# Supplementary material for: Localization techniques in quantum field theories
Source: arXiv:1608.02952 ancillary file (2016-10-13)
Supplement: Supplementary file 1 [file LocQFT.pdf]

# Localization techniques in quantum field theories

Vasily Pestun<sup>1</sup>, Maxim Zabzine<sup>2</sup>, Francesco Benini<sup>3,4</sup>, Tudor Dimofte<sup>5</sup>,  
Thomas T. Dumitrescu<sup>6</sup>, Kazuo Hosomichi<sup>7</sup>, Seok Kim<sup>8</sup>, Kimyeong Lee<sup>9</sup>,  
Bruno Le Floch<sup>10</sup>, Marcos Mariño<sup>11</sup>, Joseph A. Minahan<sup>2</sup>, David R. Morrison<sup>12</sup>,  
Sara Pasquetti<sup>13</sup>, Jian Qiu<sup>2,14,15</sup>, Leonardo Rastelli<sup>16</sup>, Shlomo S. Razamat<sup>17</sup>,  
Silvu S. Pufu<sup>18</sup>, Yuji Tachikawa<sup>19</sup>, Brian Willett<sup>20</sup>, Konstantin Zarembo<sup>21,2</sup>

<sup>1</sup>*Institut des Hautes Études Scientifique, France*

<sup>2</sup>*Department of Physics and Astronomy, Uppsala University, Sweden*

<sup>3</sup>*International School for Advanced Studies (SISSA), via Bonomea 265, 34136 Trieste, Italy*

<sup>4</sup>*Blackett Laboratory, Imperial College London, London SW7 2AZ, United Kingdom*

<sup>5</sup>*Perimeter Institute for Theoretical Physics, 31 Caroline St. N, Waterloo, ON N2J 2Y5, Canada  
(on leave) Department of Mathematics, University of California, Davis, CA 95616, USA*

<sup>6</sup>*Department of Physics, Harvard University, Cambridge, MA 02138, USA*

<sup>7</sup>*Department of Physics, National Taiwan University, Taipei 10617, Taiwan*

<sup>8</sup>*Department of Physics and Astronomy & Center for Theoretical Physics,  
Seoul National University, Seoul 151-747, Korea*

<sup>9</sup>*School of Physics, Korea Institute for Advanced Study, Seoul 130-722, Korea*

<sup>10</sup>*Princeton Center for Theoretical Science, Princeton University, Princeton, NJ 08544, USA*

<sup>11</sup>*Département de Physique Théorique et Section de Mathématiques  
Université de Genève, Genève, CH-1211 Switzerland*

<sup>12</sup>*Departments of Mathematics and Physics, University of California, Santa Barbara  
Santa Barbara, CA 93106 USA*

<sup>13</sup>*Dipartimento di Fisica, Università di Milano-Bicocca,  
Piazza della Scienza 3, I-20126 Milano, Italy*

<sup>14</sup>*Max-Planck-Institut für Mathematik, Vivatsgasse 7, 53111 Bonn, Germany*

<sup>15</sup>*Department of Mathematics, Uppsala University, Box 480, SE-75106 Uppsala, Sweden*

<sup>16</sup>*C. N. Yang Institute for Theoretical Physics, Stony Brook University, Stony Brook, NY  
11794-3840, USA*

<sup>17</sup>*Department of Physics, Technion, Haifa, 32000, Israel*

<sup>18</sup>*Joseph Henry Laboratories, Princeton University, Princeton, NJ 08544, USA*

<sup>19</sup>*Kavli Institute for the Physics and Mathematics of the Universe,  
University of Tokyo, Kashiwa, Chiba 277-8583, Japan*

<sup>20</sup>*KITP/UC Santa Barbara*

<sup>21</sup>*Nordita, KTH Royal Institute of Technology and Stockholm University, Roslagstullsbacken 23,  
SE-106 91 Stockholm, Sweden*

# Contents

|          |                                                                                                  |           |
|----------|--------------------------------------------------------------------------------------------------|-----------|
| 0.1      | Summary . . . . .                                                                                | 6         |
| 0.2      | Individual chapters . . . . .                                                                    | 7         |
| 0.3      | Volume structure . . . . .                                                                       | 12        |
|          | References . . . . .                                                                             | 12        |
| <b>1</b> | <b>Introduction to localization in quantum field theory (by Vasily Pestun and Maxim Zabzine)</b> | <b>14</b> |
| 1.1      | Main idea and history . . . . .                                                                  | 15        |
| 1.2      | Localization in diverse dimensions . . . . .                                                     | 18        |
| 1.3      | Applications of the localization technique . . . . .                                             | 29        |
|          | References . . . . .                                                                             | 31        |
| <b>2</b> | <b>Review of localization in geometry (by Vasily Pestun)</b>                                     | <b>35</b> |
| 2.1      | Equivariant cohomology . . . . .                                                                 | 36        |
| 2.2      | Classifying space and characteristic classes . . . . .                                           | 37        |
| 2.3      | Weil algebra . . . . .                                                                           | 38        |
| 2.4      | Weil model and Cartan model of equivariant cohomology . . . . .                                  | 41        |
| 2.5      | Equivariant characteristic classes in Cartan model . . . . .                                     | 43        |
| 2.6      | Standard characteristic classes . . . . .                                                        | 45        |
| 2.7      | Index formula . . . . .                                                                          | 49        |
| 2.8      | Equivariant integration . . . . .                                                                | 50        |
| 2.9      | Equivariant index formula (Dolbeault and Dirac) . . . . .                                        | 55        |
| 2.10     | Equivariant index and representation theory . . . . .                                            | 58        |
| 2.11     | Equivariant index for differential operators . . . . .                                           | 61        |
| 2.12     | Equivariant cohomological field theories . . . . .                                               | 65        |
|          | References . . . . .                                                                             | 67        |
| <b>3</b> | <b>Supersymmetric localization in two dimensions (by Francesco Benini and Bruno Le Floch)</b>    | <b>70</b> |
| 3.1      | Introduction . . . . .                                                                           | 71        |
| 3.2      | $\mathcal{N}=(2, 2)$ gauge theories on spheres . . . . .                                         | 74        |
| 3.3      | Other $\mathcal{N}=(2, 2)$ curved-space results . . . . .                                        | 90        |
| 3.4      | Elliptic genera of $\mathcal{N}=(2, 2)$ and $\mathcal{N}=(0, 2)$ theories . . . . .              | 104       |
| 3.5      | Dualities . . . . .                                                                              | 117       |

|          |                                                                                                   |            |
|----------|---------------------------------------------------------------------------------------------------|------------|
| 3.6      | Conclusion . . . . .                                                                              | 129        |
|          | References . . . . .                                                                              | 130        |
| <b>4</b> | <b>Gromov–Witten invariants and localization (by David R. Morrison)</b>                           | <b>139</b> |
| 4.1      | Introduction . . . . .                                                                            | 140        |
| 4.2      | Kähler potentials and 2-sphere partition functions . . . . .                                      | 141        |
| 4.3      | Metrics on conformal manifolds . . . . .                                                          | 144        |
| 4.4      | Quantum corrections to the Kähler potential . . . . .                                             | 152        |
| 4.5      | The two-sphere partition function and Gromov–Witten invariants . . . . .                          | 158        |
| 4.6      | Evaluating the partition function . . . . .                                                       | 161        |
| 4.7      | Appendix. $\mathcal{N} = (2, 2)$ supersymmetry in two dimensions . . . . .                        | 166        |
|          | References . . . . .                                                                              | 167        |
| <b>5</b> | <b>An introduction to supersymmetric field theories in curved space (by Thomas T. Dumitrescu)</b> | <b>174</b> |
| 5.1      | Introduction . . . . .                                                                            | 175        |
| 5.2      | Four-dimensional $\mathcal{N} = 1$ theories . . . . .                                             | 183        |
| 5.3      | Three-dimensional $\mathcal{N} = 2$ theories . . . . .                                            | 195        |
|          | References . . . . .                                                                              | 198        |
| <b>6</b> | <b>Localization on three-dimensional manifolds (by Brian Willett)</b>                             | <b>203</b> |
| 6.1      | Introduction . . . . .                                                                            | 204        |
| 6.2      | Supersymmetry on the 3-sphere . . . . .                                                           | 209        |
| 6.3      | Localization of the partition function on the 3–sphere . . . . .                                  | 220        |
| 6.4      | Lens spaces . . . . .                                                                             | 235        |
| 6.5      | $S^2 \times S^1$ partition function . . . . .                                                     | 239        |
| 6.6      | Applications . . . . .                                                                            | 247        |
|          | References . . . . .                                                                              | 265        |
| <b>7</b> | <b>Localization at large <math>N</math> in Chern–Simons–matter theories (by Marcos Mariño)</b>    | <b>271</b> |
| 7.1      | Introduction . . . . .                                                                            | 272        |
| 7.2      | The ABJM matrix model . . . . .                                                                   | 273        |
| 7.3      | Generalizations . . . . .                                                                         | 318        |
| 7.4      | Conclusions and outlook . . . . .                                                                 | 325        |
|          | References . . . . .                                                                              | 327        |
| <b>8</b> | <b>The <math>F</math>-Theorem and <math>F</math>-Maximization (by Silviu S. Pufu)</b>             | <b>334</b> |
| 8.1      | Introduction . . . . .                                                                            | 335        |
| 8.2      | The $F$ -coefficients of various CFTs . . . . .                                                   | 337        |
| 8.3      | $\mathcal{N} = 2$ SCFTs and $F$ -maximization . . . . .                                           | 347        |
| 8.4      | Conclusion . . . . .                                                                              | 360        |
|          | References . . . . .                                                                              | 361        |

|           |                                                                                                   |            |
|-----------|---------------------------------------------------------------------------------------------------|------------|
| <b>9</b>  | <b>Perturbative and nonperturbative aspects of complex Chern-Simons Theory (by Tudor Dimofte)</b> | <b>367</b> |
| 9.1       | Introduction . . . . .                                                                            | 368        |
| 9.2       | Warmup: quantization of $\mathcal{H}(T^2)$ . . . . .                                              | 370        |
| 9.3       | Complex Chern-Simons theory as a TQFT? . . . . .                                                  | 376        |
| 9.4       | Three connections to three-manifold topology . . . . .                                            | 379        |
| 9.5       | The Quantum Modularity Conjecture . . . . .                                                       | 388        |
|           | References . . . . .                                                                              | 391        |
| <b>10</b> | <b><math>\mathcal{N} = 2</math> SUSY gauge theories on <math>S^4</math> (by Kazuo Hosomichi)</b>  | <b>397</b> |
| 10.1      | Introduction . . . . .                                                                            | 398        |
| 10.2      | Construction of theories . . . . .                                                                | 401        |
| 10.3      | Partition function . . . . .                                                                      | 409        |
| 10.4      | Supersymmetric observables . . . . .                                                              | 417        |
|           | References . . . . .                                                                              | 426        |
| <b>11</b> | <b>Localization and AdS/CFT Correspondence (by Konstantin Zarembo)</b>                            | <b>431</b> |
| 11.1      | Introduction . . . . .                                                                            | 431        |
| 11.2      | $\mathcal{N} = 4$ Super-Yang-Mills theory . . . . .                                               | 432        |
| 11.3      | Circular Wilson loop . . . . .                                                                    | 433        |
| 11.4      | Higher representations and D-branes . . . . .                                                     | 440        |
| 11.5      | Wavy lines, cusp and latitude . . . . .                                                           | 449        |
| 11.6      | Operator Product Expansion . . . . .                                                              | 457        |
| 11.7      | Massive theory . . . . .                                                                          | 464        |
| 11.8      | Conclusions . . . . .                                                                             | 468        |
|           | References . . . . .                                                                              | 469        |
| <b>12</b> | <b>A brief review of the 2d/4d correspondences (by Yuji Tachikawa)</b>                            | <b>475</b> |
| 12.1      | Introduction . . . . .                                                                            | 476        |
| 12.2      | Two two-dimensional theories . . . . .                                                            | 477        |
| 12.3      | A class of four-dimensional theories . . . . .                                                    | 489        |
| 12.4      | Two supersymmetric backgrounds . . . . .                                                          | 494        |
| 12.5      | Two correspondences and an interpretation . . . . .                                               | 502        |
| 12.6      | Future directions . . . . .                                                                       | 509        |
|           | References . . . . .                                                                              | 514        |
| <b>13</b> | <b>The supersymmetric index in four dimensions (by Leonardo Rastelli and Shlomo S. Razamat)</b>   | <b>519</b> |
| 13.1      | Introduction . . . . .                                                                            | 520        |
| 13.2      | Definition of the index . . . . .                                                                 | 521        |
| 13.3      | Index of sigma models . . . . .                                                                   | 527        |
| 13.4      | Index of gauge theories . . . . .                                                                 | 529        |
| 13.5      | Index spectroscopy . . . . .                                                                      | 534        |

|                                                                                    |            |
|------------------------------------------------------------------------------------|------------|
| 13.6 Dualities and Identities . . . . .                                            | 538        |
| 13.7 Limits . . . . .                                                              | 542        |
| 13.8 Other topics and open problems . . . . .                                      | 553        |
| References . . . . .                                                               | 554        |
| <b>14 Review of localization for</b>                                               |            |
| <b>5d supersymmetric gauge theories (by Jian Qiu and Maxim Zabzine)</b>            | <b>559</b> |
| 14.1 Introduction . . . . .                                                        | 560        |
| 14.2 The basic setup . . . . .                                                     | 562        |
| 14.3 The cohomological complex . . . . .                                           | 566        |
| 14.4 Analysis of the fixed points . . . . .                                        | 573        |
| 14.5 Gauge fixing and the determinant . . . . .                                    | 578        |
| 14.6 Asymptotics and comparison with flat space . . . . .                          | 584        |
| 14.7 Appendix. Geometrical setting . . . . .                                       | 589        |
| References . . . . .                                                               | 597        |
| <b>15 Matrix models for 5d super Yang-Mills (by Joseph A. Minahan)</b>             | <b>600</b> |
| 15.1 Introduction . . . . .                                                        | 601        |
| 15.2 Matrix model for $\mathcal{N} = 1$ 5d Yang-Mills with matter . . . . .        | 602        |
| 15.3 $\mathcal{N} = 1^*$ 5d super Yang-Mills . . . . .                             | 606        |
| 15.4 Supergravity comparisons . . . . .                                            | 609        |
| 15.5 Discussion . . . . .                                                          | 611        |
| References . . . . .                                                               | 612        |
| <b>16 Holomorphic blocks and the 5d AGT correspondence (by Sara Pasquetti)</b>     | <b>615</b> |
| 16.1 Introduction . . . . .                                                        | 616        |
| 16.2 Compact manifolds and Holomorphic Block factorisation . . . . .               | 617        |
| 16.3 Chiral 5d AGT . . . . .                                                       | 633        |
| 16.4 3d & 5d partition functions as $q$ -deformed correlators . . . . .            | 644        |
| 16.5 Appendix . . . . .                                                            | 649        |
| References . . . . .                                                               | 652        |
| <b>17 Indices for 6 dimensional superconformal field theories (by Seok Kim and</b> |            |
| <b>Kimyeong Lee)</b>                                                               | <b>659</b> |
| 17.1 Introduction . . . . .                                                        | 660        |
| 17.2 Coulomb branch indices for the self-dual strings . . . . .                    | 663        |
| 17.3 Superconformal indices of the 6d (2, 0) theories . . . . .                    | 670        |
| 17.4 Discussions . . . . .                                                         | 691        |
| 17.5 Appendix. Off-shell supergravity analysis on $S^5$ . . . . .                  | 693        |
| References . . . . .                                                               | 696        |

## 0.1 Summary

This is the summary of the special volume “Localization techniques in quantum field theories” which contains 17 individual chapters.<sup>1</sup> The focus of the volume is on the localization technique and its applications in supersymmetric gauge theories. Although the ideas of equivariant localization in quantum field theory go back 30 years, here we concentrate on the recent surge in the subject during the last ten years. This subject develops rapidly and thus it is impossible to have a fully satisfactory overview of the field. This volume took about two and a half years in making, and during this period some important new results have been obtained, and it was hard to incorporate all of them. However we think that it is important to provide an overview and an introduction to this quickly developing subject. This is important both for the young researchers, who just enter the field and to established scientists as well. We have tried to do our best to review the main results during the last ten years.

The volume has two types of chapters, some chapters concentrate on the localization calculation in different dimensions by itself, and other chapters concentrate on the major applications of the localization result. Obviously, such separation is sometimes artificial. The chapters are ordered roughly according to the dimensions of the corresponding supersymmetric theories. First, we try to review the localization calculation in given dimension, and then we move to the discussion of the major applications.

The volume covers the localization calculations for the supersymmetric theories in dimensions 2,3,4 and 5. The volume discusses the applications of these calculations for theories living up to dimension 6, and for string/M theories. We have to apologize in advance for omitting from the review the new and important calculations which have appeared during last couple of years.

This volume is intended to be a single volume where the different chapters cover the different but related topics within a certain focused scope. Some chapters depend on results presented in a different chapter, but the dependency is not a simple linear order.

The whole volume, when published, could be cited as

V. Pestun and M. Zabzine, eds.,  
“Localization techniques in quantum field theories”,  
*Journal of Physics A* (2016)

The arXiv preprint version can be accessed from arXiv summary entry which lists all authors and links to all 17 individual contributions, the corresponding citation would be

[arXiv:1608.02952](https://arxiv.org/abs/1608.02952)

An individual contribution can be cited by its chapter number, for example

---

<sup>1</sup>The preprint version is available at <https://arxiv.org/src/1608.02952/anc/LocQFT.pdf> or <http://pestun.ihep.fr/pages/LocalizationReview/LocQFT.pdf>

S. Pufu, “The F-Theorem and F-Maximization,”  
Chapter 8 in V. Pestun and M. Zabzine, eds.,  
“Localization techniques in quantum field theories”,  
*Journal of Physics A* (2016)

and accessed on arXiv and cited by the arXiv number

[arXiv:1608.02960](https://arxiv.org/abs/1608.02960).

## 0.2 Individual chapters

Below we summarize the content of each individual contribution/chapter:

Chapter 1: “Introduction to localization in quantum field theory” (Vasily Pestun and Maxim Zabzine)

This is the introductory chapter to the whole volume, outlining its scope and reviewing the field as a whole. The chapter discusses shortly the history of equivariant localization both in finite and infinite dimensional setups. The derivation of the finite dimensional Berline-Vergne-Atiyah-Bott formula is given in terms of supergeometry. This derivation is formally generalized to the infinite dimensional setup in the context of supersymmetric gauge theories. The result for supersymmetric theories on spheres is presented in a uniform fashion over different dimensions, and the related index theorem calculations are reviewed. The applications of localization techniques are listed and briefly discussed.

Chapter 2: “Review of localization in geometry” (Vasily Pestun)

This chapter is a short summary of the mathematical aspects of the Berline-Vergne-Atiyah-Bott formula and Atiyah-Singer index theory. These tools are routinely used throughout the volume. The chapter reviews the definition of equivariant cohomology, and its Weyl and Cartan models. The standard characteristic classes and their equivariant versions are reviewed. The equivariant integration is discussed and the mathematical derivation of the Berline-Vergne-Atiyah-Bott formula is explained. The Atiyah-Singer index theorems and their equivariant versions are briefly reviewed.

Chapter 3: “Supersymmetric localization in two dimensions” (Francesco Benini and Bruno Le Floch)

This chapter concentrates on the localization techniques for 2d supersymmetric gauge theories and on the major applications of 2d localization results. The main example is the calculation of the partition function for  $\mathcal{N} = (2, 2)$  gauge theory on  $S^2$ . Two different approaches are presented, the Coulomb branch localization (when the result is written as an integral over the Cartan subalgebra) and the Higgs branch localization (when the answer is written

as a sum). Briefly  $\mathcal{N} = (2, 2)$  gauge theories on other curved backgrounds are discussed, and the calculation for the hemisphere is presented. The important calculation of the partition function for  $\mathcal{N} = (2, 2)$  and  $\mathcal{N} = (2, 0)$  theories on the torus is presented, this quantity is known as the elliptic genus. The result is written in terms of the Jeffrey-Kirwan residue, which is a higher dimensional analog of the residue operation. The mathematical aspects of the Jeffrey-Kirwan residue operation are briefly explained. As the main application of the localization calculation in 2d, some dualities are discussed; in particular mirror symmetry and Seiberg duality.

Chapter 4: “Gromov-Witten invariants and localization” (David Morrison)

This chapter concentrates on an important application of 2d localization calculation, see Chapter 3. The chapter provides a pedagogical introduction to the relation between the genus 0 Gromov-Witten invariants (counting of holomorphic maps) and the localization of 2d gauged linear sigma models. The relation is based on the conjecture which connects the partition function of  $\mathcal{N} = (2, 2)$  gauge theories on  $S^2$  with the Zamolodchikov metric on the conformal manifold of the theory. This relation allows to deduce the Gromov-Witten invariants on the Calabi-Yau manifold from the partition function on  $S^2$  of the corresponding linear sigma model. This chapter explains this conjecture and reviews the main step of the calculation.

Chapter 5: “An Introduction to supersymmetric field theories in curved space” (Thomas Dumitrescu)

This chapter addresses the problem of defining rigid supersymmetric theories on curved backgrounds. The systematic approach to this problem is based on the Festuccia-Seiberg work on organizing the background fields into off-shell supergravity multiplets. The chapter concentrates in details on two major examples,  $\mathcal{N} = 1$  supersymmetric theories in 4d and  $\mathcal{N} = 2$  supersymmetric theories in 3d. The full classification of supersymmetric theories on curved backgrounds can be given for the theories with four or fewer supersymmetry in four or fewer dimensions.

Chapter 6: “Localization on three-dimensional manifolds” (Brian Willett)

This chapter provides an introduction to the localization technique for 3d supersymmetric gauge theories. The 3d  $\mathcal{N} = 2$  supersymmetric theories are introduced and their formulation on curved space is briefly discussed, this is closely related to Chapter 5. The calculation of the partition function on  $S^3$  is presented in great details with the final result presented as an integral over the Cartan subalgebra of the Lie algebra of the gauge group. The calculation on the lens spaces, on  $S^2 \times S^1$  and different applications of these calculations are also discussed. The dualities between different gauge theories are briefly discussed. The factorization of the result into holomorphic blocks is also considered, and in this context the Higgs branch

localization is discussed.

Chapter 7: “Localization at large  $N$  in Chern-Simons-matter theories” (Marcos Mariño)

The result of the localization calculation in 3d is given in terms of matrix integrals, see Chapter 6. These matrix integrals are complicated and it is not easy to extract information from this answer. This chapter is devoted to the study of 3d matrix models and extracting physical information from them. The chapter concentrates on the famous ABJM model which plays a crucial role in the AdS/CFT correspondence. The M-theory expansion for the ABJM model is discussed in details and the relation to topological strings is presented.

Chapter 8: “The F-Theorem and F-Maximization” (Silviu Pufu)

The partition function on  $S^3$  for  $\mathcal{N} = 2$  supersymmetric gauge theories is written as matrix integrals which depend on the different parameters of the theory, see Chapter 6. This chapter studies the properties of the free energy (minus the logarithm of the sphere partition function), which is regarded as the measure of the degrees of freedom in the theory. In particular the chapter states and explains the F-theorem and F-maximization principles for 3d theories. The F-theorem is a 3d analogue of the Zamolodchikov’s c-theorem in 2d and the a-theorem in 4d. For 3d theories the F-theorem makes a precise statement about the idea that the number of degrees of freedom decreases along the RG flow.

Chapter 9: “Perturbative and nonperturbative aspects of complex Chern-Simons Theory” (Tudor Dimofte)

This chapter discusses another important application for the localization calculation in 3d. The chapter starts by briefly reviewing some basic facts about the complex Chern-Simons theory, the main interest is the Chern-Simons theory for  $SL(N, \mathbb{C})$ . There is a short discussion of the 3d/3d correspondence, which states that the partition function of the complex Chern-Simons theory on  $M$  is the same as the partition function of a specific supersymmetric gauge theory (whose field content depends on  $M$ ) on the lens space. The chapters finishes with a discussion of the quantum modularity conjecture.

Chapter 10: “ $\mathcal{N} = 2$  SUSY gauge theories on  $S^4$ ” (Kazuo Hosomichi)

This chapter gives a detailed exposition of the calculation of the partition function and other supersymmetric observables for  $\mathcal{N} = 2$  supersymmetric gauge theories on  $S^4$ , both round and squashed. Using off-shell supergravity, the construction of  $\mathcal{N} = 2$  supersymmetric theories on squashed  $S^4$  is presented. The localization calculation is performed and the determinants are explicitly evaluated using index theorems (review in Chapter 2). The inclusion of supersymmetric observables (Wilson loops, ’t Hooft operators and surface operators) into the localization calculation on  $S^4$  is discussed.

Chapter 11: “Localization and AdS/CFT Correspondence” (Konstantin Zarembo)

One of the major application of the localization calculation on  $S^4$  (see Chapter 10) is the application to AdS/CFT. This chapter is devoted to the study of the matrix models which appear in the calculation on  $S^4$  and its application to the AdS/CFT correspondence. Localization offers a unique laboratory for the AdS/CFT correspondence, since we are able to explore the supersymmetric gauge theory in non-perturbative domain. Using holography the localization computation can be compared to string theory and supergravity calculations.

Chapter 12: “A brief review of the 2d/4d correspondences” (Yuji Tachikawa)

From the perspective of the  $\mathcal{N} = (0, 2)$  self-dual 6d theory, this chapter explains the 2d/4d correspondence (AGT), considering the 6d theory on a product of 2d and 4d manifold. This correspondence relates the 4d computations for supersymmetric gauge theories of class  $\mathcal{S}$ , obtained by compactification of the 6d theory on the 2d manifold, to 2d computations in 2d theory obtained by compactification of 6d theory on the 4d manifold. The chapter starts by reviewing basic facts about 2d q-deformed Yang-Mills theory and the Liouville theory. The main building block of rank 1 theories considered in the chapter is the trifundamental multiplet coupled with  $SU(2)$  gauge fields. The partition function on  $S^1 \times S^3$  for such a 4d theory is computed in 2d by q-deformed Yang-Mills and the partition function on  $S^4$  is computed in 2d by the Liouville theory.

Chapter 13: “The supersymmetric index in four dimensions” (Leonardo Rastelli and Shlomo Razamat)

This chapter studies the partition function on  $S^3 \times S^1$  for  $\mathcal{N} = 1$  supersymmetric theories in 4d, also known as the 4d supersymmetric index. The chapter starts by defining the supersymmetric index and reviewing combinatorial tools to compute it in theories with a Lagrangian description. After illustrating some basic properties of the index in the simple setting of supersymmetric sigma models, the chapter turns to the discussion of the index of supersymmetric gauge theories, emphasizing physical applications. The index contains useful information about the spectrum of shortened multiplets, and how to extract this information is discussed in some detail. The most important application of the index, as a powerful tool for checking non-perturbative dualities between supersymmetric gauge theories, is illustrated in several examples. The last part of the chapter considers several interesting limits of the supersymmetric index.

Chapter 14: “Review of localization for 5d supersymmetric gauge theories” (Jian Qiu and Maxim Zabzine)

The chapter provides the introduction to localization calculation for  $\mathcal{N} = 1$  supersym-

metric gauge theories on toric Sasaki-Einstein manifolds, for example on a five-sphere  $S^5$ . The chapter starts by recalling basic facts about supersymmetry and supersymmetric gauge theories in flat 5d space. Then the construction of the supersymmetric gauge theory on the Sasaki-Einstein manifolds is explicitly given. Using the field redefinition, the supersymmetry transformations are rewritten in terms of differential forms, thus making geometrical aspects of the localization more transparent. For toric Sasaki-Einstein manifolds the localization calculation can be carried out completely, the calculation of determinants is given and the full partition function is conjectured. The chapter ends with comments about deducing the flat space results from the curved result.

Chapter 15: “Matrix models for 5d super Yang-Mills” (Joseph Minahan)

The result of 5d localization calculation is given in terms of complicated matrix models, see Chapter 14. This chapter studies the resulting matrix models. The basic properties of the matrix models are described and the 't Hooft limit is analyzed for  $\mathcal{N} = 1^*$  theory (a vector multiplet plus a hypermultiplet in the adjoint representation). For large 't Hooft coupling the free energy behaves as  $N^3$  for  $U(N)$  gauge theory and the corresponding supergravity analysis is performed. This analysis support the idea that the non-perturbative completion of 5d theory is the 6d  $\mathcal{N} = (2, 0)$  superconformal field theory.

Chapter 16: “Holomorphic blocks and the 5d AGT correspondence” (Sara Pasquetti)

This chapter further studies partition functions from 2d to 5d. In particular it concentrates on the idea that the partition function on a compact manifold can be built up from basic blocks, so-called holomorphic blocks. The main point is that the geometric decomposition of the compact manifold should have its counterpart in the appropriate decomposition of the partition function. These factorization properties are reviewed in different dimensions. The rest of the chapter concentrates on a 5d version of the AGT correspondence.

Chapter 17: “Indices for 6 dimensional superconformal field theories” (Seok Kim and Kimyeong Lee)

This chapter deals with the 6d  $(2, 0)$  superconformal field theory. This theory cannot be accessed directly, but it is related to many other supersymmetric gauge theories, e.g. it is believed to be the UV-completion of maximally supersymmetric 5d gauge theory. The relation between 5d partition function and 6d supersymmetric index is discussed in details in this chapter.

## 0.3 Volume structure

The different chapters are related to each other and the relation is not a simple linear relation, which can be shown by their ordering in the volume. Below we provide the graphical relation between different chapters. This diagram<sup>2</sup> gives the general idea.

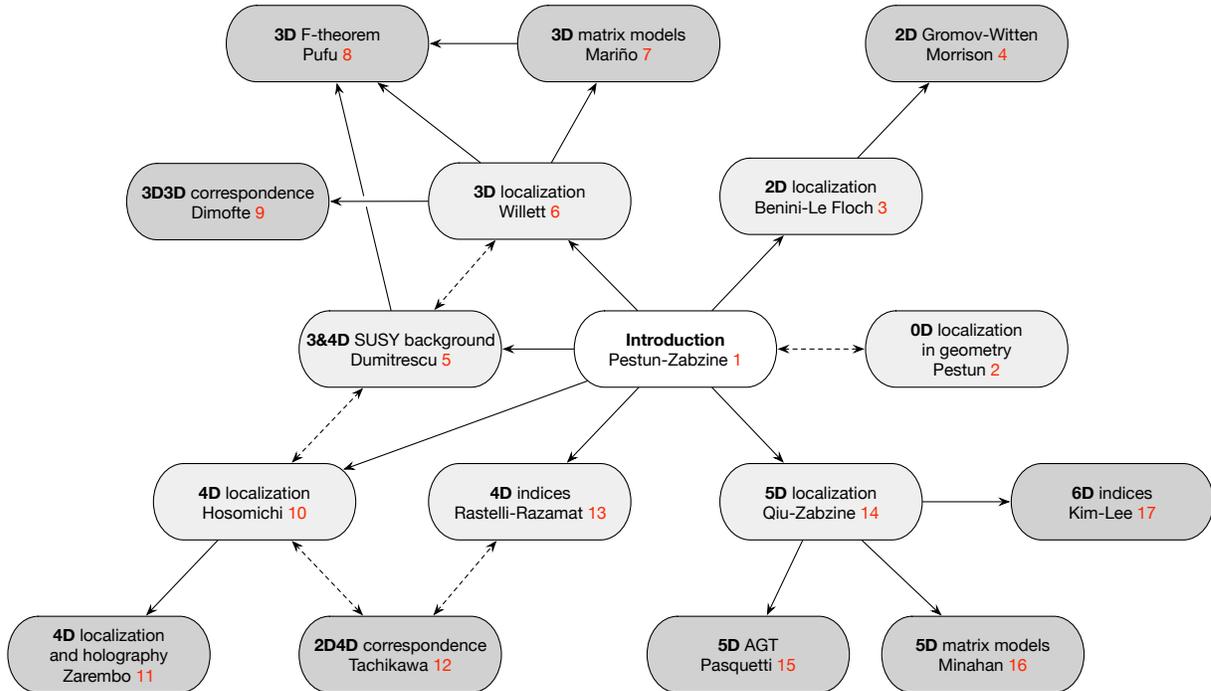

## References

- [1] V. Pestun and M. Zabzine, “Introduction to localization in quantum field theory,” *Journal of Physics A* **xx** (2016) 000, [1608.02953](#).
- [2] V. Pestun, “Review of localization in geometry,” *Journal of Physics A* **xx** (2016) 000, [1608.02954](#).
- [3] F. Benini and B. Le Floch, “Supersymmetric localization in two dimensions,” *Journal of Physics A* **xx** (2016) 000, [1608.02955](#).
- [4] D. Morrison, “Gromov-Witten invariants and localization,” *Journal of Physics A* (2016) , [1608.02956](#).
- [5] T. Dumitrescu, “An Introduction to Supersymmetric Field Theories in Curved Space,” *Journal of Physics A* **xx** (2016) 000, [1608.02957](#).
- [6] B. Willett, “Localization on three-dimensional manifolds,” *Journal of Physics A* **xx** (2016) 000, [1608.02958](#).
- [7] M. Mariño, “Localization at large  $N$  in Chern-Simons-matter theories,” *Journal of Physics A* **xx** (2016) 000, [1608.02959](#).
- [8] S. Pufu, “The F-Theorem and F-Maximization,” *Journal of Physics A* **xx** (2016) 000, [1608.02960](#).

<sup>2</sup>Special thanks to Yuji Tachikawa for the final design of the diagram

- [9] T. Dimofte, “Perturbative and nonperturbative aspects of complex Chern-Simons Theory,” *Journal of Physics A* **xx** (2016) 000, [1608.02961](#).
- [10] K. Hosomichi, “ $\mathcal{N} = 2$  SUSY gauge theories on  $S^4$ ,” *Journal of Physics A* **xx** (2016) 000, [1608.02962](#).
- [11] K. Zarembo, “Localization and AdS/CFT Correspondence,” *Journal of Physics A* **xx** (2016) 000, [1608.02963](#).
- [12] Y. Tachikawa, “A brief review of the 2d/4d correspondences,” *Journal of Physics A* **xx** (2016) 000, [1608.02964](#).
- [13] L. Rastelli and S. Razamat, “The supersymmetric index in four dimensions,” *Journal of Physics A* **xx** (2016) 000, [1608.02965](#).
- [14] J. Qiu and M. Zabzine, “Review of localization for 5D supersymmetric gauge theories,” *Journal of Physics A* **xx** (2016) 000, [1608.02966](#).
- [15] J. Minahan, “Matrix models for 5D super Yang-Mills,” *Journal of Physics A* **xx** (2016) 000, [1608.02967](#).
- [16] S. Pasquetti, “Holomorphic blocks and the 5d AGT correspondence,” *Journal of Physics A* **xx** (2016) 000, [1608.02968](#).
- [17] S. Kim and K. Lee, “Indices for 6 dimensional superconformal field theories,” *Journal of Physics A* **xx** (2016) 000, [1608.02969](#).

# Chapter 1

## Introduction to localization in quantum field theory

Vasily Pestun<sup>1</sup> and Maxim Zabzine<sup>2</sup>

<sup>1</sup>*Institut des Hautes Études Scientifique, France*

<sup>2</sup>*Department of Physics and Astronomy, Uppsala University, Sweden*  
pestun@ihes.fr, Maxim.Zabzine@physics.uu.se

### Abstract

This is the introductory chapter to the volume. We review the main idea of the localization technique and its brief history both in geometry and in QFT. We discuss localization in diverse dimensions and give an overview of the major applications of the localization calculations for supersymmetric theories. We explain the focus of the present volume.

### Contents

|            |                                                             |           |
|------------|-------------------------------------------------------------|-----------|
| <b>1.1</b> | <b>Main idea and history</b> . . . . .                      | <b>15</b> |
| <b>1.2</b> | <b>Localization in diverse dimensions</b> . . . . .         | <b>18</b> |
| 1.2.1      | Topological Yang-Mills . . . . .                            | 21        |
| 1.2.2      | Even dimensions . . . . .                                   | 23        |
| 1.2.3      | Odd dimensions . . . . .                                    | 27        |
| <b>1.3</b> | <b>Applications of the localization technique</b> . . . . . | <b>29</b> |
|            | <b>References</b> . . . . .                                 | <b>31</b> |

## 1.1 Main idea and history

According to the English dictionary<sup>1</sup> the word *localize* means to make local, fix in or assign or restrict to a particular place, locality. Both in mathematics and physics the word “localize” has multiple meanings and typically physicists with different backgrounds mean different things by localization. This volume is devoted to the extension of the Atiyah-Bott localization formula (and related statements, e.g. the Duistermaat-Heckman formula and different versions of the fixed-point theorem) in differential geometry to an infinite dimensional situation of path integral, and in particular in the context of supersymmetric quantum field theory. In quantum field theory one says “supersymmetric localization” to denote such computations. In this volume we concentrate on the development of the supersymmetric localization technique during the last ten years, 2007-2016.

In differential geometry the idea of localization can be traced back to 1926 [2], when Lefschetz proved the fixed-point formula which counts fixed points of a continuous map of a topological space to itself by using the graded trace of the induced map on the homology groups of this space. In the 1950’s, the Grothendieck-Hirzebruch-Riemann-Roch theorem expressed in the most general form the index of a holomorphic vector bundle (supertrace over graded cohomology space) in terms of certain characteristic classes. In the 1960’s, the Atiyah-Singer index theorem solved the same problem for an arbitrary elliptic complex.

In 1982 Duistermaat and Heckman [3] proved the following formula

$$\int_M \frac{\omega^n}{n!} e^{-\mu} = \sum_i \frac{e^{-\mu(x_i)}}{e(x_i)}, \quad (1.1.1)$$

where  $M$  is a symplectic compact manifold of dimension  $2n$  with symplectic form  $\omega$  and with a Hamiltonian  $U(1)$  action whose moment map is  $\mu$ . Here  $x_i$  are the fixed points of the  $U(1)$  action and they are assumed to be isolated, and  $e(x_i)$  is the product of the weights of the  $U(1)$  action on the tangent space at  $x_i$ . Later independently in 1982 Berline and Vergne [4] and in 1984 Atiyah and Bott [5] generalized the Duistermaat-Heckman formula to the case of a general compact manifold  $M$  with a  $U(1)$  action and an integral  $\int \alpha$  of an equivariantly-closed form  $\alpha$ , that is  $(d + \iota_V)\alpha = 0$ , where  $V(x)$  is the vector field corresponding to the  $U(1)$  action. The Berline-Vergne-Atiyah-Bott formula reads as

$$\int_M \alpha = \sum_i \frac{\pi^n \alpha_0(x_i)}{\sqrt{\det(\partial_\mu V^\nu(x_i))}}, \quad (1.1.2)$$

where it is assumed that  $x_i$  are isolated fixed points of the  $U(1)$  action, and  $\alpha_0$  is the zero-form component of  $\alpha$ . The Berline-Vergne-Atiyah-Bott formula has multiple generalizations, to the case of non-isolated fixed locus, to supermanifolds, to the holomorphic case, etc. The more detailed overview of this formula and its relation to equivariant cohomology is given in Chapter 2. Here we will concentrate on conceptual issues and our discussion is rather schematic.

---

<sup>1</sup>E.g. <http://www.dictionary.com>, based on the Random House Dictionary, ©Random House, Inc. 2016

Let us review the proof of the Berline-Vergne-Atiyah-Bott formula (1.1.2). We will use the language of supergeometry, since it is easier to generalize to the infinite dimensional setup. Consider the odd tangent bundle  $\Pi TM$  where  $x^\mu$  are coordinates on  $M$  and  $\psi^\mu$  are odd coordinates on the fiber (i.e., they transform as  $dx^\mu$ ). Functions  $f(x, \psi)$  correspond to differential forms and the integration measure  $d^n x d^n \psi$  on  $\Pi TM$  is canonically defined. Assume that there is a  $U(1)$  action on compact  $M$  with the corresponding vector field  $V^\mu(x)\partial_\mu$ . Define the following ‘‘supersymmetry transformations’’

$$\begin{aligned}\delta x^\mu &= \psi^\mu \\ \delta \psi^\mu &= V^\mu(x)\end{aligned}\tag{1.1.3}$$

which correspond to the equivariant differential  $d + \iota_V$ . We are interested in computation of the integral

$$Z(0) = \int_{\Pi TM} \alpha(x, \psi) d^n x d^n \psi\tag{1.1.4}$$

for  $\alpha(x, \psi)$  a ‘‘supersymmetric observable’’, i.e. an equivariantly closed form  $\delta\alpha(x, \psi) = 0$ . We can deform the integral in the following way

$$Z(t) = \int_{\Pi TM} \alpha(x, \psi) e^{-t\delta W(x, \psi)} d^n x d^n \psi ,\tag{1.1.5}$$

where  $W(x, \psi)$  is some function. Using the Stokes theorem, one can show that the integral  $Z(t)$  is independent of  $t$ , provided that  $\delta^2 W = 0$ . For example, we can choose  $W = V^\mu g_{\mu\nu} \psi^\nu$  with  $g_{\mu\nu}$  being a  $U(1)$ -invariant metric. If  $Z(t)$  is independent of  $t$ , then we can calculate the original integral at  $t = 0$  at another value of  $t$ , in particular we can send  $t$  to infinity

$$Z(0) = \lim_{t \rightarrow \infty} Z(t) = \lim_{t \rightarrow \infty} \int_{\Pi TM} \alpha(x, \psi) e^{-t\delta W(x, \psi)} d^n x d^n \psi .\tag{1.1.6}$$

Thus using the saddle point approximation for  $Z(t)$  we can calculate the exact value of  $Z(0)$ . If we choose  $W = V^\mu g_{\mu\nu} \psi^\nu$  with the invariant metric and perform the calculation we arrive at the formula (1.1.2). Let us outline the main steps of the derivation. In the integral (1.1.6)

$$\delta W = V^\mu g_{\mu\nu} V^\nu + \partial_\rho (V^\mu g_{\mu\nu}) \psi^\rho \psi^\nu\tag{1.1.7}$$

and thus in the limit  $t \rightarrow \infty$  the critical points  $x_i$  of the  $U(1)$  action dominate,  $V(x_i) = 0$ . Let us consider the contribution of one isolated point  $x_i$ , and for the sake of clarity let’s assume that  $x_i = 0$ . In the neighbourhood of this critical point 0, we can rescale coordinates as follows

$$\sqrt{t}x = \tilde{x} , \quad \sqrt{t}\psi = \tilde{\psi} ,\tag{1.1.8}$$

so that the integral expression (1.1.6) becomes

$$Z(0) = \lim_{t \rightarrow \infty} \int_{\Pi TM} \alpha\left(\frac{\tilde{x}}{\sqrt{t}}, \frac{\tilde{\psi}}{\sqrt{t}}\right) e^{-t\delta W\left(\frac{\tilde{x}}{\sqrt{t}}, \frac{\tilde{\psi}}{\sqrt{t}}\right)} d^n \tilde{x} d^n \tilde{\psi} ,\tag{1.1.9}$$

where we have used the property of the measure on  $\Pi TM$ ,  $d^n x d^n \psi = d^n \tilde{x} d^n \tilde{\psi}$ . Now in (1.1.9) we may keep track of only leading terms which are independent of  $t$ . In the exponent with  $\delta W$  only the quadratic terms are relevant

$$\delta W = H_{\mu\nu} \tilde{x}^\mu \tilde{x}^\nu + S_{\mu\nu} \tilde{\psi}^\mu \tilde{\psi}^\nu, \quad (1.1.10)$$

where the concrete form of the matrices  $H$  and  $S$  is irrelevant. In the limit  $t \rightarrow \infty$  the “supersymmetry transformations” (1.1.3) are naturally linearized

$$\begin{aligned} \delta \tilde{x}^\mu &= \tilde{\psi}^\mu \\ \delta \tilde{\psi}^\mu &= \partial_\nu V^\mu(0) \tilde{x}^\nu, \end{aligned} \quad (1.1.11)$$

and the condition  $\delta^2 W = 0$  now implies

$$H_{\mu\nu} = S_{\mu\sigma} \partial_\nu V^\sigma(0). \quad (1.1.12)$$

Now in the integral (1.1.9) we have to take the limit  $t \rightarrow \infty$  and perform the gaussian integral in even and odd coordinates

$$Z(0) = \alpha(0, 0) \frac{\pi^{\dim M/2} \text{Pf}(S)}{\sqrt{\det H}} \quad (1.1.13)$$

and using (1.1.12) we arrive at

$$Z(0) = \alpha(0, 0) \frac{\pi^{\dim M/2}}{\sqrt{\det \partial_\mu V^\nu(0)}}. \quad (1.1.14)$$

If we repeat this calculation for every fixed point, we arrive at the Berline-Vergne-Atiyah-Bott formula (1.1.2). This is the actual proof for a  $U(1)$  action on a compact  $M$ . In principle the requirement of a  $U(1)$  action can be relaxed to  $V$  being Killing vector on a compact  $M$ , since in the derivation we only use the invariance of the metric to construct the appropriate  $W$ . For non-compact spaces, one can use the Berline-Vergne-Atiyah-Bott formula as a suitable definition of the integral, for example to introduce the notion of equivariant volume etc. There are many generalizations of the above logic, for example one can construct the holomorphic version of the equivariant differential with the property  $\delta^2 = 0$  etc.

This setup can be formally generalized to the case where  $M$  is an infinite dimensional manifold.

Indeed, we can regard this as the definition of the infinite dimensional integral, provided that the formal properties are preserved. However, in the infinite dimensional case, the main challenge is to make sure that all steps of the formal proof can be suitably defined, for example the choice of a suitable  $W$  may become a non-trivial problem. In the infinite dimensional situation the matrix  $\partial_\nu V^\mu(0)$  in (1.1.11) turns into a differential operator and the (super)-determinant of this differential operator should be defined carefully.

The most interesting applications of these ideas come from supersymmetric gauge theories. In this case, one tries to recognise the supersymmetry transformations together with the

BRST-symmetry coming from the gauge fixing as some type of equivariant differential (1.1.3) acting on the space of fields (an infinite dimensional supermanifold).

In the context of the infinite-dimensional path integral, the localization construction was first proposed by Witten in his work on supersymmetric quantum mechanics [7]. In that case the infinite dimensional manifold  $M$  is the loop space  $LX$  of an ordinary smooth manifold  $X$ . In the simplest case, the  $U(1)$  action on  $LX$  comes from the rotation of the loop. Similar ideas were later applied to two-dimensional topological sigma model [8] and four dimensional topological gauge theory [9]. In the 1990's the ideas of localization were widely used in the setup of cohomological topological field theories, e.g. see [10] for nice applications of these ideas to two-dimensional Yang-Mills theory. Further development on supersymmetric localization is related to the calculation of Nekrasov's partition function, or equivariant Donaldson-Witten theory [11], based on earlier works [12–15].

The focus of this volume is on the developments starting from the work [16], where the exact partition function and the expectation values of Wilson loops for  $\mathcal{N} = 2$  supersymmetric gauge theories on  $S^4$  were calculated. In [16] the 4d  $\mathcal{N} = 2$  theory was placed on  $S^4$ , preserving 8 supercharges, and the supersymmetry transformations together with BRST-transformations were recognized as the equivariant differential on the space of fields. The zero modes were carefully treated by Atiyah-Singer index theorem, and the final result was written as a finite-dimensional integral over the Cartan algebra of the Lie algebra of the gauge group. Later this calculation was generalized and extended to other types of supersymmetric theories, other dimensions and geometries. These exact results provide a unique laboratory for the study of non-perturbative properties of gauge theories. Some contributions to this volume provide an overview of the actual localization calculation in concrete dimensions, for concrete class of theories, while other contributions look at the applications of the results and discuss their physical and mathematical significance.

## 1.2 Localization in diverse dimensions

In order to apply the localization technique to supersymmetric theories one needs to resolve a number of technical and conceptual problems. First of all, one needs to define a rigid supersymmetric theory on curved manifolds and understand what geometrical data goes into the construction. The old idea was that rigid supersymmetry on curved manifolds requires an existence of covariantly constant spinors which would correspond to the parameters in the supersymmetry transformations. The next natural generalization would be if the supersymmetry parameters satisfy the Killing spinor equations [17]. For example, all spheres admit Killing spinors and thus supersymmetric gauge theories can be constructed on spheres. However, a more systematic view on supersymmetric rigid theories on curved manifolds has been suggested in [18] giving background values to auxiliary fields in the supergravity. (More recently an approach of topological gravity was explored in [19, 20].) This approach allows in principle to analyze rigid supersymmetric theories on curved manifolds, although the analysis appears to be increasingly complicated as we deal with higher dimensions and more supersymmetry. At the moment we know how to place on a curved manifold the

supersymmetric theories, which in flat space have four or fewer supercharges, in dimension 2,3 and 4 for both Euclidean and Lorentzian signatures [21–24]. For other cases only partial results are available. For example, in four dimensions the situation for theories with eight supercharges remains open, see e.g. [25–27]. Situation is similar in five dimensions, see e.g. [28–30] and in six dimensions [31]; see also [32, 33] in the context of superspace treatment of rigid supergravity. Thus despite the surge in the activity the full classification of supersymmetric theories on curved manifolds remains an open problem. Rigid supersymmetric theories on curved manifolds are discussed in Chapter 5.

Moreover, in order to be able to carry the localization calculation explicitly and write the result in closed form, we need manifolds with enough symmetries, for example with a rich toric action. Again we do not know the full classification of curved manifolds that allow both a toric action and a rigid supersymmetric gauge theory. In 3d we know how to localize the theories with 4 supercharges on  $S^3$ , on lens spaces  $L_p$  and on  $S^2 \times S^1$ . In 4d the situation becomes more complicated, we know how to localize the theories with 8 supercharges on  $S^4$  and with 4 supercharges on  $S^3 \times S^1$ , but the general situation in 4d remains to be understood. In 5d there exists an infinite family of toric Sasaki-Einstein manifold ( $S^5$  is one of them) for which the result up to non-perturbative contributions can be written explicitly for the theories with 8 supercharges. Notice, however, that this is not the most general 5d manifolds which admit the rigid supersymmetry, e.g. a bit separated example is  $S^4 \times S^1$ . In 6d the nearly Kähler manifolds (e.g.,  $S^6$ ) will allow the theories with 16 supercharges and in 7d the toric Sasaki-Einstein manifolds (e.g.,  $S^7$ ) will allow the theories with 16 supercharges.

The best studied examples are the supersymmetric gauge theories on spheres  $S^d$ , which we are going to review briefly since they provide the nice illustration for the general results. The first results were obtained for  $S^4$  in [16], for  $S^3$  in [35], for  $S^2$  in [36, 37], for  $S^5$  in [38–40] and finally for  $S^6$  and  $S^7$  were addressed in [41]. These calculations were generalized and extended to the squashed  $S^3$  [42, 43], to the squashed  $S^4$  [27, 44], the squashed  $S^5$  [45–47] and the result for the squashed  $S^6$  and  $S^7$  was already suggested in [41]. There is also an attempt in [48] to analytically continue the partition function on  $S^d$  to generic complex values of  $d$ .

Let us describe the result for different spheres in a uniform fashion. We consider the general case of squashed spheres.

The odd and even dimensional spheres  $S^{2r-1}$  and  $S^{2r}$  lead to two types of special functions called  $S_r$  and  $\Upsilon_r$  that are used to present the result.

The main building block of these functions is the multiple inverse Gamma function  $\gamma_r(x|\epsilon_1, \dots, \epsilon_r)$ , which is a function of a variable  $x$  on the complex plane  $\mathbb{C}$  and  $r$  complex parameters  $\epsilon_1, \dots, \epsilon_r$ . This function is defined as a  $\zeta$ -regularized product

$$\gamma_r(x|\epsilon_1, \dots, \epsilon_r) = \prod_{n_1, \dots, n_r=0}^{\infty} (x + n_1\epsilon_1 + \dots + n_r\epsilon_r), \quad (1.2.1)$$

The parameters  $\epsilon_i$  should belong to an open half-plane of  $\mathbb{C}$  bounded by a real line passing through the origin. The unrefined version of  $\gamma_r$  is defined as

$$\gamma_r(x) = \gamma_r(x|1, \dots, 1) = \prod_{k=0}^{\infty} (x+k)^{\frac{(k+1)(k+2)\dots(k+r-1)}{(r-1)!}}. \quad (1.2.2)$$

The  $\Upsilon_r$ -function, obtained from the localization on  $S^{2r}$ , is defined as

$$\Upsilon_r(x|\epsilon_1, \dots, \epsilon_r) = \gamma_r(x|\epsilon_1, \dots, \epsilon_r) \gamma_r\left(\sum_{i=1}^r \epsilon_i - x|\epsilon_1, \dots, \epsilon_r\right)^{(-1)^r}. \quad (1.2.3)$$

These functions form a hierarchy with respect to a shift of  $x$  by one of  $\epsilon$ -parameters

$$\Upsilon_r(x + \epsilon_i|\epsilon_1, \dots, \epsilon_i, \dots, \epsilon_r) = \Upsilon_{r-1}^{-1}(x|\epsilon_1, \dots, \epsilon_{i-1}, \epsilon_{i+1}, \dots, \epsilon_r) \Upsilon_r(x|\epsilon_1, \dots, \epsilon_i, \dots, \epsilon_r) \quad (1.2.4)$$

The unrefined version of  $\Upsilon_r$  is defined as follows

$$\Upsilon_r(x) = \Upsilon_r(x|1, \dots, 1) = \prod_{k \in \mathbb{Z}} (k+x)^{\text{sgn}(k+1) \frac{(k+1)(k+2)\dots(k+r-1)}{(r-1)!}}. \quad (1.2.5)$$

The  $S_r$ -function, called multiple sine, obtained from localization on  $S^{2r-1}$ , is defined as

$$S_r(x|\epsilon_1, \dots, \epsilon_r) = \gamma_r(x|\epsilon_1, \dots, \epsilon_r) \gamma_r\left(\sum_{i=1}^r \epsilon_i - x|\epsilon_1, \dots, \epsilon_r\right)^{(-1)^{r-1}}. \quad (1.2.6)$$

See [49] for exposition and further references. These functions also form a hierarchy with respect to a shift of  $x$  by one of the  $\epsilon$ -parameters

$$S_r(x + \epsilon_i|\epsilon_1, \dots, \epsilon_i, \dots, \epsilon_r) = S_{r-1}^{-1}(x|\epsilon_1, \dots, \epsilon_{i-1}, \epsilon_{i+1}, \dots, \epsilon_r) S_r(x|\epsilon_1, \dots, \epsilon_i, \dots, \epsilon_r). \quad (1.2.7)$$

Notice that  $S_1(x|\epsilon) = 2 \sin(\frac{\pi x}{\epsilon})$  is a periodic function. Thus  $S_1$  is periodic by itself,  $S_2$  is periodic up to  $S_1^{-1}$ ,  $S_3$  is periodic up to  $S_2^{-1}$  etc. The unrefined version of multiple sine is defined as

$$S_r(x) = S_r(x|1, \dots, 1) = \prod_{k \in \mathbb{Z}} (k+x)^{\frac{(k+1)(k+2)\dots(k+r-1)}{(r-1)!}}. \quad (1.2.8)$$

The result for a vector multiplet with 4, 8 and 16 supercharges placed on a sphere  $S^2, S^4$  and  $S^6$  respectively is given in terms of  $\Upsilon_r$  functions as follows

$$Z_{S^{2r}} = \int_{\mathfrak{t}} da \prod_{w \in R_{\text{ad } \mathfrak{g}}} \Upsilon_r(iw \cdot a|\epsilon) e^{P_r(a)} + \dots, \quad (1.2.9)$$

where the integral is taken over the Cartan subalgebra of the gauge Lie algebra  $\mathfrak{g}$ , the  $w$  are weights of the adjoint representation of  $\mathfrak{g}$  and  $P_r(a)$  is the polynomial in  $a$  of degree  $r$ ,

$$P_r(a) = \alpha_r \text{Tr}(a^r) + \dots + \alpha_2 \text{Tr}(a^2) + \alpha_1 \text{Tr}(a). \quad (1.2.10)$$

The polynomial  $P_r(a)$  is coming from the classical action of the theory. The parameters  $\alpha_i$  are related to the Yang-Mills coupling, the Chern-Simons couplings and the FI couplings.

The sphere  $S^{2r}$  admits  $T^r$  action with two fixed points, and the parameters  $\epsilon_1, \dots, \epsilon_r$  are the squashing parameters for  $S^{2r}$  (at the same time  $\epsilon_1, \dots, \epsilon_r$  are equivariant parameters for the  $T^r$  action).

For  $S^2$ , the dots are non-perturbative contributions coming from other localization loci with non-trivial magnetic fluxes (review in Chapter 3). For  $S^4$ , the dots correspond to the contributions of point-like instantons over the north and south poles computed by the Nekrasov instanton partition function (review in Chapter 10). For the case of  $S^6$  the expression corresponds to maximally supersymmetric theory on  $S^6$ , and the nature of the dots remains to be understood.

The partition function of the vector multiplet with 4, 8, or 16 supercharges on the odd-dimensional spheres  $S^3$ ,  $S^5$  and  $S^7$ , or  $S^{2r-1}$  with  $r = 2, 3, 4$ , is given by

$$Z_{S^{2r-1}} = \int_{\mathfrak{t}} da \prod_{w \in R_{\text{ad g}}} S_r(iw \cdot a | \epsilon) e^{P_r(a)} + \dots, \quad (1.2.11)$$

where now  $\epsilon$ -parameters are equivariant parameters of the  $T^r \subset SO(2r)$  toric action on  $S^{2r-1}$ .

For  $S^3$  the dots are absent and the expression (1.2.11) provides the full results for  $\mathcal{N} = 2$  vector multiplet on  $S^3$  (review in Chapter 6). For  $S^5$  the formula (1.2.11) provides the result for  $\mathcal{N} = 1$  vector multiplet (review in Chapter 14). The theory on  $S^7$  is unique and it corresponds to the maximally supersymmetric Yang-Mills in 7d with 16 supercharges.

For the case of  $S^5$  and  $S^7$  the dots are there and they correspond to the contributions around non-trivial connection satisfying certain non-linear PDEs. There are some natural guesses about these corrections, but there are no systematic derivation and no understanding of them, especially for the case of  $S^7$ .

Our present discussion can be summarized in the following table:

| dim   | multiplet                | #super | special function         | references | derivation |
|-------|--------------------------|--------|--------------------------|------------|------------|
| $S^2$ | $\mathcal{N} = 2$ vector | 4      | $\Upsilon_1(x \epsilon)$ | [36, 37]   | Chapter 3  |
| $S^3$ | $\mathcal{N} = 2$ vector | 4      | $S_2(x \epsilon)$        | [35]       | Chapter 6  |
| $S^4$ | $\mathcal{N} = 2$ vector | 8      | $\Upsilon_2(x \epsilon)$ | [16]       | Chapter 10 |
| $S^5$ | $\mathcal{N} = 1$ vector | 8      | $S_3(x \epsilon)$        | [38–40]    | Chapter 14 |
| $S^6$ | $\mathcal{N} = 2$ vector | 16     | $\Upsilon_3(x \epsilon)$ | [41]       |            |
| $S^7$ | $\mathcal{N} = 1$ vector | 16     | $S_4(x \epsilon)$        | [41]       |            |

The contribution of matter multiplet (chiral multiplet for theories with 4 supercharges and hypermultiplets for theories with 8 supercharges) can be expressed in terms of the same special functions, see next section.

The detailed discussion of the localization calculation on the spheres and other manifolds can be found in different contributions in this volume, 2d is discussed in Chapter 3, 3d in Chapter 6, 4d in Chapter 10, 5d in Chapter 14.

Next we can schematically explain the above result.

### 1.2.1 Topological Yang-Mills

We recall that  $\mathcal{N} = 1$  super Yang-Mills theory is defined in dimension  $d = 3, 4, 6, 10$  and that the algebraic structure of supersymmetry transformations is related to an isomorphism that one can establish between  $\mathbb{R}^{d-2}$  and the famous four division algebras:

| SYM | algebra      | S                          | dim S | top SYM | equations                     | #equations | quotient    |
|-----|--------------|----------------------------|-------|---------|-------------------------------|------------|-------------|
| 3d  | $\mathbb{R}$ | $S$                        | 2     | 1d      | —                             | 0          | —           |
| 4d  | $\mathbb{C}$ | $S$                        | 4     | 2d      | $F = 0$                       | 1          | Kahler      |
| 6d  | $\mathbb{H}$ | $S^+ \otimes \mathbb{C}^2$ | 8     | 4d      | $F = -\star F$                | 3          | hyperKahler |
| 10d | $\mathbb{O}$ | $S^+$                      | 16    | 8d      | $F = -\star(F \wedge \Omega)$ | 7          | octonionic  |

In this table  $S$  denotes the  $2^{\lfloor d/2 \rfloor}$ -dimensional Dirac spinor representation of  $Spin(d)$  group. The  $S^+$  denotes the chiral (Weyl) spinor representation of  $Spin(d)$ . In all cases, one uses Majorana spinors in Lorenzian signature, or *holomorphic Dirac*<sup>2</sup> spinors in Euclidean signature. Notice the peculiarity of the 6d case where one uses chiral  $Sp(1)$ -doublet spinors with  $\mathbb{C}^2$  being the fundamental representation of the  $Sp(1) \simeq SU(2)$  R-symmetry, and that in the 10d case one uses a single copy of the chiral spinor representation. The number  $\dim S$  is often referred as the *the number of the supercharges in the theory*.

Also, it is well known that the  $\mathcal{N} = 1$  under the dimensional reduction to the dimension  $d - 2$  produces the ‘topological’ SYM which localizes to the solutions of certain first order (BPS type) elliptic equations on the gauge field strength of the curvature listed in the table. The 1d topYM is, of course, the trivial theory, with empty equations, since there is no room for the curvature 2-form in a 1-dimensional theory. The equation for 2d topYM is the equation of zero curvature, for 4d topYM it is the instanton equation of self-dual curvature (defined by the conformal structure on the 4d manifold), and for 8d topYM it is the equation of the octonionic instanton (defined by the Hodge star  $\star$  operator and the Cayley 4-form  $\Omega$  on a  $Spin(7)$ -holonomy 8d manifold).

The corresponding linearized complexes are

| topYM             | linearized complex                                                | fiber dimensions                                           |
|-------------------|-------------------------------------------------------------------|------------------------------------------------------------|
| $\mathbb{R}$ : 1d | $\Omega^0 \rightarrow \Omega^1$                                   | $\mathbf{1} \rightarrow \mathbf{1}$                        |
| $\mathbb{C}$ : 2d | $\Omega^0 \rightarrow \Omega^1 \rightarrow \Omega^2$              | $\mathbf{1} \rightarrow \mathbf{2} \rightarrow \mathbf{1}$ |
| $\mathbb{H}$ : 4d | $\Omega^0 \rightarrow \Omega^1 \rightarrow \Omega_+^2$            | $\mathbf{1} \rightarrow \mathbf{4} \rightarrow \mathbf{3}$ |
| $\mathbb{O}$ : 8d | $\Omega^0 \rightarrow \Omega^1 \rightarrow \Omega_{\text{oct}}^2$ | $\mathbf{1} \rightarrow \mathbf{8} \rightarrow \mathbf{7}$ |

(1.2.12)

Here  $\Omega^p$  is a shorthand for  $\Omega^p(X) \otimes \text{ad } \mathfrak{g}$ , that is the space of  $\mathfrak{g}$ -valued differential  $p$ -forms on  $X$ , where  $\mathfrak{g}$  is the Lie algebra of the gauge group and  $X$  is the space-time manifold. In the 4d theory the space  $\Omega_+^2$  denotes the space of self-dual 2-forms that satisfy the instanton equation  $F = -\star F$ , and in the 8d theory the space  $\Omega_{\text{oct}}^2$  is the space of 2-forms that satisfy the octonionic instanton equation  $F = -\star(F \wedge \Omega)$ .

In these complexes, the first term  $\Omega^0$  describes the tangent space to the infinite-dimensional group of gauge transformations on  $X$ , the second term  $\Omega^1$  describes the tangent space to the affine space of gauge connections on  $X$ , and the last term ( $\Omega^2$  for 2d,  $\Omega_+^2$  for 4d,  $\Omega_{\text{oct}}^2$  for 8d) describes that space where the equations are valued.

If space-time  $X$  is invariant under an isometry group  $T$ , the topological YM can be treated equivariantly with respect to the  $T$ -action. The prototypical case is the equivariant

---

<sup>2</sup>This means that the spinors  $\psi$  in Euclidean signature are taken to be complex, but algebraically speaking, only  $\psi$  appears in the theory but not its complex conjugate  $\bar{\psi}$

Donaldson-Witten theory, or 4d topYM in  $\Omega$ -background defined on  $\mathbb{R}^4$  equivariantly with respect to  $T = SO(4)$ , generating the Nekrasov partition function [11]. Special functions, like the  $\Upsilon$ -function defined by infinite products like (1.2.3) are infinite-dimensional versions of the equivariant Euler class of the tangent bundle to the space of all fields appearing after localization of the path integral by Atiyah-Bott fixed point formula (see Chapter 2 section 8.1 for more details). The equivariant Euler class can be determined by computing first the equivariant Chern class (index) of the linearized complex describing the tangent space of the topological YM theory. The  $T$ -equivariant Chern class (index) for the equation elliptic complex

$$D : \cdots \rightarrow \Gamma(E_k, X) \rightarrow \Gamma(E_{k+1}, X) \rightarrow \cdots \quad (1.2.13)$$

on space  $X$  made from sections of vector bundles  $E_\bullet$ , can be conveniently computed by the Atiyah-Singer index theorem

$$\text{ind}_T(D) = \sum_{x \in X^T} \frac{\sum_k (-1)^k \text{ch}_T(E_k)|_x}{\det_{T_x X}(1 - t^{-1})} \quad (1.2.14)$$

where  $X^T$  is the fixed point set of  $T$  on  $X$  (see Chapter 2 section 11.1 for details).

## 1.2.2 Even dimensions

First we will apply the Atiyah-Singer index theorem (review in Chapter 2 section 11.1) for the *complexified* complexes (1.2.12) on  $X = \mathbb{R}^d$  for  $d = 2, 4, 8$  topological YM with respect to the natural  $SO(d)$  equivariant action on  $\mathbb{R}^d$  with fixed point  $x = 0$ .

For  $d = 2r$  and  $r = 1, 2, 4$  we pick the Cartan torus  $T^r = U(1)^r$  in the  $SO(2r)$  with parameters  $(t_1, \dots, t_r) \in U(1)^r$ . The denominator in the Atiyah-Singer index theorem is

$$\det(1 - t^{-1})|_{\mathbb{R}^{2r}} = \prod_{s=1}^n (1 - t_s)(1 - t_s^{-1}) \quad (1.2.15)$$

The numerator is obtained by computing the graded trace over the fiber of the equation complex at the fixed point  $x = 0$ .

For equivariant 2d topYM on  $\mathbb{R}^2$  (coming from SYM with 4 supercharges):

$$\text{ind}_T(D, \mathbb{R}^2, \Omega_{\mathbb{C}}^0 \rightarrow \Omega_{\mathbb{C}}^1 \rightarrow \Omega_{\mathbb{C}}^2)_{2\text{d}} = \frac{1 - (t_1 + t_1^{-1}) + 1}{(1 - t_1)(1 - t_1^{-1})} = \frac{1}{1 - t_1} + \frac{1}{1 - t_1^{-1}} \quad (1.2.16)$$

For equivariant 4d topYM on  $\mathbb{R}^4$  (coming from SYM with 8 supercharges):

$$\begin{aligned} \text{ind}_T(D, \mathbb{R}^4, \Omega_{\mathbb{C}}^0 \rightarrow \Omega_{\mathbb{C}}^1 \rightarrow \Omega_{\mathbb{C}}^{2+})_{4\text{d}} &= \frac{1 - (t_1 + t_1^{-1} + t_2 + t_2^{-1}) + (1 + t_1 t_2 + t_1^{-1} t_2^{-1})}{(1 - t_1)(1 - t_1^{-1})(1 - t_2)(1 - t_2^{-1})} \\ &= \frac{1}{(1 - t_1)(1 - t_2)} + \frac{1}{(1 - t_1^{-1})(1 - t_2^{-1})} \end{aligned} \quad (1.2.17)$$

For equivariant 8d topYM on  $\mathbb{R}^8$  (coming from SYM with 16 supercharges), to preserve the Cayley form and the octonionic equations coming from the  $Spin(7)$  structure, the 4 parameters  $(t_1, t_2, t_3, t_4)$  should satisfy the constraint  $t_1 t_2 t_3 t_4 = 1$ . The weights on 7-dimensional bundle, whose sections are  $\Omega_{\text{oct}, \mathbb{C}}^2$ , can be computed from the weights of the chiral spinor bundle  $S^+$  modulo the trivial bundle. The chiral spinor bundle  $S^+$  can be identified (after a choice of complex structure on  $X$ ) as  $S^+ \simeq (\oplus_{p=0}^2 \Lambda^{2p} T_X^{0,1}) \otimes K^{\frac{1}{2}}$  where  $K$  is the canonical bundle on  $X = \mathbb{R}^8 \simeq \mathbb{C}^4$  equivariantly trivial with respect to the  $T^3$  action parametrized by  $(t_1, t_2, t_3, t_4)$  with  $t_1 t_2 t_3 t_4 = 1$ . Then

$$\begin{aligned} \text{ind}_T(D, \mathbb{R}^8, \Omega_{\mathbb{C}}^0 \rightarrow \Omega_{\mathbb{C}}^1 \rightarrow \Omega_{\text{oct}, \mathbb{C}}^2)_{8\text{d}} &= \frac{(1 - (\sum_{s=1}^4 (t_s + t_s^{-1}))) + (1 + \sum_{1 \leq r < s \leq 4} t_r t_s)}{\prod_{s=1}^4 (1 - t_s)(1 - t_s^{-1})} = \\ &= \frac{1}{(1 - t_1)(1 - t_2)(1 - t_3)(1 - t_4)}, \quad t_1 t_2 t_3 t_4 = 1 \end{aligned} \quad (1.2.18)$$

It is also interesting to consider the dimensional reduction of the 8d topYM (coming from the SYM with 16 supercharges) to the 6d theory. The numerator in the index is computed in the same way as (1.2.18), but the denominator is changed to the 6d determinant, hence we find

$$\begin{aligned} \text{ind}_T(D, \mathbb{R}^6, \Omega_{\mathbb{C}}^0 \rightarrow \Omega_{\mathbb{C}}^1 \rightarrow \Omega_{\mathbb{C}}^{2, \text{oct}})_{6\text{d reduction}} &= \frac{(1 - (\sum_{s=1}^4 (t_s + t_s^{-1}))) + (1 + \sum_{1 \leq r < s \leq 4} t_r t_s)}{\prod_{s=1}^3 (1 - t_s)(1 - t_s^{-1})} = \\ &= \frac{1 - t_4^{-1}}{(1 - t_1)(1 - t_2)(1 - t_3)} \stackrel{t_1 t_2 t_3 t_4 = 1}{=} \\ &= \frac{1}{(1 - t_1)(1 - t_2)(1 - t_3)} + \frac{1}{(1 - t_1^{-1})(1 - t_2^{-1})(1 - t_3^{-1})} \end{aligned} \quad (1.2.19)$$

From equations (1.2.16)(1.2.17)(1.2.19) we see that the index for the complexified vector multiplet of the 2d theory (4 supercharges), 4d theory (8 supercharges) and 6d theory (16 supercharges) on  $\mathbb{R}^{2r}$  can be uniformly written in the form

$$\text{ind}_T(D, \mathbb{R}^{2r}, \text{vector}_{\mathbb{C}}) = \frac{1 + (-1)^r \prod_{s=1}^r t_s}{\prod_{s=1}^r (1 - t_s)} = \frac{1}{\prod_{s=1}^r (1 - t_s)} + \frac{1}{\prod_{s=1}^r (1 - t_s^{-1})} \quad r = 1, 2, 3 \quad (1.2.20)$$

Hence, the equivariant index of the complexified vector multiplet in 2,4 and 6 dimensions on flat space is equivalent to the index of the Dolbeault complex plus its dual, because (see review in Chapter 2 section 9)

$$\text{ind}_T(\bar{\partial}, \mathbb{C}^{2r}, \Omega^{0, \bullet}) = \frac{1}{\prod_{s=1}^r (1 - t_s^{-1})} \quad (1.2.21)$$

The vector multiplet is in a real representation of the equivariant group: each non-zero weight eigenspace appears together with its dual. Generally, the index of a real representation has the form

$$f(t_1, \dots, t_r) + f(t_1^{-1}, \dots, t_r^{-1}) \quad (1.2.22)$$

The equivariant Euler class in the denominator of the Atiyah-Bott localization formula (Chapter 2 section 8.1 and section 12) is defined as the Pfaffian rather than the determinant, hence each pair of terms in the equivariant index, describing a weight space and its dual, corresponds to a single weight factor in the equivariant Euler class. The choice between two opposite weights leads to a sign issue, which depends on the choice of the orientation on the infinite-dimensional space of all field modes. A careful treatment leads to interesting sign factors discussed in details for example in Chapter 3.

A natural choice of orientation leads to the holomorphic projection of the vector multiplet index (1.2.20) in 2, 4 and 6 dimensions by picking only the first term in (1.2.20) so that

$$\text{ind}_T(D, \mathbb{R}^{2r}, \text{vector}_{\mathbb{C}})_{\text{hol}} = \frac{1}{\prod_{s=1}^r (1 - t_s)} \quad r = 1, 2, 3 \quad (1.2.23)$$

The supersymmetric Yang-Mills with 4, 8 and 16 supercharges can be put on the spheres  $S^2$ ,  $S^4$  and  $S^6$  as was done in [16], [36], [37], [41] and reviewed in Chapter 3 and Chapter 10.

A certain generator  $Q_\epsilon$  of the global superconformal group can be used for the localization computation. This generator  $Q_\epsilon$  is represented by a conformal Killing spinor  $\epsilon$  on a sphere  $S^{2r}$ , and satisfies  $Q_\epsilon^2 = R$  where  $R$  is a rotation isometry. There are two fixed points of  $R$  on an even-dimensional sphere, usually called the north and the south poles. It turns out that the equivariant elliptic complex of equations, describing the equations of the topological YM, is replaced by a certain equivariant transversally elliptic complex of equations. Near the north pole this complex is approximated by the equivariant topological YM theory (theory in  $\Omega$ -background), and near the south pole by its conjugate.

The index of the transversally elliptic operator can be computed by the Atiyah-Singer theorem, see for the complete treatment [54], application [16], Chapter 2 or Chapter 10. The result is that the index is contributed by the two fixed point on the sphere  $S^{2r}$ , with a particular choice of the distribution associated to the rational function, in other words with a particular choice of expansion in positive or negative powers of  $t_s$ , denoted by  $[\ ]_+$  or  $[\ ]_-$  respectively (see Chapter 2 section 11.1):

$$\text{ind}_T(D, S^{2r}, \text{vector}_{\mathbb{C}})_{\text{hol}} = \left[ \frac{1}{\prod_{s=1}^r (1 - t_s)} \right]_+ + \left[ \frac{1}{\prod_{s=1}^r (1 - t_s)} \right]_- \quad r = 1, 2, 3 \quad (1.2.24)$$

So far we have computed only the space-time geometrical part of the index. Now, suppose that the multiplet is tensored with a representation of a group  $G$  (like the gauge symmetry, R-symmetry or flavour symmetry), and let  $L_\xi \simeq \mathbb{C}$  be a complex eigenspace in representation of  $G$  with eigenweight  $\xi = e^{ix}$ . Then

$$\text{ind}_{T \times G}(D, S^{2r}, \text{vector}_{\mathbb{C}} \otimes L_\xi)_{\text{hol}} = \left[ \frac{\xi}{\prod_{s=1}^r (1 - t_s)} \right]_+ + \left[ \frac{\xi}{\prod_{s=1}^r (1 - t_s)} \right]_- \quad (1.2.25)$$

Now let  $\epsilon_s$  and  $x$  be the Lie algebra parameters associated with the group parameters  $t_s$  and  $\xi$  as

$$t_s = \exp(i\epsilon_s), \quad \xi = \exp(ix) \quad (1.2.26)$$

By definition, let  $\Upsilon_r(x|\epsilon)$  be the equivariant Euler class (Pfaffian) of the graded vector space of fields of a vector multiplet on  $S^{2r}$  with the character (index) defined by (1.2.25)

$$\Upsilon_r(x|\epsilon) = \text{eu}_{T \times G}(D, S^{2r}, \text{vector}_{\mathbb{C}} \otimes L_{\xi})_{\text{hol}}|_{t_s=e^{i\epsilon_s}, \xi=e^{ix}} \quad (1.2.27)$$

Explicitly, converting the infinite Taylor sum series of (1.2.25)

$$\left[ \frac{\xi}{\prod_{s=1}^r (1-t_s)} \right]_+ + \left[ \frac{\xi}{\prod_{s=1}^r (1-t_s)} \right]_- = \sum_{n_1=0, \dots, n_r=0}^{\infty} \xi (t_1^{n_1} \dots t_r^{n_r} + (-1)^r t_1^{-1-n_1} \dots t_r^{-1-n_r}) \quad (1.2.28)$$

into the product of weights we find the infinite-product definition of the  $\Upsilon_r(x|\epsilon)$  function

$$\Upsilon_r(x|s) \stackrel{\text{reg}}{=} \prod_{n_1=0, \dots, n_r=0}^{\infty} \left( x + \sum_{s=1}^r n_s \epsilon_s \right) \left( \epsilon - x + \sum_{s=1}^r n_s \epsilon_s \right)^{(-1)^r} \quad (1.2.29)$$

where  $\stackrel{\text{reg}}{=}$  denotes Weierstrass or  $\zeta$ -function regularization and

$$\epsilon = \epsilon_1 + \dots + \epsilon_r \quad (1.2.30)$$

The analysis for the scalar multiplet (the chiral multiplet in 2d for the theory with 4 supercharges or the hypermultiplet in 4d for the theory with 8 supercharges) is similar. On equivariant  $\mathbb{R}^{2r}$  the corresponding complex for the scalar multiplet is the Dirac operator  $S^+ \rightarrow S^-$ , which differs from the Dolbeault complex by the twist by the square root of the canonical bundle, hence

$$\text{ind}_T(D, \mathbb{R}^{2r}, \text{scalar})_{\text{hol}} = -\frac{\prod_{s=1}^r t_s^{\frac{1}{2}}}{\prod_{s=1}^r (1-t_s)} \quad r = 1, 2 \quad (1.2.31)$$

On the sphere  $S^{2r}$ , again, one takes the contribution from the north and the south pole approximated locally by  $\mathbb{R}^{2r}$  with opposite orientations, and gets

$$\text{ind}_T(D, S^{2r}, \text{scalar})_{\text{hol}} = -\left[ \frac{\prod_{s=1}^r t_s^{\frac{1}{2}}}{\prod_{s=1}^r (1-t_s)} \right]_+ - \left[ \frac{\prod_{s=1}^r t_s^{\frac{1}{2}}}{\prod_{s=1}^r (1-t_s)} \right]_- \quad r = 1, 2 \quad (1.2.32)$$

Hence, the equivariant Euler class of the graded space of sections of the scalar multiplet is obtained simply by a shift of the argument of the  $\Upsilon$ -function and inversion

$$\text{eu}_{T \times G}(D, S^{2r}, \text{scalar} \otimes L_{\xi})_{\text{hol}}|_{t_s=e^{i\epsilon_s}, w=e^{ix}} = \Upsilon_r \left( x + \frac{\epsilon}{2} \right)^{-1} \quad (1.2.33)$$

As computed in [16], [36], [37], [41] and reviewed in Chapter 3 and Chapter 10, the localization by the Atiyah-Bott formula brings the partition function of supersymmetric Yang-Mills with 4, 8 and 16 supercharges on the spheres  $S^2$ ,  $S^4$  and  $S^6$  to the form of an integral over the imaginary line contour in the complexified Lie algebra of the Cartan

torus of the gauge group (the zero mode of one of the scalar fields in the vector multiplet). The integrand is a product of the classical factor induced from the classical action and the determinant factor (the inverse of the equivariant Euler class of the tangent space to the space of fields) which has been computed above in terms of the  $\Upsilon_r$ -function. Hence, for  $r = 1, 2, 3$  we get perturbatively exact result of the partition function in the form of a finite-dimensional integral over the Cartan subalgebra of the Lie algebra of the gauge group (generalized matrix model)

$$Z_{S^{2r}, \text{pert}} = \int_{\mathfrak{t}_G} da \frac{\prod_{w \in R_{\text{ad } \mathfrak{g}}} \Upsilon_r(iw \cdot a | \epsilon)}{\prod_{w \in R_{G \times F}} \Upsilon_r(iw \cdot (a, m) + \frac{\epsilon}{2} | \epsilon)} e^{P(a)} \quad (1.2.34)$$

Hence  $Z_{S^{2r}, \text{pert}}$  is the contribution to the partition function of the trivial localization locus (all fields vanish except the zero mode  $a$  of one of the scalars of the vector multiplet and some auxiliary fields). The  $Z_{S^{2r}, \text{pert}}$  does not include the non-perturbative contributions. The factor  $e^{P(a)}$  is induced by the classical action evaluated at the localization locus. The product of  $\Upsilon_r$ -functions in the numerator comes from the vector multiplet and it runs over the weights of the adjoint representation. The product of  $\Upsilon_r$ -functions in the denominator comes from the scalar multiplet (chiral or hyper), and it runs over the weights of a complex representation  $R_G$  of the gauge group  $G$  in which the scalar multiplet transforms. In addition, by taking the matter fields multiplets to be in a representation of a flavor symmetry  $F$ , the mass parameters  $m \in \mathfrak{t}_F$  can be introduced naturally. For  $r = 3$  the denominator is empty, because the 6d gauge theory with 16 supercharges is formed only from the gauge vector multiplet.

The non-perturbative contributions come from other localization loci, such as magnetic fluxes on  $S^2$ , or instantons on  $S^4$ , and their effect modifies the equivariant Euler classes presented as  $\Upsilon_r$ -factors in (1.2.34) by certain rational factors. The 4d non-perturbative contributions are captured by fusion of Nekrasov instanton partition function with its conjugate [11, 16]. See 2d details in Chapter 3 and 4d details in Chapter 10.

Much before localization results on gauge theory on  $S^4$  were obtained, the  $\Upsilon_2$  function prominently appeared in Zamolodchikov-Zamolodchikov paper [55] on structure functions of 2d Liouville CFT. The coincidence was one of the key observations by Alday-Gaiotto-Tachikawa [56] that led to a remarkable 2d/4d correspondence (AGT) between correlators in Liouville (Toda) theory and gauge theory partition functions on  $S^4$ , see review in Chapter 12.

### 1.2.3 Odd dimensions

Next we discuss the odd dimensional spheres (in principle, this discussion is applicable for any simply connected Sasaki-Einstein manifold, i.e. the manifold  $X$  admits at least two Killing spinors). After field redefinitions, which involve the Killing spinors, the integration space for odd dimensional supersymmetric gauge theories with the gauged fixing fields can be represented as the following spaces

$$\begin{aligned} 3\text{d} : & \quad \mathcal{A}(X, \mathfrak{g}) \times \Pi\Omega^0(X, \mathfrak{g}) \times \Pi\Omega^0(X, \mathfrak{g}) \times \Pi\Omega^0(X, \mathfrak{g}) \\ 5\text{d} : & \quad \mathcal{A}(X, \mathfrak{g}) \times \Pi\Omega_H^{2,+}(X, \mathfrak{g}) \times \Pi\Omega^0(X, \mathfrak{g}) \times \Pi\Omega^0(X, \mathfrak{g}) \\ 7\text{d} : & \quad \mathcal{A}(X, \mathfrak{g}) \times \Omega_H^{3,0}(X, \mathfrak{g}) \times \Pi\Omega_H^{2,+}(X, \mathfrak{g}) \times \Pi\Omega^0(X, \mathfrak{g}) \times \Pi\Omega^0(X, \mathfrak{g}) \end{aligned} \quad (1.2.35)$$

where in all cases there are common last two factors  $\Pi\Omega^0(X, \mathfrak{g}) \times \Pi\Omega^0(X, \mathfrak{g})$  coming from the gauge fixing. The space  $\mathcal{A}(X, \mathfrak{g})$  is the space of connections on  $X$  with the Lie algebra  $\mathfrak{g}$ . The Sasaki-Einstein manifold is a contact manifold and the differential forms can be naturally decomposed into vertical and horizontal forms using the Reeb vector field  $R$  and the contact form  $\kappa$ . The horizontal plane admits a complex structure and thus the horizontal forms can be decomposed further into  $(p, q)$ -forms. For two forms we define the space  $\Omega_H^{2,+}$  as  $(2, 0)$ -forms plus  $(0, 2)$ -forms plus forms proportional to  $d\kappa$ . Thus for 5d  $\Omega_H^{2,+}$  is the space of standard self-dual forms in four dimensions (rank 3 bundle), and for 7d forms in  $\Omega_H^{2,+}$  obey the hermitian Yang-Mills conditions in six dimensions (rank 7 bundle: 3 complex components and 1 real). By just counting degrees of freedom one can check that the 3d case corresponds to an  $\mathcal{N} = 2$  vector multiplet (4 supercharges), the 5d case to an  $\mathcal{N} = 1$  vector multiplet (8 supercharges) and 7d to  $\mathcal{N} = 1$  maximally supersymmetric theory (16 supercharges). The supersymmetry square  $Q_\epsilon^2$ , which acts on this space, is given by the sum of Lie derivative along the Reeb vector field  $R$  and constant gauge transformations:  $Q_\epsilon^2 = \mathcal{L}_R + ad_a$ . Around the trivial connection, after some cancelations, the problem boils down to the calculation of the following superdeterminant

$$Z_{S^{2r-1}} = \int_{\mathfrak{t}_G} da \, \text{sdet}_{\Omega_H^{(\bullet,0)}(X, \mathfrak{g})}(\mathcal{L}_R + ad_a) e^{P_r(a)} + \dots, \quad (1.2.36)$$

and this is a uniform description for Sasaki-Einstein manifolds in 3d, 5d and 7d. In 3d the only simply connected Sasaki-Einstein manifold is  $S^3$ , while in 5d and 7d there are many examples of simply connected Sasaki-Einstein manifolds (there is a rich class of the toric Sasaki-Einstein manifolds). The determinant can be calculated in many alternative ways, and the result depends on  $X$ .

If  $X$  is a sphere  $S^{2r-1}$ , the determinant in (1.2.36), equivalently, the inverse equivariant Euler class of the normal bundle to the localization locus in the space of all fields, can be computed from the equivariant Chern character, or the index, of a certain transversally elliptic operator  $D = \pi^* \bar{\partial}$  induced from the Dobeault operator  $\bar{\partial}$  by the Hopf fibration projection  $\pi : S^{2r-1} \rightarrow \mathbb{C}\mathbb{P}^{r-1}$ .

The index, or equivariant Chern character, is easy to compute by the Atiyah-Singer fixed point theorem (see the details in Chapter 2 section 11.2). The result is

$$\text{ind}_T(D, S^{2r-1}) = \sum_{n=-\infty}^{\infty} \text{ind}_T(\bar{\partial}, \mathbb{C}\mathbb{P}^{r-1}, \mathcal{O}(n)) = \left[ \frac{1}{\prod_{k=1}^r (1 - t_k)} \right]_+ + \left[ \frac{(-1)^{r-1} t_1^{-1} \dots t_r^{-1}}{\prod_{k=1}^r (1 - t_k^{-1})} \right]_- \quad (1.2.37)$$

Converting the additive equivariant Chern character to the multiplicative equivariant Euler character, we find the definition of the multiple sine function

$$S_r(x|\epsilon) = \text{eu}_{T \times G}(S^{2r-1}, D \otimes L_\xi)_{\text{hol}}|_{t_s = e^{i\epsilon_s}, \xi = e^{ix}} \quad (1.2.38)$$

where  $L_\xi$  is a 1-dimensional complex eigenspace with character  $\xi$ . Explicitly

$$S_r(x|\epsilon) \stackrel{\text{reg}}{=} \prod_{n_1=0, \dots, n_r=0}^{\infty} \left( x + \sum_{s=1}^r n_s \epsilon_s \right) \left( \epsilon - x + \sum_{s=1}^r n_s \epsilon_s \right)^{(-1)^{r-1}} \quad (1.2.39)$$

and this leads to the formula (1.2.11) for the perturbative part of the partition function of a vector multiplet on  $S^{2r-1}$ .

For  $r = 2, 3$  we can also treat a scalar supermultiplet (a chiral multiplet for the theory with 4 supercharges or a hypermultiplet for the theory with 8 supercharges). The corresponding complex is described by an elliptic operator  $\pi^* \not{D}$  for  $\pi : S^{2r-1} \rightarrow \mathbb{C}\mathbb{P}^{r-1}$ , where  $\not{D}$  is the Dirac operator  $S^+ \rightarrow S^-$  on  $\mathbb{C}\mathbb{P}^{r-1}$ . The Dirac complex is isomorphic to the Dolbeault complex by a twist by a square root of the canonical bundle. Because of the opposite statistics, there is also an overall sign factor like in (1.2.32).

Finally, the contribution of both vector multiplet in representation  $R_{\text{ad}_g}$  and scalar multiplet in representation  $R_{G \times F}$  to the perturbative part of the partition function is computed by the finite-dimensional integral over the localization locus  $\mathfrak{t}_G$  with the following integrand made of  $S_r$  functions

$$Z_{S^{2r-1}, \text{pert}} = \int_{\mathfrak{t}_G} da \frac{\prod_{w \in R_{\text{ad}_g}} S_r(iw \cdot a | \epsilon)}{\prod_{w \in R_{G \times F}} S_r(iw \cdot (a, m) + \frac{\epsilon}{2} | \epsilon)} e^{P(a)} \quad (1.2.40)$$

Here  $F$  is a possible flavor group of symmetry, and  $m \in \mathfrak{t}_F$  is a mass parameter.

For reviews of 3d localization see Chapter 6, Chapter 7, Chapter 8, Chapter 9 and for reviews of 5d localization see Chapter 14, Chapter 15, Chapter 16.

The case of  $S^n \times S^1$  is built from the trigonometric version of  $S^n$ -result.

The trigonometric version of the  $\Upsilon_r$ -function (1.2.29) is given by

$$H_r(x | \epsilon_1, \dots, \epsilon_r) = \prod_{n_1, \dots, n_r=0}^{\infty} \left( 1 - e^{2\pi i x} e^{2\pi i n \bar{\epsilon}} \right) \left( 1 - e^{2\pi i \left( \sum_{i=1}^r \epsilon_i - x \right)} e^{2\pi i n \bar{\epsilon}} \right)^{(-1)^r}. \quad (1.2.41)$$

The trigonometric version of the multiple sine function  $S_r$  (1.2.39) is given by the multiple elliptic gamma function

$$G_r(x | \epsilon_1, \dots, \epsilon_r) = \prod_{n_1, \dots, n_r=0}^{\infty} \left( 1 - e^{2\pi i x} e^{2\pi i n \bar{\epsilon}} \right) \left( 1 - e^{2\pi i \left( \sum_{i=1}^r \epsilon_i - x \right)} e^{2\pi i n \bar{\epsilon}} \right)^{(-1)^{r-1}}. \quad (1.2.42)$$

where  $G_1$  corresponds to the  $\theta$ -function,  $G_2$  corresponds to the elliptic gamma function.

The partition function on  $S^r \times S^1$  has an interpretation as a supersymmetric index, namely a graded trace over the Hilbert space. The review of supersymmetric index in 2d is in Chapter 3, in 4d is in Chapter 13 and in 6d is in Chapter 17.

### 1.3 Applications of the localization technique

The localization technique can be applied only to a very restricted set of supersymmetric observables, e.g. partition functions, supersymmetric Wilson loops etc. Unfortunately, the localization technique does not allow us to calculate correlators of generic local operators. However, the supersymmetric localization offers a unique opportunity to study the full

non-perturbative answer for these restricted class of observables and this is a powerful tool to inspect interacting quantum field theory. As one can see from the previous section, the localization results are given in terms of complicated finite dimensional integrals. Thus one has to develop techniques to study these integrals and learn how to deduce the relevant physical and mathematical information. Some of the reviews in this volume are dedicated to the study of the localization results (sometimes in various limits) and to the applications of these results in physics and mathematics.

The original motivation of [16] was to prove the Erickson-Semenoff-Zarembo and Drukker-Gross conjecture, which expresses the expectation value of supersymmetric circular Wilson loop operators in  $\mathcal{N} = 4$  supersymmetric Yang-Mills theory in terms of a Gaussian matrix model, see review in Chapter 11. This conjecture was actively used for checks of AdS/CFT correspondence. After more general localization results became available, they were also used for stronger tests of AdS/CFT.

On the AdS side, it is relatively easy to perform the calculation, since it requires only classical supergravity. However, on the gauge theory side, we need the full non-perturbative result in order to be able to compare it with the supergravity calculation. The localization technique offers us a unique opportunity for non-perturbative checks of AdS/CFT correspondence. A number of reviews are devoted to the use of localization for AdS/CFT correspondence: for AdS<sub>4</sub>/CFT<sub>3</sub> see review in Chapter 7 and Chapter 8, for AdS<sub>5</sub>/CFT<sub>4</sub> see review in Chapter 11, for AdS<sub>7</sub>/CFT<sub>6</sub> see review in Chapter 15 and Chapter 17. The localization results for spheres (1.2.34) and (1.2.40) gave rise to new matrix models which had not been investigated before. One of the main problems is to find out how the free energy (the logarithm of the partition function) scales in the large  $N$ -limit. In 3d there is an interesting scaling  $N^{3/2}$ , and the analysis of the partition function on  $S^3$  for the ABJM model is related to different subjects such as topological string, see review in Chapter 7. On the other hand, the 5d theory establishes a rather exotic scaling  $N^3$  for the gauge theory, and it supports the relation of the 5d theory to 6d (2, 0) superconformal field theory, see review in Chapter 17.

Once we start to calculate the partition functions on different manifolds (e.g.,  $S^r$  and  $S^{r-1} \times S^1$ ), we start to realize the composite structure of the answer. Namely the answer can be built from basic objects called holomorphic blocks, this is discussed in details for 2d, 3d, 4d and 5d theories in Chapter 6 and Chapter 16. Besides, it seems that in odd dimensions the partition function may serve as a good measure for the number of degrees of freedom. This can be made more precise for the partition function on  $S^3$  which measures the number of degrees of freedom of the supersymmetric theory. Thus one can study how it behaves along the RG flow, see Chapter 8.

Another interesting application of localization appears in the context of the BPS/CFT-correspondence [66], in which BPS phenomena of 4d gauge theories are related to 2d conformal field theory or its massive, lattice, or integrable deformation. A beautiful and precise realization of this idea is the Alday-Gaiotto-Tachikawa (AGT) correspondence which relates 4d  $\mathcal{N} = 2$  gauge theory of class  $\mathcal{S}$  to Liouville (Toda) CFT on some Riemann surface  $C$ . A 4d  $\mathcal{N} = 2$  gauge theory of class  $\mathcal{S}$  is obtained by compactification of 6d (2, 0) tensor self-dual theory on  $C$ . For a review of this topic see Chapter 12.

The 3d/3d version of this correspondence is reviewed in Chapter 9 and 5d version is reviewed in Chapter 16.

The 2d supersymmetric non-linear sigma models play a prominent role in string theory and mathematical physics, but it is hard to perform direct calculations for non-linear sigma model. However some gauged linear sigma models (2d supersymmetric gauge theories) flow to non-linear sigma model. This flow allows to compute some quantities of non-linear sigma models, such as genus 0 Gromov-Witten invariants (counting of holomorphic maps from  $S^2 \simeq \mathbb{CP}^1$  to a Calabi-Yau target) by localization in 2d gauge theories on  $S^2$ . See review in Chapter 4 and Chapter 3.

Other important applications of localization calculations are explicit checks of QFT dualities. Sometimes QFT theories with different Lagrangians describe the same physical system and have the same physical dynamics, a famous example is Seiberg duality [68]. The dual theories may look very different in the description by gauge group and matter content, but have the same partition functions, provided appropriate identification of the parameters. Various checks of the duality using the localization results are reviewed in Chapter 3, Chapter 6, Chapter 8 and Chapter 13.

**Acknowledgement:** We thank all authors who contributed to this volume: Francesco Benini, Tudor Dimofte, Thomas T. Dumitrescu, Kazuo Hosomichi, Seok Kim, Kimyeong Lee, Bruno Le Floch, Marcos Mariño, Joseph A. Minahan, David Morrison, Sara Pasquetti, Jian Qiu, Leonardo Rastelli, Shlomo S. Razamat, Silvu S. Pufu, Yuji Tachikawa and Brian Willett. We are grateful for their cooperation and for their patience with long completion of this project, for many suggestions and helpful ideas. Special thanks to Joseph A. Minahan and Bruno Le Floch for a meticulous proofreading of this introduction, and to Guido Festuccia for comments.

The research of V.P. is supported by ERC grant QUASIFT. The research of M.Z. is supported by Vetenskapsrådet under grant #2014- 5517, by the STINT grant and by the grant “Geometry and Physics” from the Knut and Alice Wallenberg foundation.

## References

- [1] V. Pestun and M. Zabzine, eds., *Localization techniques in quantum field theory*, vol. xx. Journal of Physics A, 2016. 1608.02952. <https://arxiv.org/src/1608.02952/anc/LocQFT.pdf>, <http://pestun.ihes.fr/pages/LocalizationReview/LocQFT.pdf>.
- [2] S. Lefschetz, “Intersections and transformations of complexes and manifolds,” *Trans. Amer. Math. Soc.* **28** (1926) no. 1, 1–49. <http://dx.doi.org/10.2307/1989171>.
- [3] J. J. Duistermaat and G. J. Heckman, “On the variation in the cohomology of the symplectic form of the reduced phase space,” *Invent. Math.* **69** (1982) no. 2, 259–268. <http://dx.doi.org/10.1007/BF01399506>.
- [4] N. Berline and M. Vergne, “Classes caractéristiques équivariantes. Formule de localisation en cohomologie équivariante,” *C. R. Acad. Sci. Paris Sér. I Math.* **295** (1982) no. 9, 539–541.
- [5] M. F. Atiyah and R. Bott, “The moment map and equivariant cohomology,” *Topology* **23** (1984) no. 1, 1–28. [http://dx.doi.org/10.1016/0040-9383\(84\)90021-1](http://dx.doi.org/10.1016/0040-9383(84)90021-1).

- [6] V. Pestun, “Review of localization in geometry,” *Journal of Physics A* **xx** (2016) 000, [1608.02954](#).
- [7] E. Witten, “Supersymmetry and Morse theory,” *J. Differential Geom.* **17** (1982) no. 4, 661–692 (1983). <http://projecteuclid.org/euclid.jdg/1214437492>.
- [8] E. Witten, “Topological sigma models,” *Comm. Math. Phys.* **118** (1988) no. 3, 411–449. <http://projecteuclid.org/euclid.cmp/1104162092>.
- [9] E. Witten, “Topological quantum field theory,” *Comm. Math. Phys.* **117** (1988) no. 3, 353–386. <http://projecteuclid.org/euclid.cmp/1104161738>.
- [10] E. Witten, “Two-dimensional gauge theories revisited,” *J. Geom. Phys.* **9** (1992) 303–368, [arXiv:hep-th/9204083](#) [hep-th].
- [11] N. A. Nekrasov, “Seiberg-Witten prepotential from instanton counting,” *Adv. Theor. Math. Phys.* **7** (2003) no. 5, 831–864. <http://projecteuclid.org/euclid.atmp/1111510432>.
- [12] A. Losev, N. Nekrasov, and S. L. Shatashvili, “Issues in topological gauge theory,” *Nucl. Phys.* **B534** (1998) 549–611, [arXiv:hep-th/9711108](#) [hep-th].
- [13] G. W. Moore, N. Nekrasov, and S. Shatashvili, “Integrating over Higgs branches,” *Commun. Math. Phys.* **209** (2000) 97–121, [arXiv:hep-th/9712241](#) [hep-th].
- [14] A. Losev, N. Nekrasov, and S. L. Shatashvili, “Testing Seiberg-Witten solution,” [arXiv:hep-th/9801061](#) [hep-th]. <http://alice.cern.ch/format/showfull?sysnb=0266564>.
- [15] A. Losev, G. W. Moore, N. Nekrasov, and S. Shatashvili, “Four-dimensional avatars of two-dimensional RCFT,” *Nucl. Phys. Proc. Suppl.* **46** (1996) 130–145, [arXiv:hep-th/9509151](#) [hep-th].
- [16] V. Pestun, “Localization of gauge theory on a four-sphere and supersymmetric Wilson loops,” *Commun. Math. Phys.* **313** (2012) 71–129, [arXiv:0712.2824](#) [hep-th].
- [17] M. Blau, “Killing spinors and SYM on curved spaces,” *JHEP* **11** (2000) 023, [arXiv:hep-th/0005098](#) [hep-th].
- [18] G. Festuccia and N. Seiberg, “Rigid Supersymmetric Theories in Curved Superspace,” *JHEP* **06** (2011) 114, [arXiv:1105.0689](#) [hep-th].
- [19] C. Imbimbo and D. Rosa, “Topological anomalies for Seifert 3-manifolds,” *JHEP* **07** (2015) 068, [arXiv:1411.6635](#) [hep-th].
- [20] J. Bae, C. Imbimbo, S.-J. Rey, and D. Rosa, “New Supersymmetric Localizations from Topological Gravity,” *JHEP* **03** (2016) 169, [arXiv:1510.00006](#) [hep-th].
- [21] C. Klare, A. Tomasiello, and A. Zaffaroni, “Supersymmetry on Curved Spaces and Holography,” *JHEP* **08** (2012) 061, [arXiv:1205.1062](#) [hep-th].
- [22] T. T. Dumitrescu, G. Festuccia, and N. Seiberg, “Exploring Curved Superspace,” *JHEP* **08** (2012) 141, [arXiv:1205.1115](#) [hep-th].
- [23] D. Cassani, C. Klare, D. Martelli, A. Tomasiello, and A. Zaffaroni, “Supersymmetry in Lorentzian Curved Spaces and Holography,” *Commun. Math. Phys.* **327** (2014) 577–602, [arXiv:1207.2181](#) [hep-th].
- [24] C. Closset, T. T. Dumitrescu, G. Festuccia, and Z. Komargodski, “Supersymmetric Field Theories on Three-Manifolds,” *JHEP* **05** (2013) 017, [arXiv:1212.3388](#) [hep-th].
- [25] C. Klare and A. Zaffaroni, “Extended Supersymmetry on Curved Spaces,” *JHEP* **10** (2013) 218, [arXiv:1308.1102](#) [hep-th].
- [26] D. Butter, G. Inverso, and I. Lodato, “Rigid 4D  $\mathcal{N} = 2$  supersymmetric backgrounds and actions,” *JHEP* **09** (2015) 088, [arXiv:1505.03500](#) [hep-th].

- [27] V. Pestun, “Localization for  $\mathcal{N} = 2$  Supersymmetric Gauge Theories in Four Dimensions,” in *New Dualities of Supersymmetric Gauge Theories*, J. Teschner, ed., pp. 159–194. 2016. [arXiv:1412.7134 \[hep-th\]](#). <http://inspirehep.net/record/1335346/files/arXiv:1412.7134.pdf>.
- [28] Y. Pan, “Rigid Supersymmetry on 5-dimensional Riemannian Manifolds and Contact Geometry,” *JHEP* **05** (2014) 041, [arXiv:1308.1567 \[hep-th\]](#).
- [29] Y. Imamura and H. Matsuno, “Supersymmetric backgrounds from 5d N=1 supergravity,” *JHEP* **07** (2014) 055, [arXiv:1404.0210 \[hep-th\]](#).
- [30] Y. Pan and J. Schmude, “On rigid supersymmetry and notions of holomorphy in five dimensions,” *JHEP* **11** (2015) 041, [arXiv:1504.00321 \[hep-th\]](#).
- [31] H. Samtleben, E. Sezgin, and D. Tsimpis, “Rigid 6D supersymmetry and localization,” *JHEP* **03** (2013) 137, [arXiv:1212.4706 \[hep-th\]](#).
- [32] S. M. Kuzenko, “Supersymmetric Spacetimes from Curved Superspace,” *PoS CORFU2014* (2015) 140, [arXiv:1504.08114 \[hep-th\]](#).
- [33] S. M. Kuzenko, J. Novak, and G. Tartaglino-Mazzucchelli, “Symmetries of curved superspace in five dimensions,” *JHEP* **10** (2014) 175, [arXiv:1406.0727 \[hep-th\]](#).
- [34] T. Dumitrescu, “An Introduction to Supersymmetric Field Theories in Curved Space,” *Journal of Physics A* **xx** (2016) 000, [1608.02957](#).
- [35] A. Kapustin, B. Willett, and I. Yaakov, “Exact Results for Wilson Loops in Superconformal Chern-Simons Theories with Matter,” *JHEP* **03** (2010) 089, [arXiv:0909.4559 \[hep-th\]](#).
- [36] F. Benini and S. Cremonesi, “Partition Functions of  $\mathcal{N} = (2, 2)$  Gauge Theories on  $S^2$  and Vortices,” *Commun. Math. Phys.* **334** (2015) no. 3, 1483–1527, [arXiv:1206.2356 \[hep-th\]](#).
- [37] N. Doroud, J. Gomis, B. Le Floch, and S. Lee, “Exact Results in D=2 Supersymmetric Gauge Theories,” *JHEP* **05** (2013) 093, [arXiv:1206.2606 \[hep-th\]](#).
- [38] J. Kallen and M. Zabzine, “Twisted supersymmetric 5D Yang-Mills theory and contact geometry,” *JHEP* **05** (2012) 125, [arXiv:1202.1956 \[hep-th\]](#).
- [39] J. Kallen, J. Qiu, and M. Zabzine, “The perturbative partition function of supersymmetric 5D Yang-Mills theory with matter on the five-sphere,” *JHEP* **08** (2012) 157, [arXiv:1206.6008 \[hep-th\]](#).
- [40] H.-C. Kim and S. Kim, “M5-branes from gauge theories on the 5-sphere,” *JHEP* **05** (2013) 144, [arXiv:1206.6339 \[hep-th\]](#).
- [41] J. A. Minahan and M. Zabzine, “Gauge theories with 16 supersymmetries on spheres,” *JHEP* **03** (2015) 155, [arXiv:1502.07154 \[hep-th\]](#).
- [42] N. Hama, K. Hosomichi, and S. Lee, “SUSY Gauge Theories on Squashed Three-Spheres,” *JHEP* **05** (2011) 014, [arXiv:1102.4716 \[hep-th\]](#).
- [43] Y. Imamura and D. Yokoyama, “N=2 supersymmetric theories on squashed three-sphere,” *Phys. Rev.* **D85** (2012) 025015, [arXiv:1109.4734 \[hep-th\]](#).
- [44] N. Hama and K. Hosomichi, “Seiberg-Witten Theories on Ellipsoids,” *JHEP* **09** (2012) 033, [arXiv:1206.6359 \[hep-th\]](#). [Addendum: JHEP10,051(2012)].
- [45] G. Lockhart and C. Vafa, “Superconformal Partition Functions and Non-perturbative Topological Strings,” [arXiv:1210.5909 \[hep-th\]](#).
- [46] Y. Imamura, “Perturbative partition function for squashed  $S^5$ ,” [arXiv:1210.6308 \[hep-th\]](#).
- [47] H.-C. Kim, J. Kim, and S. Kim, “Instantons on the 5-sphere and M5-branes,” [arXiv:1211.0144 \[hep-th\]](#).

- [48] J. A. Minahan, “Localizing gauge theories on  $S^d$ ,” *JHEP* **04** (2016) 152, [arXiv:1512.06924 \[hep-th\]](#).
- [49] A. Narukawa, “The modular properties and the integral representations of the multiple elliptic gamma functions,” *Advances in Mathematics* **189** (2004) no. 2, 247 – 267.  
<http://www.sciencedirect.com/science/article/pii/S0001870803003670>.
- [50] F. Benini and B. Le Floch, “Supersymmetric localization in two dimensions,” *Journal of Physics A* **xx** (2016) 000, [1608.02955](#).
- [51] K. Hosomichi, “ $\mathcal{N} = 2$  SUSY gauge theories on  $S^4$ ,” *Journal of Physics A* **xx** (2016) 000, [1608.02962](#).
- [52] B. Willett, “Localization on three-dimensional manifolds,” *Journal of Physics A* **xx** (2016) 000, [1608.02958](#).
- [53] J. Qiu and M. Zabzine, “Review of localization for 5D supersymmetric gauge theories,” *Journal of Physics A* **xx** (2016) 000, [1608.02966](#).
- [54] M. F. Atiyah, *Elliptic operators and compact groups*. Springer-Verlag, Berlin, 1974. Lecture Notes in Mathematics, Vol. 401.
- [55] A. B. Zamolodchikov and A. B. Zamolodchikov, “Structure constants and conformal bootstrap in Liouville field theory,” *Nucl. Phys.* **B477** (1996) 577–605, [arXiv:hep-th/9506136 \[hep-th\]](#).
- [56] L. F. Alday, D. Gaiotto, and Y. Tachikawa, “Liouville Correlation Functions from Four-dimensional Gauge Theories,” *Lett.Math.Phys.* **91** (2010) 167–197, [arXiv:0906.3219 \[hep-th\]](#).
- [57] Y. Tachikawa, “A brief review of the 2d/4d correspondences,” *Journal of Physics A* **xx** (2016) 000, [1608.02964](#).
- [58] M. Mariño, “Localization at large  $N$  in Chern-Simons-matter theories,” *Journal of Physics A* **xx** (2016) 000, [1608.02959](#).
- [59] S. Pufu, “The F-Theorem and F-Maximization,” *Journal of Physics A* **xx** (2016) 000, [1608.02960](#).
- [60] T. Dimofte, “Perturbative and nonperturbative aspects of complex Chern-Simons Theory,” *Journal of Physics A* **xx** (2016) 000, [1608.02961](#).
- [61] J. Minahan, “Matrix models for 5D super Yang-Mills,” *Journal of Physics A* **xx** (2016) 000, [1608.02967](#).
- [62] S. Pasquetti, “Holomorphic blocks and the 5d AGT correspondence,” *Journal of Physics A* **xx** (2016) 000, [1608.02968](#).
- [63] L. Rastelli and S. Razamat, “The supersymmetric index in four dimensions,” *Journal of Physics A* **xx** (2016) 000, [1608.02965](#).
- [64] S. Kim and K. Lee, “Indices for 6 dimensional superconformal field theories,” *Journal of Physics A* **xx** (2016) 000, [1608.02969](#).
- [65] K. Zarembo, “Localization and AdS/CFT Correspondence,” *Journal of Physics A* **xx** (2016) 000, [1608.02963](#).
- [66] N. Nekrasov, “On the BPS/CFT correspondence,” *Lecture at the University of Amsterdam string theory group seminar* (2004) .
- [67] D. Morrison, “Gromov-Witten invariants and localization,” *Journal of Physics A* (2016) , [1608.02956](#).
- [68] N. Seiberg, “Electric - magnetic duality in supersymmetric nonAbelian gauge theories,” *Nucl. Phys.* **B435** (1995) 129–146, [arXiv:hep-th/9411149 \[hep-th\]](#).

# Chapter 2

## Review of localization in geometry

Vasily Pestun

*Institut des Hautes Études Scientifique, France*  
pestun@ihes.fr

### Abstract

Review of localization in geometry: equivariant cohomology, characteristic classes, Atiyah-Bott formula, Atiyah-Singer equivariant index formula, Mathai-Quillen formalism

### Contents

|            |                                                              |           |
|------------|--------------------------------------------------------------|-----------|
| <b>2.1</b> | <b>Equivariant cohomology</b>                                | <b>36</b> |
| <b>2.2</b> | <b>Classifying space and characteristic classes</b>          | <b>37</b> |
| <b>2.3</b> | <b>Weil algebra</b>                                          | <b>38</b> |
| <b>2.4</b> | <b>Weil model and Cartan model of equivariant cohomology</b> | <b>41</b> |
| 2.4.1      | Cartan model                                                 | 41        |
| 2.4.2      | Weil model                                                   | 43        |
| <b>2.5</b> | <b>Equivariant characteristic classes in Cartan model</b>    | <b>43</b> |
| <b>2.6</b> | <b>Standard characteristic classes</b>                       | <b>45</b> |
| 2.6.1      | Euler class                                                  | 45        |
| 2.6.2      | Euler class of vector bundle and Mathai-Quillen form         | 46        |
| 2.6.3      | Chern character                                              | 48        |
| 2.6.4      | Chern class                                                  | 48        |
| 2.6.5      | Todd class                                                   | 48        |
| 2.6.6      | The $\hat{A}$ class                                          | 49        |
| <b>2.7</b> | <b>Index formula</b>                                         | <b>49</b> |
| <b>2.8</b> | <b>Equivariant integration</b>                               | <b>50</b> |
| 2.8.1      | Thom isomorphism and Atiyah-Bott localization                | 51        |
| 2.8.2      | Duistermaat-Heckman localization                             | 52        |

|                   |                                                                          |           |
|-------------------|--------------------------------------------------------------------------|-----------|
| 2.8.3             | Gaussian integral example . . . . .                                      | 53        |
| 2.8.4             | Example of a two-sphere . . . . .                                        | 54        |
| <b>2.9</b>        | <b>Equivariant index formula (Dolbeault and Dirac)</b> . . . . .         | <b>55</b> |
| <b>2.10</b>       | <b>Equivariant index and representation theory</b> . . . . .             | <b>58</b> |
| <b>2.11</b>       | <b>Equivariant index for differential operators</b> . . . . .            | <b>61</b> |
| 2.11.1            | Atiyah-Singer equivariant index formula for elliptic complexes . . . . . | 61        |
| 2.11.2            | Atiyah-Singer index formula for a free action $G$ -manifold . . . . .    | 62        |
| 2.11.3            | General Atiyah-Singer index formula . . . . .                            | 63        |
| <b>2.12</b>       | <b>Equivariant cohomological field theories</b> . . . . .                | <b>65</b> |
| <b>References</b> | . . . . .                                                                | <b>67</b> |

Foundations of equivariant de Rham theory have been laid in two papers by Henri Cartan [2] [3]. The book by Guillemin and Sternberg [4] covers Cartan’s papers and treats equivariant de Rham theory from the perspective of supersymmetry. See also the book by Berline-Vergne [5], the lectures by Szabo [6] and by Cordes-Moore-Ramgoolam [7], and Vergne’s review [8].

## 2.1 Equivariant cohomology

Let  $G$  be a compact connected Lie group. Let  $X$  be a  $G$ -manifold, which means that there is a defined action  $G \times X \rightarrow X$  of the group  $G$  on the manifold  $X$ .

If  $G$  acts freely on  $X$  (all stabilizers are trivial) then the space  $X/G$  is an ordinary manifold on which the usual cohomology theory  $H^\bullet(X/G)$  is defined. If the  $G$  action on  $X$  is free, the  $G$ -equivariant cohomology groups  $H_G^\bullet(X)$  are defined to be the ordinary cohomology  $H^\bullet(X/G)$ .

If the  $G$  action on  $X$  is not free, the naive definition of the equivariant cohomology  $H_G^\bullet(X)$  fails because  $X/G$  is not an ordinary manifold. If non-trivial stabilizers exist, the corresponding points on  $X/G$  are not ordinary points but fractional or stacky points.

A proper topological definition of the  $G$ -equivariant cohomology  $H_G(X)$  sets

$$H_G^\bullet(X) = H^\bullet(X \times_G EG) = H^\bullet((X \times EG)/G) \tag{2.1.1}$$

where the space  $EG$ , called *universal bundle* [9, 10] is a topological space associated to  $G$  with the following properties

1. The space  $EG$  is contractible
2. The group  $G$  acts freely on  $EG$

Because of the property (1) the cohomology theory of  $X$  is isomorphic to the cohomology theory of  $X \times EG$ , and because of the property (2) the group  $G$  acts freely on  $X \times EG$  and hence the quotient space  $(X \times_G EG)$  has a well-defined ordinary cohomology theory.

## 2.2 Classifying space and characteristic classes

If  $X$  is a point  $pt$ , the ordinary cohomology theory  $H^\bullet(pt)$  is elementary

$$H^n(pt, \mathbb{R}) = \begin{cases} \mathbb{R}, & n = 0 \\ 0, & n > 0 \end{cases} \quad (2.2.1)$$

but the equivariant cohomology  $H_G^\bullet(pt)$  is less trivial. Indeed,

$$H_G^\bullet(pt) = H^\bullet(EG/G) = H^\bullet(BG) \quad (2.2.2)$$

where the quotient space  $BG = EG/G$  is called *classifying space*.

The terminology *universal bundle*  $EG$  and *classifying space*  $BG$  comes from the fact that any smooth principal  $G$ -bundle on a manifold  $X$  can be induced by a pullback  $f^*$  of the universal principal  $G$ -bundle  $EG \rightarrow BG$  using a suitable smooth map  $f : X \rightarrow BG$ .

The cohomology groups of  $BG$  are used to construct *characteristic classes* of principal  $G$ -bundles.

Let  $\mathfrak{g} = Lie(G)$  be the real Lie algebra of a compact connected Lie group  $G$ . Let  $\mathbb{R}[\mathfrak{g}]$  be the space of real valued polynomial functions on  $\mathfrak{g}$ , and let  $\mathbb{R}[\mathfrak{g}]^G$  be the subspace of  $Ad_G$  invariant polynomials on  $\mathfrak{g}$ .

For a principal  $G$ -bundle over a base manifold  $X$  the Chern-Weil morphism

$$\begin{aligned} \mathbb{R}[\mathfrak{g}]^G &\rightarrow H^\bullet(X, \mathbb{R}) \\ p &\mapsto p(F_A) \end{aligned} \quad (2.2.3)$$

sends an adjoint invariant polynomial  $p$  on the Lie algebra  $\mathfrak{g}$  to a cohomology class  $[p(F_A)]$  in  $H^\bullet(X)$  where  $F_A = \nabla_A^2$  is the curvature 2-form of any connection  $\nabla_A$  on the  $G$ -bundle. The cohomology class  $[p(F_A)]$  does not depend on the choice of the connection  $A$  and is called the *characteristic class* of the  $G$ -bundle associated to the polynomial  $p \in \mathbb{R}[\mathfrak{g}]^G$ .

The main theorem of Chern-Weil theory is that the ring of characteristic classes  $\mathbb{R}[\mathfrak{g}]^G$  is isomorphic to the cohomology ring  $H^\bullet(BG)$  of the classifying space  $BG$ : the Chern-Weil morphism (2.2.3) is an isomorphism

$$\mathbb{R}[\mathfrak{g}]^G \xrightarrow{\sim} H^\bullet(BG, \mathbb{R}) \quad (2.2.4)$$

For the circle group  $G = S^1 \simeq U(1)$  the universal bundle  $ES^1$  and classifying space  $BS^1$  can be modelled as

$$ES^1 \simeq S^{2n+1}, \quad BS^1 \simeq \mathbb{C}P^n \quad \text{at} \quad n \rightarrow \infty \quad (2.2.5)$$

Then the Chern-Weil isomorphism is explicitly

$$\mathbb{C}[\mathfrak{g}]^G \simeq H^\bullet(\mathbb{C}P^\infty, \mathbb{C}) \simeq \mathbb{C}[\epsilon] \quad (2.2.6)$$

where  $\epsilon \in \mathfrak{g}^\vee$  is a linear function on  $\mathfrak{g} = Lie(S^1)$  and  $\mathbb{C}[\epsilon]$  denotes the free polynomial ring on one generator  $\epsilon$ . The  $\epsilon \in H^2(\mathbb{C}\mathbb{P}^\infty, \mathbb{C})$  is negative of the first Chern class  $c_1$  of the universal bundle

$$-c_1(\gamma) = \epsilon = \frac{1}{2\pi\sqrt{-1}} \text{tr}_1 F_A(\gamma) \quad (2.2.7)$$

where  $\text{tr}_1$  denotes trace of the curvature two-form  $F_A = dA + A \wedge A$  in the fundamental complex 1-dimensional representation in which the Lie algebra of  $\mathfrak{g} = Lie(S^1)$  is represented by  $i\mathbb{R}$ . The cohomological degree of  $\epsilon$  is

$$\deg \epsilon = \deg F_A(\gamma) = 2 \quad (2.2.8)$$

Generally, for a compact connected Lie group  $G$  we reduce the Chern-Weil theory to the maximal torus  $T \subset G$  and identify

$$\mathbb{C}[\mathfrak{g}]^G \simeq \mathbb{C}[\mathfrak{t}]^{W_G} \quad (2.2.9)$$

where  $\mathfrak{t}$  is the Cartan Lie algebra  $\mathfrak{t} = Lie(T)$  and  $W_G$  is the Weyl group of  $G$ .

For example, if  $G = U(n)$  the Weyl group  $W_{U(n)}$  is the permutation group of  $n$  eigenvalues  $\epsilon_1, \dots, \epsilon_n$ . Therefore

$$H^\bullet(BU(n), \mathbb{C}) = \mathbb{C}[\mathfrak{g}]^{U(n)} \simeq \mathbb{C}[\epsilon_1, \dots, \epsilon_n]^{W_{U(n)}} \simeq \mathbb{C}[c_1, \dots, c_n] \quad (2.2.10)$$

where  $(c_1, \dots, c_n)$  are elementary symmetrical monomials called Chern classes

$$c_k = (-1)^k \sum_{i_1 \leq \dots \leq i_k} \epsilon_{i_1} \dots \epsilon_{i_k} \quad (2.2.11)$$

The classifying space for  $G = U(n)$  is

$$BU(n) = \lim_{k \rightarrow \infty} \text{Gr}_n(\mathbb{C}^{k+n}) \quad (2.2.12)$$

where  $\text{Gr}_n(V)$  denotes the space of  $n$ -planes in the vector space  $V$ .

To summarize, if  $G$  is a connected compact Lie group with Lie algebra  $\mathfrak{g} = Lie(G)$ , maximal torus  $T$  and its Lie algebra  $\mathfrak{t} = Lie(T)$ , and Weyl group  $W_G$ , then it holds

$$\boxed{H_G^\bullet(pt, \mathbb{R}) \simeq H^\bullet(BG, \mathbb{R}) \simeq \mathbb{R}[\mathfrak{g}]^G \simeq \mathbb{R}[\mathfrak{t}]^{W_G}} \quad (2.2.13)$$

## 2.3 Weil algebra

The cohomology  $H^\bullet(BG, \mathbb{R})$  of the classifying space  $BG$  can also be realized in the Weil algebra

$$\mathcal{W}_{\mathfrak{g}} := \mathbb{R}[\mathfrak{g}[1] \oplus \mathfrak{g}[2]] = \Lambda \mathfrak{g}^\vee \otimes S \mathfrak{g}^\vee \quad (2.3.1)$$

Here  $\mathfrak{g}[1]$  denotes shift of degree so that elements of  $\mathfrak{g}[1]$  are Grassmann. The space of polynomial functions  $\mathbb{R}[\mathfrak{g}[1]]$  on  $\mathfrak{g}[1]$  is the anti-symmetric algebra  $\Lambda \mathfrak{g}^\vee$  of  $\mathfrak{g}^\vee$ , and the space of polynomial functions  $\mathbb{R}[\mathfrak{g}[2]]$  on  $\mathfrak{g}[2]$  is the symmetric algebra  $S \mathfrak{g}^\vee$  of  $\mathfrak{g}^\vee$ .

The elements  $c \in \mathfrak{g}[1]$  have degree 1 and represent the connection 1-form on the universal bundle. The elements  $\phi \in \mathfrak{g}[2]$  have degree 2 and represent the curvature 2-form on the universal bundle. An odd differential on functions on  $\mathfrak{g}[1] \oplus \mathfrak{g}[2]$  can be described as an odd vector field  $\delta$  such that  $\delta^2 = 0$ . The odd vector field  $\delta$  of degree 1 represents de Rham differential on the universal bundle

$$\begin{aligned}\delta c &= \phi - \frac{1}{2}[c, c] \\ \delta \phi &= -[c, \phi]\end{aligned}\tag{2.3.2}$$

which follows from the standard relations between the connection  $A$  and the curvature  $F_A$

$$\begin{aligned}dA &= F_A - \frac{1}{2}[A, A] \\ dF_A &= -[A, F_A]\end{aligned}\tag{2.3.3}$$

This definition implies  $\delta^2 = 0$ . Indeed,

$$\begin{aligned}\delta^2 c &= \delta \phi - [\delta c, c] = -[c, \phi] - \left[\phi - \frac{1}{2}[c, c], c\right] = 0 \\ \delta^2 \phi &= -[\delta c, \phi] + [c, \delta \phi] = -\left[\phi - \frac{1}{2}[c, c], \phi\right] - [c, [c, \phi]] = 0\end{aligned}\tag{2.3.4}$$

Given a basis  $T_\alpha$  on the Lie algebra  $\mathfrak{g}$  with structure constants  $[T_\beta, T_\gamma] = f_{\beta\gamma}^\alpha T_\alpha$  the differential  $\delta$  has the form

$$\begin{aligned}\delta c^\alpha &= \phi^\alpha - \frac{1}{2}f_{\beta\gamma}^\alpha c^\beta c^\gamma \\ \delta \phi^\alpha &= -f_{\beta\gamma}^\alpha c^\beta \phi^\gamma\end{aligned}\tag{2.3.5}$$

The differential  $\delta$  can be decomposed into the sum of two differentials

$$\delta = \delta_K + \delta_{\text{BRST}}\tag{2.3.6}$$

with

$$\begin{aligned}\delta_K \phi &= 0, & \delta_{\text{BRST}} \phi &= -[c, \phi] \\ \delta_K c &= \phi, & \delta_{\text{BRST}} c &= -\frac{1}{2}[c, c]\end{aligned}\tag{2.3.7}$$

The differential  $\delta_{\text{BRST}}$  is the BRST differential (Chevalley-Eilenberg differential for Lie algebra cohomology with coefficients in the Lie algebra module  $S\mathfrak{g}^\vee$ ). The differential  $\delta_K$  is the Koszul differential (de Rham differential on  $\Omega^\bullet(\Pi\mathfrak{g})$ ).

The field theory interpretation of the Weil algebra and the differential (2.3.6) was given in [11] and [12].

The Weil algebra  $\mathcal{W}_\mathfrak{g} = \mathbb{R}[\mathfrak{g}[1] \oplus \mathfrak{g}[2]]$  is an extension of the Chevalley-Eilenberg algebra  $CE_\mathfrak{g} = \mathbb{R}[\mathfrak{g}[1]] = \Lambda\mathfrak{g}^\vee$  by the algebra  $\mathbb{R}[\mathfrak{g}[2]]^G = S\mathfrak{g}^\vee$  of symmetric polynomials on  $\mathfrak{g}$

$$CE_\mathfrak{g} \leftarrow \mathcal{W}_\mathfrak{g} \leftarrow S\mathfrak{g}^\vee\tag{2.3.8}$$

which is quasi-isomorphic to the algebra of differential forms on the universal bundle

$$G \rightarrow EG \rightarrow BG \quad (2.3.9)$$

The duality between the Weil algebra  $\mathcal{W}_{\mathfrak{g}}$  and the de Rham algebra  $\Omega^\bullet(EG)$  of differential forms on  $EG$  is provided by the Weil homomorphism

$$\mathcal{W}_{\mathfrak{g}} \rightarrow \Omega^\bullet(EG) \quad (2.3.10)$$

after a choice of a connection 1-form  $A \in \Omega^1(EG) \otimes \mathfrak{g}$  and its field strength  $F_A \in \Omega^2(EG) \otimes \mathfrak{g}$  on the universal bundle  $EG \rightarrow BG$ .

Indeed, the connection 1-form  $A \in \Omega^1(EG) \otimes \mathfrak{g}$  and field strength  $F \in \Omega^2(EG) \otimes \mathfrak{g}$  define maps  $\mathfrak{g}^\vee \rightarrow \Omega^1(EG)$  and  $\mathfrak{g}^\vee \rightarrow \Omega^2(EG)$

$$\begin{aligned} c^\alpha &\mapsto A^\alpha \\ \phi^\alpha &\mapsto F^\alpha \end{aligned} \quad (2.3.11)$$

The cohomology of the Weil algebra is trivial

$$H^n(\mathcal{W}_{\mathfrak{g}}, \delta, \mathbb{R}) = \begin{cases} \mathbb{R}, & n = 0 \\ 0, & n > 0 \end{cases} \quad (2.3.12)$$

corresponding to the trivial cohomology of  $\Omega^\bullet(EG)$ .

To define  $G$ -equivariant cohomology we need to consider  $G$  action on  $EG$ . To compute  $H_G^\bullet(pt) = H^\bullet(BG)$ , consider  $\Omega^\bullet(BG) = \Omega^\bullet(EG/G)$ .

For any principal  $G$ -bundle  $\pi : P \rightarrow P/G$  the differential forms on  $P$  in the image of the pullback  $\pi^*$  of the space of differential forms on  $P/G$  are called *basic*

$$\Omega^\bullet(P)_{\text{basic}} = \pi^* \Omega^\bullet(P/G) \quad (2.3.13)$$

Let  $L_\alpha$  be the Lie derivative in the direction of a vector field  $\alpha$  generated by a basis element  $T_\alpha \in \mathfrak{g}$ , and  $i_\alpha$  be the contraction with the vector field generated by  $T_\alpha$ .

An element  $\omega \in \Omega^\bullet(P)_{\text{basic}}$  can be characterized by two conditions

1.  $\omega$  is invariant on  $P$  with respect to the  $G$ -action:  $L_\alpha \omega = 0$
2.  $\omega$  is horizontal on  $P$  with respect to the  $G$ -action:  $i_\alpha \omega = 0$

In the Weil model the contraction operation  $i_\alpha$  is realized as

$$\begin{aligned} i_\alpha c^\beta &= \delta_\alpha^\beta \\ i_\alpha \phi^\beta &= 0 \end{aligned} \quad (2.3.14)$$

and the Lie derivative  $L_\alpha$  is defined by the usual relation

$$L_\alpha = \delta i_\alpha + i_\alpha \delta \quad (2.3.15)$$

From the definition of  $\Omega^\bullet(P)_{\text{basic}}$  for the case of  $P = EG$  we obtain

$$H_G^\bullet(pt) = H^\bullet(BG, \mathbb{R}) = H^\bullet(\Omega^\bullet(EG)_{\text{basic}}, \mathbb{R}) = H^\bullet(\mathcal{W}_{\mathfrak{g}}, \delta, \mathbb{R})_{\text{basic}} = (S\mathfrak{g}^\vee)^G \quad (2.3.16)$$

## 2.4 Weil model and Cartan model of equivariant cohomology

The isomorphism

$$H(BG, \mathbb{R}) = H(EG, \mathbb{R})_{\text{basic}} = H(\mathcal{W}_{\mathfrak{g}}, \delta, \mathbb{R})_{\text{basic}} \quad (2.4.1)$$

suggests to replace the topological model for  $G$ -equivariant cohomologies of real manifold  $X$

$$H_G(X, \mathbb{R}) = H((X \times EG)/G, \mathbb{R}) \quad (2.4.2)$$

by the *Cartan model*

$$H_G(X, \mathbb{R}) = H((\Omega^\bullet(X) \otimes S\mathfrak{g}^\vee)^G, \mathbb{R}) \quad (2.4.3)$$

or by the equivalent algebraic *Weil model*

$$H_G(X, \mathbb{R}) = H((\Omega^\bullet(X) \otimes \mathcal{W}_{\mathfrak{g}})_{\text{basic}}, \mathbb{R}) \quad (2.4.4)$$

### 2.4.1 Cartan model

Here  $(\Omega^\bullet(X) \otimes S\mathfrak{g}^\vee)^G$  denotes the  $G$ -invariant subspace in  $(\Omega^\bullet(X) \otimes S\mathfrak{g}^\vee)$  under the  $G$ -action induced from  $G$ -action on  $X$  and adjoint  $G$ -action on  $\mathfrak{g}$ .

It is convenient to think about  $(\Omega^\bullet(X) \otimes S\mathfrak{g}^\vee)$  as the space

$$\Omega_{C^\infty, \text{poly}}^{\bullet, 0}(X \times \mathfrak{g}) \quad (2.4.5)$$

of smooth differential forms on  $X \times \mathfrak{g}$  of degree 0 along  $\mathfrak{g}$  and polynomial along  $\mathfrak{g}$ .

In  $(T_a)$  basis on  $\mathfrak{g}$ , an element  $\phi \in \mathfrak{g}$  is represented as  $\phi = \phi^\alpha T_\alpha$ . Then  $(\phi^\alpha)$  is the dual basis of  $\mathfrak{g}^\vee$ . Equivalently  $\phi^\alpha$  is a linear coordinate on  $\mathfrak{g}$ .

The commutative ring  $\mathbb{R}[\mathfrak{g}]$  of polynomial functions on the vector space underlying  $\mathfrak{g}$  is naturally represented in the coordinates as the ring of polynomials in generators  $\{\phi^\alpha\}$

$$\mathbb{R}[\mathfrak{g}] = \mathbb{R}[\phi^1, \dots, \phi^{\text{rk} \mathfrak{g}}] \quad (2.4.6)$$

Hence, the space (2.4.5) can be equivalently presented as

$$\Omega_{C^\infty, \text{poly}}^{\bullet, 0}(X \times \mathfrak{g}) = \Omega^\bullet(X) \otimes \mathbb{R}[\mathfrak{g}] \quad (2.4.7)$$

Given an action of the group  $G$  on any manifold  $M$

$$\rho_g : m \mapsto g \cdot m \quad (2.4.8)$$

the induced action on the space of differential forms  $\Omega^\bullet(M)$  comes from the pullback by the map  $\rho_{g^{-1}}$

$$\rho_g : \omega \mapsto \rho_{g^{-1}}^* \omega, \quad \omega \in \Omega^\bullet(M) \quad (2.4.9)$$

In particular, if  $M = \mathfrak{g}$  and  $\omega \in \mathfrak{g}^\vee$  is a linear function on  $\mathfrak{g}$ , then (2.4.9) is the *co-adjoint action* on  $\mathfrak{g}^\vee$ .

The invariant subspace  $(\Omega^\bullet(X) \otimes \mathbb{R}[\mathfrak{g}])^G$  forms a complex with respect to the *Cartan differential*

$$d_G = d \otimes 1 + i_\alpha \otimes \phi^\alpha \quad (2.4.10)$$

where  $d : \Omega^\bullet(X) \rightarrow \Omega^{\bullet+1}(X)$  is the de Rham differential, and  $i_\alpha : \Omega^\bullet(X) \rightarrow \Omega^{\bullet-1}(X)$  is the operation of contraction of the vector field on  $X$  generated by  $T_\alpha \in \mathfrak{g}$  with differential forms in  $\Omega^\bullet(X)$ .

The Cartan model of the  $G$ -equivariant cohomology  $H_G(X)$  is

$$H_G(X) = H\left((\Omega^\bullet(X) \otimes \mathbb{R}[\mathfrak{g}])^G, d_G\right) \quad (2.4.11)$$

To check that  $d_G^2 = 0$  on  $(\Omega^\bullet(X) \otimes \mathbb{R}[\mathfrak{g}])^G$  we compute  $d_G^2$  on  $\Omega^\bullet(X) \otimes \mathbb{R}[\mathfrak{g}]$  and find

$$d_G^2 = L_\alpha \otimes \phi^\alpha \quad (2.4.12)$$

where  $L_\alpha : \Omega^\bullet(X) \rightarrow \Omega^\bullet(X)$  is the Lie derivative on  $X$

$$L_\alpha = di_\alpha + i_\alpha d \quad (2.4.13)$$

along vector field generated by  $T_\alpha$ .

The infinitesimal action by a Lie algebra generator  $T_a$  on an element  $\omega \in \Omega^\bullet(X) \otimes R[\mathfrak{g}]$  is

$$T_\alpha \cdot \omega = (L_\alpha \otimes 1 + 1 \otimes L_\alpha) \cdot \omega \quad (2.4.14)$$

where  $L_\alpha \otimes 1$  is the geometrical Lie derivative by the vector field generated by  $T_\alpha$  on  $\Omega^\bullet(X)$  and  $1 \otimes L_\alpha$  is the coadjoint action on  $\mathbb{R}[\mathfrak{g}]$

$$L_\alpha = f_{\alpha\beta}^\gamma \phi^\beta \frac{\partial}{\partial \phi^\gamma} \quad (2.4.15)$$

If  $\omega$  is a  $G$ -invariant element,  $\omega \in (\Omega^\bullet(X) \otimes R[\mathfrak{g}])^G$ , then

$$(L_\alpha \otimes 1 + 1 \otimes L_\alpha)\omega = 0 \quad (2.4.16)$$

Therefore, if  $\omega \in (\Omega^\bullet(X) \otimes R[\mathfrak{g}])^G$  it holds that

$$d_G^2 \omega = (1 \otimes \phi^\alpha L_\alpha)\omega = \phi^\alpha f_{\alpha\beta}^\gamma \phi^\beta \frac{\partial \omega}{\partial \phi^\gamma} = 0 \quad (2.4.17)$$

by the antisymmetry of the structure constants  $f_{\alpha\beta}^\gamma = -f_{\beta\alpha}^\gamma$ . Therefore  $d_G^2 = 0$  on  $(\Omega^\bullet(X) \otimes \mathbb{R}[\mathfrak{g}])^G$ .

The grading on  $\Omega^\bullet(X) \otimes \mathbb{R}[\mathfrak{g}]$  is defined by the assignment

$$\deg d = 1 \quad \deg i_{v_\alpha} = -1 \quad \deg \phi^\alpha = 2 \quad (2.4.18)$$

which implies

$$\deg d_G = 1 \quad (2.4.19)$$

Let

$$\Omega_G^n(X) = \bigoplus_k (\Omega^{n-2k} \otimes \mathbb{R}[\mathfrak{g}]^k)^G \quad (2.4.20)$$

be the subspace in  $(\Omega(X) \otimes \mathbb{R}[\mathfrak{g}])^G$  of degree  $n$  according to the grading (2.4.18).

Then

$$\dots \xrightarrow{d_G} \Omega_G^n(X) \xrightarrow{d_G} \Omega_G^{n+1}(X) \xrightarrow{d_G} \dots \quad (2.4.21)$$

is a differential complex. The equivariant cohomology groups  $H_G^\bullet(X)$  in the Cartan model are defined as the cohomology of the complex (2.4.21)

$$H_G^\bullet(X) \equiv \text{Ker } d_G / \text{Im } d_G \quad (2.4.22)$$

In particular, if  $X = pt$  is a point then

$$H_G^\bullet(pt) = \mathbb{R}[\mathfrak{g}]^G \quad (2.4.23)$$

in agreement with (2.3.16).

If  $x^\mu$  are coordinates on  $X$ , and  $\psi^\mu = dx^\mu$  are Grassman coordinates on the fibers of  $\Pi TX$ , we can represent the Cartan differential (2.4.10) in the notations more common in quantum field theory traditions

$$\begin{aligned} \delta x^\mu &= \psi^\mu \\ \delta \psi^\mu &= \phi^\alpha v_\alpha^\mu \end{aligned} \quad \delta \phi = 0 \quad (2.4.24)$$

where  $v^\mu$  are components of the vector field on  $X$  generated by a basis element  $T_\alpha$  for the  $G$ -action on  $X$ . In quantum field theory, the coordinates  $x^\mu$  are typically coordinates on the infinite-dimensional space of bosonic fields, and  $\psi^\mu$  are typically coordinates on the infinite-dimensional space of fermionic fields.

## 2.4.2 Weil model

The differential in Weil model can be presented in coordinate notations similar to (2.4.24) as follows

$$\begin{aligned} \delta x^\mu &= \psi^\mu + c^\alpha v_\alpha^\mu & \delta c^\alpha &= \phi^\alpha - \frac{1}{2} f_{\beta\gamma}^\alpha c^\beta c^\gamma \\ \delta \psi^\mu &= \phi^\alpha v_\alpha^\mu + \partial_\nu v_\alpha^\mu c^\alpha \psi^\nu & \delta \phi^\alpha &= -f_{\beta\gamma}^\alpha c^\beta \phi^\gamma \end{aligned} \quad (2.4.25)$$

In physical applications, typically  $c$  is the BRST ghost field for gauge symmetry, and Weil differential is the sum of a supersymmetry transformation and BRST transformation, for example see [13].

## 2.5 Equivariant characteristic classes in Cartan model

For a reference see [14] and [15].

Let  $G$  and  $T$  be compact connected Lie groups.

We consider a  $T$ -equivariant  $G$ -principal bundle  $\pi : P \rightarrow X$ . This means that an equivariant  $T$ -action is defined on  $P$  compatible with the  $G$ -bundle structure of  $\pi : P \rightarrow X$ . One can take that  $G$  acts from the right and  $T$  acts from the left.

The compatibility means that  $T$ -action on the total space of  $P$

- commutes with the projection map  $\pi : P \rightarrow X$
- commutes with the  $G$  action on the fibers of  $\pi : P \rightarrow X$

Let  $D_A = d + A$  be a  $T$ -invariant connection on a  $T$ -equivariant  $G$ -bundle  $P$ . Here the connection  $A$  is a  $\mathfrak{g}$ -valued 1-form on the total space of  $P$  (such a connection always exists by the averaging procedure for compact  $T$ ).

Then we define the  $T$ -equivariant connection

$$D_{A,T} = D_A + \epsilon^a i_{v_a} \quad (2.5.1)$$

and the  $T$ -equivariant curvature

$$F_{A,T} = (D_{A,T})^2 - \epsilon^a \otimes \mathcal{L}_{v_a} \quad (2.5.2)$$

where  $\epsilon^a$  are coordinates on the Lie algebra  $\mathfrak{t}$  (like the coordinates  $\phi^a$  on the Lie algebra  $\mathfrak{g}$  in the previous section defining Cartan model of  $G$ -equivariant cohomology), which is in fact is an element of  $\Omega_T^2(X) \otimes \mathfrak{g}$

$$F_{A,T} = F_A - \epsilon^a \otimes \mathcal{L}_{v_a} + [\epsilon^a \otimes i_{v_a}, 1 \otimes D_A] = F_A + \epsilon^a i_{v_a} A \quad (2.5.3)$$

Let  $X^T$  be the  $T$ -fixed point set in  $X$ . If the equivariant curvature  $F_{A,T}$  is evaluated on  $X^T$ , only the vertical component of  $i_{v_a}$  contributes to the formula (2.5.3) and  $v_a$  pairs with the vertical component of the connection  $A$  on the  $T$ -fiber of  $P$  given by  $g^{-1}dg$ . The  $T$ -action on  $G$ -fibers induces the homomorphism

$$\rho : \mathfrak{t} \rightarrow \mathfrak{g} \quad (2.5.4)$$

and let  $\rho(T_a)$  be the images of  $T_a$  basis elements of  $\mathfrak{t}$ .

An ordinary characteristic class for a principal  $G$ -bundle on  $X$  is  $[p(F_A)] \in H^{2d}(X)$  for a  $G$ -invariant degree  $d$  polynomial  $p \in \mathbb{R}[\mathfrak{g}]^G$ . Here  $F_A$  is the curvature of any connection  $A$  on the  $G$ -bundle.

In the same way, a  $T$ -equivariant characteristic class for a principal  $G$ -bundle associated to a  $G$ -invariant degree  $d$  polynomial  $p \in \mathbb{R}[\mathfrak{g}]^G$  is  $[p(F_{A,T})] \in H_T^{2d}(X)$ . Here  $F_{A,T}$  is the  $T$ -equivariant curvature of any  $T$ -equivariant connection  $A$  on the  $G$ -bundle.

Restricted to  $T$ -fixed points  $X^T$  the  $T$ -equivariant characteristic class associated to polynomial  $p \in \mathbb{R}[\mathfrak{g}]^G$  is

$$p(F_A + \epsilon^a \rho(T_a)) \quad (2.5.5)$$

In particular, if  $V$  is a representation of  $G$  and  $p$  is the Chern character of the vector bundle  $V$ , then if  $X$  is a point, the equivariant Chern characters is an ordinary character of the space  $V$  as a  $G$ -module.

## 2.6 Standard characteristic classes

For a reference see the book by Bott and Tu [16].

### 2.6.1 Euler class

Let  $G = SO(2n)$  be the special orthogonal group which preserves a Riemannian metric  $g \in S^2V^\vee$  on an oriented real vector space  $V$  of  $\dim_{\mathbb{R}} V = 2n$ .

The Euler characteristic class is defined by the adjoint invariant polynomial

$$\text{Pf} : \mathfrak{so}(2n, \mathbb{R}) \rightarrow \mathbb{R} \quad (2.6.1)$$

of degree  $n$  on the Lie algebra  $\mathfrak{so}(2n)$  called *Pfaffian* and defined as follows. For an element  $x \in \mathfrak{so}(2n)$  let  $x' \in V^\vee \otimes V$  denote representation of  $x$  on  $V$  (fundamental representation), so that  $x'$  is an antisymmetric  $(2n) \times (2n)$  matrix in some orthonormal basis of  $V$ . Let  $g \cdot x' \in \Lambda^2 V^\vee$  be the two-form associated by  $g$  to  $x'$ , and let  $v_g \in \Lambda^{2n} V^\vee$  be the standard volume form on  $V$  associated to the metric  $g$ , and  $v_g^* \in \Lambda^{2n} V$  be the dual of  $v_g$ . By definition

$$\text{Pf}(x) = \frac{1}{n!} \langle v_g^*, (g \cdot x')^{\wedge n} \rangle \quad (2.6.2)$$

For example, for the  $2 \times 2$ -blocks diagonal matrix

$$\text{Pf} \begin{pmatrix} 0 & \epsilon_1 & \dots & \dots & 0 & 0 \\ -\epsilon_1 & 0 & \dots & \dots & 0 & 0 \\ \dots & \dots & \dots & \dots & \dots & \dots \\ \dots & \dots & \dots & \dots & \dots & \dots \\ 0 & 0 & \dots & \dots & 0 & \epsilon_n \\ 0 & 0 & \dots & \dots & -\epsilon_n & 0 \end{pmatrix} = \epsilon_1 \dots \epsilon_n \quad (2.6.3)$$

For an antisymmetric  $(2n) \times (2n)$  matrix  $x'$ , the definition implies that  $\text{Pf}(x)$  is a degree  $n$  polynomial of matrix elements of  $x$  which satisfies

$$\text{Pf}(x)^2 = \det x \quad (2.6.4)$$

Let  $P$  be an  $SO(2n)$  principal bundle  $P \rightarrow X$ .

In the standard normalization the Euler class  $e(P)$  is defined in such a way that it takes values in  $H^{2n}(X, \mathbb{Z})$  and is given by

$$e(P) = \frac{1}{(2\pi)^n} [\text{Pf}(F)] \quad (2.6.5)$$

For example, the Euler characteristic of an oriented real manifold  $X$  of real dimension  $2n$  is an integer number given by

$$e(X) = \int_X e(T_X) = \frac{1}{(2\pi)^n} \int_X \text{Pf}(R) \quad (2.6.6)$$

where  $R$  denotes the curvature form of the tangent bundle  $T_X$ .

In quantum field theories the definition (2.6.2) of the Pfaffian is usually realized in terms of a Gaussian integral over the Grassmann (anticommuting) variables  $\theta$  which satisfy  $\theta_i \theta_j = -\theta_j \theta_i$ . The definition (2.6.2) is presented as

$$\text{Pf}(x) = \int d\theta_{2n} \dots d\theta_1 \exp\left(-\frac{1}{2} \theta_i x_{ij} \theta_j\right) \quad (2.6.7)$$

By definition, the integral  $[d\theta_{2n} \dots d\theta_1]$  picks the coefficient of the monomial  $\theta_1 \dots \theta_{2n}$  of an element of the the Grassman algebra generated by  $\theta$ .

## 2.6.2 Euler class of vector bundle and Mathai-Quillen form

See Mathai-Quillen [17] and Aityah-Jeffrey [18].

The Euler class of a vector bundle can be presented in a QFT formalism. Let  $E$  be an oriented real vector bundle  $E$  of rank  $2n$  over a manifold  $X$ .

Let  $x^\mu$  be local coordinates on the base  $X$ , and let their differentials be denoted  $\psi^\mu = dx^\mu$ .

Let  $h^i$  be local coordinates on the fibers of  $E$ . Let  $\Pi E$  denote the superspace obtained from the total space of the bundle  $E$  by inverting the parity of the fibers, so that the coordinates in the fibers of  $\Pi E$  are odd variables  $\chi^i$ . Let  $g_{ij}$  be the matrix of a Riemannian metric on the bundle  $E$ . Let  $A^i_\mu$  be the matrix valued 1-form on  $X$  representing a connection on the bundle  $E$ .

Using the connection  $A$  we can define an odd vector field  $\delta$  on the superspace  $\Pi T(\Pi E)$ , or, equivalently, a de Rham differential on the space of differential forms  $\Omega^\bullet(\Pi E)$ . In local coordinates  $(x^\mu, \psi^\mu)$  and  $(\chi^i, h^i)$  the definition of  $\delta$  is

$$\begin{aligned} \delta x^\mu &= \psi^\mu & \delta \chi^i &= h^i - A^i_{j\mu} \psi^\mu \chi^j \\ \delta \psi^\mu &= 0 & \delta h^i &= \delta(A^i_{j\mu} \psi^\mu \chi^j) \end{aligned} \quad (2.6.8)$$

Here  $h^i = D\chi^i$  is the *covariant* de Rham differential of  $\chi^i$ , so that under the change of framing on  $E$  given by  $\chi^i = s^i_j \tilde{\chi}^j$  the  $h^i$  transforms in the same way, that is  $h^i = s^i_j \tilde{h}^j$ .

The odd vector field  $\delta$  is nilpotent

$$\delta^2 = 0 \quad (2.6.9)$$

and is called de Rham vector field on  $\Pi T(\Pi E)$ .

Consider an element  $\alpha$  of  $\Omega^\bullet(\Pi E)$  defined by the equation

$$\alpha = \frac{1}{(2\pi)^{2n}} \exp(-t\delta V) \quad (2.6.10)$$

where  $t \in \mathbb{R}_{>0}$  and

$$V = \frac{1}{2} (g_{ij} \chi^i h^j) \quad (2.6.11)$$

Notice that since  $h^i$  has been defined as  $D\chi^i$  the definition (2.6.10) is coordinate independent.

To expand the definition of  $\alpha$  (2.6.10) we compute

$$\delta(\chi, h) = (h - A\chi, h) - (\chi, dA\chi - A(h - A\chi)) = (h, h) - (\chi, F_A\chi) \quad (2.6.12)$$

where we suppressed the indices  $i, j$ , the  $d$  denotes the de Rham differential on  $X$  and  $F_A$  the curvature 2-form on the connection  $A$

$$F_A = dA + A \wedge A \quad (2.6.13)$$

The Gaussian integration of the form  $\alpha$  along the vertical fibers of  $\Pi E$  gives

$$\frac{1}{(2\pi)^{2n}} \int [dh][d\chi] \exp\left(-\frac{1}{2}\delta(\chi, h)\right) = \frac{1}{(2\pi)^n} \text{Pf}(F_A) \quad (2.6.14)$$

which agrees with definition of the integer valued Euler class (2.6.5). The representation of the Euler class in the form (2.6.10) is called the Gaussian *Mathai-Quillen representation* of the Thom class.

The Euler class of the vector bundle  $E$  is an element of  $H^{2n}(X, \mathbb{Z})$ . If  $\dim X = 2n$ , the number obtained after integration of the fundamental cycle on  $X$

$$e(E) = \int_{\Pi T(\Pi E)} \alpha \quad (2.6.15)$$

is an integer Euler characteristic of the vector bundle  $E$ .

If  $E = TX$  the equation (2.6.15) provides the Euler characteristic of the manifold  $X$  in the form

$$e(X) = \frac{1}{(2\pi)^{\dim X}} \int_{\Pi T(\Pi TX)} \exp(-t\delta V) \stackrel{t \rightarrow 0}{=} \frac{1}{(2\pi)^{\dim X}} \int_{\Pi T(\Pi TX)} 1 \quad (2.6.16)$$

Given a section  $s$  of the vector bundle  $E$ , we can deform the form  $\alpha$  in the same  $\delta$ -cohomology class by taking

$$V_s = \frac{1}{2}(\chi, h + \sqrt{-1}s) \quad (2.6.17)$$

After integrating over  $(h, \chi)$  the the resulting differential form on  $X$  has factor

$$\exp\left(-\frac{1}{2t}s^2\right) \quad (2.6.18)$$

so it is concentrated in a neighborhood of the locus  $s^{-1}(0) \subset X$  of zeroes of the section  $s$ .

In this way the Poincare-Hopf theorem is proven: given an oriented vector bundle  $E$  on an oriented manifold  $X$ , with  $\text{rank } E = \dim X$ , the Euler characteristic of  $E$  is equal to the number of zeroes of a generic section  $s$  of  $E$  counted with orientation

$$e(E) = \sum_{x \in s^{-1}(0) \subset X} \text{sign det } ds|_x \quad (2.6.19)$$

where  $ds|_x : T_x \rightarrow E_x$  is the differential of the section  $s$  at a zero  $x \in s^{-1}(0)$ . The assumption that  $s$  is a generic section implies that  $\text{det } ds|_x$  is non-zero.

For a short reference on the Mathai-Quillen formalism see [19].

### 2.6.3 Chern character

Let  $P$  be a principal  $GL(n, \mathbb{C})$  bundle over a manifold  $X$ . The Chern character is an adjoint invariant function

$$\text{ch} : \mathfrak{gl}(n, \mathbb{C}) \rightarrow \mathbb{C} \quad (2.6.20)$$

defined as the trace in the fundamental representation of the exponential map

$$\text{ch} : x \mapsto \text{tr } e^x \quad (2.6.21)$$

The exponential map is defined by formal series

$$\text{tr } e^x = \sum_{n=0}^{\infty} \frac{1}{n!} \text{tr } x^n \quad (2.6.22)$$

The eigenvalues of the  $gl(n, \mathbb{C})$  matrix  $x$  are called *Chern roots*. In terms of the Chern roots the Chern character is

$$\text{ch}(x) = \sum_{i=1}^n e^{x_i} \quad (2.6.23)$$

### 2.6.4 Chern class

Let  $P$  be a principal  $GL(n, \mathbb{C})$  bundle over a manifold  $X$ . The Chern class  $c_k$  for  $k \in \mathbb{Z}_{>0}$  of  $x \in \mathfrak{gl}(n, \mathbb{C})$  is defined by expansion of the determinant

$$\det(1 + tx) = \sum_{k=0}^n t^k c_k \quad (2.6.24)$$

In particular

$$c_1(x) = \text{tr } x, \quad c_n(x) = \det x \quad (2.6.25)$$

In terms of Chern roots  $c_k$  is defined by elementary symmetric monomials

$$c_k = \sum_{1 \leq i_1 < i_2 < \dots < i_k \leq n} x_{i_1} \dots x_{i_k} \quad (2.6.26)$$

*Remark on integrality.* Our conventions for characteristic classes of  $GL(n, \mathbb{C})$  bundles differ from the frequently used conventions in which Chern classes  $c_k$  take value in  $H^{2k}(X, \mathbb{Z})$  by a factor of  $(-2\pi\sqrt{-1})^k$ . In our conventions the characteristic class of degree  $2k$  needs to be multiplied by  $\frac{1}{(-2\pi\sqrt{-1})^k}$  to be integral.

### 2.6.5 Todd class

Let  $P$  be a principal  $GL(n, \mathbb{C})$  bundle over a manifold  $X$ . The Todd class of  $x \in \mathfrak{gl}(n, \mathbb{C})$  is defined to be

$$\text{td}(x) = \det \frac{x}{1 - e^{-x}} = \prod_{i=1}^n \frac{x_i}{1 - e^{-x_i}} \quad (2.6.27)$$

where  $\det$  is evaluated in the fundamental representation. The ratio evaluates to a series expansion involving Bernoulli numbers  $B_k$

$$\frac{x}{1 - e^{-x}} = \sum_{k=0}^{\infty} \frac{(-1)^k}{k!} B_k x^k = 1 + \frac{x}{2} + \frac{x^2}{12} - \frac{x^4}{720} + \dots \quad (2.6.28)$$

### 2.6.6 The $\hat{A}$ class

Let  $P$  be a principal  $GL(n, \mathbb{C})$  bundle over a manifold  $X$ . The  $\hat{A}$  class of  $x \in GL(n, \mathbb{C})$  is defined as

$$\hat{A} = \det \frac{x}{e^{\frac{x}{2}} - e^{-\frac{x}{2}}} = \prod_{i=1}^n \frac{x_i}{e^{x_i/2} - e^{-x_i/2}} \quad (2.6.29)$$

The  $\hat{A}$  class is related to the Todd class by

$$\hat{A}(x) = \det e^{-\frac{x}{2}} \text{td } x \quad (2.6.30)$$

## 2.7 Index formula

For a holomorphic vector bundle  $E$  over a complex variety  $X$  of  $\dim_{\mathbb{C}} X = n$  the index  $\text{ind}(\bar{\partial}, E)$  is defined as

$$\text{ind}(\bar{\partial}, E) = \sum_{k=0}^n (-1)^k \dim H^k(X, E) \quad (2.7.1)$$

The localization theorem in  $K$ -theory gives the index formula of Grothendieck-Riemann-Roch-Hirzebruch-Atiyah-Singer relating the index to the Todd class

$$\boxed{\text{ind}(\bar{\partial}, E) = \frac{1}{(-2\pi\sqrt{-1})^n} \int_X \text{td}(T_X^{1,0}) \text{ch}(E)} \quad (2.7.2)$$

Similarly, the index of Dirac operator  $\not{D} : S^+ \otimes E \rightarrow S^- \otimes E$  from the positive chiral spinors  $S^+$  to the negative chiral spinors  $S^-$ , twisted by a vector bundle  $E$ , is defined as

$$\text{ind}(\not{D}, E) = \dim \ker \not{D} - \dim \text{coker } \not{D} \quad (2.7.3)$$

and is given by the Atiyah-Singer index formula

$$\boxed{\text{ind}(\not{D}, E) = \frac{1}{(-2\pi\sqrt{-1})^n} \int_X \hat{A}(T_X^{1,0}) \text{ch}(E)} \quad (2.7.4)$$

Notice that on a Kahler manifold the Dirac complex

$$\not{D} : S^+ \rightarrow S^-$$

is isomorphic to the Dolbeault complex

$$\dots \rightarrow \Omega^{0,p}(X) \xrightarrow{\bar{\partial}} \Omega^{0,p+1}(X) \rightarrow \dots$$

twisted by the square root of the canonical bundle  $K = \Lambda^n(T_X^{1,0})^\vee$

$$\mathcal{D} = \bar{\partial} \otimes K^{\frac{1}{2}} \tag{2.7.5}$$

consistently with the relation (2.6.30) and the Riemann-Roch-Hirzebruch-Atiyah-Singer index formula

*Remark on  $2\pi$  and  $\sqrt{-1}$  factors.* The vector bundle  $E$  in the index formula (2.7.2) can be promoted to a complex

$$\rightarrow E^\bullet \rightarrow E^{\bullet+1} \rightarrow \tag{2.7.6}$$

In particular, the  $\bar{\partial}$  index of the complex  $E^\bullet = \Lambda^\bullet(T_X^{1,0})^\vee$  of  $(\bullet, 0)$ -forms on a Kahler variety  $X$  equals the Euler characteristic of  $X$

$$e(X) = \text{ind}(\bar{\partial}, \Lambda^\bullet(T_X^{1,0})^\vee) = \sum_{q=0}^n \sum_{p=0}^n (-1)^{p+q} \dim H^{p,q}(X) \tag{2.7.7}$$

We find

$$\text{ch } \Lambda^\bullet(T_X^{1,0})^\vee = \prod_{i=1}^n (1 - e^{-x_i}) \tag{2.7.8}$$

where  $x_i$  are Chern roots of the curvature of the  $n$ -dimensional complex bundle  $T_X^{1,0}$ . Hence, the Todd index formula (2.7.2) gives

$$e(X) = \frac{1}{(2\pi\sqrt{-1})^n} \int c_n(T_X^{1,0}) \tag{2.7.9}$$

The above agrees with the Euler characteristic (2.6.6) provided it holds that

$$\det(\sqrt{-1}x_{u(n)}) = \text{Pf}(x_{\mathfrak{so}(2n)}) \tag{2.7.10}$$

where  $x_{\mathfrak{so}(2n)}$  represents the curvature of the  $2n$ -dimensional real tangent bundle  $T_X$  as  $2n \times 2n$  antisymmetric matrices, and  $x_{u(n)}$  represents the curvature of the complex holomorphic  $n$ -dimensional tangent bundle  $T_X^{(1,0)}$  as  $n \times n$  anti-hermitian matrices. That (2.7.10) holds is clear from the  $(2 \times 2)$  representation of  $\sqrt{-1}$

$$\sqrt{-1} \mapsto \begin{pmatrix} 0 & -1 \\ 1 & 0 \end{pmatrix} \tag{2.7.11}$$

## 2.8 Equivariant integration

See the paper by Atiyah and Bott [20].

## 2.8.1 Thom isomorphism and Atiyah-Bott localization

A map

$$f : F \rightarrow X$$

of manifolds induces a natural pushforward map on the homology

$$f_* : H_\bullet(F) \rightarrow H_\bullet(X)$$

and pullback on the cohomology

$$f^* : H^\bullet(X) \rightarrow H^\bullet(F)$$

In the situation when there is Poincaré duality between homology and cohomology we can construct pushforward operation on the cohomology

$$f_* : H^\bullet(F) \rightarrow H^\bullet(X) \tag{2.8.1}$$

We can display the pullback and pushforward maps on the diagram

$$H^\bullet(F) \begin{array}{c} \xrightarrow{f_*} \\ \xleftarrow{f^*} \end{array} H^\bullet(X) \tag{2.8.2}$$

For example, if  $F$  and  $X$  are compact manifolds and  $f : F \hookrightarrow X$  is the inclusion, then for the pushforward map  $f_* : H^\bullet(F) \rightarrow H^\bullet(X)$  we find

$$f_* 1 = \Phi_F \tag{2.8.3}$$

where  $\Phi_F$  is the cohomology class in  $H^\bullet(X)$  which is Poincaré dual to the manifold  $F \subset X$ : for a form  $\alpha$  on  $X$  we have

$$\int_F f^* \alpha = \int_X \Phi_F \wedge \alpha \tag{2.8.4}$$

If  $X$  is the total space of the orthogonal vector bundle  $\pi : X \rightarrow F$  over the oriented manifold  $F$  then  $\Phi_F(X)$  is called the Thom class of the vector bundle  $X$  and  $f_* : H^\bullet(F) \rightarrow H^\bullet(X)$  is the Thom isomorphism: to a form  $\alpha$  on  $F$  we associate a form  $\Phi \wedge \pi^* \alpha$  on  $X$ . The important property of the Thom class  $\Phi_F$  for a submanifold  $F \hookrightarrow X$  is

$$f^* \Phi_F = e(\nu_F) \tag{2.8.5}$$

where  $e(\nu_F)$  is the Euler class of the normal bundle to  $F$  in  $X$ . Combined with (2.8.3) the last equation gives

$$f^* f_* 1 = e(\nu_F) \tag{2.8.6}$$

as a map  $H^\bullet(F) \rightarrow H^\bullet(F)$ .

More generally, if  $f : F \hookrightarrow X$  is an inclusion of a manifold  $F$  into a manifold  $X$  the Poincaré dual class  $\Phi_F$  is isomorphic to the Thom class of the normal bundle of  $F$  in  $X$ .

Now we consider  $T$ -equivariant cohomologies for a compact abelian Lie group  $T$  acting on  $X$ . Let  $F = X^T$  be the set of  $T$  fixed points in  $X$ . Then the equivariant Euler class  $e_T(\nu_F)$  is invertible, therefore the identity map on  $H_T^\bullet(X)$  can be presented as

$$1 = f_* \frac{1}{e_T(\nu_F)} f^* \quad (2.8.7)$$

Let  $\pi^X : X \rightarrow pt$  be the map from a manifold  $X$  to a point  $pt$ . The pushforward operator  $\pi_*^X : H_T^\bullet(X) \rightarrow H_T^\bullet(pt)$  corresponds to the integration of the cohomology class over  $X$ . The pushforward is functorial. For maps  $F \xrightarrow{f} X \xrightarrow{\pi^X} pt$  we have the composition  $\pi_*^X f_* = \pi_*^F$  for  $F \xrightarrow{\pi^F} pt$ . So we arrive to the Atiyah-Bott integration formula

$$\pi_*^X = \pi_*^F \frac{f^*}{e_T(\nu_F)} \quad (2.8.8)$$

or more explicitly

$$\boxed{\int_X \alpha = \int_F \frac{f^* \alpha}{e_T(\nu_F)}} \quad (2.8.9)$$

## 2.8.2 Duistermaat-Heckman localization

A particular example where the Atiyah-Bott localization formula can be applied is a symplectic space on which a Lie group  $T$  acts in a Hamiltonian way. Namely, let  $(X, \omega)$  be a real symplectic manifold of  $\dim_{\mathbb{R}} X = 2n$  with symplectic form  $\omega$  and let compact connected Lie group  $T$  act on  $X$  in Hamiltonian way, which means that there exists a function, called *moment map* or Hamiltonian

$$\mu : X \rightarrow \mathfrak{t}^\vee \quad (2.8.10)$$

such that

$$d\mu_a = -i_a \omega \quad (2.8.11)$$

in some basis  $(T_a)$  of  $\mathfrak{t}$  where  $i_a$  is the contraction operation with the vector field generated by the  $T_a$  action on  $X$ .

The degree 2 element  $\omega_T \in \Omega^\bullet(X) \otimes St^*$  defined by the equation

$$\omega_T = \omega + \epsilon^a \mu_a \quad (2.8.12)$$

is a  $d_T$ -closed equivariant differential form:

$$d_T \omega_T = (d + \epsilon^a i_a)(\omega + \epsilon^b \mu_b) = \epsilon^a d\mu_a + \epsilon^a i_a \omega = 0 \quad (2.8.13)$$

This implies that the mixed-degree equivariant differential form

$$\alpha = e^{\omega_T} \quad (2.8.14)$$

is also  $d_T$ -closed, and we can apply the Atiyah-Bott localization formula to the integral

$$\int_X \exp(\omega_T) = \frac{1}{n!} \int_X \omega^n \exp(\epsilon^a \mu_a) \quad (2.8.15)$$

For  $T = SO(2)$  so that  $\text{Lie}(SO(2)) \simeq \mathbb{R}$  the integral (2.8.15) is the typical partition function of a classical Hamiltonian mechanical system in statistical physics with Hamiltonian function  $\mu : X \rightarrow \mathbb{R}$  and inverse temperature parameter  $-\epsilon$ .

Suppose that  $T = SO(2)$  and that the set of fixed points  $X^T$  is discrete. Then the Atiyah-Bott localization formula (2.8.9) implies

$$\boxed{\frac{1}{n!} \int_X \omega^n \exp(\epsilon^a \mu_a) = \sum_{x \in X^T} \frac{\exp(\epsilon^a \mu_a)}{e_T(\nu_x)}} \quad (2.8.16)$$

where  $\nu_x$  is the normal bundle to a fixed point  $x \in X^T$  in  $X$  and  $e_T(\nu_x)$  is the  $T$ -equivariant Euler class of the bundle  $\nu_x$ .

The rank of the normal bundle  $\nu_x$  is  $2n$  and the structure group is  $SO(2n)$ . In notations of section 2.5 we evaluate the  $T$ -equivariant characteristic Euler class of the principal  $G$ -bundle for  $T = SO(2)$  and  $G = SO(2n)$  by equation (2.5.5) for the invariant polynomial on  $\mathfrak{g} = \mathfrak{so}(2n)$  given by  $p = \frac{1}{(2\pi)^n} \text{Pf}$  according to definition (2.6.5).

### 2.8.3 Gaussian integral example

To illustrate the localization formula (2.8.16) suppose that  $X = \mathbb{R}^{2n}$  with symplectic form

$$\omega = \sum_{i=1}^n dx^i \wedge dy_i \quad (2.8.17)$$

and  $SO(2)$  action

$$\begin{pmatrix} x_i \\ y_i \end{pmatrix} \mapsto \begin{pmatrix} \cos w_i \theta & -\sin w_i \theta \\ \sin w_i \theta & \cos w_i \theta \end{pmatrix} \begin{pmatrix} x_i \\ y_i \end{pmatrix} \quad (2.8.18)$$

where  $\theta \in \mathbb{R}/(2\pi\mathbb{Z})$  parametrizes  $SO(2)$  and  $(w_1, \dots, w_n) \in \mathbb{Z}^n$ .

The point  $0 \in X$  is the *fixed point* so that  $X^T = \{0\}$ , and the normal bundle  $\nu_x = T_0X$  is an  $SO(2)$ -module of real dimension  $2n$  and complex dimension  $n$  that splits into a direct sum of  $n$  irreducible  $SO(2)$  modules with weights  $(w_1, \dots, w_n)$ .

We identify  $\text{Lie}(SO(2))$  with  $\mathbb{R}$  with basis element  $\{1\}$  and coordinate function  $\epsilon \in \text{Lie}(SO(2))^*$ . The  $SO(2)$  action (2.8.18) is Hamiltonian with respect to the moment map

$$\mu = \mu_0 + \frac{1}{2} \sum_{i=1}^n w_i (x_i^2 + y_i^2) \quad (2.8.19)$$

Assuming that  $\epsilon < 0$  and all  $w_i > 0$  we find by direct Gaussian integration

$$\frac{1}{n!} \int_X \omega^n \exp(\epsilon \mu) = \frac{(2\pi)^n}{(-\epsilon)^n \prod_{i=1}^n w_i} \exp(\epsilon \mu_0) \quad (2.8.20)$$

and the same result by the localization formula (2.8.16) because

$$e_T(\nu_x) = \frac{1}{(2\pi)^n} \text{Pf}(\epsilon\rho(1)) \quad (2.8.21)$$

according to the definition of the  $T$ -equivariant class (2.5.5) and the Euler characteristic class (2.6.5), and where  $\rho : \text{Lie}(SO(2)) \rightarrow \text{Lie}(SO(2n))$  is the homomorphism in (2.5.4) with

$$\rho(1) = \begin{pmatrix} 0 & -w_1 & \dots & \dots & 0 & 0 \\ w_1 & 0 & \dots & \dots & 0 & 0 \\ \dots & \dots & \dots & \dots & \dots & \dots \\ \dots & \dots & \dots & \dots & \dots & \dots \\ 0 & 0 & \dots & \dots & 0 & -w_n \\ 0 & 0 & \dots & \dots & w_n & 0 \end{pmatrix} \quad (2.8.22)$$

according to (2.8.18).

### 2.8.4 Example of a two-sphere

Let  $(X, \omega)$  be the two-sphere  $S^2$  with coordinates  $(\theta, \alpha)$  and symplectic structure

$$\omega = \sin \theta d\theta \wedge d\alpha \quad (2.8.23)$$

Let the Hamiltonian function be

$$H = -\cos \theta \quad (2.8.24)$$

so that

$$\omega = dH \wedge d\alpha \quad (2.8.25)$$

and the Hamiltonian vector field be  $v_H = \partial_\alpha$ . The differential form

$$\omega_T = \omega + \epsilon H = \sin \theta d\theta \wedge d\alpha - \epsilon \cos \theta$$

is  $d_T$ -closed for

$$d_T = d + \epsilon i_\alpha \quad (2.8.26)$$

Let

$$\alpha = e^{t\omega_T} \quad (2.8.27)$$

Locally there is a degree 1 form  $V$  such that  $\omega_T = d_TV$ , for example

$$V = -(\cos \theta)d\alpha \quad (2.8.28)$$

but globally  $V$  does not exist. The  $d_T$ -cohomology class  $[\alpha]$  of the form  $\alpha$  is non-zero.

The localization formula (2.8.15) gives

$$\int_X \exp(\omega_T) = \frac{2\pi}{-\epsilon} \exp(-\epsilon) + \frac{2\pi}{\epsilon} \exp(\epsilon) \quad (2.8.29)$$

where the first term is the contribution of the  $T$ -fixed point  $\theta = 0$  and the second term is the contribution of the  $T$ -fixed point  $\theta = \pi$ .

## 2.9 Equivariant index formula (Dolbeault and Dirac)

Let  $G$  be a compact connected Lie group.

Suppose that  $X$  is a complex variety and  $E$  is a holomorphic  $G$ -equivariant vector bundle over  $X$ . Then the cohomology groups  $H^\bullet(X, E)$  form representation of  $G$ . In this case the index of  $E$  (2.7.1) can be refined to *an equivariant index* or *character*

$$\mathrm{ind}_G(\bar{\partial}, E) = \sum_{k=0}^n (-1)^k \mathrm{ch}_G H^k(X, E) \quad (2.9.1)$$

where  $\mathrm{ch}_G H^i(X, E)$  is the character of a representation of  $G$  in the vector space  $H^i(X, E)$ . More concretely, the equivariant index can be thought of as a gadget that attaches to  $G$ -equivariant holomorphic bundle  $E$  a complex valued adjoint invariant function on the group  $G$

$$\mathrm{ind}_G(\bar{\partial}, E)(g) = \sum_{k=0}^n (-1)^k \mathrm{tr}_{H^k(X, E)} g \quad (2.9.2)$$

on elements  $g \in G$ . The sign alternating sum (2.9.2) is also known as *the supertrace*

$$\mathrm{ind}_G(\bar{\partial}, E)(g) = \mathrm{str}_{H^\bullet(X, E)} g \quad (2.9.3)$$

The index formula (2.7.2) is replaced by the equivariant index formula in which characteristic classes are promoted to  $G$ -equivariant characteristic classes in the Cartan model of  $G$ -equivariant cohomology with differential  $d_G = d + \phi^a i_a$  as in (2.4.10)

$$\mathrm{ind}(\bar{\partial}, E)(e^{\phi^a T_a}) = \frac{1}{(-2\pi\sqrt{-1})^n} \int_X \mathrm{td}_G(T_X) \mathrm{ch}_G(E) = \int_X e_G(T_X) \frac{\mathrm{ch}_G E}{\mathrm{ch}_G \Lambda^\bullet T_X^\vee} \quad (2.9.4)$$

Here  $\phi^a T_a$  is an element of Lie algebra of  $G$  and  $e^{\phi^a T_a}$  is an element of  $G$ , and  $T_X$  denotes the holomorphic tangent bundle of the complex manifold  $X$ .

If the set  $X^G$  of  $G$ -fixed points is discrete, then applying the localization formula (2.8.9) to the equivariant index (2.9.4) we find the equivariant Lefschetz formula

$$\boxed{\mathrm{ind}(\bar{\partial}, E)(g) = \sum_{x \in X^G} \frac{\mathrm{tr}_{E_x}(g)}{\det_{T_x^{1,0} X}(1 - g^{-1})}} \quad (2.9.5)$$

The Euler character is cancelled against the numerator of the Todd character.

### Example of $\mathbb{C}\mathbb{P}^1$

Let  $X$  be  $\mathbb{C}\mathbb{P}^1$  and let  $E = \mathcal{O}(n)$  be a complex line bundle of degree  $n$  over  $\mathbb{C}\mathbb{P}^1$ , and let  $G = U(1)$  equivariantly act on  $E$  as follows. Let  $z$  be a local coordinate on  $\mathbb{C}\mathbb{P}^1$ , and let an element  $t \in U(1) \subset \mathbb{C}^\times$  send the point with coordinate  $z$  to the point with coordinate  $tz$  so that

$$\mathrm{ch} T_0^{1,0} X = t \quad \mathrm{ch} T_\infty^{1,0} X = t^{-1} \quad (2.9.6)$$

where  $T_0^{1,0}X$  denotes the fiber of the holomorphic tangent bundle at  $z = 0$  and similarly  $T_\infty^{1,0}X$  the fiber at  $z = \infty$ . Let the action of  $U(1)$  on the fiber of  $E$  at  $z = 0$  be trivial. Then the action of  $U(1)$  on the fiber of  $E$  at  $z = \infty$  is found from the gluing relation

$$s_\infty = z^{-n}s_0 \quad (2.9.7)$$

to be of weight  $-n$ , so that

$$\text{ch } E|_{z=0} = 1, \quad \text{ch } E|_{z=\infty} = t^{-n} \quad (2.9.8)$$

Then

$$\text{ind}(\bar{\partial}, \mathcal{O}(n), \mathbb{CP}^1)(t) = \frac{1}{1-t^{-1}} + \frac{t^{-n}}{1-t} = \frac{1-t^{-n-1}}{1-t^{-1}} = \begin{cases} \sum_{k=0}^n t^{-k}, & n \geq 0 \\ 0, & n = -1, \\ -t \sum_{k=0}^{-n-2} t^k, & n < -1 \end{cases} \quad (2.9.9)$$

We can check against the direct computation. Assume  $n \geq 0$ . The kernel of  $\bar{\partial}$  is spanned by  $n+1$  holomorphic sections of  $\mathcal{O}(n)$  of the form  $z^k$  for  $k = 0, \dots, n$ , the cokernel is empty by Riemann-Roch. The section  $z^k$  is acted upon by  $t \in T$  with weight  $t^{-k}$ . Therefore

$$\text{ind}_T(\bar{\partial}, \mathcal{O}(n), \mathbb{CP}^1) = \sum_{k=0}^n t^{-k} \quad (2.9.10)$$

Even more explicitly, for illustration, choose a connection 1-form  $A$  with constant curvature  $F_A = -\frac{1}{2}in\omega$ , denoted in the patch around  $\theta = 0$  (or  $z = 0$ ) by  $A^{(0)}$  and in the patch around  $\theta = \pi$  (or  $z = \infty$ ) by  $A^{(\pi)}$

$$A^{(0)} = -\frac{1}{2}in(1 - \cos \theta)d\alpha \quad A^{(\pi)} = -\frac{1}{2}in(-1 - \cos \theta)d\alpha \quad (2.9.11)$$

The gauge transformation between the two patches

$$A^{(0)} = A^{(\pi)} - in d\alpha \quad (2.9.12)$$

is consistent with the defining  $E$  bundle transformation rule for the sections  $s^{(0)}, s^{(\pi)}$  in the patches around  $\theta = 0$  and  $\theta = \pi$

$$s^{(0)} = z^n s^{(\pi)} \quad A^{(0)} = A^{(\pi)} + z^n dz^{-n}. \quad (2.9.13)$$

The equivariant curvature  $F_T$  of the connection  $A$  in the bundle  $E$  is given by

$$F_T = -\frac{1}{2}in(\omega + \epsilon(1 - \cos \theta)) \quad (2.9.14)$$

as can be verified against the definition (2.5.3)  $F_T = F + \epsilon i_v A$ . Notice that to verify the expression for the equivariant curvature (2.9.14) in the patch near  $\theta = \pi$  one needs to take into account contributions from the vertical component  $g^{-1}dg$  of the connection  $A$  on the

total space of the principal  $U(1)$  bundle and from the  $T$ -action on the fiber at  $\theta = \pi$  with weight  $-n$ .

Then

$$\begin{aligned} \text{ch}(E)|_{\theta=0} &= \exp(F_T)|_{\theta=0} = 1 \\ \text{ch}(E)|_{\theta=\pi} &= \exp(F_T)|_{\theta=\pi} = \exp(-in\epsilon) = t^{-n} \end{aligned} \quad (2.9.15)$$

for  $t = \exp(i\epsilon)$  in agreement with (2.9.9).

A similar exercise gives the index for the Dirac operator on  $S^2$  twisted by a magnetic field of flux  $n$

$$\text{ind}(\not{D}, \mathcal{O}(n), S^2) = \frac{t^{n/2} - t^{-n/2}}{t^{1/2} - t^{-1/2}} \quad (2.9.16)$$

where now we have chosen the lift of the  $T$ -action symmetrically to be of weight  $n/2$  at  $\theta = 0$  and of weight  $-n/2$  at  $\theta = \pi$ . Also notice that up to overall multiplication by a power of  $t$  related to the choice of lift of the  $T$ -action to the fibers of the bundle  $E$ , the relation (2.7.5) holds

$$\text{ind}(\not{D}, \mathcal{O}(n), S^2) = \text{ind}(\bar{\not{D}}, \mathcal{O}(n-1), \mathbb{C}\mathbb{P}^1) \quad (2.9.17)$$

because on  $\mathbb{C}\mathbb{P}^1$  the canonical bundle is  $K = \mathcal{O}(-2)$ .

### Example of $\mathbb{C}\mathbb{P}^m$

. Let  $X = \mathbb{C}\mathbb{P}^m$  be defined by the projective coordinates  $(x_0 : x_1 : \dots : x_m)$  and  $L_n$  be the line bundle  $L_n = \mathcal{O}(n)$ . Let  $T = U(1)^{(m+1)}$  act on  $X$  by

$$(x_0 : x_1 : \dots : x_m) \mapsto (t_0^{-1}x_0 : t_1^{-1}x_1 : \dots : t_m^{-1}x_m) \quad (2.9.18)$$

and by  $t_k^n$  on the fiber of the bundle  $L_n$  in the patch around the  $k$ -th fixed point  $x_k = 1, x_{i \neq k} = 0$ . We find the index as a sum of contributions from  $m+1$  fixed points

$$\text{ind}_T(D) = \sum_{k=0}^m \frac{t_k^n}{\prod_{j \neq k} (1 - (t_j/t_k))} \quad (2.9.19)$$

For  $n \geq 0$  the index is a homogeneous polynomial in  $\mathbb{C}[t_0, \dots, t_m]$  of degree  $n$  representing the character on the space of holomorphic sections of the  $\mathcal{O}(n)$  bundle over  $\mathbb{C}\mathbb{P}^m$ .

$$\text{ind}_T(D) = \begin{cases} s_n(t_0, \dots, t_m), & n \geq 0 \\ 0, & -m \leq n < 0 \\ (-1)^m t_0^{-1} t_1^{-1} \dots t_m^{-1} s_{-n-m-1}(t_0^{-1}, \dots, t_m^{-1}), & n \leq -m-1 \end{cases} \quad (2.9.20)$$

where  $s_n(t_0, \dots, t_m)$  are complete homogeneous symmetric polynomials. This result can be quickly obtained from the contour integral representation of the sum (2.9.19)

$$\frac{1}{2\pi i} \oint_{\mathcal{C}} \frac{dz}{z} \frac{z^n}{\prod_{j=0}^m (1 - t_j/z)} = \sum_{k=0}^m \frac{t_k^n}{\prod_{j \neq k} (1 - (t_j/t_k))}, \quad (2.9.21)$$

If  $n \geq -m$  we pick the contour of integration  $\mathcal{C}$  to enclose all residues  $z = t_j$ . The residue at  $z = 0$  is zero and the sum of residues is (2.9.19). On the other hand, the same contour integral is evaluated by the residue at  $z = \infty$  which is computed by expanding all fractions in inverse powers of  $z$ , and is given by the complete homogeneous polynomial in  $t_i$  of degree  $n$ .

If  $n < -m$  we assume that the contour of integration is a small circle around the  $z = 0$  and does not include any of the residues  $z = t_j$ . Summing the residues outside of the contour, and taking that  $z = \infty$  does not contribute, we get (2.9.19) with the  $(-)$  sign. The residue at  $z = 0$  contributes by (2.9.20).

Also notice that the last line of (2.9.20) relates<sup>1</sup> to the first line by the reflection  $t_i \rightarrow t_i^{-1}$

$$\frac{t_k^n}{\prod_{j \neq k} (1 - t_j/t_k)} = \frac{(-1)^m (t_k^{-1})^{-n-m-1} (\prod_j t_j^{-1})}{\prod_{j \neq k} (1 - t_j^{-1}/t_k^{-1})} \quad (2.9.22)$$

which is the consequence of the Serre duality on  $\mathbb{C}\mathbb{P}^m$ .

## 2.10 Equivariant index and representation theory

The  $\mathbb{C}\mathbb{P}^1$  in example (2.9.16) can be thought of as a flag manifold  $SU(2)/U(1)$ , and (2.9.9) (2.9.16) as characters of  $SU(2)$ -modules. For index theory on general flag manifolds  $G_{\mathbb{C}}/B_{\mathbb{C}}$ , that is Borel-Weyl-Bott theorem<sup>2</sup>, the shift of the form (2.9.17) is a shift by the Weyl vector  $\rho = \sum_{\alpha > 0} \alpha$  where  $\alpha$  are positive roots of  $\mathfrak{g}$ .

The index formula with localization to the fixed points on a flag manifold is equivalent to the Weyl character formula.

The generalization of formula (2.9.16) for generic flag manifold appearing from a co-adjoint orbit in  $\mathfrak{g}^*$  is called *Kirillov character formula* [21], [22], [23].

Let  $G$  be a compact simple Lie group. The Kirillov character formula equates the  $T$ -equivariant index of the Dirac operator  $\text{ind}_T(D)$  on the  $G$ -coadjoint orbit of the element  $\lambda + \rho \in \mathfrak{g}^*$  with the character  $\chi_\lambda$  of the  $G$  irreducible representation with highest weight  $\lambda$ .

The character  $\chi_\lambda$  is a function  $\mathfrak{g} \rightarrow \mathbb{C}$  determined by the representation of the Lie group  $G$  with highest weight  $\lambda$  as

$$\chi_\lambda : X \mapsto \text{tr}_\lambda e^X, \quad X \in \mathfrak{g} \quad (2.10.1)$$

Let  $X_\lambda$  be an orbit of the co-adjoint action by  $G$  on  $\mathfrak{g}^*$ . Such orbit is specified by an element  $\lambda \in \mathfrak{t}^*/W$  where  $\mathfrak{t}$  is the Lie algebra of the maximal torus  $T \subset G$  and  $W$  is the Weyl group. The co-adjoint orbit  $X_\lambda$  is a homogeneous symplectic  $G$ -manifold with the canonical symplectic structure  $\omega$  defined at point  $x \in X \subset \mathfrak{g}^*$  on tangent vectors in  $\mathfrak{g}$  by the formula

$$\omega_x(\bullet_1, \bullet_2) = \langle x, [\bullet_1, \bullet_2] \rangle \quad \bullet_1, \bullet_2 \in \mathfrak{g} \quad (2.10.2)$$

The converse is also true: any homogeneous symplectic  $G$ -manifold is locally isomorphic to a coadjoint orbit of  $G$  or central extension of it.

<sup>1</sup>Thanks to Bruno Le Floch for the comment

<sup>2</sup>For a short presentation see exposition by J. Lurie at <http://www.math.harvard.edu/~lurie/papers/bwb.pdf>

The minimal possible stabilizer of  $\lambda$  is the maximal abelian subgroup  $T \subset G$ , and the maximal co-adjoint orbit is  $G/T$ . Such orbit is called a *full flag manifold*. The real dimension of the full flag manifold is  $2n = \dim G - \text{rk } G$ , and is equal to the number of roots of  $\mathfrak{g}$ . If the stabilizer of  $\lambda$  is a larger group  $H$ , such that  $T \subset H \subset G$ , the orbit  $X_\lambda$  is called a *partial flag manifold*  $G/H$ . A degenerate flag manifold is a projection from the full flag manifold with fibers isomorphic to  $H/T$ .

Flag manifolds are equipped with natural complex and Kahler structure. There is an explicitly holomorphic realization of the flag manifolds as a complex quotient  $G_{\mathbb{C}}/P_{\mathbb{C}}$  where  $G_{\mathbb{C}}$  is the complexification of the compact group  $G$  and  $P_{\mathbb{C}} \subset G_{\mathbb{C}}$  is a parabolic subgroup. Let  $\mathfrak{g} = \mathfrak{g}_- \oplus \mathfrak{h} \oplus \mathfrak{g}_+$  be the standard decomposition of  $\mathfrak{g}$  into the Cartan  $\mathfrak{h}$  algebra and the upper triangular  $\mathfrak{g}_+$  and lower triangular  $\mathfrak{g}_-$  subspaces.

The minimal parabolic subgroup is known as Borel subgroup  $B_{\mathbb{C}}$ , its Lie algebra is conjugate to  $\mathfrak{h} \oplus \mathfrak{g}_+$ . The Lie algebra of generic parabolic subgroup  $P_{\mathbb{C}} \supset B_{\mathbb{C}}$  is conjugate to the direct sum of  $\mathfrak{h} \oplus \mathfrak{g}_+$  and a proper subspace of  $\mathfrak{g}_-$ .

Full flag manifolds with integral symplectic structure are in bijection with irreducible  $G$ -representations  $\pi_\lambda$  of highest weight  $\lambda$

$$X_{\lambda+\rho} \leftrightarrow \pi_\lambda \quad (2.10.3)$$

This is known as the Kirillov correspondence in geometric representation theory.

Namely, if  $\lambda \in \mathfrak{g}^*$  is a weight, the symplectic structure  $\omega$  is integral and there exists a line bundle  $L \rightarrow X_\lambda$  with a unitary connection of curvature  $\omega$ . The line bundle  $L \rightarrow X_\lambda$  is acted upon by the maximal torus  $T \subset G$  and we can study the  $T$ -equivariant geometric objects. The Kirillov-Berline-Getzler-Vergne character formula equates the equivariant index of the Dirac operator  $\mathcal{D}$  twisted by the line bundle  $L \rightarrow X_{\lambda+\rho}$  on the co-adjoint orbit  $X_{\lambda+\rho}$  with the character  $\chi_\lambda$  of the irreducible representation of  $G$  with highest weight  $\lambda$

$$\text{ind}_T(\mathcal{D})(X_{\lambda+\rho}) = \chi_\lambda \quad (2.10.4)$$

This formula can be easily proven using the Atiyah-Singer equivariant index formula

$$\text{ind}_T(\mathcal{D})(X_{\lambda+\rho}) = \frac{1}{(-2\pi i)^n} \int_{X_{\lambda+\rho}} \text{ch}_T(L) \hat{A}_T(T_X) \quad (2.10.5)$$

and the Atiyah-Bott formula to localize the integral over  $X_{\lambda+\rho}$  to the set of fixed points  $X_{\lambda+\rho}^T$ .

The localization to  $X_{\lambda+\rho}^T$  yields the Weyl formula for the character. Indeed, the stabilizer of  $\lambda + \rho$ , where  $\lambda$  is a dominant weight, is the Cartan torus  $T \subset G$ . The co-adjoint orbit  $X_{\lambda+\rho}$  is the full flag manifold. The  $T$ -fixed points are in the intersection  $X_{\lambda+\rho} \cap \mathfrak{t}$ , and hence, the set of the  $T$ -fixed points is the Weyl orbit of  $\lambda + \rho$

$$X_{\lambda+\rho}^T = \text{Weyl}(\lambda + \rho) \quad (2.10.6)$$

At each fixed point  $p \in X_{\lambda+\rho}^T$  the tangent space  $T_{X_{\lambda+\rho}}|_p$  is generated by the root system of  $\mathfrak{g}$ . The tangent space is a complex  $T$ -module  $\oplus_{\alpha>0} \mathbb{C}_\alpha$  with weights  $\alpha$  given by the positive roots of  $\mathfrak{g}$ . Consequently, the denominator of  $\hat{A}_T$  gives the Weyl denominator, the numerator

of  $\hat{A}_T$  cancels with the Euler class  $e_T(T_X)$  in the localization formula, and the restriction of  $\text{ch}_T(L) = e^\omega$  is  $e^{w(\lambda+\rho)}$

$$\frac{1}{(-2\pi i)^n} \int_{X_{\lambda+\rho}} \text{ch}_T(L) \hat{A}(T_X) = \sum_{w \in W} \frac{e^{iw(\lambda+\rho)\epsilon}}{\prod_{\alpha > 0} (e^{\frac{1}{2}i\alpha\epsilon} - e^{-\frac{1}{2}i\alpha\epsilon})} \quad (2.10.7)$$

We conclude that the localization of the equivariant index of the Dirac operator on  $X_{\lambda+\rho}$  twisted by the line bundle  $L$  to the set of fixed points  $X_{\lambda+\rho}^T$  is precisely the Weyl formula for the character.

The Kirillov correspondence between the index of the Dirac operator of  $L \rightarrow X_{\lambda+\rho}$  and the character is closely related to the Borel-Weil-Bott theorem.

Let  $B_{\mathbb{C}}$  be a Borel subgroup of  $G_{\mathbb{C}}$ ,  $T_{\mathbb{C}}$  be the maximal torus,  $\lambda$  an integral weight of  $T_{\mathbb{C}}$ . A weight  $\lambda$  defines a one-dimensional representation of  $B_{\mathbb{C}}$  by pulling back the representation on  $T_{\mathbb{C}} = B_{\mathbb{C}}/U_{\mathbb{C}}$  where  $U_{\mathbb{C}}$  is the unipotent radical of  $B_{\mathbb{C}}$  (the unipotent radical  $U_{\mathbb{C}}$  is generated by  $\mathfrak{g}_+$ ). Let  $L_{\lambda} \rightarrow G_{\mathbb{C}}/B_{\mathbb{C}}$  be the associated line bundle, and  $\mathcal{O}(L_{\lambda})$  be the sheaf of regular local sections of  $L_{\lambda}$ . For  $w \in \text{Weyl}_G$  define the action of  $w$  on a weight  $\lambda$  by  $w * \lambda := w(\lambda + \rho) - \rho$ .

The *Borel-Weil-Bott* theorem is that for any weight  $\lambda$  one has

$$H^{l(w)}(G_{\mathbb{C}}/B_{\mathbb{C}}, \mathcal{O}(L_{\lambda})) = \begin{cases} R_{\lambda}, & w * \lambda \text{ is dominant} \\ 0, & w * \lambda \text{ is not dominant} \end{cases} \quad (2.10.8)$$

where  $R_{\lambda}$  is the irreducible  $G$ -module with highest weight  $\lambda$ , the  $w$  is an element of Weyl group such that  $w * \lambda$  is dominant weight, and  $l(w)$  is the length of  $w$ . We remark that if there exists  $w \in \text{Weyl}_G$  such that  $w * \lambda$  is dominant weight, then  $w$  is unique. There is no  $w \in \text{Weyl}_G$  such that  $w * \lambda$  is dominant if in the basis of the fundamental weights  $\Lambda_i$  some of the coordinates of  $\lambda + \rho$  vanish.

### Example

For  $G = SU(2)$  the  $G_{\mathbb{C}}/B_{\mathbb{C}} = \mathbb{C}\mathbb{P}^1$ , an integral weight of  $T_{\mathbb{C}}$  is an integer  $n \in \mathbb{Z}$ , and the line bundle  $L_n$  is the  $\mathcal{O}(n)$  bundle over  $\mathbb{C}\mathbb{P}^1$ . The Weyl weight is  $\rho = 1$ .

The weight  $n \geq 0$  is dominant and the  $H^0(\mathbb{C}\mathbb{P}^1, \mathcal{O}(n))$  is the  $SL(2, \mathbb{C})$  module of highest weight  $n$  (in the basis of fundamental weights of  $SL(2)$ ).

For weight  $n = -1$  the  $H^i(\mathbb{C}\mathbb{P}^1, \mathcal{O}(-1))$  is empty for all  $i$  as there is no Weyl transformation  $w$  such that  $w * n$  is dominant (equivalently, because  $\rho + n = 0$ ).

For weight  $n \leq -2$  the  $w$  is the  $\mathbb{Z}_2$  reflection and  $w * n = -(n + 1) - 1 = -n - 2$  is dominant and  $H^1(\mathbb{C}\mathbb{P}^1, \mathcal{O}(n))$  is an irreducible  $SL(2, \mathbb{C})$  module of highest weight  $-n - 2$ .

The relation between Borel-Weil-Bott theorem for  $G_{\mathbb{C}}/B_{\mathbb{C}}$  and the Dirac complex on  $G_{\mathbb{C}}/B_{\mathbb{C}}$  is that Dirac operator is precisely the Dolbeault operator shifted by the square root of the canonical bundle

$$S^+(X) \ominus S^-(X) = K^{\frac{1}{2}} \sum (-1)^p \Omega^{0,p}(X) \quad (2.10.9)$$

and consequently

$$\text{ind}(X_{\lambda+\rho}, \not{D} \otimes L_{\lambda+\rho}) = \text{ind}(G_{\mathbb{C}}/B_{\mathbb{C}}, \bar{\partial} \otimes L_{\lambda}) \quad (2.10.10)$$

The Borel-Bott-Weyl theorem has a generalization for partial flag manifolds. Let  $P_{\mathbb{C}}$  be a parabolic subgroup of  $G_{\mathbb{C}}$  with  $B_{\mathbb{C}} \subset P_{\mathbb{C}}$  and let  $\pi : G_{\mathbb{C}}/B_{\mathbb{C}} \rightarrow G_{\mathbb{C}}/P_{\mathbb{C}}$  denote the canonical projection. Let  $E \rightarrow G_{\mathbb{C}}/P_{\mathbb{C}}$  be a vector bundle associated to an irreducible finite dimensional  $P_{\mathbb{C}}$  module, and let  $\mathcal{O}(E)$  be the sheaf of local regular sections of  $E$ . Then  $\mathcal{O}(E)$  is isomorphic to the direct image sheaf  $\pi_*\mathcal{O}(L)$  for a one-dimensional  $B_{\mathbb{C}}$ -module  $L$  and

$$H^k(G_{\mathbb{C}}/P_{\mathbb{C}}, \mathcal{O}(E)) = H^k(G_{\mathbb{C}}/B_{\mathbb{C}}, \mathcal{O}(L))$$

For application of Kirillov theory to Kac-Moody and Virasoro algebra see [24].

## 2.11 Equivariant index for differential operators

See the book by Atiyah [25].

Let  $E_k$  be vector bundles over a manifold  $X$ . Let  $G$  be a compact Lie group acting on  $X$  and the bundles  $E_k$ . The action of  $G$  on a bundle  $E$  induces canonically a linear action on the space of sections  $\Gamma(E)$ . For  $g \in G$  and a section  $\phi \in \Gamma(E)$  the action is

$$(g\phi)(x) = g\phi(g^{-1}x), \quad x \in X \quad (2.11.1)$$

Let  $D_k$  be linear differential operators compatible with the  $G$  action, and let  $\mathcal{E}$  be the complex (that is  $D_{k+1} \circ D_k = 0$ )

$$\mathcal{E} : \Gamma(E_0) \xrightarrow{D_0} \Gamma(E_1) \xrightarrow{D_1} \Gamma(E_2) \rightarrow \dots \quad (2.11.2)$$

Since  $D_k$  are  $G$ -equivariant operators, the  $G$ -action on  $\Gamma(E_k)$  induces the  $G$ -action on the cohomology  $H^k(\mathcal{E})$ . The equivariant index of the complex  $\mathcal{E}$  is the virtual character

$$\text{ind}_G(D) : \mathfrak{g} \rightarrow \mathbb{C} \quad (2.11.3)$$

defined by

$$\text{ind}_G(D)(g) = \sum_k (-1)^k \text{tr}_{H^k(\mathcal{E})} g \quad (2.11.4)$$

### 2.11.1 Atiyah-Singer equivariant index formula for elliptic complexes

If the set  $X^G$  of  $G$ -fixed points is discrete, the Atiyah-Singer equivariant index formula is

$$\boxed{\text{ind}_G(D) = \sum_{x \in X^G} \frac{\sum_k (-1)^k \text{ch}_G(E_k)|_x}{\det_{T_x X}(1 - g^{-1})}} \quad (2.11.5)$$

For the Dolbeault complex  $E_k = \Omega^{0,k}$  and  $D_k = \bar{\partial} : \Omega^{0,k} \rightarrow \Omega^{0,k+1}$

$$\rightarrow \Omega^{0,\bullet} \xrightarrow{\bar{\partial}} \Omega^{0,\bullet+1} \rightarrow \quad (2.11.6)$$

the index (2.11.5) agrees with (2.9.5) because the numerator in (2.11.5) decomposes as  $\text{ch}_G E \text{ch}_G \Lambda^\bullet T_{0,1}^*$  and the denominator as  $\text{ch}_G \Lambda^\bullet T_{0,1}^* \text{ch}_G \Lambda^\bullet T_{1,0}^*$  and the factor  $\text{ch}_G \Lambda^\bullet T_{0,1}^*$  cancels out.

For example, the equivariant index of  $\bar{\partial} : \Omega^{0,0}(X) \rightarrow \Omega^{0,1}(X)$  on  $X = \mathbb{C}_{\langle x \rangle}$  under the  $T = U(1)$  action  $x \mapsto t^{-1}x$  where  $t \in T$  is the fundamental character is contributed by the fixed point  $x = 0$  as

$$\text{ind}_T(\mathbb{C}, \bar{\partial}) = \frac{1 - \bar{t}}{(1-t)(1-\bar{t})} = \frac{1}{1-t} = \sum_{k=0}^{\infty} t^k \quad (2.11.7)$$

where the denominator is the determinant of the operator  $1 - t$  over the two-dimensional normal bundle to  $0 \in \mathbb{C}$  spanned by the vectors  $\partial_x$  and  $\partial_{\bar{x}}$  with eigenvalues  $t$  and  $\bar{t}$ . In the numerator, 1 comes from the equivariant Chern character on the fiber of the trivial line bundle at  $x = 0$  and  $-\bar{t}$  comes from the equivariant Chern character on the fiber of the bundle of  $(0, 1)$  forms  $d\bar{x}$ .

We can compare the expansion in power series in  $t^k$  of the index with the direct computation. The terms  $t^k$  for  $k \in \mathbb{Z}_{\geq 0}$  come from the local  $T$ -equivariant holomorphic functions  $x^k$  which span the kernel of  $\bar{\partial}$  on  $\mathbb{C}_{\langle x \rangle}$ . The cokernel is empty by the Poincaré lemma. Compare with (2.9.10).

Similarly, for the  $\bar{\partial}$  complex on  $\mathbb{C}^r$  we obtain

$$\text{ind}_T(\mathbb{C}^r, \bar{\partial}) = \left[ \prod_{k=1}^r \frac{1}{(1-t_k)} \right]_+ \quad (2.11.8)$$

where  $\llbracket \rrbracket_+$  means expansion in positive powers of  $t_k$ .

For application to the localization computation on spheres of even dimension  $S^{2r}$  we can compute the index of a certain transversally elliptic operator  $D$  which naturally interpolates between the  $\bar{\partial}$ -complex in the neighborhood of one fixed point (north pole) of the  $r$ -torus  $T^r$  action on  $S^{2r}$  and the  $\bar{\partial}$ -complex in the neighborhood of another fixed point (south pole). The index is a sum of two fixed point contributions

$$\begin{aligned} \text{ind}_T(S^{2r}, D) &= \left[ \prod_{k=1}^r \frac{1}{(1-t_k)} \right]_+ + \left[ \prod_{k=1}^r \frac{1}{(1-t_k)} \right]_- \\ &= \left[ \prod_{k=1}^r \frac{1}{(1-t_k)} \right]_+ + \left[ \prod_{k=1}^r \frac{(-1)^r t_1^{-1} \dots t_r^{-1}}{(1-t_k^{-1})} \right]_- \end{aligned} \quad (2.11.9)$$

where  $\llbracket \rrbracket_+$  and  $\llbracket \rrbracket_-$  denotes the expansions in positive and negative powers of  $t_k$ .

## 2.11.2 Atiyah-Singer index formula for a free action $G$ -manifold

Suppose that a compact Lie group  $G$  acts freely on a manifold  $X$  and let  $Y = X/G$  be the quotient, and let

$$\pi : X \rightarrow Y \quad (2.11.10)$$

be the associated  $G$ -principal bundle.

Suppose that  $D$  is a  $G \times T$  equivariant operator (differential) for a complex  $(\mathcal{E}, D)$  of vector bundles  $E_k$  over  $X$  as in (2.11.2). The  $G \times T$ -equivariance means that the complex  $\mathcal{E}$  and the operator  $D$  are pullbacks by  $\pi^*$  of a  $T$ -equivariant complex  $\tilde{\mathcal{E}}$  and operator  $\tilde{D}$  on the base  $Y$

$$\mathcal{E} = \pi^* \tilde{\mathcal{E}}, \quad D = \pi^* \tilde{D} \quad (2.11.11)$$

We want to compute the  $G \times T$ -equivariant index  $\text{ind}_{G \times T}(D; X)$  for the complex  $(\mathcal{E}, D)$  on the total space  $X$  for a  $G \times T$  transversally elliptic operator  $D$  using  $T$ -equivariant index theory on the base  $Y$ . We can do that using Fourier theory on  $G$  (counting KK modes in  $G$ -fibers).

Let  $R_G$  be the set of all irreducible representations of  $G$ . For each irreducible representation  $\alpha \in R_G$  we denote by  $\chi_\alpha$  the character of this representation, and by  $W_\alpha$  the vector bundle over  $Y$  associated to the principal  $G$ -bundle (2.11.10). Then, for each irrep  $\alpha \in R_G$  we consider a complex  $\tilde{\mathcal{E}} \otimes W_\alpha$  on  $Y$  obtained by tensoring  $\tilde{\mathcal{E}}$  with the vector bundle  $W_\alpha$  over  $Y$ . The Atiyah-Singer formula is

$$\text{ind}_{G \times T}(D; X) = \sum_{\alpha \in R_G} \text{ind}_T(\tilde{D} \otimes W_\alpha; Y) \chi_\alpha. \quad (2.11.12)$$

### Example of $S^{2r-1}$

We consider an example immediately relevant for localization on odd-dimensional spheres  $S^{2r-1}$  which are subject to the equivariant action of the maximal torus  $T^r$  of the isometry group  $SO(2r)$ . The sphere  $\pi : S^{2r-1} \rightarrow \mathbb{C}\mathbb{P}^{r-1}$  is the total space of the  $S^1$  Hopf fibration over the complex projective space  $\mathbb{C}\mathbb{P}^{r-1}$ .

We will apply the equation (2.11.12) for a transversally elliptic operator  $D$  induced from the Dolbeault operator  $\tilde{D} = \bar{\partial}$  on  $\mathbb{C}\mathbb{P}^{r-1}$  by the pullback  $\pi^*$ .

To compute the index of operator  $D = \pi^* \bar{\partial}$  on  $\pi : S^{2r-1} \rightarrow \mathbb{C}\mathbb{P}^{r-1}$  we apply (2.11.12) and use (2.9.20) and obtain

$$\text{ind}(D, S^{2r-1}) = \sum_{n=-\infty}^{\infty} \text{ind}_T(\bar{\partial}, \mathbb{C}\mathbb{P}^{r-1}, \mathcal{O}(n)) = \left[ \frac{1}{\prod_{k=1}^r (1 - t_k)} \right]_+ + \left[ \frac{(-1)^{r-1} t_1^{-1} \dots t_r^{-1}}{\prod_{k=1}^r (1 - t_k^{-1})} \right]_- \quad (2.11.13)$$

where  $[\ ]_+$  and  $[\ ]_-$  denotes the expansion in positive and negative powers of  $t_k$ . See further review in Chapter 1.

### 2.11.3 General Atiyah-Singer index formula

The Atiyah-Singer index formula for the Dolbeault and Dirac complexes and the equivariant index formula (2.11.5) can be generalized to a generic situation of an equivariant index of transversally elliptic complex (2.11.2).

Let  $X$  be a real manifold. Let  $\pi : T^*X \rightarrow X$  be the cotangent bundle. Let  $\{E^\bullet\}$  be an indexed set of vector bundles on  $X$  and  $\pi^* E^\bullet$  be the vector bundles over  $T^*X$  defined by the pullback.

The symbol  $\sigma(D)$  of a differential operator  $D : \Gamma(E) \rightarrow \Gamma(F)$  (2.11.2) is a linear operator  $\sigma(D) : \pi^*E \rightarrow \pi^*F$  which is defined by taking the highest degree part of the differential operator and replacing all derivatives  $\frac{\partial}{\partial x^\mu}$  by the conjugate coordinates  $p^\mu$  in the fibers of  $T^*X$ .

For example, for the Laplacian  $\Delta : \Omega^0(X, \mathbb{R}) \rightarrow \Omega^0(X, \mathbb{R})$  with highest degree part in some coordinate system  $\{x^\mu\}$  given by  $\Delta = g^{\mu\nu} \partial_\mu \partial_\nu$  where  $g^{\mu\nu}$  is the inverse Riemannian metric, the symbol of  $\Delta$  is a  $\text{Hom}(\mathbb{R}, \mathbb{R})$ -valued (i.e. number valued) function on  $T^*X$  given by

$$\sigma(\Delta) = g^{\mu\nu} p_\mu p_\nu \quad (2.11.14)$$

where  $p_\mu$  are conjugate coordinates (momenta) on the fibers of  $T^*X$ .

A differential operator  $D : \Gamma(E) \rightarrow \Gamma(F)$  is elliptic if its symbol  $\sigma(D) : \pi^*E \rightarrow \pi^*F$  is an isomorphism of vector bundles  $\pi^*E$  and  $\pi^*F$  on  $T^*X$  outside of the zero section  $X \subset T^*X$ .

The index of a differential operator  $D$  depends only on the topological class of its symbol in the topological K-theory of vector bundles on  $T^*X$ . The Atiyah-Singer formula for the index of the complex (2.11.2) is

$$\boxed{\text{ind}_G(D, X) = \frac{1}{(2\pi)^{\dim_{\mathbb{R}} X}} \int_{T^*X} \hat{A}_G(\pi^*T_X) \text{ch}_G(\pi^*E^\bullet)} \quad (2.11.15)$$

Here  $T^*X$  denotes the total space of the cotangent bundle of  $X$  with canonical orientation such that  $dx^1 \wedge dp_1 \wedge dx^2 \wedge dp_2 \dots$  is a positive element of  $\Lambda^{\text{top}}(T^*X)$ .

Let  $n = \dim_{\mathbb{R}} X$ . Let  $\pi^*T_X$  denote the vector bundle of dimension  $n$  over the total  $T^*X$  obtained as pullback of  $T_X \rightarrow X$  to  $T^*X$ . The  $\hat{A}_G$ -character of  $\pi^*T_X$  is

$$\hat{A}_G(\pi^*T_X) = \det_{\pi^*T_X} \left( \frac{R_G}{e^{R_G/2} - e^{-R_G/2}} \right) \quad (2.11.16)$$

where  $R_G$  denotes the  $G$ -equivariant curvature of the bundle  $\pi^*T_X$ . Notice that the argument of  $\hat{A}$  is  $n \times n$  matrix where  $n = \dim_{\mathbb{R}} T_X$  (real dimension of  $X$ ) while if general index formula is specialized to Dirac operator on Kahler manifold  $X$  as in (2.7.4) the argument of the  $\hat{A}$ -character is an  $n \times n$  matrix where  $n = \dim_{\mathbb{C}} T_X^{1,0}$  (complex dimension of  $X$ ).

Even though the integration domain  $T^*X$  is non-compact the integral (2.11.16) is well-defined because of the ( $G$ -transversal) ellipticity of the complex  $\pi^*E$ .

For illustration take the complex to be  $E_0 \xrightarrow{D} E_1$ . Since  $\sigma(D) : \pi^*E_0 \rightarrow \pi^*E_1$  is an isomorphism outside of the zero section we can pick a smooth connection on  $\pi^*E_0$  and  $\pi^*E_1$  such that its curvature on  $E_0$  is equal to the curvature on  $E_1$  away from a compact tubular neighborhood  $U_\epsilon X$  of  $X \subset T^*X$ . Then  $\text{ch}_G(\pi^*E^\bullet)$  is explicitly vanishing away from  $U_\epsilon X$  and the integration over  $T^*X$  reduces to integration over the compact domain  $U_\epsilon X$ .

It is clear that under localization to the fixed points of the  $G$ -action on  $X$  the general formula (2.11.16) reduces to the fixed point formula (2.11.5). This is due to the fact that the numerator in the  $\hat{A}$ -character  $\det_{\pi^*T_X} R_G = \text{Pf}_{T_X^*}(R_G)$  is the Euler class of the tangent bundle  $T_{T_X^*}$  to  $T^*X$  which cancels with the denominator in (2.8.9), while the restriction of the denominator of (2.11.16) to fixed points is equal to (2.11.16) or (2.11.5), because  $\det e^{R_G} = 1$ , since  $R_G$  is a curvature of the tangent bundle  $T_X$  with orthogonal structure group.

## 2.12 Equivariant cohomological field theories

Certain field theories first have been interpreted as cohomological and topological field theories by Witten, see [27], [28].

Often the path integral for supersymmetric field theories can be represented in the form

$$Z = \int_X \alpha \tag{2.12.1}$$

where  $X$  is the superspace (usually of infinite dimension) of all fields of the theory. Moreover, the integrand measure  $\alpha$  is closed with respect to an odd operator  $\delta$  which is typically constructed as a sum of a supersymmetry algebra generator and a BRST charge

$$\delta\alpha = 0 \tag{2.12.2}$$

The integrand is typically a product of an exponentiated action functional  $S$ , perhaps with insertion of a non-exponentiated observable  $\mathcal{O}$

$$\alpha = e^{-S} \mathcal{O} \tag{2.12.3}$$

so that both  $S$  and  $\mathcal{O}$  are  $\delta$ -closed

$$\delta S = 0, \quad \delta \mathcal{O} = 0. \tag{2.12.4}$$

If  $X$  is a supermanifold, such as a total space  $\Pi E$  of a vector bundle  $E$  (over a base  $Y$ ) with parity inversed fibers, the equivariant Euler characteristic class (Pfaffian) in the Atiyah-Bott formula (2.8.9) is replaced by the graded (super) version of the Pfaffian. The weights associated to fermionic components contribute inversely compared to the weights associated to bosonic components.

Typically, in quantum field theories the base  $Y$  of the bundle  $E \rightarrow Y$  is the space of fields. Certain differential equations (like BPS equations) are represented by a section  $s : Y \rightarrow E$ . The zero set of the section  $s^{-1}(0) \subset Y$  are the field configurations which solve the equations. For example, in topological self-dual Yang-Mills theory (Donaldson-Witten theory) the space  $Y$  is the infinite-dimensional affine space of all connections on a principal  $G$ -bundle on a smooth four-manifold  $M_4$ . In a given framing, connections are represented by adjoint-valued 1-forms on  $M_4$ , so  $Y \simeq \Omega^1(M_4) \otimes \text{ad } \mathfrak{g}$ . A fiber of the vector bundle  $E$  at a given connection  $A$  on the  $G$ -bundle on  $M_4$  is the space of adjoint-valued two-forms  $\Omega^{2+}(M_4) \otimes \text{ad } \mathfrak{g}$ . The section  $s : \Omega^1(M_4) \otimes \text{ad } \mathfrak{g} \rightarrow \Omega_2$  is represented by the self-dual part of the curvature form

$$A \mapsto F_A^+ \tag{2.12.5}$$

The zeroes of the section  $s = 0$  are connections  $A$  that are solutions of the equation  $F_A^+ = 0$ . The integrand  $\alpha$  is the Mathai-Quillen representative of the Thom class for the bundle  $E \rightarrow Y$  like in (2.6.10) and (2.6.17). The integral over the space of all fields  $X = \Pi E$  localizes to the integral over the zeroes  $s^{-1}(0)$  of the section, which in the Donaldson-Witten example is the moduli space of self-dual connections, called *instanton moduli space*.

The functional integral version of the localization formula of Atiyah-Bott has the same formal form

$$\boxed{\int_X \alpha = \int_F \frac{f^* \alpha}{e(\nu_F)}} \quad (2.12.6)$$

except that in the quantum field theory version the space  $X$  is an infinite-dimensional superspace of fields. The  $F$  denotes the localization locus in the space of fields. Let  $\Phi_F \in H^\bullet(X)$  be the Poincaré dual class to  $F$ , or Thom class of the inclusion  $f : F \hookrightarrow X$  which provides the isomorphism

$$f_* : H^\bullet(F) \rightarrow H^\bullet(X) \quad (2.12.7)$$

$$f_* : 1 \mapsto \Phi_F \quad (2.12.8)$$

Let  $\nu_F$  be the normal bundle to  $F$  in  $X$ . In quantum field theory language the space  $F$  is called the moduli space or localization locus, and  $\nu_F$  is the space of linearized fluctuations of fields transversal to the localization locus. The cohomology class of  $f^* \Phi_F$  in  $H^\bullet(F)$  is equal to the Euler class of the normal bundle  $\nu_F$

$$[f^* \Phi_F] = e(\nu_F) \quad (2.12.9)$$

The localization (2.8.9) from  $X$  to  $F$  exists whenever the locus  $F$  is such that there exists an inverse to the Euler class  $e(\nu_F)$  of its normal bundle in  $X$ . Two examples of such  $F$  have been considered above:

(i) if  $X = \Pi E$  is the total space of a vector bundle  $E \rightarrow Y$  with parity inversed fibers, then  $F \subset Y \subset X$  can be taken to be the set of zeroes  $F = s^{-1}(0)$  of a generic section  $s : Y \rightarrow E$

(ii) If  $X$  is a  $G$ -manifold for a compact group  $G$ , then  $F$  can be taken to be  $F = X^G$ , the set of  $G$ -fixed points on  $X$

The formula (2.12.6) is more general than these examples. In practice, in quantum field theory problems, the localization locus  $F$  is found by deforming the form  $\alpha$  to

$$\alpha_t = \alpha \exp(-t\delta V) \quad (2.12.10)$$

Here  $t \in \mathbb{R}$  is a deformation parameter, and  $V$  is a fermionic functional on the space of fields, such that  $\delta V$  has a trivial cohomology class (the cohomology class  $\delta V$  is automatically trivial on effectively compact spaces, but on a non-compact space of fields, which usually appears in quantum field theory path integrals, one has to take extra care of the contributions from the boundary at infinity to ensure that  $\delta V$  has trivial cohomology class).

If the even part of the functional  $\delta V$  is positive definite, then by sending the parameter  $t \rightarrow \infty$  we can see that the integral

$$\int_X \alpha \exp(-t\delta V) \quad (2.12.11)$$

localizes to the locus  $F \subset X$  where  $\delta V$  vanishes. Such locus  $F$  has an invertible Euler class of its normal bundle in  $X$  and the localization formula (2.12.6) holds.

In some quantum field theory problems, a compact Lie group  $G$  acts on  $X$  and  $\delta$  is isomorphic to an equivariant de Rham differential in the Cartan model of  $G$ -equivariant cohomology of  $X$ , so that an element  $\mathbf{a}$  of the Lie algebra of  $G$  appears as a parameter of the partition function  $Z$ .

Then the partition function  $Z(\mathbf{a})$  can be interpreted as an element of  $H_G^\bullet(pt)$ , and the Atiyah-Bott localization formula can be applied to compute  $Z(\mathbf{a})$ .

There are two types of equivariant partition functions.

In the partition functions of the first type  $Z(\mathbf{a})$ , the variable  $\mathbf{a}$  is a *parameter* of the quantum field theory such as a coupling constant, a background field, a choice of vacuum, an asymptotics of fields or a boundary condition. Such a partition function is typical for a quantum field theory on a non-compact space, such as the Nekrasov partition function of equivariant gauge theory on  $\mathbb{R}_{\epsilon_1, \epsilon_2}^4$  [29].

In the partition function of the second type, the variable  $\mathbf{a}$  is actually a *dynamical field* of the quantum field theory, so that the complete partition function is defined by integration of the partial partition function  $\tilde{Z}(\mathbf{a}) \in H_G^\bullet(pt)$

$$Z = \int_{\mathbf{a} \in \mathfrak{g}} \mu(\mathbf{a}) \tilde{Z}(\mathbf{a}) \tag{2.12.12}$$

where  $\mu(a)$  is a certain adjoint invariant volume form on the Lie algebra  $\mathfrak{g}$ . The partition function  $Z$  of second type is typical for quantum field theories on compact space-times reviewed in this volume, such as the partition function of a supersymmetric gauge theory on  $S^4$  [13] reviewed in Chapter 10, or on spheres of other dimensions, see summary of results in Chapter 1.

## Acknowledgements

The author is grateful to Bruno Le Floch for a careful proofreading and comments on this chapter. The author is supported by ERC QUASIFT grant.

## References

- [1] V. Pestun and M. Zabzine, eds., *Localization techniques in quantum field theory*, vol. xx. Journal of Physics A, 2016. 1608.02952. <https://arxiv.org/src/1608.02952/anc/LocQFT.pdf>, <http://pestun.ihep.fr/pages/LocalizationReview/LocQFT.pdf>.
- [2] H. Cartan, “Notions d’algèbre différentielle; application aux groupes de Lie et aux variétés où opère un groupe de Lie,” *Colloque de topologie (espaces fibrés), Bruxelles, 1950* (1951) 15–27.
- [3] H. Cartan, “La transgression dans un groupe de Lie et dans un espace fibré principal,” *Colloque de topologie (espaces fibrés), Bruxelles, 1950* (1951) 57–71.
- [4] V. W. Guillemin and S. Sternberg, *Supersymmetry and equivariant de Rham theory*. Mathematics Past and Present. Springer-Verlag, Berlin, 1999. <http://dx.doi.org/10.1007/978-3-662-03992-2>. With an appendix containing two reprints by Henri Cartan [ MR0042426 (13,107e); MR0042427 (13,107f)].

- [5] N. Berline, E. Getzler, and M. Vergne, *Heat kernels and Dirac operators*. Grundlehren Text Editions. Springer-Verlag, Berlin, 2004. Corrected reprint of the 1992 original.
- [6] R. J. Szabo, “Equivariant localization of path integrals,” [arXiv:hep-th/9608068 \[hep-th\]](#).
- [7] S. Cordes, G. W. Moore, and S. Ramgoolam, “Large N 2-D Yang-Mills theory and topological string theory,” *Commun. Math. Phys.* **185** (1997) 543–619, [hep-th/9402107](#).
- [8] M. Vergne, “Applications of Equivariant Cohomology,” [math/0607389](#).
- [9] J. Milnor, “Construction of universal bundles. I,” *Ann. of Math. (2)* **63** (1956) 272–284.
- [10] J. Milnor, “Construction of universal bundles. II,” *Ann. of Math. (2)* **63** (1956) 430–436.
- [11] H. Kanno, “Weyl Algebra Structure and Geometrical Meaning of BRST Transformation in Topological Quantum Field Theory,” *Z. Phys.* **C43** (1989) 477.
- [12] J. M. F. Labastida and M. Pernici, “A Gauge Invariant Action in Topological Quantum Field Theory,” *Phys. Lett.* **B212** (1988) 56.
- [13] V. Pestun, “Localization of gauge theory on a four-sphere and supersymmetric Wilson loops,” *Commun.Math.Phys.* **313** (2012) 71–129, [arXiv:0712.2824 \[hep-th\]](#).
- [14] R. Bott and L. W. Tu, *Equivariant characteristic classes in the Cartan model*. World Sci. Publ., River Edge, NJ, 2001.
- [15] N. Berline and M. Vergne, “The equivariant Chern character and index of  $G$ -invariant operators. Lectures at CIME, Venise 1992.”
- [16] R. Bott and L. W. Tu, *Differential forms in algebraic topology*, vol. 82 of *Graduate Texts in Mathematics*. Springer-Verlag, New York-Berlin, 1982.
- [17] V. Mathai and D. Quillen, “Superconnections, Thom classes, and equivariant differential forms,” *Topology* **25** (1986) no. 1, 85–110. [http://dx.doi.org/10.1016/0040-9383\(86\)90007-8](http://dx.doi.org/10.1016/0040-9383(86)90007-8).
- [18] M. F. Atiyah and L. Jeffrey, “Topological Lagrangians and cohomology,” *J. Geom. Phys.* **7** (1990) no. 1, 119–136.
- [19] S. Wu, “Mathai-Quillen formalism,” [arXiv:hep-th/0505003 \[hep-th\]](#).
- [20] M. F. Atiyah and R. Bott, “The moment map and equivariant cohomology,” *Topology* **23** (1984) no. 1, 1–28.
- [21] A. A. Kirillov, *Lectures on the orbit method*, vol. 64 of *Graduate Studies in Mathematics*. American Mathematical Society, Providence, RI, 2004. <http://dx.doi.org/10.1090/gsm/064>.
- [22] B. Kostant, “Quantization and unitary representations. I. Prequantization.”
- [23] A. A. Kirillov, “Merits and demerits of the orbit method,” *Bull. Amer. Math. Soc. (N.S.)* **36** (1999) no. 4, 433–488. <http://dx.doi.org/10.1090/S0273-0979-99-00849-6>.
- [24] A. Alekseev and S. L. Shatashvili, “Path Integral Quantization of the Coadjoint Orbits of the Virasoro Group and 2D Gravity,” *Nucl. Phys.* **B323** (1989) 719.
- [25] M. F. Atiyah, *Elliptic operators and compact groups*. Springer-Verlag, Berlin, 1974. Lecture Notes in Mathematics, Vol. 401.
- [26] V. Pestun and M. Zabzine, “Introduction to localization in quantum field theory,” *Journal of Physics A* **xx** (2016) 000, [1608.02953](#).
- [27] E. Witten, “Introduction to cohomological field theories,” *Int.J.Mod.Phys.* **A6** (1991) 2775–2792.
- [28] E. Witten, “Topological Quantum Field Theory,” *Commun.Math.Phys.* **117** (1988) 353.

- [29] N. A. Nekrasov, “Seiberg-Witten prepotential from instanton counting,” *Adv.Theor.Math.Phys.* **7** (2004) 831–864, [arXiv:hep-th/0206161 \[hep-th\]](#). To Arkady Vainshtein on his 60th anniversary.
- [30] K. Hosomichi, “ $\mathcal{N} = 2$  SUSY gauge theories on  $S^4$ ,” *Journal of Physics A* **xx** (2016) 000, [1608.02962](#).

# Chapter 3

## Supersymmetric localization in two dimensions

Francesco Benini<sup>1,2</sup> and Bruno Le Floch<sup>3</sup>

<sup>1</sup>*International School for Advanced Studies (SISSA), via Bonomea 265, 34136 Trieste, Italy*

<sup>2</sup>*Blackett Laboratory, Imperial College London, London SW7 2AZ, United Kingdom*

<sup>3</sup>*Princeton Center for Theoretical Science, Princeton University, Princeton, NJ 08544, USA*

fbenini@sissa.it, blefloch@princeton.edu

### Abstract

This is an introductory review to localization techniques in supersymmetric two-dimensional gauge theories. In particular we describe how to construct Lagrangians of  $\mathcal{N}=(2,2)$  theories on curved spaces, and how to compute their partition functions and certain correlators on the sphere, the hemisphere and other curved backgrounds. We also describe how to evaluate the partition function of  $\mathcal{N}=(0,2)$  theories on the torus, known as the elliptic genus. Finally we summarize some of the applications, in particular to probe mirror symmetry and other non-perturbative dualities.

### Contents

|            |                                                                  |           |
|------------|------------------------------------------------------------------|-----------|
| <b>3.1</b> | <b>Introduction</b>                                              | <b>71</b> |
| <b>3.2</b> | <b><math>\mathcal{N}=(2,2)</math> gauge theories on spheres</b>  | <b>74</b> |
| 3.2.1      | Multiplets, Lagrangians and supersymmetry                        | 75        |
| 3.2.2      | BPS equations                                                    | 77        |
| 3.2.3      | Coulomb branch localization                                      | 79        |
| 3.2.4      | The A-system                                                     | 82        |
| 3.2.5      | Higgs branch localization                                        | 84        |
| 3.2.6      | One-loop determinants                                            | 87        |
| <b>3.3</b> | <b>Other <math>\mathcal{N}=(2,2)</math> curved-space results</b> | <b>90</b> |

|            |                                                                                                                  |            |
|------------|------------------------------------------------------------------------------------------------------------------|------------|
| 3.3.1      | Local operator insertions . . . . .                                                                              | 90         |
| 3.3.2      | Twisted multiplets on the sphere . . . . .                                                                       | 92         |
| 3.3.3      | Localization on the hemisphere . . . . .                                                                         | 95         |
| 3.3.4      | $\Omega$ -deformed A-twist on the sphere . . . . .                                                               | 98         |
| 3.3.5      | General supersymmetric backgrounds . . . . .                                                                     | 100        |
| <b>3.4</b> | <b>Elliptic genera of <math>\mathcal{N}=(2, 2)</math> and <math>\mathcal{N}=(0, 2)</math> theories . . . . .</b> | <b>104</b> |
| 3.4.1      | Multiplets, Lagrangians and supersymmetry . . . . .                                                              | 107        |
| 3.4.2      | The localization formula and the JK residue . . . . .                                                            | 108        |
| 3.4.3      | The derivation . . . . .                                                                                         | 112        |
| 3.4.4      | Extensions and applications . . . . .                                                                            | 114        |
| <b>3.5</b> | <b>Dualities . . . . .</b>                                                                                       | <b>117</b> |
| 3.5.1      | Mirror symmetry . . . . .                                                                                        | 118        |
| 3.5.2      | Seiberg duality with unitary groups . . . . .                                                                    | 121        |
| 3.5.3      | Variants of Seiberg duality . . . . .                                                                            | 124        |
| 3.5.4      | $\mathcal{N}=(0, 2)$ trialities . . . . .                                                                        | 127        |
| <b>3.6</b> | <b>Conclusion . . . . .</b>                                                                                      | <b>129</b> |
|            | <b>References . . . . .</b>                                                                                      | <b>130</b> |

## 3.1 Introduction

Two-dimensional theories, despite the low dimensionality, are interesting for a number of reasons: they often appear in statistical physics and condensed matter physics; they share many properties with four-dimensional theories but are more tractable and yet quite non-trivial; they play a central role in string theory; they endow intricate mathematical problems and structures. Particularly tractable are supersymmetric theories, and we will be mostly concerned with 2d  $\mathcal{N}=(2, 2)$  and  $\mathcal{N}=(0, 2)$  supersymmetry. Those theories appear on the worldsheet of strings compactified down to four dimensions with  $\mathcal{N}=2$  or  $\mathcal{N}=1$  supersymmetry. They also exhibit dualities, which identify low-energy limits of pairs of theories, similar to 4d Seiberg duality [2]. Two-dimensional non-linear sigma models (NLSMs) with Kähler or Calabi-Yau target space, or bundles on such spaces, are related to mathematical problems such as mirror symmetry, Gromov-Witten invariants and quantum sheaf cohomology. Gauged linear sigma models (GLSMs), namely two-dimensional supersymmetric gauge theories, can provide convenient ultraviolet (UV) descriptions of NLSMs [3] thus proving to be extraordinary computational tools. Finally, GLSMs are also used as microscopic descriptions of surface operators in higher dimensions and as worldsheet theories for brane intersections (such as M-strings).

In this review we summarize recent results in supersymmetric localization techniques for two-dimensional theories, and applications to Calabi-Yau manifolds and dualities. The first half of the review concerns  $\mathcal{N}=(2, 2)$  theories on curved (compact) spaces: their construction and the computation of the corresponding Euclidean path-integral—that we will generically call a “partition function”. Curved-space Lagrangians can be obtained by coupling the supersymmetric theory to supergravity, and then switching on background values for the

metric and the other bosonic fields in the graviton multiplet [4] (also Chapter 5). While the flat space  $\mathcal{N}=(2,2)$  supersymmetry algebra admits both a vector and an axial  $U(1)$  R-symmetry, a mixed anomaly prevents them from being simultaneously gauged: the curved space background must break one, giving rise to A-type and B-type backgrounds, respectively. Supersymmetric supergravity backgrounds on compact orientable Riemann surfaces and preserving the vector R-symmetry were classified in [6].<sup>1</sup> With the topology of the sphere, one finds the well-known A- (and  $\bar{A}$ -) twist [8] with  $\pm 1$  units of R-symmetry flux, as well as an “ $\Omega$ -deformation” thereof [9, 10] (see subsection 3.3.4)—but also “untwisted” backgrounds [11–13] (see section 3.2 and subsection 3.3.2) with zero net R-symmetry flux, analogous to the seminal setup of Pestun on  $S^4$  [14]. The genus  $g = 1$  case includes flat tori (see section 3.4). For all these cases, we show how partition functions can be computed. For  $g > 1$ , the only solution is the A-twist and we will not discuss it further.

To begin with, in section 3.2 we follow [11–13] and perform supersymmetric localization for  $\mathcal{N}=(2,2)$  chiral and vector multiplets on squashed-sphere untwisted backgrounds preserving the vector R-symmetry  $R$ . Since continuous deformations of the coefficients in kinetic and superpotential terms in the action do not affect the path-integral (as those terms are  $\mathcal{Q}$ -exact with respect to a supercharge  $\mathcal{Q}$ ), the partition function is independent of gauge couplings and wave-function renormalization and it is thus a renormalization group (RG) invariant. It is a non-trivial non-perturbative function of R-charges and twisted chiral parameters: twisted masses and flavor fluxes (background field strengths coupled to flavor symmetries) as well as Fayet-Iliopoulos (FI) parameters and theta angles (appearing in the twisted superpotential).

To showcase the supersymmetric localization method, we go through this relatively tractable case in detail. The path integral localizes to fixed-points of  $\mathcal{Q}$  (see subsection 3.2.2) and quadratic fluctuations around these. Their contribution (see subsection 3.2.6) is found by adding to the action a  $\mathcal{Q}$ -exact and  $\mathcal{Q}$ -closed deformation term  $t\delta_{\mathcal{Q}}V$ : the limit  $t \rightarrow \infty$  localizes the path integral further to saddle-points of  $\delta_{\mathcal{Q}}V$ . It turns out that using two different deformation terms one can get different-looking expressions (3.2.17) and (3.2.40). The first one (see subsection 3.2.3), called *Coulomb branch formula*, is a sum over gauge fluxes and an integral over a Coulomb branch parameter of the theory, which converges for generic FI/theta parameters. We show in subsection 3.2.4 that it obeys a system of differential equations called the A-system. The second one (see subsection 3.2.5), called *Higgs branch formula*, is an expansion in some corner of the FI/theta moduli space: it involves a sum over solutions (dubbed Higgs branches) of the D-term equations, with non-perturbative contributions from point-like (anti-)vortices at the (South) North pole.  $\mathcal{Q}$ -invariant operators can also be included in both expressions (see subsection 3.3.1).

The two forms are useful in different settings. Higgs branch expressions are used to confirm Seiberg-like dualities, as discussed in subsection 3.5.2. For instance,  $U(K)$  and  $U(N - K)$  gauge theories with  $N$  fundamental chiral multiplets are expected to have the same low-energy limit. Their sphere partition functions are shown to be equal by mapping the  $\binom{N}{K}$  solutions of D-term equations of one theory to the  $\binom{N}{N-K}$  solutions for the other, and equating (anti-)vortex contributions order by order in the number of vortices. More

---

<sup>1</sup>A more general classification was provided in [7].

complicated variants of this duality can also be checked using Higgs branch expressions (see [subsection 3.5.3](#)).

On the other hand, Coulomb branch expressions are useful to characterize “phases” of GLSMs. Let us consider briefly a famous example: a  $U(1)$  vector multiplet and chiral multiplets  $P, X_1, \dots, X_5$  of charges  $(-5, +1, \dots, +1)$  with a superpotential  $W = P G_5(X)$  for some homogeneous degree 5 polynomial  $G_5$ . For FI parameter  $\zeta \gg 0$  this GLSM flows to an NLSM on the quintic hypersurface  $\{G_5(X) = 0\} \subset \mathbb{CP}^4$ , while for  $\zeta \ll 0$  the GLSM flows to an orbifolded Landau-Ginzburg model with a single classical vacuum. The distinction between these two phases can be seen in the sphere partition function: the Coulomb branch integral can be expanded as a sum of residues of poles to one side or the other of the integration contour depending on whether  $2\pi\zeta \lesseqgtr 5 \log 5$  (see [\[15, 16\]](#) for more general discussions).

We also use the Coulomb branch integral as our starting point when investigating mirror symmetry in [subsection 3.5.1](#). As explained in [Chapter 4](#), metric deformations of the NLSM’s target Calabi-Yau decompose into complex structure deformations and Kähler structure deformations, which correspond respectively to superpotential and twisted superpotential terms in the GLSM action. The partition function  $Z_A$  preserving  $R$  gives the Kähler potential  $K_K = -\log Z_A$  on the moduli space of Kähler structure deformations [\[13, 18–20\]](#). Important enumerative geometry data of the Calabi-Yau manifold, namely its genus-zero Gromov-Witten invariants, can then be extracted from the  $\zeta \gg 0$  expansion of  $Z_A$ . The Kähler potential on the moduli space of complex structure deformations is similarly  $K_C = -\log Z_B$  in terms of the partition function  $Z_B$  of the GLSM on a supergravity background that preserves the axial R-symmetry [\[21\]](#). We compute  $Z_B$  in [subsection 3.3.2](#). Mirror symmetry states that pairs of Calabi-Yau manifolds have identical moduli spaces, with complex structure and Kähler structure deformations interchanged. Accordingly, we describe in [subsection 3.5.1](#) how  $Z_A$  of a GLSM is equal to  $Z_B$  of a GLSM flowing to an NLSM on the mirror Calabi-Yau.

Another important case where localization was performed is the hemisphere [\[22–24\]](#) (see [subsection 3.3.3](#)), which is the simplest case of a manifold with boundaries. GLSMs on the hemisphere can be used to describe open strings with Calabi-Yau target space: boundary conditions for fields on the hemisphere are branes in the target. The hemisphere partition function has an integral and a series representations, like the sphere partition function  $Z_A$  (although the contour is difficult to work out in general). We do not discuss the real projective plane calculation of [\[25\]](#), which gives information about orientifold planes in the Calabi-Yau target.

As is well-known, Kähler potentials are only defined up to Kähler transformations  $K \rightarrow K + f(z) + \overline{f(\overline{z})}$  where  $z$  is a holomorphic coordinate on the given Kähler manifold (here a moduli space of metric deformations of a Calabi-Yau). This translates to a multiplicative ambiguity of sphere partition functions, which can be traced to a freedom in choosing how FI parameters (promoted to twisted chiral multiplets) couple to background supergravity [\[6, 13, 19\]](#). Derivatives  $\partial\overline{\partial} \log Z$  of the Kähler potential remain unambiguous. An analysis of supergravity counterterms [\[20\]](#) shows that there is no such universal content for general  $\mathcal{N}=(0, 2)$  theories on the sphere. In order to find physical observables, one needs to compute correlators. For some  $\mathcal{N}=(0, 2)$  deformations of  $\mathcal{N}=(2, 2)$  GLSMs, placed on the sphere using the  $A/2$ -twist,

correlators were computed using supersymmetric localization in [26].

The review is organized as follows. In [section 3.2](#) we calculate the (squashed) sphere partition function of  $\mathcal{N}=(2,2)$  GLSMs using the two different localization approaches. In [section 3.3](#) we extend the results in various ways: we discuss the inclusion of operators, twisted chiral and twisted vector multiplets, the hemisphere, the  $\Omega$ -deformed A-twist, ending with a general discussion of  $\mathcal{N}=(2,2)$  supersymmetry on curved spaces. In [section 3.4](#) we turn to a second major localization result in two dimensions: the (equivariant) elliptic genus of  $\mathcal{N}=(2,2)$  and  $\mathcal{N}=(0,2)$  theories, namely their partition function on a flat torus. Contrarily to the sphere, the torus has non-trivial cycles and we include flat background connections. The elliptic genus is an important probe of supersymmetry breaking and is one of the rare RG invariant quantities available to test dualities between  $\mathcal{N}=(0,2)$  theories. After defining the elliptic genus and its modularity properties, we describe  $\mathcal{N}=(0,2)$  multiplets and Lagrangians in [subsection 3.4.1](#), then give the localization formula (3.4.28) in [subsection 3.4.2](#) followed by an outline of the derivation in [subsection 3.4.3](#), and we end with several extensions and applications in [subsection 3.4.4](#). In [section 3.5](#) we highlight some applications of the sphere and torus partition functions. We begin with a check of Abelian mirror symmetry in [subsection 3.5.1](#). Then we check that Seiberg-dual  $\mathcal{N}=(2,2)$  theories have equal sphere partition functions and equal elliptic genera in [subsection 3.5.2](#) before turning to generalizations in [subsection 3.5.3](#). We compare elliptic genera for the  $\mathcal{N}=(0,2)$  triality in [subsection 3.5.4](#). We conclude in [section 3.6](#) with a brief discussion of topics that were not included in the review.

## 3.2 $\mathcal{N}=(2,2)$ gauge theories on spheres

This section is devoted to partition functions of  $\mathcal{N}=(2,2)$  Euclidean gauge theories on the round [11, 12] and squashed [13] sphere. The aims are to show localization at work and to obtain two exact expressions, (3.2.17) and (3.2.40), for the  $S^2$  partition function.

In terms of the standard flat superspace [3], the basic  $\mathcal{N}=(2,2)$  multiplets are: chiral superfields defined by  $\bar{D}_\pm \Phi = 0$ ; vector superfields with gauge transformation  $V \cong V + \Lambda + \bar{\Lambda}$  for  $\Lambda$  chiral; twisted chiral superfields defined by  $\bar{D}_+ \tilde{\Phi} = D_- \tilde{\Phi} = 0$ ; twisted vector superfields with gauge transformation  $\tilde{V} \cong \tilde{V} + \Lambda_t + \bar{\Lambda}_t$  for  $\Lambda_t$  twisted chiral. The field-strength multiplets  $\Sigma = \bar{D}_+ D_- V$  and  $\tilde{\Sigma} = \bar{D}_+ \bar{D}_- \tilde{V}$  are twisted chiral and chiral, respectively. Twisted and untwisted multiplets are interchanged by a  $\mathbb{Z}_2$  automorphism of the  $\mathcal{N}=(2,2)$  superalgebra, that also exchanges the vector  $U(1)_R$  and axial  $U(1)_A$  R-symmetries. One can write down kinetic terms for the basic multiplets,

$$\int d^2\theta d^2\bar{\theta} (\bar{\Phi}\Phi + \tilde{\bar{\Phi}}\tilde{\Phi}),$$

including (twisted) chirals and field strengths. Besides, one can write superpotential interactions terms (top component of a composite chiral field  $W$ ) and twisted superpotential terms (top component of a composite twisted chiral field  $\tilde{W}$ ).

We focus in this section on gauged linear sigma models built from vector and chiral multiplets. The components of chiral multiplets (a complex scalar  $\phi$ , a complex Dirac spinor

$\psi$  and a complex auxiliary scalar  $F$ ) transform in some representation  $\mathfrak{R}$  of a gauge and flavor symmetry group  $G \times G_f$ , their conjugates  $(\bar{\phi}, \bar{\psi}, \bar{F})$  transform in  $\bar{\mathfrak{R}}$ , while the vector multiplet components (a real gauge field  $A_i$ , real scalars  $\eta, \sigma$ , complex Dirac fermions  $\lambda, \bar{\lambda}$  and a real auxiliary scalar  $D$ ) transform in the adjoint representation of  $G$ .

In [subsection 3.2.1](#) we place these GLSMs on the sphere in a way that preserves  $U(1)_R$ , describe how supersymmetries act and write supersymmetric Lagrangians. Other  $\mathcal{N}=(2,2)$  theories and backgrounds are considered in [section 3.3](#). We choose a localization supercharge  $\mathcal{Q}$  whose square rotates the sphere around its poles. In [subsection 3.2.2](#) we find that  $\mathcal{Q}$ -invariant field configurations are generically parametrized by a discrete gauge flux  $\mathfrak{m}$  through  $S^2$  and a vector multiplet scalar  $\sigma$ . When chiral multiplets are not charged under  $U(1)_R$ , we note the existence of additional vortex and antivortex configurations near the poles for particular values of  $\sigma$  named Higgs-branch roots. In [subsection 3.2.3](#) we localize using a deformation term that eliminates (anti)vortices and expresses the partition function as a sum over fluxes and an integral over the Coulomb branch parameter  $\sigma$  of one-loop determinants computed later. The partition function obeys a system of differential equations [15], shown in [subsection 3.2.4](#), that are (anti)holomorphic in certain combinations of Fayet-Iliopoulos (FI) parameters and theta angles. It must thus be a sum of products of a holomorphic solution and an antiholomorphic solution. We reproduce the factorization for a large class of GLSMs in [subsection 3.2.5](#) (in the absence of R-charges) by a different choice of deformation term which interpolates between the Coulomb branch integral and a sum over Higgs branches. Each term in this sum factorizes into (anti)holomorphic vortex partition functions due to (anti)vortices at the (South) North pole. These can be obtained explicitly by expressing the Coulomb branch integral as a sum of residues. We end in [subsection 3.2.6](#) by outlining how one-loop determinants for fluctuations around saddle points are computed, correcting a sign in the process.

### 3.2.1 Multiplets, Lagrangians and supersymmetry

We now place vector and chiral multiplets and their Lagrangians on squashed spheres which preserve a  $U(1) \subset SU(2)$  isometry of  $S^2$ . The metric, vielbein, and spin connection are<sup>2</sup>

$$ds^2 = \delta_{ab} e^a e^b, \quad e^1 = f(\theta) d\theta, \quad e^2 = r \sin(\theta) d\varphi, \quad \omega = \frac{r \cos \theta}{f(\theta)} d\varphi, \quad (3.2.1)$$

where  $\varphi$  is  $2\pi$ -periodic,  $0 \leq \theta \leq \pi$ , and  $f(0) = f(\pi) = r$  to avoid conical singularities at the North ( $\theta = 0$ ) and South ( $\theta = \pi$ ) poles. The full covariant derivative is  $D_i = \nabla_i - iA_i$  in terms of the metric-covariant derivative  $\nabla_i$  and (dynamical and background) gauge fields  $A_i$ . Using the vielbein,  $D_1 = f(\theta)^{-1} D_\theta$  and  $D_2 = (r \sin(\theta))^{-1} D_\varphi$ .

The metric is conformally flat, hence the generators of superconformal transformations are those of flat space. Among those, supercharges which square to isometries of the sphere generate the Poincaré superalgebra  $\mathfrak{su}(2|1)$  for the round sphere  $f(\theta) = r$ , and  $\mathfrak{su}(1|1)$  in

<sup>2</sup>This metric assumes that lengths of meridian circles are monotonic from the equator to each pole. Final results will only involve the equatorial radius  $r$ .

general. Explicitly, we will use a supercharge  $\mathcal{Q} \in \mathfrak{su}(1|1)$  whose square is  $\mathcal{Q}^2 = J + R/2$ , where  $J$  is the  $U(1)$  rotation and  $R$  is a  $U(1)$  vector R-symmetry.

Thanks to conformal flatness, the action of superconformal transformations (and  $\mathcal{Q}$  in particular) on vector and chiral multiplets is known. It is conveniently written in terms of conformal Killing spinors  $\epsilon$ , namely solutions of  $\nabla_i \epsilon = \gamma_i \tilde{\epsilon}$  for some  $\tilde{\epsilon}$ . Unfortunately the conformal map between the squashed sphere and the plane is quite unwieldy, thus the resulting conformal Killing spinors are complicated. Another approach, which works for non-conformally-flat spaces in higher dimensions [27, 28], is to keep spinors simple by introducing an R-symmetry background gauge field  $V_i$ . For definiteness we choose<sup>3</sup>

$$\epsilon = e^{i\theta\gamma_1/2} e^{i\varphi/2} \epsilon_0, \quad \bar{\epsilon} = e^{i\theta\gamma_1/2} e^{-i\varphi/2} \bar{\epsilon}_0, \quad \text{with } \gamma_3 \epsilon_0 = \epsilon_0 \text{ and } \gamma_3 \bar{\epsilon}_0 = -\bar{\epsilon}_0 \quad (3.2.2)$$

and the normalization  $\bar{\epsilon}\epsilon = \bar{\epsilon}_0\epsilon_0 = 1$ . These spinors span the space of solutions to  $\nabla_i \epsilon = i\gamma_i \epsilon/2r$  on the round sphere. On squashed spheres they are solutions to the R-covariant conformal Killing spinor equation

$$D_i \epsilon = (\nabla_i - iV_i)\epsilon = \frac{i\gamma_i \epsilon}{2f(\theta)} \quad D_i \bar{\epsilon} = (\nabla_i + iV_i)\bar{\epsilon} = \frac{i\gamma_i \bar{\epsilon}}{2f(\theta)} \quad (3.2.3)$$

with a connection  $V = \frac{1}{2}\left(1 - \frac{r}{f(\theta)}\right) d\varphi$  smooth everywhere. Note that supersymmetry transformations of vector and chiral multiplets must likewise be made covariant by including  $V$  in every covariant derivative, with the R-charge of each field as its coefficient.

Let us now write the supersymmetry variations  $\delta_{\mathcal{Q}}$  of vector and chiral multiplet components under the supercharge  $\mathcal{Q}$  built from  $\epsilon, \bar{\epsilon}$ . We only list the supersymmetry transformations of fermions (we have also shifted the auxiliary field  $D$  by  $\sigma/r$ ), and refer to [6, 11, 12, 21] for the complete expressions:

$$\begin{aligned} \delta_{\mathcal{Q}} \lambda &= (iV_m^+ \gamma^m - D)\epsilon & \text{where} & & V_i^\pm &= \mp D_i \sigma + \varepsilon_{ij} D^j \eta \\ \delta_{\mathcal{Q}} \bar{\lambda} &= (iV_m^- \gamma^m + D)\bar{\epsilon} & & & V_3^\pm &= F_{12} \pm i[\sigma, \eta] - \eta/f(\theta) \end{aligned} \quad (3.2.4)$$

$$\begin{aligned} \delta_{\mathcal{Q}} \psi &= \left( i\gamma^i D_i \phi + i\sigma \phi + \gamma_3 \eta \phi - q\phi/(2f(\theta)) \right) \epsilon + \bar{\epsilon} F \\ \delta_{\mathcal{Q}} \bar{\psi} &= \left( i\gamma^i D_i \bar{\phi} + i\bar{\phi} \sigma - \gamma_3 \bar{\phi} \eta - q\bar{\phi}/(2f(\theta)) \right) \bar{\epsilon} + \epsilon \bar{F}. \end{aligned} \quad (3.2.5)$$

The implicit summations on the first and second line are over  $m = 1, 2, 3$ .

The most general renormalizable action with  $\mathcal{N}=(2, 2)$  supersymmetry involving only vector and chiral multiplets takes the form

$$S = S_{\text{v.m.}} + S_{\tilde{W}} + S_{\text{c.m.}} + S_W. \quad (3.2.6)$$

The vector multiplet action  $S_{\text{v.m.}}$ , the chiral multiplet action  $S_{\text{c.m.}}$  and the superpotential term  $S_W$  are dimensional reductions of their 4d  $\mathcal{N}=1$  counterparts, with corrections of order  $1/r$  and  $1/r^2$  to preserve supersymmetry on the squashed sphere.

<sup>3</sup>Our conventions for spinor components of chiral and vector multiplets and our choice of Killing spinors follow [11] for consistency with the rest of the review. They differ from [12, 13] by factors of  $e^{i\pi(1-\gamma^3)/4}$ . Note that  $e^{i\pi(1-\gamma^3)/4} \gamma^i e^{-i\pi(1-\gamma^3)/4} = \varepsilon^{ij} \gamma_j$ . Moreover the contraction of spinor indices is  $\psi\chi = \psi_\alpha \varepsilon^{\alpha\beta} \chi_\beta$ , namely the symbol  $\psi\chi$  stands for  $\psi^T \begin{pmatrix} 0 & 1 \\ -1 & 0 \end{pmatrix} \chi$  in standard matrix notation.

The twisted superpotential term  $S_{\tilde{W}}$  is analogous to the superpotential term  $S_W$ : a (twisted) superpotential is the top component of a polynomial in (twisted) chiral multiplets. In theories of vector and chiral multiplets the only twisted chiral multiplet available is the field strength  $\Sigma$  of the vector multiplet, and the most commonly used twisted superpotential in a gauge theory is linear in  $\Sigma$ . The twisted superpotential term  $S_{\tilde{W}}$  is then—for each  $U(1)$  gauge group—the familiar FI D-term and a topological term measuring the gauge field flux  $\mathbf{m}$  through  $S^2$ . The coefficients  $\zeta$  (FI parameter) and  $\vartheta$  (theta angle) combine into a complexified FI parameter  $z = e^{-2\pi\zeta + i\vartheta}$ .

Finally, one can endow chiral multiplets with twisted masses by coupling the flavor symmetry group to an external (non-dynamical) vector multiplet and giving it a supersymmetric background value. We solve the BPS equations in (3.2.14) and find that the background is parametrized by a real scalar  $\tau$  and a discrete flux  $\mathbf{n}$ . The action  $S_{\text{c.m.}}$  and the supersymmetry transformations (3.2.5) of a chiral multiplet then depend on its R-charge  $q$ , its twisted mass  $\tau$  and the flux  $\mathbf{n}$ .

Except for the twisted superpotential term  $S_{\tilde{W}}$ , all terms in the action (3.2.6) are  $\mathcal{Q}$ -exact and  $\mathcal{Q}$ -invariant. Explicitly, the corresponding Lagrangian densities are

$$\begin{aligned}\mathcal{L}_{\text{v.m.}} &= \delta_{\mathcal{Q}}\delta_{\bar{\epsilon}} \text{Tr}\left(\bar{\lambda}\lambda/2 - 2\sigma D + \sigma^2/f(\theta)\right) \\ \mathcal{L}_{\text{c.m.}} &= \delta_{\mathcal{Q}}\delta_{\bar{\epsilon}}\left(\bar{\psi}\psi - 2i\bar{\phi}\sigma\phi + (q-1)\bar{\phi}\phi/f(\theta)\right) \\ \mathcal{L}_W &= \delta_{\mathcal{Q}}\left(\psi_{(W)}\epsilon + \bar{\epsilon}\bar{\psi}_{(\bar{W})}\right).\end{aligned}\tag{3.2.7}$$

Therefore, any  $\mathcal{Q}$ -invariant observable is independent of the coefficients in  $S_{\text{v.m.}}$ ,  $S_{\text{c.m.}}$  and  $S_W$ , and can only depend on parameters in the twisted superpotential (FI parameters, theta angles) and in supersymmetry transformations (R-charges, twisted masses, background fluxes). In particular, these observables are independent of the gauge couplings  $g_{\text{YM}}$  hence are invariant under the RG flow, which makes them very powerful probes of the low-energy limit of GLSMs.

### 3.2.2 BPS equations

The localization argument guarantees that only  $\mathcal{Q}$ -invariant field configurations (and quadratic fluctuations nearby) contribute to  $\mathcal{Q}$ -invariant path integrals. The variations  $\delta_{\mathcal{Q}}$  of bosons involve fermionic fields hence vanish automatically and we are left with solving  $\delta_{\mathcal{Q}}\lambda = \delta_{\mathcal{Q}}\bar{\lambda} = 0$  and  $\delta_{\mathcal{Q}}\psi = \delta_{\mathcal{Q}}\bar{\psi} = 0$  for the spinors  $\epsilon, \bar{\epsilon}$  defining  $\mathcal{Q}$ .

The vanishing of gluino variations (3.2.4) implies

$$iV_3^{\pm} \mp V_1^{\pm} \sin\theta = D \cos\theta \quad \text{and} \quad iV_2^{\pm} \pm V_1^{\pm} \cos\theta = D \sin\theta.\tag{3.2.8}$$

The integration contour is fixed by convergence of the path integral: the bosons  $A_i, \eta, \sigma$ , and  $D$  in vector multiplets are real, thus  $V_m^{\pm}$  are real as well. In one of the localization calculations we will replace  $D$  by its complex on-shell value, thus we now keep  $D$  general when solving the BPS equations. Extracting the real and imaginary parts of (3.2.8) yields

$V_1^\pm = \text{Re } D = 0$ ,  $V_2^\pm = \sin \theta \text{ Im } D$  and  $V_3^\pm = \cos \theta \text{ Im } D$ . Therefore, the BPS equations read

$$0 = D_2 \eta = D_1 \sigma = D_2 \sigma = [\eta, \sigma] \quad (3.2.9)$$

$$D_1 \eta = -\sin \theta \text{ Im } D \quad \text{and} \quad F_{12} - \frac{\eta}{f(\theta)} = \cos \theta \text{ Im } D. \quad (3.2.10)$$

Fixing the gauge  $A_\theta = 0$ , equations (3.2.10) imply  $\partial_\theta(A_\varphi + r\eta \cos \theta) = 0$ . Solving in either region  $0 \leq \theta < \pi$  or  $0 < \theta \leq \pi$  one gets  $A = (k - r \cos \theta \eta) d\varphi$  where  $k$  is fixed by continuity at the pole to be  $k^+ = r\eta(0)$  and  $k^- = -r\eta(\pi)$ , respectively. The two  $A$  are gauge equivalent away from the poles provided the flux  $\mathbf{m} = \frac{1}{2\pi} \int F = r\eta(0) + r\eta(\pi) = k^+ - k^-$  is GNO quantized [29] namely has integer eigenvalues on any representation of  $G$ . The remaining equations imply that the constant  $\sigma$  commutes with all  $\eta(\theta, \varphi)$  and that

$$\partial_\varphi \eta = i[k^\pm, \eta] \quad (3.2.11)$$

with a constant  $k^\pm$  depending on the gauge. Periodicity in  $\varphi$  requires  $\eta$  to lie in integer eigenspaces of  $k^\pm$  (in the adjoint representation), which coincide due to GNO quantization of  $k^+ - k^-$ .

We now turn to the BPS equations of the chiral multiplet. Linear combinations of  $\delta_{\mathcal{Q}}\psi = 0$  and the complex conjugate of  $\delta_{\mathcal{Q}}\bar{\psi} = 0$  yield  $0 = F = \sigma\phi$  and

$$0 = \cos \frac{\theta}{2} (D_1 + iD_2)\phi - \sin \frac{\theta}{2} \left( \eta + \frac{q}{2f(\theta)} \right) \phi = \sin \frac{\theta}{2} (D_1 - iD_2)\phi - \cos \frac{\theta}{2} \left( \eta - \frac{q}{2f(\theta)} \right) \phi. \quad (3.2.12)$$

Taking into account  $A = (k^\pm - r \cos \theta \eta) d\varphi$  from above, the equations imply

$$0 = F = \sigma\phi = \left( \sin \theta \partial_\theta - f(\theta)\eta + \frac{q}{2} \cos \theta \right) \phi = \left( \partial_\varphi - ik^\pm + \frac{iq}{2f(\theta)/r} \right) \phi. \quad (3.2.13)$$

Periodicity in  $\varphi$  requires  $\phi$  to lie in the integer eigenspaces of  $k^\pm - iqr/2f(\theta)$  for all  $\theta$ , but this is only possible if  $q = 0$  (or if the sphere is round). At the poles, (3.2.12) imply additionally to first order in  $\theta$  that  $\phi$  is (anti)holomorphic at the (South) North pole.

In subsection 3.2.3 we will keep  $D$  real and assume that all R-charges are positive (and the sphere is squashed), so that  $\phi = 0$ . Since  $\text{Im } D = 0$  we now have  $\partial_\theta \eta = 0$  hence  $\eta$  is equal to its value at the poles and is constant. Altogether,

$$f(\theta) F_{12} = \eta = \frac{\mathbf{m}}{2r}, \quad \sigma = \text{constant}, \quad 0 = [\eta, \sigma] = D = \phi = F. \quad (3.2.14)$$

The path integral localizes to these ‘‘Coulomb branch’’ configurations, so named in analogy to the Coulomb branch of the flat space theory. Since  $\eta$  and  $\sigma$  commute, a constant gauge transformation reduces them to the Cartan algebra  $\mathfrak{t}$  of  $G$ . Another outcome of this computation concerns non-dynamical vector multiplets: one can turn on a flux  $\mathbf{m}^{\text{ext}} = \mathbf{n}$  and a real twisted mass  $\sigma^{\text{ext}} = \tau$  for each chiral multiplet, as announced in subsection 3.2.1.

In subsection 3.2.5 we will assume that all R-charges vanish and alter the contour of integration of  $D$  (equivalently we evaluate its Gaussian path integral) to localize onto complex saddle points of the deformation term chosen there. Namely,

$$D = -i(\phi\bar{\phi} - \chi) \quad (3.2.15)$$

where we will choose a “deformation” FI parameter  $\chi$  for each  $U(1)$  gauge factor. Besides Coulomb branch configurations similar to (3.2.14) with  $\phi = 0$ , there are now Higgs branch (and mixed branch) configurations with  $\phi \neq 0$ . Writing a twisted mass  $\tau_I$  for each chiral multiplet  $\phi_I$  explicitly, the constraint  $(\sigma + \tau_I)\phi_I = 0$  only allows non-zero  $\phi$  at particular points on the Coulomb branch. For generic twisted masses at most rank  $G$  different chiral multiplets can be non-zero. Due to (3.2.13),  $\phi(\theta, \varphi) \sim (e^{i\varphi} \sin \theta)^{k^\pm} \phi_0$  near the poles, hence regular non-zero solutions  $\phi$  must additionally lie in the non-negative integer eigenspaces of  $k^\pm$ . The remaining BPS equations

$$\partial_\theta \eta = f(\theta) \sin \theta (\phi\bar{\phi} - \chi), \quad \sin \theta \partial_\theta \phi = f(\theta) \eta \phi \quad (3.2.16)$$

have not been analysed in full generality. For  $G = U(N)$  with (anti)fundamental matter and generic twisted masses we will find that all contributions to the localized path integral are suppressed as  $\chi \rightarrow \infty$  except those in which the group is fully Higgsed. The condition is that the non-vanishing chiral multiplets span  $\mathbb{C}^N$ : then  $(\sigma + \tau_I)\phi_I = 0$  fixes  $\sigma$ , and more importantly all eigenvalues of  $k^\pm$  must be non-negative integers. While in the Coulomb branch localization scheme only the difference  $k^+ - k^-$  was GNO quantized, in the Higgs branch localization scheme  $\chi \rightarrow \infty$  both  $k^+$  and  $k^-$  are quantized (and non-negative). We will interpret  $k^\pm$  as counting vortices at the North pole and antivortices at the South pole.

### 3.2.3 Coulomb branch localization

In this section we assume for simplicity that all R-charges are in the range  $0 < q < 2$ . In all models of interest this condition can be made to hold by mixing the R-charge with  $U(1)$  gauge charges if needed. Other values for the R-charges can be reached by analytic continuation.

Recall the localization argument: we add a  $\mathcal{Q}$ -invariant deformation term  $t\delta_{\mathcal{Q}}\mathcal{V}$  to the action and take  $t \rightarrow \infty$  thus making the saddle-point approximation exact. Any  $\mathcal{Q}$ -invariant observable then reduces to an integral over saddle points of its classical value at these saddles, with a measure given by a Gaussian integral (one-loop determinant) of quadratic fluctuations around the saddles. Additionally, saddle points that are not  $\mathcal{Q}$ -invariant cannot contribute since the Grassmann integral of a constant vanishes. This second argument would not be necessary if we used the canonical deformation term  $\delta_{\mathcal{Q}}(\lambda \overline{\delta_{\mathcal{Q}}\lambda} + \psi \overline{\delta_{\mathcal{Q}}\psi})$  since the saddle points of its bosonic part are precisely  $\mathcal{Q}$ -invariant configurations. However, we use the  $\mathcal{Q}$ -closed and  $\mathcal{Q}$ -exact deformation term  $S_{\text{v.m.}} + S_{\text{c.m.}}$  in (3.2.7). It is straightforward to check that all  $\mathcal{Q}$ -invariant configurations (3.2.14) are saddle points.

The (squashed) sphere partition function of a 2d  $\mathcal{N}=(2, 2)$  GLSM with gauge group  $G$  and chiral multiplets in the representation  $\mathfrak{R} = \bigoplus_I \mathfrak{R}_I$  (each with an R-charge  $q_I$ , a background flux  $\mathbf{n}_I$ , and a twisted mass  $\tau_I$ ) is then a sum over GNO-quantized fluxes ( $\mathbf{m}$  has integer

eigenvalues on any representation of  $G$ ) and an integral over the Cartan algebra  $\mathfrak{t}$  of  $G$  of classical and one-loop factors

$$Z_{S^2} = \frac{r^{c/3}}{|\text{Weyl}(G)|} \sum_{\mathfrak{m}} \int_{\mathfrak{t}} \frac{d(r\sigma)}{(2\pi)^{\text{rank } G}} Z_{\text{cl}}(z, \bar{z}; r\sigma, \mathfrak{m}) Z_{\text{gauge}}(r\sigma, \mathfrak{m}) Z_{\text{matter}}(q, r\sigma + r\tau, \mathfrak{m} + \mathfrak{n}) . \quad (3.2.17)$$

The order  $|\text{Weyl}(G)|$  of the Weyl group appears due to residual discrete gauge redundancy in  $\mathfrak{t}$ . The result only depends on the squashed sphere through its equatorial radius  $r$ . We explain in [subsection 3.2.6](#) how to compute vector multiplet and chiral multiplet one-loop determinants: they are products over positive roots  $\alpha$  of  $G$  and over weights  $\rho$  of each representation  $\mathfrak{R}_I$ ,

$$\begin{aligned} Z_{\text{gauge}} &= \prod_{\alpha > 0} (-1)^{\alpha(\mathfrak{m})} \left[ r^2 \alpha(\sigma)^2 + \frac{\alpha(\mathfrak{m})^2}{4} \right] \\ Z_{\text{matter}} &= \prod_{I, \rho} \frac{\Gamma\left(\frac{q_I}{2} - ir\tau_I - \frac{n_I}{2} - ir\rho(\sigma) - \frac{\rho(\mathfrak{m})}{2}\right)}{\Gamma\left(1 - \frac{q_I}{2} + ir\tau_I - \frac{n_I}{2} + ir\rho(\sigma) - \frac{\rho(\mathfrak{m})}{2}\right)} . \end{aligned} \quad (3.2.18)$$

For the common case of a linear twisted superpotential  $\widetilde{W}$  with an FI parameter  $\zeta_\ell$  and a theta term  $\vartheta_\ell$  for each  $U(1)$  gauge factor, the classical contribution is

$$Z_{\text{cl}} = \prod_{\ell} z_{\ell}^{\text{Tr}_{\ell}(ir\sigma + \frac{\mathfrak{m}}{2})} \bar{z}_{\ell}^{\text{Tr}_{\ell}(ir\sigma - \frac{\mathfrak{m}}{2})} \quad (3.2.19)$$

where  $z_{\ell} = e^{-2\pi\zeta_{\ell} + i\vartheta_{\ell}}$  and we denote  $\text{Tr}_{\ell}$  the projection onto the  $\ell$ -th  $U(1)$  factor: for  $G = \prod_{\ell} U(N_{\ell})$  these really are traces. To be more precise, (3.2.19) involves renormalized FI parameters at the scale  $1/r$ ,

$$z_{\ell} = (rM_{\text{UV}})^{\sum_I Q_I^{\ell}} z_{\ell}^{\text{UV}} , \quad (3.2.20)$$

where  $z^{\text{UV}}$  are bare parameters at some UV scale  $M_{\text{UV}}$  and  $Q_I^{\ell}$  are charges of chiral multiplets under the  $\ell$ -th  $U(1)$  factor. We obtain this dependence on  $r$  from zeta function regularization when computing one-loop determinant in [subsection 3.2.6](#), and also obtain the overall power  $r^{c/3}$ ,

$$\frac{c}{3} = \sum_I (1 - q_I) \dim \mathfrak{R}_I - \dim G . \quad (3.2.21)$$

For theories that flow to a superconformal field theory (SCFT),  $c$  is the central charge. The equatorial radius  $r$  is also used as a scale for twisted masses and  $\sigma$ .

Several comments are in order. The partition function only depends on parameters in the twisted superpotential (here  $z, \bar{z}$ ), on R-charges, twisted masses and background fluxes. This is expected since the coupling constants  $g_{\text{YM}}$  and superpotential couplings multiply  $\mathcal{Q}$ -exact terms. In particular any superpotential simply specializes  $Z_{S^2}$  by fixing some linear combinations of the R-charges to 2. The partition function depends holomorphically on the combinations  $\frac{q_I}{2} - ir\tau_I$  hence it can be extended to R-charges beyond  $0 < q < 2$ .

Another extension is to include  $\mathcal{Q}$ -invariant operators in the path integral, such as  $\text{Tr}_{\ell}(i\sigma + \eta)$  at the North pole or  $\text{Tr}_{\ell}(i\sigma - \eta)$  at the South pole: this is achieved by including

| Groups with $(-1)^{2\delta(\mathbf{m})} = 1$                                   | Groups with $(-1)^{2\delta(\mathbf{m})}$ a discrete theta angle  |
|--------------------------------------------------------------------------------|------------------------------------------------------------------|
| $SU(MN)/\mathbb{Z}_M$ with $M$ odd or $N$ even                                 | $SU(MN)/\mathbb{Z}_M$ with $M$ even and $N$ odd                  |
| $SO(2N)$                                                                       | $SO(2N+1)$                                                       |
| $SO(8N)/\mathbb{Z}_2, SO(8N+2)/\mathbb{Z}_2$                                   | $SO(8N+4)/\mathbb{Z}_2, SO(8N+6)/\mathbb{Z}_2$                   |
| $Sp(4N)/\mathbb{Z}_2, Sp(4N+3)/\mathbb{Z}_2, E_6/\mathbb{Z}_3$                 | $Sp(4N+1)/\mathbb{Z}_2, Sp(4N+2)/\mathbb{Z}_2, E_7/\mathbb{Z}_2$ |
| Simply-connected groups: $SU(N),$<br>$Spin(N), Sp(N), E_6, E_7, E_8, F_4, G_2$ | Quotients $Spin(4N)/\mathbb{Z}_2$ other than $SO(4N)$            |

Table 3.1: Effect of the vector multiplet one-loop determinant sign  $(-1)^{2\delta(\mathbf{m})}$  for connected compact simple groups. It is trivial when the Weyl vector  $\delta$  is a weight, and otherwise corresponds to a  $\mathbb{Z}_2$  discrete theta angle. For  $U(N)$  the sign shifts the (continuous) theta angle by  $\pi$  if  $N$  is even.

their on-shell values  $\text{Tr}_\ell(i\sigma \pm \frac{\mathbf{m}}{2r})$  in the integrand (3.2.17), and will be further discussed in subsection 3.3.1. These insertions can be realized by taking derivatives with respect to  $\log z_\ell$  and  $\log \bar{z}_\ell$ , respectively. This is a manifestation of the fact that the integrand in (3.2.17) factorizes as a function of  $z$  and  $i\sigma + \frac{\mathbf{m}}{2r}$  times a function of  $\bar{z}$  and  $i\sigma - \frac{\mathbf{m}}{2r}$ . This factorization will play an important role later.

Note that the sign

$$\prod_{\alpha>0} (-1)^{\alpha(\mathbf{m})} = e^{2\pi i \delta(\mathbf{m})}, \quad (3.2.22)$$

which we will derive later, was originally missed. It was correctly predicted in [24, 30, 31]. For many groups this sign is +1 because the Weyl vector  $\delta$  (half sum of positive roots) is a weight of  $G$ . An important exception is  $U(N)$  with  $N$  even: then the sign is equivalent to a shift of the theta angle by  $\pi$ . Table 3.1 gives a list for simple groups.

We expect the one-loop determinants of two chiral multiplets  $X$  and  $Y$  with opposite gauge and flavor charges and with R-charges  $q$  and  $2-q$  to cancel. Indeed, such chiral multiplets can be integrated out by including a superpotential mass term  $W = \mu XY$  with  $\mu \rightarrow \infty$ , and  $W$  does not affect the partition function. Omitting external sources here for brevity,

$$\prod_{\rho} \frac{\Gamma\left(\frac{q}{2} - ir\rho(\sigma) - \frac{\rho(\mathbf{m})}{2}\right)}{\Gamma\left(1 - \frac{q}{2} + ir\rho(\sigma) - \frac{\rho(\mathbf{m})}{2}\right)} \frac{\Gamma\left(1 - \frac{q}{2} + ir\rho(\sigma) + \frac{\rho(\mathbf{m})}{2}\right)}{\Gamma\left(\frac{q}{2} - ir\rho(\sigma) + \frac{\rho(\mathbf{m})}{2}\right)} = \prod_{\rho} (-1)^{\rho(\mathbf{m})}. \quad (3.2.23)$$

We have used  $\Gamma(x + \mathbf{m}/2)/\Gamma(1 - x + \mathbf{m}/2) = (-1)^{\mathbf{m}}\Gamma(x - \mathbf{m}/2)/\Gamma(1 - x - \mathbf{m}/2)$  which is a consequence of Euler's identity  $\Gamma(y)\Gamma(1-y) = \pi/\sin \pi y$ . Since weights sum to zero for simple factors of  $G$ , the sign simply shifts theta angles of some  $U(1)$  gauge factors by  $\pi$ .

The one-loop determinant of a vector multiplet can be recast as that of a collections of chiral multiplets of R-charge  $q = 2$  and gauge charges equal to the roots  $\alpha$  of  $G$ . This can be understood in terms of the Higgs mechanism. If the theory had an extra chiral multiplet of R-charge 0 in the adjoint representation, we could give a VEV to its diagonal components without breaking the R-symmetry. The VEV would break the gauge group to its maximal

torus  $U(1)^{\text{rank } G}$ , and give a mass both to vector and chiral multiplet components along the roots  $\alpha$ . Taking into account the observation above, we have schematically the relations:  $Z_{\text{gauge}} = 1/\prod_{\alpha} Z_{\text{chiral}}^{(\alpha), q=0} = \prod_{\alpha} Z_{\text{chiral}}^{(\alpha), q=2}$ . This fact implies that  $Z_{S^2}$  of a non-Abelian GLSM is the specialization of  $Z_{S^2}$  of an associated ‘‘Cartan theory’’ which has gauge group  $U(1)^{\text{rank } G}$ , has rank  $G$  parameters  $z_{\ell}$ , and has one chiral multiplet for each weight  $w$  of  $\mathfrak{R}$  and one for each root  $\alpha$  of  $G$ . The original partition function is retrieved by setting  $z_{\ell} = 1$  for each FI parameter that does not correspond to a  $U(1)$  factor of the original theory.

### 3.2.4 The A-system

Remarkably, the partition function (3.2.17) obeys a system of differential equations that are holomorphic in the  $z_{\ell}$  and a similar system for  $\bar{z}_{\ell}$ . We first review the results of [15], which apply to abelian GLSMs and to non-abelian GLSMs through their associated Cartan theory. Set  $r = 1$  for brevity. Consider a GLSM with abelian gauge group  $G = U(1)^N$  and chiral multiplets of charges  $Q_I^{\ell}$  under the  $\ell$ -th gauge group factor. Its partition function is

$$Z_{S^2} = \sum_{\mathbf{m} \in \mathbb{Z}^N} \int_{\mathbb{R}^N} \frac{d^N \sigma}{(2\pi)^N} \prod_{\ell=1}^N \left[ z_{\ell}^{i\sigma_{\ell} + \frac{\mathbf{m}_{\ell}}{2}} \bar{z}_{\ell}^{i\sigma_{\ell} - \frac{\mathbf{m}_{\ell}}{2}} \right] \prod_I \left[ \frac{\Gamma\left(\frac{q_I}{2} - i\tau_I - \frac{\mathbf{n}_I}{2} - Q_I^{\ell}(i\sigma_{\ell} + \frac{\mathbf{m}_{\ell}}{2})\right)}{\Gamma\left(1 - \frac{q_I}{2} + i\tau_I - \frac{\mathbf{n}_I}{2} + Q_I^{\ell}(i\sigma_{\ell} - \frac{\mathbf{m}_{\ell}}{2})\right)} \right] \quad (3.2.24)$$

with an implicit summation over  $\ell$ . If we shift the summation on  $\mathbf{m}$  by any  $\mathbf{u} \in \mathbb{Z}^N$  and the contour for each  $\sigma_{\ell}$  by  $-iu_{\ell}/2$  (the contour encounters no pole), then the classical action is multiplied by  $z_{\ell}^{\mathbf{u}_{\ell}}$  and the arguments of gamma functions are shifted by  $-Q_I^{\ell} \mathbf{u}_{\ell}$  in the numerator. Extracting these shifts from the gamma function arguments yields some factors linear in  $i\sigma_{\ell} + \mathbf{m}_{\ell}/2$  which can be reproduced by acting on  $Z_{S^2}$  with the holomorphic differential operators  $z_{\ell} \partial / \partial z_{\ell}$ . We find that for any  $\mathbf{u} \in \mathbb{Z}^N$ ,

$$\begin{aligned} & \prod_{I, Q_I^{\ell} \mathbf{u}_{\ell} > 0} \left( \frac{q_I}{2} - i\tau_I - \frac{\mathbf{n}_I}{2} - Q_I^{\ell} \frac{\partial}{\partial \log z_{\ell}} \right)_{Q_I^{\ell} \mathbf{u}_{\ell}} Z_{S^2} \\ &= \left( \prod_{\ell=1}^N z_{\ell}^{\mathbf{u}_{\ell}} \right) \prod_{I, Q_I^{\ell} \mathbf{u}_{\ell} < 0} \left( \frac{q_I}{2} - i\tau_I - \frac{\mathbf{n}_I}{2} - Q_I^{\ell} \frac{\partial}{\partial \log z_{\ell}} \right)_{-Q_I^{\ell} \mathbf{u}_{\ell}} Z_{S^2} \end{aligned} \quad (3.2.25)$$

in terms of Pochhammer symbols  $(x)_n = \prod_{i=0}^{n-1} (x+i) = \Gamma(x+n)/\Gamma(x)$ . The same system with  $z_{\ell} \rightarrow (-1)^{\sum_I Q_I^{\ell}} \bar{z}_{\ell}$  and  $\mathbf{n} \rightarrow -\mathbf{n}$  holds.

This ‘‘A-system’’ of equations—a slight generalization of the GKZ (Gel’fand, Kapranov, Zelevinski) A-hypergeometric systems—is highly redundant: the equation for  $\mathbf{u} + \mathbf{u}'$  is a consequence of those for  $\mathbf{u}$  and  $\mathbf{u}'$ , at least if  $Q_I^{\ell} \mathbf{u}_{\ell}$  and  $Q_I^{\ell} \mathbf{u}'_{\ell}$  have the same sign for all  $I$ . The space of holomorphic solutions to (3.2.25) is typically finite-dimensional, so  $Z_{S^2}$  is a linear combination of holomorphic times antiholomorphic solutions:

$$Z_{S^2} = \sum_k C_k \mathcal{F}_k(z) \tilde{\mathcal{F}}_k(\bar{z}). \quad (3.2.26)$$

For GLSMs that flow in the infrared to NLSMs on Calabi-Yau manifolds, the differential equations are the well-known Picard-Fuchs differential equations and the functions  $\mathcal{F}_k$  are periods of the mirror Calabi-Yau.

For non-Abelian examples it turns out that many solutions to the associated Cartan theory's A-system are absent from explicit factorizations of  $Z_{S^2}$  into (3.2.26). This suggests the existence of more stringent differential equations whose set of solutions would capture exactly the (anti)holomorphic dependence of  $Z_{S^2}$ . Let us focus for concreteness on SQCD, namely  $G = U(N)$  with  $N_f$  fundamental and  $N_f$  antifundamental chiral multiplets. We replace the single FI parameter  $z$  by  $z_\ell$ ,  $1 \leq \ell \leq N$  as in the associated Cartan theory, but we write the vector multiplet one-loop determinant as a differential operator rather than as a chiral multiplet determinant. Concretely:

$$Z_{S^2}^{\text{SQCD}}(z, \bar{z}) = \frac{1}{N!} \left[ \prod_{k < j}^N \left( iz_k \frac{\partial}{\partial z_k} - iz_j \frac{\partial}{\partial z_j} \right) \left( i\bar{z}_k \frac{\partial}{\partial \bar{z}_k} - i\bar{z}_j \frac{\partial}{\partial \bar{z}_j} \right) \prod_{\ell=1}^N Z_{S^2}^{N=1}(z_\ell, \bar{z}_\ell) \right]_{\substack{z_\ell = (-1)^{N-1} z \\ \bar{z}_\ell = (-1)^{N-1} \bar{z}}} . \quad (3.2.27)$$

The sign  $(-1)^{N-1}$  comes from  $(-1)^{\alpha(m)}$  in the vector multiplet one-loop determinant (see Table 3.1). The partition function  $Z_{S^2}^{N=1}$  of SQED (an Abelian theory) obeys the A-system, which reduces in this case to a single equation ( $\mathbf{u} = 1$ ):

$$\left[ \prod_{I=1}^{N_f} \left( \frac{q_I}{2} - i\tau_I - \frac{\mathbf{n}_I}{2} - \frac{\partial}{\partial \log z_\ell} \right) - z_\ell \prod_{I=1}^{N_f} \left( \frac{q_I}{2} - i\tau_I - \frac{\mathbf{n}_I}{2} + \frac{\partial}{\partial \log z_\ell} \right) \right] Z_{S^2}^{N=1} = 0 . \quad (3.2.28)$$

The space of holomorphic solutions to this  $N_f^{\text{th}}$  order differential equation is spanned by  $N_f$  functions  $\mathcal{F}_I(z)$  for  $I = 1, \dots, N_f$ . The antiholomorphic counterpart  $z \rightarrow \bar{z}$  also holds, so in an appropriate basis  $Z_{S^2}^{N=1}(z, \bar{z}) = \sum_I C_I \mathcal{F}_I(z) \mathcal{F}_I(\bar{z})$ . Expand each SQED partition function  $Z_{S^2}^{N=1}$  in (3.2.27) as such a sum, so as to get  $(N_f)^N$  factorized terms in total. Note that the holomorphic differential operator in (3.2.27) is antisymmetric in the  $z_k$ , hence only  $\binom{N_f}{N}$  terms remain.<sup>4</sup>

We now show that these  $\binom{N_f}{N}$  terms are solutions of an ordinary differential equation of order  $\binom{N_f}{N}$  in  $z\partial/\partial z$ , rather than a system of differential equations in  $z_\ell\partial/\partial z_\ell$ . By expanding the differential operator in (3.2.27) into a sum of monomials which are products of derivatives acting on individual factors  $Z_{S^2}^{N=1}(z_j, \bar{z}_j)$ , then setting  $z_j = (-1)^{N-1}z$  and  $\bar{z}_j = (-1)^{N-1}\bar{z}$  as indicated in (3.2.27), one writes the SQCD partition function as (3.2.29) below, for  $p_j = j$ . Consider more generally

$$F_p(z, \bar{z}) = \varepsilon_{\ell_1 \dots \ell_N} \prod_{j=1}^N \left[ \left( iz \frac{\partial}{\partial z} \right)^{p_j-1} \left( i\bar{z} \frac{\partial}{\partial \bar{z}} \right)^{\ell_j-1} Z_{S^2}^{N=1}(z, \bar{z}) \right] \quad (3.2.29)$$

for integers  $p_j \geq 1$ . Reordering the  $p_j$  only affects signs, and  $F_p$  vanishes if any  $p_i = p_j$ . The  $iz\partial/\partial z$  derivative of  $F_p$  is a sum of  $N$  such functions (each with one  $p_j \rightarrow p_j + 1$ ). On the

<sup>4</sup>For  $N_f < N$ , localization gives a vanishing result for  $Z_{S^2}$ : this is due to supersymmetry breaking.

other hand, the GKZ equation (3.2.28) for  $Z_{S^2}^{N=1}(z, \bar{z})$  expresses its  $N_f$ <sup>th</sup> derivative as a linear combination of its lower derivatives. Thus  $F_p$  with any  $p_j > N_f$  can be written as a sum of terms with lower  $p$ . All derivatives of  $Z_{S^2}^{\text{SQCD}} = F_{1,2,\dots,N}$  are hence linear combinations (with known holomorphic coefficients) of the  $\binom{N_f}{N}$  functions  $F_p$  for which all  $1 \leq p_j \leq N_f$ . This establishes the existence of a holomorphic differential equation of order  $\binom{N_f}{N}$  obeyed by the SQCD partition function (coefficients can be made polynomial in  $z$ ).

This proof extends to quiver gauge theories, and gives bounds on the number of terms needed in the factorization of  $Z_{S^2}$  that are stronger than those deduced from the GKZ system of the associated Cartan theory. On the other hand the proof is not constructive; no closed form expression for the differential equation is known at present.

### 3.2.5 Higgs branch localization

As we have just seen, the sphere partition function of a GLSM can be factorized into holomorphic times antiholomorphic functions of its complexified FI parameters. We now interpret the factors physically as being due to vortices at the poles, by localizing the path integral directly into this form. After this ‘‘Higgs branch’’ localization was found for 2d  $\mathcal{N}=(2,2)$  theories [11, 12], it was used to explain a similar factorization in 3d  $\mathcal{N}=2$  theories [32, 33] and 4d  $\mathcal{N}=1$  theories [34, 35].

Because the Coulomb branch result (3.2.17) is analytic in  $\frac{q_I}{2} - ir\tau_I$ , we can work with  $q_I = 0$ . We also ignore fluxes for external vector multiplets for simplicity, and set  $r = 1$ . Of course, we assume that the theory has  $U(1)$  gauge factors as otherwise the factorization property is vacuously true.

We localize using in addition to  $\mathcal{L}_{\text{v.m.}} + \mathcal{L}_{\text{c.m.}}$  the deformation term [11]

$$\mathcal{L}_{\text{Higgs}} = \delta_{\mathcal{Q}} \text{Tr} \left[ -i(\phi\bar{\phi} - \chi)\delta_{\mathcal{Q}}\sigma \right]. \quad (3.2.30)$$

For each  $U(1)$  gauge factor, it includes a parameter  $\chi$  which will play the role of an FI parameter. The trace denotes the natural pairing between  $\bar{\phi}$  and  $(\delta_{\mathcal{Q}}\sigma)\phi$  on the one hand, and the projection onto each  $U(1)$  gauge factor with coefficients  $\chi$  on the other hand. The bosonic part of this deformation term includes  $iD(\phi\bar{\phi} - \chi)$ , and leads to the on-shell value  $D = -i(\phi\bar{\phi} - \chi)$  up to unimportant coefficients. After integrating out  $D$ , saddle points of the deformation term are exactly the  $\mathcal{Q}$ -invariant configurations analyzed in subsection 3.2.2:

$$\eta(\theta, \varphi) = e^{i\varphi[k^{\pm}, \cdot]} \eta(\theta, 0), \quad \phi(\theta, \varphi) = e^{i\varphi k^{\pm}} \phi(\theta, 0), \quad (3.2.31)$$

$$\partial_{\theta}\eta = f(\theta) \sin \theta (\phi\bar{\phi} - \chi), \quad \sin \theta \partial_{\theta}\phi = f(\theta) \eta\phi, \quad (3.2.32)$$

where  $k^+ = \eta(0)$  is used in the simply-connected region  $0 \leq \theta < \pi$  while  $k^- = -\eta(\pi)$  in the region  $0 < \theta \leq \pi$ . The remaining fields are a constant  $\sigma$  which commutes with all  $\eta(\theta, \varphi)$  and such that  $(\sigma + \tau_I)\phi_I = 0$  for all flavors  $I$ , and  $A = (k^{\pm} - \cos \theta \eta) d\varphi$  whose flux  $\mathfrak{m} = k^+ - k^-$  is GNO quantized. We have also seen that any non-zero  $\phi$  lies among non-negative integer eigenspaces of  $k^{\pm}$ . Since  $(\sigma, k^{\pm})$  commute pairwise, a constant gauge transformation diagonalizes them.

The partition function localizes to an integral over all solutions to these equations, and one should compute one-loop determinants. One technique described in [subsection 3.2.6](#) to compute one-loop determinants involves localization to fixed points of  $\mathcal{Q}^2$ , namely the poles. One-loop determinants are then a product of contributions from each pole that only depend on values of the  $\mathcal{Q}$ -invariant field configuration at those points. The one-loop determinants (3.2.18) computed in the Coulomb branch factorize as functions of  $i\sigma \pm \frac{\mathbf{m}}{2}$ , which we associated to the North and South poles by considering correlators of the  $\mathcal{Q}$ -invariant operators  $i\sigma \pm \eta$  in [subsection 3.2.3](#). We deduce that the one-loop determinant is, more generally,

$$Z_{1\text{-loop}} = \prod_{\alpha > 0} (-1)^{\alpha(\mathbf{m})} \alpha(i\sigma + \eta(0)) \alpha(i\sigma - \eta(\pi)) \prod_{I,w} \frac{\Gamma(-i\tau_I - w(i\sigma + \eta(0)))}{\Gamma(1 + i\tau_I + w(i\sigma - \eta(\pi)))}. \quad (3.2.33)$$

Both  $k^+ \mp k^- = \eta(0) \pm \eta(\pi)$  are integrals over the squashed sphere. One is the flux:

$$\eta(0) + \eta(\pi) = \frac{1}{2\pi} \int_0^\pi d\theta \int_0^{2\pi} d\varphi \partial_\theta(-\eta \cos \theta) = \frac{1}{2\pi} \int F = \mathbf{m} \quad (3.2.34)$$

and fluxes through each hemisphere are  $k^+ = \eta(0)$  and  $-k^- = \eta(\pi)$ . The other is the integral of the  $D$ -term equation with the volume form:

$$\eta(0) - \eta(\pi) = \int_0^\pi d\theta (-\partial_\theta \eta) = \frac{1}{2\pi} \int (\chi - \phi\bar{\phi}) d\text{vol}_2 \equiv \Delta. \quad (3.2.35)$$

For a fixed flux  $\mathbf{m}$ , each ratio of Gamma functions in (3.2.33) has the asymptotics

$$\left| \frac{\Gamma(-i\tau_I - w(i\sigma + \mathbf{m}/2 + \Delta/2))}{\Gamma(1 + i\tau_I + w(i\sigma - \mathbf{m}/2 + \Delta/2))} \right| \stackrel{w(\Delta) \rightarrow \pm\infty}{\equiv} e^{-(2w(\Delta)+1)(\log|w(\Delta)|-1)+O(1)}. \quad (3.2.36)$$

Taking the product over weights  $w$ , we expect the one-loop determinant to be suppressed for large  $\Delta$ . We shall prove for a class of theories that in the appropriate limit  $\chi \rightarrow \pm\infty$  the one-loop determinant indeed is suppressed for all saddle points except those for which the  $D$ -term  $\phi\bar{\phi} - \chi$  is small throughout the sphere. The path integral localizes in this limit to solutions to  $\phi\bar{\phi} = \chi$  with vortices at the poles.

Let us focus for concreteness on  $U(N)$  SQCD with  $N_f$  fundamental and  $N_a \leq N_f$  antifundamental chiral multiplets of generic twisted masses  $\tau_I$  and  $\tilde{\tau}_I$  respectively. The case  $N_a \geq N_f$  is obtained by charge conjugation. We assume  $N_f \geq N$  to avoid supersymmetry breaking. The results extend to  $\prod_\ell U(N_\ell)$  quiver gauge theories by considering gauge groups one by one, and perhaps to more general matter contents.

Consider a smooth  $\mathcal{Q}$ -invariant configuration, and diagonalize  $\sigma$  by a constant gauge transformation. At most  $N$  chiral multiplets are non-zero: in each eigenspace of  $\sigma$ , at most one chiral multiplet is non-zero because of  $(\sigma + \tau_I)\phi_I = 0$  for fundamentals and  $\tilde{\phi}_I(-\sigma + \tilde{\tau}_I) = 0$  for antifundamentals. Focus first on a non-zero fundamental  $\phi_I \neq 0$ . The trace of (3.2.32) in the eigenspace  $\sigma = -\tau_I$  implies (with no summation on  $I$  in this paragraph)

$$\sin \theta \partial_\theta(\bar{\phi}_I \phi_I) = 2f(\theta)\bar{\phi}_I \eta \phi_I, \quad \partial_\theta(\bar{\phi}_I \eta \phi_I) = f(\theta) \sin \theta (\bar{\phi}_I \phi_I - \chi)\bar{\phi}_I \phi_I. \quad (3.2.37)$$

We prove by contradiction that  $\bar{\phi}_I \phi_I \leq \chi$  for any such non-zero solution (in particular  $\chi > 0$ ). Consider the infimum  $\theta_0$  of angles at which  $\bar{\phi}_I \phi_I \geq \chi$  (if it exists). The derivative of  $\bar{\phi}_I \phi_I$  must be non-negative, thus  $\bar{\phi}_I \eta \phi_I \geq 0$ . These two inequalities continue to hold for  $\theta \in [\theta_0, \pi]$  since derivatives are non-negative. However, we know that  $\phi_I$  is among non-positive eigenspaces of  $\eta(\pi) = -k^-$ , thus the second inequality must be saturated everywhere, hence  $\eta \phi_I = 0$  and we find constant  $\phi_I$  solutions with  $|\phi_I|^2 = \chi$ . Similarly, solutions where an antifundamental  $\tilde{\phi}_I \neq 0$  is non-zero obey  $|\tilde{\phi}_I|^2 \leq -\chi$  hence require  $\chi < 0$ . Collecting these results, we deduce in particular that the  $D$ -term  $\chi \mathbb{1}_N - \phi_I \bar{\phi}_I + \tilde{\phi}_I \tilde{\phi}_I$  is positive semidefinite for  $\chi > 0$  and negative semidefinite for  $\chi < 0$ . Furthermore, its trace is at least  $|\chi|$  (in absolute value) unless  $N$  chiral multiplets are non-zero, fully Higgsing the gauge group (fixing  $\sigma$ ).

The (diagonal) matrix  $\Delta$  is the integral (3.2.35) of this semidefinite matrix. One consequence is that  $\text{Tr } \Delta \rightarrow \pm\infty$  (with the same sign as  $\chi$ ) in the limits  $\chi \rightarrow \pm\infty$ , except for saddle points for which  $N$  chiral multiplets are non-zero and the  $D$ -term equation is approximately obeyed throughout the sphere. Another consequence is that all eigenvalues of  $\Delta$  have the same sign as  $\text{Tr } \Delta$ ; then taking the product of (3.2.36) over all weights we find that the full one-loop determinant is suppressed as  $\text{Tr } \Delta \rightarrow +\infty$  (for  $N_a > N_f$  instead it would be suppressed as  $\text{Tr } \Delta \rightarrow -\infty$  while for  $N_a = N_f$  it is suppressed in both limits). Therefore, the only saddle points that contribute as  $\chi \rightarrow +\infty$  are those with  $N$  non-zero fundamental chiral multiplets. The requirement that  $\phi$  belongs to non-negative integer eigenspaces of  $k^\pm$  at poles then forces all eigenvalues of  $k^\pm$  to be non-negative integers.

At the (South) North pole  $\phi_I$  obeys BPS (anti)vortex equations. The eigenvalues of  $k^\pm$  control the asymptotics  $\phi_I \sim (e^{i\varphi} \sin \theta)^{k^\pm} \phi_I^\circ$  at the poles thus counting (anti)vortices there. Since the integral of  $D$  is  $k^+ + k^-$ , the distance over which  $|\phi_I|^2$  goes from 0 at the poles to  $\chi$  must scale like  $k^\pm / \sqrt{\chi}$ : vortices become point-like as  $\chi \rightarrow \infty$ .

Altogether, the path integral is a sum over  $\binom{N_f}{N}$  Higgs branches  $H$ , namely choices of  $N$  flavors with  $\phi_I \neq 0$ , and over vorticities  $k_j^\pm$  ( $j = 1, \dots, N$ ). The classical action for each such configuration is evaluated using that the gauge flux and integrated  $D$ -term are  $k^+ \mp k^-$ , and the result factorizes: contributions from (anti)vortices at the (South) North pole depend (anti)holomorphically on  $z$ . After some massaging,

$$Z_{S^2}^{\text{SQCD}} = \sum_{\substack{H \subset \{1, \dots, N_f\} \\ \#H=N}} \left[ \prod_{J \in H} \frac{(z\bar{z})^{-i\tau_J} \prod_{I \notin H} \gamma(-i\tau_I + i\tau_J)}{\prod_{I=1}^{N_a} \gamma(1 + i\tilde{\tau}_I + i\tau_J)} f_H(z) f_H((-1)^{N_f - N_a} \bar{z}) \right] \quad (3.2.38)$$

$$f_{\{J_1, \dots, J_N\}}(x) = \sum_{k_1, \dots, k_N \geq 0} \prod_{j=1}^N \frac{x^{k_j} \prod_{I=1}^{N_a} (-i\tilde{\tau}_I - i\tau_{J_j})_{k_j}}{\prod_{i=1}^N (i\tau_{J_i} - i\tau_{J_j} - k_i)_{k_j} \prod_{I \notin \{J_i\}} (-i\tau_I + i\tau_{J_j} - k_j)_{k_j}} \quad (3.2.39)$$

where  $\gamma(y) = \Gamma(y)/\Gamma(1-y)$  and  $z$  is the renormalized value (3.2.20). Up to a relabeling of parameters, the function  $f_H(z)$  coincides with previously known vortex partition functions computed in the Omega background. This is unsurprising as point-like vortices are unaffected by the precise IR regulator (sphere or Omega background). The sign difference  $(-1)^{N_f - N_a}$  between vortices and antivortices is explained by noting that  $\mathcal{Q}^2$  rotates counterclockwise around one pole but clockwise around the other, hence one should map the rotation parameter

$1/r \rightarrow -1/r$ , and by noting that the renormalized  $z$  includes a factor  $r^{N_f - N_a}$ .

We have glossed over a technical difficulty: the one-loop determinant (3.2.36) is singular for chiral multiplets  $\phi_I$  that acquire a non-zero value in a given Higgs branch. The corresponding zero-mode of  $\phi_I$  is removed by the  $D$ -term equation, in other words integrating out  $D$  makes  $\phi_I$  massive. To derive (3.2.38) we have eliminated these zero-modes by taking the appropriate residues, but fixing signs is not straightforward in this approach. On the other hand, we know that Coulomb branch and Higgs branch localization must yield the same result. One can derive the Higgs branch expression (3.2.38) from the Coulomb branch integral (if  $N_a < N_f$  or  $N_a = N_f$  and the true FI parameter  $\zeta > 0$ ) by closing the integration contours and writing the integral as a sum of residues. From the Coulomb branch integral,  $k^\pm$  appear as the flux  $\mathbf{m} = k^+ - k^-$  and integers  $k_j^+ + k_j^- \geq 0$  labeling poles of gamma functions. Factorization is due to the fact that the integrand in the Coulomb branch expression is a product of a function of  $z$  and  $i\sigma + \mathbf{m}/2$  by a function of  $\bar{z}$  and  $i\sigma - \mathbf{m}/2$ .

In more general theories, the Higgs branch localization result takes the form

$$Z_{S^2} = \sum_{\text{Higgs branches}} Z_{\text{cl}} Z'_{1\text{-loop}} Z_{\text{vortex}} Z_{\text{antivortex}} . \quad (3.2.40)$$

The sum ranges over constant solutions to  $(\sigma + \tau_I)\phi_I = 0$  and to the  $D$ -term equation  $\phi\bar{\phi} = \chi$ , which form a discrete set for generic twisted masses.<sup>5</sup> The factors are a classical contribution from these constant solutions, a one-loop determinant with poles removed as outlined above, and (anti)holomorphic contributions from point-like (anti)vortices at the poles. The detailed expression can in principle be obtained by localizing onto the Higgs branch as we have just done for SQCD, but solutions to the BPS equations have not been investigated in general.

A simpler approach to obtain (3.2.40) is to start from the Coulomb branch integral and close contours: as for SQCD, the residues organize themselves into a factorized form. This leads to vortex partition functions which were also later computed in the Omega background [36]. The relevant sets of poles are described in subsection 4.6.2. We apply this technique to compare partition functions of dual theories in subsection 3.5.2.

### 3.2.6 One-loop determinants

The first step in computing one-loop determinants around a  $\mathcal{Q}$ -invariant configuration  $\Phi_0$  is to write the quadratic Lagrangian for fluctuations  $\delta\Phi$ , including a gauge fixing term. The Lagrangian takes the form  $\delta\Phi \Delta[\Phi_0] \delta\Phi$  for some operator  $\Delta$  whose bosonic part  $\Delta_b$  is essentially a Laplacian, and whose fermionic part  $\Delta_f$  is essentially a Dirac operator. The one-loop determinant reads

$$Z_{1\text{-loop}}[\Phi_0] = \frac{\det \Delta_f[\Phi_0]}{\det \Delta_b[\Phi_0]} , \quad (3.2.41)$$

where we omit the usual square root by considering  $\Delta_b$  as a complex operator rather than a real operator on the same space of fields. Additionally, the operators  $\Delta_b$  and  $\Delta_f$  split into direct sums of contributions from the vector and chiral multiplets, which decompose further

---

<sup>5</sup>In theories with a complicated matter content, this should be checked explicitly.

into individual roots or weights. Three techniques are commonly used to evaluate these determinants.

The most pedestrian approach (for the round sphere only) is to decompose fields into spherical harmonics. In this decomposition  $\Delta_b$  and  $\Delta_f$  are block diagonal, with blocks involving a finite number of modes. The determinant of each block is straightforward to evaluate, and in their product, contributions of many bosonic and fermionic modes cancel.

A second approach harnesses the cancellation by constructing two eigenmodes of  $\Delta_f$  for each eigenmode of  $\Delta_b$ , and viceversa. The pairing fails to be exactly 2-to-1 for some modes, which thus contribute to the ratio of determinants (3.2.41). Only these eigenvalues need to be computed, instead of the whole spectrum of  $\Delta$ .

The third approach is more systematic. To begin with, find a basis  $(X, X')$  of the fluctuation fields such that  $\mathcal{Q}X = X'$  and  $\mathcal{Q}X' = \mathcal{R}X$  where  $\mathcal{R} = \mathcal{Q}^2$  is bosonic. Separate pairs  $(X_0, X'_0)$  with  $X_0$  bosonic and  $X'_0$  fermionic from pairs  $(X_1, X'_1)$  with opposite statistics, and write down the part of  $V$  quadratic in fluctuations as

$$V^{(2)} = X'_0 D_{00} X_0 + X_1 D_{10} X_0 + X'_0 D_{01} X'_1 + X_1 D_{11} X'_1 . \quad (3.2.42)$$

The operators  $\Delta_b$  and  $\Delta_f$  are read from  $\mathcal{Q}V^{(2)}$ . After some linear algebra, the constraint  $\mathcal{Q}^2 V^{(2)} = 0$  implies that<sup>6</sup>

$$\frac{\det \Delta_f}{\det \Delta_b} = \frac{\det' \mathcal{R}_1}{\det' \mathcal{R}_0} = \frac{\det_{\text{coker } D_{10}} \mathcal{R}_1}{\det_{\text{ker } D_{10}} \mathcal{R}_0} = \prod_i \mathcal{R}(i)^{-m_i} , \quad (3.2.43)$$

where  $i$  indexes eigenvalues  $\mathcal{R}(i)$  of  $\mathcal{R}$ , and  $m_i$  is the multiplicity of  $\mathcal{R}(i)$  in  $\text{ker } D_{10}$  minus that in  $\text{coker } D_{10}$ . These eigenvalues and multiplicities are read from the  $\mathcal{R}$ -equivariant index

$$\text{ind}_{\mathcal{R}}(D_{10}) = \text{Tr}_{\text{ker } D_{10}} e^{t\mathcal{R}} - \text{Tr}_{\text{coker } D_{10}} e^{t\mathcal{R}} = \sum_i m_i e^{t\mathcal{R}(i)} , \quad (3.2.44)$$

itself computed as a sum over fixed points of  $\mathcal{R}$ , thanks to the Atiyah-Bott-Berline-Vergne equivariant localization formula [37, 38].

Each of these methods requires lengthy calculations for which we refer to appendices of [11–13]. To clarify a sign that was originally missed (in the vector multiplet one-loop determinant) we must describe some salient points. By continuity, squashing cannot affect signs, so we focus for simplicity on the round sphere  $f(\theta) = r$  and let  $r = 1$ .

As a warm-up before the vector multiplet, consider the one-loop determinant for fluctuations of a chiral multiplet along a particular weight  $w$  of  $\mathfrak{R}$ . Denote by  $w(\mathbf{m})$  and  $w(\sigma)$  the (on-shell) components of the vector multiplet when acting on this weight. One finds the eigenvalues of  $\Delta_b$  by expanding fields in (spin) spherical harmonics:  $\left(J + \frac{1}{2}\right)^2 - \left(iw(\sigma) + \frac{1-q}{2}\right)^2$  with multiplicity  $2J + 1$  for  $J - \frac{|w(\mathbf{m})|}{2} \in \mathbb{Z}_{\geq 0}$ . The fermionic Lagrangian is

$$\mathcal{L}_f^{\text{c.m.}(w)} = i\bar{\psi} \Delta_f^{\text{c.m.}(w)} \psi = i\bar{\psi} \left( -\not{D} - w(\mathbf{m})/2 + (iw(\sigma) - q/2)\gamma^3 \right) \psi , \quad (3.2.45)$$

---

<sup>6</sup>For a non-degenerate deformation term,  $\Delta_f$  and  $\Delta_b$  have no zero-modes transverse to the localization locus.  $\mathcal{R}_0$  and  $\mathcal{R}_1$  can have such zero-modes, which should be omitted from  $\det \mathcal{R}_1 / \det \mathcal{R}_0$ , however these are transverse to  $\text{coker } D_{10}$  and  $\text{ker } D_{10}$ .

where  $\mathcal{D} = \gamma^i D_i$  involves a flux  $w(\mathbf{m})$  through the sphere. Note that we extracted a factor of  $i$  from  $\Delta_f$ : this multiplies the determinant by an overall constant phase which only affects the normalization of the partition function. The operator  $\mathcal{D}$  has  $|w(\mathbf{m})|$  zero-modes of chirality  $\text{sign } w(\mathbf{m})$ , and it has, for each  $J - |w(\mathbf{m})|/2 - 1/2 \in \mathbb{Z}_{\geq 0}$ ,  $2J + 1$  pairs of modes with eigenvalues  $\pm i\sqrt{(J + 1/2)^2 - w(\mathbf{m})^2/4}$  interchanged by  $\gamma^3$ . The operator  $\Delta_f$  thus decomposes into blocks with the following determinant (the matrix is expressed in a basis of eigenmodes of  $\mathcal{D}$ )

$$\det \begin{pmatrix} -i\sqrt{(J + 1/2)^2 - w(\mathbf{m})^2/4} - w(\mathbf{m})/2 & -iw(\sigma) + q/2 \\ -iw(\sigma) + q/2 & i\sqrt{(J + 1/2)^2 - w(\mathbf{m})^2/4} - w(\mathbf{m})/2 \end{pmatrix} \quad (3.2.46)$$

$$= \left( J + \frac{1-q}{2} + iw(\sigma) \right) \left( J + \frac{1+q}{2} - iw(\sigma) \right),$$

as well as  $|w(\mathbf{m})|$  eigenvalues  $-w(\mathbf{m})/2 + (iw(\sigma) - q/2) \text{sign } w(\mathbf{m})$ . Combining these ingredients,

$$\frac{\det \Delta_f^{\text{c.m.}(w)}}{\det \Delta_b^{\text{c.m.}(w)}} = \left( -w(\mathbf{m})/2 - (q/2 - iw(\sigma)) \text{sign } w(\mathbf{m}) \right)^{|w(\mathbf{m})|}$$

$$\times \frac{\prod_{J=(|w(\mathbf{m})|+1)/2}^{\infty} \left( J + 1/2 - q/2 + iw(\sigma) \right)^{2J+1} \left( J + 1/2 + q/2 - iw(\sigma) \right)^{2J+1}}{\prod_{J=|w(\mathbf{m})|/2}^{\infty} \left( J + 1 - q/2 + iw(\sigma) \right)^{2J+1} \left( J + q/2 - iw(\sigma) \right)^{2J+1}}$$

$$= \left( -\text{sign } w(\mathbf{m}) \right)^{|w(\mathbf{m})|} \prod_{J=|w(\mathbf{m})|/2}^{\infty} \frac{J + 1 - q/2 + iw(\sigma)}{J + q/2 - iw(\sigma)}. \quad (3.2.47)$$

The infinite product is divergent and we apply zeta-function regularization, namely replace  $\prod_{k \geq 0} (x + k)$  by  $\sqrt{2\pi}/\Gamma(x)$ . Combining the contributions from all weights  $w$  of the chiral multiplet representation, we get the chiral multiplet one-loop determinant

$$\mathcal{Z}_{1\text{-loop}}^{\text{c.m.}} = \prod_w \frac{\left( -\text{sign } w(\mathbf{m}) \right)^{|w(\mathbf{m})|} \Gamma\left(\frac{q}{2} - iw(\sigma) + \frac{|w(\mathbf{m})|}{2}\right)}{\Gamma\left(1 - \frac{q}{2} + iw(\sigma) + \frac{|w(\mathbf{m})|}{2}\right)} = \prod_w \frac{\Gamma\left(\frac{q}{2} - iw(\sigma) - \frac{w(\mathbf{m})}{2}\right)}{\Gamma\left(1 - \frac{q}{2} + iw(\sigma) - \frac{w(\mathbf{m})}{2}\right)}. \quad (3.2.48)$$

The last equality can be proven using  $\Gamma(x + 1) = x\Gamma(x)$ .

We now move on to the vector multiplet, with an emphasis on signs rather than the precise factors. The quadratic action, hence the one-loop determinant, splits into contributions from each root  $\alpha$  of  $G$ . Again we denote by  $\alpha(\mathbf{m})$  and  $\alpha(\sigma)$  the relevant on-shell components of the vector multiplet. The bosonic operator  $\Delta_b^\alpha$ , taking into account ghosts, is positive definite as for the chiral multiplet hence will not affect signs in the final result. The fermionic action is closely related to the action (3.2.45) of an adjoint chiral multiplet of R-charge  $q = 0$ . It is

$$\mathcal{L}_f^{\text{v.m.}(\alpha)} = -i\bar{\lambda}\Delta_f^{\text{v.m.}(\alpha)}\lambda = -i\bar{\lambda}\left(-\mathcal{D} + \frac{1}{2}[w(\mathbf{m}), \cdot] + i\gamma^3[w(\sigma), \cdot]\right)\lambda, \quad (3.2.49)$$

which differs from its chiral multiplet counterpart for the same weight  $\alpha$  in two respects: we extracted a different overall factor  $-i$  instead of  $i$ , and more importantly the sign in front of

$w(\mathbf{m})$  changed. Keeping track of the effect of this change on the eigenvalues found previously gives

$$\det \Delta_f^{\text{v.m.}(\alpha)} = \left( -\text{sign } \alpha(\mathbf{m}) \right)^{|\alpha(\mathbf{m})|} \left( \frac{|\alpha(\mathbf{m})|}{2} + i\alpha(\sigma) \right)^{|\alpha(\mathbf{m})|} \prod_{J=\frac{|\alpha(\mathbf{m})|+1}{2}}^{\infty} \left( \left( J + \frac{1}{2} \right)^2 + \alpha(\sigma)^2 \right)^{2J+1}. \quad (3.2.50)$$

Upon taking the product over the roots  $\alpha$ , the signs for positive and negative roots combine:

$$\prod_{\alpha} \left( -\text{sign } \alpha(\mathbf{m}) \right)^{|\alpha(\mathbf{m})|} = \prod_{\alpha>0} (-1)^{\alpha(\mathbf{m})} = e^{2\pi i \delta(\mathbf{m})} \quad (3.2.51)$$

where  $\delta$  is the Weyl vector, half-sum of the positive roots, and  $2\delta(\mathbf{m}) \in \mathbb{Z}$  may be odd. The other contributions in (3.2.50) combine into positive factors, and most are cancelled by bosonic factors. Altogether, the vector multiplet one-loop determinant is

$$Z_{1\text{-loop}}^{\text{v.m.}} = e^{2\pi i \delta(\mathbf{m})} \prod_{\alpha>0} \left[ \frac{\alpha(\mathbf{m})^2}{4} + \alpha(\sigma)^2 \right]. \quad (3.2.52)$$

More precisely, the one-loop determinant omits factors for roots with  $\alpha(\mathbf{m}) = 0$ . We include these factors nevertheless: they arise as Vandermonde determinants when replacing the integral over all scalars  $\sigma$  in the Lie algebra of  $G$  commuting with  $\mathbf{m}$  by an integral over the Cartan subalgebra only.

Had we kept the radius explicitly, it would appear as  $1/r^2$  in each factor of (3.2.52) and  $1/r$  in each factor of (3.2.47). The zeta-function regularized form of  $\prod_{k \geq 0} (x + k/r)$  is  $\sqrt{2\pi} r^{rx-1/2} / \Gamma(rx)$ , thus the one-loop determinant listed above are multiplied altogether by

$$r^{-\dim G + \text{rank } G} \prod_w r^{1-q+2irw(\sigma)} = r^{c/3 + \text{rank } G + 2ir \sum_w w(\sigma)}, \quad (3.2.53)$$

with  $c/3 = \sum_w (1-q) - \dim G$  as in (3.2.21). This power of  $r$ , together with the power  $r^{-\text{rank } G}$  due to integrating over  $r\sigma$  rather than  $\sigma$ , yields the overall power  $r^{c/3}$  and the renormalization (3.2.20) of FI parameters in subsection 3.2.3.

### 3.3 Other $\mathcal{N}=(2, 2)$ curved-space results

In this section we will briefly present some of the main directions in which the simple computation of the  $S^2$  partition function has been developed.

#### 3.3.1 Local operator insertions

Besides the computation of pure Euclidean partition functions, localization is also extremely powerful in computing expectation values and correlators of BPS operators: both local

and non-local, both order and disorder.<sup>7</sup> In order to be computable, the operators must be invariant under the supercharge  $\mathcal{Q}$  used to localize, in other words they must be BPS. However the superalgebra on a curved manifold may be quite different from the flat-space one, therefore localization on  $S^2$  (or other curved manifolds) grants us access to correlators that go beyond the standard “chiral rings” on flat space.

Let us discuss local operators on  $S^2$ .<sup>8</sup> It follows from (3.2.4)-(3.2.5) that the order operators invariant under  $\mathcal{Q}$  are the field-strength twisted chiral operators  $\Sigma$ —whose bottom components are the complex scalars  $(\sigma - i\eta)$ —at the North pole  $x_N$ , and their conjugates  $\bar{\Sigma}$  at the South pole  $x_S$  (since  $\mathcal{Q}^2 = J + R/2$ ,  $\mathcal{Q}$ -closed local operators must sit at fixed points of  $J$ ). For order operators the localization prescription is simply to insert the operator into the integrand, in this case  $\sigma \mp i\mathbf{m}/2r$  for  $\Sigma$  and  $\bar{\Sigma}$ , respectively. Schematically and setting  $r = 1$ , non-normalized correlators are given by

$$\left\langle \mathcal{O}_N(\Sigma(x_N)) \mathcal{O}_S(\bar{\Sigma}(x_S)) \right\rangle_{\text{n.n.}} = \frac{1}{|\text{Weyl}|} \sum_{\mathbf{m}} \int_{\mathfrak{t}} \frac{d^{\text{rank}} \sigma}{(2\pi)^{\text{rank}}} \mathcal{O}_N\left(\sigma - \frac{i\mathbf{m}}{2}\right) \mathcal{O}_S\left(\sigma + \frac{i\mathbf{m}}{2}\right) Z_{\text{cl},1\text{-loop}} \quad (3.3.1)$$

where  $\mathcal{O}_{N,S}$  are arbitrary gauge-invariant polynomial functions, while normalized correlators are further divided by  $Z_{S^2}$ .

There is a subtlety, though. Since we are forced to place all chiral operators at the same point (and similarly for anti-chirals), one might expect contact terms to show up. Such contact terms can be understood in terms of operator mixings [40]. Indeed the correlators (3.3.1) do not satisfy the flat-space chiral ring relations. It turns out [10, 41] that they realize a sort of non-commutative deformation of the chiral ring. Let us present the simple example of  $\mathbb{C}\mathbb{P}^{N-1}$ , *i.e.* the  $U(1)$  GLSM with  $N$  chiral multiplets of charge 1. With a trick similar to the one used in subsection 3.2.4, one can show that the correlators satisfy

$$\left\langle \Sigma^N \mathcal{O}_N(\Sigma) \mathcal{O}_S(\bar{\Sigma}) \right\rangle = \left(\frac{i}{r}\right)^N z \left\langle \mathcal{O}_N\left(\Sigma - \frac{i}{r}\right) \mathcal{O}_S(\bar{\Sigma}) \right\rangle, \quad (3.3.2)$$

where  $\Sigma$  and  $\bar{\Sigma}$  are inserted at the North and South pole, respectively. In the limit  $r \rightarrow \infty$  this reproduces the twisted chiral ring of the GLSM, namely  $\Sigma^N = \left(\frac{i}{r}\right)^N z$ ,<sup>9</sup> which coincides with the quantum cohomology of  $\mathbb{C}\mathbb{P}^{N-1}$  [42]. To interpret the deformation, we rewrite (non-normalized) correlators of  $\Sigma$  as derivatives of the partition function,  $\Sigma \rightarrow \frac{z}{ir} \frac{\partial}{\partial z}$ , which obviously do not commute with  $z$ . Then (3.3.2) reduces to the A-system equation for  $\mathbb{C}\mathbb{P}^{N-1}$ ,  $\left(\frac{\partial}{\partial \log z}\right)^N - (-1)^N z = 0$ , and the non-commutative ring is the  $\mathcal{D}$ -module obtained as quotient of the Weyl algebra by that equation.

An interesting class of local disorder operators is given by vortex operators.<sup>10</sup> They are

<sup>7</sup>By “order” operators we mean standard polynomial functions of the fundamental fields in the Lagrangian, while “disorder” operators are defined as singular boundary conditions for the fields in the path-integral at points or submanifolds [39].

<sup>8</sup>Wilson line operators can be easily computed as well, see [12].

<sup>9</sup>On flat space this should be written as  $\Sigma^N = (iM_{\text{UV}})^N z_{\text{UV}}$ , where the UV Fayet-Iliopoulos term is related to the renormalized one as in (3.2.20).

<sup>10</sup>They are the equivalent of vortex line operators in 3d, and of certain simple surface operators in 4d.

defined by the singular behavior of the gauge field  $A$  around a point,

$$A \sim \gamma d\varphi, \quad (3.3.3)$$

where  $\varphi$  is an angular coordinate around that point and  $\gamma \in \mathfrak{g}$ . The definition (3.3.3) is in a gauge where matter fields are regular, therefore it corresponds to a point-like insertion of magnetic flux:  $F_{12} = 2\pi\gamma \delta^2(x)$ . On  $S^2$  we can insert BPS local vortex operators at the two poles, and the supersymmetric operator also involve the local source  $D = 2\pi i\gamma \delta^2(x)$ . In [43] the correlator of two vortex operators at the two poles, and labelled by  $\gamma^{N,S}$ , has been computed with localization techniques in  $\mathcal{N}=(2,2)$  simple gauge theories. A useful trick is the equivalence between gauge theories in the presence of (quantized) vortex operators and on orbifolds [44]. In the Abelian case the result is that the correlators, as functions of  $\gamma$ , are piecewise constant with jumps at certain specific values. In the non-Abelian case, instead, there is a dependence on the Levi subgroup specified by  $\gamma$ , which is the reductive subgroup of  $G$  commuting with  $\gamma$ . In both cases the partition function still factorizes as in subsection 3.2.5.

### 3.3.2 Twisted multiplets on the sphere

So far we have considered the simplest type of  $\mathcal{N}=(2,2)$  gauge theories: those made of vector and chiral multiplets. Things become even more interesting when including other types of multiplets. The addition of twisted chiral multiplets has been studied in [13]. A twisted chiral multiplet  $Y : (y, \chi, G)$  satisfies  $\overline{D}_+ Y = D_- Y = 0$  and it comprises a complex scalar  $y$ , a Dirac fermion  $\chi$  and a complex auxiliary scalar  $G$ . One can write Lagrangians for them on the sphere that preserve the  $\mathfrak{su}(2|1)$  supersymmetry algebra of  $S^2$ , and apply localization to compute partition functions and correlators.<sup>11</sup> Twisted chiral multiplets must be neutral under vector multiplets, however they can couple to the field-strength twisted chiral multiplet  $\Sigma$  through a twisted superpotential  $\widetilde{W}$ .

The supersymmetric action on  $S^2$  follows from the Lagrangian

$$\mathcal{L}_{\text{t.c.m.}} = D^i \bar{y} D_i y + i \bar{\chi} \gamma^i D_i \chi + \left| G + \frac{\Delta}{r} y \right|^2. \quad (3.3.4)$$

The parameter  $\Delta$  is the Weyl weight of the twisted chiral multiplet. In the special case  $\Delta = 1$ , the action is the same as for an Abelian vector multiplet, because with the identifications  $y = \sigma - i\eta$ ,  $\chi = \lambda$  and  $G = D - iF_{12}$  we construct the field-strength twisted chiral multiplet.

The interaction term  $\mathcal{L}_{\widetilde{W}}$  has been already considered in subsection 3.2.1. In the context of mirror symmetry, as we will see in subsection 3.5.1, particularly important is the non-minimal coupling  $\widetilde{W} = \Sigma Y$  between a vector multiplet and twisted chiral multiplets, where  $Y$  plays the role of a dynamical FI term.

One can perform localization with respect to the same supercharge  $\mathcal{Q}$  used before [13]. From the BPS equations  $\delta\chi = \delta\bar{\chi} = 0$ , one obtains the conditions

$$y = \text{const.}, \quad G + \frac{\Delta}{r} y = 0, \quad (3.3.5)$$

<sup>11</sup>In fact, [13] generalizes the construction to squashed rotationally-invariant spheres which preserve only an  $\mathfrak{su}(1|1)$  superalgebra. It turns out that the localization computations do not depend on the squashing.

in other words the complex scalar  $y$  can be an arbitrary constant on the sphere. The Lagrangian  $\mathcal{L}_{\text{t.c.m.}}$  is  $\mathcal{Q}$ -exact and can be used as a localization term. The one-loop determinant is trivial, in the sense that it does not depend on  $y$ . Thus, for a system of twisted chiral multiplets  $Y_I$  the localization formula reads

$$Z_{S^2} = \int \left( \prod_I d^2 y_I \right) e^{-4\pi i r \tilde{W}(y) - 4\pi i r \overline{\tilde{W}}(\bar{y})}, \quad (3.3.6)$$

where the index  $I$  runs over the twisted chiral multiplets. As we will see in [subsection 3.5.1](#), this expression can be used to confirm the mirrors [\[45\]](#) of Hori and Vafa.

The superalgebra on  $S^2$  we have considered so far—that we will call  $\mathfrak{su}(2|1)_A$ —is a subalgebra of the  $\mathcal{N}=(2,2)$  superconformal algebra whose bosonic part comprises  $\mathfrak{su}(2)$  rotations of  $S^2$  and the  $\mathfrak{u}(1)$  vector-like R-symmetry. There exists, though, another inequivalent choice,  $\mathfrak{su}(2|1)_B$ , which instead contains the  $\mathfrak{u}(1)$  axial R-symmetry [\[21\]](#). The two are swapped by the  $\mathbb{Z}_2$  mirror outer automorphism that exchanges the R-symmetries and exchanges multiplets with twisted multiplets. Those superalgebras contain supercharges  $\mathcal{Q}_A$  and  $\mathcal{Q}_B$ , respectively. The charge  $\mathcal{Q}_A$  annihilates twisted chiral operators at the North pole and their conjugates at the South pole: it can be used to compute their correlators on  $S^2$  (as we saw in [subsection 3.3.1](#)), as well as the Zamolodchikov metric on the Kähler moduli space of conformal fixed points. Those quantities are independent of complex structure moduli because chiral (superpotential) deformations are  $\mathcal{Q}_A$ -exact. Likewise,  $\mathcal{Q}_B$  annihilates chiral operators at the North pole and their conjugates at the South pole, it can be used to compute their correlators on  $S^2$  and the Zamolodchikov metric on the complex structure moduli space of fixed points [\[21\]](#). They will be independent of Kähler moduli because twisted chiral (twisted superpotential) deformations are  $\mathcal{Q}_B$ -exact.

At this point, the easiest way to construct  $\mathfrak{su}(2|1)_B$ -invariant actions on  $S^2$  and compute their path-integrals with localization is to exploit the  $\mathbb{Z}_2$  mirror automorphism. Thus, the  $\mathfrak{su}(2|1)_B$  partition function of a gauge theory of vector and chiral multiplets is equal to the  $\mathfrak{su}(2|1)_A$  partition function of a theory of twisted vector and twisted chiral multiplets. In this way, we can perform all computations in the  $\mathfrak{su}(2|1)_A$  framework we have used to far, provided we study all types of twisted multiplets, in particular twisted vector multiplets.

A twisted vector multiplet is a real multiplet  $\tilde{V}$  subject to gauge redundancy by a twisted chiral multiplet:  $\tilde{V} \cong \tilde{V} + \Lambda_t + \bar{\Lambda}_t$ . It has the same components as a standard vector multiplet,  $\tilde{V} : (A_\mu, \sigma, \bar{\sigma}, \eta, \bar{\eta}, D)$ , but the supersymmetry transformations are different. In particular, the field strength sits in the chiral multiplets  $\tilde{\Sigma} : (\sigma, \eta, D + iF)$  and its conjugate, the transformation of which we have already discussed. Twisted chiral multiplets can be minimally coupled to twisted vector multiplets; in Wess-Zumino gauge, the transformations of the former pick up a dependence on the latter. One can then write down supersymmetric actions on  $S^2$  [\[21\]](#), in particular the Yang-Mills Lagrangian for  $\tilde{V}$  equals the kinetic Lagrangian for the chiral multiplet  $\tilde{\Sigma}$ . The FI term sits in a linear superpotential term for  $\tilde{\Sigma}$ .

An important point to stress is that charged twisted chiral multiplets contribute to the gauge- $U(1)_R$  anomaly. Since  $U(1)_R$  is part of the supersymmetry algebra on  $S^2$  (rather than being an outer automorphism as on flat space), such an anomaly would spoil supersymmetry.

Therefore, only theories for which the sums of the charges of twisted chirals under Abelian twisted vectors vanish can preserve supersymmetry on  $S^2$  quantum mechanically.<sup>12</sup>

Both kinetic actions are  $\mathcal{Q}$ -exact and can be used for localization [21]. The bosonic part of the Lagrangian reads

$$\begin{aligned} \mathcal{L}_{\text{kin}}|_{\text{bos}} = & \frac{1}{2g^2} \text{Tr} \left( |D_\mu \sigma|^2 + \frac{1}{4} [\sigma, \bar{\sigma}]^2 + F^2 + \tilde{D}^2 \right) \\ & + |D_\mu y|^2 + |G|^2 + \frac{1}{2} (|\sigma y|^2 + |\bar{\sigma} y|^2) + \frac{g^2}{2} (y\bar{y} - \chi)^2, \end{aligned} \quad (3.3.7)$$

where  $\tilde{D} \equiv D + ig^2(y\bar{y} - \chi)$  and  $\chi$  is the matrix of FI terms that commutes with the gauge generators. Under the standard reality conditions, that Lagrangian is semipositive definite. The path-integral localizes<sup>13</sup> to its zeros modulo gauge transformations, that is the manifold

$$\mathcal{M} = \left\{ y \mid y = \text{const.}, y\bar{y} - \chi = 0 \right\} / G = \mathbb{C}^{|\mathfrak{R}|} //_\chi G \quad (3.3.8)$$

with all other fields vanishing. Therefore,  $\mathcal{M}$  is a Kähler quotient of  $\mathbb{C}^{|\mathfrak{R}|}$  at levels  $\chi$  of the moment map, where  $|\mathfrak{R}|$  is the dimension of the matter representation.

Let us consider the Abelian case discussed in [21]: the gauge group is  $U(1)^{N_c}$  and there are  $N_f$  twisted chiral multiplets of charges  $Q_{I=1\dots N_f}^{a=1\dots N_c}$  subject to  $\sum_I Q_I^a = 0$ . The one-loop determinant turns out to be

$$Z_{1\text{-loop}} = \det(M^\dagger M), \quad (3.3.9)$$

where  $M$  is the  $N_f \times N_c$  matrix  $M_I^a = Q_I^a y_I$ . Obviously it must have  $N_f \geq N_c$ , otherwise the gauginos have fermionic zero-modes and the determinant vanishes. After some algebra, the partition function can be written as

$$Z_{S^2} = \int \frac{d^{N_f} y \wedge d^{N_f} \bar{y}}{(2\pi)^{N_c}} \det(M^\dagger M) \prod_a \delta(2\mu_a + \chi_a) e^{-4\pi i r \tilde{W}(y) - 4\pi i r \bar{\tilde{W}}(\bar{y})}, \quad (3.3.10)$$

where the functions

$$\mu_a = -\frac{1}{2} \sum_I Q_I^a |y_I|^2 \quad (3.3.11)$$

are the moment maps for the gauge action. Twisted chiral and antichiral operators are easily inserted at the North and South pole, respectively, by including  $\mathcal{O}_{\text{NP}}(Y)$  and  $\mathcal{O}_{\text{SP}}(\bar{Y})$  in the integrand.

An interesting check performed in [21] in models with a low-energy geometric description as Calabi-Yau NLSMs, is that the partition function assumes the form

$$Z_{S^2} = i^{\dim \mathcal{M}} \int_{\mathcal{M}} \Omega \wedge \bar{\Omega} = e^{-\mathcal{K}_C} \quad (3.3.12)$$

<sup>12</sup>The same statement is true if we try to use the B-type topological twist [46].

<sup>13</sup>As always, one should be careful to include the gauge-fixing sector. The details can be found in the reference.

in terms of the nonvanishing holomorphic top form  $\Omega$ . Thus, the sphere partition function computes the Kähler potential on the complex structure moduli space.

There are other multiplets that represent the  $\mathcal{N}=(2, 2)$  supersymmetry algebra, such as semichiral multiplets, semichiral vector multiplets and large vector multiplets [47, 48]. The most general  $\mathcal{N}=(2, 2)$  NLSM contains chiral, twisted chiral and semichiral multiplets, and has a non-Kähler target with bi-Hermitian [49] (also known as generalized Kähler [50, 51]) geometry with torsion. Some of those models can be realized at the IR of GLSMs constructed out of the more general multiplets. For instance, the sphere partition function of GLSMs with semichiral multiplets has been computed in [52].

### 3.3.3 Localization on the hemisphere

A very interesting development of the localization programme is to consider theories on manifolds with boundaries. This is an extremely rich and interesting problem in its own right, it allows to discuss domain walls and interfaces between different phases, it relates with lower-dimensional theories that may live along the boundary, and in the 2d case it makes contact with the physics of D-branes via string theory.

As a first step, [22–24] study 2d  $\mathcal{N}=(2, 2)$  gauge theories on the hemisphere (topology of the disk  $D_2$ ) and compute their partition function with localization. The result  $Z_{D_2}(\mathcal{B})$  depends on the boundary conditions—or D-brane—at the boundary, and they mainly focus on B-branes [46, 53–55]. The partition function depends holomorphically on twisted chiral parameters and it is independent of chiral parameters. In fact, it computes the inner product  $\langle \mathcal{B} | \mathbb{1} \rangle$  between two states in the Ramond sector, one generated by the identity operator<sup>14</sup> and the other by the boundary conditions, and this is called the *central charge* of the D-brane [53]. For theories that flow to NLSMs on Kähler manifolds, the large-volume limit reproduces the known geometric expression [56], however the localization formula contains all quantum corrections (to be compared with [45, 54]). This can help in identifying the precise correspondence between the original B-brane and the mirror A-brane.

The partition function takes the form of an integral of a meromorphic form, and the choice of contour is related to the choice of boundary conditions for vector multiplets. There is no a priori rule to decide the boundary conditions, but the convergence of the integral imposes strong constraints. Near the phase boundaries, a convergent contour can be found only for a very restricted class of branes, and this reproduces the *grade restriction rule* found in [55] in some specific cases, generalizing it to non-Abelian GLSMs and non-Calabi-Yau geometries.

Let us briefly describe the localization computation of  $Z_{D_2}(\mathcal{B})$  [22–24]. The hemisphere is parametrized by  $\theta$  in the range  $[0, \frac{\pi}{2}]$  and the boundary breaks the superalgebra  $\mathfrak{su}(2|1)_A$  to  $\mathfrak{su}(1|1)_A$ , whose bosonic  $\mathfrak{u}(1)$  subalgebra is a combination of rotations and vector-like R-symmetry rotations. To construct the kinetic actions for vector and chiral multiplets, one can use the same  $\mathcal{Q}$ -exact expressions as on  $S^2$ , however they will now involve boundary

---

<sup>14</sup>More generally, one can compute  $\langle \mathcal{B} | \mathcal{O} \rangle$  by inserting the twisted chiral operator  $\mathcal{O}$  at the pole.

terms (we set  $r = 1$ ):

$$\begin{aligned} \delta_{\mathcal{Q}}\delta_{\bar{\epsilon}} \int d\text{vol}_2 \text{Tr} \left( \bar{\lambda}\lambda/2 - 2D\sigma + \sigma^2 \right) &= \int d\text{vol}_2 \mathcal{L}_{\text{v.m.}} + \oint_{\theta=\frac{\pi}{2}} d\varphi \mathcal{L}_{\text{v.m.}}^{\text{bd}} \\ \delta_{\mathcal{Q}}\delta_{\bar{\epsilon}} \int d\text{vol}_2 \left( \bar{\psi}\psi - 2i\bar{\phi}\sigma\phi + (q-1)\bar{\phi}\phi \right) &= \int d\text{vol}_2 \mathcal{L}_{\text{c.m.}} + \oint_{\theta=\frac{\pi}{2}} d\varphi \mathcal{L}_{\text{c.m.}}^{\text{bd}} . \end{aligned} \quad (3.3.13)$$

Likewise, the FI and  $\vartheta$ -terms as well as more general twisted superpotential interactions are corrected by boundary terms to be supersymmetric. However the variation of the superpotential is a boundary term:

$$\delta\mathcal{L}_W = iD_\mu \left( \bar{\epsilon}\gamma^\mu\psi_i \partial_i W(\phi) \right) + iD_\mu \left( \epsilon\gamma^\mu\bar{\psi}_{\bar{i}} \partial_{\bar{i}} W(\bar{\phi}) \right) \quad (3.3.14)$$

called the Warner term [57]. This is not easily canceled by a boundary term as before.

To cancel the variation of the superpotential, we need to construct the so-called Chan-Paton boundary interaction [55]. First we need a  $\mathbb{Z}_2$ -graded vector space

$$\mathcal{V} = \mathcal{V}^e \oplus \mathcal{V}^o . \quad (3.3.15)$$

We can think of the space  $\text{End}(\mathcal{V})$  as a superalgebra, and take the odd endomorphisms to anticommute with the fermionic fields. Then  $\mathcal{V}$  must furnish a unitary representation of  $G \times G_F \times U(1)_R$ , *i.e.* its coordinates are assigned R-charges  $q_*$  and a gauge/flavor representation  $\rho_*$ . Finally we should construct two polynomials  $\mathfrak{Q}(\phi)$ ,  $\bar{\mathfrak{Q}}(\bar{\phi})$  (complex conjugate in Lorentzian signature) with values in  $\text{End}(\mathcal{V})^o$ , invariant under  $G \times G_F$  and with R-charge 1 and  $-1$ , respectively, such that

$$\mathfrak{Q}(\phi)^2 = W(\phi) \mathbb{1}_{\mathcal{V}} , \quad \bar{\mathfrak{Q}}(\bar{\phi})^2 = \bar{W}(\bar{\phi}) \mathbb{1}_{\mathcal{V}} . \quad (3.3.16)$$

These equations are called a *matrix factorization* of  $W$ , and  $\mathfrak{Q}$  is called a *tachyon profile*. With it we construct the super-connection

$$\mathcal{A}_\varphi = \rho_*(A_\varphi + i\sigma) + \frac{R}{2} - \frac{i}{2}\{\mathfrak{Q}, \bar{\mathfrak{Q}}\} + \frac{1}{2}(\psi_+ - \psi_-)^i \partial_i \mathfrak{Q} + \frac{1}{2}(\bar{\psi}_+ - \bar{\psi}_-)^i \partial_i \bar{\mathfrak{Q}} \quad (3.3.17)$$

and the boundary interaction is given by the supertrace

$$\text{Str}_{\mathcal{V}} \left[ \text{Pexp} \left( i \oint d\varphi \mathcal{A}_\varphi \right) \right] . \quad (3.3.18)$$

One can show that the SUSY variation of the Chan-Paton interaction cancels the Warner term [55]. The term  $\{\mathfrak{Q}, \bar{\mathfrak{Q}}\}$  represents a boundary potential.

At this point one should specify boundary conditions invariant under supersymmetry and compatible with the Euler-Lagrange equations. The issue is somehow delicate, and details can be found in [22–24]. The boundary conditions for vector multiplets include  $D_\theta\sigma = 0$  and  $F_{\mu\nu} = 0$ , therefore—compared to the  $S^2$  case—the BPS moduli space does not include the flux parameter  $\mathfrak{m}$ . For chiral multiplets there are two options: Neumann or Dirichlet.

Neumann boundary conditions include  $D_\theta\phi = D_\theta\bar{\phi} = 0$  and describe directions along the D-brane (in target space). Dirichlet boundary conditions include  $\phi = \bar{\phi} = 0$  and describe directions perpendicular to the D-brane. The BPS equations fix  $\sigma = D = \text{const}$ . The one-loop determinants are

$$\begin{aligned} Z_{\text{gauge}} &= \prod_{\alpha>0} i\alpha(\sigma) \sin(i\pi\alpha(\sigma)) \\ Z_{\text{matter}}^{\text{Neu}} &= \prod_{w\in\mathfrak{R}} \Gamma(-iw(\sigma)) , & Z_{\text{matter}}^{\text{Dir}} &= \prod_{w\in\mathfrak{R}} \frac{-2\pi i e^{\pi w(\sigma)}}{\Gamma(1+iw(\sigma))} . \end{aligned} \quad (3.3.19)$$

As usual, twisted masses are introduced by including an external vector multiplet with scalar component  $\tau$ , and R-charges are accounted by the shift  $\tau \rightarrow \tau + iq/2$ . The final localization formula is

$$Z_{D_2}(\mathcal{B}) = \frac{1}{|\text{Weyl}(G)|} \int \frac{d^N\sigma}{(2\pi)^N} z^{i\sigma} \text{Str}_{\mathcal{V}}[e^{-2\pi\sigma}] Z_{1\text{-loop}} \quad (3.3.20)$$

where  $z = e^{-2\pi\zeta + i\vartheta}$  is the exponential of the complexified FI parameter and  $N = \text{rank } G$ . As we have discussed before, the integration contour should be defined with care: it should be a deformation of the real contour  $\sigma \in \mathbb{R}^N$  which ensures convergence, and only for a very restricted set of branes can this be achieved for all values of  $z$  [24].

To clarify the role of the Chan-Paton interaction, let us give a simple example of D0-branes on  $\mathbb{C}^n$ . The model has  $n$  free chiral multiplets with flavor symmetry  $G_F = U(n)$ . To describe D0-branes one can simply impose Dirichlet boundary conditions in all directions, which does not break  $U(n)$ . There is no gauge sector and the partition function reads

$$Z_{D_2}(\text{D0}) = \prod_{j=1}^n \frac{-2\pi i e^{\pi\tau_j}}{\Gamma(1+i\tau_j)} \quad (3.3.21)$$

where  $\tau_j$  are the twisted masses (equivariant parameters). On the other hand, we can impose Neumann boundary conditions and construct a boundary interaction. To construct  $\mathcal{V}$  we take fermionic oscillators  $\{\eta_i, \bar{\eta}^j\} = \delta_i^j$  and a Clifford vacuum  $|0\rangle$  such that  $\bar{\eta}^j|0\rangle = 0$ : then we identify  $\mathcal{V}$  with the fermionic Fock space. We choose the tachyon profile

$$\mathfrak{Q}(\phi) = \phi^i \eta_i , \quad \bar{\mathfrak{Q}}(\bar{\phi}) = \bar{\phi}_j \bar{\eta}^j . \quad (3.3.22)$$

Clearly  $\mathfrak{Q}(\phi)^2 = \bar{\mathfrak{Q}}(\bar{\phi})^2 = 0$ . As  $\eta_i$  generate the Fock space and transform in the antifundamental representation of  $U(n)$ , one gets  $\text{Str}_{\mathcal{V}}[e^{-2\pi\tau}] = \prod_j (1 - e^{2\pi\tau_j})$ . Hence

$$Z_{D_2}(\text{D0}) = \prod_{j=1}^n (1 - e^{2\pi\tau_j}) \Gamma(-i\tau_j) = \prod_{j=1}^n \frac{-2\pi i e^{\pi\tau_j}}{\Gamma(1+i\tau_j)} . \quad (3.3.23)$$

We have indicated the boundary conditions in the same way as before, namely as D0, because they realize the same D-brane in the IR, and indeed the central charges agree. The boundary interaction creates a potential  $\{\mathfrak{Q}, \bar{\mathfrak{Q}}\} = \bar{\phi}^i \phi_i$  whose only minimum is at the origin, therefore at low energies it gives the same D-brane as by imposing Dirichlet boundary conditions. This

is a simple example of tachyon condensation [58]: one can describe all lower-dimensional branes using space-filling branes and a suitable boundary tachyon profile.

An important outcome of the localization computation is the expression for the D-brane central charge in large-volume geometric phases [24]:

$$Z_{D_2}(\mathcal{B}) = \int_X \hat{\Gamma}_X e^{B+i\omega/2\pi} \text{ch}(\mathcal{B}) . \quad (3.3.24)$$

Here  $X$  is the Kähler target manifold,  $\omega$  its Kähler class,  $B$  is the B-field and  $\text{ch}(\mathcal{B})$  is the Chern character of the complex of holomorphic vector bundles that specifies the brane (see [24] for details). Moreover  $\hat{\Gamma}_X$  is the *Gamma class* of the holomorphic tangent bundle of  $X$ , defined in the standard way in terms of the Chern roots by the function

$$\hat{\Gamma}(x) = \Gamma\left(1 - \frac{x}{2\pi i}\right) . \quad (3.3.25)$$

The formula was already known to mathematicians [59–61],<sup>15</sup> and the appearance of  $\hat{\Gamma}_X$  from the perturbative part of the NLSM path-integral has also been confirmed in [62]. A similar analysis for orientifold planes, as opposed to D-branes, has been done in [25] by studying the partition function of GLSMs on  $\mathbb{R}\mathbb{P}^2$ , and an expression for the central charge in large-volume geometric phases has been found.

### 3.3.4 $\Omega$ -deformed A-twist on the sphere

The modern “Coulomb branch localization” framework initiated by Pestun [14] can be applied to well-studied setups to obtain new interesting results. In particular, the canonical way to preserve supersymmetry on a curved manifold is to perform the so-called *topological twist* [63]: one turns on a background vector field that couples to the R-symmetry, equal and opposite to (some component of) the spin connection. On  $S^2$ , the A-type topological twist corresponds to one unit of magnetic flux for the vector R-symmetry  $R$ .<sup>16</sup> Thus, the A-twist [8] consists of a supersymmetric background for 2d  $\mathcal{N}=(2, 2)$  theories—different from the one we have discussed so far—preserving an  $\mathfrak{su}(1|1)_A$  subalgebra (the bosonic  $\mathfrak{u}(1)$  is the vector-like  $R$ ).

The interesting observables in the A-model [8, 46] are correlation functions of twisted chiral operators at non-coincident points (and their descendants). For gauge theories, they are gauge-invariant polynomials  $\mathcal{O}(\Sigma(p))$  of the field-strength twisted multiplet at points  $p$ . Those operators form a chiral ring, and the correlations functions are independent of the insertion points  $p$ . For theories that flow to NLSMs, the correlators equal the structure constants of the quantum cohomology ring of the target.

Localization has been applied to topologically twisted theories since the beginning, however in a form more similar to the “Higgs branch localization” in which the path-integral localizes to holomorphic maps in A-twisted NLSMs, and to point-like vortices in A-twisted GLSMs (see

<sup>15</sup>In particular notice that  $\hat{\Gamma}_X$  appears in place of the A-roof class  $\hat{A}_X$ .

<sup>16</sup>In the B-type twist one turns on one unit of flux for the axial R-symmetry. Since the two are equivalent, up to the  $\mathbb{Z}_2$  automorphisms that swaps multiplets with twisted multiplets, we shall consider the A-twist only.

*e.g.* [3, 64]). It turns out that Coulomb branch localization can be applied as well, producing compact and easily-calculable expressions for correlators in A-twisted gauge theories on  $S^2$  [9, 10] and yielding new results in non-Abelian theories.

The A-twisted background can be generalized into a sort of  $\Omega$ -deformed  $S^2$  [6]:<sup>17</sup> the superalgebra is still  $\mathfrak{su}(1|1)$ , however the  $\mathfrak{u}(1)$  bosonic subalgebra is a linear combination of  $R$  and rotations of  $S^2$  along an axis, controlled by a parameter  $\epsilon_\Omega$ . This deformation had already appeared in the mathematical literature, starting with the work of Givental [65]. Since rotations are part of the supersymmetry algebra, for  $\epsilon_\Omega \neq 0$  local operators can only be inserted at the North and South poles.

Localization can be applied to the more general  $\Omega$ -deformed A-twist as well [9, 10]. The BPS configurations are parametrized by the Cartan part of the complex scalar  $\sigma$  in the vector multiplet, as well as by diagonal magnetic fluxes  $\mathbf{m}$  in the coroot lattice  $\Gamma_t$ . For a theory with exponentiated complex FI term  $z = e^{-2\pi\zeta + i\vartheta}$  the classical action is

$$Z_{\text{cl}} = z^{\text{Tr } \mathbf{m}}. \quad (3.3.26)$$

The one-loop determinants for vector and chiral multiplets are

$$Z_{1\text{-loop}}^{\text{gauge}} = \prod_{\alpha > 0} \left[ \alpha(\sigma)^2 - \frac{\alpha(\mathbf{m})^2 \epsilon_\Omega^2}{4} \right], \quad Z_{1\text{-loop}}^{\text{chiral}} = \prod_{w \in \mathfrak{R}} \prod_{j = -\frac{|B_w|-1}{2}}^{\frac{|B_w|-1}{2}} \left( \frac{1}{w(\sigma) + j \epsilon_\Omega} \right)^{\text{sign } B_w} \quad (3.3.27)$$

where  $B_w = w(\mathbf{m}) - q_w + 1$ . Here  $q_w$  are the R-charges, which on the A-twisted background have to be chosen integral (because of Dirac quantization). Each operator insertion  $\mathcal{O}(\Sigma)$  brings an extra factor

$$\mathcal{O}\left(\sigma \pm \epsilon_\Omega \frac{\mathbf{m}}{2}\right).$$

The sign is  $\pm$  for insertions at the North/South pole, while for  $\epsilon_\Omega = 0$  operators can be inserted at any point. Then the localization formula is

$$\left\langle \prod_i \mathcal{O}_i \right\rangle_\Omega = \frac{1}{|\text{Weyl}(G)|} \sum_{\mathbf{m} \in \Gamma_t} \left[ \sum_{\sigma_* \in \mathfrak{M}_{\text{sing}}} \text{JK-Res}_{\sigma=\sigma_*}(\mathbf{Q}(\sigma_*), \eta) \prod_i \mathcal{O}_i Z_{\text{cl}} Z_{1\text{-loop}} + \text{bdry} \right]. \quad (3.3.28)$$

This formula has a similar flavor to the previous ones, however the integration is over a specific middle-dimensional contour in the complex  $\sigma$ -plane which effectively computes a weighted sum of residues of the integrand at the singular points  $\sigma_* \in \mathfrak{M}_{\text{sing}}$ . This particular contour is called the Jeffrey-Kirwan residue [66]: its importance for recent localization computations has been recognized in [67] in the context of the elliptic genus, and we will explain it in detail in section 3.4, including the notation used in (3.3.28). The JK residue depends on the choice of an auxiliary parameter  $\eta \in \mathfrak{t}$ , while the last term represents boundary contributions at infinity of the  $\sigma$ -plane. The sum of all contributions does not depend on  $\eta$ , however for certain choices the boundary contribution vanishes making the computation easier. More details can be found in [9, 10].

<sup>17</sup>A geometric way to understand this deformation is to start in 3d with an  $S^2$ -bundle over  $S^1$  in which  $S^2$  rotates by an angle  $\epsilon_\Omega$  as we wind around  $S^1$ . Then reduce on  $S^1$  to 2d [9].

### 3.3.5 General supersymmetric backgrounds

To study supersymmetric backgrounds more general than the  $\mathcal{N}=(2, 2)$  massive superalgebras on the round  $S^2$  or the A-twist, one can employ a systematic method developed by Festuccia and Seiberg in four dimensions [4], and adapted to the two-dimensional case in [6] (the method is summarized in Chapter 5). The method consists in coupling the flat-space supersymmetric theory of interest to some off-shell supergravity,<sup>18</sup> giving an expectation value to the bosonic fields in the graviton multiplet (including the metric and the auxiliary fields), and then taking a rigid limit in which the Newton constant goes to zero but the background remains fixed. In this limit, supersymmetry of the background is guaranteed by the vanishing of gravitino variations (possibly including gaugino variations, when they are part of the graviton multiplet).

The two-dimensional Lorentzian  $\mathcal{N}=(2, 2)$  superalgebra can have at most the R-symmetry group automorphism  $U(1)_{\text{left}} \times U(1)_{\text{right}} \simeq U(1)_R \times U(1)_A$ , *i.e.* a vector and an axial part. We restrict to theories with a vector-like R-symmetry, then the algebra admits a complex central charge  $Z$ .<sup>19</sup> On Euclidean flat space, the supersymmetry algebra is

$$\{Q_\alpha, \tilde{Q}_\beta\} = [2\gamma^\mu P_\mu + 2i\mathbb{P}_+ Z - 2i\mathbb{P}_- \tilde{Z}]_{\alpha\beta}, \quad \{Q_\alpha, Q_\beta\} = \{\tilde{Q}_\alpha, \tilde{Q}_\beta\} = 0, \quad (3.3.29)$$

where  $\mathbb{P}_\pm$  are the projectors on positive/negative chirality spinors. Tilded quantities are complex conjugate in Lorentzian signature, but are independent complexified quantities in Euclidean signature. To  $Q_\pm, \tilde{Q}_\pm$  we assign R-charges  $-1$  and  $+1$ , respectively.

Theories with an R-symmetry have an  $\mathcal{R}$ -multiplet<sup>20</sup> containing the conserved operators

$$\mathcal{R}_\mu : \quad (T_{\mu\nu}, S_{\alpha\mu}, \tilde{S}_{\alpha\mu}, j_\mu^R, j_\mu^Z, j_\mu^{\tilde{Z}}), \quad (3.3.30)$$

namely the stress tensor, the supersymmetry currents, and the currents for R-symmetry and central charges. Correspondingly, there exists an off-shell 2d supergravity—dimensional reduction of new minimal 4d supergravity [69–71]—whose graviton multiplet couples to the  $\mathcal{R}$ -multiplet. In a Wess-Zumino gauge it contains the fields

$$\mathcal{G}_\mu : \quad (g_{\mu\nu}, \Psi_{\alpha\mu}, \tilde{\Psi}_{\alpha\mu}, V_\mu, C_\mu, \tilde{C}_\mu), \quad (3.3.31)$$

namely the metric, the gravitinos and the gauge fields coupling to R- and central charges. The gauge fields  $V_\mu, C_\mu, \tilde{C}_\mu$  appear in covariant derivatives,  $D_\mu = \nabla_\mu - iqV_\mu + \frac{z}{2}\tilde{C}_\mu - \frac{\tilde{z}}{2}C_\mu$ , as well as through their field strengths. It is convenient to introduce the dual field strengths

$$\mathcal{H} = -i\varepsilon^{\mu\nu}\partial_\mu C_\nu, \quad \tilde{\mathcal{H}} = -i\varepsilon^{\mu\nu}\partial_\mu \tilde{C}_\nu. \quad (3.3.32)$$

<sup>18</sup>This step has the technical limitation that we need an off-shell formulation both for supergravity and the quantum field theory. Thus, it becomes difficult to apply the method when the number of supercharges is large.

<sup>19</sup>The  $\mathcal{N}=(2, 2)$  superalgebra admits two complex central charges, each breaking one of the two R-symmetries. A superconformal theory cannot have central charges.

<sup>20</sup>For a discussion of supercurrent multiplets in two dimensions see [68].

The gravitino variations—which will be referred to as the generalized Killing spinor (GKS) equations—are:

$$\begin{aligned} 0 &= \frac{1}{2}\delta\Psi_\mu = (\nabla_\mu - iV_\mu)\epsilon - \frac{1}{2}\begin{pmatrix} \mathcal{H} & 0 \\ 0 & \widetilde{\mathcal{H}} \end{pmatrix}\gamma_\mu\epsilon + \dots \\ 0 &= \frac{1}{2}\delta\widetilde{\Psi}_\mu = (\nabla_\mu + iV_\mu)\widetilde{\epsilon} - \frac{1}{2}\begin{pmatrix} \widetilde{\mathcal{H}} & 0 \\ 0 & \mathcal{H} \end{pmatrix}\gamma_\mu\widetilde{\epsilon} + \dots \end{aligned} \quad (3.3.33)$$

In the rightmost terms we used conventions in which the chirality matrix is  $\gamma_3 = \begin{pmatrix} 1 & 0 \\ 0 & -1 \end{pmatrix}$ . The two supersymmetry parameters  $\epsilon$ ,  $\widetilde{\epsilon}$  are complex Dirac spinors with R-charges 1,  $-1$  respectively, and no central charges. The dots represent terms that vanish when we set  $\Psi_\mu = \widetilde{\Psi}_\mu = 0$ . These equations have to be solved for the background fields as well as for  $\epsilon$ ,  $\widetilde{\epsilon}$ , and the number of solutions for the latter is the number of preserved supercharges.

From the off-shell supergravity transformations of fields (which can be found in [6]) one deduces the deformed supersymmetry algebra on a background:<sup>21</sup>

$$\begin{aligned} \{\delta_\epsilon, \delta_{\widetilde{\epsilon}}\} &= i\mathcal{L}_K - i\epsilon\mathbf{Q}\widetilde{\epsilon} \\ \{\delta_{\epsilon_1}, \delta_{\epsilon_2}\} &= \{\delta_{\widetilde{\epsilon}_1}, \delta_{\widetilde{\epsilon}_2}\} = 0 \end{aligned} \quad \mathbf{Q} = \begin{pmatrix} z - \sigma - \frac{r}{2}\mathcal{H} & 0 \\ 0 & \widetilde{z} - \widetilde{\sigma} - \frac{r}{2}\widetilde{\mathcal{H}} \end{pmatrix} \quad (3.3.34)$$

acting on a field  $\varphi_{q,z,\widetilde{z}}$  of fixed charges. The first term is a gauge-covariant Lie derivative, and it represents a translation along the vector field

$$K^\mu = \epsilon\gamma^\mu\widetilde{\epsilon}. \quad (3.3.35)$$

It follows from the GKS equations that such a vector field is Killing,  $\nabla_{(\mu}K_{\nu)} = 0$  and  $\mathcal{L}_K\mathcal{H} = \mathcal{L}_K\widetilde{\mathcal{H}} = 0$ , unless it vanishes. The second term is a mix of R-symmetry,  $Z/\widetilde{Z}$ -symmetry and gauge/global symmetry rotations.

Let us discuss some important solutions to (3.3.33) (the full set of solutions is presented in [6]). The first solution, known for a long time [8], is the *topological A-twist*:

$$V_\mu = -\frac{1}{4}\omega_\mu^{ab}\varepsilon_{ab}, \quad \epsilon = \begin{pmatrix} 0 \\ \epsilon_- \end{pmatrix}, \quad \widetilde{\epsilon} = \begin{pmatrix} \widetilde{\epsilon}_+ \\ 0 \end{pmatrix}, \quad \mathcal{H} = 0, \quad \widetilde{\mathcal{H}} = 0 \quad (3.3.36)$$

where  $\omega_\mu^{ab}$  is the spin connection and  $\epsilon_-, \widetilde{\epsilon}_+$  are constant.<sup>22</sup> This solution exists on any orientable Riemann surface  $\Sigma$ . There are two Killing spinors of opposite R-charge and chirality. On a compact Riemann surface of genus  $g$ , the background has  $(g-1)$  units of R-symmetry flux:  $\frac{1}{2\pi}\int_\Sigma dV = g-1$ . In particular the R-charge of all gauge-invariant operators should be quantized:

$$q(g-1) \in \mathbb{Z}. \quad (3.3.37)$$

<sup>21</sup>The contraction of spinor indices is  $\psi_\chi = \psi_\alpha\varepsilon^{\alpha\beta}\chi_\beta$ , namely the symbol  $\psi_\chi$  stands for  $\psi^T\begin{pmatrix} 0 & 1 \\ -1 & 0 \end{pmatrix}\chi$  in standard matrix notation. Moreover in this subsection  $\sigma$  indicates the full complex scalar in the vector multiplet, indicated by  $\sigma - i\eta$  before.

<sup>22</sup>More generally,  $\mathcal{H}$  could be an arbitrary function; this does not affect the supersymmetry algebra. We cannot turn on holonomies for  $V_\mu$  because  $\epsilon, \widetilde{\epsilon}$  (and the supercharges) would no longer be periodic and there would not be solutions.

The deformed supersymmetry algebra, in the absence of central charges, is simply<sup>23</sup>

$$\delta_\epsilon^2 = \delta_{\tilde{\epsilon}}^2 = 0, \quad \{\delta_\epsilon, \delta_{\tilde{\epsilon}}\} = 0. \quad (3.3.38)$$

Similarly, there is the  $\bar{A}$ -twist with  $1 - g$  units of R-symmetry flux. For  $g > 1$  these are the only two solutions.

For  $g = 0$  (topologically  $S^2$ ), if the metric has a rotational symmetry around an axis, there exists a one-parameter family of deformations called the  $\Omega$ -background in [6]. Let  $K^\mu$  be the Killing vector field, which for definiteness we can take as  $K = \partial_\varphi$  in the coordinates (3.2.1). Then

$$V_\mu = -\frac{1}{2}\omega_\mu^{12}, \quad \epsilon = \begin{pmatrix} \epsilon_\Omega K_{\hat{z}} \\ 1 \end{pmatrix} \epsilon_-, \quad \tilde{\epsilon} = \begin{pmatrix} 1 \\ -\epsilon_\Omega K_{\hat{z}} \end{pmatrix} \tilde{\epsilon}_+, \quad \mathcal{H} = -\frac{i}{2}\epsilon_\Omega \varepsilon^{\mu\nu} \partial_\mu K_\nu, \quad \tilde{\mathcal{H}} = 0, \quad (3.3.39)$$

where  $\epsilon_\Omega$  is a complex parameter. We have used the flat complex index that follows from  $e^{\hat{z}} = e^{\hat{1}} + ie^{\hat{2}}$ . In practice we can identify  $C_\mu = \frac{\epsilon_\Omega}{2} K_\mu$ . The background preserves two complex supercharges of opposite R-charge, and the deformed supersymmetry algebra is

$$\{\delta_\epsilon, \delta_{\tilde{\epsilon}}\} = i\epsilon_\Omega \mathcal{L}_K^{s'} + i\epsilon_- \tilde{\epsilon}_+ Z, \quad (3.3.40)$$

where  $\mathcal{L}_K^{s'}$  is a Lie derivative covariant with respect to gauge/flux rotations, not with respect to  $R$ ,  $Z$  and  $\tilde{Z}$ , but where the spin  $s$  is replaced by  $s' = s + \frac{g}{2}$ . This is the background that we considered in subsection 3.3.4.

On  $S^2$  there is a second class of interesting solutions with no net R-symmetry flux: they give *untwisted* backgrounds. The simplest case is that of a round  $S^2$ , then

$$V_\mu = 0, \quad \mathcal{H} = \tilde{\mathcal{H}} = \frac{i}{r}, \quad \nabla_\mu \epsilon = \frac{i}{2r} \gamma_\mu \epsilon, \quad \nabla_\mu \tilde{\epsilon} = \frac{i}{2r} \gamma_\mu \tilde{\epsilon}. \quad (3.3.41)$$

The spinors solve the Killing spinor equation: on the round  $S^2$  there are four solutions—two for  $\epsilon$  and two for  $\tilde{\epsilon}$ —so the number of preserved supersymmetries is maximal. With no central charges the deformed supersymmetry algebra is

$$\{\delta_\epsilon, \delta_{\tilde{\epsilon}}\} = i\mathcal{L}_K - \frac{\epsilon\tilde{\epsilon}}{2r} R, \quad (3.3.42)$$

and the Killing vectors  $K^\mu$  generate the  $\mathfrak{so}(3)$  isometry algebra of  $S^2$ . The full superalgebra is  $\mathfrak{su}(2|1)$ . Notice that the background is not the analytic continuation of a real background in Lorentzian signature, and this in general breaks reflection positivity. However, if the theory is superconformal, the auxiliary fields  $\mathcal{H}$ ,  $\tilde{\mathcal{H}}$  couple to redundant operators and reflection positivity is recovered.

As described in subsection 3.2.1, on more general topological spheres with only  $U(1)$  isometry one can still preserve two supercharges of opposite R-charge without twisting. Considering for definiteness the metric  $ds^2 = f(\theta)^2 d\theta^2 + r^2 \sin^2 \theta d\varphi^2$ , the background is

$$V = \frac{1}{2} \left(1 - \frac{r}{f}\right) d\varphi, \quad \epsilon = e^{\frac{i}{2}\theta\gamma_1} e^{\frac{i}{2}\varphi} \begin{pmatrix} \epsilon_0 \\ 0 \end{pmatrix}, \quad \tilde{\epsilon} = e^{\frac{i}{2}\theta\gamma_1} e^{-\frac{i}{2}\varphi} \begin{pmatrix} 0 \\ \tilde{\epsilon}_0 \end{pmatrix}, \quad \mathcal{H} = \tilde{\mathcal{H}} = \frac{i}{f} \quad (3.3.43)$$

<sup>23</sup>With central charges one finds the  $\mathfrak{su}(1|1)$  superalgebra  $\{\delta_\epsilon, \delta_{\tilde{\epsilon}}\} = i\epsilon_- \tilde{\epsilon}_+ (z - \sigma)$ .

with constant  $\epsilon_0, \tilde{\epsilon}_0$ .

One last example we want to mention is that of  $\mathcal{N}=(2, 2)$  theories with both vector and axial R-symmetries, placed on a flat  $T^2$ . In this case one can turn on a flat connection for, say, the left-moving R-symmetry  $U(1)_{\text{left}}$ . As a result the left-moving supercharges are lifted, however there remain the two right-moving supercharges with opposite charge under  $U(1)_{\text{right}}$ . This case is discussed in [section 3.4](#).

Supersymmetric actions on the curved backgrounds are constructed in a way similar to flat space: the supersymmetry variations of gauge-invariant D-terms and F-terms are total derivatives, therefore their spacetime integrals are supersymmetric invariants. The top D-term component of a neutral general supermultiplet with  $q = 0$  can be used to construct the super-Yang-Mills and matter kinetic actions,  $\mathcal{L}_D = D$ . For instance from the D-term of  $-\frac{1}{2}\tilde{\Phi}e^{-2\mathcal{V}}\Phi$  one obtains the kinetic action of a chiral multiplet  $\Phi$ :

$$\begin{aligned} \mathcal{L}_\Phi = & D_\mu \tilde{\phi} D^\mu \phi + \tilde{\phi} D \phi + \frac{1}{2} \left( \frac{q}{2} R_s + \mathcal{H} \tilde{z} + \tilde{\mathcal{H}} z \right) \tilde{\phi} \phi + \frac{1}{2} \tilde{\phi} \{ \mathbf{Q}, \tilde{\mathbf{Q}} \} \phi \\ & - \tilde{F} F + i \tilde{\psi} \gamma^\mu D_\mu \psi + i \tilde{\psi} \tilde{\mathbf{Q}} \psi + i \sqrt{2} \tilde{\psi} \tilde{\lambda} \phi + i \sqrt{2} \tilde{\phi} \lambda \psi \end{aligned} \quad (3.3.44)$$

where  $R_s$  is the scalar curvature. For NLSMs one uses the D-term of the Kähler potential  $K(\tilde{\Phi}, \Phi)$ . From the D-term of a gauge-invariant multiplet whose lowest component is  $\frac{1}{2} \text{Tr} \tilde{\sigma} \sigma$  one obtains the SYM action

$$\begin{aligned} \mathcal{L}_\mathcal{V} = & \frac{1}{2} \left( F_{12} - \frac{1}{2} \tilde{\mathcal{H}} \sigma + \frac{1}{2} \mathcal{H} \tilde{\sigma} \right)^2 + \frac{1}{2} D_\mu \tilde{\sigma} D^\mu \sigma + \frac{1}{8} [\sigma, \tilde{\sigma}]^2 \\ & + i \tilde{\lambda} \gamma^\mu D_\mu \lambda - i \tilde{\lambda} \begin{pmatrix} [\tilde{\sigma}, \cdot] & 0 \\ 0 & [\sigma, \cdot] \end{pmatrix} \lambda - \frac{1}{2} \left( D + \frac{1}{2} \tilde{\mathcal{H}} \sigma + \frac{1}{2} \mathcal{H} \tilde{\sigma} \right)^2 \end{aligned} \quad (3.3.45)$$

with trace implicit. The top F-term component of a neutral chiral multiplet with  $q = 2$ ,  $z = \tilde{z} = 0$  gives superpotential interactions,

$$\mathcal{L}_W = F_W + \tilde{F}_W, \quad (3.3.46)$$

where  $F_W$  is the F-term component of the superpotential  $W(\Phi)$ :<sup>24</sup>

$$F_W = \frac{\partial W}{\partial \phi_i} F_i - \frac{1}{2} \frac{\partial^2 W}{\partial \phi_i \partial \phi_j} \psi_j \psi_i, \quad \tilde{F}_W = \frac{\partial \tilde{W}}{\partial \tilde{\phi}_i} \tilde{F}_i + \frac{1}{2} \frac{\partial^2 \tilde{W}}{\partial \tilde{\phi}_i \partial \tilde{\phi}_j} \tilde{\psi}_j \tilde{\psi}_i. \quad (3.3.47)$$

The top component of a twisted chiral multiplet with  $q = z = \tilde{z} = 0$  (called twisted F-term or G-term) can be corrected to give supersymmetric actions, since  $\delta(G - i\tilde{\mathcal{H}}\omega)$  is a total derivative (here  $\omega$  is the lowest component of a twisted chiral multiplet). The twisted superpotential action is then

$$\mathcal{L}_\mathcal{W} = G_\mathcal{W} - i\tilde{\mathcal{H}}\mathcal{W}(\omega) + \tilde{G}_\mathcal{W} + i\mathcal{H}\tilde{\mathcal{W}}(\tilde{\omega}), \quad (3.3.48)$$

---

<sup>24</sup>Integrating out  $F_i, \tilde{F}_i$  one obtains the real positive potential  $\sum_i |\frac{\partial W}{\partial \phi_i}|^2$ . Alternatively, to keep the fields  $F_i, \tilde{F}_i$  one should redefine them with an  $i$ , then the kinetic action is positive-definite and the superpotential action is imaginary.

where

$$G_{\mathcal{W}} = \frac{\partial \mathcal{W}}{\partial \omega_i} G_i - \frac{1}{2} \frac{\partial^2 \mathcal{W}}{\partial \omega_i \partial \omega_j} \eta_j \eta_i \quad (3.3.49)$$

is the G-term of the twisted superpotential  $\mathcal{W}$ .

### 3.4 Elliptic genera of $\mathcal{N}=(2, 2)$ and $\mathcal{N}=(0, 2)$ theories

We discuss now the Euclidean path-integral of two-dimensional  $\mathcal{N}=(2, 2)$  supersymmetric theories on a torus  $T^2$ . This quantity, called the *elliptic genus*, was first introduced in the physics literature in [72–74] in the context of free orbifolds and in [75, 76] in the context of non-linear sigma models. As usual, the path-integral on a circle computes the trace over a Hilbert space of states, and we start from such a Hamiltonian definition:

$$Z_{T^2}(\tau, z, u) = \text{Tr}_{\text{RR}} (-1)^F q^{H_L} \bar{q}^{H_R} y^J \prod_a x_a^{K_a} . \quad (3.4.1)$$

The trace is over the Ramond sector of the Hilbert space of the theory on a spatial circle, *i.e.* one takes periodic boundary conditions for fermions. Then  $F$  is the fermion number, we define the parameters

$$q = e^{2\pi i \tau} , \quad y = e^{2\pi i z} , \quad x_a = e^{2\pi i u_a} , \quad (3.4.2)$$

and  $q$  specifies the complex structure of a torus  $w \cong w + 1 \cong w + \tau$ , with  $\tau = \tau_1 + i\tau_2$ .  $H_L$  and  $H_R$  are the left- and right-moving Hamiltonians respectively, defined in Euclidean signature in terms of Hamiltonian and momentum as  $2H_L = H + iP$ ,  $2H_R = H - iP$ . We assume that the theory has a left-moving  $U(1)$  R-symmetry  $J$  (which might be discrete if the theory is not conformal) and a flavor group  $K$  (with Cartan generators  $K_a$ ). Their fugacities are  $y$  and  $x_a$ . Given a charge vector  $\rho^a$ , we use the notation  $x^\rho = \prod_a x_a^{\rho^a} = e^{2\pi i \rho^a u_a}$ . We also write  $\rho(u) = \rho^a u_a$ , considering  $\rho \in \mathfrak{k}^*$  and  $u \in \mathfrak{k}$ , where  $\mathfrak{k}$  is the Cartan algebra of the flavor symmetry group  $K$ . The elliptic genus with  $u_a \neq 0$  is sometimes called the equivariant elliptic genus, while setting  $z = u_a = 0$  the elliptic genus reduces to the Witten index. The  $q \rightarrow 0$  limit of the elliptic genus is called the  $\chi_y$  genus.

Physically, the elliptic genus is interesting because it detects spontaneous supersymmetry breaking: if supersymmetry is broken, then the Witten index is zero (although the opposite is not necessarily true) [77]. Moreover, if the theory is superconformal the operators  $H_L, H_R, J$  equal the zero-mode generators  $L_0, \bar{L}_0, J_0$  of the superconformal algebra<sup>25</sup> and the elliptic genus is equal to the *superconformal index*, which counts superconformal primary operators in flat space.

Mathematically, the elliptic genus of a NLSM with complex target manifold  $X$  is a topological invariant—related to the elliptic cohomology of  $X$  [75]—equal to the Euler characteristic of a specific infinite-dimensional formal vector space  $E_{q,y}$ . The Witten index equals the Euler number of  $X$ . See *e.g.* [80].

<sup>25</sup>When not uniquely fixed, *e.g.* by the superpotential, the superconformal R-symmetries can be determined through the *c*-extremization principle of [78, 79].

If the theory has a discrete spectrum (at least in the equivariant sense), then the elliptic genus is a holomorphic function of  $q$  because the contributions from states with  $H_R \neq 0$  cancels between pairs of states with opposite values of  $(-1)^F$ . The genus has very interesting modular transformation properties as well. Since the spectrum of the Ramond sector is invariant under charge conjugation:

$$Z_{T^2}(\tau, z, u) = Z_{T^2}(\tau, -z, -u) . \quad (3.4.3)$$

When the R-symmetry is non-anomalous and the theory flows to an IR fixed point, the modular transformations of the elliptic genus are:

$$Z_{T^2}\left(\frac{a\tau + b}{c\tau + d}, \frac{z}{c\tau + d}, \frac{u}{c\tau + d}\right) = \exp\left[\frac{\pi ic}{c\tau + d}\left(\frac{c_L}{3}z^2 - 2\mathcal{A}_L^a u_a z\right)\right] Z_{T^2}(\tau, z, u) \quad (3.4.4)$$

for  $\begin{pmatrix} a & b \\ c & d \end{pmatrix} \in SL(2, \mathbb{Z})$ . Here  $c_L$  is the left-moving IR central charge, proportional to the 't Hooft anomaly of  $J$ , while  $\mathcal{A}_L^a$  is the 't Hooft anomaly between  $J$  and  $K_a$ :

$$c_L = -3 \sum_{\text{fermions}} \gamma_3 J^2, \quad \mathcal{A}_L^a = \sum_{\text{fermions}} \gamma_3 J K_a . \quad (3.4.5)$$

The sums are taken over all fermions in the theory, and  $\gamma_3$  is the chirality matrix that we take positive (negative) on right (left) movers. For a NLSM on a Calabi-Yau manifold  $X$  of complex dimension  $d = c_L/3$ , the elliptic genus is a Jacobi form of weight zero and index  $d/2$ .

Later on, the elliptic genus of Gepner models was computed using the known characters of  $\mathcal{N}=2$  superconformal algebras [81, 82]. Then it was realized that the elliptic genus of Landau-Ginzburg models can be computed by localization [83], which led to a formula for the elliptic genus of Gepner models using the orbifold Landau-Ginzburg description [84–87]. In this review we will be mostly concerned with the more recent computation of the elliptic genus of gauge theories [67, 88, 89] with localization techniques. The resulting formula agrees with that of Landau-Ginzburg models in case the gauge group is trivial, and with known mathematical results of the elliptic genus of complete intersections in toric varieties [90, 91] when the theory has a smooth geometric phase.

It turns out that one can equally well consider the elliptic genus of theories with only  $\mathcal{N}=(0, 2)$  supersymmetry. Mathematically, they describe more general bundles than the tangent bundle on  $X$ . Their equivariant elliptic genus is defined as

$$Z_{T^2}(\tau, u) = \text{Tr}_R (-1)^F q^{H_L} \bar{q}^{H_R} \prod_a x_a^{K_a} . \quad (3.4.6)$$

If the theory has a low-energy description as a NLSM with target a holomorphic vector bundle over a compact complex manifold, as in the models in [92], the elliptic genus encodes the Euler characteristic of that vector bundle [93].<sup>26</sup>

---

<sup>26</sup>Setting  $u_a = 0$ , the equivariant elliptic genus reduces to the partition function of the chiral CFT associated to the half-twisted model.

If the theory has discrete spectrum, the elliptic genus is a holomorphic function of  $\tau$  with the following modular transformation properties:

$$Z_{T^2}\left(\frac{a\tau + b}{c\tau + d}, \frac{u}{c\tau + d}\right) = \epsilon(a, b, c, d)^{c_R - c_L} \exp\left[-\frac{\pi i c}{c\tau + d} \mathcal{A}^{ab} u_a u_b\right] Z_{T^2}(\tau, u) \quad (3.4.7)$$

for  $\begin{pmatrix} a & b \\ c & d \end{pmatrix} \in SL(2, \mathbb{Z})$ . The multiplier system  $\epsilon(a, b, c, d)$  is a phase, independent of  $u_a$ , universally defined by

$$\frac{\eta\left(\frac{a\tau + b}{c\tau + d}\right)}{\theta_1\left(\frac{a\tau + b}{c\tau + d} \middle| \frac{u}{c\tau + d}\right)} = \epsilon(a, b, c, d) e^{-\frac{i\pi c}{c\tau + d} x^2} \frac{\eta(\tau)}{\theta_1(\tau|u)}. \quad (3.4.8)$$

It is through  $\epsilon$  that the gravitational anomaly shows up. In the theories under consideration,  $c_R - c_L$  equals three times the number of right-moving minus left-moving fermions, while  $\mathcal{A}^{ab}$  are the flavor 't Hooft anomalies:

$$c_R - c_L = 3 \sum_{\text{fermions}} \gamma_3, \quad \mathcal{A}^{ab} = \sum_{\text{fermions}} \gamma_3 K_a K_b. \quad (3.4.9)$$

One could also consider alternative elliptic genera where the trace is taken in the Neveu-Schwartz sector (on one or both sides), as in [88]. The resulting functions are all equivalent, because easily related by spectral flow.

**The Jeffrey-Kirwan residue.** The main focus in this review is the computation of the elliptic genera of gauge theories, through localization techniques. Such a computation has been done in [67, 88, 89] for the simplest theories, building on [83, 94], and then generalized in many ways, for instance in [95–98]. In particular, the expression found in [67, 89] involves a particular type of higher-dimensional residue operation called the *Jeffrey-Kirwan* (JK) *residue* defined in [66] and motivated by [99]. Schematically:

$$Z_{T^2} = \sum_{u_*} \text{JK-Res}_{u=u_*} Z_{1\text{-loop}}(u)$$

where  $Z_{1\text{-loop}}$  is a meromorphic top-form on an  $r$ -dimensional complex manifold ( $r$  is the rank of the gauge group), and the sum is over all singular points. The JK residue depends on a choice of vector  $\eta$ , however the total sum does not (and the parameter  $\eta$  is just auxiliary). The details are presented below.

Such a residue operation arises from a careful treatment of the bosonic and fermionic zero-modes in the problem. It has then been realized that very similar systems of zero-modes arise in many other localization contexts, for instance for the Witten index in one dimension [100, 101], for the Nekrasov partition function [102] in four [103] and five [104] dimensions, for the topological twist in two dimensions [9, 10, 26] and its higher-dimensional generalizations [9]. In all these cases, the result of localization for gauge theories takes the form of a JK residue, possibly with extra boundary contributions.

### 3.4.1 Multiplets, Lagrangians and supersymmetry

In the path-integral formulation, the elliptic genus equals the Euclidean path-integral of the theory on a flat  $T^2$ , in the presence of flat connections  $A^R$  and  $A^{\text{flav}}$  for the R- and flavor symmetries, respectively, coupled to the R- and flavor symmetry currents:

$$z = \oint_t A^R - \tau \oint_s A^R, \quad u_a = \oint_t A^{a\text{-th flav}} - \tau \oint_s A^{a\text{-th flav}}, \quad (3.4.10)$$

where  $t, s$  are the temporal and spatial cycles.<sup>27</sup> This is equivalent to specifying non-trivial boundary conditions twisted by the R- and flavor charges, along both the spatial and temporal cycles. Since the background is flat, the actions are just the standard ones. In the  $\mathcal{N}=(2, 2)$  case we have already discussed multiplets, supersymmetry transformations and actions for gauge theories in [section 3.2](#) and [section 3.3](#). So, let us move the  $\mathcal{N}=(0, 2)$  case.

We are interested in  $\mathcal{N}=(0, 2)$  gauge theories. The reader can consult [\[3, 92, 105\]](#) for more details. Using the complex coordinate  $w$ , the supersymmetry parameters satisfy  $\gamma^w \epsilon = \gamma^{\bar{w}} \bar{\epsilon} = 0$ . It is convenient to write spinors in components, in particular the SUSY parameters are  $\epsilon^+, \bar{\epsilon}^+$ . We consider theories formulated in terms of chiral, Fermi and vector multiplets.

First we have a chiral multiplet  $\Phi = (\phi, \bar{\phi}, \psi^-, \bar{\psi}^-)$  with variations

$$\begin{aligned} \delta\phi &= -i\bar{\epsilon}^+ \psi^- & \delta\psi^- &= 2i\epsilon^+ D_{\bar{w}}\phi \\ \delta\bar{\phi} &= -i\epsilon^+ \bar{\psi}^- & \delta\bar{\psi}^- &= 2i\bar{\epsilon}^+ D_{\bar{w}}\bar{\phi}. \end{aligned} \quad (3.4.11)$$

Second we have a Fermi multiplet  $\Lambda = (\psi^+, \bar{\psi}^+, G, \bar{G})$  with variations

$$\begin{aligned} \delta\psi^+ &= \bar{\epsilon}^+ G + i\epsilon^+ E & \delta G &= 2\epsilon^+ D_{\bar{w}}\psi^+ - \epsilon^+ \psi_E^- \\ \delta\bar{\psi}^+ &= \epsilon^+ \bar{G} + i\bar{\epsilon}^+ \bar{E} & \delta\bar{G} &= 2\bar{\epsilon}^+ D_{\bar{w}}\bar{\psi}^+ - \bar{\epsilon}^+ \bar{\psi}_E^-. \end{aligned} \quad (3.4.12)$$

Here  $\mathcal{E}(\Phi_i) = (E, \bar{E}, \psi_E^-, \bar{\psi}_E^-)$  is a chiral multiplet, holomorphic function of the fundamental chiral multiplets in the theory, and it is part of the definition of  $\Lambda$ . Notice that  $E = E(\phi_i)$  and its fermionic partner is  $\psi_E^- = \sum_i \psi_i^- \partial E / \partial \phi_i$ . Third we have a vector multiplet  $V = (A_\mu, \lambda^+, \bar{\lambda}^+, D)$  with variations

$$\begin{aligned} \delta A_w &= \frac{1}{2}(\epsilon^+ \bar{\lambda}^+ - \bar{\epsilon}^+ \lambda^+) & \delta \bar{\lambda}^+ &= \bar{\epsilon}^+ (-D - iF_{12}) & \delta(-D - iF_{12}) &= 2\epsilon^+ D_{\bar{w}} \bar{\lambda}^+ \\ \delta A_{\bar{w}} &= 0 & \delta \lambda^+ &= \epsilon^+ (-D + iF_{12}) & \delta(-D + iF_{12}) &= 2\bar{\epsilon}^+ D_{\bar{w}} \lambda^+. \end{aligned} \quad (3.4.13)$$

Comparing with [\(3.4.12\)](#), notice that the fields in the second and third column form a Fermi multiplet  $\Upsilon = (\bar{\lambda}^+, \lambda^+, -D - iF_{12}, -D + iF_{12})$  with  $\mathcal{E} = 0$ .

The supersymmetric action for chiral multiplets comes from the Lagrangian

$$\mathcal{L}_\Phi = D_\mu \bar{\phi} D^\mu \phi + i\bar{\phi} D\phi + 2\bar{\psi}^- D_w \psi^- - \bar{\psi}^- \lambda^+ \phi + \bar{\phi} \bar{\lambda}^+ \psi^-, \quad (3.4.14)$$

---

<sup>27</sup>Choosing a constant connection  $A_\mu^R$ , we have  $z = (-2i\tau_2) A_\mu^R$  and similarly for the flavor holonomies.

for Fermi multiplets we have

$$\mathcal{L}_\Lambda = -2\bar{\psi}^+ D_{\bar{w}}\psi^+ + \bar{E}E + \bar{G}G + \bar{\psi}^+\psi_E^- - \bar{\psi}_E^-\psi^+, \quad (3.4.15)$$

and for vector multiplets we have

$$\mathcal{L}_\Upsilon = \text{Tr} \left[ F_{12}^2 + D^2 - 2\bar{\lambda}^+ D_{\bar{w}}\lambda^+ \right]. \quad (3.4.16)$$

The last one equals the Lagrangian for the Fermi multiplet  $\Upsilon$ . Interactions are specified by holomorphic functions  $J^a(\phi)$  of the chiral multiplets (and anti-holomorphic functions  $\bar{J}^a(\bar{\phi})$  of their partners), where  $a$  parametrizes the Fermi multiplets in the theory:

$$\mathcal{L}_J = \sum_a \left( iG_a J^a - \psi_a^+ \psi_J^{-a} \right), \quad \mathcal{L}_{\bar{J}} = \sum_a \left( i\bar{G}_a \bar{J}^a - \bar{\psi}_a^+ \bar{\psi}_{\bar{J}}^{-a} \right). \quad (3.4.17)$$

Their supersymmetry variation is a total derivative as long as

$$\sum_a E_a(\phi) J^a(\phi) = 0. \quad (3.4.18)$$

It turns out that all these actions are  $\mathcal{Q}$ -exact. This reflects the fact that the elliptic genus is a ‘‘topological invariant’’, unaffected by continuous deformations of the parameters in the theory. Defining the anticommuting supercharge  $\mathcal{Q}$  by using commuting spinor parameters and choosing them  $\epsilon^+ = \bar{\epsilon}^+ = 1$ , the action of  $\mathcal{Q}$  is then immediately read off from the supersymmetry variations and one finds, up to total derivatives:

$$\begin{aligned} \mathcal{L}_\Phi &= \mathcal{Q} \left( 2i\bar{\phi} D_w \psi^- - i\bar{\phi} \lambda^+ \phi \right), & \mathcal{L}_\Lambda &= \mathcal{Q} \left( \bar{\psi}^+ G - i\bar{E} \psi^+ \right) \\ \mathcal{L}_J &= \mathcal{Q} \left( \sum_a i\psi_a^+ J^a \right), & \mathcal{L}_\Upsilon &= -\mathcal{Q} \text{Tr} \left( \lambda^+ (D + iF_{12}) \right). \end{aligned} \quad (3.4.19)$$

The  $\mathcal{N}=(2,2)$  theories can be regarded as special cases of  $\mathcal{N}=(0,2)$ , in which the left-moving R-symmetry appears as a flavor symmetry. To reduce from  $(2,2)$  to  $(0,2)$  supersymmetry, we define projectors  $P_\pm = (1 \pm \gamma_3)/2$ . Then the chiral multiplet  $\Phi_{(2,2)}$  splits into a chiral multiplet  $\Phi = (\phi, \bar{\phi}, P_- \psi, P_- \bar{\psi})$  and a Fermi multiplet  $\Lambda = (P_+ \psi, P_+ \bar{\psi}, F, \bar{F})$ . The vector multiplet  $V_{(2,2)}$  splits into a vector multiplet  $V$  and an adjoint chiral multiplet  $\Sigma = (\sigma, \bar{\sigma}, P_- \lambda, P_- \bar{\lambda})$ . If  $\Phi_{(2,2)}$  is charged under  $V_{(2,2)}$ , then its Fermi component  $\Lambda$  has  $\mathcal{E} = \Sigma\Phi$  (where  $\Sigma$  acts in the correct representation). Superpotential interactions  $W(\Phi_{(2,2)})$  become interactions  $J^a(\phi) = \partial W / \partial \phi_a$ . A twisted chiral multiplet  $Y_{(2,2)}$  (which must be neutral) splits into a chiral and a Fermi multiplet. In particular the twisted chiral multiplet  $\Sigma_{(2,2)}$  constructed out of  $V_{(2,2)}$  splits into  $\Upsilon$  and  $\Sigma$ . A twisted superpotential  $\widetilde{W}(\Sigma_{(2,2)})$  becomes an interaction  $J^\Upsilon(\sigma) = \partial \widetilde{W} / \partial \sigma$ , and a complexified Fayet-Iliopoulos term is simply a constant  $J^\Upsilon = \frac{\theta}{2\pi} + i\zeta$ .

### 3.4.2 The localization formula and the JK residue

We will first present the formula for the elliptic genus obtained from localization in [67, 89], and then outline its derivation in the next subsection.

The localization computation proceeds along the same steps as in [section 3.2](#). First, the moduli space of BPS configurations is parametrized by flat  $G$ -connection on  $T^2$  modulo gauge transformations, where  $G$  is the gauge group. For simplicity, we will assume that the non-Abelian part of  $G$  is connected and simply-connected.<sup>28</sup> Let  $\mathfrak{h}$  be the Cartan algebra of  $G$ , then the Cartan torus of  $G$  can be identified with  $\mathfrak{h}/\Gamma_{\mathfrak{h}}$  where  $\Gamma_{\mathfrak{h}}$  is the coroot lattice. We define

$$\mathfrak{M} = \mathfrak{h}_{\mathbb{C}}/(\Gamma_{\mathfrak{h}} + \tau\Gamma_{\mathfrak{h}}) , \quad (3.4.20)$$

then the moduli space is  $\mathfrak{M}/\text{Weyl}(G)$ . We parametrize the complexified Cartan algebra  $\mathfrak{h}_{\mathbb{C}}$  by  $u_a$ , then  $\mathfrak{M}$  is the product of  $r$  copies of  $T^2$  where  $r = \text{rank } G$ . Similarly, we introduce variables  $\xi_b$  on the complexified Cartan algebra of the flavor group  $K$  and fugacities  $\zeta_b = e^{2\pi i \xi_b}$ .

Second, the one-loop determinants produce a meromorphic  $(r, 0)$ -form  $Z_{1\text{-loop}}(\tau, z, u, \xi)$ . In the  $\mathcal{N}=(2, 2)$  case, for a gauge theory with chiral multiplets transforming in the (possibly reducible) representation  $\mathfrak{R}$ , such a form is

$$Z_{1\text{-loop}} = \left( \frac{2\pi\eta(q)^3}{\theta_1(q, y^{-1})} \right)^r \prod_{\alpha \in G} \frac{\theta_1(q, x^\alpha)}{\theta_1(q, y^{-1}x^\alpha)} \prod_{\rho \in \mathfrak{R}} \frac{\theta_1(q, y^{R_\rho/2-1}\zeta^{K_\rho}x^\rho)}{\theta_1(q, y^{R_\rho/2}\zeta^{K_\rho}x^\rho)} du_1 \cdots du_r . \quad (3.4.21)$$

The first product is over the roots  $\alpha$  of  $G$ , while the second one is over the weights  $\rho$  of  $\mathfrak{R}$ . The elliptic Dedekind and Jacobi functions are defined as

$$\eta(q) = q^{\frac{1}{24}} \prod_{n=1}^{\infty} (1 - q^n) , \quad \theta_1(q, y) = -iq^{\frac{1}{8}}y^{\frac{1}{2}} \prod_{n=1}^{\infty} (1 - q^n)(1 - yq^n)(1 - y^{-1}q^{n-1}) . \quad (3.4.22)$$

Finally,  $R_\rho/2$  is the left-moving R-charge (if the axial R-charge is zero, then  $R_\rho$  is the vector R-charge) and  $K_\rho$  is the flavor weight of the chiral multiplet associated to the weight  $\rho$ . These charges are constrained by superpotential interactions, and this is the only place where the superpotential appears. If extra (neutral) twisted chiral multiplets  $\Sigma_c$  with axial R-charge  $R_c^{(A)}$  are present, one should also include the factor

$$\prod_c \frac{\theta_1(q, y^{-R_c^{(A)}/2+1})}{\theta_1(q, y^{-R_c^{(A)}/2})} .$$

In the  $\mathcal{N}=(0, 2)$  case, for a theory with chiral multiplets in representation  $\mathfrak{R}_{\text{chiral}}$  and Fermi multiplets in representation  $\mathfrak{R}_{\text{Fermi}}$ , the meromorphic form is

$$Z_{1\text{-loop}} = \left( \frac{2\pi\eta(q)^2}{i} \right)^r \prod_{\alpha \in G} i \frac{\theta_1(q, x^\alpha)}{\eta(q)} \prod_{\rho \in \mathfrak{R}_{\text{chiral}}} \frac{i\eta(q)}{\theta_1(q, \zeta^{K_\rho}x^\rho)} \prod_{\rho \in \mathfrak{R}_{\text{Fermi}}} i \frac{\theta_1(q, \zeta^{K_\rho}x^\rho)}{\eta(q)} du_1 \cdots du_r . \quad (3.4.23)$$

Note that the only difference between  $u$  and  $\xi$  is that  $u$  will be integrated over. We will sometimes keep  $\xi$  implicit in the following formulæ.

<sup>28</sup>Non-simply-connected and disconnected groups can be treated as well, see *e.g.* [89].

The meromorphic form  $Z_{1\text{-loop}}$  has poles in  $u$ , along hyperplanes corresponding to all chiral and off-diagonal vector multiplets for  $\mathcal{N}=(2,2)$ , and to chiral multiplets for  $\mathcal{N}=(0,2)$ . Each of those multiplets introduces a singular hyperplane  $H_i \subset \mathfrak{M}$ . We will use the index  $i$  for them, and call  $Q_i \in \mathfrak{h}^*$  the weight of the multiplet under the gauge group. For the different types of multiplets we have:

$$\begin{aligned} \text{vector}_{(2,2)} : H_i &= \left\{ \begin{array}{l} -z + Q_i(u) = 0 \pmod{\mathbb{Z} + \tau\mathbb{Z}} \end{array} \right\}, & Q_i &= \alpha \\ \text{chiral}_{(2,2)} : H_i &= \left\{ \begin{array}{l} \frac{R_i}{2}z + Q_i(u) + K_i(\xi) = 0 \pmod{\mathbb{Z} + \tau\mathbb{Z}} \end{array} \right\}, & Q_i &= \rho \\ \text{chiral}_{(0,2)} : H_i &= \left\{ \begin{array}{l} Q_i(u) + K_i(\xi) = 0 \pmod{\mathbb{Z} + \tau\mathbb{Z}} \end{array} \right\}, & Q_i &= \rho. \end{aligned} \tag{3.4.24}$$

Note that a single  $H_i$  can contain multiple parallel disconnected hyperplanes. We denote by  $\mathbf{Q} = \{Q_i\}$  the set of all charge covectors. Then we define

$$\mathfrak{M}_{\text{sing}} = \bigcup_i H_i \tag{3.4.25}$$

in  $\mathfrak{M}$ , and we denote by  $\mathfrak{M}_{\text{sing}}^* \subset \mathfrak{M}_{\text{sing}}$  the set of isolated points in  $\mathfrak{M}$  where at least  $r$  linearly-independent hyperplanes meet:

$$\mathfrak{M}_{\text{sing}}^* = \left\{ u_* \in \mathfrak{M} \mid \text{at least } r \text{ linearly independent } H_i \text{'s meet at } u_* \right\}. \tag{3.4.26}$$

Given  $u_* \in \mathfrak{M}_{\text{sing}}^*$ , we denote by  $\mathbf{Q}(u_*)$  the set of charges of the hyperplanes meeting at  $u_*$ :

$$\mathbf{Q}(u_*) = \{Q_i \mid u_* \in H_i\}. \tag{3.4.27}$$

Next, one has to choose a generic<sup>29</sup> non-zero  $\eta \in \mathfrak{h}^*$ . Then, the elliptic genus is given by the formula:<sup>30</sup>

$$Z_{T^2}(\tau, z, \xi) = \frac{1}{|\text{Weyl}(G)|} \sum_{u_* \in \mathfrak{M}_{\text{sing}}^*} \text{JK-Res}_{u=u_*}(\mathbf{Q}(u_*), \eta) Z_{1\text{-loop}}(\tau, z, u, \xi). \tag{3.4.28}$$

Here JK-Res is the Jeffrey-Kirwan residue operation, which is explained in detail below. It is locally constant as a function of  $\eta$ , but it can jump as  $\eta$  crosses from one chamber to another. Nonetheless the sum on the right hand side is independent of  $\eta$ .

<sup>29</sup>Denote by  $\text{Cone}_{\text{sing}}(\mathbf{Q}) \subset \mathfrak{h}^*$  the union of the cones generated by all subsets of  $\mathbf{Q}$  with  $r-1$  elements. Then each connected component of  $\mathfrak{h}^* \setminus \text{Cone}_{\text{sing}}(\mathbf{Q})$  is called a *chamber*. By a ‘‘generic’’ covector we mean an  $\eta \notin \text{Cone}_{\text{sing}}(\mathbf{Q})$ : such  $\eta$  identifies a chamber in  $\mathfrak{h}^*$ .

<sup>30</sup>For a technical reason, one has to assume the following condition on the gauge theory charges: *For any  $u_* \in \mathfrak{M}_{\text{sing}}^*$ , the set  $\mathbf{Q}(u_*)$  is contained in a half-space of  $\mathfrak{h}^*$ .* A hyperplane arrangement with this property at  $u_*$  is called *projective* [106]. Notice that if the number of hyperplanes at  $u_*$  is exactly  $r$ , the arrangement is automatically projective. When the condition is not met, one needs to relax the constraints on R- and flavor charges coming from the superpotential, resolve  $u_*$  into multiple singularities which are separately projective, and eventually take a limit where the charges are the desired ones. If at every  $u_*$  the number of hyperplanes meeting at  $u_*$  is exactly  $r$ , we call the situation *non-degenerate*.

## The Jeffrey-Kirwan residue

The Jeffrey-Kirwan residue operation has been introduced in [66]; there are several equivalent formulations available in the literature, and we follow [106]. We define the residue at  $u_* = 0$ ; for generic  $u_*$  one just shifts the coordinates. Consider  $n$  hyperplanes meeting at  $u = 0 \in \mathbb{C}^r$ :

$$H_i = \{u \in \mathbb{C}^r \mid Q_i(u) = 0\} \quad (3.4.29)$$

for  $i = 1, \dots, n$  and with  $Q_i \in (\mathbb{R}^r)^*$ . Here we indicate the set of charges  $\mathbf{Q}(u_*) = \{Q_i\}$  simply by  $\mathbf{Q}_*$ : the charges define the hyperplanes  $H_i$  and give them an orientation. The set  $\mathbf{Q}_*$  defines a hyperplane arrangement (for further details on hyperplane arrangements see *e.g.* [107]). The coefficients defining the hyperplanes are all real, *i.e.* we are dealing with a complexified central arrangement. A residue operation is a linear functional on the space of meromorphic  $r$ -forms that are holomorphic on the complement of the arrangement, such that it annihilates exterior derivatives of rational  $(r - 1)$ -forms.

Take a meromorphic  $r$ -form  $\omega$  defined in a neighborhood  $U$  of  $u = 0$ , and holomorphic on the complement of  $\bigcup_i H_i$ . When  $n = r$ , we can define the residue of  $\omega$  at  $u = 0$  by its integral over  $\prod_{i=1}^r \mathcal{C}_i$ , where each  $\mathcal{C}_i$  is a small circle around  $H_i$  (and the overall sign depends on the order of the  $H_i$ 's). This stems from the fact that the homology group  $H_r(U \setminus \bigcup_{i=1}^r H_i, \mathbb{Z}) = \mathbb{Z}$ , and therefore there is a natural generator defined up to a sign. When  $n > r$  however,  $H_r(U \setminus \bigcup_{i=1}^n H_i, \mathbb{Z}) = \mathbb{Z}^{c_{n,r}}$  with  $c_{n,r} > 1$ , and it is imperative to specify the precise cycle to choose.

For a projective arrangement and given an  $\eta \in (\mathbb{R}^r)^*$ , the Jeffrey-Kirwan residue is the linear functional defined by the conditions:

$$\text{JK-Res}_{u=0}(\mathbf{Q}_*, \eta) \frac{dQ_{j_1}(u)}{Q_{j_1}(u)} \wedge \dots \wedge \frac{dQ_{j_r}(u)}{Q_{j_r}(u)} = \begin{cases} \text{sign det}(Q_{j_1} \dots Q_{j_r}) & \text{if } \eta \in \text{Cone}(Q_{j_1} \dots Q_{j_r}) \\ 0 & \text{otherwise} \end{cases} \quad (3.4.30)$$

where Cone denotes the cone spanned by the vectors in the argument. We can rewrite it as

$$\text{JK-Res}_{u=0}(\mathbf{Q}_*, \eta) \frac{du_1 \wedge \dots \wedge du_r}{Q_{j_1}(u) \dots Q_{j_r}(u)} = \begin{cases} \frac{1}{|\text{det}(Q_{j_1} \dots Q_{j_r})|} & \text{if } \eta \in \text{Cone}(Q_{j_1} \dots Q_{j_r}) \\ 0 & \text{otherwise} \end{cases} \quad (3.4.31)$$

after choosing coordinates  $u_a$  on  $\mathfrak{h}$ . The definition (3.4.30)-(3.4.31) is in general vastly over-determined since there are many relations between the forms  $\bigwedge_{\alpha=1}^r dQ_{j_\alpha} / Q_{j_\alpha}$ , but it has been proven in [108] that (3.4.30) is consistent, and it is given by an integral over an explicit cycle. A constructive definition of the JK residue, as a sum of iterated standard residues, has been given in [106] and reviewed in [67].

In the simplest case of  $r = 1$ , applying (3.4.31) one finds

$$\text{JK-Res}_{u=0}(\{q\}, \eta) \frac{du}{u} = \begin{cases} \text{sign}(q) & \text{if } \eta q > 0, \\ 0 & \text{if } \eta q < 0. \end{cases} \quad (3.4.32)$$

Substituting into (3.4.28), one finds that the elliptic genus in the rank-1 case is given by

$$Z_{T^2} = \frac{1}{|\text{Weyl}(G)|} \sum_{u_+ \in \mathfrak{M}_{\text{sing}}^+} \frac{1}{2\pi i} \oint_{u=u_+} Z_{1\text{-loop}} = -\frac{1}{|\text{Weyl}(G)|} \sum_{u_- \in \mathfrak{M}_{\text{sing}}^-} \frac{1}{2\pi i} \oint_{u=u_-} Z_{1\text{-loop}} \quad (3.4.33)$$

by choosing  $\eta = 1$  and  $\eta = -1$  respectively, where  $\mathfrak{M}_{\text{sing}}^{+(-)}$  is the subset of singularities with positive (negative) associated charge. In other words, one should sum (with sign) the residues coming from fields of either positive or negative charge. As the sum of all residues vanishes, the result is independent of the choice of  $\eta$ .

### 3.4.3 The derivation

Let us briefly sketch how the formula (3.4.28) is derived. The formula and its derivation was first obtained in [67, 89] and then extended in [9, 10, 26, 100].

The standard localization procedure reduces the path-integral to an integral over the BPS supermanifold of zero-modes, schematically

$$Z_{T^2} = \int_{\mathcal{M}_{\text{BPS}}} \mathcal{D}\varphi_0 e^{-S[\varphi_0]} Z_{1\text{-loop}}[\varphi_0]. \quad (3.4.34)$$

In the present case, it turns out that  $\mathcal{M}_{\text{BPS}}$  contains fermionic zero-modes as well as singular loci with extra bosonic zero-modes. With a suitable regulator, the two problems solve each other and one is left with a contour integral within the bosonic component of  $\mathcal{M}_{\text{BPS}}$ .

Solving the bosonic BPS equations—read off from (3.4.11), (3.4.12) and (3.4.13)—chiral and Fermi multiplets are set to zero and one finds the moduli space of flat connections on  $T^2$  modulo gauge transformations. In the simplest case of a gauge group  $G$  with connected and simply-connected non-Abelian part (and arbitrary Abelian part):

$$\mathcal{M}_{\text{BPS}} \Big|_{\text{bos}} = \mathfrak{M}/\text{Weyl}(G), \quad \mathfrak{M} = \mathfrak{h}_{\mathbb{C}}/(\Gamma_{\mathfrak{h}} + \tau\Gamma_{\mathfrak{h}}). \quad (3.4.35)$$

Here  $\mathfrak{M}$  is  $r$  copies of  $T^2$  and we parametrize it by the variables  $u$ .

Around each of the BPS configurations, besides the bosonic zero-modes that parametrize  $\mathcal{M}_{\text{BPS}} \Big|_{\text{bos}}$  there are also fermionic zero-modes and together they form complete supermultiplets. Each bosonic zero-mode is paired with a fermionic zero-mode coming from the Cartan gaugini (in  $\mathcal{N}=(0, 2)$  notation). The right-moving Cartan gaugini  $\lambda$  are not lifted because they are charged only under the R-symmetry, and we cannot turn on a flat connection for the R-symmetry without breaking supersymmetry. In a gauge where  $A_\mu$  is constant, we can identify (up to unimportant coefficients)  $u = A_{\bar{w}}$ , then the fermionic zero-modes are constant  $\lambda^+$ ,  $\bar{\lambda}^+$ . We can close the supersymmetry algebra “off-shell” if we introduce an auxiliary bosonic zero-mode  $D_0$ , which is the constant profile of  $D$ . The supersymmetry algebra follows from (3.4.13):

$$\begin{aligned} Qu = 0, & & Q\bar{u} = \frac{1}{2}\bar{\lambda}^+, & & Q\bar{\lambda}^+ = 0, & & Q\lambda^+ = -D_0, & & QD_0 = 0 \\ \tilde{Q}u = 0, & & \tilde{Q}\bar{u} = -\frac{1}{2}\lambda^+, & & \tilde{Q}\lambda^+ = 0, & & \tilde{Q}\bar{\lambda}^+ = -D_0, & & \tilde{Q}D_0 = 0. \end{aligned} \quad (3.4.36)$$

We used that the flux is zero and all modes are constant on  $T^2$ .

The one-loop determinants, keeping the dependence on  $D_0$  which serves as a regulator of the final expression, are easy to compute using the Hamiltonian definition. For instance, for an  $\mathcal{N}=(2, 2)$  chiral multiplet of charge weight  $\rho$  one finds

$$\mathcal{Z}^{(2,2) \text{ chiral}}(u, \bar{u}, D_0) = \prod_{m,n} \frac{(m + n\tau + (1 - \frac{R}{2})z - \rho(u))(m + n\bar{\tau} + \frac{R}{2}\bar{z} + \rho(\bar{u}))}{|m + n\tau + \frac{R}{2}z + \rho(u)|^2 + i\rho(D_0)}. \quad (3.4.37)$$

The determinants reduce to  $Z_{1\text{-loop}}$  in (3.4.21) and (3.4.23) for  $D_0 = 0$ . Then they develop singularities on  $\mathfrak{M}$  along the hyperplanes  $H_i$  because extra bosonic zero-modes appear, but there are no divergences for generic  $D_0 \neq 0$ .

The last step is to integrate over the moduli space of BPS configurations. For simplicity, let us restrict to the case that  $G$  has rank 1. Since all action terms are  $\mathcal{Q}$ -exact, we perform localization simply by sending to zero all interactions. The singular hyperplanes—which in this case are just points—arise because we take the limit  $\mathbf{e} \rightarrow 0$ , where  $\mathbf{e}$  is the gauge coupling. In the weakly-interacting theory the contribution from the neighborhood of a singular point  $u_* \in \mathfrak{M}_{\text{sing}}$  where there are  $M$  quasi-zero-modes  $\phi_i$ —whose charges  $Q_i$  have the same sign by the assumption in footnote 30—is roughly:

$$I = \int d^{2M}\phi \exp \left[ - \sum_i |Q_i(u - u_*)|^2 |\phi_i|^2 - \frac{\mathbf{e}^2}{2} \left( \zeta - \sum_i Q_i |\phi_i|^2 \right)^2 \right], \quad (3.4.38)$$

where  $\zeta$  is the FI term. The second term comes from the D-term potential and it ensures that the integral is convergent, even at  $u = u_*$ . By rescaling  $\phi_i \rightarrow |Q_i \mathbf{e}|^{-1/2} \phi_i$  we can find an upper bound  $|I| \lesssim C/\mathbf{e}^M$  for some constant  $C$ . Therefore, we can split the integral over  $\mathfrak{M}$  into two pieces, removing from  $\mathfrak{M}$  an  $\varepsilon$ -neighborhood  $\Delta_\varepsilon$  of  $\mathfrak{M}_{\text{sing}}$ . The integral over  $\Delta_\varepsilon$  is bounded by  $\varepsilon^2/\mathbf{e}^M$  up to constants, therefore in a scaling limit  $\mathbf{e}, \varepsilon \rightarrow 0$  in which  $\varepsilon^2/\mathbf{e}^M \rightarrow 0$  as well, it does not contribute. We thus have

$$Z_{T^2} = \frac{1}{|\text{Weyl}(G)|} \lim_{\mathbf{e}, \varepsilon \rightarrow 0} \int_{\mathfrak{M} \setminus \Delta_\varepsilon} d^2u \int_{\mathbb{R}+i\eta} dD_0 \int d\lambda^+ d\bar{\lambda}^+ \mathcal{Z}(u, \bar{u}, \lambda^+, \bar{\lambda}^+, D_0). \quad (3.4.39)$$

We have restored the dependence on the zero-mode  $D_0$  of the auxiliary field, since it will be used as a regulator momentarily. Then  $\mathcal{Z}$  is the effective partition function obtained by integrating out all massive modes. Setting  $\lambda^+ = \bar{\lambda}^+ = 0$  and in the  $\mathbf{e} \rightarrow 0$  limit it gives what we have written in (3.4.37), and further setting  $D_0 = 0$  it gives the one-loop determinants in (3.4.21) and (3.4.23). The function  $\mathcal{Z}$  is holomorphic in  $D_0$  around the origin as long as  $u \notin \Delta_\varepsilon$ . Therefore we have the freedom to shift the real integration contour on the complex  $D_0$ -plane along the imaginary direction, as long as this shift is small: in (3.4.39) we have called  $\eta$  such a shift.

The partition function  $\mathcal{Z}(u, \bar{u}, \lambda^+, \bar{\lambda}^+, D_0)$  depends on the gaugino zero-modes because of the Lagrangian couplings  $\lambda\psi\phi$  to the matter fields we have integrated out. As noticed in [9, 10], the dependence is fixed by supersymmetry. From the algebra (3.4.36) it follows

$$0 = \tilde{Q}\mathcal{Z} = -\frac{\lambda^+}{2} \frac{\partial \mathcal{Z}}{\partial \bar{u}} - D_0 \frac{\partial \mathcal{Z}}{\partial \bar{\lambda}^+} \quad \Rightarrow \quad \frac{\partial^2 \mathcal{Z}}{\partial \lambda^+ \partial \bar{\lambda}^+} = -\frac{1}{2D_0} \frac{\partial \mathcal{Z}}{\partial \bar{u}} \Big|_{\lambda^+ = \bar{\lambda}^+ = 0}. \quad (3.4.40)$$

The integral over the fermionic zero-modes produces a total derivative, and by Stoke's theorem we obtain the contour integral expression

$$Z_{T^2} = \frac{1}{|\text{Weyl}(G)|} \lim_{\epsilon, \epsilon \rightarrow 0} \int_{\partial\Delta_\epsilon} du \int_{\mathbb{R}+i\eta} \frac{dD_0}{D_0} \mathcal{Z}(u, \bar{u}, D_0). \quad (3.4.41)$$

Consider a component of  $\partial\Delta_\epsilon$  around a point  $u_* \in \mathfrak{M}_{\text{sing}}$ . Suppose that we have chosen  $\eta > 0$ . From the unregularized expression in (3.4.37) of the chiral one-loop determinant, we see that the poles in the complex  $D_0$ -plane are in the half  $\rho \text{Im } D_0 > 0$ . If  $\rho < 0$  the poles are in the negative half-plane. As  $\epsilon \rightarrow 0$  they collapse towards  $D_0 = 0$ , because the term in absolute value is of order  $\epsilon$  on the contour  $\partial\Delta_\epsilon$ , however the contour  $\mathbb{R} + i\eta$  is safely far from them. The  $D_0$ -integral remains finite as  $\epsilon \rightarrow 0$ , and then the  $u$ -integral vanishes because its contour shrinks. On the contrary, if  $\rho > 0$  the poles are in the upper  $D_0$ -half-plane and, as  $\epsilon \rightarrow 0$ , they would cross the contour  $\mathbb{R} + i\eta$ . To avoid that, we shift the contour to  $\mathbb{R} - i\eta$  and we collect minus the residue at  $D_0 = 0$ . As before, the integral along  $\mathbb{R} - i\eta$  does not yield any contribution as  $\epsilon \rightarrow 0$ . Minus the residue at  $D_0 = 0$ , though, gives

$$\lim_{\epsilon, \epsilon \rightarrow 0} \int_{\partial\Delta_\epsilon} du \mathcal{Z}(u, \bar{u}, 0) = \text{Res}_{u=u_*} Z_{1\text{-loop}}(u),$$

up to constants that can be fixed in one known example. Had we chosen  $\eta < 0$  instead, a similar argument goes through and one obtains minus the residue at  $u = u_*$  if  $\rho < 0$ , zero if  $\rho > 0$ .

We reach the conclusion that for  $\eta > 0$  we collect the residues of  $Z_{1\text{-loop}}(u)$  at the points  $u_* \in \mathfrak{M}_{\text{sing}}^+$  corresponding to chiral fields with positive charges, while for  $\eta < 0$  we collect minus the residues at the points  $u_* \in \mathfrak{M}_{\text{sing}}^-$  corresponding to chiral fields with negative charges, reproducing (3.4.33). The generic higher-rank case is much more intricate, but conceptually very similar, and it leads to the JK residue. We refer the reader to the references for details.

### 3.4.4 Extensions and applications

The localization formula we presented has been generalized in many ways. The authors of [96, 97] have considered gauge theories with Stückelberg fields, which in the IR may realize non-compact sigma models a prototype of which is the  $SL(2, \mathbb{R})/U(1)$  (cigar) coset. The resulting genus is a Jacobi-like form that is non-holomorphic in the modular parameter  $\tau$  of the torus, with mock modular behavior. The reason is that those models have a continuous spectrum above a threshold, even when equivariant parameters are turned on, and the density of states of bosons and fermions in the continuum need not be equal.

The prototype  $\mathcal{N}=(2, 2)$  GLSM is the one introduced by Hori and Kapustin in [109]. The model has a  $U(1)$  vector field  $V$ , a chiral multiplet  $\Phi$  of charge 1, and a chiral Stückelberg field  $P$  that transforms as

$$P \rightarrow P + i\Lambda \quad (3.4.42)$$

under super-gauge transformations  $V \rightarrow V - i\Lambda + i\bar{\Lambda}$ . Moreover the imaginary part of  $p$  (the scalar in  $P$ ) is periodic,  $p \sim p + 2\pi i$ . The action is

$$S = \frac{1}{4\pi} \int d^2w d^4\theta \left[ \bar{\Phi} e^V \Phi + \frac{k}{4} (P + \bar{P} + V)^2 - \frac{1}{2e^2} \bar{\Sigma} \Sigma \right], \quad (3.4.43)$$

where  $k > 0$  and  $\Sigma$  is the field-strength twisted chiral multiplet. When written in components, the imaginary part of  $p$  acts as a standard Stückelberg field that gives the photon a mass, while the real part is a dynamical FI term. Integrating out the massive photon and after some RG flow, one obtains the  $SL(2, \mathbb{R})_k/U(1)$  SCFT with central charge  $c = 3 + \frac{6}{k}$ , which in the large  $k$  limit has a description as the NLSM with cigar target

$$ds^2 = 2k \left( du^2 + \tanh^2 u d\psi^2 \right) \quad (3.4.44)$$

with  $\psi \cong \psi + 2\pi$ , and a non-trivial background dilaton [110].

When computing the elliptic genus with localization, the presence of the field  $P$  introduces many differences. First, the action involving  $P$  is naively  $\mathcal{Q}$ -exact but in fact it gives rise to a non-trivial boundary term in field space [109], therefore the final answer will depend on  $k$ . Luckily,  $P$  appears quadratically in the action and so its path-integral can be computed exactly.

Second, the field  $P$  has fermionic zero-modes  $\chi^-, \bar{\chi}^-$  coupled to the gaugino zero-modes  $\lambda^+, \bar{\lambda}^+$ . Therefore, when integrating over the fermionic zero-modes they are absorbed at tree level and we simply generate a constant factor—instead of a total derivative as before. The integration over the bosonic zero-modes of  $P$  and the massive modes is standard, and the details can be found in [96, 97, 111]. A point to note is that the imaginary part of  $p$  is a periodic scalar which admits winding modes:  $p_2(w + 1) = p_2(w) + 2\pi n$ ,  $p_2(w + \tau) = p_2(w) + 2\pi m$ . The path-integral over  $P$  then gives

$$Z_P = \frac{k}{D_0 \tau_2} \frac{\theta_1(q, y)}{\eta(q)^3} \sum_{m, n \in \mathbb{Z}} \exp \left[ -\frac{\pi k}{\tau_2} \left( m + n\tau + u + \frac{z}{k} \right) \left( m + n\bar{\tau} + \bar{u} + \frac{z}{k} \right) \right]. \quad (3.4.45)$$

The one-loop determinant of the chiral multiplet is also modified. The UV left-moving R-symmetry  $J_\mu$  is anomalous and the IR conserved superconformal R-symmetry is obtained by mixing with the gauge-invariant quantity  $A_\mu + \partial_\mu p_2$ . The R-symmetry background experienced by  $\Phi$  thus depends on the winding numbers  $(m, n)$ :

$$Z_\Phi = y^{\rho m} \frac{\theta_1(q, y^{R/2-1} x^\rho)}{\theta_1(q, y^{R/2} x^\rho)}, \quad (3.4.46)$$

where  $\rho$  is the gauge charge. Putting everything together, and generalizing to multiple chiral multiplets  $\Phi_i$ , one finds the formula:

$$Z_{T^2} = k \int_{T^2} \frac{d^2u}{\tau_2} \prod_i \frac{\theta_1(q, y^{\frac{R_i}{2}-1} x^{\rho_i})}{\theta_1(q, y^{\frac{R_i}{2}} x^{\rho_i})} \sum_{m, n \in \mathbb{Z}} y^{n \sum_i \rho_i} e^{-\frac{\pi k}{\tau_2} (m + n\tau + u + \frac{z}{k}) (m + n\bar{\tau} + \bar{u} + \frac{z}{k})}. \quad (3.4.47)$$

The cigar coset theory corresponds to a single field with  $\rho = 1$  and  $R = 0$ . Notice that in the presence of multiple chiral multiplets with coincident poles, the integral is divergent and it should be regularized with care.

The expression above is not holomorphic in  $\tau$ : it is the product of a usual Jacobi form and an Appell-Lerch sum. The latter are intimately related to a very interesting class of functions called mock modular forms [112–114]. Their key feature is that they transform as modular forms, but they suffer from a holomorphic anomaly.

The example above can obviously be generalized to more Abelian groups and matter contents. As an interesting application, [115] studies the equivariant elliptic genera of a class of gravitational instantons that are given by hyper-Kähler four-manifolds of asymptotically locally flat (ALF) type. The simplest of these spaces is the Taub-NUT manifold, while more general constructions yield the multi-center  $A_k$  ALF spaces of Gibbons and Hawking [116] and other spaces. Taub-NUT can be obtained from an  $\mathcal{N}=(4, 4)$  GLSM consisting of a  $U(1)$  vector multiplet, a hypermultiplet of charge 1 and a neutral Stückelberg hypermultiplet [117].<sup>31</sup> The model has  $SU(2)^3$  R-symmetry and  $U(1)_f$  flavor symmetry (one  $SU(2)$  corresponds to rotations of  $\mathbb{R}^3$ , while  $U(1)_f$  rotates the circle). The coupling  $k$  controls the size of the asymptotic circle, and in the  $k \rightarrow \infty$  limit the model turns into  $\mathbb{C}^2$ . Localization in this case gives<sup>32</sup>

$$Z_{T^2} = k \int_{\mathbb{C}} \frac{d^2 u}{\tau_2} \frac{\theta_1(q, xy\zeta_1) \theta_1(q, xy^{-1}\zeta_1)}{\theta_1(q, x\zeta_1\zeta_2) \theta_1(q, x\zeta_1\zeta_2^{-1})} e^{-\frac{k\pi}{\tau_2}|u|^2}, \quad (3.4.48)$$

where we have used the sum over winding sectors to “unfold” the integral over the whole complex plane. Here  $\zeta_1, \zeta_2, y$  are fugacities for  $U(1)_f$  and for two left-moving R-symmetries, respectively. In the  $k \rightarrow \infty$  limit one obtains the equivariant elliptic genus of  $\mathbb{C}^2$ , which equals the integrand of (3.4.48) evaluated at  $u = 0$  and it is holomorphic in  $\tau$ .

Physically, the equivariant deformations produce a potential roughly proportional to the length of the orbits of the associated  $U(1)$  actions. In the case of Taub-NUT the potential produced by  $\zeta_1 = e^{2\pi i \xi_1}$  is

$$V = \frac{\xi_1^2}{\frac{1}{k} + \frac{1}{|\vec{x}|^2}}, \quad (3.4.49)$$

where  $\vec{x}$  is a coordinate on  $\mathbb{R}^3$ . Around the origin ( $\vec{x} = 0$ ) the potential is quadratic and it gives a discrete IR spectrum, while at large  $|\vec{x}|$  it is a constant allowing for a continuous spectrum of scattering states. The latter are responsible for the loss of holomorphy in  $\tau$ .

One can also generalize the elliptic genus to the *twining genera*: in the minimal  $\mathcal{N}=(0, 2)$  case, given a theory with a discrete symmetry  $g$  that commutes with the right-moving supersymmetry algebra, they are defined as

$$Z_g(\tau, u) = \text{Tr}_{\text{R}} (-1)^F g q^{H_L} \bar{q}^{H_R} \prod_a x_a^{K_a} \quad (3.4.50)$$

<sup>31</sup>In  $\mathcal{N}=(2, 2)$  notation, the model has a vector multiplet  $V$ , two neutral chiral multiplets  $\Phi, \Psi$ , two chiral multiplets  $Q, \tilde{Q}$  of charges  $\pm 1$ , and a Stückelberg chiral multiplet  $P$ . There is also a superpotential  $W = \tilde{Q}\Phi Q + \Phi\Psi$ .

<sup>32</sup>In this model the R-symmetry current is not anomalous, therefore the Stückelberg field has no R-charge.

with an insertion of  $g$  into the trace. These objects decompose into characters of the discrete symmetry group, and therefore contain valuable information about the spectrum of the theory. As shown in [95], it is easy to extend the localization computation to the twining genera. If the symmetry element  $g$  acts on chiral and Fermi multiplets as

$$g \Phi_i = e^{2\pi i \alpha_i} \Phi_i, \quad g \Lambda_i = e^{2\pi i \beta_i} \Lambda_i, \quad (3.4.51)$$

the corresponding one-loop determinants are modified to

$$Z_{\Phi_i} = \frac{i \eta(q) e^{\pi i \alpha_i}}{\theta_1(q, e^{2\pi i \alpha_i} x^{\rho_i})}, \quad Z_{\Lambda_i} = \frac{i \theta_1(q, e^{2\pi i \beta_i} x^{\rho_i})}{\eta(q) e^{\pi i \beta_i}}. \quad (3.4.52)$$

Then one takes the JK residue at the (possibly shifted) poles. The formula has been used for instance in [95] to study the twining genera of  $\mathcal{N}=(0, 4)$  NLSM with K3 target under the action of elements of  $M_{24}$ , the largest Mathieu group, in connection with the so-called “moonshine conjectures”.

For  $\mathcal{N}=(0, 2)$  gauge theories, the elliptic genus is one of the few quantities that can be computed non-pertubatively via localization.<sup>33</sup> Therefore it constitutes a crucial test of conjectured IR dualities among different gauge theories. One example are the trialities of [118], which will be discussed in subsection 3.5.4.

To conclude, we mention two recent applications of the elliptic genus of gauge theories. One is in the context of “AGT correspondences” [119] (see also Chapter 12). Through the compactification of M5-branes on  $T^2 \times \mathcal{M}_4$ , where  $\mathcal{M}_4$  is an arbitrary four-manifold, one can try to relate the elliptic genus of certain  $\mathcal{N}=(0, 2)$  gauge theories (which depend on  $\mathcal{M}_4$ ) and the Vafa-Witten partition function [121] of 4d  $\mathcal{N}=4$  SYM on  $\mathcal{M}_4$ . This program has been initiated in [122]. Another application is to interpret the partition functions of certain 6d SCFTs as the generating functions of the elliptic genera of their BPS strings [123] (see Chapter 17).

## 3.5 Dualities

The supersymmetric observables exactly computed in previous sections provide powerful means to test dualities. We review in this section a few such applications of the sphere partition function and the elliptic genus. First we consider mirror symmetry in subsection 3.5.1, comparing sphere partition functions of 2d  $\mathcal{N}=(2, 2)$  GLSMs which flow to mirror Calabi-Yau manifolds. In subsection 3.5.2 we discuss Seiberg-like dualities between 2d  $\mathcal{N}=(2, 2)$  gauge theories with  $U(N)$  gauge groups and (anti)fundamental matter. Then in subsection 3.5.3 we list generalizations, while subsection 3.5.4 describes 2d  $\mathcal{N}=(0, 2)$  dualities which have been checked using the elliptic genus.

---

<sup>33</sup>For deformations of  $\mathcal{N}=(2, 2)$  gauge theories, one can also compute correlators on  $S^2$  [26].

### 3.5.1 Mirror symmetry

Numerous NLSMs with Calabi-Yau target spaces can be realized as the low-energy limit of gauged linear sigma models. The Calabi-Yau moduli space coincides with the conformal manifold of the NLSM, which is typically spanned by exactly marginal (chiral and twisted chiral) operators of the GLSM. Twisted chiral operators alter the (complexified) Kähler structure of the Calabi-Yau, while chiral operators alter its complex structure. Both the moduli space of Kähler structure deformations and that of complex structure deformations are Kähler manifolds, whose metric derives from a Kähler potential.

As reviewed in Chapter 4, these Kähler potentials can be efficiently computed from GLSM sphere partition functions [13, 18–20]. Placing a GLSM on the sphere preserves either the vector or the axial R-symmetry. These two choices lead to distinct partition functions  $Z_A$  and  $Z_B$ , computed in section 3.2 and subsection 3.3.2. Both are independent of the superrenormalizable gauge coupling hence are invariant under the RG flow. The first one depends only on twisted chiral parameters (FI parameters, theta angles, twisted masses, vector R-charges) and gives the Kähler potential  $\mathcal{K}_K$  on the moduli space of Kähler structure deformations, while the second one depends only on chiral parameters (the superpotential) and gives the Kähler potential  $\mathcal{K}_C$  on the moduli space of complex structure deformations:

$$Z_A = e^{-\mathcal{K}_K} \quad \text{and} \quad Z_B = e^{-\mathcal{K}_C} . \quad (3.5.1)$$

This streamlines the extraction of genus zero Gromov-Witten invariants from  $\mathcal{K}_K$  (see [18, 62, 125, 126]). Remarkably, most known Calabi-Yau manifolds are paired such that the moduli space of complex structure deformations of one is identical to the moduli space of Kähler structure deformations of the other and viceversa. The manifolds are called mirrors of each other. The interchange of  $\mathcal{K}_K$  and  $\mathcal{K}_C$  can be shown by proving that  $Z_A$  of one GLSM is equal to  $Z_B$  of the other.

Mirror symmetry generalizes to GLSMs whose low-energy limit is an NLSM on a Kähler manifold (with non-negative first Chern class) rather than a Calabi-Yau manifold: a large class of GLSMs have Landau-Ginzburg models as their mirrors [45]. In this section, we prove following [13, 21] (an example was worked out in [11]) that  $Z_A$  of a GLSM is equal to  $Z_B$  of the Landau-Ginzburg mirror proposed by Hori and Vafa. In fact, to avoid switching back and forth between the backgrounds that preserve  $\mathfrak{su}(2|1)_A$  and  $\mathfrak{su}(2|1)_B$ , we apply to the Landau-Ginzburg model the involution of the superconformal algebra which exchanges these two subalgebras and exchanges vector/chiral multiplets with twisted vector/chiral multiplets. As a result, we wish to write  $Z_A$  of a GLSM (computed in section 3.2) as  $Z_A$  of a Landau-Ginzburg model of twisted chiral multiplets (computed in subsection 3.3.2).

The key mathematical identity is (omitting irrelevant constant factors)<sup>34</sup>

$$\frac{\Gamma(a)}{\Gamma(1+b)} = \int_0^\infty dt e^{-t} t^{a-1} \int_{\text{Hankel}} ds e^s s^{-b-1} = \int_{-\infty}^\infty \int_{-\pi}^\pi d^2 Y \exp\left(-e^{-Y} - aY + e^{-\bar{Y}} + b\bar{Y}\right), \quad (3.5.2)$$

where  $Y \cong Y + 2\pi i$  is periodic and  $a + b \in \mathbb{Z}$ . This identity applies readily to the one-loop determinant (3.2.18) of a chiral multiplet:

$$Z_{1\text{-loop}}^{\text{chiral}} = \prod_w \frac{\Gamma\left(\frac{q}{2} - ir\tau - \frac{n}{2} - irw(\sigma) - \frac{w(\mathbf{m})}{2}\right)}{\Gamma\left(1 - \frac{q}{2} + ir\tau - \frac{n}{2} + irw(\sigma) - \frac{w(\mathbf{m})}{2}\right)} = \prod_w \int d^2 Y_w e^{-\frac{q}{2}(Y_w + \bar{Y}_w)} e^{-4\pi ir \widetilde{W}_w - 4\pi ir \bar{\widetilde{W}}_w} \quad (3.5.3)$$

where the twisted superpotential  $\widetilde{W}$  involves the bottom component  $\Sigma = r\sigma - i\mathbf{m}/2$  of the field strength twisted chiral multiplet:

$$4\pi ir \widetilde{W}_w = e^{-Y_w} - \left(ir\tau + \frac{n}{2} + iw(\Sigma)\right) Y_w. \quad (3.5.4)$$

For non-zero R-charges, the weight factor  $\exp[-\frac{q}{2}(Y_w + \bar{Y}_w)]$  is naturally absorbed in the integration measure (up to a constant) by using the variables  $\widetilde{X}_w = \exp(-\frac{q}{2}Y_w)$ .

Translating the full partition function of a GLSM to the variables  $Y$  and  $\Sigma$  yields

$$Z_{\text{GLSM}} = \int d^2 \Sigma \prod_{\alpha > 0} \left[ e^{\pi\alpha(\Sigma - \bar{\Sigma})} \alpha(\Sigma) \alpha(\bar{\Sigma}) \right] \prod_{I,w} \left[ \int d^2 Y_w^I e^{-\frac{q_I}{2}(Y_w^I + \bar{Y}_w^I)} \right] e^{-4\pi ir \widetilde{W} - 4\pi ir \bar{\widetilde{W}}} \quad (3.5.5)$$

where  $\Sigma$  has a GNO quantized imaginary part, we dropped a factor of  $r^{c/3}$  and numerical constants, and where

$$4\pi ir \widetilde{W} = \sum_\ell \left[ \left( \vartheta_\ell + 2\pi i \zeta_\ell \right) \text{Tr}_\ell \Sigma \right] + \sum_{I,w} \left[ e^{-Y_w^I} - \left( ir\tau_I + \frac{n_I}{2} + iw(\Sigma) \right) Y_w^I \right]. \quad (3.5.6)$$

This twisted superpotential was found much earlier [45] to be generated by vortices.

Equation (3.5.5) is the  $Z_A$  partition function (3.3.6) of a Landau-Ginzburg model with twisted chiral multiplets  $\Sigma$  and  $Y$  in a certain target space (whose volume form leads to the non-trivial integration measure) and subject to the twisted superpotential (3.5.6), or equivalently the  $Z_B$  partition function of a model with chiral multiplets. We can go further in the case of Landau-Ginzburg models mirror to Abelian GLSMs: then  $\Sigma$  appears only linearly in the twisted superpotential hence plays the role of a Lagrange multiplier. Integrating it out yields delta function constraints between the variables  $Y^I$ :

$$i\vartheta_\ell - 2\pi\zeta_\ell + \sum_I Y^I Q_I^\ell \in 2\pi i \mathbb{Z}. \quad (3.5.7)$$

---

<sup>34</sup>The Hankel contour goes around the cut of  $s^{-b-1}$  along the negative real axis, at a constant distance  $\epsilon > 0$  above and below it. To prove the second equality, either redefine  $Y = -\log t$  and  $\bar{Y} = -\log s$ , or decompose  $Y = x + iy$  and recognize that the last expression is the Fourier transform  $2\pi \int_{-\infty}^{+\infty} dx e^{(b-a)x} J_{a+b}(2e^{-x})$  of the Bessel function of the first kind.

Here  $Q_I^\ell$  denotes the charge of the  $I$ -th chiral multiplet under the  $\ell$ -th gauge group and we have dropped the index  $w$  as each irreducible representation is one-dimensional. Each of the  $N$  constraints (3.5.7) eliminates one of the  $N_f$  twisted chiral multiplets  $Y^I$ . The twisted superpotential reads

$$4\pi i r \widetilde{W} = \sum_{I=1}^{N_f} \left[ e^{-Y^I} - \left( i r \tau_I + \frac{\mathbf{n}_I}{2} \right) Y^I \right] \quad (3.5.8)$$

and the integration measure reduces to (up to permutations of the  $Y^I$ 's)

$$\prod_{I=1}^{N_f-N} \int d^2 Y^I e^{-\frac{q'_I}{2}(Y^I + \bar{Y}^I)} \quad (3.5.9)$$

where  $q'_I$  are certain combinations of R-charges, most conveniently determined by mixing the R-symmetry with gauge symmetries so that R-charges of eliminated twisted chiral multiplets vanish. Switching to variables  $\widetilde{X}^I = \exp(-\frac{q'_I}{2} Y^I)$  yields a Landau-Ginzburg model whose target space is flat, but with a conical singularity at  $\widetilde{X} = 0$ .

Let us consider as an example the quintic hypersurface in  $\mathbb{CP}^4$ . We start with a  $U(1)$  GLSM with 5 chiral multiplets  $X_i$  of gauge charge +1 and R-charge  $q$  and a chiral multiplet  $P$  of gauge charge  $-5$  and R-charge  $q_P = 2 - 5q$ , with a superpotential  $W = P G_5(X)$  where  $G_5$  is a generic homogeneous polynomial of degree 5. The parameter  $q$  mixes the R-symmetry with the gauge symmetry. Following the steps above, we introduce twisted chiral fields  $Y_1, \dots, Y_5, Y_P$  then integrate out  $\Sigma$  and obtain the constraint (3.5.7), namely  $5Y_P = 2\pi\zeta - i\vartheta + Y_1 + \dots + Y_5 \pmod{2\pi i}$ . For convenience, mix the R-symmetry with the gauge symmetry to set  $q \rightarrow 2/5$  so that  $q_P = 0$ . The variables  $\widetilde{X}_i = \exp(-Y_i/5) \in \mathbb{C}^*/\mathbb{Z}_5$  absorb the integration measure, at the cost of an orbifold singularity at the origin. In those variables, the twisted superpotential of the Landau-Ginzburg model reads

$$4\pi i r \widetilde{W} = \widetilde{G}_5(\widetilde{X}) = \widetilde{X}_1^5 + \widetilde{X}_2^5 + \widetilde{X}_3^5 + \widetilde{X}_4^5 + \widetilde{X}_5^5 + e^{(-2\pi\zeta + i\vartheta)/5} \widetilde{X}_1 \widetilde{X}_2 \widetilde{X}_3 \widetilde{X}_4 \widetilde{X}_5. \quad (3.5.10)$$

This model does not depend on the 101 parameters in the original superpotential  $P G_5(X)$ , hence it can only be the mirror of the quintic GLSM at a specific point in the moduli space. Since the theories coincide at that point, their whole moduli spaces must be the same, but let us describe more precisely how this comes about. Continuing from  $Z_A$  of the Landau-Ginzburg model, we add a  $U(1)$  twisted vector multiplet under which each  $\widetilde{X}_i$  has charge +1 and a twisted chiral multiplet  $\widetilde{P}$  of charge  $-5$  and replace  $\widetilde{W}$  by  $\widetilde{P} \widetilde{G}_5(\widetilde{X})$  to make it gauge invariant. The  $Z_A$  partition function (3.3.10) of this twisted GLSM coincides with that of the Landau-Ginzburg model. The twisted GLSM is a special case of the quintic GLSM with multiplets replaced by twisted multiplets and  $G_5 \rightarrow \widetilde{G}_5$ . When its FI parameter  $\chi$  is negative, the low-energy limit is the Landau-Ginzburg model (3.5.10): the D-term equation  $\sum_i |\widetilde{X}_i|^2 - 5|\widetilde{P}|^2 = \chi$  forces  $P \neq 0$  and the F-term equation then sets all  $\widetilde{X}_i = 0$ . When  $\chi > 0$  instead, the low-energy limit is an NLSM on the quintic hypersurface  $\widetilde{G}_5 = 0$ , orbifolded as described above. This orbifold has fixed points and curves. Blowing up the singularities

requires a choice of 100 volume parameters which combine with  $\chi$  to reproduce the 101 chiral parameters of the original GLSM. The NLSM on the blown-up orbifold of  $\{\tilde{G}_5 = 0\}$  could also be described by a twisted  $U(1)^{101}$  GLSM with 106 twisted chiral multiplets, but this is somewhat cumbersome.

The partition functions  $Z_A$  and  $Z_B$  of mirror theories have also been proven equal for all complete intersections in products of weighted projective spaces.

### 3.5.2 Seiberg duality with unitary groups

We now describe a 2d  $\mathcal{N}=(2, 2)$  analogue of 4d  $\mathcal{N}=1$  Seiberg duality, explain how sphere partition functions and elliptic genera of the dual theories are compared, and deduce some variants of this duality in the next subsection. The first such  $\mathcal{N}=(2, 2)$  dualities were analyzed in [127].

The duality states that two theories (named “electric” and “magnetic” theories) have the same infrared limit. The electric theory has a  $U(K)$  gauge group,  $N_f$  fundamental chiral multiplets  $\phi_F$  ( $1 \leq F \leq N_f$ ), and  $N_a$  antifundamental chiral multiplets  $\tilde{\phi}_A$  ( $1 \leq A \leq N_a$ ). We assume  $N \leq \max(N_f, N_a)$ , as otherwise supersymmetry is spontaneously broken (both the elliptic genus and the sphere partition function vanish, see footnote 4) and there is no duality. The magnetic theory has the same field content with

$$(K, N_f, N_a) \rightarrow (K', N'_f, N'_a) = (\max(N_f, N_a) - K, N_a, N_f)$$

and additionally it has  $N_a N_f$  gauge singlet chiral multiplets  $M_{AF}$  with a cubic superpotential  $W = M_{AF} \tilde{\phi}'_F \phi'_A$ . The complexified FI parameters  $t = 2\pi\zeta + i\vartheta$  and the vector R-charges are

$$(-1)^{N'_f - K'} e^{-t'} = [(-1)^{N_f - K} e^{-t}]^{-1} \text{ namely } \zeta' = -\zeta, \quad \vartheta' = -\vartheta + \min(N_f, N_a)\pi \quad (3.5.11)$$

$$q'_A = 1 - \tilde{q}_A, \quad \tilde{q}'_F = 1 - q_F, \quad q'^{(M)}_{AF} = \tilde{q}_A + q_F. \quad (3.5.12)$$

These R-charges give the superpotential R-charge 2 as required by supersymmetry, and are also consistent with the matching of chiral rings:  $M_{AF}$  is mapped to the meson  $\tilde{\phi}'_A \phi'_F$  of the electric theory. The flavor symmetry  $S[U(N_f) \times U(N_a)]$  shared by the two theories can be coupled to a background vector multiplet to include twisted masses and flavor fluxes (the same in both theories), and  $M$  transforms in the bifundamental representation of  $U(N_f) \times U(N_a)$ .

Charge conjugation lets us assume  $N_a \leq N_f$ . It would in fact be enough to check the duality for  $N_a = N_f$ , then decouple chiral multiplets by giving them large twisted masses.

Let us compare elliptic genera of the two theories [67, 88]. Recall that the elliptic genus  $Z_{T^2}(\tau, z, \xi)$  depends on the period  $\tau$  of  $T^2$ , an R-symmetry holonomy  $z$ , and flavor symmetry holonomies  $\xi$  in the flavor Cartan algebra. It is a sum of JK residues (3.4.28) of  $Z_{1\text{-loop}}(\tau, z, u, \xi)$  at values of the gauge holonomies  $u$  (in the gauge Cartan algebra) where this meromorphic (rank  $G, 0$ )-form has poles. More precisely, each component of  $u$  lies in a torus  $\mathbb{C}/(\mathbb{Z} + \tau\mathbb{Z})$

and similarly for  $\xi$ . For the electric theory,<sup>35</sup>

$$Z_{1\text{-loop}}(\tau, z, u, \xi, \tilde{\xi}) = \frac{1}{K!} \left( \frac{2\pi\eta(q)^3}{\theta_1(\tau| - z)} \right)^K \prod_{i \neq j}^K \frac{\theta_1(\tau|u_i - u_j)}{\theta_1(\tau|u_i - u_j - z)} \\ \times \prod_{i=1}^K \left( \prod_{F=1}^{N_f} \frac{\theta_1(\tau|u_i - \xi_F + (\frac{q_F}{2} - 1)z)}{\theta_1(\tau|u_i - \xi_F + \frac{q_F}{2}z)} \prod_{A=1}^{N_a} \frac{\theta_1(\tau| - u_i + \tilde{\xi}_A + (\frac{\tilde{q}_A}{2} - 1)z)}{\theta_1(\tau| - u_i + \tilde{\xi}_A + \frac{\tilde{q}_A}{2}z)} \right) d^K u . \quad (3.5.13)$$

In the following we omit R-charges by shifting  $\xi_F \rightarrow \xi_F + (q_F/2)z$  and  $\tilde{\xi}_A \rightarrow \tilde{\xi}_A - (\tilde{q}_A/2)z$ .

Consider first the case  $N_a = N_f$ . The elliptic genus is a sum of residues of (3.5.13) at a set of poles which depends on a choice of auxiliary parameter  $\eta$  in the gauge Cartan algebra. Choosing  $\eta = (1, \dots, 1)$  selects poles due to fundamental chiral multiplets, at  $u_i = \xi_{F_i}$  for  $1 \leq i \leq K$ , with all  $F_i$  distinct. Altogether, poles which contribute are labelled by  $K$ -element subsets  $\mathcal{I}$  of  $\{1, \dots, N_f\}$ :

$$Z_{T^2}^{U(K)}(\tau, z, \xi, \tilde{\xi}) = \sum_{\mathcal{I} \in \mathcal{C}(K, N_f)} \prod_{F \in \mathcal{I}} \left( \prod_{E \notin \mathcal{I}} \frac{\theta_1(\tau|\xi_F - \xi_E - z)}{\theta_1(\tau|\xi_F - \xi_E)} \prod_{A=1}^{N_a} \frac{\theta_1(\tau| - \xi_F + \tilde{\xi}_A - z)}{\theta_1(\tau| - \xi_F + \tilde{\xi}_A)} \right) \\ = \left( \prod_{F=1}^{N_f} \prod_{A=1}^{N_a} \frac{\theta_1(\tau| - \xi_F + \tilde{\xi}_A - z)}{\theta_1(\tau| - \xi_F + \tilde{\xi}_A)} \right) Z_{T^2}^{U(N_f - K)}(\tau, z, -\frac{z}{2} - \xi, \frac{z}{2} - \tilde{\xi}) . \quad (3.5.14)$$

Besides straightforward rearrangements, the second line uses  $\theta_1(\tau| - z) = -\theta_1(\tau|z)$ . Restoring the R-charges by  $\xi_F \rightarrow \xi_F - (q_F/2)z$  and  $\tilde{\xi}_A \rightarrow \tilde{\xi}_A + (\tilde{q}_A/2)z$ , we recognize the genus of the dual theory with R-charges (3.5.12).

For  $N_a \neq N_f$  the left-moving  $U(1)$  R-symmetry is anomalous and reduces to  $\mathbb{Z}_{|N_f - N_a|}$ . The R-symmetry fugacity  $y$  must obey  $y^{N_f - N_a} = 1$ , as  $Z_{1\text{-loop}}$  is multiplied by  $y^{N_f - N_a}$  upon shifting any component of  $u$  by  $\tau$ . Unfortunately,  $Z_{1\text{-loop}}$  is ill-defined at  $y = 1$  so the localization calculation of the elliptic genus fails in that case (and whenever  $y^K = 1$ ). However, we can introduce  $N_f - N_a$  chiral multiplets  $P_j$  in the  $\det^{-1}$  representation of  $U(K)$  to cancel the R-symmetry anomaly and allow generic  $y$ , then take the limit  $y^{N_f - N_a} \rightarrow 1$ . Provided we choose R-charges of  $P_j$  to be  $q_j = q + 2j$  for some  $q$ , their one-loop determinant contributions to the elliptic genus cancel as  $y^{N_f - N_a} \rightarrow 1$  (for  $y = 1$  a physical explanation is that one can turn on twisted masses for the  $P_j$ ):

$$\left( \prod_{j=1}^{N_f - N_a} \frac{\theta_1(q, y^{q/2 + j - 1} x^{-1})}{\theta_1(q, y^{q/2 + j} x^{-1})} \right) \xrightarrow{y^{N_f - N_a} \rightarrow 1} 1 . \quad (3.5.15)$$

The elliptic genus of the theory enriched with the  $P_j$  can be computed with  $\eta = (1, \dots, 1)$  as above and yields exactly (3.5.14) once one takes the limit (3.5.15). For the allowed values  $(N_f - N_a)z \in \mathbb{Z}$ , the above turns out to simplify to

$$Z_{T^2}^{U(K)}(\tau, z, \xi, \tilde{\xi})_{y^{N_f - N_a} = 1} = y^{-KN_a/2} \binom{N_f}{K}_y = y^{-KN_a/2} \frac{\prod_{j=N_f+1-K}^{N_f} (y^{j/2} - y^{-j/2})}{\prod_{j=1}^K (y^{j/2} - y^{-j/2})} . \quad (3.5.16)$$

<sup>35</sup>With a slight abuse of notation, we identify  $\theta_1(\tau|z) \equiv \theta_1(q, y)$  where, as usual,  $q = e^{2\pi i\tau}$  and  $y = e^{2\pi iz}$ .

The elliptic genus vanishes for  $y^K \neq 1$ : this could be derived by using  $\eta = (-1, \dots, -1)$  in the theory without  $P_j$ . Incidentally, we learn by setting  $y = 1$  that the theories have  $\binom{N_f}{K}$  vacua.

The equality of elliptic genera implies that BPS states of the dual theories have identical flavor and R-symmetry charges, but does not fix the map of (complexified) FI parameters nor the superpotential. These are fixed by comparing A-type and B-type sphere partition functions, respectively.

Next, we sketch the proof [11, 41, 128] that A-type sphere partition functions  $Z_{S^2}^A$  of the two theories coincide. This probes their twisted chiral rings (these have also been proven isomorphic). As described in subsection 3.2.5 the partition function can be localized to (3.2.38): a ‘‘Higgs branch configuration’’ (labeled by  $\mathcal{I}$  below) in the bulk of the sphere with vortices at the North pole and antivortices at the South pole. In detail,

$$Z_{S^2}^A = \sum_{\mathcal{I} \in \mathcal{C}(K, N_f)} Z_0^{\mathcal{I}} Z_+^{\mathcal{I}}(e^{-t}) Z_-^{\mathcal{I}}(e^{-\bar{t} + i\pi(N_f - N_a)}) \quad (3.5.17)$$

where the semiclassical contribution  $Z_0^{\mathcal{I}}$  and the (anti)vortex contributions  $Z_{\pm}^{\mathcal{I}}$  are expressed in terms of the combinations  $\Sigma_F^{\pm} = q_F/2 + ir\tau_F \pm \mathbf{n}_F/2$  of R-charge, twisted mass and flavor flux of fundamental chiral multiplets and similarly  $\tilde{\Sigma}_A^{\pm} = -\tilde{q}_A/2 + ir\tilde{\tau}_A \pm \tilde{\mathbf{n}}_A/2$  for antifundamentals:

$$Z_0^{\mathcal{I}} = \prod_{F \in \mathcal{I}} \left( e^{-t\Sigma_F^+ - \bar{t}\Sigma_F^-} \prod_{E \notin \mathcal{I}} \frac{\Gamma(\Sigma_E^+ - \Sigma_F^+)}{\Gamma(1 - \Sigma_E^- + \Sigma_F^-)} \prod_{A=1}^{N_a} \frac{\Gamma(\Sigma_F^+ - \tilde{\Sigma}_A^+)}{\Gamma(1 - \Sigma_F^- + \tilde{\Sigma}_A^-)} \right) \quad (3.5.18)$$

$$Z_{\pm}^{\mathcal{I}}(x) = \sum_{(k_F \geq 0)_{F \in \mathcal{I}}} \prod_{F \in \mathcal{I}} \frac{x^{k_F} \prod_{A=1}^{N_a} (\Sigma_F^{\pm} - \tilde{\Sigma}_A^{\pm})_{k_F}}{\prod_{E \in \mathcal{I}} (-\Sigma_E^{\pm} + \Sigma_F^{\pm} - k_E)_{k_F} \prod_{E \notin \mathcal{I}} (\Sigma_E^{\pm} - \Sigma_F^{\pm} - k_F)_{k_F}}. \quad (3.5.19)$$

Dual partition functions are compared term by term. The semiclassical parts  $Z_{0,\text{electric}}^{\mathcal{I}}$  and  $Z_{0,\text{magnetic}}^{\{1, \dots, N_f\} \setminus \mathcal{I}}$  are equal up to simple factors elaborated on below. Terms of order  $x^k$  for some  $k \geq 0$  in the vortex partition functions can be recast as a  $k$ -dimensional contour integral such that the poles on one side of the contour are labelled by  $(k_F \geq 0)_{F \in \mathcal{I}}$  with  $\sum_F k_F = k$ . Provided  $N_a \leq N_f - 2$ , there is no pole at infinity and the sum of residues is equal to a sum over poles on the other side of the contour, which reproduces the  $k$ -vortex partition function of the dual theory. For  $|N_a - N_f| \leq 1$  the integrand is singular at infinity and more tedious calculations are needed. The result is

$$Z_{U(K)}^{N_f, N_a}(\Sigma^{\pm}, \tilde{\Sigma}^{\pm}; t) = a_+ \left( e^{-t - i\pi K'} \right) a_- \left( e^{-\bar{t} + i\pi K'} \right) \times \prod_{F, A} \frac{\Gamma(\Sigma_F^+ - \tilde{\Sigma}_A^+)}{\Gamma(1 - \Sigma_F^- + \tilde{\Sigma}_A^-)} Z_{U(K')}^{N_a, N_f} \left( \tilde{\Sigma}^{\pm} + \frac{1}{2}, \Sigma^{\pm} - \frac{1}{2}; t' \right) \quad (3.5.20)$$

where the factors  $a_{\pm}$  depend on  $\Sigma_F^{\pm}$  and  $\tilde{\Sigma}_A^{\pm}$  and are (anti)holomorphic functions of  $t$ :

$$a_{\pm}(z) = z^{-K'/2} \prod_{F=1}^{N_f} \left[ e^{\pm i\pi K'} z \right]^{\Sigma_F^{\pm}} \prod_{A=1}^{N_a} \left[ e^{\pm i\pi K'} \right]^{\tilde{\Sigma}_A^{\pm}} G_{\pm}(z) \quad (3.5.21)$$

and the last function is  $G_{\pm}(z) = 1$  for  $N_a \leq N_f - 2$ ,  $G_{\pm}(z) = e^{\mp z}$  for  $N_a = N_f - 1$ , and  $G_{\pm}(z) = (1+z)^{K' - \sum_F \Sigma_F^{\pm} + \sum_A \tilde{\Sigma}_A^{\pm}}$  for  $N_a = N_f$ . The last two factors in (3.5.20) are the partition function of the dual theory with its mesons: shifts of  $\Sigma^{\pm}$  and  $\tilde{\Sigma}^{\pm}$  by  $\frac{1}{2}$  realize the map of R-charges (3.5.12). The factors  $a_{\pm}$  are ambiguities due to finite renormalization of the partition function, but in quiver gauge theories they become physical and have neat interpretations in terms of cluster algebras [41] or Liouville/Toda correlation functions [128]. The phase of  $a_+ a_-$  comes from a background twisted superpotential that depends on  $t$  and on the background field strength (twisted chiral) multiplets incorporating twisted masses and flavor fluxes. The absolute value is independent of these background fields and can be ignored for our purposes. It comes from improving the R-symmetry current. Ambiguities of the sphere partition function under multiplication by (anti)holomorphic functions of  $t$  play an important role in Chapter 4.

We will not elaborate on the comparison of B-type sphere partition functions performed very recently in [129]. It yields that if the electric theory is endowed with a superpotential  $W = W(\tilde{\phi}_A \phi_F)$ , then the magnetic theory has the superpotential  $W(M_{AF}) + M_{AF} \tilde{\phi}'_F \phi'_A$ . This is consistent with the matching of chiral rings  $M_{AF} = \tilde{\phi}_A \phi_F$  and  $\tilde{\phi}'_F \phi'_A = 0$ .

### 3.5.3 Variants of Seiberg duality

We now turn to consequences and analogues of the  $\mathcal{N}=(2,2)$  Seiberg duality.

The  $\mathcal{N}=(2,2)$   $SU(K)$  gauge theory with  $N_f$  fundamental chiral multiplets is dual to the theory with  $K \rightarrow K' = N_f - K$ , as described in [127]. Chiral rings are generated by baryons, which match provided R-charges are  $q'_F = -q_F + \sum_F q_F/K'$ . Chiral multiplets of the two theories are in the (anti)fundamental of an  $SU(N_f)$  flavor symmetry and have charges  $1/K$  and  $1/K'$  under a  $U(1)$  baryonic symmetry. Elliptic genera are shown to match in [67, 88]. A-type sphere partition functions are shown to match [11] by integrating partition functions of the analogous  $U(K)$  and  $U(N_f - K)$  theories:

$$\begin{aligned} Z_{SU(K)}^{N_f}(q_F) &= \int_0^{2\pi} \frac{d\vartheta}{2\pi} \int_{-\infty}^{\infty} 4\pi d\zeta Z_{U(K)}^{N_f}(q_F; \zeta, \vartheta) \\ &= \int_0^{2\pi} \frac{d\vartheta}{2\pi} \int_{-\infty}^{\infty} 4\pi d\zeta Z_{U(N_f-K)}^{N_f}(q'_F; -\zeta, -\vartheta + \#\pi) = Z_{SU(N_f-K)}^{N_f}(q'_F). \end{aligned} \quad (3.5.22)$$

We have used that partition functions of  $U(K)$  and  $U(N_f - K)$  theories are equal up to (3.5.21), namely powers of  $e^{-t}$  and  $e^{-\tilde{t}}$  that can be absorbed by shifting the Coulomb branch parameter  $\sigma$  and the flux  $\mathbf{m}$ . This shifts R-charges from  $1 - q_F$  to  $q'_F$  given above, and affects twisted masses and flavor fluxes in the same way, compatible with flavor symmetries.

In the presence of  $N_a \leq N_f - 2$  additional antifundamental chiral multiplets, all steps of (3.5.22) go through ( $\zeta$ -dependent factors prevent the last step for  $N_a = N_f - 1$  and  $N_a = N_f$ ) and yield

$$Z_{SU(K)}^{N_f, N_a}(q_F, \tilde{q}_A) = \prod_{F,A} \gamma(\tilde{q}_A/2 + q_F/2) Z_{SU(N_f-K)}^{N_a, N_f} \left( 2 - \tilde{q}_A + \frac{1}{K'} \sum_F q_F, -q_F + \frac{1}{K'} \sum_F q_F \right). \quad (3.5.23)$$

At first this suggests that the two theories may be dual. However, chiral rings do not match: the mesons  $\tilde{\phi}_A \phi_F$  and baryons  $\phi_{F_1} \wedge \cdots \wedge \phi_{F_K}$  of the electric theory match with the singlets and baryons of the magnetic theory, but there is no chiral operator in the magnetic theory with the same R-charge as antibaryons  $\tilde{\phi}_{A_1} \wedge \cdots \wedge \tilde{\phi}_{A_K}$ . The lack of duality is confirmed by noting that elliptic genera fail to match. A similar situation was observed in [30] where two GLSMs with equal  $Z_A$  were shown to flow to different SCFTs, whose Calabi-Yau target spaces thus have the same quantum Kähler moduli space despite having different complex structure moduli spaces.

The same technique gives pairs of  $U(K)$  and  $U(K')$  theories that have equal sphere partition functions but are not all dual. Start from the equality of partition functions of  $U(K)$  and  $U(N_f - K)$  theories with  $N_f$  fundamentals and  $N_a \leq N_f - 2$  antifundamentals and additional singlets for the magnetic theory<sup>36</sup>. Add  $L$  singlets on both sides and gauge a  $U(1) \subset S[U(N_f) \times U(N_a)] \times U(1)^L$  flavor symmetry, then shift its generator by that of  $U(1) \subset U(K)$  or  $U(1) \subset U(N_f - K)$ . Integrate over FI and theta parameters associated to the mixed  $U(1)$ . This yields partition functions of  $U(K)$  and  $U(N_f - K)$  theories with matter in  $N_f$  fundamental,  $N_a$  antifundamental, and  $L$  singlet representations of the  $SU$  gauge group and with arbitrary  $U(1)$  gauge charges. As in dualities above, the magnetic theory has  $N_f N_a$  additional singlets, now charged under the  $U(1)$  gauge group. Despite sphere partition functions being equal, the theories are not expected to be dual in general: their chiral rings typically do not match due to antibaryons dressed by singlets. It would be interesting to find out which of these pairs of theories are indeed dual. In [127], the duality was established for  $N_a = 0$ ,  $L = 1$ , and with a superpotential  $W = P G_d(B)$  where  $P$  is the additional singlet in the  $\det^{-d}$  representation of  $U(K)$ , and  $G_d(B)$  is a degree  $d$  polynomial in the baryons  $B$ . See also [130] for the case of  $N_a = 1$  multiplets in the  $\square \otimes \det^{-1}$  representation and other negative powers of  $\det$  (then chiral rings contain no  $U(1)$ -invariant antibaryons).

Quiver gauge theories with  $U(N_i)$  gauge and flavor symmetry factors and bifundamental chiral multiplets have multiple duals. These are obtained by gauging part of the flavor symmetry  $S[U(N_f) \times U(N_a)]$  in the duality between  $U(K)$  and  $U(\max(N_a, N_f) - K)$  theories above. Denote by  $a_{ij} \geq 0$  the number of chiral multiplets in the antifundamental representation of  $U(N_i)$  and the fundamental of  $U(N_j)$  for  $i \neq j$ . Let  $N_f(k) = \sum_i N_i a_{ik}$  and  $N_a(k) = \sum_j a_{kj} N_j$  be the numbers of (anti)fundamental chiral multiplets for the node  $U(N_k)$ . For any gauge factor  $U(N_k)$  there exists a dual with

$$N_k \rightarrow N'_k = \max\left(N_f(k), N_a(k)\right) - N_k, \quad a'_{ij} = \begin{cases} a_{ij} + a_{ik} a_{kj} & \text{if } i \neq k \text{ and } j \neq k \\ a_{ji} & \text{if } i = k \text{ or } j = k \end{cases} \quad (3.5.24)$$

with cubic superpotential terms coupling the  $N_j a'_{jk} = a_{kj} N_j$  fundamental and  $a'_{ki} N_i = N_i a_{ik}$  antifundamental chiral multiplets of  $U(N'_k)$  with the corresponding  $N_i a_{ik} a_{kj} N_j$  singlets of  $U(N'_k)$  while preserving the  $U(N_i)$  and  $U(N_j)$  symmetries. The map of (complexified) FI parameters is more elaborate: for example in quivers with all  $N_a(i) = N_f(i)$  so that FI

<sup>36</sup>To ease the parallel description of dual theories we have charge conjugated one theory.

parameters do not run

$$z'_k = z_k^{-1} \quad \text{and for } k \neq i, \quad z'_i = z_i z_k^{a_{ki}} (z_k + 1)^{a_{ik} - a_{ki}} \quad (3.5.25)$$

in terms of the Kähler parameters  $z_j = \exp(-t_j + i\pi(N_f(j) - N_j))$ . One can typically apply further Seiberg dualities to other nodes in the quiver, obtaining a web of dualities. However, after dualizing the node  $U(N_k)$ , the quiver gauge theory involves adjoint matter if  $a_{ik} \neq 0 \neq a_{ki}$  for some  $i$ : then one cannot apply Seiberg duality to  $U(N_i)$ . This motivates the restriction to quivers such that for any of the dual descriptions, whenever  $a_{ij} \neq 0 \neq a_{ji}$  for some  $i \neq j$ , there exists a quadratic superpotential giving mass to  $2 \min(a_{ij}, a_{ji})$  of these bifundamental chiral multiplets, which can thus be removed without affecting the infrared limit. The condition is difficult to check, but has been proven for various classes of quivers. Then all dual quivers can be taken to have  $a_{ij} = 0$  or  $a_{ji} = 0$  for all  $i, j$ , and the matter content is equally described by the antisymmetric matrix  $B_{ij} = a_{ij} - a_{ji}$ . In [41] it was observed that  $B$ , together with the beta function of FI parameters, and the  $z_j$ , reproduce the structure of cluster seeds. Dualities act on this data as cluster mutations. The connection between cluster algebras and 2d  $\mathcal{N}=(2, 2)$  quiver dualities is stronger than in higher dimensions, as it concerns not only the quiver described by  $B$  but also cluster coefficients and cluster variables.

Seiberg duality can also be realized as an explicit symmetry in a 2d CFT [128]: the A-type sphere partition function of  $U(K)$  gauge theories with  $N_f$  fundamental and  $N_a \leq N_f$  antifundamental chiral multiplets is equal to a correlator in the  $A_{N_f-1}$  Toda CFT. Toda CFT charge conjugation reproduces precisely  $K' = N_f - K$  and the map of FI parameters, R-charges and twisted masses. This instance of the AGT correspondence goes further: one can include adjoint matter and obtain two other dualities.

- A generalization of  $\mathcal{N}=(2, 2)^*$  dualities studied in [41]. The duality relates  $U(K)$  and  $U(K')$  gauge theories with  $N$  fundamental,  $N$  antifundamental and one adjoint chiral multiplet  $X$  with a superpotential  $W = \sum_{F=1}^N \tilde{\phi}_F X^{l_F} \phi_F$  for arbitrary integers  $l_F \geq 0$ . The magnetic theory has  $K' = \sum_F l_F - K$  colors (for  $K' < 0$  supersymmetry is broken and there is no duality). When all  $l_F = 1$ , the theories are  $\mathcal{N}=(2, 2)^*$  theories (mass deformations of  $\mathcal{N}=(4, 4)$  SQCD). A-type sphere partition functions of the two theories were proven to be equal in [128]. Chiral rings are generated by  $\tilde{\phi}_A X^k \phi_F$  with  $0 \leq k < l_A, l_F$  and by  $\text{Tr } X^k$  for  $0 \leq k < K$  or  $0 \leq k < K'$  depending on the theory. This mismatch has not been investigated but might be cured by the superpotential. Just like Seiberg duality, (part of the) flavor symmetries can be gauged to produce dualities between quivers.
- An  $\mathcal{N}=(2, 2)$  Kutasov-Schwimmer duality. The electric theory has  $U(K)$  gauge group with  $N_f$  fundamentals,  $N_a$  antifundamentals and one adjoint  $X$  with superpotential  $W = \text{Tr } X^{l+1}$  for some  $l \geq 1$ . The magnetic theory is identical with  $(K, N_f, N_a, l) \rightarrow (\max(N_f, N_a)l - K, N_a, N_f, l)$  and  $lN_f N_a$  gauge singlets  $M_{jFA}$  for  $0 \leq j < l$ , with a superpotential  $W = M_{jAF} \tilde{\phi}'_F X'^j \phi'_A + \text{Tr } X'^{(l+1)}$ . Chiral rings match under  $X \rightarrow X'$  and  $\tilde{\phi}_A X^j \phi_F \rightarrow M_{jAF}$ . A-type sphere partition functions were proven to be equal in [128].

It would be interesting to investigate the existence of analogues of Brodie dualities, where the electric and magnetic theories have two adjoint chiral multiplets  $X$  and  $Y$  subject to a superpotential  $W = \text{Tr}(X^{k+1} + XY^2)$ .

Orthogonal and symplectic gauge groups were considered by Hori [131]. For instance, the  $USp(2k)$  gauge theory with  $2p + 1$  fundamentals  $\phi_I$  and  $m$  singlets  $M^a$  subject to a cubic superpotential  $W = A_a^{[IJ]} M^a \langle \phi_I, \phi_J \rangle$  with generic coefficients  $A_a^{[IJ]}$  is dual to the theory with  $k \rightarrow p - k$  and  $m \rightarrow \binom{2p+1}{2} - m$  provided these numbers are positive. Sphere partition functions of these dual theories have not been compared: the usual method of comparing Higgs branch expressions fails due to the absence of FI parameter. Gauging a  $U(1)$  flavor symmetry gives further dualities [30, 132], whose gauge group  $U(1) \times USp(2k)$  (and its  $\mathbb{Z}_2$  quotient) allow FI-theta parameters. Sphere partition functions have been compared for theories whose low-energy limit has a Calabi-Yau threefold target space. Presumably, integrating over the FI-theta parameters as in (3.5.22) should help prove that Hori duals have equal A-type sphere partition function.

### 3.5.4 $\mathcal{N}=(0, 2)$ trialities

We describe dualities [118] between  $\mathcal{N}=(0, 2)$  theories with a gauge group  $U(K)$  and (anti)fundamental matter. The theories are expected to flow at intermediate energy scales to NLSMs on bundles over Grassmannians [133] and each duality is due to an isomorphism between bundles over  $Gr(K, N)$  and  $Gr(N - K, N)$  [134].

We let  $N_P, N_\Phi, N_\Psi$  denote the number of antifundamental chirals  $P$ , fundamental chirals  $\Phi$ , and antifundamental Fermi multiplets  $\Psi$  (which could be mapped to fundamental ones by exchanging  $E$  and  $J$  interactions). The  $SU(K)$  gauge anomaly  $N_P/2 + N_\Phi/2 - N_\Psi/2 - K$  due to fermions in the matter and vector multiplets must vanish, thus  $K = (N_P + N_\Phi - N_\Psi)/2$ . The  $U(1)$  gauge anomaly  $N_P K + N_\Phi K - N_\Psi K = 2K^2$  of these multiplets is cancelled<sup>37</sup> by adding two Fermi multiplets  $\Omega_{1,2}$  with  $U(1)$  charge  $K$ , *i.e.*, in the determinant representation of  $U(K)$ . For convenience, we also include  $N_P N_\Phi$  neutral Fermi multiplets  $\Gamma$  with a J-term interaction  $\Gamma P \Phi$ .

Theories with  $(N_P, N_\Phi, N_\Psi)$  equal to the same  $(N_1, N_2, N_3)$  up to cyclic permutations, depicted by the quivers in Figure 3.1, are expected to flow to the same infrared fixed point. As evidence, we show that the elliptic genus<sup>38</sup> is invariant under cyclic permutations of  $(N_P, N_\Phi, N_\Psi)$ . The classical flavor symmetry is  $S[U(N_P) \times U(N_\Phi) \times U(N_\Psi) \times U(2)]$  with holonomies  $(\xi_i^P, \xi_i^\Phi, \xi_i^\Psi, \xi_i^\Omega)$  modulo gauge transformations, but mixed flavor-gauge anomalies reduce Abelian symmetries to a two-dimensional subgroup: this can be used for instance to fix the  $U(1)_\Omega$  holonomy  $\sum_i \xi_i^\Omega = -\sum_i \xi_i^P - \sum_i \xi_i^\Phi + \sum_i \xi_i^\Psi$  (we took  $\Phi$  in the  $\square$  of  $SU(N_\Phi)$ ). Up to a constant, the elliptic genus is a sum of residues of

$$\frac{\prod_{\ell=1}^2 \theta(\xi_\ell^\Omega + \sum_a u_a) \prod_{a=1}^K \prod_{i=1}^{N_\Psi} \theta(\xi_i^\Psi - u_a) \prod_{j=1}^{N_P} \prod_{k=1}^{N_\Phi} \theta(\xi_j^P - \xi_k^\Phi)}{\prod_{a=1}^K \prod_{i=1}^{N_P} \theta(\xi_i^P - u_a) \prod_{j=1}^{N_\Phi} \theta(u_a - \xi_j^\Phi)} \prod_{a \neq b}^K \theta(u_a - u_b) \theta'(0)^K d^K u$$

<sup>37</sup>One could consider  $SU(K)$  gauge theories and omit  $\Omega_{1,2}$ .

<sup>38</sup>While [118] work in the NSNS sector we work in the RR sector; results are related by spectral flow.

|             | $P$          | $\Phi$       | $\Psi$       | $\Gamma$     | $\Omega$     |
|-------------|--------------|--------------|--------------|--------------|--------------|
| $U(K)$      | $\square$    | $\square$    | $\square$    | $\mathbf{1}$ | $\det$       |
| $U(N_P)$    | $\square$    | $\mathbf{1}$ | $\mathbf{1}$ | $\square$    | $\mathbf{1}$ |
| $U(N_\Phi)$ | $\mathbf{1}$ | $\square$    | $\mathbf{1}$ | $\square$    | $\mathbf{1}$ |
| $U(N_\Psi)$ | $\mathbf{1}$ | $\mathbf{1}$ | $\square$    | $\mathbf{1}$ | $\mathbf{1}$ |
| $SU(2)$     | $\mathbf{1}$ | $\mathbf{1}$ | $\mathbf{1}$ | $\mathbf{1}$ | $\square$    |

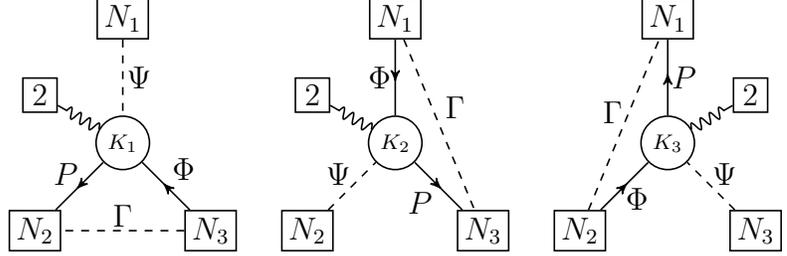

Figure 3.1: Quivers for three  $\mathcal{N}=(0, 2)$  theories related by triality:  $K_i = (N_1 + N_2 + N_3)/2 - N_i$  and  $(N_P, N_\Phi, N_\Psi)$  is one of  $(N_2, N_3, N_1)$ ,  $(N_3, N_1, N_2)$ ,  $(N_1, N_2, N_3)$ . The table lists how the chirals  $P, \Phi$  and Fermis  $\Psi, \Gamma, \Omega$  transform under the gauge group  $U(K) = U(\frac{1}{2}(N_P + N_\Phi - N_\Psi))$  and the classical flavor symmetry  $S[U(N_P) \times U(N_\Phi) \times U(N_\Psi) \times U(2)]$  which loses one Abelian factor due to a flavor-gauge anomaly.

where  $\theta(u) = \theta_1(\tau|u)/i\eta(q) = -\theta(-u)$  has zeros at  $\mathbb{Z} + \tau\mathbb{Z}$ , no poles, and  $\theta'(0) = 2\pi i\eta(q)^2$ . Several sets of poles give the same sum of residues: poles due to  $P$  (at  $\{u_a\} = \{\xi_j^P | j \in J\}$  for each set of  $K$  distinct flavors  $J \subset \{1, \dots, N_P\}$ ) with residue

$$\frac{\prod_{\ell=1}^2 \theta(\xi_\ell^\Omega + \sum_{j \in J} \xi_j^P) \prod_{j \in J} \prod_{i=1}^{N_\Psi} \theta(\xi_i^\Psi - \xi_j^P) \prod_{j \notin J} \prod_{k=1}^{N_\Phi} \theta(\xi_j^P - \xi_k^\Phi)}{\prod_{j \in J} \prod_{i \notin J} \theta(\xi_i^P - \xi_j^P)}; \quad (3.5.26)$$

or poles due to  $\Phi$  (at  $\{u_a\} = \{\xi_j^\Phi | j \in J\}$  for  $J \subset \{1, \dots, N_\Phi\}$ ) with residue

$$\frac{\prod_{\ell=1}^2 \theta(\xi_\ell^\Omega + \sum_{j \in J} \xi_j^\Phi) \prod_{j \notin J} \prod_{i=1}^{N_P} \theta(\xi_i^P - \xi_j^\Phi) \prod_{j \in J} \prod_{k=1}^{N_\Psi} \theta(\xi_k^\Psi - \xi_j^\Phi)}{\prod_{j \in J} \prod_{i \notin J} \theta(\xi_i^\Phi - \xi_j^\Phi)}. \quad (3.5.27)$$

Up to a sign, (3.5.26) is mapped to (3.5.27) under  $(N_P, \xi^P) \rightarrow (N_\Phi, \xi^\Phi) \rightarrow (N_\Psi, \xi^\Psi) \rightarrow (N_P, \xi^P)$  and  $J \rightarrow J^c$ . One also has a shift  $\xi_i^\Omega \rightarrow \xi_i^\Omega - \sum_j \xi_j^\Omega - \sum_j \xi_j^P$  fixed by the above constraint on  $\sum \xi^\Omega$ . Elliptic genera of theories in Figure 3.1 are thus equal, with  $S[U(N_1) \times U(N_2) \times U(N_3) \times SU(2)]$  flavor symmetries identified. Another outcome of the calculation is that the elliptic genus vanishes if  $K > N_P$  or  $K > N_\Phi$  in any frame, which is equivalent to  $K < 0$  in a dual frame. This suggests that supersymmetry is broken unless  $(N_1, N_2, N_3)$  obey the triangle inequality.

Lack of space forces us to only mention variants of the Gaiotto-Gukov-Putrov triality. Gauging flavor symmetries leads to dualities between  $\mathcal{N}=(0, 2)$  quiver gauge theories with bifundamental chiral/Fermi multiplets and Fermi multiplets in determinant representations; however, most quivers have either gauge anomalies or spontaneous supersymmetry breaking. Such quivers were obtained from brane brick models in [135]. As shown in [136], a twisted dimensional reduction of the 6d (2,0) theory on  $S^2 \times \Sigma$  yields  $\mathcal{N}=(0, 4)$  Lagrangians labelled by pants decompositions of  $\Sigma$ , and changes in pants decomposition give  $\mathcal{N}=(0, 4)$  dualities. Similarly, twisted dimensional reductions on  $S^2$  of 4d  $\mathcal{N}=1$  and 4d  $\mathcal{N}=2$  dualities yield two-dimensional (0, 2) or (0, 4) or (2, 2) dualities [137], in particular an  $SU(K)$  variant of the (0, 2) triality above. All of these dualities are checked by comparing elliptic genera. The dimensional reduction is based on [9, 138] (see also [139–141]).

## 3.6 Conclusion

We have reviewed the main localization calculations in two dimensions on the sphere (section 3.2), other curved backgrounds (section 3.3) and the torus (section 3.4), and discussed applications to mirror symmetry and gauge theory dualities (section 3.5). We now conclude this review by mentioning other developments.

Two-dimensional gauge theory descriptions of several non-critical strings in 6d SCFTs have been tested by comparing topological vertex results to the elliptic genus of a string. As discussed in Chapter 17, this was done for M-strings [123, 142–144] (namely M2-branes suspended between M5-branes), E-strings [145, 146] (M2-branes suspended between M5- and M9-branes), little strings [147] (strings on type IIA or IIB NS5-branes), and for a class of 6d  $\mathcal{N}=(1, 0)$  SCFTs engineered from F-theory [148, 149].

Nekrasov’s instanton partition function of 4d  $\mathcal{N}=2$  theories such as  $SU(N)$  super-Yang-Mills can be reproduced by an appropriate (R-preserving)  $S^2$  partition function [150].<sup>39</sup> The 4d theory is engineered by  $N$  fractional D3-branes on  $\mathbb{C}^2/\mathbb{Z}_2$  and its instantons by  $k$  D(−1)-branes. Blowing up the singular point yields a D1–D5 brane system, described in the gauge theory limit by a 2d  $\mathcal{N}=(2, 2)$   $U(k)$  GLSM on the blown-up sphere  $\mathbb{C}P^1$ . In the zero-radius limit, its sphere partition function reproduces the equivariant volume of the ADHM moduli space of  $k$  instantons, while for non-zero radius it captures genus zero Gromov-Witten invariants of the ADHM moduli space [16, 152]. This construction was later used to extract spectra of hydrodynamic quantum integrable systems [153, 154].

Another appearance of integrable models in relation to 2d localization is that elliptic genera give solutions to Yang-Baxter equations [155, 156]. In this context, the Yang-Baxter equation amounts to the invariance of the genus under  $\mathcal{N}=(2, 2)$  Seiberg-like dualities.

We have already mentioned that twisted dimensional reductions of 4d  $\mathcal{N}=1$  theories on a sphere yield 2d  $\mathcal{N}=(0, 2)$  theories and that 4d dualities become 2d dualities. The 2d  $\mathcal{N}=(0, 2)$  elliptic genus is thus a limit of a  $T^2 \times S^2$  partition function [9]. Similarly, the partition function of 3d  $\mathcal{N}=2$  theories on Lens spaces, described in Chapter 6, reduces to an  $S^2$  partition function when the circle fiber of the Lens space shrinks to zero size (see also [158, 159]). The  $S^2$  partition function also appears when localizing 4d  $\mathcal{N}=2$  theories on  $S^4$  on their Higgs branch [160, 161].

In four-dimensional supersymmetric gauge theories, a class of surface operators can be constructed by coupling a two-dimensional theory to the bulk fields supersymmetrically (see also Chapter 10). Superconformal indices of coupled 2d/4d systems were computed in [88] (see [163, 164] for related 5d calculations) and led to discovering the node-hopping duality (see also [165]): coupling the same 2d  $\mathcal{N}=(2, 2)$  theory to different fields in a 4d  $\mathcal{N}=2$  quiver theory gives the same surface operator at low energies. The AGT correspondence relates the node-hopping duality to crossing symmetry in a 2d CFT [128]: the  $S^4$  partition function of the 4d theory is identified with a Toda CFT correlator, adding a surface operator on  $S^2 \subset S^4$  corresponds to inserting a (degenerate) vertex operator in the correlator, and different

---

<sup>39</sup>In a different approach [151], for 4d  $\mathcal{N}=2$  theories engineered by string theories on a Calabi-Yau three-fold  $X$ , the Seiberg-Witten Kähler potential can be obtained as that of  $X$ , itself derived from the  $S^2$  partition function of a GLSM flowing to an NLSM on  $X$ .

choices of couplings correspond to different OPEs of that vertex operator with others. Kähler parameters (the 4d gauge coupling and 2d FI/theta parameters) correspond to positions of vertex operators in the correlator and are expected to transform non-trivially under node-hopping. The map could be found by comparing  $S^2 \subset S^4$  partition functions of these 2d/4d systems, but instanton-vortex partition functions which appear when localizing [166] are unknown. It would be interesting to derive them.

## Acknowledgements

We are grateful to Nikolay Bobev, Cyril Closset, Stefano Cremonesi, Nima Doroud, Richard Eager, Jaume Gomis, Kentaro Hori, Sungjay Lee, Daniel S. Park, Mauricio Romo, Yuji Tachikawa, Ran Yacoby, Alberto Zaffaroni and Peng Zhao for collaborations and insightful discussions over the years on some of the material presented here. F.B. is supported in part by the Royal Society as a Royal Society University Research Fellowship holder, and by the MIUR-SIR grant RBSI1471GJ “Quantum Field Theories at Strong Coupling: Exact Computations and Applications”.

## References

- [1] V. Pestun and M. Zabzine, eds., *Localization techniques in quantum field theory*, vol. xx. Journal of Physics A, 2016. 1608.02952. <https://arxiv.org/src/1608.02952/anc/LocQFT.pdf>, <http://pestun.ihep.fr/pages/LocalizationReview/LocQFT.pdf>.
- [2] N. Seiberg, “Electric - magnetic duality in supersymmetric nonAbelian gauge theories,” *Nucl. Phys.* **B435** (1995) 129–146, [arXiv:hep-th/9411149](https://arxiv.org/abs/hep-th/9411149) [hep-th].
- [3] E. Witten, “Phases of N=2 theories in two-dimensions,” *Nucl. Phys.* **B403** (1993) 159–222, [arXiv:hep-th/9301042](https://arxiv.org/abs/hep-th/9301042) [hep-th].
- [4] G. Festuccia and N. Seiberg, “Rigid Supersymmetric Theories in Curved Superspace,” *JHEP* **06** (2011) 114, [arXiv:1105.0689](https://arxiv.org/abs/1105.0689) [hep-th].
- [5] T. Dumitrescu, “An Introduction to Supersymmetric Field Theories in Curved Space,” *Journal of Physics A* **xx** (2016) 000, 1608.02957.
- [6] C. Closset and S. Cremonesi, “Comments on  $\mathcal{N} = (2, 2)$  supersymmetry on two-manifolds,” *JHEP* **07** (2014) 075, [arXiv:1404.2636](https://arxiv.org/abs/1404.2636) [hep-th].
- [7] J. Bae, C. Imbimbo, S.-J. Rey, and D. Rosa, “New Supersymmetric Localizations from Topological Gravity,” *JHEP* **03** (2016) 169, [arXiv:1510.00006](https://arxiv.org/abs/1510.00006) [hep-th].
- [8] E. Witten, “Topological Sigma Models,” *Commun. Math. Phys.* **118** (1988) 411.
- [9] F. Benini and A. Zaffaroni, “A topologically twisted index for three-dimensional supersymmetric theories,” *JHEP* **07** (2015) 127, [arXiv:1504.03698](https://arxiv.org/abs/1504.03698) [hep-th].
- [10] C. Closset, S. Cremonesi, and D. S. Park, “The equivariant A-twist and gauged linear sigma models on the two-sphere,” *JHEP* **06** (2015) 076, [arXiv:1504.06308](https://arxiv.org/abs/1504.06308) [hep-th].
- [11] F. Benini and S. Cremonesi, “Partition Functions of  $\mathcal{N} = (2, 2)$  Gauge Theories on  $S^2$  and Vortices,” *Commun. Math. Phys.* **334** (2015) no. 3, 1483–1527, [arXiv:1206.2356](https://arxiv.org/abs/1206.2356) [hep-th].

- [12] N. Doroud, J. Gomis, B. Le Floch, and S. Lee, “Exact Results in D=2 Supersymmetric Gauge Theories,” *JHEP* **05** (2013) 093, [arXiv:1206.2606 \[hep-th\]](#).
- [13] J. Gomis and S. Lee, “Exact Kahler Potential from Gauge Theory and Mirror Symmetry,” *JHEP* **04** (2013) 019, [arXiv:1210.6022 \[hep-th\]](#).
- [14] V. Pestun, “Localization of gauge theory on a four-sphere and supersymmetric Wilson loops,” *Commun. Math. Phys.* **313** (2012) 71–129, [arXiv:0712.2824 \[hep-th\]](#).
- [15] J. Halverson, V. Kumar, and D. R. Morrison, “New Methods for Characterizing Phases of 2D Supersymmetric Gauge Theories,” *JHEP* **09** (2013) 143, [arXiv:1305.3278 \[hep-th\]](#).
- [16] G. Bonelli, A. Sciarappa, A. Tanzini, and P. Vasko, “Vortex partition functions, wall crossing and equivariant Gromov-Witten invariants,” *Commun. Math. Phys.* **333** (2015) no. 2, 717–760, [arXiv:1307.5997 \[hep-th\]](#).
- [17] D. Morrison, “Gromov-Witten invariants and localization,” *Journal of Physics A* (2016) , 1608.02956.
- [18] H. Jockers, V. Kumar, J. M. Lapan, D. R. Morrison, and M. Romo, “Two-Sphere Partition Functions and Gromov-Witten Invariants,” *Commun. Math. Phys.* **325** (2014) 1139–1170, [arXiv:1208.6244 \[hep-th\]](#).
- [19] E. Gerchkovitz, J. Gomis, and Z. Komargodski, “Sphere Partition Functions and the Zamolodchikov Metric,” *JHEP* **11** (2014) 001, [arXiv:1405.7271 \[hep-th\]](#).
- [20] J. Gomis, Z. Komargodski, P.-S. Hsin, A. Schwimmer, N. Seiberg, and S. Theisen, “Anomalies, Conformal Manifolds, and Spheres,” [arXiv:1509.08511 \[hep-th\]](#).
- [21] N. Doroud and J. Gomis, “Gauge theory dynamics and Kahler potential for Calabi-Yau complex moduli,” *JHEP* **12** (2013) 99, [arXiv:1309.2305 \[hep-th\]](#).
- [22] S. Sugishita and S. Terashima, “Exact Results in Supersymmetric Field Theories on Manifolds with Boundaries,” *JHEP* **11** (2013) 021, [arXiv:1308.1973 \[hep-th\]](#).
- [23] D. Honda and T. Okuda, “Exact results for boundaries and domain walls in 2d supersymmetric theories,” *JHEP* **09** (2015) 140, [arXiv:1308.2217 \[hep-th\]](#).
- [24] K. Hori and M. Romo, “Exact Results In Two-Dimensional (2,2) Supersymmetric Gauge Theories With Boundary,” [arXiv:1308.2438 \[hep-th\]](#).
- [25] H. Kim, S. Lee, and P. Yi, “Exact partition functions on  $\mathbb{RP}^2$  and orientifolds,” *JHEP* **02** (2014) 103, [arXiv:1310.4505 \[hep-th\]](#).
- [26] C. Closset, W. Gu, B. Jia, and E. Sharpe, “Localization of twisted  $\mathcal{N}=(0,2)$  gauged linear sigma models in two dimensions,” [arXiv:1512.08058 \[hep-th\]](#).
- [27] N. Hama, K. Hosomichi, and S. Lee, “SUSY Gauge Theories on Squashed Three-Spheres,” *JHEP* **05** (2011) 014, [arXiv:1102.4716 \[hep-th\]](#).
- [28] N. Hama and K. Hosomichi, “Seiberg-Witten Theories on Ellipsoids,” *JHEP* **09** (2012) 033, [arXiv:1206.6359 \[hep-th\]](#). [Addendum: *JHEP*10,051(2012)].
- [29] P. Goddard, J. Nuyts, and D. I. Olive, “Gauge Theories and Magnetic Charge,” *Nucl. Phys.* **B125** (1977) 1.
- [30] K. Hori and J. Knapp, “Linear sigma models with strongly coupled phases - one parameter models,” *JHEP* **11** (2013) 070, [arXiv:1308.6265 \[hep-th\]](#).
- [31] K. Hori, C. Y. Park, and Y. Tachikawa, “2d SCFTs from M2-branes,” *JHEP* **11** (2013) 147, [arXiv:1309.3036 \[hep-th\]](#).

- [32] M. Fujitsuka, M. Honda, and Y. Yoshida, “Higgs branch localization of 3d  $\mathcal{N} = 2$  theories,” *PTEP* **2014** (2014) no. 12, 123B02, [arXiv:1312.3627 \[hep-th\]](#).
- [33] F. Benini and W. Peelaers, “Higgs branch localization in three dimensions,” *JHEP* **05** (2014) 030, [arXiv:1312.6078 \[hep-th\]](#).
- [34] W. Peelaers, “Higgs branch localization of  $\mathcal{N} = 1$  theories on  $S^3 \times S^1$ ,” *JHEP* **08** (2014) 060, [arXiv:1403.2711 \[hep-th\]](#).
- [35] Y. Yoshida, “Factorization of 4d  $\mathcal{N}=1$  superconformal index,” [arXiv:1403.0891 \[hep-th\]](#).
- [36] T. Fujimori, T. Kimura, M. Nitta, and K. Ohashi, “2d Partition Function in Omega-background and Vortex/Instanton Correspondence,” *JHEP* **12** (2015) 110, [arXiv:1509.08630 \[hep-th\]](#).
- [37] M. F. Atiyah and R. Bott, “The Moment map and equivariant cohomology,” *Topology* **23** (1984) 1–28.
- [38] N. Berline and M. Vergne, “Classes caractéristiques équivariantes. Formule de localisation en cohomologie équivariante,” *C.R.Acad.Sci.Paris* **295** (1982) 539–541.
- [39] G. ’t Hooft, “On the Phase Transition Towards Permanent Quark Confinement,” *Nucl. Phys.* **B138** (1978) 1.
- [40] E. Gerchkovitz, J. Gomis, N. Ishtiaque, A. Karasik, Z. Komargodski, and S. S. Pufu, “Correlation Functions of Coulomb Branch Operators,” [arXiv:1602.05971 \[hep-th\]](#).
- [41] F. Benini, D. S. Park, and P. Zhao, “Cluster Algebras from Dualities of 2d  $\mathcal{N} = (2, 2)$  Quiver Gauge Theories,” *Commun. Math. Phys.* **340** (2015) no. 1, 47–104, [arXiv:1406.2699 \[hep-th\]](#).
- [42] E. Witten, “The Verlinde algebra and the cohomology of the Grassmannian,” [arXiv:hep-th/9312104 \[hep-th\]](#).
- [43] K. Hosomichi, “Orbifolds, Defects and Sphere Partition Function,” [arXiv:1507.07650 \[hep-th\]](#).
- [44] I. Biswas, “Parabolic bundles as orbifold bundles,” *Duke Math. J.* **88** (1997) no. 2, 305–325. <http://dx.doi.org/10.1215/S0012-7094-97-08812-8>.
- [45] K. Hori and C. Vafa, “Mirror symmetry,” [arXiv:hep-th/0002222 \[hep-th\]](#).
- [46] E. Witten, “Mirror manifolds and topological field theory,” [arXiv:hep-th/9112056 \[hep-th\]](#).
- [47] T. Buscher, U. Lindstrom, and M. Rocek, “New Supersymmetric  $\sigma$  Models With Wess-Zumino Terms,” *Phys. Lett.* **B202** (1988) 94.
- [48] U. Lindstrom, M. Rocek, I. Ryb, R. von Unge, and M. Zabzine, “New  $\mathcal{N} = (2,2)$  vector multiplets,” *JHEP* **08** (2007) 008, [arXiv:0705.3201 \[hep-th\]](#).
- [49] S. J. Gates, Jr., C. M. Hull, and M. Rocek, “Twisted Multiplets and New Supersymmetric Nonlinear Sigma Models,” *Nucl. Phys.* **B248** (1984) 157.
- [50] M. Gualtieri, *Generalized Complex Geometry*. PhD thesis, Oxford University, 2003. [arXiv:math/0401221 \[math.DG\]](#).
- [51] M. Gualtieri, “Generalized Complex Geometry,” *Ann. of Math. (2)* **174** (2011) 75–123, [arXiv:math/0703298 \[math.DG\]](#).
- [52] F. Benini, P. M. Cricigno, D. Jain, and J. Nian, “Semichiral Fields on  $S^2$  and Generalized Kähler Geometry,” [arXiv:1505.06207 \[hep-th\]](#).
- [53] H. Ooguri, Y. Oz, and Z. Yin, “D-branes on Calabi-Yau spaces and their mirrors,” *Nucl. Phys.* **B477** (1996) 407–430, [arXiv:hep-th/9606112 \[hep-th\]](#).
- [54] K. Hori, A. Iqbal, and C. Vafa, “D-branes and mirror symmetry,” [arXiv:hep-th/0005247 \[hep-th\]](#).

- [55] M. Herbst, K. Hori, and D. Page, “Phases Of  $N=2$  Theories In 1+1 Dimensions With Boundary,” [arXiv:0803.2045 \[hep-th\]](#).
- [56] R. Minasian and G. W. Moore, “K theory and Ramond-Ramond charge,” *JHEP* **11** (1997) 002, [arXiv:hep-th/9710230 \[hep-th\]](#).
- [57] N. P. Warner, “Supersymmetry in boundary integrable models,” *Nucl. Phys.* **B450** (1995) 663–694, [arXiv:hep-th/9506064 \[hep-th\]](#).
- [58] A. Sen, “Tachyon condensation on the brane anti-brane system,” *JHEP* **08** (1998) 012, [arXiv:hep-th/9805170 \[hep-th\]](#).
- [59] S. Hosono, “Central charges, symplectic forms, and hypergeometric series in local mirror symmetry,” [arXiv:hep-th/0404043 \[hep-th\]](#).
- [60] L. Katzarkov, M. Kontsevich, and T. Pantev, “Hodge theoretic aspects of mirror symmetry,” [arXiv:0806.0107 \[math.AG\]](#).
- [61] H. Iritani, “An integral structure in quantum cohomology and mirror symmetry for toric orbifolds,” *Adv. Math.* **222** (2009) no. 3, 1016–1079, [0903.1463 \[math.AG\]](#).
- [62] J. Halverson, H. Jockers, J. M. Lapan, and D. R. Morrison, “Perturbative Corrections to Kaehler Moduli Spaces,” *Commun. Math. Phys.* **333** (2015) no. 3, 1563–1584, [arXiv:1308.2157 \[hep-th\]](#).
- [63] E. Witten, “Topological Quantum Field Theory,” *Commun. Math. Phys.* **117** (1988) 353.
- [64] D. R. Morrison and M. R. Plesser, “Summing the instantons: Quantum cohomology and mirror symmetry in toric varieties,” *Nucl. Phys.* **B440** (1995) 279–354, [arXiv:hep-th/9412236 \[hep-th\]](#).
- [65] A. B. Givental, “Equivariant Gromov-Witten Invariants,” *Internat. Math. Res. Notices* **13** (1996) 613, [arXiv:alg-geom/9603021 \[alg-geom\]](#).
- [66] L. C. Jeffrey and F. C. Kirwan, “Localization for nonabelian group actions,” *Topology* **34** (1995) no. 2, 291–327, [arXiv:alg-geom/9307001](#). [http://dx.doi.org/10.1016/0040-9383\(94\)00028-J](http://dx.doi.org/10.1016/0040-9383(94)00028-J).
- [67] F. Benini, R. Eager, K. Hori, and Y. Tachikawa, “Elliptic Genera of 2d  $\mathcal{N} = 2$  Gauge Theories,” *Commun. Math. Phys.* **333** (2015) no. 3, 1241–1286, [arXiv:1308.4896 \[hep-th\]](#).
- [68] T. T. Dumitrescu and N. Seiberg, “Supercurrents and Brane Currents in Diverse Dimensions,” *JHEP* **07** (2011) 095, [arXiv:1106.0031 \[hep-th\]](#).
- [69] M. F. Sohnius and P. C. West, “An Alternative Minimal Off-Shell Version of  $N=1$  Supergravity,” *Phys. Lett.* **B105** (1981) 353.
- [70] M. Sohnius and P. C. West, “The Tensor Calculus and Matter Coupling of the Alternative Minimal Auxiliary Field Formulation of  $N = 1$  Supergravity,” *Nucl. Phys.* **B198** (1982) 493.
- [71] S. J. Gates, M. T. Grisaru, M. Rocek, and W. Siegel, “Superspace Or One Thousand and One Lessons in Supersymmetry,” *Front. Phys.* **58** (1983) 1–548, [arXiv:hep-th/0108200 \[hep-th\]](#).
- [72] A. N. Schellekens and N. P. Warner, “Anomalies and Modular Invariance in String Theory,” *Phys. Lett.* **B177** (1986) 317.
- [73] A. N. Schellekens and N. P. Warner, “Anomaly Cancellation and Selfdual Lattices,” *Phys. Lett.* **B181** (1986) 339.
- [74] K. Pilch, A. N. Schellekens, and N. P. Warner, “Path Integral Calculation of String Anomalies,” *Nucl. Phys.* **B287** (1987) 362.
- [75] E. Witten, “Elliptic Genera and Quantum Field Theory,” *Commun. Math. Phys.* **109** (1987) 525.

- [76] E. Witten, “The Index of the Dirac Operator in Loop Space,” in *Elliptic Curves and Modular Form in Algebraic Topology*, Lecture Notes in Mathematics. 1988.  
<http://alice.cern.ch/format/showfull?sysnb=0088339>.
- [77] E. Witten, “Constraints on Supersymmetry Breaking,” *Nucl. Phys.* **B202** (1982) 253.
- [78] F. Benini and N. Bobev, “Exact two-dimensional superconformal R-symmetry and c-extremization,” *Phys. Rev. Lett.* **110** (2013) no. 6, 061601, [arXiv:1211.4030](https://arxiv.org/abs/1211.4030) [[hep-th](#)].
- [79] F. Benini and N. Bobev, “Two-dimensional SCFTs from wrapped branes and c-extremization,” *JHEP* **06** (2013) 005, [arXiv:1302.4451](https://arxiv.org/abs/1302.4451) [[hep-th](#)].
- [80] V. Gritsenko, “Elliptic genus of Calabi-Yau manifolds and Jacobi and Siegel modular forms,” [arXiv:math/9906190](https://arxiv.org/abs/math/9906190) [[math](#)].
- [81] T. Eguchi, H. Ooguri, A. Taormina, and S.-K. Yang, “Superconformal Algebras and String Compactification on Manifolds with SU(N) Holonomy,” *Nucl. Phys.* **B315** (1989) 193.
- [82] H. Ooguri, “Superconformal Symmetry and Geometry of Ricci Flat Kahler Manifolds,” *Int. J. Mod. Phys.* **A4** (1989) 4303–4324.
- [83] E. Witten, “On the Landau-Ginzburg description of N=2 minimal models,” *Int. J. Mod. Phys.* **A9** (1994) 4783–4800, [arXiv:hep-th/9304026](https://arxiv.org/abs/hep-th/9304026) [[hep-th](#)].
- [84] P. Berglund and M. Henningson, “Landau-Ginzburg orbifolds, mirror symmetry and the elliptic genus,” *Nucl. Phys.* **B433** (1995) 311–332, [arXiv:hep-th/9401029](https://arxiv.org/abs/hep-th/9401029) [[hep-th](#)].
- [85] T. Kawai, Y. Yamada, and S.-K. Yang, “Elliptic genera and N=2 superconformal field theory,” *Nucl. Phys.* **B414** (1994) 191–212, [arXiv:hep-th/9306096](https://arxiv.org/abs/hep-th/9306096) [[hep-th](#)].
- [86] T. Kawai and S.-K. Yang, “Duality of orbifoldized elliptic genera,” *Prog. Theor. Phys. Suppl.* **118** (1995) 277–298, [arXiv:hep-th/9408121](https://arxiv.org/abs/hep-th/9408121) [[hep-th](#)].
- [87] P. Berglund and M. Henningson, “On the elliptic genus and mirror symmetry,” [arXiv:hep-th/9406045](https://arxiv.org/abs/hep-th/9406045) [[hep-th](#)].
- [88] A. Gadde and S. Gukov, “2d Index and Surface operators,” *JHEP* **03** (2014) 080, [arXiv:1305.0266](https://arxiv.org/abs/1305.0266) [[hep-th](#)].
- [89] F. Benini, R. Eager, K. Hori, and Y. Tachikawa, “Elliptic genera of two-dimensional N=2 gauge theories with rank-one gauge groups,” *Lett. Math. Phys.* **104** (2014) 465–493, [arXiv:1305.0533](https://arxiv.org/abs/1305.0533) [[hep-th](#)].
- [90] X. Ma and J. Zhou, “Elliptic genera of complete intersections,” *Internat. J. Math.* **16** (2005) no. 10, 1131–1155, [arXiv:math/0411081](https://arxiv.org/abs/math/0411081) [[math.AG](#)]. <http://dx.doi.org/10.1142/S0129167X05003259>.
- [91] S. Guo and J. Zhou, “Elliptic genera of complete intersections in weighted projective spaces,” *Internat. J. Math.* **22** (2011) no. 5, 695–712. <http://dx.doi.org/10.1142/S0129167X11007008>.
- [92] J. Distler and S. Kachru, “(0,2) Landau-Ginzburg theory,” *Nucl. Phys.* **B413** (1994) 213–243, [arXiv:hep-th/9309110](https://arxiv.org/abs/hep-th/9309110) [[hep-th](#)].
- [93] T. Kawai and K. Mohri, “Geometry of (0,2) Landau-Ginzburg orbifolds,” *Nucl. Phys.* **B425** (1994) 191–216, [arXiv:hep-th/9402148](https://arxiv.org/abs/hep-th/9402148) [[hep-th](#)].
- [94] P. A. Grassi, G. Policastro, and E. Scheidegger, “Partition Functions, Localization, and the Chiral de Rham complex,” [arXiv:hep-th/0702044](https://arxiv.org/abs/hep-th/0702044) [[HEP-TH](#)].
- [95] S. Harrison, S. Kachru, and N. M. Paquette, “Twining Genera of (0,4) Supersymmetric Sigma Models on K3,” *JHEP* **04** (2014) 048, [arXiv:1309.0510](https://arxiv.org/abs/1309.0510) [[hep-th](#)].

- [96] S. Murthy, “A holomorphic anomaly in the elliptic genus,” *JHEP* **06** (2014) 165, [arXiv:1311.0918 \[hep-th\]](#).
- [97] S. K. Ashok, N. Doroud, and J. Troost, “Localization and real Jacobi forms,” *JHEP* **04** (2014) 119, [arXiv:1311.1110 \[hep-th\]](#).
- [98] D. Israel and M. Sarkis, “New supersymmetric index of heterotic compactifications with torsion,” *JHEP* **12** (2015) 069, [arXiv:1509.05704 \[hep-th\]](#).
- [99] E. Witten, “Two-dimensional gauge theories revisited,” *J. Geom. Phys.* **9** (1992) 303–368, [arXiv:hep-th/9204083 \[hep-th\]](#).
- [100] K. Hori, H. Kim, and P. Yi, “Witten Index and Wall Crossing,” *JHEP* **01** (2015) 124, [arXiv:1407.2567 \[hep-th\]](#).
- [101] C. Cordova and S.-H. Shao, “An Index Formula for Supersymmetric Quantum Mechanics,” [arXiv:1406.7853 \[hep-th\]](#).
- [102] N. A. Nekrasov, “Seiberg-Witten prepotential from instanton counting,” *Adv. Theor. Math. Phys.* **7** (2003) no. 5, 831–864, [arXiv:hep-th/0206161 \[hep-th\]](#).
- [103] S. Nakamura, “On the Jeffrey-Kirwan residue of BCD-instantons,” *PTEP* **2015** (2015) no. 7, 073B02, [arXiv:1502.04188 \[hep-th\]](#).
- [104] C. Hwang, J. Kim, S. Kim, and J. Park, “General instanton counting and 5d SCFT,” *JHEP* **07** (2015) 063, [arXiv:1406.6793 \[hep-th\]](#).
- [105] J. Distler, “Notes on (0,2) superconformal field theories,” in *Trieste HEP Cosmology 1994:0322-351*, pp. 0322–351. 1995. [arXiv:hep-th/9502012 \[hep-th\]](#).
- [106] A. Szenes and M. Vergne, “Toric reduction and a conjecture of Batyrev and Materov,” *Invent. Math.* **158** (2004) no. 3, 453–495, [arXiv:math/0306311 \[math.AT\]](#).  
<http://dx.doi.org/10.1007/s00222-004-0375-2>.
- [107] P. Orlik and H. Terao, *Arrangements of Hyperplanes*, vol. 300 of *Grundlehren der mathematischen Wissenschaften*. Springer-Verlag, Berlin-Heidelberg-New York, 1992.
- [108] M. Brion and M. Vergne, “Arrangement of hyperplanes. I. Rational functions and Jeffrey-Kirwan residue,” *Ann. Sci. École Norm. Sup. (4)* **32** (1999) 715–741, [arXiv:math/9903178 \[math.DG\]](#).
- [109] K. Hori and A. Kapustin, “Duality of the fermionic 2-D black hole and N=2 Liouville theory as mirror symmetry,” *JHEP* **08** (2001) 045, [arXiv:hep-th/0104202 \[hep-th\]](#).
- [110] E. Witten, “On string theory and black holes,” *Phys. Rev.* **D44** (1991) 314–324.
- [111] S. K. Ashok and J. Troost, “Elliptic genera and real Jacobi forms,” *JHEP* **01** (2014) 082, [arXiv:1310.2124 \[hep-th\]](#).
- [112] S. P. Zwegers, *Moch theta functions*. PhD thesis, Utrecht, 2002. [arXiv:0807.4834](#).
- [113] D. Zagier, “Ramanujan’s mock theta functions and their applications [d’après Zwegers and Bringmann-Ono],” in *Séminaire BOURBAKI, 60 ème année, n. 986*. 2006-2007.
- [114] A. Dabholkar, S. Murthy, and D. Zagier, “Quantum Black Holes, Wall Crossing, and Mock Modular Forms,” [arXiv:1208.4074 \[hep-th\]](#).
- [115] J. A. Harvey, S. Lee, and S. Murthy, “Elliptic genera of ALE and ALF manifolds from gauged linear sigma models,” *JHEP* **02** (2015) 110, [arXiv:1406.6342 \[hep-th\]](#).
- [116] G. W. Gibbons and S. W. Hawking, “Gravitational Multi - Instantons,” *Phys. Lett.* **B78** (1978) 430.
- [117] D. Tong, “NS5-branes, T duality and world sheet instantons,” *JHEP* **07** (2002) 013, [arXiv:hep-th/0204186 \[hep-th\]](#).

- [118] A. Gadde, S. Gukov, and P. Putrov, “(0, 2) trialities,” *JHEP* **03** (2014) 076, [arXiv:1310.0818 \[hep-th\]](#).
- [119] L. F. Alday, D. Gaiotto, and Y. Tachikawa, “Liouville Correlation Functions from Four-dimensional Gauge Theories,” *Lett. Math. Phys.* **91** (2010) 167–197, [arXiv:0906.3219 \[hep-th\]](#).
- [120] Y. Tachikawa, “A brief review of the 2d/4d correspondences,” *Journal of Physics A* **xx** (2016) 000, [1608.02964](#).
- [121] C. Vafa and E. Witten, “A Strong coupling test of S duality,” *Nucl. Phys.* **B431** (1994) 3–77, [arXiv:hep-th/9408074 \[hep-th\]](#).
- [122] A. Gadde, S. Gukov, and P. Putrov, “Fivebranes and 4-manifolds,” [arXiv:1306.4320 \[hep-th\]](#).
- [123] B. Haghighat, A. Iqbal, C. Kozkaz, G. Lockhart, and C. Vafa, “M-Strings,” *Commun. Math. Phys.* **334** (2015) no. 2, 779–842, [arXiv:1305.6322 \[hep-th\]](#).
- [124] S. Kim and K. Lee, “Indices for 6 dimensional superconformal field theories,” *Journal of Physics A* **xx** (2016) 000, [1608.02969](#).
- [125] E. Sharpe, “Predictions for Gromov-Witten invariants of noncommutative resolutions,” *J. Geom. Phys.* **74** (2013) 256–265, [arXiv:1212.5322 \[hep-th\]](#).
- [126] Y. Honma and M. Manabe, “Exact Kahler Potential for Calabi-Yau Fourfolds,” *JHEP* **05** (2013) 102, [arXiv:1302.3760 \[hep-th\]](#).
- [127] K. Hori and D. Tong, “Aspects of Non-Abelian Gauge Dynamics in Two-Dimensional  $\mathcal{N}=(2, 2)$  Theories,” *JHEP* **05** (2007) 079, [arXiv:hep-th/0609032 \[hep-th\]](#).
- [128] J. Gomis and B. Le Floch, “M2-brane surface operators and gauge theory dualities in Toda,” [arXiv:1407.1852 \[hep-th\]](#).
- [129] N. Doroud. Private communication, 2016.
- [130] K. Ueda and Y. Yoshida, “Equivariant A-twisted GLSM and Gromov–Witten invariants of CY 3-folds in Grassmannians,” [arXiv:1602.02487 \[hep-th\]](#).
- [131] K. Hori, “Duality In Two-Dimensional (2,2) Supersymmetric Non-Abelian Gauge Theories,” *JHEP* **10** (2013) 121, [arXiv:1104.2853 \[hep-th\]](#).
- [132] A. Gerhardus and H. Jockers, “Dual Pairs of Gauged Linear Sigma Models and Derived Equivalences of Calabi-Yau threefolds,” [arXiv:1505.00099 \[hep-th\]](#).
- [133] A. Gadde, S. Gukov, and P. Putrov, “Exact Solutions of 2d Supersymmetric Gauge Theories,” [arXiv:1404.5314 \[hep-th\]](#).
- [134] B. Jia, E. Sharpe, and R. Wu, “Notes on nonabelian (0,2) theories and dualities,” *JHEP* **08** (2014) 017, [arXiv:1401.1511 \[hep-th\]](#).
- [135] S. Franco, S. Lee, and R.-K. Seong, “Brane Brick Models and 2d (0,2) Triality,” [arXiv:1602.01834 \[hep-th\]](#).
- [136] P. Putrov, J. Song, and W. Yan, “(0, 4) dualities,” [arXiv:1505.07110 \[hep-th\]](#).
- [137] A. Gadde, S. S. Razamat, and B. Willett, “On the reduction of 4d  $\mathcal{N} = 1$  theories on  $\mathbb{S}^2$ ,” *JHEP* **11** (2015) 163, [arXiv:1506.08795 \[hep-th\]](#).
- [138] C. Closset and I. Shamir, “The  $\mathcal{N} = 1$  Chiral Multiplet on  $T^2 \times S^2$  and Supersymmetric Localization,” *JHEP* **03** (2014) 040, [arXiv:1311.2430 \[hep-th\]](#).
- [139] M. Honda and Y. Yoshida, “Supersymmetric index on  $T^2 \times S^2$  and elliptic genus,” [arXiv:1504.04355 \[hep-th\]](#).

- [140] M. Honda, “N=2 minimal model from 4d supersymmetric theory,” [arXiv:1508.06111 \[hep-th\]](#).
- [141] S. Cecotti, J. Song, C. Vafa, and W. Yan, “Superconformal Index, BPS Monodromy and Chiral Algebras,” [arXiv:1511.01516 \[hep-th\]](#).
- [142] B. Haghighat, C. Kozcaz, G. Lockhart, and C. Vafa, “Orbifolds of M-strings,” *Phys. Rev.* **D89** (2014) no. 4, 046003, [arXiv:1310.1185 \[hep-th\]](#).
- [143] K. Hosomichi and S. Lee, “Self-dual Strings and 2D SYM,” *JHEP* **01** (2015) 076, [arXiv:1406.1802 \[hep-th\]](#).
- [144] Y. Sugimoto, “The Enhancement of Supersymmetry in M-strings,” [arXiv:1508.02125 \[hep-th\]](#).
- [145] J. Kim, S. Kim, K. Lee, J. Park, and C. Vafa, “Elliptic Genus of E-strings,” [arXiv:1411.2324 \[hep-th\]](#).
- [146] J. Kim, S. Kim, and K. Lee, “Higgsing towards E-strings,” [arXiv:1510.03128 \[hep-th\]](#).
- [147] J. Kim, S. Kim, and K. Lee, “Little strings and T-duality,” [arXiv:1503.07277 \[hep-th\]](#).
- [148] B. Haghighat, A. Klemm, G. Lockhart, and C. Vafa, “Strings of Minimal 6d SCFTs,” *Fortsch. Phys.* **63** (2015) 294–322, [arXiv:1412.3152 \[hep-th\]](#).
- [149] A. Gadde, B. Haghighat, J. Kim, S. Kim, G. Lockhart, and C. Vafa, “6d String Chains,” [arXiv:1504.04614 \[hep-th\]](#).
- [150] G. Bonelli, A. Sciarappa, A. Tanzini, and P. Vasko, “The Stringy Instanton Partition Function,” *JHEP* **01** (2014) 038, [arXiv:1306.0432 \[hep-th\]](#).
- [151] D. S. Park and J. Song, “The Seiberg-Witten Kahler Potential as a Two-Sphere Partition Function,” *JHEP* **01** (2013) 142, [arXiv:1211.0019 \[hep-th\]](#).
- [152] M. Manabe, “Stringy Instanton Counting and Topological Strings,” *JHEP* **07** (2015) 097, [arXiv:1501.00064 \[hep-th\]](#).
- [153] G. Bonelli, A. Sciarappa, A. Tanzini, and P. Vasko, “Six-dimensional supersymmetric gauge theories, quantum cohomology of instanton moduli spaces and  $gl(N)$  Quantum Intermediate Long Wave Hydrodynamics,” *JHEP* **07** (2014) 141, [arXiv:1403.6454 \[hep-th\]](#).
- [154] G. Bonelli, A. Sciarappa, A. Tanzini, and P. Vasko, “Quantum Cohomology and Quantum Hydrodynamics from Supersymmetric Quiver Gauge Theories,” [arXiv:1505.07116 \[hep-th\]](#).
- [155] M. Yamazaki and W. Yan, “Integrability from 2d  $\mathcal{N} = (2, 2)$  dualities,” *J. Phys.* **A48** (2015) 394001, [arXiv:1504.05540 \[hep-th\]](#).
- [156] J. Yagi, “Quiver gauge theories and integrable lattice models,” *JHEP* **10** (2015) 065, [arXiv:1504.04055 \[hep-th\]](#).
- [157] B. Willett, “Localization on three-dimensional manifolds,” *Journal of Physics A* **xx** (2016) 000, [1608.02958](#).
- [158] F. Benini, T. Nishioka, and M. Yamazaki, “4d Index to 3d Index and 2d TQFT,” *Phys. Rev.* **D86** (2012) 065015, [arXiv:1109.0283 \[hep-th\]](#).
- [159] M. Yamazaki, “Four-dimensional superconformal index reloaded,” *Theor. Math. Phys.* **174** (2013) 154–166. [Teor. Mat. Fiz.174,177(2013)].
- [160] H.-Y. Chen and T.-H. Tsai, “On Higgs Branch Localization of Seiberg-Witten Theories on Ellipsoid,” [arXiv:1506.04390 \[hep-th\]](#).
- [161] Y. Pan and W. Peelaers, “Ellipsoid partition function from Seiberg-Witten monopoles,” *JHEP* **10** (2015) 183, [arXiv:1508.07329 \[hep-th\]](#).

- [162] K. Hosomichi, “ $\mathcal{N} = 2$  SUSY gauge theories on  $S^4$ ,” *Journal of Physics A* **xx** (2016) 000, [1608.02962](#).
- [163] D. Gaiotto and H.-C. Kim, “Surface defects and instanton partition functions,” [arXiv:1412.2781](#) [[hep-th](#)].
- [164] M. Bullimore, H.-C. Kim, and P. Koroteev, “Defects and Quantum Seiberg-Witten Geometry,” *JHEP* **05** (2015) 095, [arXiv:1412.6081](#) [[hep-th](#)].
- [165] H.-Y. Chen and H.-Y. Chen, “Heterotic Surface Defects and Dualities from 2d/4d Indices,” *JHEP* **10** (2014) 004, [arXiv:1407.4587](#) [[hep-th](#)].
- [166] J. Lamy-Poirier, “Localization of a supersymmetric gauge theory in the presence of a surface defect,” [arXiv:1412.0530](#) [[hep-th](#)].

# Chapter 4

## Gromov–Witten invariants and localization

David R. Morrison

*Departments of Mathematics and Physics  
University of California, Santa Barbara  
Santa Barbara, CA 93106 USA  
drm@math.ucsb.edu*

### Abstract

We give a pedagogical review of the computation of Gromov–Witten invariants via localization in 2D gauged linear sigma models. We explain the relationship between the two-sphere partition function of the theory and the Kähler potential on the conformal manifold. We show how the Kähler potential can be assembled from classical, perturbative, and non-perturbative contributions, and explain how the non-perturbative contributions are related to the Gromov–Witten invariants of the corresponding Calabi–Yau manifold. We then explain how localization enables efficient calculation of the two-sphere partition function and, ultimately, the Gromov–Witten invariants themselves.

### Contents

|            |                                                           |            |
|------------|-----------------------------------------------------------|------------|
| <b>4.1</b> | <b>Introduction</b>                                       | <b>140</b> |
| <b>4.2</b> | <b>Kähler potentials and 2-sphere partition functions</b> | <b>141</b> |
| <b>4.3</b> | <b>Metrics on conformal manifolds</b>                     | <b>144</b> |
| 4.3.1      | Nonlinear sigma models                                    | 144        |
| 4.3.2      | Gauged linear sigma models                                | 146        |
| 4.3.3      | Phases of an abelian GLSM                                 | 148        |
| <b>4.4</b> | <b>Quantum corrections to the Kähler potential</b>        | <b>152</b> |
| 4.4.1      | Nonlinear $\sigma$ -model action and the effective action | 152        |

|            |                                                                                              |            |
|------------|----------------------------------------------------------------------------------------------|------------|
| 4.4.2      | Perturbative corrections to the Kähler potential . . . . .                                   | 154        |
| 4.4.3      | Nonperturbative corrections and Gromov–Witten invariants . . . . .                           | 155        |
| <b>4.5</b> | <b>The two-sphere partition function and Gromov–Witten invariants . . . . .</b>              | <b>158</b> |
| 4.5.1      | The $S^2$ partition function for a GLSM . . . . .                                            | 158        |
| 4.5.2      | The hemisphere partition function and the $tt^*$ equations . . . . .                         | 159        |
| 4.5.3      | Extracting Gromov–Witten invariants from the partition function . . . . .                    | 160        |
| <b>4.6</b> | <b>Evaluating the partition function . . . . .</b>                                           | <b>161</b> |
| 4.6.1      | Analytic structure of the partition function . . . . .                                       | 161        |
| 4.6.2      | Residues and phases . . . . .                                                                | 162        |
| 4.6.3      | Gromov–Witten invariants of an example . . . . .                                             | 163        |
| <b>4.7</b> | <b>Appendix. <math>\mathcal{N} = (2, 2)</math> supersymmetry in two dimensions . . . . .</b> | <b>166</b> |
|            | <b>References . . . . .</b>                                                                  | <b>167</b> |

## 4.1 Introduction

Many of the early studies of conformal field theories in two dimensions were motivated by the connection of these theories to perturbative string theory. When the string theory is being compactified on a compact manifold  $X$  (typically a Calabi–Yau manifold), the resulting conformal field theory can be described in terms of the nonlinear sigma model with target space  $X$ . One of the interesting features of these theories is the phenomenon of *mirror symmetry* [2–4]: two different Calabi–Yau manifolds  $X$  and  $Y$  can lead to conformal field theories which are identical save for a relabeling of the action of the superconformal algebra.

The celebrated paper of Candelas, de la Ossa, Green, and Parkes [5] exploited mirror symmetry to provide a new way to calculate instanton contributions to the sigma model (now known as “Gromov–Witten invariants” [6, 7]), appealing to the fact that instanton-corrected correlation functions in one theory corresponded to correlation functions in the other theory which receive no quantum corrections. This powerful method, eventually formalized as a mathematical “Mirror Theorem” [8, 9], only works when the mirror partner of a given Calabi–Yau manifold is known. Subsequent developments in mathematics (cf. [10]) suggest that it should be possible to determine the Gromov–Witten invariants without recourse to the mirror, and that has now been achieved in a physics context as well [11]. This new physical method for finding Gromov–Witten invariants is the subject of the present review.

The method is a by-product of a recent theme in the study of supersymmetric quantum field theories, which formulates a given theory on a sphere or product of spheres, and evaluates physical quantities such as the partition function by means of localization. This theme was pioneered in four dimensions by Pestun [12], and has subsequently been extended to a number of different dimensions and contexts, many of which are covered in this volume.

For theories in dimension two with  $\mathcal{N} = (2, 2)$  supersymmetry, the formulation on the two-sphere and the corresponding localization computations were carried out in [13, 14]. The authors of [11] then recognized that there was a connection between the partition function on the two-sphere and the Zamolodchikov metric on the conformal manifold of the theory,

formulating this as a precise conjecture. They also showed how the conjecture would enable the calculation of Gromov–Witten invariants from the data of the partition function, without needing a mirror Calabi–Yau manifold.

Compelling arguments in favor of the conjecture were soon given in [15, 16]. We present here instead a more recent argument [17] which explains the result as arising from an anomaly of the conformal field theory. We review that argument in Section 4.2.

In Section 4.3 we then discuss two kinds of sigma models: the nonlinear sigma model with Calabi–Yau target space (including the classical Kähler potential on the conformal manifold), and the “gauged linear sigma model” of [18], which is where we shall carry out our localization computations. Quantum corrections to the Kähler potential, including the non-perturbative corrections associated to Gromov–Witten invariants, are discussed in Section 4.4.

The determination of the two-sphere partition function via localization, and the corresponding method for calculating Gromov–Witten invariants, is reviewed in Section 4.5. Finally, in Section 4.6 we discuss the evaluation of the partition function via residues and show how to obtain Gromov–Witten invariants explicitly. We have collected supplementary material in an Appendix (Section 4.7).

We have drawn heavily upon [19, 20], [11], [21, 22], [17] in preparing this review.

## 4.2 Kähler potentials and 2-sphere partition functions

Let us consider the exactly marginal operators for a two-dimensional conformal field theory. These are operators  $\mathcal{O}_I$  having the property that, if added to the action with coupling constants  $\lambda^I$

$$\delta S = \frac{1}{\pi} \sum_I \int d^2x \lambda^I \mathcal{O}_I(x) , \quad (4.2.1)$$

they leave the theory conformally invariant. The coupling constants  $\lambda^I$  parameterize the *conformal manifold*  $\mathcal{M}$  of the theory, and the two-point functions

$$\langle \mathcal{O}_I(x) \mathcal{O}_J(y) \rangle = \frac{g_{IJ}(\lambda^K)}{(x-y)^4} \quad (4.2.2)$$

determine the *Zamolodchikov metric*  $g_{IJ}$  on  $\mathcal{M}$  [23].

In momentum space the two-point functions (4.2.2) take the form

$$\langle \mathcal{O}_I(p) \mathcal{O}_J(-p) \rangle \sim p^4 \log \left( \frac{\Lambda^2}{p^2} \right) . \quad (4.2.3)$$

Having a logarithmic behavior with cutoff  $\Lambda$  does not violate scale invariance since any rescaling of  $\Lambda$  can be compensated with a contact term. However, although they do not spoil conformal invariance, these logarithms lead to the non-conservation of the dilatation charge in the presence of non-vanishing background fields (the original “conformal anomaly”). This can be detected by promoting the couplings  $\lambda^I$  to fields [24]. Then the anomaly induces a term in the energy-momentum trace of the rough form

$$T^\mu_\mu = g_{IJ} \lambda^I \square \lambda^J + \dots . \quad (4.2.4)$$

In this section, we shall discuss a further conformal anomaly under variation of the 2D metric, following [17]. This anomaly was first observed in [25], and is again consistent with scale invariance due to the possibility of contact terms in the two-point function.

We assume as in [17] that the given conformal field theory can be regulated in a diffeomorphism-invariant way, including a metric  $\gamma_{\mu\nu}$  on the 2D spacetime as well as spacetime-dependent couplings  $\lambda^I$ . The partition function of the theory on this spacetime then depends on the metric and couplings, taking the form  $Z[\gamma_{\mu\nu}; \lambda^I]$ .

We consider an infinitesimal Weyl transformation

$$\delta_\sigma \gamma_{\mu\nu} = 2\gamma_{\mu\nu} \delta\sigma \quad (4.2.5)$$

(where the infinitesimal  $\delta\sigma$  has compact support) and ask for the corresponding variation  $\delta_\sigma \log Z$  of the partition function. A precise form of the infinitesimal Weyl variation of  $\log Z$  is derived in [25] and takes the form

$$\delta_\sigma \log Z = \frac{c}{24\pi} \int d^2x \delta\sigma \sqrt{\gamma} R - \frac{1}{4\pi} \int d^2x \delta\sigma \sqrt{\gamma} g_{IJ} \gamma^{\mu\nu} \partial_\mu \lambda^I \partial_\nu \lambda^J, \quad (4.2.6)$$

where  $R$  is the Ricci scalar. The first term is a universal contribution due to the central charge  $c$  of the theory. It is argued in [17] that no anomalies other than (4.2.6) are possible.

The ‘‘conformal anomaly’’ functional (4.2.6) describes a sigma model with target space  $\mathcal{M}$ , and is not the Weyl variation of any local counterterm. It is therefore cohomologically nontrivial.

There *is* an allowed local counterterm of the form

$$\int d^2x \sqrt{\gamma} R F(\lambda^I) \quad (4.2.7)$$

whose Weyl variation is

$$\delta_\sigma \int d^2x \sqrt{\gamma} R F(\lambda^I) = -2 \int d^2x \sqrt{\gamma} \square (\delta\sigma) F(\lambda^I). \quad (4.2.8)$$

Thus, (4.2.6) can be shifted by terms of the form (4.2.8).

In the case of an  $\mathcal{N} = (2, 2)$  theory,<sup>1</sup> exactly marginal operators can either be chiral or twisted chiral:

$$\delta S = \frac{1}{\pi} \int d^2x \left( \sum_I \lambda^I \int d^2\theta \mathcal{O}_I(x, \theta) + \sum_A \tilde{\lambda}^A \int d^2\theta \tilde{\mathcal{O}}_A(x, \theta) + \text{c.c.} \right), \quad (4.2.9)$$

where  $\mathcal{O}_I$  is chiral and  $\tilde{\mathcal{O}}_A$  is twisted chiral. The analysis in [17] assumes that the parameters  $\lambda^I$  and  $\tilde{\lambda}^A$  can be promoted to background chiral and twisted chiral superfields respectively, and we make the same assumption.

We wish to supersymmetrize the conformal anomaly (4.2.6) and the counterterm (4.2.7). In order to do so, we place the theory in curved superspace [26]. The possibilities for doing

---

<sup>1</sup>We establish some notation and properties for these theories in an Appendix (Section 4.7).

so with  $\mathcal{N} = (2, 2)$  supersymmetry were analyzed in [27, 28], and amount to a coupling to supergravity.

There are two distinct supergravities to which we could couple, known as  $U(1)_V$  and  $U(1)_A$  [29]; the label indicates whether the  $U(1)$  symmetry preserved in the Poincaré supergravity theory is vector or axial. From the point of view of the  $\mathcal{N} = (2, 2)$  SCFT, the theory has an  $R$ -symmetry of the form  $U(1)_V \times U(1)_A$ , and we can couple either factor (but not both) to a background gauge field. As in [17], we assume<sup>2</sup> that the theory can be regularized so as to preserve diffeomorphism invariance, supersymmetry, and either  $U(1)_V$  or  $U(1)_A$ ; once this is done, the other  $R$ -symmetry cannot be preserved by the regularization scheme. In particular, our assumptions imply that there are no gravitational anomalies and that  $c_L = c_R$ .

Since every two-dimensional metric is conformally flat, the conformal factor  $\sigma$  may be used to specify the metric. When we supersymmetrize, the conformal factor becomes part of a superfield. In the case of  $U(1)_A$  supergravity, it is the scalar in a chiral superfield  $\Sigma$  while in the case of  $U(1)_V$  supergravity it is the scalar in a twisted chiral superfield  $\tilde{\Sigma}$ .<sup>3</sup> We will focus on the case of  $U(1)_V$  in this discussion, although a similar discussion holds for  $U(1)_A$  (and was carried out in [17]).

The supersymmetrization of the conformal anomaly (4.2.6) is straightforward. In the regularization which preserves  $U(1)_V$  it takes the form

$$\delta_{\tilde{\Sigma}} \log Z_V = \frac{c}{24\pi} \int d^2x d^4\theta (\delta\tilde{\Sigma} + \delta\bar{\tilde{\Sigma}})(\tilde{\Sigma} + \bar{\tilde{\Sigma}}) - \frac{1}{4\pi} \int d^2x d^4\theta \left( \delta\tilde{\Sigma} K(\lambda, \bar{\lambda}, \tilde{\lambda}, \bar{\tilde{\lambda}}) + \text{c.c.} \right), \quad (4.2.10)$$

using superconformal gauge. In fact, the classification of anomalies allows one to conclude [17] that  $K$  is real and

$$K = K_c(\lambda, \bar{\lambda}) - K_{tc}(\tilde{\lambda}, \bar{\tilde{\lambda}}), \quad (4.2.11)$$

so that  $\mathcal{M} = \mathcal{M}_c \times \mathcal{M}_{tc}$  is metrically a product.<sup>4</sup> The Kähler potential on  $\mathcal{M}_c$  is  $K_c$  which depends only on the chiral parameters and the Kähler potential on  $\mathcal{M}_{tc}$  is  $K_{tc}$  which depends only on the twisted chiral parameters. We conclude that the conformal anomaly can be written in the form

$$\begin{aligned} \delta_{\tilde{\Sigma}} \log Z_V &= \frac{c}{24\pi} \int d^2x d^4\theta (\delta\tilde{\Sigma} + \delta\bar{\tilde{\Sigma}})(\tilde{\Sigma} + \bar{\tilde{\Sigma}}) \\ &\quad - \frac{1}{4\pi} \int d^2x d^4\theta (\delta\tilde{\Sigma} + \delta\bar{\tilde{\Sigma}}) (K_c(\lambda, \bar{\lambda}) - K_{tc}(\tilde{\lambda}, \bar{\tilde{\lambda}})). \end{aligned} \quad (4.2.12)$$

We also need a supersymmetric version of the allowed local counterterm. In the  $U(1)_V$  case this takes the form [16]

$$S_V = \frac{1}{4\pi} \int d^2x d^2\theta \tilde{\mathcal{R}} F(\tilde{\lambda}) + \text{c.c.} = \frac{1}{4\pi} \int d^2x d^4\theta \tilde{\Sigma} F(\tilde{\lambda}) + \text{c.c.} \quad (4.2.13)$$

<sup>2</sup>This issue is discussed in detail in [27] building on the general framework of [26] (see also [30]).

<sup>3</sup>If there is any danger of confusion, we shall indicate the  $R$ -symmetry in our notation and refer to these superfields as  $\Sigma_R$  or  $\tilde{\Sigma}_R$ .

<sup>4</sup>This product structure holds at smooth points; at certain singular points we may need to take the quotient of the product by a finite group [31, 32].

where  $\widetilde{\mathcal{R}} = \overline{D^2 \widetilde{\Sigma}}$  is the twisted chiral curvature superfield in superconformal gauge. The counterterm (4.2.13) depends only on the twisted chiral parameters  $\widetilde{\lambda}$  and the dependence is holomorphic. Under a super-Weyl transformation,

$$\delta_{\widetilde{\Sigma}} S_V = \frac{1}{4\pi} \int d^2x d^4\theta \left( \delta \widetilde{\Sigma} F(\widetilde{\lambda}) + \delta \widetilde{\Sigma} \overline{F}(\widetilde{\lambda}) \right) . \quad (4.2.14)$$

The effect of adding a local counterterm of the form (4.2.13) is to shift the twisted chiral Kähler potential

$$K_{tc} \rightarrow K_{tc} + F(\widetilde{\lambda}) + \overline{F}(\widetilde{\lambda}) . \quad (4.2.15)$$

The chiral Kähler potential  $K_c$  is unchanged by the addition of counterterms.

The conformal anomaly will affect the partition function whenever the theory is placed on a curved manifold with non-trivial topology. In particular, for compactification on a two-sphere, both the dependence on the radius (via the central charge) and the radius-independent part of the anomaly will be visible in the partition function. If we compactify so as to preserve the  $U(1)_A$  symmetry, the partition function will detect  $K_c(\lambda, \overline{\lambda})$  and be independent of  $\widetilde{\lambda}$ ; on the other hand, if we compactify so as to preserve the  $U(1)_V$  symmetry (as we will do here), the partition function takes the form

$$Z_{S^2} = \left( \frac{r}{r_0} \right)^{c/3} e^{-K_{tc}(\widetilde{\lambda}, \widetilde{\lambda})} \quad (4.2.16)$$

(where  $r_0$  is a fixed scale), as conjectured in [11].<sup>5</sup> This quantity is independent of scale and can be calculated in the ultraviolet, for example on a gauged linear sigma model, or directly in the infrared.

## 4.3 Metrics on conformal manifolds

We now introduce two classes of  $\mathcal{N} = (2, 2)$  theories which give rise to conformal theories in the infrared.

### 4.3.1 Nonlinear sigma models

A nonlinear sigma model whose target is a Calabi–Yau manifold  $X$  of complex dimension  $n$  is a 2D quantum field theory with  $\mathcal{N} = (2, 2)$  supersymmetry which is expected to flow to a conformal theory of central charge  $c = 3n$  in the infrared. In fact, the  $\beta$ -function of such a theory vanishes at one-loop, although there are in general higher loop corrections [33].<sup>6</sup> We choose the action of the  $\mathcal{N} = (2, 2)$  algebra on the nonlinear sigma model in such a way that the chiral marginal operators correspond to the harmonic  $(n - 1, 1)$ -forms on  $X$ , and the twisted chiral marginal operators correspond to the harmonic  $(1, 1)$ -forms. Thus, the chiral conformal manifold  $\mathcal{M}_c$  corresponds to the “moduli space of  $X$ ” studied in algebraic

<sup>5</sup>The radial dependence was suppressed in [11].

<sup>6</sup>In spite of these perturbative corrections, one still expects a CFT in the infrared [34].

geometry which specifies the possible complex structures on  $X$ . The twisted chiral conformal manifold  $\mathcal{M}_{tc}$ , however, has no straightforward identification in mathematics. Near the “large radius limit” boundary point it is parameterized by the choice of complexified Kähler form on  $X$ , which is a complex combination of the Kähler form  $\omega$  and the Kalb–Ramond two-form field  $B$  (which is only well-defined up to shifts by an integral two-form). For this reason,  $\mathcal{M}_{tc}$  is sometimes referred to as the “complexified Kähler moduli space,” with coordinate  $t = i\omega + B$ .

The Zamolodchikov metric on the chiral conformal manifold  $\mathcal{M}_c$  can be identified [35] with the Weil–Peterson metric which was described by Tian [36] and Todorov [37]. For this description, we consider the family of complex manifolds  $\mathcal{X} \xrightarrow{\pi} \mathcal{M}_c$  corresponding to the variation of complex structure, and let  $\Omega$  be a nonvanishing relative holomorphic  $n$ -form on  $\pi^{-1}(U)$  over an open set  $U \subset \mathcal{M}_c$ . Then the function

$$K_c := -\log \left( i^{n^2} \int_X \Omega \wedge \bar{\Omega} \right) , \quad (4.3.1)$$

which is a real-valued function on  $U$ , is a Kähler potential for the Zamolodchikov metric restricted to  $U$ . Any other choice of  $\Omega$  takes the form  $e^{-F} \Omega$  for a nonvanishing holomorphic function  $e^{-F}$  on  $U$ . If we make such a change, then

$$\begin{aligned} -\log \left( i^{n^2} \int_X \Omega \wedge \bar{\Omega} \right) &\mapsto -\log \left( i^{n^2} \int_X e^{-F-\bar{F}} \Omega \wedge \bar{\Omega} \right) \\ &= -\log \left( i^{n^2} \int_X \Omega \wedge \bar{\Omega} \right) + F + \bar{F} , \end{aligned} \quad (4.3.2)$$

as expected for a Kähler potential. Due to some powerful non-renormalization theorems [24, 38], this formula for the Kähler potential on  $\mathcal{M}_c$  is not subject to quantum corrections.

On the other hand, the twisted chiral conformal manifold  $\mathcal{M}_{tc}$  has a classical approximation in terms of the Kähler cone  $\mathcal{K}_X$  of  $X$ , complexified to  $H^2(X, \mathbb{R}) + i\mathcal{K}_X$  by the inclusion of the Kalb–Ramond field. In the simplest case,<sup>7</sup> there are line bundles  $\mathcal{L}_j$  whose first Chern classes  $c_1(\mathcal{L}_j)$  form a basis for  $H^2(X, \mathbb{Z})$  and also generate the Kähler cone:

$$\mathcal{K}_X = \mathbb{R}_{>0} c_1(\mathcal{L}_1) + \cdots + \mathbb{R}_{>0} c_1(\mathcal{L}_s). \quad (4.3.3)$$

If  $t_1, \dots, t_s$  are the corresponding complex coordinates on  $H^2(X, \mathbb{R}) + i\mathcal{K}_X$ , then  $e^{2\pi i t_1}, \dots, e^{2\pi i t_s}$  are local coordinates on the twisted chiral conformal manifold. With respect to these coordinates, the Kähler potential for the Zamolodchikov metric on  $\mathcal{M}_{tc}$  has a classical expression

$$K_{tc} = -\log \left( \frac{1}{(2\pi)^n} \exp \left( \sum t_j \mathcal{F}_j \right) \wedge \overline{\exp \left( \sum t_j \mathcal{F}_j \right)} \right) + \cdots , \quad (4.3.4)$$

where  $\mathcal{F}_j$  is the curvature of a connection on the bundle  $\mathcal{L}_j$ , expressed as a 2-form (with indices suppressed), and the exponential is computed as a power series in which differential forms of even degree are multiplied using the wedge product.

<sup>7</sup>Other cases can be handled by expressing  $\mathcal{K}_X$  as a union of such “integer basis” cones up to automorphism; see [39].

Using the fact that  $L_j := c_1(\mathcal{L}_j)$  is an integral cohomology class represented by the differential form  $\frac{i}{2\pi}\mathcal{F}_j$ , (4.3.4) can be rewritten in terms of integral cohomology (evaluated on the fundamental homology class  $[X]$ ) as

$$e^{-K_{tc}} = \left( \exp \left( \sum 2 \operatorname{Im}(t_j) L_j \right) \right) [X] + \dots \quad (4.3.5)$$

where in this formula, the multiplication in the power series expansion is represented by cup product. Only the term in the exponential of degree  $n$  contributes to this classical expression, which can be written as

$$e^{-K_{tc}} = \frac{1}{n!} \left( \sum 2 \operatorname{Im}(t_j) L_j \right)^n [X] + \dots \quad (4.3.6)$$

and depends on the intersection pairings among the integral divisors  $L_j$ , which are specified by the cohomology ring of  $X$ .

In either form, this classical expression is subject to both perturbative and non-perturbative corrections, to be discussed in the next section.

### 4.3.2 Gauged linear sigma models

Another approach to conformal field theories on Calabi–Yau manifolds is to start with a Lagrangian theory in the UV known as a *gauged linear sigma model* [18].

A gauged linear sigma model (GLSM) is formulated in  $\mathcal{N} = (2, 2)$  superspace, and involves a compact gauge group  $G$  as well as  $N$  chiral matter multiplets transforming in a representation  $\Psi : G \rightarrow U(N)$ . We denote the corresponding representation of the Lie algebra  $\mathfrak{g}$  of  $G$  by  $\psi : \mathfrak{g} \rightarrow \mathfrak{u}(N)$ , so that<sup>8</sup>

$$\Psi(e^{2\pi i Y}) = e^{2\pi i \psi(Y)} \quad (4.3.7)$$

for  $Y \in \mathfrak{g}$ . To streamline our later analysis, we fix a Cartan subgroup  $H \subset G$  (i.e., a maximal connected abelian subgroup) with corresponding Cartan subalgebra  $\mathfrak{h} \subset \mathfrak{g}$ , and choose coordinates  $\phi_J$  on the complex vector space  $\mathbb{C}^N$  such that each  $\phi_J$  is a simultaneous eigenvector for  $\Psi|_H$ . The eigenvalues of  $\Psi_H$  can be specified by means of the *weight lattice*  $\Lambda_{\text{wt}} \subset \mathfrak{h}^*$  of  $G$ , which gives the eigenvalues for the corresponding representation of  $\mathfrak{h}$ . That is, for each  $\phi_J$  there is a weight vector  $w_J \in \Lambda_{\text{wt}} \subset \mathfrak{h}^*$  such that for  $h = e^{2\pi i Y} \in H$ ,

$$\Psi(h)(\phi_J) = e^{2\pi i w_J \cdot Y} \phi_J, \quad (4.3.8)$$

using a dot to denote the pairing between  $\mathfrak{h}^*$  and  $\mathfrak{h}$ .

One of the interaction terms in the Lagrangian is specified by means of a  $G$ -invariant “superpotential” polynomial  $W(\phi_1, \dots, \phi_N)$ . We will also construct a term in the Lagrangian from Lie algebra characters  $\xi : \mathfrak{g} \rightarrow \mathfrak{u}(1)$  which arise from one-dimensional representations  $\Xi : G \rightarrow U(1)$ . It is convenient to choose a basis  $\xi_1, \dots, \xi_k$  for the lattice of such characters.

---

<sup>8</sup>We follow the usual physics convention of putting an  $i$  in the exponential map so that the Lie algebra consists of Hermitian operators. We also put a factor of  $2\pi$  to clarify the integral structure.

All of these characters are trivial on the commutator  $[\mathfrak{g}, \mathfrak{g}]$  and so factor through the projection to the abelianization  $\mathfrak{a} = \mathfrak{g}/[\mathfrak{g}, \mathfrak{g}]$ .

To construct the GLSM, we begin with  $N$  chiral superfields  $\Phi_J$  (i.e., satisfying  $\bar{D}_+\Phi_J = \bar{D}_-\Phi_J = 0$ ) interacting via the holomorphic superpotential  $W(\Phi_1, \dots, \Phi_N)$ . The model is invariant under the action of  $G$  (via  $\Psi$ ) on  $\mathbb{C}^N$  and we gauge this action, preserving  $\mathcal{N} = (2, 2)$  supersymmetry, by introducing a  $\mathfrak{g}$ -valued vector multiplet  $V$  with invariant field strength  $\Sigma = \frac{1}{\sqrt{2}}\bar{D}_+D_-V$ . This last field is *twisted chiral*, which means that  $\bar{D}_+\Sigma = D_-\Sigma = 0$ . We include a topological theta angle  $\vartheta$  and a Fayet–Iliopoulos D-term with coefficient  $\zeta$ , each taking values in<sup>9</sup>  $\mathfrak{a}^* = \text{Ann}([\mathfrak{g}, \mathfrak{g}]) \subset \mathfrak{g}^*$ . These terms are naturally written in terms of the complex combination<sup>10</sup>  $\tau = i\zeta + \frac{1}{2\pi}\vartheta$  or its exponential  $z = e^{2\pi i\tau} = e^{-2\pi\zeta + i\vartheta}$ . We introduce a pairing between  $\mathfrak{a}^*$  and  $\mathfrak{g}$  defined by

$$\langle \tau, \Sigma \rangle := \sum \tau_a \text{tr}_{\xi_a}(\Sigma), \quad (4.3.9)$$

which is independent of the choice of basis. The resulting Lagrangian density is

$$\begin{aligned} \mathcal{L} = & \int d^4\theta \left( \|e^{\psi(V)}\Phi\|^2 - \frac{1}{4e^2}\|\Sigma\|^2 \right) \\ & + \left( \int d\theta^+ d\theta^- W(\Phi_1, \dots, \Phi_N) + \text{c.c.} \right) \\ & + \left( \frac{i}{\sqrt{2}} \int d\theta^+ d\bar{\theta}^- \langle \tau, \Sigma \rangle + \text{c.c.} \right), \end{aligned} \quad (4.3.10)$$

where for simplicity of notation, we have set all gauge couplings of irreducible factors of  $G$  to a single value  $e$ . The marginal couplings of these theories are the coefficients<sup>11</sup> of the superpotential (for  $\mathcal{M}_c$ ) and the choice of D-term coefficient and  $\theta$ -angle (for  $\mathcal{M}_{tc}$ ).

We will assume that these theories admit both a vector-like symmetry  $U(1)_V$  and an axial-like symmetry  $U(1)_A$ . In flat space, a given action of  $U(1)_V \times U(1)_A$  may be modified by a global symmetry but on  $S^2$ , changing the charges of the fields (other than by adding gauge charges) produces a distinct theory [13, 14]. For this reason, we shall regard the specification of these charges as part of the data of the theory. We design our choice with the expectation that, should the theory flow to a superconformal theory in the IR, the specified  $U(1)_V \times U(1)_A$  will become the  $R$ -symmetry which is part of the superconformal algebra. In general we allow these  $R$ -charges to be rational numbers, although for many purposes it is best if they are integers up to gauge transformation. We will study this theory on  $S^2$  preserving the  $U(1)_V$  symmetry, in order to analyze the metric on the twisted chiral conformal manifold.

<sup>9</sup>Globally, as discussed in [40–42], we should identify  $e^{-2\pi\zeta + i\vartheta}$  with an element of  $\text{Hom}(\pi_1(G), \mathbb{C}^*)^{G_0}$ , where  $G_0$  is the connected component of  $G$ .

<sup>10</sup>Both  $\tau$  and  $z$  are local coordinates on the twisted chiral conformal manifold. To avoid cluttering our formulas, we suppress the “tilde” on these variables which should be present for consistency with the notation of Section 4.2.

<sup>11</sup>More precisely, the coefficients account for the marginal chiral couplings with some redundancy; see [43] or [20] for an account of this.

Having specified an  $R$ -charge  $q \in \mathbb{Q}$  for a given superfield, the general form of the vector-like symmetry is

$$e^{i\alpha F_V} : \mathcal{F}(x^\mu, \theta^\pm, \bar{\theta}^\pm) \mapsto e^{i\alpha q} \mathcal{F}(x^\mu, e^{-i\alpha} \theta^\pm, e^{i\alpha} \bar{\theta}^\pm) \quad (4.3.11)$$

while the general form of the axial-like symmetry is

$$e^{i\beta F_A} : \mathcal{F}(x^\mu, \theta^\pm, \bar{\theta}^\pm) \mapsto e^{i\beta q} \mathcal{F}(x^\mu, e^{\mp i\beta} \theta^\pm, e^{\pm i\beta} \bar{\theta}^\pm) . \quad (4.3.12)$$

Note that the superpotential, if nonzero, must have  $R$ -charge 2.

In flat space, such a symmetry can have an anomaly in the presence of gauge fields. A quick computation [18, 19] shows that the anomaly is given by a function on the Lie algebra proportional to  $V \mapsto \text{tr}(\psi(V))$ ; we require that this vanish identically so that the symmetries are not anomalous. Since the action of the continuous part of  $G$  on the monomial  $\Phi_1 \cdots \Phi_N$  is via  $\exp(\text{tr}(\psi(V)))$ , this is the same as requiring that  $\Phi_1 \cdots \Phi_N$  be invariant under the continuous part of the gauge group  $G$ . In addition, in order to ensure integral  $R$ -charges up to gauge transformation, we require that  $\Phi_1 \cdots \Phi_N$  be invariant under the entire group  $G$  [44]. In other words, we must require that

$$\Psi(G) \subset SU(N), \quad (4.3.13)$$

and we will impose that requirement henceforth.

Finally, using the  $R$ -symmetry and calculating as in [45], one finds that the central charge  $c$  of the fixed-point CFT is determined by

$$\frac{c}{3} = d - \sum_{J=1}^N q_J , \quad (4.3.14)$$

where the sum extends over all of the chiral superfields, and where  $d$  is the difference between the number of chiral fields and the number of gauge fields.

### 4.3.3 Phases of an abelian GLSM

As explained in detail in [18], a GLSM with an abelian gauge group and an anomaly-free  $R$ -symmetry (i.e.,  $\sum w_J = 0$ ) can be described very explicitly at low energy and in many cases coincides with a nonlinear sigma model with target a Calabi–Yau manifold. In such cases, the correspondence only holds when the FI-parameters are in a certain range of values, and the typical GLSM has other phases with different low-energy descriptions in addition to the geometric phase(s).

The low-energy analysis begins by mapping out the space of classical vacua of the theory. The algebraic equations of motion for the auxiliary fields  $D_a$  in the vector multiplets and  $F_J$  in the chiral multiplets can be solved:

$$D_a = -e^2 \left( \sum_{J=1}^N (w_J)_a |\phi_J|^2 - \zeta_a \right) \quad (4.3.15)$$

$$F_J = -\frac{\partial W}{\partial \phi_J} . \quad (4.3.16)$$

The potential energy for the bosonic zero modes is then

$$U = \frac{1}{2e^2} \sum_{a=1}^h D_a^2 + \sum_{J=1}^N |F_J|^2 + \sum_{a,b} \bar{\sigma}_a \sigma_b \sum_{J=1}^N (w_J)_a (w_J)_b |\phi_J|^2, \quad (4.3.17)$$

where  $\phi_J, \sigma_a$  are the lowest components of  $\Phi_J, \Sigma_a$  respectively. The space of classical vacua is the quotient by  $G$  of the set of zeros of  $U$ .

Suppressing any solutions with  $\sigma \neq 0$  (which are absent for generic values of the parameters), the space of solutions is

$$(D^{-1}(0) \cap \text{Crit}(W))/G \subset D^{-1}(0)/G. \quad (4.3.18)$$

Since  $G$  is abelian, this quotient has a description as a toric variety of dimension  $N - h$ , as we now review. The group  $G$  has a natural complexification  $G_{\mathbb{C}}$  in which each  $U(1)$  factor is promoted to the complex group  $\mathbb{C}^*$ ; the action of  $G$  on  $V$  extends to an action of  $G_{\mathbb{C}}$ . For any choice of FI-parameters, the space  $D^{-1}(0)/G$  has a description as a GIT quotient

$$\mathbb{C}^N // G_{\mathbb{C}} = (\mathbb{C}^N - Z_{\zeta})/G_{\mathbb{C}}, \quad (4.3.19)$$

where  $Z_{\zeta}$  is the union of all  $G_{\mathbb{C}}$ -orbits which do not meet  $D^{-1}(0)$ . (The dependence on the FI-parameters  $\zeta$  comes from their inclusion in the D-term equation (4.3.15)).

The nature of the quotient space changes as  $\zeta$  varies, and can be systematically described by a construction known as the “secondary fan” [46–49]. Let  $\mathcal{J} \subset \{1, \dots, N\}$  be a collection of  $h$  indices such that the weight vectors  $\{w_J, J \in \mathcal{J}\}$  are linearly independent; we wish to know if  $D^{-1}(0)$  contains entries in which

$$\phi_J = 0 \text{ for all } J \notin \mathcal{J}. \quad (4.3.20)$$

(If so, then the corresponding orbit  $\mathcal{O}_{\mathcal{J}}$  lies in the quotient space.<sup>12</sup>) To answer this, note that if we impose (4.3.20) then the D-term equations become

$$\zeta = \sum_{J \in \mathcal{J}} |\phi_J|^2 w_J. \quad (4.3.21)$$

In other words, since all coefficients on the right side of (4.3.21) are nonnegative,  $\zeta$  must lie in the cone  $\mathcal{C}_{\mathcal{J}}$  in FI-parameter-space  $\mathfrak{a}^*$  which is generated by the weight vectors  $\{w_J, J \in \mathcal{J}\}$ .

Thus, for a given  $\zeta \in \mathfrak{a}^*$ , to determine which orbits  $\mathcal{O}_{\mathcal{J}}$  lie in  $D^{-1}(0)/G$  we simply determine which cones  $\mathcal{C}_{\mathcal{J}}$  contain  $\zeta$ . This decomposition into cones describes the *secondary fan*, and the regions it defines in  $\mathfrak{a}^*$  are called the *phases* of the GLSM.

To illustrate this construction, we work it out in a particular example<sup>13</sup> which we will follow throughout the paper. We use an example which has been studied extensively in the literature [50–52], [19], [53–55].

<sup>12</sup>A bit more concretely, for each  $\mathcal{G}_{\mathcal{J}}$  containing  $\zeta$ , the complementary set of indices  $\{1, \dots, N\} - \mathcal{J}$  labels the coordinates for one of the toric coordinate charts of  $D^{-1}(0)/G$ .

<sup>13</sup>The example we use is an abelian GLSM, which does not exhibit the full power of the localization method to compute Gromov–Witten invariants, since those invariants can also be computed by mirror symmetry for abelian GLSMs with a geometric phase. However, we avoid some of the complications of nonabelian GLSMs by working with this particular example.

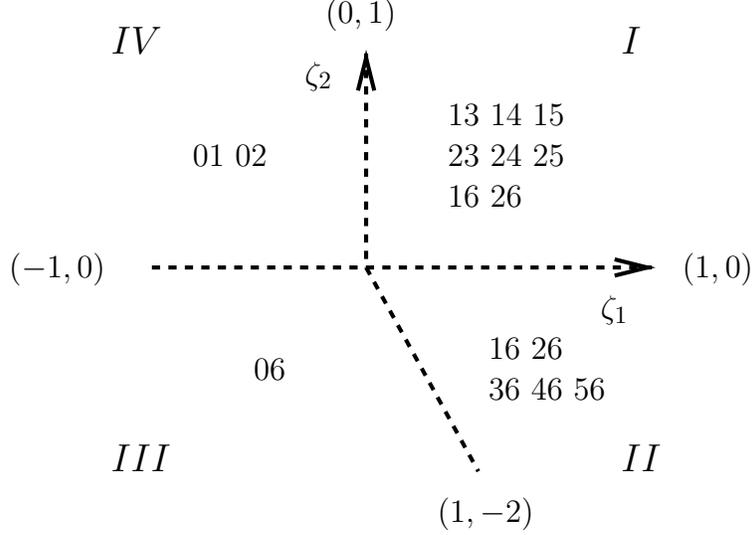

Figure 4.1: Secondary fan data for the example.

Consider an anti-canonical hypersurface in the toric variety obtained from the weighted projective fourfold  $\mathbb{P}^{(1,1,2,2,2)}$  by blowing up its singular locus. This can be described by a GLSM as follows. Let  $(\gamma_1, \gamma_2) \in G = U(1) \times U(1)$  act on the vector space  $\mathbb{C}^7$  via

$$(\phi_0, \phi_1, \dots, \phi_6) \mapsto (\gamma_1^{-4} \phi_0, \gamma_2 \phi_1, \gamma_2 \phi_2, \gamma_1 \phi_3, \gamma_1 \phi_4, \gamma_1 \phi_5, \gamma_1 \gamma_2^{-2} \phi_6) . \quad (4.3.22)$$

We specify  $R$ -charges of these fields in terms of two arbitrary rational parameters  $q_1$  and  $q_2$  to be determined later, as

|             |            |                  |                          |              |          |
|-------------|------------|------------------|--------------------------|--------------|----------|
| field       | $\phi_0$   | $\phi_1, \phi_2$ | $\phi_3, \phi_4, \phi_5$ | $\phi_6$     |          |
| $R$ -charge | $2 - 4q_1$ | $q_2$            | $q_1$                    | $q_1 - 2q_2$ | (4.3.23) |

For the superpotential, which is a  $G$ -invariant polynomial of  $R$ -charge two, we choose

$$W(\phi_0, \phi_1, \dots, \phi_6) = \phi_0 F_{(4,0)}(\phi_1, \dots, \phi_6), \quad (4.3.24)$$

where  $F_{(4,0)}$  is a generic homogeneous polynomial of bi-degree  $(4, 0)$  with respect to the gauge group  $G = U(1) \times U(1)$ .

The D-term equations are

$$\zeta_1 = -4|\phi_0|^2 + |\phi_3|^2 + |\phi_4|^2 + |\phi_5|^2 + |\phi_6|^2 , \quad (4.3.25)$$

$$\zeta_2 = |\phi_1|^2 + |\phi_2|^2 - 2|\phi_6|^2 . \quad (4.3.26)$$

We then find the secondary fan data which is illustrated in Figure 4.1: for each pair  $\{J, J'\}$  we have indicated the region(s) which are included in the cone generated by  $w_J$  and  $w_{J'}$ . This leads to four phases, labeled by Roman numerals in the Figure.

Note that the cones  $\mathcal{C}_{\mathcal{J}}$  are not necessarily phase regions in and of themselves; in the example,  $\mathcal{C}_{16}$  is the union of phases I and II.

The geometry of the various quotients is best described by determining the sets  $Z_\zeta$  which are excluded from the quotient. If we label those sets according to phase region, then by examining which variables are allowed to vanish together, we find that

$$Z_I = \{\phi_1 = \phi_2 = 0\} \cup \{\phi_3 = \phi_4 = \phi_5 = \phi_6 = 0\} \quad (4.3.27)$$

$$Z_{II} = \{\phi_1 = \phi_2 = \phi_3 = \phi_4 = \phi_5 = 0\} \cup \{\phi_6 = 0\} \quad (4.3.28)$$

$$Z_{III} = \{\phi_0 = 0\} \cup \{\phi_6 = 0\} \quad (4.3.29)$$

$$Z_{IV} = \{\phi_0 = 0\} \cup \{\phi_1 = \phi_2 = 0\} \quad (4.3.30)$$

Each phase has a geometric description [19]: in phase I, we get a line bundle over the blowup of  $\mathbb{P}^{(1,1,2,2,2)}$  along its singular locus, in phase II, we get a line bundle over  $\mathbb{P}^{(1,1,2,2,2)}$  itself, in phase III we get  $\mathbb{C}^5/\mathbb{Z}_8$ , and in phase IV we get

$$\left(\mathbb{C}^3 \times \mathcal{O}_{\mathbb{P}^1}(2)\right)/\mathbb{Z}_4. \quad (4.3.31)$$

The phase of relevance for comparison to the nonlinear sigma model is the geometric phase, phase I.

We still must impose the F-term equations, and in doing so, we can be more specific concerning our “generic” assumptions about the superpotential (4.3.24). We assume that  $F_{(4,0)}(\phi_1, \phi_2, \phi_3, \phi_4, \phi_5, 1)$  is a transverse homogeneous polynomial in 5 variables (which means that the origin is the only common zero of the partial derivatives), and that  $F_{(4,0)}(\phi_1, \phi_2, \phi_3, \phi_4, \phi_5, 0)$ , which is independent of  $\phi_1$  and  $\phi_2$ , is a transverse homogeneous polynomial of 3 variables. The F-term equations are

$$\frac{\partial W}{\partial \phi_J} = 0, \quad J = 0, \dots, 6. \quad (4.3.32)$$

To solve the F-term equations, we note that  $\partial W/\partial \phi_0 = F$ , and that  $\phi_0$  divides  $\partial W/\partial \phi_J$  for  $J \neq 0$ . Thus, one solution is

$$\phi_0 = F = 0. \quad (4.3.33)$$

If  $\phi_0 \neq 0$  but  $\phi_6 = 0$ , then  $(\partial F/\partial \phi_j)|_{\phi_6=0} = 0$  for  $J = 3, 4, 5$ , which implies (by transversality) that

$$\phi_3 = \phi_4 = \phi_5 = \phi_6 = 0. \quad (4.3.34)$$

Moreover, there is no monomial appearing in  $F$  which involves only the variables  $\phi_1$  and  $\phi_2$ , so  $F$  vanishes on the locus (4.3.34) and we see that (4.3.34) provides a second solution to the F-term equations. Finally, if  $\phi_0 \neq 0$  and  $\phi_6 \neq 0$ , then the transversality of  $F(\phi_1, \phi_2, \phi_3, \phi_4, \phi_5, 1)$  implies that

$$\phi_1 = \phi_2 = \phi_3 = \phi_4 = \phi_5 = 0 \quad (4.3.35)$$

is also a solution (because there is no power of  $\phi_6$  is a monomial).

In phase I, we see that that only possible solution is  $\{\phi_0 = F = 0\}$ . This defines a hypersurface  $F = 0$  inside the zero-section  $\{\phi_0 = 0\}$  of the line bundle. In other words, we get a hypersurface in the blowup of  $\mathbb{P}^{(1,1,2,2,2)}$  along its singular locus. The requirement (4.3.13)

(guaranteeing anomaly-free  $R$ -symmetry and integral  $R$ -charges up to gauge transformation) is precisely the condition for the hypersurface to be Calabi–Yau. This is a general phenomenon for toric hypersurfaces [56].

The other solutions to the F-term equations are relevant in other phases: in phase II, we again get (4.3.33); in phase III, we get (4.3.35); and in phase IV, we get (4.3.34).

## 4.4 Quantum corrections to the Kähler potential

In this section, we discuss quantum effects in the  $\mathcal{N} = (2, 2)$  supersymmetric two-dimensional nonlinear  $\sigma$ -model on a Calabi–Yau manifold  $X$  of arbitrary dimension. As noted above, the Kähler potential  $K_c$  on the chiral conformal manifold is not subject to corrections. However, the Kähler potential  $K_{tc}$  on the twisted chiral conformal manifold is subject to perturbative corrections which have been determined in detail in [22], as well as non-perturbative instanton corrections described in terms of Gromov–Witten invariants. We describe the perturbative corrections both in terms of expressions in the Riemannian curvature (integrated over  $X$ ) and in terms of cohomology classes (evaluated on the fundamental homology class of  $X$ ).

### 4.4.1 Nonlinear $\sigma$ -model action and the effective action

Under the renormalization group an  $\mathcal{N} = (2, 2)$  supersymmetric, two-dimensional, nonlinear  $\sigma$ -model with Kähler target space  $X$  (of complex dimension  $n$ ), flows in the infrared to a conformal fixed point characterized by vanishing  $\beta$ -functions. In this section, the  $\beta$ -function of the target space Kähler form is of particular interest, which vanishes at tree level but is nonzero at one-loop:

$$\frac{1}{\alpha'}\beta_{i\bar{j}} = R_{i\bar{j}} + \Delta\omega_{i\bar{j}}(\alpha') = R_{i\bar{j}} + \alpha'^3 \frac{\zeta(3)}{48} T_{i\bar{j}} + O(\alpha'^5) . \quad (4.4.1)$$

Here  $\alpha'$  is the coupling constant in the nonlinear  $\sigma$ -model. At leading one-loop order, the Ricci tensor  $R_{i\bar{j}}$  appears;  $\Delta\omega_{i\bar{j}}$  then comprises all higher loop corrections, which are exact in cohomology, i.e.,  $\Delta\omega = d\rho$  with some global one form  $\rho$  on  $X$  [34, 57]. The tensor  $T_{i\bar{j}}$  is the first non-vanishing subleading correction at four loops [58], which has been explicitly calculated in [59]. (The five-loop correction at order  $O(\alpha'^4)$  has been shown to vanish [60].) Thus, at leading order the vanishing  $\beta$ -function  $\beta_{i\bar{j}} = 0$  requires a Ricci-flat Kähler metric and hence a Calabi–Yau target space. However, this Ricci-flat Calabi–Yau target space metric gets further corrected at higher loops.

To analyze these corrections, it is useful to adopt an effective action point of view for the target space geometry. Namely, we interpret the condition for the vanishing  $\beta$ -function as the Euler–Lagrange equation for the metric  $g_{i\bar{j}}$  arising from an action functional [58, 61]. The relevant effective action  $\mathcal{S}_{\text{eff}}[g]$  takes the form

$$\mathcal{S}_{\text{eff}}[g] = \int \sqrt{g} [R(g) + \Delta S(\alpha', g)] , \quad (4.4.2)$$

with the corrections  $\Delta S(\alpha', R)$ . The leading correction arises at fourth loop order  $\alpha'^3$  and enjoys the expansion

$$\Delta S(\alpha', g) = \alpha'^3 S^{(4)}(g) + \alpha'^5 S^{(6)}(g) + \dots \quad (4.4.3)$$

Here the  $n$ -th loop correction  $S^{(n)}(g)$  is a scalar functional of the metric tensor and the Riemann tensor. A proposal for the structure of these terms was put forward in [62].

Since the effective action  $\mathcal{S}_{\text{eff}}[g]$  gets corrected beyond the leading contribution, we expect the classical metric on  $\mathcal{M}_{tc}$  to receive further corrections from higher loop orders. Using mirror symmetry, the tree level term and four-loop correction in the case of Calabi–Yau threefolds were determined to be [5]

$$e^{-K_{tc}} = \frac{1}{3!} \left( \sum_{j=1}^s 2 \operatorname{Im} t_j L_j \right)^3 [X] + \alpha'^3 \left( -\frac{1}{4\pi^3} \zeta(3) c_3(X) \cup \left( \sum_{j=1}^s 4\pi \operatorname{Im} t_j L_j \right)^0 \right) [X] + O(e^{2\pi i t}) , \quad (4.4.4)$$

expressed in terms of the Chern class  $c_3(X)$  and a special value of the Riemann  $\zeta$ -function. The appearance of the  $\zeta$ -value  $\zeta(3)$  (of transcendental weight three) indicates its origin as a four-loop counterterm of the  $\mathcal{N} = (2, 2)$  supersymmetric nonlinear  $\sigma$ -model [59].

In general, further corrections in  $\alpha'$  appear for Calabi–Yau target spaces of higher dimension  $n > 3$ . They take the following form in which  $\alpha'$  is indicated explicitly (although it is set equal to 1 elsewhere in this review):

$$e^{-K_{tc}} = \left( \exp \left( \sum_{j=1}^s 2 \operatorname{Im} t_j L_j \right) + \frac{1}{(2\pi)^n} \sum_{k=0}^n \alpha'^k \chi_k \right) [X] + O(e^{2\pi i t}) , \quad (4.4.5)$$

where the characteristic class  $\chi_k$  arises from the perturbative loop corrections at loop order  $k + 1$ . (Thanks to [60] we expect  $\chi_4$  to vanish.) Due to the appearance of higher curvature tensors in the corrections  $\Delta\omega_{i\bar{j}}$  of the  $\beta$ -function (4.4.1), we can expect that integrating such curvature tensors can be expressed in terms of the Chern classes of the tangent bundle of the target space  $X$ . Furthermore, the loop corrections appearing in  $\Delta\omega_{i\bar{j}}$  at a given loop order  $k + 1$ , i.e., at order  $\alpha'^k$ , give rise to corrections with transcendental degree  $k$ , which is a general property of loop corrections of supersymmetric two-dimensional  $\sigma$ -models [63]. As a result, the cohomology classes  $\chi_k$  are homogeneous elements of transcendental degree  $k$  in the graded polynomial ring over all products of multiple  $\zeta$ -values up to transcendental weight  $k$

$$\chi_k \in H^{2k}(X, \mathbb{Q})[\zeta(m)_{2 \leq m \leq k}, \zeta(m_1, m_2)_{2 \leq m_1 + m_2 \leq k}, \dots, \zeta(1, \dots, 1)]_k . \quad (4.4.6)$$

The transcendental weight of a multiple  $\zeta$ -value  $\zeta(m_1, \dots, m_a)$  is given by the sum  $m_1 + \dots + m_a$ , and the multiple zeta functions  $\zeta(m_1, \dots, m_a)$  generalize the Riemann zeta function according to [64]

$$\zeta(m_1, \dots, m_a) = \sum_{n_1 > n_2 > \dots > n_a} \frac{1}{n_1^{m_1} \dots n_a^{m_a}} . \quad (4.4.7)$$

Note that there are many non-trivial relations over  $\mathbb{Q}$  among such multiple  $\zeta$ -values; see for instance [65].

## 4.4.2 Perturbative corrections to the Kähler potential

Perturbative corrections to  $e^{-K_{tc}}$  were found in [22], assuming that all corrections take the universal form (4.4.5), by using mirror symmetry and period computations to determine the values of  $\chi_k$ . The answers can be expressed in terms of a characteristic class known as the “gamma class” [66–70], [55], but we will take a more direct approach and present the corrections explicitly both in terms of Riemannian curvature and in terms of Chern classes.

The corrections to the Kähler potential involve the Riemann curvature tensor, which we denote by  $\mathcal{R}$  (suppressing indices) and regard as a differential-form-valued endomorphism of the tangent bundle of  $M$ . If we take the trace over tangent bundle indices, we obtain a 2-form  $\text{tr}(\mathcal{R})$  which is just the familiar Ricci tensor  $R_{ij}$  with indices suppressed. We will also consider traces of higher powers (i.e., composing the endomorphism with itself a number of times):  $\text{tr}(\mathcal{R}^\ell)$  defines a  $2\ell$ -form.

We can now state the perturbative corrections to the classical metric (4.3.4) which were derived in [22], in the case of  $c_1(X) = 0$ :

$$K_{tc} = -\log \frac{1}{(2\pi)^n} \int_X \exp \left( 2 \text{Re} \left( \sum t_j \mathcal{F}_j \right) - 2 \sum_{k=1}^{\infty} \frac{\zeta(2k+1)}{2k+1} \text{tr} \left( (i\mathcal{R}/2\pi)^{2k+1} \right) \right) + \mathcal{O}(e^{2\pi it}) . \quad (4.4.8)$$

To write this in terms of integer cohomology classes, we need to use Newton’s identities which express  $\sum_{j=1}^n x_j^\ell$  in terms of the elementary symmetric functions  $\sigma_1, \sigma_2, \dots, \sigma_n$  of  $\{x_1, x_2, \dots, x_n\}$ . If we write

$$\sum_{j=1}^n x_j^\ell = P_\ell(\sigma_1, \sigma_2, \dots, \sigma_\ell) , \quad (4.4.9)$$

then by Chern–Weil theory,

$$\int_X \text{tr} \left( (i\mathcal{R}/2\pi)^\ell \right) = P_\ell(c_1, c_2, \dots, c_\ell) . \quad (4.4.10)$$

Thus, we can express the perturbative corrections to (4.3.5) in the form

$$e^{-K_{tc}} = \exp \left( \sum 2 \text{Im}(t_j) L_j - \frac{2}{(2\pi)^n} \sum_{k=1}^{\infty} \frac{\zeta(2k+1)}{2k+1} P_{2k+1}(c_1, c_2, \dots, c_{2k+1}) \right) [X] + \mathcal{O}(e^{2\pi it}) , \quad (4.4.11)$$

where  $c_1 = 0$ ,  $c_2, c_3, \dots$  are the Chern classes of  $X$ .

For Calabi–Yau threefolds, the perturbative correction (4.4.4) found in [5] gives the complete answer. However, in order to evaluate these expressions for Calabi–Yau manifolds of higher dimension, it is convenient to have the first several (odd) Newton’s identities at our disposal, which we give with  $\sigma_1$  set to 0:

$$\begin{aligned} P_1|_{\sigma_1=0} &= 0 \\ P_3|_{\sigma_1=0} &= 3\sigma_3 \\ P_5|_{\sigma_1=0} &= -5\sigma_2\sigma_3 + 5\sigma_5 \\ P_7|_{\sigma_1=0} &= 7\sigma_2^2\sigma_3 - 7\sigma_2\sigma_5 - 7\sigma_3\sigma_4 + 7\sigma_7 \end{aligned} \quad (4.4.12)$$

Setting  $c_1 = 0$  and expanding the exponential in (4.4.11), we find the first few perturbative corrections

$$\begin{aligned}
\chi_3 &= -2\zeta(3)c_3 \\
\chi_4 &= 0 \\
\chi_5 &= 2\zeta(5)(c_2c_3 - c_5) \\
\chi_6 &= 2\zeta(3)^2c_3^2 \\
\chi_7 &= -2\zeta(7)(c_2^2c_3 - c_3c_4 - c_2c_5 + c_7)
\end{aligned}
\tag{4.4.13}$$

in terms of the Chern classes  $c_k$  of the Calabi–Yau  $n$ -fold  $X$ . The contributions  $\chi_3$  and  $\chi_4$  are exactly what appear in [5, 71].

### 4.4.3 Nonperturbative corrections and Gromov–Witten invariants

The nonperturbative corrections to a two-dimensional nonlinear sigma model are due to instantons, i.e., action-minimizing maps from a Euclidean spacetime to the target manifold, and the relevant corrections to the metric on  $\mathcal{M}_{tc}$  are given by instantons of genus zero.

In order to describe the instanton corrections to the Zamolodchikov metric, we must first describe instanton corrections to certain other quantities in the theory. The twisted chiral operators in the theory have a natural ring structure determined by the two-point and three-point genus zero correlation functions in terms of a “Frobenius algebra” structure [72]. This determination goes as follows: given a ring  $R$  with a nondegenerate bilinear form

$$(-, -) : R \times R \rightarrow \mathbb{C}, \tag{4.4.14}$$

there is a natural trilinear map

$$\langle ABC \rangle := (A \star B, C), \tag{4.4.15}$$

where  $\star$  denotes the product in the ring. (When evaluated on a basis of  $R$ , this gives the structure constants for the ring.) Conversely, whenever we are given a bilinear form (4.4.14) and a trilinear form (4.4.15), we get a product on  $R$ .

These two-point and three-point correlation functions can be computed equally well in the closely related “topological sigma model” [7], in which the spins of the fields are modified and a suitable projection is performed.<sup>14</sup> The twisted chiral operators in the topological theory can be identified with harmonic forms (or their cohomology classes) on the target manifold  $X$ , and the ring structure in the classical theory is simply the cup product pairing in cohomology. However, this ring structure is deformed by instanton contributions [7, 74, 75] in the quantum theory, giving rise to the “quantum cohomology ring” of  $X$  (which is known to be associative [76–78]).

To describe the instanton contributions, we represent cohomology classes  $A$ ,  $B$ , and  $C$  by algebraic cycles on  $X$ ; the correlation function is calculated by integrating over the space of maps  $\pi$  from the genus one spacetime with three points  $p, q, r$  specified such that  $\pi(p)$

---

<sup>14</sup>We are considering here the “A-model” of [73].

lies in  $A$ ,  $\pi(q)$  lies in  $B$ , and  $\pi(r)$  lies in  $C$ ; a standard localization procedure reduces the computation to determining the space of volume-minimizing maps. The classical contribution to the correlation function comes from constant maps, and simply counts common points of intersection of  $A$ ,  $B$ , and  $C$ . Since the two-point function can also be expressed in terms of intersections, the Frobenius algebra construction reproduces the familiar cup product on cohomology (which counts intersections of the corresponding algebraic cycles), as mentioned above.

For nonconstant maps, it turns out that the image of  $\pi$  has a deformation space whose dimension is expected to be  $\dim X - 3$  (since the spacetime has genus zero).<sup>15</sup> Imposing the conditions on  $\pi(p)$ ,  $\pi(q)$ , and  $\pi(r)$  then cuts down the dimension to zero, and the corresponding maps can be counted. If we fix the homology class  $\eta$  of the image, then the Gromov–Witten invariant  $GW_{0,3}^{X,\eta}(A, B, C)$ , which has a precise mathematical definition, is intended to count the number of maps.

Each instanton contribution is weighted by the instanton action  $e^{\int_{\eta} S} = e^{2\pi i \tau \cdot \eta}$ , which we often denote by  $q^\eta$ . The quantum product can be written as

$$A \star B := A \cup B + \sum_{\eta} (A \star B)_{\eta} q^{\eta} \quad (4.4.16)$$

where  $(A \star B)_{\eta}$  is the unique class satisfying

$$((A \star B)_{\eta} \cup C) [X] = GW_{0,3}^{X,\eta}(A, B, C) \quad (4.4.17)$$

for all  $C$ . We can restrict the sum (4.4.16) to only range over those classes  $\eta$  in  $H_2(X, \mathbb{Z})$  whose intersection with each Kähler class is nonnegative.

Due to orbifold singularities in the deformation spaces, the mathematical definition of Gromov–Witten invariants only guarantees that they are rational numbers, not integers. The physical reason for this is understood, and stems from a “multiple covering” phenomenon. If the map  $\pi$  factors through a multiple covering  $S^2 \rightarrow S^2$  of degree  $m$ , then the homology class of the image takes the form  $\eta = m\varphi$  but, as argued in [82] in dimension three and [83] in arbitrary dimension (see also [84]), the count of maps is the same.

We can take this into account by defining a modified Gromov–Witten invariant  $\widetilde{GW}_{0,3}^{X,\varphi}(A, B, C)$  which should only count the maps of degree one. If we collect terms according to degree one maps, we find a total instanton contribution of

$$\sum_{\varphi \in H_2(X, \mathbb{Z})} \widetilde{GW}_{0,3}^{X,\varphi}(A, B, C) \frac{q^{\varphi}}{1 - q^{\varphi}} = \sum_{\varphi \in H_2(X, \mathbb{Z})} \widetilde{GW}_{0,3}^{X,\varphi}(A, B, C) \sum_{m=1}^{\infty} q^{m\varphi} . \quad (4.4.18)$$

Extracting the coefficient of  $q^\eta$ , we obtain a formula

$$GW_{0,3}^{X,\eta}(A, B, C) = \sum_{\eta=m\varphi} \widetilde{GW}_{0,3}^{X,\varphi}(A, B, C) \quad (4.4.19)$$

---

<sup>15</sup>When the deformation space fails to have the expected dimension, there is a natural way to integrate over the excess deformations to still produce a “count” of maps satisfying the three conditions [79–81].

which can be used to define the modified Gromov–Witten invariants. They are expected to be integers.

For Calabi–Yau threefolds, there is one further modification which can be made to the definitions. The expected dimension of the deformation spaces in that case is zero, so we expect only a finite number of possibilities (in a fixed homology class) for the image of  $\pi$ . For each rational curve of class  $\varphi$ , there are  $(A \cdot \varphi)$  choices for the location of  $\pi(p)$ ,  $(B \cdot \varphi)$  choices for the location of  $\pi(q)$ , and  $(C \cdot \varphi)$  choices for the location of  $\pi(r)$ . It is then natural to define the “Gromov–Witten instanton number” of genus 0 and class  $\varphi$  to be

$$N_\varphi = \frac{\widetilde{GW}_{0,3}^{X,\varphi}(A, B, C)}{(A \cdot \varphi)(B \cdot \varphi)(C \cdot \varphi)} \quad (4.4.20)$$

which is expected to be an integer, independent of  $A, B, C$ , that counts the number of rational curves in class  $\varphi$ .

Having spelled out in detail how instantons determine the quantum cohomology ring, we can now explain the nonperturbative corrections to the Zamolchikov metric. If we substitute

$$2\operatorname{Im}(t_j) = i(\bar{t}_j - t_j) \quad (4.4.21)$$

into the perturbative expression for the metric (4.4.11), we obtain an expression involving cup products between twisted chiral operators (labeled by  $t_j$ ) and their complex conjugates (labeled by  $\bar{t}_j$ ). For the former, we can make computations in the quantum cohomology ring instead, replacing  $\cup$  by  $\star$ . For the latter, we should use the complex-conjugated cohomology ring, with instanton actions  $\bar{q}^\eta$  rather than  $q^\eta$ . That is, we can do those computations in complex-conjugated quantum cohomology, replacing  $\cup$  by  $\bar{\star}$ .

In other words, the prescription for nonperturbative corrections to the perturbative formula (4.4.11) is: perform the multiplications among holomorphic terms using  $\star$  and among anti-holomorphic terms using  $\bar{\star}$ ; then multiply the pieces together using cup product.<sup>16</sup>

Let us spell this out explicitly for Calabi–Yau threefolds. The perturbative expression can be written as

$$\frac{i}{6}(\sum t_j L_j)^3 - \frac{i}{2}(\sum t_j L_j)^2(\sum \bar{t}_j L_j) + \frac{i}{2}(\sum t_j L_j)(\sum \bar{t}_j L_j)^2 - \frac{i}{6}(\sum \bar{t}_j L_j)^3 - \frac{\zeta(3)}{4\pi^3}c_3(X). \quad (4.4.22)$$

---

<sup>16</sup>This prescription matches the formulas in [11] in dimension three and [71] in dimension four, as well as considerations from mirror symmetry.

When nonperturbative corrections are included, this becomes

$$\begin{aligned}
& \frac{i}{6} \left( \sum t_j t_k t_\ell \left( (L_j \cup L_k \cup L_\ell)[X] + \sum_\eta GW_{0,3}^{X,\eta}(L_j, L_k, L_\ell) q^\eta \right) \right) \\
& - \frac{i}{2} \left( \sum t_j t_k \bar{t}_\ell \left( (L_j \cup L_k \cup L_\ell)[X] + \sum_\eta GW_{0,3}^{X,\eta}(L_j, L_k, L_\ell) q^\eta \right) \right) \\
& + \frac{i}{2} \left( \sum t_j \bar{t}_k \bar{t}_\ell \left( (L_j \cup L_k \cup L_\ell)[X] + \sum_\eta GW_{0,3}^{X,\eta}(L_j, L_k, L_\ell) \bar{q}^\eta \right) \right) \\
& - \frac{i}{6} \left( \sum \bar{t}_j \bar{t}_k \bar{t}_\ell \left( (L_j \cup L_k \cup L_\ell)[X] + \sum_\eta GW_{0,3}^{X,\eta}(L_j, L_k, L_\ell) \bar{q}^\eta \right) \right) - \frac{\zeta(3)}{4\pi^3} c_3(X).
\end{aligned} \tag{4.4.23}$$

## 4.5 The two-sphere partition function and Gromov–Witten invariants

### 4.5.1 The $S^2$ partition function for a GLSM

Consider an  $\mathcal{N} = (2, 2)$  GLSM with gauge group  $G$ , chiral fields  $\Phi_J$  of  $R$ -charge  $q_J$  on which  $G$  acts by the representation  $\Psi : S \rightarrow SU(N)$ , superpotential  $W$ , and complexified FI-parameters  $\frac{\vartheta}{2\pi} + i\zeta \in \text{Ann}([\mathfrak{g}, \mathfrak{g}]_{\mathbb{C}}) \subset \mathfrak{g}_{\mathbb{C}}^*$ . As in Section 4.3.2, we fix a Cartan subgroup  $H$  of  $G$  and weights  $w_J \in \Lambda_{\text{wt}} \subset \mathfrak{h}^*$  describing the eigenvalues of  $\Psi|_H$ .<sup>17</sup>

The possible fluxes of the gauge theory through the 2-sphere are GNO quantized [85], which means that they are integer-valued functions on the weight lattice, i.e., elements  $\mathfrak{m}$  of the coweight lattice  $\Lambda_{\text{wt}}^{\vee} \subset \mathfrak{h}$ . The combinations  $i\sigma \pm \frac{\mathfrak{m}}{2}$  are what appear in the formulas.

In [13, 14], a computation of  $Z_{S^2}$  for a 2-sphere of radius  $r$  is made by expanding on the Coulomb branch and using localization, after modifying the Lagrangian appropriately to put the theory on  $S^2$ . The original papers include twisted masses related to flavor symmetries of the theory but we shall not include those as they are not relevant for our application. Since we are only studying the theories which are conformal in the infrared, the only dependence on the radius is through a multiplicative factor. Some additional notation:  $|\mathcal{W}|$  denotes the order of the Weyl group of  $G$ ,  $\Delta^+$  denotes the set of positive roots of  $G$  (a subset of the weight lattice), and  $\rho = \frac{1}{2}(\sum_{\alpha \in \Delta^+} \alpha)$  is the Weyl vector. Here is the final formula, which assumes that all  $R$ -charges have been chosen in the range  $0 < q < 2$ :

$$\frac{Z_{S^2}(z, \bar{z})}{(r/r_0)^{c/3}} = \frac{1}{|\mathcal{W}|} \sum_{\mathfrak{m} \in \Lambda_{\text{wt}}^{\vee}} \int_{\mathfrak{h}} \left( \prod_{\mu=1}^{\text{rank}(G)} \frac{d\sigma_{\mu}}{2\pi} \right) Z_{\text{class}}(\sigma, \mathfrak{m}) Z_{\text{gauge}}(\sigma, \mathfrak{m}) Z_{\text{matter}}(\sigma, \mathfrak{m}), \tag{4.5.1}$$

<sup>17</sup>Note that we are organizing things slightly differently from the way the matter representation is described in [13, 14]. With our conventions, each  $\phi_J$  spans a one-dimensional space which is preserved by the action of  $H$  and thus is identified with a weight of the representation  $\Psi$ . In [13, 14], the representation was decomposed into irreducible representations of  $G$  (labeled by  $\phi_J$ , each of which had additional indices in those papers), and then each of those irreducible representations was decomposed into weight spaces.

where

$$\begin{aligned}
Z_{\text{class}} &= \exp\langle \log z, i\sigma + \frac{\mathbf{m}}{2} \rangle \exp\langle \log \bar{z}, i\sigma - \frac{\mathbf{m}}{2} \rangle = e^{-4\pi(\zeta, i\sigma) + \langle i\vartheta, \mathbf{m} \rangle} \\
Z_{\text{gauge}} &= (-1)^{2\rho \cdot \mathbf{m}} \prod_{\alpha \in \Delta^+} \left( (\alpha \cdot \sigma)^2 + \frac{1}{4}(\alpha \cdot \mathbf{m})^2 \right), \\
Z_{\text{matter}} &= \prod_J \frac{\Gamma\left(\frac{q_J}{2} - w_J \cdot i\sigma - \frac{1}{2}w_J \cdot \mathbf{m}\right)}{\Gamma\left(1 - \frac{q_J}{2} + w_J \cdot i\sigma - \frac{1}{2}w_J \cdot \mathbf{m}\right)}.
\end{aligned} \tag{4.5.2}$$

We have included an overall sign in  $Z_{\text{gauge}}$ , missing in [13, 14], whose necessity was pointed out in [55, 86].

## 4.5.2 The hemisphere partition function and the $tt^*$ equations

As discussed above, the partition function of a GLSM has been evaluated on a 2-sphere [13, 14]. The partition function has also been evaluated on a hemisphere, that is, a half-sphere  $D^2$  equipped with the spherical metric [55, 86, 87], as well as on real projective 2-space [88]. A full discussion of these results is beyond the scope of this review, but we will briefly present the result for the hemisphere, following [55].

We need to specify BPS boundary conditions for the GLSM along the boundary of the hemisphere, and the natural type of boundary conditions to use are ‘‘B-branes’’ [89, 90]. The spectrum of B-branes is locally constant over  $\mathcal{M}_{tc}$ , and the data needed to specify B-branes in a GLSM was thoroughly analyzed in [54].

Having specified some B-brane data  $\mathcal{B}$ , the partition function  $Z_{D^2, \mathcal{B}}$  on a hemisphere of radius  $r$  is evaluated explicitly in [55]. The dependence on the radius is via an overall factor (which is the square root of the corresponding factor in  $Z_{S^2}$ ). The dependence of the hemisphere partition function on the choice  $\mathcal{B}$  of B-brane comes through a factor  $f_{\mathcal{B}}(\sigma)$  in the integrand described in [55], to which we refer for further details (see also [42]).

In order to evaluate the partition function, an appropriate integration contour  $\gamma \subset \mathfrak{h}_{\mathbb{C}}$  must be chosen. With this understood, the result of [55] is:

$$\frac{Z_{D^2, \mathcal{B}}(z, \bar{z})}{(r/r_0)^{c/6}} = \frac{1}{|\mathcal{W}|} \int_{\gamma} \prod_{\mu=1}^{\text{rank}(G)} \frac{d\sigma_{\mu}}{2\pi} e^{-4\pi i(\zeta, \sigma)} \prod_{\alpha \in \Delta^+} \alpha \cdot \sigma \sinh(\pi \alpha \cdot \sigma) \prod_J \Gamma\left(\frac{q_J}{2} - w_J \cdot i\sigma\right) f_{\mathcal{B}}(\sigma), \tag{4.5.3}$$

where  $\zeta = -\frac{1}{2\pi} \text{Re} \log z$ . The authors of [55] interpret this formula as specifying a BPS charge for each choice of boundary condition, and they verify that it agrees with the BPS charge in circumstances under which both can be computed.

It is natural to expect that the hemisphere partition function will play an important role in some yet-to-be-established holomorphic factorization property for two-sphere partition functions. Indeed, for the analogous three-dimensional gauge theories with  $\mathcal{N} = 2$  supersymmetry, the partition function computed in [91, 92] displays such a factorization. (This fact was noted in [93], and further explored in [94].) The authors of [55] have taken an important step in this direction in the 2D case by analyzing the GLSM partition function on an annulus and studying how it can be used to glue together the results on the two hemispheres to reproduce

the result on the sphere. Their calculation is not completely general, but for theories with a geometric phases they verify that such a factorization result does indeed hold.

An alternate approach to such a factorization result might proceed by means of the “ $tt^*$  equations” of [95], as suggested in [11, 15]. The  $tt^*$  equations describe the Zamolodchikov metric in terms of topological twists of the GLSM: it is equal to the overlap of ground states in the  $A$ -twisted GLSM on one hemisphere, and an  $\bar{A}$ -twisted GLSM on the other hemisphere. The authors of [15] carry out a computation of such an overlap by means of a calculation on the squashed two-sphere, which has different limiting interpretations as the squashing parameter is varied. We refer to [15] for further details.

### 4.5.3 Extracting Gromov–Witten invariants from the partition function

We now explain how, with the Euler characteristic  $\chi(X) = c_3(X)$  as additional input, the relationship between the Kähler potential and the two-sphere partition function can be used to extract the Gromov–Witten invariants from the partition function  $Z_{S^2}$  in the case of a Calabi–Yau threefold  $X$ . The form of the partition function which we have determined for a nonlinear sigma model depends on a choice of coordinates, so our task is to use the asymptotic behavior of  $Z_{S^2}$  to determine the appropriate coordinates. For ease of exposition, in this section we will assume that we have chosen FI coordinates so that a neighborhood of  $\{z_a = 0 \text{ for all } a\}$  describes a geometric phase of the GLSM.

To bring the partition function  $Z_{S^2}(z, \bar{z})$  into an appropriate normal form and to extract the Gromov–Witten invariants, we use the following algorithm:

1. Evaluate  $Z_{S^2}(z, \bar{z}) = e^{-K_{tc}}$  by contour integration as an expansion around large volume. (We will discuss this step in more detail in the next section.) The result can be expressed in terms of logarithmic coordinates  $\tau_j = \frac{1}{2\pi i} \log z_j$ , and the goal is to find a change of coordinates from  $\tau_j$  to  $t_j$ .
2. Isolate the perturbative  $\zeta(3)$  term and perform a Kähler transformation  $K = K' + X^0(z) + \overline{X^0(z)}$  in order to reproduce the constant term  $-\frac{\zeta(3)}{4\pi^3} \chi(X)$  in (4.4.4) and (4.4.23); (The initial  $\zeta(3)$  term might have a non-constant coefficient, which gives rise to a nontrivial Kähler transformation.)
3. Read off the holomorphic part of the coefficient of  $\bar{\tau}_j \bar{\tau}_k = \frac{1}{(2\pi i)^2} \log \bar{z}_j \log \bar{z}_k$ , which should then be identified with

$$-\frac{i}{2} \sum_{\ell} (L_j \cup L_k \cup L_{\ell})[X] t_{\ell} . \quad (4.5.4)$$

Use this to extract the NLSM coordinates  $t_{\ell}$ , which must have the form

$$t_{\ell} = \frac{\log z_{\ell}}{2\pi i} + f_{\ell}(z) , \quad (4.5.5)$$

where  $f_{\ell}(z)$  is a holomorphic function. This determines the NLSM coordinates up to the undetermined constants  $f_{\ell}(0)$ .

4. Invert the GLSM/NLSM map<sup>18</sup> (4.5.5) to obtain the  $z_\ell$  as a function of  $t_\ell$ ,

$$z_\ell = e^{-2\pi i f_\ell(0)} \left( q_\ell + O(q^2) \right), \quad (4.5.6)$$

where  $q_\ell := e^{2\pi i t_\ell}$ ;

5. Fix the constant terms  $f_\ell(0)$  by demanding the lowest order terms in the instanton expansion be positive; and, finally,
6. Read off the (rational) Gromov–Witten invariants  $GW_{0,3}^{X,\eta}(A, B, C)$  from the coefficients in the  $q$ -expansion. The (integral) Gromov–Witten instanton numbers  $N_\eta$  of genus zero (roughly, the “number of rational curves”) can then be obtained from the multi-covering formulas (4.4.19) and (4.4.20).

## 4.6 Evaluating the partition function

The low-energy effective theory describing the dynamics of the GLSM depends on the value of the FI-parameters [18]. The space of FI-parameters can be divided into phase regions depending on the character of the low-energy dynamics as explained in Section 4.3.3. In this section we show how this phase structure is closely related to structure of the integrand of the two-sphere partition function, and how this observation can be used to determine Gromov–Witten invariants explicitly.

The idea is stated rather simply: when  $Z_{S^2}$  is evaluated by the method of residues, the contour prescription depends on the value of the FI-parameters, which in turn affects the set of poles that contribute to the integral. At certain codimension-one walls in FI-parameter space the structure of poles contributing to the  $Z_{S^2}$  integral can change, signaling the presence of a GLSM phase transition along that wall. In particular, for abelian GLSMs we show that this phase structure is precisely the same secondary fan which governs the low-energy physics. Furthermore, we also describe how phases of non-abelian GLSMs can be understood in terms of phases of an associated “Cartan” theory.

### 4.6.1 Analytic structure of the partition function

When the integrand in equation (4.5.1) is analytically continued to complex values of  $\sigma \in \mathfrak{h}_\mathbb{C}$ , it becomes a meromorphic function of the integration variables. In order to evaluate this integral by means of residues, we need to identify the location of all poles in that integrand. We observe that the gauge factor  $Z_{\text{gauge}}$  never contributes poles and the integrand has the same analytic structure if this term is omitted. In fact, if we retain the same matter content but restrict the gauge group to a Cartan subgroup  $H$ , then up to a constant, we simply omit the previous  $Z_{\text{gauge}}$  factor while retaining the  $Z_{\text{classical}}$  and  $Z_{\text{matter}}$  factors. For the purposes

---

<sup>18</sup>This is the analogue of the much-studied “mirror map” relating chiral and twisted chiral conformal manifolds of a mirror pair [43].

of analyzing the analytic structure of the integrand, we may thus restrict ourselves to abelian gauge theories without loss of generality. See [30] for a further discussion of this point.

The partition function for an abelian GLSM with  $G = H = U(1)^h$  is

$$\frac{Z_{S^2}(z, \bar{z})}{(r/r_0)^{c/3}} = \sum_{\mathbf{m} \in \mathbb{Z}^h} \int_{\mathfrak{h}} \left( \prod_{\mu=1}^h \frac{d\sigma_\mu}{2\pi} \right) e^{-4\pi\langle \zeta, i\sigma \rangle + \langle i\vartheta, \mathbf{m} \rangle} \prod_J \frac{\Gamma\left(\frac{q_J}{2} - w_J \cdot i\sigma - \frac{1}{2}w_J \cdot \mathbf{m}\right)}{\Gamma\left(1 - \frac{q_J}{2} + w_J \cdot i\sigma - \frac{1}{2}w_J \cdot \mathbf{m}\right)}, \quad (4.6.1)$$

assuming as in (4.5.1) that  $0 < q_J < 2$ . Recall that  $\Gamma(z)$  is a meromorphic function in the complex plane with simple poles at  $z = -n$ ,  $n \in \mathbb{Z}_{\geq 0}$ , with residue  $\text{Res}_{z=-n} \Gamma(z) = \frac{(-1)^n}{n!}$  and an essential singularity at  $z = \infty$ . Taking into account cancellations between zeros and poles, the  $J^{\text{th}}$  factor in the final product of the integrand in (4.6.1) has poles along the hyperplanes

$$H_J^{(k)} : \quad \frac{q_J}{2} - w_J \cdot i\sigma - \frac{1}{2}w_J \cdot \mathbf{m} = -k, \quad k \in \mathbb{Z}_{\geq 0}, \quad k \geq w_J \cdot \mathbf{m}. \quad (4.6.2)$$

The partition function integrand can be regarded as a meromorphic function on the space  $\mathbb{C}^{\text{rank}(\mathfrak{g})}$  with poles along the hyperplanes  $H_i^{(k)}$ , which we refer to as *polar divisors*. Note that the collection of hyperplanes  $H_J^{(k)}$  is contained in the half space  $\text{Re}(w_J \cdot i\sigma) \geq 0$ , and also satisfies  $\text{Im}(w_J \cdot i\sigma) = 0$ . The analytic structure of the integrand will be relevant in what follows, as we will evaluate the integral in (4.6.1) through the method of residues after choosing an appropriate way to close the integration contour in  $\mathfrak{h}_{\mathbb{C}}$ .

## 4.6.2 Residues and phases

We use the multi-dimensional residue method [97, 98] to evaluate the  $h$ -dimensional integral in (4.6.1) for an abelian GLSM in terms of ‘‘Grothendieck residues.’’ The integration contour  $\mathfrak{h} = \mathbb{R}^h$  must be replaced by a closed contour  $\gamma$  which meets none of the polar divisors. This is done using a multi-dimensional analogue of the familiar Jordan lemma which replaces an improper integral over the real axis by a contour integral enclosing poles in the lower half-plane; the latter can be evaluated using residues. This can be done provided that the integrand in the lower half-plane dies off at infinity in a suitable way.

Here, we do the same thing for each complex variable in  $\mathfrak{h}_{\mathbb{C}}$ . The resulting integral is of a meromorphic  $h$ -form over an  $h$ -dimensional compact cycle  $\gamma$  which does not intersect the poles of the integrand. By Stokes’ theorem, if we vary the integration cycle without crossing any of the polar divisors, the value of the integral does not change. In particular, since a change of basis of  $\mathfrak{h}$  can be described by a path between the two bases leading to a one-parameter family of contours  $\gamma_t$ ; as long as none of the intermediate contours  $\gamma_t$  intersect any of the polar divisors, the integral does not change. For our primary integral (4.6.1), the growth rate is controlled by the exponential factor and so it is the sign of  $\text{Re}\langle \zeta, i\sigma \rangle$  which matters; if that sign remains positive then the contours  $\gamma_t$  will not encounter the polar divisors.

Each possible transverse intersection of  $h$  polar divisors is associated to an  $h$ -element subset  $\mathcal{J} \subset \{1, \dots, N\}$  such that the  $h$  vectors  $\{w_J, J \in \mathcal{J}\}$  are linearly independent; as in Section 4.3.3, we let  $\mathfrak{J}$  denote the set of all such subsets  $\mathcal{J}$ . The corresponding polar divisors

$H_J^{(k)}$  for all  $J \in \mathcal{J}$  and  $k \in \mathbb{Z}_{\geq 0}$  (defined in (4.6.2)), intersect in an infinite discrete point set that we denote by  $P_{\mathcal{J}}$ . The residue of the integrand at any point  $p \in P_{\mathcal{J}}$  is well defined and can be evaluated.

To determine whether the residues at the points of  $P_{\mathcal{J}}$  contribute to the integrand, we consider the basis  $\{w_J, J \in \mathcal{J}\}$  of  $\mathfrak{h}^*$ , and express the FI-parameters as  $\zeta = \sum_{J \in \mathcal{J}} \zeta_J w_J$ , (which is possible since  $\{w_J \mid J \in \mathcal{J}\}$  is linearly independent). If  $\zeta_J > 0$  for all  $J \in \mathcal{J}$ , then with respect to the dual coordinates  $\sigma_m u$  of  $\mathfrak{h}$ , the contours all close in the lower half-plane and the residues at the points of  $P_{\mathcal{J}}$  are to be included in the integrand. If one or more  $\zeta_J$  is negative, then at least one of the contours closes in the upper half-plane rather than the lower half-plane, and the residue is excluded.

Thus, the cones  $\mathcal{C}_{\mathcal{J}}$  which determine the phase structure of the theory (as explained in Section 4.3.3) also determine which residues to include in an evaluation of the two-sphere partition function (4.6.1).

Let  $\mathcal{C}$  denote the (non-empty) intersection of all cones  $\mathcal{C}_{\mathcal{J}}$  that contain  $\zeta$ . The partition function, for  $\zeta = -\frac{1}{2\pi}z \in \mathcal{C}$ , can be evaluated as

$$\frac{Z_{S^2}(z, \bar{z})}{(r/r_0)^{c/3}} = \sum_{\substack{\mathcal{J} \in \mathfrak{J}, \\ \zeta \in \mathcal{C}_{\mathcal{J}}}} \sum_{p \in P_{\mathcal{J}}} \text{Res}_{\sigma=\sigma_p} \left( \sum_{m \in \mathbb{Z}^s} e^{-4\pi(\zeta, i\sigma) + \langle i\vartheta, m \rangle} \prod_{J=1}^N \frac{\Gamma(\frac{q_J}{2} - w_J \cdot (i\sigma + \frac{m}{2}))}{\Gamma(1 - \frac{q_J}{2} + w_J \cdot (i\sigma - \frac{m}{2}))} \right), \quad (4.6.3)$$

where  $\sigma_p$  denotes the coordinates of the point  $p \in P_{\mathcal{J}}$ . The above expression is an infinite series, whose convergence is controlled by the exponential factor  $e^{-4\pi(\zeta, i\sigma) + \langle i\vartheta, m \rangle}$ , up to a finite shift of  $i\zeta + \frac{1}{2\pi}\vartheta$  due to the exponential asymptotics of the remainder of the integrand. When  $\zeta$  is sufficiently deep inside the cone  $\mathcal{C}$  all summations are convergent.

We thus see that the expression (4.6.1) for  $Z_{S^2}$  is an integral of Mellin–Barnes type, which allows comparison of the behavior in different regions of the FI-parameter space. The Mellin–Barnes technique had been used earlier to study GLSMs [99–101] but here it arises as a property of the two-sphere partition function integrand, rather than being introduced as a mathematical tool to aid in understanding the theory.

### 4.6.3 Gromov–Witten invariants of an example<sup>19</sup>

We consider again the example arising from the resolution of the degree eight hypersurface in the weighted projective space  $\mathbb{P}^{(1,1,2,2,2)}$ , using the GLSM description introduced in Section 4.3.3. The  $R$ -charges on the vector space  $\mathbb{C}^7$  are specified by the (rational) charge vector  $(2 - 4q_1, q_2, q_2, q_1, q_1, q_1, q_1 - 2q_2)$  as a function of the two rational parameters  $q_1$  and  $q_2$ . The requirement of all  $R$ -charges being positive gives the inequalities

$$0 < q_2 < \frac{q_1}{2} < \frac{1}{4}, \quad (4.6.4)$$

<sup>19</sup>I am grateful to my collaborators Jim Halverson, Hans Jockers, Vijay Kumar, Joshua Lapan, and Mauricio Romo for their assistance with this example.

and then it turns out that all  $R$ -charges are less than 2 as well. Deep in the geometric phase (phase I), we can simplify the expression for the partition function (4.5.1) by evaluating the  $\sigma$ -integration of the partition function with the help of residue calculus. Since all the Kähler parameters  $\zeta_\ell$  are positive, we close the  $\sigma$ -integrations in the lower half-planes of the complexified  $\sigma$ -planes. The residues which contribute to the integral correspond to the cones  $C_{\mathcal{J}}$  illustrated in the first quadrant of Figure 4.1. Computing the residues and bearing in mind the charge condition (4.6.4), a straightforward but somewhat tedious algebraic manipulation yields the partition function

$$\begin{aligned}
Z_{S^2}(z, \bar{z}) &= |z_1|^{q_1} |z_2|^{q_2} \operatorname{Res}_{\tilde{\epsilon}=0} \left[ \frac{\pi^5 \sin 4\pi \epsilon_1}{\sin^3 \pi \epsilon_1 \cdot \sin^2 \pi \epsilon_2 \cdot \sin \pi (\epsilon_1 - 2\epsilon_2)} \right. \\
&\quad \times \left( \sum_{k_1, k_2=0}^{+\infty} \frac{\Gamma(4(k_1 - \epsilon_1) + 1) z_1^{k_1 - \epsilon_1} z_2^{k_2 - \epsilon_2}}{\Gamma((k_1 - \epsilon_1) + 1)^3 \Gamma(k_2 - \epsilon_2 + 1)^2 \Gamma(k_1 - \epsilon_1 - 2(k_2 - \epsilon_2) + 1)} \right) \\
&\quad \times \left. \left( \sum_{k_1, k_2=0}^{+\infty} \frac{\Gamma(4(k_1 - \epsilon_1) + 1) \bar{z}_1^{k_1 - \epsilon_1} \bar{z}_2^{k_2 - \epsilon_2}}{\Gamma((k_1 - \epsilon_1) + 1)^3 \Gamma(k_2 - \epsilon_2 + 1)^2 \Gamma(k_1 - \epsilon_1 - 2(k_2 - \epsilon_2) + 1)} \right) \right]. \tag{4.6.5}
\end{aligned}$$

We identify the partition function with the exponentiated Kähler potential, and we follow the algorithm in Section 4.5.3 to arrive at the Kähler potential in flat coordinates. Using the Euler characteristic  $\chi = -168$  as an overall normalization for the  $\zeta(3)$  term, we obtain the transformed Kähler potential  $K'(z, \bar{z})$

$$e^{-K'(z, \bar{z})} = -\frac{1}{8\pi^3 |z_1|^{q_1} |z_2|^{q_2}} \frac{Z_{S^2}(z, \bar{z})}{|X^0(z)|^2}, \quad X^0(z) = \sum_{k_1, k_2=0}^{\infty} \frac{(4k_1)!}{(k_1!)^3 (k_2!)^2 (k_1 - 2k_2)!} z_1^{k_1} z_2^{k_2}. \tag{4.6.6}$$

We observe that the relevant Kähler transformation involves the “fundamental period”  $X^0(z)$  familiar from the toric mirror symmetry program [56, 102]. (This is a common feature of all of the examples which have been computed explicitly [11].) From the  $(\log z_k \log z_\ell)$  terms,  $k, \ell = 1, 2$ , we extract the NLSM coordinates, which have the expansions

$$\begin{aligned}
2\pi i t_1 &= \log z_1 + 104 z_1 - z_2 + 9\,780 z_1^2 + 48 z_1 z_2 - \frac{3}{2} z_2^2 + \dots, \\
2\pi i t_2 &= \log z_2 + 48 z_1 + 2 z_2 + 6\,408 z_1^2 - 96 z_1 z_2 + 3 z_2^2 + \dots.
\end{aligned} \tag{4.6.7}$$

Inverting these maps, from the Kähler potential we find the triple intersection numbers of the Calabi–Yau hypersurface

$$L_1^3 = 8, \quad L_1^2 L_2 = 0, \quad L_1 L_2^2 = 4, \quad L_2^3 = 0, \tag{4.6.8}$$

where  $L_1$  and  $L_2$  are the divisors associated to the Kähler coordinates  $t_1$  and  $t_2$ , and the genus zero Gromov–Witten instanton numbers  $N_{d_1, d_2}$  of degree  $(d_1, d_2)$  listed in Table 4.1. These same numbers had earlier been calculated by means of mirror symmetry [50] but the present calculation is direct.

Our example Calabi–Yau threefold  $X$  exhibits an extremal transition to a different Calabi–Yau threefold  $\widehat{X}$  [50]. Such extremal transitions have been studied in detail in [103–107],

| $N_{d_1, d_2}$ | $d_1=0$ | 1   | 2      | 3         | 4             | 5               | 6                   |
|----------------|---------|-----|--------|-----------|---------------|-----------------|---------------------|
| $d_2=0$        | –       | 640 | 10 032 | 288 384   | 10 979 984    | 495 269 504     | 24 945 542 832      |
| 1              | 4       | 640 | 72 224 | 7 539 200 | 757 561 520   | 74 132 328 704  | 7 117 563 990 784   |
| 2              | 0       | 0   | 10 032 | 7 539 200 | 2 346 819 520 | 520 834 042 880 | 95 728 361 673 920  |
| 3              | 0       | 0   | 0      | 288 384   | 757 561 520   | 520 834 042 880 | 212 132 862 927 264 |
| 4              | 0       | 0   | 0      | 0         | 10 979 984    | 74 132 328 704  | 95 728 361 673 920  |
| 5              | 0       | 0   | 0      | 0         | 0             | 495 269 504     | 7 117 563 990 784   |
| 6              | 0       | 0   | 0      | 0         | 0             | 0               | 24 945 542 832      |
| 7              | 0       | 0   | 0      | 0         | 0             | 0               | 0                   |

Table 4.1: Gromov–Witten instanton numbers of the blown up degree eight Calabi–Yau hypersurface in  $\mathbb{P}^{(1,1,2,2,2)}$  (genus zero).

and a transition arises for the given example as follows. As the curves in the homology class dual to the divisor  $L_2$  in  $X$  are blown down,  $X$  develops (generically) four nodal singularities. The resulting singular threefold  $X_{\text{sing}}$  is a degree eight hypersurface in  $\mathbb{P}^{(1,1,2,2,2)}$  with the nodal points induced from the singularities of the weighted projective space. Alternatively, we may embed  $X_{\text{sing}}$  into  $\mathbb{P}^5$  as the complete intersection of the degree two polynomial  $\widehat{F}_2(\eta_1, \dots, \eta_6) = \eta_1\eta_2 - \eta_3^2$  and a degree four polynomial  $\widehat{F}_4(\eta_1, \dots, \eta_6)$  with the homogeneous coordinates  $\eta_1, \dots, \eta_6$  of  $\mathbb{P}^5$ .  $X_{\text{sing}}$  embedded in  $\mathbb{P}^{(1,1,2,2,2)}$  is associated to the degree eight polynomial  $F_8(\phi_1, \dots, \phi_5) = \widehat{F}_4(\phi_1^2, \phi_2^2, \phi_1\phi_2, \phi_3, \phi_4, \phi_5)$  in terms of the weighted homogeneous coordinates  $\phi_1, \dots, \phi_5$  of  $\mathbb{P}^{(1,1,2,2,2)}$ . Perturbing the polynomial  $\widehat{F}_2$ , we obtain the smooth and deformed Calabi–Yau threefold  $\widehat{X}$  as the complete intersection of degree  $(2, 4)$  in  $\mathbb{P}^5$ .

Due to this extremal transition, the genus zero Gromov–Witten instanton numbers of  $\widehat{X}$  appear as the sum [108]

$$N_\delta(\widehat{X}) = \sum_{d=0}^{+\infty} N_{\delta, d}(X) . \quad (4.6.9)$$

From Table 4.1, we extract the invariants

$$N_\delta(\widehat{X}) = 1\,280, 92\,288, 15\,655\,168, 3\,883\,902\,528, 1\,190\,923\,282\,176, \dots , \quad (4.6.10)$$

which are in agreement with the genus zero Gromov–Witten instanton numbers of  $\mathbb{P}^5[2, 4]$  calculated (again using mirror symmetry) in [109].

## Acknowledgments

I would like to thank Jim Halverson, Hans Jockers, Vijay Kumar, Josh Lapan, Ronen Plesser, and Mauricio Romo for collaboration on various of the results presented here. I particularly thank Nati Seiberg for sharing insights about his work, some of which is also presented here. I also thank Chris Beem, Francesco Benini, Eduardo Cattani, Cyril Closset, Jacques

Distler, Jaume Gomis, Rajesh Gopakumar, Antonella Grassi, Simeon Hellerman, Kentaro Hori, Shinobu Hosono, Nabil Iqbal, Zohar Komargodsky, Peter Koroteev, Sungjay Lee, Bruno Le Floch, Jan Manschot, Greg Moore, Joe Polchinski, Eric Sharpe, Samson Shatashvili, Yuji Tachikawa, Cumrun Vafa, and Edward Witten for useful discussions and correspondence. I would also like to thank the Institut Henri Poincaré for hospitality during the final stages of this project. This work was supported in part by National Science Foundation Grant PHY-1307513 (USA) and by the Centre National de la Recherche Scientifique (France).

## 4.7 Appendix. $\mathcal{N} = (2, 2)$ supersymmetry in two dimensions

We study two-dimensional theories with  $\mathcal{N} = (2, 2)$  supersymmetry. There are two basic types of supermultiplet, the notation for which is obtained by dimensional reduction from that of [110]. A *chiral supermultiplet* has components  $(\phi, \psi, F)$  while a *vector supermultiplet* has components  $(v, \sigma, \lambda, D)$ .

In Euclidean signature, we use a complex coordinate  $z$  on spacetime, and consider  $\sqrt{dz}$  and  $\sqrt{d\bar{z}}$  as bases for the two spinor bundles  $S_+$  and  $S_-$  of opposite chirality. In components, we can write

$$\psi = \psi_- \sqrt{dz} + \psi_+ \sqrt{d\bar{z}}. \quad (4.7.1)$$

In Minkowski signature, with time coordinate  $x^0$  and spatial coordinate  $x^1$ , the metric has components  $\eta_{00} = -1$ ,  $\eta_{11} = 1$ ,  $\eta_{01} = 0$ . The fermionic coordinates  $\theta^\pm$  and  $\bar{\theta}^\pm$  are complex, related by complex conjugation (i.e.,  $(\theta^\pm)^* = \bar{\theta}^\pm$ ). The  $\pm$  indices denote chirality. In particular,

$$\begin{bmatrix} \cosh \gamma & \sinh \gamma \\ \sinh \gamma & \cosh \gamma \end{bmatrix} \in SO(1, 1) \quad (4.7.2)$$

acts by  $e^{\pm\gamma/2}$  on  $\theta^\pm$  and also by  $e^{\pm\gamma/2}$  on  $\bar{\theta}^\pm$ .

A superfield is a function  $\Phi$  of these variables, and can be expanded into the thetas.  $\Phi$  is bosonic if  $[\theta^\alpha, \Phi] = 0$  and fermionic if  $\{\theta^\alpha, \Phi\} = 0$ .

We introduce the combinations  $x^\pm := x^0 \pm x^1$  and the corresponding differential operators

$$\partial_\pm = \frac{\partial}{\partial x^\pm} := \frac{1}{2} \left( \frac{\partial}{\partial x^0} \pm \frac{\partial}{\partial x^1} \right). \quad (4.7.3)$$

There are two natural sets of differential operators on superspace:

$$\mathcal{Q}^\pm = \frac{\partial}{\partial \theta^\pm} + i\bar{\theta}^\pm \partial_\pm \quad (4.7.4)$$

$$\bar{\mathcal{Q}}^\pm = -\frac{\partial}{\partial \bar{\theta}^\pm} - i\theta^\pm \partial_\pm \quad (4.7.5)$$

which satisfy  $\{\mathcal{Q}_\pm, \bar{\mathcal{Q}}_\pm\} = -2i\partial_\pm$ , and

$$D^\pm = \frac{\partial}{\partial\theta^\pm} - i\bar{\theta}^\pm\partial_\pm \quad (4.7.6)$$

$$\bar{D}^\pm = -\frac{\partial}{\partial\bar{\theta}^\pm} + i\theta^\pm\partial_\pm \quad (4.7.7)$$

which anti-commute with the first set, and satisfy  $\{D_\pm, \bar{D}_\pm\} = 2i\partial_\pm$ .

A *chiral superfield*  $\Phi$  satisfies  $\bar{D}_\pm\Phi = 0$ . Its component description is:

$$\Phi(x^\mu, \theta^\pm, \bar{\theta}^\pm) = \phi(y^\pm) + \theta^\alpha\psi_\alpha(y^\pm) + \theta^+\theta^-F(y^\pm) \quad (4.7.8)$$

where  $y^\pm = x^\pm - i\theta^\pm\bar{\theta}^\pm$  and  $F(y^\pm)$  is a non-propagating ‘‘auxiliary’’ field in the multiplet.. A *twisted chiral superfield*  $U$  satisfies  $\bar{D}_+U = D_-U = 0$ .

A vector multiplet is a real superfield  $V = V(x^\mu, \theta^\pm, \bar{\theta}^\pm)$  which under a gauge transformation  $\Phi \mapsto e^{iA}\Phi$  transforms as  $V \mapsto V + i(\bar{A} - A)$ , so that the Lagrangian

$$\int d^4\theta\bar{\Phi}e^V\Phi$$

is invariant under gauge transformations.

There is a gauge transformation putting the gauge field into *Wess-Zumino gauge*, where it takes the form

$$V = \theta^-\bar{\theta}^-(v_0 - v_1) + \theta^+\bar{\theta}^+(v_0 + v_1) - \theta^-\bar{\theta}^+\sigma - \theta^+\bar{\theta}^-\bar{\sigma} + i\theta^-\theta^+(\bar{\theta}^-\bar{\lambda}_- + \bar{\theta}^+\bar{\lambda}_+) \\ + i\bar{\theta}^+\bar{\theta}^-(\theta^-\lambda_- + \theta^+\lambda_+) + \theta^-\theta^+\bar{\theta}^+\bar{\theta}^-D \quad (4.7.9)$$

where  $\sigma$  is a complex scalar field,  $\lambda_\pm$  and  $\bar{\lambda}_\pm$  define a Dirac fermion, and  $D$  is an auxiliary real scalar field. The components  $v_\mu$  define the covariant derivatives  $D_\mu = \partial_\mu + iv_\mu$ .

The field strength of  $V$  is

$$\Sigma := \bar{D}_+D_-V \quad (4.7.10)$$

and it has a component expansion

$$\Sigma = \sigma(\tilde{y}) + i\theta^+\bar{\lambda}_+(\tilde{y}) - i\bar{\theta}^-\lambda_-(\tilde{y}) + \theta^+\bar{\theta}^-[D(\tilde{y}) - iv_{01}(\tilde{y})], \quad (4.7.11)$$

where  $\tilde{y}^\pm := x^\pm \mp i\theta^\pm\bar{\theta}^\pm$  and  $v_{01} = \partial_0v_1 - \partial_1v_0$  is the curvature of the connection.

## References

- [1] V. Pestun and M. Zabzine, eds., *Localization techniques in quantum field theory*, vol. xx. Journal of Physics A, 2016. 1608.02952. <https://arxiv.org/src/1608.02952/anc/LocQFT.pdf>, <http://pestun.ihes.fr/pages/LocalizationReview/LocQFT.pdf>.
- [2] B. R. Greene and M. R. Plesser, ‘‘Duality in Calabi–Yau Moduli Space,’’ *Nucl. Phys. B* **338** (1990) 15–37.

- [3] P. Candelas, M. Lynker, and R. Schimmrigk, “Calabi–Yau Manifolds in Weighted  $\mathbb{P}_4$ ,” *Nucl. Phys. B* **341** (1990) 383–402.
- [4] P. S. Aspinwall, C. A. Lütken, and G. G. Ross, “Construction and Couplings of Mirror Manifolds,” *Phys. Lett. B* **241** (1990) 373–380.
- [5] P. Candelas, X. C. de la Ossa, P. S. Green, and L. Parkes, “A Pair of Calabi–Yau Manifolds as an Exactly Soluble Superconformal Theory,” *Nucl. Phys. B* **359** (1991) 21–74.
- [6] M. Gromov, “Pseudo Holomorphic Curves in Symplectic Manifolds,” *Invent. Math.* **82** (1985) 307–347.
- [7] E. Witten, “Topological Sigma Models,” *Commun. Math. Phys.* **118** (1988) 411–449.
- [8] A. B. Givental, “Equivariant Gromov–Witten invariants,” *Internat. Math. Res. Notices* (1996) no. 13, 613–663, [arXiv:alg-geom/9603021](#).
- [9] B. H. Lian, K. Liu, and S.-T. Yau, “Mirror Principle. I,” *Asian J. Math.* **1** (1997) no. 4, 729–763, [arXiv:alg-geom/9712011](#).
- [10] Y. Cooper and A. Zinger, “Mirror Symmetry for Stable Quotients Invariants,” *Michigan Math. J.* **63** (2014) no. 3, 571–621, [arXiv:1201.6350](#) [[math.AG](#)].
- [11] H. Jockers, V. Kumar, J. M. Lapan, D. R. Morrison, and M. Romo, “Two-Sphere Partition Functions and Gromov–Witten Invariants,” *Commun. Math. Phys.* **325** (2014) 1139–1170, [arXiv:1208.6244](#) [[hep-th](#)].
- [12] V. Pestun, “Localization of Gauge Theory on a Four-Sphere and Supersymmetric Wilson Loops,” *Commun. Math. Phys.* **313** (2012) 71–129, [arXiv:0712.2824](#) [[hep-th](#)].
- [13] F. Benini and S. Cremonesi, “Partition Functions of  $\mathcal{N} = (2, 2)$  Gauge Theories on  $S^2$  and Vortices,” *Commun. Math. Phys.* **334** (2015) no. 3, 1483–1527, [arXiv:1206.2356](#) [[hep-th](#)].
- [14] N. Doroud, J. Gomis, B. Le Floch, and S. Lee, “Exact Results in D=2 Supersymmetric Gauge Theories,” *JHEP* **1305** (2013) 093, [arXiv:1206.2606](#) [[hep-th](#)].
- [15] J. Gomis and S. Lee, “Exact Kähler Potential from Gauge Theory and Mirror Symmetry,” *JHEP* **1304** (2013) 019, [arXiv:1210.6022](#) [[hep-th](#)].
- [16] E. Gerchkovitz, J. Gomis, and Z. Komargodski, “Sphere Partition Functions and the Zamolodchikov Metric,” *JHEP* **1411** (2014) 001, [arXiv:1405.7271](#) [[hep-th](#)].
- [17] J. Gomis, P.-S. Hsin, Z. Komargodski, A. Schwimmer, N. Seiberg, and S. Theisen, “Anomalies, Conformal Manifolds, and Spheres,” *JHEP* **1603** (2016) 022, [arXiv:1509.08511](#) [[hep-th](#)].
- [18] E. Witten, “Phases of  $N = 2$  Theories in Two Dimensions,” *Nucl. Phys. B* **403** (1993) 159–222, [arXiv:hep-th/9301042](#).
- [19] D. R. Morrison and M. R. Plesser, “Summing the Instantons: Quantum Cohomology and Mirror Symmetry in Toric Varieties,” *Nucl. Phys. B* **440** (1995) 279–354, [arXiv:hep-th/9412236](#).
- [20] D. R. Morrison and M. R. Plesser, “Towards Mirror Symmetry as Duality for Two-Dimensional Abelian Gauge Theories,” in *Trieste Conference on S-Duality and Mirror Symmetry*, vol. 46 of *Nucl. Phys. B Proc. Suppl.*, pp. 177–186. 1996. [arXiv:hep-th/9508107](#).
- [21] J. Halverson, V. Kumar, and D. R. Morrison, “New Methods for Characterizing Phases of 2D Supersymmetric Gauge Theories,” *JHEP* **1309** (2013) 143, [arXiv:1305.3278](#) [[hep-th](#)].
- [22] J. Halverson, H. Jockers, J. M. Lapan, and D. R. Morrison, “Perturbative Corrections to Kähler Moduli Spaces,” *Commun. Math. Phys.* **333** (2015) 1563–1584, [arXiv:1308.2157](#) [[hep-th](#)].
- [23] A. Zamolodchikov, “Irreversibility of the Flux of the Renormalization Group in a 2D Field Theory,” *JETP Lett.* **43** (1986) 730–732.

- [24] N. Seiberg, “Naturalness Versus Supersymmetric Nonrenormalization Theorems,” *Phys. Lett. B* **318** (1993) 469–475, [arXiv:hep-ph/9309335](#).
- [25] H. Osborn, “Weyl Consistency Conditions and a Local Renormalization Group Equation for General Renormalizable Field Theories,” *Nucl. Phys. B* **363** (1991) 486–526.
- [26] G. Festuccia and N. Seiberg, “Rigid Supersymmetric Theories in Curved Superspace,” *JHEP* **1106** (2011) 114, [arXiv:1105.0689 \[hep-th\]](#).
- [27] C. Closset and S. Cremonesi, “Comments on  $\mathcal{N} = (2, 2)$  Supersymmetry on Two-Manifolds,” *JHEP* **1407** (2014) 075, [arXiv:1404.2636 \[hep-th\]](#).
- [28] J. Bae, C. Imbimbo, S.-J. Rey, and D. Rosa, “New Supersymmetric Localizations from Topological Gravity,” *JHEP* **03** (2016) 169, [arXiv:1510.00006 \[hep-th\]](#).
- [29] P. S. Howe and G. Papadopoulos, “N=2, D = 2 Supergeometry,” *Class. Quant. Grav.* **4** (1987) 11–21.
- [30] A. Adams, H. Jockers, V. Kumar, and J. M. Lapan, “N=1 Sigma Models in  $AdS_4$ ,” *JHEP* **1112** (2011) 042, [arXiv:1104.3155 \[hep-th\]](#).
- [31] M. Bershadsky, C. Vafa, and V. Sadov, “D-Strings on D-Manifolds,” *Nucl. Phys. B* **463** (1996) 398–414, [hep-th/9510225](#).
- [32] S. Katz, D. R. Morrison, and M. R. Plesser, “Enhanced Gauge Symmetry in Type II String Theory,” *Nucl. Phys. B* **477** (1996) 105–140, [arXiv:hep-th/9601108](#).
- [33] M. T. Grisaru, A. E. M. van de Ven, and D. Zanon, “Two-Dimensional Supersymmetric Sigma-Models on Ricci-Flat Kähler Manifolds are Not Finite,” *Nucl. Phys. B* **277** (1986) no. 2, 388–408.
- [34] D. Nemeschansky and A. Sen, “Conformal Invariance of Supersymmetric  $\sigma$ -Models on Calabi-Yau Manifolds,” *Phys. Lett. B* **178** (1986) no. 4, 365–369.
- [35] P. Candelas, T. Hubsch, and R. Schimmrigk, “Relation Between the Weil-Petersson and Zamolodchikov Metrics,” *Nucl. Phys. B* **329** (1990) 583–590.
- [36] G. Tian, “Smoothness of the Universal Deformation Space of Compact Calabi–Yau Manifolds and its Peterson–Weil Metric,” in *Mathematical Aspects of String Theory*, S.-T. Yau, ed., pp. 629–646. World Scientific, Singapore, 1987.
- [37] A. N. Todorov, “The Weil-Petersson Geometry of the Moduli Space of  $SU(n \geq 3)$  (Calabi–Yau) Manifolds, I,” *Commun. Math. Phys.* **126** (1989) 325–246.
- [38] M. T. Grisaru, W. Siegel, and M. Rocek, “Improved Methods for Supergraphs,” *Nucl. Phys. B* **159** (1979) 429–250.
- [39] D. R. Morrison, “Compactifications of Moduli Spaces Inspired by Mirror Symmetry,” in *Journées de Géométrie Algébrique d’Orsay (Juillet 1992)*, vol. 218 of *Astérisque*, pp. 243–271. Société Mathématique de France, 1993. [arXiv:alg-geom/9304007](#).
- [40] K. Hori, “Duality In Two-Dimensional (2,2) Supersymmetric Non-Abelian Gauge Theories,” *JHEP* **10** (2013) 121, [arXiv:1104.2853 \[hep-th\]](#).
- [41] K. Hori and J. Knapp, “Linear Sigma Models With Strongly Coupled Phases – One Parameter Models,” *JHEP* **11** (2013) 070, [arXiv:1308.6265 \[hep-th\]](#).
- [42] J. Knapp, M. Romo, and E. Scheidegger, “Hemisphere Partition Function and Analytic Continuation to the Conifold Point,” [arXiv:1602.01382 \[hep-th\]](#).
- [43] P. S. Aspinwall, B. R. Greene, and D. R. Morrison, “The Monomial-Divisor Mirror Map,” *Internat. Math. Res. Notices* (1993) 319–337, [arXiv:alg-geom/9309007](#).

- [44] P. S. Aspinwall and M. R. Plesser, “General Mirror Pairs for Gauged Linear Sigma Models,” *JHEP* **11** (2015) 029, [arXiv:1507.00301 \[hep-th\]](#).
- [45] E. Silverstein and E. Witten, “Global  $U(1)$  R Symmetry and Conformal Invariance of (0,2) Models,” *Phys. Lett. B* **328** (1994) 307–311, [arXiv:hep-th/9403054](#).
- [46] I. M. Gel’fand, A. V. Zelevinskiĭ, and M. M. Kapranov, “Newton Polyhedra of Principal  $A$ -Determinants,” *Soviet Math. Dokl.* **40** (1990) 278–281.
- [47] I. M. Gel’fand, A. V. Zelevinskiĭ, and M. M. Kapranov, “Discriminants of Polynomials in Several Variables and Triangulations of Newton Polyhedra,” *Leningrad Math. J.* **2** (1991) 449–505.
- [48] L. J. Billera, P. Filliman, and B. Sturmfels, “Constructions and Complexity of Secondary Polytopes,” *Adv. Math.* **83** (1990) no. 2, 155–179.
- [49] P. S. Aspinwall, B. R. Greene, and D. R. Morrison, “Calabi–Yau Moduli Space, Mirror Manifolds and Spacetime Topology Change in String Theory,” *Nucl. Phys. B* **416** (1994) 414–480, [arXiv:hep-th/9309097](#).
- [50] P. Candelas, X. de la Ossa, A. Font, S. Katz, and D. R. Morrison, “Mirror Symmetry for Two Parameter Models – I,” *Nucl. Phys. B* **416** (1994) 481–562, [arXiv:hep-th/9308083](#).
- [51] S. Hosono, A. Klemm, S. Theisen, and S.-T. Yau, “Mirror Symmetry, Mirror Map and Applications to Calabi–Yau Hypersurfaces,” *Commun. Math. Phys.* **167** (1995) 301–350, [arXiv:hep-th/9308122](#).
- [52] P. S. Aspinwall, B. R. Greene, and D. R. Morrison, “Measuring Small Distances In  $N=2$  Sigma Models,” *Nucl. Phys. B* **420** (1994) 184–242, [arXiv:hep-th/9311042](#).
- [53] D. R. Morrison, “Through the Looking Glass,” in *Mirror Symmetry III*, D. H. Phong, L. Vinet, and S.-T. Yau, eds., vol. 10 of *AMS/IP Stud. Adv. Math.*, pp. 263–277. International Press, Cambridge, 1999. [arXiv:alg-geom/9705028](#).
- [54] M. Herbst, K. Hori, and D. Page, “Phases Of  $N = 2$  Theories In 1+1 Dimensions With Boundary,” [arXiv:0803.2045 \[hep-th\]](#).
- [55] K. Hori and M. Romo, “Exact Results In Two-Dimensional (2,2) Supersymmetric Gauge Theories With Boundary,” [arXiv:1308.2438 \[hep-th\]](#).
- [56] V. V. Batyrev, “Dual Polyhedra and Mirror Symmetry for Calabi–Yau Hypersurfaces in Toric Varieties,” *J. Algebraic Geom.* **3** (1994) no. 3, 493–535, [arXiv:alg-geom/9310003](#).
- [57] P. S. Howe, G. Papadopoulos, and K. Stelle, “Quantizing the  $N=2$  Super Sigma Model in Two-Dimensions,” *Phys. Lett. B* **174** (1986) 405–410.
- [58] D. J. Gross and E. Witten, “Superstring Modifications of Einstein’s Equations,” *Nucl. Phys. B* **277** (1986) no. 1, 1–10.
- [59] M. T. Grisaru, A. E. M. van de Ven, and D. Zanon, “Four-Loop  $\beta$ -Function for the  $N = 1$  and  $N = 2$  Supersymmetric Nonlinear Sigma Model in Two Dimensions,” *Phys. Lett. B* **173** (1986) no. 4, 423–428.
- [60] M. T. Grisaru, D. I. Kazakov, and D. Zanon, “Five-Loop Divergences for the  $N = 2$  Supersymmetric Nonlinear Sigma-Model,” *Nucl. Phys. B* **287** (1987) no. 1, 189–204.
- [61] D. Zanon, “Four-Loop  $\sigma$ -Model Beta-Functions Versus  $\alpha'^3$  Corrections to Superstring Effective Actions,” in *Super Field Theories (NATO ASI Series)*, H. C. Lee, V. Elias, G. Kunstatter, R. B. Mann, and K. S. Viswanathan, eds., vol. 160 of *Series B: Physics*, pp. 275–282. Plenum Press, 1986.
- [62] M. D. Freeman, C. N. Pope, M. F. Sohnius, and K. S. Stelle, “Higher-Order  $\sigma$ -Model Counterterms and the Effective Action for Superstrings,” *Phys. Lett. B* **178** (1986) no. 2-3, 199–204.

- [63] D. J. Broadhurst, J. Gracey, and D. Kreimer, “Beyond the Triangle and Uniqueness Relations: Nonzeta Counterterms at Large  $N$  from Positive Knots,” *Z. Phys. C* **75** (1997) 559–574, [arXiv:hep-th/9607174 \[hep-th\]](#).
- [64] D. Zagier, “Values of Zeta Functions and Their Applications,” in *First European Congress of Mathematics, Vol. II (Paris, 1992)*, vol. 120 of *Progr. Math.*, pp. 497–512. Birkhäuser, Basel, 1994.
- [65] J. Blümlein, D. J. Broadhurst, and J. A. M. Vermaseren, “The Multiple Zeta Value Data Mine,” *Comput. Phys. Comm.* **181** (2010) no. 3, 582–625, [arXiv:0907.2557 \[math-ph\]](#).
- [66] A. Libgober, “Chern Classes and the Periods of Mirrors,” *Math. Res. Lett.* **6** (1999) no. 2, 141–149, [arXiv:math.AG/9803119](#).
- [67] H. Iritani, “Real and Integral Structures in Quantum Cohomology I: Toric Orbifolds,” [arXiv:0712.2204 \[math.AG\]](#).
- [68] H. Iritani, “An Integral Structure in Quantum Cohomology and Mirror Symmetry for Toric Orbifolds,” *Adv. Math.* **222** (2009) no. 3, 1016–1079, [arXiv:0903.1463 \[math.AG\]](#).
- [69] H. Iritani, “Quantum Cohomology and Periods,” *Ann. Inst. Fourier (Grenoble)* **61** (2011) no. 7, 2909–2958, [arXiv:1101.4512 \[math.AG\]](#).
- [70] L. Katzarkov, M. Kontsevich, and T. Pantev, “Hodge Theoretic Aspects of Mirror Symmetry,” in *From Hodge Theory to Integrability and TQFT  $tt^*$ -Geometry*, vol. 78 of *Proc. Sympos. Pure Math.*, pp. 87–174. Amer. Math. Soc., Providence, RI, 2008. [arXiv:0806.0107 \[math.AG\]](#).
- [71] Y. Honma and M. Manabe, “Exact Kähler Potential for Calabi–Yau Fourfolds,” *JHEP* **1305** (2013) 102, [arXiv:1302.3760 \[hep-th\]](#).
- [72] B. Dubrovin, “Geometry of 2D Topological Field Theories,” in *Integrable Systems and Quantum Groups (Montecatini Terme, 1993)*, vol. 1620 of *Lecture Notes in Math.*, pp. 120–348. Springer, Berlin, 1996. [arXiv:hep-th/9407018](#).
- [73] E. Witten, “Mirror Manifolds and Topological Field Theory,” in *Essays on Mirror Manifolds*, pp. 120–158. Int. Press, Hong Kong, 1992. [arXiv:hep-th/9112056](#).
- [74] E. Witten, “On the Structure of the Topological Phase of Two-Dimensional Gravity,” *Nucl. Phys. B* **340** (1990) 281–332.
- [75] C. Vafa, “Topological Mirrors and Quantum Rings,” in *Essays on Mirror Manifolds*, pp. 96–119. Int. Press, Hong Kong, 1992. [arXiv:hep-th/9111017](#).
- [76] E. Witten, “Two-Dimensional Gravity and Intersection Theory on Moduli Space,” in *Surveys in Differential Geometry (Cambridge, MA, 1990)*, pp. 243–310. Lehigh Univ., Bethlehem, PA, 1991.
- [77] R. Dijkgraaf, H. L. Verlinde, and E. P. Verlinde, “Topological Strings in  $d < 1$ ,” *Nucl. Phys. B* **352** (1991) 59–86.
- [78] B. Dubrovin, “Integrable Systems in Topological Field Theory,” *Nucl. Phys. B* **379** (1992) 627–689.
- [79] M. Kontsevich and Y. Manin, “Gromov-Witten classes, Quantum Cohomology, and Enumerative Geometry,” *Commun. Math. Phys.* **164** (1994) 525–562, [arXiv:hep-th/9402147](#).
- [80] Y. Ruan and G. Tian, “A Mathematical Theory of Quantum Cohomology,” *J. Differential Geom.* **42** (1995) no. 2, 259–367.
- [81] J. Li and G. Tian, “Virtual Moduli Cycles and Gromov-Witten Invariants of Algebraic Varieties,” *J. Amer. Math. Soc.* **11** (1998) no. 1, 119–174, [arXiv:alg-geom/9602007](#).
- [82] P. S. Aspinwall and D. R. Morrison, “Topological Field Theory and Rational Curves,” *Commun. Math. Phys.* **151** (1993) 245–262, [arXiv:hep-th/9110048](#).

- [83] B. R. Greene, D. R. Morrison, and M. R. Plesser, “Mirror Manifolds in Higher Dimension,” *Commun. Math. Phys.* **173** (1995) 559–598, [arXiv:hep-th/9402119](#).
- [84] A. Klemm and R. Pandharipande, “Enumerative Geometry of Calabi-Yau 4-Folds,” *Commun. Math. Phys.* **281** (2008) 621–653, [arXiv:math.AG/0702189](#).
- [85] P. Goddard, J. Nuyts, and D. I. Olive, “Gauge Theories and Magnetic Charge,” *Nucl. Phys. B* **125** (1977) 1–28.
- [86] D. Honda and T. Okuda, “Exact Results for Boundaries and Domain Walls in 2d Supersymmetric Theories,” *JHEP* **09** (2015) 140, [arXiv:1308.2217 \[hep-th\]](#).
- [87] S. Sugishita and S. Terashima, “Exact Results in Supersymmetric Field Theories on Manifolds with Boundaries,” *JHEP* **11** (2013) 021, [arXiv:1308.1973 \[hep-th\]](#).
- [88] H. Kim, S. Lee, and P. Yi, “Exact Partition Functions on  $\mathbb{RP}^2$  and Orientifolds,” *JHEP* **02** (2014) 103, [arXiv:1310.4505 \[hep-th\]](#).
- [89] K. Becker, M. Becker, and A. Strominger, “Fivebranes, Membranes and Nonperturbative String Theory,” *Nucl. Phys. B* **456** (1995) 130–152, [arXiv:hep-th/9507158](#).
- [90] H. Ooguri, Y. Oz, and Z. Yin, “D-Branes on Calabi-Yau Spaces and their Mirrors,” *Nucl. Phys. B* **477** (1996) 407–430, [arXiv:hep-th/9606112](#).
- [91] A. Kapustin, B. Willett, and I. Yaakov, “Exact Results for Wilson Loops in Superconformal Chern-Simons Theories with Matter,” *JHEP* **1003** (2010) 089, [arXiv:0909.4559 \[hep-th\]](#).
- [92] N. Hama, K. Hosomichi, and S. Lee, “SUSY Gauge Theories on Squashed Three-Spheres,” *JHEP* **1105** (2011) 014, [arXiv:1102.4716 \[hep-th\]](#).
- [93] S. Pasquetti, “Factorisation of  $N = 2$  Theories on the Squashed 3-Sphere,” *JHEP* **1204** (2012) 120, [arXiv:1111.6905 \[hep-th\]](#).
- [94] C. Beem, T. Dimofte, and S. Pasquetti, “Holomorphic Blocks in Three Dimensions,” *JHEP* **1412** (2014) 177, [arXiv:1211.1986 \[hep-th\]](#).
- [95] S. Cecotti and C. Vafa, “Topological Antitopological Fusion,” *Nucl. Phys. B* **367** (1991) 359–461.
- [96] F. Benini and B. Le Floch, “Supersymmetric localization in two dimensions,” *Journal of Physics A* **xx** (2016) 000, [1608.02955](#).
- [97] P. Griffiths and J. Harris, *Principles of Algebraic Geometry*. John Wiley & Sons, New York, 1978.
- [98] A. K. Tsikh, *Multidimensional Residues and their Applications*, vol. 103 of *Translations of Mathematical Monographs*. Amer. Math. Soc., Providence, R. I., 1992.
- [99] M. Passare, A. K. Tsikh, and A. A. Cheshel, “Multiple Mellin-Barnes Integrals as Periods of Calabi-Yau Manifolds with Several Moduli,” *Theor. Math. Phys.* **109** (1997) 1544–1555, [arXiv:hep-th/9609215](#).
- [100] R. P. Horja, *Hypergeometric Functions and Mirror Symmetry in Toric Varieties*. PhD thesis, Duke University, 1999. [arXiv:math.AG/9912109](#).
- [101] L. A. Borisov and R. P. Horja, “Mellin-Barnes Integrals as Fourier-Mukai Transforms,” *Adv. Math.* **207** (2006) no. 2, 876–927, [arXiv:math.AG/0510486](#).
- [102] V. V. Batyrev and L. A. Borisov, “On Calabi-Yau Complete Intersections in Toric Varieties,” in *Higher-Dimensional Complex Varieties (Trento, 1994)*, pp. 39–65. de Gruyter, Berlin, 1996. [arXiv:alg-geom/9412017](#).
- [103] C. H. Clemens, “Double Solids,” *Adv. in Math.* **47** (1983) no. 2, 107–230.

- [104] R. Friedman, “Simultaneous Resolution of Threefold Double Points,” *Math. Ann.* **274** (1986) no. 4, 671–689.
- [105] M. Reid, “The Moduli Space of 3-Folds with  $K = 0$  May Nevertheless Be Irreducible,” *Math. Ann.* **278** (1987) no. 1-4, 329–334.
- [106] P. Candelas, P. S. Green, and T. Hubsch, “Rolling Among Calabi–Yau Vacua,” *Nucl. Phys. B* **330** (1990) 49–102.
- [107] B. R. Greene, D. R. Morrison, and A. Strominger, “Black Hole Condensation and the Unification of String Vacua,” *Nucl. Phys. B* **451** (1995) 109–120, [arXiv:hep-th/9504145](#).
- [108] A.-M. Li and Y. Ruan, “Symplectic Surgery and Gromov-Witten Invariants of Calabi-Yau 3-Folds,” *Invent. Math.* **145** (2001) no. 1, 151–218, [arXiv:math.AG/9803036](#).
- [109] A. Libgober and J. Teitelbaum, “Lines on Calabi–Yau Complete Intersections, Mirror Symmetry, and Picard–Fuchs Equations,” *Internat. Math. Res. Notices* (1993) no. 1, 29–39, [arXiv:alg-geom/9301001](#).
- [110] J. Wess and J. Bagger, *Supersymmetry and Supergravity*. Princeton University Press, Princeton, N.J., 1983.

[7]

# Chapter 5

## An introduction to supersymmetric field theories in curved space

Thomas T. Dumitrescu

*Department of Physics, Harvard University, Cambridge, MA 02138, USA*

`tdumitre@physics.harvard.edu`

### Abstract

In this review, we give a pedagogical introduction to a systematic framework for constructing and analyzing supersymmetric field theories on curved spacetime manifolds. The framework is based on the use of off-shell supergravity background fields. We present the general principles, which broadly apply to theories with different amounts of supersymmetry in diverse dimensions, as well as specific applications to  $\mathcal{N} = 1$  theories in four dimensions and their three-dimensional cousins with  $\mathcal{N} = 2$  supersymmetry.

### Contents

|            |                                                               |            |
|------------|---------------------------------------------------------------|------------|
| <b>5.1</b> | <b>Introduction</b>                                           | <b>175</b> |
| 5.1.1      | Background fields and partition functions                     | 176        |
| 5.1.2      | Supersymmetric theories                                       | 178        |
| 5.1.3      | Overview of the formalism                                     | 180        |
| 5.1.4      | Outline                                                       | 183        |
| <b>5.2</b> | <b>Four-dimensional <math>\mathcal{N} = 1</math> theories</b> | <b>183</b> |
| 5.2.1      | Stress-tensor multiplets and off-shell supergravities         | 183        |
| 5.2.2      | Theories with an $R$ -symmetry                                | 186        |
| 5.2.3      | Lagrangians                                                   | 189        |
| 5.2.4      | Constraining the partition function                           | 190        |
| 5.2.5      | Example: $S^3 \times S^1$                                     | 193        |
| 5.2.6      | Theories without an $R$ -symmetry                             | 194        |

|                   |                                                                |            |
|-------------------|----------------------------------------------------------------|------------|
| <b>5.3</b>        | <b>Three-dimensional <math>\mathcal{N} = 2</math> theories</b> | <b>195</b> |
| 5.3.1             | Theories with an $R$ -symmetry on curved manifolds             | 195        |
| 5.3.2             | Constraining the partition function                            | 196        |
| 5.3.3             | Example: round and squashed $S^3$                              | 196        |
| 5.3.4             | $F$ -maximization and correlation functions                    | 197        |
| <b>References</b> |                                                                | <b>198</b> |

## 5.1 Introduction

A standard tool in quantum field theory (QFT) is to probe the theory with non-dynamical sources, or background fields. The consequences of symmetries can then be systematically analyzed by assigning spurious transformation rules to the background fields. In supersymmetric theories, all sources must therefore reside in multiplets of supersymmetry, or superfields. This constrains the extent to which they can affect protected supersymmetric, or BPS, quantities. A typical example is the effective superpotential in four-dimensional theories with  $\mathcal{N} = 1$  supersymmetry, which must be a locally holomorphic function of coupling constants that reside in background chiral superfields [2]. This constraint makes it possible to determine the effective superpotential exactly in a large class of theories; see [3] for a classic exposition of this powerful approach to analyzing the dynamics of supersymmetric field theories.

Much recent work has involved placing supersymmetric field theories on a manifold  $\mathcal{M}$  with a non-trivial metric or topology, while preserving some (though generally not all) supercharges.<sup>1</sup> The partition function  $Z_{\mathcal{M}}$  on  $\mathcal{M}$  (which may be decorated with suitable background fields or operator insertions) is BPS and can sometimes be computed exactly, e.g. using supersymmetric localization techniques.<sup>2</sup> A systematic approach to constructing and analyzing supersymmetric field theories on curved manifolds  $\mathcal{M}$  was presented in [7]. It extends the principle that all background fields should reside in superfields to the metric  $g_{\mu\nu}$  on  $\mathcal{M}$  by embedding it in an off-shell supergravity multiplet.

The purpose of this review is twofold: first, to outline in broad strokes the supergravity-based approach of [7], which is very general and applies to all supersymmetric field theories. Second, to present some applications to four-dimensional  $\mathcal{N} = 1$  theories (section 5.2) and their three-dimensional cousins with  $\mathcal{N} = 2$  supersymmetry (section 5.3). These examples illustrate the general framework and showcase its utility for deriving exact results, often without recourse to explicit localization computations, or even a Lagrangian.

---

<sup>1</sup> The study of supersymmetric field theories on non-trivial manifolds was pioneered by Witten, see for instance [4, 5].

<sup>2</sup> The basic idea behind supersymmetric localization is reviewed below; see Chapter 1 for a broader and more detailed exposition.

### 5.1.1 Background fields and partition functions

Throughout, background gauge fields coupling to conserved currents will play a crucial role. As an example, consider a theory with a  $U(1)$  flavor symmetry. The corresponding conserved current  $j_\mu$  can be coupled to a background gauge field  $a_\mu$ ,

$$\Delta\mathcal{L} = a^\mu j_\mu + \mathcal{O}(a^2) . \quad (5.1.1)$$

The  $\mathcal{O}(a^2)$  seagull terms are tuned to ensure invariance of the Lagrangian under gauge transformations of  $a_\mu$ , which enforces current conservation,  $\partial^\mu j_\mu = 0$ . Small field variations around  $a_\mu = 0$  are captured by correlation functions of  $j_\mu$  in the undeformed theory.

Every relativistic QFT possesses a conserved, symmetric stress tensor  $T_{\mu\nu}$ . (If the theory is also conformally invariant, then  $T_{\mu\nu}$  can be chosen such that  $T_\mu^\mu = 0$ .) The appropriate source is a background spacetime metric  $g_{\mu\nu}$ . Depending on the signature of spacetime, it may be a Lorentzian or a Riemannian metric. Below, we will mostly discuss field theories on compact, Euclidean spacetime manifolds, which require a Riemannian  $g_{\mu\nu}$ . Around flat space,  $g_{\mu\nu} = \delta_{\mu\nu}$ , the theory couples to a metric deformation  $\Delta g_{\mu\nu}$  via the stress tensor,<sup>3</sup>

$$g_{\mu\nu} = \delta_{\mu\nu} + \Delta g_{\mu\nu} , \quad \Delta\mathcal{L} = -\frac{1}{2} \Delta g^{\mu\nu} T_{\mu\nu} + \mathcal{O}(\Delta g^2) . \quad (5.1.2)$$

Here the indices are raised and lowered using the flat metric  $\delta_{\mu\nu}$ . When the perturbation  $\Delta g_{\mu\nu}$  is small, its effect is captured by correlation functions of  $T_{\mu\nu}$  in flat space. The conservation equation  $\partial^\mu T_{\mu\nu} = 0$  is enforced by choosing the  $\mathcal{O}(\Delta g^2)$  gravitational seagull terms so that the Lagrangian is invariant under diffeomorphisms that also act on the background metric  $g_{\mu\nu}$ . Such a diffeomorphism-invariant Lagrangian can then be studied on an arbitrary Riemannian manifold  $\mathcal{M}$ , which may be curved or possess non-trivial topology.<sup>4</sup>

The stress tensor is not unique: it can be redefined by improvement terms, such as

$$T'_{\mu\nu} = T_{\mu\nu} + \left( \partial_\mu \partial_\nu - \delta_{\mu\nu} \partial^2 \right) \mathcal{O} , \quad (5.1.3)$$

where  $\mathcal{O}$  is a well-defined scalar operator. Both  $T_{\mu\nu}$  and  $T'_{\mu\nu}$  are acceptable stress tensors: they are symmetric, conserved, and integrate to the momentum operators  $P_\mu$ . Consequently, we can use either one to place the theory in curved space. The improvement terms in (5.1.3) then give rise to curvature couplings,

$$\mathcal{L}' = \mathcal{L} - \frac{1}{2} R[g] \mathcal{O} , \quad (5.1.4)$$

where  $R[g]$  is the Ricci scalar of the metric  $g_{\mu\nu}$ .<sup>5</sup> More general improvements can involve a four-index tensor  $\mathcal{O}_{\mu\nu\rho\lambda}$  that couples to the full Riemann tensor  $R_{\mu\nu\rho\lambda}$ . We can also modify the Lagrangian by adding local, diffeomorphism-invariant terms that only involve the background

<sup>3</sup> Unless stated otherwise, we follow the conventions of [8]. Whenever possible, they coincide with those of [9].

<sup>4</sup> Additional care is required if the field theory has gravitational anomalies (see for instance [10]).

<sup>5</sup> In the conventions of [9], a round  $S^d$  of radius  $r$  has constant negative scalar curvature  $R = -\frac{d(d-1)}{r^2}$ .

metric. These do not change the correlation functions of  $T_{\mu\nu}$  at separated points, but they can give rise to contact terms at coincident points.

Given a QFT on a manifold  $\mathcal{M}$ , it is interesting to study its partition function,

$$Z_{\mathcal{M}}[g_{\mu\nu}, a_{\mu}, \dots] = \int \mathcal{D}\Psi e^{-\int \mathcal{L}_{\mathcal{M}}[\Psi; g_{\mu\nu}, a_{\mu}, \dots]} . \quad (5.1.5)$$

In addition to the metric  $g_{\mu\nu}$  on  $\mathcal{M}$ , we can also couple a background gauge field  $a_{\mu}$  to every flavor current of the theory, as in (5.1.1). The ellipses in (5.1.5) denote other background fields. Below, we will see that supersymmetric theories are naturally equipped with a variety of other background fields that must be considered in conjunction with  $g_{\mu\nu}$  and  $a_{\mu}$ . In general,  $Z_{\mathcal{M}}$  suffers from IR and UV divergences. The IR divergences can often be cured by taking  $\mathcal{M}$  to be a compact manifold.<sup>6</sup> As in flat space, the UV divergences are regulated by introducing a short-distance cutoff. The resulting dependence of  $Z_{\mathcal{M}}$  on the regularization scheme is captured by local counterterms in the background fields. In UV-complete quantum field theories, only finitely many such counterterms are needed. Given a set of background fields, the possible counterterms can be enumerated once and for all. If the regulator preserves certain symmetries, e.g. diffeomorphisms, the counterterms must also respect these symmetries.

The scheme-independent part of the partition function  $Z_{\mathcal{M}}$  captures the universal long-distance physics of the QFT. For instance, the functional dependence of  $Z_{\mathcal{M}}$  on the sources  $g_{\mu\nu}, a_{\mu}$ , etc. encodes correlation functions of the corresponding local operators  $T_{\mu\nu}, j_{\mu}$  etc. on  $\mathcal{M}$ . Partition functions can also detect non-local degrees of freedom, which are activated by the topology of  $\mathcal{M}$ . A typical example is Chern-Simons theory on a three-manifold, which possesses no local operators but leads to non-trivial partition functions [11].

In conformal field theories (CFTs), the conformal symmetry can be used to relate properties of the theory on different manifolds. A typical example is the operator-state correspondence, which identifies states on  $S^{d-1} \times \mathbb{R}$  in Hamiltonian (i.e. radial) quantization with local operators. Similarly, correlation functions of local operators on  $\mathbb{R}^d$  are conformally related to correlation functions on  $S^d$ , where the IR fluctuations of the CFT are naturally regulated by the finite spacetime volume. Note that conformal symmetry fixes the improvement terms (5.1.3), and hence the curvature couplings (5.1.4), by singling out a preferred, traceless stress tensor.

A quantity that has received much recent attention is the entanglement entropy. For the special case of vacuum entanglement across a spherical entangling surface in a CFT, the entanglement entropy can be obtained from the partition function  $Z_{S^d}$  on a round sphere [12]. More precisely, the statement applies to the universal, scheme-independent parts of both quantities. These can in turn be used to define a quantity that is known (in  $1 \leq d \leq 4$  dimensions) or believed to decrease monotonically under renormalization-group (RG) flow (see for instance Chapter 8 and references therein).

---

<sup>6</sup> This is not sufficient to ensure that  $Z_{\mathcal{M}}$  is IR finite, since the integral in (5.1.5) may have bosonic zero modes even if  $\mathcal{M}$  is compact.

## 5.1.2 Supersymmetric theories

As is the case for most observables in interacting QFTs, the partition functions discussed in section 5.1.1 are generally not (exactly) computable. The situation is better in supersymmetric theories: BPS observables, which are annihilated by some of the supercharges, are often tightly constrained; in favorable situations, they can even be determined exactly.

Placing supersymmetric field theories on a non-trivial manifold  $\mathcal{M}$  with a curved metric  $g_{\mu\nu}$  generally breaks all flat-space supercharges. Intuitively, this can be understood from the linearized coupling (5.1.2) of the stress tensor to the background metric  $g_{\mu\nu}$ , since  $T_{\mu\nu}$  is not a BPS operator, i.e.  $[Q, T_{\mu\nu}] \neq 0$  for every flat-space supercharge  $Q$ . More precisely, placing a flat-space theory on  $\mathcal{M}$  by minimally coupling it to the metric  $g_{\mu\nu}$  leads to a curved-space supercharge for each covariantly constant spinor  $\zeta$  on  $\mathcal{M}$ ,

$$\nabla_\mu \zeta = 0 . \tag{5.1.6}$$

This equation is very restrictive. For instance, the only compact four-manifolds that admit covariantly constant spinors are flat tori  $T^4$  and K3 surfaces with Ricci-flat Kähler metrics. Similar statements apply to background flavor gauge fields  $a_\mu$ , which typically break supersymmetry because the associated flavor current  $j_\mu$  is not a BPS operator. A notable exception occurs for flat connections, which can always be turned on without breaking supersymmetry.<sup>7</sup>

In this review we will follow [7] and explain how the condition (5.1.6) can be relaxed in a systematic way. Consequently, some supersymmetry can be preserved for a much larger class of manifolds  $\mathcal{M}$  and background fields  $g_{\mu\nu}, a_\mu$ . If  $\mathcal{M}$  does not admit covariantly constant spinors, this is achieved by coupling the flat-space field theory to background fields in a special, non-minimal way. As we will see, a crucial role is played by additional background fields that are necessarily present in supersymmetric theories. The resulting curved-space Lagrangian  $\mathcal{L}_\mathcal{M}$  is invariant under the action of one or several supercharges, whose algebra may be deformed. The corresponding spinor parameters satisfy equations that generalize (5.1.6).

Under favorable conditions, the partition function  $Z_\mathcal{M}$  of a supersymmetric field theory on a curved manifold  $\mathcal{M}$  can be computed exactly using supersymmetric localization. (See Chapter 1 for an overview with references.) The theory is frequently assumed to have a presentation in terms of fields and a Lagrangian. In the simplest case, the curved-space Lagrangian  $\mathcal{L}_\mathcal{M}$  is invariant under a nilpotent supercharge  $Q$ , i.e.  $Q^2 = 0$ , which can be used to deform the path integral expression (5.1.5) for the partition function while preserving  $Q$ ,

$$Z_\mathcal{M}(t) = \int \mathcal{D}\Psi e^{-\int \mathcal{L}_\mathcal{M} + t\{Q, \mathcal{O}\}} , \tag{5.1.7}$$

for some fermionic operator  $\mathcal{O}$ . In order to ensure that the deformed action in the exponent of (5.1.7) is  $Q$ -invariant for every value of  $t$ , it is convenient (but not necessary) to realize the supercharge  $Q$  off shell. The variation of  $Z_\mathcal{M}(t)$  with respect to the parameter  $t$  vanishes,

---

<sup>7</sup> This is not true for flat  $R$ -symmetry background gauge fields, which can break supersymmetry.

because the change in the integrand is  $Q$ -exact,<sup>8</sup>

$$\frac{d}{dt}Z_{\mathcal{M}}(t) = \langle \{Q, \mathcal{O}\} \rangle = 0 . \quad (5.1.8)$$

This shows that  $Z_{\mathcal{M}} = Z_{\mathcal{M}}(0)$  can be computed by evaluating (5.1.7) for any choice of  $t$ , including  $t \rightarrow \infty$ . For suitable choices of the operator  $\mathcal{O}$ , this limit localizes the path integral to semiclassical field configurations, with  $t^{-1} \rightarrow 0$  playing the role of Planck's constant. The semiclassical saddle points depend on the choice of  $Q$  and  $\mathcal{O}$ , i.e. they are typically not saddle points of the undeformed theory with Lagrangian  $\mathcal{L}_{\mathcal{M}}$ .

The bulk of this review volume is dedicated to explicit localization computations of supersymmetric partition functions  $Z_{\mathcal{M}}$ , perhaps in the presence of additional insertions (see Chapter 1 and references therein). The techniques and results reviewed below serve as a basis for such calculations. In particular, we will address the following questions:

- 1.) When and how can a supersymmetric field theory be placed on a curved manifold  $\mathcal{M}$  while preserving some supersymmetry?
- 2.) What additional data does the resulting supersymmetric Lagrangian  $\mathcal{L}_{\mathcal{M}}$  on  $\mathcal{M}$  depend on, beyond the data that was already present in flat space?
- 3.) How does supersymmetry constrain the dependence of the partition function  $Z_{\mathcal{M}}$  on this data?

As we will see, these questions can be answered within a uniform, largely model-independent framework, which crucially relies on supersymmetry, but not explicit localization computations. In fact, most of the results reviewed below do not require a Lagrangian description of the field theory.<sup>9</sup> Before outlining the general framework in section 5.1.3, we will examine a few representative examples of supersymmetric field theories in non-trivial backgrounds.

The only way to preserve all flat-space supercharges on a compact manifold  $\mathcal{M}$  without turning on any background fields other than the metric is to take  $\mathcal{M}$  to be a flat torus  $T^d$ , with periodic boundary conditions for fermions. The corresponding partition function  $Z_{T^d}$  is the Witten index [4], which counts the supersymmetric vacua of the theory on  $T^{d-1} \times \mathbb{R}$ , weighted by their fermion number.<sup>10</sup>

As was already discussed around (5.1.6) above, a covariantly constant spinor leads to a supercharge on  $\mathcal{M}$ , but such spinors only exist for very special choices of  $\mathcal{M}$ , such as Calabi-Yau manifolds. A more general prescription for preserving supersymmetry, which applies to a larger class of manifolds, is known as twisting [5]: assume that the supersymmetric theory has a continuous  $R$ -symmetry  $G_R$ , and that the Riemannian holonomy group of

---

<sup>8</sup> This argument requires the path integral to converge sufficiently rapidly so that it is legitimate to integrate by parts in field space. See [14] for a detailed discussion of some examples where this assumption breaks down.

<sup>9</sup> See Chapter 12 for some examples of localization calculations in non-Lagrangian theories.

<sup>10</sup> The Witten index may be ill defined if there are bosonic zero modes that are not lifted when the flat-space theory is compactified on a torus.

the metric  $g_{\mu\nu}$  on  $\mathcal{M}$  is  $G_{\text{hol}}$ . If a given flat-space supercharge  $Q$  is a singlet under the diagonal subgroup  $(G_R \times G_{\text{hol}})|_{\text{diag}}$ , then  $Q$  can be preserved on  $\mathcal{M}$ . (In flat space, the holonomy group  $G_{\text{hol}}$  acts via Euclidean rotations.) A prototypical example is topologically twisted  $\mathcal{N} = 2$  Yang-Mills theory on an oriented Riemannian four-manifold [5]. Here  $G_R = SU(2)_R$  and  $G_{\text{hol}} = SO(4) = SU(2) \times SU(2)$ . One of the  $SU(2)$  factors of  $G_{\text{hol}}$  is twisted by the  $SU(2)_R$  symmetry to yield a single scalar supercharge on  $\mathcal{M}$ , which can be used to show that the partition function  $Z_{\mathcal{M}}$  is independent of the metric  $g_{\mu\nu}$  on  $\mathcal{M}$ . For this reason, the twist is referred to as topological. However, not all twists give rise to topological theories. For instance, four-dimensional  $\mathcal{N} = 1$  theories with a  $U(1)_R$  symmetry can be twisted on an arbitrary Kähler surface  $\mathcal{M}$ , for which  $G_{\text{hol}} = U(2)$  [16, 17]. Now the twisted theory depends on the complex structure of  $\mathcal{M}$ , and hence it is not topological.

Twisted theories are often described by performing a field redefinition to variables that are adapted to the geometric structure that underlies the twist. For instance, topologically twisted  $\mathcal{N} = 2$  theories can be described by fields that are differential forms on  $\mathcal{M}$ , while holomorphically twisted  $\mathcal{N} = 1$  theories on a Kähler surface  $\mathcal{M}$  lead to fields that are complex  $(p, q)$  forms on  $\mathcal{M}$ . However, the twisting procedure can also be implemented by coupling the original, untwisted supersymmetric field theory to a background  $R$ -symmetry gauge field  $A_{\mu}^{(R)}$ , which is tuned to cancel part of the spin connection [17, 18]. The preserved supercharge on  $\mathcal{M}$  is parametrized by an  $R$ -charged spinor  $\zeta$  that satisfies,

$$\left(\nabla_{\mu} - iA_{\mu}^{(R)}\right)\zeta = 0, \quad (5.1.9)$$

which generalizes (5.1.6).

Much recent activity has revolved around supersymmetric field theories on backgrounds that go beyond the basic twisting paradigm. Two prototypical examples of such backgrounds arose in the study of four-dimensional  $\mathcal{N} = 2$  theories with an  $SU(2)_R$  symmetry. (We will encounter additional examples below.) The first is the  $\Omega$ -background of [19, 20], which can be viewed as an equivariant deformation of the topological twist on  $\mathbb{R}^4 = \mathbb{R}_{\varepsilon_1}^2 \times \mathbb{R}_{\varepsilon_2}^2$  by an isometry that rotates two orthogonal  $\mathbb{R}^2$  planes inside  $\mathbb{R}^4$ . The rotation angles are determined by the equivariant parameters  $\varepsilon_{1,2}$ . This background preserves more supercharges than the topological twist, and the corresponding partition function  $Z_{\Omega}$  explicitly depends on  $\varepsilon_{1,2}$ , as well as some flat-space coupling constants, in a complicated and interesting way. The second example is a background on a round  $S^4$ , which preserves all eight supercharges [21]. The supersymmetry algebra is deformed to  $OSp(2|4)$ , whose bosonic subalgebra contains the  $SO(2)_R$  Cartan subalgebra of the  $SU(2)_R$  symmetry and the  $Sp(4) = SO(5)$  isometries of  $S^4$ . The partition function  $Z_{S^4}$  can depend on some flat-space couplings and the radius of the sphere. See [22] and Chapter 10 for a review of these two backgrounds and some of their applications.

### 5.1.3 Overview of the formalism

As was noted at the beginning of section 5.1.2, the obstruction to preserving supersymmetry on an arbitrary curved manifold  $\mathcal{M}$  is due to the fact that the stress tensor  $T_{\mu\nu}$  is not a

BPS operator. In supersymmetric theories  $T_{\mu\nu}$  resides in a supermultiplet, together with other bosonic and fermionic operators  $\mathcal{J}_B^i$  and  $\mathcal{J}_F^i$ . As we will review in section 5.2.1, the structure of the stress-tensor multiplet reflects very general properties of the field theory (e.g. the spacetime dimension, the amount of supersymmetry, the presence or absence of possible  $R$ -symmetries, or whether the theory is superconformal), but is otherwise largely model independent. Moreover, every supersymmetric field theory must have a stress tensor multiplet, even if the theory is strongly coupled or does not have a Lagrangian description.

The bosonic superpartners  $\mathcal{J}_B^i$  of the stress tensor can be coupled to suitable bosonic background fields  $\mathcal{B}_B^i$  and added to the Lagrangian (5.1.2),

$$\Delta\mathcal{L} = -\frac{1}{2}\Delta g^{\mu\nu}T_{\mu\nu} + \sum_i \mathcal{B}_B^i \mathcal{J}_B^i + (\text{seagull terms}) , \quad (5.1.10)$$

where we casually refer to all higher-order terms in the background fields as seagull terms. For special choices of  $\Delta g^{\mu\nu}$  and the other bosonic sources  $\mathcal{B}_B^i$ , the deformation  $\Delta\mathcal{L}$  can preserve some supersymmetry, due to cancellations between the supersymmetry transformations of  $T_{\mu\nu}$  and  $\mathcal{J}_B^i$ . At higher order, we must also ensure supersymmetry of the seagull terms, which can lead to additional conditions.<sup>11</sup>

Following [2], it was explained in [7] that the constraints of supersymmetry on the bosonic sources  $g_{\mu\nu}$ ,  $\mathcal{B}_B^i$  are best understood by embedding them into a supermultiplet. Their fermionic superpartners  $\mathcal{B}_F^i$ , which source the operators  $\mathcal{J}_F^i$  in the stress-tensor multiplet, are set to zero in the Lagrangian (5.1.10). As was emphasized in [7], the sources must reside in an off-shell supergravity multiplet, because they are non-dynamical background fields that couple to the stress-tensor supermultiplet. This construction can be viewed as a rigid limit of dynamical off-shell supergravity, where the fluctuations of the supergravity fields are frozen by scaling the Planck mass to infinity,  $M_p \rightarrow \infty$ . We will therefore refer to this construction of supersymmetric field theories on  $\mathcal{M}$  as rigid supersymmetry.

The requirement that  $\Delta\mathcal{L}$  in (5.1.2) should preserve a supercharge  $Q$  amounts to the statement that the  $Q$ -variation of all fermionic sources should vanish,

$$\delta_Q \mathcal{B}_F^i = 0 . \quad (5.1.11)$$

The left-hand side of this equation is a non-trivial bosonic expression, which involves the sources  $g_{\mu\nu}$ ,  $\mathcal{B}_B^i$  and the spinor  $\zeta$  that parametrizes the supercharge  $Q$ . The equations (5.1.11) simultaneously determine the allowed supersymmetric configurations for the bosonic background fields and the corresponding spinor parameter  $\zeta$ .

Even at this level of generality, we can make the following observations:

- The fermionic sources  $\mathcal{J}_F^i$  always include at least one background gravitino  $\Psi_\mu$ , whose supersymmetry variation takes the schematic form  $\delta_Q \Psi_\mu = \nabla_\mu \zeta + \dots$ . Imposing (5.1.11)

---

<sup>11</sup> A well-known example arises in four-dimensional  $\mathcal{N} = 2$  theories with a continuous flavor symmetry  $G$ . We can turn on complex mass parameters  $m$  that are valued in the (complexified) Lie algebra of  $G$ . At linear order, all such  $m$  are supersymmetric, but at quadratic order supersymmetry requires that  $[m, m^\dagger] = 0$ . See [24] for a recent discussion with references.

then leads to a differential equation for the spinor parameter  $\zeta$  that generalizes (5.1.6) and (5.1.9). We will follow standard practice and refer to such equations as (generalized) Killing spinor equations. A given configuration of background fields admits multiple supercharges if it satisfies (5.1.11) for each supercharge  $Q$ , i.e. if the Killing spinor equations in this background admit multiple independent solutions.

- Both the generalized Killing spinor equations and the rigid supersymmetry algebra on  $\mathcal{M}$  follow from the structure of the background off-shell supergravity multiplet. The rigid supersymmetry algebra is realized as a subalgebra of the (infinite-dimensional) algebra of supergravity gauge transformations. As we will review in section 5.2, a given field theory may admit several inequivalent stress-tensor supermultiplets. In this case it can be coupled to different off-shell supergravities,<sup>12</sup> which generally lead to inequivalent Killing spinor equations, and hence to different supersymmetric backgrounds.
- A rigid supersymmetric background is characterized by a full set of bosonic supergravity background fields, i.e. specifying only the metric does not determine the background. In particular, there are distinct backgrounds that have the same metric but lead to different partition functions. In general, they may arise from different off-shell supergravities, preserve different amounts of supersymmetry, or lead to different supersymmetry algebras.
- In Lorentzian signature, unitarity fixes the reality properties of the fields in the supergravity multiplet so that the Lagrangian (5.1.10) is real. In Euclidean signature, we are free to contemplate background fields that do not satisfy the reality conditions needed for unitarity (more precisely, reflection positivity). This greatly enriches the set of Euclidean backgrounds, and some interesting supersymmetric backgrounds can only be obtained in this way. (We will, however, always assume that the background metric  $g_{\mu\nu}$  is a standard Riemannian metric.) Observables (e.g. partition functions) computed in such non-unitary backgrounds in general do not possess standard reality properties. Nevertheless, they often encode interesting information about the underlying unitarity field theory.
- If the flat-space field theory has a Lagrangian description in terms of fields, then the Lagrangian and the supersymmetry transformation rules for the fields in curved space follow from the corresponding formulas in the appropriate matter-coupled off-shell supergravity.<sup>13</sup> These formulas are universal, i.e. they apply for arbitrary configurations of the supergravity fields. Once a given supersymmetric background has been found, the Lagrangian and the transformation rules in this background can be obtained by specializing the general formulas.

---

<sup>12</sup> Under certain conditions, distinct off-shell supergravities may be equivalent on shell, but this will not play a role in our discussion.

<sup>13</sup> The formalism only requires the supergravity fields to be off shell. For explicit computations, it is often convenient to also realize some supercharges off shell in the matter sector (see for instance Chapter 10).

It is straightforward to extend the preceding discussion to supersymmetric configurations of bosonic background fields residing in other supermultiplets. Supersymmetry requires the variations of all fermionic sources in the multiplet to vanish, as in (5.1.11). Below we will apply this to background gauge fields that couple to conserved flavor currents. However, the supergravity multiplet enjoys a special status, since it determines the number of supercharges and their algebra. Activating additional background fields that reside in other supermultiplets may preserve these supercharges, or it may break them to a (possibly trivial) subalgebra.

## 5.1.4 Outline

In the remainder of this review, we will illustrate the rigid supersymmetry formalism using  $\mathcal{N} = 1$  theories in four dimensions (section 5.2) and  $\mathcal{N} = 2$  theories in three dimensions (section 5.3). We discuss different stress-tensor and supergravity multiplets, and describe some of the corresponding supersymmetric backgrounds. We explain how to construct supersymmetric Lagrangians on these backgrounds and describe the data they depend on, paying particular attention to the data that originates from the coupling to the curved manifold  $\mathcal{M}$ . Finally, we explain to what extent this data can affect the partition function  $Z_{\mathcal{M}}$ . We will mostly focus on theories with a  $U(1)_R$  symmetry, but we also mention some results for theories that do not have such a symmetry.

We consider two examples in detail:  $\mathcal{N} = 1$  theories on  $S^3 \times S^1$  and  $\mathcal{N} = 2$  theories on a round or squashed  $S^3$ . The former background can be used to define an index that tracks supersymmetric operators along RG flows (it is closely related to the superconformal index, see Chapter 13). The latter backgrounds play a crucial role in  $F$ -maximization and can be used to compute correlation functions of conserved currents (see Chapter 8).

## 5.2 Four-dimensional $\mathcal{N} = 1$ theories

### 5.2.1 Stress-tensor multiplets and off-shell supergravities

As was explained in section 5.1.3, the procedure of placing a supersymmetric theory on a curved manifold commences with a choice of stress-tensor supermultiplet in flat space. The different possibilities that can arise in four-dimensional  $\mathcal{N} = 1$  theories were described in [26, 27]. (See also [28] for an early discussion.) Here we will restrict ourselves to the three most common multiplets. We will describe them in superspace (using the conventions of [9]) as well as in components. In all cases, the supersymmetry transformations of the component fields implicitly follow from the superspace description. In section 5.2.4 we will explicitly write out some of these transformation rules for theories with a  $U(1)_R$  symmetry.

- 1.) The stress-tensor multiplet of an  $\mathcal{N} = 1$  superconformal theory (SCFT) is a real superfield  $\mathcal{J}_\mu$  that satisfies

$$\overline{D}^{\dot{\alpha}} \mathcal{J}_{\alpha\dot{\alpha}} = 0, \quad \mathcal{J}_{\alpha\dot{\alpha}} = \sigma_{\alpha\dot{\alpha}}^\mu \mathcal{J}_\mu. \quad (5.2.1)$$

The component fields in  $\mathcal{J}_\mu$  are given by

$$\mathcal{J}_\mu = \left( j_\mu^{(R)}, S_{\mu\alpha}, T_{\mu\nu} \right), \quad (5.2.2)$$

where  $j_\mu^{(R)}$  is the superconformal  $U(1)_R$  current,  $S_{\mu\alpha}$  is the supersymmetry current, and  $T_{\mu\nu}$  is the stress tensor. All three currents are conserved, and the currents  $S_{\mu\alpha}, T_{\mu\nu}$  are traceless, i.e.  $\bar{\sigma}^{\mu\dot{\alpha}\alpha} S_{\mu\alpha} = T_\mu^\mu = 0$ .

- 2.) The majority of four-dimensional  $\mathcal{N} = 1$  theories (with or without an  $R$ -symmetry) admit a Ferrara-Zumino (FZ) stress-tensor multiplet [29].<sup>14</sup> The FZ-multiplet is given by a real superfield  $\mathcal{J}_\mu^{\text{FZ}}$ , such that

$$\bar{D}^{\dot{\alpha}} \mathcal{J}_{\alpha\dot{\alpha}}^{\text{FZ}} = D_\alpha X, \quad \bar{D}_{\dot{\alpha}} X = 0, \quad (5.2.3)$$

where  $\mathcal{J}_{\alpha\dot{\alpha}}^{\text{FZ}} = \sigma_{\alpha\dot{\alpha}}^\mu \mathcal{J}_\mu^{\text{FZ}}$ , as in (5.2.1). The component fields in the FZ-multiplet are

$$\mathcal{J}_\mu^{\text{FZ}} = (j_\mu, S_{\mu\alpha}, x, T_{\mu\nu}). \quad (5.2.4)$$

Here  $j_\mu$  is a non-conserved vector operator,  $S_{\mu\alpha}$  is the conserved supersymmetry current,  $x$  is a complex scalar, and  $T_{\mu\nu}$  is the conserved, symmetric stress tensor. The chiral superfield  $X$  is the trace submultiplet of the FZ-multiplet,<sup>15</sup>

$$X = \left( x, \sigma_{\alpha\dot{\alpha}}^\mu \bar{S}_\mu^{\dot{\alpha}}, T_\mu^\mu + i\partial^\mu j_\mu \right). \quad (5.2.5)$$

When  $X = 0$ , the FZ-multiplet reduces to the superconformal multiplet, as can be seen by comparing (5.2.3) and (5.2.1). In this case the vector operator  $j_\mu$  in the FZ-multiplet becomes the conserved superconformal  $U(1)_R$  current, and  $S_{\mu\alpha}, T_{\mu\nu}$  become traceless.

- 3.) Non-conformal theories with a  $U(1)_R$  symmetry possess a stress-tensor multiplet  $\mathcal{R}_\mu$ , whose bottom component is the conserved  $R$ -current  $j_\mu^{(R)}$ . In superspace,

$$\bar{D}^{\dot{\alpha}} \mathcal{R}_{\alpha\dot{\alpha}} = \chi_\alpha, \quad \bar{D}_{\dot{\alpha}} \chi_\alpha = 0, \quad D^\alpha \chi_\alpha = \bar{D}_{\dot{\alpha}} \bar{\chi}^{\dot{\alpha}}. \quad (5.2.6)$$

The component fields residing in the  $\mathcal{R}$ -multiplet are given by

$$\mathcal{R}_\mu = \left( j_\mu^{(R)}, S_{\mu\alpha}, T_{\mu\nu}, C_{\mu\nu} \right). \quad (5.2.7)$$

Here  $C_{\mu\nu} = C_{[\mu\nu]}$  is a conserved two-form current, which can give rise to a string charge in the supersymmetry algebra [27]. The superfield  $\chi_\alpha$ , which satisfies the same constraints as an abelian field-strength multiplet, is the trace submultiplet of the  $\mathcal{R}$ -multiplet. Setting  $\chi_\alpha = 0$  leads to the superconformal multiplet (5.2.1).

<sup>14</sup> The only known exceptions are abelian gauge theories with Fayet-Iliopoulos terms, and their analogues in the context of (gauged) sigma models [26, 27, 30, 31].

<sup>15</sup> Unlike unitary superconformal multiplets, which possess a unique lowest-weight state, multiplets of Poincaré supersymmetry may be reducible (i.e. they may contain non-trivial submultiplets) without being decomposable into smaller multiplets. See [27] for a discussion in the context of stress-tensor multiplets.

Some theories have more than one stress-tensor multiplet. For instance, a theory with an FZ-multiplet may possess a  $U(1)_R$  symmetry, in which case it also admits an  $\mathcal{R}$ -multiplet. In this case the two multiplets are related by a supersymmetric analogue of the improvement transformation (5.1.3) for the stress tensor.

The off-shell supergravity multiplets that couple to the conformal stress-tensor multiplet, the FZ-multiplet and the  $\mathcal{R}$ -multiplet are conformal supergravity [32], as well as the old [33,34] and new [35,36] minimal formulations of off-shell supergravity. (See [37] for a recent discussion of conformal and old minimal supergravity; additional details on new minimal supergravity can be found in [38].) In principle, we can use any set of off-shell supergravity fields, as long as the flat-space theory admits the corresponding stress-tensor multiplet. In practice, it is often useful to consider non-conformal supergravity, even if the flat-space theory is conformal. The reason is that, quantum mechanically, even CFTs must be defined using a UV cutoff, which breaks conformal symmetry but can often be chosen to preserve supersymmetry. If the theory is conformal, we expect the non-conformal supergravity fields to decouple as the UV cutoff is taken to infinity. However, some remnants of the regulator, and hence of the non-conformal supergravity fields, may survive:

- The allowed supersymmetric counterterms that parametrized the UV ambiguities (i.e. the scheme dependence) of the partition function  $Z_{\mathcal{M}}$  are governed by the non-conformal supergravity theory that couples to the combined SCFT-regulator system. The non-conformal gravity fields can in principle be decoupled by fine-tuning these counterterms, but in practice one is typically left with an ambiguity parametrized by local counterterms that involve the non-conformal supergravity fields.<sup>16</sup> This plays an important role in elucidating the properties of supersymmetric partition functions and interpreting the results of explicit localization computations. See for instance [39–47] and references therein for a sampling of the recent literature.
- The decoupling of the non-conformal supergravity fields can be spoiled by superconformal anomalies, which cannot (even in principle) be removed by fine-tuning the allowed supersymmetric counterterms. Examples are Weyl anomalies in even dimensions, which render  $T_{\mu}^{\mu} \neq 0$  in the presence of certain background fields. Such anomalies are, for instance, discussed in [47–49], as well as Chapter 4. A different, global superconformal anomaly in three dimensions was described in [40].

In light of the above, we will only consider the non-conformal old and new minimal supergravity theories.<sup>17</sup> Moreover, most of our discussion will focus on the new minimal formulation, because field theories with a  $U(1)_R$  symmetry are typically under better theoretical control.

---

<sup>16</sup> Relevant counterterms are multiplied by positive powers of the UV cutoff  $\Lambda$ , so that they are easily identified and adjusted. It is typically more difficult to isolate the effects of marginal counterterms.

<sup>17</sup> Even though we will not do so here, it is often convenient to formulate non-conformal supergravity theories as coupled systems consisting of a conformal supergravity multiplet and one or several compensating matter multiplets that can be used to Higgs the conformal symmetry.

## 5.2.2 Theories with an $R$ -symmetry

The coupling of theories with a  $U(1)_R$  symmetry to supergravity background fields proceeds via the  $\mathcal{R}$ -multiplet (5.2.6) and (5.2.7), whose component fields we repeat here for convenience,

$$\mathcal{R}_\mu = \left( j_\mu^{(R)}, S_{\mu\alpha}, T_{\mu\nu}, C_{\mu\nu} \right) . \quad (5.2.8)$$

The appropriate background fields reside in the new minimal supergravity multiplet [35, 36],

$$\mathcal{H}_\mu = \left( A_\mu^{(R)}, \Psi_{\mu\alpha}, g_{\mu\nu}, B_{\mu\nu} \right) . \quad (5.2.9)$$

In addition to the metric  $g_{\mu\nu}$  and the gravitino  $\Psi_{\mu\alpha}$ , this multiplet contains a  $U(1)_R$  gauge field  $A_\mu^{(R)}$ , which couples to the conserved  $R$ -current  $j_\mu^{(R)}$ , and a two-form gauge field  $B_{\mu\nu}$ , which couples to the conserved two-form current  $C_{\mu\nu}$ . We will often use the Hodge dual of its field strength, which is a covariantly conserved vector field,<sup>18</sup>

$$V^\mu = \frac{i}{2} \varepsilon^{\mu\nu\rho\lambda} \partial_\nu B_{\rho\lambda} , \quad \nabla_\mu V^\mu = 0 . \quad (5.2.10)$$

The only fermionic field in the new minimal supergravity multiplet (5.2.9) is the gravitino  $\Psi_{\mu\alpha}$ .

As explained around (5.1.11), the supersymmetric configurations of the bosonic background fields are determined by setting the supersymmetry variations of the gravitino to zero. In new minimal supergravity, these variations take the following form,

$$\delta\Psi_{\mu\alpha} = -2 \left( \nabla_\mu - iA_\mu^{(R)} \right) \zeta_\alpha - iV^\nu \sigma_{\mu\alpha\dot{\alpha}} \bar{\sigma}_\nu^{\dot{\alpha}\beta} \zeta_\beta , \quad (5.2.11)$$

$$\delta\bar{\Psi}_\mu^{\dot{\alpha}} = -2 \left( \nabla_\mu + iA_\mu^{(R)} \right) \bar{\zeta}^{\dot{\alpha}} + iV^\nu \bar{\sigma}_\mu^{\dot{\alpha}\alpha} \sigma_{\nu\alpha\dot{\beta}} \bar{\zeta}^{\dot{\beta}} . \quad (5.2.12)$$

These formulas are valid in Lorentzian signature, where the left-handed spinor  $\zeta_\alpha$  of  $R$ -charge +1 and the right-handed spinor  $\bar{\zeta}_{\dot{\alpha}}$  of  $R$ -charge +1 are related by complex conjugation, while  $A_\mu^{(R)}$  and  $V_\mu$  are real.

In Euclidean signature, the left-handed and right-handed spinors are independent and no longer related by complex conjugation. We will emphasize this by writing tildes instead of bars, e.g.  $\tilde{\zeta}_{\dot{\alpha}}$  instead of  $\bar{\zeta}_{\dot{\alpha}}$  and  $\tilde{\sigma}_\mu$  instead of  $\bar{\sigma}_\mu$ . (In Euclidean signature, we follow the conventions of [8].) Moreover, the Lorentzian reality conditions on  $A_\mu^{(R)}$  and  $V_\mu$  may be relaxed at the expense of unitarity. In general, a supercharge  $Q$  is characterized by a pair  $(\zeta, \tilde{\zeta})$  of left- and right-handed Killing spinors, but in new minimal supergravity we can always consider supercharges  $(\zeta, 0)$  or  $(0, \tilde{\zeta})$  of definite  $R$ -charge. (In section 5.2.6 we will discuss theories without an  $R$ -symmetry, where this decomposition of  $(\zeta, \tilde{\zeta})$  is generally not possible.) A supercharge  $Q$  of  $R$ -charge  $-1$  corresponds to a Killing spinor  $\zeta$  for which the right-hand side of (5.2.11) vanishes,

$$\left( \nabla_\mu - iA_\mu^{(R)} \right) \zeta = -\frac{i}{2} V^\nu \sigma_\mu \tilde{\sigma}_\nu \zeta . \quad (5.2.13)$$

<sup>18</sup> The factor of  $i$  in (5.2.10) is absent in Lorentzian signature, where both  $B_{\mu\nu}$  and  $V^\mu$  are real.

Similarly, a supercharge  $\tilde{Q}$  of  $R$ -charge  $+1$  corresponds to a Killing spinor  $\tilde{\zeta}$  for which the right-hand side of (5.2.12) vanishes,

$$\left(\nabla_\mu + iA_\mu^{(R)}\right)\tilde{\zeta} = \frac{i}{2}V^\nu\tilde{\sigma}_\mu\sigma_\nu\tilde{\zeta} . \quad (5.2.14)$$

Note that these equations reduce to (5.1.9), which describes twisting, when the background field  $V^\mu$  vanishes.

As explained in section 5.1.3, the rigid supersymmetry algebra satisfied by the supercharges  $Q$  or  $\tilde{Q}$  descends from the algebra of local supergravity transformations. In new minimal supergravity, this algebra includes local supersymmetry transformations (parametrized by arbitrary spinors  $\zeta, \tilde{\zeta}$ ), as well as diffeomorphisms, local Lorentz transformations, and  $R$ -symmetry gauge transformations [35, 36]. If we restrict to Killing spinors that satisfy (5.2.13) and (5.2.14), this algebra simplifies and reduces to the rigid supersymmetry algebra satisfied by the supercharges  $Q, \tilde{Q}$ . On a field  $\Phi$  with  $U(1)_R$  charge  $r$  and arbitrary spin, the algebra is given by

$$\begin{aligned} \{\delta_Q, \delta_{\tilde{Q}}\}\Phi &= 2i\mathcal{L}'_K\Phi , & K^\mu &= \zeta\sigma^\mu\tilde{\zeta} , \\ \delta_Q^2\Phi &= \delta_{\tilde{Q}}^2\Phi = 0 . \end{aligned} \quad (5.2.15)$$

The infinitesimal variations anticommute because we take the spinors  $\zeta, \tilde{\zeta}$  to be commuting. It follows from the Killing spinor equations (5.2.13) and (5.2.14) that  $K^\mu$  is a Killing vector. The operator  $\mathcal{L}'_K$  denotes a modified Lie derivative along  $K$ , which is twisted by the  $R$ -symmetry,

$$\mathcal{L}'_K\Phi = \mathcal{L}_K\Phi - irK^\mu\left(A_\mu^{(R)} + \frac{3}{2}V_\mu\right)\Phi . \quad (5.2.16)$$

Here  $\mathcal{L}_K$  is the ordinary Lie derivative.<sup>19</sup> Due to the twist, the  $R$ -charge can appear on the right-hand side of the supersymmetry algebra, unlike in standard flat-space supersymmetry.

The solutions to the generalized Killing spinor equations (5.2.13) and (5.2.14) were analyzed in [7, 51, 52], and the conditions for the existence of one or several supercharges were deduced. In particular, it was found that a single supercharge  $Q$  of  $R$ -charge  $-1$  exists if and only if  $\mathcal{M}$  is a complex manifold, i.e. it admits an integrable complex structure  $J^\mu{}_\nu$ , and  $g_{\mu\nu}$  is a compatible Hermitian metric. Since there is only one supercharge, it follows from (5.2.15) that it must square to zero, i.e.  $\delta_Q^2 = 0$ . In section 5.2.5 we will discuss complex manifolds with topology  $S^3 \times S^1$  that preserve up to four supercharges.

The Killing spinor  $\zeta$  corresponding to a single supercharge  $Q$  on a complex manifold  $\mathcal{M}$  is simply related to the complex structure  $J^\mu{}_\nu$  on  $\mathcal{M}$ ,

$$J^\mu{}_\nu = -\frac{2i}{|\zeta|^2}\zeta^\dagger\sigma^\mu{}_\nu\zeta . \quad (5.2.17)$$

<sup>19</sup> Its action on spinors  $\chi_\alpha, \tilde{\chi}_{\dot{\alpha}}$  is given by

$$\mathcal{L}_K\chi = \nabla_\mu\chi - \frac{1}{2}\nabla_\mu K_\nu\sigma^{\mu\nu}\chi , \quad \mathcal{L}_K\tilde{\chi} = \nabla_\mu\tilde{\chi} - \frac{1}{2}\nabla_\mu K_\nu\tilde{\sigma}^{\mu\nu}\tilde{\chi} .$$

The background fields  $A_\mu^{(R)}$  and  $V_\mu$  are essentially determined by  $J^\mu{}_\nu$  and the Hermitian metric  $g_{\mu\nu}$ . Here we will only quote the formula for  $V^\mu$ ,

$$V^\mu = \frac{1}{2} \nabla_\nu J^\nu{}_\mu , \quad (5.2.18)$$

up to a freely adjustable piece that will play no role in our discussion. (See [8] for additional details, including the formula for  $A_\mu^{(R)}$ .) Note that  $V^\mu$  vanishes when  $\mathcal{M}$  is Kähler, so that  $J^\mu{}_\nu$  is covariantly constant. As discussed around (5.1.9), this is precisely the case that allows for twisting by the  $U(1)_R$  symmetry. Therefore, the supergravity construction reduces to twisting in the appropriate limit, but it is more general. For instance, it allows complex manifolds  $\mathcal{M}$  that are not Kähler, such as the  $S^3 \times S^1$  backgrounds discussed in section 5.2.5. This is only possible because of the additional field  $V^\mu$  supplied by new minimal supergravity.

An important fact that carries over from twisting is that the supercharge  $Q$  on the complex manifold  $\mathcal{M}$  transforms as a scalar under holomorphic coordinate changes [52]. This will play a crucial role in section 5.2.4, where we analyze the dependence of the partition function  $Z_{\mathcal{M}}$  on the geometry of  $\mathcal{M}$ .

It is straightforward to extend the preceding discussion to background gauge fields  $a_\mu$ , which couple to conserved flavor currents  $j_\mu$  [8, 53]. Here we will focus on a single  $U(1)$  current. In flat space, it resides in a real linear superfield  $\mathcal{J}$ , which satisfies

$$D^2 \mathcal{J} = \bar{D}^2 \mathcal{J} = 0 . \quad (5.2.19)$$

In components,

$$\mathcal{J} = \left( J , j_\alpha , \bar{j}_{\dot{\alpha}} , j_\mu \right) , \quad \partial^\mu j_\mu = 0 . \quad (5.2.20)$$

The corresponding background gauge field  $a_\mu$  resides in a vector multiplet  $\mathcal{V}$ . In Wess-Zumino gauge,

$$\mathcal{V} = \left( D , \lambda_\alpha , \bar{\lambda}_{\dot{\alpha}} , a_\mu \right) . \quad (5.2.21)$$

Here  $D$  is a real auxiliary field and  $\lambda_\alpha$  is the gaugino. In order to determine the allowed supersymmetric configurations of the bosonic background fields  $a_\mu, D$  on a complex manifold  $\mathcal{M}$  with supercharge  $Q$ , we follow the same logic as above and set

$$\delta_Q \lambda = i\zeta D + \sigma^{\mu\nu} \zeta f_{\mu\nu} = 0 , \quad f_{\mu\nu} = \partial_\mu a_\nu - \partial_\nu a_\mu . \quad (5.2.22)$$

This leads to the following constraints,

$$f^{0,2} = 0 , \quad D = -\frac{1}{2} J^{\mu\nu} f_{\mu\nu} , \quad (5.2.23)$$

where  $f^{0,2}$  is the anti-holomorphic  $(0, 2)$  component of the two-form  $f_{\mu\nu}$ . Therefore, supersymmetric background gauge fields are in one-to-one correspondence with holomorphic line bundles over the complex manifold  $\mathcal{M}$ .

### 5.2.3 Lagrangians

As was emphasized in section 5.1.3, the rigid supersymmetry approach cleanly separates between the allowed supersymmetric backgrounds and their supersymmetry algebras (which were discussed in section 5.2.2), and supersymmetric Lagrangians on these backgrounds. These Lagrangians only depend on a choice of background supergravity multiplet, but not on the specific field configuration of the supergravity fields. They can be straightforwardly obtained from the corresponding formulas in new-minimal supergravity [35, 36, 38].

Consider, for instance, a free chiral multiplet  $\Phi = (\phi, \psi_\alpha, F)$  of  $R$ -charge  $r$ , and its conjugate anti-chiral multiplet  $\tilde{\Phi} = (\tilde{\phi}, \tilde{\psi}_{\dot{\alpha}}, \tilde{F})$  of  $R$ -charge  $-r$ , with flat-space Lagrangian

$$\mathcal{L}_{\mathbb{R}^4} = \partial^\mu \tilde{\phi} \partial_\mu \phi - i \tilde{\psi} \tilde{\sigma}^\mu \partial_\mu \psi - \tilde{F} F . \quad (5.2.24)$$

The corresponding curved-space Lagrangian in the presence of supergravity background fields is given by [7],

$$\mathcal{L}_{\mathcal{M}} = \mathcal{L}_{\mathbb{R}^4} \Big|_{\text{covariant}} + V^\mu \left( i \tilde{\phi} \overleftrightarrow{D}_\mu \phi + \tilde{\psi} \tilde{\sigma}_\mu \psi \right) - r \left( \frac{1}{4} R - 3V^\mu V_\mu \right) \tilde{\phi} \phi . \quad (5.2.25)$$

Here  $D_\mu = \partial_\mu - irA_\mu^{(R)}$  is the  $R$ -covariant derivative, and  $\mathcal{L}_{\mathbb{R}^4} \Big|_{\text{covariant}}$  is the covariantization of (5.2.24) with respect to diffeomorphisms and  $R$ -symmetry gauge transformations. It describes the minimal coupling of  $\mathcal{L}_{\mathbb{R}^4}$  to background fields. However, supersymmetry requires the presence of additional, non-minimal terms in the Lagrangian (5.2.25). Moreover, these terms explicitly depend on the  $R$ -charge  $r$  of  $\Phi$ , i.e. on the choice of  $\mathcal{R}$ -multiplet that was used to couple the flat-space theory to background supergravity. This agrees with the general discussion in section 5.1.3: the coupling to  $\mathcal{M}$  proceeds through the stress-tensor multiplet and different multiplets lead to different theories in curved space. Here the ability to freely assign any  $R$ -charge  $r$  to  $\Phi$  reflects the freedom to choose an  $\mathcal{R}$ -multiplet from a continuous family of such multiplets. In other situations the  $R$ -charge may be fixed, e.g. in the presence of a superpotential  $W = \Phi^n$  we must set  $r = \frac{2}{n}$ .<sup>20</sup>

The non-minimal terms in (5.2.25) also require a corresponding modification of the supersymmetry transformations,

$$\begin{aligned} \delta \phi &= \sqrt{2} \zeta \psi , \\ \delta \psi &= \sqrt{2} \zeta F + i \sqrt{2} \sigma^\mu \tilde{\zeta} \left( \partial_\mu - irA_\mu^{(R)} \right) \phi , \\ \delta F &= \sqrt{2} \tilde{\zeta} \tilde{\sigma}^\mu \left( \nabla_\mu - i(r-1)A_\mu^{(R)} - \frac{i}{2} V_\mu \right) \psi , \end{aligned} \quad (5.2.26)$$

and similarly for the conjugate fields in the anti-chiral multiplet  $\tilde{\Phi}$ . Given a solution  $\zeta$  of the Killing spinor equation (5.2.13), we can substitute the corresponding background fields

---

<sup>20</sup> Note that the curvature coupling  $\sim rR\tilde{\phi}\phi$  in (5.2.25) may lead to a tachyonic instability if the curvature  $R$  has a definite sign and  $|r|$  is too large. This is born out in explicit examples, e.g. some supersymmetric partition functions are only meaningful if the  $R$ -charges are restricted to a certain range.

into the Lagrangian (5.2.25) and verify that it is supersymmetric under (5.2.26), provided we use (5.2.13).

Broadly speaking, the curved-space Lagrangian  $\mathcal{L}_{\mathcal{M}}$  depends on three kinds of data:

- 1.) Data that was already present in the flat-space Lagrangian  $\mathcal{L}_{\mathbb{R}^4}$ .
- 2.) The choice of  $\mathcal{R}$ -multiplet that is used to couple the flat-space theory to supergravity background fields. For a theory with a Lagrangian description, this amounts to a set of  $R$ -charge assignments for the fields.
- 3.) Various geometric structures on  $\mathcal{M}$ , i.e. the complex structure  $J^\mu{}_\nu$ , the Hermitian metric  $g_{\mu\nu}$ , and possibly background flavor gauge fields described by holomorphic line bundles over  $\mathcal{M}$ . These structures emerge from the Killing spinor equations (5.2.13) and (5.2.14), as well as (5.2.22) for background gauge fields.

We will now explain how supersymmetry constrains the dependence of the partition function  $Z_{\mathcal{M}}$  on this data, focusing on the curved-space data summarized in 2.) and 3.) above.

#### 5.2.4 Constraining the partition function

We can use supersymmetry to constrain the dependence of the partition function  $Z_{\mathcal{M}}$  on continuous data. The basic idea is to vary the data by a small amount, schematically denoted by  $\Delta\mathcal{M}$ , and check whether the corresponding small change  $\Delta\mathcal{L}_{\mathcal{M}}$  in the Lagrangian is  $Q$ -exact. If this is the case, the partition function does not depend on the deformation,

$$\Delta\mathcal{L}_{\mathcal{M}} = (\Delta\mathcal{M}) \{Q, \mathcal{O}\}, \quad \Delta Z_{\mathcal{M}} \sim \langle \{Q, \mathcal{O}\} \rangle = 0. \quad (5.2.27)$$

The same logic underlies the localization argument, which was sketched around (5.1.7) and (5.1.8).

A head-on analysis of this problem is possible [53], but it is complicated by the fact that the curved-space Lagrangian and the supersymmetry transformations depend on the continuous data that we would like to vary. Here we will explain a simple but powerful method for sidestepping these complications, which has the added advantage of not requiring a Lagrangian. The simplification proceeds in two steps:

- 1.) If we work around flat space, with a nearly flat metric, then the deformation Lagrangian  $\Delta\mathcal{L}_{\mathcal{M}}$  consists of operators in the stress-tensor multiplet of the flat-space theory, i.e. the  $\mathcal{R}$ -multiplet (5.2.7). The known supersymmetry transformations of these operators can be used to determine which terms in  $\Delta\mathcal{L}_{\mathcal{M}}$  are  $Q$ -exact.
- 2.) These results can be extended to arbitrary complex manifolds by using the fact that the supercharge  $Q$  is a scalar under holomorphic coordinate transformations.

This logic is standard in the context of topological twisting (see for instance [5, 16]), where  $Q$  is a scalar under all coordinate changes and a suitably defined stress-tensor  $\hat{T}_{\mu\nu}$  is  $Q$ -exact in flat space,  $\hat{T}_{\mu\nu} = \{Q, \Lambda_{\mu\nu}\}$ . This is generally sufficient to ensure that the partition function  $Z_{\mathcal{M}}$  on any four-manifold  $\mathcal{M}$  does not depend on the metric  $g_{\mu\nu}$ .

Following [8], we will now apply this argument to constrain the dependence of the partition function  $Z_{\mathcal{M}}$  on a complex manifold  $\mathcal{M}$  on the complex structure  $J^\mu{}_\nu$  and the Hermitian metric  $g_{\mu\nu}$ . To this end, we introduce local holomorphic coordinates  $z^i$  ( $i = 1, 2$ ), in which the non-zero components of the complex structure and the metric are given by

$$J^i{}_j = i\delta^i{}_j, \quad J^{\bar{i}}{}_{\bar{j}} = -i\delta^{\bar{i}}{}_{\bar{j}}, \quad g_{i\bar{j}}. \quad (5.2.28)$$

In these coordinates, infinitesimal variations  $\Delta J^\mu{}_\nu, \Delta g_{\mu\nu}$  of the complex structure and the metric must satisfy the following constraints,

$$\begin{aligned} \Delta J^i{}_j &= \Delta J^{\bar{i}}{}_{\bar{j}} = 0, & \partial_{\bar{j}}\Delta J^i{}_k - \partial_k\Delta J^i{}_{\bar{j}} &= 0, \\ \Delta g_{i\bar{j}} &= \text{anything}, & \Delta g_{ij} &= \frac{i}{2}(\Delta J_{ij} + \Delta J_{j\bar{i}}). \end{aligned} \quad (5.2.29)$$

The first line ensures that  $J^\mu{}_\nu + \Delta J^\mu{}_\nu$  is also an integrable complex structure (at first order in the variation), while the second line is the statement that the deformed metric  $g_{\mu\nu} + \Delta g_{\mu\nu}$  should be Hermitian with respect to the deformed complex structure. Complex structure deformations of the form

$$\Delta J^i{}_{\bar{j}} = 2i\partial_{\bar{j}}\varepsilon^i, \quad (5.2.30)$$

are induced by an infinitesimal diffeomorphism parametrized by the vector field  $\varepsilon^\mu$ . This leads to a cohomology problem for non-trivial complex structure deformations: they correspond to classes in  $H^{0,1}(\mathcal{M}, T^{1,0}\mathcal{M})$ . If  $\mathcal{M}$  is compact (as we are assuming here), this is a finite-dimensional vector space, i.e. there is a finite number of complex structure moduli. See [54] for an introduction to the deformation theory of complex manifolds.

We begin with the linearized couplings of the bosonic operators (5.2.8) in the  $\mathcal{R}$ -multiplet to the bosonic new minimal supergravity fields (5.2.9) (this is (5.1.10), specialized to new minimal supergravity),<sup>21</sup>

$$\Delta\mathcal{L} = -\frac{1}{2}\Delta g^{\mu\nu}T_{\mu\nu} + A^{(R)\mu}j_\mu^{(R)} + B^{\mu\nu}C_{\mu\nu}. \quad (5.2.31)$$

We can now substitute the deformations (5.2.29) into this formula. (This requires the formula for  $B_{\mu\nu}$  in (5.2.18) and the formula for  $A_\mu^{(R)}$  in [8].) We find that

$$\Delta\mathcal{L} = -\Delta g^{i\bar{j}}\mathcal{T}_{i\bar{j}} - i\sum_j \Delta J^{\bar{i}}{}_j \mathcal{T}_{\bar{i}i} + i\sum_j \Delta J^i{}_{\bar{j}} (\mathcal{T}_{ij} + i\partial_{\bar{j}}j_i^{(R)}), \quad (5.2.32)$$

where we have defined the following (complex) linear combination of operators in the  $\mathcal{R}$ -multiplet,

$$\mathcal{T}_{\mu\nu} = T_{\mu\nu} + \frac{1}{4}C_{\mu\nu} - \frac{i}{4}\varepsilon_{\mu\nu\rho\lambda}\partial^\rho j^{(R)\lambda} - \frac{i}{2}\partial_\nu j_\mu^{(R)}. \quad (5.2.33)$$

<sup>21</sup> Our operator  $C_{\mu\nu}$  was denoted by  $\frac{i}{4}\varepsilon_{\mu\nu\rho\lambda}\mathcal{F}^{\rho\lambda}$  in [8].

We can now ask whether any of these operators are  $Q$ -exact, and hence do not affect the partition function when they appear in (5.2.32). The only fermionic operators in the  $\mathcal{R}$ -multiplet are the supersymmetry current  $S_{\mu\alpha}$  and its conjugate  $\tilde{S}_{\mu\dot{\alpha}}$ , whose  $Q$ -variations are given by

$$\{Q, S_{\mu\alpha}\} = 0, \quad \{Q, \tilde{S}_{\mu\dot{\alpha}}\} = 2i (\tilde{\sigma}^\nu \zeta)_{\dot{\alpha}} \mathcal{T}_{\mu\nu}. \quad (5.2.34)$$

Using the relation (5.2.17) between the Killing spinor  $\zeta$  and the complex structure  $J^\mu{}_\nu$ , it can be shown that the second relation in (5.2.34) amounts to the statement that all operators of the form  $\mathcal{T}_{\mu\bar{i}}$ , for any index  $\mu$ , are  $Q$ -exact. Comparing with (5.2.32) shows that:

- 1.) The partition function  $Z_{\mathcal{M}}$  does not depend on the Hermitian metric  $g_{i\bar{j}}$ .
- 2.) The partition function  $Z_{\mathcal{M}}$  depends on  $\Delta J^i{}_{\bar{j}}$ , but not on its complex conjugate  $\Delta J^{\bar{i}}{}_j$ , i.e. it is a holomorphic function of the complex structure moduli.<sup>22</sup>

These results lead to the following observations:

- Since  $Z_{\mathcal{M}}$  does not depend on the metric, we can rescale  $g_{i\bar{j}} \rightarrow \lambda^2 g_{i\bar{j}}$  for some constant  $\lambda$ . This uniform scale transformation can be identified with RG flow, and hence  $Z_{\mathcal{M}}$  can be computed in the UV or in the deep IR of any non-trivial RG flow. An immediate consequence is that  $Z_{\mathcal{M}}$  must be invariant under IR dualities, such as Seiberg duality [55].
- The arguments above apply to small (infinitesimal) deformations, and hence they only show that  $Z_{\mathcal{M}}$  is a locally holomorphic function of the complex structure moduli. There are generally interesting singularities at certain loci in moduli space. Even the metric independence of  $Z_{\mathcal{M}}$  may only hold for sufficiently small deformations (see for instance [14]).
- We can repeat the preceding analysis for flavor current multiplets. The upshot is that  $Z_{\mathcal{M}}$  only depends on background gauge fields through the corresponding holomorphic line bundles [8]. In particular, it is a locally holomorphic function of the bundle moduli. If  $\mathcal{M}$  is compact, there are finitely many of them.

So far we have discussed the dependence of  $Z_{\mathcal{M}}$  on the geometric structures supplied by the background fields. We can use similar methods to analyze its dependence on the choice of  $U(1)_R$  symmetry that is used to couple the flat-space field theory to  $\mathcal{M}$ . A detailed discussion can be found in [53]. Here we only recall that, in flat space, the  $R$ -symmetry is not unique whenever there is an abelian flavor symmetry that can mix with it. However, in a non-trivial background the  $R$ -charges may be quantized, and hence not continuously variable (see for instance [8, 52]). Only special classes of complex manifolds allow a continuously variable  $R$ -symmetry.<sup>23</sup>

<sup>22</sup> Note that  $Z_{\mathcal{M}}$  cannot depend on trivial deformations that vanish in cohomology, since these are induced by background diffeomorphisms.

<sup>23</sup> The precise condition is that the canonical bundle  $\mathcal{K}$  of the complex manifold  $\mathcal{M}$  must be topologically trivial, i.e. its Chern class must vanish,  $c_1(\mathcal{K}) = 0$ .

### 5.2.5 Example: $S^3 \times S^1$

We will now briefly summarize an application of the general results discussed above to complex manifolds with topology  $S^3 \times S^1$ . (See [8] for additional details.) It follows from results of Kodaira [56] that every such complex manifold must be a primary Hopf surface, which comes in two types. We will focus on a primary Hopf surface of the first type,  $\mathcal{M}^{p,q}$ , which is defined by the following holomorphic quotient,

$$\mathcal{M}^{p,q} = \{\mathbb{C}^2 - (0,0)\} / \{(w,z) \sim (pw,qz)\} , \quad 0 < |p| \leq |q| < 1 . \quad (5.2.35)$$

Here  $p, q$  are complex structure moduli of the Hopf surface. The results summarized in section 5.2.4 imply that the partition function  $Z_{\mathcal{M}^{p,q}}$  is a locally holomorphic function of  $p, q$ . If there are abelian background gauge fields, it must also be locally holomorphic in the corresponding bundle modulus  $u$ . (It can be shown that there is only one such modulus on  $\mathcal{M}^{p,q}$ .) Partition functions on Hopf surfaces were directly studied in [57, 58] using localization techniques.

It can be shown [8] that  $Z_{\mathcal{M}}(p, q, u)$  coincides with the supersymmetric index  $\mathcal{I}(p, q, u)$  for states on  $S^3 \times \mathbb{R}$  defined in [59] (see also [7, 60, 61]), with general complex fugacities  $p, q, u$ .<sup>24</sup> If the theory is an SCFT, this index coincides with the superconformal index of [61], which counts BPS operators, but in general it is distinct. In particular, it is defined away from the conformal point and can be tracked along RG flows. See Chapter 13 for a more detailed discussion.

It is worth commenting on the  $S^3 \times \mathbb{R}$  background of new minimal supergravity that is used to define the index [7, 62]. It preserves four supercharges that anticommute to an  $SU(2|1)$  superalgebra. The bosonic subalgebra  $SU(2) \times U(1)$  contains one of the  $SU(2)$  factors of the  $SU(2)_\ell \times SU(2)_r$  isometry of  $S^3$ , and a  $U(1)$  factor that is a linear combination of time translations along  $\mathbb{R}$  and the  $R$ -charge. The supergravity background fields are given by

$$ds^2 = d\tau^2 + r^2 d\Omega_3 , \quad V = \pm \frac{i}{r} d\tau , \quad A^{(R)} = -\frac{1}{2} V . \quad (5.2.36)$$

Here  $r$  is the radius of the round  $S^3$ , and the sign of  $V$  depends on whether the  $SU(2) \subset SU(2|1)$  is identified with  $SU(2)_\ell$  or  $SU(2)_r$ . The choice of  $A^{(R)}$  is such that the supercharges are time independent. Note that the background fields are consistent with reflection positivity in Euclidean signature, since the  $\tau$ -components of  $V$  and  $A^{(R)}$  are purely imaginary, i.e. they would be real in Lorentzian signature. The non-conformal index  $\mathcal{I}(p, q, u)$  is defined as the Witten index of the theory on  $S^3 \times \mathbb{R}$  in Hamiltonian quantization,

$$\mathcal{I}(p, q, u) = \text{Tr}_{\mathcal{H}_{S^3}} \left( (-1)^F p^{J_\ell + J_r - \frac{R}{2}} q^{J_\ell - J_r - \frac{R}{2}} u^{Q_{\text{flavor}}} \right) . \quad (5.2.37)$$

Here  $\mathcal{H}_{S^3}$  is the Hilbert space of states on  $S^3$ ,  $J_\ell$  and  $J_r$  are the Cartan generators of  $SU(2)_\ell$  and  $SU(2)_r$ ,  $R$  is the  $U(1)_R$  charge, and  $Q_{\text{flavor}}$  is the  $U(1)$  flavor charge associated with the fugacity  $u$ .

<sup>24</sup> More precisely, the equality between  $Z_{\mathcal{M}}$  and  $\mathcal{I}$  holds up to a scheme-independent factor, which arises from anomalies and can be interpreted as a supersymmetric Casimir energy [46, 57].

## 5.2.6 Theories without an $R$ -symmetry

Theories without a  $U(1)_R$  symmetry do not possess an  $\mathcal{R}$ -multiplet, and hence they cannot be coupled to the new minimal supergravity background fields. Consequently, the discussion in the preceding subsections does not apply to them. A prominent example of such a theory is pure  $\mathcal{N} = 1$  supersymmetric Yang-Mills theory, where the  $U(1)_R$  symmetry is explicitly broken by an anomaly. However, even theories without an  $R$ -symmetry typically possess an FZ-multiplet (5.2.4), which can be coupled to the old minimal supergravity background fields [33, 34],

$$\mathcal{H}_\mu = \left( b_\mu, \Psi_{\mu\alpha}, M, \widetilde{M}, g_{\mu\nu} \right). \quad (5.2.38)$$

Here  $b_\mu$  is a well-defined (i.e. non-gauge) vector field, and  $M, \widetilde{M}$  are complex scalars. In Lorentzian signature  $\widetilde{M} = \overline{M}$ , but in Euclidean signature they may be independent.

The Killing spinor equations that follow from setting the supersymmetry variation of the gravitino  $\Psi_{\mu\alpha}$  to zero are given by [7]

$$\nabla_\mu \zeta = \frac{i}{6} M \sigma_\mu \tilde{\zeta} + \frac{i}{3} b_\mu \zeta + \frac{i}{3} b^\nu \sigma_{\mu\nu} \zeta, \quad (5.2.39)$$

and a similar equation with  $\zeta \leftrightarrow \tilde{\zeta}$ ,  $M \leftrightarrow -\widetilde{M}$ , and  $i \leftrightarrow -i$ . Note that, unlike in the new minimal case (5.2.13), the Killing spinor equation mixes the left- and right-handed spinors  $\zeta$  and  $\tilde{\zeta}$ , which leads to new backgrounds that cannot arise in new minimal supergravity.

The supersymmetric backgrounds that satisfy (5.2.39) were classified in [7, 63–65]. A simple background that highlights the qualitative differences between the old and new minimal cases is a round  $S^4$  of radius  $r$  with

$$M = \widetilde{M} = -\frac{3i}{r}, \quad b_\mu = 0. \quad (5.2.40)$$

Since  $S^4$  is not a complex manifold, it cannot arise as a background in new minimal supergravity. Moreover, the non-zero values for  $M, \widetilde{M}$  necessarily break the  $R$ -symmetry of the field theory, even if it was present in flat space. Finally, note that  $M, \widetilde{M}$  are not complex conjugates, and hence the background does not respect reflection positivity unless these fields decouple. This happens if the flat-space theory is superconformal, in which case it can be mapped to  $S^4$  by a conformal transformation that preserves unitarity. In a non-conformal theory, the violation of unitarity is necessary in order to avoid a no-go theorem that forbids unitary supersymmetric theories in de Sitter space, and hence reflection positive supersymmetric theories on compact spheres. The  $S^4$  background admits a squashing deformation that only preserves the isometry group  $SO(4) \subset SO(5)$ . Unfortunately, neither the round nor the squashed  $S^4$  appear to be amenable to localization calculations (see for instance the recent discussion in [45]).

## 5.3 Three-dimensional $\mathcal{N} = 2$ theories

### 5.3.1 Theories with an $R$ -symmetry on curved manifolds

Here we briefly sketch extensions of the results summarized in section 5.2 to three-dimensional theories with  $\mathcal{N} = 2$  supersymmetry. We only discuss theories with a  $U(1)_R$  symmetry. Now the  $\mathcal{R}$ -multiplet consists of the following operators [27],

$$\mathcal{R} = \left( j_\mu^{(R)}, S_{\mu\alpha}, T_{\mu\nu}, j_\mu^{(Z)}, J \right) . \quad (5.3.1)$$

Here  $j_\mu^{(R)}$  is the  $R$ -current,  $S_{\mu\alpha}$  is the supersymmetry current,  $T_{\mu\nu}$  is the stress tensor,  $j_\mu^{(Z)}$  is the central charge current, and  $J$  is a scalar operator. All operators other than  $J$  are conserved currents. The corresponding background supergravity fields constitute the analogue of new minimal supergravity in three dimensions (see for instance [66] and references therein),

$$\mathcal{H} = \left( A_\mu^{(R)}, \Psi_{\mu\alpha}, g_{\mu\nu}, C_\mu, H \right) . \quad (5.3.2)$$

Now the condition  $\delta_Q \Psi_{\mu\alpha} = 0$  leads to the following generalized Killing spinor equation for the allowed supersymmetric backgrounds [51, 67],

$$\left( \nabla_\mu - A_\mu^{(R)} \right) \zeta = -\frac{1}{2} H \gamma_\mu \zeta + \frac{i}{2} V_\mu \zeta - \frac{1}{2} \varepsilon_{\mu\nu\rho} V^\nu \gamma^\rho \zeta . \quad (5.3.3)$$

Here  $V^\mu = -i\varepsilon^{\mu\nu\rho} \partial_\nu C_\rho$  is the dual field strength of  $C_\mu$  in Euclidean signature. A solution  $\zeta$  to these equations exists if and only if the three-manifold  $\mathcal{M}$  admits a geometric structure known as a transversely holomorphic foliation (THF), and the metric is a compatible transversely Hermitian metric (see [8] for additional details). This structure is comprised of the following ingredients:

- 1.) A nowhere vanishing unit vector field  $\xi^\mu$ , which provides a local  $2 + 1$  decomposition of the manifold  $\mathcal{M}$ .
- 2.) An integrable complex structure  $J$  on the two-dimensional spaces transverse to  $\xi^\mu$ , such that  $J$  is invariant along  $\xi^\mu$ , i.e.  $\mathcal{L}_\xi J = 0$ .

In the compact case, such manifolds have been classified [68–70]. Topologically, they must be Seifert manifolds or  $T^2$  bundles over  $S^1$ . Compact hyperbolic three-manifolds are not allowed.

As is already clear from the definition, manifolds that carry a THF are very similar to complex manifolds. For instance, both admit complex  $(p, q)$  differential forms, a  $\bar{\partial}$ -operator, a corresponding Dolbeault cohomology, and holomorphic line bundles. As in four dimensions, these holomorphic line bundles correspond to supersymmetric configurations of background gauge fields for abelian flavor symmetries. Both a THF, and the holomorphic line bundles over it, generally come in infinite families labeled by a finite number of holomorphic moduli. As in the discussion around (5.2.30), these moduli (which are finite in number if  $\mathcal{M}$  is compact) correspond to certain  $\bar{\partial}$ -cohomology classes. See section 5 of [8] for an introduction to THFs and their moduli.

### 5.3.2 Constraining the partition function

In addition to the flat-space couplings and the choice of  $R$ -symmetry, the Lagrangian on  $\mathcal{M}$  now depends on a choice of THF, a transversely Hermitian metric, and holomorphic line bundles corresponding to background flavor gauge fields. Repeating the arguments in section 5.2.4 in this case, we find that (see [8] for a detailed discussion):

- The partition function  $Z_{\mathcal{M}}$  does not depend on the transversely Hermitian metric.
- $Z_{\mathcal{M}}$  is a locally holomorphic function of the THF moduli.
- The partition function depends holomorphically on line bundle moduli corresponding to background flavor gauge fields.

### 5.3.3 Example: round and squashed $S^3$

In  $\mathcal{N} = 2$  theories with a  $U(1)_R$  symmetry, the partition function on a round  $S^3$  is computable using supersymmetric localization techniques [71–73] (see also Chapter 6). This result has been generalized to a large variety of squashed spheres, see for instance [75–83]. These squashed spheres often have the feature that their metric contains arbitrary functions, in addition to various continuous parameters. Explicit localization computations of partition functions on these squashed spheres indicate that:

- The partition function only depends on the background geometry through a single complex parameter  $b$ , known as the squashing parameter. We will therefore denote the partition function by  $Z_{S_b^3}$ .
- Some deformations of the background fields do not affect  $Z_{S_b^3}$  (i.e. they do not change  $b$ ), even though the metric changes.

These observations can be understood using the results of [8] summarized in section 5.3.2 above.<sup>25</sup> It follows from the classification of [68–70] that the moduli space of THFs on three-manifolds diffeomorphic to  $S^3$  (i.e. squashed spheres) is one complex dimensional.<sup>26</sup> Therefore all squashed-sphere partition functions should only depend on one complex modulus, which can be identified with the squashing parameter  $b$ . It also shows that more complicated squashings will not lead to new partition functions.

Similarly, distinct squashed spheres that give rise to the same value of  $b$  correspond to the same choice of THF, but possibly different transversely Hermitian metrics, which do not affect the partition function.

---

<sup>25</sup> Some of these results (for special backgrounds and theories) were subsequently reproduced from a different point of view in [84]. We thank the authors for emphasizing their work to us.

<sup>26</sup> There is another, isolated branch of the moduli space, which consists of a single point, but it will not be important for us here (see [8] for additional details).

### 5.3.4 $F$ -maximization and correlation functions

The SUSY theories on  $S^3 \times S^1$  and  $S^3$  discussed in sections 5.2.5 and 5.3.3 above explicitly depend on a choice of  $U(1)_R$  symmetry, which affects their curvature couplings. In a superconformal theory, there is a distinguished choice of  $U(1)_R$  symmetry, which resides in the superconformal algebra. In four-dimensional  $\mathcal{N} = 1$  theories, it can be determined in flat space using anomalies and  $a$ -maximization [48, 85].

The analogous principle for three-dimensional  $\mathcal{N} = 2$  theories is  $F$ -maximization [72]. Since this is the subject of Chapter 8, we will only make a few remarks. Consider the partition function  $Z_{S^3}$  on a round  $S^3$ , together with a supersymmetric background gauge field for the conserved flavor current  $j_\mu$ . This partition function only depends on one holomorphic line bundle modulus  $u$ ,

$$Z_{S^3} = e^{-F(u)} , \quad F(u) = F(m + it) . \quad (5.3.4)$$

Here  $t \in \mathbb{R}$  controls the mixing of the flavor symmetry with the  $R$ -symmetry, while  $m$  is a real mass parameter associated with the flavor symmetry. The fact that the  $m$ - and  $t$ -dependence of  $F$  descends from a single holomorphic function of  $u$  was first observed in [72]. A general explanation was given in [53].

Derivatives of the free energy  $F$  with respect to  $t$  compute integrated correlation functions of  $j_\mu$  or its superpartners on  $S^3$ . In an SCFT, one-point functions should vanish, so that

$$\partial_t \text{Re}F \Big|_{\text{SCFT}} = 0 . \quad (5.3.5)$$

Surprisingly, the first derivative of the imaginary part  $\text{Im}F$  need not vanish, due to a global superconformal anomaly that can arise in three dimensions [39, 40].

Taking more derivatives with respect to  $t$  leads to higher-point correlation functions of  $j_\mu$ , for instance

$$\partial_t^2 \text{Re}F \Big|_{\text{SCFT}} = -\frac{\pi^2}{2} \tau . \quad (5.3.6)$$

Here  $\tau$  is the coefficient of the current two-point function at separated points in flat space. In a unitary theory  $\tau$  must be positive,

$$\langle j_\mu(x) j_\nu(0) \rangle = \frac{\tau}{16\pi^2} \left( \delta^{\mu\nu} \partial^2 - \partial^\mu \partial^\nu \right) \frac{1}{x^2} , \quad \tau > 0 . \quad (5.3.7)$$

The conditions in (5.3.5), (5.3.6), and (5.3.7) amount to the statement of  $F$ -maximization, which can be used to solve for the superconformal value  $t = t_*$  of the mixing parameter. Once this value has been found, we can use (5.3.6) to compute the value of  $\tau$  in the SCFT. Similarly, we can slightly squash the sphere away from the round point  $b = 1$  to extract the positive coefficient  $C_T > 0$  that appears in the stress-tensor two-point function at separated points [67],

$$C_T \sim \partial_b^2 \text{Re}F \Big|_{b=1} . \quad (5.3.8)$$

## Acknowledgments

I am grateful to C. Closset, G. Festuccia, Z. Komargodski, and N. Seiberg for collaboration on some of the work reviewed here. My work is supported by the Fundamental Laws Initiative at Harvard University, as well as DOE grant DE-SC0007870 and NSF grant PHY-1067976.

## References

- [1] V. Pestun and M. Zabzine, eds., *Localization techniques in quantum field theory*, vol. xx. Journal of Physics A, 2016. 1608.02952. <https://arxiv.org/src/1608.02952/anc/LocQFT.pdf>, <http://pestun.ihep.fr/pages/LocalizationReview/LocQFT.pdf>.
- [2] N. Seiberg, “Naturalness versus supersymmetric nonrenormalization theorems,” *Phys. Lett.* **B318** (1993) 469–475, [arXiv:hep-ph/9309335](https://arxiv.org/abs/hep-ph/9309335) [hep-ph].
- [3] K. A. Intriligator and N. Seiberg, “Lectures on supersymmetric gauge theories and electric-magnetic duality,” *Nucl. Phys. Proc. Suppl.* **45BC** (1996) 1–28, [arXiv:hep-th/9509066](https://arxiv.org/abs/hep-th/9509066) [hep-th].
- [4] E. Witten, “Constraints on Supersymmetry Breaking,” *Nucl. Phys.* **B202** (1982) 253.
- [5] E. Witten, “Topological Quantum Field Theory,” *Commun. Math. Phys.* **117** (1988) 353.
- [6] V. Pestun and M. Zabzine, “Introduction to localization in quantum field theory,” *Journal of Physics A* **xx** (2016) 000, 1608.02953.
- [7] G. Festuccia and N. Seiberg, “Rigid Supersymmetric Theories in Curved Superspace,” *JHEP* **06** (2011) 114, [arXiv:1105.0689](https://arxiv.org/abs/1105.0689) [hep-th].
- [8] C. Closset, T. T. Dumitrescu, G. Festuccia, and Z. Komargodski, “The Geometry of Supersymmetric Partition Functions,” *JHEP* **01** (2014) 124, [arXiv:1309.5876](https://arxiv.org/abs/1309.5876) [hep-th].
- [9] J. Bagger and J. Wess, *Supersymmetry and Supergravity*. Princeton University Press, 1992.
- [10] L. Alvarez-Gaume and E. Witten, “Gravitational Anomalies,” *Nucl. Phys.* **B234** (1984) 269.
- [11] E. Witten, “Quantum Field Theory and the Jones Polynomial,” *Commun. Math. Phys.* **121** (1989) 351–399.
- [12] H. Casini, M. Huerta, and R. C. Myers, “Towards a derivation of holographic entanglement entropy,” *JHEP* **05** (2011) 036, [arXiv:1102.0440](https://arxiv.org/abs/1102.0440) [hep-th].
- [13] S. Pufu, “The F-Theorem and F-Maximization,” *Journal of Physics A* **xx** (2016) 000, 1608.02960.
- [14] G. W. Moore and E. Witten, “Integration over the u plane in Donaldson theory,” *Adv. Theor. Math. Phys.* **1** (1997) 298–387, [arXiv:hep-th/9709193](https://arxiv.org/abs/hep-th/9709193) [hep-th].
- [15] Y. Tachikawa, “A brief review of the 2d/4d correspondences,” *Journal of Physics A* **xx** (2016) 000, 1608.02964.
- [16] E. Witten, “Supersymmetric Yang-Mills theory on a four manifold,” *J. Math. Phys.* **35** (1994) 5101–5135, [arXiv:hep-th/9403195](https://arxiv.org/abs/hep-th/9403195) [hep-th].
- [17] A. Johansen, “Twisting of  $N = 1$  SUSY gauge theories and heterotic topological theories,” *Int. J. Mod. Phys.* **A10** (1995) 4325–4358, [arXiv:hep-th/9403017](https://arxiv.org/abs/hep-th/9403017) [hep-th].
- [18] A. Karlhede and M. Rocek, “Topological Quantum Field Theory and  $N = 2$  Conformal Supergravity,” *Phys. Lett.* **B212** (1988) 51.

- [19] N. A. Nekrasov, “Seiberg-Witten prepotential from instanton counting,” *Adv. Theor. Math. Phys.* **7** (2003) no. 5, 831–864, [arXiv:hep-th/0206161 \[hep-th\]](#).
- [20] N. Nekrasov and A. Okounkov, “Seiberg-Witten theory and random partitions,” *Prog. Math.* **244** (2006) 525–596, [arXiv:hep-th/0306238 \[hep-th\]](#).
- [21] V. Pestun, “Localization of gauge theory on a four-sphere and supersymmetric Wilson loops,” *Commun. Math. Phys.* **313** (2012) 71–129, [arXiv:0712.2824 \[hep-th\]](#).
- [22] V. Pestun, “Localization for  $\mathcal{N} = 2$  Supersymmetric Gauge Theories in Four Dimensions,” in *New Dualities of Supersymmetric Gauge Theories*, J. Teschner, ed., pp. 159–194. 2016. [arXiv:1412.7134 \[hep-th\]](#).
- [23] K. Hosomichi, “ $\mathcal{N} = 2$  SUSY gauge theories on  $S^4$ ,” *Journal of Physics A* **xx** (2016) 000, [1608.02962](#).
- [24] C. Cordova, T. T. Dumitrescu, and K. Intriligator, “Deformations of Superconformal Theories,” [arXiv:1602.01217 \[hep-th\]](#).
- [25] L. Rastelli and S. Razamat, “The supersymmetric index in four dimensions,” *Journal of Physics A* **xx** (2016) 000, [1608.02965](#).
- [26] Z. Komargodski and N. Seiberg, “Comments on Supercurrent Multiplets, Supersymmetric Field Theories and Supergravity,” *JHEP* **07** (2010) 017, [arXiv:1002.2228 \[hep-th\]](#).
- [27] T. T. Dumitrescu and N. Seiberg, “Supercurrents and Brane Currents in Diverse Dimensions,” *JHEP* **07** (2011) 095, [arXiv:1106.0031 \[hep-th\]](#).
- [28] S. J. Gates, M. T. Grisaru, M. Rocek, and W. Siegel, “Superspace Or One Thousand and One Lessons in Supersymmetry,” *Front. Phys.* **58** (1983) 1–548, [arXiv:hep-th/0108200 \[hep-th\]](#).
- [29] S. Ferrara and B. Zumino, “Transformation Properties of the Supercurrent,” *Nucl. Phys.* **B87** (1975) 207.
- [30] Z. Komargodski and N. Seiberg, “Comments on the Fayet-Iliopoulos Term in Field Theory and Supergravity,” *JHEP* **06** (2009) 007, [arXiv:0904.1159 \[hep-th\]](#).
- [31] T. T. Dumitrescu, Z. Komargodski, and M. Sudano, “Global Symmetries and D-Terms in Supersymmetric Field Theories,” *JHEP* **11** (2010) 052, [arXiv:1007.5352 \[hep-th\]](#).
- [32] M. Kaku, P. K. Townsend, and P. van Nieuwenhuizen, “Properties of Conformal Supergravity,” *Phys. Rev.* **D17** (1978) 3179.
- [33] K. S. Stelle and P. C. West, “Minimal Auxiliary Fields for Supergravity,” *Phys. Lett.* **B74** (1978) 330–332.
- [34] S. Ferrara and P. van Nieuwenhuizen, “The Auxiliary Fields of Supergravity,” *Phys. Lett.* **B74** (1978) 333.
- [35] M. F. Sohnius and P. C. West, “An Alternative Minimal Off-Shell Version of  $N=1$  Supergravity,” *Phys. Lett.* **B105** (1981) 353–357.
- [36] M. Sohnius and P. C. West, “The Tensor Calculus and Matter Coupling of the Alternative Minimal Auxiliary Field Formulation of  $N = 1$  Supergravity,” *Nucl. Phys.* **B198** (1982) 493–507.
- [37] D. Z. Freedman and A. Van Proeyen, *Supergravity*. Cambridge University Press, 2012.
- [38] S. Ferrara and S. Sabharwal, “Structure of New Minimal Supergravity,” *Annals Phys.* **189** (1989) 318–351.
- [39] C. Closset, T. T. Dumitrescu, G. Festuccia, Z. Komargodski, and N. Seiberg, “Contact Terms, Unitarity, and F-Maximization in Three-Dimensional Superconformal Theories,” *JHEP* **10** (2012) 053, [arXiv:1205.4142 \[hep-th\]](#).

- [40] C. Closset, T. T. Dumitrescu, G. Festuccia, Z. Komargodski, and N. Seiberg, “Comments on Chern-Simons Contact Terms in Three Dimensions,” *JHEP* **09** (2012) 091, [arXiv:1206.5218 \[hep-th\]](#).
- [41] E. Gerchkovitz, J. Gomis, and Z. Komargodski, “Sphere Partition Functions and the Zamolodchikov Metric,” *JHEP* **11** (2014) 001, [arXiv:1405.7271 \[hep-th\]](#).
- [42] L. Di Pietro and Z. Komargodski, “Cardy formulae for SUSY theories in  $d = 4$  and  $d = 6$ ,” *JHEP* **12** (2014) 031, [arXiv:1407.6061 \[hep-th\]](#).
- [43] J. Gomis and N. Ishtiaque, “Kähler potential and ambiguities in 4d  $\mathcal{N} = 2$  SCFTs,” *JHEP* **04** (2015) 169, [arXiv:1409.5325 \[hep-th\]](#).
- [44] B. Assel, D. Cassani, and D. Martelli, “Supersymmetric counterterms from new minimal supergravity,” *JHEP* **11** (2014) 135, [arXiv:1410.6487 \[hep-th\]](#).
- [45] G. Knodel, J. T. Liu, and L. A. Pando Zayas, “On  $\mathcal{N}=1$  partition functions without R-symmetry,” *JHEP* **03** (2015) 132, [arXiv:1412.4804 \[hep-th\]](#).
- [46] B. Assel, D. Cassani, L. Di Pietro, Z. Komargodski, J. Lorenzen, and D. Martelli, “The Casimir Energy in Curved Space and its Supersymmetric Counterpart,” *JHEP* **07** (2015) 043, [arXiv:1503.05537 \[hep-th\]](#).
- [47] J. Gomis, P.-S. Hsin, Z. Komargodski, A. Schwimmer, N. Seiberg, and S. Theisen, “Anomalies, Conformal Manifolds, and Spheres,” *JHEP* **03** (2016) 022, [arXiv:1509.08511 \[hep-th\]](#).
- [48] D. Anselmi, D. Z. Freedman, M. T. Grisaru, and A. A. Johansen, “Nonperturbative formulas for central functions of supersymmetric gauge theories,” *Nucl. Phys.* **B526** (1998) 543–571, [arXiv:hep-th/9708042 \[hep-th\]](#).
- [49] D. Cassani and D. Martelli, “Supersymmetry on curved spaces and superconformal anomalies,” *JHEP* **10** (2013) 025, [arXiv:1307.6567 \[hep-th\]](#).
- [50] D. Morrison, “Gromov-Witten invariants and localization,” *Journal of Physics A* (2016) , 1608.02956.
- [51] C. Klare, A. Tomasiello, and A. Zaffaroni, “Supersymmetry on Curved Spaces and Holography,” *JHEP* **08** (2012) 061, [arXiv:1205.1062 \[hep-th\]](#).
- [52] T. T. Dumitrescu, G. Festuccia, and N. Seiberg, “Exploring Curved Superspace,” *JHEP* **08** (2012) 141, [arXiv:1205.1115 \[hep-th\]](#).
- [53] C. Closset, T. T. Dumitrescu, G. Festuccia, and Z. Komargodski, “From Rigid Supersymmetry to Twisted Holomorphic Theories,” *Phys. Rev.* **D90** (2014) no. 8, 085006, [arXiv:1407.2598 \[hep-th\]](#).
- [54] K. Kodaira, *Complex Manifolds and Deformation of Complex Structures*. Springer, 1986.
- [55] N. Seiberg, “Electric - magnetic duality in supersymmetric nonAbelian gauge theories,” *Nucl. Phys.* **B435** (1995) 129–146, [arXiv:hep-th/9411149 \[hep-th\]](#).
- [56] K. Kodaira, “Complex structures on  $S^1 \times S^3$ ,” *Proceedings of the National Academy of Sciences* **55** (1966) no. 2, 240–243.
- [57] B. Assel, D. Cassani, and D. Martelli, “Localization on Hopf surfaces,” *JHEP* **08** (2014) 123, [arXiv:1405.5144 \[hep-th\]](#).
- [58] T. Nishioka and I. Yaakov, “Generalized indices for  $\mathcal{N} = 1$  theories in four-dimensions,” *JHEP* **12** (2014) 150, [arXiv:1407.8520 \[hep-th\]](#).
- [59] C. Romelsberger, “Counting chiral primaries in  $\mathcal{N} = 1$ ,  $d=4$  superconformal field theories,” *Nucl. Phys.* **B747** (2006) 329–353, [arXiv:hep-th/0510060 \[hep-th\]](#).

- [60] F. A. Dolan and H. Osborn, “Applications of the Superconformal Index for Protected Operators and q-Hypergeometric Identities to N=1 Dual Theories,” *Nucl. Phys.* **B818** (2009) 137–178, [arXiv:0801.4947 \[hep-th\]](#).
- [61] J. Kinney, J. M. Maldacena, S. Minwalla, and S. Raju, “An Index for 4 dimensional super conformal theories,” *Commun. Math. Phys.* **275** (2007) 209–254, [arXiv:hep-th/0510251 \[hep-th\]](#).
- [62] D. Sen, “Supersymmetry in the Space-time  $R \times S^3$ ,” *Nucl. Phys.* **B284** (1987) 201.
- [63] H. Samtleben and D. Tsimpis, “Rigid supersymmetric theories in 4d Riemannian space,” *JHEP* **05** (2012) 132, [arXiv:1203.3420 \[hep-th\]](#).
- [64] J. T. Liu, L. A. Pando Zayas, and D. Reichmann, “Rigid Supersymmetric Backgrounds of Minimal Off-Shell Supergravity,” *JHEP* **10** (2012) 034, [arXiv:1207.2785 \[hep-th\]](#).
- [65] T. T. Dumitrescu and G. Festuccia, “Exploring Curved Superspace (II),” *JHEP* **01** (2013) 072, [arXiv:1209.5408 \[hep-th\]](#).
- [66] S. M. Kuzenko, U. Lindstrom, M. Rocek, I. Sachs, and G. Tartaglino-Mazzucchelli, “Three-dimensional  $\mathcal{N} = 2$  supergravity theories: From superspace to components,” *Phys. Rev.* **D89** (2014) no. 8, 085028, [arXiv:1312.4267 \[hep-th\]](#).
- [67] C. Closset, T. T. Dumitrescu, G. Festuccia, and Z. Komargodski, “Supersymmetric Field Theories on Three-Manifolds,” *JHEP* **05** (2013) 017, [arXiv:1212.3388 \[hep-th\]](#).
- [68] M. Brunella and É. Ghys, “Umbilical foliations and transversely holomorphic flows,” *J. Differential Geom* **41** (1995) no. 1, 1–19.
- [69] M. Brunella, “On transversely holomorphic flows I,” *Inventiones mathematicae* **126** (1996) no. 2, 265–279.
- [70] É. Ghys, “On transversely holomorphic flows II,” *Inventiones mathematicae* **126** (1996) no. 2, 281–286.
- [71] A. Kapustin, B. Willett, and I. Yaakov, “Exact Results for Wilson Loops in Superconformal Chern-Simons Theories with Matter,” *JHEP* **03** (2010) 089, [arXiv:0909.4559 \[hep-th\]](#).
- [72] D. L. Jafferis, “The Exact Superconformal R-Symmetry Extremizes Z,” *JHEP* **05** (2012) 159, [arXiv:1012.3210 \[hep-th\]](#).
- [73] N. Hama, K. Hosomichi, and S. Lee, “Notes on SUSY Gauge Theories on Three-Sphere,” *JHEP* **03** (2011) 127, [arXiv:1012.3512 \[hep-th\]](#).
- [74] B. Willett, “Localization on three-dimensional manifolds,” *Journal of Physics A* **xx** (2016) 000, [1608.02958](#).
- [75] N. Hama, K. Hosomichi, and S. Lee, “SUSY Gauge Theories on Squashed Three-Spheres,” *JHEP* **05** (2011) 014, [arXiv:1102.4716 \[hep-th\]](#).
- [76] Y. Imamura, “Relation between the 4d superconformal index and the  $S^3$  partition function,” *JHEP* **09** (2011) 133, [arXiv:1104.4482 \[hep-th\]](#).
- [77] Y. Imamura and D. Yokoyama, “N=2 supersymmetric theories on squashed three-sphere,” *Phys. Rev.* **D85** (2012) 025015, [arXiv:1109.4734 \[hep-th\]](#).
- [78] D. Martelli, A. Passias, and J. Sparks, “The gravity dual of supersymmetric gauge theories on a squashed three-sphere,” *Nucl. Phys.* **B864** (2012) 840–868, [arXiv:1110.6400 \[hep-th\]](#).
- [79] T. Nishioka and I. Yaakov, “Supersymmetric Renyi Entropy,” *JHEP* **10** (2013) 155, [arXiv:1306.2958 \[hep-th\]](#).
- [80] D. Martelli and A. Passias, “The gravity dual of supersymmetric gauge theories on a two-parameter deformed three-sphere,” *Nucl. Phys.* **B877** (2013) 51–72, [arXiv:1306.3893 \[hep-th\]](#).

- [81] L. F. Alday, D. Martelli, P. Richmond, and J. Sparks, “Localization on Three-Manifolds,” *JHEP* **10** (2013) 095, [arXiv:1307.6848 \[hep-th\]](#).
- [82] J. Nian, “Localization of Supersymmetric Chern-Simons-Matter Theory on a Squashed  $S^3$  with  $SU(2) \times U(1)$  Isometry,” *JHEP* **07** (2014) 126, [arXiv:1309.3266 \[hep-th\]](#).
- [83] A. Tanaka, “Localization on round sphere revisited,” *JHEP* **11** (2013) 103, [arXiv:1309.4992 \[hep-th\]](#).
- [84] C. Imbimbo and D. Rosa, “Topological anomalies for Seifert 3-manifolds,” *JHEP* **07** (2015) 068, [arXiv:1411.6635 \[hep-th\]](#).
- [85] K. A. Intriligator and B. Wecht, “The Exact superconformal R symmetry maximizes a,” *Nucl. Phys.* **B667** (2003) 183–200, [arXiv:hep-th/0304128 \[hep-th\]](#).

# Chapter 6

## Localization on three-dimensional manifolds

Brian Willett

*KITP/UC Santa Barbara*  
bwillett@kitp.ucsb.edu

### Abstract

In this review article we describe the localization of three dimensional  $\mathcal{N} = 2$  supersymmetric theories on compact manifolds, including the squashed sphere,  $S_b^3$ , the lens space,  $S_b^3/\mathbb{Z}_p$ , and  $S^2 \times S^1$ . We describe how to write supersymmetric actions on these spaces, and then compute the partition functions and other supersymmetric observables by employing the localization argument. We briefly survey some applications of these computations.

### Contents

|            |                                                               |            |
|------------|---------------------------------------------------------------|------------|
| <b>6.1</b> | <b>Introduction</b>                                           | <b>204</b> |
| 6.1.1      | Review of $3d \mathcal{N} = 2$ Field Theories                 | 205        |
| <b>6.2</b> | <b>Supersymmetry on the 3-sphere</b>                          | <b>209</b> |
| 6.2.1      | Round sphere                                                  | 210        |
| 6.2.2      | Supersymmetry on general 3-manifolds                          | 214        |
| 6.2.3      | Squashed 3-sphere                                             | 217        |
| <b>6.3</b> | <b>Localization of the partition function on the 3-sphere</b> | <b>220</b> |
| 6.3.1      | Round $S^3$                                                   | 222        |
| 6.3.2      | Squashed $S^3$                                                | 228        |
| 6.3.3      | Operator insertions                                           | 233        |
| <b>6.4</b> | <b>Lens spaces</b>                                            | <b>235</b> |
| 6.4.1      | Localization on $L(p, 1)$                                     | 235        |
| <b>6.5</b> | <b><math>S^2 \times S^1</math> partition function</b>         | <b>239</b> |

|                   |                                                                            |            |
|-------------------|----------------------------------------------------------------------------|------------|
| 6.5.1             | Supersymmetric backgrounds . . . . .                                       | 239        |
| 6.5.2             | Localization on $S^2 \times S^1$ . . . . .                                 | 241        |
| 6.5.3             | Loop operators . . . . .                                                   | 244        |
| 6.5.4             | Superconformal index . . . . .                                             | 245        |
| <b>6.6</b>        | <b>Applications . . . . .</b>                                              | <b>247</b> |
| 6.6.1             | Applications discussed in accompanying articles . . . . .                  | 248        |
| 6.6.2             | Dualities . . . . .                                                        | 251        |
| 6.6.3             | Factorization, holomorphic blocks, and Higgs branch localization . . . . . | 255        |
| 6.6.4             | Limits of partition functions . . . . .                                    | 259        |
| <b>References</b> | <b>. . . . .</b>                                                           | <b>265</b> |

## 6.1 Introduction

Supersymmetry provides a variety of tools for analyzing strongly coupled quantum field theories. An important example is supersymmetric localization, which is a powerful method for computing exact results in supersymmetric quantum field theories. In the 90's this idea was used to great effect in computing observables in certain topologically twisted theories (*e.g.*, [2]). More recently, starting with the work [3], there has been a wave of exact results for non-topological observables on compact manifolds for theories in various dimensions and with various amounts of supersymmetry. This has led to exciting progress and new insights about these theories, as described in the accompanying articles in this issue.

In this article we will study these observables in the context of three dimensional  $\mathcal{N} = 2$  supersymmetric theories. This is a rich class of theories, which exhibit many interesting properties, and an enormous amount of work (which we can not hope to summarize here) has focused on these models. They provide an ideal setting for investigation, being rich enough to exhibit many non-trivial phenomena, such as confinement, whose study may teach us general lessons about quantum field theories, while also enjoying enough symmetry and rigid structure that many of their properties can be deduced analytically. In particular, as we will describe in this article, this structure allows the exact computation of the partition function and other supersymmetric observables on a variety of compact curved manifolds. We will describe how localization reduces the path integral to a finite dimensional matrix model, which renders it eminently computable, and thus allows one to obtain exact results in strongly interacting quantum field theories. These results have led to a deeper understanding of these models, and have had many interesting applications, some of which we will briefly survey.

The outline of this article is as follows. In the remainder of the introduction, we review some basic properties of  $3d \mathcal{N} = 2$  theories in flat space. Then in section 2 we will describe how to write supersymmetric actions on curved backgrounds, starting with the round  $S^3$  and then moving to more general backgrounds using a supergravity analysis. In section 3 we describe the computation of the partition functions on round and squashed 3-spheres, using the localization argument. In section 4 we discuss supersymmetric theories on lens spaces, and compute their partition functions. In section 5 we discuss the partition function

on  $S^2 \times S^1$ , and its relation to the superconformal index. Finally in section 6 we briefly survey some applications of these partition function computations. This article is meant as an introduction and overview of some of the work that has been done on  $3d \mathcal{N} = 2$  localization, and as such, most of the content will be familiar to the experts.

### 6.1.1 Review of $3d \mathcal{N} = 2$ Field Theories

The theories we will consider in this article are three dimensional theories with  $\mathcal{N} = 2$  supersymmetry, *i.e.*, four real supercharges. This is the same amount of supersymmetry as in  $4d \mathcal{N} = 1$  theories, and many properties of the  $3d$  superalgebra can be deduced by reduction from four dimensions. Let us first describe some basic properties of these theories in flat three dimensional spacetime, in preparation for studying them on curved backgrounds in the next section. For more background on theories with  $\mathcal{N} = 2$  supersymmetry, see, *e.g.*, [4].

The  $\mathcal{N} = 2$  algebra contains supercharges  $\mathcal{Q}_\alpha$  and  $\mathcal{Q}_\alpha^\dagger$ , which satisfy the algebra:<sup>1</sup>

$$\{\mathcal{Q}_\alpha, \mathcal{Q}_\beta\} = \{\mathcal{Q}_\alpha^\dagger, \mathcal{Q}_\beta^\dagger\} = 0, \quad \{\mathcal{Q}_\alpha, \mathcal{Q}_\beta^\dagger\} = 2\gamma_{\alpha\beta}^\mu P_\mu + 2i\epsilon_{\alpha\beta} Z \quad (6.1.1)$$

Here  $P_\mu$  is the momentum,  $Z$  is the real central charge, and  $\gamma^\mu$  are the Pauli matrices.

We can build Lagrangians for field theories with  $\mathcal{N} = 2$  supersymmetry using two basic types of field multiplets: chiral multiplets and vector multiplets. These can be defined using a superspace formalism obtained by dimensionally reducing the  $4d \mathcal{N} = 1$  superspace formalism. Chiral multiplets  $\Phi$  satisfy  $\bar{\mathcal{D}}_\alpha \Phi = 0$ , and consist of the following component fields:

$$\text{complex scalar } \phi, \quad \text{complex spinor } \psi, \quad \text{auxiliary complex scalar } F \quad (6.1.2)$$

The action of supersymmetry on these fields is summarized by introducing an operator  $\delta = \zeta \mathcal{Q} + \tilde{\zeta} \mathcal{Q}^\dagger$ , labeled by constant spinors  $\zeta, \tilde{\zeta}$ .<sup>2</sup>

$$\begin{aligned} \delta\phi &= \sqrt{2}\zeta\psi \\ \delta\psi &= \sqrt{2}\zeta F - \sqrt{2}i\gamma^\mu\tilde{\zeta}\partial_\mu\phi \\ \delta F &= -\sqrt{2}i\tilde{\zeta}\gamma^\mu\partial_\mu\psi \end{aligned} \quad (6.1.3)$$

One can check that this gives a representation of the algebra (6.1.1) with  $Z = 0$ .

Vector multiplets satisfy  $V = V^\dagger$ , and have a gauge symmetry  $V \sim V + \Lambda + \Lambda^\dagger$ , for  $\Lambda$  a chiral multiplet. In Wess-Zumino gauge, they consist of fields:

$$\text{vector } A_\mu, \quad \text{real scalar } \sigma, \quad \text{complex spinor } \lambda, \quad \text{auxiliary real scalar } D \quad (6.1.4)$$

which all lie in the adjoint representation of the gauge group. They have the following transformation laws:<sup>3</sup>

<sup>1</sup>Throughout this article we will work in Euclidean signature.

<sup>2</sup>In this article, our notations and spinor conventions will mostly follow [5].

<sup>3</sup>Here  $\tilde{\lambda}$  denotes the field that would be Hermitian conjugate to  $\lambda$  in Lorentzian signature; here they are treated as independent fields.

$$\begin{aligned}
\delta A_\mu &= -i(\zeta\gamma_\mu\tilde{\lambda} + \tilde{\zeta}\gamma_\mu\lambda), \\
\delta\sigma &= -\zeta\tilde{\lambda} + \tilde{\zeta}\lambda, \\
\delta\lambda &= (iD - \frac{i}{2}\epsilon^{\mu\nu\rho}\gamma_\rho F_{\mu\nu} - i\gamma^\mu D_\mu\sigma)\zeta, \\
\delta\tilde{\lambda} &= (-iD - \frac{i}{2}\epsilon^{\mu\nu\rho}\gamma_\rho F_{\mu\nu} + i\gamma^\mu D_\mu\sigma)\tilde{\zeta}, \\
\delta D &= \zeta\gamma^\mu D_\mu\tilde{\lambda} - \tilde{\zeta}\gamma^\mu D_\mu\lambda - [\zeta\tilde{\lambda}, \sigma] - [\tilde{\zeta}\lambda, \sigma]
\end{aligned} \tag{6.1.5}$$

Supersymmetry transformations take one out of Wess-Zumino gauge, so one must supplement them by a suitable gauge transformation. This also modifies the supersymmetry transformations of the chiral by terms involving the gauge multiplet fields:

$$\begin{aligned}
\delta\phi &= \sqrt{2}\zeta\psi, \\
\delta\psi &= \sqrt{2}\zeta F - \sqrt{2}i\gamma^\mu\tilde{\zeta}D_\mu\phi + \sqrt{2}i\sigma\phi\tilde{\zeta}, \\
\delta F &= -\sqrt{2}i\tilde{\zeta}\gamma^\mu D_\mu\psi - \sqrt{2}i\sigma\tilde{\zeta}\psi + 2i\tilde{\zeta}\tilde{\lambda}\phi,
\end{aligned} \tag{6.1.6}$$

The action in flat space can be written as a sum of  $D$ -term and  $F$ -term contributions:

$$S = \int d^3x \left( \int d^4\theta K(\Phi, \Phi^\dagger, V) + \int d^2\theta W(\Phi) + c.c. \right) \tag{6.1.7}$$

where  $K$  is the Kahler potential and  $W$  is the superpotential. The standard choice for kinetic term of the chiral multiplet, which we will always take, is:

$$K(\Phi, \Phi^\dagger, V) = \Phi^\dagger e^V \Phi \tag{6.1.8}$$

which gives the following Lagrangian when expanded in component fields:

$$\mathcal{L}_{chi} = D_\mu\tilde{\phi}D^\mu\phi + \tilde{\phi}(\sigma^2 + D)\phi - i\tilde{\psi}\gamma^\mu D_\mu\psi - i\tilde{\psi}\sigma\psi + \sqrt{2}i(\tilde{\phi}\lambda\psi + \tilde{\psi}\tilde{\lambda}\phi) - \tilde{F}F \tag{6.1.9}$$

For the vector multiplet, there are two choices for the kinetic term. First we can consider a supersymmetric extension of the Chern-Simons (CS) kinetic term:

$$\mathcal{L}_{CS} = \frac{i}{4\pi}\text{Tr}_{CS}(e^{\mu\nu\rho}(A_\mu\partial_\nu A_\rho + \frac{2i}{3}A_\mu A_\nu A_\rho) + 2iD\sigma + 2\tilde{\lambda}\lambda) \tag{6.1.10}$$

Here invariance under large gauge transformations imposes a quantization law for the trace function  $Tr_{CS}$ . For example, if the gauge group is  $U(N)$  then  $Tr_{CS} = k\text{Tr}_F$ , with  $\text{Tr}_F$  the trace in the fundamental representation and  $k$  an integer.

These kinetic terms for the matter and gauge fields preserve scale invariance classically. It is a non-trivial consequence of  $\mathcal{N} = 2$  supersymmetry that a theory defined by the above chiral multiplet kinetic term and with a Chern-Simons kinetic term for the gauge multiplet

preserves scale invariance on the quantum level [6]. However, for a generic theory the chiral fields will undergo wave function renormalization.

Another choice of kinetic term for the gauge field is the Yang-Mills Lagrangian:

$$\mathcal{L}_{YM} = \frac{1}{g^2} \text{Tr} \left( \frac{1}{4} F^{\mu\nu} F_{\mu\nu} + \frac{1}{2} D^\mu \sigma D_\mu \sigma - i \tilde{\lambda} \gamma^\mu D_\mu \lambda + i \tilde{\lambda} [\sigma, \lambda] - \frac{1}{2} D^2 \right) \quad (6.1.11)$$

The gauge coupling  $g^2$  has dimensions of mass, and so this term breaks scale invariance.

We can also consider superpotential terms for the chiral multiplets, defined by a holomorphic function  $W(\Phi_i)$ :

$$\mathcal{L}_W = \int d^2\theta W(\Phi_i) + c.c. = \frac{\partial W}{\partial \Phi_i}(\phi_i) F_i + \frac{\partial^2 W}{\partial \Phi_i \partial \Phi_j}(\phi_i) \psi_i \psi_j + c.c. \quad (6.1.12)$$

An example is a complex mass term: given two chiral fields  $X$  and  $Y$ , a superpotential term  $W = mXY$  leads to a mass  $m$  for the fields in both chiral multiplets, and they can be integrated out at energies below  $m$ . A quartic superpotential leads to a sextic scalar potential, and is classically marginal. The superpotential must be invariant under any gauge symmetry of the theory, and it restricts the flavor symmetry.

#### *Real mass and FI parameters*

In addition to dynamical vector multiplets, one can turn on background vector multiplets which couple to the flavor symmetries of the theories. We should think of these background fields as classical, taking fixed values which appear as parameters in the action. In order to preserve supersymmetry, these background fields must be in configurations which would be acted on trivially by the supersymmetry transformations if these were dynamical fields. These are often called ‘‘BPS configurations.’’ One can check that this imposes  $\sigma$  be constant, and all other vector multiplet fields vanish. For a chiral multiplet with charge  $q$  under a global symmetry, if we couple a background gauge field to this symmetry and set  $\sigma = m$ , one finds additional terms in the action:

$$\mathcal{L}_{chi} = \dots + q^2 m^2 \tilde{\phi} \phi - i q m \tilde{\psi} \psi \quad (6.1.13)$$

corresponding to a mass  $qm$  for the both the bosonic and fermionic excitations. This also modifies the supersymmetry transformations giving:

$$\delta \psi = \dots + \sqrt{2} i q m \phi \tilde{\zeta}, \quad \delta F = \dots - \sqrt{2} i q m \tilde{\zeta} \psi \quad (6.1.14)$$

Turning on a real mass parameter shifts the central charge  $Z \rightarrow Z + m\mathcal{F}$ , where  $\mathcal{F}$  is the corresponding flavor symmetry charge, and so modifies the commutation relations through (6.1.1).

If the gauge group is  $U(1)$ , then the field strength  $F_{\mu\nu}$  can be used to define a conserved current:

$$J_{top}^\mu = \star F^\mu \quad (6.1.15)$$

This is conserved as a result of the Bianchi identity for  $F_{\mu\nu}$ . The charged objects of this symmetry are monopole operators, and the charged excitations are vortices (see, *e.g.*, [4]). To gauge this symmetry with a vector multiplet  $\mathcal{V}'$ , we write the supersymmetric completion of the linear coupling  $A'_\mu J_{top}^\mu = \epsilon^{\mu\nu\rho} A'_\mu \partial_\nu A_\rho$ , which is an off-diagonal Chern-Simons term:

$$\frac{i}{2\pi} (\epsilon^{\mu\nu\rho} A'_\mu \partial_\nu A'_\rho + iD\sigma' + i\sigma D' + \tilde{\lambda}\lambda' + \tilde{\lambda}'\lambda) \quad (6.1.16)$$

To turn on a real mass for this symmetry, we can take this to be a background vector multiplet with a constant value for the scalar  $\sigma' = \zeta$ , which gives rise to a Fayet-Iliopoulos (FI) term:

$$\mathcal{L}_{FI} = -\frac{1}{2\pi} \zeta D \quad (6.1.17)$$

More generally, we can allow an FI parameter for any  $U(1)$  factor of  $G$ . Namely, if we let  $\lambda_a$  run over a basis of Weyl-invariant weights of  $G$ , the most general FI term is given by:

$$\mathcal{L}_{FI} = -\frac{1}{2\pi} \sum_a \zeta^a \lambda_a(D) \quad (6.1.18)$$

#### *$U(1)_R$ symmetry and superconformal symmetry*

The  $\mathcal{N} = 2$  algebra includes a  $U(1)$  symmetry rotating the supercharges  $\mathcal{Q} \rightarrow e^{i\alpha} \mathcal{Q}$  and  $\mathcal{Q}^\dagger \rightarrow e^{-i\alpha} \mathcal{Q}^\dagger$ . For a free theory, the  $U(1)_R$  symmetry acts on the fields as:

$$\phi \rightarrow e^{i\alpha/2} \phi, \quad \psi \rightarrow e^{-i\alpha/2} \psi, \quad F \rightarrow e^{-3i\alpha/2} F, \quad \lambda \rightarrow e^{i\alpha} \lambda \quad (6.1.19)$$

We will refer to this as the  $UV$  R-symmetry, as it corresponds the free UV fixed point of a  $3d$  gauge theory. In general, we can define a new  $U(1)_R$  symmetry by adding to it some  $U(1)$  flavor symmetry, *i.e.*, a symmetry which commutes with the superalgebra (and so acts on all fields in a given multiplet identically). This does not affect the action of the symmetry on the supercharges, but shifts the R-charges of all chiral multiplet fields charged under the symmetry. When we consider a generic interacting Lagrangian, our choices of  $U(1)_R$  symmetry may be limited if some symmetries are broken, or the R-symmetry may be explicitly broken, *e.g.*, by a superpotential.

As mentioned above, one can construct Chern-Simons-matter theories which are exactly conformal. More generally, since the Yang-Mills term is relevant, non-conformal gauge theories in three dimensions will typically flow to non-trivial superconformal field theories. Such theories are invariant under a larger  $\mathfrak{osp}(2|2, 2)$  superalgebra, whose bosonic subalgebra includes the  $\mathfrak{so}(3, 1)$  conformal algebra and  $\mathfrak{u}(1)$  R-symmetry. In a superconformal theory, there is a privileged choice of R-symmetry, determined by the condition that its current sits in the same superconformal multiplet as the traceless stress-energy tensor. In a generic theory, the superconformal R-charges of the basic fields are irrational numbers, and are difficult to compute a priori. We will see in section 6 that the 3-sphere partition function gives a tool for computing these charges directly.

## Extended Supersymmetry

We can also consider theories which have additional supersymmetry, namely,  $\mathcal{N}$  real spinor supercharges,  $\mathcal{Q}_\alpha^a$ ,  $a = 1, \dots, \mathcal{N}$  for  $\mathcal{N} > 2$ . For our purposes such theories can always be treated as  $\mathcal{N} = 2$  theories by picking a distinguished  $\mathcal{N} = 2$  subalgebra and treating them as  $\mathcal{N} = 2$  theories with a specialized field content and action. However, theories with  $\mathcal{N} \geq 3$  supersymmetry enjoy more robust non-renormalization properties. For example, their superconformal  $U(1)$  R-symmetry is the UV R-symmetry, a consequence of the fact that the  $U(1)$  R-symmetry sits inside a larger non-abelian group,  $SO(\mathcal{N})$ , and so cannot be mixed with a  $U(1)$  flavor symmetry.<sup>4</sup>

The most important example will be  $\mathcal{N} = 4$  supersymmetry, which can be obtained by reduction from  $4d$   $\mathcal{N} = 2$  supersymmetry. Here the field content can be organized into hypermultiplets, which consists of a pair of chiral multiplets,  $(q, \tilde{q})$ , in conjugate representations of the gauge and flavor symmetry groups, and vector multiplets, which consist of a  $\mathcal{N} = 2$  vector multiplet and an adjoint chiral multiplet  $\Phi$ . The actions are constrained to have the canonical kinetic terms, and a superpotential coupling:

$$W = \tilde{q}\Phi q \tag{6.1.20}$$

With both a Yang-Mills and Chern-Simons term, one can only realize  $\mathcal{N} \leq 3$  supersymmetry. However, with only a Chern-Simons term, one can find theories with large amounts of supersymmetry, such as the  $\mathcal{N} \geq 4$  theories of Gaiotto-Witten [8], and the  $\mathcal{N} \geq 5$  ABJ(M) theories [9, 10] and related  $\mathcal{N} = 8$  BLG theories [11, 12].

## 6.2 Supersymmetry on the 3-sphere

Many interesting results about three dimensional theories with  $\mathcal{N} = 2$  and higher supersymmetry have been obtained by studying the theories in flat space. In this article, our goal will be to study these theories on compact curved manifolds. One reason to do this is that on a compact manifold, the partition function of the theory is a finite, well-defined observable. We will see below that in many cases, this observable can be computed exactly, even in strongly coupled theories. These partition functions can then be related to certain information about the flat space theory, and so these exact results will give us a powerful tool for studying these theories.

In order to begin we need to write down actions for these theories on curved spacetimes, and it will be crucial that these actions preserve some supersymmetry. One way to proceed is to topologically twist the theories, à la Witten [2], which gives rise to a scalar supercharge which can be preserved on a generic manifold. To obtain a scalar supercharge in  $3d$ , we need at least an  $SO(3)$  R-symmetry, and so  $\mathcal{N} \geq 3$  supersymmetry, and this leads to the theories studied, *e.g.*, in [13].

---

<sup>4</sup>This may fail to be true if the theory is “bad” in the sense of [7].

An alternative approach is to restrict our attention to conformal field theories. These can then be conformally mapped from  $\mathbb{R}^3$  to any conformally flat space. In the case of a supersymmetric theory, the conformal algebra combines with the supersymmetry algebra to form the larger superconformal algebra, and this will be preserved on any such conformally flat background. With this motivation we first consider to the case of the round 3-sphere, which can be conformally mapped to  $\mathbb{R}^3$ , *e.g.*, by stereographic projection. Superconformal invariance will motivate us to write an action on  $S^3$  which preserves some supersymmetry, following [14].

However, we will see that this approach is quite limited, and requires some ad hoc reasoning to find a consistent action of supersymmetry on the fields. A more general picture has emerged, using supergravity, in which one finds a much larger class of geometries on which one can place theories supersymmetrically. In the present case, this construction can be thought of as performing a partial topological twist using the  $U(1)_R$  symmetry of the  $\mathcal{N} = 2$  algebra, which can produce a scalar supercharge when one is able to reduce the structure group of the tangent bundle to  $U(1)$ . The round sphere background is then a special case of this more general construction. After reviewing some relevant aspects of the general construction, we apply it to a set of manifolds which are topologically 3-spheres but with non-round metrics, so-called “squashed spheres,” and describe the supersymmetric backgrounds one can define here.

## 6.2.1 Round sphere

Given a conformally invariant theory in flat space, there is a unique way to couple it to a conformally flat manifold while preserving conformal invariance. For a superconformal theory, this coupling will also preserve the superconformal invariance. As a simple example, if we take the free chiral multiplet, the conformally coupled action is:

$$S = \int \sqrt{g} d^3x \left( \partial_\mu \tilde{\phi} \partial^\mu \phi + \frac{R}{8} \tilde{\phi} \phi - i \tilde{\psi} \gamma^\mu \nabla_\mu \psi - \tilde{F} F \right) \quad (6.2.1)$$

where  $R$  is the Ricci scalar<sup>5</sup> of the metric  $g_{\mu\nu}$ . One finds that this is invariant under the following superconformal symmetries:

$$\begin{aligned} \delta \phi &= \sqrt{2} \zeta \psi, \\ \delta \psi &= \sqrt{2} \zeta F - \sqrt{2} i \gamma^\mu \tilde{\zeta} \partial_\mu \phi - \frac{\sqrt{2} i}{3} \gamma^\mu (\nabla_\mu \tilde{\zeta}) \phi, \\ \delta F &= -\sqrt{2} i \tilde{\zeta} \gamma^\mu \nabla_\mu \psi \end{aligned} \quad (6.2.2)$$

provided that  $\zeta$  and  $\tilde{\zeta}$  are “Killing spinors,” *i.e.*, they satisfy:<sup>6</sup>

<sup>5</sup>We use a convention where the Ricci scalar curvature of the round  $S^3$  is positive, namely,  $R = \frac{6}{\ell^2}$ , where  $\ell$  is the radius.

<sup>6</sup>Solutions to this equation are sometimes called “conformal Killing spinors” or “twistor spinors,” while the term “Killing spinors” is sometimes reserved for those spinors with  $\zeta'$  proportional to  $\zeta$ . For ease of language we will refer to solutions of (6.2.3) (and its generalization in (6.2.15) below) simply as Killing spinors.

$$\nabla_\mu \zeta = \gamma_\mu \zeta', \quad (6.2.3)$$

and similarly for  $\tilde{\zeta}$ , where one computes  $\zeta' = \frac{1}{3}\gamma^\mu \nabla_\mu \zeta$ . This equation has the important property of being conformally covariant: under a rescaling  $g \rightarrow e^{2\Omega}g$  of the metric, we can rescale a Killing spinor as  $\zeta \rightarrow e^{\Omega/2}\zeta$  to get a Killing spinor for the new geometry. In flat space, there are 4 independent solutions: taking  $\zeta$  constant reproduces the supersymmetry transformations in (6.1.3), and taking  $\zeta = x^\mu \gamma_\mu \zeta_o$  for  $\zeta_o$  constant gives the special superconformal symmetries. Letting  $\zeta$  and  $\tilde{\zeta}$  run over these solutions, we see that there are 8 independent superconformal symmetries, which generate the superconformal algebra  $\mathfrak{osp}(2|2, 2)$ . Using the conformal covariance, this holds also on an arbitrary conformally flat background.

For the gauge multiplet, recall that the Yang-Mills term is not conformally invariant in 3 dimensions. However, the Chern-Simons term is conformal (in fact, topological), and can be written on an arbitrary manifold:

$$\mathcal{L}_{CS} = \frac{i}{4\pi} \text{Tr}_{CS}(\epsilon^{\mu\nu\rho}(A_\mu \partial_\nu A_\rho + \frac{2i}{3} A_\mu A_\nu A_\rho) + 2iD\sigma + 2\tilde{\lambda}\lambda) \quad (6.2.4)$$

This is invariant under the transformations:<sup>7</sup>

$$\begin{aligned} \delta A_\mu &= -i(\zeta \gamma_\mu \tilde{\lambda} + \tilde{\zeta} \gamma_\mu \lambda) \\ \delta \sigma &= -\zeta \tilde{\lambda} + \tilde{\zeta} \lambda \\ \delta \lambda &= (iD - \frac{i}{2} \epsilon^{\mu\nu\rho} \gamma_\rho F_{\mu\nu} - i\gamma^\mu D_\mu \sigma) \zeta - \frac{2i}{3} \sigma \gamma^\mu \nabla_\mu \zeta \\ \delta \tilde{\lambda} &= (-iD - \frac{i}{2} \epsilon^{\mu\nu\rho} \gamma_\rho F_{\mu\nu} + i\gamma^\mu D_\mu \sigma) \tilde{\zeta} + \frac{2i}{3} \sigma \gamma^\mu \nabla_\mu \tilde{\zeta} \\ \delta D &= \zeta \gamma^\mu D_\mu \tilde{\lambda} - \tilde{\zeta} \gamma^\mu D_\mu \lambda - [\zeta \tilde{\lambda}, \sigma] - [\tilde{\zeta} \lambda, \sigma] - iV_\mu (\zeta \gamma^\mu \tilde{\lambda} + \tilde{\zeta} \gamma^\mu \lambda) + \frac{1}{3} (\nabla_\mu \zeta \gamma^\mu \tilde{\lambda} - \nabla_\mu \tilde{\zeta} \gamma^\mu \lambda) \end{aligned} \quad (6.2.5)$$

It is straightforward to modify the action and SUSY transformation of the free chiral multiplet to couple it to a gauge multiplet while preserving superconformal invariance; we will summarize these below in a more general context.

These supersymmetries generate the superconformal algebra  $\mathfrak{osp}(2|2, 2)$ . Demanding an action which preserves the full superconformal algebra explicitly is very restrictive, and excludes many interesting superconformal theories which we can only obtain by RG flow from a non-conformal UV description. We can get further by relaxing the condition that we preserve the full superconformal algebra, and preserve only a subalgebra.

---

<sup>7</sup>In fact, the action is invariant under these transformations not only when  $\zeta$  and  $\tilde{\zeta}$  are Killing spinors, but for arbitrary spinors, which is related to the infinite dimensional diffeomorphism symmetry of this action. Since we will typically be interested in gauge theories coupled to matter, we will always impose the spinors are Killing spinors.

To see how this works, let us now specialize to the round  $S^3$ , of radius  $\ell$ .<sup>8</sup> This space is conformally flat, being conformally mapped to flat space by the stereographic projection, and so we expect to be able to place superconformal theories on this geometry.

First let us find the Killing spinors. It is convenient to recall that  $S^3$  is the group manifold of  $SU(2)$ , and so is acted on by left- and right-multiplication, which gives rise to the  $SU(2)_{left} \times SU(2)_{right}$  isometry group. Then we can take a vielbein,  $e_i^{left}$ ,  $i = 1, 2, 3$ , which is invariant under left-multiplication. In this basis the spin-connection is  $\omega_{ijk} = \frac{1}{\ell}\epsilon_{ijk}$ , and the spinor covariant derivative is:

$$\nabla_i \zeta = \partial_i \zeta - \frac{i}{2\ell} \gamma_i \zeta \quad (6.2.6)$$

Thus taking  $\zeta$  to be constant in this basis, one finds two linearly independent solutions to (6.2.3) with  $\zeta' = -\frac{i}{2\ell}\zeta$ . There are two other solutions with  $\zeta' = \frac{i}{2\ell}\zeta$  which can similarly be seen using a right-invariant vielbein.

Let us now declare that we are only interested in the subalgebra of the superconformal algebra generated by the left-invariant Killing spinors. These generate the superalgebra  $\mathfrak{osp}(2|2)$ , whose bosonic subalgebra consists of the  $\mathfrak{su}(2)_{left}$  isometry and the  $\mathfrak{u}(1)_R$  symmetry. The  $SU(2)_{right}$  symmetry commutes with these generators, and so the global symmetry algebra is  $\mathfrak{osp}(2|2) \times \mathfrak{su}(2)_{right}$ . In particular, this algebra does not contain dilatations, and so we might hope to find scale non-invariant actions. Indeed, letting  $\zeta$  be one of the left-invariant Killing spinors and  $\tilde{\zeta}$  its adjoint, one can compute that (up to total derivatives):

$$\begin{aligned} & \delta_\zeta \delta_{\tilde{\zeta}} \text{Tr} \left( \frac{1}{2} \tilde{\lambda} \lambda + i \sigma D \right) = \\ & = (\zeta \tilde{\zeta}) \text{Tr} \left( \frac{1}{4} F^{\mu\nu} F_{\mu\nu} + \frac{1}{2} D^\mu \sigma D_\mu \sigma - \frac{1}{2} (D + \frac{i}{\ell} \sigma)^2 - i \tilde{\lambda} \gamma^\mu D_\mu \lambda - \frac{1}{2\ell} \tilde{\lambda} \lambda + i \tilde{\lambda} [\sigma, \lambda] \right) \end{aligned} \quad (6.2.7)$$

Which is a curved-space analogue of the Yang-Mills action (6.1.11), and reduces to it as  $\ell \rightarrow \infty$ . This action is manifestly invariant under the two left-invariant supersymmetries.<sup>9</sup> Note that it explicitly breaks scale-invariance. In particular, this action must not be invariant under the two right-invariant supersymmetries, since if it were it would be invariant under the full superconformal algebra which they generate.

Once we sacrifice full conformal invariance, we can also try to construct non-conformally coupled actions for the scalars. In [15, 16] such actions were found which assign to a chiral multiplet a general R-charge  $r$  (the case  $r = \frac{1}{2}$  corresponding to the conformally coupled chiral):

$$\mathcal{L}_{chi} = D_\mu \tilde{\phi} D^\mu \phi + \tilde{\phi} (\sigma^2 + \frac{i(2r-1)}{\ell} \sigma + D + \frac{r(2-r)}{\ell^2}) \phi$$

---

<sup>8</sup>We could work in units where the radius of the sphere,  $\ell$ , is one, but it will be instructive to keep track of it.

<sup>9</sup>Namely, this follows from the fact that  $\delta_\zeta^2 = 0$  and  $\{\delta_\zeta, \delta_{\tilde{\zeta}}\}$  is a translation, which preserves the quantity inside the trace, up to a total derivative.

$$-i\tilde{\psi}\gamma^\mu D_\mu\psi - i\tilde{\psi}(\sigma + \frac{i}{\ell}(r - \frac{1}{2}))\psi + \sqrt{2}i(\tilde{\phi}\lambda\psi + \tilde{\psi}\tilde{\lambda}\phi) - \tilde{F}F \quad (6.2.8)$$

This is preserved by:

$$\begin{aligned} \delta\phi &= \sqrt{2}\zeta\psi, \\ \delta\psi &= \sqrt{2}\zeta F - \sqrt{2}i\gamma^\mu\tilde{\zeta}D_\mu\phi + \sqrt{2}i\sigma\phi\tilde{\zeta} - \sqrt{2}\frac{r}{\ell}\tilde{\zeta}\phi, \\ \delta F &= -\sqrt{2}i\tilde{\zeta}\gamma^\mu D_\mu\psi - \sqrt{2}i\sigma\tilde{\zeta}\psi + 2i\tilde{\zeta}\tilde{\lambda}\phi + \frac{\sqrt{2}}{\ell}(r - \frac{1}{2})\tilde{\zeta}\psi \end{aligned} \quad (6.2.9)$$

One computes that these transformations realize the algebra:

$$\delta_\zeta^2 = \delta_{\tilde{\zeta}}^2 = 0, \quad \{\delta_\zeta, \delta_{\tilde{\zeta}}\}\varphi = -i(v^\mu D_\mu)\varphi + \frac{1}{\ell}\mathcal{R}\varphi \quad (6.2.10)$$

where  $v^\mu = \tilde{\zeta}\gamma^\mu\zeta$  generates an infinitesimal  $SU(2)_{left}$  rotation, and  $\mathcal{R}$  is the R-charge, *i.e.*, acting as  $r$  for  $\phi$ ,  $r-1$  for  $\psi$ , and  $r-2$  for  $F$ . Note these reduce to the flat space gauge-coupled chiral multiplet action and supersymmetry algebra as  $\ell \rightarrow \infty$ .

Let us summarize what we have done so far. We have found an action on a round 3-sphere which preserves some superalgebra, namely,  $\mathfrak{osp}(2|2) \times \mathfrak{su}(2)_{right}$ . If our theory happened to be conformal, this sits inside the larger  $\mathfrak{osp}(2|2, 2)$  superconformal algebra, but we need not restrict to conformal theories. However, suppose we place the theory on a very large  $S^3$ , such that  $\frac{1}{\ell}$  is much larger than any relevant scale in the flat space theory. We have seen that the actions above are then well-approximated by the flat space actions. Thus as we undergo RG flow, the theory will flow very close to the flat space IR superconformal fixed point before it feels the effects of the non-zero curvature. But then we are effectively coupling a conformal theory to the curvature of  $S^3$ , and so, provided the  $\mathfrak{osp}(2|2)$  action we have chosen in the UV properly sits inside the superconformal  $\mathfrak{osp}(2|2, 2)$  group, we will obtain the IR SCFT conformally coupled to  $S^3$  [15].

Distinct  $\mathfrak{osp}(2|2)$  subalgebras differ by mixing the R-symmetry with a  $U(1)$  flavor symmetry of the theory, so to ensure we are studying the conformally coupled IR SCFT, we need to pick the R-symmetry to be the privileged  $U(1)_R$  superconformal symmetry, whose current sits in the same multiplet as the traceless stress energy tensor. If our theory has  $\mathcal{N} \geq 3$  supersymmetry, this is just the UV R-symmetry, while in the generic case we will have to determine these superconformal R-charges somehow (see section 6). But once we do, we can be sure that the  $\ell \rightarrow \infty$  limit of any  $S^3$  observables we compute correspond to those we would obtain if we conformally coupled the IR SCFT to  $S^3$ . As we will see below, the  $S^3$  observables we will compute are typically independent of  $\ell$ , making this correspondence even more straightforward.

### *Real masses and FI terms*

So far we have discussed mapping a conformal theory to the round  $S^3$ . However, one can consider certain deformations which take one away from the conformally mapped action, but give rise to interesting observables which probe the global symmetries of the theory.

Recall that in flat space we can add a real mass parameter associated to each  $U(1)$  subgroup of the global symmetry by coupling this symmetry to a background  $U(1)$  gauge multiplet and turning on a constant classical background value for the scalar, with all other fields vanishing. This preserved SUSY because this background was BPS. On  $S^3$ , we can similarly couple to a background vector multiplet in a BPS configuration. From (6.2.5), one can check that the following configuration is preserved by the supersymmetry transformations:

$$\sigma_{BG} = i\ell D_{BG} \equiv \frac{\hat{m}}{\ell} = \text{constant} \quad (6.2.11)$$

where it is convenient to work in terms of a dimensionless parameter  $\hat{m}$ . This modifies the chiral multiplet Lagrangian as:

$$\mathcal{L}_{chi} = \dots + \frac{q^2 \hat{m}^2 + 2i(r-1)q\hat{m}}{\ell^2} \tilde{\phi}\phi - i\frac{q\hat{m}}{\ell} \tilde{\psi}\psi \quad (6.2.12)$$

As in flat space, since the gauge scalar appears in the supersymmetry transformations of the chiral multiplet, such a term modifies these transformations, giving rise to a central extension of the algebra (6.2.10).

Note that for large  $\ell$ , the Lagrangian (6.2.12) goes over to the flat space chiral multiplet Lagrangian with a real mass  $\hat{m}/\ell$  (6.1.13). In particular, to get a finite real mass in the  $\ell \rightarrow \infty$  limit, one must scale  $\hat{m}$  with  $\ell$ . We will return to this issue in section 6.

Similarly, one can turn on a background vector multiplet coupled to the  $U(1)_J$  symmetry of a dynamical  $U(1)$  gauge field. This gives rise to a term:

$$\mathcal{L}_{FI} = \frac{1}{2\pi} \left( -D \frac{\hat{\zeta}}{\ell} + i\sigma \frac{\hat{\zeta}}{\ell^2} \right) \quad (6.2.13)$$

which is the  $S^3$ -analogue of the FI-term in flat space (6.1.17), and approaches it in the  $\ell \rightarrow \infty$  limit.

## 6.2.2 Supersymmetry on general 3-manifolds

In writing supersymmetric actions on the round sphere, we were initially motivated by superconformal invariance, but were soon led to consider non-conformally-invariant actions. Moreover, finding supersymmetric actions and transformation laws of the fields involved some guesswork. Once we allow such actions, one can ask whether we might also work on non-conformally-flat geometries, and whether there is a systematic method for constructing supersymmetric backgrounds on such manifolds. This was found to be the case in a series of papers, starting with [17]. The basic philosophy is to look for background, off-shell configurations of certain supergravity theories which preserve some rigid supersymmetry, and which can be coupled to quite general supersymmetric field theories via a certain multiplet

containing the stress-energy tensor. We refer to the accompanying article in Chapter 5 for a more in-depth discussion of this program.

The present case of interest, that of three dimensional  $\mathcal{N} = 2$  theories with a  $U(1)_R$  symmetry, was considered in [5]. They found that the appropriate supergravity theory is the three dimensional “new minimal” formalism, and found conditions under which a given background admits rigid supersymmetries. To describe these supergravity backgrounds explicitly, let us review the field content of new minimal supergravity in three dimensions. The fields are:

$$\begin{aligned} \text{metric } g_{\mu\nu}, \quad \text{R-symmetry gauge field } A_\mu^{(R)}, \quad \text{2-form gauge field } B_{\mu\nu}, \\ \text{central charge symmetry gauge field } C_\mu, \quad \text{gravitino } \psi_\mu, \tilde{\psi}_\mu \end{aligned} \quad (6.2.14)$$

We will often work in terms of the (Hodge duals of the) field strengths,  $H = \frac{i}{2}\epsilon^{\mu\nu\rho}\partial_\mu B_{\nu\rho}$ ,  $V^\mu = -i\epsilon^{\mu\nu\rho}\partial_\nu C_\rho$ . To have a rigid supersymmetry, we must find backgrounds which admit supersymmetry transformations such that  $\delta\psi_\mu = 0$ , which gives the conditions:

$$\begin{aligned} (\nabla_\mu - iA_\mu^{(R)})\zeta &= -\frac{1}{2}H\gamma_\mu\zeta - iV_\mu\zeta - \frac{1}{2}\epsilon_{\mu\nu\rho}V^\nu\gamma^\rho\zeta \\ (\nabla_\mu + iA_\mu^{(R)})\tilde{\zeta} &= -\frac{1}{2}H\gamma_\mu\tilde{\zeta} + iV_\mu\tilde{\zeta} + \frac{1}{2}\epsilon_{\mu\nu\rho}V^\nu\gamma^\rho\tilde{\zeta} \end{aligned} \quad (6.2.15)$$

where  $\zeta$  and  $\tilde{\zeta}$  have R-charge 1 and  $-1$ , respectively. We will also refer to solutions to this equation, which generalizes (6.2.3),<sup>10</sup> as Killing spinors.

The existence of a solution to one of these equations on a manifold was shown to be equivalent to the manifold admitting a transversally holomorphic fibration, which is an odd-dimensional analogue of a complex structure. In this article we will specialize to the case where there exists solutions to both equations, *i.e.*, two Killings spinors,  $\zeta$  and  $\tilde{\zeta}$ , of opposite R-charge. This further implies that the combination:

$$K^\mu = \zeta\gamma^\mu\tilde{\zeta} \quad (6.2.16)$$

is a nowhere-vanishing Killing vector. Conversely, if the manifold admits a nowhere vanishing real<sup>11</sup> Killing vector, then one can construct a background preserving two supercharges of opposite R-charge. Namely, if such a Killing vector exists, then we can find local coordinates  $(\psi, z, \bar{z})$  such that the metric locally takes the form:

$$ds^2 = \Omega(z, \bar{z})^2(d\psi + a)^2 + c(z, \bar{z})dzd\bar{z} \quad (6.2.17)$$

where  $a = a_z(z, \bar{z})dz + \bar{a}_{\bar{z}}(z, \bar{z})d\bar{z}$  and  $K^\mu = \frac{\partial}{\partial\psi}$ . We can cover the manifold by such charts which are related by  $\psi' = \psi + \alpha(z, \bar{z})$ ,  $z = \beta(z)$ ,  $\bar{z} = \bar{\beta}(\bar{z})$ , with  $\alpha$  real and  $\beta$  holomorphic.

Then the supergravity background fields and Killing spinors can be written explicitly in terms of  $K^\mu$  and these adapted coordinates. While this holds in general, we will make one

<sup>10</sup>Namely, this is essentially the generalization of (6.2.3) where  $\zeta$  is a section of a line bundle with connection  $A^{(R)}$ .

<sup>11</sup>The case of a complex Killing vector is more restrictive, and we will discuss an example in section 5.

simplifying assumption, which will be satisfied in all the examples we consider, which is that  $\Omega(z, \bar{z}) = 1$ , which amounts to requiring  $\|K\|^2 = 1$ . Note this can always be arranged by a conformal transformation, and this turns out not to affect any supersymmetric observables [19], so there is not much loss in making this assumption. With this assumption, we can take the following vielbein:

$$e_1 - ie_2 = c(z, \bar{z})dz, \quad e_1 + ie_2 = c(z, \bar{z})d\bar{z}, \quad e_3 = d\psi + a \quad (6.2.18)$$

and the spin connection is given by:

$$\omega_{12} = -\omega_{21} = F_a e_3 + \omega_{12}^{(2d)}, \quad \omega_{23} = -\omega_{32} = -F_a e_1, \quad \omega_{31} = -\omega_{13} = -F_a e_2 \quad (6.2.19)$$

where we have defined  $F_a(z, \bar{z}) = 2i(\partial_{\bar{z}}a_z - \partial_z a_{\bar{z}})$ , which is independent of the choice of chart, and  $\omega_{12}^{(2d)}$  is the spin connection associated to the  $2d$  metric  $c^2 dz d\bar{z}$ . Then one can check that if we take:

$$h = iF_a, \quad V^\mu = 0, \quad A^{(R)} = F_a e_3 + \frac{1}{2}\omega_{12}^{(2d)} \quad (6.2.20)$$

Then the Killing spinor equations (6.2.15) are solved by simply taking:

$$\zeta = \begin{pmatrix} 1 \\ 0 \end{pmatrix}, \quad \tilde{\zeta} = \begin{pmatrix} 0 \\ 1 \end{pmatrix}, \quad (6.2.21)$$

Let us record here the SUSY transformations of the gauge and chiral multiplets on a general background, which we will use in the examples below. For the gauge multiplet we find:

$$\begin{aligned} \delta A_\mu &= -i(\zeta\gamma_\mu\tilde{\lambda} + \tilde{\zeta}\gamma_\mu\lambda) \\ \delta\sigma &= -\zeta\tilde{\lambda} + \tilde{\zeta}\lambda \\ \delta\lambda &= (i(D + \sigma H) - \frac{i}{2}\epsilon^{\mu\nu\rho}\gamma_\rho F_{\mu\nu} - i\gamma^\mu(D_\mu\sigma + iV_\mu\sigma))\zeta \\ \delta\tilde{\lambda} &= (-i(D + \sigma H) - \frac{i}{2}\epsilon^{\mu\nu\rho}\gamma_\rho F_{\mu\nu} + i\gamma^\mu(D_\mu\sigma - iV_\mu\sigma))\tilde{\zeta} \\ \delta D &= D_\mu(\zeta\gamma^\mu\tilde{\lambda} - \tilde{\zeta}\gamma^\mu\lambda) - [\zeta\tilde{\lambda}, \sigma] - [\tilde{\zeta}\lambda, \sigma] - iV_\mu(\zeta\gamma^\mu\tilde{\lambda} + \tilde{\zeta}\gamma^\mu\lambda) - H(\zeta\tilde{\lambda} - \tilde{\zeta}\lambda) \end{aligned} \quad (6.2.22)$$

and for a chiral multiplet of R-charge  $r$  we find:

$$\begin{aligned} \delta\phi &= \sqrt{2}\zeta\psi, \\ \delta\psi &= \sqrt{2}\zeta F - \sqrt{2}i\gamma^\mu\tilde{\zeta}D_\mu\phi + \sqrt{2}i\sigma\phi\tilde{\zeta} + r\sqrt{2}iH\tilde{\zeta}\phi, \\ \delta F &= -\sqrt{2}iD_\mu(\tilde{\zeta}\gamma^\mu\psi) - \sqrt{2}i\sigma\tilde{\zeta}\psi + 2i\tilde{\zeta}\tilde{\lambda}\phi - \sqrt{2}i(r-2)H\tilde{\zeta}\psi \end{aligned} \quad (6.2.23)$$

Here the covariant derivative  $D_\mu$  is defined by:

$$D_\mu = \nabla_\mu - iA_\mu - i\mathcal{R}A_\mu^{(R)} \quad (6.2.24)$$

and these realize the algebra  $su(1|1)$ :

$$\delta_\zeta^2 = \delta_{\tilde{\zeta}}^2 = 0, \quad \{\delta_\zeta, \delta_{\tilde{\zeta}}\} = \mathcal{L}'_K + \mathcal{R}h\zeta\tilde{\zeta} \quad (6.2.25)$$

where  $\mathcal{R}$  is the R-charge of the field being acted on, and  $\mathcal{L}'_K$  is a R-symmetry covariant Lie derivative along  $K^\mu$ .

One can write supersymmetric Lagrangians for the gauge multiplet and chiral multiplet, analogous to the chiral  $D$ -term and Yang-Mills term above. These are given by:<sup>12</sup>

$$\delta_\zeta\delta_{\tilde{\zeta}}\left(\frac{1}{2}\tilde{\psi}\psi + i\tilde{\phi}\sigma\phi + iH(r-1)\tilde{\phi}\phi\right) = (\zeta\tilde{\zeta})\mathcal{L}_{chi} \quad (6.2.26)$$

$$\begin{aligned} \mathcal{L}_{chi} = & \mathcal{D}_\mu\tilde{\phi}\mathcal{D}^\mu\phi + \tilde{\phi}(\sigma^2 + \frac{r}{4}R + \frac{1}{2}(r - \frac{1}{2})V^\mu V_\mu + r(r - \frac{1}{2})H^2 + 2H(r - \frac{1}{2})\sigma + D)\phi \\ & - i\tilde{\psi}\gamma^\mu D_\mu\psi - i\tilde{\psi}(\sigma + (r - \frac{1}{2})H)\psi + \sqrt{2}i(\tilde{\phi}\lambda\psi + \tilde{\psi}\tilde{\lambda}\phi) - \tilde{F}F \end{aligned} \quad (6.2.27)$$

$$\delta_\zeta\delta_{\tilde{\zeta}}\text{Tr}\left(\frac{1}{2}\tilde{\lambda}\lambda + i\sigma D\right) = (\zeta\tilde{\zeta})\mathcal{L}_{YM} \quad (6.2.28)$$

$$\begin{aligned} \mathcal{L}_{YM} = & \text{Tr}\left(\frac{1}{4}F^{\mu\nu}F_{\mu\nu} + \frac{1}{2}D^\mu\sigma D_\mu\sigma - \frac{1}{2}(D + \sigma H)^2 + \frac{i}{2}\sigma\epsilon^{\mu\nu\rho}V_\mu F_{\nu\rho} - \frac{1}{2}V^\mu V_\mu\sigma^2\right. \\ & \left. - i\tilde{\lambda}\gamma^\mu(D_\mu + \frac{i}{2}V_\mu)\lambda + \frac{i}{2}H\tilde{\lambda}\lambda + i\tilde{\lambda}[\sigma, \lambda]\right) \end{aligned} \quad (6.2.29)$$

Just as on the round sphere, one can also turn on supersymmetric real mass and FI terms by coupling background vector multiplets in appropriate BPS configurations. We will describe these in more detail in the examples below.

### 6.2.3 Squashed 3-sphere

From the previous section, it is clear that the round sphere background should admit a large set of deformations of its metric and other background fields while still preserving some supersymmetry. These deformations of the metric lead to spaces which are often referred to as “squashed spheres,” or “ellipsoids.” There are infinitely many distinct ways one can supersymmetrically squash the sphere, and many have been discussed in the literature (see, *e.g.*, [20–23]). However, it turns out that these can all be labeled by a single complex parameter, usually called  $b$ , the “squashing parameter,” such that the partition function and supersymmetric observables depend on the background only through  $b$ . This was studied

<sup>12</sup>Here  $\mathcal{D}_\mu = D_\mu + ir_0V_\mu$ , where  $r_0$  is the UV R-symmetry generator.

systematically in [19], where it was shown that deformations of the background which preserve  $b$  only affect the action by a  $Q$ -exact term in the action, and so do not affect supersymmetric observables.<sup>13</sup>

A simple way to construct supersymmetry-preserving geometries which are topologically 3-spheres is by using the Hopf fibration, *i.e.*, exhibiting it as a  $U(1)$  fibration, with metric:

$$ds^2 = (d\psi + a)^2 + c^2 dz d\bar{z} \quad (6.2.30)$$

where now  $\psi \sim \psi + 2\pi$ ,  $c^2 dz d\bar{z}$  is any smooth metric on  $S^2$ , and  $a$  is a connection on  $S^2$  with Chern number 1. In this case the integral curves of  $K = \partial_\psi$  are the fibers of the Hopf fibration. However, it turns out that these geometries all give the same answer for supersymmetric observables as the round sphere. Note one can define such backgrounds for general fibrations over general Riemann surfaces, as considered in [25, 26].

A more general answer can be obtained if we consider metrics on  $S^3$  which admit two independent isometries. To construct such metrics, let us define coordinates  $(\chi, \theta, \phi)$  by:

$$z_1 = \cos \chi e^{i\varphi}, \quad z_2 = \sin \chi e^{i\theta} \quad (6.2.31)$$

which parameterize the subset  $S^3 \subset \mathbb{C}^2$  defined by  $|z_1|^2 + |z_2|^2 = 1$ . Here  $\chi \in [0, \frac{\pi}{2}]$ ,  $\varphi \sim \varphi + 2\pi$ , and  $\theta \sim \theta + 2\pi$ . These are called “toroidal coordinates,” as the surfaces of constant  $\chi$  are tori swept out by  $\theta$  and  $\phi$ , where at  $\chi = 0$  (respectively  $\chi = \frac{\pi}{2}$ ), the cycle corresponding to  $\varphi$  (respectively  $\theta$ ) degenerates, and the torus degenerates to a circle (see Figure 1). The round sphere metric in these coordinates is:

$$ds^2 = \ell^2 (d\chi^2 + \cos^2 \chi d\varphi^2 + \sin^2 \chi d\theta^2) \quad (6.2.32)$$

Let us consider a more general metric which preserves a  $U(1) \times U(1)$  subgroup of the  $SU(2) \times SU(2)$  isometry of the round sphere. We take:

$$ds^2 = f(\chi)^2 d\chi^2 + \ell_1^2 \cos^2 \chi d\varphi^2 + \ell_2^2 \sin^2 \chi d\theta^2 \quad (6.2.33)$$

Here  $\ell_i$  are constants, and  $f$  is an arbitrary smooth positive function on  $[0, \frac{\pi}{2}]$ , with the only restriction that  $f(\chi = 0) = \ell_1$  and  $f(\chi = \frac{\pi}{2}) = \ell_2$ , as otherwise the space will have conical singularities along these circles. We will see below that the supersymmetric observables on this space depend only on the “squashing parameter”  $b$ , defined by:<sup>14</sup>

$$b \equiv \sqrt{\ell_1/\ell_2} \quad (6.2.34)$$

In particular, they are essentially independent of the function  $f(\chi)$ .

<sup>13</sup>See also [24] for an alternative approach, using three dimensional topological gravity, to constructing supersymmetric backgrounds and determining which geometric parameters supersymmetric observables may depend on.

<sup>14</sup>Here we require  $b$  to be real, but one can find more general supersymmetric backgrounds corresponding to complex  $b$  [27].

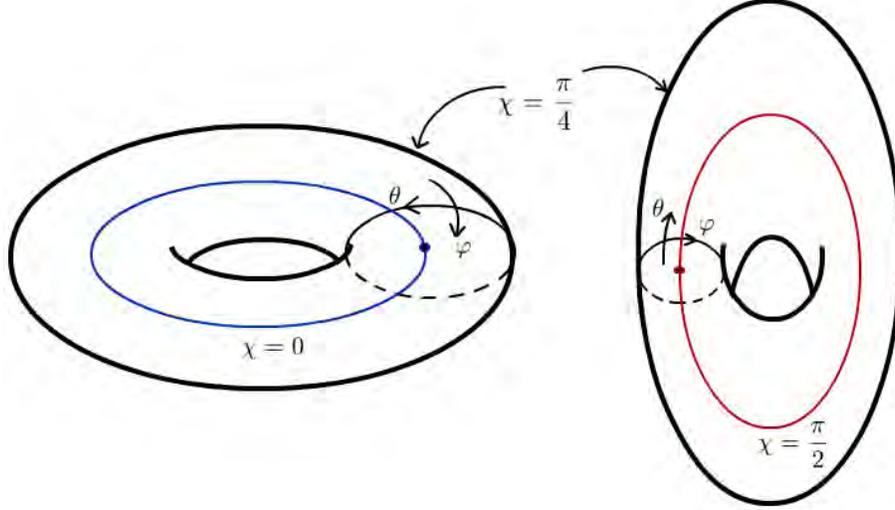

Figure 6.1: The (squashed) sphere in toroidal coordinates, cut open along the torus at  $\chi = \frac{\pi}{4}$ .

A general Killing vector on this space has the form  $\alpha\partial_\varphi + \beta\partial_\theta$  for constants  $\alpha, \beta$ . In order to use the supergravity background derived above, we demand that the norm of  $K$  be constant, *i.e.*:

$$\|K\|^2 = \alpha^2 l_1^2 \cos^2 \chi + \beta^2 l_2^2 \sin^2 \chi = \text{constant} \quad (6.2.35)$$

This imposes  $\beta/\alpha = l_1/l_2 = b^2$ , and so we find a suitable Killing vector is:

$$K = l_1^{-1}\partial_\varphi + l_2^{-1}\partial_\theta \quad (6.2.36)$$

Then we can locally write the metric in the form (6.2.17) by defining local coordinates (here  $z = x + iy, \bar{z} = x - iy$ ):

$$x = \int_{x_0}^x \frac{f(\chi)}{\sin \chi \cos \chi} d\chi, \quad y = -l_2\varphi + l_1\theta, \quad \psi = l_1\varphi \cos^2 \chi + l_2\theta \sin^2 \chi \quad (6.2.37)$$

and one can check that the metric (6.2.33) can be written:

$$ds^2 = (d\psi + a)^2 + c(z, \bar{z})dzd\bar{z} \quad (6.2.38)$$

Where the 1-form  $a$  and scalar  $c$  are given by (writing these in toroidal coordinates for simplicity):

$$a = 2(-l_1\varphi + l_2\theta) \sin \chi \cos \chi d\chi, \quad c = \sin \chi \cos \chi \quad (6.2.39)$$

One can check that they are independent of  $\psi$  and  $d\psi$ , and that  $\partial_\psi = K$ . Then, from (6.2.18), we take the vielbein:

$$e_1 = f(\chi)d\chi, \quad e_2 = -l_2d\varphi + l_1d\theta, \quad e_3 = l_1d\varphi \cos^2 \chi + l_2d\theta \sin^2 \chi \quad (6.2.40)$$

Note that, for general  $b$ , the coordinate  $\psi$  is not periodic, *i.e.*, this metric is not compatible with an  $S^1$  fibration. The integral curves of  $K$  do not close at generic  $\chi$  unless  $b^2 = p/q$  is rational, in which case they give rise to  $(p, q)$  torus knots. However, for all  $b$ , the integral curves of  $K$  at  $\chi = 0, \frac{\pi}{2}$  are circles, and we will see below that one can insert supersymmetric loop operators along these circles.

Now we can use the machinery introduced in the previous section to write supersymmetric actions on this space. From (6.2.20), we compute

$$H = \frac{i}{f}, \quad V_\mu = 0, \quad A^{(R)} = \frac{1}{2}\left(1 - \frac{\ell_1}{f}\right)d\varphi + \frac{1}{2}\left(1 - \frac{\ell_2}{f}\right)d\theta \quad (6.2.41)$$

Here we have performed an  $R$ -symmetry gauge transformation to ensure that  $A_\mu^{(R)}$  is everywhere regular. In this gauge, the Killing spinors are given by:

$$\zeta = e^{i(\varphi+\theta)/2} \begin{pmatrix} 1 \\ 0 \end{pmatrix}, \quad \tilde{\zeta} = e^{-i(\varphi+\theta)/2} \begin{pmatrix} 0 \\ 1 \end{pmatrix}, \quad (6.2.42)$$

Note that for the round sphere,  $f(\chi) = \ell_1 = \ell_2 = \ell$ . Then  $H = \frac{i}{\ell}$  and  $A^{(R)}$  vanishes, and one can check that the SUSY transformations and actions reproduce those we found in section 2.1, giving rise to one of the left-invariant Killing spinors and its conjugate. The existence of two additional Killing spinors, and the larger  $\mathfrak{osp}(2|2)$  algebra, is a consequence of the extra symmetry of the round sphere. One can also construct squashed sphere backgrounds which preserve four supercharges [20, 21], but we will not consider them here.

### 6.3 Localization of the partition function on the 3–sphere

In the previous section we found actions for a  $3d \mathcal{N} = 2$  theories on a general squashed sphere background which reduce to the flat space actions as the radius  $\ell$  of the sphere was taken to infinity, and preserve a deformed supersymmetry algebra for all  $\ell$ . In this section we will put these actions to work, and use them to compute exact, non-perturbative results in strongly coupled quantum field theories. Although we will study the theories on curved, compact backgrounds, we will see these results also teach us about the theories in flat space.

The fact that we are working on a compact space opens up the possibility to consider the partition function, *i.e.*, the (unnormalized) path integral with no operator insertions, as a well-defined observable in the theory. As we will see below, the partition function is a very rich observable, with many physical applications. We will also be able to compute the expectation value of certain supersymmetric operators. In the case of conformal theories on the round sphere, these expectation values can be related to ones in the flat space theory. We will study further applications in section 6.

To start, let us pick some flat space  $3d \mathcal{N} = 2$  gauge theory which we would like to study. This amounts to a choice of the following data:

- A gauge group  $G$ . Then the field content will include a vector multiplet in the adjoint representation of  $G$ .
- Representations  $R_i$  of  $G$  for the chiral multiplets
- Kinetic terms for the vector and chiral multiplets. The latter will always be the canonical one, while for the former we may include the standard Yang-Mills term as well as...
- A Chern-Simons term defined by some properly quantized trace  $\text{Tr}_{CS}$  on the Lie algebra  $\mathfrak{g}$ . Here we allow  $\text{Tr}_{CS} = 0$  if there is no CS term.
- A gauge-invariant superpotential  $W(\Phi_i)$  for the chiral multiplets. This superpotential must preserve a  $U(1)_R$  symmetry.

We have seen in the previous section how to write an action on a 3-sphere of radius  $\ell$  which preserves some supersymmetry, and reduces to the original flat space action as  $\ell \rightarrow \infty$ . To do this, we must choose a  $U(1)_R$  symmetry, which assigns an R-charge  $r_i$  to the  $i$ th chiral multiplet; at this point this choice is arbitrary, but we will return to this issue below. We denote this action  $S$ , and write it schematically as:

$$S[\Phi] = S_{YM}[\Phi] + S_{chi}[\Phi] + S_W[\Phi] + S_{CS}[\Phi] \quad (6.3.1)$$

where  $\Phi$  denotes the fields of the theory. Then we would like to compute the Euclidean signature path-integral:

$$\mathcal{Z} = \int \mathcal{D}\Phi e^{-S[\Phi]} \quad (6.3.2)$$

or more generally, the expectation value of a supersymmetric operator  $\mathcal{O}$ :

$$\langle \mathcal{O} \rangle = \frac{1}{\mathcal{Z}} \int \mathcal{D}\Phi e^{-S[\Phi]} \mathcal{O}[\Phi] \quad (6.3.3)$$

As in many articles in this review, the key principle that will allow us to compute these observables is the localization argument, which we review now. We recall from the previous section that  $S_{YM}$  and  $S_{chi}$  are total  $\delta_\zeta$  variations. Thus we can change their coefficients without affecting these observables, provided that  $\delta_\zeta \mathcal{O} = 0$ . Thus we consider the deformed action:

$$S'_t[\Phi] = tS_{YM}[\Phi] + tS_{chi}[\Phi] + S_W[\Phi] + S_{CS}[\Phi] \quad (6.3.4)$$

When we take  $t$  very large, since  $S_{YM}$  and  $S_{chi}$  are positive semi-definite, the path integral gets contributions only from field configurations near the locus of zero modes of these kinetic terms:

$$\mathcal{M}_{BPS} = \{\Phi_o \mid S_{YM}[\Phi_o] = S_{chi}[\Phi_o] = 0\} \quad (6.3.5)$$

These are the saddle points of the path integral in the large  $t$  limit. As we will see shortly, this space is finite dimensional, and in fact, coincides precisely with the set of BPS configurations, as in (6.2.11).

Then to find the contribution to the path integral from a region near some fixed  $\Phi_o$  we write:

$$\Phi = \Phi_o + t^{-1/2}\Phi' \quad (6.3.6)$$

and we expand the action to leading order in  $t^{-1}$ :

$$S'_t[\Phi] = S_{YM}^{quad}[\Phi_o; \Phi'] + S_{chi}^{quad}[\Phi_o; \Phi'] + S_W[\Phi_o] + S_{CS}[\Phi_o] + O(t^{-1}) \quad (6.3.7)$$

where the superscript “quad” denotes that we consider only the quadratic part of these actions (treating  $\Phi_o$  as a background field), since the higher order terms will be suppressed by powers of  $t^{-1}$ . The integration over  $\Phi'$  for a fixed  $\Phi_o$  is a computation in a gaussian theory, and can be performed explicitly. We define:

$$\mathcal{Z}_{1-loop}[\Phi_o] = \int \mathcal{D}\Phi' e^{-S_{YM}^{quad}[\Phi_o; \Phi'] - S_{chi}^{quad}[\Phi_o; \Phi']} \quad (6.3.8)$$

It then only remains to perform the finite dimensional integral over the zero-modes  $\Phi_o$ :

$$\mathcal{Z} = \int_{\mathcal{M}_{BPS}} d\Phi_o e^{-S_W[\Phi_o] - S_{CS}[\Phi_o]} \mathcal{Z}_{1-loop}[\Phi_o] \quad (6.3.9)$$

$$\langle \mathcal{O} \rangle = \frac{1}{\mathcal{Z}} \int_{\mathcal{M}_{BPS}} d\Phi_o \mathcal{O}[\Phi_o] e^{-S_W[\Phi_o] - S_{CS}[\Phi_o]} \mathcal{Z}_{1-loop}[\Phi_o] \quad (6.3.10)$$

A priori these expressions are the leading approximations in the large  $t$  limit, but since the answer is independent of  $t$ , these approximations are exact for all  $t$ , and in particular for our original action.

Let us now see how these computations go through in detail using the actions we have derived in the previous section.

### 6.3.1 Round $S^3$

We start, as in the previous section, with the relatively simpler case of the round 3-sphere.

#### *Gauge multiplet*

Recall from (6.2.7) that the supersymmetric Yang-Mills term on  $S^3$  can be written as:

$$\begin{aligned} S_{YM} &= \delta_\zeta \delta_{\bar{\zeta}} \int \sqrt{g} d^3x \frac{1}{\zeta \bar{\zeta}} \text{Tr} \left( \frac{1}{2} \tilde{\lambda} \lambda + i\sigma D \right) = \\ &= \int \sqrt{g} d^3x \text{Tr} \left( \frac{1}{4} F^{\mu\nu} F_{\mu\nu} + \frac{1}{2} D^\mu \sigma D_\mu \sigma - \frac{1}{2} \left( D + \frac{i}{\ell} \sigma \right)^2 - i\tilde{\lambda} \gamma^\mu D_\mu \lambda - \frac{1}{2\ell} \tilde{\lambda} \lambda + i\tilde{\lambda} [\sigma, \lambda] \right) \end{aligned} \quad (6.3.11)$$

To make the path-integral well-defined, we should work with the gauge-fixed theory. Thus we introduce ghosts  $c, \bar{c}, b$  and add the ghost action:<sup>15</sup>

$$S_g = \int \sqrt{g} d^3x \text{Tr}(D_\mu \bar{c} D^\mu c + b \nabla^\mu A_\mu) \quad (6.3.12)$$

which imposes the gauge  $\nabla^\mu A_\mu = 0$ . The action  $S_g$  is invariant under a fermionic BRST symmetry,  $\delta_{BRST}$ , and one can check that  $S_{YM} + S_g$  is exact under the sum of  $\delta_\zeta$  and  $\delta_{BRST}$ , so we can add them both to the action without affecting the result of the path-integral.

Since (6.3.11) is written as a sum of squares, we can immediately see the zeros of this action, or BPS configurations, are given by:

$$F_{\mu\nu} = 0, \quad D_\mu \sigma = 0, \quad D + \frac{i}{\ell} \sigma = 0 \quad (6.3.13)$$

Since  $H^1(S^3, \mathbb{R}) = 0$ , the first equation implies that  $A_\mu$  is pure gauge, and our gauge-fixing condition imposes that in fact  $A_\mu = 0$ . The second equation then says that  $\sigma$  is constant. Thus the BPS configurations are:<sup>16</sup>

$$\sigma = i\ell D \equiv \frac{\hat{\sigma}_o}{\ell} = \text{constant} \quad (6.3.14)$$

These are labeled by an element  $\hat{\sigma}_o$  of the Lie algebra  $\mathfrak{g}$  of the gauge group. Without loss we can take  $\hat{\sigma}_o$  to lie in a Cartan subalgebra  $\mathfrak{h}$  of  $\mathfrak{g}$ .

Next we need to compute the 1-loop determinant from fluctuations around one of these configurations. Thus we expand:

$$A_\mu = t^{-1/2} A'_\mu, \quad \sigma = \frac{\hat{\sigma}_o}{\ell} + t^{-1/2} \sigma', \quad D = -\frac{i}{\ell^2} \hat{\sigma}_o + t^{-1/2} D', \quad \lambda = t^{-1/2} \lambda' \quad (6.3.15)$$

Here  $\sigma'$  should be taken to not include its zero mode, as this is accounted for in the integral over  $\hat{\sigma}_o$  we will perform in a moment. We plug these into the Yang-Mills action above and expand to leading order in  $t^{-1}$  to find the quadratic action:

$$\begin{aligned} tS'_{YM}[\sigma_o] = \int \sqrt{g} d^3x \text{Tr} & \left( \frac{1}{4} F'^{\mu\nu} F'_{\mu\nu} + \frac{1}{2} \partial^\mu \sigma' \partial_\mu \sigma' - \frac{1}{2\ell^2} [A'_\mu, \hat{\sigma}_o]^2 - \frac{1}{2} (D' + \frac{i}{\ell} \sigma')^2 \right. \\ & \left. - i \tilde{\lambda}' \gamma^\mu \nabla_\mu \lambda' - \frac{1}{2\ell} \tilde{\lambda}' \lambda' + \frac{i}{\ell} \tilde{\lambda}' [\hat{\sigma}_o, \lambda'] \right) + O(t^{-1}) \end{aligned} \quad (6.3.16)$$

where  $F'_{\mu\nu} = \partial_\mu A'_\nu - \partial_\nu A'_\mu$ .

<sup>15</sup>Here we should not integrate over the zero mode of  $c$ . This can be treated more carefully by introducing ghosts of ghosts.

<sup>16</sup>The factor of  $\ell^{-1}$  in the equation defining  $\hat{\sigma}_o$  is to make it dimensionless, which will be convenient below.

Now we need to compute the path-integral of this gaussian theory. We decompose the gauge field as:

$$A'_\mu = B_\mu + \partial_\mu \varphi \quad (6.3.17)$$

where  $B_\mu$  is divergenceless, *i.e.*,  $\nabla^\mu B_\mu = 0$ . Then one can check that the integrals over  $\sigma'$ ,  $\varphi$ ,  $c$  and  $\bar{c}$  all give determinants which cancel. Next we expand  $B_\mu$  and  $\lambda'$  in a basis  $X_\alpha$  of the Lie algebra, such that  $[\hat{\sigma}_o, X_\alpha] = \alpha(\hat{\sigma}_o)X_\alpha$ . The remaining action is then:

$$\int \sqrt{g} d^3x \sum_{\alpha \in Ad(G)} \left( \frac{1}{2} B^\mu_{-\alpha} (-\nabla^2 + \frac{1}{\ell^2} \alpha(\hat{\sigma}_o)^2) B_{\mu\alpha} + \tilde{\lambda}'_{-\alpha} (-i\gamma^\mu \nabla_\mu + \frac{i}{\ell} \alpha(\hat{\sigma}_o) - \frac{1}{2\ell}) \lambda'_\alpha \right) \quad (6.3.18)$$

and so the 1-loop determinant is given by:

$$\mathcal{Z}_{1-loop}^{gauge}(\sigma_o) = \prod_{\alpha \in Ad(G)} \frac{\det(-i\gamma^\mu \nabla_\mu + \frac{i}{\ell} \alpha(\sigma_o) - \frac{1}{2\ell})}{\det(-\nabla^2 + \frac{1}{\ell^2} \alpha(\hat{\sigma}_o)^2)} \quad (6.3.19)$$

where in the denominator the operator is understood to act on divergenceless vector fields.

To compute these determinants, we note that the scalars, spinors, and vectors on the round  $S^3$  fall into the following representations of the  $SU(2)_{left} \times SU(2)_{right}$  isometry group:

$$\begin{aligned} \text{scalars} & \quad \oplus_{j \geq 0} \left( \frac{j}{2}, \frac{j}{2} \right), & \quad \nabla^2 \text{ eigenvalue} & \rightarrow \frac{1}{\ell^2} j(j+2) \\ \text{spinors} & \quad \oplus_{j \geq 0} \left( \frac{j}{2}, \frac{j+1}{2} \right) \oplus \left( \frac{j+1}{2}, \frac{j}{2} \right), & \quad i\gamma^\mu \nabla_\mu \text{ eigenvalue} & \rightarrow \pm \frac{1}{\ell} \left( j + \frac{3}{2} \right) \\ \text{divergenceless vectors} & \quad \oplus_{j \geq 0} \left( \frac{j}{2}, \frac{j+2}{2} \right) \oplus \left( \frac{j+2}{2}, \frac{j}{2} \right), & \quad \nabla^2 \text{ eigenvalue} & \rightarrow \frac{1}{\ell^2} (j+2)^2 \end{aligned} \quad (6.3.20)$$

Thus we find (canceling factors of  $\ell$ ):

$$\mathcal{Z}_{1-loop}^{gauge}(\sigma_o) = \prod_{\alpha \in Ad(G)} \prod_{j=0}^{\infty} \frac{((-j-2 + i\alpha(\hat{\sigma}_o))(j+1 + i\alpha(\hat{\sigma}_o)))^{(j+1)(j+2)}}{(\alpha(\hat{\sigma}_o)^2 + (j+2)^2)^{(j+1)(j+3)}} \quad (6.3.21)$$

Many of these eigenvalues cancel, and we end up with:

$$\mathcal{Z}_{1-loop}^{gauge}[\sigma_o] = \prod_{\alpha \in Ad(G)} \prod_{j=1}^{\infty} \frac{(j + i\alpha(\hat{\sigma}_o))^{j+1}}{(j - i\alpha(\hat{\sigma}_o))^{j-1}}$$

After zeta-function regularization, this can be written as:

$$\mathcal{Z}_{1-loop}^{gauge}(\sigma_o) = \prod_{\alpha \in Ad(G)} \frac{2 \sinh \pi \alpha(\sigma_o)}{\pi \alpha(\sigma_o)} \quad (6.3.22)$$

The cancellation of most of the eigenvalues is a consequence of the supersymmetry which acts on the fluctuations about the BPS configuration. We will see it continues to hold even on the general geometry of the squashed sphere, and in fact will be what ultimately allows us to evaluate the ratio of determinants of the more complicated operators which will appear there.

### *Chiral multiplet*

Next we turn to the chiral multiplet. For simplicity, we may take the gauge multiplet fields to lie in their BPS configurations, since any other configurations will be strongly suppressed by the gauge multiplet  $\delta$ -exact term. We use the kinetic term of the chiral multiplet of  $R$ -charge  $r$  from (6.2.8), for a fixed BPS configuration labeled by  $\hat{\sigma}_o$ :

$$\mathcal{L}_{chi} = \partial_\mu \tilde{\phi} \partial^\mu \phi + \frac{1}{\ell^2} \tilde{\phi} (\hat{\sigma}_o^2 + 2i(r-1)\hat{\sigma}_o + r(2-r))\phi - i\tilde{\psi} \gamma^\mu \nabla_\mu \psi - \frac{i}{\ell} \tilde{\psi} (\hat{\sigma}_o + i(r - \frac{1}{2}))\psi - \tilde{F}F \quad (6.3.23)$$

One can check that this action has no zero modes apart from the trivial one, with all fields vanishing.<sup>17</sup> This action is already quadratic, so all that remains is to compute the path integral for this gaussian theory. After expanding the modes in a weight basis  $e_\rho$  of the representation  $R$  in which the chiral transforms, we find the partition function is given by:

$$\mathcal{Z}_{1-loop}^{chiral}(\hat{\sigma}_o) = \prod_{\rho \in R} \frac{\det(-i\gamma^\mu \nabla_\mu - \frac{i}{\ell}(\rho(\hat{\sigma}_o) + i(r - \frac{1}{2})))}{\det(-\nabla^2 + \frac{1}{\ell^2}(\rho(\hat{\sigma}_o)^2 + 2i(r-1)\rho(\hat{\sigma}_o) + r(2-r)))} \quad (6.3.24)$$

We can compute the eigenvalues of these operators using (6.3.20):

$$\begin{aligned} \mathcal{Z}_{1-loop}^{chiral}(\hat{\sigma}_o) &= \prod_{\rho \in R} \prod_{j=0}^{\infty} \frac{(\pm(j + \frac{3}{2}) - i\rho(\hat{\sigma}_o) + r - \frac{1}{2})^{(j+1)(j+2)}}{(j(j+2) + \rho(\sigma_o)^2 + 2i(r-1)\rho(\hat{\sigma}_o) + r(2-r))^{(j+1)^2}} \\ &= \prod_{\rho \in R} \prod_{j=0}^{\infty} \frac{((j+1 - i\rho(\hat{\sigma}_o) + r)(-j-2 - i\rho(\hat{\sigma}_o) + r))^{(j+1)(j+2)}}{((j+r - i\rho(\hat{\sigma}_o))(j+2-r + i\rho(\hat{\sigma}_o)))^{(j+1)^2}} = \prod_{\rho \in R} \prod_{j=0}^{\infty} \frac{(j + i\rho(\hat{\sigma}_o) + 2 - r)^{j+1}}{(j - i\rho(\hat{\sigma}_o) + r)^{j+1}} \\ &= \prod_{\rho \in R} \mathcal{Z}_{chi}^r(\rho(\hat{\sigma}_o)) \end{aligned} \quad (6.3.25)$$

where we define the 1-loop determinant of a chiral multiplet of  $R$ -charge  $r$  and coupled to a background gauge scalar  $\hat{\sigma}$  as:

$$\mathcal{Z}_{chi}^r(\hat{\sigma}) = s_{b=1}(i(1-r) - \hat{\sigma}) \quad (6.3.26)$$

where  $s_b(x)$  is the double-sine function, defined for general  $b$  by:

<sup>17</sup>This will also follow from the fact that the fluctuations we will compute in a moment have no zero-modes.

$$s_b(x) = \prod_{m,n \geq 0} \frac{(m + \frac{1}{2})b + (n + \frac{1}{2})b^{-1} - ix}{(m + \frac{1}{2})b + (n + \frac{1}{2})b^{-1} + ix} \quad (6.3.27)$$

For theories with  $\mathcal{N} \geq 3$  supersymmetry, the matter content is organized into hypermultiplets, which are pairs of chiral multiplets with R-charge  $\frac{1}{2}$ . Here one finds a simplification using:<sup>18</sup>

$$\mathcal{Z}_{chi}^{r=\frac{1}{2}}(\pm\rho(\sigma_o)) = s_{b=1}(\frac{i}{2} \pm \rho(\hat{\sigma}_o)) = \frac{1}{2 \cosh \pi \rho(\hat{\sigma}_o)} \quad (6.3.28)$$

In addition, the adjoint chiral multiplet in the  $\mathcal{N} = 4$  vector multiplet has R-charge 1, and one can check that its contribution is trivial.

### *Classical contribution*

Next we must consider the contribution from the original action when we plug in the BPS configuration,  $\sigma = i\ell D = \frac{\hat{\sigma}_o}{\ell}$ , and all other fields vanishing. The original kinetic terms for the gauge and chiral multiplets do not contribute, since, by construction, they vanish on the BPS configurations. For the Chern-Simons term, if we plug the BPS configuration into (6.2.4), we find:

$$S_{CS}[\hat{\sigma}_o] = \frac{i}{4\pi} \int \sqrt{g} d^3x \text{Tr}_{CS}(2i(\frac{\hat{\sigma}_o}{\ell})(\frac{\hat{\sigma}_o}{i\ell^2})) = \frac{i \text{vol}(S^3)}{2\pi\ell^3} \text{Tr}_{CS}(\hat{\sigma}_o^2) = \pi i \text{Tr}_{CS}(\hat{\sigma}_o^2) \quad (6.3.29)$$

where we used  $\text{vol}(S^3) = 2\pi^2\ell^3$ .

The superpotential term does not directly contribute to the matrix model, since it depends only on the fields in the chiral multiplet, which are zero at the saddle point. However, it does contribute in an indirect way, by restricting the allowed R-charges and the flavor symmetry group of the theory.

### *Background Fields*

So far we have considered the action without any mass or FI deformations, however, these are easily incorporated by recalling that they correspond to background BPS configurations of vector multiplets coupled to global symmetries.

To incorporate them, let us assume the flavor symmetry group of the theory is  $H$ , so that the total symmetry acting on the chiral multiplets is  $G \times H$ . Then we can couple a classical background gauge multiplet to the flavor symmetry group  $H$ , and then a real mass parameter is just a BPS configuration for this gauge multiplet, which is labeled by an element  $\hat{m}$  of the Lie algebra of  $H$ . Thus if we can decompose the chirals into weights  $(\rho, \omega)$  of the

---

<sup>18</sup>Here we are only considering flavor symmetries commuting with the full  $\mathcal{N} = 4$  superalgebra. One could also turn on a real mass for the  $U(1)$  subgroup of the  $SO(4)$  R-symmetry commuting with our chosen  $\mathcal{N} = 2$  subalgebra, however, in this case the 1-loop determinants would not simplify.

representation  $\tilde{R}$  of  $G \times H$  in which they sit, we find the 1-loop determinant with the real mass turned on is:

$$\prod_{(\rho, \omega) \in \tilde{R}} \mathcal{Z}_{chi}^r(\rho(\hat{\sigma}_o) + \omega(\hat{m})) \quad (6.3.30)$$

Similarly, an FI term is a classical background  $U(1)$  gauge multiplet which couples to the dynamical gauge field via an off-diagonal CS term, as in (6.2.13). Thus it modifies the classical contribution via a term (in the notation of (6.1.18)):

$$S_{FI} = 2\pi i \hat{\zeta}^a \lambda_a(\hat{\sigma}_o) \quad (6.3.31)$$

### Integration over BPS configurations

Putting the above pieces together, we see the contribution from a BPS configuration labeled by  $\hat{\sigma}_o$ , which we have taken to lie in a Cartan subalgebra  $\mathfrak{h}$  of  $\mathfrak{g}$ , is given by:

$$\begin{aligned} & e^{-S_{CS}[\hat{\sigma}_o] - S_{FI}[\hat{\sigma}_o]} \mathcal{Z}_{1-loop}^{gauge}(\hat{\sigma}_o) \mathcal{Z}_{1-loop}^{chi}(\hat{\sigma}_o) \\ &= e^{-\pi i Tr_{CS}(\hat{\sigma}_o^2) - 2\pi i \hat{\zeta}^a \lambda_a(\hat{\sigma}_o)} \prod_{\alpha \in Ad(G)} \frac{2 \sinh \pi \alpha(\hat{\sigma}_o)}{\pi \alpha(\hat{\sigma}_o)} \prod_i \prod_{(\rho, \omega) \in \tilde{R}_i} \mathcal{Z}_{chi}^{r_i}(\rho(\hat{\sigma}_o) + \omega(\hat{m})) \end{aligned} \quad (6.3.32)$$

where  $R_i$  runs over the irreducible representations of  $G \times H$  in which the chiral multiplets lie.

The final step is to integrate over these BPS configurations, *i.e.*, to integrate  $\hat{\sigma}_o$  over the Lie algebra  $\mathfrak{g}$ . Using the Weyl integration formula we can reduce this to an integral over our chosen Cartan subalgebra  $\mathfrak{h}$ . This induces a Vandermonde determinant factor, which precisely cancels the denominator in the 1-loop contribution of the gauge multiplet, and we finally arrive at:

$$\mathcal{Z}_{S^3}(\hat{\eta}, \hat{m}) = \frac{1}{|\mathcal{W}|} \int_{\mathfrak{h}} d\hat{\sigma}_o e^{-\pi i Tr_{CS}(\hat{\sigma}_o^2) - 2\pi i \hat{\zeta}^a \lambda_a(\hat{\sigma}_o)} \prod_{\alpha \in Ad(G)} 2 \sinh \pi \alpha(\hat{\sigma}_o) \prod_i \prod_{(\rho, \omega) \in \tilde{R}_i} \mathcal{Z}_{chi}^{r_i}(\rho(\hat{\sigma}_o) + \omega(\hat{m})) \quad (6.3.33)$$

where  $|\mathcal{W}|$  is the rank of the Weyl group of  $G$ .

### R-symmetry

Let us close this section with some comments about the choice of R-symmetry used in coupling the theory to the sphere. As discussed in section 1, given an R-symmetry, we can always define a new one by mixing it with a  $U(1)$  flavor symmetry of the theory. Note from (6.3.26) that the 1-loop determinant of a chiral multiplet is a holomorphic function of  $\hat{\sigma} + ir$ ,

*i.e.*, an imaginary shift of  $\hat{\sigma}$  has the same effect as changing the R-charge of the chiral. Then to implement the mixing of the R-symmetry with a  $U(1)$  flavor symmetry corresponding to a Lie algebra element  $\hat{\mu} \in \mathfrak{h}$ , we should shift:

$$\hat{m} \rightarrow \hat{m} + i\hat{\mu}, \quad (6.3.34)$$

as this will shift the R-charges of all chiral multiplets charged under this flavor symmetry appropriately. In other words, we see that the partition function is naturally a holomorphic function of the parameter  $\hat{m}$ , with the real and imaginary parts of  $\hat{m}$  determining the real mass and  $U(1)_R$  symmetry, respectively.

As discussed in the previous section, in order to compute the  $S^3$  partition function of the conformally mapped IR fixed point of the theory, we must determine the correct superconformal R-symmetry. We will see in section 6 how the  $S^3$  partition function itself gives a solution to this problem.

### 6.3.2 Squashed $S^3$

Having successfully computed the partition function on the round sphere, let us consider the more general geometries discussed in section 2.3, which we recall are defined by a metric:

$$ds^2 = f(\chi)^2 d\chi^2 + \ell_1^2 \cos^2 \chi d\varphi^2 + \ell_2^2 \sin^2 \chi d\theta^2 \quad (6.3.35)$$

Here the philosophy will be very much the same: we deform the action by a  $\delta$ -exact term which localizes the path-integral to a finite dimensional space of configurations. We will see the space we localize to is essentially the same as on the round  $S^3$ . However, although this reduces us to a gaussian theory, we must compute the spectrum of differential operators on this general background, which is a difficult problem. However, we will see that supersymmetry again helps to make this calculation quite tractable.

The first step is to determine the space of BPS configurations. From (6.2.29), noting that  $V^\mu = 0$  on the squashed sphere background, we find the bosonic piece is:

$$\mathcal{L}_{YM,bos} = \text{Tr} \left( \frac{1}{4} F^{\mu\nu} F_{\mu\nu} + \frac{1}{2} D^\mu \sigma D_\mu \sigma - \frac{1}{2} (D + \sigma H)^2 \right) \quad (6.3.36)$$

Similarly to the round sphere, the zeros of this action are constant values for  $\sigma$  and  $D$ , labeled by a Lie algebra element  $\hat{\sigma}_o$ :

$$\sigma = -D/H \equiv \frac{\hat{\sigma}_o}{\ell} = \text{constant} \quad (6.3.37)$$

where we have defined  $\ell = \sqrt{\ell_1 \ell_2}$ , and we recall  $H = -i/f$ . As on the round sphere, the chiral multiplet does not contribute additional zero modes.

Let us now compute the 1-loop determinants for such a BPS configuration.

*Chiral Multiplet*

This time we will start with the chiral multiplet. The chiral kinetic term, expanded about the BPS configuration for the gauge multiplet labeled by  $\hat{\sigma}_o$ , is:

$$\begin{aligned} \mathcal{L}_{chi} = & \partial_\mu \tilde{\phi} \partial^\mu \phi + \frac{1}{\ell^2} \tilde{\phi} (\hat{\sigma}_o^2 + \frac{r}{4} \hat{R} + r(r - \frac{1}{2}) H^2 + 2\hat{H}(r - 1) \hat{\sigma}_o) \phi \\ & - i\tilde{\psi} \gamma^\mu \nabla_\mu \psi - \frac{i}{\ell} \tilde{\psi} (\hat{\sigma}_o + (r - \frac{1}{2}) \hat{H}) \psi - \tilde{F} F \end{aligned} \quad (6.3.38)$$

where we defined  $\hat{H} = \ell H = \frac{i\ell}{f}$ , and  $\hat{R} = \ell^2 R$ , where  $R$  is the Ricci scalar associated to the metric (6.3.35). The 1-loop determinant is then given by:

$$\mathcal{Z}_{1-loop}^{chi}(\hat{\sigma}_o) = \prod_{\rho \in R} \left( \frac{\det \mathcal{O}_F(\rho(\hat{\sigma}_o))}{\det \mathcal{O}_B(\rho(\hat{\sigma}_o))} \right)^{1/2} \quad (6.3.39)$$

where:

$$\begin{aligned} \mathcal{O}_B(\hat{\sigma}) &= -\nabla^2 + \frac{1}{\ell^2} (\hat{\sigma}^2 + \frac{r}{4} \hat{R} + r(r - \frac{1}{2}) H^2 + 2\hat{H}(r - 1) \hat{\sigma}) \\ \mathcal{O}_F(\hat{\sigma}) &= -i\gamma^\mu \nabla_\mu - \frac{i}{\ell} (\hat{\sigma} + (r - \frac{1}{2}) \hat{H}) \end{aligned} \quad (6.3.40)$$

The determinants of these operators on such a general background as the one we are considering here would be quite difficult to compute. However, supersymmetry turns out to pair many of the bosonic and fermionic modes, leading to a large cancellation in (6.3.39), and so we need only to find the unpaired modes [20, 28, 29].

To see how this works, it is useful to reorganize the fields in the chiral multiplet as:

$$\begin{aligned} \varphi_e &\equiv \phi & \varphi'_e &\equiv 2(\tilde{\zeta}\zeta)F - 2i\tilde{\zeta}\gamma^\mu\tilde{\zeta}D_\mu\phi \\ \varphi_o &\equiv \sqrt{2}\tilde{\zeta}\psi, & \varphi'_o &\equiv \sqrt{2}\zeta\psi \end{aligned} \quad (6.3.41)$$

Then, defining  $\mathcal{Q} = \delta_\zeta + \delta_{\tilde{\zeta}}$ , the supersymmetry transformations can be summarized as:

$$\mathcal{Q}\varphi_{e,o} = \varphi'_{o,e}, \quad \mathcal{Q}\varphi'_{e,o} = \mathcal{H}\varphi_{o,e} \quad (6.3.42)$$

where:

$$\mathcal{H} = \mathcal{Q}^2 = iK^\mu D_\mu + i\sigma\phi - \mathcal{R}H \quad (6.3.43)$$

Here  $\varphi_{e,o}$  take values in the same vector space, which we will denote  $\mathcal{V}_0$ , consisting of scalar fields on  $S_b^3$  of R-charge  $r$ , and similarly  $\varphi_{e',o'}$  take values in  $\mathcal{V}_1$ , consisting of scalar fields of R-charge  $r - 2$ . Now we can write the  $\mathcal{Q}$ -exact kinetic term as:

$$\mathcal{L}_{chi} = \begin{pmatrix} \tilde{\varphi}_e & \tilde{\varphi}_{e'} \end{pmatrix} \mathcal{O}_B \begin{pmatrix} \varphi_e \\ \varphi_{e'} \end{pmatrix} + \begin{pmatrix} \tilde{\varphi}_o & \tilde{\varphi}_{o'} \end{pmatrix} \mathcal{O}_F \begin{pmatrix} \varphi_o \\ \varphi_{o'} \end{pmatrix} \quad (6.3.44)$$

where one can show that:

$$\mathcal{O}_B = \begin{pmatrix} \mathcal{D}_{00} & \mathcal{D}_{01} \\ \mathcal{D}_{10} & \mathcal{D}_{11}\mathcal{H}_1 \end{pmatrix}, \quad \mathcal{O}_F = \begin{pmatrix} \mathcal{D}_{00}\mathcal{H}_0 & \mathcal{D}_{01} \\ \mathcal{D}_{10} & \mathcal{D}_{11} \end{pmatrix} \quad (6.3.45)$$

where  $\mathcal{D}_{ab}$  are certain differential operators, and the subscripts are to emphasize which spaces the operators act on. Supersymmetry implies these operators commute with  $\mathcal{H}$ , in the sense that:

$$[\mathcal{D}_{00}, \mathcal{H}_0] = 0, \quad [\mathcal{D}_{11}, \mathcal{H}_1] = 0, \quad \mathcal{D}_{10}\mathcal{H}_0 = \mathcal{H}_1\mathcal{D}_{10}, \quad \mathcal{D}_{01}\mathcal{H}_1 = \mathcal{H}_0\mathcal{D}_{01} \quad (6.3.46)$$

Now if we decompose:

$$\mathcal{V}_0 = \ker_{\mathcal{D}_{01}} \oplus \mathcal{V}_0^\perp, \quad \mathcal{V}_1 = \text{coker}_{\mathcal{D}_{01}} \oplus \mathcal{V}_1^\perp \quad (6.3.47)$$

then  $\mathcal{D}_{01}$  acts as an isomorphism between  $\mathcal{V}_0^\perp$  and  $\mathcal{V}_1^\perp$ , and a short linear algebra argument shows that the contributions from these subspaces cancel in (6.3.39). Then we are left with:

$$\mathcal{Z}_{1-loop} = \left( \frac{\det_{\ker_{\mathcal{D}_{01}}}(\mathcal{D}_{00}\mathcal{H}_0) \det_{\text{coker}_{\mathcal{D}_{01}}}(\mathcal{D}_{11})}{\det_{\ker_{\mathcal{D}_{01}}}(\mathcal{D}_{00}) \det_{\text{coker}_{\mathcal{D}_{01}}}(\mathcal{D}_{11}\mathcal{H}_1)} \right)^{1/2} = \left( \frac{\det_{\ker_{\mathcal{D}_{01}}}(\mathcal{H}_0)}{\det_{\text{coker}_{\mathcal{D}_{01}}}(\mathcal{H}_1)} \right)^{1/2} \quad (6.3.48)$$

Note we have simplified the problem considerably: rather than compute the spectrum of a second order differential operator on the entire space of fields, we need only compute the spectrum of the first order differential operator  $\mathcal{H}$  on the subspace of fields annihilated by  $\mathcal{D}_{01}$  or its adjoint,  $\mathcal{D}_{10}$ . These are given explicitly by:

$$\mathcal{D}_{01} = -i\zeta\gamma^\mu\zeta D_\mu, \quad \mathcal{D}_{10} = i\tilde{\zeta}\gamma^\mu\tilde{\zeta} D_\mu \quad (6.3.49)$$

Let us look for solutions to  $\mathcal{D}_{01}\phi = 0$  of the form  $\phi = g_{m,n}(\chi)e^{im\varphi+n\theta}$ . This gives a first order ODE for  $g_{m,n}(\chi)$ :

$$\left( \frac{\ell}{f} \frac{d}{d\chi} - \frac{b \sin \chi}{\cos \chi} (m - rA_\theta^{(R)}) - \frac{\cos \chi}{b \sin \chi} (n + rA_\phi^{(R)}) \right) g_{m,n} = 0 \quad (6.3.50)$$

which implies that its behavior near  $\chi = 0, \frac{\pi}{2}$  is:

$$g_{m,n}(\chi) \sim \sin^m \chi \cos^n \chi \quad (6.3.51)$$

Thus regularity of the solutions imposes  $m, n \geq 0$ . One then computes the eigenvalues of  $\mathcal{H}$  as:

$$\lambda_{m,n} = \frac{1}{\ell} (mb + nb^{-1} + i\hat{\sigma} - \frac{Q}{2}(r-2)), \quad m, n \geq 0 \quad (6.3.52)$$

where recall  $b = \sqrt{\ell_1/\ell_2}$ , and  $Q = b + b^{-1}$ . A similar computation for  $\mathcal{D}_{10}$ , which acts on modes in the conjugate representation, gives:

$$\hat{\lambda}_{m,n} = \frac{1}{\ell} (mb + nb^{-1} - i\hat{\sigma} + \frac{Q}{2}r), \quad m, n \geq 0 \quad (6.3.53)$$

Thus we find:

$$\mathcal{Z}_{chi}^r(\hat{\sigma}) = \prod_{m,n} \frac{mb + nb^{-1} + i\hat{\sigma} + \frac{Q}{2}(2-r)}{mb + nb^{-1} - i\hat{\sigma} + \frac{Q}{2}r} = s_b\left(\frac{iQ}{2}(1-r) - \hat{\sigma}\right) \quad (6.3.54)$$

where the double sine function is defined in (6.3.27).

Another way to compute the ratio (6.3.39), which was utilized in [28], is to note that it is closely related to the  $\mathcal{G}$ -equivariant index of the operator  $\mathcal{D}_{01}$ :

$$\mathcal{I} = \text{Tr}_{\ker \mathcal{D}_{01}} \mathcal{H} - \text{Tr}_{\text{coker } \mathcal{D}_{01}} \mathcal{H} \quad (6.3.55)$$

where  $\mathcal{G} = U(1)_\varphi \times U(1)_\theta \times U(1)_R \times G$ , and  $\mathcal{H}$  is a particular generator in this group. This can be computed by the Atiyah-Singer index theorem, and reduces to a computation at the fixed points of the group action, which are the circles at  $\chi = 0, \frac{\pi}{2}$ . From this index one can extract the ratio of determinants in (6.3.39). We refer to [28] for the details of this computation. Note this implies the results depends only on the details of the differential operator in the neighborhood of this locus, which gives an explanation for why the ratio of determinants, and hence the partition function, does not depend on the detailed form of the metric away from this locus, and in particular on the function  $f(\chi)$ .

### *Gauge Multiplet*

For the gauge multiplet, one can proceed analogously as above, and we refer to [28, 30] for details. There is also a shortcut to the answer, which we will describe here. First we mention the useful formula:

$$\mathcal{Z}_{chi}^r(\hat{\sigma}) \mathcal{Z}_{chi}^{2-r}(-\hat{\sigma}) = 1 \quad (6.3.56)$$

This is a consequence of the fact that a superpotential term  $W = XY$  causes the chirals  $X$  and  $Y$  to gain a mass, and so they do not contribute to the low energy theory, and so must not contribute to the partition function. Such a superpotential mass restricts the gauge/flavor charges of the two chirals to be opposite, and their R-charges to sum to 2, giving rise to (6.3.56). Such a formula holds quite generally for supersymmetric partition functions of theories with a  $U(1)_R$  symmetry on various manifolds, and in various dimensions.

Now suppose we have a non-abelian gauge group  $G$ . The modes of the vector multiplet along the Cartan containing  $\hat{\sigma}_o$  are uncharged, and so contribute a numerical factor. Then, following [31], we can consider a mode corresponding to a root  $\alpha$ . If the gauge group is Higgsed such that the generator corresponding to  $\alpha$  is broken, this mode will eat a chiral multiplet charged as  $-\alpha$  and these will combine to give a massive vector multiplet, which will not contribute to the index. This chiral multiplet must have no flavor and R-charges. Thus we have the relation:

$$\mathcal{Z}_{gauge\ mode}(\alpha(\hat{\sigma}_o)) \mathcal{Z}_{chi}^{r=0}(-\alpha(\hat{\sigma}_o)) = 1 \quad (6.3.57)$$

which, combined with (6.3.56), gives:

$$\mathcal{Z}_{gauge\ mode}(\alpha(\hat{\sigma}_o)) = \mathcal{Z}_{chi}^{r=2}(\alpha(\hat{\sigma}_o)) \quad (6.3.58)$$

Again, this formula holds fairly generally for supersymmetric partition functions of theories with a  $U(1)_R$  symmetry. On the squashed sphere, since the roots come in positive/negative pairs, one can write:

$$\mathcal{Z}_{1-loop}^{gauge}(\hat{\sigma}_o) = \prod_{\alpha \in Ad(G)} \mathcal{Z}_{chi}^{r=2}(\alpha(\hat{\sigma}_o)) = \prod_{\alpha > 0} 4 \sinh \pi b \alpha(\hat{\sigma}_o) \sinh \pi b^{-1} \alpha(\hat{\sigma}_o) \quad (6.3.59)$$

Note this correctly reproduces the round sphere gauge multiplet contribution when  $b = 1$ .

### *Classical Contribution and real masses*

As on the round sphere, the only part of the original action which contributes at the BPS locus is the Chern-Simons term. We find:

$$S_{CS}[\hat{\sigma}_o] = \frac{i}{4\pi} \int \sqrt{g} d^3x Tr_{CS} \left( 2 \frac{1}{\ell^3} i \hat{H} \hat{\sigma}_o^2 \right) \quad (6.3.60)$$

One computes:

$$\int \sqrt{g} d^3x i \hat{H} = \int d\chi d\varphi d\theta \ell_1 \ell_2 \ell \sin \chi \cos \chi = 2\pi^2 \ell^3 \quad (6.3.61)$$

where we have use  $i \hat{H} = \frac{\ell}{f(\chi)}$  and  $\ell_1 \ell_2 = \ell^2$ . Thus we find, as on the round sphere:

$$S_{CS}[\hat{\sigma}_o] = \pi i Tr_{CS}(\sigma_o)^2 \quad (6.3.62)$$

One can also introduce real mass parameters and FI terms by turning on BPS configurations for background gauge fields, and they enter the partition function in an analogous way as for the round sphere. The R-charge of a chiral again appears in a complex combination with the real mass  $\hat{m}$ , and a shift of the R-symmetry is now implemented by a shift:

$$\hat{m} \rightarrow \hat{m} + \frac{iQ}{2} \hat{\mu}, \quad (6.3.63)$$

### *Putting it together*

After collecting the above ingredients and integrating over the BPS configurations labeled by  $\hat{\sigma}_o$  using the Weyl integration formula, we arrive at the final answer for the squashed sphere partition function:

$$\mathcal{Z}_{S_b^3}(\hat{\zeta}, \hat{m}) = \frac{1}{|\mathcal{W}|} \int_{\mathfrak{h}} d\hat{\sigma}_o e^{-\pi i Tr_{CS}(\hat{\sigma}_o^2) - 2\pi i \zeta^a \lambda_a(\hat{\sigma}_o)} \prod_{\alpha > 0} 4 \sinh \pi b \alpha(\hat{\sigma}_o) \sinh \pi b^{-1} \alpha(\hat{\sigma}_o) \times$$

$$\times \prod_i \prod_{(\rho, \omega) \in R_i} \mathcal{Z}_{chi}^{r_i}(\rho(\hat{\sigma}_o) + \omega(\hat{m})) \quad (6.3.64)$$

In particular, note that it depends on the geometry of the sphere only through the parameter  $b = \sqrt{\ell_1/\ell_2}$ .

### 6.3.3 Operator insertions

In addition to the partition function, we can also include operator insertions in the path integral, provided they are invariant under the supercharge we have used to localize. In this way, we can compute the expectation values of supersymmetric operators. On the round sphere, this setup is conformally equivalent to flat space, and so, provided we properly normalize the expectation values by dividing by the partition function, these results also give the expectation values of supersymmetric operators in the flat space theory.

One choice of supersymmetric operator is the scalar in a chiral multiplet, which we can see from (6.2.23) is invariant under  $\delta_{\zeta}$ . However, this will evaluate to zero on the locus  $\mathcal{M}_{BPS}$ , and so have zero expectation value.<sup>19</sup> On the other hand, there are interesting loop operators we can consider.

#### *Wilson loops*

First consider the following supersymmetric completion of a Wilson loop:

$$W = \text{Tr}_S \mathcal{P} \exp e^{i \oint_{\gamma} (A - i\sigma d|x|)} \quad (6.3.65)$$

where  $\mathcal{P} \exp$  is the path-ordered exponential, and  $S$  is the representation of  $G$  in which we take the trace. This is supersymmetric provided that the quantity in the exponent is supersymmetric. Using (6.2.22), one can check:

$$\delta_{\zeta}(A_{\mu} - i\sigma K^{\mu}) = 0 \quad (6.3.66)$$

Thus this operator is supersymmetric provided  $\gamma$  is an integral curve of the Killing vector  $K^{\mu}$ .

On the round sphere, all the integral curves of  $K^{\mu}$  close to give great circles. On a squashed sphere, recall that:

$$K \propto b \partial_{\varphi} + b^{-1} \partial_{\theta} \quad (6.3.67)$$

Thus the integral curves close for generic  $b$  only at  $\chi = 0$  and  $\chi = \frac{\pi}{2}$ , where either  $\varphi$  or  $\theta$  degenerate. For  $b^2 = p/q$  rational, they close also for generic  $\chi$ , and give  $(p, q)$  torus knots.

To compute the expectation value of a Wilson line, we evaluate it on a BPS configuration and insert this into the integral over  $\mathcal{M}_{BPS}$ . Taking the loop at  $\chi = 0$  for concreteness, we compute:

---

<sup>19</sup>We can also see this from the fact that any gauge-invariant chiral operator has positive R-charge by a unitarity argument, and so must have zero expectation value.

$$W[\hat{\sigma}_o] = \text{Tr}_S e^{\frac{1}{\ell} \oint_{\gamma} \hat{\sigma}_o d|x|} = \text{Tr}_S e^{2\pi b \hat{\sigma}_o} \quad (6.3.68)$$

with the loop at  $\chi = \frac{\pi}{2}$  contributing a similar factor with  $b \rightarrow b^{-1}$ . Thus a Wilson loop is computed by including in (6.3.64) an additional insertion of:

$$\text{Tr}_S e^{2\pi b \pm \hat{\sigma}_o} = \sum_{\rho \in S} e^{2\pi b \pm \rho(\hat{\sigma}_o)} \quad (6.3.69)$$

### Vortex loops

In addition to Wilson loops, one can consider vortex loop operators [28, 32]. These can be defined by coupling a background flavor gauge field in a certain singular BPS configuration. For example, if we place such a defect at  $\chi = 0$ , we impose

$$F_{BG} = \frac{1}{\ell_1} \hat{\alpha} \frac{\delta(\chi)}{\chi}, \quad D_{BG} = \frac{i}{\ell_1} \hat{\alpha} \frac{\delta(\chi)}{\chi} \quad (6.3.70)$$

where  $\hat{\alpha}$  is an element of the Lie algebra of the flavor symmetry. The delta function for  $F_{BG}$  imposes that the background gauge field has a holonomy  $e^{2\pi i \hat{\alpha}}$  around the loop at  $\chi = 0$ . Equivalently, the periodicity of modes of chiral multiplets which are charged under this symmetry are shifted. For example, a scalar mode transforming in a weight  $\omega$  of the flavor symmetry group will have:

$$\phi(\chi, \varphi + 2\pi, \theta) = e^{2\pi i \omega(\hat{\alpha})} \phi(\chi, \varphi, \theta), \Rightarrow \phi(\chi, \varphi, \theta) = \sum_{m,n} \phi_{m,n}(\chi) e^{im\varphi + n\theta}, \quad m - \omega(\hat{\alpha}), n \in \mathbb{Z} \quad (6.3.71)$$

Since this background is supersymmetric, the same cancellation argument used in section 3.2 holds, and one finds a contribution only from modes in the (co)kernel of  $\mathcal{D}_{oe}$ . However, because of the shift in the quantization of  $m$ , the eigenvalues are now (considering a mode with weight  $\rho$  under the gauge group and  $\omega$  under the flavor symmetry group):

$$\begin{aligned} \lambda_{m,n} &= \frac{1}{\ell} ((m + \omega(\hat{\alpha}))b + nb^{-1} + i\rho(\hat{\sigma}_o) - \frac{Q}{2}(r-2)), \quad m, n \in \mathbb{Z}_{\geq 0} \\ \hat{\lambda}_{m,n} &= \frac{1}{\ell} ((m - \omega(\hat{\alpha}))b + nb^{-1} - i\rho(\hat{\sigma}_o) + \frac{Q}{2}r) \end{aligned} \quad (6.3.72)$$

where we use the fact that the modes on the second line are in the conjugate representation, and so the quantization of  $m$  is shifted oppositely. Thus the 1-loop determinant for the chiral multiplet is modified to:

$$\mathcal{Z}_{1-loop}(\hat{\sigma}_o; \hat{\alpha}) = \prod_{(\rho, \omega)} s_b \left( \frac{iQ}{2} (1-r) + ib\omega(\hat{\alpha}) - \rho(\hat{\sigma}_o) \right) \quad (6.3.73)$$

One can similarly define a defect loop at  $\chi = \frac{\pi}{2}$ , which is related by  $b \rightarrow b^{-1}$ .

A related observable is the supersymmetric Reyni entropy, defined in [33].

## 6.4 Lens spaces

In this section we study  $3d \mathcal{N} = 2$  theories on lens spaces. A lens space is a certain  $\mathbb{Z}_p$  quotient of  $S^3$ . Namely, if we think of the round  $S^3$  as the subset of  $\mathbb{C}^2$  defined by  $|z_1|^2 + |z_2|^2 = 1$ , then the lens space  $L(p, q)$ , for  $p, q$  relatively prime positive integers, is defined by imposing the relation:

$$(z_1, z_2) \sim (e^{2\pi i/p} z_1, e^{-2\pi i q/p} z_2) \quad (6.4.1)$$

This action is free, and the resulting quotient space is a smooth manifold.

We will restrict our attention to the spaces  $L(p, 1)$ . In this case, the  $\mathbb{Z}_p$  action is a subgroup of the  $SU(2)_r$  isometry group. Since this group commutes with the superalgebra  $\mathfrak{osp}(2|2)$  preserved on the round sphere, we expect to be able to place theories supersymmetrically on this space without too much difficulty.

In addition to this  $\mathbb{Z}_p$  quotient of the round sphere, we can also consider the quotient of the squashed geometries considered above, with metric:

$$ds^2 = f(\chi)d\chi^2 + \ell_1^2 \cos^2 \chi d\varphi^2 + \ell_2^2 \sin^2 \chi d\theta^2 \quad (6.4.2)$$

Then we get a space which is topologically  $L(p, 1)$  by imposing:

$$(\chi, \varphi, \theta) \sim (\chi, \varphi + \frac{2\pi}{p}, \theta - \frac{2\pi}{p}) \quad (6.4.3)$$

The lens space partition function is an interesting observable for a few reasons. First, it generalizes the  $S_b^3$  partition function, which is the special case  $p = 1$ , and so gives a more refined observable of a supersymmetric quantum field theory, *e.g.*, leading to richer tests of dualities [34], and more general dual supergravity geometries [35]. In addition, unlike the sphere, the lens space has non-trivial topology, and supports non-trivial gauge bundles. This means that, unlike the  $S_b^3$  partition function, the lens space partition function is sensitive to issues related to the global structure of the gauge group [36]. Finally, as we will see in section 6, the sphere, lens space, and  $S^2 \times S^1$  partition functions all arise from more a basic object, called the ‘‘holomorphic block,’’ and studying the lens space partition function can lead one to a better understanding of this more general picture. Thus let us turn now to the computation of these partition functions.

### 6.4.1 Localization on $L(p, 1)$

We can use the techniques of the previous sections to place theories supersymmetrically on these spaces, and compute their partition functions. This problem was studied in [34, 35, 37, 38].

Since these spaces are locally equivalent to the 3-sphere geometries we discussed previously, and since the supersymmetry transformations and the actions they preserve were determined by local considerations, we can carry them over to this geometry essentially unchanged. The localization argument proceeds as above, and we find that the the path integral localizes to:

$$F_{\mu\nu} = 0, \quad D_\mu \sigma = 0, \quad D + H\sigma = 0 \quad (6.4.4)$$

On  $S^3$  the first equation implied  $A_\mu = 0$ , but here we must be more careful, since  $L(p, 1)$  supports non-trivial flat connections. Namely, recall that the flat  $G$ -connections on a manifold  $\mathcal{M}$  are labeled by elements of the set:

$$\text{Hom}(\pi_1(\mathcal{M}), G) / \text{conjugation} \quad (6.4.5)$$

Since the lens space is a free  $\mathbb{Z}_p$  quotient of the simply connected space  $S^3$ , we have:

$$\pi_1(L(p, 1)) = \mathbb{Z}_p \quad (6.4.6)$$

Thus a flat connection is labeled by an element  $g \in G$  with  $g^p = 1$ , up to conjugation. Then, taking  $g$  to lie in the maximal torus, we can write:

$$g = e^{\frac{2\pi i}{p} \mathbf{m}} \quad (6.4.7)$$

where  $\mathbf{m}$  is an element of the  $\Lambda/(p\Lambda)$ , where  $\Lambda$  is the coweight lattice of  $G$ . For example, if we take  $G = U(N)$ , then we can write:

$$g = \text{diag}(e^{2\pi i \mathbf{m}_1/p}, e^{2\pi i \mathbf{m}_2/p}, \dots, e^{2\pi i \mathbf{m}_N/p}) \quad (6.4.8)$$

where  $\mathbf{m}_j \in \mathbb{Z}_p$ , and using the residual Weyl-symmetry, we can take  $\mathbf{m}_1 \leq \mathbf{m}_2 \leq \dots \leq \mathbf{m}_N$ . So the distinct flat  $U(N)$  connections on  $L(p, 1)$  are labeled by such a non-decreasing sequence of integers mod  $p$ .

The remaining equations in (6.4.4) imply that the BPS configurations are:

$$\sigma = -\frac{D}{H} \equiv \frac{\hat{\sigma}_o}{\ell} = \text{constant}, \quad [\hat{\sigma}_o, \mathbf{m}] = 0 \quad (6.4.9)$$

The last equation follows from  $D_\mu \sigma = 0$ , and means that we can take  $\hat{\sigma}_o$  and  $g$  to lie in the same Cartan. Thus the space of BPS configurations is:

$$(\mathfrak{g} \times \Lambda/(p\Lambda)) / \mathcal{W} \quad (6.4.10)$$

where  $\mathcal{W}$  is the Weyl group.

### *Classical contribution*

As on the sphere, the only piece of the original action which evaluates to a non-zero value on the BPS configurations is the Chern-Simons term. Now it gets a contribution both from the constant value of the scalars  $\sigma$  and  $D$ , as well as from the flat gauge field. The contribution from the former is simply:

$$\frac{i}{4\pi} \int \sqrt{g} d^3x \text{Tr}_{CS} \left( 2 \frac{1}{\ell^3} i \hat{H} \hat{\sigma}_o^2 \right) = \frac{\pi i}{p} \text{Tr}_{CS}(\hat{\sigma}_o^2) \quad (6.4.11)$$

which is related to (6.3.62) by a factor of  $p$ , owing to the fact that  $\text{vol}(L(p, 1)) = \text{vol}(S^3)/p$ .

To find the contribution from the flat connection labeled by  $\mathbf{m}$ , we must take extra care because the gauge field lives in a non-trivial bundle. To properly define the Chern-Simons functional on such a bundle, we should exhibit it as a boundary of a 4-manifold  $\mathcal{M}_4$  with a principal bundle, and use the relation:

$$\int_{\partial\mathcal{M}_4} \text{Tr}_{CS}(A \wedge dA + \frac{2i}{3}A \wedge A \wedge A) = \int_{\mathcal{M}_4} \text{Tr}_{CS}F \wedge F \quad (6.4.12)$$

Then, as argued in [35], we can take  $\mathcal{M}_4$  to be the total space of the bundle  $\mathcal{O}(p) \rightarrow \mathbb{CP}^1$ , and one can show:

$$S_{CS}[A] = -\frac{\pi i}{p} \text{Tr}_{CS}(\mathbf{m}^2) \quad (6.4.13)$$

Thus the total classical contribution in the matrix model is:

$$S_{CS}[\hat{\sigma}_o, \mathbf{m}] = \frac{\pi i}{p} \text{Tr}_{CS}(\hat{\sigma}_o^2 - \mathbf{m}^2) \quad (6.4.14)$$

### 1-loop determinants

Let us now compute the 1-loop determinant from fluctuations about a fixed configuration labeled by  $\hat{\sigma}_o, \mathbf{m}$ . A convenient way to proceed is to lift the actions to the covering space,  $S_b^3$ , and then impose the fields have the correct periodicity under the  $\mathbb{Z}_p$  action. Namely, for a field  $\phi$  transforming with weight  $\rho$  under the gauge group, we impose (for  $\omega$  a generator of the  $\mathbb{Z}_p$  isometry):

$$\omega \cdot \phi = e^{\frac{2\pi i}{p} \rho(\mathbf{m})} \phi \quad (6.4.15)$$

More explicitly, taking toroidal coordinates  $(\chi, \varphi, \theta)$  which are acted on by  $\omega \cdot (\chi, \varphi, \theta) = (\chi, \varphi + \frac{2\pi}{p}, \theta - \frac{2\pi}{p})$ , and expanding  $\phi$  into Fourier modes:

$$\phi(\chi, \varphi, \theta) = \phi_{m,n}(\chi) e^{im\varphi + in\theta} \quad (6.4.16)$$

this imposes:

$$\phi_{m,n}(\chi) = 0 \quad \text{unless} \quad m - n = \rho(\mathbf{m}) \pmod{p} \quad (6.4.17)$$

Now we need to compute the determinants of the differential operators which appear in the quadratic pieces of the  $Q$ -exact terms for the gauge and chiral multiplets. Fortunately, since these are locally identical to those on  $S_b^3$ , we have already done most of the work. In particular, we can use the same cancellation argument as above, and find that the only modes that contribute are those in the (co)kernel of the appropriate  $\mathcal{D}_{oe}$  operator. The eigenvalues we found were, for the chiral multiplet:

$$\lambda_{m,n} = mb + nb^{-1} + i\hat{\sigma} + \frac{Q}{2}(2 - r) \quad (6.4.18)$$

$$\hat{\lambda}_{m,n} = mb + nb^{-1} - i\hat{\sigma} + \frac{Q}{2}r$$

for  $m, n \geq 0$ . The only modification we must make here is to impose the periodicity (6.4.17). Thus if we define a modified double-sine function:

$$s_b^{(p)}(x; k) = \prod_{m,n \geq 0, m-n=k \pmod{p}} \frac{(m + \frac{1}{2})b + (n + \frac{1}{2})b^{-1} - ix}{(m + \frac{1}{2})b + (n + \frac{1}{2})b^{-1} + ix} \quad (6.4.19)$$

we find:<sup>20</sup>

$$\mathcal{Z}_{chi}^r(\hat{\sigma}_o, \mathbf{m}) = s_b^{(p)}\left(\frac{iQ}{2}(1-r) - \rho(\hat{\sigma}_o); \rho(\mathbf{m})\right) \quad (6.4.20)$$

For the gauge multiplet, one can perform a similar computation, or alternatively apply the general argument above that off-diagonal gauge multiplet modes contribute as adjoint chiral multiplets of R-charge 2, and write:

$$\mathcal{Z}_{gauge}(\hat{\sigma}_o, \mathbf{m}) = \prod_{\alpha \in Ad(G)} s_b^{(p)}(-iQ - \alpha(\hat{\sigma}_o); \alpha(\mathbf{m})) \quad (6.4.21)$$

which can be shown to simplify to:

$$\mathcal{Z}_{gauge}(\hat{\sigma}_o, \mathbf{m}) = \prod_{\alpha > 0} 4 \sinh \frac{\pi b}{p} \alpha(\hat{\sigma}_o + i\mathbf{m}) \sinh \frac{\pi b^{-1}}{p} \alpha(\hat{\sigma}_o - i\mathbf{m}) \quad (6.4.22)$$

### *Background fields*

As on  $S_b^3$ , it is natural to turn on background vector multiplets in BPS configurations coupled to flavor symmetries. In the present case, this includes a constant value for the scalar  $\sigma$ , and corresponding value for  $D$ , as on  $S_b^3$ , and this reduces to the flat space real mass parameter as the manifold is taken very large. In addition, we can turn on flat connections, labeled by an element  $\mathbf{n}$  in the coweight lattice of the flavor symmetry group, which modify the partition function in the expected way. The possibility to turn on these backgrounds is a consequence of the non-trivial topology of the manifold, and they do not have a flat space analogue.

### *Summing over BPS configurations*

Putting together the classical contribution and 1-loop piece, we must finally integrate over  $\sigma_i$  sum over all holonomies  $g$ . As on  $S^3$ , we can use the Weyl-integration formula

---

<sup>20</sup>In [39] it was suggested that an additional sign factor  $e^{\frac{\pi i}{2r}([k](r-[k])-(r-1)k^2)}$  be included in the 1-loop determinant of a chiral multiplet, where  $[k] \in \{0, \dots, r-1\}$  such that  $[k] = k \pmod{r}$ . Relatedly, in [40] it was argued that the Chern-Simons contribution (6.4.14) should have an additional sign  $(-1)^{Tr_{CS} m^2}$ . These signs are necessary to ensure factorization of the chiral multiplet partition function into holomorphic blocks (see section 6.3), but have not been derived from a localization argument.

to reduce the integral of  $\hat{\sigma}_o$  over the entire Lie algebra to one over the Cartan. However, in a sector with holonomy  $\mathbf{m}$ , the generators of the gauge group with  $\alpha(\mathbf{m}) \neq 0$  are broken, and correspondingly the Vandermonde determinant is modified to  $\prod_{\alpha>0|\alpha(\mathbf{m})=0} \alpha(\hat{\sigma}_o)^2$ . This precisely cancels the denominator of (6.4.22). Thus we find:

$$\begin{aligned} \mathcal{Z}(\hat{\zeta}, \mathbf{w}; \hat{m}, \mathbf{n}) &= \frac{1}{|\mathcal{W}|} \sum_{\mathbf{m} \in \Lambda/(\rho\Lambda)} \int_{\mathfrak{h}} d\hat{\sigma}_o e^{-\frac{\pi i}{p} \text{Tr}_{CS}(\hat{\sigma}_o^2 - \mathbf{m}^2) - \frac{2\pi i}{p} (\hat{\zeta}^a \lambda_a(\hat{\sigma}_o) - \mathbf{w}^a \lambda_a(\mathbf{m}))} \times \\ &\times \prod_{\alpha>0} 4 \sinh \frac{\pi b}{p} \alpha(\hat{\sigma}_o + i\mathbf{m}) \sinh \frac{\pi b^{-1}}{p} \alpha(\hat{\sigma}_o - i\mathbf{m}) \prod_i \prod_{(\rho, \omega) \in R_i} s_b^{(p)} \left( \frac{iQ}{2} (1 - r_i) + \rho(\hat{\sigma}_o) + \omega(\hat{m}); \rho(\mathbf{m}) + \omega(\mathbf{n}) \right) \end{aligned} \quad (6.4.23)$$

$$(6.4.24)$$

## 6.5 $S^2 \times S^1$ partition function

In this section we discuss  $3d \mathcal{N} = 2$  theories on  $S^2 \times S^1$ . As we will see, the partition function on this space has the interpretation, for conformal theories, of computing the superconformal index, which counts local operators in the flat space theory. We start, as in the previous sections, by writing backgrounds on  $S^2 \times S^1$  which preserve some supersymmetry.

### 6.5.1 Supersymmetric backgrounds

To start, let us consider the round  $S^2 \times S^1$ , with metric:<sup>21</sup>

$$ds^2 = dx^2 + d\theta^2 + \sin^2 \theta d\phi^2 \quad (6.5.1)$$

where  $x \sim x + \tau$ .

As above, to place theories supersymmetrically on this space we must choose appropriate background supergravity fields so that we can construct a solution to the Killing spinor equation (6.2.15). One option is to use the Killing vector generating translations along the  $S^1$  to construct two supercharges of opposite R-charge. From (6.2.20), we find the supergravity fields are then:

$$H = V^\mu = 0, \quad A^{(R)} = \omega_{12}^{(S^2)} \quad (6.5.2)$$

where  $\omega_{12}^{(S^2)}$  is the spin connection on  $S^2$ . This means that this background includes a unit flux through  $S^2$  for the  $U(1)_R$  gauge field; in other words, we are performing a partial topological twist along the  $S^2$  directions. In particular, we must impose that the R-charges of all fields are

---

<sup>21</sup>In this section we work in units where the radius of the  $S^2$  is one.

integers, so that they live in well-defined bundles. This background leads to the “topologically twisted index” considered in [31].

In this article we will focus instead on another background, studied in [41, 42], which has no  $R$ -symmetry flux, and is closely related to the superconformal index, as we will discuss below. To motivate the background, we can proceed as for the round  $S^3$  in section 2 and use the fact that there is a conformal transformation mapping  $\mathbb{R}^3$  to  $\mathbb{S}^2 \times \mathbb{R}$ . With some work, one finds the flat space Killing spinors map to Killing spinors which satisfy:

$$\nabla_\mu \zeta_\pm = \pm \frac{1}{2} \gamma_\mu \gamma_3 \zeta_\pm \quad (6.5.3)$$

Namely, taking a vielbein:

$$e_1 = d\theta, \quad e_2 = \sin \theta d\phi, \quad e_3 = dx \quad (6.5.4)$$

We can write:

$$\zeta_\pm = e^{\pm x/2} \left( a e^{i\phi/2} \begin{pmatrix} \cos \frac{\theta}{2} \\ \pm \sin \frac{\theta}{2} \end{pmatrix} + b e^{-i\phi/2} \begin{pmatrix} \sin \frac{\theta}{2} \\ \mp \cos \frac{\theta}{2} \end{pmatrix} \right) \quad (6.5.5)$$

Letting  $\zeta$  and  $\tilde{\zeta}$  run over these four solutions, we see can construct the 8 independent superconformal symmetries, which generate the superconformal algebra  $\mathfrak{osp}(2|2, 2)$ .

Note the  $x$ -dependence of these Killing spinors is incompatible with compactifying this space to  $S^2 \times S^1$ . We can fix this by introducing an imaginary, flat  $R$ -symmetry connection with holonomy along the  $x$ -direction, which we can arrange to leave half of the Killing spinors periodic: two of  $R$ -charge 1 and two of  $R$ -charge  $-1$ . On general grounds, two Killing spinors of opposite  $R$ -charge anti-commute to a Killing vector, and in the present case, we find that the Killing vectors are complex:

$$\tilde{\zeta} \gamma^\mu \zeta = \frac{\partial}{\partial x} \mp i \frac{\partial}{\partial \phi} \quad (6.5.6)$$

where we take  $\zeta = \zeta_+$  and  $\tilde{\zeta} = \zeta_-$ , with the top sign corresponding to  $(a, b) = (1, 0)$  and the bottom to  $(a, b) = (0, 1)$ .

These supercharges generate the subalgebra  $\mathfrak{osp}(2|2)$  of the superconformal algebra. This subalgebra does not contain dilatations, and so, as for the round  $S^3$ , we expect we can also couple non-conformal theories to this background. We can do this systematically using the supergravity analysis of section 2.2. Namely, we can read off the background supergravity fields from by comparing (6.2.15) to (6.5.3) to find:

$$H = 0, \quad V_\mu = A_\mu^{(R)} = -i \delta_{\mu 3} \quad (6.5.7)$$

Then the supersymmetry preserving actions for the gauge and chiral multiplets can be read off, and one finds:

$$\begin{aligned} \mathcal{L}_{chi} = & D_\mu \tilde{\phi} D^\mu \phi + \tilde{\phi} \left( (1 - 2r) D_3 + r(1 - r) + \sigma^2 + D \right) \phi \\ & - i \tilde{\psi} \gamma^\mu \left( D_\mu + \left( r - \frac{1}{2} \right) \delta_{\mu 3} \right) \psi - i \tilde{\psi} \sigma \psi + \sqrt{2} i (\tilde{\phi} \lambda \psi + \tilde{\psi} \tilde{\lambda} \phi) - \tilde{F} F \end{aligned} \quad (6.5.8)$$

$$\mathcal{L}_{YM} = \text{Tr} \left( \left( \frac{1}{2} \star F_\mu + D_\mu \sigma + \delta_{\mu 3} \sigma \right)^2 - \frac{1}{2} D^2 - i \tilde{\lambda} \gamma^\mu (D_\mu + \frac{1}{2} \delta_{\mu 3}) \lambda + i \tilde{\lambda} [\sigma, \lambda] \right) \quad (6.5.9)$$

One can also construct supersymmetric backgrounds for more general (but still axially symmetric) metrics on  $S^2$ , but for simplicity we will restrict our attention to the round  $S^2$ .

### 6.5.2 Localization on $S^2 \times S^1$

Next we localize the path integral. First, we observe that the Yang-Mills action (6.5.9) is written as sums of squares, and vanishes on the following BPS locus:

$$\star F_\mu + D_\mu \sigma + \delta_{\mu 3} \sigma = D = 0 \quad (6.5.10)$$

To find the solutions, note that we may turn on a constant value  $\alpha$  for  $A_3$  without affecting  $F_{\mu\nu}$ , giving rise to a holonomy  $z \equiv e^{i\tau\alpha}$  for the gauge field around the  $S^1$ . Also, we can turn a constant value of  $\sigma$  provided that  $F_{\mu\nu}$  has constant flux through  $S^2$ . This flux is quantized, labeled by an element  $\mathbf{m}$  of the coweight lattice  $\Lambda_{cw}$ , and we are led to the following space of BPS configurations:

$$A_\mu = \alpha dx + \mathbf{m} A_{Dir}, \quad \sigma = -\mathbf{m} \quad (6.5.11)$$

where  $A_{Dir}$  is the unit-flux Dirac monopole on  $S^2$ , *i.e.*,  $dA_{Dir} = \frac{1}{2} \text{vol}(S^2)$ . Here we must also impose  $[\alpha, \mathbf{m}] = 0$ , and we will take them to lie in a chosen Cartan subalgebra.

Let us fix a BPS background for the gauge multiplet, labeled by  $\alpha$  and  $\mathbf{m}$ . Then, proceeding as in section 3, we can decompose the chiral multiplet into weights  $\rho$  of the representation, and expand the action to quadratic order around this background, to find:

$$\begin{aligned} S_{chi}^{quad} = \sum_{\rho \in R} \int \sqrt{g} d^3 x \left( \tilde{\phi}_\rho (-D_3^2 - D^{(\rho(\mathbf{m}))}_i D^{(\rho(\mathbf{m}))}_i + (1 - 2r) D_3 + r(1 - r) + \rho(\mathbf{m})^2) \phi_\rho - \tilde{F} F \right. \\ \left. - i \tilde{\psi} (\gamma^i D_i^{(\rho(\mathbf{m}))} + \gamma^3 D_3 + \rho(\mathbf{m}) + (\frac{1}{2} - r) \gamma_3) \psi \right) \end{aligned} \quad (6.5.12)$$

Here we defined  $D_i^{(m)}$ ,  $i = 1, 2$ , for integer  $m$ , to be the gauge-covariant derivative on  $S^2$  with  $m$  units of magnetic flux. Also,  $D_3 = \partial_x + i\alpha$  is the gauge-covariant derivative along the  $S^1$  direction.

To compute the determinants, let us focus for simplicity on a single chiral multiplet of R-charge  $r$ , coupled to a  $U(1)$  gauge field holonomy  $e^{i\tau\alpha}$  and flux  $m$ ; the general case is a straightforward extension. Following [41, 42], we use the fact that the Laplacian and Dirac operators in the background of a magnetic flux  $m$  can be diagonalized using the so-called ‘‘monopole spherical harmonics’’ [43]:

$$Y_{j, j_3}^{(m)}, \quad j = |m|, |m| + 1, \dots, \quad j_3 = -j, -j + 1, \dots, j \quad (6.5.13)$$

For the bosons we use the relation:

$$-D_i^{(m)} D_i^{(m)} Y_{j,j_3}^{(m)} = (j(j+1) - m^2) Y_{j,j_3}^{(m)} \quad (6.5.14)$$

Expanding also in angular momenta  $2\pi in/\tau$ ,  $n \in \mathbb{Z}$ , along the  $S^1$  direction, we find the bosonic eigenvalues are:

$$\begin{aligned} \lambda_B &= ((2\pi n - \alpha)/\tau + i\frac{r}{2})^2 + j(j+1) + \frac{i(1-2r)}{\tau}(2\pi n - \alpha) + r(1-r) \\ &= (j + \frac{r}{2} + \frac{1}{\tau}(2\pi in + i\alpha))(j + 1 - \frac{r}{2} - \frac{1}{\tau}(2\pi in - i\alpha)), \quad j = |m|, |m| + 1, \dots \end{aligned} \quad (6.5.15)$$

For the fermions, we look for a solution of the form  $\begin{pmatrix} A Y_{j,j_3}^{(m+\frac{1}{2})} \\ B Y_{j,j_3}^{(m-\frac{1}{2})} \end{pmatrix}$ . For  $j \geq |m| + \frac{1}{2}$ , there are two independent solutions,  $\lambda_F^\pm$  and one finds they contribute to the determinant through a factor:

$$\lambda_F^+ \lambda_F^- = (j + \frac{1}{2} - \frac{r}{2} - \frac{1}{\tau}(2\pi in - i\alpha))(j + \frac{r}{2} + \frac{1}{\tau}(2\pi in - i\alpha)) \quad j = |m| + \frac{1}{2}, |m| + \frac{3}{2}, \dots \quad (6.5.16)$$

while for  $j = |m| - \frac{1}{2}$ , only one solution exists, with eigenvalue:

$$\lambda_F = j + \frac{r}{2} + \frac{1}{\tau}(2\pi in - i\alpha), \quad j = |m| - \frac{1}{2} \quad (6.5.17)$$

Putting this together, we are left with the following 1-loop determinant:

$$\mathcal{Z}_{chi}^r = \prod_{n \in \mathbb{Z}} \frac{\prod_{j=|m|+\frac{1}{2}}^{\infty} (j + \frac{1}{2} - \frac{r}{2} - \frac{1}{\tau}(2\pi in - i\alpha))^{2j+1} \prod_{j=|m|-\frac{1}{2}}^{\infty} (j + \frac{r}{2} + \frac{1}{\tau}(2\pi in - i\alpha))^{2j+1}}{\prod_{j=|m|}^{\infty} ((j + \frac{r}{2} + \frac{1}{\tau}(2\pi in + i\alpha))(j + 1 - \frac{r}{2} - \frac{1}{\tau}(2\pi in - i\alpha)))^{2j+1}} \quad (6.5.18)$$

As usual, there is significant cancellation between the bosons and fermions, and this simplifies to:

$$\mathcal{Z}_{1-loop}^{chiral} = \prod_{n \in \mathbb{Z}} \prod_{j=0}^{\infty} \frac{j + |m| + 1 - \frac{r}{2} - \frac{1}{\tau}(2\pi in - i\alpha)}{j + |m| + \frac{r}{2} + \frac{1}{\tau}(2\pi in - i\alpha)} \quad (6.5.19)$$

The infinite product over the  $S^1$  angular momenta can be performed using  $\prod_{n \in \mathbb{Z}} (2\pi in + z) = e^{-z/2}(1 - e^z)$ , and after some regularization, we are left with:<sup>22</sup>

---

<sup>22</sup>The phase factor was argued in [44, 45] to be necessary to correctly account for the fermion number of monopole operators in the superconformal index (see section 5.4 below); it should arise from a more careful regularization of the 1-loop determinants in the background magnetic flux. Provided the theory is free of parity anomalies, the total phase from all chiral multiplets and Chern-Simons terms in the theory will combine to give a sign.

$$\mathcal{Z}_{chi}^r(z, m; q) = e^{-i\pi m|m|/2} (q^{1-r/2} z^{-1})^{|m|/2} \prod_{j=0}^{\infty} \frac{1 - q^{1-r/2+|m|/2+j} z^{-1}}{1 - q^{r/2+|m|/2+j} z} \quad (6.5.20)$$

where we have defined  $q = e^{-\tau}$  and  $z = e^{i\tau\alpha}$ . As shown in [44], this can be conveniently rewritten as (defining  $(z; q) = \prod_{j=0}^{\infty} (1 - zq^j)$ ):

$$\mathcal{Z}_{chi}^r(z, m; q) = e^{-i\pi m^2/2} (q^{1-r/2} z^{-1})^{|m|/2} \frac{(q^{1-r/2+m/2} z^{-1}; q)}{(q^{r/2+m/2} z; q)} \quad (6.5.21)$$

One can proceed similarly to find the 1-loop contribution of the vector multiplet; we refer to [41, 42] for details. Here we will use the same shortcut as in sections 3.2 and 4 to note that this contribution is the same as that of an R-charge 2 chiral in the adjoint representation, which one computes to be:

$$\mathcal{Z}_{1-loop}^{gauge} = \prod_{\alpha \in Ad(G)} q^{-|\alpha(m)|/2} (1 - z^\alpha q^{|\alpha(m)|}) \quad (6.5.22)$$

### *Classical contribution and background fields*

As usual, the only source of a classical contribution is a Chern-Simons term. For the background in (6.5.11) the supersymmetric Chern-Simons term gets a contribution from the gauge field. A naive computation gives:

$$S_{CS} = \frac{i}{4\pi} \int_{S^2 \times S^1} \text{Tr}_{CS}(A \wedge dA) = \frac{i}{4\pi} \int_{S^2 \times S^1} \text{Tr}_{CS}(\alpha dx \wedge \text{mvol}(S^2)) = i\tau \text{Tr}_{CS}(\alpha \mathbf{m}) \quad (6.5.23)$$

More precisely, since the gauge field lives in a non-trivial bundle, one should exhibit  $S^2 \times S^1$  as the boundary of a 4-manifold and extend the bundle there, as in section 4. In [45] it was conjectured (see also footnote 20) that the correct contribution of the CS term contains an additional phase:

$$e^{-S_{CS}} = e^{-i \text{Tr}_{CS}(\tau \alpha \mathbf{m} + \pi \mathbf{m}^2)} \quad (6.5.24)$$

For example, for a  $U(N)$  gauge theory with  $\text{Tr}_{CS}$  equal to  $k$  times the trace in the fundamental representation, this leads to:

$$e^{-S_{CS}} = \prod_i (-1)^{km_i} z_i^{-km_i} \quad (6.5.25)$$

We can also couple background gauge fields to flavor symmetries and put them in fixed BPS configurations. These are labeled by a holonomy  $\mu \in H$  along the  $S^1$  and a flux  $n \in \Lambda_H$  through the  $S^2$ , where  $H$  is the flavor symmetry group and  $\Lambda_H$  is its coweight lattice. This modifies the chiral multiplet contribution in the expected way. In addition, a  $U(1)$  gauge field with holonomy  $w$  and flux  $n$  coupled to the  $U(1)_J$  topological symmetry for a dynamical  $U(1)$  gauge field, with holonomy  $z$  and flux  $m$ , leads to an insertion:

$$e^{-S_{FI}} = z^{-n} w^{-m} \quad (6.5.26)$$

*Final result*

Putting this all together, we find the  $S^2 \times S^1$  partition function is given by:

$$\begin{aligned} \mathcal{Z}_{S^2 \times S^1}(\mu, s, w, n; q) &= \sum_{m \in \Lambda_{cw}} \frac{1}{|\mathcal{W}|} \int_{\mathbb{T}^{r_G}} \prod_{i=1}^{r_G} \frac{dz_i}{z_i} e^{-S_{CS} - S_{FI}} \prod_{\alpha \in Ad(G)} q^{-|\alpha(m)|/2} (1 - z^\alpha q^{|\alpha(m)|}) \\ &\times \prod_i \prod_{(\rho, \omega) \in R_i} \mathcal{Z}_{chi}^{r_i}(z^\rho \mu^\omega, \rho(m) + \omega(s); q) \end{aligned} \quad (6.5.27)$$

### 6.5.3 Loop operators

We can also consider the expectation value of supersymmetric loop operators on  $S^2 \times S^1$ . To preserve supersymmetry, these must sit at the fixed points of the rotations of the  $S^2$ , *i.e.*, the north and south poles.

First consider the supersymmetric Wilson loop. We can place the following operators at the poles of the  $S^2$ , and wrapping the  $S^1$ , while preserving some supersymmetry:

$$W = \text{Tr}_R \mathcal{P} \exp \left( \oint (iA \mp \sigma d|x|) \right) \quad (6.5.28)$$

where the top (bottom) sign corresponds to the north (south) pole. Evaluating this on the saddle point configuration (6.5.11), we find its contribution is:

$$\sum_{\rho \in R} e^{\rho(i\alpha \pm \tau m)} = \sum_{\rho \in R} z^\alpha q^{\pm \alpha(m)} \quad (6.5.29)$$

where  $\rho$  runs over the weights of the representation  $R$ . Thus the expectation value of this Wilson loop is given by inserting the above expression in the matrix model.

One can also consider vortex loop operators on  $S^2 \times S^1$  [28]. Similarly to  $S^3$ , these correspond to turning on singular profiles for background fields in a vector multiplet coupled to a flavor symmetry generator  $\alpha \in \mathfrak{h}$ , which impose that the matter fields charged under this symmetry incur a holonomy as they wind the loop. However, note that if a loop wraps the north pole, it is also wrapping the south pole! Therefore, if we include a vortex loop corresponding to  $\alpha_+$  at the north pole and  $\alpha_-$  at the south pole, then provided there is no flux for the flavor symmetry gauge field, we must have  $\rho(\alpha_+ + \alpha_-) \in \mathbb{Z}$  for all weights of fields which appear in the theory. More generally if we include flux, this condition is modified to:

$$\rho(\alpha_+ + \alpha_- + \mathfrak{s}) \in \mathbb{Z} \quad (6.5.30)$$

The localization in this background can be performed using an index theorem [28], and much like on  $S^3$ , the result is given by shifting the argument of the flavor symmetry parameters in the partition function:

$$\langle V_{n.p.}(\alpha_+) V_{s.p.}(\alpha_-) \rangle = \mathcal{I}(\mu q^{(\alpha_+ + \alpha_-)/2}, \mathfrak{s} + \frac{1}{2}(\alpha_+ - \alpha_-); q) \quad (6.5.31)$$

### 6.5.4 Superconformal index

Given a superconformal theory in  $D$  dimensions, a useful object to study is the superconformal index [46]. This can be defined as a trace over the space of local operators of the theory which is weighted by global symmetry charges in a clever way, designed so that it receives contributions only from protected short multiplets. Under continuous deformations of the theory, short multiplets can only enter or leave the spectrum if they can combine to form long multiplets, but by construction these do not contribute to the index. Therefore the index is invariant under such continuous deformations, and this property is what underlies its usefulness.

In more detail, let us pick a supercharge  $\mathcal{Q}$ , and let  $\mathcal{F}_i$  be a complete basis of global symmetries commuting with  $\mathcal{Q}$ . Then we define:

$$\mathcal{I}(\mu_i, \beta) = \text{Tr}(-1)^F e^{\beta \delta} e^{\mu_i F_i} \quad (6.5.32)$$

where  $\delta = \{\mathcal{Q}, \mathcal{Q}^\dagger\}$ . The  $(-1)^F$  weighting signals that this is a Witten index: states which are not annihilated by  $\delta$  come in boson/fermion pairs, and cancel out of the trace, and so it only receives contribution from states annihilated by  $\delta$ ; in particular it is independent of  $\beta$ . It is also independent of continuous deformations of the theory. If one can continuously deform the theory to a weakly coupled point, one can then compute the superconformal index there, and in doing so learn about the local operators in the strongly coupled CFT one started with.

This kind of argument is very similar to the localization argument, and this is not a coincidence. Namely, by the usual state-operator correspondence in CFTs, the space of local operators can be identified with the Hilbert space of the theory on  $S^{D-1} \times \mathbb{R}$ , and the superconformal index can be interpreted as the trace over this Hilbert space with certain operator insertions. This partition function can then often be computed by a localization argument.

The superconformal index in various dimensions has had many recent applications, and is discussed in some of the accompanying review articles; we refer to Chapter 13 and Chapter 17 for more details.

Let us specialize now to three dimensional  $\mathcal{N} = 2$  SCFTs. Then the supercharges have the following global symmetry charges:<sup>23</sup>

---

<sup>23</sup>Here the conjugation operation is the one appropriate to radial quantization on  $S^2 \times \mathbb{R}$ , and relates an ordinary supercharge to a special superconformal supercharge.

|                                 | $\Delta$       | $R$ | $j_3$          | $F_a$ |
|---------------------------------|----------------|-----|----------------|-------|
| $\mathcal{Q}_1$                 | $\frac{1}{2}$  | 1   | $-\frac{1}{2}$ | 0     |
| $\mathcal{Q}_2$                 | $\frac{1}{2}$  | 1   | $\frac{1}{2}$  | 0     |
| $\tilde{\mathcal{Q}}_1$         | $\frac{1}{2}$  | -1  | $-\frac{1}{2}$ | 0     |
| $\tilde{\mathcal{Q}}_2$         | $\frac{1}{2}$  | -1  | $\frac{1}{2}$  | 0     |
| $\mathcal{Q}_1^\dagger$         | $-\frac{1}{2}$ | -1  | $\frac{1}{2}$  | 0     |
| $\mathcal{Q}_2^\dagger$         | $-\frac{1}{2}$ | -1  | $-\frac{1}{2}$ | 0     |
| $\tilde{\mathcal{Q}}_1^\dagger$ | $-\frac{1}{2}$ | 1   | $\frac{1}{2}$  | 0     |
| $\tilde{\mathcal{Q}}_2^\dagger$ | $-\frac{1}{2}$ | 1   | $-\frac{1}{2}$ | 0     |

(6.5.33)

where  $\Delta$  is the Hamiltonian on  $S^2$ ,  $R$  is the  $U(1)_R$  charge, and  $j_3$  is the Cartan charge of the  $SU(2)$  rotation group of  $S^2$ . One computes:

$$\delta = \{\mathcal{Q}_1^\dagger, \mathcal{Q}_1\} = \Delta - R - j_3 \quad (6.5.34)$$

Then, from the table, we see that the charges  $\Delta - j_3$  and  $F_a$  (as well as  $\delta$ ) all commute with  $\mathcal{Q}_1$ , and so from (6.5.32) we see the appropriate index to compute here is:

$$\mathcal{I}(q; \mu_a) = \text{Tr}(-1)^F e^{\beta(\Delta - R - j_3)} e^{\beta'(\Delta + j_3)} e^{i\rho_a F_a} \quad (6.5.35)$$

This trace will only get contributions from states with  $\Delta - R - j_3 = 0$ .

This index can also be interpreted as the partition function on  $S^2 \times S^1_\tau$ , where  $\tau = \beta + \beta'$  is the coefficient of  $\Delta$  in (6.5.35), with certain twisted boundary conditions for the fields, namely:

$$\Phi(x + \tau) \sim e^{\beta(\Delta - R - j_3)} e^{\beta'(\Delta + j_3)} e^{i\rho_a F_a} \Phi(x) \quad (6.5.36)$$

as well as periodic boundary conditions for the fermions. To make connection with the partition function computed above, let us use the freedom to choose  $\beta$  to set  $\beta = \beta'$ , so that the  $j_3$  dependence drops out, and then:

$$\Phi(x + \tau) \sim e^{\tau(\Delta - \frac{1}{2}R)} e^{i\rho_a F_a} \Phi(x) \quad (6.5.37)$$

These twisted boundary conditions can be traded for flat background gauge fields with appropriate holonomies along the  $S^1$ , namely:<sup>24</sup>

$$A_\mu^{(R)} - \frac{3}{2}V_\mu = \frac{i}{2}\delta_{3\mu}, \quad A_\mu^{flavor,a} = \frac{\rho_a}{\tau}\delta_{3\mu} \quad (6.5.38)$$

Comparing to (6.5.7) and (6.5.11), we see this is precisely the partition function we computed in the previous subsection, specialized to zero background fluxes. We have now argued that it is a protected object by two different (but related) means: 1) this compact curved background preserves some supercharges, and so the partition function can be computed by localization,

<sup>24</sup>Here the combination of background fields in the first equation is what couples to R-symmetry current in a superconformal theory [5].

and 2) it is related to a Witten index in the radially quantized theory. One can find a more general background corresponding a more general value of  $\beta$ , where the  $S^2$  will be fibered non-trivially over the  $S^1$ , but of course one will find that the partition function is independent of  $\beta$ .

However, the localization argument was somewhat more general, in that it could be defined for non-conformal theories as well. As we argued for  $S^3$ , if we use the superconformal R-symmetry to couple to the curved background, the partition function we compute using the UV description will agree with that of the conformally mapped IR CFT. Thus we can use localization to compute this quantity, and thus learn about the spectrum of local operators in the CFT.

### *Extended supersymmetry*

For 3d theories with  $\mathcal{N} = 4$  supersymmetry, there is an  $SU(2)_H \times SU(2)_C$  R-symmetry group, and the index takes the general form:

$$\mathcal{I}(\mu_a; t, q) = \text{Tr}_{\mathcal{H}_{S^2}} (-1)^F q^{\Delta - \frac{1}{2}(R_H + R_C)} t^{R_H - R_C} \mu_a^{F_a} \quad (6.5.39)$$

where  $F_a$  are the flavor symmetries of the theory which commute with the  $\mathcal{N} = 4$  algebra, and  $R_H$  and  $R_C$  are the Cartan generators of the two  $SU(2)$  R-symmetry factors. From the  $\mathcal{N} = 2$  point of view,  $t$  is simply another flavor fugacity, but it plays a special role in this context.

There are some useful limits one can define for this index, in which it simplifies significantly, and probes interesting information about the moduli spaces of these theories [49]. Namely, first consider taking  $q, t^{-1} \rightarrow 0$  while holding  $x = tq^{1/2}$  finite. In this limit we are computing:

$$\mathcal{I}(x) = \text{Tr}_{\mathcal{H}_H} (-1)^F x^{\Delta - R_C} \quad (6.5.40)$$

where  $\mathcal{H}_H$  denotes the subspace of states for which  $\Delta = R_H$ . The operators corresponding to these states are closely related to the ones which get a VEV on the Higgs branch of the theory, and it turns out to compute the Hilbert series of the Higgs branch [50]. Thus this limit is denoted the ‘‘Higgs limit’’ of the index. One can similarly define the ‘‘Coulomb limit,’’ where  $q, t \rightarrow 0$  while  $\tilde{x} = t^{-1}q^{1/2}$  is held finite, and these are exchanged under 3d mirror symmetry.

## 6.6 Applications

In this section we give a brief survey of some of the applications of these localization computations. This overview will necessarily omit many interesting topics due to lack of space, and the topics which appear may reflect the author’s biases more so than the importance of the topic.

### 6.6.1 Applications discussed in accompanying articles

Several of these applications are covered in more depth in accompanying review articles. Here we will give a very brief summary of each and refer to the accompanying articles for a more in-depth discussion and references.

#### *Large $N$ gauge theories and AdS/CFT*

The accompanying article in Chapter 7 discusses the partition functions for large  $N$  gauge theories, and applications to the AdS/CFT correspondence. The AdS/CFT correspondence provides a non-perturbative definition of quantum gravity theories by relating them to ordinary quantum field theories which live on the asymptotic boundary of spacetime. In particular, there are many explicit examples relating  $d$  dimensional supersymmetric gauge theories to string or M-theory on certain asymptotically  $AdS_{d+1}$  geometries. A characteristic feature of this duality is that it relates the strong coupling region of one side to the weak coupling region of the other; for example, in the limit where the quantum and stringy effects are small on the gravity side, the gauge theory typically has very large rank and strong coupling. Thus it can be difficult to compute quantities on both sides and thus check the duality. However, localization provides the means to perform exact computations even in strongly coupled gauge theories, and so is an extremely valuable tool in understanding this duality, and by extension, various features of string and M-theory.

In the case  $d = 3$ , the most well-studied example of the AdS/CFT correspondence involves the ABJM theory [9]. This is a CFT which has a Lagrangian description as an  $\mathcal{N} = 4$   $U(N) \times U(N)$  theory with two bifundamental hypermultiplets and Chern-Simons level  $k$  and  $-k$  for the two gauge group factors. The supersymmetry can be shown to enhance to  $\mathcal{N} = 6$  for generic  $k$ , and  $\mathcal{N} = 8$  for  $k = 1, 2$ . It provides a low energy description of  $N$  M2 branes propagating on  $\mathbb{C}^4/\mathbb{Z}_k$ . One can construct an AdS dual description by taking the large  $N$  limit. Here, one can either hold  $k$  finite, obtaining a description in terms of M-theory on  $AdS_4 \times S^7/\mathbb{Z}_k$ , or take an 't Hooft limit with  $\lambda = \frac{N}{k}$  held finite, in which case one finds type IIA string theory on  $AdS_4 \times \mathbb{CP}^3$ . In the large  $N$  and large  $\lambda$  limit the gravitational side becomes weakly coupled, and can be well described in a perturbative expansion around the appropriate supergravity theory.

To compare the supergravity predictions to the gauge theory, we can compute the partition function of ABJM theory at large  $N$ . The partition function of the ABJM theory is given by:<sup>25</sup>

$$\mathcal{Z}_{ABJM}(N, k) = \frac{1}{N!^2} \int d^N \sigma d^N \tilde{\sigma} e^{ik\pi \sum_j (\sigma_j^2 - \tilde{\sigma}_j^2)} \frac{\prod_{i < j} (2 \sinh \pi(\sigma_i - \sigma_j))^2 (2 \sinh \pi(\tilde{\sigma}_i - \tilde{\sigma}_j))^2}{\prod_{i, j} (2 \cosh \pi(\sigma_i - \tilde{\sigma}_j))^2}$$

While localization has simplified tremendously the problem of evaluating the path integral, for large  $N$  this is still a formidable integral to compute. However, mathematicians and

<sup>25</sup>In this section, for notational simplicity, we will replace  $\hat{\sigma}_o \rightarrow \sigma$  and  $\hat{m} \rightarrow m$ .

physicists have devised several techniques for evaluating large- $N$  matrix models as a systematic expansion in  $1/N$ . A convenient way to organize the computation is in terms of a genus expansion:

$$F_{ABJM}(N, k) \equiv \log \mathcal{Z}(N, k) = \sum_{g \geq 0} F_g(\lambda) g_s^{2g-2}$$

where  $\lambda = \frac{N}{k}$  is held finite, and  $g_s = \frac{2\pi i}{N\lambda}$ , so that this is a perturbative  $\frac{1}{N}$  expansion. Here  $F_0(\lambda)$  corresponds to the genus-zero free energy, and can be compared to the supergravity predictions. It can be computed exactly in terms of generalized hypergeometric functions, and interpolates between its expansion for large and small  $\lambda$ , which are given by:

$$\frac{1}{N^2} F_0(\lambda) \approx \begin{cases} -\log(2\pi\lambda) + \frac{3}{2} + 2 \log 2, & \lambda \ll 1 \\ \frac{\pi\sqrt{2}}{3\sqrt{\lambda}}, & \lambda \gg 1 \end{cases}$$

For the weak coupling limit of small  $\lambda$  we see the expected  $N^2$  scaling for the free energy of a weakly coupled gauge theory. However, for large  $\lambda$  we see the striking  $N^{3/2}$  behavior which is predicted by supergravity.

Many techniques have been developed to compute the higher genus corrections  $F_g(\lambda)$ , and much is known about the non-perturbative corrections as well. Similar computations can also be performed in other, less supersymmetric  $3d$  gauge theories with gravity duals. We refer to the accompanying article in Chapter 7 for more details and references.

#### *F-theorem and the F-maximization*

The accompanying article in Chapter 8 discusses the free energy  $F$  of a three dimensional conformal field theory, which can be defined as:

$$F = -\log |\mathcal{Z}_{S^3}|$$

This quantity plays an important role in understanding the network of RG flows between  $3d$  conformal field theories. Namely, given a flow from a UV CFT to an IR CFT, the  $F$ -theorem states that:

$$F_{UV} > F_{IR}$$

This can be used to rule out various RG flows. In particular, it implies that RG flow is irreversible, as it forbids flow from the IR CFT back to the UV CFT. Intuitively one can think of  $F$  as measuring the degrees of freedom of the theory, which one expects to decrease upon RG flow. However, unlike the analogous quantities  $a$  and  $c$  in 2 and 4 dimensions,  $F$  is not related to a local quantity, and can be non-trivial even in topological theories, which have no local degrees of freedom. The  $F$ -theorem was proven in [53] by relating this quantity to the entanglement entropy of a disk in flat space, and using the strong-subadditivity of entanglement entropy.

The above considerations hold in a general CFT, but in general the free energy is very difficult to compute. One can perform computations in a free theory, in a large  $N$  or  $\epsilon$ -expansion, or even holographically, but in a general interacting CFT one has little hope of computing  $F$ . However, in the context of  $\mathcal{N} = 2$  theories, we have seen  $\mathcal{Z}_{S^3}$ , and therefore  $F$ , can be computed exactly using localization. These  $\mathcal{N} = 2$  theories have provided a useful testing ground for the  $F$ -theorem and its implications for RG flows between  $3d$  theories.

A related application is  $F$ -maximization. Recall that to compute the  $S^3$  partition function, one must pick a  $U(1)_R$  symmetry. A general R-symmetry can be obtained by mixing the UV R-symmetry with any  $U(1)$  flavor symmetry  $F_i$  of the theory:

$$R_{t_i} = R_{UV} + \sum_i t_i F_i$$

One may perform the computation for any such choice of R-symmetry, and the answer will be some function  $\mathcal{Z}_{S^3}(t_i)$ . However, only for the unique superconformal R-symmetry, whose current sits in the same super-multiplet as the traceless stress energy tensor of the IR CFT, will the answer agree with that of the conformally coupled IR CFT. In general the superconformal R-charges of chiral fields may be quite complicated, irrational numbers, and without a prescription to find them one seems to be unable to compute the  $S^3$  partition function of the IR CFT.

Fortunately the  $S^3$  partition function itself provides the solution to this problem. Namely, it was argued in [15] that the superconformal R-symmetry is the one that extremizes  $F$ , namely:

$$\frac{\partial}{\partial t_i} F(t_i) = -\frac{\partial}{\partial t_i} \log |\mathcal{Z}_{S^3}| = 0 \quad \text{for the superconformal R-symmetry}$$

This follows because the derivatives of  $F$  are related to (integrated) 1-point functions of local operators on  $S^3$ , which must vanish in a CFT. One can also show that the second derivatives with respect to the  $t_i$  are related to 2-point functions of currents, which must be positive by unitarity, and using this one can show that  $F$  is actually (locally) maximized at the superconformal R-charge.

The  $F$ -theorem gives an algorithmic way to compute the superconformal R-symmetry of a  $3d$   $\mathcal{N} = 2$  SCFT, provided there are no accidental  $U(1)$  flavor symmetries in the IR. In this way it is analogous to  $4d$   $a$ -maximization, however, the procedure here is technically more complicated, as one is extremizing integrals of transcendental functions, rather than cubic polynomials as in  $4d$ . Note also that if one deforms the theory by adding a superpotential which breaks some flavor symmetry, then, provided there are no accidental symmetries in the IR, this reduces the space of  $t_i$ 's, and so the  $F$ -maximization procedure is bound to land us on a smaller  $F$  than in the UV theory, relating the  $F$ -maximization principle to the  $F$ -theorem.

### *3d-3d correspondence*

In Chapter 9 the so-called  $3d - 3d$  correspondence is discussed. Consider the  $6d$   $\mathcal{N} = (0, 2)$  SCFT of type  $A_{N-1}$  (there are also versions for the other ADE groups) placed on  $\mathcal{M}_3 \times S^3_b/\mathbb{Z}_k$ ,

where  $\mathcal{M}_3$  is an arbitrary 3-manifold along which we perform a certain topological twist. Then this system has two dual description, depending on whether we compactify on the  $\mathcal{M}_3$  or lens space factor:

- As  $SL(N, \mathbb{C})$  Chern-Simons theory on  $\mathcal{M}_3$  at level  $k + is$ , where  $is = k \frac{1-b^2}{1+b^2}$ .
- As a certain  $3d \mathcal{N} = 2$  SCFT, denoted by  $T_N[\mathcal{M}_3]$ , on  $S_b^3/\mathbb{Z}_k$ .

In many cases an explicit Lagrangian description for  $T_N[\mathcal{M}_3]$  can be obtained by decomposing the three manifold into a triangulation, assigning a certain building block theory to each tetrahedron, and implementing certain gluing rules to reassemble these into the full  $T_N[\mathcal{M}_3]$  theory. Different triangulations of the manifold can give rise to superficially different theories, which are then related by duality.

This correspondence is analogous to the AGT correspondence, which relates  $4d \mathcal{N} = 2$  theories to Toda theory on punctured Riemann surfaces  $\Sigma$ . In particular, the theory  $T_N[\Sigma \times S^1]$  is just the dimensional reduction of the corresponding  $4d$  theory, and in particular has  $\mathcal{N} = 4$  supersymmetry.

There are many observables one can map across this correspondence; the basic example is the partition function:

$$\mathcal{Z}_{S_b^3/\mathbb{Z}_k}[T_N[\mathcal{M}_3]] = \mathcal{Z}_{SL(N, \mathbb{C})_{k,s}}[\mathcal{M}_3]$$

This correspondence gives rise to important new connections in physics and mathematics. It leads to new perspectives on complex Chern-Simons theory, which gives rise to rich invariants of three-manifolds, and provides a useful description of three-dimensional gravity.

## 6.6.2 Dualities

We have seen that the supersymmetric partition function on a compact manifold  $\mathcal{M}_3$  is an RG-invariant observable of a theory. This means it can serve as a powerful test of IR dualities, *i.e.*, pairs of UV Lagrangian descriptions which are conjectured to flow to equivalent SCFTs in the IR. Namely, we can compute the partition function of both theories in a proposed duality using their UV description, and check whether they agree, as they must if they are indeed equivalent in the IR. If we consider the partition function as a function of generic real mass parameters associated to the global symmetries of the theories, the matching of this (in general, quite complicated) function serves as a powerful test of the duality, and in particular of the mapping of global symmetries across the duality. In some cases we can also map loop operators across the duality. In this section we give a few typical examples of such duality checks. Many others exist in the literature; see [34, 55–59] for a small sampling.

### *Mirror Symmetry*

Mirror symmetry was originally proposed in [60, 61] as a duality between  $3d \mathcal{N} = 4$  gauge theories motivated by the following type *IIB* string construction, consisting of *D5*, *D3*, and *NS5* branes arranged as follows:<sup>26</sup>

|            | 0 | 1 | 2 | 3 | 4 | 5 | 6 <sup>c</sup> | 7 | 8 | 9 |
|------------|---|---|---|---|---|---|----------------|---|---|---|
| <i>D3</i>  | x | x | x |   |   |   | x              |   |   |   |
| <i>D5</i>  | x | x | x |   |   |   |                | x | x | x |
| <i>NS5</i> | x | x | x | x | x | x |                |   |   |   |

At low energies, gravity decouples and we find an effective description as the following  $3d \mathcal{N} = 4$  gauge theory:

- For each segment of  $N$  *D3* branes between consecutive *NS5* branes, there is a  $U(N)$  gauge group factor.
- For each *NS5* brane, there is a bifundamental hypermultiplet coupled to the two corresponding adjacent  $U(N)$  factors. A displacement of the *NS5* brane in the 789 direction gives rise to a relative FI term between these factors.
- For each *D5* brane, there is a fundamental hypermultiplet in the  $U(N)$  factor corresponding to the *D3* brane it intersects. A displacement of the *D5* brane in the 345 direction gives rise to a mass for the hypermultiplet.

If we apply *S*-duality to this type *IIB* configuration, the *D5* and *NS5* branes are interchanged, and we find a quite different  $3d$  gauge theory description. These two gauge theories are then expected to flow to equivalent SCFTs in the IR. An example dual pair is shown in Figure 2. A characteristic feature of mirror symmetry is that masses and FI parameters are exchanged.

Let us check this with a supersymmetric partition function [62, 63]. The simplest example is the round 3 sphere. We've seen in (6.3.28) that for  $\mathcal{N} = 4$  theories the contributions to the matrix model simplify, and the free hypermultiplet of real mass  $m$  has partition function:

$$\mathcal{Z}_{hyp}(m) = \frac{1}{2 \cosh(\pi m)} \quad (6.6.1)$$

The simplest example of mirror symmetry is a duality between a free hypermultiplet of real mass  $m$  and a  $U(1)$  gauge theory with a single charged hypermultiplet, and FI term  $m$ . This corresponds to the identity:

$$\mathcal{Z}_{U(1)_{N_f=1}}(m) = \int d\sigma e^{2\pi i m \sigma} \frac{1}{2 \cosh \pi \sigma} = \mathcal{Z}_{hyp}(m) \quad (6.6.2)$$

which is just the statement that the hyperbolic secant is invariant under Fourier transform. This is analogous to the argument of [64] that abelian mirror symmetry is essentially a functional Fourier transform identity.

---

<sup>26</sup>Here an  $x$  denotes that the brane extends along this dimension, the superscript  $c$  denotes that the 6th dimension is compactified.

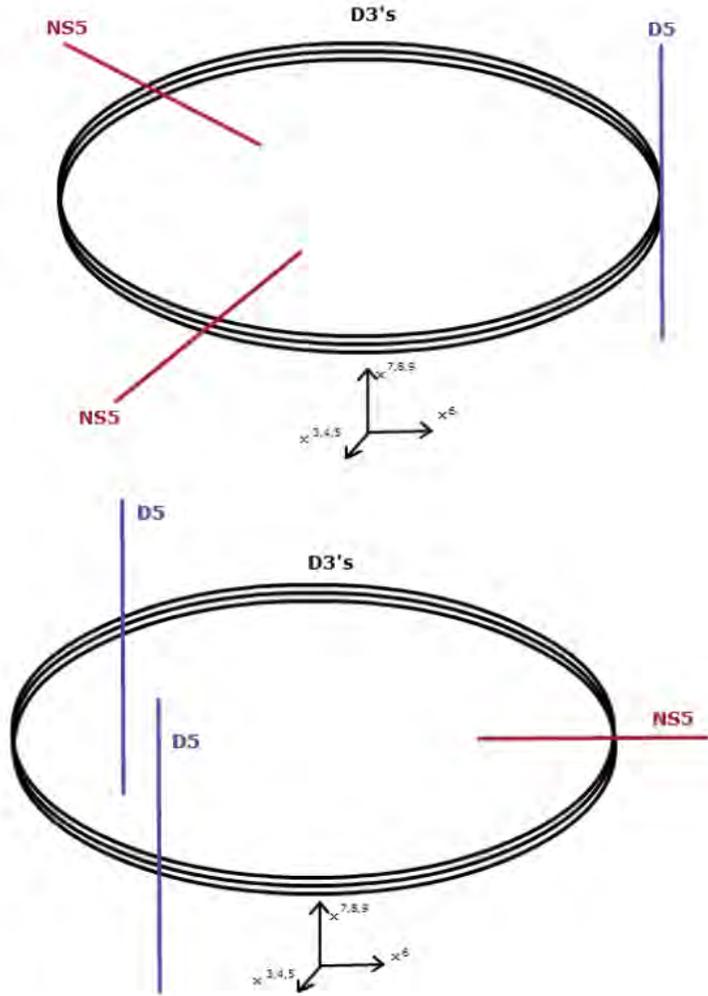

Figure 6.2: Two dual brane configurations. In the top, the low energy gauge theory is  $U(3) \times U(3)$  with bifundamental hypermultiplets and a fundamental hypermultiplet in one of the gauge factors. In the bottom, the low energy gauge theory is  $U(3)$  with an adjoint hypermultiplet and two fundamental hypermultiplets. These gauge theories are mirror dual.

For a general such gauge theory, the matrix model can be written by following the rules in section 3, *i.e.*:

$$\text{For the } ath \text{ } U(N) \text{ gauge multiplet} \rightarrow \prod_{i < j} (2 \sinh \pi(\sigma_a^i - \sigma_a^j))^2 \quad (6.6.3)$$

$$\text{For a fundamental hyper in } ath \text{ gauge group} \rightarrow \frac{1}{\prod_{i=1}^N 2 \cosh(\pi \sigma_a^i)}$$

$$\text{For the bifund. hyper connecting the } ath \text{ and } (a+1)th \text{ gauge group} \rightarrow \frac{1}{\prod_{i,j=1}^N 2 \cosh \pi(\sigma_a^i - \sigma_{a+1}^j)}$$

In this form the contribution of the D5 and NS5 branes are qualitatively different, and it is difficult to see that there is a duality exchanging them.

To make the duality manifest, we enumerate the five-branes by an index  $\alpha \in \mathbb{Z}_M$ , where  $M$  is the total number of fivebranes, and we write:

$$\mathcal{Z} = \int \prod_{\alpha=1}^M \frac{1}{N!} \sum_{\pi_\alpha \in S_N} (-1)^{\pi_\alpha} \prod_{i=1}^N d\sigma_\alpha^i d\tau_\alpha^i e^{2\pi i \tau_\alpha^i (\sigma_\alpha^i - \sigma_{\alpha+1}^{\pi_\alpha(i)})} \mathcal{I}_\alpha(\sigma_\alpha^i, \tau_\alpha^i)$$

$$\mathcal{I}_\alpha(\sigma, \tau) = \begin{cases} \frac{1}{2 \cosh(\pi\sigma)} & \text{if the } \alpha\text{th fivebrane is an D5 brane} \\ \frac{1}{2 \cosh(\pi\tau)} & \text{if the } \alpha\text{th fivebrane is a NS5 brane} \end{cases} \quad (6.6.4)$$

where  $S_N$  is the permutation group of  $N$  elements. Integrating out all of the  $\tau_\alpha^j$  variables gives delta functions which identify all  $\sigma$  variables between consecutive NS5 branes, and leads to a single  $U(N)$  gauge group for this interval. Using:

$$\sum_{\pi \in S_N} (-1)^\pi \frac{1}{2 \cosh \pi(x^i - y^{\pi(i)})} = \frac{\prod_{i < j} 2 \sinh \pi(x^i - x^j) 2 \sinh \pi(y^i - y^j)}{\prod_{i,j} 2 \cosh \pi(x^i - y^j)} \quad (6.6.5)$$

which follows from the Cauchy determinant formula, one can check this correctly reproduces the ingredients in (6.6.3). However, in the form (6.6.4) the symmetry under exchange of NS5 and D5 branes is manifest, corresponding to the exchange of  $\tau_\alpha^i$  and  $\sigma_\alpha^i$ . Thus we have shown the  $S^3$  partition functions for mirror dual theories are equal.

### *Seiberg-like dualities*

Another class of 3d dualities are often referred to as Seiberg-like dualities, as they are qualitatively similar to 4d Seiberg dualities [65]. These include the dualities of Aharony [66], Giveon-Kutasov [67], and others [45, 55, 58, 59, 68–70].

These dualities were checked at the level of supersymmetric partition functions in several papers, *e.g.*, [55, 71–73], and others. As an illustrative example, we take the  $U(N)$  version of the duality of Giveon and Kutasov, which relates the following 3d  $\mathcal{N} = 2$  gauge theories:

- *Theory A* -  $U(N_c)$  with CS term at level  $k > 0$  and  $N_f$  fundamental flavors  $(q_a, \tilde{q}_b)$ .
- *Theory B* -  $U(\hat{N}_c)$ , where  $\hat{N}_c = k + N_f - N_c$ , with CS level  $-k$ ,  $N_f$  fundamental flavors  $(Q^a, \tilde{Q}^b)$ , and  $N_f^2$  singlet mesons  $M_{ab}$ , with superpotential:

$$W = Q^a M_{ab} \tilde{Q}^b \quad (6.6.6)$$

These theories have a global symmetry  $SU(N_f) \times SU(N_f) \times U(1)_A \times U(1)_J$ . We can compute the  $S_b^3$  partition functions of these theories, refined by real mass parameters  $(m_a, \tilde{m}_a, \mu, \zeta)$  for these symmetries. One finds:

$$\mathcal{Z}_A(m_a, \tilde{m}_a, \mu, \zeta) = \tag{6.6.7}$$

$$= \frac{1}{N_c!} \int \prod_{j=1}^{N_c} d\sigma_j e^{-\pi i k \sigma_j^2 - 2\pi i \zeta \sigma_j} \prod_{a=1}^{N_f} s_b(\pm \sigma_j + m_a + \mu) \prod_{i < j} (2 \sinh \pi b^\pm (\sigma_i - \sigma_j))$$

$$\mathcal{Z}_B(m_a, \tilde{m}_a, \mu, \zeta) = \prod_{a,b=1}^{N_f} s_b(m_a + \tilde{m}_b + 2\mu) \times \tag{6.6.8}$$

$$\times \frac{1}{\hat{N}_c!} \int \prod_{j=1}^{\hat{N}_c} d\sigma_j e^{\pi i k \sigma_j^2 - 2\pi i \zeta \sigma_j} \prod_{a=1}^{N_f} s_b\left(\frac{iQ}{2} \pm \sigma_j - m_a - \mu\right) \prod_{i < j} (2 \sinh \pi b^\pm (\sigma_i - \sigma_j))$$

where we use the notation  $f(x_\pm) = f(x_+)f(x_-)$ . For theory  $B$ , the first line corresponds to the contribution of the singlets  $M_{ab}$ . Here we have parameterized the global symmetry parameters for theory  $B$ , including the R-charges, according to the mapping of these symmetries across the duality.

To compare these, one must pay attention to contact terms for global symmetries [74]. These manifest in the partition function as relative Chern-Simons terms for background gauge fields coupled to global symmetries, which must be included in order to correctly match correlation functions across the duality. In the present example, taking these into account, one finds the precise relation between the partition functions implied by the duality is [72]:

$$\mathcal{Z}_A(m_a, \tilde{m}_a, \mu, \zeta) = e^{\phi(m_a, \tilde{m}_a, \mu, \zeta)} \mathcal{Z}_B(m_a, \tilde{m}_a, \mu, \zeta)$$

$$\begin{aligned} \text{where } \phi(m_a, \tilde{m}_a, \mu, \zeta) \equiv & \frac{\pi i}{12} (k^2 + 3(k + N_f)(N_f - 2) + 2) + \pi i \zeta^2 - \frac{k\pi i}{2} \sum_a (m_a^2 + \tilde{m}_a^2) \\ & + \pi i N_f (N_f - k) \mu^2 + \pi N_f (k + N_f - 2N_c) \mu \end{aligned} \tag{6.6.9}$$

The identity of these integrals of double sine functions is highly non-trivial, and was proven relatively recently in [75]. The method of proof is to take a certain limit of identities between integrals of elliptic gamma functions, which correspond physically to identities of the  $4d$  supersymmetric index of Seiberg dual theories. Correspondingly, these  $3d$  dualities can be derived from the  $4d$  dualities by reduction on a circle [45], and we will mention this limit of the  $4d$  index below.

In addition to matching partition functions, one can match the expectation values of supersymmetric loop operators across dualities. See [28, 32, 76, 77] for some examples.

### 6.6.3 Factorization, holomorphic blocks, and Higgs branch localization

In this section we describe an interesting factorization property enjoyed by all of the partition functions discussed in this article. For example, for the squashed sphere partition function, and for a suitable class of theories, it was observed in [78] that the partition function can be written as:

$$\mathcal{Z}_{S_b^3}(m_a) = \sum_{\alpha} B_{\alpha}(x_a; q) \tilde{B}_{\alpha}(\tilde{x}_a; \tilde{q}) \quad (6.6.10)$$

where the index  $\alpha$  labels vacua of the mass-deformed theory, and  $B_{\alpha}$  (respectively,  $\tilde{B}_{\alpha}$ ) are certain holomorphic functions of  $q = e^{2\pi i b^2}$  and  $x_a = e^{2\pi i b m_a}$  (respectively,  $\tilde{q} = e^{2\pi i b^{-2}}$  and  $\tilde{x}_a = e^{2\pi i b^{-1} m_a}$ ). A similar factorization was conjectured for the supersymmetric index [44], and these were described in a unified framework in [79]. The lens space partition function was subsequently also shown to factorize similarly [39, 40], as well as the topological twisted index [39]. A remarkable fact is that in all cases, the partition functions of a given theory on any of these manifolds are built out of the same objects  $B_{\alpha}$ , the so-called ‘‘holomorphic blocks.’’

The basic observation that connects these various partition functions is that all of the corresponding spaces,  $S^3$ ,  $S^3/\mathbb{Z}_p$ , and  $S^2 \times S^1$ , admit a Heegard decomposition as a union of two solid tori,  $D^2 \times S^1$ . Namely, starting with two disjoint solid tori, whose boundaries are two-dimensional tori, we perform a large diffeomorphism on one of boundaries before gluing them together. Such large diffeomorphisms are labeled by the group  $SL(2, \mathbb{Z})$ , and for various choices of elements  $g \in SL(2, \mathbb{Z})$  we find the following topological spaces:

$$g = \text{Id} \rightarrow S^2 \times S^1, \quad g = S = \begin{pmatrix} 0 & 1 \\ -1 & 0 \end{pmatrix} \rightarrow S^3, \quad g = \begin{pmatrix} 1 & 0 \\ -p & 1 \end{pmatrix} \rightarrow S^3/\mathbb{Z}_p, \quad (6.6.11)$$

This observation is only true at the level of the topology of the spaces, however the partition functions we have computed are not topological, so extra care must be taken.

Nevertheless, one proceeds by defining a partition function on  $D^2 \times_q S^1$ , where the subscript denotes that the disk is fibered over the circle, and rotates by an angle  $-i \log q$  as one goes around the circle. In order to preserve supersymmetry, one performs a partial topological twist, *i.e.*, one turns on a background R-symmetry gauge field with flux  $\pm \frac{1}{2}$  through the  $D^2$ , the two choices being related by parity. This topological twist renders the partition function invariant under changes of the metric of the disk. Then we can deform the disk to a so-called ‘‘Melvin cigar,’’ with a long throat that is asymptotically a flat cylinder, so that the total space is asymptotically  $T^2 \times \mathbb{R}$ . The long Euclidean time evolution on the flat  $T^2$  has the effect of projecting the state to a ground state  $\alpha$  of the theory, which therefore labels the boundary conditions on this space. Finally, for each  $U(1)$  flavor symmetry factor, one may also turn on a real mass and flat connections with holonomy along the  $S^1$ , which combine into a complex quantity  $x_a$ . Then we define the holomorphic block  $B_{\alpha}$  to be the partition function on this supersymmetric background:

$$B_{\alpha}(x_a; q) = \mathcal{Z}_{D^2 \times_q S^1}(x_a; \alpha) \quad (6.6.12)$$

To make the connection to the partition functions we have computed above, we use the fact just mentioned that they are each topologically a union of two copies of  $D^2 \times S^1$ . If these two copies can be similarly deformed, by a  $Q$ -exact deformation, to two copies of the

cigar geometry above, then we can insert a complete set of states at some point in the long  $T^2 \times \mathbb{R}$  region. Since only ground states contribute, we then find an expression:

$$\sum_{\alpha} B_{\alpha}(x_a; q) B_{\alpha}(\tilde{x}_a, \tilde{q}) \quad (6.6.13)$$

where  $\tilde{q} = g \cdot q$ ,  $\tilde{x} = g \cdot x$ , and  $g$  implements the action of the large diffeomorphism, acting as:

$$g = \begin{pmatrix} a & b \\ c & d \end{pmatrix} \in SL(2, \mathbb{Z}) \quad \Rightarrow \quad q = e^{2\pi i \tau} \rightarrow \tilde{q} = e^{\pm 2\pi i \frac{a\tau + b}{c\tau + d}}, \quad x = e^{2\pi i \mu} \rightarrow \tilde{x} = e^{\pm 2\pi i \frac{\mu}{c\tau + d}} \quad (6.6.14)$$

where the sign corresponds to the option to change orientation before gluing. This argument is analogous to that of the  $tt^*$  program in  $2d$  [80], where the  $S^2$  partition function is shown to be fused from a topological and anti-topological twisted disk partition functions. Indeed, the holomorphic blocks reduce to these  $2d$  blocks as one takes the radius of the circle to zero.

To give a concrete example, consider a free chiral multiplet charged under a  $U(1)$  flavor symmetry. By itself, this theory suffers from a parity anomaly, so we add a level  $-\frac{1}{2}$  background Chern-Simons term for the flavor symmetry, as well as a flavor-R contact term. Then this theory, which is sometimes denoted  $\mathcal{T}_{\Delta}$ , has a single block, given by:

$$B_{\Delta}(x; q) = (qx^{-1}; q)_{\infty} = \begin{cases} \prod_{j=0}^{\infty} (1 - q^{j+1}x^{-1}) & |q| < 1 \\ \prod_{j=0}^{\infty} (1 - q^{-j}x^{-1})^{-1} & |q| > 1 \end{cases} \quad (6.6.15)$$

For the case of the  $S$ -fusing, which should give the  $S_b^3$  partition function, we find (taking  $b^2$  to have positive imaginary part, so that  $|q|, |\tilde{q}|^{-1} < 1$ ):

$$B_{\Delta}(x; q) B_{\Delta}(\tilde{x}; \tilde{q}) = \prod_{j=0}^{\infty} \frac{1 - q^{j+1}x^{-1}}{1 - \tilde{q}^j \tilde{x}^{-1}} = e^{\frac{\pi i}{2}(\mu - \frac{iQ}{2})^2} s_b\left(\frac{iQ}{2} - \mu\right) \quad (6.6.16)$$

with the parameters defined as below (6.6.10). This indeed correctly reproduce the  $S_b^3$  partition function of a free chiral multiplet with the chosen contact terms. On the other hand, for the identity fusing, which should give the  $S^2 \times S^1$  partition function, we have  $\tilde{q} = q^{-1}$ , and the block variables  $x$  and  $\tilde{x}$  can be shown to be related to the variables  $z$  and  $m$  in the index by  $x = zq^{-m/2}$  and  $\tilde{x} = z^{-1}q^{-m/2}$  [79]. Thus we find:

$$B_{\Delta}(x; q) B_{\Delta}(\tilde{x}; \tilde{q}) = \frac{(q^{1+m/2}z^{-1}; q)}{(q^{m/2}z; q)} \quad (6.6.17)$$

and comparing to (6.5.21), we see this correctly reproduces the index of the theory on  $S^2 \times S^1$ . A similar result holds also for the other partition functions.

In general, in a gauge theory, there are typically many blocks, and a contour integral prescription for computing them was given in [79], which can be derived using certain difference operators acting on the blocks derived from studying loop operators supported at the tip of the cigar. Subsequently the blocks were derived directly by localization in [81].

### Higgs branch localization

An alternative way to exhibit the partition functions in the factorized form (6.6.10) is by an alternative localization prescription, called ‘‘Higgs branch localization,’’ considered in [82, 83]. This is to be contrasted with the localization we studied above, which might be called ‘‘Coulomb branch localization,’’ since the BPS configurations which we localize to, and then sum over, involve a constant value for the scalar  $\sigma$ , which parameterizes the Coulomb branch in flat space.

To arrive at the Higgs branch localization, we add a new  $\delta$ -exact term (here we work on  $S_b^3$ ; a similar argument applies on the other spaces):

$$\mathcal{L}_H = t \delta \text{Tr} \left( \frac{i}{2} (\tilde{\zeta} \lambda - \tilde{\lambda} \zeta) H(\phi) \right) = t \text{Tr} \left( \left( \frac{1}{2} \star F_3 - i(D + h\sigma) \right) H(\phi) \right) + \text{fermions} \quad (6.6.18)$$

where  $H(\phi)$  is an arbitrary function of the scalar fields in the chiral multiplets of the theory, which is valued in the adjoint representation of the gauge group. By the usual argument, the addition of this term does not affect the result of the path-integral. However, it does change the set of field configurations we localize to in the  $t \rightarrow \infty$  limit. A convenient choice for  $H$  turns out to be:

$$H(\phi) = \zeta - \sum_{i,a} T_{adj}^a \tilde{\phi}_i T_{R_i}^a \phi_i \quad (6.6.19)$$

where  $\zeta$  is a real parameter, which should not appear the final answer. As shown in [83], this term, in combination with the usual  $\delta$ -exact term, has the effect of localizing to the solutions of the following equations:

$$\begin{aligned} 0 = \star F_3 + \frac{\sigma_I}{f} + H(\phi) &= \star F_1 + D_2 \sigma_I = \star F_2 - D_1 \sigma_I = D_3 \sigma_I = D_i \sigma_R & (6.6.20) \\ 0 = (\sigma_R + m_i) \phi_i &= D_3 \phi_i - i(\sigma_I + \frac{r}{f}) \phi_i = (D_1 - iD_2) \phi_i = F_i \end{aligned}$$

where we express vectors in terms of the vielbein (6.2.40), and  $\sigma = \sigma_R + i\sigma_I$ . If we look for solutions with  $F_{\mu\nu} = 0$ , these equations simplify to  $H(\phi) = (\sigma_R + m_i) \phi_i = 0$ , which are precisely the equations which would define a Higgs vacuum in flat space. For appropriate matter content, and generic real masses, these solutions are discrete, and so we find a number of such solutions equal to the number of Higgs vacua.

More generally, if we relax the condition  $F_{\mu\nu} = 0$ , we find that, in the region near the circles at  $\chi = 0$  ( $\chi = \frac{\pi}{2}$ ), the equations (6.6.20) are approximately those of a BPS (anti-)vortex on  $\mathbb{R}^2 \times S^1$ . Far from these circles the solution must take the form:

$$\phi_i = \phi_i^* e^{-im\theta - in\phi}, \quad A = -md\theta - nd\phi \quad (6.6.21)$$

where  $\phi_i^*$  is a Higgs vacuum, *i.e.*,  $H(\phi_i^*) = 0$ , and  $m, n$  are non-negative integers, which label the (anti-)vortex numbers at the  $\chi = 0$  ( $\chi = \frac{\pi}{2}$ ) circles. Thus we find an infinite tower of

such BPS vortex configurations, and one can compute the contribution to the path integral from these configurations in terms of the  $3d$  vortex partition function,  $\mathcal{Z}_{vortex}$ , and one finds, schematically:

$$\sum_{\text{Higgs vacua}} \mathcal{Z}_{vortex} \mathcal{Z}_{anti-vortex} \quad (6.6.22)$$

In general there may be other BPS configurations one must sum over (namely, ‘‘Coulomb-like’’ configurations involving a non-zero value for  $\sigma$ ), however, in cases where it is possible to mass deform the theory such that all vacua are isolated Higgs vacua, this expression computes the full partition function, and gives an alternate derivation of the factorized form (6.6.10).

Similar factorizations of partition functions exist also in  $2d$ ,  $4d$ , and  $5d$ , with the latter discussed in more detail in the accompanying review article in Chapter 16.

### 6.6.4 Limits of partition functions

In this section we consider various limits of the parameters on which the partition function depends.

#### Large real masses

Given a  $3d$   $\mathcal{N} = 2$  theory in flat space, we can turn on real mass parameters to initiate an RG flow to a new fixed point. Above, we have seen above that it is possible to turn on a curved-space analogue of real mass parameters while preserving a deformed supersymmetry algebra. These do not give rise to an RG flow to a different theory, but instead give a richer observable of the original theory, generalizing the undeformed partition function and probing the global symmetries of the theory. A natural question is whether these two kinds of real mass deformations are related.

Recall that the supersymmetric actions we have written on curved geometries had the important property that they reduced locally to the flat space actions as the size of the manifold was taken to infinity. This ensures that when we couple the flat space UV action to these geometries, we find the same result as if we had first flowed to low energies in flat space, and then coupled the IR CFT to these backgrounds. Suppose that instead we wish to take our flat space theory to be one deformed by some real mass parameters. Then, considering first the case of the round  $S^3$ , if we compare (6.1.13) and (6.2.12) we see that in order to obtain a flat space action with a finite real mass parameter  $m$  as  $\ell \rightarrow \infty$ , we must take:

$$\hat{m} = m\ell \quad (6.6.23)$$

Now the  $S^3$  partition function is no longer independent of  $\ell$ , and so if we want to study the IR fixed point of this flat space action, we must take the limit  $\ell \rightarrow \infty$ , in other words, we must study the partition function in the limit  $\hat{m} \rightarrow \infty$ . Let us see how this works in some examples.

*Chiral multiplet*

First consider a chiral multiplet which is coupled with charge  $Q$  to a dynamical gauge multiplet, with scalar  $\sigma$ , as well as to a background gauge multiplet with scalar  $M$ . Then turning on a flat space real mass for this chiral multiplet corresponds to taking the  $M \rightarrow \infty$  limit of the partition function, and one finds (generalizing now to the squashed sphere):<sup>27</sup>

$$\begin{aligned} s_b(-M - Q\sigma) \underset{M \rightarrow \infty}{\sim} \exp\left(\frac{\pi i}{2} \text{sgn}(M) \left( (M + Q\sigma)^2 - \frac{1}{12}(b^2 + b^{-2}) \right)\right) \\ = e^{\pi i Q |M| \sigma} e^{\frac{1}{2} \pi i \text{sgn}(M) Q^2 \sigma^2} e^{\frac{1}{2} \pi i \text{sgn}(M) M^2 - \frac{1}{12}(b^2 + b^{-2})} \end{aligned} \quad (6.6.24)$$

Let us compare this to what we obtain if we integrate out a charged chiral multiplet in flat space. As discussed in [4], this induces effective Chern-Simons and FI terms for the gauge multiplet:

$$\zeta_{eff} = -\frac{1}{2} Q |M|, \quad k_{eff} = -\frac{1}{2} Q^2 \text{sgn}(M) \quad (6.6.25)$$

Comparing to (6.6.24), we see this induces precisely the expected contribution of these terms in the  $S_b^3$  partition function. In addition we find a flavor-flavor contact term, which can be removed if desired by the addition of a local counterterm.

We can similarly take a large real mass limit in the supersymmetric index. From (6.5.11), turning on a BPS configuration with background flux  $n$  for a  $U(1)$  flavor symmetry sets the background fields to be (reinstating the radius  $\ell$  of the  $S^2$ , and taking  $\omega_{\mu\nu}$  as the volume form of a unit sphere):

$$F_{\mu\nu} = -\frac{1}{\ell^2} n \omega_{\mu\nu} \quad \sigma = \frac{1}{\ell} n \quad (6.6.26)$$

Thus to obtain a finite real mass,  $\sigma = m$ , in the flat space limit, we should scale:

$$n = m\ell \quad (6.6.27)$$

In this limit the effect of the background flux is negligible, and so we correctly reproduce the flat space action of a chiral multiplet with real mass  $m$ . The contribution of a charge  $Q$  chiral multiplet in the background of a dynamical gauge field configuration labeled by  $z_g$  and  $m_g$  gives:

$$\begin{aligned} \mathcal{Z}_{chi}^{r=1}(z_g^Q, Qm_g + n) &= e^{-\frac{1}{2} \pi i Q^2 m^2} (z_g^{-Q})^{\frac{|Qm_g+n|}{2}} \prod_{j=0}^{\infty} \frac{1 - q^{\frac{1}{2} + \frac{|Qm_g+n|}{2} + j} z_g^{-Q}}{1 - q^{\frac{1}{2} + \frac{|Qm_g+n|}{2} + j} z_g^Q} \\ &\underset{n \rightarrow \infty}{\sim} e^{-\frac{1}{2} \pi i Q^2 m^2} (z_g^{-Q})^{\frac{1}{2} \text{sgn}(n)(n+Qm_g)} = z_g^{-\frac{1}{2} Q |n|} e^{-\frac{1}{2} \pi i Q^2 m^2} z_g^{-\frac{1}{2} Q^2 m_g} \end{aligned} \quad (6.6.28)$$

---

<sup>27</sup>Here we take  $r = 1$  for simplicity; a more general  $r$  can be obtained by analytic continuation of  $M$  or  $\sigma$ , and will introduce additional flavor-R and/or gauge-R contact terms

which again produces the expected Chern-Simons and FI term contributions, as in (6.6.25).

### Gauge theory

The situation in a gauge theory is more complicated. For concreteness, let us consider the  $S_b^3$  partition function of a  $U(N_c)$  gauge theory with  $N_f$  flavors and no CS term. Let us turn on a real mass  $M$  for the  $N_f$ th flavor, which we will take very large. Specifically, we consider:

$$\lim_{M \rightarrow \infty} \mathcal{Z}_{U(N_c), N_f}(\mu_{N_f}, M) = \tag{6.6.29}$$

$$\lim_{M \rightarrow \infty} \frac{1}{N_c!} \int \prod_{j=1}^{N_c} \left( e^{-2\pi i \zeta \sigma_j} \left( \prod_{a=1}^{N_f-1} s_b(\pm(\sigma_j + m_a) + \mu_a) \right) s_b(\pm(\sigma_j + M) + \mu_{N_f}) \right) \prod_{i < j} 2 \sinh \pi b^\pm(\sigma_i - \sigma_j)$$

where we suppress in the argument of  $\mathcal{Z}$  the masses of the other flavors, which are remaining light, and the FI parameter.

A naive guess would be to just take the large  $M$  limit of the integrand, using the formula (6.6.24) to simplify the contribution of the massive flavor. We find the integrand becomes:

$$e^{2\pi i M N_c (\frac{iQ}{2} + \mu_{N_f})} \frac{1}{N_c!} \prod_{j=1}^{N_c} e^{-2\pi i (\zeta - \frac{iQ}{2} - \mu_{N_f}) \sigma_j} \prod_{a=1}^{N_f-1} s_b(\pm(\sigma_j + m_a) + \mu_a) \prod_{i < j} 2 \sinh \pi b^\pm(\sigma_i - \sigma_j) \tag{6.6.30}$$

which, up to an overall factor, is the integrand for a  $U(N_c)$  theory with  $N_f - 1$  flavors, as we might have expected.

However, this turns out to be incorrect, in general. Namely, when we take the limit of an integral, we must make sure we capture the dominant contribution. In some cases this contribution may remain at finite  $\sigma_j$  as  $M \rightarrow \infty$ , in which case taking the limit at the level of the integrand as we did above is justified. In the present case, a more careful analysis [45] shows that this is the case only when:

$$\frac{Q}{2}(N_f - N_c - 1) - \text{Im} \mu_{N_f} > 0 \tag{6.6.31}$$

When this is not true, one finds instead that it is appropriate to shift one of the eigenvalues,  $\sigma_{N_c} = \sigma' + M$ , and one finds the integrand in (6.6.29) becomes:<sup>28</sup>

$$\exp \left( 2\pi i (M((N_f - 1)\frac{iQ}{2} + (N_c - 1)\mu_{N_f} + \sum_{a=1}^{N_f-1} \mu_a) + \sum_{a=1}^{N_f-1} m_a(-\frac{iQ}{2} - \mu_a + \zeta - \mu_{N_f})) \right) \times$$

$$\times \frac{1}{(N_c - 1)!} \prod_{j=1}^{N_c-1} \left( e^{-2\pi i (\zeta - \mu_{N_f}) \sigma_j} \prod_{a=1}^{N_f-1} s_b(\pm(\sigma_j + m_a) + \mu_a) \right) \prod_{i < j} 2 \sinh \pi b^\pm(\sigma_i - \sigma_j)$$

<sup>28</sup>The Weyl factor  $\frac{1}{N_c!}$  has been replaced by  $\frac{1}{(N_c-1)!}$  because we have multiplied by  $N_c$  to account for the choices to shift  $\sigma_{j < N_c}$  rather than  $\sigma_{N_c}$ , which all give equivalent results

$$\times e^{-2\pi i(\zeta + \frac{iQ}{2}(N_f - N_c) - \sum_{a=1}^{N_f-1} \mu_a)\sigma'} s_b(\pm\sigma' + \mu_{N_f}) \quad (6.6.32)$$

Here we find the  $S_b^3$  partition function of a  $U(1) \times U(N_c - 1)$  theory. The  $U(1)$  sector, parameterized by  $\sigma'$ , is decoupled from the  $U(N_c - 1)$  sector, and one can dualize it into singlet chiral multiplets. Thus we find a  $U(N_c - 1)$  theory with  $N_f - 1$  flavors, and some additional singlets. To summarize, we have found that:

$$\mathcal{Z}_{U(N_c), N_f}(M, \mu_{N_f}) \underset{M \rightarrow \infty}{\sim} \begin{cases} e^{f_1(M, \mu_{N_f})} \mathcal{Z}_{U(N_c), N_f-1} & (6.6.31) \text{ satisfied} \\ e^{f_2(M, \mu_{N_f})} \mathcal{Z}_{U(N_c-1), N_f-1} & (6.6.31) \text{ not satisfied} \end{cases} \quad (6.6.33)$$

where  $f_i$  are simple divergent factors, which can be stripped off in either case to obtain a finite answer.

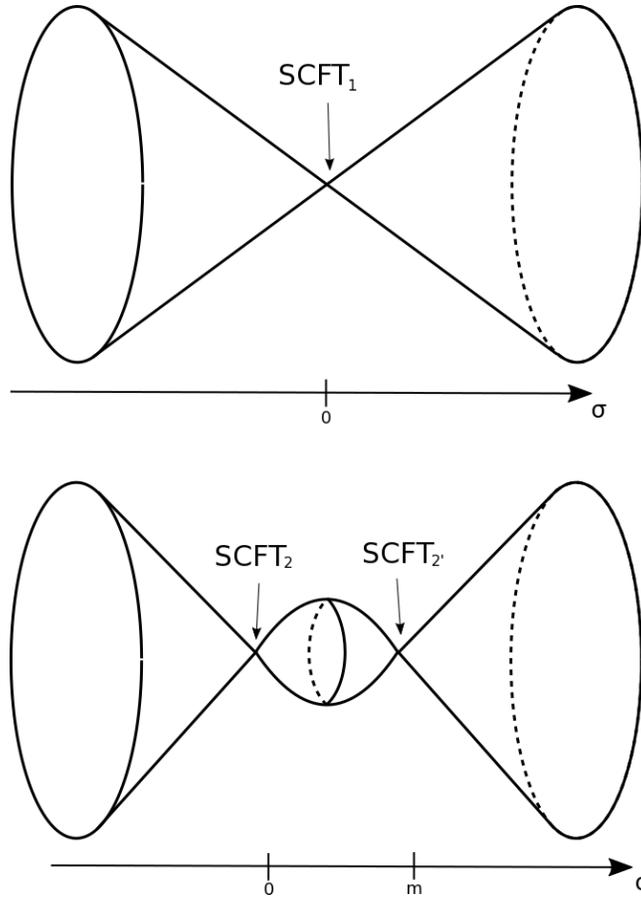

Figure 6.3: In the top, the Coulomb branch of the undeformed theory, with a single interacting fixed point at  $\sigma_j = 0$ . In the bottom, the Coulomb branch of the theory with a real mass  $m$ , which deforms the moduli space, and there are now two points with non-trivial SCFTs.

To understand the physics of these two possible limits, note that turning on a real mass parameter in flat space typically deforms the moduli space of the theory, and the resulting

moduli space may have multiple points where an interacting SCFT resides (see Figure 3). In the present example, when we turn on a finite real mass  $m$  deformation in flat space, the moduli space is deformed and two interacting fixed points appear, one at  $\sigma = \text{diag}(0, \dots, 0)$ , and one at  $\sigma = \text{diag}(0, \dots, -m)$ . The low energy theories describing these two points are precisely the two we have found above. Depending on the inequality, one or the other of these SCFTs will have the dominant contribution to the  $S_b^3$  partition function in the large real mass limit.

If we start with a pair of dual theories and add dual real mass deformations, there must exist a mapping of the resulting SCFTs which relates them by duality. This can be a useful method for producing new dualities from known ones [45, 85, 86]. In this example, the original theory has an Aharony dual description as a  $U(\hat{N}_c)$  theory with  $N_f$  flavors, where  $\hat{N}_c = N_f - N_c$ , and taking the corresponding limit there one finds:

$$\lim_{M \rightarrow \infty} \mathcal{Z}_{U(\hat{N}_c), N_f}(M, \mu_{N_f}) = \begin{cases} e^{f_1(M, \mu_{N_f})} \mathcal{Z}_{U(\hat{N}_c-1), N_f-1} & \text{(6.6.31) satisfied} \\ e^{f_2(M, \mu_{N_f})} \mathcal{Z}_{U(\hat{N}_c), N_f-1} & \text{(6.6.31) not satisfied} \end{cases} \quad (6.6.34)$$

The duality of the original theories implies their  $S_b^3$  partition functions are equal for all  $M$ . Then if we are in the case where (6.6.31) is satisfied, for example, then we see the divergent factors on the two sides agree and can be stripped off, and taking the  $M \rightarrow \infty$  limit we obtain an identity:

$$\mathcal{Z}_{U(N_c), N_f} = \mathcal{Z}_{U(N_f - N_c - 1), N_f} \quad (6.6.35)$$

which correctly reproduces the identity for a new Aharony dual pair with  $N_f - 1$  flavors. When (6.6.31) is not satisfied, we find the identity for a different dual pair. Note that, in order to correctly obtain the duality with  $N_f - 1$  flavors, it was crucial to understand the multiple saddles in the  $M \rightarrow \infty$  limit of the partition function. In particular, taking the naive limit on both sides would have led us to an incorrect duality.

## Dimensional reduction

As a final application, we consider limits of supersymmetric partition functions which connect theories in different dimensions.

First, we consider the supersymmetric index for four dimensional theories with  $\mathcal{N} = 1$  supersymmetry. This is reviewed in the accompanying article in Chapter 13. The index can be written as a trace over states on  $S^3$ :

$$\mathcal{I}(p, q, \mu_a) = \text{Tr}(-1)^F p^{j_\ell + j_r - \frac{R}{2}} q^{j_\ell - j_r - \frac{R}{2}} \prod_a \mu_a^{F_a} \quad (6.6.36)$$

where  $j_\ell$  and  $j_r$  are the Cartan of the  $SU(2)_\ell$  and  $SU(2)_r$  isometries of  $S^3$ ,  $R$  is the R-symmetry, and  $F_a$  are flavor fugacities. The index of a chiral multiplet charged under a symmetry with fugacity  $z$  is given by the elliptic gamma function,  $\Gamma_e(z; p, q)$ .

As discussed in Chapter 13, the index can also be interpreted as a partition function on  $S_b^3 \times S_\tau^1$ , where  $\tau$  is the ratio of the radius of the  $S^1$  to that of the  $S_b^3$ , and is related to the parameters above by [45, 87]:

$$p = e^{2\pi i \tau b}, \quad q = e^{2\pi i \tau b^{-1}}, \quad \mu_a = e^{2\pi i \tau m_a} \quad (6.6.37)$$

where  $m_a$  is the  $A_4$  component of background gauge field coupled to the flavor symmetry  $F_a$ . If we now send the radius  $\tau$  to zero, we find, for a chiral multiplet [87–89]:

$$\Gamma_e(z = e^{2\pi i \tau \sigma}, p = e^{2\pi i \tau b}, q = e^{2\pi i \tau b^{-1}}) \rightarrow e^{\frac{\pi i}{6\tau}(\sigma - Q)} s_b(\sigma) \quad (6.6.38)$$

More generally, one can consider this limit for a gauge theories, in which case the compact integral over the gauge fugacities  $z_i$  in  $4d$  descends to the non-compact integral over  $\sigma_i$  as  $\tau \rightarrow 0$ , and we recover the dimensionally reduced theory, with however a constraint on their real mass parameters owing to anomalies in four dimensions. This constraint can be attributed to a superpotential which is generated when we compactify the four dimensional theories on a circle [45]. If we start with a dual pair of theories in four dimensions, taking this limit implies the identity of their  $3d$  reductions, with this superpotential term.

One can similarly consider a limit of the partition function of a  $4d$   $\mathcal{N} = 1$  theory on  $L(p, 1) \times S_\tau^1$  as  $\tau \rightarrow 0$ , and we recover the partition function on  $L(p, 1)$ , up to a simple divergent factor [38].

We can also take limits starting from three dimensions. First consider the  $S^2 \times S^1$  partition function. Then we expect the limit where the radius of the  $S^1$  goes to zero to give the partition function on  $S^2$ . To see this for a chiral multiplet, recall that its  $S^2 \times S^1$  index is:

$$\mathcal{I}_{chi}(z, m; q) = e^{-\frac{1}{2}\pi i m^2} (q^{\frac{1-r}{2}} z^{-1})^{\frac{m}{2}} \frac{(q^{1-\frac{r}{2}+\frac{m}{2}} z^{-1}; q)}{(q^{\frac{r}{2}+\frac{m}{2}} z; q)} \quad (6.6.39)$$

where we recall  $(z; q) = \prod_{j=0}^{\infty} (1 - zq^j)$ . Then writing  $q = e^{-\tau}$ ,  $z = e^{i\tau\eta}$ , and using the identity [90]:

$$\lim_{z \rightarrow 1} \frac{(z^s; z)}{(z^t; z)} (1 - z)^{s-t} = \frac{\Gamma(t)}{\Gamma(s)} \quad (6.6.40)$$

we find:

$$\mathcal{I}_{chi}(z, m; q) \xrightarrow{\tau \rightarrow 0} \tau^{2i\eta+1-r} e^{-\frac{1}{2}\pi i m^2} \frac{\Gamma(\frac{r}{2} - i\eta - \frac{m}{2})}{\Gamma(1 - \frac{r}{2} + i\eta - \frac{m}{2})} \quad (6.6.41)$$

As described in the accompanying article in Chapter 3, the ratio of gamma functions on the RHS describes the contribution of a chiral multiplet on  $S^2$ , and there is an additional divergent factor arising from integrating out the KK modes. For a gauge theory, the finite integral over the holonomy decompactifies into a real integral over  $\sigma$ , much as in the limit of the  $4d$  index. In addition, the infinite sum over monopole fluxes remains, giving a similar infinite sum over fluxes which appears in the  $S^2$  partition function.

We can also start with the lens space  $S^3/\mathbb{Z}_p$ , and consider the  $p \rightarrow \infty$  limit. In this limit, the circle fiber of the lens space shrinks to zero size, and so we again expect the geometry to approach that of  $S^2$ . Thus one expects the  $p \rightarrow \infty$  limit of the lens space partition function to go over to the partition function on  $S^2$  [90]. Indeed, recall the lens space partition function of a chiral multiplet:

$$s_b^{(p)}(iQ(1-r) + \sigma; \mathbf{m}) = \prod_{m, n \geq 0, m+n=\mathbf{m} \pmod{p}} \frac{(m + \frac{1}{2})b + (n + \frac{1}{2})b^{-1} - i(iQ(1-r) + \sigma)}{(m + \frac{1}{2})b + (n + \frac{1}{2})b^{-1} + i(iQ(1-r) + \sigma)} \quad (6.6.42)$$

we see that, as  $p \rightarrow \infty$ , this becomes a single infinite product over  $k \geq 0$ , where

$$n = m - \mathbf{m} = k, \quad \mathbf{m} \geq 0, \quad m = n + \mathbf{m} = k, \quad (6.6.43)$$

and so:

$$s_b^{(p \rightarrow \infty)}(iQ(1-r) + \sigma; \mathbf{m}) = \prod_{k \geq 0} \frac{k + \frac{|\mathbf{m}|}{2} + 1 - \frac{r}{2} + i\sigma}{k + \frac{|\mathbf{m}|}{2} + \frac{r}{2} - i\sigma} \quad (6.6.44)$$

which again reproduces the  $S^2$  partition function of a chiral multiplet. For a gauge theory, as we take  $p \rightarrow \infty$ , the finite sum over  $\mathbf{m}$  gives rise to the infinite sum over monopole fluxes on  $S^2$ .

## Acknowledgements

The author would like to thank Ofer Aharony, Anton Kapustin, Nathan Seiberg, Shlomo Razamat, and Itamar Yaakov for collaborations on some of the work discussed in this article. This research was supported in part by the National Science Foundation under Grant No. NSF PHY11-25915.

## References

- [1] V. Pestun and M. Zabzine, eds., *Localization techniques in quantum field theory*, vol. xx. Journal of Physics A, 2016. 1608.02952. <https://arxiv.org/src/1608.02952/anc/LocQFT.pdf>, <http://pestun.ihes.fr/pages/LocalizationReview/LocQFT.pdf>.
- [2] E. Witten, “Topological Quantum Field Theory,” *Commun. Math. Phys.* **117** (1988) 353.
- [3] V. Pestun, “Localization of gauge theory on a four-sphere and supersymmetric Wilson loops,” *Commun. Math. Phys.* **313** (2012) 71–129, [arXiv:0712.2824](https://arxiv.org/abs/0712.2824) [hep-th].
- [4] O. Aharony, A. Hanany, K. A. Intriligator, N. Seiberg, and M. J. Strassler, “Aspects of N=2 supersymmetric gauge theories in three-dimensions,” *Nucl. Phys.* **B499** (1997) 67–99, [arXiv:hep-th/9703110](https://arxiv.org/abs/hep-th/9703110) [hep-th].
- [5] C. Closset, T. T. Dumitrescu, G. Festuccia, and Z. Komargodski, “Supersymmetric Field Theories on Three-Manifolds,” *JHEP* **05** (2013) 017, [arXiv:1212.3388](https://arxiv.org/abs/1212.3388) [hep-th].

- [6] D. Gaiotto and X. Yin, “Notes on superconformal Chern-Simons-Matter theories,” *JHEP* **08** (2007) 056, [arXiv:0704.3740 \[hep-th\]](#).
- [7] D. Gaiotto and E. Witten, “S-Duality of Boundary Conditions In N=4 Super Yang-Mills Theory,” *Adv. Theor. Math. Phys.* **13** (2009) no. 3, 721–896, [arXiv:0807.3720 \[hep-th\]](#).
- [8] D. Gaiotto and E. Witten, “Janus Configurations, Chern-Simons Couplings, And The theta-Angle in N=4 Super Yang-Mills Theory,” *JHEP* **06** (2010) 097, [arXiv:0804.2907 \[hep-th\]](#).
- [9] O. Aharony, O. Bergman, D. L. Jafferis, and J. Maldacena, “N=6 superconformal Chern-Simons-matter theories, M2-branes and their gravity duals,” *JHEP* **10** (2008) 091, [arXiv:0806.1218 \[hep-th\]](#).
- [10] O. Aharony, O. Bergman, and D. L. Jafferis, “Fractional M2-branes,” *JHEP* **11** (2008) 043, [arXiv:0807.4924 \[hep-th\]](#).
- [11] J. Bagger and N. Lambert, “Modeling Multiple M2’s,” *Phys. Rev.* **D75** (2007) 045020, [arXiv:hep-th/0611108 \[hep-th\]](#).
- [12] A. Gustavsson, “Algebraic structures on parallel M2-branes,” *Nucl. Phys.* **B811** (2009) 66–76, [arXiv:0709.1260 \[hep-th\]](#).
- [13] L. Rozansky and E. Witten, “HyperKahler geometry and invariants of three manifolds,” *Selecta Math.* **3** (1997) 401–458, [arXiv:hep-th/9612216 \[hep-th\]](#).
- [14] A. Kapustin, B. Willett, and I. Yaakov, “Exact Results for Wilson Loops in Superconformal Chern-Simons Theories with Matter,” *JHEP* **03** (2010) 089, [arXiv:0909.4559 \[hep-th\]](#).
- [15] D. L. Jafferis, “The Exact Superconformal R-Symmetry Extremizes Z,” *JHEP* **05** (2012) 159, [arXiv:1012.3210 \[hep-th\]](#).
- [16] N. Hama, K. Hosomichi, and S. Lee, “Notes on SUSY Gauge Theories on Three-Sphere,” *JHEP* **03** (2011) 127, [arXiv:1012.3512 \[hep-th\]](#).
- [17] G. Festuccia and N. Seiberg, “Rigid Supersymmetric Theories in Curved Superspace,” *JHEP* **06** (2011) 114, [arXiv:1105.0689 \[hep-th\]](#).
- [18] T. Dumitrescu, “An Introduction to Supersymmetric Field Theories in Curved Space,” *Journal of Physics A* **xx** (2016) 000, [1608.02957](#).
- [19] C. Closset, T. T. Dumitrescu, G. Festuccia, and Z. Komargodski, “The Geometry of Supersymmetric Partition Functions,” *JHEP* **01** (2014) 124, [arXiv:1309.5876 \[hep-th\]](#).
- [20] N. Hama, K. Hosomichi, and S. Lee, “SUSY Gauge Theories on Squashed Three-Spheres,” *JHEP* **05** (2011) 014, [arXiv:1102.4716 \[hep-th\]](#).
- [21] Y. Imamura and D. Yokoyama, “N=2 supersymmetric theories on squashed three-sphere,” *Phys. Rev.* **D85** (2012) 025015, [arXiv:1109.4734 \[hep-th\]](#).
- [22] D. Martelli and J. Sparks, “The gravity dual of supersymmetric gauge theories on a biaxially squashed three-sphere,” *Nucl. Phys.* **B866** (2013) 72–85, [arXiv:1111.6930 \[hep-th\]](#).
- [23] J. Nian, “Localization of Supersymmetric Chern-Simons-Matter Theory on a Squashed  $S^3$  with  $SU(2) \times U(1)$  Isometry,” *JHEP* **07** (2014) 126, [arXiv:1309.3266 \[hep-th\]](#).
- [24] C. Imbimbo and D. Rosa, “Topological anomalies for Seifert 3-manifolds,” *JHEP* **07** (2015) 068, [arXiv:1411.6635 \[hep-th\]](#).
- [25] J. Kallen, “Cohomological localization of Chern-Simons theory,” *JHEP* **08** (2011) 008, [arXiv:1104.5353 \[hep-th\]](#).
- [26] K. Ohta and Y. Yoshida, “Non-Abelian Localization for Supersymmetric Yang-Mills-Chern-Simons Theories on Seifert Manifold,” *Phys. Rev.* **D86** (2012) 105018, [arXiv:1205.0046 \[hep-th\]](#).

- [27] D. Martelli and A. Passias, “The gravity dual of supersymmetric gauge theories on a two-parameter deformed three-sphere,” *Nucl. Phys.* **B877** (2013) 51–72, [arXiv:1306.3893 \[hep-th\]](#).
- [28] N. Drukker, T. Okuda, and F. Passerini, “Exact results for vortex loop operators in 3d supersymmetric theories,” *JHEP* **07** (2014) 137, [arXiv:1211.3409 \[hep-th\]](#).
- [29] K. Hosomichi, “A review on SUSY gauge theories on  $S^3$ ,” *Math. Phys. Stud.* **9783319187693** (2016) 307–338, [arXiv:1412.7128 \[hep-th\]](#).
- [30] L. F. Alday, D. Martelli, P. Richmond, and J. Sparks, “Localization on Three-Manifolds,” *JHEP* **10** (2013) 095, [arXiv:1307.6848 \[hep-th\]](#).
- [31] F. Benini and A. Zaffaroni, “A topologically twisted index for three-dimensional supersymmetric theories,” *JHEP* **07** (2015) 127, [arXiv:1504.03698 \[hep-th\]](#).
- [32] A. Kapustin, B. Willett, and I. Yaakov, “Exact results for supersymmetric abelian vortex loops in 2+1 dimensions,” *JHEP* **06** (2013) 099, [arXiv:1211.2861 \[hep-th\]](#).
- [33] T. Nishioka and I. Yaakov, “Supersymmetric Renyi Entropy,” *JHEP* **10** (2013) 155, [arXiv:1306.2958 \[hep-th\]](#).
- [34] Y. Imamura and D. Yokoyama, “ $S^3/Z_n$  partition function and dualities,” *JHEP* **11** (2012) 122, [arXiv:1208.1404 \[hep-th\]](#).
- [35] L. F. Alday, M. Fluder, and J. Sparks, “The Large N limit of M2-branes on Lens spaces,” *JHEP* **10** (2012) 057, [arXiv:1204.1280 \[hep-th\]](#).
- [36] O. Aharony, N. Seiberg, and Y. Tachikawa, “Reading between the lines of four-dimensional gauge theories,” *JHEP* **08** (2013) 115, [arXiv:1305.0318 \[hep-th\]](#).
- [37] D. Gang, “Chern-Simons theory on  $L(p,q)$  lens spaces and Localization,” [arXiv:0912.4664 \[hep-th\]](#).
- [38] F. Benini, T. Nishioka, and M. Yamazaki, “4d Index to 3d Index and 2d TQFT,” *Phys. Rev.* **D86** (2012) 065015, [arXiv:1109.0283 \[hep-th\]](#).
- [39] F. Nieri and S. Pasquetti, “Factorisation and holomorphic blocks in 4d,” *JHEP* **11** (2015) 155, [arXiv:1507.00261 \[hep-th\]](#).
- [40] Y. Imamura, H. Matsuno, and D. Yokoyama, “Factorization of the  $S^3/Z_n$  partition function,” *Phys. Rev.* **D89** (2014) no. 8, 085003, [arXiv:1311.2371 \[hep-th\]](#).
- [41] S. Kim, “The Complete superconformal index for  $N=6$  Chern-Simons theory,” *Nucl. Phys.* **B821** (2009) 241–284, [arXiv:0903.4172 \[hep-th\]](#). [Erratum: *Nucl. Phys.*B864,884(2012)].
- [42] Y. Imamura and S. Yokoyama, “Index for three dimensional superconformal field theories with general R-charge assignments,” *JHEP* **04** (2011) 007, [arXiv:1101.0557 \[hep-th\]](#).
- [43] T. T. Wu and C. N. Yang, “Dirac monopole without strings: Monopole harmonics,” *Nucl. Phys. B* **107**, 365 (1976).
- [44] T. Dimofte, D. Gaiotto, and S. Gukov, “3-Manifolds and 3d Indices,” *Adv. Theor. Math. Phys.* **17** (2013) no. 5, 975–1076, [arXiv:1112.5179 \[hep-th\]](#).
- [45] O. Aharony, S. S. Razamat, N. Seiberg, and B. Willett, “3d dualities from 4d dualities,” *JHEP* **07** (2013) 149, [arXiv:1305.3924 \[hep-th\]](#).
- [46] J. Kinney, J. M. Maldacena, S. Minwalla, and S. Raju, “An Index for 4 dimensional super conformal theories,” *Commun. Math. Phys.* **275** (2007) 209–254, [arXiv:hep-th/0510251 \[hep-th\]](#).
- [47] L. Rastelli and S. Razamat, “The supersymmetric index in four dimensions,” *Journal of Physics A* **xx** (2016) 000, [1608.02965](#).

- [48] S. Kim and K. Lee, “Indices for 6 dimensional superconformal field theories,” *Journal of Physics A* **xx** (2016) 000, [1608.02969](#).
- [49] S. S. Razamat and B. Willett, “Down the rabbit hole with theories of class  $\mathcal{S}$ ,” *JHEP* **10** (2014) 99, [arXiv:1403.6107 \[hep-th\]](#).
- [50] S. Cremonesi, A. Hanany, and A. Zaffaroni, “Monopole operators and Hilbert series of Coulomb branches of  $3d \mathcal{N} = 4$  gauge theories,” *JHEP* **01** (2014) 005, [arXiv:1309.2657 \[hep-th\]](#).
- [51] M. Mariño, “Localization at large  $N$  in Chern-Simons-matter theories,” *Journal of Physics A* **xx** (2016) 000, [1608.02959](#).
- [52] S. Pufu, “The F-Theorem and F-Maximization,” *Journal of Physics A* **xx** (2016) 000, [1608.02960](#).
- [53] H. Casini and M. Huerta, “On the RG running of the entanglement entropy of a circle,” *Phys. Rev. D* **85** (2012) 125016, [arXiv:1202.5650 \[hep-th\]](#).
- [54] T. Dimofte, “Perturbative and nonperturbative aspects of complex Chern-Simons Theory,” *Journal of Physics A* **xx** (2016) 000, [1608.02961](#).
- [55] F. Benini, C. Closset, and S. Cremonesi, “Comments on 3d Seiberg-like dualities,” *JHEP* **10** (2011) 075, [arXiv:1108.5373 \[hep-th\]](#).
- [56] V. P. Spiridonov and G. S. Vartanov, “Elliptic hypergeometry of supersymmetric dualities II. Orthogonal groups, knots, and vortices,” *Commun. Math. Phys.* **325** (2014) 421–486, [arXiv:1107.5788 \[hep-th\]](#).
- [57] D. Jafferis and X. Yin, “A Duality Appetizer,” [arXiv:1103.5700 \[hep-th\]](#).
- [58] A. Kapustin, H. Kim, and J. Park, “Dualities for 3d Theories with Tensor Matter,” *JHEP* **12** (2011) 087, [arXiv:1110.2547 \[hep-th\]](#).
- [59] J. Park and K.-J. Park, “Seiberg-like Dualities for 3d  $N=2$  Theories with  $SU(N)$  gauge group,” *JHEP* **10** (2013) 198, [arXiv:1305.6280 \[hep-th\]](#).
- [60] K. A. Intriligator and N. Seiberg, “Mirror symmetry in three-dimensional gauge theories,” *Phys. Lett. B* **387** (1996) 513–519, [arXiv:hep-th/9607207 \[hep-th\]](#).
- [61] J. de Boer, K. Hori, H. Ooguri, and Y. Oz, “Mirror symmetry in three-dimensional gauge theories, quivers and D-branes,” *Nucl. Phys. B* **493** (1997) 101–147, [arXiv:hep-th/9611063 \[hep-th\]](#).
- [62] A. Kapustin, B. Willett, and I. Yaakov, “Nonperturbative Tests of Three-Dimensional Dualities,” *JHEP* **10** (2010) 013, [arXiv:1003.5694 \[hep-th\]](#).
- [63] S. Benvenuti and S. Pasquetti, “3D-partition functions on the sphere: exact evaluation and mirror symmetry,” *JHEP* **05** (2012) 099, [arXiv:1105.2551 \[hep-th\]](#).
- [64] A. Kapustin and M. J. Strassler, “On mirror symmetry in three-dimensional Abelian gauge theories,” *JHEP* **04** (1999) 021, [arXiv:hep-th/9902033 \[hep-th\]](#).
- [65] N. Seiberg, “Electric - magnetic duality in supersymmetric nonAbelian gauge theories,” *Nucl. Phys. B* **435** (1995) 129–146, [arXiv:hep-th/9411149 \[hep-th\]](#).
- [66] O. Aharony, “IR duality in  $d = 3$   $N=2$  supersymmetric  $USp(2N(c))$  and  $U(N(c))$  gauge theories,” *Phys. Lett. B* **404** (1997) 71–76, [arXiv:hep-th/9703215 \[hep-th\]](#).
- [67] A. Giveon and D. Kutasov, “Seiberg Duality in Chern-Simons Theory,” *Nucl. Phys. B* **812** (2009) 1–11, [arXiv:0808.0360 \[hep-th\]](#).
- [68] H. Kim and J. Park, “Aharony Dualities for 3d Theories with Adjoint Matter,” *JHEP* **06** (2013) 106, [arXiv:1302.3645 \[hep-th\]](#).

- [69] O. Aharony and D. Fleischer, “IR Dualities in General 3d Supersymmetric SU(N) QCD Theories,” *JHEP* **02** (2015) 162, [arXiv:1411.5475 \[hep-th\]](#).
- [70] A. Kapustin, “Seiberg-like duality in three dimensions for orthogonal gauge groups,” [arXiv:1104.0466 \[hep-th\]](#).
- [71] A. Kapustin, B. Willett, and I. Yaakov, “Tests of Seiberg-like Duality in Three Dimensions,” [arXiv:1012.4021 \[hep-th\]](#).
- [72] B. Willett and I. Yaakov, “N=2 Dualities and Z Extremization in Three Dimensions,” [arXiv:1104.0487 \[hep-th\]](#).
- [73] C. Hwang, K.-J. Park, and J. Park, “Evidence for Aharony duality for orthogonal gauge groups,” *JHEP* **11** (2011) 011, [arXiv:1109.2828 \[hep-th\]](#).
- [74] C. Closset, T. T. Dumitrescu, G. Festuccia, Z. Komargodski, and N. Seiberg, “Contact Terms, Unitarity, and F-Maximization in Three-Dimensional Superconformal Theories,” *JHEP* **10** (2012) 053, [arXiv:1205.4142 \[hep-th\]](#).
- [75] F. Van de Bult, “Hyperbolic Hypergeometric Functions,” *Thesis* (2007) .
- [76] A. Kapustin and B. Willett, “Wilson loops in supersymmetric Chern-Simons-matter theories and duality,” [arXiv:1302.2164 \[hep-th\]](#).
- [77] B. Assel and J. Gomis, “Mirror Symmetry And Loop Operators,” *JHEP* **11** (2015) 055, [arXiv:1506.01718 \[hep-th\]](#).
- [78] S. Pasquetti, “Factorisation of N = 2 Theories on the Squashed 3-Sphere,” *JHEP* **04** (2012) 120, [arXiv:1111.6905 \[hep-th\]](#).
- [79] C. Beem, T. Dimofte, and S. Pasquetti, “Holomorphic Blocks in Three Dimensions,” *JHEP* **12** (2014) 177, [arXiv:1211.1986 \[hep-th\]](#).
- [80] S. Cecotti and C. Vafa, “Topological-anti-topological fusion,” *Nuclear Physics B* **367** (1991) 359–461.
- [81] Y. Yoshida and K. Sugiyama, “Localization of 3d  $\mathcal{N} = 2$  Supersymmetric Theories on  $S^1 \times D^2$ ,” [arXiv:1409.6713 \[hep-th\]](#).
- [82] M. Fujitsuka, M. Honda, and Y. Yoshida, “Higgs branch localization of 3d  $\mathfrak{d}\mathfrak{I}\mathfrak{S}\mathfrak{I} = 2$  theories,” *PTEP* **2014** (2014) no. 12, 123B02, [arXiv:1312.3627 \[hep-th\]](#).
- [83] F. Benini and W. Peelaers, “Higgs branch localization in three dimensions,” *JHEP* **05** (2014) 030, [arXiv:1312.6078 \[hep-th\]](#).
- [84] S. Pasquetti, “Holomorphic blocks and the 5d AGT correspondence,” *Journal of Physics A* **xx** (2016) 000, [1608.02968](#).
- [85] V. Niarchos, “Seiberg dualities and the 3d/4d connection,” *JHEP* **07** (2012) 075, [arXiv:1205.2086 \[hep-th\]](#).
- [86] A. Amariti and C. Klare, “Chern-Simons and RG Flows: Contact with Dualities,” *JHEP* **08** (2014) 144, [arXiv:1405.2312 \[hep-th\]](#).
- [87] Y. Imamura, “Relation between the 4d superconformal index and the  $S^3$  partition function,” *JHEP* **09** (2011) 133, [arXiv:1104.4482 \[hep-th\]](#).
- [88] F. A. H. Dolan, V. P. Spiridonov, and G. S. Vartanov, “From 4d superconformal indices to 3d partition functions,” *Phys. Lett.* **B704** (2011) 234–241, [arXiv:1104.1787 \[hep-th\]](#).
- [89] A. Gadde and W. Yan, “Reducing the 4d Index to the  $S^3$  Partition Function,” *JHEP* **12** (2012) 003, [arXiv:1104.2592 \[hep-th\]](#).

- [90] F. Benini and S. Cremonesi, “Partition Functions of  $\mathcal{N} = (2, 2)$  Gauge Theories on  $S^2$  and Vortices,” *Commun. Math. Phys.* **334** (2015) no. 3, 1483–1527, [arXiv:1206.2356 \[hep-th\]](#).
- [91] F. Benini and B. Le Floch, “Supersymmetric localization in two dimensions,” *Journal of Physics A* **xx** (2016) 000, [1608.02955](#).

# Chapter 7

## Localization at large $N$ in Chern–Simons–matter theories

Marcos Mariño

*Département de Physique Théorique et Section de Mathématiques*  
*Université de Genève, Genève, CH-1211 Switzerland*  
Marcos.Marino@unige.ch

### Abstract

We review some exact results for the matrix models appearing in the localization of Chern–Simons–matter theories, focusing on the structure of non-perturbative effects and on the M-theory expansion of ABJM theory. We also summarize some of the results obtained for other Chern–Simons–matter theories, as well as recent applications to topological strings.

### Contents

|            |                                                        |            |
|------------|--------------------------------------------------------|------------|
| <b>7.1</b> | <b>Introduction</b>                                    | <b>272</b> |
| <b>7.2</b> | <b>The ABJM matrix model</b>                           | <b>273</b> |
| 7.2.1      | A short review of ABJM theory                          | 273        |
| 7.2.2      | The 't Hooft expansion                                 | 277        |
| 7.2.3      | The M-theory expansion                                 | 285        |
| <b>7.3</b> | <b>Generalizations</b>                                 | <b>318</b> |
| 7.3.1      | The 't Hooft expansion of Chern–Simons–matter theories | 318        |
| 7.3.2      | The Fermi gas approach to Chern–Simons–matter theories | 321        |
| 7.3.3      | Topological strings                                    | 323        |
| <b>7.4</b> | <b>Conclusions and outlook</b>                         | <b>325</b> |
|            | <b>References</b>                                      | <b>327</b> |

## 7.1 Introduction

The use of localization techniques in superconformal gauge theories, pioneered in [2], has led to many new exact results in QFT. Typically, these techniques give expressions for the partition functions or correlation functions of the theory in terms of a matrix integral, and the number of variables of this integral scales as the rank of the gauge group  $N$ . Although the resulting expressions are relatively explicit, it is not so easy to evaluate them analytically for small  $N$ , and it is even harder to determine their behavior as  $N$  grows large. However, this is precisely the regime that one wants to study in applications of localization to the AdS/CFT correspondence.

In this paper we will review some aspects of the large  $N$  solution to the matrix integrals appearing in the localization of Chern–Simons–matter theories [3]. The first exact results for their large  $N$  limits were found in [4,5], where the planar Wilson loop vevs and the planar free energy of ABJM theory [6] were calculated explicitly. Many subsequent works, following [7], have studied the strict large  $N$  limit of these theories and compared them with their gravity counterparts<sup>1</sup>. However, in this review we will focus on the rich structures appearing *beyond* the strict large  $N$  limit: the determination of exact planar free energies, the 't Hooft  $1/N$  expansion beyond the planar limit, and specially the structure of non-perturbative effects at large  $N$ , which are invisible in the 't Hooft expansion. We will also focus on the results for the partition functions on the three-sphere. There have been studies of these theories on other three-manifolds, and also of other observables, such as Wilson loops, but we will not consider these extensions here.

Going beyond the strict large  $N$  limit is not easy, and so far the only theory for which we have a rather complete picture is ABJM theory (and its close cousin, ABJ theory [8].) After considerable effort, a detailed expression for the full  $1/N$  expansion of the partition function of ABJM theory, including non-perturbative corrections, is now available. This is arguably the most complete result obtained so far for a gauge theory observable in the general framework of the  $1/N$  expansion (of course, simpler models have been solved with the same level of detail, but they do not have the same level of complexity.) Therefore, section 2 (which comprises most of this review), is devoted to a relatively self-contained explanation of this result, since many of its ingredients are scattered across the literature. In section 3, we summarize what is known beyond the strict large  $N$  limit in other Chern–Simons–matter theories. We also comment on some related developments in topological string theory. Finally, in section 4 we list some conclusions and open problems.

While preparing this review for publication, another review paper on this subject appeared [9].

---

<sup>1</sup>By strict large  $N$  limit, we mean the dominant term in the large  $N$  expansion. This contains less information than the exact planar limit, since it is given by its leading term at strong 't Hooft coupling.

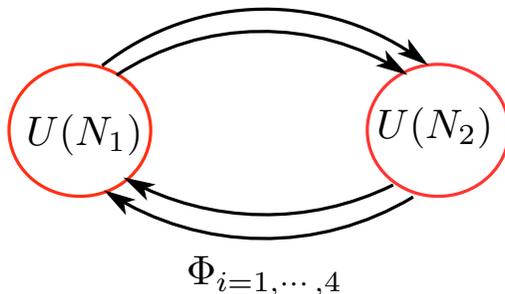

Figure 7.1: The quiver for ABJ(M) theory. The two nodes represent the  $U(N_{1,2})$  Chern–Simons theories (with opposite levels) and the arrows between the nodes represent the four matter multiplets in the bifundamental representation.

## 7.2 The ABJM matrix model

### 7.2.1 A short review of ABJM theory

ABJM theory and its generalization, also called ABJ theory, were proposed in [6, 8] to describe  $N$  M2 branes on  $\mathbb{C}^4/\mathbb{Z}_k$ . They are particular examples of supersymmetric Chern–Simons–matter theories and their basic ingredient is a pair of vector multiplets with gauge groups  $U(N_1)$ ,  $U(N_2)$ , described by two supersymmetric Chern–Simons theories with opposite levels  $k$ ,  $-k$ . In addition, we have four matter supermultiplets  $\Phi_i$ ,  $i = 1, \dots, 4$ , in the bifundamental representation of the gauge group  $U(N_1) \times U(N_2)$ . This theory can be represented as a quiver with two nodes, which stand for the two supersymmetric Chern–Simons theories, and four edges between the nodes representing the matter supermultiplets (see Fig. 7.1). In addition, there is a superpotential involving the matter fields, which after integrating out the auxiliary fields in the Chern–Simons–matter system, reads (on  $\mathbb{R}^3$ )

$$W = \frac{4\pi}{k} \text{Tr} \left( \Phi_1 \Phi_2^\dagger \Phi_3 \Phi_4^\dagger - \Phi_1 \Phi_4^\dagger \Phi_3 \Phi_2^\dagger \right). \quad (7.2.1)$$

In this expression we have used the standard superspace notation for  $\mathcal{N} = 1$  supermultiplets in 4d. When the two gauge groups have identical rank, i.e.  $N_1 = N_2 = N$ , the theory is called ABJM theory. The generalization in which  $N_1 \neq N_2$  is called ABJ theory. More details on the construction of these theories can be found in [10, 11]. In most of this review we will focus on ABJM theory, which has two parameters:  $N$ , the common rank of the gauge group, and  $k$ , the Chern–Simons level. Note that, in this theory, all the fields are in the adjoint representation of  $U(N)$  or in the bifundamental representation of  $U(N) \times U(N)$ . Therefore, they have two color indices and one can use the standard ’t Hooft rules [12] to perform a  $1/N$  expansion. Since  $k$  plays the rôle of the inverse gauge coupling  $1/g^2$ , the natural ’t Hooft parameter is given by

$$\lambda = \frac{N}{k}. \quad (7.2.2)$$

One of the most important aspects of ABJM theory is that, at large  $N$ , it describes a non-trivial background of  $M$  theory, as it was already postulated in [13]. In the large distance limit in which  $M$ -theory can be described by supergravity, this is nothing but the Freund–Rubin background

$$X_{11} = \text{AdS}_4 \times \mathbb{S}^7 / \mathbb{Z}_k. \quad (7.2.3)$$

If we represent  $\mathbb{S}^7$  inside  $\mathbb{C}^4$  as

$$\sum_{i=1}^4 |z_i|^2 = 1, \quad (7.2.4)$$

the action of  $\mathbb{Z}_k$  in (7.2.3) is simply given by

$$z_i \rightarrow e^{\frac{2\pi i}{k}} z_i. \quad (7.2.5)$$

The metric on  $\text{AdS}_4 \times \mathbb{S}^7$  depends on a single parameter, the radius  $L$ , and by using metrics on  $\text{AdS}_4$  and  $\mathbb{S}^7$  of unit radius, we have

$$ds^2 = L^2 \left( \frac{1}{4} ds_{\text{AdS}_4}^2 + ds_{\mathbb{S}^7}^2 \right). \quad (7.2.6)$$

As it is well-known, the Freund–Rubin background also involves a non-zero flux for the four-form field strength  $G$  of 11d SUGRA, see for example [14] for an early review of eleven-dimensional supergravity on this background.

The AdS/CFT correspondence between ABJM theory and  $M$ -theory in the above Freund–Rubin background comes with a dictionary between the gauge theory parameters and the  $M$ -theory parameters. The parameter  $k$  in the gauge theory has a purely geometric interpretation and it is the same  $k$  appearing in the modding out by  $\mathbb{Z}_k$  in (7.2.3) and (7.2.5). The parameter  $N$  corresponds to the number of M2 branes, which lead to the non-zero flux of  $G$ , and also determines the radius of the background. One finds,

$$\left( \frac{L}{\ell_p} \right)^6 = 32\pi^2 k N, \quad (7.2.7)$$

where  $\ell_p$  is the eleven-dimensional Planck constant. It should be emphasized that the above relation is in principle only valid in the large  $N$  limit, and it has been argued that it is corrected due to a shift in the M2 charge [15, 16]. According to this argument, the physical charge determining the radius is not  $N$ , but rather

$$Q = N - \frac{1}{24} \left( k - \frac{1}{k} \right). \quad (7.2.8)$$

The geometric,  $M$ -theory description in terms of the background (7.2.3) emerges when

$$N \rightarrow \infty, \quad k \text{ fixed}. \quad (7.2.9)$$

The corresponding regime in the dual gauge theory will be called the *M-theory regime*. In this regime, one looks for asymptotic expansions of the observables at large  $N$  but  $k$  fixed. This is the so-called *M-theory expansion* of the gauge theory.

It has been known for a while that the above Freund–Rubin background of M-theory can be used to find a background of type IIA superstring theory of the form

$$X_{10} = \text{AdS}_4 \times \mathbb{CP}^3. \quad (7.2.10)$$

This is due to the existence of the Hopf fibration,

$$\begin{array}{ccc} \mathbb{S}^1 & \rightarrow & \mathbb{S}^7 \\ & & \downarrow \\ & & \mathbb{CP}^3 \end{array} \quad (7.2.11)$$

and the circle of this fibration can be used to perform a non-trivial reduction from M-theory to type IIA theory [17]. In order to have a perturbative regime for the type IIA superstring, we need the circle to be small, and this is achieved when  $k$  is large. Indeed, by using the standard dictionary relating M-theory and type IIA theory, we find that the string coupling constant  $g_{\text{st}}$  is given by

$$g_{\text{st}}^2 = \frac{1}{k^2} \left( \frac{L}{\ell_s} \right)^2, \quad (7.2.12)$$

where  $\ell_s$  is the string length. On the other hand, we also have from this dictionary that

$$\lambda = \frac{1}{32\pi^2} \left( \frac{L}{\ell_s} \right)^4, \quad (7.2.13)$$

where  $\lambda$  is the 't Hooft parameter (7.2.2). We conclude that the perturbative regime of the type IIA superstring corresponds to the 't Hooft  $1/N$  expansion, in which

$$N \rightarrow \infty, \quad \lambda = \frac{N}{k} \quad \text{fixed}, \quad (7.2.14)$$

i.e. the genus expansion in the 't Hooft regime of the gauge theory corresponds to the perturbative genus expansion of the superstring. In addition, the regime of strong 't Hooft coupling corresponds to the point-particle limit of the superstring, in which  $\alpha'$  corrections are suppressed.

A very important aspect of ABJM theory is that there are two different regimes to consider: the M-theory regime (7.2.9), and the standard 't Hooft regime (7.2.14). The existence of a well-defined M-theory limit is somewhat surprising from the gauge theory point of view. This limit is more like a thermodynamic limit of the theory, in which the number of degrees of freedom goes to infinity but the coupling constant remains fixed. General aspects of this limit have been discussed in [18].

One of the consequences of the AdS/CFT correspondence is that the partition function of the Euclidean ABJM theory on  $\mathbb{S}^3$  should be equal to the partition function of the Euclidean version of M-theory/string theory on the dual AdS backgrounds [19], i.e.

$$Z(\mathbb{S}^3) = Z(X), \quad (7.2.15)$$

where  $X$  is the eleven-dimensional background (7.2.3) or the ten-dimensional background (7.2.10), appropriate for the M-theory regime or the 't Hooft regime, respectively. In the M-theory limit we can use the supergravity approximation to compute the M-theory partition function, which is just given by the classical action of eleven-dimensional supergravity evaluated on-shell, i.e. on the metric of (7.2.3). This requires a regularization of IR divergences but eventually leads to a finite result, which gives a prediction for the behavior of the partition function of ABJM theory at large  $N$  and fixed  $k$  (see [11] for a review of these issues). If we define the free energy of the theory as the logarithm of the partition function,

$$F(N, k) = \log Z(N, k), \quad (7.2.16)$$

one finds, from the supergravity approximation to M-theory [20],

$$F(N, k) \approx -\frac{\pi\sqrt{2}}{3}k^{1/2}N^{3/2}, \quad N \gg 1. \quad (7.2.17)$$

The  $N^{3/2}$  behavior of the free energy is a famous prediction of AdS/CFT [21] for the large  $N$  behavior of a theory of M2 branes.

The AdS/CFT prediction (7.2.15) can be also studied in the 't Hooft regime. The free energy of the gauge theory on the sphere has a large  $N$  expansion which we will write as

$$F(N, k) = \sum_{g \geq 0} F_g(\lambda) g_s^{2g-2}, \quad (7.2.18)$$

where

$$g_s = \frac{2\pi i}{k}. \quad (7.2.19)$$

This expansion is of course equivalent to a  $1/N$  expansion, since  $g_s = 2\pi i\lambda/N$ , and the 't Hooft parameter is kept fixed. In the string theory side, it corresponds to the genus expansion of the free energy. In particular, the planar free energy  $F_0(\lambda)$  of the gauge theory should agree with the superstring free energy at tree level, i.e. at genus zero. When  $\lambda$  is large, the string is small as compared to the AdS radius, and we can use the point-particle approximation to string theory, i.e. we can approximate the genus zero free energy by the type IIA supergravity result. One obtains in this way a prediction for the planar free energy of ABJM theory at strong 't Hooft coupling, of the form

$$F_0(\lambda) \approx \frac{4\pi^3\sqrt{2}}{3}\lambda^{3/2}, \quad \lambda \gg 1. \quad (7.2.20)$$

Interestingly, both predictions are equivalent, in the sense that one can obtain (7.2.20) from (7.2.17) by setting  $k = N/\lambda$ , and viceversa. This is not completely obvious from the point of view of the gauge theory, since it could happen that higher genus corrections in the 't Hooft expansion contribute to the M-theory limit. That this is not the case has been conjectured in [18] to be a general fact and it has been called “planar dominance.” It seems to be a general property of Chern–Simons–matter theories with both an M-theory expansion and a 't Hooft

expansion. Note as well that, as explained in detail in [11], the behavior of the planar free energy at weak 't Hooft coupling is very different from the prediction (7.2.20). Therefore, the planar free energy should be a non-trivial interpolating function between the weakly coupled regime and the strongly coupled regime.

In order to analyze in detail the implications of the large  $N$  duality between ABJM theory and M-theory on the AdS background (7.2.3), it is extremely useful to be able to perform reliable computations on the gauge theory side. The techniques of localization pioneered in [2] have led to a wonderful result for the partition function of ABJM theory on the three-sphere  $S^3$ , due to [3]. This result expresses this partition function, which *a priori* is given by a complicated path integral, in terms of a matrix model (i.e. a path integral in zero dimensions). We will refer to it as the ABJM matrix model, and it takes the following form (the derivation of this and similar expressions can be found in Chapter 6):

$$\begin{aligned}
 Z(N, k) &= \frac{1}{N!^2} \int \frac{d^N \mu}{(2\pi)^N} \frac{d^N \nu}{(2\pi)^N} \frac{\prod_{i < j} \left[ 2 \sinh \left( \frac{\mu_i - \mu_j}{2} \right) \right]^2 \left[ 2 \sinh \left( \frac{\nu_i - \nu_j}{2} \right) \right]^2}{\prod_{i, j} \left[ 2 \cosh \left( \frac{\mu_i - \nu_j}{2} \right) \right]^2} \exp \left[ \frac{ik}{4\pi} \sum_{i=1}^N (\mu_i^2 - \nu_i^2) \right].
 \end{aligned}
 \tag{7.2.21}$$

In the remaining of this review, we will analyze this matrix model in detail. We will study it in different regimes and we will try to extract lessons and consequences for the AdS/CFT correspondence.

## 7.2.2 The 't Hooft expansion

### The planar limit

In order to test the prediction (7.2.20), it would be useful to have an explicit expression for  $F_0(\lambda)$ , and eventually for the full series of genus  $g$  free energies  $F_g(\lambda)$ . This is in principle a formidable problem, involving the resummation of double-line diagrams with a fixed genus in the perturbative expansion of the total free energy. However, since the partition function is given by the matrix integral (7.2.21), we can try to obtain the  $1/N$  expansion directly in the matrix model. The large  $N$  expansion of matrix models has been extensively studied since the seminal work of Brézin, Itzykson, Parisi and Zuber [22], and there are by now many different techniques to solve this problem. The first step in this calculation is of course to obtain the planar free energy  $F_0(\lambda)$ , which is the dominant term at large  $N$ .

A detailed review of the calculation of the planar free energy of the ABJM matrix model can be found in [11], and we won't repeat it here. We will just summarize the most important aspects of the solution. As usual, at large  $N$ , the eigenvalues of the matrix model “condense” around cuts in the complex plane. This means that the equilibrium values of the eigenvalues  $\mu_i, \nu_i, i = 1, \dots, N$ , fall into two arcs in the complex plane as  $N$  becomes large. The equilibrium conditions for the eigenvalues  $\mu_i, \nu_i$  can be found immediately from the integrand

of the matrix integral:

$$\begin{aligned}\frac{ik}{2\pi}\mu_i &= -\sum_{j \neq i}^N \coth \frac{\mu_i - \mu_j}{2} + \sum_{j=1}^N \tanh \frac{\mu_i - \nu_j}{2}, \\ \frac{ik}{2\pi}\nu_i &= \sum_{j \neq i}^N \coth \frac{\nu_i - \nu_j}{2} - \sum_{j=1}^N \tanh \frac{\nu_i - \mu_j}{2}.\end{aligned}\tag{7.2.22}$$

In standard matrix models, it is useful to think about the equilibrium values of the eigenvalues as the result of a competition between a confining one-body potential and a repulsive two-body potential. Here we can not do that, since the one-body potential is imaginary. One way to go around this is to use analytic continuation: we rotate  $k$  to an imaginary value, and then at the end of the calculation we rotate it back. This is the procedure followed originally in [5]. We consider then the saddle-point equations

$$\begin{aligned}\mu_i &= \frac{t_1}{N_1} \sum_{j \neq i}^{N_1} \coth \frac{\mu_i - \mu_j}{2} + \frac{t_2}{N_2} \sum_{j=1}^{N_2} \tanh \frac{\mu_i - \nu_j}{2}, \\ \nu_i &= \frac{t_2}{N_2} \sum_{j \neq i}^{N_2} \coth \frac{\nu_i - \nu_j}{2} + \frac{t_1}{N_1} \sum_{j=1}^{N_1} \tanh \frac{\nu_i - \mu_j}{2}.\end{aligned}\tag{7.2.23}$$

where

$$t_i = g_s N_i, \quad i = 1, 2.\tag{7.2.24}$$

The planar free energy obtained from these equations will be a function only of  $t_1$  and  $t_2$ , and to recover the planar free energy of the original ABJM matrix model we have to set

$$t_1 = -t_2 = \frac{2\pi i}{k} N.\tag{7.2.25}$$

The equations (7.2.23), for real  $g_s$ , are equivalent to the original ones (7.2.22) after rotating  $k$  to the imaginary axis, and then performing an analytic continuation  $N_2 \rightarrow -N_2$ . At large  $N_i$ , and for real  $g_s$ ,  $t_i$ , the eigenvalues  $\mu_i$ ,  $i = 1, \dots, N_1$  and  $\nu_j$ ,  $j = 1, \dots, N_2$ , condense around two cuts in the real axis,  $\mathcal{C}_{1,2}$  (respectively.) Due to the symmetries of the problem, these cuts are symmetric around the origin. We will denote by  $[-A, A]$ ,  $[-B, B]$ , respectively.

It turns out that the equations (7.2.23) are the saddle-point equations for the so-called lens space matrix model studied in [23–25], whose planar solution is well-known. To write down the solution, one introduces a resolvent  $\omega(z)$ , as defined in [25]:

$$\omega(z) = g_s \left\langle \sum_{i=1}^{N_1} \coth \left( \frac{z - \mu_i}{2} \right) \right\rangle + g_s \left\langle \sum_{a=1}^{N_2} \tanh \left( \frac{z - \nu_a}{2} \right) \right\rangle.\tag{7.2.26}$$

In terms of the variable  $Z = e^z$ , it is given by

$$\omega(z)dz = -t \frac{dZ}{Z} + 2g_s \left\langle \sum_{i=1}^{N_1} \frac{dZ}{Z - e^{\mu_i}} \right\rangle + 2g_s \left\langle \sum_{a=1}^{N_2} \frac{dZ}{Z + e^{\nu_a}} \right\rangle,\tag{7.2.27}$$

where

$$t = t_1 + t_2. \quad (7.2.28)$$

In the planar approximation, the sum over eigenvalues can be replaced by an integration involving their densities, and we have that

$$\omega_0(z) = -t + 2t_1 \int_{\mathcal{C}_1} \rho_1(\mu) \frac{Z}{Z - e^\mu} d\mu + 2t_2 \int_{\mathcal{C}_2} \rho_2(\nu) \frac{Z}{Z + e^\nu} d\nu, \quad (7.2.29)$$

where  $\rho_1(\mu)$ ,  $\rho_2(\nu)$  are the large  $N$  densities of eigenvalues on the cuts  $\mathcal{C}_1$ ,  $\mathcal{C}_2$ , respectively, normalized as

$$\int_{\mathcal{C}_1} \rho_1(\mu) d\mu = \int_{\mathcal{C}_2} \rho_2(\nu) d\nu = 1. \quad (7.2.30)$$

A standard discontinuity argument tells us that

$$\begin{aligned} \rho_1(X) dX &= -\frac{1}{4\pi i t_1} \frac{dX}{X} (\omega_0(X + i\epsilon) - \omega_0(X - i\epsilon)), & X \in \mathcal{C}_1, \\ \rho_2(Y) dY &= \frac{1}{4\pi i t_2} \frac{dY}{Y} (\omega_0(Y + i\epsilon) - \omega_0(Y - i\epsilon)), & Y \in \mathcal{C}_2. \end{aligned} \quad (7.2.31)$$

The planar resolvent turns out to have the explicit expression [24, 25]

$$\omega_0(Z) = \log \left( \frac{e^{-t}}{2} \left[ f(Z) - \sqrt{f^2(Z) - 4e^{2t} Z^2} \right] \right). \quad (7.2.32)$$

Notice that  $e^{\omega_0}$  has a square root branch cut involving the function

$$\sigma(Z) = f^2(Z) - 4e^{2t} Z^2 = (Z - a)(Z - 1/a)(Z + b)(Z + 1/b), \quad (7.2.33)$$

where  $a^{\pm 1}, b^{\pm 1}$  are the endpoints of the cuts in the  $Z = e^z$  plane (i.e.  $A = \log a$ ,  $B = \log b$ ). They are determined, in terms of the parameters  $t_1, t_2$  by the normalization conditions for the densities (7.2.30). We will state the final results in ABJM theory. A detailed derivation can be found in the original papers [4, 5] and in the review [11].

In the ABJM case we have to consider the special case or “slice” given in (7.2.25), therefore  $t = 0$ . One can parametrize the endpoints of the cut in terms of a single parameter  $\kappa$ , as

$$a + \frac{1}{a} = 2 + i\kappa, \quad b + \frac{1}{b} = 2 - i\kappa. \quad (7.2.34)$$

The 't Hooft coupling  $\lambda$  turns out to be a non-trivial function of  $\kappa$ , determined by the normalization of the density. In order for  $\lambda$  to be real and well-defined,  $\kappa$  has to be real as well, and one finds the equation [4]

$$\lambda(\kappa) = \frac{\kappa}{8\pi} {}_3F_2 \left( \frac{1}{2}, \frac{1}{2}, \frac{1}{2}; 1, \frac{3}{2}; -\frac{\kappa^2}{16} \right). \quad (7.2.35)$$

Notice that the endpoints of the cuts are in general complex, i.e. the cuts  $\mathcal{C}_1, \mathcal{C}_2$  are arcs in the complex plane. This is a consequence of the analytic continuation and it has been

verified in numerical simulations of the original saddle-point equations (7.2.22) [7]. Using similar techniques (see again [11]), one finds a very explicit expression for the derivative of the planar free energy,

$$\partial_\lambda F_0(\lambda) = \frac{\kappa}{4} G_{3,3}^{2,3} \left( \begin{matrix} \frac{1}{2}, & \frac{1}{2}, & \frac{1}{2} \\ 0, & 0, & -\frac{1}{2} \end{matrix} \middle| -\frac{\kappa^2}{16} \right) + \frac{\pi^2 i \kappa}{2} {}_3F_2 \left( \begin{matrix} \frac{1}{2}, & \frac{1}{2}, & \frac{1}{2} \\ 1, & \frac{3}{2} \end{matrix}; -\frac{\kappa^2}{16} \right). \quad (7.2.36)$$

This is written in terms of the auxiliary variable  $\kappa$ , but by using the explicit map (7.2.35), one can re-express it in terms of the 't Hooft coupling, and one finds the following expansion around  $\lambda = 0$ ,

$$\partial_\lambda F_0(\lambda) = -8\pi^2 \lambda \left( \log \left( \frac{\pi \lambda}{2} \right) - 1 \right) + \frac{16\pi^4 \lambda^3}{9} + \mathcal{O}(\lambda^5). \quad (7.2.37)$$

It is easy to see that this reproduces the perturbative, weak coupling expansion of the matrix integral. This also fixes the integration constant, and one can write

$$F_0(\lambda) = \int_0^\lambda d\lambda' \partial_{\lambda'} F_0(\lambda'). \quad (7.2.38)$$

To study the strong 't Hooft coupling behavior, we notice from (7.2.35) that large  $\lambda \gg 1$  requires  $\kappa \gg 1$ . More concretely, we find the following expansion at large  $\kappa$ :

$$\lambda(\kappa) = \frac{\log^2(\kappa)}{2\pi^2} + \frac{1}{24} + \mathcal{O}\left(\frac{1}{\kappa^2}\right), \quad \kappa \gg 1. \quad (7.2.39)$$

This suggests to define the shifted coupling

$$\hat{\lambda} = \lambda - \frac{1}{24}. \quad (7.2.40)$$

Notice from (7.2.8) that this shift is precisely the one needed in order for  $\hat{\lambda}$  to be identified with  $Q/k$ , at leading order in the string coupling constant. The relationship (7.2.39) is immediately inverted to

$$\kappa \approx e^{\pi\sqrt{2\hat{\lambda}}}, \quad \lambda \gg 1. \quad (7.2.41)$$

To compute the planar free energy, we have to analytically continue the r.h.s. of (7.2.36) to  $\kappa = \infty$ , and we obtain

$$\partial_\lambda F_0(\lambda) = 2\pi^2 \log \kappa + \frac{4\pi^2}{\kappa^2} {}_4F_3 \left( 1, 1, \frac{3}{2}, \frac{3}{2}; 2, 2, 2; -\frac{16}{\kappa^2} \right). \quad (7.2.42)$$

After integrating w.r.t.  $\lambda$ , we find,

$$F_0(\hat{\lambda}) = \frac{4\pi^3 \sqrt{2}}{3} \hat{\lambda}^{3/2} + \frac{\zeta(3)}{2} + \sum_{\ell \geq 1} e^{-2\pi\ell\sqrt{2\hat{\lambda}}} f_\ell \left( \frac{1}{\pi\sqrt{2\hat{\lambda}}} \right), \quad (7.2.43)$$

where  $f_\ell(x)$  is a polynomial in  $x$  of degree  $2\ell - 3$  (for  $\ell \geq 2$ ). The leading term in (7.2.43) agrees precisely with the prediction from the AdS dual in (7.2.20). The series of exponentially small corrections in (7.2.43) were interpreted in [5] as coming from worldsheet instantons of type IIA theory wrapping the  $\mathbb{CP}^1$  cycle in  $\mathbb{CP}^3$ . This is a novel type of correction in AdS<sub>4</sub> dualities which is not present in the large  $N$  dual to  $\mathcal{N} = 4$  super Yang–Mills theory, see [26] for a preliminary investigation of these effects.

An important aspect of the above planar solution is the following. As we explained above, in finding this solution it is useful to take into account the relationship to the lens space matrix model of [23, 24] discovered in [4]. On the other hand, this matrix model computes, in the  $1/N$  expansion, the partition function of topological string theory on a non-compact Calabi–Yau (CY) known as local  $\mathbb{P}^1 \times \mathbb{P}^1$ , and in particular its planar free energy is given by the genus zero free energy or prepotential of this topological string theory. Local  $\mathbb{P}^1 \times \mathbb{P}^1$  has two complexified Kähler parameters  $T_{1,2}$ . It turns out that the ABJM slice in which  $N_1 = N_2$  corresponds to the “diagonal” geometry in which  $T_1 = T_2$ . The relationship of ABJM theory to this topological string theory has been extremely useful in deriving exact answers for many of these quantities, and we will find it again in the sections to follow. For example, the constant term involving  $\zeta(3)$  in (7.2.43) is well-known in topological string theory and it gives the constant map contribution to the genus zero free energy. The series of worldsheet instantons appearing in (7.2.43) is related to the worldsheet instantons of genus zero in topological string theory. There is however one subtlety: the genus zero free energy in (7.2.43) is the one appropriate to the so-called “orbifold frame” studied in [24], and then it is analytically continued to large  $\lambda$ , which in topological string theory corresponds to the so-called large radius regime. This is not a natural procedure to follow from the point of view of topological strings on local  $\mathbb{P}^1 \times \mathbb{P}^1$ , where quantities in the orbifold frame are typically expanded around the orbifold point.

### Higher genus corrections

The analysis of the previous subsection gives us the leading term in the  $1/N$  expansion, but it is of course an important and interesting problem to compute the higher genus free energies with  $g \geq 1$ . This involves computing subleading  $1/N$  corrections to the free energy of the ABJM matrix model. The computation of such corrections in Hermitian matrix models has a long history, and a general algorithm solving the problem was found in [27]. However, this algorithm is difficult to implement in practice. In some examples, one can use a more efficient method, developed in the context of topological string theory, which is known as the direct integration of the holomorphic anomaly equations. This method was introduced in [28], and applied to the ABJM matrix model in [5]. The  $F_g(\lambda)$  obtained by this method are written in terms of modular forms. The modular parameter is given by

$$\tau = i \frac{K' \left( \frac{i\kappa}{4} \right)}{K \left( \frac{i\kappa}{4} \right)}. \quad (7.2.44)$$

In this equation,  $K(k)$  is the elliptic integral of the first kind,  $K'(k) = K(k')$ , and

$$(k')^2 = 1 - k^2 \tag{7.2.45}$$

is the complementary modulus.  $\tau$  is related to the second derivative of the planar free energy by

$$\frac{i}{4\pi^3} \partial_\lambda^2 F_0(\lambda) = \tau - 1, \tag{7.2.46}$$

which is a standard relation in special geometry. The genus one free energy is given by

$$F_1(\lambda) = -\log \eta(\tau - 1) - \frac{1}{2} \log(2), \tag{7.2.47}$$

where  $\eta(\tau)$  is Dedekind's eta function. The higher genus free energies are expressed in terms of  $E_2(\tau)$ , the standard Eisenstein series, and the Jacobi theta functions

$$b = \vartheta_2^4(\tau), \quad d = \vartheta_4^4(\tau). \tag{7.2.48}$$

They have the general structure

$$F_g(\lambda) = \frac{1}{(bd^2)^{g-1}} \sum_{k=0}^{3g-3} E_2^k(\tau) p_k^{(g)}(b, d), \quad g \geq 2, \tag{7.2.49}$$

where  $p_k^{(g)}(b, d)$  are polynomials in  $b, d$  of modular weight  $6g - 6 - 2k$ . For example, for the genus two free energy one finds the explicit expression

$$F_2(\lambda) = \frac{1}{432bd^2} \left( -\frac{5}{3} E_2^3 + 3bE_2^2 - 2E_4E_2 \right) + \frac{16b^3 + 15db^2 - 15d^2b + 2d^3}{12960bd^2}. \tag{7.2.50}$$

The higher genus  $F_g$  can be found recursively, although there is no known closed form expression or generating functional for them. A detailed analysis for the very first  $g$  shows that they have the following structure, in terms of the auxiliary variable  $\kappa$  [29]<sup>2</sup>:

$$F_g = c_g + f_g \left( \frac{1}{\log \kappa} \right) + \mathcal{O} \left( \frac{1}{\kappa^2} \right), \quad g \geq 2, \tag{7.2.51}$$

where

$$c_g = -\frac{4^{g-1} |B_{2g} B_{2g-2}|}{g(2g-2)(2g-2)!} \tag{7.2.52}$$

involves the Bernoulli numbers  $B_{2g}$ , and

$$f_g(x) = \sum_{j=0}^g c_j^{(g)} x^{2g-3+j} \tag{7.2.53}$$

---

<sup>2</sup>The constant contribution  $c_g$  was not originally included in [5, 29], but this omission was corrected in [30].

is a polynomial. Physically, the equation (7.2.51) tells us that the higher genus free energy has a constant contribution, a polynomial contribution in inverse powers of  $\lambda^{1/2}$ , going like

$$F_g(\lambda) - c_g \approx \lambda^{\frac{3}{2}-g}, \quad \lambda \gg 1, \quad g \geq 2, \quad (7.2.54)$$

and an infinite series of corrections due to worldsheet instantons of genus  $g$ . The quantities appearing here have a natural interpretation in the context of topological string theory, since the  $F_g(\lambda)$  are simply the orbifold higher genus free energies of local  $\mathbb{P}^1 \times \mathbb{P}^1$ . The constants (7.2.52) are the well-known constant map contributions to the higher genus free energies, and the worldsheet instantons of type IIA superstring theory appearing in  $F_g(\lambda)$  come from the worldsheet instantons of the topological string.

In [29] it was noted that, if we drop the worldsheet instanton corrections in the  $F_g(\lambda)$ , the expansion of the free energy has a simple expression in terms of a variable  $\zeta$  defined by

$$\zeta = 32\pi^2 k (N - B(k)), \quad (7.2.55)$$

where

$$B(k) = \frac{k}{24} + \frac{1}{3k}. \quad (7.2.56)$$

The free energy truncated in this way, which we will denote by  $F^{(p)}(N, k)$  (where the superscript means perturbative), has the following expansion,

$$F^{(p)}(N, k) = -\frac{1}{384\pi^2 k} \zeta^{3/2} + \frac{1}{6} \log \left[ \frac{\pi^3 k^3}{\zeta^{3/2}} \right] + A(k) + \sum_{n=1}^{\infty} d_{n+1} \pi^{2n} k^n \zeta^{-3n/2}, \quad (7.2.57)$$

where the coefficients  $d_n$  are just rational numbers,

$$d_2 = -\frac{80}{3}, \quad d_3 = 5120, \quad d_4 = -\frac{18104320}{9}, \quad d_5 = 1184890880, \quad \dots \quad (7.2.58)$$

and the constant term  $A(k)$  is an appropriate resummation at all genera of the contribution from the constant maps. Its explicit expression was first found in [30] and it was slightly simplified in [31] to the form,

$$A(k) = \frac{2\zeta(3)}{\pi^2 k} \left( 1 - \frac{k^3}{16} \right) + \frac{k^2}{\pi^2} \int_0^{\infty} dx \frac{x}{e^{kx} - 1} \log(1 - e^{-2x}). \quad (7.2.59)$$

It can be expanded, around  $k = \infty$ , as

$$A(k) = -\frac{k^2}{8\pi^2} \zeta(3) + \frac{1}{2} \log(2) + 2\zeta'(-1) + \frac{1}{6} \log \left( \frac{\pi}{2k} \right) + \sum_{g \geq 2} \left( \frac{2\pi}{k} \right)^{2g-2} (-1)^g c_g, \quad (7.2.60)$$

where the  $c_g$  are given in (7.2.52). The expansion (7.2.57) is remarkable, both physically and mathematically. First of all, it was shown in [32] that it can be resummed in terms of the well-known Airy function: after exponentiation, one finds that the partition function has the form

$$Z^{(p)}(N, k) = e^{A(k)} C^{-1/3}(k) \text{Ai} \left[ C^{-1/3}(k) (N - B(k)) \right], \quad (7.2.61)$$

where

$$C(k) = \frac{2}{\pi^2 k}. \quad (7.2.62)$$

The expression (7.2.61) gives an excellent approximation to the integral (7.2.21) for large  $N$  and fixed  $k$  [30]. On the other hand, from a physical point of view, if we assume that the parameter  $\zeta$  gives the right “renormalized” dictionary between the gauge theory data and the geometry, i.e., if

$$\left(\frac{L}{\ell_p}\right)^6 = \zeta, \quad (7.2.63)$$

then (7.2.57) is the expected expansion for a free energy in a theory of quantum gravity in eleven dimensions. Indeed, an  $\ell$ -loop term for a vacuum diagram in gravity in  $d$  dimensions goes like (see for example [33, 34])

$$\left(\frac{\ell_p}{L}\right)^{(d-2)(\ell-1)}, \quad (7.2.64)$$

which for  $d = 11$  agrees with the expansion parameter  $\zeta^{-3/2}$  appearing in (7.2.57). The log term in (7.2.57) should correspond to a one-loop correction in supergravity, and this was checked by a direct computation in [35], providing in this way a test of the AdS/CFT correspondence beyond the planar limit (in type IIA, this correction comes from the genus one free energy).

The 't Hooft expansion (7.2.18) gives an asymptotic series for the free energy, at fixed 't Hooft parameter. General arguments (see [36] for an early statement and [37] for a recent review) suggest that this series diverges factorially. The divergence of the series is controlled by a large  $N$  instanton with action  $A_{\text{st}}(\lambda)$ . The correction due to such an instanton is proportional to the exponentially suppressed factor,

$$\exp(-A_{\text{st}}(\lambda)/g_s). \quad (7.2.65)$$

An explicit expression for the instanton action  $A_{\text{st}}(\lambda)$  was conjectured in [29]. When  $\lambda$  is real and sufficiently large, it is given by

$$A_{\text{st}}(\lambda) = \frac{i\kappa}{4\pi} G_{3,3}^{2,3} \left( \begin{matrix} \frac{1}{2}, & \frac{1}{2}, & \frac{1}{2} \\ 0, & 0, & -\frac{1}{2} \end{matrix} \middle| -\frac{\kappa^2}{16} \right) - \frac{\pi\kappa}{2} {}_3F_2 \left( \begin{matrix} 1, & 1, & 1 \\ 2, & 2, & 2 \end{matrix}; 1, \frac{3}{2}; -\frac{\kappa^2}{16} \right) - \pi^2, \quad (7.2.66)$$

and it is essentially proportional to the derivative of the free energy (7.2.36). The function  $A_{\text{st}}(\lambda)$  is complex, and at strong coupling it behaves like,

$$-iA_{\text{st}}(\lambda) = 2\pi^2\sqrt{2\lambda} + \pi^2 i + \mathcal{O}(e^{-2\pi\sqrt{2\lambda}}), \quad \lambda \gg 1. \quad (7.2.67)$$

Since the genus  $g$  amplitudes are real, the complex instanton governing the large order behavior of the  $1/N$  expansion must appear together with its complex conjugate, and it leads to an oscillatory asymptotics. If we write

$$A_{\text{st}}(\lambda) = |A_{\text{st}}(\lambda)| e^{i\theta(\lambda)}. \quad (7.2.68)$$

we have the behavior,

$$F_g(\lambda) - c_g \sim (2g)! |A_{\text{st}}(\lambda)|^{-2g} \cos(2g\theta(\lambda) + \delta(\lambda)), \quad g \gg 1, \quad (7.2.69)$$

where  $\delta(\lambda)$  is a function of the 't Hooft coupling, which in simple cases is determined by the one-loop corrections around the instanton. The oscillatory asymptotics in (7.2.69) suggests that the 't Hooft expansion is Borel summable. This was tested in [38] by detailed numerical calculations. However, the Borel resummation of the expansion does not reproduce the correct values of the free energy at finite  $N$  and  $k$ . The contribution of the complex instanton, which is of order (7.2.65), should be added in an appropriate way to the Borel-resummed 't Hooft expansion in order to reconstruct the exact answer for the free energy. In practice, this means that one should consider “trans-series” incorporating these exponentially small effects (see for example [37] for an introduction to trans-series.)

The resummation of the perturbative free energies in (7.2.61) in terms of an Airy function suggests another approach to the problem. Conceptually, the resummation of the genus expansion in type IIA superstring theory should be achieved by going to M-theory. The non-perturbative effects appearing in (7.2.65) should also appear naturally in an M-theory approach: by using (7.2.67), we see that they have the form, for  $\lambda \gg 1$ ,

$$\exp\left(-\sqrt{2\pi}k^{1/2}N^{1/2}\right). \quad (7.2.70)$$

In view of the AdS/CFT dictionary (7.2.7), the exponent in (7.2.70) goes like

$$k^{1/2}N^{1/2} \sim \left(\frac{L}{\ell_p}\right)^3. \quad (7.2.71)$$

This is the expected dependence on  $L$  for the action of a membrane instanton in M-theory, which corresponds to a D2-brane in type IIA theory. In [29], it was shown that a D2 brane wrapping the  $\mathbb{RP}^3$  cycle inside  $\mathbb{CP}^3$  would lead to the correct strong coupling limit of the action (7.2.67). Therefore, by going to M-theory, we could in principle incorporate not only the worldsheet instantons which were not taken into account in (7.2.61), but also the non-perturbative effects due to membrane instantons. In fact, it is well-known that in M-theory membrane and worldsheet instantons appear on equal footing [40].

### 7.2.3 The M-theory expansion

In the M-theory expansion,  $N$  is large and  $k$  is fixed, corresponding to the regime (7.2.9). The original study of the ABJM matrix model (7.2.21) in [4, 5] was done in the 't Hooft regime (7.2.14). It is now time to see if we can understand the matrix model directly in the M-theory regime and solve the problems raised at the end of the previous section: can we resum the genus expansion in some way? Can we incorporate the non-perturbative effects due to membrane instantons?

### The strict large $N$ limit

The first direct study of the M-theory regime of the matrix model (7.2.21) was performed in [7]. What should we expect in this regime, based on the results from the 't Hooft expansion? First of all, note that, in this regime,  $\lambda$  scales with  $N$ , therefore the M-theory regime corresponds to strong 't Hooft coupling. If we analyze the planar solution at strong coupling, we find that the endpoints of the cuts for the eigenvalues  $\mu_i, \nu_i$ , given in (7.2.34), behave like,

$$\begin{aligned} A &\approx \pi \sqrt{\frac{2N}{k} - \frac{1}{12} + \frac{i\pi}{2}}, \\ B &\approx \pi \sqrt{\frac{2N}{k} - \frac{1}{12} - \frac{i\pi}{2}}. \end{aligned} \quad (7.2.72)$$

Therefore, the equilibrium positions for the eigenvalues occur around arcs in the complex plane, and the real part of their endpoints grows like  $N^{1/2}$  at fixed  $k$ . Note that  $A$  and  $B$  are related by complex conjugation, in agreement with the symmetry of the equations (7.2.22) under  $\mu_i \rightarrow \nu_i^*$ . Although the above result is obtained by looking at the strong coupling behavior of the planar limit, it was verified in [7] by a numerical analysis of the equations (7.2.22) at large  $N$  and fixed  $k$ . It suggests the following ansatz for the M-theory limit of the distribution of the eigenvalues,

$$\mu_j = N^{1/2}x_j + iy_j, \quad \nu_j = N^{1/2}x_j - iy_j, \quad j = 1, \dots, N, \quad (7.2.73)$$

where  $x_j, y_j$  are of order one at large  $N$ . If we assume that the values of  $x_j, y_j$  become dense at large  $N$ , as suggested both by the planar limit and the numerical analysis, we should introduce a continuous parameter in the standard way,

$$\frac{j}{N} \rightarrow \xi \in [0, 1], \quad (7.2.74)$$

so that the limiting distributions are described by functions  $x(\xi), y(\xi)$ . We also introduce the density of eigenvalues

$$\rho(x) = \frac{d\xi}{dx}. \quad (7.2.75)$$

A detailed analysis performed in [7] shows that, when  $N$  is large, the free energy of the matrix model can be written as a functional of  $\rho(x)$  and  $y(x) = y(\xi(x))$ ,

$$-F(N, k) = N^{3/2} \left[ \frac{k}{\pi} \int dx x \rho(x) y(x) + \int dx \rho^2(x) f(2y(x)) - \frac{m}{2\pi} \left( \int dx \rho(x) - 1 \right) \right]. \quad (7.2.76)$$

Here,  $f(t)$  is a periodic function of  $t$ , with period  $2\pi$ , and given by

$$f(t) = \pi^2 - t^2, \quad t \in [-\pi, \pi]. \quad (7.2.77)$$

The last term in (7.2.76) involves, as usual, a Lagrange multiplier  $m$  imposing the normalization of  $\rho(x)$ . As stressed in [7], the above functional is local in the functions  $\rho(x), y(x)$ , in

contrast to the standard functional for the planar limit of matrix model, which involves an interaction between  $\rho(x)$  and  $\rho(x')$  at different points  $x, x'$ . The reason is that the non-local part of the interaction between the eigenvalues cancels due to the presence of the cosh term in the denominator of (7.2.21). Varying the functional (7.2.76) w.r.t.  $\rho(x)$  and  $y(x)$ , one obtains the two equations

$$\begin{aligned} 2\pi\rho(x)f'(2y(x)) &= -kx, \\ 4\pi\rho(x)f(2y(x)) &= m - 2kxy(x), \end{aligned} \tag{7.2.78}$$

which are solved by

$$\rho(x) = \frac{m}{4\pi^3}, \quad y(x) = \frac{\pi^2 kx}{2m}. \tag{7.2.79}$$

The support of  $\rho(x), y(x)$  is the interval  $[-x_*, x_*]$ . One fixes  $x_*$  and  $m$  from the normalization of  $\rho$  and by minimizing  $-F$ . This gives

$$x_* = \pi\sqrt{\frac{2}{k}}, \quad m = \frac{2\pi^3}{x_*}. \tag{7.2.80}$$

Therefore,

$$y(x_*) = \frac{\pi}{2}, \tag{7.2.81}$$

in agreement with the planar solution at strong coupling (7.2.72). Evaluating the free energy for the functions (7.2.79) and the values (7.2.80) of  $x_*, m$ , one finds

$$-F(N, k) \approx \frac{\pi\sqrt{2}}{3}k^{1/2}N^{3/2}, \quad N \gg 1, \tag{7.2.82}$$

which agrees with the prediction of M-theory (7.2.17). Note that the density of eigenvalues  $\rho(x)$  in (7.2.79) is a constant. This agrees again with the strong coupling limit of the planar densities of eigenvalues  $\rho_1(X), \rho_2(Y)$  in (7.2.31), as shown in [41].

The result (7.2.57), obtained by a partial resummation of the 't Hooft expansion, shows that the M-theory expansion of the ABJM free energy has subleading corrections at large  $N$ , as well as non-perturbative corrections coming from worldsheet instantons. Can we derive these corrections directly from a study of the ABJM matrix model? In particular, we would like to obtain in the M-theory expansion a quantitative understanding of the non-perturbative corrections of the form (7.2.70), which are invisible in the 't Hooft expansion. As shown in [42], the next-to-leading correction to (7.2.82) at large  $N$  and fixed  $k$  can be computed by extending the analysis of [7] that we have just reviewed. However, this just captures the leading effect due to the shift of  $\lambda$  incorporated in the variable  $\hat{\lambda}$  of (7.2.40), which is the variable appearing naturally in the planar expression (7.2.43). Including further corrections seems difficult to do in the approach of [7]. This motivates another approach which was started in [43] and has been very useful in understanding the corrections to the strict large  $N$  limit.

## The Fermi gas approach

There is a long tradition relating matrix integrals to fermionic theories. One reason for this is that the Vandermonde determinant

$$\Delta(\mu) = \prod_{i < j} (\mu_i - \mu_j) \quad (7.2.83)$$

appearing in these integrals can be regarded, roughly speaking, as a Slater determinant in a theory of  $N$  one-dimensional fermions with positions  $\mu_i$ . For example, the fact that this factor vanishes whenever two particles are at the same point can be regarded as a manifestation of Pauli's exclusion principle.

The rewriting of the ABJM matrix integral in terms of fermionic quantities can be regarded as a variant of this idea. It should be remarked however that the Fermi gas approach that we will explain in this section is not a universal technique which can be applied to any matrix integral with a Vandermonde-like interaction. It rather requires a specific type of eigenvalue interaction, which turns out to be typical of many matrix integrals appearing in the localization of Chern–Simons–matter theories.

The starting point for the Fermi gas approach is the observation that the interaction term in the matrix integral (7.2.21) can be rewritten by using the Cauchy identity,

$$\begin{aligned} \frac{\prod_{i < j} \left[ 2 \sinh \left( \frac{\mu_i - \mu_j}{2} \right) \right] \left[ 2 \sinh \left( \frac{\nu_i - \nu_j}{2} \right) \right]}{\prod_{i, j} 2 \cosh \left( \frac{\mu_i - \nu_j}{2} \right)} &= \det_{ij} \frac{1}{2 \cosh \left( \frac{\mu_i - \nu_j}{2} \right)} \\ &= \sum_{\sigma \in S_N} (-1)^{\epsilon(\sigma)} \prod_i \frac{1}{2 \cosh \left( \frac{\mu_i - \nu_{\sigma(i)}}{2} \right)}. \end{aligned} \quad (7.2.84)$$

In this equation,  $S_N$  is the permutation group of  $N$  elements, and  $\epsilon(\sigma)$  is the signature of the permutation  $\sigma$ . After some manipulations spelled out in detail in [44], one obtains [43, 44]

$$Z(N, k) = \frac{1}{N!} \sum_{\sigma \in S_N} (-1)^{\epsilon(\sigma)} \int \frac{d^N x}{(2\pi k)^N} \prod_{i=1}^N \rho(x_i, x_{\sigma(i)}), \quad (7.2.85)$$

where

$$\rho(x_1, x_2) = \frac{1}{2\pi k} \frac{1}{\left(2 \cosh \frac{x_1}{2}\right)^{1/2}} \frac{1}{\left(2 \cosh \frac{x_2}{2}\right)^{1/2}} \frac{1}{2 \cosh \left(\frac{x_1 - x_2}{2k}\right)}. \quad (7.2.86)$$

The expression (7.2.85) can be immediately identified [45] as the canonical partition function of a one-dimensional ideal Fermi gas of  $N$  particles, where (7.2.86) is the canonical density matrix. Notice that, by using the Cauchy identity again, with  $\mu_i = \nu_i$ , we can rewrite (7.2.85) as a matrix integral involving one single set of  $N$  eigenvalues,

$$Z(N, k) = \frac{1}{N!} \int \prod_{i=1}^N \frac{dx_i}{4\pi k} \frac{1}{2 \cosh \frac{x_i}{2}} \prod_{i < j} \left( \tanh \left( \frac{x_i - x_j}{2k} \right) \right)^2. \quad (7.2.87)$$

The canonical density matrix (7.2.86) is related to the Hamiltonian operator  $\mathbf{H}$  in the usual way,

$$\rho(x_1, x_2) = \langle x_1 | \rho | x_2 \rangle, \quad \rho = e^{-\mathbf{H}}, \quad (7.2.88)$$

where the inverse temperature  $\beta = 1$  is fixed. We will come back to the construction of the Hamiltonian shortly.

Since ideal quantum gases are better studied in the grand canonical ensemble, the above representation suggests to look at the grand canonical partition function, defined by

$$\Xi(\mu, k) = 1 + \sum_{N \geq 1} Z(N, k) e^{N\mu}. \quad (7.2.89)$$

Here,  $\mu$  is the chemical potential. The grand canonical potential is

$$\mathcal{J}(\mu, k) = \log \Xi(\mu, k). \quad (7.2.90)$$

A standard argument (presented for example in [45]) tells us that

$$\mathcal{J}(\mu, k) = - \sum_{\ell \geq 1} \frac{(-\kappa)^\ell}{\ell} Z_\ell, \quad (7.2.91)$$

where

$$\kappa = e^\mu \quad (7.2.92)$$

is the fugacity, and

$$Z_\ell = \text{Tr} \rho^\ell = \int dx_1 \cdots dx_\ell \rho(x_1, x_2) \rho(x_2, x_3) \cdots \rho(x_{\ell-1}, x_\ell) \rho(x_\ell, x_1). \quad (7.2.93)$$

As is well-known, the canonical and the grand-canonical formulations are equivalent, and the canonical partition function is recovered from the grand canonical one by integration,

$$Z(N, k) = \oint \frac{d\kappa}{2\pi i} \frac{\Xi(\mu, k)}{\kappa^{N+1}}. \quad (7.2.94)$$

Since we are dealing with an ideal gas, all the physics is in principle encoded in the spectrum of the Hamiltonian  $\mathbf{H}$ . This spectrum is defined by,

$$\rho |\varphi_n\rangle = e^{-E_n} |\varphi_n\rangle, \quad n = 0, 1, \dots, \quad (7.2.95)$$

or, equivalently, by the integral equation associated to the kernel (7.2.86),

$$\int \rho(x, x') \varphi_n(x') dx' = e^{-E_n} \varphi_n(x), \quad n = 0, 1, \dots \quad (7.2.96)$$

It can be verified that this spectrum is indeed discrete and the energies are real. This is because, as it can be easily checked, (7.2.86) defines a positive, trace-class operator on  $L^2(\mathbb{R})$ , and the above properties of the spectrum follow from standard results in the theory of such operators (see, for example, [46]). The thermodynamics is completely determined by the

spectrum: the grand canonical partition function is given by the Fredholm determinant associated to the integral operator (7.2.86),

$$\Xi(\mu, k) = \det(1 + \kappa\rho) = \prod_{n \geq 0} (1 + \kappa e^{-E_n}). \quad (7.2.97)$$

In terms of the density of eigenvalues

$$\rho(E) = \sum_{n \geq 0} \delta(E - E_n), \quad (7.2.98)$$

we also have the standard formula

$$\mathcal{J}(\mu, k) = \int_0^\infty dE \rho(E) \log(1 + \kappa e^{-E}). \quad (7.2.99)$$

What can we learn from the ABJM partition function in the Fermi gas formalism? The first thing we can do is to derive the strict large  $N$  limit of the free energy, including the correct coefficient. To do this, we have to be more precise about the Hamiltonian of the theory, which is defined implicitly by (7.2.88) and (7.2.86). Let us first write the density matrix (7.2.86) as

$$\rho = e^{-\frac{1}{2}U(\mathbf{x})} e^{-T(\mathbf{p})} e^{-\frac{1}{2}U(\mathbf{x})}. \quad (7.2.100)$$

In this equation,  $\mathbf{x}, \mathbf{p}$  are canonically conjugate operators,

$$[\mathbf{x}, \mathbf{p}] = i\hbar, \quad (7.2.101)$$

and

$$\hbar = 2\pi k. \quad (7.2.102)$$

Note that  $\hbar$  is the inverse coupling constant of the gauge theory/string theory, therefore semiclassical or WKB expansions in the Fermi gas correspond to strong coupling expansions in gauge theory/string theory. Finally, the potential  $U(x)$  in (7.2.100) is given by

$$U(x) = \log\left(2 \cosh \frac{x}{2}\right), \quad (7.2.103)$$

and the kinetic term  $T(p)$  is given by the same function,

$$T(p) = \log\left(2 \cosh \frac{p}{2}\right). \quad (7.2.104)$$

Indeed, we have

$$\begin{aligned} \langle x' | \rho | x \rangle &= e^{-\frac{1}{2}U(x') - \frac{1}{2}U(x)} \int dp dp' \langle x' | p \rangle \langle p | e^{-T(p)} | p' \rangle \langle p' | x \rangle \\ &= e^{-\frac{1}{2}U(x') - \frac{1}{2}U(x)} \int \frac{dp}{2\pi\hbar} \frac{e^{\frac{i}{\hbar}p(x'-x)}}{2 \cosh\left(\frac{p}{2}\right)} = \frac{1}{2\pi k} e^{-\frac{1}{2}U(x') - \frac{1}{2}U(x)} \frac{1}{2 \cosh\left(\frac{x-x'}{2k}\right)}, \end{aligned} \quad (7.2.105)$$

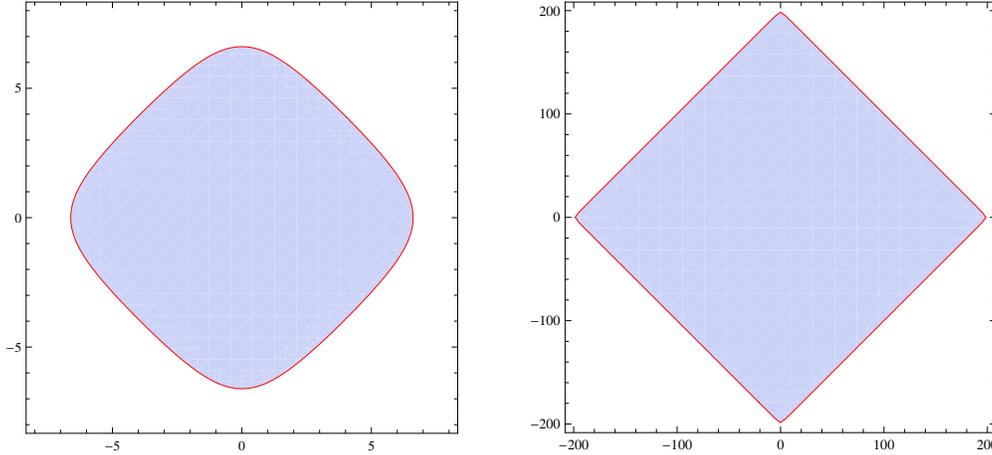

Figure 7.2: The Fermi surface (7.2.108) for ABJM theory in the  $q = x-p$  plane, for  $E = 4$  (left) and  $E = 100$  (right). When the energy is large, the Fermi surface approaches the polygon (7.2.109).

which is (7.2.86). The resulting Hamiltonian is not standard. First of all, the kinetic term leads to an operator involving an infinite number of derivatives (by expanding it around  $p = 0$ ), and it should be regarded as a difference operator, as we will see later. Second, the ordering of the operators in (7.2.100) shows that the Hamiltonian we are dealing with is not the sum of the kinetic term plus the potential, but it includes  $\hbar$  corrections due to non-trivial commutators. This is for example what happens when one considers quantum theories on the lattice: the standard Hamiltonian is only recovered in the continuum limit, which sets the commutators to zero. All these complications can be treated appropriately, and we will address some of them in this expository article, but let us first try to understand what happens when  $N$  is large.

The potential in (7.2.103) is a confining one, and at large  $x$  it behaves linearly,

$$U(x) \approx \frac{|x|}{2}, \quad |x| \rightarrow \infty. \quad (7.2.106)$$

When the number of particles in the gas,  $N$ , is large, the typical energies are large, and we are in the semiclassical regime. In that case, we can ignore the quantum corrections to the Hamiltonian and take its classical limit

$$H_{\text{cl}}(x, p) = U(x) + T(p). \quad (7.2.107)$$

Standard semiclassical considerations indicate that the number of particles  $N$  is given by the area of the Fermi surface, defined by

$$H_{\text{cl}}(x, p) = E, \quad (7.2.108)$$

divided by  $2\pi\hbar$ , the volume of an elementary cell. However, for large  $E$ , we can replace  $U(x)$  and  $T(p)$  by their leading behaviors at large argument, so that the Fermi surface is well approximated by the polygon,

$$\frac{|x|}{2} + \frac{|p|}{2} = E. \quad (7.2.109)$$

This can be seen in Fig. 7.2, where we show the Fermi surface computed from (7.2.108) for two values of the energies, a moderate one and a large one. For the large one, the Fermi surface is very well approximated by the polygon of (7.2.109). The area of this polygon is  $8E^2$ . Therefore, by using the relation between the grand potential and the average number of particles,

$$\frac{\partial \mathcal{J}(\mu, k)}{\partial \mu} = \langle N(\mu, k) \rangle \approx \frac{8\mu^2}{2\pi\hbar}, \quad (7.2.110)$$

we obtain immediately

$$\mathcal{J}(\mu, k) \approx \frac{2\mu^3}{3\pi^2 k}. \quad (7.2.111)$$

To compute the free energy, we note that, at large  $N$ , the contour integral (7.2.94) can be computed by a saddle-point approximation, which leads to the standard Legendre transform,

$$F(N, k) \approx \mathcal{J}(\mu_*, k) - \mu_* N, \quad (7.2.112)$$

where  $\mu_*$  is the function of  $N$  and  $k$  defined by (7.2.110), i.e.

$$\mu_* \approx \frac{\sqrt{2}}{2} \pi k^{1/2} N^{1/2}. \quad (7.2.113)$$

In this way, we immediately recover the result (7.2.82) from (7.2.112). In particular, the scaling  $3/2$  is a simple consequence from the analysis: it is the expected scaling for a Fermi gas in one dimension with a linearly confining potential and an ultra-relativistic dispersion relation  $T(p) \propto |p|$  at large  $p$ . This is arguably the simplest derivation of the result (7.2.82), as it uses only elementary notions in Statistical Mechanics. Note that in this derivation we have considered the M-theory regime in which  $N$  is large and  $k$  is fixed, and we have focused on the strict large  $N$  limit considered in [7] and reviewed in the last section. The main question is now: can we use the Fermi gas formulation to obtain explicit results for the corrections to the strict large  $N$  limit? In the next sections we will address this question.

## The WKB expansion of the Fermi gas

In the Fermi gas approach, the physics of the partition function is encoded in a quantum ideal gas. Although the gas is non-interacting, its one-particle Hamiltonian is complicated, and the energy levels  $E_n$  in (7.2.95) are not known in closed form. What can we do in this situation? As we have seen in (7.2.102), the parameter  $k$  corresponds to the Planck constant of the quantum Fermi gas. Therefore, we can try a systematic development around  $k = 0$ , i.e. a semiclassical WKB approximation. Such an approach should give a way of computing corrections to (7.2.111) and (7.2.82). Of course, we are not *a priori* interested in the physics at

small  $k$ , but rather at *finite*  $k$ , and in particular at integer  $k$ . However, the expansion at small  $k$  gives important clues about the problem at finite  $k$  and it can be treated systematically.

There are two ways of working out the WKB expansion: we can work directly at the level of the grand potential, or we can work at the level of the energy spectrum. Let us first consider the problem at the level of the grand potential. It turns out that, in order to perform a systematic semiclassical expansion, the most useful approach is Wigner's phase space formulation of Quantum Mechanics (in fact, this formulation was originally introduced by Wigner in order to understand the semiclassical expansion of thermodynamic quantities.) A detailed application of this formalism to the ABJM Fermi gas can be found in [43, 47]. The main idea of the method is to map quantum-mechanical operators to functions in classical phase space through the Wigner transform. Under this map, the product of operators famously becomes the  $\star$  or Moyal product (see for example [48] for a review, and [49] for an elegant summary with applications). This approach is particularly useful in view of the nature of our Hamiltonian  $\mathbf{H}$ , which includes quantum corrections. The Wigner transform of  $\mathbf{H}$  has the structure

$$H_W(x, p) = H_{\text{cl}}(x, p) + \sum_{n \geq 1} \hbar^{2n} H_W^{(n)}(x, p), \quad (7.2.114)$$

where  $H_{\text{cl}}(x, p)$  is the classical Hamiltonian introduced in (7.2.107). Proceeding in this way, we obtain a systematic  $\hbar$  expansion of all the quantities of the theory. The WKB expansion of the grand potential reads,

$$\mathcal{J}^{\text{WKB}}(\mu, k) = \sum_{n \geq 0} \mathcal{J}_n(\mu) k^{2n-1}. \quad (7.2.115)$$

Note that this is principle an approximation to the full function  $\mathcal{J}(\mu, k)$ , since it does not take into account non-perturbative effects in  $\hbar$ . The functions  $\mathcal{J}_n(\mu)$  in this expansion can be in principle computed in closed form, although their calculation becomes more and more cumbersome as  $n$  grows. The leading term  $n = 0$  is however relatively easy to compute [43]. We first notice that the traces (7.2.93) have a simple semiclassical limit,

$$Z_\ell \approx \int \frac{dx dp}{2\pi\hbar} e^{-\ell H_{\text{cl}}(x, p)}, \quad \hbar \rightarrow 0, \quad (7.2.116)$$

which is just the classical average, with an appropriate measure which includes the volume of the elementary quantum cell  $2\pi\hbar$ . By using the integral

$$\int_{-\infty}^{\infty} \frac{d\xi}{\left(2 \cosh \frac{\xi}{2}\right)^\ell} = \frac{\Gamma^2(\ell/2)}{\Gamma(\ell)}, \quad (7.2.117)$$

we find

$$k Z_\ell \approx \frac{1}{2\pi} \frac{\Gamma^4(\ell/2)}{\Gamma^2(\ell)}, \quad \hbar \rightarrow 0, \quad (7.2.118)$$

and

$$\mathcal{J}_0(\mu) = - \sum_{\ell=1}^{\infty} \frac{(-\kappa)^\ell}{4\pi^2} \frac{\Gamma^4(\ell/2)}{\ell \Gamma^2(\ell)}. \quad (7.2.119)$$

This expression is convenient when  $\kappa$  is small, i.e. for  $\mu \rightarrow -\infty$ . To make contact with the large  $N$  limit, we need to consider the limit of large, positive chemical potential,  $\mu \rightarrow +\infty$ . As we will see in the next section, this can be done by using a Mellin–Barnes integral, and one finds

$$\mathcal{J}_0(\mu) = \frac{2\mu^3}{3\pi^2} + \frac{\mu}{3} + \frac{2\zeta(3)}{\pi^2} + J_0^{\text{M2}}(\mu), \quad (7.2.120)$$

where

$$J_0^{\text{M2}}(\mu) = \sum_{\ell=1}^{\infty} \left( a_{0,\ell} \mu^2 + b_{0,\ell} \mu + c_{0,\ell} \right) e^{-2\ell\mu}, \quad (7.2.121)$$

and  $a_{0,\ell}$ ,  $b_{0,\ell}$  and  $c_{0,\ell}$  are computable coefficients. The leading, cubic term in  $\mu$  in (7.2.120) is the one we found in (7.2.111). The subleading term in  $\mu$  gives a correction of order  $N^{1/2}$  to the leading behavior (7.2.82). The function  $J_0^{\text{M2}}(\mu)$  involves an infinite series of exponentially small corrections in  $\mu$ . Note that, although this result for  $\mathcal{J}_0(\mu)$  is semiclassical in  $\hbar$ , it goes beyond the leading result at large  $N$  in (7.2.82). This is because it takes into account the exact classical Fermi surface (7.2.108), rather than its polygonal approximation (7.2.109). Therefore, we see that, already at this level, the Fermi gas approach makes it possible to go beyond the strict large  $N$  limit.

Of particular interest are the exponentially small terms in  $\mu$  in (7.2.121). What is their meaning? By taking into account that, at large  $N$ ,  $\mu$  is given in (7.2.113), one finds that these corrections to  $\mathcal{J}(\mu, k)$  lead to corrections in  $Z(N, k)$  precisely of the form (7.2.70). We recall that these were found originally in the matrix model as non-perturbative effects in the 't Hooft expansion. We conclude that the exponentially small corrections in  $\mu$  in (7.2.121), which in the Fermi gas approach appear already in the semi-classical approximation, correspond to non-perturbative corrections to the genus expansion, and should be identified as membrane instanton contributions.

It is possible to go beyond the leading order of the WKB expansion of the grand potential and compute the corrections appearing in (7.2.115). The function  $\mathcal{J}_1(\mu)$  was also derived in [43] and its large  $\mu$  expansion has the following form,

$$\mathcal{J}_1(\mu) = \frac{\mu}{24} - \frac{1}{12} + \mathcal{O}\left(\mu^2 e^{-2\mu}\right). \quad (7.2.122)$$

Moreover, the following non-renormalization theorem can be proved [43]: for  $n \geq 2$ , the  $n$ -th order correction to the WKB expansion is given by a  $\mu$ -independent constant  $A_n$ , and a function which is exponentially suppressed as  $\mu \rightarrow \infty$ , i.e.

$$\mathcal{J}_n(\mu) = A_n + \mathcal{O}\left(\mu^2 e^{-2\mu}\right), \quad n \geq 2. \quad (7.2.123)$$

The exponentially small terms appearing in the functions  $\mathcal{J}_n(\mu)$  with  $n \geq 1$  have the same structure as for  $n = 0$ . We then conclude that, in the WKB approximation, i.e. as a power series in  $k$  around  $k = 0$ , the grand potential has the structure

$$\mathcal{J}^{\text{WKB}}(\mu, k) = J^{(\text{p})}(\mu) + J^{\text{M2}}(\mu, k). \quad (7.2.124)$$

In this equation, the perturbative piece  $J^{(p)}(\mu)$  is given by

$$J^{(p)}(\mu) = \frac{C(k)}{3}\mu^3 + B(k)\mu + A(k), \quad (7.2.125)$$

where  $B(k)$  and  $C(k)$  were defined in (7.2.56), and (7.2.62), respectively, and  $A(k)$  is given by the formal power series expansion

$$A(k) = \sum_{n \geq 0} A_n k^{2n-1}, \quad (7.2.126)$$

where

$$A_0 = \frac{2\zeta(3)}{\pi^2}, \quad A_1 = -\frac{1}{12}, \quad (7.2.127)$$

as one finds from (7.2.120) and (7.2.122). This series turns out to be the asymptotic expansion around  $k = 0$  of the function defined in (7.2.59) (and this is why we have used the same notation for both). Therefore, the function  $A(k)$  has two different asymptotic expansions: one of them gives the constants  $A_n$  appearing in the WKB analysis of the grand potential, as we have just seen. The other one gives the genus  $g$ , constant map contributions to the free energy  $c_g$  which appear in the 't Hooft expansion, as we saw in (7.2.60). The second term in the r.h.s. of (7.2.124) has the structure,

$$J^{M2}(\mu) = \sum_{\ell=1}^{\infty} (a_{\ell}(k)\mu^2 + b_{\ell}(k)\mu + c_{\ell}(k)) e^{-2\ell\mu}, \quad (7.2.128)$$

where the coefficients have the WKB expansion,

$$a_{\ell}(k) = \sum_{n \geq 0} a_{n,\ell} k^{2n-1}. \quad (7.2.129)$$

Similar expansions hold for  $b_{\ell}(k)$ ,  $c_{\ell}(k)$ .

We can now plug the result (7.2.124) in (7.2.94). In the  $\mu$ -plane, this is an integral from  $-\pi i$  to  $\pi i$ :

$$Z(N, k) = \frac{1}{2\pi i} \int_{-\pi i}^{\pi i} \frac{d\mu}{2\pi i} e^{\mathcal{J}(\mu, k) - N\mu}. \quad (7.2.130)$$

If we neglect exponentially small corrections in  $N$ , we can deform the contour  $[-\pi i, \pi i]$  to the contour  $\mathcal{C}$  shown in Fig. 7.3. Therefore, we find that, up to these corrections,

$$Z(N, k) \approx \frac{1}{2\pi i} \int_{\mathcal{C}} \exp(J^{(p)}(\mu) - \mu N) d\mu. \quad (7.2.131)$$

The above integral is given by an Airy function, and we immediately recover the result (7.2.61) for the perturbative  $1/N$  expansion at fixed  $k$ . As explained before, this includes all the  $1/N$  corrections to the partition function in a single strike.

We see that the Fermi gas approach leads to a powerful derivation of the Airy function behavior of the partition function. In this approach, such a derivation just requires computing the grand potential at next-to-leading order in the WKB expansion. Although this is a one-loop result, it is exact in  $k$  if we neglect exponentially small corrections in  $\mu$ . Therefore, a one-loop calculation in the grand-canonical ensemble leads to an all-orders result in the canonical ensemble.

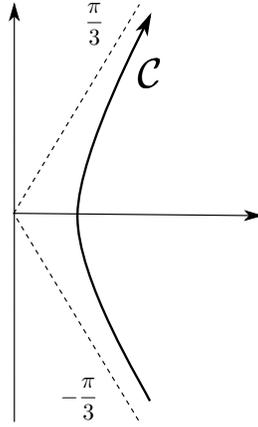

Figure 7.3: The contour  $\mathcal{C}$  in the complex plane of the chemical potential.

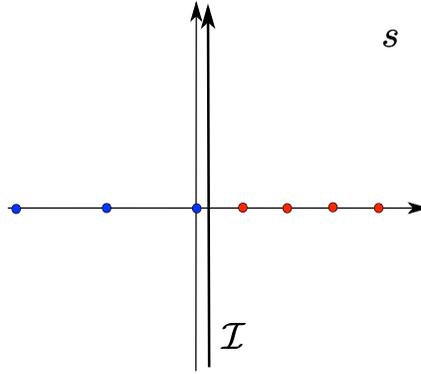

Figure 7.4: The contour  $\mathcal{I}$  in the complex  $s$  plane. By closing the contour to the right, we encircle the poles at  $s = n$ ,  $n \in \mathbb{Z}_{>0}$ . By closing the contour to the left, we encircle the poles at  $s = -2n$ ,  $n \in \mathbb{Z}_{\geq 0}$ .

### From the WKB expansion to the refined topological string

In order to complete our understanding of the WKB expansion of the Fermi gas, we should determine the coefficients appearing in the expansion (7.2.128). We can in principle compute them order by order in powers of  $k$  by using standard semiclassical techniques, but it would be much better to know the full expansion explicitly. As first noted in [50], it turns out that there is an elegant and powerful answer for the all-orders WKB grand potential, which involves the *refined* topological string of local  $\mathbb{P}^1 \times \mathbb{P}^1$  in the so-called Nekrasov–Shatashvili (NS) limit [51]. A good starting point for understanding this connection is to formulate the problem of computing the semiclassical limit  $\mathcal{J}_0(\mu)$  in a way which makes contact with the theory of periods of CY manifolds.

Let us consider again the expression (7.2.119) for the semiclassical grand potential, and

let us write this infinite sum as a Mellin–Barnes integral,

$$\mathcal{J}_0(\kappa) = -\frac{1}{4\pi^2} \int_{\mathcal{I}} \frac{ds}{2\pi i} \frac{\Gamma(-s)\Gamma(s/2)^4}{\Gamma(s)} \kappa^s, \quad (7.2.132)$$

where the contour  $\mathcal{I}$  runs parallel to the imaginary axis, see Fig. 7.4<sup>3</sup>. It can be deformed so that the integral encloses the poles of  $\Gamma(-s)$  at  $s = n$ ,  $n = 1, \dots$  (in the clockwise direction). The residues at these poles give back the infinite series in (7.2.119). We can however deform the contour in the opposite direction, so that it encloses the poles at

$$s = -2m, \quad m = 0, 1, 2, \dots, \quad (7.2.133)$$

and we find

$$\mathcal{J}_0(\kappa) = -\frac{1}{4\pi^2} \sum_{n=0}^{\infty} \text{Res}_{s=-2n} \left[ \frac{\Gamma(-s)\Gamma(s/2)^4}{\Gamma(s)} \kappa^s \right]. \quad (7.2.134)$$

The pole at  $s = 0$  gives

$$\frac{2}{3\pi^2} \mu^3 + \frac{1}{3} \mu + \frac{2\zeta(3)}{\pi^2}, \quad (7.2.135)$$

which is precisely the leading part of (7.2.120) as  $\mu \rightarrow \infty$ . To understand the contribution of the rest of the poles, let us consider the following differential operator,

$$\mathcal{L} = \theta^3 - 4z\theta(2\theta + 1)^2, \quad (7.2.136)$$

where

$$\theta = z \frac{d}{dz}. \quad (7.2.137)$$

A basis of solutions to the equation

$$\mathcal{L}\Pi = 0 \quad (7.2.138)$$

can be obtained by using the Frobenius method. One first considers the so-called fundamental period or solution,

$$\varpi_0(z, \rho) = \sum_{n \geq 0} a_n(\rho) z^{n+\rho}, \quad (7.2.139)$$

where

$$a_n(\rho) = 16^n \frac{\Gamma^2\left(n + \rho + \frac{1}{2}\right) \Gamma(n + \rho)}{\Gamma^3(n + \rho + 1)} \frac{\Gamma^3(\rho + 1)}{\Gamma^2\left(\rho + \frac{1}{2}\right) \Gamma(\rho)}. \quad (7.2.140)$$

The Frobenius method instruct us to look at the functions,

$$\varpi_k(z) = \left. \frac{d^k \varpi_0(z, \rho)}{d\rho^k} \right|_{\rho=0}. \quad (7.2.141)$$

---

<sup>3</sup>The Mellin–Barnes technique to study the grand potential was independently developed in [52].

For  $k = 1, 2, 3$ , they have the following structure,

$$\begin{aligned}\varpi_1(z) &= \log z + \widetilde{\varpi}_1(z), \\ \varpi_2(z) &= (\log z)^2 + 2 \log z \widetilde{\varpi}_1(z) + \widetilde{\varpi}_2(z), \\ \varpi_3(z) &= (\log z)^3 + 3 (\log z)^2 \widetilde{\varpi}_1(z) + 3 \log z \widetilde{\varpi}_2(z) + \widetilde{\varpi}_3(z),\end{aligned}\tag{7.2.142}$$

where the  $\widetilde{\varpi}_k(z)$  are power series in  $z$ ,

$$\widetilde{\varpi}_k(z) = \sum_{n=1}^{\infty} \left( \frac{d^k a_n(\rho)}{d\rho^k} \right)_{\rho=0} z^n.\tag{7.2.143}$$

We have, for example,

$$\begin{aligned}\widetilde{\varpi}_1(z) &= \sum_{n=1}^{\infty} \frac{1}{n} \left( \frac{\Gamma\left(n + \frac{1}{2}\right)}{\Gamma\left(\frac{1}{2}\right)n!} \right)^2 (16z)^n, \\ \widetilde{\varpi}_2(z) &= \sum_{n=1}^{\infty} \frac{4}{n} \left( \frac{\Gamma\left(n + \frac{1}{2}\right)}{\Gamma\left(\frac{1}{2}\right)n!} \right)^2 \left[ \psi\left(n + \frac{1}{2}\right) - \psi(n + 1) + 2 \log 2 - \frac{1}{2n} \right] (16z)^n.\end{aligned}\tag{7.2.144}$$

When  $k = 1, 2$ , the functions  $\varpi_k(z)$  give solutions to the equation (7.2.138). After some simple manipulations, it is easy to see that the contribution to  $\mathcal{J}_0(\kappa)$  of the residue at  $s = -2n$ ,  $n \neq 0$ , is given by

$$-\frac{1}{8\pi^2} \text{Res}_{\epsilon=0} \frac{\Gamma\left(1 - \frac{\epsilon}{2}\right)^4 \Gamma\left(\frac{\epsilon}{2}\right)^4 \Gamma\left(n - \frac{\epsilon}{2}\right) \Gamma\left(n - \frac{\epsilon}{2} + \frac{1}{2}\right)^2}{\Gamma(1 - \epsilon)\Gamma(\epsilon) \Gamma\left(n - \frac{\epsilon}{2} + 1\right)^3} (4/\kappa)^{2n-\epsilon}.\tag{7.2.145}$$

By setting  $\rho = -\epsilon/2$  and comparing to (7.2.140), we find

$$\mathcal{J}_0(\mu) = -\frac{1}{12\pi^2} \varpi_3(z) - \frac{1}{6} \varpi_1(z) + \frac{2\zeta(3)}{\pi^2},\tag{7.2.146}$$

where

$$z = e^{-2\mu}.\tag{7.2.147}$$

We also have

$$\begin{aligned}\sum_{\ell=1}^{\infty} a_{0,\ell} z^\ell &= -\frac{1}{\pi^2} \widetilde{\varpi}_1(z), \\ \sum_{\ell=1}^{\infty} b_{0,\ell} z^\ell &= \frac{1}{2\pi^2} \widetilde{\varpi}_2(z), \\ \sum_{\ell=1}^{\infty} c_{0,\ell} z^\ell &= -\frac{1}{12\pi^2} \widetilde{\varpi}_3(z) - \frac{1}{6} \widetilde{\varpi}_1(z).\end{aligned}\tag{7.2.148}$$

The structure above indicates a connection to topological string theory. The differential operator (7.2.136) is the Picard–Fuchs operator describing the genus zero topological string

on local  $\mathbb{P}^1 \times \mathbb{P}^1$  (see for example [53]). In this context, it is useful to define a so-called flat coordinate  $t$  and a genus zero free energy  $F_0(t)$  by the equations,

$$\begin{aligned} t &= -\varpi_1(z), \\ \frac{\partial F_0}{\partial t} &= \frac{1}{2}\varpi_2(z) - \frac{\pi^2}{3}, \end{aligned} \tag{7.2.149}$$

so that

$$F_0(t) = \frac{t^3}{6} - \frac{\pi^2 t}{3} - 2\zeta(3) - 4e^{-t} - \frac{9}{2}e^{-2t} - \dots \tag{7.2.150}$$

In terms of these quantities, one finds

$$\mathcal{J}_0(\mu) = \frac{1}{2\pi^2} \left( t \frac{\partial F_0}{\partial t} - 2F_0 \right). \tag{7.2.151}$$

We would like to understand now the higher order WKB corrections to the grand potential in the context of topological string theory, in line with what we have done for the leading, semiclassical function  $\mathcal{J}_0(\mu)$ . To do this, and following [54], we will look at the WKB expansion of the energy levels, i.e. we will consider the spectral problem defined by (7.2.95), (7.2.96). The first step is to reformulate (7.2.95) as a spectral problem for a difference equation. Let us define

$$|\psi\rangle = e^{\frac{1}{2}U(x)}|\phi\rangle. \tag{7.2.152}$$

It follows from (7.2.100) that (7.2.95) can be written as (we remove the indices for the discrete energies)

$$e^{U(x)}e^{T(p)}|\psi\rangle = e^E|\psi\rangle, \tag{7.2.153}$$

or, equivalently, in the coordinate representation,

$$\psi(x + i\pi k) + \psi(x - i\pi k) = \frac{e^E}{2 \cosh\left(\frac{x}{2}\right)}\psi(x). \tag{7.2.154}$$

This difference equation is equivalent to the original problem (7.2.95) provided some analyticity and boundary conditions are imposed on the function  $\psi(x)$ . Let us denote by  $\mathcal{S}_a$  the strip in the complex  $x$ -plane defined by

$$|\operatorname{Im}(x)| < a. \tag{7.2.155}$$

Let us also denote by  $A(\mathcal{S}_a)$  those functions  $g$  which are bounded and analytic in the strip, continuous on its closure, and for which  $g(x + iy) \rightarrow 0$  as  $x \rightarrow \pm\infty$  through real values, when  $y \in \mathbb{R}$  is fixed and satisfies  $|y| < a$ . It can be seen, by using for example the results in [55], that the equivalence of (7.2.154) and (7.2.95) requires that  $\psi(x)$  belongs to the space  $A(\mathcal{S}_{\pi k})$ .

The difference equation (7.2.154) can be solved in the WKB approximation, just as the Schrödinger equation (see for example [56]). One introduces a WKB ansatz,

$$\psi(x, \hbar) = \exp\left(\frac{1}{\hbar}S(x, \hbar)\right), \tag{7.2.156}$$

where

$$S(x, \hbar) = \sum_{n \geq 0} S_n(x) \hbar^n, \quad (7.2.157)$$

and we remember that  $\hbar$  is given by (7.2.102). The leading order approximation gives

$$S'_0(x) = p(x). \quad (7.2.158)$$

This defines a curve in phase space

$$y = p(x), \quad (7.2.159)$$

as well as a differential on that curve

$$\lambda(x) = p(x)dx. \quad (7.2.160)$$

In the case of the difference equation (7.2.154), the curve (7.2.159) is nothing but the equation for the Fermi surface (7.2.108). Geometrically, this is a curve of genus one, with two one-cycles  $A$  and  $B$ . The  $B$  period of the differential  $\lambda$  gives the classical volume of phase space,

$$\text{vol}_0(E) = \oint_B \lambda, \quad (7.2.161)$$

and the Bohr–Sommerfeld quantization condition says that this volume is quantized as

$$\text{vol}_0(E) = 2\pi\hbar \left( n + \frac{1}{2} \right), \quad n = 0, 1, 2, \dots \quad (7.2.162)$$

The quantum corrections in (7.2.157) can be also interpreted geometrically: we introduce a “quantum” differential

$$\lambda(x; \hbar) = \partial_x S(x, \hbar) dx, \quad (7.2.163)$$

and the perturbative, “quantum” volume of phase space is defined as

$$\text{vol}_p(E; \hbar) = \oint_B \lambda(x; \hbar) = \sum_{n \geq 0} \text{vol}_n(E) \hbar^{2n}. \quad (7.2.164)$$

As it is well-known since the work of Dunham [57], this leads to a quantum-corrected quantization condition of the form

$$\text{vol}_p(E) = 2\pi\hbar \left( n + \frac{1}{2} \right), \quad n = 0, 1, 2, \dots \quad (7.2.165)$$

It is straightforward to do an analysis of this problem order by order in  $\hbar$ , but exact as a function of  $E$ . The classical volume is given essentially by a Meijer function [43],

$$\text{vol}_0(E) = \frac{e^E}{\pi} G_{3,3}^{2,3} \left( \frac{e^{2E}}{16} \middle| \begin{matrix} \frac{1}{2}, \frac{1}{2}, \frac{1}{2} \\ 0, 0, -\frac{1}{2} \end{matrix} \right) - 4\pi^2, \quad (7.2.166)$$

which has the following behavior at large  $E$ ,

$$\text{vol}_0(E) = 8E^2 - \frac{4\pi^2}{3} + \mathcal{O}(E e^{-2E}). \quad (7.2.167)$$

The leading term is nothing but the area of the polygon (7.2.109). The corrections incorporate the difference between the volume, as computed by the exact Fermi surface, and the volume as computed in the polygonal approximation. One can also find [54],

$$\text{vol}_1(E) = \frac{e^{-E} \left( (32 e^{-2E} - 1) E(k_E) - K(k_E) \right)}{6 (16 e^{-2E} - 1)}, \quad (7.2.168)$$

where  $K(k_E)$ ,  $E(k_E)$  are elliptic integrals of the first and second kind, respectively, with modulus

$$k_E^2 = 1 - \frac{e^{2E}}{16}. \quad (7.2.169)$$

As we will explain in a moment, this calculation is the counterpart of the perturbative calculation of  $\mathcal{J}_n(\mu)$  that we considered in the previous section. What we really need, in order to understand the theory in the M-theory regime, is an approach which is exact in  $k$  (i.e. in  $\hbar$ ) but leads to an expansion at large  $E$ , since this corresponds to large  $N$ . In the case of the WKB problem we are analyzing here, we need to resum the WKB expansion of the perturbative volume at all orders in  $\hbar$ , but order by order in  $e^{-2E}$ . To do this, we will relate the spectral problem (7.2.95) to another one, which makes contact with the refined topological string [54]. Let us consider

$$\left( e^{\mathbf{u}} + z_1 e^{-\mathbf{u}} + e^{\mathbf{v}} + z_2 e^{-\mathbf{v}} - 1 \right) |\psi\rangle = 0, \quad (7.2.170)$$

where  $\mathbf{u}$ ,  $\mathbf{v}$  are operators satisfying the commutation relation,

$$[\mathbf{v}, \mathbf{u}] = \frac{i\hbar}{2}, \quad (7.2.171)$$

and  $z_1, z_2$  are complex parameters. If we do the following change of variables,

$$\mathbf{v} = \frac{\mathbf{x} + \mathbf{p}}{2} + \frac{i\pi k}{4} - E, \quad \mathbf{u} = \frac{\mathbf{x} - \mathbf{p}}{2} - \frac{i\pi k}{4} - E, \quad (7.2.172)$$

and consider the specialization

$$z_1 = q^{1/2} z \quad z_2 = q^{-1/2} z, \quad (7.2.173)$$

where

$$z = e^{-2E} \quad (7.2.174)$$

and

$$q = e^{\frac{i\hbar}{2}} = e^{\pi i k}, \quad (7.2.175)$$

the equation (7.2.170) becomes the difference equation (7.2.154). Note that the change of variables (7.2.172) is a canonical transformation, i.e. its classical version preserves the volume element of phase space, up to an overall factor. It turns out that the difference equation (7.2.170) appears in the context of refined topological string theory [58] (see also [59, 60]). It implements the “quantization” of the mirror curve of local  $\mathbb{P}^1 \times \mathbb{P}^1$ , and it leads to the

NS limit of the refined topological string. In particular, the periods of the exact quantum differential (or *quantum periods*) can be calculated as an expansion at small  $z_1, z_2$  but exactly in  $\hbar$  [50, 58]. Note that, in this context, the variables  $z_1, z_2$  are interpreted as complex deformation parameters of the mirror curve. In the case at hand, we have two quantum  $A$ -periods and two quantum  $B$ -periods, denoted by  $\Pi_{A_I}(z_1, z_2; \hbar), \Pi_{B_I}(z_1, z_2; \hbar), I = 1, 2$ . The  $A$ -periods have the structure

$$\Pi_{A_I}(z_1, z_2; \hbar) = \log z_I + \tilde{\Pi}_A(z_1, z_2; \hbar), \quad I = 1, 2. \quad (7.2.176)$$

The two quantum  $B$ -periods are related by the exchange of the moduli,

$$\Pi_{B_2}(z_1, z_2; \hbar) = \Pi_{B_1}(z_2, z_1; \hbar), \quad (7.2.177)$$

and they have the structure

$$\begin{aligned} \Pi_{B_1}(z_1, z_2; \hbar) &= -\frac{1}{8} \left( \log^2 z_1 - 2 \log z_1 \log z_2 - \log^2 z_2 \right) + \frac{1}{2} \log z_2 \tilde{\Pi}_A(z_1, z_2; \hbar) \\ &\quad + \frac{1}{4} \tilde{\Pi}_B(z_1, z_2; \hbar). \end{aligned} \quad (7.2.178)$$

The expansion of the periods around  $z_1 = z_2 = 0$  is given, to the very first orders, by,

$$\begin{aligned} \tilde{\Pi}_A(z_1, z_2; \hbar) &= 2(z_1 + z_2) + 3(z_1^2 + z_2^2) + 2(4 + q + q^{-1})z_1z_2 + \frac{20}{3}(z_1^3 + z_2^3) \\ &\quad + 2(16 + 6q + 6q^{-1} + q^2 + q^{-2})z_1z_2(z_1 + z_2) + \mathcal{O}(z_i^4), \\ \tilde{\Pi}_B(z_1, z_2; \hbar) &= 8 \left[ \frac{q+1}{2(q-1)} \log q \right] z_1 + 4 \left[ 1 + \frac{5q^2 + 8q + 5}{2(q^2 - 1)} \log q \right] z_1^2 \\ &\quad + 8 \left[ 1 + \frac{(1+q)^3}{2q(q-1)} \log q \right] z_1z_2 + 4z_2^2 + \mathcal{O}(z_i^3), \end{aligned} \quad (7.2.179)$$

where  $q$  is given in (7.2.175). In general, on a local CY manifold with  $n$  moduli, the quantum  $A$  periods define a “quantum” mirror map [58], relating the flat coordinates  $t_I$  to the complex moduli  $z_I, I = 1, \dots, n$ , while the quantum  $B$  periods define the NS free energy,  $F^{\text{NS}}$ ,

$$-t_I(\hbar) = \Pi_{A_I}(z_I; \hbar), \quad \frac{\partial F^{\text{NS}}}{\partial t_I} = \frac{1}{\hbar} \Pi_{B_I}(z_I; \hbar), \quad I = 1, \dots, n. \quad (7.2.180)$$

The NS free energy has an asymptotic expansion around  $\hbar = 0$ , of the form

$$F^{\text{NS}}(t_I; \hbar) = \sum_{n \geq 0} F_n^{\text{NS}}(t_I) \hbar^{2n-1}, \quad (7.2.181)$$

and the leading order term

$$F_0^{\text{NS}}(t_I) = F_0(t_I) \quad (7.2.182)$$

is the standard prepotential of the local CY manifold. The knowledge of the quantum mirror map and of the NS free energy, as a function of the flat coordinates  $t_I$ , is equivalent to knowing both periods.

Let us now come back to the problem of calculating (7.2.164). This is a quantum period for the spectral curve defined by (7.2.154), but this curve is just a specialization of (7.2.170) with the dictionary (7.2.173) and after a canonical transformation. Therefore, (7.2.164) should be a combination of the quantum periods of local  $\mathbb{P}^1 \times \mathbb{P}^1$ , specialized to the “slice” (7.2.173). Let us denote

$$\begin{aligned}\tilde{\Pi}_A(z; \hbar) &\equiv \tilde{\Pi}_A(q^{1/2}z, q^{-1/2}z; \hbar) = \sum_{\ell \geq 1} \hat{a}_\ell(\hbar) z^\ell, \\ \tilde{\Pi}_B(z; \hbar) &\equiv \frac{1}{2} \left( \tilde{\Pi}_B(q^{1/2}z, q^{-1/2}z; \hbar) + \tilde{\Pi}_B(q^{-1/2}z, q^{1/2}z; \hbar) \right) = \sum_{\ell \geq 1} \hat{b}_\ell(\hbar) z^\ell,\end{aligned}\tag{7.2.183}$$

where  $\hat{a}_\ell(\hbar)$ ,  $\hat{b}_\ell(\hbar)$  have the  $\hbar$ -expansion,

$$\hat{a}_\ell(\hbar) = \sum_{n=0}^{\infty} \hat{a}_\ell^{(n)} \hbar^{2n}, \quad \hat{b}_\ell(\hbar) = \sum_{n=0}^{\infty} \hat{b}_\ell^{(n)} \hbar^{2n}.\tag{7.2.184}$$

Note that the classical limits of  $\tilde{\Pi}_{A,B}(z; \hbar)$  are the power series  $\tilde{\omega}_{1,2}(z)$  written down in (7.2.144). Requiring the combination of quantum periods to have the correct classical limit, and that only even powers of  $\hbar$  appear, we find,

$$\begin{aligned}\text{vol}_p(E; \hbar) &= 4\Pi_{B_1}(q^{1/2}z, q^{-1/2}z; \hbar) + 4\Pi_{B_2}(q^{1/2}z, q^{-1/2}z; \hbar) - \frac{4\pi^2}{3} - \frac{\hbar^2}{12} \\ &= 8E^2 - \frac{4\pi^2}{3} + \frac{\hbar^2}{24} - 8E \sum_{\ell \geq 1} \hat{a}_\ell(\hbar) e^{-2\ell E} + 2 \sum_{\ell \geq 1} \hat{b}_\ell(\hbar) e^{-2\ell E}.\end{aligned}\tag{7.2.185}$$

This is the resummation we were looking for, and solves the problem of computing the perturbative, quantum volume of phase space by re-expressing it in terms of quantities associated to the quantum mirror symmetry of local  $\mathbb{P}^1 \times \mathbb{P}^1$ .

Let us make contact with the grand potential. Of course, this is not independent of the quantum volume of phase space, since in an ideal gas the spectrum of the Hamiltonian determines the thermodynamics. From the expression (7.2.97) as a Fredholm determinant, we have

$$\mathcal{J}(\mu, k) = \sum_{n \geq 0} \log \left( 1 + e^{\mu - E_n} \right).\tag{7.2.186}$$

For the moment being we will restrict ourselves to the perturbative regime, but at all orders in the WKB expansion (as we will see, there are important non-perturbative corrections in  $\hbar$ ). The perturbative energies will be denoted by  $E_n^p$ , and they are determined by the WKB quantization condition (7.2.165), which defines in fact an implicit function  $E^p(n)$  for arbitrary values of  $n$ . In order to perform the sum over discrete energy levels, we will use the Euler–Maclaurin formula, which reads

$$\sum_{n \geq 0} f(n) = \int_0^\infty f(n) dn + \frac{1}{2} (f(0) + f(\infty)) + \sum_{r \geq 1} \frac{B_{2r}}{(2r)!} \left( f^{(2r-1)}(\infty) - f^{(2r-1)}(0) \right).\tag{7.2.187}$$

Notice that, in general, this formula gives an asymptotic expansion for the sum. In our case, the function  $f(n)$  is given by

$$f(n) = \log \left( 1 + e^{\mu - E^{\text{P}}(n)} \right). \quad (7.2.188)$$

Since  $E^{\text{P}}(n) \rightarrow \infty$  as  $n \rightarrow \infty$ , we have  $f(\infty) = 0$ ,  $f^{(2r-1)}(\infty) = 0$  for all  $r \geq 1$ . The first terms of (7.2.187) give,

$$\int_{E_0^{\text{P}}}^{\infty} \frac{dn(E)}{dE} \log \left( 1 + e^{\mu - E} \right) dE + \frac{1}{2} f(0) = \frac{1}{2\pi\hbar} \int_{E_0^{\text{P}}}^{\infty} \frac{\text{vol}_{\text{p}}(E)}{1 + e^{E-\mu}} dE. \quad (7.2.189)$$

In deriving this equation, we first changed variables from  $n$  to  $E$ , by using

$$n(E) = \frac{\text{vol}_{\text{p}}(E)}{2\pi\hbar} - \frac{1}{2}, \quad (7.2.190)$$

we integrated by parts, and we took into account that

$$\frac{\text{vol}_{\text{p}}(E_0^{\text{P}})}{2\pi\hbar} = \frac{1}{2}, \quad (7.2.191)$$

as well as the asymptotic behavior

$$\text{vol}(E) \approx E^2, \quad E \rightarrow \infty. \quad (7.2.192)$$

We conclude that the WKB expansion of the grand potential is related to the perturbative quantum volume as

$$\mathcal{J}^{\text{WKB}}(\mu, k) = \frac{1}{2\pi\hbar} \int_{E_0^{\text{P}}}^{\infty} \frac{\text{vol}_{\text{p}}(E) dE}{e^{E-\mu} + 1} - \sum_{r \geq 1} \frac{B_{2r}}{(2r)!} f^{(2r-1)}(0). \quad (7.2.193)$$

A clarification is needed concerning the above derivation. The first term in the l.h.s. of (7.2.189) looks identical to the standard formula (7.2.99) which one finds in textbooks. However, (7.2.189) has an infinite number of corrections due to the Euler–Maclaurin formula. How is this compatible with (7.2.99)? The answer is that in (7.2.99) the function  $\rho(E)$  is not really smooth, but rather a sum of delta functions. In contrast, in (7.2.189) we use a smooth function, the perturbative quantum volume. The price to pay for using a smooth function, in a situation in which one has a discrete set eigenvalues, is precisely including the corrections to the Euler–Maclaurin formula (see for example [61] for a discussion on the discrete versus the smooth density of eigenvalues).

We can now plug the expansion (7.2.185) in the r.h.s. of (7.2.193) and integrate term by term. The resulting integrals can be done by using the Mellin transform, see [54] for the details, and one finds in the end

$$\begin{aligned} \mathcal{J}^{\text{WKB}}(\mu, k) &= \frac{2\mu^3}{3k\pi^2} + \left( \frac{1}{3k} + \frac{k}{24} \right) \mu + \hat{A}(\hbar) \\ &+ \sum_{\ell \geq 1} \left( -\frac{\hat{a}_{\ell}(\hbar)}{\pi^2 k} \mu^2 + \frac{\hat{b}_{\ell}(\hbar)}{2\pi^2 k} \mu + \frac{\hat{c}_{\ell}(\hbar)}{2\pi^2 k} \right) e^{-2\ell\mu} - \sum_{\ell \geq 0} \frac{\hat{d}_{\ell}(\hbar)}{2\pi^2 k} e^{-(2\ell+1)\mu}. \end{aligned} \quad (7.2.194)$$

Here,  $A(\hbar)$ ,  $\widehat{c}_\ell(\hbar)$  and  $\widehat{d}_\ell(\hbar)$  have complicated expressions which can be found in [54]. They involve  $E^p(n)$  and its derivatives, evaluated at  $n = 0$ , as well as the coefficients  $\widehat{a}_\ell(\hbar)$ ,  $\widehat{b}_\ell(\hbar)$ . By comparing (7.2.194) with (7.2.124), we find that the coefficients appearing in (7.2.128) are related to the coefficients of the quantum periods introduced before by

$$a_\ell(k) = -\frac{\widehat{a}_\ell(\hbar)}{\pi^2 k}, \quad b_\ell(k) = \frac{\widehat{b}_\ell(\hbar)}{2\pi^2 k}. \quad (7.2.195)$$

Note that, in the classical limit  $k \rightarrow 0$ , we recover the first two equations in (7.2.148). This relationship between the WKB expansion of the grand potential and the quantum periods of local  $\mathbb{P}^1 \times \mathbb{P}^1$  was first conjectured in [50], and it can be checked against explicit calculations of both sets of coefficients. The above argument explains why this relation holds: it is due to the fact that the WKB solution of the spectral problem of the ABJM Fermi gas can be mapped to the problem of computing these quantum periods. This method also provides explicit, but complicated expressions for the remaining coefficients,  $\widehat{A}(\hbar)$ ,  $\widehat{c}_\ell(\hbar)$  and  $\widehat{d}_\ell(\hbar)$ . In order to have a result consistent with the perturbative results for  $\mathcal{J}_n(\mu)$ , one should have  $\widehat{d}_\ell(\hbar) = 0$  for all  $\ell \geq 0$ . This can be verified in the very first orders of a power series expansion around  $k = 0$  [54].

We can also give a more conceptual understanding of the quantum corrections to the grand potential. We have shown that the coefficients  $a_\ell(k)$  and  $b_\ell(k)$  in  $\mathcal{J}^{\text{WKB}}(\mu, k)$  can be obtained by promoting the periods  $\varpi_{1,2}(z)$  (which encode their classical limit) to quantum periods. However,  $\mathcal{J}_0(\mu)$  is itself a classical period, as we showed in (7.2.146) and (7.2.151). Therefore, the full function  $\mathcal{J}^{\text{WKB}}(\mu, k)$  should be obtained by promoting this period to its quantum counterpart. For example, one can write down a quantum version of (7.2.151) by using the NS free energy defined in (7.2.180). To do this, we focus on the period appearing in (7.2.151), which in a general CY with  $n$  moduli is given by

$$\varpi_3 = 2F_0 - \sum_{i=1}^n t_i \frac{\partial F_0}{\partial t_i}. \quad (7.2.196)$$

This can be written in a more natural way by introducing the so-called homogeneous coordinates

$$t_i = \frac{X_i}{X_0}, \quad i = 1, \dots, n. \quad (7.2.197)$$

Here,  $X_0$  plays the rôle of the inverse string coupling constant, which in our case is  $1/\hbar$ . Let us define the homogeneous prepotential  $\mathcal{F}_0(X_0, X_i)$  as

$$\mathcal{F}_0(X_0, X_i) = X_0^2 F_0 \left( \frac{X_i}{X_0} \right). \quad (7.2.198)$$

Then, one has (see for example [62])

$$\frac{1}{X_0} \frac{\partial \mathcal{F}_0}{\partial X_0} = 2F_0 - \sum_{i=1}^n t_i \frac{\partial F_0}{\partial t_i}. \quad (7.2.199)$$

It follows from (7.2.151) that

$$\frac{1}{k} \mathcal{J}_0(\mu) = -\frac{1}{\pi} \frac{\partial \mathcal{F}_0}{\partial X_0}. \quad (7.2.200)$$

The natural generalization of the homogeneous prepotential, including all the corrections in  $\hbar$ , involves the NS free energy introduced in (7.2.180).

$$\mathcal{F}(X_0, X_i) = X_0 F^{\text{NS}} \left( \frac{X_i}{X_0}; \frac{1}{X_0} \right) = X_0^2 F_0 \left( \frac{X_i}{X_0} \right) + \dots \quad (7.2.201)$$

Therefore, the generalization of (7.2.200) to an all-orders formula is

$$\mathcal{J}^{\text{WKB}}(\mu, k) = -\frac{1}{\pi} \frac{\partial}{\partial X_0} \left[ X_0 F^{\text{NS}} \left( \frac{X}{X_0}; \frac{1}{X_0} \right) \right], \quad (7.2.202)$$

where, after performing the derivative, we set  $X_0 = 1/\hbar$ ,  $X = X_0 t$  and  $\hbar = 2\pi k$ . This formula for the all-orders modified grand potential in the WKB approximation,  $\mathcal{J}^{\text{WKB}}(\mu, k)$ , was first proposed in [50] based on detailed calculations of the WKB expansion. We can now interpret it as the quantum version of the period  $\varpi_3$  of special geometry.

The above considerations suggest that we write the WKB grand potential in the way first proposed in [63]. In quantum mirror symmetry, one introduces a quantum mirror map depending on  $\hbar$ . In terms of the variables of the grand potential, this amounts to introducing an “effective” chemical potential  $\mu_{\text{eff}}$  through the equation,

$$\mu_{\text{eff}} = \mu + \frac{1}{C(k)} \sum_{\ell \geq 1} a_\ell(k) e^{-2\ell\mu}. \quad (7.2.203)$$

In the equation (7.2.151), we re-expressed the semiclassical grand potential in terms of the “flat” coordinate  $t$ . In the all-orders WKB expansion, one should re-express it in terms of the effective chemical potential introduced before. After doing this, one obtains

$$\mathcal{J}^{\text{WKB}}(\mu, k) = J^{(\text{p})}(\mu, k) + J^{\text{M}^2}(\mu, k) = J^{(\text{p})}(\mu_{\text{eff}}, k) + \mu_{\text{eff}} \tilde{J}_b(\mu_{\text{eff}}, k) + \tilde{J}_c(\mu_{\text{eff}}, k). \quad (7.2.204)$$

The two functions  $\tilde{J}_b(\mu_{\text{eff}}, k)$  and  $\tilde{J}_c(\mu_{\text{eff}}, k)$ , when expanded at large  $\mu_{\text{eff}}$ , define the coefficients  $\tilde{b}_\ell(k)$ ,  $\tilde{c}_\ell(k)$ :

$$\tilde{J}_b(\mu_{\text{eff}}, k) = \sum_{\ell=1}^{\infty} \tilde{b}_\ell(k) e^{-2\ell\mu_{\text{eff}}}, \quad \tilde{J}_c(\mu_{\text{eff}}, k) = \sum_{\ell=1}^{\infty} \tilde{c}_\ell(k) e^{-2\ell\mu_{\text{eff}}}. \quad (7.2.205)$$

In terms of generating functionals for the three sets of coefficients appearing in  $J^{\text{M}^2}(\mu, k)$ ,

$$J_a(\mu, k) = \sum_{\ell=1}^{\infty} a_\ell(k) e^{-2\ell\mu}, \quad J_b(\mu, k) = \sum_{\ell=1}^{\infty} b_\ell(k) e^{-2\ell\mu}, \quad J_c(\mu, k) = \sum_{\ell=1}^{\infty} c_\ell(k) e^{-2\ell\mu}, \quad (7.2.206)$$

we have

$$\begin{aligned} \tilde{J}_b(\mu_{\text{eff}}, k) &= J_b(\mu, k) - \frac{J_a(\mu, k)^2}{C(k)}, \\ \tilde{J}_c(\mu_{\text{eff}}, k) &= J_c(k, \mu) - \frac{J_a(\mu, k) J_b(\mu, k)}{C(k)} - \frac{B(k)}{C(k)} J_a(\mu, k) + \frac{2J_a(\mu, k)^3}{3C(k)^2}. \end{aligned} \quad (7.2.207)$$

As a final step, we can put together the decomposition (7.2.204) with the formula (7.2.202). It was conjectured in [58] (and confirmed in many examples [64]) that the NS free energy of a general, toric CY manifold, defined in terms of quantum periods, agrees with the NS limit of the refined topological string energy, which can be computed with many other methods (the refined topological vertex [65], the refined holomorphic anomaly equations of [66], and the geometric perspective on refined BPS invariants in [67]). In particular, the NS free energy can be expressed in terms of *refined BPS invariants* [65, 67], which are integer invariants encoding enumerative information on the local CY manifold. One has the following formula for the instanton part of the NS free energy, i.e. for the part involving exponentially small corrections at large  $t_I$ :

$$F_{\text{NS}}^{\text{inst}}(t, \hbar) = \sum_{j_L, j_R} \sum_{w, \mathbf{d}} N_{j_L, j_R}^{\mathbf{d}} \frac{\sin \frac{\hbar w}{2} (2j_L + 1) \sin \frac{\hbar w}{2} (2j_R + 1)}{2w^2 \sin^3 \frac{\hbar w}{2}} e^{-w \mathbf{d} \cdot \mathbf{t}}. \quad (7.2.208)$$

In this formula,  $\mathbf{t}$  is the vector of Kähler parameters  $t_I$ , and  $\mathbf{d}$  is the vector of degrees. The refined BPS invariants, denoted by  $N_{j_L, j_R}^{\mathbf{d}}$ , depend on the degrees and on two half-integer spins,  $j_L$  and  $j_R$ . Note that, when expressed in terms of the  $z_I$ s, the  $t_I$  depend as well on  $\hbar$ , as explained in (7.2.180). It follows from (7.2.208) and (7.2.204) that the coefficient  $\tilde{b}_\ell(k)$  has the following expression [50]

$$\tilde{b}_\ell(k) = -\frac{\ell}{2\pi} \sum_{j_L, j_R} \sum_{\ell=dw} \sum_{d_1+d_2=d} N_{j_L, j_R}^{d_1, d_2} q^{\frac{w}{2}(d_1-d_2)} \frac{\sin \frac{\pi k w}{2} (2j_L + 1) \sin \frac{\pi k w}{2} (2j_R + 1)}{w^2 \sin^3 \frac{\pi k w}{2}}. \quad (7.2.209)$$

In this equation,  $N_{j_L, j_R}^{d_1, d_2}$  are the refined BPS invariants of the CY manifold local  $\mathbb{P}^1 \times \mathbb{P}^1$ . The extra factor of  $q$  appearing in this formula is due to the choice of  $z_{1,2}$  in (7.2.173). In addition, one finds the following formula for the coefficient  $\tilde{c}_\ell(k)$ ,

$$\tilde{c}_\ell(k) = -k^2 \frac{\partial}{\partial k} \left( \frac{\tilde{b}_\ell(k)}{2\ell k} \right). \quad (7.2.210)$$

This relationship was first conjectured in [63], and verified in many examples. As explained above, this relation follows from the fact that the full WKB grand potential can be regarded as the quantum version of the period given in (7.2.151). This interpretation of the WKB grand potential also explains the fact that the quantum corrections  $\mathcal{J}_n^{\text{WKB}}(\mu)$  can be obtained by acting with differential operators on  $\mathcal{J}_0^{\text{WKB}}(\mu)$  [52, 68], since this is a known property of quantum periods [69].

## The TBA approach

The ABJM Fermi gas can be studied with a different tool, which in principle is exact: a TBA-like system which determines the grand potential through a set of coupled non-linear integral equations. This TBA-like system was first considered in [70], in the context of  $\mathcal{N} = 2$  models in two dimensions, but its relevance to the study of integral kernels was first noticed by Al. Zamolodchikov in [71]. His results were further elaborated and justified in the work

of Tracy and Widom [55]. Although TBA-like systems have been very useful in the study of integrable models in QFT, in the case of the ABJM Fermi gas this approach has had a limited use, as we will eventually explain. Nevertheless, it makes it possible to compute in an efficient way the partition functions  $Z(N, k)$  for finite  $N$  [72, 73], and is well suited for a WKB analysis [74].

In [71], the following type of integral kernel is considered:

$$\rho(\theta, \theta') = \frac{1}{2\pi} \frac{\exp(-u(\theta) - u(\theta'))}{2 \cosh \frac{\theta - \theta'}{2}}. \quad (7.2.211)$$

Under suitable assumptions on the potential function  $u(\theta)$ , this kernel is of trace class. The spectral problem

$$\int_{-\infty}^{\infty} \rho(\theta, \theta') f(\theta') = \lambda f(\theta) \quad (7.2.212)$$

leads to a discrete set of eigenvalues  $\lambda_n$ ,  $n = 0, 1, \dots$ . The Fredholm determinant of the operator  $\rho$  is defined by

$$\Xi(\kappa) = \prod_{n \geq 0} (1 + \kappa \lambda_n) \quad (7.2.213)$$

and it is an entire function of  $\kappa$ . We will regard  $\Xi$  as a grand canonical partition function, as in (7.2.97). The grand potential is then given by

$$\mathcal{J}(z) = \log \Xi(z), \quad (7.2.214)$$

and it has the expansion (7.2.91). Let us now introduce the iterated integral

$$R_\ell(\theta) = e^{-2u(\theta)} \int_{-\infty}^{\infty} \frac{e^{-2u(\theta_1) - \dots - 2u(\theta_\ell)}}{\cosh \frac{\theta - \theta_1}{2} \cosh \frac{\theta_1 - \theta_2}{2} \dots \cosh \frac{\theta_\ell - \theta}{2}} d\theta_1 \dots d\theta_\ell, \quad \ell \geq 1, \quad (7.2.215)$$

and

$$R_0(\theta) = e^{-2u(\theta)}. \quad (7.2.216)$$

Notice that

$$\int_{-\infty}^{\infty} d\theta R_\ell(\theta) = (4\pi)^{\ell+1} Z_{\ell+1}, \quad (7.2.217)$$

where  $Z_\ell$  is the coefficient appearing in (7.2.91). The generating series

$$R(\theta|\kappa) = \sum_{\ell \geq 0} \left(-\frac{\kappa}{4\pi}\right)^\ell R_\ell(\theta) \quad (7.2.218)$$

satisfies

$$\int_{-\infty}^{\infty} \frac{d\theta}{4\pi} R(\theta|\kappa) = \sum_{\ell \geq 0} (-\kappa)^\ell Z_{\ell+1} = \frac{\partial \mathcal{J}}{\partial \kappa}. \quad (7.2.219)$$

It was conjectured in [71] and proved in [55] that the function  $R(\theta|\kappa)$  can be obtained by using TBA-like equations. We first define

$$\begin{aligned} R_+(\theta|\kappa) &= \frac{1}{2} (R(\theta|\kappa) + R(\theta - \kappa)), \\ R_-(\theta|\kappa) &= \frac{1}{2} (R(\theta|\kappa) - R(\theta - \kappa)). \end{aligned} \quad (7.2.220)$$

Let us now consider the TBA-like system

$$\begin{aligned} 2u(\theta) &= \epsilon(\theta) + \int_{-\infty}^{\infty} \frac{d\theta'}{2\pi} \frac{\log(1 + \eta^2(\theta'))}{\cosh(\theta - \theta')}, \\ \eta(\theta) &= -\kappa \int_{-\infty}^{\infty} \frac{d\theta'}{2\pi} \frac{e^{-\epsilon(\theta')}}{\cosh(\theta - \theta')}. \end{aligned} \tag{7.2.221}$$

Then, one has that

$$\begin{aligned} R_+(\theta|\kappa) &= e^{-\epsilon(\theta)}, \\ R_-(\theta|\kappa) &= R_+(\theta|\kappa) \int_{-\infty}^{\infty} \frac{d\theta'}{\pi} \frac{\arctan \eta(\theta')}{\cosh^2(\theta - \theta')}. \end{aligned} \tag{7.2.222}$$

This conjecture has been proved in [55] for general  $u(\theta)$ . In general, the system (7.2.221) has to be solved numerically, although an exact solution exists for  $u(\theta) = e^\theta$  in terms of Airy functions [75].

It is obvious that the ABJM Fermi gas is a particular case of the above formalism, up to a simple change of variables. Indeed, if we set

$$x = k\theta, \tag{7.2.223}$$

and compare with (7.2.215), we find

$$\rho^{\ell+1}(x, x) = \langle x | \rho^{\ell+1} | x \rangle = \frac{1}{(4\pi)^{\ell+1} k} R_\ell(x), \tag{7.2.224}$$

where we have denoted

$$R_\ell(x) \equiv R_\ell\left(\theta = \frac{x}{k}\right). \tag{7.2.225}$$

The function  $R_\ell(\theta)$  is calculated with the TBA system (7.2.221) and the potential

$$u(\theta) = \frac{1}{2} \log\left(2 \cosh \frac{k\theta}{2}\right), \tag{7.2.226}$$

which depends explicitly on  $k$ . The grand potential is given by

$$\frac{\partial \mathcal{J}}{\partial \kappa} = \frac{1}{4\pi k} \int_{-\infty}^{\infty} dx R(x|\kappa). \tag{7.2.227}$$

Notice that the function  $R(x|\kappa)$  can be written as

$$R(x|\kappa) = \frac{4\pi k}{\kappa} \left\langle x \left| \frac{1}{e^{\mathbf{H}-\mu} + 1} \right| x \right\rangle, \tag{7.2.228}$$

where the Hamiltonian  $\mathbf{H}$  is defined by an equation similar to (7.2.88),

$$\langle \theta | e^{-\mathbf{H}} | \theta' \rangle = \rho(\theta, \theta'), \tag{7.2.229}$$

and  $\kappa$  is the fugacity (7.2.92). The expression (7.2.228), is up to an overall factor, the diagonal value of the number of particles in an ideal Fermi gas with Hamiltonian  $\mathbf{H}$ .

There is an important property of the TBA system of [71] which is worth discussing in some detail: the functions  $\epsilon(\theta)$ ,  $\eta(\theta)$  make it possible to calculate *both*  $R(x|\kappa)$  and  $R(x|-\kappa)$ . The last quantity is given by

$$R(x|-\kappa) = \frac{4\pi k}{\kappa} \left\langle x \left| \frac{1}{e^{\mathbf{H}-\mu} - 1} \right| x \right\rangle, \quad (7.2.230)$$

and it corresponds to the same one-particle Hamiltonian (7.2.229) but with *Bose–Einstein* statistics. If we now take into account the expression (7.2.213), we deduce that for Bose–Einstein statistics there is a physical singularity at

$$\kappa = \lambda_0^{-1} > 0 \quad (7.2.231)$$

where  $\lambda_0$  is the largest eigenvalue of the operator  $\rho(x_1, x_2)$ . This singularity corresponds of course to the onset of Bose–Einstein condensation in the gas, and as a consequence the functions  $R_{\pm}(x|\kappa)$  will have singularities in the  $x$ -plane for  $\kappa \geq \lambda_0^{-1}$ . But this is precisely the regime in which we are interested in the case of the ABJM Fermi gas, since large  $N$  corresponds to  $\mu \gg 1$ . Of course, the singularity at large and positive  $\kappa$  *cancels*, once one adds up  $R_+$  and  $R_-$ , but it appears in intermediate steps and leads to technical problems. For example, it is very difficult to use the TBA approach presented in this section to obtain numerical information on the grand potential at large fugacity  $\kappa$ , since the standard iteration of the integral equation does not converge when  $\kappa$  is moderately large.

One can then try the opposite regime and perform an expansion around  $\kappa = 0$  of all the quantities involved in the TBA system [72, 73]. By doing this, one can compute the coefficients  $Z_\ell$  recursively, up to very large  $\ell$ , and obtain in this way exact results for the partition functions  $Z(N, k)$ , for  $N = 1, 2, \dots$ . In practice,  $k$  is taken to be a small integer, and no surprisingly the cases  $k = 1, 2$  are the easiest ones: for these values of  $k$ , ABJM theory has extended  $\mathcal{N} = 8$  supersymmetry [76–79], and one would expect additional simplifications. For example, for  $k = 2$ , one finds, for the very first values of  $N$ ,

$$Z(1, 2) = \frac{1}{8}, \quad Z(2, 2) = \frac{1}{32\pi^2}, \quad Z(3, 2) = \frac{10 - \pi^2}{512\pi^2}. \quad (7.2.232)$$

Another use of the TBA approach was proposed in [74], where it was noticed that, for  $k \rightarrow 0$ , the kernel of the Fermi gas becomes a delta function, and the TBA system becomes algebraic. Exploiting this observation, one can perform a systematic expansion of all the quantities around  $k = 0$ , and calculate the functions  $\mathcal{J}_n(\mu)$  directly to high order in  $n$ .

## A conjecture for the exact grand potential

So far we have obtained two different pieces of information on the matrix model of ABJM theory: on the one hand, the full 't Hooft expansion of the partition function, and on the other hand, the full WKB expansion of the grand potential. Can we put these two pieces

of information together? It turns out that the 't Hooft expansion can be incorporated in the grand potential, but this requires a subtle handling of the relationship between the canonical and the grand-canonical ensemble. In the standard thermodynamic relationship, the canonical partition function is given by the integral (7.2.130). As we have seen in the derivation of (7.2.131), it is very convenient to extend the integration contour to infinity, along the Airy contour  $\mathcal{C}$  shown in Fig. 7.3. However, this cannot be done without changing the value of the integral: As already noted in [43], if we extend the contour in (7.2.130) to infinity, we will add to the partition function non-perturbative terms of order

$$\sim e^{-\mu/k}, \quad (7.2.233)$$

If we want to understand the structure of the non-perturbative effects in the ABJM partition function, we have to handle this issue with care. A clever way of proceeding was found by Hatsuda, Moriyama and Okuyama in [80]. Following their work, we will introduce an auxiliary object, which we will call the *modified* grand potential, denoted it by  $J(\mu, k)$ . The modified grand potential is *defined* by the equality

$$Z(N, k) = \int_{\mathcal{C}} \frac{d\mu}{2\pi i} e^{J(\mu, k) - N\mu}, \quad (7.2.234)$$

where  $\mathcal{C}$  is the Airy contour shown in Fig. 7.3. As it was noticed in [80], if we know  $J(\mu, k)$ , we can recover the conventional grand potential  $\mathcal{J}(\mu, k)$  by the relation

$$e^{\mathcal{J}(\mu, k)} = \sum_{n \in \mathbb{Z}} e^{J(\mu + 2\pi i n, k)}. \quad (7.2.235)$$

Indeed, if we plug this in (7.2.130), we can use the sum over  $n$  to extend the integration region from  $[-\pi i, \pi i]$  to the full imaginary axis. If we then deform the contour to  $\mathcal{C}$ , we obtain (7.2.234). Note that the difference between  $J(\mu, k)$  and  $\mathcal{J}(\mu, k)$  involves non-perturbative terms of the form (7.2.233), and it is not seen in a perturbative calculation around  $k = 0$ . Therefore the WKB calculation of the full grand potential still gives the perturbative expansion of the modified grand potential, and we have

$$J(\mu, k) = \mathcal{J}^{\text{WKB}}(\mu, k) + \mathcal{O}(e^{-\mu/k}). \quad (7.2.236)$$

Let us now try to understand how to incorporate the information of the 't Hooft expansion in the grand potential. It is much better to use the modified grand potential, due to the fact that the relationship (7.2.234) involves an integration going to infinity. Let us denote the 't Hooft contribution to the modified grand potential by  $J^{\text{'t Hooft}}(\mu, k)$ . If we plug this function in the r.h.s. of (7.2.234), we should obtain the 't Hooft expansion of the standard free energy. This requires doing the integral by a saddle point calculation at  $k \rightarrow \infty$ , and it also requires the following scaling for the modified grand potential (see [81] for a related discussion),

$$J^{\text{'t Hooft}}(\mu, k) = \sum_{g=0}^{\infty} k^{2-2g} J_g\left(\frac{\mu}{k}\right). \quad (7.2.237)$$

This can be regarded as the 't Hooft expansion of the modified grand potential, and contains exactly the same information than the 't Hooft expansion of the canonical partition function. As usual in the saddle-point expansion of a Laplace transform, the leading terms, which are the genus zero pieces  $J_0$  and  $-F_0/(4\pi^2)$ , are related by a Legendre transform: we first solve for the 't Hooft parameter  $\lambda$ , in terms of  $\mu/k$ , through the equation

$$\frac{\mu}{k} = \frac{1}{4\pi^2} \frac{dF_0}{d\lambda}, \quad (7.2.238)$$

and then we have,

$$J_0\left(\frac{\mu}{k}\right) = -\frac{1}{4\pi^2} \left( F_0(\lambda) - \lambda \frac{dF_0}{d\lambda} \right). \quad (7.2.239)$$

Similarly, the genus one grand potential  $J_1$  is related to the genus one free energy  $F_1$  through the equation

$$J_1\left(\frac{\mu}{k}\right) = F_1(\lambda) + \frac{1}{2} \log \left( 2\pi k^2 \partial_\mu^2 J_0\left(\frac{\mu}{k}\right) \right), \quad (7.2.240)$$

which takes into account the one-loop correction to the saddle-point. Since the integration contour in (7.2.234) goes to infinity, doing the saddle-point expansion with Gaussian integrals is fully justified and no error terms of the form (7.2.233) are introduced in this way. This is clearly one of the advantages of using the modified grand potential, instead of the standard grand potential.

We should recall now that the genus  $g$  free energies  $F_g$  are given by the topological string free energies of local  $\mathbb{P}^1 \times \mathbb{P}^1$ , in the so-called orbifold frame. It turns out that the Laplace transform which takes us to the grand potential has an interpretation in topological string theory: as shown in [43] by using the general theory of [82], it is the transformation that takes us from the orbifold frame to the so-called large radius frame. Therefore, we can interpret  $J^{\text{'t Hooft}}(\mu, k)$  as the total free energy of the topological string on local  $\mathbb{P}^1 \times \mathbb{P}^1$  at large radius. This free energy has a polynomial piece, which reproduces precisely the perturbative piece (7.2.125), and then an infinite series of corrections of the form,

$$e^{-4\mu/k}. \quad (7.2.241)$$

These corrections, after the inverse Legendre transform, give back the worldsheet instanton corrections that we found in the 't Hooft expansion of the free energy. Notice however that, from the point of view of the Fermi gas approach, these are non-perturbative in  $\hbar$ , and correspond to instanton-type corrections in the spectral problem (7.2.95) [43, 54].

The large radius free energy of local  $\mathbb{P}^1 \times \mathbb{P}^1$  is a well studied quantity (in fact, it has been much more studied than the orbifold free energies). In particular, there is a surprising result of Gopakumar and Vafa [83], valid for any CY manifold, which makes it possible to resum the genus expansion in (7.2.237). In our case, this means that we can resum the genus expansion, order by order in  $\exp(-4\mu/k)$  [80]. The result can be written as,

$$J^{\text{'t Hooft}}(\mu, k) = \frac{C(k)}{3} \mu^3 + B(k) \mu + A(k) + J^{\text{WS}}(\mu, k), \quad (7.2.242)$$

where

$$J^{\text{WS}}(\mu, k) = \sum_{m \geq 1} (-1)^m d_m(k) e^{-\frac{4m\mu}{k}}, \quad (7.2.243)$$

and the coefficients  $d_m(k)$  are given by

$$d_m(k) = \sum_{g \geq 0} \sum_{m=wd} n_g^d \left( 2 \sin \frac{2\pi w}{k} \right)^{2g-2}. \quad (7.2.244)$$

In this equation, we sum over the positive integers  $w, d$  satisfying the constraint  $wd = m$ . The quantities  $n_g^d$  are integer numbers called Gopakumar–Vafa (GV) invariants. One should note that, for any given  $d$ , the  $n_d^g$  are different from zero only for a finite number of  $g$ , therefore (7.2.244) is well-defined as a formal power series in  $\exp(-4\mu/k)$ . The GV invariants can be computed by various techniques, and in the case of non-compact CY manifolds, there are algorithms to determine them for all possible values of  $d$  and  $g$  (like for example the theory of the topological vertex [84].) It is important to note that it is only when we use the modified grand potential that we obtain the results (7.2.242), (7.2.243) for the 't Hooft expansion. If we use the standard grand potential, there are additional contributions coming from the “images” of the modified grand potential in the sum (7.2.235). Note also that the resummation of (7.2.237) leads to a resummation of the genus  $g$  free energies  $F_g(\lambda)$ , i.e. the terms of the same order in the expansion parameters

$$\exp\left(-2\pi\sqrt{\hat{\lambda}}\right), \quad \frac{1}{\sqrt{\lambda}} \quad (7.2.245)$$

can be resummed to all genera.

We have now the most important pieces of the total grand potential,  $J^{\text{WS}}(\mu, k)$ , given in (7.2.243), and  $J^{\text{M}^2}(\mu, k)$ , given in (7.2.204). From the point of view of the 't Hooft expansion,  $J^{\text{WS}}(\mu, k)$  is a resummation of a perturbative series, while  $J^{\text{M}^2}(\mu, k)$  contains non-perturbative information. Conversely, from the point of view of the WKB expansion,  $J^{\text{M}^2}(\mu, k)$  is the resummation of a perturbative expansion, while  $J^{\text{WS}}(\mu, k)$  is non-perturbative. One would be tempted to conclude that the total, modified grand potential is given by

$$J^{(\text{p})}(\mu, k) + J^{\text{M}^2}(\mu, k) + J^{\text{WS}}(\mu, k). \quad (7.2.246)$$

However, it can be seen that this is not the case: there is a “mixing” of the “membrane” and “worldsheet” contributions, which was found experimentally in [63]. It was noted in that reference that agreement with the calculations done at low orders in the expansion was achieved by promoting

$$\mu \rightarrow \mu_{\text{eff}} \quad (7.2.247)$$

in  $J^{\text{WS}}(\mu, k)$ . From the point of view of the 't Hooft expansion, the corrections added in this form are again non-perturbative. It was noted in [54] that the prescription (7.2.247) is natural from the point of view of the spectral problem: in calculating instanton corrections to the WKB result for the volume (7.2.185), the weight of an instanton should involve the quantum A-period, which means that one should use  $\mu_{\text{eff}}$  rather than  $\mu$ .

Then, the final proposal for the modified grand potential, putting together all the pieces from [4, 5, 43, 50, 63, 74, 80], is the following:

$$J(\mu, k) = J^{(p)}(\mu, k) + J^{\text{WS}}(\mu_{\text{eff}}, k) + J^{\text{M}^2}(\mu, k). \quad (7.2.248)$$

When the function (7.2.248) is expanded at large  $\mu$ , one finds exponentially small corrections in  $\mu$  of the form,

$$\exp \left\{ - \left( \frac{4n}{k} + 2\ell \right) \mu \right\}. \quad (7.2.249)$$

In [74] these mixed terms were interpreted as bound states of worldsheet instantons and membrane instantons in the M-theory dual.

One of the most important properties of the proposal (7.2.248) is the following. It is easy to see, by looking at the explicit expressions (7.2.243) and (7.2.244), that  $J^{\text{WS}}(\mu, k)$  is singular for any rational  $k$ . This is a puzzling result, since it implies that the genus resummation of the free energies  $F_g$  is also singular for infinitely many values of  $k$ , including the integer values for which the theory is in principle well-defined non-perturbatively. It is however clear that this divergence is an artifact of the genus expansion, since the original matrix integral (7.2.21), as well as its Fermi gas form (7.2.87), are perfectly well-defined for any real value of  $k$ . What is going on?

It was first proposed in [80] that the divergences in the resummation of the genus expansion of  $J^{\text{WS}}(\mu, k)$  should be cured by other terms in the modified grand potential, in such a way that the total result is finite. It turns out that  $J^{\text{M}^2}(\mu, k)$  is also singular, and its singularities cancel those of  $J^{\text{WS}}(\mu, k)$  in such a way that the total  $J(\mu, k)$  is finite. This remarkable property of  $J(\mu, k)$  was called in [74] the HMO cancellation mechanism. Originally, this mechanism was used as a way to understand the structure of  $J^{\text{M}^2}(\mu, k)$  at finite  $k$ . In [50] it was shown that this cancellation is a consequence of the structure of the the modified grand potential, and it can be proved by using the underlying geometric structure of  $J^{\text{M}^2}(\mu, k)$  and  $J^{\text{WS}}(\mu, k)$ . Let us review this proof here.

The poles in  $J^{\text{M}^2}(\mu, k)$  are due to simple poles appearing in the coefficients  $\tilde{b}_\ell(k)$  in (7.2.209), and to double poles in the coefficients  $\tilde{c}_\ell(k)$  given in (7.2.210). On the other hand, the coefficients  $d_m(k)$  are singular due to the double poles with  $g = 0$  in the formula (7.2.244). The Gopakumar–Vafa invariants appearing in (7.2.244) can be also expressed in terms of the refined BPS invariants appearing in (7.2.209), and one has

$$d_m(k) = \sum_{j_L, j_R} \sum_{m=dn} \sum_{d_1+d_2=d} N_{j_L, j_R}^{d_1, d_2} \frac{2j_R + 1}{\left(2 \sin \frac{2\pi n}{k}\right)^2} \frac{\sin \left(\frac{4\pi n}{k}(2j_L + 1)\right)}{n \sin \frac{4\pi n}{k}}. \quad (7.2.250)$$

Using these results, it is easy to see that the poles cancel. The coefficient (7.2.250) has double poles when  $k \in 2n/\mathbb{N}$ . The coefficient (7.2.209) has a simple pole when  $k \in 2\mathbb{N}/w$ , and the coefficient  $\tilde{c}_\ell(k)$  has a double pole at the same values of  $k$ . These poles contribute to terms of the same order in  $e^{-\mu_{\text{eff}}}$  when  $k$  is of the form

$$k = \frac{2n}{w} = \frac{2m}{\ell}. \quad (7.2.251)$$

We have then to examine the pole structure of (7.2.204) at these values of  $k$ . Since both (7.2.250) and (7.2.209) involve a sum over refined BPS invariants, we can look at the contribution to the pole structure of each of these invariants. In the worldsheet instanton contribution, the singular part around  $k = 2n/w$  associated to the refined BPS invariant  $N_{j_L, j_R}^{d_1, d_2}$  is

$$\frac{(-1)^m}{\pi^2} \left[ \frac{n}{w^4 \left(k - \frac{2n}{w}\right)^2} + \frac{1}{k - \frac{2n}{w}} \left( \frac{1}{w^3} + \frac{m}{nw^2} \mu_{\text{eff}} \right) \right] (1 + 2j_L)(1 + 2j_R) N_{j_L, j_R}^{d_1, d_2} e^{-\frac{2mw}{n} \mu_{\text{eff}}}. \quad (7.2.252)$$

The singular part in  $\mu_{\text{eff}} \tilde{J}_b(\mu_{\text{eff}}, k)$  associated to the same invariant is given by

$$- \frac{e^{\pi i k w (d_1 - d_2)/2}}{\pi^2} \frac{\ell}{w^3 \left(k - \frac{2n}{w}\right)} (-1)^{n(2j_L + 2j_R - 1)} (1 + 2j_L)(1 + 2j_R) N_{j_L, j_R}^{d_1, d_2} \mu_{\text{eff}} e^{-2\ell \mu_{\text{eff}}}. \quad (7.2.253)$$

Using (7.2.210), we find that the corresponding singular part in  $\tilde{J}_c(\mu_{\text{eff}}, k)$  is given by

$$- \frac{e^{\pi i k w (d_1 - d_2)/2}}{\pi^2} \left[ \frac{n}{w^4 \left(k - \frac{2n}{w}\right)^2} + \frac{1}{w^3 \left(k - \frac{2n}{w}\right)} \right] (-1)^{n(2j_L + 2j_R - 1)} (1 + 2j_L)(1 + 2j_R) N_{j_L, j_R}^{d_1, d_2} e^{-2\ell \mu_{\text{eff}}} \quad (7.2.254)$$

By using (7.2.251), one notices that

$$e^{\pi i k w (d_1 - d_2)/2} = (-1)^m \quad (7.2.255)$$

and it is easy to see that all poles in (7.2.252) cancel against the poles in (7.2.253) and (7.2.254), for any value of  $\mu_{\text{eff}}$ , provided that

$$(-1)^{n(2j_L + 2j_R - 1)} = 1. \quad (7.2.256)$$

However, this is the case, since for local  $\mathbb{P}^1 \times \mathbb{P}^1$ , the only non-vanishing BPS indices  $N_{j_L, j_R}^{d_1, d_2}$  have

$$2j_L + 2j_R - 1 \equiv 0 \pmod{2}. \quad (7.2.257)$$

This can be justified with a geometric argument explained in [50].

The HMO cancellation mechanism is conceptually important for a deeper understanding of the non-perturbative structure of M-theory. In the M-theory expansion, we have to resum the worldsheet instanton contributions to the free energy at fixed  $k$  and large  $N$ , which is precisely what the Gopakumar–Vafa representation (7.2.243) does for us. However, after this resummation, the resulting expression is singular and displays an infinite number of poles. We obtain a finite result only when the contribution of membrane instantons has been added. This shows very clearly that a theory based solely on fundamental strings is fundamentally incomplete, and that additional extended objects are needed in M-theory. Of course, this has been clear since the advent of M-theory, but the above calculation shows that the contribution of membranes is not just a correction to the contribution of fundamental strings; it is crucial

to remove the poles and to make the amplitude well-defined. Conversely, a theory based only on membrane instantons will be also incomplete and will require fundamental strings in order to make sense.

The result (7.2.248) is the current proposal for the grand potential of the ABJM matrix model. It is a remarkable exact result. From the point of view of gauge theory, it encodes the full  $1/N$  expansion, at all genera, as well as non-perturbative corrections at large  $N$  (due presumably to some form of large  $N$  instanton). From the point of view of M-theory, it incorporates both membrane instantons and worldsheet instantons. This can be seen very clearly by writing

$$e^{J(\mu,k)} = e^{J^{(p)}(\mu,k)} \sum_{l,n} a_{l,n}(k) \mu^n e^{-l\mu}, \quad (7.2.258)$$

where  $l$  is of the form  $2p + 4q/k$ , and  $p, q$  are non-negative integers. Plugging this in (7.2.234), we find

$$Z(N, k) = \frac{e^{A(k)}}{(C(k))^{1/3}} \sum_{l,n} a_{l,n} \left( -\frac{\partial}{\partial N} \right)^n \text{Ai} \left( \frac{N + l - B(k)}{(C(k))^{1/3}} \right), \quad (7.2.259)$$

where  $\text{Ai}(z)$  is again the Airy function. The first term in this expansion is of course (7.2.61), while the remaining terms are non-perturbative corrections, exponentially suppressed as  $N$  becomes large. The conjectural formula (7.2.259) provides an *exact* and *convergent* series for the partition function  $Z(N, k)$ , in the M-theory expansion. It is remarkable that, in the framework of M-theory, the asymptotic and divergent expansions in the string coupling constant are promoted to convergent series.

It is instructive to compare these results for  $Z(N, k)$  with the well-known number theory results for the number of partitions  $p(N)$  of an integer  $N$ . For  $N$  large, the leading asymptotic behavior of  $p(N)$  is given by Hardy–Ramanujan formula,

$$p(N) \sim \exp \left( \pi \sqrt{\frac{2N}{3}} \right), \quad N \gg 1. \quad (7.2.260)$$

This leading asymptotics was dramatically improved by Rademacher into a convergent series expression. In our case, the analogue of the Hardy–Ramanujan formula is the SUGRA result (7.2.17), while (7.2.259) is the analogue of the Rademacher expansion.

As noted in [85], one interesting aspect of the formulae (7.2.234) and (7.2.259) is the following. In principle, the partition function  $Z(N, k)$  is only defined for integer  $N$ , since it is given by a matrix integral for  $N$  variables. However, using (7.2.234) or (7.2.259), one can define  $Z(N, k)$  for arbitrary complex  $N$ , and the resulting function seems to be entire. It is not clear how natural is this promotion of a function defined on integer values of  $N$ , to a function on the complex plane. This is similar to the promotion of the factorial to the Gamma function. It is known that this problem has many solutions (for example, Hadamard’s Gamma function also does the job). There is in fact another way to promote  $Z(N, k)$  to a function defined on a larger domain, which is by performing a Borel resummation of the  $1/N$  expansion. This type of promotion, in the context of matrix models, was first worked out in [86] for a unitary matrix model, and it has been recently explored in much detail

in [87], in the case of the quartic matrix model. In general, in order to recover the exact non-perturbative answer, even for integer  $N$ , one has to add (Borel-resummed) instanton contributions to the resummed  $1/N$  series. In the case of ABJM theory, the results of [38] indicate that such contributions must be present, although their precise form is not known yet. It would be very interesting to see if these two different ways of extrapolating  $Z(N, k)$  to non-integer  $N$  (namely, the exact formulae (7.2.234), (7.2.259), and the Borel resummation of the  $1/N$  expansion and its instanton corrections) lead to the same function. If so, this would be a strong indication that this is the natural function picked up by the underlying mathematical structures of the problem.

The result (7.2.248) is relatively complicated, since it involves an enormous amount of information, including the all-genus Gopakumar–Vafa invariants of local  $\mathbb{P}^1 \times \mathbb{P}^1$ , and the quantum periods of this manifold to all orders. However, there are certain cases in which (7.2.248) can be simplified, as first noted in [85]. This happens when  $k = 1$  or  $k = 2$  and ABJM theory has enhanced  $\mathcal{N} = 8$  supersymmetry. In the underlying topological string theory, only the genus zero and genus one free energies contribute, so we have a sort of “non-renormalization theorem.” In these cases, as shown in [85], one can write down closed formulae for the modified grand potential and for the grand canonical partition function. The simplest case is  $k = 2$ , and one finds

$$\Xi(\mu, 2) = \exp \left\{ \frac{\mu}{4} + F_1 + F_1^{\text{NS}} - \frac{1}{\pi^2} \left( F_0(\lambda) - \lambda \partial_\lambda F_0(\lambda) + \frac{\lambda^2}{2} \partial_\lambda^2 F_0(\lambda) \right) \right\} \vartheta_3(\bar{\xi}, \bar{\tau}). \quad (7.2.261)$$

In this equation,  $F_0(\lambda)$  is the planar free energy of ABJM theory defined by (7.2.36), and  $\lambda$  is given, as a function of  $\kappa$  (or  $\mu$ ) by (7.2.35). In (7.2.261),  $\vartheta_3(\bar{\xi}, \bar{\tau})$  is a Jacobi theta function with arguments

$$\begin{aligned} \bar{\xi} &= \frac{i}{4\pi^3} \left( \lambda \partial_\lambda^2 F_0(\lambda) - \partial_\lambda F_0(\lambda) \right), \\ \bar{\tau} &= \frac{i}{8\pi^3} \partial_\lambda^2 F_0(\lambda). \end{aligned} \quad (7.2.262)$$

Note that  $\bar{\tau}$  is related to the parameter  $\tau$  in (7.2.46) by the linear relation  $\bar{\tau} = (\tau - 1)/2$ .  $F_1$  is the genus one free energy introduced in (7.2.47). Finally,  $F_1^{\text{NS}}$  is the next-to-leading term in the  $\hbar$  expansion (7.2.181), and it has the explicit expression

$$F_1^{\text{NS}}(t) = -\frac{1}{6}\mu - \frac{1}{24} \log(1 + 16 e^{-2\mu}). \quad (7.2.263)$$

It can be checked [85] that the small  $\kappa$  expansion of (7.2.261) reproduces the values of the partition function (7.2.232) and all the values computed in [80]. In addition, from the study of the zeroes of the theta function in (7.2.261), one finds an exact quantization condition determining the energy levels in (7.2.95) for  $k = 2$ . This quantization condition takes the form of a Bohr–Sommerfeld formula,

$$\text{vol}(E, 2) = 8\pi^2 \left( n + \frac{1}{2} \right), \quad n = 0, 1, 2, \dots, \quad (7.2.264)$$

where the exact quantum volume function has the form

$$\begin{aligned} \text{vol}(E, 2) = & 8\pi \frac{K'(4i e^{-E})}{K(4i e^{-E})} \left( E + 2e^{-2E} {}_4F_3 \left( 1, 1, \frac{3}{2}, \frac{3}{2}; 2, 2, 2; -16 e^{-2E} \right) \right) \\ & - \frac{4}{\pi} G_{3,3}^{3,2} \left( -16 e^{-2E} \left| \begin{array}{c} \frac{1}{2}, \frac{1}{2}, 1 \\ 0, 0, 0 \end{array} \right. \right). \end{aligned} \tag{7.2.265}$$

In this equation,  $K(k)$  is the elliptic integral of the first kind, and  $G_{3,3}^{3,2}$  is a Meijer function. The spectrum obtained from the above quantization condition has been checked in detail against numerical calculations starting from (7.2.95) [54, 85]. Similar considerations can be made for  $k = 1$ , see [85] for detailed formulae. The exact quantum volume (7.2.265) was first proposed in [54], based on some simplifying assumptions which turn out to hold only in the maximally supersymmetric cases of ABJM theory. In the general case, the quantization condition proposed in [54] receives corrections, as pointed out in [88] based on a numerical analysis of the spectrum. These corrections can be derived analytically within the framework proposed in [89], which provides an exact quantization condition for arbitrary  $k$ . As in the maximally supersymmetric cases, the quantization condition in [89] is based on finding the zeroes of the spectral determinant, which is in turn determined by (7.2.235) and (7.2.248).

## 7.3 Generalizations

In the previous section, we have focused on ABJM theory, for simplicity. However, many of the above results can be extended, in one way or another, to other Chern–Simons–matter theories. Not surprisingly, and as a general rule, the more supersymmetry the theory has, the more explicit are the results that one can obtain. In this section we will make a brief overview of these generalizations, which should mostly serve as a guide to the growing literature on the subject.

### 7.3.1 The 't Hooft expansion of Chern–Simons–matter theories

Localization can be applied to a large range of Chern–Simons–matter theories with  $\mathcal{N} \geq 2$  supersymmetry [3, 90, 91]. The partition function of such theories is reduced in this way to a matrix integral, which can then be studied in the 't Hooft expansion with conventional techniques. However, for most of these theories, obtaining even the planar free energy has been a very difficult task, due to the sheer complexity of the resulting matrix integrals. Some results exist for ABJM theory with fundamental matter [41], for the generalization of ABJM theory in which the levels are different [92] (also known as Gaiotto–Tomasiello theory [93]), and for a single Chern–Simons theory coupled to adjoint hypermultiplets [94]. In addition, T. Suyama has provided some general results for a class of  $\mathcal{N} \geq 3$  Chern–Simons–matter theories [95, 96].

One case where we have much information is ABJ theory [8]. As shown in [4, 5], the 't Hooft expansion of this theory is still completely controlled by topological string theory on

local  $\mathbb{P}^1 \times \mathbb{P}^1$ . Since this is now a two-parameter problem, computing the genus  $g$  free energies is technically more complicated, but one can determine the analogue of the function  $J^{\text{WS}}(\mu, k)$  for ABJ theory in terms of Gopakumar–Vafa invariants in a completely straightforward way.

Perhaps the simplest theory, beyond ABJ(M) theory, where the planar limit of the free energy is known, is the superconformal field theory in three dimensions consisting of supersymmetric  $U(N)$  Yang–Mills theory, coupled to a single adjoint hypermultiplet and to  $N_f$  fundamental hypermultiplets. When  $N_f = 1$ , this theory is related by mirror symmetry to  $\mathcal{N} = 8$  super Yang–Mills theory, therefore to ABJM theory with  $k = 1$  [44]. From the point of view of M-theory, this gauge theory is supposed to describe  $N$  M2 branes probing the space [79, 97]

$$\mathbb{C}^2 \times (\mathbb{C}^2/\mathbb{Z}_{N_f}), \quad (7.3.1)$$

where  $\mathbb{Z}_{N_f}$  acts on  $\mathbb{C}^2$  as

$$e^{2\pi i/N_f} \cdot (a, b) = (e^{2\pi i/N_f} a, e^{-2\pi i/N_f} b). \quad (7.3.2)$$

The corresponding quotient is an  $A_{N_f-1}$  singularity, which can be resolved to give a multi-Taub-NUT space, as expected from the engineering of the theory in terms of D6 branes. The large  $N$  dual description of this theory is in terms of M-theory on  $\text{AdS}_4 \times \mathbb{S}^7/\mathbb{Z}_{N_f}$ , where the action of  $\mathbb{Z}_{N_f}$  is the one inherited by the action on  $\mathbb{C}^2 \times \mathbb{C}^2$ .

The rules for localization of Chern–Simons–matter theories obtained in [3, 90, 91] (see Chapter 6) imply that the partition function on the three-sphere  $\mathbb{S}^3$  is given by the matrix integral

$$Z(N, N_f) = \frac{1}{N!} \int \prod_{i=1}^N \frac{dx_i}{4\pi} \frac{1}{(2 \cosh \frac{x_i}{2})^{N_f}} \prod_{i < j} \left( \tanh \left( \frac{x_i - x_j}{2} \right) \right)^2. \quad (7.3.3)$$

The tanh interaction between the eigenvalues includes both a sinh factor due to the Yang–Mills vector multiplet, and a  $1/\cosh$  due to the hypermultiplet in the adjoint representation. Notice that, when  $N_f = 1$ , this model leads to the same matrix integral than ABJM theory with  $k = 1$ , in the representation (7.2.87). The natural 't Hooft parameter for this model is

$$\lambda = \frac{N}{N_f}, \quad (7.3.4)$$

where  $N_f$  is the number of flavours (in fact, we should rather call this parameter the Veneziano parameter, since it takes into account the scaling of the number of flavors with the rank of the gauge group). The matrix model (7.3.3) was called the  $N_f$  matrix model in [98], where it was analyzed in detail. It turns out that this model can be mapped to an  $O(2)$  matrix model [99] and studied with the techniques of [100, 101] (similarly to what was done in [94]). The planar solution turns out to be very simple. Let us write the large  $N$  expansion of the free energy as

$$F(N, N_f) = \sum_{g \geq 0} N_f^{2-2g} F_g(\lambda). \quad (7.3.5)$$

As in the ABJM matrix model, in order to write the planar solution, we need to introduce an auxiliary parameter  $k$ , related to the 't Hooft parameter (7.3.4) by

$$\lambda = -\frac{1}{8} + \frac{(1+k)^2}{8\pi^2} K'(k)^2. \quad (7.3.6)$$

Then, the planar free energy is given, as a function of  $k$ , by

$$\frac{d^2 F_0}{d\lambda^2} = -2\pi \frac{K(k)}{K'(k)}. \quad (7.3.7)$$

The integration constants can be fixed by a perturbative calculation in the matrix model (7.3.3). The planar free energy can be expanded at strong 't Hooft coupling, and it has the behavior

$$F_0(\lambda) = -\frac{\pi\sqrt{2}}{3} \hat{\lambda}^{3/2} + \frac{1}{8} \left( \log(2) - \frac{\zeta(3)}{\pi^2} \right) + F_0^{\text{WS}}(\lambda), \quad (7.3.8)$$

where

$$F_0^{\text{WS}}(\lambda) = -\frac{e^{-2\pi\sqrt{2\hat{\lambda}}}}{4\pi^2} \left( 1 + 2\pi\sqrt{2\hat{\lambda}} \right) - \frac{e^{-4\pi\sqrt{2\hat{\lambda}}}}{32\pi^2} \left( 7 + 28\pi\sqrt{2\hat{\lambda}} + 64\pi^2\hat{\lambda} \right) + \dots \quad (7.3.9)$$

and the variable  $\hat{\lambda}$  is defined by

$$\hat{\lambda} = \lambda + \frac{1}{8}. \quad (7.3.10)$$

This shift is reminiscent of the shift in  $-1/24$  which appears in the planar solution of ABJM theory, in (7.2.40). The constant appearing in the second term of (7.3.8) was determined numerically in [98], and then conjectured analytically in [31].

The expansion of the planar free energy found above is conceptually very similar to what was found in ABJM theory: the leading term displays the expected  $N^{3/2}$  behavior, and the coefficient is in agreement with the expectations from the M-theory dual (this was already checked in the strict large  $N$  limit in [102]). The subleading, exponentially small corrections appearing in (7.3.9) have the expected form of worldsheet instanton corrections. However, they do *not* have the structure that one would expect from a topological string theory on a CY manifold. This is easier to see by considering the grand potential of the theory in the 't Hooft expansion, i.e. the analogue of the quantity (7.2.239) in ABJM theory. Its structure turns out to be more complicated than the one in ABJM theory, and in particular it does not have the simpler structure appearing in topological string theory.

Unfortunately, it is hard to calculate  $1/N$  corrections to the above result. The genus one free energy was determined in [98] by using matrix model techniques, but beyond that nothing is known. In [31], some all-genus results for the worldsheet instantons were guessed up to third order in the instanton expansion, but much work remains to be done if we want to understand the  $N_f$  matrix model at the level of precision that we have achieved for the ABJM matrix model.

### 7.3.2 The Fermi gas approach to Chern–Simons–matter theories

As we have seen, the Fermi gas approach to ABJM theory is very powerful, and it can be applied to other Chern–Simons–matter theories. However, it also has some limitations. It relies on algebraic identities (such as (7.2.84)) which make it possible to rewrite the relevant matrix models, in the form of the canonical partition function of an ideal Fermi gas. This can be done for a large class of  $\mathcal{N} \geq 3$  theories, but in the case of  $\mathcal{N} = 2$  theories the resulting gas is interacting [103] and much harder to analyze.

Let us mention some generalizations of the Fermi gas approach. The  $\mathcal{N} = 3$  models where it can be applied more successfully are the necklace quiver gauge theories constructed in [104, 105]. These theories are given by a Chern–Simons quiver with gauge groups and levels,

$$U(N)_{k_1} \times U(N)_{k_2} \times \cdots \times U(N)_{k_r}. \quad (7.3.11)$$

Each node is labelled with the letter  $a = 1, \dots, r$ . There are bifundamental chiral superfields  $A_{aa+1}, B_{aa-1}$  connecting adjacent nodes, and in addition there can be  $N_{f_a}$  matter superfields  $(Q_a, \tilde{Q}_a)$  in each node, in the fundamental representation. We will write

$$k_a = n_a k, \quad (7.3.12)$$

and we will assume that

$$\sum_{a=1}^r n_a = 0. \quad (7.3.13)$$

The matrix model computing the  $\mathbb{S}^3$  partition function of such a necklace quiver gauge theory is given by

$$Z(N, n_a, N_{f_a}, k) = \frac{1}{(N!)^r} \int \prod_{a,i} \frac{d\lambda_{a,i}}{2\pi} \frac{\exp\left[\frac{in_a k}{4\pi} \lambda_{a,i}^2\right]}{\left(2 \cosh \frac{\lambda_{a,i}}{2}\right)^{N_{f_a}}} \prod_{a=1}^r \frac{\prod_{i<j} \left[2 \sinh\left(\frac{\lambda_{a,i} - \lambda_{a,j}}{2}\right)\right]^2}{\prod_{i,j} 2 \cosh\left(\frac{\lambda_{a,i} - \lambda_{a+1,j}}{2}\right)}. \quad (7.3.14)$$

To construct the corresponding Fermi gas, we define a kernel corresponding to a pair of connected nodes  $(a, b)$  by,

$$K_{ab}(x', x) = \frac{1}{2\pi k} \frac{\exp\left\{i \frac{n_b x^2}{4\pi k}\right\}}{2 \cosh\left(\frac{x' - x}{2k}\right)} \left[2 \cosh \frac{x}{2k}\right]^{-N_{f_b}}, \quad (7.3.15)$$

where we set  $x = \lambda/k$ . If we use the Cauchy identity (7.2.84), it is easy to see that we can write the grand canonical partition function for this theory in the form (7.2.97), where now [106]

$$\rho = \hat{K}_{r1} \hat{K}_{12} \cdots \hat{K}_{r-1,r} \quad (7.3.16)$$

is the product of the kernels (7.3.15) around the quiver. Therefore, we still have a Fermi gas, albeit the Hamiltonian is quite complicated, and we can apply the same techniques that were used for ABJM theory in the previous section. For example, it is possible to analyze the gas

in the thermodynamic limit [43]. One can show that, at large  $\mu$ , the grand potential of the theory is still of the form

$$\mathcal{J}(\mu, k) \approx \frac{C\mu^3}{3} + B\mu, \quad \mu \gg 1. \quad (7.3.17)$$

The coefficient  $C$  for a general quiver is also determined, as in ABJM theory, by the volume of the Fermi surface at large energy. This limit is a polygon and one finds,

$$\pi^2 C = \text{vol} \left\{ (x, y) : \sum_{j=1}^r \left| y - \left( \sum_{i=1}^{j-1} k_i \right) x \right| + \left( \sum_{j=1}^r N_{f_j} \right) |x| < 1 \right\}, \quad (7.3.18)$$

which can be computed in closed form [107]. The  $B$  coefficient can be obtained in a case by case basis, although no general formula is known for all  $\mathcal{N} = 3$  quivers (a general formula is however known for a class of special quivers which preserve  $\mathcal{N} = 4$  supersymmetry, see [68].)

The result (7.3.17) has two important consequences. First, the free energy at large  $N$  has the behavior

$$F(N) \approx -\frac{2}{3} C^{-1/2} N^{3/2}. \quad (7.3.19)$$

It can be seen [43], by using the results of [107], that this agrees with the prediction from the M-theory dual (this was also verified in [7, 107] with the techniques that we reviewed in section 7.2.3). Second, by using the same techniques as in ABJM theory, we conclude that the M-theory expansion of the partition function is also given, at leading order, by an Airy function:

$$Z(N) \approx C^{-1/3}(k) \text{Ai} \left[ C^{-1/3} (N - B) \right]. \quad (7.3.20)$$

A Fermi gas formulation also exists for  $\mathcal{N} = 3$  theories with other gauge groups [42, 108, 109], and one finds again the Airy behavior (7.3.20). This behavior is arguably one of the most important results obtained from the Fermi gas approach, and it has been conjectured in [43] that it is *universal*. More precisely, it was conjectured that, in any Chern–Simons–matter theory which displays the  $N^{3/2}$  behavior for the strict large  $N$  limit of its partition function, the leading term of the M-theory expansion will have the form (7.3.20). The subleading, universal logarithmic prediction for  $Z(N)$  implied by (7.3.20) has been also tested by [35], and it has been argued that the full Airy function can be obtained from a localization computation in AdS supergravity [110].

Of course, one of the most important advantages of the Fermi gas approach is that it makes it possible to calculate non-perturbative corrections to the 't Hooft expansion. However, for theories other than ABJM theory, this has been in general difficult. An exception is again ABJ theory. The Fermi gas formulation of this theory requires some work, but it has been achieved in the papers [111, 112] (a different formulation has been proposed in [113].) A conjectural formula for the modified grand potential of this theory has been finally proposed in [113, 114]. It has exactly the same properties that we found in ABJM theory: poles appear in the resummation of the genus expansion, and they are cancelled by non-perturbative contributions (presumably coming from membrane instantons), just as in the HMO mechanism of [80].

For other theories which admit a Fermi gas description, the computation of non-perturbative contributions at the level of detail that was done in ABJ(M) theory remains largely an open problem. However, all the existing results indicate that generically the 't Hooft expansion of these theories is radically *insufficient*: not only there are non-perturbative corrections to it, but in addition the resummation of the genus expansion has poles which have to be cured by these non-perturbative effects through a generalization of the HMO mechanism. This pattern has been observed in the  $N_f$  matrix model [31, 98], in some  $\mathcal{N} = 4$  quiver theories [68, 115–117], and in theories involving orientifolds, where new types of instanton effects appear [118–120].

The Fermi gas approach has had other applications. For example, in [121] it is shown that the mirror symmetry relating some Chern–Simons–matter theories can be understood as a canonical transformation of the one-dimensional fermions.

### 7.3.3 Topological strings

One of the key ingredients for the exact determination of the grand potential of ABJM theory has been the relationship to topological string theory. Conversely, one might hope that the structures emerging in the context of Chern–Simons–matter theories are relevant for a better understanding of topological strings. In particular, as already pointed out in [122], the results of [43] suggest a Fermi gas approach to topological string theory on toric CY manifolds which has been pursued in [50, 54, 123]. When the CY  $X$  is given by the canonical bundle

$$\mathcal{O}(K_S) \rightarrow S \tag{7.3.21}$$

over a del Pezzo surface  $S$ , a detailed proposal has been presented in [124] and further developed in [125–133] (see [134] for a review.) The proposal of [124] gives a correspondence between topological string theory on  $X$ , and the spectral properties of a quantum-mechanical operator  $\rho_S$  obtained by quantizing the mirror curve to  $X$ . This correspondence shares many ingredients of the gauge theory/string theory correspondence, since the topological string emerges in the large  $N$  limit of the quantum-mechanical system. In addition, it provides a non-perturbative definition of (closed) topological string theory on  $X$ . The resulting picture is also very similar to the theory of the ABJM partition function reviewed in this article, since the operator  $\rho_S$  plays the rôle of the canonical density matrix of the Fermi gas (7.2.86). For example, in the case of local  $\mathbb{P}^2$ , the mirror curve is given by

$$W(x, y) = e^x + e^y + e^{-x-y} = u, \tag{7.3.22}$$

where  $u$  is the complex deformation moduli and we have chosen appropriate coordinates. The relevant operator is

$$\rho_{\mathbb{P}^2} = (e^x + e^y + e^{-x-y})^{-1}, \tag{7.3.23}$$

where  $x, y$  are canonically conjugate Heisenberg operators, as in (7.2.101). In contrast to what happens in ABJM theory, the kernel of the operator  $\rho_S$  is not elementary. However, in some cases (like the operator for local  $\mathbb{P}^2$ ), it can be calculated explicitly in terms of Faddeev’s quantum dilogarithm [125].

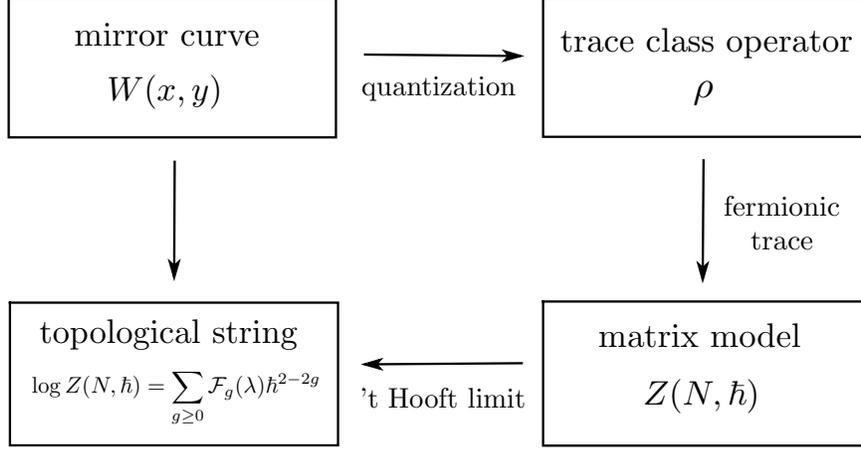

Figure 7.5: Given a toric CY threefold, the quantization of its mirror curve leads to a trace class operator  $\rho$ . The standard topological string free energy is obtained as the 't Hooft limit of its fermionic traces  $Z(N, \hbar)$ .

We can now consider a Fermi gas of  $N$  particles whose canonical density matrix is given by  $\rho_S$ . Its canonical partition function  $Z(N, \hbar)$  has a matrix model representation similar to (7.2.85),

$$Z_S(N, \hbar) = \frac{1}{N!} \sum_{\sigma \in S_N} (-1)^{\epsilon(\sigma)} \int d^N x \prod_i \rho_S(x_i, x_{\sigma(i)}) = \frac{1}{N!} \int d^N x \det(\rho_S(x_i, x_j)), \quad (7.3.24)$$

where

$$\rho_S(x, x') = \langle x | \rho_S | x' \rangle \quad (7.3.25)$$

is the kernel of  $\rho_S$ . The  $1/N$  expansion of this matrix model, in the 't Hooft limit

$$N \rightarrow \infty, \quad \frac{N}{\hbar} = \lambda = \text{fixed}, \quad (7.3.26)$$

gives the all-genus topological string free energies,

$$\log Z(N, \hbar) = \sum_{g \geq 0} \mathcal{F}_g^S(\lambda) \hbar^{2-2g}, \quad (7.3.27)$$

where  $\lambda$  parametrizes the moduli space of the local del Pezzo. Therefore, the genus expansion of the topological string on  $X$  is realized as the asymptotic expansion of a well-defined quantity,  $Z_S(N, \hbar)$ . In addition, there are non-perturbative corrections to this expansion which are captured by the refined topological string free energy of the CY manifold, in the NS limit. The structure of the correspondence is summarized in Fig. 7.5.

This picture can be made very concrete in many examples. For example, for local  $\mathbb{P}^2$ , the matrix model takes the form [126],

$$Z_{\mathbb{P}^2}(N, \hbar) = \frac{1}{N!} \int_{\mathbb{R}^N} \frac{d^N u}{(2\pi)^N} \prod_{i=1}^N e^{-V_{\mathbb{P}^2}(u_i, \hbar)} \frac{\prod_{i < j} 4 \sinh\left(\frac{u_i - u_j}{2}\right)^2}{\prod_{i, j} 2 \cosh\left(\frac{u_i - u_j}{2} + \frac{i\pi}{6}\right)}, \quad (7.3.28)$$

where

$$V_{\mathbb{P}^2}(u, \hbar) = \frac{\hbar u}{2\pi} + \log \left[ \frac{\Phi_b \left( \frac{bu}{2\pi} + \frac{ib}{3} \right)}{\Phi_b \left( \frac{bu}{2\pi} - \frac{ib}{3} \right)} \right]. \quad (7.3.29)$$

In this equation,  $\Phi_b(x)$  is Faddeev's quantum dilogarithm (where we use the conventions of [53, 125]) and  $b$  is related to  $\hbar$  by

$$b^2 = \frac{3\hbar}{2\pi}. \quad (7.3.30)$$

The function  $V_{\mathbb{P}^2}(u, \hbar)$  appearing here is relatively complicated. However, it is completely determined by the operator (7.3.23). It has an asymptotic expansion at large  $\hbar$  which can be used to compute the asymptotic expansion of the matrix integral (7.3.28) in the 't Hooft regime (7.2.14), as explained in [126]. In fact, this matrix integral is structurally very similar to the generalizations of the  $O(2)$  matrix model considered in [135], and might be exactly solvable in the planar limit.

Another geometry where the integral kernel of the operator can be written in detail is local  $\mathbb{P}^1 \times \mathbb{P}^1$  [136]. The expression (7.3.24) leads to an  $O(2)$  matrix model, which can be regarded as a generalization of the ABJ matrix model of [111, 112]. In [137], the field theory limit of topological string theory on local  $\mathbb{P}^1 \times \mathbb{P}^1$  was implemented directly in the integral kernel found in [136]. In this limit, one recovers the integral kernel studied in [71] in connection with the Painlevé III equation. On the topological string side, the field theory limit leads to Seiberg–Witten theory [138]. Based on this, [137] provided a Fermi gas picture of Seiberg–Witten theory, as well as a proof of the conjecture of [124] for local  $\mathbb{P}^1 \times \mathbb{P}^1$ , in the field theory limit.

## 7.4 Conclusions and outlook

In this paper we have reviewed in detail the large  $N$  solution to the matrix model calculating the partition function of ABJM theory and other Chern–Simons–matter theories, beyond the strict large  $N$  limit. This analysis has given us unexpected and valuable information. First of all, it has made possible to derive the famous  $N^{3/2}$  scaling of M2 branes theories from the gauge theory point of view. This result turns out to be just the tip of the iceberg: a detailed treatment of the ABJM matrix integral has led to many new exact results on the  $1/N$  expansion of this interacting QFT. We have now, thanks to the localized matrix model, the full 't Hooft expansion of the free energy, at all orders in the genus expansion. We also have a conjectural exact result for the partition function which includes all non-perturbative corrections at large  $N$ .

This non-perturbative result shows that the 't Hooft expansion is fundamentally incomplete, and instanton effects are crucial to obtain a meaningful answer. From the point of view of the dual superstring theory, it shows in a quantitative and precise way that the genus expansion is incomplete, and one needs membrane instantons coming from M-theory in order to have a consistent answer. The results obtained for ABJM theory can be generalized, to some extent, to other Chern–Simons–matter theories. Although much more work is needed for generic

Chern–Simons–matter theories, the same pattern emerges, and non-perturbative effects are crucial in order to understand the theory.

The work done so far in this field leads to many interesting and important open problems for the future. Let us mention four of them.

First of all, although many of the ingredients of the conjectural solution for the exact grand potential have been justified analytically, we are still lacking a complete derivation of the result (even by physics standards.) Mathematically, this is a challenging problem, since it amounts to computing the exact spectral determinant of the operator (7.2.86). At some point, these loopholes should be addressed seriously. Such a derivation might also be useful in the second problem: in order to have a complete picture of the non-perturbative aspects of more general Chern–Simons–matter theories, one should develop techniques to analyze the resulting matrix models. Even in the case of  $\mathcal{N} = 3$  theories, where a Fermi gas formulation is possible, we lack the necessary technology to analyze their spectrum in full detail. Concrete progress in this field will depend much on our ability to develop this technology. It is likely that the same tools which will fill out the loopholes in the derivation of (7.2.248) will make it also possible to obtain analytic results in other theories.

It is clear, in view of the AdS/CFT correspondence, that all these analytic results on Chern–Simons–matter theories give us precise predictions on the structure of the M-theory partition function on  $\text{AdS}_4$  backgrounds. In particular, they provide many interesting predictions for the counting on worldsheet instantons and membrane instantons (in a sense, these results can be regarded as a generalization of mirror symmetry, in which the matrix model computes instanton corrections due to extended configurations in superstring theory and M-theory.) It would be very interesting to see to which extent these predictions can be tested with the current technology.

Finally, as we pointed out briefly in section 7.3.3, the mathematical structures appearing in the study of the partition function of Chern–Simons–matter theories provide a non-perturbative formulation of the topological string on toric CY manifolds. It has been speculated in [124] that this formulation might be understood in terms of a theory of M2 branes. For example, the partition function (7.3.24) has, at large  $N$  and fixed  $\hbar$ , the  $N^{3/2}$  behavior typical of these theories. Such a formulation would clearly shed new light on topological string theory and lead to new perspectives in enumerative geometry. In relation to this, it has been recently noted that the matrix model for topological strings on local  $\mathbb{P}^2$ , when  $\hbar = 2\pi$ , computes as well the partition function of ABJM theory with  $k = 1$  and on an ellipsoid with deformation parameter  $b^2 = 3$  [139], making in this way an explicit connection between M2 brane theories and the non-perturbative formulation of topological strings proposed in [124, 126], for this particular case. It would be interesting to understand whether this is a happy coincidence or there is a more systematic relation between theories of M2 branes and topological strings.

## Acknowledgements

I would like to thank Sayantani Bhattacharyya, Flavio Calvo, Santiago Codesido, Ricardo Couso, Nadav Drukker, Alba Grassi, Yasuyuki Hatsuda, Johan Källén, Rinat Kashaev, Albrecht Klemm, Sanefumi Moriyama, Kazumi Okuyama, Pavel Putrov, Marc Schiereck, Ashoke Sen, Masoud Soroush and Szabolcs Zakany for the collaborations which led to most of the results presented in this review paper. Special thanks to Alba Grassi, Yasuyuki Hatsuda and Kazuo Hosomichi for a careful reading of the manuscript. I would also like to thank the coordinators of this project, Vasily Pestun and Maxim Zabzine, for inviting me to write a contribution. This work is supported in part by the Fonds National Suisse, subsidies 200021-156995 and 200020-141329, and by the NCCR 51NF40-141869 “The Mathematics of Physics” (SwissMAP).

## References

- [1] V. Pestun and M. Zabzine, eds., *Localization techniques in quantum field theory*, vol. xx. Journal of Physics A, 2016. [1608.02952](https://arxiv.org/src/1608.02952/anc/LocQFT.pdf). <https://arxiv.org/src/1608.02952/anc/LocQFT.pdf>, <http://pestun.ihes.fr/pages/LocalizationReview/LocQFT.pdf>.
- [2] V. Pestun, “Localization of gauge theory on a four-sphere and supersymmetric Wilson loops,” *Commun. Math. Phys.* **313**, 71 (2012) [arXiv:0712.2824 [hep-th]].
- [3] A. Kapustin, B. Willett and I. Yaakov, “Exact Results for Wilson Loops in Superconformal Chern-Simons Theories with Matter,” *JHEP* **1003**, 089 (2010) [arXiv:0909.4559 [hep-th]].
- [4] M. Mariño and P. Putrov, “Exact Results in ABJM Theory from Topological Strings,” *JHEP* **1006**, 011 (2010) [arXiv:0912.3074 [hep-th]].
- [5] N. Drukker, M. Mariño, P. Putrov, “From weak to strong coupling in ABJM theory,” *Commun. Math. Phys.* **306**, 511-563 (2011). [arXiv:1007.3837 [hep-th]].
- [6] O. Aharony, O. Bergman, D. L. Jafferis and J. Maldacena, “N=6 superconformal Chern-Simons-matter theories, M2-branes and their gravity duals,” *JHEP* **0810**, 091 (2008) [arXiv:0806.1218 [hep-th]].
- [7] C. P. Herzog, I. R. Klebanov, S. S. Pufu and T. Tesileanu, “Multi-Matrix Models and Tri-Sasaki Einstein Spaces,” *Phys. Rev. D* **83**, 046001 (2011) [arXiv:1011.5487 [hep-th]].
- [8] O. Aharony, O. Bergman and D. L. Jafferis, “Fractional M2-branes,” *JHEP* **0811**, 043 (2008) [arXiv:0807.4924].
- [9] Y. Hatsuda, S. Moriyama and K. Okuyama, “Exact instanton expansion of the ABJM partition function,” *PTEP* **2015**, no. 11, 11B104 (2015) [arXiv:1507.01678 [hep-th]].
- [10] J. Bagger, N. Lambert, S. Mukhi and C. Papageorgakis, “Multiple Membranes in M-theory,” *Phys. Rept.* **527**, 1 (2013) [arXiv:1203.3546 [hep-th]].
- [11] M. Mariño, “Lectures on localization and matrix models in supersymmetric Chern-Simons-matter theories,” *J. Phys. A* **44**, 463001 (2011) [arXiv:1104.0783 [hep-th]].
- [12] G. 't Hooft, “A Planar Diagram Theory for Strong Interactions,” *Nucl. Phys. B* **72**, 461 (1974).
- [13] J. M. Maldacena, “The Large N limit of superconformal field theories and supergravity,” *Adv. Theor. Math. Phys.* **2**, 231-252 (1998). [hep-th/9711200].
- [14] M. J. Duff, B. E. W. Nilsson, C. N. Pope, “Kaluza-Klein Supergravity,” *Phys. Rept.* **130**, 1-142 (1986).

- [15] O. Bergman and S. Hirano, “Anomalous radius shift in  $\text{AdS}_4/\text{CFT}_3$ ,” *JHEP* **0907**, 016 (2009) [arXiv:0902.1743].
- [16] O. Aharony, A. Hashimoto, S. Hirano, P. Ouyang, “D-brane Charges in Gravitational Duals of 2+1 Dimensional Gauge Theories and Duality Cascades,” *JHEP* **1001**, 072 (2010). [arXiv:0906.2390 [hep-th]].
- [17] B. E. W. Nilsson and C. N. Pope, “Hopf Fibration of Eleven-dimensional Supergravity,” *Class. Quant. Grav.* **1**, 499 (1984).
- [18] T. Azeyanagi, M. Fujita and M. Hanada, “From the planar limit to M-theory,” *Phys. Rev. Lett.* **110**, no. 12, 121601 (2013) [arXiv:1210.3601 [hep-th]].
- [19] E. Witten, “Anti-de Sitter space and holography,” *Adv. Theor. Math. Phys.* **2**, 253 (1998) [arXiv:hep-th/9802150].
- [20] R. Emparan, C. V. Johnson and R. C. Myers, “Surface terms as counterterms in the AdS/CFT correspondence,” *Phys. Rev. D* **60**, 104001 (1999) [arXiv:hep-th/9903238].
- [21] I. R. Klebanov and A. A. Tseytlin, “Entropy of near-extremal black p-branes,” *Nucl. Phys. B* **475** (1996) 164 [hep-th/9604089].
- [22] E. Brézin, C. Itzykson, G. Parisi, J. B. Zuber, “Planar Diagrams,” *Commun. Math. Phys.* **59**, 35 (1978).
- [23] M. Mariño, “Chern-Simons theory, matrix integrals, and perturbative three manifold invariants,” *Commun. Math. Phys.* **253**, 25-49 (2004). [hep-th/0207096].
- [24] M. Aganagic, A. Klemm, M. Mariño, C. Vafa, “Matrix model as a mirror of Chern-Simons theory,” *JHEP* **0402**, 010 (2004). [hep-th/0211098].
- [25] N. Halmagyi, V. Yasnov, “The Spectral curve of the lens space matrix model,” *JHEP* **0911**, 104 (2009). [hep-th/0311117].
- [26] A. Cagnazzo, D. Sorokin, L. Wulff, “String instanton in  $\text{AdS}_4 \times \mathbb{CP}^3$ ,” *JHEP* **1005**, 009 (2010). [arXiv:0911.5228 [hep-th]].
- [27] B. Eynard and N. Orantin, “Invariants of algebraic curves and topological expansion,” *Commun. Num. Theor. Phys.* **1**, 347 (2007) [math-ph/0702045].
- [28] M. x. Huang and A. Klemm, “Holomorphic Anomaly in Gauge Theories and Matrix Models,” *JHEP* **0709**, 054 (2007) [hep-th/0605195].
- [29] N. Drukker, M. Mariño and P. Putrov, “Nonperturbative aspects of ABJM theory,” *JHEP* **1111**, 141 (2011) [arXiv:1103.4844 [hep-th]].
- [30] M. Hanada, M. Honda, Y. Honma, J. Nishimura, S. Shiba and Y. Yoshida, “Numerical studies of the ABJM theory for arbitrary N at arbitrary coupling constant,” *JHEP* **1205**, 121 (2012) [arXiv:1202.5300 [hep-th]].
- [31] Y. Hatsuda and K. Okuyama, “Probing non-perturbative effects in M-theory,” *JHEP* **1410**, 158 (2014) [arXiv:1407.3786 [hep-th]].
- [32] H. Fuji, S. Hirano and S. Moriyama, “Summing Up All Genus Free Energy of ABJM Matrix Model,” *JHEP* **1108**, 001 (2011) [arXiv:1106.4631 [hep-th]].
- [33] C. P. Burgess, “Quantum gravity in everyday life: General relativity as an effective field theory,” *Living Rev. Rel.* **7**, 5 (2004) [gr-qc/0311082].
- [34] A. Sen, “Logarithmic Corrections to Schwarzschild and Other Non-extremal Black Hole Entropy in Different Dimensions,” *JHEP* **1304**, 156 (2013) [arXiv:1205.0971 [hep-th]].
- [35] S. Bhattacharyya, A. Grassi, M. Mariño and A. Sen, “A One-Loop Test of Quantum Supergravity,” *Class. Quant. Grav.* **31**, 015012 (2014) [arXiv:1210.6057 [hep-th]].

- [36] S. H. Shenker, “The Strength of nonperturbative effects in string theory,” in O. Alvarez, E. Marinari, P. Windey (eds.), *Random surfaces and quantum gravity*, Plenum Press, New York, 1991.
- [37] M. Mariño, “Lectures on non-perturbative effects in large  $N$  gauge theories, matrix models and strings,” *Fortsch. Phys.* **62**, 455 (2014) [arXiv:1206.6272 [hep-th]].
- [38] A. Grassi, M. Mariño and S. Zakany, “Resumming the string perturbation series,” *JHEP* **1505**, 038 (2015) [arXiv:1405.4214 [hep-th]].
- [39] D. Dorigoni, “An Introduction to Resurgence, Trans-Series and Alien Calculus,” arXiv:1411.3585 [hep-th].
- [40] K. Becker, M. Becker and A. Strominger, “Five-branes, membranes and nonperturbative string theory,” *Nucl. Phys. B* **456**, 130 (1995) [hep-th/9507158].
- [41] R. C. Santamaria, M. Mariño and P. Putrov, “Unquenched flavor and tropical geometry in strongly coupled Chern-Simons-matter theories,” *JHEP* **1110**, 139 (2011) [arXiv:1011.6281 [hep-th]].
- [42] M. Mezei and S. S. Pufu, “Three-sphere free energy for classical gauge groups,” *JHEP* **1402**, 037 (2014) [arXiv:1312.0920 [hep-th], arXiv:1312.0920].
- [43] M. Mariño and P. Putrov, “ABJM theory as a Fermi gas,” *J. Stat. Mech.* **1203**, P03001 (2012) [arXiv:1110.4066 [hep-th]].
- [44] A. Kapustin, B. Willett, I. Yaakov, “Nonperturbative Tests of Three-Dimensional Dualities,” *JHEP* **1010**, 013 (2010). [arXiv:1003.5694 [hep-th]].
- [45] R. P. Feynman, *Statistical Mechanics*, Westview Press, Boulder, 1998.
- [46] B. Simon, *Operator theory*, American Mathematical Society, 2015.
- [47] A. Klemm, M. Mariño, M. Schiereck and M. Soroush, “ABJM Wilson loops in the Fermi gas approach,” *Z. Naturforsch. A* **68**, 178 (2013) [arXiv:1207.0611 [hep-th]].
- [48] M. Hillery, R. F. O’Connell, M. O. Scully, E. P. Wigner, “Distribution functions in physics: Fundamentals,” *Phys. Rept.* **106**, 121 (1984).
- [49] B. Grammaticos, A. Voros, “Semiclassical Approximations For Nuclear Hamiltonians. 1. Spin Independent Potentials,” *Annals Phys.* **123**, 359 (1979).
- [50] Y. Hatsuda, M. Mariño, S. Moriyama and K. Okuyama, “Non-perturbative effects and the refined topological string,” *JHEP* **1409**, 168 (2014) [arXiv:1306.1734 [hep-th]].
- [51] N. A. Nekrasov and S. L. Shatashvili, “Quantization of Integrable Systems and Four Dimensional Gauge Theories,” arXiv:0908.4052 [hep-th].
- [52] Y. Hatsuda, “Spectral zeta function and non-perturbative effects in ABJM Fermi-gas,” *JHEP* **1511**, 086 (2015) [arXiv:1503.07883 [hep-th]].
- [53] A. Klemm and E. Zaslow, “Local mirror symmetry at higher genus,” hep-th/9906046.
- [54] J. Kallen and M. Mariño, “Instanton effects and quantum spectral curves,” *Annales Henri Poincare* **17**, no. 5, 1037 (2016) [arXiv:1308.6485 [hep-th]].
- [55] C. A. Tracy, H. Widom, “Proofs of two conjectures related to the thermodynamic Bethe ansatz,” *Commun. Math. Phys.* **179**, 667-680 (1996). [solv-int/9509003].
- [56] R. B. Dingle and G. J. Morgan, “WKB methods for difference equations. I, II,” *Appl. Sci. Res.* **18** (1967/1968) 221–237; 238–245.
- [57] J. L. Dunham, “The Wentzel–Brillouin–Kramers method of solving the wave equation,” *Phys. Rev.* **41**, 713 (1932).

- [58] M. Aganagic, M. C. N. Cheng, R. Dijkgraaf, D. Krefl and C. Vafa, “Quantum Geometry of Refined Topological Strings,” JHEP **1211**, 019 (2012) [arXiv:1105.0630 [hep-th]].
- [59] A. Mironov and A. Morozov, “Nekrasov Functions and Exact Bohr-Zommerfeld Integrals,” JHEP **1004**, 040 (2010) [arXiv:0910.5670 [hep-th]].
- [60] N. Nekrasov, V. Pestun and S. Shatashvili, “Quantum geometry and quiver gauge theories,” arXiv:1312.6689 [hep-th].
- [61] M. Brack and R. K. Bhaduri, *Semiclassical physics*, Addison–Wesley, 1997.
- [62] S. Hosono, A. Klemm, S. Theisen and S. T. Yau, “Mirror symmetry, mirror map and applications to complete intersection Calabi-Yau spaces,” Nucl. Phys. B **433**, 501 (1995) [hep-th/9406055].
- [63] Y. Hatsuda, S. Moriyama and K. Okuyama, “Instanton Bound States in ABJM Theory,” JHEP **1305**, 054 (2013) [arXiv:1301.5184 [hep-th]].
- [64] M. x. Huang, A. Klemm, J. Reuter and M. Schiereck, “Quantum geometry of del Pezzo surfaces in the Nekrasov-Shatashvili limit,” JHEP **1502**, 031 (2015) [arXiv:1401.4723 [hep-th]].
- [65] A. Iqbal, C. Kozcaz and C. Vafa, “The Refined topological vertex,” JHEP **0910**, 069 (2009) [hep-th/0701156].
- [66] M. x. Huang and A. Klemm, “Direct integration for general  $\Omega$  backgrounds,” Adv. Theor. Math. Phys. **16**, no. 3, 805 (2012) [arXiv:1009.1126 [hep-th]].
- [67] J. Choi, S. Katz and A. Klemm, “The refined BPS index from stable pair invariants,” Commun. Math. Phys. **328**, 903 (2014) [arXiv:1210.4403 [hep-th]].
- [68] S. Moriyama and T. Nosaka, “Partition Functions of Superconformal Chern-Simons Theories from Fermi Gas Approach,” JHEP **1411**, 164 (2014) [arXiv:1407.4268 [hep-th]].
- [69] M. x. Huang, “On Gauge Theory and Topological String in Nekrasov-Shatashvili Limit,” JHEP **1206**, 152 (2012) [arXiv:1205.3652 [hep-th]].
- [70] S. Cecotti, P. Fendley, K. A. Intriligator and C. Vafa, “A New supersymmetric index,” Nucl. Phys. B **386**, 405 (1992) [hep-th/9204102].
- [71] A. B. Zamolodchikov, “Painleve III and 2-d polymers,” Nucl. Phys. B **432**, 427 (1994) [hep-th/9409108].
- [72] P. Putrov and M. Yamazaki, “Exact ABJM Partition Function from TBA,” Mod. Phys. Lett. A **27**, 1250200 (2012) [arXiv:1207.5066 [hep-th]].
- [73] Y. Hatsuda, S. Moriyama and K. Okuyama, “Exact Results on the ABJM Fermi Gas,” JHEP **1210**, 020 (2012) [arXiv:1207.4283 [hep-th]].
- [74] F. Calvo and M. Mariño, “Membrane instantons from a semiclassical TBA,” JHEP **1305**, 006 (2013) [arXiv:1212.5118 [hep-th]].
- [75] P. Fendley, “Airy functions in the thermodynamic Bethe ansatz,” Lett. Math. Phys. **49**, 229 (1999) [hep-th/9906114].
- [76] M. K. Benna, I. R. Klebanov and T. Klose, “Charges of Monopole Operators in Chern-Simons Yang-Mills Theory,” JHEP **1001**, 110 (2010) [arXiv:0906.3008 [hep-th]].
- [77] A. Gustavsson and S. J. Rey, “Enhanced  $N=8$  Supersymmetry of ABJM Theory on  $R^{*8}$  and  $R^{*8}/Z(2)$ ,” arXiv:0906.3568 [hep-th].
- [78] O. K. Kwon, P. Oh and J. Sohn, “Notes on Supersymmetry Enhancement of ABJM Theory,” JHEP **0908**, 093 (2009) [arXiv:0906.4333 [hep-th]].
- [79] D. Bashkirov and A. Kapustin, “Supersymmetry enhancement by monopole operators,” JHEP **1105**, 015 (2011) [arXiv:1007.4861 [hep-th]].

- [80] Y. Hatsuda, S. Moriyama and K. Okuyama, “Instanton Effects in ABJM Theory from Fermi Gas Approach,” *JHEP* **1301**, 158 (2013) [arXiv:1211.1251 [hep-th]].
- [81] V. A. Kazakov, I. K. Kostov and N. A. Nekrasov, “D particles, matrix integrals and KP hierarchy,” *Nucl. Phys. B* **557**, 413 (1999) [hep-th/9810035].
- [82] M. Aganagic, V. Bouchard and A. Klemm, “Topological Strings and (Almost) Modular Forms,” *Commun. Math. Phys.* **277**, 771 (2008) [hep-th/0607100].
- [83] R. Gopakumar and C. Vafa, “M theory and topological strings. 2.,” hep-th/9812127.
- [84] M. Aganagic, A. Klemm, M. Mariño and C. Vafa, “The Topological vertex,” *Commun. Math. Phys.* **254**, 425 (2005) [hep-th/0305132].
- [85] S. Codesido, A. Grassi and M. Mariño, “Exact results in  $\mathcal{N} = 8$  Chern-Simons-matter theories and quantum geometry,” *JHEP* **1507**, 011 (2015) [arXiv:1409.1799 [hep-th]].
- [86] M. Mariño, “Nonperturbative effects and nonperturbative definitions in matrix models and topological strings,” *JHEP* **0812**, 114 (2008) [arXiv:0805.3033 [hep-th]].
- [87] R. Couso-Santamaria, R. Schiappa and R. Vaz, “Finite N from Resurgent Large N,” *Annals Phys.* **356**, 1 (2015) [arXiv:1501.01007 [hep-th]].
- [88] X. f. Wang, X. Wang and M. x. Huang, “A Note on Instanton Effects in ABJM Theory,” *JHEP* **1411**, 100 (2014) [arXiv:1409.4967 [hep-th]].
- [89] A. Grassi, Y. Hatsuda and M. Mariño, “Quantization conditions and functional equations in ABJ(M) theories,” *J. Phys. A* **49**, no. 11, 115401 (2016) [arXiv:1410.7658 [hep-th]].
- [90] N. Hama, K. Hosomichi and S. Lee, “Notes on SUSY Gauge Theories on Three-Sphere,” *JHEP* **1103**, 127 (2011) [arXiv:1012.3512 [hep-th]].
- [91] D. L. Jafferis, “The Exact Superconformal R-Symmetry Extremizes Z,” *JHEP* **1205**, 159 (2012) [arXiv:1012.3210 [hep-th]].
- [92] T. Suyama, “On Large N Solution of Gaiotto-Tomasiello Theory,” *JHEP* **1010**, 101 (2010) [arXiv:1008.3950 [hep-th]].
- [93] D. Gaiotto and A. Tomasiello, “The gauge dual of Romans mass,” *JHEP* **1001**, 015 (2010) [arXiv:0901.0969 [hep-th]].
- [94] T. Suyama, “On Large N Solution of N=3 Chern-Simons-adjoint Theories,” *Nucl. Phys. B* **867**, 887 (2013) [arXiv:1208.2096 [hep-th]].
- [95] T. Suyama, “Eigenvalue Distributions in Matrix Models for Chern-Simons-matter Theories,” *Nucl. Phys. B* **856**, 497 (2012) [arXiv:1106.3147 [hep-th]].
- [96] T. Suyama, “A Systematic Study on Matrix Models for Chern-Simons-matter Theories,” *Nucl. Phys. B* **874**, 528 (2013) [arXiv:1304.7831 [hep-th]].
- [97] F. Benini, C. Closset and S. Cremonesi, “Chiral flavors and M2-branes at toric CY4 singularities,” *JHEP* **1002**, 036 (2010) [arXiv:0911.4127 [hep-th]].
- [98] A. Grassi and M. Mariño, “M-theoretic matrix models,” *JHEP* **1502**, 115 (2015) [arXiv:1403.4276 [hep-th]].
- [99] I. K. Kostov, “ $O(n)$  Vector Model on a Planar Random Lattice: Spectrum of Anomalous Dimensions,” *Mod. Phys. Lett. A* **4**, 217 (1989).
- [100] B. Eynard and C. Kristjansen, “Exact solution of the  $O(n)$  model on a random lattice,” *Nucl. Phys. B* **455**, 577 (1995) [hep-th/9506193].

- [101] B. Eynard and C. Kristjansen, “More on the exact solution of the  $O(n)$  model on a random lattice and an investigation of the case  $|n| > 2$ ,” Nucl. Phys. B **466**, 463 (1996) [hep-th/9512052].
- [102] D. L. Jafferis, I. R. Klebanov, S. S. Pufu and B. R. Safdi, “Towards the F-Theorem: N=2 Field Theories on the Three-Sphere,” JHEP **1106**, 102 (2011) [arXiv:1103.1181 [hep-th]].
- [103] M. Mariño and P. Putrov, “Interacting fermions and N=2 Chern-Simons-matter theories,” JHEP **1311**, 199 (2013) [arXiv:1206.6346 [hep-th]].
- [104] D. L. Jafferis and A. Tomasiello, “A Simple class of N=3 gauge/gravity duals,” JHEP **0810**, 101 (2008) [arXiv:0808.0864 [hep-th]].
- [105] Y. Imamura and K. Kimura, “On the moduli space of elliptic Maxwell-Chern-Simons theories,” Prog. Theor. Phys. **120**, 509 (2008) [arXiv:0806.3727 [hep-th]].
- [106] I. K. Kostov, “Solvable statistical models on a random lattice,” Nucl. Phys. Proc. Suppl. **45A**, 13 (1996) [hep-th/9509124].
- [107] D. R. Gulotta, C. P. Herzog and S. S. Pufu, “From Necklace Quivers to the F-theorem, Operator Counting, and T(U(N)),” JHEP **1112**, 077 (2011) [arXiv:1105.2817 [hep-th]].
- [108] B. Assel, N. Drukker and J. Felix, “Partition Functions of 3d  $\hat{D}$ -Quivers and Their Mirror Duals from 1d Free Fermions,” arXiv:1504.07636 [hep-th].
- [109] S. Moriyama and T. Nosaka, “Superconformal Chern-Simons Partition Functions of Affine D-type Quiver from Fermi Gas,” JHEP **1509**, 054 (2015) [arXiv:1504.07710 [hep-th]].
- [110] A. Dabholkar, N. Drukker and J. Gomes, “Localization in supergravity and quantum  $AdS_4/CFT_3$  holography,” JHEP **1410**, 90 (2014) [arXiv:1406.0505 [hep-th]].
- [111] H. Awata, S. Hirano and M. Shigemori, “The Partition Function of ABJ Theory,” Prog. Theor. Exp. Phys. , 053B04 (2013) [arXiv:1212.2966].
- [112] M. Honda, “Direct derivation of ”mirror” ABJ partition function,” JHEP **1312**, 046 (2013) [arXiv:1310.3126 [hep-th]].
- [113] S. Matsumoto and S. Moriyama, “ABJ Fractional Brane from ABJM Wilson Loop,” JHEP **1403**, 079 (2014) [arXiv:1310.8051 [hep-th]].
- [114] M. Honda and K. Okuyama, “Exact results on ABJ theory and the refined topological string,” JHEP **1408**, 148 (2014) [arXiv:1405.3653 [hep-th]].
- [115] S. Moriyama and T. Nosaka, “ABJM membrane instanton from a pole cancellation mechanism,” Phys. Rev. D **92**, no. 2, 026003 (2015) [arXiv:1410.4918 [hep-th]].
- [116] S. Moriyama and T. Nosaka, “Exact Instanton Expansion of Superconformal Chern-Simons Theories from Topological Strings,” JHEP **1505**, 022 (2015) [arXiv:1412.6243 [hep-th]].
- [117] Y. Hatsuda, M. Honda and K. Okuyama, “Large N non-perturbative effects in  $\mathcal{N} = 4$  superconformal Chern-Simons theories,” JHEP **1509**, 046 (2015) [arXiv:1505.07120 [hep-th]].
- [118] S. Moriyama and T. Suyama, “Instanton Effects in Orientifold ABJM Theory,” arXiv:1511.01660 [hep-th].
- [119] K. Okuyama, “Probing non-perturbative effects in M-theory on orientifolds,” JHEP **1601**, 054 (2016) [arXiv:1511.02635 [hep-th]].
- [120] M. Honda, “Exact relations between M2-brane theories with and without Orientifolds,” arXiv:1512.04335 [hep-th].
- [121] N. Drukker and J. Felix, “3d mirror symmetry as a canonical transformation,” JHEP **1505**, 004 (2015) [arXiv:1501.02268 [hep-th]].

- [122] M. Mariño, “Topological strings at strong string coupling,” talk given in november 2011 at the Banff workshop *New recursion formulae and integrability for Calabi–Yau spaces*, <http://www.birs.ca/events/2011/5-day-workshops/11w5114/videos>.
- [123] M. x. Huang and X. f. Wang, “Topological Strings and Quantum Spectral Problems,” JHEP **1409**, 150 (2014) [arXiv:1406.6178 [hep-th]].
- [124] A. Grassi, Y. Hatsuda and M. Mariño, “Topological Strings from Quantum Mechanics,” arXiv:1410.3382 [hep-th].
- [125] R. Kashaev and M. Mariño, “Operators from mirror curves and the quantum dilogarithm,” arXiv:1501.01014 [hep-th].
- [126] M. Mariño and S. Zakany, “Matrix models from operators and topological strings,” *Annales Henri Poincare* **17**, no. 5, 1075 (2016) [arXiv:1502.02958 [hep-th]].
- [127] J. Gu, A. Klemm, M. Mariño and J. Reuter, “Exact solutions to quantum spectral curves by topological string theory,” JHEP **1510**, 025 (2015) [arXiv:1506.09176 [hep-th]].
- [128] X. Wang, G. Zhang and M. x. Huang, “New Exact Quantization Condition for Toric Calabi-Yau Geometries,” *Phys. Rev. Lett.* **115**, 121601 (2015) [arXiv:1505.05360 [hep-th]].
- [129] S. Codesido, A. Grassi and M. Mariño, “Spectral Theory and Mirror Curves of Higher Genus,” arXiv:1507.02096 [hep-th].
- [130] K. Okuyama and S. Zakany, “TBA-like integral equations from quantized mirror curves,” arXiv:1512.06904 [hep-th].
- [131] A. K. Kashani-Poor, “Quantization condition from exact WKB for difference equations,” arXiv:1604.01690 [hep-th].
- [132] A. Grassi, “Spectral determinants and quantum theta functions,” arXiv:1604.06786 [hep-th].
- [133] M. Mariño and S. Zakany, “Exact eigenfunctions and the open topological string,” arXiv:1606.05297 [hep-th].
- [134] M. Mariño, “Spectral Theory and Mirror Symmetry,” arXiv:1506.07757 [math-ph].
- [135] I. K. Kostov, “Exact solution of the six vertex model on a random lattice,” *Nucl. Phys. B* **575**, 513 (2000) [hep-th/9911023].
- [136] R. Kashaev, M. Mariño and S. Zakany, “Matrix models from operators and topological strings, 2,” arXiv:1505.02243 [hep-th].
- [137] G. Bonelli, A. Grassi and A. Tanzini, “Seiberg-Witten theory as a Fermi gas,” arXiv:1603.01174 [hep-th].
- [138] S. H. Katz, A. Klemm and C. Vafa, “Geometric engineering of quantum field theories,” *Nucl. Phys. B* **497**, 173 (1997) [hep-th/9609239].
- [139] Y. Hatsuda, “ABJM on ellipsoid and topological strings,” arXiv:1601.02728 [hep-th].

# Chapter 8

## The $F$ -Theorem and $F$ -Maximization

Silviu S. Pufu

*Joseph Henry Laboratories, Princeton University, Princeton, NJ 08544, USA*  
spufu@Princeton.EDU

### Abstract

This contribution contains a review of the role of the three-sphere free energy  $F$  in recent developments related to the  $F$ -theorem and  $F$ -maximization. The  $F$ -theorem states that for any Lorentz-invariant RG trajectory connecting a conformal field theory  $\text{CFT}_{\text{UV}}$  in the ultraviolet to a conformal field theory  $\text{CFT}_{\text{IR}}$ , the  $F$ -coefficient decreases:  $F_{\text{UV}} > F_{\text{IR}}$ . I provide many examples of CFTs where one can compute  $F$ , approximately or exactly, and discuss various checks of the  $F$ -theorem.  $F$ -maximization is the principle that in an  $\mathcal{N} = 2$  SCFT, viewed as the deep IR limit of an RG trajectory preserving  $\mathcal{N} = 2$  supersymmetry, the superconformal R-symmetry maximizes  $F$  within the set of all R-symmetries preserved by the RG trajectory. I review the derivation of this result and provide examples.

### Contents

|            |                                                                           |            |
|------------|---------------------------------------------------------------------------|------------|
| <b>8.1</b> | <b>Introduction</b>                                                       | <b>335</b> |
| <b>8.2</b> | <b>The <math>F</math>-coefficients of various CFTs</b>                    | <b>337</b> |
| 8.2.1      | $F$ in free field theories                                                | 337        |
| 8.2.2      | $F$ in perturbative expansions                                            | 340        |
| 8.2.3      | $F$ in theories with holographic duals                                    | 344        |
| 8.2.4      | $F$ in supersymmetric theories                                            | 345        |
| <b>8.3</b> | <b><math>\mathcal{N} = 2</math> SCFTs and <math>F</math>-maximization</b> | <b>347</b> |
| 8.3.1      | Non-conformal theories on $S^3$                                           | 348        |
| 8.3.2      | Supersymmetric localization                                               | 352        |
| 8.3.3      | $F$ -maximization                                                         | 353        |
| 8.3.4      | Examples                                                                  | 356        |

|                          |     |
|--------------------------|-----|
| 8.4 Conclusion . . . . . | 360 |
| References . . . . .     | 361 |

## 8.1 Introduction

A central problem in theoretical physics is to find the laws that govern the low-energy dynamics of a physical system whose microscopic description is either fully known or, more often than not, only approximately known. The conceptual framework in which this problem is usually formulated is that of the Renormalization Group (RG) flow—a motion in the space of theories that captures the effective degrees of freedom as they change with the energy scale used to probe the system. Based on the intuition that the effective number of degrees of freedom decreases during this process, one expects that there exist quite general constraints that limit the set of possible RG trajectories. In practice, such constraints could be extremely valuable because they could rule out or predict the kinds of low-energy dynamics that a given system might exhibit. The goal of this Chapter is to discuss such a constraint, called the  $F$ -theorem, which applies to relativistic RG flows in three space-time dimensions, as well as to review a few related developments.

If one insists on Lorentz invariance, as we will do in the present Chapter, a common picture is that the RG flow interpolates between two scale-invariant theories: one valid at high energies (the ultraviolet fixed point) and one valid at low energies (the infrared fixed point). In many cases, the symmetry of these scale-invariant theories is augmented to the conformal group, which in addition to Lorentz transformations and dilatations also includes special conformal transformations.<sup>1</sup> Let us therefore restrict our attention to RG flows between two conformal field theories (CFTs). The statement of the  $F$ -theorem is that each CFT can be assigned a number  $F$ , equal to the regularized  $S^3$  free energy,  $F \equiv -\log|Z_{S^3}|$ , as will be discussed in more detail shortly, with the property that whenever there exists an RG flow between a UV CFT and an IR CFT, one has  $F_{\text{UV}} > F_{\text{IR}}$ . In other words, the  $F$ -coefficient always decreases under RG flow. Consequently, the RG flow is not reversible: if there exists a relativistic RG flow between CFT<sub>1</sub> in the UV and CFT<sub>2</sub> in the IR, a relativistic RG flow between CFT<sub>2</sub> in the UV and CFT<sub>1</sub> in the IR is ruled out.

The  $F$ -theorem is a rather recent development that applies to three-dimensional QFTs. It has older analogs in other numbers of space-time dimensions. For instance, in two space-time dimensions, Zamolodchikov [5] showed that the central charge  $c$  always decreases under RG flow, a result known as the  $c$ -theorem. Similarly, in four-dimensional theories, Cardy [6] conjectured that the Weyl anomaly coefficient  $a$  has a similar property. This result is known as the  $a$ -theorem and was proven recently by Komargodski and Schwimmer [7]. Likewise, in one space-time dimension (i.e. for quantum mechanical systems) it has been proven that the thermal free energy decreases under RG flow, a statement known as the  $g$ -theorem [8, 9].

---

<sup>1</sup>There are known exceptions, however. For instance, free Maxwell theory in three dimensions is scale invariant, but not conformally invariant in the ultraviolet. See for example [2–4].

There is a significant difference between even and odd space-time dimensions, however. The coefficients  $c$  and  $a$  in two and four space-time dimensions, respectively, correspond to anomalies that are not present in odd space-time dimensions. These anomaly coefficients appear in correlation functions at separated points and can therefore be calculated from correlation functions of local operators. The  $F$ -coefficient, on the other hand, is a non-local quantity. Indeed, it can be non-vanishing even in topological field theories that have no local degrees of freedom, as will be shown in the case of Chern-Simons theory in Section 8.2.1. Despite these differences between even and odd space-time dimensions, a unified treatment in all dimensions can be achieved by considering the sphere partition function of the Euclidean CFT.

There are two different paths that led to the development of the  $F$ -theorem. The first path involves supersymmetric gauge theories. Three-dimensional superconformal field theories (SCFTs) with  $\mathcal{N} = 2$  supersymmetry possess a global  $U(1)_R$  R-symmetry<sup>2</sup> that appears in the superconformal algebra, just as in the case with  $\mathcal{N} = 1$  SCFTs in four dimensions. This symmetry is important because it determines various unitarity bounds—for instance, the scaling dimensions of all scalar operators must be at least equal to the magnitude of their  $U(1)_R$  charge, and scalar operators that saturate this bound have very special properties. Given an SCFT, it is desirable to determine the  $U(1)_R$  charges of the various operators of the theory.

In general, the determination of the  $U(1)_R$  symmetry is a very difficult problem even for theories with Lagrangian descriptions where the SCFT of interest is realized as the infrared limit of an RG flow, because generically the  $U(1)_R$  R-symmetry appears as an emergent symmetry only at the IR fixed point. In cases where the SCFT of interest can be reached via an  $\mathcal{N} = 2$ -preserving RG flow that does preserve some R-symmetry  $U(1)_R^{\text{RG}}$  and there are no accidental symmetries at the IR fixed point, the  $U(1)_R$  symmetry that appears in the superconformal algebra of the IR SCFT can be a linear combination of  $U(1)_R^{\text{RG}}$  and other abelian flavor symmetries preserved throughout the RG flow. It was proposed by Jafferis in [10] and later refined in [11, 12] that a procedure called  $F$ -maximization can be used to determine this linear combination. As will be discussed in more detail in Section 8.3, the procedure involves maximizing the  $S^3$  free energy  $F$  over a family of QFTs. A similar procedure for  $\mathcal{N} = 1$  theories in four dimensions called  $a$ -maximization [13] had been known previously and involved maximizing the anomaly coefficient  $a$ . Since the four-dimensional anomaly coefficient  $a$  and the three-dimensional  $S^3$  free energy  $F$  play similar roles, and since the 4-d  $a$ -coefficient was expected to be monotonic under RG flow, it was proposed in [11] that the  $F$ -coefficient should have the same property. Many tests of this proposal were performed both in supersymmetric and non-supersymmetric RG trajectories [11, 14–16].

The second path to the development of the  $F$ -theorem starts from the work of Myers and Sinha [17, 18], who studied RG flows for quantum field theories with holographic duals. For Lorentz-invariant holographic RG flows between  $d$ -dimensional CFTs, they identified a quantity  $a_d$  that decreases monotonically. Let  $a_d^*$  denote the value of  $a_d$  at an RG fixed point. It can be shown that in  $d = 2$  one has  $a_2^* = c$  and in  $d = 4$  one has  $a_4^* = a$ , and thus the

---

<sup>2</sup>An R-symmetry is a symmetry that does not commute with the supersymmetry generators.

quantity  $a_d^*$  provides a generalization of these conformal anomaly coefficients to arbitrary  $d$ . As explained in [18], the quantity  $a_d^*$  can also be interpreted as the universal part in the vacuum entanglement entropy between a ball of radius  $R$  and its complement. (In general, this entanglement entropy is divergent, being proportional to the area of the boundary of the ball in units of the UV cutoff. In a CFT it is possible to subtract unambiguously the power divergences and identify a universal contribution.) The connection between the three-dimensional  $a_3^*$  and the  $F$ -coefficient as defined above was made in [19], where it was shown that for any CFT, the universal part of the vacuum entanglement entropy between a ball and its complement is equal precisely to the  $F$ -coefficient.

This second line of development was taken further by Liu and Mezei [20], who defined for any 3-d Lorentz-invariant RG flow the notion of renormalized entanglement entropy (REE), which is a finite quantity which agrees with the  $F$ -coefficient at the UV and IR fixed points. As shown further by Casini and Huerta [21], the REE interpolates monotonically between  $F_{UV}$  and  $F_{IR}$  in any Lorentz-invariant RG flow, thus establishing the  $F$ -theorem. This proof of the  $F$ -theorem is based on the strong subadditivity property of entanglement entropy and generalizes a similar proof of the  $c$ -theorem in 2-d [22]. Extending this proof to dimensions higher than three is currently still an open problem.

In the rest of this Chapter I provide more details on these recent developments. I focus on the definition of  $F$  as the universal part in the  $S^3$  free energy as opposed to its definition in terms of entanglement entropy, partly because this definition is more closely related to the topics presented in this volume, and partly because it renders  $F$  more easily computable in many cases. In Section 8.2 I discuss the computation of the  $F$ -coefficient in free theories and in various approximations such as the  $1/N$  expansion or the  $\epsilon$  expansion, as well as in supersymmetric theories. These computations provide many checks of the  $F$ -theorem. In Section 8.3 I discuss the  $F$ -maximization principle and show how it can be applied in a few simple examples.

## 8.2 The $F$ -coefficients of various CFTs

### 8.2.1 $F$ in free field theories

Let us begin with presenting the computation of  $F$  in free field theories, where  $F$  can be easily calculated by performing a Gaussian integral [15, 23, 24].

#### Free real scalar field

To calculate the  $F$ -coefficient of a free massless real scalar field, we start with the action for a conformally coupled scalar:

$$\mathcal{S}_S = \frac{1}{2} \int d^3x \sqrt{g} \left[ \partial_\mu \phi \partial^\mu \phi + \frac{\mathcal{R}}{8} \phi^2 \right]. \quad (8.2.1)$$

The conformal coupling term,  $\mathcal{R}\phi^2/8$ , guarantees that this action is invariant under Weyl rescalings  $g_{\mu\nu}(x) \rightarrow e^{2\Omega(x)}g_{\mu\nu}(x)$ ,  $\phi(x) \rightarrow e^{-\Omega(x)/2}\phi(x)$ , for any  $\Omega(x)$ . Equivalently, the

conformal coupling guarantees that the correlation functions of  $\phi$  computed on a conformally flat space from the action (8.2.1) agree with those obtained by conformal transformation of the flat space ones. On an  $S^3$  of unit radius, we have that the Ricci scalar is  $\mathcal{R} = 6$ . The  $S^3$  free energy is therefore

$$F_S = -\log|Z_S| = \frac{1}{2} \text{tr} \log \left( -\nabla^2 + \frac{3}{4} \right). \quad (8.2.2)$$

The operator  $-\nabla^2 + \frac{3}{4}$  has eigenvalues

$$n(n+2) + \frac{3}{4} = \left(n + \frac{1}{2}\right) \left(n + \frac{3}{2}\right), \quad n = 0, 1, 2, \dots, \quad (8.2.3)$$

each appearing with degeneracy  $(n+1)^2$ . The free energy is thus

$$F_S = \frac{1}{2} \sum_{n=0}^{\infty} (n+1)^2 \log \left[ \left(n + \frac{1}{2}\right) \left(n + \frac{3}{2}\right) \right]. \quad (8.2.4)$$

This sum is cubically divergent, but it can be regularized in zeta-function regularization, or by simply multiplying each term by an exponential damping factor  $e^{-\epsilon(n+\frac{1}{2})(n+\frac{3}{2})}$ , with  $\epsilon > 0$ , and removing the power divergences in  $1/\epsilon$  in an expansion at small  $\epsilon$ . The regularized value of  $F_S$  is [23–25]

$$F_S = \frac{\log 2}{8} - \frac{3\zeta(3)}{16\pi^2} \approx 0.0638. \quad (8.2.5)$$

A notable feature of this answer is that it is strictly positive, as can be inferred from the  $F$ -theorem as follows. While the theory of a free massless scalar considered above is a CFT, the theory of a free massive scalar is not. Instead, a free massive scalar can be thought of as an RG trajectory connecting the CFT of a free massless scalar in the UV and an empty theory (a theory with no local or non-local operators) in the IR. The empty theory is a trivial CFT that should be assigned  $F_{\text{empty}} = 0$ . That  $F_S > F_{\text{empty}} = 0$  is thus a necessary condition for the  $F$ -theorem to hold.

### Free Dirac fermion

The next example of a free theory that we discuss is a free massless Dirac fermion (two-component complex spinor), for which the action on  $S^3$  can be written as

$$\mathcal{S}_D = \int d^3x \sqrt{g} \psi^\dagger (i\mathcal{D}) \psi, \quad (8.2.6)$$

where  $\mathcal{D}$  is the Dirac operator. The free energy is

$$F_D = -\log|Z_D| = -\text{tr} \log(i\mathcal{D}). \quad (8.2.7)$$

As in the case of a massless scalar, writing  $F_D$  as a sum over the eigenvalues of  $i\not{D}$  yields a divergent answer that can be regularized, for instance, using zeta function regularization. For a free massless Dirac fermion, the regularized value of  $F_D$  is

$$F_D = \frac{\log 2}{4} + \frac{3\zeta(3)}{8\pi^2} \approx 0.219. \quad (8.2.8)$$

As in the scalar case discussed above, there exists an RG trajectory corresponding to a free massive fermion that connects the CFT of a free Dirac fermion to the empty theory for which  $F_{\text{empty}} = 0$ . That  $F_D > 0$  is consistent with the  $F$ -theorem.

For a free Majorana fermion, we have

$$F_M = \frac{1}{2}F_D = \frac{\log 2}{8} + \frac{3\zeta(3)}{16\pi^2} \approx 0.109. \quad (8.2.9)$$

A free minimal  $\mathcal{N} = 1$  multiplet consisting of a free real scalar and a free Majorana fermion therefore has

$$F_S + F_M = \frac{\log 2}{4} \approx 0.173. \quad (8.2.10)$$

The  $F$ -coefficients of a free massless  $\mathcal{N} = 2$  chiral multiplet (consisting of a free massless complex scalar and a free massless Dirac fermion) and a free massless hypermultiplet (consisting of two massless complex scalars and two massless Dirac fermions) are twice and four times the value quoted in (8.2.10), respectively:

$$F_{\text{chiral}} = 2(F_S + F_M) = \frac{\log 2}{2} \approx 0.347, \quad F_{\text{hyper}} = 4(F_S + F_M) = \log 2 \approx 0.693. \quad (8.2.11)$$

### Chern-Simons theory

Another case in which the  $F$ -coefficient can be computed is that of Chern-Simons theory at level  $k$ , described by the 3-d action

$$\mathcal{S}_{\text{CS}} = \frac{ik}{4\pi} \int \text{tr} \left[ A \wedge dA - \frac{2i}{3} A \wedge A \wedge A \right], \quad (8.2.12)$$

where the gauge field  $A$  transforms in the adjoint representation of the gauge group. In the case of  $U(N)$  (or  $SU(N)$ ) the Chern-Simons level  $k$  is quantized in integer units provided that “tr” is the trace in the fundamental representation. In the  $N = 1$  case, an explicit evaluation of the Gaussian integral as in the scalar and fermion cases above, one obtains In this case

$$F_{\text{CS}} = \frac{1}{2} \log k. \quad (8.2.13)$$

More generally, for  $U(N)$  Chern-Simons theory at level  $k$ , we have, when  $N > 1$ , [26]

$$F_{\text{CS}}(k, N) = \frac{N}{2} \log(k + N) - \sum_{j=1}^{N-1} (N - j) \log \left( 2 \sin \frac{\pi j}{k + N} \right). \quad (8.2.14)$$

It is worth noting that in Maxwell theory on an  $S^3$  of radius  $R$ , we have [16] (see also [27])

$$F_{\text{Maxwell}} = -\frac{\log e^2 R}{2} + \frac{\zeta(3)}{4\pi^2}. \quad (8.2.15)$$

This theory is not conformal, because  $e^2$  has dimensions of mass. When  $R \rightarrow 0$ , we have  $F_{\text{Maxwell}} \rightarrow \infty$ , which is again in agreement with the  $F$ -theorem as applied to the case of the Maxwell-Chern-Simons theory, which can be thought of as an RG flow between Maxwell theory in the UV and Chern-Simons theory at level  $k$  in the IR.

## 8.2.2 $F$ in perturbative expansions

In theories that are not free, the  $F$ -coefficient is more difficult to calculate. As we now describe, it can be calculated approximately in various perturbative expansions. In Sections 8.2.4 and 8.3, we will describe the computation of  $F$  in supersymmetric theories, where it can be computed exactly.

### Theories with many flavors

Theories with many flavors, such as the critical  $O(N)$  vector model, become approximately free when the number of flavors is taken to infinity, and the  $F$ -coefficient of such a theory approaches that of the corresponding free theory. A general class of such theories are Chern-Simons theories coupled to charged bosons and fermions, such as a  $U(1)$  gauge theory with Chern-Simons level  $k$  to which we couple  $N_b$  complex scalars with charge  $q_b$  and  $N_f$  Dirac fermions with charge  $q_f$  with the action on  $\mathbb{R}^3$  given by

$$\begin{aligned} \mathcal{S} = \frac{ik}{4\pi} \int A \wedge dA + \int d^3x \left[ \sum_{a=1}^{N_b} [ |(\partial_\mu - iq_b A_\mu)\phi_a|^2 + s|\phi_a|^2 ] \right. \\ \left. + \sum_{\alpha=1}^{N_f} \psi_\alpha^\dagger (i\not{D} + q_f \not{A}) \psi_\alpha + \frac{u}{2} \left( \sum_{a=1}^{N_b} |\phi_a|^2 \right)^2 \right] + \dots \end{aligned} \quad (8.2.16)$$

Here, the ellipses denote other possible interactions, such as a Maxwell term for the gauge field, or a sextic boson coupling, which are believed to be irrelevant at large distances. This action does not include fermion mass terms or Yukawa terms, as these can be projected out by imposing discrete symmetries.

An interesting limit of (8.2.16) is that where  $N_f$ ,  $N_b$ , and  $k$  are all taken to infinity together. In this limit, one can argue that, upon tuning the boson mass parameter  $s$ , the IR physics is described by an interacting conformal field theory. To leading order, the  $F$ -coefficient is given by that of  $N_b$  free complex scalars and  $N_f$  free Dirac fermions, namely

$$F = 2N_b F_S + N_f F_D + \dots, \quad (8.2.17)$$

where  $F_S$  and  $F_D$  are given in (8.2.5) and (8.2.8), respectively.

The first correction to (8.2.17) can be computed as follows [16]. The first step is to decouple the quartic scalar interaction with the help of a dynamical Hubbard-Stratanovich field  $\lambda$ , thus making the replacement

$$\frac{u}{2} \left( \sum_{a=1}^{N_b} |\phi_a|^2 \right)^2 \rightarrow i\lambda \sum_{a=1}^{N_b} |\phi_a|^2 + \frac{\lambda^2}{2u} \quad (8.2.18)$$

in (8.2.16). Integrating over  $\lambda$ , one recovers the quartic scalar interaction. At low energies,  $u$  grows and the term  $\lambda^2/u$  can be dropped. One can then consider the resulting action on any conformally flat space:

$$\begin{aligned} \mathcal{S} = & \int d^3x \sqrt{g} \left[ \sum_{a=1}^{N_b} \left[ |(\partial_\mu - iq_b A_\mu)\phi_a|^2 + \left( \frac{\mathcal{R}}{8} + i\lambda \right) |\phi_a|^2 \right] \right. \\ & \left. + \sum_{\alpha=1}^{N_f} \psi_\alpha^\dagger (i\mathcal{D} + q_f \mathcal{A}) \psi_\alpha + \frac{ik}{4\pi} \int A \wedge dA \right] \end{aligned} \quad (8.2.19)$$

In the case of an  $S^3$  of unit radius, we have  $\mathcal{R} = 6$ , as before.

Performing the Gaussian path integral over the bosons and fermions, the  $S^3$  partition function becomes

$$Z = \int DA_\mu D\lambda \exp[-\mathcal{S}_{\text{eff}}[A_\mu, \lambda]] , \quad (8.2.20)$$

with

$$\mathcal{S}_{\text{eff}}[A_\mu, \lambda] = N_b \text{tr} \log \left( -(\nabla_\mu - iq_b A_\mu)^2 + \lambda + \frac{3}{4} \right) - N_f \text{tr} \log(i\mathcal{D} + q_f \mathcal{A}) + \frac{ik}{4\pi} \int A \wedge dA . \quad (8.2.21)$$

When  $N_f$ ,  $N_b$ , and  $k$  are large, the typical fluctuations of both the gauge field and the Lagrange multiplier are suppressed, and one can calculate  $Z$  in a saddle point approximation:

$$\begin{aligned} Z \approx & e^{-\mathcal{S}_{\text{eff}}[0,0]} \int DA_\mu D\lambda \exp \left[ -\frac{1}{2} \int d^3x d^3y A_\mu(x) A_\nu(y) \left( -\frac{\delta^2 \mathcal{S}_{\text{eff}}[A_\mu, \lambda]}{\delta A_\mu(x) \delta A_\nu(y)} \Big|_{A=\lambda=0} \right) \right. \\ & \left. - \frac{1}{2} \int d^3x d^3y \lambda(x) \lambda(y) \left( \frac{\delta^2 \mathcal{S}_{\text{eff}}[A_\mu, \lambda]}{\delta \lambda(x) \delta \lambda(y)} \Big|_{A=\lambda=0} \right) \right] , \end{aligned} \quad (8.2.22)$$

obtained by expanding the effective action (8.2.21) to quadratic order in the fluctuations and re-exponentiating. (The first derivatives with respect to  $\lambda$  and  $A_\mu$ , as well as the mixed second derivative vanish due to conformal invariance of the  $A = \lambda = 0$  theory.)

The quantity  $\mathcal{S}_{\text{eff}}[0, 0]$  reduces to the functional determinants in the free theory computed in the previous section. It gives precisely

$$\mathcal{S}_{\text{eff}}[0, 0] = 2N_b F_S + N_f F_D . \quad (8.2.23)$$

The Gaussian integral in (8.2.22) over  $A_\mu$  and  $\lambda$  is rather complicated, but was performed in [16]. The final result for  $F$  is

$$F = 2N_b F_S + N_f F_D + \frac{1}{2} \log \left[ \pi \sqrt{\left( \frac{q_f^2 N_f + q_b^2 N_b}{8} \right)^2 + \left( \frac{k}{\pi} \right)^2} \right] - \frac{\zeta(3)}{8\pi^2} + \dots, \quad (8.2.24)$$

where the corrections are suppressed at large  $N_f$ ,  $N_b$ , and  $k$ .

A particular case of (8.2.24) gives an approximate expression for the  $F$ -coefficient of the critical  $O(N)$  vector model. Indeed, setting  $N_b = N/2$ , as the fields appearing in the critical  $O(N)$  model are real scalars, as well as setting  $N_f = 0$ ,  $q_b = 0$ , and removing the topological contribution  $\frac{1}{2} \log k$  from (8.2.24), one obtains

$$F_{\text{critical}}(N) = N F_S - \frac{\zeta(3)}{8\pi^2} + O(1/N). \quad (8.2.25)$$

The correction to the free theory result given by the second term in (8.2.24) is a particular case of a more general setup, where instead of gauging a spin-1 current we gauge one of the higher spin currents of the free theory [28]. A related approximation scheme can be developed in the case of double trace deformations of large  $N$  vector models [15, 28].

### **$F$ from the $\epsilon$ expansion**

Another perturbative expansion that is commonly used in the theory of critical phenomena is the  $\epsilon$  expansion [29] (for a review, see [30]). This method is successfully used, for instance, to estimate certain critical exponents in CFTs such as the 3-d Ising model, and these estimates agree quite well with experimental measurements and lattice simulations. The idea of the  $\epsilon$  expansion is to continue the CFT of interest to non-integer space-time dimensions and identify the number of spacetime dimensions  $d = d_*$  where the theory can become free, or more generally, where the theory can be solved exactly. Then one can develop a perturbative expansion in  $\epsilon = d - d_*$  and extrapolate these results to the value of  $d$  of interest.

In recent work, Refs. [31–33] applied the  $\epsilon$  expansion method to the computation of the  $F$ -coefficient in theories such as the critical  $O(N)$  vector models, Gross-Neveu models, and quantum electrodynamics with charged fermionic matter. In general, it is expected that the free energy  $F^{(d)}$  on a round  $S^d$  should diverge (even after removing non-universal divergences) when  $d$  approaches an even integer due to the presence of a conformal anomaly. Indeed, when  $d$  is an even integer, the  $S^d$  free energy has a universal logarithmic dependence on the radius of the sphere proportional to the conformal anomaly coefficient—in  $d = 2$  the coefficient of the logarithmic divergence equals  $\frac{\pi}{6}c$  in the convention where a free non-compact real scalar has  $c = 1$ , while in  $d = 4$  this coefficient equals  $\frac{\pi}{2}a$  in the convention where a free real scalar has  $a = 1/90$ . The theories studied in [31–33] are solvable precisely in even  $d$ , where these divergences occur. To obtain a finite quantity, Refs. [31–33] defined

$$\tilde{F}^{(d)} = -F^{(d)} \sin \frac{\pi d}{2}. \quad (8.2.26)$$

After removing non-universal divergences, the quantity  $\tilde{F}^{(d)}$  is finite in all  $d$ . It interpolates between  $F$  in  $d = 3$  and the anomaly coefficients in  $d = 2$  and  $d = 4$ .

The critical  $O(N)$  vector model merges with the free CFT of  $N$  scalar fields in  $d = 4$ , and in  $d = 4 - \epsilon$  dimensions, with  $\epsilon \ll 1$ , it is thus weakly coupled. In [31, 32] it was found that

$$\begin{aligned} \tilde{F}_{O(N)}^{(4-\epsilon)} &= N\tilde{F}_S^{(4-\epsilon)} - \frac{\pi N(N+2)}{576(N+8)^2}\epsilon^3 - \frac{\pi N(N+2)(13N^2+370N+1588)}{6912(N+8)^4}\epsilon^4 \\ &+ \frac{\pi N(N+2)}{414720(N+8)^6} \left[ 10368(N+8)(5N+22)\zeta(3) - 647N^4 - 32152N^3 \right. \\ &\left. - 606576N^2 - 3939520N + 30\pi^2(N+8)^4 - 8451008 \right] \epsilon^5 + O(\epsilon^6), \end{aligned} \quad (8.2.27)$$

where

$$\tilde{F}_S^{(d)} = \frac{1}{\Gamma(1+d)} \int_0^1 du u \sin(\pi u) \Gamma\left(\frac{d}{2} + u\right) \Gamma\left(\frac{d}{2} - u\right) \quad (8.2.28)$$

represents the value of  $\tilde{F}^{(d)}$  of a free conformally coupled scalar. In  $d = 3$ , (8.2.28) reduces to (8.2.5).

Of particular interest is the  $N = 1$  case where the critical  $O(N)$  vector model is nothing but the critical Ising theory. In this case  $O(1) = \mathbb{Z}_2$ , and the critical Ising theory can be thought of the IR fixed point of a real scalar with a quartic potential,

$$S_{\text{Ising}} = \int d^d x \left[ (\partial_\mu \phi)^2 + m^2 \phi^2 + \lambda \phi^4 \right], \quad (8.2.29)$$

upon tuning the mass  $m$  to zero. When continued in  $d$ , it is well-known that the critical Ising theory has  $c = 1/2$  in  $d = 2$ , corresponding to  $\tilde{F}^{(2)} = \pi/12$  exactly. Using this exact value in  $d = 2$  and (8.2.27) close to  $d = 4$ , one can then construct an interpolating function and estimate that, in  $d = 3$  [31, 32]

$$\frac{F_{\text{Ising}}}{F_S} \approx 0.976. \quad (8.2.30)$$

The  $F$ -coefficient of the 3-d Ising CFT is thus fairly close to that of a free scalar field, but slightly smaller than the latter as required by the  $F$ -theorem. That the ratio (8.2.30) is close to 1 indicates that the 3-d Ising CFT is in some sense fairly close to the free scalar CFT in the space of all CFTs. For comparison, the scaling dimension of  $\phi$  in the Ising CFT is  $\Delta_\phi^{\text{Ising}} \approx 0.518$ , which is fairly close to the free scalar value  $\Delta_\phi^{\text{free}} = 1/2$ , but the scaling dimension of  $\phi^2$  is rather different being  $\Delta_{\phi^2}^{\text{Ising}} \approx 1.412$  in the Ising CFT and  $\Delta_{\phi^2}^{\text{free}} \approx 1$  in the free theory. As another comparison, the two-point function of the canonically normalized stress energy tensor  $T_{\mu\nu}$  obeys  $\langle T_{\mu\nu}(x)T_{\rho\sigma}(0) \rangle_{\text{Ising}} \approx 0.947 \langle T_{\mu\nu}(x)T_{\rho\sigma}(0) \rangle_{\text{free}}$ , so again this quantity in the interacting theory is very close to the free field result.

It is worth noting that Refs. [31–33] also conjectured that  $\tilde{F}^{(d)}$  may obey a generalized version of the  $F$ -theorem as well as of the  $F$ -maximization principle to be discussed in Section 8.3. (See also [34].)

### 8.2.3 $F$ in theories with holographic duals

Another class of CFTs where one can calculate the  $F$ -coefficient approximately are CFTs with holographic duals. Quite generally, suppose we have such a CFT whose vacuum is dual to the  $AdS_4$  solution of the classical equations of motion of an effective 4-d two-derivative gravity (or supergravity) theory with negative cosmological constant. Let  $L$  be the radius of curvature of  $AdS_4$ . In Einstein frame, the two-derivative classical Euclidean action can be written as

$$S = \frac{1}{16\pi G_4} \int d^4x \sqrt{g} \left( -R - \frac{6}{L^2} + \mathcal{L}_{\text{matter}} \right), \quad (8.2.31)$$

where  $G_4$  is the 4-d Newton constant, and  $\mathcal{L}_{\text{matter}}$  is the matter Lagrangian that we assume vanishes on the (Euclidean)  $AdS_4$  solution of the equations of motion.

In the regime where classical two-derivative supergravity is a good approximation, the  $F$ -coefficient of the dual field theory is simply equal to the regularized value of the Euclidean on-shell action. The Euclidean continuation of  $AdS_4$  is the hyperbolic space  $\mathbb{H}^4$ , whose line element is

$$ds^2 = L^2(dr^2 + \sinh^2 r ds_{S^3}^2), \quad (8.2.32)$$

where  $ds_{S^3}^2$  is the metric on a round three-sphere of unit curvature radius. The Ricci scalar of (8.2.32) is  $R = -12/L^2$ , and so plugging (8.2.32) into (8.2.31), we can write the on-shell action as

$$F = \frac{3}{8\pi G_4 L^2} \text{Vol}(\mathbb{H}^4). \quad (8.2.33)$$

The volume of  $\mathbb{H}^4$  is of course infinite, but it can be regularized by imposing a cutoff that obeys the  $SO(4)$  symmetry:

$$\text{Vol}(\mathbb{H}^4) = L^4 \text{Vol}(S^3) \int_0^{\log \Lambda} dr \sinh^3 r = L^4 \text{Vol}(S^3) \left[ \frac{\Lambda^3}{24} - \frac{3\Lambda}{8} + \frac{2}{3} + \dots \right]. \quad (8.2.34)$$

After throwing away the power divergences in  $\Lambda$  and using  $\text{Vol}(S^3) = 2\pi^2$ , we obtain  $\text{Vol}(\mathbb{H}^4) = \frac{4}{3}\pi^2 L^4$ . From (8.2.33), we deduce that [11, 35]

$$F = \frac{\pi L^2}{2G_4} \quad (8.2.35)$$

in the classical gravity approximation. To find an explicit expression for  $F$  in terms of field theory data, one has to use the AdS/CFT dictionary on a case-by-case basis to relate  $L^2/G_4$  to quantities defined in the field theory.

An interesting class of examples of CFTs with  $AdS_4$  duals are the infrared limits of the effective theories on  $N$  coincident M2-branes placed at the tip of a Calabi-Yau cone. If  $Y_7$  is the seven-dimensional Sasaki-Einstein manifold that is the base of this cone, then these

CFTs are dual to the  $AdS_4 \times Y_7$  solution of eleven-dimensional supergravity with  $N$  units of seven-form flux threading  $Y_7$ . It can be shown that in this case [35]

$$F = N^{3/2} \sqrt{\frac{2\pi^6}{27 \text{Vol}(Y_7)}}, \quad (8.2.36)$$

to leading order at large  $N$ .

That in the theories on  $N$  coincident M2-branes the number of degrees of freedom scales as  $N^{3/2}$  at large  $N$  was first noticed by Klebanov and Tseytlin [36] in the computation of the thermal free energy. A field theory explanation of the  $N^{3/2}$  scaling of the  $F$ -coefficient was provided with the help of supersymmetric localization, as will be reviewed in the next section.

### 8.2.4 $F$ in supersymmetric theories

Besides free theories, the  $F$ -coefficient can also be computed exactly in superconformal field theories (SCFTs) that have Lagrangian descriptions, where one can use the technique of supersymmetric localization. The idea [37] of supersymmetric localization is as follows. In a supersymmetric theory, the value of a functional integral does not change if we add a term to the action that is  $Q$ -exact,  $Q$  being a supercharge under which the action is invariant. Moreover, if this  $Q$ -exact term has a positive-definite bosonic part, then adding it with a large coefficient allows for the evaluation of the functional integral in the saddle point approximation, which in this limit becomes exact. The saddles on which the functional integral localizes are those on which the  $Q$ -exact term vanishes. In favorable circumstances, as is the case of  $\mathcal{N} \geq 2$  theories on  $S^3$ , the localization locus is finite dimensional, so the partition function can be expressed as a finite dimensional integral.

Building on the work of [38], the technique of supersymmetric localization was first applied to three-dimensional SCFTs on  $S^3$  in [39]. Ref. [39] focused on the case of SCFTs with Lagrangian descriptions of the type constructed in [40, 41] whose Lagrangians are invariant under superconformal transformations. All theories of this type that preserve  $\mathcal{N} \geq 3$  supersymmetry have this property. These results were then further generalized to  $\mathcal{N} = 2$  SCFTs that are embedded as deep IR limits of RG flows triggered by relevant superpotential interactions [10]. As will be explained in the next section, in these  $\mathcal{N} = 2$  examples one also has to supplement the supersymmetric localization with the technique of  $F$ -maximization [10–12]. It is not currently known how to calculate the  $F$ -coefficient of SCFTs with only  $\mathcal{N} = 1$  supersymmetry using similar methods. In the remainder of this section, let us focus on  $\mathcal{N} \geq 3$  SCFTs with exactly marginal Lagrangians as in [40, 41], and defer the discussion of  $\mathcal{N} = 2$  SCFTs to Section 8.3.

The field content of these  $\mathcal{N} \geq 3$  SCFTs can be described in terms of vector multiplets and hypermultiplets. While we provide explicit Lagrangians in an  $\mathcal{N} = 2$  notation and more details of the supersymmetric localization computation in the next section, let us now simply state the results in the case of  $\mathcal{N} \geq 3$  SCFTs and provide a few examples. Let our  $\mathcal{N} = 3$  SCFT have gauge group  $G$ , written as a product of simple factors,  $G = G^1 \times G^2 \times \cdots \times G^n$ , and with the Chern-Simons level of each factor denoted by  $k_a$ . The matter content consists

of hypermultiplets  $\mathcal{H}_i$  transforming in representations  $R_i$  of the gauge group. For such a theory, it is explained in detail in Chapter 6 that upon using the technique of supersymmetric localization the partition function takes the form

$$Z = \frac{1}{|\mathcal{W}|} \int \prod_{\text{Cartan}} d\sigma \exp \left[ \frac{i}{4\pi} \text{tr}_k \sigma^2 \right] \frac{\det_{\text{Ad}} (2 \sinh(\pi\sigma))}{\prod_{\substack{\text{hypers} \\ \text{in rep } R_i}} \det_{R_i} (2 \cosh(\pi\sigma))}. \quad (8.2.37)$$

Here,  $\sigma$  is an element of the Lie algebra that lies along the Cartan subalgebra; in particular, it can be written as  $\sigma = \sigma_a h_a$ . The determinant of  $f(\sigma)$  in a representation  $R$  with weights  $w_a^i$ , with  $i$  ranging from 1 to the  $\dim R$ , is defined as

$$\det_R f(\sigma) \equiv \prod_i f(\sum_a \sigma_a w_a^i). \quad (8.2.38)$$

The determinant in the adjoint in the numerator of (8.2.37) is defined as (8.2.38) but without including the zero weights (i.e. the Cartan elements) in the product. Lastly,  $|\mathcal{W}|$  is the order of the Weyl group of the gauge group.

### Examples

As a first example, let us consider  $\mathcal{N} = 4$   $U(1)$  super-QED with  $N$  hypermultiplets of unit gauge charge.  $\mathcal{N} = 4$  supersymmetry requires  $k = 0$  in this case. From (8.2.37), we have [16]

$$Z = \frac{1}{2^N} \int_{-\infty}^{\infty} \frac{d\lambda}{\cosh^N(\pi\lambda)} = \frac{\Gamma\left(\frac{N}{2}\right)}{2^N \sqrt{\pi} \Gamma\left(\frac{N+1}{2}\right)}. \quad (8.2.39)$$

Extracting  $F = -\log|Z|$  and expanding it at large  $N$  we obtain

$$F = N \log 2 + \frac{1}{2} \log \left( \frac{N\pi}{2} \right) - \frac{1}{4N} + \frac{1}{24N^3} + \dots. \quad (8.2.40)$$

Quite nicely, this expression matches the first few terms of (8.2.24), as can be easily checked after noting that  $N$  hypermultiplets contain  $N_b = 4N$  real scalar fields and  $N_f = 2N$  Dirac fermions. In addition, when  $N = 1$ , (8.2.39) gives  $Z = \frac{1}{2}$ , or  $F = \log 2$ , which is the same value of  $F$  as for a free hypermultiplet—see (8.2.11). Indeed,  $\mathcal{N} = 4$  SQED with one charged hypermultiplet is known to be mirror dual to a free (twisted) hypermultiplet [43].

Another application of (8.2.37) is to SCFTs with holographic duals [14, 35, 44–46], where it provides a field theory explanation for the effective number of degrees of freedom of theories on coincident M2-branes mentioned in Section 8.2.3. One of the simplest such examples is that of  $N$  M2-brane placed at a  $\mathbb{C}^4/\mathbb{Z}_k$  singularity, where the space  $Y_7$  appearing in (8.2.36) is a freely acting  $\mathbb{Z}_k$  orbifold of the 7-sphere,  $Y_7 = S^7/\mathbb{Z}_k$ . The dual field theory is an  $\mathcal{N} = 6$  theory, which in  $\mathcal{N} = 3$  language is a  $U(N) \times U(N)$  gauge theory with Chern-Simons levels  $k$  and  $-k$  for the two gauge groups, and with matter given by two bi-fundamental

hypermultiplets [47].<sup>3</sup> Eq. (8.2.37) takes the form

$$Z = \frac{1}{(N!)^2} \int \left( \prod_{i=1}^N d\lambda_i d\tilde{\lambda}_i \right) \frac{\prod_{i<j} \left( 4 \sinh [\pi(\lambda_i - \lambda_j)] \sinh [\pi(\tilde{\lambda}_i - \tilde{\lambda}_j)] \right)^2}{\prod_{i,j} \left( 2 \cosh [\pi(\lambda_i - \tilde{\lambda}_j)] \right)^2} e^{i\pi k \sum_i (\lambda_i^2 - \tilde{\lambda}_i^2)}. \quad (8.2.41)$$

This integral can be solved through a variety of methods [35, 44, 46]. At large  $N$  and fixed  $k$ , it gives

$$F = \frac{\pi\sqrt{2}}{3} k^{1/2} N^{3/2} + O(N^{1/2}), \quad (8.2.42)$$

thus reproducing the supergravity expectation (8.2.36) after using  $\text{Vol}(S^7/\mathbb{Z}_k) = \pi^4/(3k)$ . (See also Chapter 7 for a calculation of  $F$  in a ‘t Hooft-like limit where  $N$  is taken to infinity while keeping  $N/k$  fixed.) This field theory calculation of  $F$  provides, in this example, a derivation of the  $N^{3/2}$  scaling behavior of the number of degrees of freedom on  $N$  coincident M2-branes without relying on the dual supergravity description. Various other generalizations to other 3-d theories with supergravity duals were considered in [11, 14, 35, 45, 49–57]. They are rather stringent tests of the corresponding holographic dualities.

### 8.3 $\mathcal{N} = 2$ SCFTs and $F$ -maximization

In generalizing the technique of supersymmetric localization to  $\mathcal{N} = 2$  SCFTs with Lagrangian descriptions one faces the following challenge. In flat space, most of these SCFTs are described as IR fixed points of non-trivial RG flows, and one simply cannot write down a Lagrangian for these IR fixed points that is superconformal, as was the case for the  $\mathcal{N} \geq 3$  SCFTs. Consequently, one cannot use the stereographic projection map to put a generic  $\mathcal{N} = 2$  SCFT on  $S^3$  directly, without having to rely on its definition as the IR limit of an RG trajectory. In general, mapping the RG trajectory from  $\mathbb{R}^3$  to  $S^3$  is ambiguous because there are many curvature couplings one can add in this process.

The ambiguities in mapping from  $\mathbb{R}^3$  to  $S^3$  can be fixed and one can generalize the technique of supersymmetric localization if the RG trajectory on  $\mathbb{R}^3$  preserves a  $U(1)$  R-symmetry. If flavor symmetries are also present throughout the RG trajectory, then this  $U(1)_R$  symmetry may not be unique, because any linear combination of a given  $U(1)$  R-symmetry and any of the  $U(1)$  flavor symmetries is also an R-symmetry.

For any choice of  $U(1)_R$  symmetry preserved by the RG flow, it is possible to map the RG flow from  $\mathbb{R}^3$  to  $S^3$  uniquely by requiring that the curvature couplings are such that the RG flow on  $S^3$  preserves an  $SU(2|1) \times SU(2)$  symmetry, whose bosonic part consists of the  $SO(4) = SU(2) \times SU(2)$  isometry group of  $S^3$  as well as the  $U(1)_R$  symmetry mentioned

---

<sup>3</sup>In  $\mathcal{N} = 4$  notation, the matter fields consist of a bi-fundamental hypermultiplet and a bi-fundamental twisted hypermultiplet. The distinction between hypermultiplets and twisted hypermultiplets is lost when restricting to  $\mathcal{N} = 3$  supersymmetry.

above. (There is only a discrete choice as to which  $SU(2)$  subgroup of  $SO(4)$  is part of  $SU(2|1)$ .) In the case of Chern-Simons matter theories, explicit Lagrangians invariant under  $SU(2|1) \times SU(2)$  were constructed in [10, 58], and a more systematic approach based on coupling the flat space theory to a background supergravity multiplet was developed in [12, 59, 60]. (See also Chapter 5.)

### 8.3.1 Non-conformal theories on $S^3$

To be concrete, let us briefly review the construction of these  $SU(2|1) \times SU(2)$  invariant actions on  $S^3$ .<sup>4</sup> (See also Chapter 6.) As mentioned above, there is a discrete choice in constructing such actions corresponding to which  $SU(2)$  subgroup of the  $SO(4) \cong SU(2)_L \times SU(2)_R$  isometry group of  $S^3$  is the one contained in  $SU(2|1)$ . This choice is manifested in which Killing spinors are chosen as supersymmetry transformation parameters. We choose to construct actions invariant under supersymmetry transformations with  $\epsilon, \tilde{\epsilon}$  obeying

$$\nabla_\mu \epsilon = \frac{i}{2a} \sigma_\mu \epsilon, \quad \nabla_\mu \tilde{\epsilon} = \frac{i}{2a} \sigma_\mu \tilde{\epsilon}, \quad (8.3.1)$$

where  $a$  is the radius of the sphere. These spinors are invariant under  $SU(2)_L$ , but transform under  $SU(2)_R$  as a doublet, provided that we work in a frame given by  $SU(2)_L$ -invariant one forms on  $S^3$ —see footnote 4. Therefore, if one chooses the transformation parameters to obey (8.3.1), the theories we will consider on  $S^3$  are invariant under  $SU(2|1)_R \times SU(2)_L$ , where  $SU(2)_R$  is contained in  $SU(2|1)_R$ . Similar actions can be obtained using  $SU(2)_R$ -invariant spinors by formally sending  $a \rightarrow -a$  in (8.3.1) and in all the formulas below.

Just as in the case of  $\mathcal{N} = 1$  supersymmetric theories in four dimensions, the explicit actions can be constructed from vector multiplets and chiral multiplets as follows. Let us write the gauge group as a product of simple factors,

$$G^1 \times G^2 \times \cdots \times G^n, \quad (8.3.2)$$

and denote the vector multiplet associated to each simple factor by  $\mathcal{V}^a = (A_\mu^a, \lambda^a, \sigma^a, D^a)$ ,  $a = 1, \dots, n$ , where  $A_\mu^a$  is a gauge field,  $\lambda^a$  is the gaugino, and  $\sigma^a$  and  $D^a$  are scalar fields, all transforming in the adjoint representation of  $G^a$ . A chiral multiplet  $\Phi^i = (Z^i, \chi^i, F^i)$ , with  $Z^i$  and  $F^i$  scalar fields and  $\chi^i$  a two-component spinor, can in general transform in any representation of the product gauge group (8.3.2). In Lorentzian signature  $A_\mu^a$ ,  $\sigma^a$ , and  $D^a$  would be real, while the other fields would be complex. Let us denote  $\tilde{\lambda}^a = i\sigma_2 \lambda^{a*}$ ,  $\tilde{\chi}^i = i\sigma_2 \chi^{i*}$ ,  $\tilde{Z}^i = Z^{i*}$ , and  $\tilde{F}^i = F^{i*}$ . In Euclidean signature, we should allow  $A_\mu^a$ ,  $\sigma^a$ , and  $D^a$  to be complex and thus formally treat the tilde'd fields as independent from the untilded'd ones.

<sup>4</sup>We use the notation in [62]. In particular, we take the Euclidean gamma matrices to be given by the Pauli matrices,  $\gamma^i = \sigma^i$ , where  $i$  is a frame index that is raised and lowered with the flat 3-d Euclidean metric. We use the frame  $e_\mu^i$  given by the left-invariant one-forms. In this frame the spacetime covariant derivative on a spinor  $\psi$  can be written as  $\nabla_\mu \psi = (\partial_\mu + \frac{i}{2} \gamma_\mu) \psi$ , where  $\gamma_\mu = \gamma_i e_\mu^i$ .

We would like to construct an action on  $S^3$  that is invariant under  $SU(2|1) \times SU(2)$ . The transformations of the fields under the fermionic part of this superalgebra, with independent supersymmetry parameters  $\epsilon$  and  $\tilde{\epsilon}$  obeying (8.3.1), can be realized on the fields as

$$\begin{aligned}
\delta A_\mu &= -\frac{i}{2}\epsilon^T(i\sigma_2)\sigma_\mu\tilde{\lambda} - \frac{i}{2}\tilde{\epsilon}^T(i\sigma_2)\sigma_\mu\lambda, \\
\delta\sigma &= -\frac{1}{2}\epsilon^T(i\sigma_2)\tilde{\lambda} + \frac{1}{2}\tilde{\epsilon}^T(i\sigma_2)\lambda, \\
\delta D &= -\frac{1}{2}\epsilon^T(i\sigma_2)\left(\sigma^\mu\nabla_\mu\tilde{\lambda} - \frac{i}{2a}\tilde{\lambda}\right) + \frac{1}{2}\tilde{\epsilon}^T(i\sigma_2)\left(\sigma^\mu\nabla_\mu\lambda - \frac{i}{2a}\lambda\right), \\
\delta\lambda &= \left(\frac{1}{2}\sigma^{\mu\nu}F_{\mu\nu} + i\sigma^\mu\partial_\mu\sigma + iD - \frac{1}{a}\sigma\right)\epsilon, \\
\delta\tilde{\lambda} &= \left(\frac{1}{2}\sigma^{\mu\nu}F_{\mu\nu} - i\sigma^\mu\partial_\mu\sigma - iD + \frac{1}{a}\sigma\right)\tilde{\epsilon}
\end{aligned} \tag{8.3.3}$$

for a vector multiplet, and

$$\begin{aligned}
\delta Z &= i\epsilon^T(i\sigma_2)\chi, \\
\delta\tilde{Z} &= i\tilde{\epsilon}^T(i\sigma_2)\tilde{\chi}, \\
\delta F &= \tilde{\epsilon}^T(i\sigma_2)\left(i\sigma^\mu\nabla_\mu\chi + i\left(\sigma - i\frac{r-1/2}{a}\right)\chi - \tilde{\lambda}Z\right), \\
\delta\tilde{F} &= \epsilon^T(i\sigma_2)\left(i\sigma^\mu\nabla_\mu\tilde{\chi} + i\left(\sigma - i\frac{r-1/2}{a}\right)\tilde{\chi} + \lambda\tilde{Z}\right), \\
\delta\chi &= F\epsilon + \left(\sigma^\mu\nabla_\mu Z - \sigma Z + \frac{ir}{a}Z\right)\tilde{\epsilon}, \\
\delta\tilde{\chi} &= \left(\sigma^\mu\nabla_\mu\tilde{Z} - \sigma\tilde{Z} + \frac{ir}{a}\tilde{Z}\right)\epsilon + \tilde{F}\tilde{\epsilon}
\end{aligned} \tag{8.3.4}$$

for a chiral multiplet. Indeed, in the  $a \rightarrow \infty$  limit, the supersymmetry transformations rules listed above are the usual ones from flat space. The  $1/a$  corrections are precisely what is needed in order to realize the commutation rules of the  $SU(2|1)$  algebra: writing the supersymmetry variations in terms of the supercharges,

$$\delta = i\epsilon^T(i\sigma_2)Q + i\tilde{\epsilon}^T(i\sigma_2)\tilde{Q}, \tag{8.3.5}$$

it is straightforward to check that (8.3.3)–(8.3.4) imply

$$\{Q, \tilde{Q}^T i\sigma_2\} = \sigma^\mu J_i + i\sigma + \frac{1}{a}R, \tag{8.3.6}$$

where  $J_i$  is an  $SU(2)_R$  isometry, and  $R$  is the R-charge. For a chiral multiplet  $(Z, \chi, F)$ , the R-charges are  $(r, r-1, r-2)$ . The anti-chiral multiplet  $(\tilde{Z}, \tilde{\chi}, \tilde{F})$  has opposite R-charges.

The total action on  $S^3$  preserving  $SU(2|1) \times SU(2)$ , with a given choice of  $U(1)_R$  R-symmetry contained in  $SU(2|1)$ , can be written as a sum of four terms:

$$S = S_{\text{CS}} + S_{\text{kin}} + S_{\text{superpot}} + S_{\text{top}}. \tag{8.3.7}$$

The first term corresponds to a possible Chern-Simons interaction term with level  $k^a$  for the gauge group factor  $G^a$ . To avoid clutter, let us write down the Chern-Simons term for a vector multiplet  $\mathcal{V} = (A_\mu, \lambda, \sigma, D)$  with level  $k$ , thus dropping the superscript  $a$ :

$$S_{\text{CS}}[\mathcal{V}; k] = \frac{ik}{4\pi} \int d^3x \text{tr} \left[ \epsilon^{\mu\nu\rho} \left( A_\mu \partial_\nu A_\rho - \frac{2i}{3} A_\mu [A_\nu, A_\rho] \right) - \sqrt{g} (\tilde{\lambda}^T (i\sigma_2) \lambda + 2i\sigma D) \right]. \quad (8.3.8)$$

This is simply the supersymmetrized version of the Chern-Simons term in (8.2.12). The second term in (8.3.7) includes the kinetic terms for the chiral multiplets. The kinetic term for a chiral multiplet  $\Phi = (Z, \chi, F)$  with  $U(1)_R$  charge  $r$  is

$$\begin{aligned} S_{\text{kin}}[\Phi, r] = & \int d^3x \sqrt{g} \text{tr} \left( \nabla^\mu \tilde{Z} \nabla_\mu Z + \tilde{Z} \left( \sigma - i \frac{r-1/2}{a} \right)^2 Z + i \tilde{\chi}^T (i\sigma_2) \sigma^\mu \nabla_\mu \chi \right. \\ & + i \tilde{\chi}^T (i\sigma_2) \left( \sigma - i \frac{r-1/2}{a} \right) \chi - \tilde{F} F \\ & \left. + \lambda^T (i\sigma_2) \tilde{Z} \chi + \tilde{\chi}^T (i\sigma_2) Z \tilde{\lambda} - \left( D - \frac{r-1/2}{a^2} \right) \tilde{Z} Z + \frac{3}{4a^2} \tilde{Z} Z \right). \end{aligned} \quad (8.3.9)$$

Here,  $\nabla_\mu$  includes the gauge covariant derivative, namely  $\nabla_\mu \chi = (\partial_\mu + \frac{i}{2} \gamma_\mu - i A_\mu) \chi$ ,  $\nabla_\mu Z = (\partial_\mu - i A_\mu) Z$ , etc. (See footnote 4 for our frame and gamma matrix conventions.) The total Chern-Simons and kinetic terms are

$$S_{\text{CS}} = \sum_{a=1}^n S_{\text{CS}}[\mathcal{V}^a; k_a], \quad S_{\text{kin}} = \sum_i S_{\text{kin}}[\Phi^i, r_i], \quad (8.3.10)$$

where the sum is over all chiral multiplets  $\Phi^i$  with R-charge  $r_i$ . These terms are invariant under (8.3.3)–(8.3.4) for any choices of  $r_i$ .

The third term in (8.3.7),  $S_{\text{superpot}}$ , corresponds to superpotential interactions and is given by

$$S_{\text{superpot}} = \int d^3x \sqrt{g} \left[ F^i W_i + \frac{1}{2} W_{ij} \chi^i \sigma_2 \chi^j + \tilde{F}^i \tilde{W}_i + \frac{1}{2} \tilde{W}_{ij} \tilde{\chi}^i \sigma_2 \tilde{\chi}^j \right], \quad (8.3.11)$$

where  $W = W(Z_i)$ ,  $\tilde{W} = \tilde{W}(\tilde{Z}_i)$ ,  $W_i = \frac{\partial W(Z_i)}{\partial Z^i}$ , etc. This term is invariant under (8.3.3)–(8.3.4) only if the superpotential satisfies

$$(r_i - 2) W_i + \sum_j r_j W_{ij} Z^j = 0. \quad (8.3.12)$$

This condition is obeyed if  $W$  is a sum of monomials in the  $Z^i$  with the property that the sum of the R-charges of each monomial equals two. It thus follows that the trial R-charges  $r_i$  are not arbitrary, but that they are constrained by the condition that the superpotential should have R-charge two.

It is worth noting that if one sends  $r_i \rightarrow r_i + i m_i a$  in the action above, the parameters  $m_i$  are nothing but “real masses” for the chiral multiplets. The  $S^3$  action is therefore holomorphic

in  $r_i + im_i$ , a property first noticed in [10] and later explained in [12]. The explanation of this holomorphy provided in [12] is that a change in  $r_i + im_i$  can be realized by coupling one of the conserved currents of the theory to a background vector multiplet, and then giving supersymmetry-preserving expectation values to the scalars in the background vector multiplet. See also Chapter 5. We will return to this point of view shortly.

The last term in (8.3.7) is more subtle, but can become important in a gauge theory where the gauge group has a  $U(1)$  or  $U(N)$  factor with no Chern-Simons interactions. (In other situations it may be ignored.) For every such factor, the contribution to the last term in (8.3.7) is an FI term

$$S_{\text{top}}[\mathcal{V}; r_{\text{top}}] = \frac{r_{\text{top}}}{2\pi a} \int d^3x \sqrt{g} \operatorname{tr} \left( iD + \frac{\sigma}{a} \right), \quad (8.3.13)$$

with parameter  $r_{\text{top}}$ ; the total term is

$$S_{\text{top}} = \sum_a S_{\text{top}}[\mathcal{V}; r_{\text{top}}^a]. \quad (8.3.14)$$

As written in (8.3.13), real coefficients  $r_{\text{top}}^a$  correspond to pure imaginary FI parameters. As we will now explain, the coefficients  $r_{\text{top}}^a$  are in some sense on the same footing as the R-charges  $r_i$  in (8.3.10) in that they are part of the definition of which  $U(1)_R$  symmetry was used to place the theory on  $S^3$ .

Indeed, for a  $U(1)$  or  $U(N)$  gauge group factor, one can construct the conserved current

$$j_{\text{top}}^\mu = \frac{1}{4\pi} \epsilon^{\mu\nu\rho} \operatorname{tr} F_{\nu\rho}, \quad (8.3.15)$$

usually referred to as a topological current because its conservation follows simply from the Bianchi identity obeyed by  $F_{\mu\nu}$ . No operators constructed as polynomials in the matter fields alone are charged under  $j_{\text{top}}^\mu$ . The only operators charged under  $j_{\text{top}}^\mu$  can be monopole operators [63, 64], which are defined through certain boundary conditions that the gauge field as well as the other fields in the  $\mathcal{N} = 2$  vector multiplet should satisfy close to the insertion point. These operators can only carry integer units of topological charge  $q_{\text{top}} = \int d^2x j_{\text{top}}^0 \in \mathbb{Z}$ . In a supersymmetric theory, these operators may carry R-charge as well as other flavor charges. For instance, a half-BPS monopole operators  $\mathcal{M}$  of charge  $q_{\text{top}}$  has R-charge

$$\gamma(|q_{\text{top}}|) + r_{\text{top}} q_{\text{top}} \quad (8.3.16)$$

where  $\gamma(|q_{\text{top}}|)$  can be computed at one-loop and depends only on the absolute value of  $q_{\text{top}}$  [65, 66], and  $r_{\text{top}}$  is the parameter in (8.3.13). Thus, in specifying the  $U(1)_R$  symmetry used to place a Chern-Simons matter theory on  $S^3$  requires specifying both the R-charges  $r_i$  of the chiral matter fields and the R-charge parameters  $r_{\text{top}}$  of the chiral monopole operators.

Just as if one sends  $r_i \rightarrow r_i + im_i a$  can introduce a real mass deformation of the  $S^3$  theory, sending  $r_{\text{top}} \rightarrow r_{\text{top}} + i\zeta$  introduces an FI parameter  $\zeta$ . The  $S^3$  partition function is thus holomorphic in  $r_{\text{top}} + i\zeta$ , as can be understood from the fact that  $r_{\text{top}} + i\zeta$  arises as the

expectation value of a background vector multiplet that couples to the conserved current multiplet that contains the topological current (8.3.15). See [12] and Chapter 5.

The explicit construction of  $SU(2|1) \times SU(2)$ -invariant theories on  $S^3$  presented above can be rephrased in a more abstract language [12, 59, 60]. Suppose we start with the non-conformal theory on  $\mathbb{R}^3$  that is believed to flow to our SCFT of interest in the IR—in other words, suppose we start with the flat space  $a \rightarrow \infty$  limit of (8.3.7) and try to deduce the various terms proportional to  $1/a$  and  $1/a^2$  in (8.3.3)–(8.3.13). We choose a  $U(1)_R$  symmetry preserved by this non-conformal theory in flat space. One can find a unique super-multiplet  $\mathcal{R}_\mu$  that contains the  $U(1)_R$  current, the stress-energy tensor, the supersymmetry current, a conserved current corresponding to the central charge of the supersymmetry algebra, and a string current. This multiplet can then be coupled to a background supergravity multiplet. The supergravity multiplet contains the metric  $g_{\mu\nu}$ , the gravitino, two Abelian gauge fields, and a two-form gauge field. The various terms proportional to  $1/a$  and  $1/a^2$  in (8.3.3)–(8.3.13) correspond to non-vanishing background values for the fields in the  $\mathcal{H}_\mu$  multiplet required in order to preserve supersymmetry. See [12, 59, 60] as well as Chapter 5 for more details.

### 8.3.2 Supersymmetric localization

The  $S^3$  partition function of Chern-Simons matter theories with the action (8.3.7) can be computed using supersymmetric localization [10, 58] building on the work of [39]. The idea is that

$$Z = \int e^{-S} = \int e^{-S_t}, \quad S_t \equiv S + t \int d^3x \sqrt{g} \{Q, P\}, \quad (8.3.17)$$

for some suitable operator  $P$  and supercharge  $Q$  such that the bosonic part of  $\{Q, P\}$  is positive definite. Taking  $t \rightarrow \infty$  in (8.3.17), one can evaluate this expression in the saddle point approximation by considering quadratic fluctuations around the configurations where  $\{Q, P\} = 0$ :

$$Z = e^{-S} \Big|_{\{Q, P\}=0} \times (\text{1-loop det}). \quad (8.3.18)$$

The choice

$$P = \{Q, \lambda\}^\dagger \lambda + \{Q, \chi\}^\dagger \chi + \tilde{\chi} \{Q, \tilde{\chi}\}^\dagger \quad (8.3.19)$$

obeys the properties mentioned above. Moreover,  $\{Q, P\} = 0$  implies that all the fields vanish except for  $\sigma^a$  and  $D^a$ , which are required to take constant values related by

$$\{Q, P\} = 0 \quad \implies \quad D^a = -\frac{i\sigma^a}{a}. \quad (8.3.20)$$

On this configuration, only the first and last terms in (8.3.7) have a non-zero contribution. For a vector multiplet  $\mathcal{V}$  with Chern-Simons level  $k$  and imaginary FI parameter  $r_{\text{loc}}$ , this

classical contribution is

$$S_{\text{classical}}[\mathcal{V}; k; r_{\text{top}}] = - \int d^3x \sqrt{g} \left[ \frac{ik}{2\pi a} \text{tr} \sigma^2 - \frac{r_{\text{top}}}{\pi a^2} \text{tr} \sigma \right] = -i\pi a^2 k \text{tr} \sigma^2 - 2\pi r_{\text{top}} a \text{tr} \sigma, \quad (8.3.21)$$

where we used the fact that the volume of a three-sphere of radius  $a$  is  $2\pi^2 a^3$ . We will set the radius of the sphere to  $a = 1$  from now on.

The computation of the one-loop determinants is tedious and performed in detail in Chapter 6. Here, we will only list the results. The one-loop determinant for a vector multiplet  $\mathcal{V}$  is

$$Z_{1\text{-loop}}[\mathcal{V}] = \det_{\text{Ad}}(2 \sinh(\pi\sigma)), \quad (8.3.22)$$

where the determinant in the adjoint representation is defined as in (8.2.38), but without including the zero weights in the product. For a chiral multiplet  $\Phi$  of R-charge  $r$  transforming in representation  $R$  of the gauge group, the one-loop determinant is

$$Z_{1\text{-loop}}[\Phi; r] = \det_R e^{\ell(1-r+i\sigma)}, \quad (8.3.23)$$

where the determinant in representation  $R$  was defined in (8.2.38), and the function  $\ell(z)$  is defined by  $\ell'(z) = -\pi z \cot \pi z$  and  $\ell(0) = 0$ . Explicitly,

$$\ell(z) = -z \log(1 - e^{2\pi iz}) + \frac{i}{2} \left( \pi z^2 + \frac{1}{\pi} \text{Li}_2(e^{2\pi iz}) \right) - \frac{i\pi}{12}. \quad (8.3.24)$$

Combining these expressions, we can write the partition function as [10]

$$Z = \frac{1}{|\mathcal{W}|} \int_{\text{Cartan}} d\sigma \prod_a \left[ e^{i\pi k_a \text{tr}(\sigma^a)^2 - 2\pi r_{\text{top}}^a \text{tr} \sigma^a} \det_{\text{Ad}}(2 \sinh(\pi\sigma^a)) \right] \prod_i \det_{R_i} e^{\ell(1-r_i+i\sigma)}. \quad (8.3.25)$$

Here  $|\mathcal{W}|$  is the order of the Weyl group of the gauge group.

### 8.3.3 $F$ -maximization

In Section 8.3.1 we started with a non-conformal theory on  $\mathbb{R}^3$  preserving a  $U(1)_R$  R-symmetry  $R$  and used this R-symmetry to couple this theory to curvature in a supersymmetric way. We wrote down an action on  $S^3$  preserving  $SU(2|1) \times SU(2)$  where  $U(1)_R$  appears in the  $SU(2|1)$  algebra. In Section 8.3.2 we explained how to evaluate the  $S^3$  partition function  $Z$  for this theory. We now discuss in more detail the freedom one has in this construction, and how one can determine the  $U(1)_R$  symmetry that is part of the superconformal algebra of the IR SCFT on  $\mathbb{R}^3$ .

As mentioned above, if in addition to a  $U(1)_R$  symmetry, the non-conformal theory on  $\mathbb{R}^3$  also preserves Abelian flavor symmetry, then there is no unique choice for the  $U(1)_R$  symmetry that can be used in the above construction. Indeed, if the  $U(1)_R$  current for some

(canonical) choice of the  $U(1)_R$  symmetry is  $j_\mu^{(R_0)}$ , and the Abelian flavor currents are  $j_\mu^I$ , where  $I = 1, \dots, F$ ,  $F$  being the number of flavor symmetries, then

$$j_\mu^R = j_\mu^{R_0} + \sum_{I=1}^F t_I j_\mu^I, \quad (8.3.26)$$

with arbitrary  $t_I$ , is also an R-symmetry current. The flavor currents  $j_\mu^I$  could be either acting on the matter fields or could be topological currents as in (8.3.15) or, more generally, they could be linear combinations of both types of terms. Eq. (8.3.26) represents a possible mixing of the R-symmetry with the Abelian flavor symmetries. For each choice of the  $t_I$  we can construct a different  $SU(2|1) \times SU(2)$ -invariant theory on  $S^3$ , and so the localization computation in Section 8.3.2 yields an  $S^3$  partition function  $Z(t_I)$  that depends on the  $t_I$ . Indeed, for a chiral multiplet  $\Phi_i$  we can consider R-charges

$$r_i = r_{i0} + \sum_{I=1}^F t_I q_i^I, \quad (8.3.27)$$

where  $q_i^I$  is the flavor charge of  $\Phi_i$  under the flavor symmetry generated by  $j_\mu^I$ . Upon substitution of (8.3.27) into (8.3.4), it can be seen that  $t_I q_i^I$  appears in the transformation rules precisely as an expectation value for the background vector multiplet  $\mathcal{V}_I^{\text{bg}}$  that couples to the conserved current multiplet that contains  $j_\mu^I$ . This expectation value is

$$A_{I\mu}^{\text{bg}} = \lambda_I^{\text{bg}} = 0, \quad \sigma_I^{\text{bg}} = -\frac{it_I}{a}, \quad D_I^{\text{bg}} = -\frac{t_I}{a^2}. \quad (8.3.28)$$

From the transformation rules of a vector multiplet (8.3.3), we see that the configuration (8.3.28) is supersymmetric. Similarly, for a monopole operator, we can consider the R-charge parameters  $r_{\text{top}}^a$  appearing in (8.3.14) to be

$$r_{\text{top}}^a = r_{\text{top}0}^a + \sum_{I=1}^F t_I q^{Ia}, \quad (8.3.29)$$

where  $q^{Ia}$  is the charge of the monopole operator under the flavor symmetry  $j_\mu^I$ . (For a monopole operator to be charged under  $j_\mu^I$ , it must be that  $j_\mu^I$  must contain a linear combination of topological symmetries.) The term (8.3.13) in the action is then precisely the coupling of the background vector multiplet in (8.3.28) to the conserved current multiplet containing the topological current.

Let us recall why we placed a non-conformal theory on  $S^3$  in the first place: we wanted to learn about the SCFT that sits in the deep IR of the RG flow on  $\mathbb{R}^3$ . This SCFT is invariant under an unambiguous  $U(1)_R$  symmetry that appears in the superconformal algebra. Thus the superconformal  $U(1)_R$  symmetry must correspond to a specific value  $t_I = t_{I*}$  of the parameters  $t_I$  appearing in (8.3.26). The statement of  $F$ -maximization is that the function

$$F(t_I) \equiv -\log|Z(t_I)| = -\text{Re} \log Z(t_I) \quad (8.3.30)$$

is locally maximized at  $t_I = t_{I^*}$ .<sup>5</sup>  $F$ -maximization is thus a procedure for determining the R-symmetry that appears in the superconformal algebra in cases where mixing with Abelian flavor symmetries is possible.

Showing that (8.3.30) is maximized at  $t_I = t_{I^*}$  requires a careful analysis of contact terms and various relations required by supersymmetry. Intuitively, from (8.3.28), we see that taking derivatives of  $Z(t_I)$  with respect to  $t_I$  corresponds to insertions of the integrated operator in the supermultiplet containing  $j_\mu^I$  that couples to  $t_I$  via (8.3.28). Thus, derivatives of  $Z(t_I)$  evaluated at  $t_I = t_{I^*}$  can be expressed in terms of integrated correlation functions of operators in the conserved current multiplet in the SCFT, which are all parameterized by just a few numbers. In particular, the first derivative  $\partial F/\partial t_I$  should vanish when  $t_I = t_{I^*}$  because it equals an integrated one-point function in a CFT. The second derivative of  $\partial^2 F/\partial t_I \partial t_J$  equals an integrated two-point function, which in a unitary CFT it must have certain positivity properties. These positivity properties lead to the conclusion that  $F$  has a local maximum at  $t_I = t_{I^*}$ .

To be more precise, at the SCFT fixed point, the correlation functions of the canonically normalized flavor currents and R-symmetry current take the form

$$\begin{aligned} \langle j_I^\mu(x) j_J^\nu(0) \rangle &= \frac{\tau_{IJ}}{16\pi^2} (\delta^{\mu\nu} \partial^2 - \partial^\mu \partial^\nu) \frac{1}{x^2} + \frac{i\kappa_{IJ}}{2\pi} \epsilon^{\mu\nu\rho} \partial_\rho \delta^{(3)}(x), \\ \langle j_R^\mu(x) j_R^\nu(0) \rangle &= \frac{\tau_{RR}}{16\pi^2} (\delta^{\mu\nu} \partial^2 - \partial^\mu \partial^\nu) \frac{1}{x^2} + \frac{i\kappa_{RR}}{2\pi} \epsilon^{\mu\nu\rho} \partial_\rho \delta^{(3)}(x), \\ \langle j_I^\mu(x) j_R^\nu(0) \rangle &= \frac{i\kappa_{IR}}{2\pi} \epsilon^{\mu\nu\rho} \partial_\rho \delta^{(3)}(x), \end{aligned} \quad (8.3.31)$$

where  $\tau_{IJ}$  and  $\tau_{RR}$  are universal real constants that are positive by unitarity, while the contact terms proportional to the real coefficients  $\kappa_{IJ}$ ,  $\kappa_{IR}$  and  $\kappa_{RR}$  can in general depend on the precise UV completion of the theory. By relating the correlation functions of other operators in the flavor current and  $\mathcal{R}_\mu$  multiplets to (8.3.31), one can show that [12]

$$-\log Z(t_I) = -\log Z(t_{I^*}) + i2\pi\kappa_{IR}(t_I - t_{I^*}) - \frac{1}{2} \left( \frac{\pi^2}{2} \tau_{IJ} - 2\pi i\kappa_{IJ} \right) (t_I - t_{I^*})(t_J - t_{J^*}) + \dots \quad (8.3.32)$$

Recalling that we defined  $F = -\log|Z| = -\text{Re} \log Z$ , we can infer from (8.3.32) that

$$\left. \frac{\partial F}{\partial t_I} \right|_{t=t^*} = 0, \quad \left. \frac{\partial^2 F}{\partial t_I \partial t_J} \right|_{t=t^*} = -\frac{\pi^2}{2} \tau_{IJ}. \quad (8.3.33)$$

Unitarity requires  $\tau_{IJ} > 0$ , and so (8.3.33) provides a proof of the  $F$ -maximization principle.

---

<sup>5</sup>If one constructs Chern-Simons matter theories as in Section 8.3.1, with R-charge  $r_i$  for each chiral multiplet and R-charge parameters  $r_{\text{top}}^a$  for each Abelian gauge group factor, then the  $S^3$  partition function will have flat directions. The number of flat directions is given by the number of Abelian gauge group factors. They correspond to shifting the R-charges by any multiple of the gauge charge. (For more details, see Section 2.3 of [11].) Consequently,  $F$  depends only on the R-charges of gauge invariant operators, and  $F$ -maximization should be performed modulo these flat directions.

It is worth emphasizing that, as described above, the function  $F(t_I)$  carries useful information about the SCFT even away from  $t_I = t_{I^*}$ . In particular, one can extract the two-point function coefficients  $\tau_{IJ}$  from the second derivative of  $F$  [12]:

$$\tau_{IJ} = -\frac{2}{\pi^2} \left. \frac{\partial^2 F}{\partial t_I \partial t_J} \right|_{t=t_*}. \quad (8.3.34)$$

Such a relation currently provides the only way of calculating the value of  $\tau_{IJ}$  in strongly-coupled SCFTs and has been used, for instance, as a key input in the 3-d supersymmetric conformal bootstrap analysis of various  $\mathcal{N} = 2$  SCFTs [67–71].

Note that  $F$ -maximization implies that in the case where there are no accidental symmetries at the IR fixed point, the  $F$ -coefficient does decrease under supersymmetric RG flows triggered by superpotential deformations [12]. Indeed, at the UV fixed point, where one should neglect the superpotential, there are more flavor symmetries that can mix with the R-symmetry, so  $F$ -maximization has to be performed over a larger set of trial R-charges than in the presence of the superpotential. Consequently,  $F_{\text{UV}} > F_{\text{IR}}$  in these examples.

### 8.3.4 Examples

#### $\mathcal{N} = 2$ super-Ising CFT and Wess-Zumino models

Perhaps the simplest example of an  $\mathcal{N} = 2$  SCFT where one can use the methods described above to compute its  $F$  coefficient is the critical  $\mathcal{N} = 2$  super-Ising model. It can be described in terms of a single chiral multiplet  $\Phi = (Z, \chi, F)$  with a cubic superpotential interaction  $W = g\Phi^3$ ,  $g$  being a dimensionful coupling constant. This non-conformal theory is believed to flow in the infrared to an  $\mathcal{N} = 2$  SCFT—the  $\mathcal{N} = 2$  super-Ising CFT. The superpotential does not preserve any flavor symmetries. The only R-symmetry is that under which  $\Phi$  has R-charge  $r = 1/3$ . The  $F$ -coefficient of this theory can be read off from (8.3.25) to be

$$F_{\mathcal{N} = 2 \text{ Ising}} = -\ell(2/3) \approx 0.259. \quad (8.3.35)$$

This value is smaller than that of a free chiral multiplet  $F_{\text{chiral}} \approx 0.347$  (see (8.2.11)), which is the UV CFT fixed point of the RG flow  $W = g\Phi^3$ .

The  $\mathcal{N} = 2$  super-Ising CFT is one of many Wess-Zumino models [72] that are believed to flow to interacting SCFTs in the infrared. (For a review, see [73].) For instance, one can construct supersymmetric generalization of the critical  $O(N)$  vector model by considering  $N + 1$  chiral multiplets  $\Phi_i = (Z_i, \chi_i, F_i)$  with the  $O(N)$ -invariant cubic superpotential

$$W = g \Phi_{N+1} \sum_{i=1}^N \Phi_i^2. \quad (8.3.36)$$

These models have been studied in the  $1/N$  expansion [74], the  $4 - \epsilon$  expansion [75–78], and more recently using supersymmetric localization [31, 79] and the conformal bootstrap [67, 68].<sup>6</sup>

---

<sup>6</sup>These models provide a counterexample to a possible conjecture stating that the coefficient  $c_T$  appearing in the two-point function of the canonically normalized stress tensor decreases along RG flow [79].

| $N$                                | 1    | 2    | 3    | 4    | 5    | 6    | 7    | 8    | 9    | 10   |
|------------------------------------|------|------|------|------|------|------|------|------|------|------|
| $r_i = r$ (for $i = 1, \dots, N$ ) | .708 | .667 | .632 | .605 | .586 | .572 | .562 | .554 | .548 | .543 |
| $r_{N+1} = 2 - 2r$                 | .584 | .667 | .737 | .790 | .828 | .856 | .876 | .892 | .904 | .914 |

Table 8.1: The superconformal R-charges  $r_i$  at the IR fixed point of (8.3.36).

The RG flow triggered by (8.3.36) preserves a  $U(1)_R$  symmetry as well as an  $O(N) \times U(1)$  flavor symmetry. Under the  $O(N)$  symmetry, the  $\Phi_i$  transform as a vector and  $\Phi_{N+1}$  is a singlet, while under the flavor  $U(1)$   $\Phi_i$  has charge  $+1$  for  $i = 1, \dots, N$  and charge  $-2$  for  $i = N + 1$ . Since there is one Abelian flavor symmetry, there is a one-parameter family of R-charge assignments consistent with the  $O(N)$ -invariance of the theory and with the fact that the superpotential has R-charge two:

$$\begin{aligned} r_i &= r, & \text{for } i = 1, \dots, N, \\ r_{N+1} &= 2 - 2r. \end{aligned} \tag{8.3.37}$$

Using (8.3.25), one finds

$$F = -N\ell(1 - r) - \ell(2r - 1). \tag{8.3.38}$$

The  $F$ -maximization principle states that one should maximize (8.3.38) with respect to  $r$  in order to find the value of  $r$  attained at the SCFT fixed point. Doing so, one obtains the values of  $r$  given in Table 8.1. Since the multiplets  $\Phi_i = (Z_i, \chi_i, F_i)$  are chiral, the values of  $r$  given in Table 8.1 also determine the scaling dimensions of  $Z_i$  and  $\chi_i$  to be  $\Delta_{Z_i} = r_i$  and  $\Delta_{\chi_i} = r_i + \frac{1}{2}$ , respectively.

In the case  $N = 2$ , one can make the redefinitions  $X = \Phi_3$ ,  $Y = \Phi_1 + i\Phi_2$ , and  $Z = \Phi_1 - i\Phi_2$  and rewrite the superpotential (8.3.36) as  $W = gXYZ$ . This theory is the “XYZ model.” It is invariant under permuting  $X$ ,  $Y$ , and  $Z$ , and consequently at the IR fixed point one expects the R-charges of  $X$ ,  $Y$ , and  $Z$  to be equal. Since these charges must add up to two, we must have  $r_X = r_Y = r_Z = 2/3$ . Indeed, one can check that when  $N = 2$ , (8.3.38) is maximized when  $r = 2/3$ .

Wess-Zumino models of the same type as above also provide an example that emphasizes the limitation of the  $F$ -maximization principle of not incorporating accidental symmetries. When using  $F$ -maximization, one assumes that the RG flow ends at an SCFT where no accidental symmetries are present. This assumption may of course be wrong. For instance, one can show that the assumption of no accidental symmetries is indeed incorrect in the following generalization of (8.3.36):

$$W = g_1 \Phi_{N+1} \sum_{i=1}^N \Phi_i^2 + g_2 \Phi_{N+1}^3, \tag{8.3.39}$$

where  $g_1$  and  $g_2$  are coupling constants. The RG flow triggered by (8.3.39) preserves an  $O(N) \times \mathbb{Z}_3$  flavor symmetry and a unique  $U(1)_R$  symmetry under which all the  $\Phi_i$  have

R-charge  $2/3$ . It is tempting to assume that the IR limit of (8.3.39) is a unitary SCFT where all the  $\Phi_i$  have R-charge  $2/3$ , but this assumption was recently proven to be incorrect if  $N > 2$  using the conformal bootstrap [67]. Based on arguments coming from the  $4 - \epsilon$  expansion, what is believed to happen in the model (8.3.39) when  $N > 2$  is that the coupling  $g_2$  flows to zero in the IR, the flavor symmetry thus being enhanced to  $O(N) \times U(1)$ . The IR fixed point of (8.3.39) is then believed to be the same as that of (8.3.36).

### $\mathcal{N} = 2$ SQED and a test of dualities

As another example, one can consider  $\mathcal{N} = 2$  supersymmetric quantum electrodynamics with  $N$  pairs of conjugate flavors that we denote by  $\Phi_i$  (of gauge charge  $+1$ ) and  $\tilde{\Phi}_i$  (of gauge charge  $-1$ ), with  $i = 1, \dots, N$ , and vanishing superpotential. One can also add a Chern-Simons term with level  $k$  for the  $U(1)$  vector multiplet. This theory has the following flavor symmetries: a  $U(1)$  flavor symmetry under which both  $\Phi_i$  and  $\tilde{\Phi}_i$  have the same charge; an  $SU(N)$  symmetry under which the  $\Phi_i$  transform as a fundamental and  $\tilde{\Phi}_i$  as an anti-fundamental; a topological  $U(1)$  symmetry generated by  $*F$ ; as well as a charge conjugation symmetry that flips the sign of the fields in the vector multiplet and interchanges  $\Phi_i$  with  $\tilde{\Phi}_i$ . If we want to preserve the  $SU(N)$  symmetry and the charge conjugation symmetry, then the R-symmetry can only mix with the flavor  $U(1)$  under which  $\Phi_i$  and  $\tilde{\Phi}_i$  have the same charge. Thus, one can consider a family of R-charge assignments

$$r_{\Phi_i} = r_{\tilde{\Phi}_i} = r \quad (8.3.40)$$

parameterized by  $r$ . The  $S^3$  partition function is<sup>7</sup>

$$Z(r) = \int_{-\infty}^{\infty} d\sigma e^{i\pi k \sigma^2} e^{N(\ell(1-r+i\sigma)+\ell(1-r-i\sigma))}. \quad (8.3.41)$$

It is straightforward to calculate numerically this integral and maximize  $F = -\log|Z|$  with respect to  $r$ . One can also develop an analytical approximation in the regime where  $N$  and  $k$  are both taken to be large, with the ratio  $\kappa = 2k/(N\pi)$  fixed. One finds the value of  $r$  that maximizes  $F$  to be [16]

$$r = \frac{1}{2} - \frac{2}{\pi^2(1+\kappa^2)} \frac{1}{N} - \frac{2[\pi^2 - 12 + \kappa^2(4 - 2\pi^2) + \pi^2\kappa^4]}{\pi^4(1+\kappa^2)^3} \frac{1}{N^2} + O(N^{-3}). \quad (8.3.42)$$

The corresponding  $F$ -coefficient is

$$F = N \log 2 + \frac{1}{2} \log \left( \frac{N\pi}{2} \sqrt{1+\kappa^2} \right) + \left( \frac{\kappa^2 - 1}{4(1+\kappa^2)^2} + \frac{2}{\pi^2(1+\kappa^2)^2} \right) \frac{1}{N} + O(N^{-2}). \quad (8.3.43)$$

It can be checked that the analytical approximation (8.3.42)–(8.3.43) matches quite well the numerical results even at fairly small values of  $N$ . It also matches the large  $N$  expansion in (8.2.24), if one identifies  $N_b = N_f = 2N$ . See [16] for more details.

---

<sup>7</sup>We set  $r_{\text{top}} = 0$ , thus assigning the monopole operators with topological charge  $+q_{\text{top}}$  and  $-q_{\text{top}}$  equal R-charges. Such an assignment is consistent with the charge conjugation symmetry. When  $k \neq 0$ , this assignment can also be thought of as fixing the flat direction mentioned in Footnote 5.

An interesting particular case is SQED with only one pair of conjugate chiral multiplets of unit gauge charge and no Chern-Simons interactions, namely  $k = 0$  and  $N = 1$ , where it can be checked numerically that the value of  $r$  that maximizes  $F$  is  $r = 1/3$ . Indeed, in this case the  $S^3$  partition function can be written as [10]

$$Z(r) = \int_{-\infty}^{\infty} d\sigma e^{\ell(1-r+i\sigma)+\ell(1-r-i\sigma)} = e^{2\ell(r)+\ell(1-2r)}, \quad (8.3.44)$$

where the last equality can be checked numerically, for instance. This is nothing but the  $S^3$  partition function of the  $XYZ$  model (see the discussion following (8.3.25)) with R-charge assignments  $r_X = 2r$ ,  $r_Y = 1 - r$ ,  $r_Z = 1 - r$ . Indeed, the SQED with 1 pair of conjugate chirals is known to be dual to the  $XYZ$  model [80]. That  $F$  is maximized when  $r = 1/3$  is consistent with the fact that in the  $XYZ$  model  $F$  is maximized for the symmetric R-charge assignment  $r_X = r_Y = r_Z = 2/3$ . The expression (8.3.44) is not just a check of the duality between the  $XYZ$  model and SQED, but it also provides some insight into how the duality works. In particular, the chiral field  $X$  is dual to an operator of R-charge  $2r$  (this is  $\tilde{Q}Q$ ), while  $Y$  and  $Z$  are dual to operators of R-charge  $1 - r$  (these are monopole operators). Other tests of dualities using the  $S^3$  partition function were performed, for example, in [81–90].

### Examples in holography

The  $\mathcal{N} = 2$  SCFTs with holographic duals provide a richer set of examples in which one can calculate  $F$  via supersymmetric localization and compare it to the supergravity expectation. For instance, there are many SCFTs that are conjectured to be dual to M-theory backgrounds of the form  $AdS_4 \times Y_7$ , where  $Y_7$  is a Sasaki-Einstein space, realized by placing  $N$  coincident M2-branes at tip of the Calabi-Yau cone over  $Y_7$ . In these instances, supergravity predicts that the  $F$ -coefficient is given by (8.2.36). There have been many field theory computations of  $F$  in  $\mathcal{N} = 2$  SCFTs that match this supergravity result. See, for example, [11, 49, 51, 84, 91–93].

Moving away from SCFTs, one may wonder whether it is possible to calculate the  $S^3$  in supergravity and reproduce from a holographic computation the entire function of the trial R-charges, even before performing  $F$ -maximization in the field theory. This question was studied in [62] in the context of ABJM theory [47]. ABJM theory is a  $U(N)_k \times U(N)_{-k}$  Chern-Simons-matter theory that in general preserves  $\mathcal{N} = 6$  supersymmetry that is believed to be enhanced to  $\mathcal{N} = 8$  when  $k = 1$  or  $2$ . In  $\mathcal{N} = 2$  notation, the field content of ABJM theory consists of two  $U(N)$  vector multiplets with Chern-Simons interactions  $k$  and  $-k$ , with matter content consisting of two chiral multiplets  $\mathcal{Z}_i$ ,  $i = 1, 2$  transforming as a bifundamental of  $U(N) \times U(N)$  and two chiral multiplets  $\mathcal{W}_i$ ,  $i = 1, 2$ , transforming in the conjugate representation. The superpotential is of the form

$$W \propto \epsilon^{ik} \epsilon^{jl} \text{tr} [\mathcal{W}_i \mathcal{Z}_j \mathcal{W}_k \mathcal{Z}_l], \quad (8.3.45)$$

with a precise coefficient fixed by the extended supersymmetry of the theory. The extended supersymmetry also fixes the R-charges of the chiral operators to  $r_{\mathcal{W}_i} = r_{\mathcal{Z}_i} = 1/2$ , so there

is no need to perform  $F$ -maximization in this case. However, one can nevertheless consider a 3-parameter family of trial R-charges given by arbitrary  $r_{\mathcal{W}_i}$  and  $r_{\mathcal{Z}_i}$  with the constraint

$$r_{\mathcal{W}_1} + r_{\mathcal{W}_2} + r_{\mathcal{Z}_1} + r_{\mathcal{Z}_2} = 2 \tag{8.3.46}$$

that ensures that the superpotential has R-charge 2.<sup>8</sup> This R-charge assignment preserves only  $\mathcal{N} = 2$  supersymmetry. Using (8.3.25) and the matrix model technique developed in [35] one can show that at large  $N$  the  $S^3$  free energy takes the form [11]

$$F = \frac{\sqrt{2}\pi k^{1/2} N^{3/2}}{3} 4\sqrt{r_{\mathcal{W}_1} r_{\mathcal{W}_2} r_{\mathcal{Z}_1} r_{\mathcal{Z}_2}} + O(N^{1/2}). \tag{8.3.47}$$

This expression agrees with (8.2.42) when  $r_{\mathcal{W}_i} = r_{\mathcal{Z}_i} = 1/2$ .

In the case  $k = 1$ , the 3-parameter R-charge deformations mentioned above are dual to holographic RG flows that asymptote to  $\mathbb{H}^4 \times S^7$  in the UV. These flows were constructed in [62] in a 4-d model that can be uplifted to a background of 11-d supergravity. This model involves Einstein gravity coupled to three complex scalar fields, each of which corresponds to one of the three parameters in the family of R-charge assignments. Upon a careful use of holographic renormalization and supersymmetry, Ref. [62] obtained a perfect match of the 4-d on-shell supergravity action with (8.3.47).<sup>9</sup>

## 8.4 Conclusion

In this contribution I reviewed some of the recent developments related to the  $S^3$  free energy of various supersymmetric and non-supersymmetric CFTs in three dimensions, in particular the  $F$ -theorem and the  $F$ -maximization principle and some of their applications. In Section 8.2 I have shown how the  $F$ -coefficient can be computed in various approximation schemes, and how these results are consistent with the  $F$ -theorem in several examples. In Section 8.3 I explained how  $F$  can be computed exactly in SCFTs with  $\mathcal{N} \geq 2$  supersymmetry, and as a byproduct how one can determine the R-charges (or scaling dimensions) of the various chiral operators of these SCFTs by maximizing the  $F$  over a set of trial R-charges, both in general and in a few examples.

The irreversibility of the RG trajectories that is required by the  $F$ -theorem is a fundamental property of relativistic quantum field theory in three dimensions. An interesting open problem remains to prove the  $F$ -theorem in a way that uses directly the properties of the  $S^3$  partition function, without appealing to the notion of entanglement entropy. Perhaps a related future direction would be to construct a function that interpolates between  $F_{UV}$  and  $F_{IR}$  monotonically along any RG trajectory and that is stationary at the UV and IR fixed points. The proof of the  $F$ -theorem using entanglement entropy [19, 21] that I did not review here does

---

<sup>8</sup>We may  $r_{\text{top}}^a = 0$  as a choice in order to fix the flat directions mentioned in Footnote 5. These parameters were included in the analysis performed in [11].

<sup>9</sup>See also [94–102] for other constructions of supergravity backgrounds dual to deformations of supersymmetric field theories on curved manifolds.

provide a strictly monotonic interpolating function, namely the renormalized entanglement entropy proposed in [20], but this function may or may not be stationary at the UV and IR fixed points [103, 104]. Lastly, it would be interesting to investigate whether there exists an analog of the  $F$ -theorem in a larger odd number of spacetime dimensions. For instance, in five dimensions there are a few examples of RG trajectories between pairs of CFTs that obey a conjectured  $F$ -theorem [105, 106], but there is no general proof of such a result.

## Acknowledgments

I am particularly grateful to Shai Chester, Dan Freedman, Simone Giombi, Dan Gulotta, Chris Herzog, Luca Iliesiu, Daniel Jafferis, Igor Klebanov, Jaehoon Lee, Tatsuma Nishioka, Subir Sachdev, Ben Safdi, Grisha Tarnopolsky, Tibi Tesileanu, and Ran Yacoby for collaboration on the various projects mentioned or reviewed here. This work was supported in part by the US NSF under Grant No. PHY-1418069.

## References

- [1] V. Pestun and M. Zabzine, eds., *Localization techniques in quantum field theory*, vol. xx. Journal of Physics A, 2016. 1608.02952. <https://arxiv.org/src/1608.02952/anc/LocQFT.pdf>, <http://pestun.ihep.fr/pages/LocalizationReview/LocQFT.pdf>.
- [2] R. Jackiw and S. Y. Pi, “Tutorial on Scale and Conformal Symmetries in Diverse Dimensions,” *J. Phys.* **A44** (2011) 223001, [arXiv:1101.4886](https://arxiv.org/abs/1101.4886) [math-ph].
- [3] A. Dymarsky, Z. Komargodski, A. Schwimmer, and S. Theisen, “On Scale and Conformal Invariance in Four Dimensions,” [arXiv:1309.2921](https://arxiv.org/abs/1309.2921) [hep-th].
- [4] A. Dymarsky, K. Farnsworth, Z. Komargodski, M. A. Luty, and V. Prilepina, “Scale Invariance, Conformality, and Generalized Free Fields,” [arXiv:1402.6322](https://arxiv.org/abs/1402.6322) [hep-th].
- [5] A. Zamolodchikov, “Irreversibility of the Flux of the Renormalization Group in a 2D Field Theory,” *JETP Lett.* **43** (1986) 730–732.
- [6] J. L. Cardy, “Is There a c Theorem in Four-Dimensions?,” *Phys.Lett.* **B215** (1988) 749–752.
- [7] Z. Komargodski and A. Schwimmer, “On Renormalization Group Flows in Four Dimensions,” *JHEP* **1112** (2011) 099, [arXiv:1107.3987](https://arxiv.org/abs/1107.3987) [hep-th].
- [8] I. Affleck and A. W. W. Ludwig, “Exact conformal-field-theory results on the multichannel Kondo effect: Single-fermion Green’s function, self-energy, and resistivity,” *Phys. Rev.* **B48** (1993) no. 10, 7297.
- [9] I. Affleck and A. W. W. Ludwig, “Universal noninteger ‘ground state degeneracy’ in critical quantum systems,” *Phys. Rev. Lett.* **67** (1991) 161–164.
- [10] D. L. Jafferis, “The Exact Superconformal R-Symmetry Extremizes  $Z$ ,” *JHEP* **1205** (2012) 159, [arXiv:1012.3210](https://arxiv.org/abs/1012.3210) [hep-th].
- [11] D. L. Jafferis, I. R. Klebanov, S. S. Pufu, and B. R. Safdi, “Towards the F-Theorem:  $\mathcal{N} = 2$  Field Theories on the Three-Sphere,” *JHEP* **1106** (2011) 102, [arXiv:1103.1181](https://arxiv.org/abs/1103.1181) [hep-th].

- [12] C. Closset, T. T. Dumitrescu, G. Festuccia, Z. Komargodski, and N. Seiberg, “Contact Terms, Unitarity, and F-Maximization in Three-Dimensional Superconformal Theories,” *JHEP* **1210** (2012) 053, [arXiv:1205.4142 \[hep-th\]](#).
- [13] K. A. Intriligator and B. Wecht, “The Exact superconformal R symmetry maximizes a,” *Nucl.Phys.* **B667** (2003) 183–200, [arXiv:hep-th/0304128 \[hep-th\]](#).
- [14] D. R. Gulotta, C. P. Herzog, and S. S. Pufu, “From Necklace Quivers to the F-theorem, Operator Counting, and T(U(N)),” *JHEP* **1112** (2011) 077, [arXiv:1105.2817 \[hep-th\]](#).
- [15] I. R. Klebanov, S. S. Pufu, and B. R. Safdi, “F-Theorem without Supersymmetry,” *JHEP* **1110** (2011) 038, [arXiv:1105.4598 \[hep-th\]](#).
- [16] I. R. Klebanov, S. S. Pufu, S. Sachdev, and B. R. Safdi, “Entanglement Entropy of 3-d Conformal Gauge Theories with Many Flavors,” *JHEP* **1205** (2012) 036, [arXiv:1112.5342 \[hep-th\]](#).
- [17] R. C. Myers and A. Sinha, “Seeing a c-theorem with holography,” *Phys.Rev.* **D82** (2010) 046006, [arXiv:1006.1263 \[hep-th\]](#).
- [18] R. C. Myers and A. Sinha, “Holographic c-theorems in arbitrary dimensions,” *JHEP* **1101** (2011) 125, [arXiv:1011.5819 \[hep-th\]](#).
- [19] H. Casini, M. Huerta, and R. C. Myers, “Towards a derivation of holographic entanglement entropy,” *JHEP* **1105** (2011) 036, [arXiv:1102.0440 \[hep-th\]](#).
- [20] H. Liu and M. Mezei, “A Refinement of entanglement entropy and the number of degrees of freedom,” *JHEP* **1304** (2013) 162, [arXiv:1202.2070 \[hep-th\]](#).
- [21] H. Casini and M. Huerta, “On the RG running of the entanglement entropy of a circle,” *Phys.Rev.* **D85** (2012) 125016, [arXiv:1202.5650 \[hep-th\]](#).
- [22] H. Casini and M. Huerta, “A c-theorem for the entanglement entropy,” *J. Phys.* **A40** (2007) 7031–7036, [arXiv:cond-mat/0610375 \[cond-mat\]](#).
- [23] J. R. Quine and J. Choi, “Zeta regularized products and functional determinants on spheres,” *Rocky Mountain J. Math.* **26** (1996) no. 2, 719–729.
- [24] H. Kumagai, “The determinant of the Laplacian on the  $n$ -sphere,” *Acta Arith.* **91** (1999) no. 3, 199–208.
- [25] M. Marino, “Lectures on localization and matrix models in supersymmetric Chern-Simons-matter theories,” *J.Phys.A* **A44** (2011) 463001, [arXiv:1104.0783 \[hep-th\]](#).
- [26] E. Witten, “Quantum Field Theory and the Jones Polynomial,” *Commun. Math. Phys.* **121** (1989) 351–399.
- [27] C. A. Agon, M. Headrick, D. L. Jafferis, and S. Kasko, “Disk entanglement entropy for a Maxwell field,” *Phys. Rev.* **D89** (2014) no. 2, 025018, [arXiv:1310.4886 \[hep-th\]](#).
- [28] S. Giombi, I. R. Klebanov, S. S. Pufu, B. R. Safdi, and G. Tarnopolsky, “AdS Description of Induced Higher-Spin Gauge Theory,” *JHEP* **1310** (2013) 016, [arXiv:1306.5242 \[hep-th\]](#).
- [29] K. G. Wilson and M. E. Fisher, “Critical exponents in 3.99 dimensions,” *Phys. Rev. Lett.* **28** (1972) 240–243.
- [30] K. G. Wilson and J. B. Kogut, “The Renormalization group and the epsilon expansion,” *Phys. Rept.* **12** (1974) 75–200.
- [31] S. Giombi and I. R. Klebanov, “Interpolating between  $a$  and  $F$ ,” *JHEP* **03** (2015) 117, [arXiv:1409.1937 \[hep-th\]](#).

- [32] L. Fei, S. Giombi, I. R. Klebanov, and G. Tarnopolsky, “Generalized  $F$ -Theorem and the  $\epsilon$  Expansion,” [arXiv:1507.01960 \[hep-th\]](#).
- [33] S. Giombi, I. R. Klebanov, and G. Tarnopolsky, “Conformal QED $_d$ ,  $F$ -Theorem and the  $\epsilon$  Expansion,” [arXiv:1508.06354 \[hep-th\]](#).
- [34] J. A. Minahan, “Localizing gauge theories on  $S^d$ ,” *JHEP* **04** (2016) 152, [arXiv:1512.06924 \[hep-th\]](#).
- [35] C. P. Herzog, I. R. Klebanov, S. S. Pufu, and T. Tesileanu, “Multi-Matrix Models and Tri-Sasaki Einstein Spaces,” *Phys. Rev.* **D83** (2011) 046001, [arXiv:1011.5487 \[hep-th\]](#).
- [36] I. R. Klebanov and A. A. Tseytlin, “Entropy of near extremal black p-branes,” *Nucl. Phys.* **B475** (1996) 164–178, [arXiv:hep-th/9604089 \[hep-th\]](#).
- [37] E. Witten, “Topological Quantum Field Theory,” *Commun. Math. Phys.* **117** (1988) 353.
- [38] V. Pestun, “Localization of gauge theory on a four-sphere and supersymmetric Wilson loops,” *Commun. Math. Phys.* **313** (2012) 71–129, [arXiv:0712.2824 \[hep-th\]](#).
- [39] A. Kapustin, B. Willett, and I. Yaakov, “Exact Results for Wilson Loops in Superconformal Chern-Simons Theories with Matter,” *JHEP* **03** (2010) 089, [arXiv:0909.4559 \[hep-th\]](#).
- [40] J. H. Schwarz, “Superconformal Chern-Simons theories,” *JHEP* **11** (2004) 078, [arXiv:hep-th/0411077 \[hep-th\]](#).
- [41] D. Gaiotto and X. Yin, “Notes on superconformal Chern-Simons-Matter theories,” *JHEP* **08** (2007) 056, [arXiv:0704.3740 \[hep-th\]](#).
- [42] B. Willett, “Localization on three-dimensional manifolds,” *Journal of Physics A* **xx** (2016) 000, [1608.02958](#).
- [43] K. A. Intriligator and N. Seiberg, “Mirror symmetry in three-dimensional gauge theories,” *Phys. Lett.* **B387** (1996) 513–519, [arXiv:hep-th/9607207 \[hep-th\]](#).
- [44] N. Drukker, M. Marino, and P. Putrov, “From weak to strong coupling in ABJM theory,” *Commun. Math. Phys.* **306** (2011) 511–563, [arXiv:1007.3837 \[hep-th\]](#).
- [45] R. C. Santamaria, M. Marino, and P. Putrov, “Unquenched flavor and tropical geometry in strongly coupled Chern-Simons-matter theories,” *JHEP* **10** (2011) 139, [arXiv:1011.6281 \[hep-th\]](#).
- [46] M. Marino and P. Putrov, “ABJM theory as a Fermi gas,” *J. Stat. Mech.* **1203** (2012) P03001, [arXiv:1110.4066 \[hep-th\]](#).
- [47] O. Aharony, O. Bergman, D. L. Jafferis, and J. Maldacena, “ $\mathcal{N} = 6$  superconformal Chern-Simons-matter theories, M2-branes and their gravity duals,” *JHEP* **10** (2008) 091, [arXiv:0806.1218 \[hep-th\]](#).
- [48] M. Mariño, “Localization at large  $N$  in Chern-Simons-matter theories,” *Journal of Physics A* **xx** (2016) 000, [1608.02959](#).
- [49] D. Martelli and J. Sparks, “The large  $N$  limit of quiver matrix models and Sasaki-Einstein manifolds,” *Phys. Rev.* **D84** (2011) 046008, [arXiv:1102.5289 \[hep-th\]](#).
- [50] S. Cheon, H. Kim, and N. Kim, “Calculating the partition function of  $\mathcal{N} = 2$  Gauge theories on  $S^3$  and AdS/CFT correspondence,” *JHEP* **05** (2011) 134, [arXiv:1102.5565 \[hep-th\]](#).
- [51] M. Gabella, D. Martelli, A. Passias, and J. Sparks, “The free energy of  $\mathcal{N} = 2$  supersymmetric AdS $_4$  solutions of M-theory,” *JHEP* **10** (2011) 039, [arXiv:1107.5035 \[hep-th\]](#).
- [52] D. R. Gulotta, J. P. Ang, and C. P. Herzog, “Matrix Models for Supersymmetric Chern-Simons Theories with an ADE Classification,” *JHEP* **01** (2012) 132, [arXiv:1111.1744 \[hep-th\]](#).

- [53] D. R. Gulotta, C. P. Herzog, and T. Nishioka, “The ABCDEF’s of Matrix Models for Supersymmetric Chern-Simons Theories,” *JHEP* **04** (2012) 138, [arXiv:1201.6360 \[hep-th\]](#).
- [54] P. M. Crichigno, C. P. Herzog, and D. Jain, “Free Energy of  $D_n$  Quiver Chern-Simons Theories,” *JHEP* **03** (2013) 039, [arXiv:1211.1388 \[hep-th\]](#).
- [55] A. Amariti and S. Franco, “Free Energy vs Sasaki-Einstein Volume for Infinite Families of M2-Brane Theories,” *JHEP* **09** (2012) 034, [arXiv:1204.6040 \[hep-th\]](#).
- [56] B. Assel, J. Estes, and M. Yamazaki, “Large N Free Energy of 3d N=4 SCFTs and  $AdS_4/CFT_3$ ,” *JHEP* **09** (2012) 074, [arXiv:1206.2920 \[hep-th\]](#).
- [57] A. Guarino, D. L. Jafferis, and O. Varela, “String Theory Origin of Dyonically  $\mathcal{N} = 8$  Supergravity and Its Chern-Simons Duals,” *Phys. Rev. Lett.* **115** (2015) no. 9, 091601, [arXiv:1504.08009 \[hep-th\]](#).
- [58] N. Hama, K. Hosomichi, and S. Lee, “Notes on SUSY Gauge Theories on Three-Sphere,” *JHEP* **03** (2011) 127, [arXiv:1012.3512 \[hep-th\]](#).
- [59] G. Festuccia and N. Seiberg, “Rigid Supersymmetric Theories in Curved Superspace,” *JHEP* **06** (2011) 114, [arXiv:1105.0689 \[hep-th\]](#).
- [60] C. Closset, T. T. Dumitrescu, G. Festuccia, Z. Komargodski, and N. Seiberg, “Comments on Chern-Simons Contact Terms in Three Dimensions,” *JHEP* **09** (2012) 091, [arXiv:1206.5218 \[hep-th\]](#).
- [61] T. Dumitrescu, “An Introduction to Supersymmetric Field Theories in Curved Space,” *Journal of Physics A* **xx** (2016) 000, [1608.02957](#).
- [62] D. Z. Freedman and S. S. Pufu, “The holography of  $F$ -maximization,” *JHEP* **03** (2014) 135, [arXiv:1302.7310 \[hep-th\]](#).
- [63] V. Borokhov, A. Kapustin, and X.-k. Wu, “Monopole operators and mirror symmetry in three-dimensions,” *JHEP* **12** (2002) 044, [arXiv:hep-th/0207074 \[hep-th\]](#).
- [64] V. Borokhov, A. Kapustin, and X.-k. Wu, “Topological disorder operators in three-dimensional conformal field theory,” *JHEP* **11** (2002) 049, [arXiv:hep-th/0206054 \[hep-th\]](#).
- [65] F. Benini, C. Closset, and S. Cremonesi, “Chiral flavors and M2-branes at toric CY4 singularities,” *JHEP* **02** (2010) 036, [arXiv:0911.4127 \[hep-th\]](#).
- [66] D. L. Jafferis, “Quantum corrections to  $\mathcal{N} = 2$  Chern-Simons theories with flavor and their  $AdS_4$  duals,” *JHEP* **08** (2013) 046, [arXiv:0911.4324 \[hep-th\]](#).
- [67] S. M. Chester, S. Giombi, L. V. Iliesiu, I. R. Klebanov, S. S. Pufu, and R. Yacoby, “Accidental Symmetries and the Conformal Bootstrap,” *JHEP* **01** (2016) 110, [arXiv:1507.04424 \[hep-th\]](#).
- [68] S. M. Chester, L. V. Iliesiu, S. S. Pufu, and R. Yacoby, “Bootstrapping  $O(N)$  Vector Models with Four Supercharges in  $3 \leq d \leq 4$ ,” [arXiv:1511.07552 \[hep-th\]](#).
- [69] S. M. Chester, J. Lee, S. S. Pufu, and R. Yacoby, “The  $\mathcal{N} = 8$  superconformal bootstrap in three dimensions,” *JHEP* **09** (2014) 143, [arXiv:1406.4814 \[hep-th\]](#).
- [70] N. Bobev, S. El-Showk, D. Mazac, and M. F. Paulos, “Bootstrapping SCFTs with Four Supercharges,” *JHEP* **08** (2015) 142, [arXiv:1503.02081 \[hep-th\]](#).
- [71] C. Beem, W. Peelaers, and L. Rastelli, “Deformation quantization and superconformal symmetry in three dimensions,” [arXiv:1601.05378 \[hep-th\]](#).
- [72] J. Wess and B. Zumino, “Supergauge Transformations in Four-Dimensions,” *Nucl. Phys.* **B70** (1974) 39–50.

- [73] M. J. Strassler, “An Unorthodox introduction to supersymmetric gauge theory,” in *Strings, Branes and Extra Dimensions: TASI 2001: Proceedings*, pp. 561–638. 2003. [arXiv:hep-th/0309149](#) [[hep-th](#)].
- [74] P. M. Ferreira and J. A. Gracey, “The Beta function of the Wess-Zumino model at  $O(1/N^2)$ ,” *Nucl. Phys.* **B525** (1998) 435–456, [arXiv:hep-th/9712138](#) [[hep-th](#)].
- [75] P. M. Ferreira and J. A. Gracey, “Nonzeta knots in the renormalization of the Wess-Zumino model?,” *Phys. Lett.* **B424** (1998) 85–92, [arXiv:hep-th/9712140](#) [[hep-th](#)].
- [76] P. M. Ferreira, I. Jack, and D. R. T. Jones, “The Quasiinfrared fixed point at higher loops,” *Phys. Lett.* **B392** (1997) 376–382, [arXiv:hep-ph/9610296](#) [[hep-ph](#)].
- [77] I. Jack and D. R. T. Jones, “Quasiinfrared fixed points and renormalization group invariant trajectories for nonholomorphic soft supersymmetry breaking,” *Phys. Rev.* **D61** (2000) 095002, [arXiv:hep-ph/9909570](#) [[hep-ph](#)].
- [78] I. Jack, D. R. T. Jones, and A. Pickering, “The soft scalar mass beta function,” *Phys. Lett.* **B432** (1998) 114–119, [arXiv:hep-ph/9803405](#) [[hep-ph](#)].
- [79] T. Nishioka and K. Yonekura, “On RG flow of  $\tau_{RR}$  for supersymmetric field theories in three-dimensions,” *Journal of High Energy Physics* **2013** (2013) no. 5, 1–20.
- [80] O. Aharony, A. Hanany, K. A. Intriligator, N. Seiberg, and M. J. Strassler, “Aspects of  $\mathcal{N} = 2$  supersymmetric gauge theories in three-dimensions,” *Nucl. Phys.* **B499** (1997) 67–99, [arXiv:hep-th/9703110](#) [[hep-th](#)].
- [81] B. Willett and I. Yaakov, “ $\mathcal{N} = 2$  Dualities and  $Z$  Extremization in Three Dimensions,” [arXiv:1104.0487](#) [[hep-th](#)].
- [82] A. Kapustin, B. Willett, and I. Yaakov, “Nonperturbative Tests of Three-Dimensional Dualities,” *JHEP* **10** (2010) 013, [arXiv:1003.5694](#) [[hep-th](#)].
- [83] A. Kapustin, B. Willett, and I. Yaakov, “Tests of Seiberg-like Duality in Three Dimensions,” [arXiv:1012.4021](#) [[hep-th](#)].
- [84] A. Amariti, C. Klare, and M. Siani, “The Large  $N$  Limit of Toric Chern-Simons Matter Theories and Their Duals,” *JHEP* **10** (2012) 019, [arXiv:1111.1723](#) [[hep-th](#)].
- [85] B. R. Safdi, I. R. Klebanov, and J. Lee, “A Crack in the Conformal Window,” *JHEP* **04** (2013) 165, [arXiv:1212.4502](#) [[hep-th](#)].
- [86] A. Kapustin, “Seiberg-like duality in three dimensions for orthogonal gauge groups,” [arXiv:1104.0466](#) [[hep-th](#)].
- [87] D. Jafferis and X. Yin, “A Duality Appetizer,” [arXiv:1103.5700](#) [[hep-th](#)].
- [88] A. Kapustin, H. Kim, and J. Park, “Dualities for 3d Theories with Tensor Matter,” *JHEP* **12** (2011) 087, [arXiv:1110.2547](#) [[hep-th](#)].
- [89] T. Morita and V. Niarchos, “F-theorem, duality and SUSY breaking in one-adjoint Chern-Simons-Matter theories,” *Nucl. Phys.* **B858** (2012) 84–116, [arXiv:1108.4963](#) [[hep-th](#)].
- [90] F. Benini, C. Closset, and S. Cremonesi, “Comments on 3d Seiberg-like dualities,” *JHEP* **10** (2011) 075, [arXiv:1108.5373](#) [[hep-th](#)].
- [91] D. Gang, C. Hwang, S. Kim, and J. Park, “Tests of  $\text{AdS}_4/\text{CFT}_3$  correspondence for  $\mathcal{N} = 2$  chiral-like theory,” *JHEP* **02** (2012) 079, [arXiv:1111.4529](#) [[hep-th](#)].
- [92] D. R. Gulotta, C. P. Herzog, and S. S. Pufu, “Operator Counting and Eigenvalue Distributions for 3D Supersymmetric Gauge Theories,” *JHEP* **11** (2011) 149, [arXiv:1106.5484](#) [[hep-th](#)].

- [93] H. Kim and N. Kim, “Operator Counting for  $\mathcal{N} = 2$  Chern-Simons Gauge Theories with Chiral-like Matter Fields,” *JHEP* **05** (2012) 152, [arXiv:1202.6637 \[hep-th\]](#).
- [94] D. Martelli, A. Passias, and J. Sparks, “The gravity dual of supersymmetric gauge theories on a squashed three-sphere,” *Nucl. Phys.* **B864** (2012) 840–868, [arXiv:1110.6400 \[hep-th\]](#).
- [95] D. Martelli and J. Sparks, “The gravity dual of supersymmetric gauge theories on a biaxially squashed three-sphere,” *Nucl. Phys.* **B866** (2013) 72–85, [arXiv:1111.6930 \[hep-th\]](#).
- [96] D. Martelli, A. Passias, and J. Sparks, “The supersymmetric NUTs and bolts of holography,” *Nucl. Phys.* **B876** (2013) 810–870, [arXiv:1212.4618 \[hep-th\]](#).
- [97] D. Martelli and A. Passias, “The gravity dual of supersymmetric gauge theories on a two-parameter deformed three-sphere,” *Nucl. Phys.* **B877** (2013) 51–72, [arXiv:1306.3893 \[hep-th\]](#).
- [98] D. Farquet, J. Lorenzen, D. Martelli, and J. Sparks, “Gravity duals of supersymmetric gauge theories on three-manifolds,” *JHEP* **08** (2016) 080, [arXiv:1404.0268 \[hep-th\]](#).
- [99] D. Farquet and J. Sparks, “Wilson loops and the geometry of matrix models in  $\text{AdS}_4/\text{CFT}_3$ ,” *JHEP* **01** (2014) 083, [arXiv:1304.0784 \[hep-th\]](#).
- [100] D. Farquet and J. Sparks, “Wilson loops on three-manifolds and their M2-brane duals,” *JHEP* **12** (2014) 173, [arXiv:1406.2493 \[hep-th\]](#).
- [101] N. Bobev, H. Elvang, D. Z. Freedman, and S. S. Pufu, “Holography for  $\mathcal{N} = 2^*$  on  $S^4$ ,” *JHEP* **07** (2014) 001, [arXiv:1311.1508 \[hep-th\]](#).
- [102] N. Bobev, H. Elvang, U. Kol, T. Olson, and S. S. Pufu, “Holography for  $\mathcal{N} = 1^*$  on  $S^4$ ,” [arXiv:1605.00656 \[hep-th\]](#).
- [103] I. R. Klebanov, T. Nishioka, S. S. Pufu, and B. R. Safdi, “Is Renormalized Entanglement Entropy Stationary at RG Fixed Points?,” *JHEP* **10** (2012) 058, [arXiv:1207.3360 \[hep-th\]](#).
- [104] H. Liu and M. Mezei, “Probing renormalization group flows using entanglement entropy,” *JHEP* **01** (2014) 098, [arXiv:1309.6935 \[hep-th\]](#).
- [105] D. L. Jafferis and S. S. Pufu, “Exact results for five-dimensional superconformal field theories with gravity duals,” *JHEP* **05** (2014) 032, [arXiv:1207.4359 \[hep-th\]](#).
- [106] L. Fei, S. Giombi, and I. R. Klebanov, “Critical  $O(N)$  models in  $6 - \epsilon$  dimensions,” *Phys. Rev.* **D90** (2014) no. 2, 025018, [arXiv:1404.1094 \[hep-th\]](#).

# Chapter 9

## Perturbative and nonperturbative aspects of complex Chern-Simons Theory

Tudor Dimofte

*Perimeter Institute for Theoretical Physics, 31 Caroline St. N, Waterloo, ON N2J 2Y5, Canada*  
*(on leave) Department of Mathematics, University of California, Davis, CA 95616, USA*  
tudor@math.ucdavis.edu

### Abstract

We present an elementary review of some aspects of Chern-Simons theory with complex gauge group  $SL(N, \mathbb{C})$ . We discuss some of the challenges in defining the theory as a full-fledged TQFT, as well as some successes inspired by the 3d-3d correspondence. The 3d-3d correspondence relates partition functions (and other aspects) of complex Chern-Simons theory on a 3-manifold  $M$  to supersymmetric partition functions (and other observables) in an associated 3d theory  $T[M]$ . Many of these observables may be computed by supersymmetric localization. We present several prominent applications to 3-manifold topology and number theory in light of the 3d-3d correspondence.

### Contents

|            |                                                              |            |
|------------|--------------------------------------------------------------|------------|
| <b>9.1</b> | <b>Introduction</b>                                          | <b>368</b> |
| <b>9.2</b> | <b>Warmup: quantization of <math>\mathcal{H}(T^2)</math></b> | <b>370</b> |
| 9.2.1      | Equivariant quantization                                     | 374        |
| 9.2.2      | Holomorphic polarizations and CFT                            | 375        |
| <b>9.3</b> | <b>Complex Chern-Simons theory as a TQFT?</b>                | <b>376</b> |
| 9.3.1      | Symmetries, regularizations, and the 3d-3d correspondence    | 378        |
| <b>9.4</b> | <b>Three connections to three-manifold topology</b>          | <b>379</b> |

|                   |                                                                       |            |
|-------------------|-----------------------------------------------------------------------|------------|
| 9.4.1             | Hyperbolic volumes, twisted torsion, and large $N$ . . . . .          | 379        |
| 9.4.2             | State-integral models and angle structures . . . . .                  | 381        |
| 9.4.3             | Embedded surfaces and M2 branes in the 3d index ( $k = 0$ ) . . . . . | 386        |
| <b>9.5</b>        | <b>The Quantum Modularity Conjecture</b> . . . . .                    | <b>388</b> |
| <b>References</b> | . . . . .                                                             | <b>391</b> |

## 9.1 Introduction

Chern-Simons theory with complex gauge group came to prominence in the late 80's, partly as a tool for understanding three-dimensional gravity with a negative cosmological constant [2–5]. Many early developments were due to Witten. Since then, it has found a multitude of applications and deep connections with many parts of theoretical physics and mathematics. A highly incomplete list includes:

- Many further applications of  $SL(2, \mathbb{C})$  Chern-Simons theory (and its  $SL(2, \mathbb{R}) \times SL(2, \mathbb{R})$  cousin) to three-dimensional quantum gravity and AdS/CFT. Similarly,  $SL(N, \mathbb{C})$  Chern-Simons at large  $N$  has been used to describe higher-spin theories of gravity [6, 7].
- Chern-Simons theory with gauge group  $SL(N, \mathbb{C})$  can naturally be embedded in string/M-theory, opening up many powerful perspectives and techniques for analyzing the former. As a notable example, the compactification of  $N$  M5 branes on the product of an ellipsoidally deformed lens space  $L(k, 1)_b \simeq S_b^3/\mathbb{Z}_k$  and a three-manifold  $M$  (with a topological twist along  $M$ ) leads equivalently to  $SL(N, \mathbb{C})$  Chern-Simons theory at level  $k$  on  $M$  [8–10] or an  $\mathcal{N} = 2$  supersymmetric theory  $T_N[M]$  on the lens space [11–14]. This duality, known as the 3d-3d correspondence, fits into a series of dualities involving the compactification of five-branes on various  $d$ -dimensional manifolds  $M^d$ , including the AGT correspondence [15] and the duality of Gukov-Gadde-Putrov relating Vafa-Witten partition functions on  $M^4$  and elliptic genera [16].
- There is a multitude of applications to three-dimensional geometry and topology. Fundamentally, partition functions of complex Chern-Simons theory on three-manifolds  $M$  provide new topological invariants, generalizing the famous invariants (including knot polynomials) associated with compact Chern-Simons theory [17, 18]. As yet, a systematic computation of the complex invariants only exists for certain classes of manifolds (*e.g.* hyperbolic ones [19–22]), though new tools to attack the general case are under development [23, 24].

The perturbative expansion of  $SL(2, \mathbb{C})$  Chern-Simons theory on a three-manifold  $M$  encodes various topological invariants of  $M$ , such as its hyperbolic volume and twisted analytic torsion. In the case that  $M = S^3 \setminus K$  is a knot complement in  $S^3$ , it was conjectured by Gukov [25] that this expansion agrees with a (highly nontrivial) asymptotic limit of colored Jones polynomials of  $K$ , providing physical motivation for a mathematical statement known as the Volume Conjecture [26, 27]. The relation between

complex Chern-Simons theory and knot polynomials is essentially a result of analytic continuation, albeit a subtle one [28].

The perturbative expansion of  $SL(2, \mathbb{C})$  Chern-Simons theory on knot complements has been successfully reproduced [29–31] using the topological recursion of Eynard-Orantin [32], a far-reaching formalism for the quantization of spectral curves.

The study of five-brane systems related to complex Chern-Simons theory recently led to a vast generalization of the Volume Conjecture, involving asymptotic limits of colored HOMFLY polynomials and their categorification [33].

- There are several hints that complex Chern-Simons theory has quasi-modular properties, *cf.* [12,34], though a complete physical characterization of these properties is still missing. The asymptotic expansions of  $SL(2, \mathbb{C})$  Chern-Simons theory around various singular points in the space of coupling constants (levels) [35], related by an action of the modular group, provide evidence for the Quantum Modularity Conjecture of Zagier [36].
- There are close connections between complex Chern-Simons theory and the mathematical theory of cluster algebras, *cf.* [37,38]. Cluster algebras play an essential role in the (local) description and quantization of phase spaces that complex Chern-Simons theory attaches to two-dimensional boundaries, *cf.* [39–41], and Chern-Simons theory on three-manifolds is associated with cluster-algebra morphisms.
- Very recently,  $SL(2, \mathbb{C})$  Chern-Simons theory at integer levels (in terms of (9.2.1) below, this means  $k \in \mathbb{Z}$  and  $is \in \mathbb{Z}$ ) has been proposed as an effective theory of quantum Hall systems [42]. Excitingly, this may lead to tests of complex Chern-Simons theory in the lab.

In this short review, we will only be able to touch upon a few of these topics and connections. We will actually begin in Section 9.2 with some basic concepts in complex Chern-Simons theory, including the definition of the Hilbert spaces  $\mathcal{H}[\Sigma]$  assigned to two-dimensional oriented manifolds. One of the most prominent distinctions between Chern-Simons theory with complex and compact gauge groups is that, in the complex case, these Hilbert spaces are infinite-dimensional. As an illustrative example, we will outline the simple quantization of the torus Hilbert space  $\mathcal{H}[T^2]$  for gauge group  $SL(2, \mathbb{C})$ , and its dependence on the coupling constants or “levels” of the theory. We also review some features of the refined or *equivariant* quantization of Hilbert spaces recently developed by Gukov and Pei [23].

This prepares us in Section 9.3 to discuss one of the most fundamental *open* problems in complex Chern-Simons theory: defining the theory as a full TQFT. In essence, this means being able to assign Hilbert spaces  $\mathcal{H}[\Sigma]$  to any oriented surface and wavefunctions  $\mathcal{Z}[M] \in \mathcal{H}[\partial M]$  to any oriented three-manifold, in such a way that the standard cutting-and-gluing axioms of Atiyah and Segal are obeyed [43]. As we shall review, the difficulty with cutting and gluing in complex Chern-Simons theory stems from the infinite-dimensional nature of Hilbert spaces, and the fact that, naively, wavefunctions often vanish or diverge. Some very promising routes to overcoming these difficulties are suggested by embedding

complex Chern-Simons theory in string/M-theory, and using additional symmetries to regulate zeroes or infinities [23, 24, 44]. Interestingly, these symmetries are related to categorification of Chern-Simons theory.

In the second half of this review, we then discuss a few relations between complex Chern-Simons theory and the topology and geometry of three-manifolds. In each case, we view these relations in light of string/M-theory and the 3d-3d correspondence. In Section 9.4, we will discuss 1) asymptotic expansions of  $SL(N, \mathbb{C})$  Chern-Simons partition functions, their relation to hyperbolic volumes, and their behavior at large  $N$  *vis à vis* holography of five-brane systems; 2) state-sum/integral models for  $SL(N, \mathbb{C})$  Chern-Simons theory, their relation to positive angle structures on ideal triangulations of three-manifolds, and the corresponding implication for positivity of operator dimensions in theories  $T[M]$  built from ideal triangulations; 3) the interpretation of the  $SL(N, \mathbb{C})$  partition function at level  $k = 0$  as counting surfaces in a three-manifold  $M$ , BPS operators in  $T[M]$ , and BPS M2 branes ending on wrapped M5 branes in M-theory (related to recent mathematical work [45]). In Section 9.5, we will state some of the observations and conjectures about “quantum” modularity in Chern-Simons theory.

We emphasize that the 3d-3d correspondence provides the main link between complex Chern-Simons theory and localization methods in supersymmetric gauge theories, which are the focus of this collection of articles. Particularly relevant are the reviews of T. Dumitrescu (Chapter 5) and B. Willett (Chapter 6). The basic idea is that whenever  $T[M]$  can be explicitly described as (say) a gauge theory, its partition function on spaces such as  $S^3$  or  $S^3/\mathbb{Z}_k$  is readily computed by supersymmetric localization. This has led to new formulations and refinements of Chern-Simons partition functions on  $M$ , which in turn produce invariants of 3-manifolds,

$$\begin{array}{ccc}
 & \text{complex CS theory on } M \\
 & + \text{ refinement/categorification...} \\
 \swarrow & & \searrow \\
 \text{SUSY localization for } T[M] & & \text{topological invariants of } M
 \end{array} \tag{9.1.1}$$

Unfortunately, we will not say very much about connections of complex Chern-Simons theory to cluster algebras, topological recursion, categorification, gravity, or many other fascinating topics. We hope that some of the references above will guide readers interested in these subjects.

## 9.2 Warmup: quantization of $\mathcal{H}(T^2)$

To get a feel for the structure of complex Chern-Simons theory, we begin with a (seemingly) elementary exercise: the quantization of the phase space that  $SL(2, \mathbb{C})$  Chern-Simons theory attaches to a two-torus.

First, some generalities. As discussed in [5], the action of complex Chern-Simons theory on a Euclidean three-manifold  $M$  takes the form

$$I_{k,s} = \frac{1}{2}(k + is)S_{CS}(\mathcal{A}) + \frac{1}{2}(k - is)S_{CS}(\overline{\mathcal{A}}), \tag{9.2.1}$$

where  $S_{CS} = \frac{1}{4\pi} \int_M \text{Tr}(\mathcal{A} \wedge \mathcal{A} + \frac{2}{3} \mathcal{A} \wedge \mathcal{A} \wedge \mathcal{A})$  is the usual Chern-Simons functional. Here  $\mathcal{A}$  is a connection on an  $SL(2, \mathbb{C})$  bundle over  $M$ , and  $\bar{\mathcal{A}}$  is its complex conjugate. The group  $SL(2, \mathbb{C})$  contains  $SU(2)$  as its maximal compact subgroup (in fact, as a complex manifold,  $SL(2, \mathbb{C}) \simeq T^*SU(2)$ ), and on a compact 3-manifold  $M$  there can be large gauge transformations  $g : M \rightarrow SL(2, \mathbb{C})$  that wrap nontrivially around the compact  $SU(2)$ . The path-integral integration measure  $\exp(iI_{k,s})$  is invariant under large gauge transformations on a closed  $M$  so long as  $k \in \mathbb{Z}$ . On the other hand, the coupling constant  $s$  is unconstrained.

For a unitary theory — which in Euclidean space means that partition functions are conjugated under orientation reversal — the action must be real, which forces  $s$  to be real. We will assume this to be true in the quantization below, though eventually in partition functions we will find that we can analytically continue  $s$  in a straightforward manner. There also exist exotic unitarity structures with  $s$  imaginary [5], which will lead to slightly different Hilbert spaces.

As an aside, in the relation to 3d Euclidean gravity with a negative cosmological constant, one identifies the Hermitian and anti-Hermitian parts of  $\mathcal{A} = w + ie$  as a vielbein ( $e$ ) and a spin connection ( $w$ ). The part of the action  $I_{k,s}$  proportional to  $s$  becomes the usual Einstein-Hilbert action, while the part proportional to  $k$  is a gravitational Chern-Simons term [3]. The classical solutions of Chern-Simons theory on a three-manifold  $M$  are flat  $SL(2, \mathbb{C})$  connections, which become identified with (possibly degenerate) metrics of constant negative curvature, *i.e.* hyperbolic metrics, in 3d gravity.

Geometric quantization of complex Chern-Simons theory on a general surface  $\Sigma$  was first discussed in [5] and recently revisited in [48], using a holomorphic polarization. A more modern perspective on quantization, based on the topological A-model, appears in [49], following [50] (see also [51]). In the case of  $\Sigma = T^2$ , we can take a more pedestrian approach, following [21, 22].

The Hilbert space that Chern-Simons theory assigns to any surface  $\Sigma$  is a quantization of the classical phase space

$$\mathcal{P}[\Sigma] = \mathcal{M}_{\text{flat}}(SL(2, \mathbb{C}), \Sigma) \simeq \text{Hom}(\pi_1(\Sigma), SL(2, \mathbb{C})). \quad (9.2.2)$$

This is the space of complex flat connections on  $\Sigma$  (modulo gauge transformations), or equivalently, the space of representations of the fundamental group of  $\Sigma$  in  $SL(2, \mathbb{C})$ . The space  $\mathcal{P}[\Sigma]$  is a finite-dimensional complex symplectic variety, possibly singular, equipped with the Atiyah-Bott holomorphic symplectic form

$$\Omega = \int_{\Sigma} \delta \mathcal{A} \wedge \delta \mathcal{A}. \quad (9.2.3)$$

Of course, the actual symplectic form we use for quantization should be real; the Chern-Simons action (9.2.1) tells us to take

$$\omega_{k,s} = \frac{k + is}{4\pi} \Omega + \frac{k - is}{4\pi} \bar{\Omega} = \frac{k}{2\pi} \text{Re} \Omega - \frac{s}{2\pi} \text{Im} \Omega. \quad (9.2.4)$$

Famously, the space  $\mathcal{P}[\Sigma]$  is hyperkähler. It admits an entire  $\mathbb{C}\mathbb{P}^1$  of complex structures, one of which is singled out in the description (9.2.2) as a space of complex flat connections.

The other complex structures can be made manifest by rewriting  $\mathcal{P}[\Sigma]$  as Hitchin's moduli space  $\mathcal{P}[\Sigma] \simeq \mathcal{M}_{\text{Hit}}(SU(2), \Sigma)$  associated to the compact group  $SU(2)$  [52]. Similarly, the space  $\mathcal{P}[\Sigma]$  admits a  $\mathbb{C}\mathbb{P}^1$  of real symplectic forms, spanned by the hyperkähler triplet  $(\omega_I, \omega_J, \omega_K)$ , where  $\omega_I = \text{Re } \Omega$  and  $\omega_J = \text{Im } \Omega$  above. The third form  $\omega_J$  is a Kähler form in our chosen complex structure. Notably,  $\frac{1}{4\pi^2}\omega_I$  represents a nontrivial *integral* cohomology class in  $H^2(\mathcal{P}[\Sigma], \mathbb{Z})$ , while  $\omega_J, \omega_K$  are cohomologically trivial. This provides another explanation for the quantization of the level  $k$ : in geometric quantization, one requires  $\omega_{k,s}$  to be the first Chern class of a line bundle, which can only happen if it has integral periods, whence  $k \in \mathbb{Z}$ , but  $s$  is unconstrained.

Now let us specialize to  $\Sigma = T^2$ . Flat connections on a torus are determined by the holonomies  $\rho_A, \rho_B$  along the  $A$  and  $B$  cycles, up to  $SL(2, \mathbb{C})$  conjugation. Since the fundamental group  $\pi_1(T^2) = \mathbb{Z}^2$  is abelian, the holonomies commute and can be simultaneously diagonalized.<sup>1</sup> Letting  $x, y$  denote their eigenvalues, we find

$$\mathcal{P}[T^2] = (\mathbb{C}^* \times \mathbb{C}^*)/\mathbb{Z}_2 \simeq \{(x, y) \in (\mathbb{C}^*)^2\}/(x, y) \sim (x^{-1}, y^{-1}). \quad (9.2.5)$$

The  $\mathbb{Z}_2$  action here is just that of the Weyl group, acting as residual gauge transformations. The holomorphic symplectic form is

$$\Omega = 2 \frac{dy}{y} \wedge \frac{dx}{x}, \quad (9.2.6)$$

reflecting the nontrivial intersection of  $A$  and  $B$  cycles on  $T^2$ , whence

$$\omega_{k,s} = \frac{k}{\pi} (d \log |y| \wedge d \log |x| - d \arg y \wedge d \arg x) - \frac{s}{\pi} (d \log |y| \wedge d \arg x + d \arg y \wedge d \log |x|). \quad (9.2.7)$$

As anticipated, the period of  $\frac{1}{2\pi}\omega_{k,s}$  on the compact  $(S^1 \times S^1)/\mathbb{Z}_2$  cycle in  $\mathcal{P}[T^2]$  is equal to  $k$ , and is properly quantized.

In order to diagonalize the real symplectic form  $\omega_{k,s}$ , we define  $b$  to be the complex number with  $\text{Re}(b) > 0$  and

$$b^2 = \frac{k - is}{k + is}, \quad (9.2.8)$$

and make a change of variables<sup>2</sup> from  $(x, y) \in (\mathbb{C}^*)^2$  to  $(\mu, \nu; m, n) \in \mathbb{R}^2 \times (\mathbb{R}/2k\mathbb{Z})^2$ :

$$\begin{aligned} x &= \exp \frac{i\pi}{k} (-ib\mu - m), & \bar{x} &= \exp \frac{i\pi}{k} (-ib^{-1}\mu + m), \\ y &= \exp \frac{i\pi}{k} (-ib\nu - n), & \bar{y} &= \exp \frac{i\pi}{k} (-ib^{-1}\nu + n). \end{aligned} \quad (9.2.9)$$

Notice that if  $s$  is real then  $|b| = 1$ , so  $(x, y)$  and  $(\bar{x}, \bar{y})$  are complex conjugates, as written. Then the symplectic form collapses to

$$\omega_{k,s} = \frac{\pi}{k} d\nu \wedge d\mu - \frac{\pi}{k} dn \wedge dm. \quad (9.2.10)$$

<sup>1</sup>More precisely: the holonomies can simultaneously be put in Jordan normal form.

<sup>2</sup>The new variables absorb some powers of the coupling constants  $k, b$ , which obfuscates the effect of the classical limit  $k \rightarrow \infty$ , *e.g.* in (9.2.11). It is important to keep in mind that the natural functions on the phase space are still  $x, \bar{x}, y, \bar{y}$ .

We proceed to quantize the space as if it were just  $\mathbb{C}^* \times \mathbb{C}^*$ , and restore Weyl invariance later. The functions  $\nu, \mu$  and  $n, m$  can simply be quantized to operators with canonical commutation relations

$$-[\boldsymbol{\nu}, \boldsymbol{\mu}] = [\mathbf{n}, \mathbf{m}] = \frac{k}{i\pi}. \quad (9.2.11)$$

Of course, since  $m$  is periodic the spectrum of  $\mathbf{n}$  is quantized, and vice versa; altogether, both the eigenvalues of both  $\mathbf{m}$  and  $\mathbf{n}$  must belong to  $\mathbb{Z}/(2k\mathbb{Z})$ . The well-defined operators are actually quantizations  $\mathbf{x}, \bar{\mathbf{x}}, \mathbf{y}, \bar{\mathbf{y}}$  of the  $\mathbb{C}^*$ -valued functions in (9.2.9), with  $\mathbf{x} = \exp \frac{i\pi}{k} \left( -ib\boldsymbol{\mu} - \mathbf{m} \right)$ , etc. For these we find

$$\mathbf{y}\mathbf{x} = q^{\frac{1}{2}}\mathbf{x}\mathbf{y}, \quad \bar{\mathbf{y}}\bar{\mathbf{x}} = \tilde{q}^{\frac{1}{2}}\bar{\mathbf{x}}\bar{\mathbf{y}}; \quad \mathbf{x}\bar{\mathbf{y}} = \bar{\mathbf{y}}\mathbf{x}, \quad \mathbf{y}\bar{\mathbf{x}} = \bar{\mathbf{x}}\mathbf{y}, \quad (9.2.12)$$

with

$$q^{\frac{1}{2}} := \exp \frac{2\pi i}{k+is} = \exp \frac{i\pi}{k}(b^2+1), \quad \tilde{q}^{\frac{1}{2}} := \exp \frac{2\pi i}{k-is} = \exp \frac{i\pi}{k}(b^{-2}+1). \quad (9.2.13)$$

Thus, abstractly, we see that the quantized operator algebra consists of two independent Weyl algebras (or “quantum torus” algebras), one in  $\mathbf{x}, \mathbf{y}$  and one in  $\bar{\mathbf{x}}, \bar{\mathbf{y}}$ .

There are many equivalent ways to represent the operator algebra on a Hilbert space  $\mathcal{H}[T^2]$ . The simplest is to take

$$\mathcal{H}[T^2]_{k,s} = L^2(\mathbb{R}) \otimes \mathbb{C}^{2|k|} \simeq \{f(\mu, m)\} \quad (9.2.14)$$

to consist of functions of a real variable  $\mu$  and an integer  $m \in \mathbb{Z}/(2k\mathbb{Z})$ . Equivalently, we may take functions of  $x$  and  $\bar{x}$ . Formally, in geometric quantization, this corresponds to choosing a particular “real” polarization — taking sections of a line bundle  $\mathcal{L} \rightarrow \mathcal{P}[\Sigma]$  with  $c_1(\mathcal{L}) = \omega_{k,s}$  that are covariantly constant with respect to  $\nu$  and  $n$ . The operators  $\mathbf{x}, \bar{\mathbf{x}}$  act on  $f(\mu, m)$  as multiplication by  $x, \bar{x}$ , while  $\mathbf{y}, \bar{\mathbf{y}}$  are shifts

$$\mathbf{y}f(\mu, m) = f(\mu + ib, m - 1), \quad \bar{\mathbf{y}}f(\mu, m) = f(\mu + ib^{-1}, m + 1). \quad (9.2.15)$$

To restore Weyl-invariance, we restrict to the  $\mathbb{Z}_2$ -invariant part of the Hilbert space, *i.e.* functions that are even

$$f(\mu, m) = f(-\mu, -m). \quad (9.2.16)$$

Correspondingly, we should restrict to a subalgebra of the operator algebra that is invariant under  $(\mathbf{x}, \bar{\mathbf{x}}, \mathbf{y}, \bar{\mathbf{y}}) \rightarrow (\mathbf{x}^{-1}, \bar{\mathbf{x}}^{-1}, \mathbf{y}^{-1}, \bar{\mathbf{y}}^{-1})$ . This subalgebra is generated by operators  $\mathbf{X} = \mathbf{x} + \mathbf{x}^{-1}$ ,  $\mathbf{Y} = \mathbf{y} + \mathbf{y}^{-1}$ , and  $\mathbf{T} = \mathbf{x}\mathbf{y} + \mathbf{x}^{-1}\mathbf{y}^{-1}$  (and their conjugates), which obey

$$\mathbf{X}^2 + \mathbf{Y}^2 + q^{-\frac{1}{2}}\mathbf{T}^2 = \mathbf{X}\mathbf{T}\mathbf{Y} + 2(1 + q^{-1}). \quad (9.2.17)$$

When  $k = 0$ , complex Chern-Simons theory still make sense (as long as  $s \neq 0$ ), but the above quantization procedure requires a slight modification [20]. The change of variables (9.2.9) does not make sense, and is not necessary, since  $\omega_{k=0,s}$  is already diagonalized. Indeed,

$\omega_{k=0,s}$  is the canonical symplectic form on  $\mathbb{C}^* \times \mathbb{C}^*$  when viewed as the cotangent bundle  $T^*(S^1 \times S^1)$ . We expect quantization to produce  $\mathcal{H}[T^2]_{0,s} = L^2(\mathbb{Z} \times \mathbb{Z})$ . To see it, simply write  $(x, y) = (e^{\frac{\pi}{s}m+i\theta}, e^{\frac{\pi}{s}n+i\phi})$ . The symplectic form becomes

$$\omega_{k=0,s} = -dn \wedge d\theta + dm \wedge d\phi. \quad (9.2.18)$$

These canonically-conjugate functions are quantized to operators with  $[\boldsymbol{\theta}, \mathbf{n}] = -[\boldsymbol{\phi}, \mathbf{m}] = i$ . Since  $\theta, \phi$  are periodic with period  $2\pi$ , the eigenvalues of  $\mathbf{m}, \mathbf{n}$  must be integers. We can represent the operator algebra (say) on functions  $f(m, n)$  of two integers, such that

$$\begin{aligned} \mathbf{x} f(m, n) &= q^{\frac{m}{4}} f(m, n-1), & \bar{\mathbf{x}} f(m, n) &= \tilde{q}^{-\frac{m}{4}} f(m, n+1), \\ \mathbf{y} f(m, n) &= q^{\frac{n}{4}} f(m+1, n), & \bar{\mathbf{y}} f(m, n) &= \tilde{q}^{-\frac{n}{4}} f(m-1, n), \end{aligned} \quad (9.2.19)$$

where now (9.2.13) reduces to

$$q^{\frac{1}{4}} = \tilde{q}^{-\frac{1}{4}} := \exp \frac{\pi}{s}. \quad (9.2.20)$$

With these new definitions of  $q$  and  $\tilde{q}$ , the operators satisfy the standard quantum-torus relations (9.2.12). Alternatively, and equivalently, we may take the Hilbert space to contain functions  $g(m, \zeta)$  of an integer  $m$  and a phase  $\zeta = e^{i\theta}$ , with

$$\begin{aligned} \mathbf{x} g(m, \zeta) &= q^{\frac{m}{4}} \zeta g(m, \zeta), & \bar{\mathbf{x}} g(m, \zeta) &= \tilde{q}^{-\frac{m}{4}} \zeta^{-1} g(m, \zeta), \\ \mathbf{y} g(m, \zeta) &= q^{\frac{n}{4}} g(m+1, q^{\frac{1}{4}} \zeta), & \bar{\mathbf{y}} g(m, \zeta) &= \tilde{q}^{-\frac{n}{4}} g(m-1, \tilde{q}^{-\frac{n}{4}} \zeta). \end{aligned} \quad (9.2.21)$$

Again, we impose Weyl-invariance at the end by restricting to even functions  $f(m, n) = f(-m, -n)$  or  $g(m, \zeta) = g(-m, \zeta^{-1})$ .

### 9.2.1 Equivariant quantization

There are several things to notice about (9.2.14). Perhaps the most salient is that, unlike in the case of Chern-Simons theory with compact gauge group [17, 53], the Hilbert space is infinite-dimensional. This is no surprise, since it comes from quantizing a noncompact phase space. One may also recognize the  $\mathbb{C}^{2k}$  factor as being related to the standard Hilbert space for  $SU(2)$  theory at (bare) level  $k$ . Indeed, if we ignore  $\mu$  and consider functions  $f(m)$  of an integer  $m \in \mathbb{Z}/(2k\mathbb{Z})$ , such that  $f(m) = f(-m)$  as in (9.2.16), we find exactly  $|k|+1$  independent values  $f(0), f(1), \dots, f(|k|)$  that determine a state in the finite-dimensional Hilbert space of  $SU(2)$  Chern-Simons.

What is less obvious, in particular for general  $\Sigma$ , is that the infinite-dimensional Hilbert space of complex Chern-Simons theory admits an additional  $U(1)_t$  symmetry, introduced in [23]. The graded components of  $\mathcal{H}[\Sigma]$  (*i.e.* the subspaces of fixed  $U(1)_t$  charge) turn out to be finite-dimensional, and in particular the subspace of zero charge is just the familiar  $SU(2)$  Hilbert space.

The extra  $U(1)_t$  symmetry comes from viewing  $\mathcal{P}[\mathcal{M}] \simeq \mathcal{M}_{\text{Hit}}(SU(2), \Sigma)$  as the Hitchin moduli space. There is a canonical  $U(1)_t$  metric isometry of the Hitchin moduli space that rotates the  $\mathbb{CP}^1$  of complex structures about an axis. In particular, it rotates  $\omega_J = \text{Im}(\Omega)$

and  $\omega_K$  into each other. This is an isometry of our quantization problem at least when  $s = 0$ , since it preserves  $\omega_{k,s=0}$ , and leads to the desired symmetry of  $\mathcal{H}[\Sigma]_{k,0}$ . (Since the Hilbert space, abstractly, does not depend on  $s$ , one might then hope to endow even spaces at  $s \neq 0$  with the symmetry.)

In the case  $\Sigma = T^2$ , it is easy to describe the  $U(1)_t$  symmetry: when we view  $\mathcal{P}[T^2] \simeq T^*(S^1 \times S^1)/\mathbb{Z}_2 \approx T^*\mathcal{M}_{\text{flat}}(SU(2), T^2)$  as the cotangent bundle of the space of flat  $SU(2)$  connections,  $U(1)_t$  simply rotates the cotangent fibers. The  $U(1)_t$ -invariant subspace of  $\mathcal{H}[T^2]_{k,s=0}$  simply consists of the functions  $f(\mu, m)$  that are independent of  $\mu$  — *i.e.* the  $SU(2)$  Hilbert space we found above. The full  $U(1)_t$  action is trickier to describe in the polarization we are using. Roughly, one observes that at  $s = 0$  and  $b = 1$  the variables  $x, \bar{x}$  can be written as

$$x = z\eta^{-m}, \quad \bar{x} = z\eta^m, \quad (9.2.22)$$

where  $z = \exp(\pi\mu/k)$  and  $\eta = \exp(i\pi/k)$ . Then, on functions of  $f(z, m)$  that are analytic in  $z$ , the  $U(1)_t$  symmetry just acts as rotations  $z \rightarrow e^{i\theta}z$ . The subspaces of fixed  $U(1)_t$  weight contain monomials in  $z$ . After imposing Weyl invariance, the graded dimension of the Hilbert space becomes

$$\begin{aligned} \dim_{U(1)_t} \mathcal{H}[T^2]_{k,s=0} &:= \sum_{w \in \mathbb{Z}} t^w \dim \mathcal{H}[T^2]_{k,s=0}^{\text{weight } w} = |k| + 1 + 2|k|(t + t^2 + t^3 + \dots) \\ &= |k| + 1 + \frac{2|k|t}{1-t}. \end{aligned} \quad (9.2.23)$$

## 9.2.2 Holomorphic polarizations and CFT

Often in geometric quantization of Chern-Simons theory, one uses a holomorphic polarization instead of the real polarization above. In Chern-Simons theory with compact gauge group (*cf.* [53]), this means to choose a complex structure ‘ $\tau$ ’ on a surface  $\Sigma$ , to write the connection one-form as  $A = A_z dz + A_{\bar{z}} d\bar{z}$  in local complex coordinates, and, when quantizing, to define the Hilbert space to consist of sections of the line bundle  $\mathcal{L} \rightarrow \mathcal{P}[\Sigma]$  that are covariantly constant with respect to  $A_{\bar{z}}$ .

Naively, it may appear that choosing such a complex polarization needlessly complicates the problem. However, a complex polarization has three great advantages. First, it allows one to ask analyze the Hilbert space varies with the choice of complex structure. Locally the variation is trivial, expressed formally by saying that the bundle of Hilbert spaces over the space of complex structures (*i.e.* over the Teichmüller space of  $\Sigma$ ) has a projectively flat connection. However, globally, one derives an action of the mapping class group of  $\Sigma$  on the Chern-Simons Hilbert space. Second, and related to this idea, a holomorphic polarization allows one to identify the Hilbert space of Chern-Simons theory with the space of conformal blocks in a particular boundary CFT. In the case of compact Chern-Simons theory, the boundary CFT is a famously WZW model [17]. The projectively flat connection on Teichmüller space is the Knizhnik-Zamolodchikov connection of the CFT. Finally, for generic surfaces  $\Sigma$  a real polarization as above simply isn’t available! Thus, using a holomorphic polarization is the only way to go.

In the case of complex Chern-Simons theory, there are actually multiple choices of complex polarizations. If we write a complex connection and its conjugate as  $\mathcal{A} = \mathcal{A}_z dz + \mathcal{A}_{\bar{z}} d\bar{z}$ ,  $\bar{\mathcal{A}} = \bar{\mathcal{A}}_z dz + \bar{\mathcal{A}}_{\bar{z}} d\bar{z}$ , then we can ask that sections of  $\mathcal{L}$  be covariantly constant with respect to

$$(A) \quad \mathcal{A}_{\bar{z}}, \quad \bar{\mathcal{A}}_z \quad \text{or} \quad (B) \quad (\text{some components of}) \quad \bar{\mathcal{A}}_{\bar{z}}, \quad \bar{\mathcal{A}}_z. \quad (9.2.24)$$

The first choice was analyzed by Witten [5], and leads to a boundary CFT whose conformal blocks must contain contributions from both chiral and anti-chiral sectors. This polarization plays a central role in the relation between  $SL(2, \mathbb{C})$  Chern-Simons theory and quantum Hall systems [42, 54]. The second choice is related to Liouville theory coupled to parafermions [55, 56].

### 9.3 Complex Chern-Simons theory as a TQFT?

Now, having seen very explicitly that complex Chern-Simons Hilbert spaces are infinite-dimensional (and exactly how they're infinite-dimensional), let us think a bit about the properties of partition functions.

For a closed three-manifold  $M$ , it is expected that the complex Chern-Simons partition function takes the form

$$\mathcal{Z}[M]_{k,s} = \sum_{\text{flat } \alpha} \frac{1}{|\text{Stab}(\alpha)|} \mathcal{B}_\alpha(q^{\frac{1}{2}}) \tilde{\mathcal{B}}_\alpha(\tilde{q}^{\frac{1}{2}}). \quad (9.3.1)$$

The sum here is over flat complex connections  $\alpha$  on  $M$ , which are the critical points of the Chern-Simons path integral; and  $\mathcal{B}_\alpha, \tilde{\mathcal{B}}_\alpha$  are holomorphic and antiholomorphic contributions to the path integral from quantum fluctuations around the critical point, with  $q, \tilde{q}$  defined by (9.2.13). The prefactor  $|\text{Stab}(\alpha)|$  is the volume of the stabilizer of  $\alpha$ , *i.e.* the volume of the subgroup of the gauge group that preserves a particular flat connection.

One certainly expects such a formula to be valid perturbatively, due to standard properties of path integrals in quantum field theory. (The perturbative version of (9.3.1) formed the basis for the physical explanation of the Volume Conjecture in [25].) It was argued in [28], however, that the formula is actually valid non-perturbatively as well. Roughly, one should think of (9.3.1) as expanding the integration cycle in the Chern-Simons path integral into a sum of integration cycles  $\Gamma_\alpha$  defined by gradient flow off of each critical point with respect to the Chern-Simons action. The  $\Gamma_\alpha$  can further be written as products<sup>3</sup> of cycles  $\gamma_\alpha \times \tilde{\gamma}_\alpha$  in the space of (holomorphic)  $\times$  (anti-holomorphic) connections, leading to the factorization  $\mathcal{B}_\alpha(q^{\frac{1}{2}}) \tilde{\mathcal{B}}_\alpha(\tilde{q}^{\frac{1}{2}})$ .<sup>4</sup>

For a three-manifold with boundary  $\Sigma$ , the same type of formula holds after properly accounting for boundary conditions. In particular, the sum is over flat connections with a fixed

<sup>3</sup>In general, there could be a nontrivial matrix  $n_{\alpha\beta}$  connecting holomorphic and anti-holomorphic sectors. However, when one considers unitary Chern-Simons theory with an integration contour  $\Gamma$  along which  $\bar{\mathcal{A}}$  is honestly the conjugate of  $\mathcal{A}$ , the matrix is just the identity.

<sup>4</sup>The 3d-3d correspondence relates holomorphic-antiholomorphic factorization in complex Chern-Simons theory to a rather nontrivial statement about lens-space partition functions of 3d  $\mathcal{N} = 2$  theories  $T[M]$  [57].

behavior at  $\Sigma$ , and each summand becomes a wavefunction in  $\mathcal{H}[\Sigma]_{k,s}$ . For example if  $\Sigma = T^2$  is a torus, we would fix A-cycle holonomy eigenvalues  $x, \bar{x}$  of a flat connection as in Section 9.2, and the individual wavefunctions would have the factorized form  $\mathcal{B}_\alpha(x, q^{\frac{1}{2}})\tilde{\mathcal{B}}_\alpha(\bar{x}, \tilde{q}^{\frac{1}{2}})$ .

What can we learn from (9.3.1)? In the best-case scenario, there is a finite number of flat connections on  $M$ , and all the flat connections have finite-volume stabilizers. This would lead to a finite, well-defined (in principle)  $\mathcal{Z}[M]_{k,s}$ . In contrast:

- If a flat connection  $\alpha$  is isolated but its stabilizer has infinite volume, its contribution to (9.3.1) vanishes.
- If flat connections come in a continuous family on which the Chern-Simons action is constant, then the contribution to (9.3.1) can be infinite.

Unfortunately, the best-case scenario never holds, and both of these potentially bad situations can arise. We consider some examples.

If  $M$  is hyperbolic (meaning that it admits a hyperbolic metric), it is expected that there are a finite number of  $SL(2, \mathbb{C})$  flat connections on  $M$ . Intuitively, for hyperbolic  $M$  the fundamental group  $\pi_1(M)$  is sufficiently complicated that the representations  $\pi_1(M) \rightarrow SL(2, \mathbb{C})$  are isolated.<sup>5</sup> Then the partition function is finite. As we discuss in Section 9.4.2, the partition function can actually be computed. However, there is always at least one flat connection  $\alpha_{\text{abel}}$  whose holonomies belong to the maximal torus  $GL(1, \mathbb{C}) \subset SL(2, \mathbb{C})$ . The stabilizer of  $\alpha_{\text{abel}}$  contains constant  $GL(1, \mathbb{C})$ -valued gauge transformations; since  $GL(1, \mathbb{C})$  has infinite volume,  $\alpha_{\text{abel}}$  does not contribute at all to the partition function. This becomes hugely problematic when trying to formulate complex Chern-Simons as a TQFT, as all flat connections must be accounted for during cutting and gluing [44].

There are some simple manifolds whose fundamental group  $\pi_1(M)$  is abelian. For example, if  $M$  is a lens space  $L(p, r) \simeq S^3/\mathbb{Z}_p$ , the fundamental group is  $\mathbb{Z}_p$ . In this case, every single flat connection has holonomy in the maximal torus of the gauge group, the volume of the stabilizer is always infinite, and  $\mathcal{Z}[M]$  vanishes identically.

In the opposite extreme are manifolds  $M$  on which the flat connections are not isolated. In this case, we expect that  $\mathcal{Z}[M]$  diverges. For example, consider  $M = \Sigma \times S^1$ . Then  $\mathcal{M}_{\text{flat}}(G_{\mathbb{C}}, M) = \mathcal{M}_{\text{flat}}(G_{\mathbb{C}}, \Sigma) \times T_{\mathbb{C}}$  (where  $T_{\mathbb{C}}$  is the maximal torus of  $G_{\mathbb{C}}$ ). The partition function is

$$\mathcal{Z}[M]_{k,s} = \text{Tr}_{\mathcal{H}[M]_{k,s}} \mathbf{1} = \dim \mathcal{H}[M]_{k,s} = \infty. \quad (9.3.2)$$

Both the zeroes and infinities appearing here obstruct the definition of consistent cutting and gluing rules needed to make Chern-Simons theory a TQFT. The zeroes and infinities have to be regularized. While no systematic approach to regularization has been formulated so far, there are exist several promising and exciting proposals. Almost all of them are motivated by string/M-theory and the 3d-3d correspondence.

---

<sup>5</sup>On hyperbolic  $M$ , one particular flat  $SL(2, \mathbb{C})$  connection — the one corresponding to the global hyperbolic metric — is well known to be isolated [58, 59]. Computational experiments suggest that in fact all flat connections  $SL(2, \mathbb{C})$  are isolated, but there exists no general proof of this statement.

### 9.3.1 Symmetries, regularizations, and the 3d-3d correspondence

In principle, the 3d-3d correspondence itself may suffice to resolve the difficulties with cutting and gluing in complex Chern-Simons theory.<sup>6</sup> The correspondence assigns to a closed 3-manifold  $M$  and a Lie algebra  $\mathfrak{g}$  of type *ADE* (and a bit of extra discrete data) a three-dimensional field theory  $T_G[M]$  with the property that that

$$\begin{aligned} & \text{partition function of } T_G[M] \text{ on squashed lens space } L(k, 1)_b \\ &= G_{\mathbb{C}} \text{ Chern-Simons partition function } \mathcal{Z}[M]_{k,s} \text{ with } is = k \frac{1-b^2}{1+b^2}. \end{aligned} \tag{9.3.3}$$

where  $\mathfrak{g} = \text{Lie}(G)$ . When  $G_{\mathbb{C}} = SL(N, \mathbb{C})$ , the theory  $T_{G_{\mathbb{C}}}[M]$  is the effective low-energy worldvolume theory of  $N$  M5 branes compactified on  $M$ ; the branes wrap  $M \times \mathbb{R}^3$  in the M-theory geometry  $T^*M \times \mathbb{R}^5$ . Similarly, the correspondence assigns to a three-manifold  $M$  with boundary  $\Sigma$  a boundary condition  $T_G[M]$  for the four-dimensional theory  $T_G[\Sigma]$  of class  $\mathcal{S}$  [62, 63].

Typically  $T_G[M]$  is an  $\mathcal{N} = 2$  superconformal theory, though both supersymmetry and conformal invariance might be broken. Unfortunately, it is not completely understood what conditions on  $M$  guarantee  $\mathcal{N} = 2$  superconformal theories. We assume for the present heuristic argument that we do have  $\mathcal{N} = 2$  superconformal theories.

The basic idea, then, would be to replace  $G_{\mathbb{C}}$  Chern-Simons theory on  $M$  with  $T_{G_{\mathbb{C}}}[M]$ , which is a much more powerful object. Even when the Chern-Simons partition functions  $\mathcal{Z}[M]_{k,s}$  (equivalently, lens-space partition functions of  $T_G[M]$ ) are ill-defined, the theory  $T_G[M]$  itself should still make sense. Moreover, the theories  $T_G[M]$  obey cutting and gluing rules. Gluing  $M = N_1 \cup_{\Sigma} N_2$  corresponds to “sandwiching” the four-dimensional theory  $T_G[\Sigma]$  between boundary conditions  $T_G[N_1]$  and  $T_G[N_2]$ , and colliding the boundaries together to produce a new effective theory  $T_G[N_1 \cup_{\Sigma} N_2]$ . In this way, we reproduce the structure of a three-dimensional TQFT. If we should ever want to recover Chern-Simons partition functions, we just place the superconformal theories on a lens space  $L(k, 1)_b$ .

There are two practical difficulties with this proposal that will hopefully be overcome soon. First, the full theories  $T_G[M]$  are not actually known for most manifolds, for any nonabelian  $G$ . A construction using ideal triangulations was outlined in [14, 38] (also [64, 65]); however, that construction produces subsectors of the full theories  $T_G[M]$  that are missing some branches of vacua, the same way partition functions of Chern-Simons theory on hyperbolic manifolds are “missing” abelian flat connections. Examples of complete theories  $T_G[M]$  for a handful of manifolds (including a hyperbolic one) were postulated in [44], and theories for lens spaces  $M = L(p, r)$  were studied in [23, 24, 44].

The second difficulty, or potential shortcoming, is that zeroes and infinities still remain in the actual Chern-Simons partition functions. Here, however, another solution presents itself: the theories  $T_G[M]$  often have extra symmetries; and parameters associated to these symmetries (twisted masses or fugacities) can be used to refine the squashed-lens-space  $L(k, 1)_b$  partition functions of  $T_G[M]$  — thus literally regularizing the Chern-Simons zeroes and infinities.

---

<sup>6</sup>We will not review the 3d-3d correspondence here. For recent reviews and discussions, especially in the context of Chern-Simons theory and TQFT, see [23, 24, 44, 60] as well as the related [61].

We already met one such symmetry in Section 9.2.1: the  $U(1)_t$  that gave an equivariant quantization of the Hilbert space  $\mathcal{H}[\Sigma]_{k,s=0}$ . Via the 3d-3d correspondence, this Hilbert space is mapped to the BPS Hilbert space of the 4d class- $\mathcal{S}$  theory  $T_G[\Sigma]$  on  $\mathbb{R} \times L(k, 1)_{b=1}$ . This 4d theory has an additional R-symmetry  $U(1)_t$  that commutes with the supercharge used to define the “BPS” Hilbert space, and provides the  $U(1)_t$  grading.

Similarly, the three-dimensional theory  $T_G[\Sigma \times S^1]$  (obtained by compactifying  $T_G[\Sigma]$  on a circle) has  $\mathcal{N} = 4$  rather than  $\mathcal{N} = 2$  supersymmetry. The larger R-symmetry group of the  $\mathcal{N} = 4$  theory contains  $U(1)_t$ , and including its twisted mass in partition functions leads to finite answers that encapsulate the graded dimension (9.2.23).

Theories  $T_G[M]$  for Seifert-fibered three-manifolds  $M$  should also retain this  $U(1)_t$  symmetry. In this case, it can ultimately be traced back to an exceptional isometry<sup>7</sup> of the  $M$ -theory geometry  $T^*M \times \mathbb{R}^5$ . A simple example of such a manifold is a lens space  $M = L(p, r)$ , whose refined partition functions were analyzed in [24], and put precisely into the factorized form (9.3.1) — with the factors  $1/|\text{Stab}(\alpha)| = 1/\infty$  now regularized.

When  $M$  is generic (*e.g.* hyperbolic) this exceptional  $U(1)_t$  symmetry is, unfortunately, absent. It was nevertheless proposed in [44] that there exists yet *another* symmetry  $U(1)_{t'}$  in any theory  $T_G[M]$ , related to the standard  $U(1)$  R-symmetry of three-dimensional  $\mathcal{N} = 2$  theories — as well as to categorification of colored knot polynomials. This  $U(1)_{t'}$  was used to regularize Chern-Simons partition functions for the trefoil and figure-eight knot complements (Seifert-fibered and hyperbolic manifolds, respectively), producing sums of the form (9.3.1) that included all flat connections, even abelian ones.

## 9.4 Three connections to three-manifold topology

As discussed in Section 9.3, the partition function of Chern-Simons theory with gauge group  $G_{\mathbb{C}}$  will take a finite, well-defined value on manifolds  $M$  that only admit finitely many flat  $G_{\mathbb{C}}$  connections. For  $G_{\mathbb{C}} = SL(2, \mathbb{C})$  and possibly  $G_{\mathbb{C}} = SL(N, \mathbb{C})$ , hyperbolic manifolds are expected to be of this type. (Indeed, there exist systematic computations of partition functions for hyperbolic manifolds with boundary of genus  $\geq 1$ .) One may then try to relate properties of the partition function with the topology of  $M$ . We proceed to outline some of the more striking relations. In each case, M-theory and/or the 3d-3d correspondence provides valuable insight.

### 9.4.1 Hyperbolic volumes, twisted torsion, and large $N$

The most fundamental relation between complex Chern-Simons theory and hyperbolic geometry has been understood for a long time, and concerns the semi-classical asymptotic expansion of partition functions [3] (see also [25, 67]). It is easiest to formulate it first in terms of the “holomorphic blocks”  $\mathcal{B}_\alpha, \tilde{\mathcal{B}}_\alpha$  appearing in (9.3.1), labelled by flat connections

---

<sup>7</sup>This very same symmetry played a central role in defining refined (compact) Chern-Simons theory on Seifert-fibered manifolds [66].

$\alpha$  :

$$\begin{aligned} \text{as } k + is \rightarrow \infty \text{ or } q^{\frac{1}{2}} = e^{\frac{2\pi i}{k+is}} \rightarrow 1, \quad \mathcal{B}_\alpha(q^{\frac{1}{2}}) &\sim \sqrt{\frac{4\pi^3}{\tau(\alpha)}} e^{\frac{i(k+is)}{8\pi} S_{CS}(\alpha)}; \\ \text{as } k - is \rightarrow \infty \text{ or } \tilde{q}^{\frac{1}{2}} = e^{\frac{2\pi i}{k-is}} \rightarrow 1, \quad \tilde{\mathcal{B}}_\alpha(\tilde{q}^{\frac{1}{2}}) &\sim \sqrt{\frac{4\pi^3}{\tau(\alpha)^*}} e^{\frac{i(k-is)}{8\pi} S_{CS}(\alpha)^*}; \end{aligned} \quad (9.4.1)$$

where  $S_{CS}(\alpha)$  is the classical Chern-Simons action evaluated on a particular flat connection and  $\tau(\alpha)$  is the analytic Ray-Singer torsion twisted by the flat connection  $\alpha$  [68]. This is the standard result expected from Chern-Simons perturbation theory [69]. In the presence of a boundary, the classical action and torsion on the RHS depend on the choice of boundary conditions (boundary holonomies) for  $\alpha$ . From (9.3.1), it then follows that if both  $k + is \rightarrow \infty$  and  $k - is \rightarrow \infty$

$$\mathcal{Z}[M]_{k,s} \sim \sum_{\text{flat } \alpha} \frac{1}{|\text{Stab}(\alpha)|} \frac{4\pi^3}{|\tau(\alpha)|} e^{\frac{ik}{4\pi} \text{Re } S_{CS}(\alpha) - \frac{is}{4\pi} \text{Im } S_{CS}(\alpha)}. \quad (9.4.2)$$

The formula is particularly meaningful if  $s$  is analytically continued to (say) positive imaginary values. Then each term in (9.4.2) shows exponential growth or decay at large  $|s|$ , controlled by  $\text{Im } S_{CS}(\alpha)$ .

Now suppose that  $M$  is hyperbolic, meaning that it admits a hyperbolic metric. The hyperbolic metric is unique (given suitable boundary conditions) and is a topological invariant of  $M$  [58, 59]. Moreover, the vielbein and spin connection of the hyperbolic metric can be rewritten as a flat  $SL(2, \mathbb{C})$  connection  $\alpha_{\text{hyp}} = w + ie$ , with the property that  $\text{Im } S_{CS}(\alpha_{\text{hyp}}) = \text{Vol}(M)$  is the hyperbolic volume of  $M$ . The real part  $\text{Re } S_{CS}(\alpha_{\text{hyp}})$  is known as the Chern-Simons invariant of the hyperbolic structure, and provides a natural complexification of the hyperbolic volume [70, 71]. It is also useful to note that the connection  $\alpha_{\text{hyp}}$  necessarily has a trivial stabilizer – the connection is fundamentally non-abelian.

Therefore, if the gauge group is  $SL(2, \mathbb{C})$  and  $M$  is hyperbolic, the sum (9.4.2) contains a term that is controlled by the hyperbolic volume of  $M$ . Typically,  $\text{Im } S_{CS}(\alpha_{\text{hyp}})$  is larger than the “volume” of any other flat connection, and the entire sum (9.4.2) is dominated by the hyperbolic volume. (It is expected that  $\text{Im } S_{CS}(\alpha_{\text{hyp}})$  always dominates, but no general result of this type has been proven.)

It is often useful to strip off the holomorphic part of the asymptotic expansion. This can be done by taking a *singular* limit: we fix  $k = 1$ , analytically continue  $s$  to imaginary values, and send  $s \rightarrow -ik = -i$ . This has the effect of sending  $q \rightarrow 1$  but  $\tilde{q} \rightarrow 0$ , which trivializes the anti-holomorphic blocks,  $\tilde{\mathcal{B}}_\alpha(\tilde{q}^{\frac{1}{2}}) \rightarrow 1$ . In this singular limit, we expect

$$\mathcal{Z}[M]_{1,s} \sim \sum_{\text{flat } \alpha} \frac{1}{|\text{Stab}(\alpha)|} \sqrt{\frac{4\pi^3}{\tau(\alpha)}} e^{-\frac{1}{\hbar} S_{CS}(\alpha)} \quad \text{as } \hbar = 2\pi i \frac{1 - is}{1 + is} \rightarrow 0. \quad (9.4.3)$$

This sort of limit played a major role in early analyses of partition functions for complex Chern-Simons theory [49, 72], though it was not realized at the time that the partition functions (derived from quantum Teichmüller theory) being analyzed had fixed level  $k = 1$ .

The fact that the perturbative expansion of complex Chern-Simons theory (or individual holomorphic blocks, as in (9.4.1)) contains geometric invariants of  $M$  played a major role in providing a physical justification for the Volume Conjecture, and generalizing it. The original Volume Conjecture [26, 27] claims that a particular double-scaling limit of colored Jones polynomials of a knot  $K \subset S^3$  leads to exponential growth, controlled by the hyperbolic volume of the knot complement  $\text{Vol}(S^3 \setminus K)$ . This was justified in [25] by embedding  $SU(2)$  Chern-Simons theory (which computes colored Jones polynomials) into a holomorphic sector of  $SL(2, \mathbb{C})$  Chern-Simons theory, and arguing that the asymptotic expansions of  $SU(2)$  and (holomorphic)  $SL(2, \mathbb{C})$  theories should coincide. The argument immediately led to generalizations, involving higher-order terms in the asymptotic expansion and a dependence on boundary conditions, which have been carefully checked in many computations, cf. [49, 67, 73].

It is also interesting to consider “large- $N$ ” limits in complex Chern-Simons theory, taking the gauge group to be  $SL(N, \mathbb{C})$  and sending  $N \rightarrow \infty$ . Physically, such limits are most conveniently studied by realizing Chern-Simons theory on a stack of  $N$  M5 branes (Section 9.3.1), and using AdS/CFT or large- $N$  duality. A study of the five-brane system [74–76] predicts that the leading asymptotic growth of the partition function  $\mathcal{Z}[M]_{k,s}$  as in (9.4.2) scales as  $N^3 \text{Vol}(M)$  at large  $N$  [38]. This is not surprising: the hyperbolic flat  $SL(2, \mathbb{C})$  connection can be embedded into  $SL(N, \mathbb{C})$  by using the  $N$ -dimensional representation  $\rho_N : SL(2, \mathbb{C}) \rightarrow SL(N, \mathbb{C})$ , and the Chern-Simons functional evaluates to  $\sim N^3 \text{Vol}(M)$  on  $\rho_N(\alpha_{\text{hyp}})$ , cf. [77]. As long as (9.4.2) is dominated by the flat connection  $\rho_N(\alpha_{\text{hyp}})$  for any  $N$ , one quickly recovers the scaling prediction. Much more non-trivially, the M-theory analysis predicts that the logarithm of the *torsion*  $\tau(\rho_N(\alpha_{\text{hyp}}))$  will grow as  $N^3 \text{Vol}(M)$  [78, 79] at large  $N$  as well. This latter result was recently proved by Porti and Menal-Ferrer [80].

## 9.4.2 State-integral models and angle structures

When  $M = S^3 \setminus K$  is an oriented hyperbolic knot or link complement (or, more generally, an oriented hyperbolic manifold with non-empty boundary of genus  $\geq 1$ ), there exists a systematic construction of  $SL(2, \mathbb{C})$  Chern-Simons partition functions  $\mathcal{Z}[M]_{k,s}$  for all levels  $k, s$ . The full definition of these partition functions appears in [81, 82] for  $k = 0$ , and [21, 22] for  $k \neq 0$ , respectively. It is a culmination of much previous work, including [19, 49, 72, 83, 84] for  $k = 1$ ; [20] for  $k = 0$  (and indirectly [85–87]); and (indirectly, via 3d-3d correspondence) [88, 89] for  $k > 1$ . The definition extends to  $SL(N, \mathbb{C})$  using techniques of [38].

The construction of these partition functions uses a topological ideal triangulation of the three-manifold  $M = \cup_{i=1}^N \Delta_i$ . This is a tiling of  $M$  by truncated tetrahedra  $\Delta_i$ , as in Figure 9.4.1, such that 1) various pairs of large hexagonal faces are glued together; but 2) the small triangles at the truncated vertices are left untouched, and become part of the boundary  $\partial M$ .

One then proceeds in standard TQFT fashion. For gauge group  $SL(2, \mathbb{C})$  (or more precisely,  $PSL(2, \mathbb{C})$ ), the boundary of each tetrahedron is assigned a Hilbert space  $\mathcal{H}[\partial\Delta]_{k,s} \simeq L^2(\mathbb{R}) \otimes \mathbb{C}^k$ . The Hilbert space comes from quantizing an open subset of the space of flat connections on  $\partial\Delta$ , viewed as a four-punctured sphere; in this case  $\mathcal{P}[\partial\Delta]^{\text{open}} \simeq \mathbb{C}^* \times \mathbb{C}^*$ , and the quantization of Section 9.2 applies in a straightforward manner, with no Weyl quotient.

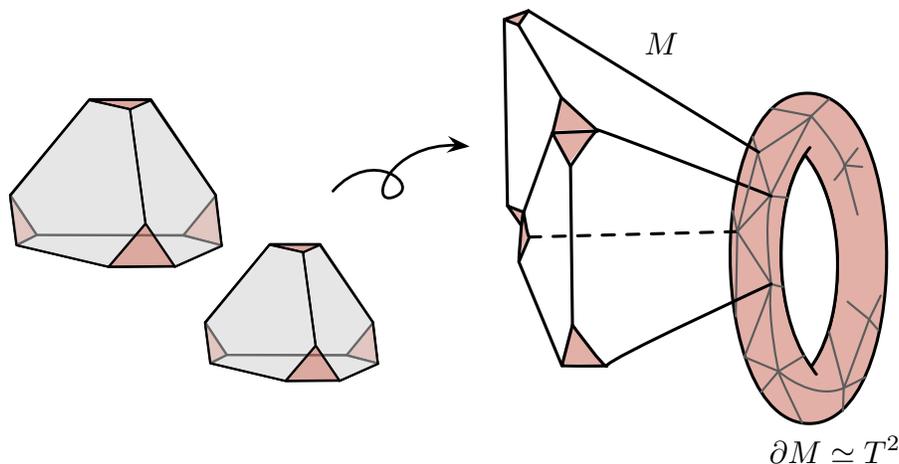

Figure 9.4.1: Ideal (*i.e.* truncated) tetrahedra, glued together along their large hexagonal faces to form an ideal triangulation of a knot complement  $M$ . The small triangular faces at truncated vertices become part of the boundary of  $M$ .

Each tetrahedron is assigned a canonical partition function  $\mathcal{Z}[\Delta]_{k,s} \in \mathcal{H}[\partial\Delta]_{k,s}$ , which has the form of a “quantum dilogarithm” function; for  $|k| \geq 1$ , this is

$$\mathcal{Z}[\Delta_i]_{k,s}(\mu_i, m_i) = \prod_{r=0}^{\infty} \frac{1 - q^{1+r} z_i^{-1}}{1 - \tilde{q}^{-r} \bar{z}_i^{-1}}, \quad (9.4.4)$$

with  $q, \tilde{q}$  as in (9.2.13) or (9.2.20) and  $z_i = e^{\frac{2\pi b}{k} \mu_i - \frac{2\pi i}{k} m_i}$ ,  $\bar{z}_i = e^{\frac{2\pi b^{-1}}{k} \mu_i + \frac{2\pi i}{k} m_i}$  as in (9.2.9). (For  $k = 0$ , see Section 9.4.3.)

The partition function  $\mathcal{Z}[M]_{k,s}$  is then obtained by taking a product  $\prod_{i=1}^N \mathcal{Z}[\Delta_i]_{k,s}(\mu_i, m_i)$ , and integrating out all pairs of variables  $(\mu_i, m_i)$  associated to the interior of  $M$ , leaving behind some variables associated to the boundary. It is slightly tricky to describe this operation in precise terms, because the tetrahedron Hilbert space  $\mathcal{H}[\partial\Delta]_{k,s}$  does not easily factorize into contributions from the tetrahedron’s four large faces.<sup>8</sup> The right prescription comes from viewing gluing in TQFT somewhat more globally, as a quantum symplectic reduction. It turns out that the combinatorics of ideal triangulations have some fundamental symplectic properties, first discovered by Neumann and Zagier [90,91], that allow the quantum symplectic reduction to be defined.

As an example, take  $M = S^3 \setminus K$  to be a knot complement. In this case, there is a canonical “A-cycle” on the boundary torus  $\partial M = T^2$ , defined by a small loop linking the knot  $K$  in  $S^3$  (called the meridian cycle); and there is a canonical boundary condition for  $SL(2, \mathbb{C})$  connections, defined by requiring their holonomy along the meridian cycle to have trivial eigenvalues. (Crucially, this does not require the actual holonomy to be trivial; in  $SL(2, \mathbb{C})$

<sup>8</sup>The Hilbert space *can* be factorized by introducing some redundant degrees of freedom [19], in a manner directly analogous to Kashaev’s quantization of Teichmüller space [40].

there are parabolic matrices  $\begin{pmatrix} 1 & \\ & 1 \end{pmatrix}$  with trivial eigenvalues.) In the notation of Section 9.2, the boundary condition sets  $x = \bar{x} = 1$ , or restricts functions  $f(\mu, m) \in \mathcal{H}[T^2]_{k,s}$  to their values at  $\mu = m = 0$ . Suppose that the knot complement is glued from  $N$  tetrahedra  $\Delta_i$ . The combinatorics of the triangulation define a “Neumann-Zagier datum”

$$\mathbf{A}, \mathbf{B} \in \text{Mat}_{N \times N}(\mathbb{Z}), \quad \nu, \in \mathbb{Z}^N \quad (9.4.5)$$

consisting of two  $N \times N$  integer matrices  $\mathbf{A}, \mathbf{B}$  (that encode adjacency relations for edges of the tetrahedra and satisfy the symplectic property  $\mathbf{A}\mathbf{B}^T - \mathbf{B}\mathbf{A}^T = I_{N \times N}$ ) and a vector  $\nu$  of  $N$  integers. A precise definition is given in [73]. Then the partition function  $\mathcal{Z}[M]_{k,s} = \mathcal{Z}[M]_{k,s}(0, 0)$  with the canonical boundary condition takes the concise form [35]

$$\mathcal{Z}[M]_{k,s} = \frac{C}{k^N \sqrt{\det \mathbf{B}}} \sum_{m \in (\mathbb{Z}/k\mathbb{Z})^N} \int d^N \mu (-\zeta^{\frac{1}{2}})^{m\mathbf{B}^{-1}\mathbf{A}m} e^{-\frac{i\pi}{k} \mu \mathbf{B}^{-1} \mathbf{A} \mu - \frac{\pi}{k} (b+b^{-1}) \mu \mathbf{B}^{-1} \nu} \prod_{i=1}^N \mathcal{Z}[\Delta]_{k,s}(\mu_i, m_i), \quad (9.4.6)$$

with  $\zeta = e^{\frac{2\pi i}{k}}$ . The prefactor  $C = \zeta^{\frac{1}{4}} f \mathbf{B}^{-1} \nu e^{\frac{i\pi}{4k} (b^2 - b^{-2})} f \mathbf{B}^{-1} \nu$  depends on an integer solution  $(f, f'') \in \mathbb{Z}^{2N}$  to  $\mathbf{A}f + \mathbf{B}f'' = \nu$ .

There are several things to note about this partition function:

- It approximately takes the form of a “state sum” or “state integral,” with the partition function (9.4.4) assigned to every tetrahedron building-block. The “state variables”  $m_i \in \mathbb{Z}/k\mathbb{Z}$  and  $\mu_i$  are summed/integrated over. The number of sums/integrals is the same as the number of tetrahedra which is also the same as the number of internal edges in the triangulation.
- As explained in [22, 35], the partition function is only defined up to an overall phase, of the form  $\zeta^{\frac{a}{24}} e^{\frac{i\pi}{12k} (a'b^2 + a''b^{-2})}$ ,  $a, a', a'' \in \mathbb{Z}$ . This subsumes the standard *framing ambiguity* in complex Chern-Simons theory [5], which would modify the partition function by a factor of  $e^{-\frac{i\pi}{2k} (b+b^{-1})^2}$  upon shifting the framing of the tangent bundle of  $M$ .
- Each tetrahedron building-block manifestly admits a holomorphic-antiholomorphic factorization as in (9.3.1). The full partition function is also expected to admit such a factorization; this was demonstrated for some simple examples in [22]. (See also [57, 92] for  $k = 0$ ,  $k = 1$  examples.)
- Perhaps most interestingly, the precise definition of the integration contour in (9.4.6) and the convergence of the integral depends crucially on the existence of a *positive angle structure* on the triangulation being used. This is ultimately what restricts the computation to a particular class of 3-manifolds that includes all hyperbolic ones. It also beautifully makes contact with the three-dimensional superconformal theory  $T[M]$  defined combinatorially in [14] using an ideal triangulation — the definition of  $T[M]$  does not make sense (cannot produce a superconformal theory) unless a positive angle structure exists. We proceed to explain this idea momentarily.

- Via the 3d-3d correspondence, the integral (9.4.6) has a dual interpretation as a partition function of  $T[M]$  on the lens space  $S^3/\mathbb{Z}_k$ . This partition function is computed by localization methods, as in Section 4.1 of B. Willett’s article, Chapter 6. Each  $\mathcal{Z}[\Delta]_{k,s}(\mu_i, m_i)$  is the contribution of a chiral multiplet to the partition function, and the additional prefactor comes from background Chern-Simons terms involving flavor and R-symmetries.
- Changes of ideal triangulations are generated by 2–3 Pachner moves, which replace a pair of tetrahedra glued along a common face by a triplet glued along three common faces and a central edge. The state-integral (9.4.6) is invariant under 2–3 moves that preserve the positive or non-negative angle structure (as appropriate), due to a 5-term integral identity for the quantum dilogarithm (9.4.4). In the case  $k = 1$ , this identity was first discovered by Faddeev [93] (see also [94]).

An angle structure on a topological ideal triangulation is an assignment of real parameters (“angles”) to the six long edges of each tetrahedron, in such a way that 1) angles on opposite edges are equal (leaving three angles  $\alpha_i, \alpha'_i, \alpha''_i$  per tetrahedron  $\Delta_i$ ); 2) the sum of angles around any tetrahedron vertex equals  $\pi$  (thus  $\alpha_i + \alpha'_i + \alpha''_i = \pi$ ); and 3) the sum of angles around every internal edge in the triangulation equals  $2\pi$ . In terms of the Neumann-Zagier gluing datum (9.4.5) for a knot complement, the last condition translates to<sup>9</sup>

$$\mathbf{A}\alpha + \mathbf{B}\alpha'' = \pi\nu. \quad (9.4.7)$$

The idea of an angle structure is motivated by hyperbolic geometry. In an ideal triangulation by *hyperbolic* tetrahedra, the dihedral angles precisely obey the three conditions above [59].

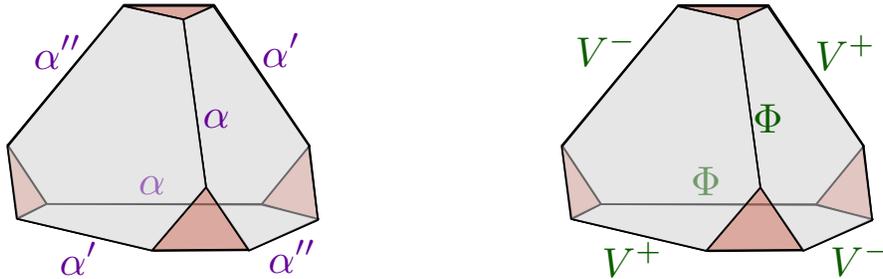

Figure 9.4.2: Left: dihedral angles assigned to edges of an oriented ideal tetrahedron, obeying  $\alpha + \alpha' + \alpha'' = \pi$ . Right: operators of the tetrahedron theory  $T[\Delta]$  assigned to the same edges; these operators have R-charges  $\rho, \rho', \rho''$  that obey  $\rho + \rho' + \rho'' = 1$ .

A positive (respectively, non-negative) angle structure is one where all angles additionally obey  $\alpha_i, \alpha'_i, \alpha''_i > 0$  ( $\geq 0$ ). An oriented hyperbolic three-manifold with genus-one boundary

<sup>9</sup>Technically, only  $N-1$  out of the  $N$  components of (9.4.7) correspond to internal edges; the last component of (9.4.7) relates to a boundary condition at  $\partial M = T^2$ , and can be removed from the angle-structure analysis. We are bypassing such subtleties in this heuristic discussion.

always admits an triangulation with non-negative dihedral angles, hence there a triangulation with a non-negative angle structure [95]. It is conjectured and strongly believed that the same holds for strictly positive angle structures. (As evidence for this, the default triangulations produced by the computer program `SnapPy` [96] for the first few thousand hyperbolic knot complements all admit positive angle structures.)

It was shown in [81,82] that analogue of the partition function (9.4.6) at  $k = 0$  (*cf.* Section 9.4.3) is well-defined when the triangulation admits a non-negative angle structure. Similarly, it was shown in [19] for  $k = 1$  and [21, 22] for  $|k| \geq 1$  that the partition function (9.4.6) is well defined if the triangulation admits a positive angle structure. In each case, the angle structure specifies a canonical convergent integration contour.

The combinatorial construction of theories  $T[M]$  given in [14] translates the ingredients of the state-integral (9.4.6) to operations in three-dimensional  $\mathcal{N} = 2$  gauge theories. One starts by associating a theory  $T[\Delta_i]$  containing a single chiral multiplet  $\Phi_i$  (*i.e.* a free complex boson  $\phi_i$  and a complex fermion  $\psi_i$ ) to each tetrahedron. In addition to the chiral (BPS) operator  $\Phi_i$ , the theory  $T[\Delta_i]$  contains two elementary chiral monopole operators  $V_i^\pm$ , which exist only in the presence of a monopole background for the flavor symmetry of the theory.<sup>10</sup> Geometrically, the three operators  $\Phi_i, V_i^+, V_i^-$  are associated to three pairs of  $\Delta_i$ , as on the RHS of Figure 9.4.2. Moreover,  $T[\Delta_i]$  has an R-symmetry<sup>11</sup>  $U(1)_R$  that rotates  $(\phi_i, \psi_i)$  with charges  $(\rho_i, \rho_i - 1)$  for some (undetermined)  $\rho_i \in \mathbb{R}$ . One usually just says that  $\Phi_i$  has R-charge  $\rho_i$ . The other BPS operators  $V_i^+, V_i^-$  have some R-charges  $\rho'_i, \rho''_i$ , subject to a single relation  $\rho_i + \rho'_i + \rho''_i = 1$ .

Even for the theory of a single tetrahedron, R-charges are beginning to look like angles, and it is tempting to identify  $\rho_i = \alpha_i/\pi$  (etc.). The analogy persists upon gluing. The theory  $T[M]$  of [14] is defined by taking a tensor product of  $N$  tetrahedron theories  $\otimes_{i=1}^N T[\Delta_i]$ , gauging some flavor symmetries, and (most importantly here) adding superpotential interactions  $W = \sum_{E=1}^N \mathcal{O}_E$  containing a chiral operator  $\mathcal{O}_E$  for every internal edge  $E$  of the triangulation  $M = \cup_{i=1}^N \Delta_i$ . If all the tetrahedron edges identified with  $E$  are labelled by elementary chiral fields  $\Phi_i$ , one simply constructs  $\mathcal{O}_E$  as a product  $\prod_i \Phi_i$  of these surrounding fields. For edges identified with monopole operators, the prescription is more subtle. In either case, one finds that the R-charge of  $\mathcal{O}_E$  is a sum of the R-charges  $\rho_i, \rho'_i$ , or  $\rho''_i$  associated to operators on the tetrahedron edges identified with  $E$ . The superpotential breaks  $U(1)_R$  R-symmetry unless the charge of every  $\mathcal{O}_E$  is exactly 2.

Now, in order for the gauge theory  $T[M]$  to flow (in a straightforward way) to a superconformal theory in the infrared, two conditions are necessary: 1) some  $U(1)_R$  R-symmetry must be preserved; and 2) there must exist a choice of  $U(1)_R$  symmetry such that the charges of all chiral operators are non-negative, because in a superconformal theory R-charges are proportional to operator dimensions. This means that we must be able to choose  $\rho_i, \rho'_i, \rho''_i$  for

<sup>10</sup>One does not usually talk about “flavor” monopole operators like  $V_i^\pm$ , but they are essential in the construction of theories  $T[M]$ , and the relation between these theories and geometry. They can easily be seen in the generalized index of a free chiral multiplet [87], and can also be understood as ordinary monopole operators if the flavor symmetry of  $T[\Delta_i]$  were weakly gauged.

<sup>11</sup>This is a global symmetry that does not commute with supersymmetry, and is related to an  $SO(2)$  automorphism of the 3d  $\mathcal{N} = 2$  SUSY algebra.

individual tetrahedra in such a way that the sums of these charges around any internal edge  $E$  is 2, and all these charges are non-negative. Together with the relation  $\rho_i + \rho'_i + \rho''_i = 1$ , the conditions become equivalent to the existence of a non-negative angle structure.

### 9.4.3 Embedded surfaces and M2 branes in the 3d index ( $k = 0$ )

The partition function of complex Chern-Simons theory at level  $k = 0$  is rather special. Via the 3d-3d correspondence, it takes the form of a supersymmetric index [20]. Schematically:

$$\mathcal{Z}[M]_{k=0,s} = \mathcal{Z}[T[M] \text{ on } S^2 \times_q S^1] = \text{Tr}_{\mathcal{H}[T[M] \text{ on } S^2]} (-1)^R q^{\frac{R}{2} + J_3}, \quad (9.4.8)$$

with  $q = \exp \frac{4\pi}{s}$  as usual. Here  $S^2 \times_q S^1$  denotes a geometry that is fibered over  $S^1$ , in such a way that  $S^2$  rotates around an axis (by an amount  $\pi/s$ ) as  $S^1$  is traversed. Just as in our discussion around (9.3.2), the partition function of any quantum field theory in such a geometry can be expressed as a trace. In this case, it becomes a trace over the Hilbert space of  $T[M]$  on  $S^2$ , weighted by the spin ( $J_3$ ) and R-charge ( $R$ ) of states. Due to the factor  $(-1)^R$ , this trace behaves like an Euler character (physically, a Witten index [97]). In particular, only “BPS states” in the cohomology of a particular supercharge contribute. While the “BPS sector” of the Hilbert space containing such states is infinite-dimensional, it is expected to have finite  $q$ -graded dimension when  $M$  is sufficiently nice (*e.g.* hyperbolic), so that (9.4.8) produces a well-defined formal Laurent series in  $q$ . Less obviously, if  $T[M]$  is a superconformal theory, then superconformal symmetry requires the existence of an R-charge assignment such that only non-negative powers of  $q$  appear in (9.4.8) [20].

In the case that  $T[M]$  is superconformal, one can also use the state-operator correspondence to recast the RHS of (9.4.8) as a sum over BPS *operators* of  $T[M]$  rather than states. Then the index counts the number of operators with given spin and R-charge. Combining this perspective with the 3d-3d correspondence really makes the geometry of  $M$  come to life, in the following way.

Recall that for gauge group  $G_{\mathbb{C}} = SL(N, \mathbb{C})$ , the theory  $T[M]$  is the effective theory of  $N$  M5 branes wrapped on  $M \times \mathbb{R}^3$  inside the eleven-dimensional background  $T^*M \times \mathbb{R}^5$ . From this perspective, at least some of the BPS operators in  $T[M]$  should come from M2 branes that end on the stack of M5 branes, such that their boundary  $\partial(\text{M2}) = \Sigma \times \{0\} \subset M \times \mathbb{R}^3$  wraps a surface in  $M$ . One might therefore expect that

$$\text{The index } \mathcal{Z}[M]_{k=0,s} \text{ “counts” surfaces in } M. \quad (9.4.9)$$

Alternatively, we may think of  $T[M]$  as the effective theory obtained by compactifying the 6d (2,0) theory of type  $A_{N-1}$  on  $M$ . The local BPS operators of  $T[M]$  can come from 1) local operators of the 6d theory; or 2) surface operators in the 6d theory, corresponding to the boundaries of M2 branes in the M-theory picture above. Thus, a more refined statement of (9.4.9) would be that the index counts surfaces in  $M$  decorated by local operators.

The first hint that (9.4.9) could be true came in work of Gukov, Gadde, and Putrov [98]. They investigated the index for knot complements  $M = S^3 \setminus K$ , and found contributions from boundary-incompressible surfaces. These are incompressible surfaces  $\Sigma$  whose boundary

$\partial\Sigma = S^1 \subset \partial M$  wraps a particular nontrivial cycle on the torus boundary of  $M$ . The corresponding operators  $\mathcal{O}_\Sigma$  and all of their powers  $\mathcal{O}_\Sigma^2, \mathcal{O}_\Sigma^3, \dots$  (corresponding to multiply-wrapped surfaces) are expected to contribute to the index, and this is exactly what [98] found.

To make a more precise statement, we should recall that the index  $\mathcal{Z}[M]_{k=0,s}(m, n)$  of a knot complement depends on two integers  $m, n$ , as in (9.2.19). On one hand, these integers are magnetic and electric (flavor) charges in the space of local BPS operators of  $T[M]$ . On the other hand, these charges label homology classes  $(m, n) \in H_1(\partial M, \mathbb{Z})$ . For an operator  $\mathcal{O}_\Sigma$  corresponding to a surface in  $M$ , the charges  $(m_\Sigma, n_\Sigma)$  measure the homology class of the boundary curve  $\partial\Sigma \subset \partial M$ .

In the case of a boundary-incompressible surface  $\Sigma$ , the expectation is that the operator  $\mathcal{O}_\Sigma$  preserves not one but two supercharges. This implies that if  $\mathcal{O}_\Sigma$  has  $\frac{R}{2} + J_3 = Q_\Sigma$ , so that it contributes  $q^{Q_\Sigma}$  to the index in some charge sector  $(m_\Sigma, n_\Sigma)$ , then the  $d$ -th power  $\mathcal{O}_\Sigma^d$  has  $\frac{R}{2} + J_3 = dQ_\Sigma$  and contributes  $q^{dQ_\Sigma}$  to the index in charge sector  $(dm_\Sigma, dn_\Sigma)$ . One can therefore detect the presence of such operators in the index because they force the minimal power of  $q$  appearing in  $\mathcal{Z}[M]_{k=0,s}(dm, dn)$  to grow linearly as  $d \rightarrow \infty$  whenever  $(m, n)$  coincides with the charge  $(m_\Sigma, n_\Sigma)$  of an incompressible surface. In contrast, for generic  $(m, n)$ , the growth of  $\mathcal{Z}[M]_{k=0,s}(dm, dn)$  as  $d \rightarrow \infty$  is quadratic.<sup>12</sup> Famously, the set of possible charges of incompressible surfaces  $(m_\Sigma, n_\Sigma)$  is finite [102].

The simplest example of such behavior occurs not for a knot complement but for a single ideal tetrahedron  $M = \Delta$ . The index  $\mathcal{Z}[\Delta]_{k=0,s}(m, n)$  is defined by

$$\sum_{n \in \mathbb{Z}} \mathcal{Z}[\Delta]_{k=0,s}(m, n) \zeta^n = \prod_{r=0}^{\infty} \frac{1 - q^{1+r} x^{-1}}{1 - q^r \tilde{x}^{-1}}, \quad (9.4.10)$$

where  $x = q^{\frac{m}{2}} \zeta$  and  $\tilde{x} = q^{\frac{m}{2}} \zeta^{-1}$  (cf. (9.2.21)). Explicitly,

$$\mathcal{Z}[\Delta]_{k=0,s}(m, n) = \sum_{r=(-n)_+}^{\infty} \frac{q^{-\left(r+\frac{1}{2}n\right)m}}{\prod_{i=1}^r (1 - q^{-i}) \prod_{j=1}^{r+n} (1 - q^j)}, \quad (9.4.11)$$

where  $(-n)_+ = \max(-n, 0)$ . There are three rays in the  $(m, n)$  lattice along which the leading power of  $q$  grows linearly:  $\gamma = (0, -d)$ ,  $\gamma' = (d, 0)$ , and  $\gamma'' = (-d, d)$  for  $d \geq 0$ . In terms of the theory  $T[\Delta]$ , these three rays correspond to powers of the three operators  $\Phi, V^+, V^-$  that were discussed at the end of Section 9.4.2. Geometrically, they correspond to the three “local” incompressible surfaces shown in Figure 9.4.3. (These surfaces are boundary-incompressible if the boundary of the ideal tetrahedron is understood as a four-punctured sphere. They are the basic building blocks of what are known as normal surfaces in three-manifold topology [103].)

The boundary-incompressible surfaces in  $M$  lead to very special operators that are unconstrained, in the sense that all their powers contribute to the index, with purely additive

---

<sup>12</sup>Similar behavior appears in certain stable limits of the Jones polynomial [99]. In both cases, the behavior can partially be explained by observing that 1) one is studying  $q$ -series that are solutions to recursion relations coming from the  $A$ -polynomial of a knot [20, 25, 100]; and 2) boundary slopes of the  $A$ -polynomial are related to boundary slopes of incompressible surfaces [101]. See [20, App. D] for further remarks.

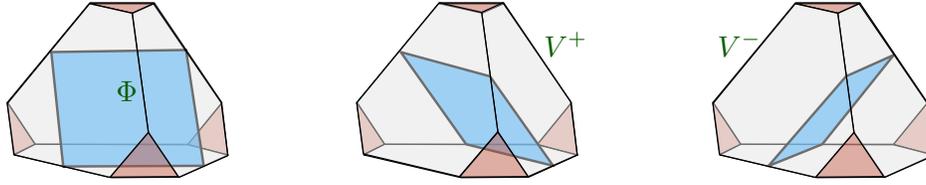

Figure 9.4.3: Three incompressible surfaces inside an ideal tetrahedron, corresponding to three unconstrained operators in the theory  $T[\Delta]$ .

$\frac{R}{2} + J_3$  charge. In general, one might expect to find operators whose powers do obey various relations, and do not have additive charges. Excitingly, in recent mathematical work [45], Hodgson, Hoffman, Garoufalidis, and Rubinstein found that it was possible to rewrite the *entire* index  $\mathcal{Z}[M]_{k=0,s}$  of a knot complement as a sum over surfaces,

$$\mathcal{Z}[M]_{k=0,s}(m, n) = \sum_{\Sigma \text{ s.t. } [\partial\Sigma] = (m, n)} w_{\Sigma}(q), \quad (9.4.12)$$

where the sum is over all normal surfaces in a given triangulation of  $M$ , making the expected relation (9.4.9) true in a precise sense. The main contribution to the weights  $w_{\Sigma}(q)$  looks like a product of tetrahedron indices, corresponding to the tetrahedra in the triangulation. It would be very interesting to understand these weights in terms of local operators of the 6d  $(2, 0)$  theory, bound to the surface  $\Sigma$ .

## 9.5 The Quantum Modularity Conjecture

Our final topic concerns the relation between complex Chern-Simons theory and Zagier's Quantum Modularity Conjecture (QMC) [36]. Strictly speaking, the QMC concerns certain limits of colored Jones polynomials of knots in  $S^3$ . Physically, colored Jones polynomials have to do with  $SU(2)$  Chern-Simons theory. However, by embedding  $SU(2)$  theory into a holomorphic sector of  $SL(2, \mathbb{C})$  theory, one can use complex Chern-Simons theory to study the very same limits [35]. Moreover,  $SL(2, \mathbb{C})$  theory and its various stringy realizations may have a chance of explaining some of the subtler aspects of the conjecture.

To formulate a precise statement, we begin by recalling that the colored Jones polynomials  $J_K(N, q)$  of a knot  $K \subset S^3$  are expectation values in  $SU(2)$  Chern-Simons theory of Wilson loops in the  $N$ -dimensional representation [17, 104, 105]. Physically, the parameter  $q = \exp \frac{2\pi i}{k}$  encodes the renormalized level  $k \in \mathbb{Z}$  of the  $SU(2)$  theory, but (as the name suggest) the Jones polynomials can be analytically continued to Laurent polynomials in a formal variable  $q$ . For any  $k$ -th root of unity  $q^k = 1$ , the Jones polynomials are periodic  $J_K(N, q) = J_K(N + k, q)$ .

The colored Jones polynomials can equivalently be defined using the wavefunction of  $SU(2)$  Chern-Simons at renormalized level  $k$  on the knot complement  $M = S^3 \setminus K$ . (The bare level appearing in the Lagrangian is  $k - 2$ .) Recall, *e.g.* from Section 9.2, that the Hilbert space  $\mathcal{H}[T^2]_k$  in compact Chern-Simons theory is  $k - 1$  dimensional. The  $SU(2)$

wavefunction  $\mathcal{Z}[M]_k$  is thus a vector in  $\mathbb{C}^{k-1}$ , whose components are precisely the Jones polynomials  $J_K(1, e^{\frac{2\pi i}{k}})$ ,  $J_K(2, e^{\frac{2\pi i}{k}})$ ,  $\dots$ ,  $J_K(k-1, e^{\frac{2\pi i}{k}})$ .

For any rational number  $\alpha = a/c$ , Zagier defines

$$\mathcal{J}_K(\alpha) := J_K(c, e^{\frac{2\pi i a}{c}}). \quad (9.5.1)$$

Crucially, this is just outside the natural range of states in  $SU(2)$  Chern-Simons at renormalized level  $c$ , hinting that some analytic continuation will be necessary for a physical interpretation of (9.5.1) (just like it was in the Volume Conjecture).

The QMF states in part that  $\mathcal{J}_K(\alpha)$  shows exponential growth as  $\alpha$  tends to any fixed rational number  $\alpha_0$  through rational values, with the rate of growth governed by the hyperbolic volume of  $M = S^3 \setminus K$ . Specifically, let  $\begin{pmatrix} a & b \\ c & d \end{pmatrix} \in SL(2, \mathbb{Z})$  with  $c > 0$ , and let  $X \rightarrow \infty$  in a fixed coset of  $\mathbb{Q}/\mathbb{Z}$  (for example:  $X = 1, 2, 4, 5, \dots$  or  $X = \frac{3}{4}, \frac{7}{4}, \frac{11}{4}, \dots$  with constant denominators). Set  $\hbar = 2\pi i/(cX + d)$ . Then, conjecturally, there is an asymptotic expansion

$$\mathcal{J}_K\left(\frac{aX + b}{cX + d}\right) \sim \mathcal{J}_K(X) \left(\frac{2\pi i}{\hbar}\right)^{\frac{3}{2}} e^{\frac{1}{c\hbar} S_{CS}(\text{geom})} \phi_{K, a/c}(\hbar), \quad (9.5.2)$$

where  $S_{CS}(\text{geom}) = \text{CS}(M) + i\text{Vol}(M)$  is the volume of the geometric flat connection on  $M$ , containing the hyperbolic volume as in Section 9.4.1; and  $\phi_{K, a/c}(\hbar)$  is a formal power series in  $\hbar$  that depends only on  $a/c \bmod 1$ . Moreover, it was conjectured that after dividing by the leading coefficient to make  $\tilde{\phi}_{K, a/c}(\hbar) = \phi_{K, a/c}(\hbar)/\phi_{K, a/c}(0)$  monic, the subleading coefficients all belong to the trace field of  $K$  adjoined a  $c$ -th root of unity  $\Gamma_K(e^{\frac{2\pi i a}{c}})$ . (The number field  $\Gamma_K$  contains the traces of all holonomies of the geometric flat  $SL(2, \mathbb{C})$  connection on  $M$ .)

For  $\begin{pmatrix} a & b \\ c & d \end{pmatrix} = \begin{pmatrix} 0 & -1 \\ 1 & 0 \end{pmatrix}$  and  $X = 1, 2, 3, \dots \in \mathbb{N}$ , the QMC (9.5.2) reduces to the usual Volume Conjecture.<sup>13</sup> Heuristically, one may think of the Volume Conjecture as studying a limit of colored Jones polynomials as  $q \rightarrow 1$ , and the QMC as studying limits where  $q$  approaches all the rational points on the unit circle.

In order to embed the QMC in  $SL(2, \mathbb{C})$  Chern-Simons theory, one can consider singular limits very similar to (9.4.3).<sup>14</sup> Namely, it was argued in [35] that when fixing the integer level  $k$  and sending  $s \rightarrow -ik$  in complex Chern-Simons theory, or equivalently  $(k+is, k-is) \rightarrow (2k, 0)$ , the knot-complement partition function has an asymptotic expansion

$$\mathcal{Z}[M]_{k,s} \stackrel{s \rightarrow -ik}{\sim} \left(\frac{2\pi i}{\hbar}\right)^{\frac{3}{2}} e^{\frac{1}{k\hbar} S_{CS}(\text{geom})} \phi_{K, 1/k}(\hbar), \quad \hbar = 2\pi i \frac{k-is}{k+is} \quad (9.5.3)$$

with the same series as in (9.5.2). Using the state-sum construction (9.4.6) (on one hand) and detailed computations of Garoufalidis and Zagier for asymptotics of colored Jones polynomials (on the other hand), the agreement between (9.5.2) and (9.5.3) was verified in dozens of

<sup>13</sup>The number-theoretic properties of the asymptotic expansion in the Volume Conjecture were explored from a physical perspective in [49], leading to the notion of an Arithmetic Quantum Field Theory.

<sup>14</sup>There may be other ways to embed the QMC into complex Chern-Simons theory. It was proposed in [106] that setting  $(k+is, k-is) \rightarrow (a, c)$  to finite integer values, which is a perfectly regular limit in complex Chern-Simons, may also be related to the QMC.

examples. By performing a saddle-point expansion of the state-sum model, one also deduces that coefficients of  $\tilde{\phi}_{K,1/k}(\hbar)$  lie in the number field  $\Gamma_K(e^{\frac{2\pi i}{k}})$  as desired.

In terms of the 3d-3d correspondence, the singular limit in (9.5.3) corresponds to computing the partition function of  $T[M]$  on a squashed lens space  $L(k, 1)_b \simeq S_b^3/\mathbb{Z}_k$ , and sending to zero the squashing parameter  $b^2 \rightarrow 0$ . The  $1/k$  dependence in the leading asymptotic can be explained from the simple fact that the lens space is a  $k$ -fold quotient of the three-sphere. It would be interesting to make further physical predictions for the QMC by relating the partition functions of  $T[M]$  on different lens spaces  $L(k, 1)_b$ , or more generally  $L(c, a)_b$ .

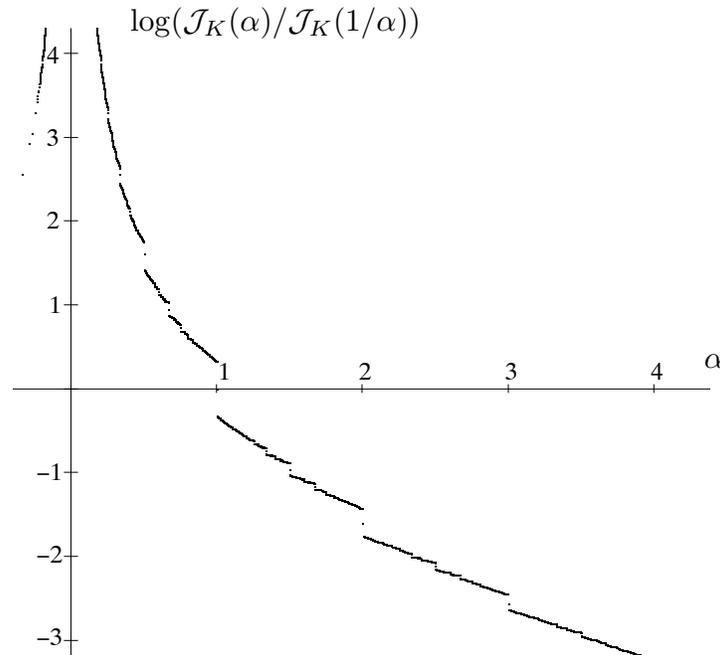

Figure 9.5.1: The graph of  $\mathcal{J}_K(\alpha)/\mathcal{J}_K(1/\alpha)$  when  $K$  is the figure-eight knot, from [36].

Another observation of [36] is that, for hyperbolic several knots, the ratio  $\mathcal{J}_K(\alpha)/\mathcal{J}_K(\gamma(\alpha))$  for  $\gamma \in SL(2, \mathbb{Z})$  has some very interesting finite behavior. This ratio measures the *failure* of  $\mathcal{J}_K(\alpha)$  to be truly “modular.” For the figure-eight knot, a graph of this function appears in [36, Fig. 4], reproduced above. The graph is almost monotonic (it violates monotonicity at a very fine scales) and discontinuous at all rational points  $a/c$ , the size of the discontinuity being roughly proportional to the denominator  $|c|$ .

If we turn this graph on its side, any condensed matter theorist would recognize it immediately: it is the plot of Hall resistivity as a function of magnetic field in a two-dimensional electron system. The plot has plateaus at rational points, due to the fractional quantum Hall effect. It is extremely tempting to think that this must be related to the effective complex Chern-Simons theory in quantum-Hall systems [42]; the connection is investigated in [54].

## Acknowledgements

I am grateful to Stavros Garoufalidis, Sergei Gukov, Neil Hoffman, Craig Hodgson, Hyam Rubinstein, Daniel Jafferis, and Cumrun Vafa for many insightful discussions on the themes that entered this review.

## References

- [1] V. Pestun and M. Zabzine, eds., *Localization techniques in quantum field theory*, vol. xx. Journal of Physics A, 2016. 1608.02952. <https://arxiv.org/src/1608.02952/anc/LocQFT.pdf>, <http://pestun.ihe.fr/pages/LocalizationReview/LocQFT.pdf>.
- [2] A. Achucarro and P. K. Townsend, “A Chern-Simons action for three-dimensional anti-de Sitter supergravity theories,” *Phys. Lett.* **B180** (1986) 89–92.
- [3] E. Witten, “2+1 Dimensional Gravity as an Exactly Soluble System,” *Nucl. Phys.* **B311** (1988) no. 1, 46–78. <http://www.ams.org/mathscinet/search/publications.html?pg1=MR&s1=MR974271>.
- [4] E. Witten, “Topology-Changing Amplitudes in (2+1)-Dimensional Gravity,” *Nucl. Phys.* **B323** (1989) 113. <http://adsabs.harvard.edu/abs/1989NuPhB.323..113W>.
- [5] E. Witten, “Quantization of Chern-Simons Gauge Theory with Complex Gauge Group,” *Comm. Math. Phys.* **137** (1991) 29–66.
- [6] A. Campoleoni, S. Fredenhagen, S. Pfenninger, and S. Theisen, “Asymptotic symmetries of three-dimensional gravity coupled to higher-spin fields,” *JHEP* **1011** (2010) 007, 1008.4744v2. <http://arxiv.org/abs/1008.4744v2>.
- [7] M. R. Gaberdiel and R. Gopakumar, “Minimal Model Holography,” *J. Phys.* **A46** (2013) 214002, 1207.6697v2. <http://arxiv.org/abs/1207.6697v2>.
- [8] C. Cordova and D. L. Jafferis, “Complex Chern-Simons from M5-branes on the Squashed Three-Sphere,” 1305.2891v1. <http://arxiv.org/abs/1305.2891v1>.
- [9] S. Lee and M. Yamazaki, “3d Chern-Simons Theory from M5-branes,” *JHEP* **1312** (2013) 035, 1305.2429v2. <http://arxiv.org/abs/1305.2429v2>.
- [10] J. Yagi, “3d TQFT from 6d SCFT,” *JHEP* **1308** (2013) 017, 1305.0291v1. <http://arxiv.org/abs/1305.0291v1>.
- [11] T. Dimofte, S. Gukov, and L. Hollands, “Vortex Counting and Lagrangian 3-manifolds,” *Lett. Math. Phys.* **98** (2011) 225–287, 1006.0977v1. <http://arxiv.org/abs/1006.0977v1>.
- [12] T. Dimofte and S. Gukov, “Chern-Simons Theory and S-duality,” *JHEP* **1305** (2013) 109, 1106.4550v1. <http://arxiv.org/abs/1106.4550v1>.
- [13] Y. Terashima and M. Yamazaki, “SL(2,R) Chern-Simons, Liouville, and Gauge Theory on Duality Walls,” *JHEP* **1108** (2011) 135, 1103.5748v1. <http://arxiv.org/abs/1103.5748v1>.
- [14] T. Dimofte, D. Gaiotto, and S. Gukov, “Gauge Theories Labelled by Three-Manifolds,” *Comm. Math. Phys.* **325** (2014) 367–419, 1108.4389v1. <http://arxiv.org/abs/1108.4389v1>.
- [15] L. F. Alday, D. Gaiotto, and Y. Tachikawa, “Liouville Correlation Functions from Four-Dimensional Gauge Theories,” *Lett. Math. Phys.* **91** (2010) no. 2, 167–197, 0906.3219v1. <http://arxiv.org/abs/0906.3219v1>.
- [16] A. Gadde, S. Gukov, and P. Putrov, “Fivebranes and 4-manifolds,” 1306.4320v1. <http://arxiv.org/abs/1306.4320v1>.

- [17] E. Witten, “Quantum Field Theory and the Jones Polynomial,” *Comm. Math. Phys.* **121** (1989) no. 3, 351–399.
- [18] N. Reshetikhin and V. Turaev, “Invariants of 3-manifolds via link polynomials and quantum groups,” *Invent. Math.* **103** (1991) no. 3, 547–597.  
<http://www.springerlink.com/index/U416971M947560R7.pdf>.
- [19] J. E. Andersen and R. Kashaev, “A TQFT from quantum Teichmüller theory,” **1109.6295v1**.  
<http://arxiv.org/abs/1109.6295v1>.
- [20] T. Dimofte, D. Gaiotto, and S. Gukov, “3-Manifolds and 3d Indices,” *Adv. Theor. Math. Phys.* **17** (2013) 975–1076, **1112.5179v1**. <http://arxiv.org/abs/1112.5179v1>.
- [21] J. E. Andersen and R. Kashaev, “Complex Quantum Chern-Simons,” **1409.1208v1**.  
<http://arxiv.org/abs/1409.1208v1>.
- [22] T. Dimofte, “Complex Chern-Simons theory at level  $k$  via the 3d-3d correspondence,” *Comm. Math. Phys.* **339** (2015) no. 2, 619–662, **1409.0857v1**. <http://arxiv.org/abs/1409.0857v1>.
- [23] S. Gukov and D. Pei, “Equivariant Verlinde formula from fivebranes and vortices,” **1501.01310v1**.  
<http://arxiv.org/abs/1501.01310v1>.
- [24] D. Pei and K. Ye, “A 3d-3d appetizer,” **1503.04809v1**. <http://arxiv.org/abs/1503.04809v1>.
- [25] S. Gukov, “Three-Dimensional Quantum Gravity, Chern-Simons Theory, and the A-Polynomial,” *Commun. Math. Phys.* **255** (2005) no. 3, 577–627, **hep-th/0306165v1**.  
<http://arxiv.org/abs/hep-th/0306165v1>.
- [26] R. M. Kashaev, “The hyperbolic volume of knots from quantum dilogarithm,” *Lett. Math. Phys.* **39** (1997) 269–265, **q-alg/9601025v2**. <http://arxiv.org/abs/q-alg/9601025v2>.
- [27] H. Murakami and J. Murakami, “The colored Jones polynomials and the simplicial volume of a knot,” *Acta Math.* **186** (2001) no. 1, 85–104, **math/9905075v2**. <http://arxiv.org/abs/math/9905075v2>.
- [28] E. Witten, “Analytic Continuation of Chern-Simons Theory,” *Chern-Simons gauge theory: 20 Years After (AMS/IP Stud. Adv. Math.)* (2011) 347–446, **1001.2933v2**.  
<http://arxiv.org/abs/1001.2933v4>.
- [29] R. Dijkgraaf and H. Fuji, “The Volume Conjecture and Topological Strings,” *Fortschr. Phys.* **57** (2009) no. 9, 825–856, **0903.2084v2**. <http://arxiv.org/abs/0903.2084v2>.
- [30] S. Gukov and P. Sułkowski, “A-polynomial, B-model, and Quantization,” *JHEP* **1202** (2012) 070, **1108.0002v1**. <http://arxiv.org/abs/1108.0002v1>.
- [31] G. Borot and B. Eynard, “All-order asymptotics of hyperbolic knot invariants from non-perturbative topological recursion of A-polynomials,” **1205.2261v2**. <http://arxiv.org/abs/1205.2261v2>.
- [32] B. Eynard and N. Orantin, “Invariants of Algebraic Curves and Topological Expansion,” *Commun. Number Theory Phys.* **1** (2007) no. 2, 347–452, **math-ph/0702045v4**.  
<http://arxiv.org/abs/math-ph/0702045v4>.
- [33] H. Fuji, S. Gukov, and P. Sułkowski, “Volume Conjecture: Refined and Categorified,” **1203.2182v1**.  
<http://arxiv.org/abs/1203.2182v1>.
- [34] S. Gukov, P. Putrov, and C. Vafa, “Fivebranes and 3-manifold homology,” **1602.05302v1**.  
<http://arxiv.org/abs/1602.05302v1>.
- [35] T. Dimofte and S. Garoufalidis, “Quantum modularity and complex Chern-Simons theory,” **1511.05628v1**. <http://arxiv.org/abs/1511.05628v1>.
- [36] D. Zagier, “Quantum Modular Forms,” *Quanta of Maths, Clay Math. Proc.* **11** (2010) 659–675. AMS, Providence, RI.

- [37] Y. Terashima and M. Yamazaki, “3d N=2 Theories from Cluster Algebras,” *PTEP* **023** (2014) B01, [1301.5902v1](https://arxiv.org/abs/1301.5902v1). <http://arxiv.org/abs/1301.5902v1>.
- [38] T. Dimofte, M. Gabella, and A. B. Goncharov, “K-Decompositions and 3d Gauge Theories,” [1301.0192v1](https://arxiv.org/abs/1301.0192v1). <http://arxiv.org/abs/1301.0192v1>.
- [39] L. Chekhov and V. V. Fock, “Quantum Teichmüller Space,” *Theoret. and Math. Phys.* **120** (1999) no. 3, 1245–1259, [math/9908165v2](https://arxiv.org/abs/math/9908165v2). <http://arxiv.org/abs/math/9908165v2>.
- [40] R. M. Kashaev, “Quantization of Teichmüller Spaces and the Quantum Dilogarithm,” *Lett. Math. Phys.* **43** (1998) no. 2, 105–115. <http://www.ams.org/mathscinet/search/publications.html?pg1=MR&s1=MR1607296>.
- [41] V. V. Fock and A. B. Goncharov, “Cluster ensembles, quantization and the dilogarithm,” *Annales Scientifiques L’Ecole Normal Supérieur, 4-e series* **t.42** (2009) 865–930, [math/0311245v5](https://arxiv.org/abs/math/0311245v5). <http://arxiv.org/abs/math/0311245v5>.
- [42] C. Vafa, “Fractional Quantum Hall Effect and M-Theory,” [1511.03372v3](https://arxiv.org/abs/1511.03372v3). <http://arxiv.org/abs/1511.03372v3>.
- [43] M. Atiyah, “Geometry and Physics of Knots,” *Cambridge Univ. Press, Cambridge* (1990) 78pp. <http://books.google.com/books?hl=en&lr=&id=l0WaaHA5rBcC&oi=fnd&pg=PA291&dq=%2522atiyah%2522+%2522knots%2522&ots=55BgFRpwVT&sig=1Rg8AWBVtC1bLt7986jgkMk4Vw>.
- [44] H.-J. Chung, T. Dimofte, S. Gukov, and P. Sulkowski, “3d-3d Correspondence Revisited,” [1405.3663v1](https://arxiv.org/abs/1405.3663v1). <http://arxiv.org/abs/1405.3663v1>.
- [45] S. Garoufalidis, C. Hodgson, N. Hoffman, and H. Rubinstein, “The 3D-index and normal surfaces,” [arXiv:1604.02688](https://arxiv.org/abs/1604.02688) [[math.GT](https://arxiv.org/abs/1604.02688)].
- [46] T. Dumitrescu, “An Introduction to Supersymmetric Field Theories in Curved Space,” *Journal of Physics A* **xx** (2016) 000, [1608.02957](https://arxiv.org/abs/1608.02957).
- [47] B. Willett, “Localization on three-dimensional manifolds,” *Journal of Physics A* **xx** (2016) 000, [1608.02958](https://arxiv.org/abs/1608.02958).
- [48] J. E. Andersen and N. L. Gammelgaard, “The Hitchin-Witten Connection and Complex Quantum Chern-Simons Theory,” [1409.1035v1](https://arxiv.org/abs/1409.1035v1). <http://arxiv.org/abs/1409.1035v1>.
- [49] T. Dimofte, S. Gukov, J. Lenells, and D. Zagier, “Exact Results for Perturbative Chern-Simons Theory with Complex Gauge Group,” *Comm. Num. Thy. and Phys.* **3** (2009) no. 2, 363–443, [0903.2472v1](https://arxiv.org/abs/0903.2472v1). <http://arxiv.org/abs/0903.2472v1>.
- [50] S. Gukov and E. Witten, “Branes and Quantization,” *Adv. Theor. Math. Phys.* **13** (2009) no. 5, 1445–1518, [0809.0305v2](https://arxiv.org/abs/0809.0305v2). <http://arxiv.org/abs/0809.0305v2>.
- [51] S. Gukov, “Quantization via Mirror Symmetry,” [1011.2218v1](https://arxiv.org/abs/1011.2218v1). <http://arxiv.org/abs/1011.2218v1>.
- [52] N. Hitchin, “The self-duality equations on a Riemann surface,” *Proc. London Math. Soc* (1987) . <http://plms.oxfordjournals.org/cgi/reprint/s3-55/1/59.pdf>.
- [53] S. Axelrod, S. D. Pietra, and E. Witten, “Geometric Quantization of Chern-Simons Gauge Theory,” *J. Diff. Geom.* **33** (1991) no. 3, 787–902. <http://www.ams.org/mathscinet/search/publications.html?pg1=MR&s1=MR1100212>.
- [54] T. Dimofte, S. Gukov, and C. Vafa, “Work in progress,”.
- [55] T. Nishioka and Y. Tachikawa, “Para-Liouville/Toda central charges from M5-branes,” *Phys. Rev. D* **84** (2011) 046009, [1106.1172v1](https://arxiv.org/abs/1106.1172v1). <http://arxiv.org/abs/1106.1172v1>.
- [56] C. Cordova and D. L. Jafferis, “Toda Theory From Six Dimensions,” [arXiv:1605.03997](https://arxiv.org/abs/1605.03997) [[hep-th](https://arxiv.org/abs/1605.03997)].

- [57] C. Beem, T. Dimofte, and S. Pasquetti, “Holomorphic Blocks in Three Dimensions,” [1211.1986v1](https://arxiv.org/abs/1211.1986v1).  
<http://arxiv.org/abs/1211.1986v1>.
- [58] G. Mostow, “Strong Rigidity of Locally Symmetric Spaces,” *Ann. Math. Studies, Princeton Univ. Press, Princeton, NJ* **78** (1973) .  
<http://books.google.com/books?hl=en&lr=&id=xTOSFmrFrWoC&oi=fnd&pg=PA3&dq=%2522mostow%2522+%2522strong%2522&ots=kACCab0aTW&sig=igChC-yXFJUQLgjr8FoYi6YU5jc>.
- [59] W. Thurston, “The Geometry and Topology of Three-Manifolds,” *Lecture notes at Princeton University* (1980) .  
<http://pi.unl.edu/~mbrittenham2/classwk/990s08/public/thurston.notes.pdf/6a.pdf>.
- [60] T. Dimofte, “3d Superconformal Theories from Three-Manifolds,” *Math. Phys. Stud.* **9783319187693** (2016) 339–373, [1412.7129v1](https://arxiv.org/abs/1412.7129v1). <http://arxiv.org/abs/1412.7129v1>. J. Teschner, ed.
- [61] D. Gang, N. Kim, M. Romo, and M. Yamazaki, “Aspects of Defects in 3d-3d Correspondence,” [1510.05011v1](https://arxiv.org/abs/1510.05011v1). <http://arxiv.org/abs/1510.05011v1>.
- [62] D. Gaiotto, “N=2 dualities,” *JHEP* **1208** (2012) 034, [0904.2715v1](https://arxiv.org/abs/0904.2715v1).  
<http://arxiv.org/abs/0904.2715v1>.
- [63] D. Gaiotto, G. W. Moore, and A. Neitzke, “Four-dimensional wall-crossing via three-dimensional field theory,” *Comm. Math. Phys.* **299** (2010) no. 1, 163–224, [0807.4723v1](https://arxiv.org/abs/0807.4723v1).  
<http://arxiv.org/abs/0807.4723v1>.
- [64] S. Cecotti, C. Cordova, and C. Vafa, “Braids, Walls, and Mirrors,” [1110.2115v1](https://arxiv.org/abs/1110.2115v1).  
<http://arxiv.org/abs/1110.2115v1>.
- [65] C. Cordova, S. Espahbodi, B. Haghighat, A. Rastogi, and C. Vafa, “Tangles, Generalized Reidemeister Moves, and Three-Dimensional Mirror Symmetry,” [1211.3730v1](https://arxiv.org/abs/1211.3730v1).  
<http://arxiv.org/abs/1211.3730v1>.
- [66] M. Aganagic and S. Shakirov, “Knot Homology from Refined Chern-Simons Theory,” [1105.5117v1](https://arxiv.org/abs/1105.5117v1).  
<http://arxiv.org/abs/1105.5117v1>.
- [67] S. Gukov and H. Murakami, “SL(2,C) Chern-Simons theory and the asymptotic behavior of the colored Jones polynomial,” *Lett. Math. Phys.* **86** (2008) no. 2-3, 79–98, [math/0608324v2](https://arxiv.org/abs/math/0608324v2).  
<http://arxiv.org/abs/math/0608324v2>.
- [68] D. B. Ray and I. M. Singer, “R-torsion and the Laplacian on Riemannian manifolds,” *Adv. in Math.* **7** (1971) 145–210.  
<http://www.ams.org/mathscinet/search/publications.html?pg1=MR&s1=MR0295381>.
- [69] D. Bar-Natan and E. Witten, “Perturbative expansion of Chern-Simons theory with non-compact gauge group,” *Comm. Math. Phys.* **141** (1991) no. 2, 423–440.  
<http://www.springerlink.com/index/G417376W368T0806.pdf>.
- [70] J. Cheeger and J. Simons, “Differential characters and geometric invariants,” *Lecture Notes in Math.* **1167** (1985) 50–80. Springer, Berlin.
- [71] S.-S. Chern and J. Simons, “Characteristic forms and geometric invariants,” *Ann. of Math* **99** (1974) no. 2, 48–69.
- [72] K. Hikami, “Generalized Volume Conjecture and the A-Polynomials - the Neumann-Zagier Potential Function as a Classical Limit of Quantum Invariant,” *J. Geom. Phys.* **57** (2007) no. 9, 1895–1940, [math/0604094v1](https://arxiv.org/abs/math/0604094v1). <http://arxiv.org/abs/math/0604094v1>.
- [73] T. D. Dimofte and S. Garoufalidis, “The quantum content of the gluing equations,” *Geom. Topol.* **17** (2013) no. 3, 1253–1315, [1202.6268v1](https://arxiv.org/abs/1202.6268v1). <http://arxiv.org/abs/1202.6268v1>.

- [74] M. Henningson and K. Skenderis, “The Holographic Weyl anomaly,” *JHEP* **9807** (1998) 023, [hep-th/9806087v2](http://arxiv.org/abs/hep-th/9806087v2). <http://arxiv.org/abs/hep-th/9806087v2>.
- [75] J. A. Harvey, R. Minasian, and G. Moore, “Non-abelian Tensor-multiplet Anomalies,” *JHEP* **9809** (1998) 004, [hep-th/9808060v1](http://arxiv.org/abs/hep-th/9808060v1). <http://arxiv.org/abs/hep-th/9808060v1>.
- [76] J. P. Gauntlett, N. Kim, and D. Waldram, “M-Fivebranes Wrapped on Supersymmetric Cycles,” *Phys. Rev.* **D63** (2001) 126001, [hep-th/0012195v2](http://arxiv.org/abs/hep-th/0012195v2). <http://arxiv.org/abs/hep-th/0012195v2>.
- [77] S. Garoufalidis, D. P. Thurston, and C. K. Zickert, “The complex volume of  $SL(n, \mathbb{C})$ -representations of 3-manifolds,” [1111.2828v1](http://arxiv.org/abs/1111.2828v1). <http://arxiv.org/abs/1111.2828v1>.
- [78] D. Martelli, A. Passias, and J. Sparks, “The gravity dual of supersymmetric gauge theories on a squashed three-sphere,” *Nucl. Phys.* **B864** (2012) 840–868, [1110.6400v3](http://arxiv.org/abs/1110.6400v3). <http://arxiv.org/abs/1110.6400v3>.
- [79] D. Gang, N. Kim, and S. Lee, “Holography of 3d-3d correspondence at Large N,” *JHEP* **1504** (2015) 091, [1409.6206v1](http://arxiv.org/abs/1409.6206v1). <http://arxiv.org/abs/1409.6206v1>.
- [80] P. Menal-Ferrer and J. Porti, “Higher dimensional Reidemeister torsion invariants for cusped hyperbolic 3-manifolds,” *J. of Topol.* **7** (2014) no. 1, 69–119, [1110.3718v2](http://arxiv.org/abs/1110.3718v2). <http://arxiv.org/abs/1110.3718v2>.
- [81] S. Garoufalidis, “The 3D index of an ideal triangulation and angle structures,” [1208.1663v1](http://arxiv.org/abs/1208.1663v1). <http://arxiv.org/abs/1208.1663v1>.
- [82] S. Garoufalidis, C. D. Hodgson, J. H. Rubinstein, and H. Segerman, “1-efficient triangulations and the index of a cusped hyperbolic 3-manifold,” [1303.5278v1](http://arxiv.org/abs/1303.5278v1). <http://arxiv.org/abs/1303.5278v1>.
- [83] T. Dimofte, “Quantum Riemann Surfaces in Chern-Simons Theory,” *Adv. Theor. Math. Phys.* **17** (2013) 479–599, [1102.4847v1](http://arxiv.org/abs/1102.4847v1). <http://arxiv.org/abs/1102.4847v1>.
- [84] J. E. Andersen and R. Kashaev, “A new formulation of the Teichmüller TQFT,” [1305.4291v1](http://arxiv.org/abs/1305.4291v1). <http://arxiv.org/abs/1305.4291v1>.
- [85] S. Kim, “The complete superconformal index for  $N=6$  Chern-Simons theory,” *Nucl. Phys.* **B821** (2009) 241–284, [0903.4172v5](http://arxiv.org/abs/0903.4172v5). <http://arxiv.org/abs/0903.4172v5>.
- [86] Y. Imamura and S. Yokoyama, “Index for three dimensional superconformal field theories with general R-charge assignments,” *JHEP* **1104** (2011) 007, [1101.0557v3](http://arxiv.org/abs/1101.0557v3). <http://arxiv.org/abs/1101.0557v3>.
- [87] A. Kapustin and B. Willett, “Generalized Superconformal Index for Three Dimensional Field Theories,” [1106.2484v1](http://arxiv.org/abs/1106.2484v1). <http://arxiv.org/abs/1106.2484v1>.
- [88] F. Benini, T. Nishioka, and M. Yamazaki, “4d Index to 3d Index and 2d TQFT,” *Phys. Rev.* **D86** (2012) 065015, [1109.0283v2](http://arxiv.org/abs/1109.0283v2). <http://arxiv.org/abs/1109.0283v2>.
- [89] Y. Imamura, H. Matsuno, and D. Yokoyama, “Factorization of  $S^3/Z_n$  partition function,” *Phys. Rev.* **D89** (2014) 085003, [1311.2371v3](http://arxiv.org/abs/1311.2371v3). <http://arxiv.org/abs/1311.2371v3>.
- [90] W. D. Neumann and D. Zagier, “Volumes of hyperbolic three-manifolds,” *Topology* **24** (1985) no. 3, 307–332.
- [91] W. Neumann, “Combinatorics of Triangulations and the Chern-Simons Invariant for Hyperbolic 3-Manifolds,” in *Topology '90, Ohio State Univ. Math. Res. Inst. Publ.* **1** (1992) . <http://www.math.columbia.edu/~neumann/preprints/cspaper.pdf>.
- [92] S. Garoufalidis and R. Kashaev, “From state integrals to q-series,” [1304.2705v1](http://arxiv.org/abs/1304.2705v1). <http://arxiv.org/abs/1304.2705v1>.

- [93] L. Faddeev, “Current-Like Variables in Massive and Massless Integrable Models,” in *Quantum groups and their applications in physics (Varenna 1994)*, *Proc. Internat. School Phys. Enrico Fermi, 127, IOS, Amsterdam* (1996) 117–135. <http://arxiv.org/abs/hep-th/9408041>.
- [94] L. D. Faddeev and R. M. Kashaev, “Quantum Dilogarithm,” *Modern Phys. Lett.* **A9** (1994) no. 5, 427–434, [hep-th/9310070v1](http://arxiv.org/abs/hep-th/9310070v1). <http://arxiv.org/abs/hep-th/9310070v1>.
- [95] C. Petronio and J. Weeks, “Partially Flat Ideal Triangulations of Cusped Hyperbolic 3-Manifolds,” *Osaka J. Math.* **37** (2000) no. 2, 453–466. [http://www.projecteuclid.org/DPubS/Repository/1.0/Disseminate?handle=euclid.ojm/1200789209&view=body&content-type=pdf\\_1](http://www.projecteuclid.org/DPubS/Repository/1.0/Disseminate?handle=euclid.ojm/1200789209&view=body&content-type=pdf_1).
- [96] M. Culler, N. Dunfield, and J. R. Weeks, “SnapPy, a computer program for studying the geometry and topology of 3-manifolds,”. <http://snappy.computop.org>. <http://snappy.computop.org>.
- [97] E. Witten, “Constraints on supersymmetry breaking,” *Nucl. Phys.* **B202** (1982) no. 2, 253–316. <http://www.ams.org/mathscinet/search/publications.html?pg1=MR&s1=MR668987>.
- [98] A. Gadde, S. Gukov, and P. Putrov, “Walls, Lines, and Spectral Dualities in 3d Gauge Theories,” [1302.0015v1](http://arxiv.org/abs/1302.0015v1). <http://arxiv.org/abs/1302.0015v1>.
- [99] S. Garoufalidis, “The Jones slopes of a knot,” *Quant. Topol.* **2** (2011) 43–69, [0911.3627v4](http://arxiv.org/abs/0911.3627v4). <http://arxiv.org/abs/0911.3627v4>.
- [100] S. Garoufalidis, “On the Characteristic and Deformation Varieties of a Knot,” *Geom. Topol. Monogr.* **7** (2004) 291–304, [math/0306230v4](http://arxiv.org/abs/math/0306230v4). <http://arxiv.org/abs/math/0306230v4>.
- [101] D. Cooper, M. Culler, H. Gillet, D. Long, and P. Shalen, “Plane Curves Associated to Character Varieties of 3-Manifolds,” *Invent. Math.* **118** (1994) no. 1, 47–84. <http://www.springerlink.com/index/R865T605G509312U.pdf>.
- [102] A. Hatcher, “On the boundary curves of incompressible surfaces,” *Pacific J. Math.* **99** (1982) 373–377.
- [103] J. H. Rubinstein, “An algorithm to recognize the 3-sphere,” *Proc. International Congress of Math.* **1** (1994) no. 2, 601–611. Birkhauser, Basel.
- [104] V. F. R. Jones, “A polynomial invariant for knots via von Neumann algebras,” *Bull. Amer. Math. Soc. (N.S.)* **12** (1985) no. 1, 103–111. <http://www.ams.org/mathscinet/search/publications.html?pg1=MR&s1=MR766964>.
- [105] V. G. Turaev, “The Yang-Baxter equation and invariants of links,” *Invent. Math.* **92** (1988) no. 3, 527–553. <http://www.ams.org/mathscinet/search/publications.html?pg1=MR&s1=MR939474>.
- [106] S. Garoufalidis and R. Kashaev, “Evaluation of state integrals at rational points,” *Comm. Num. Thy. Phys.* **9** (2015) no. 3, 549–582, [1411.6062v2](http://arxiv.org/abs/1411.6062v2). <http://arxiv.org/abs/1411.6062v2>.

# Chapter 10

## $\mathcal{N} = 2$ SUSY gauge theories on $S^4$

Kazuo Hosomichi

*Department of Physics, National Taiwan University, Taipei 10617, Taiwan*  
hosomiti@phys.ntu.edu.tw

### Abstract

We review exact results in  $\mathcal{N} = 2$  supersymmetric gauge theories defined on  $S^4$  and its deformation. We first summarize the construction of rigid SUSY theories on curved backgrounds based on off-shell supergravity, then explain how to apply localization principle to supersymmetric path integrals. Closed formulae for partition function as well as expectation values of non-local BPS observables are presented.

### Contents

|                                                                       |            |
|-----------------------------------------------------------------------|------------|
| <b>10.1 Introduction</b>                                              | <b>398</b> |
| <b>10.2 Construction of theories</b>                                  | <b>401</b> |
| 10.2.1 Conformal Killing spinors on $S^4$                             | 401        |
| 10.2.2 Generalized Killing spinors and $\mathcal{N} = 2$ Supergravity | 401        |
| 10.2.3 Transformation laws and Lagrangians                            | 402        |
| 10.2.4 Examples of SUSY backgrounds                                   | 406        |
| <b>10.3 Partition function</b>                                        | <b>409</b> |
| 10.3.1 Localization principle                                         | 409        |
| 10.3.2 Gauge fixing                                                   | 411        |
| 10.3.3 Determinants and index                                         | 412        |
| 10.3.4 $\mathcal{N} = 4$ SYM and Gaussian matrix model                | 416        |
| <b>10.4 Supersymmetric observables</b>                                | <b>417</b> |
| 10.4.1 Wilson loops                                                   | 417        |
| 10.4.2 't Hooft loops                                                 | 417        |
| 10.4.3 Surface operators                                              | 423        |
| <b>References</b>                                                     | <b>426</b> |

## 10.1 Introduction

Four-dimensional  $\mathcal{N} = 2$  supersymmetric gauge theories are known to be mathematically highly constrained, and yet they can accommodate a variety of interesting physical phenomena. One can therefore ask general questions about physics of strong gauge interactions in these theories and expect a rather precise answer. The first non-trivial result was obtained by Seiberg and Witten [2, 3] for the structure of Coulomb branch moduli space as well as the mass of BPS particles. By combining the constraints from  $\mathcal{N} = 2$  supersymmetry together with electro-magnetic duality, they determined the exact prepotential which encodes the full low-energy effective Lagrangian, including the contribution of instantons which were otherwise very difficult to evaluate at that time.

Another powerful approach to 4D  $\mathcal{N} = 2$  theories is localization, which makes use of supersymmetry to reduce the difficult problem of infinite-dimensional path integral to a much simpler problem. There is a class of 4D topological field theories, called topologically twisted theories [4], which are obtained from  $\mathcal{N} = 2$  theories by changing the spin of fields according to their quantum numbers under the internal symmetry  $SU(2)_R$ . Once the SUSY localization is applied to those theories, path integral can be shown to reduce to a finite-dimensional integral on instanton moduli spaces. Nekrasov later proposed the so-called Omega-deformation [5–8] of the topologically twisted theories, which further simplifies the integrals on moduli spaces by using the rotational symmetry of  $\mathbb{R}^4$ . The resulting path integral is called Nekrasov’s instanton partition function, and is expressed as a sum over point-like instanton configurations localized at the origin. Nekrasov’s partition function was shown to reproduce the prepotential of  $\mathcal{N} = 2$  theories in the limit of small Omega-deformation. Moreover, it has given us a new insight into the connection between  $\mathcal{N} = 2$  gauge theories and other branches of physics and mathematics, such as topological strings or integrable systems.

**Pestun’s pioneering work** Application of localization principle to quantum field theories has been long restricted to topological field theories with scalar supersymmetry. A major breakthrough was made by Pestun [9] who constructed  $\mathcal{N} = 2$  supersymmetric gauge theories on the four-sphere  $S^4$  and derived closed formulae for partition function as well as expectation values of certain Wilson loops [9]. This article reviews his result and some of the subsequent work on exact supersymmetric observables in  $\mathcal{N} = 2$  supersymmetric gauge theories on  $S^4$  and its deformations.

The original motivation of the work [9] was to prove a conjecture which arose from the study of AdS/CFT correspondence, that the expectation values of supersymmetric circular Wilson loops in  $\mathcal{N} = 4$  super Yang-Mills theory are given by Gaussian matrix integral [10, 11]. Instead of topological field theories with scalar SUSY, Pestun constructed physical  $\mathcal{N} = 2$  SUSY theories on  $S^4$  via conformal map from flat  $\mathbb{R}^4$ . By a successful application of SUSY localization principle, the path integral was shown to reduce to a finite-dimensional integral. A one-parameter (mass) deformation of the  $\mathcal{N} = 4$  SYM called  $\mathcal{N} = 2^*$  theory was studied in detail, and it was found that the integrand simplifies dramatically at a special value of the mass. In this way, it was analytically shown that the  $S^4$  partition function is precisely given by a Gaussian matrix integral [9, 12]. See Chapter 11 for more detail on the application of

localization to the problems in AdS/CFT.

Pestun’s work is the first nontrivial example in which a coherent and fully explicit prescription was given for physical supersymmetric models on curved spaces, from the construction of theories to the evaluation of supersymmetric observables. Exact formulae were obtained later for partition functions of supersymmetric gauge theories on  $S^3$  [14–16],  $S^2$  [17, 18] and  $S^5$  [19–21] by following basically the same program. Together with the supersymmetric partition functions on  $S^1 \times S^d$  called superconformal indices, the sphere partition functions are now regarded as powerful analytic tools to explore non-perturbative aspects of SUSY gauge theories. In particular, for CFTs with right number of supersymmetry in even dimensions, it was shown that the sphere partition function is protected from regularization ambiguity and computes the Kähler potential for the space of marginal couplings [22, 23].

Important applications of Pestun’s result have been made for a family of 4D  $\mathcal{N} = 2$  theories of “class S” [24], that are known to show up on the worldvolume of multiple M5-branes (5 + 1-dimensional object in M-theory) wrapped on punctured Riemann surfaces. In particular, Alday, Gaiotto and Tachikawa (AGT) discovered a surprising correspondence between exact  $S^4$  partition functions of the class S superconformal theories for two M5-branes and correlation functions of 2D Liouville conformal field theory [25] (see Chapter 12). Generalization to gauge groups of higher rank and Toda conformal field theories was soon proposed by Wyllard [27]. This discovery brought us with another new insight into the mathematical structure underlying 4D  $\mathcal{N} = 2$  gauge theories. It also triggered an extensive study of similar correspondences between quantum field theories in different dimensions that follow from compactifications of multiple M5-branes.

**Squashing** Supersymmetric gauge theories and exact physical observables have also been studied on manifolds which are less symmetric than sphere. One motivation for this generalization arose from the AGT relation, since the partition function on the round  $S^4$  was shown to correspond to Toda CFTs at a special (self-dual) value of the coupling,  $b = 1$ . Nontrivial results along this line of generalization were first obtained in [28] and [29] for 3D  $\mathcal{N} = 2$  supersymmetric theories on certain squashed spheres with a background vector field turned on. The supersymmetry there is characterized by generalized Killing spinors with a specific coupling to the vector field.

For theories with different amount of SUSY and in other dimensions, the most natural framework to explore supersymmetric curved backgrounds is off-shell supergravity [30], See Chapter 5. For 4D  $\mathcal{N} = 2$  theories this idea was employed in [32] to construct supersymmetric ellipsoid backgrounds, which depend on a squashing parameter  $b$  measuring the deformation from the round sphere geometry. The partition function on this background was shown to reproduce the correlators of Toda CFTs at general values of the coupling. The rigid supersymmetric backgrounds were systematically classified and deformations of  $S^4$  were studied within  $\mathcal{N} = 1$  off-shell supergravity in [33–37], and in [38] within  $\mathcal{N} = 2$  supergravity. Different versions of deformations of the round  $S^4$  have been studied in [39, 40], while the backgrounds of other topologies, such as products of spheres and  $AdS$  spaces, have been

studied in [41–45], where the results have been used to study the loop correction to the entropy of certain charged black holes. Supersymmetric deformations of the round sphere geometry have also been applied to the computation of Rényi entropy in gauge theories in  $D = 3, 4, 5$ ; see [46–50].

**Supersymmetric observables** Localization techniques have also been applied to compute expectation values of various supersymmetric observables. An important class of observables in 4D  $\mathcal{N} = 2$  theories are supersymmetric Wilson and ’t Hooft loop operators, defined from the worldlines of electrically or magnetically charged particles. It is a remarkable feature of  $\mathcal{N} = 2$  supersymmetric theories that one can make quantitative statements about properties of these particles, in particular how they are exchanged among each other under S-duality [24]. Also, a number of nontrivial conjectures on the expectation values of loop operators have been proposed from AGT relation and checked explicitly [51–53]. The effect of deformations of the theories on Wilson loop and local observables were studied in [54].

Another important class of nonlocal operators are surface operators, which have two dimensional worldvolume inside four dimensions. See [55] for a review. They are defined either by introducing two-dimensional field theory degrees of freedom on the surface or by imposing singular behavior on gauge and other fields along the surface. They were first introduced in [56] in the study of geometric Langlands program within the framework of 4D  $\mathcal{N} = 4$  SYM theory. Interesting progress has been made for surface operators in  $\mathcal{N} = 2$  supersymmetric theories through the comparison of the gauge theory analysis with the results from topological string or predictions from AGT relation [51, 57–65].

**Conventions** Throughout this article, we use the indices  $\alpha, \beta, \dots$  and  $\dot{\alpha}, \dot{\beta}, \dots$  for 4D chiral and anti-chiral spinors. The indices are raised and lowered by the antisymmetric invariant tensors  $\epsilon^{\alpha\beta}, \epsilon^{\dot{\alpha}\dot{\beta}}, \epsilon_{\alpha\beta}, \epsilon_{\dot{\alpha}\dot{\beta}}$  with nonzero elements

$$\epsilon^{12} = -\epsilon^{21} = -\epsilon_{12} = \epsilon_{21} = 1. \quad (10.1.1)$$

Following Wess-Bagger [66] we suppress the pairs of undotted indices contracted in the up-left, down-right order, or pairs of dotted indices contracted in the down-left, up-right order. We also use the set of  $2 \times 2$  matrices  $(\sigma^a)_{\alpha\dot{\alpha}}$  and  $(\bar{\sigma}^a)^{\dot{\alpha}\alpha}$  with  $a = 1, \dots, 4$  satisfying standard algebras. In terms of Pauli’s matrices  $\boldsymbol{\tau}^a$  they are given by

$$\begin{aligned} \sigma^a &= -i\boldsymbol{\tau}^a, & \bar{\sigma}^a &= i\boldsymbol{\tau}^a, & (a = 1, 2, 3) \\ \sigma^4 &= 1, & \bar{\sigma}^4 &= 1. \end{aligned} \quad (10.1.2)$$

We also use  $\sigma_{ab} = \frac{1}{2}(\sigma_a \bar{\sigma}_b - \sigma_b \bar{\sigma}_a)$  and  $\bar{\sigma}_{ab} = \frac{1}{2}(\bar{\sigma}_a \sigma_b - \bar{\sigma}_b \sigma_a)$ . Note that  $\sigma_{ab}$  is anti-self-dual, i.e.  $\sigma_{ab} = -\frac{1}{2}\epsilon_{abcd}\sigma_{cd}$ , while  $\bar{\sigma}_{ab}$  is self-dual.

For 4D  $\mathcal{N} = 2$  theories on flat space, supersymmetry is parametrized by constant spinors  $\xi_{\alpha A}$  and  $\bar{\xi}_A^{\dot{\alpha}}$ . The index  $A = 1, 2$  indicates that they transform as doublet under  $SU(2)$  R-symmetry which commutes with the generators of Poincaré symmetry but rotates the supercharges. In addition,  $\xi_{\alpha A}$  and  $\bar{\xi}_A^{\dot{\alpha}}$  carry  $U(1)$  R-charges  $+1$  and  $-1$ . Throughout this article, these SUSY parameters are Grassmann-even quantities.

| bosons         |                                      |  | $q_{\mathbb{R}}$ | fermions          |                       |  | $q_{\mathbb{R}}$ |
|----------------|--------------------------------------|--|------------------|-------------------|-----------------------|--|------------------|
| $g_{mn}$       | metric                               |  | 0                | $\psi_{mA}$       | chiral gravitino      |  | +1               |
| $(V_m)^A_B$    | gauge field for $SU(2)_{\mathbb{R}}$ |  | 0                | $\bar{\psi}_{mA}$ | anti-chiral gravitino |  | -1               |
| $\tilde{V}_m$  | gauge field for $U(1)_{\mathbb{R}}$  |  | 0                | $\eta_A$          | chiral spinor         |  | +1               |
| $T_{mn}$       | anti-self-dual tensor                |  | +2               | $\bar{\eta}_A$    | anti-chiral spinor    |  | -1               |
| $\bar{T}_{mn}$ | self-dual tensor                     |  | -2               |                   |                       |  |                  |
| $M$            | scalar                               |  | 0                |                   |                       |  |                  |

Table 10.2.1: fields and their  $U(1)_{\mathbb{R}}$  charges  $q_{\mathbb{R}}$  in off-shell 4D  $\mathcal{N} = 2$  supergravity

## 10.2 Construction of theories

Here we review the construction of  $\mathcal{N} = 2$  supersymmetric gauge theories on  $S^4$  using off-shell supergravity. We then present a number of nontrivial supergravity backgrounds with rigid supersymmetry, including the supersymmetric deformation of  $S^4$  into ellipsoids.

### 10.2.1 Conformal Killing spinors on $S^4$

As the round  $S^4$  is conformally flat, 4D  $\mathcal{N} = 2$  superconformal theories can be constructed on  $S^4$  by a conformal map from flat  $\mathbb{R}^4$ . Let  $\ell$  be the radius of  $S^4$ . The superconformal symmetry is then described by conformal Killing spinors satisfying

$$\begin{aligned}
D_m \xi_A &\equiv \left( \partial_m + \frac{1}{4} \Omega_m^{ab} \sigma_{ab} \right) \xi_A = -i \sigma_m \bar{\xi}'_A, & D_m \bar{\xi}'_A &= -\frac{i}{4\ell^2} \bar{\sigma}_m \xi_A, \\
D_m \bar{\xi}_A &\equiv \left( \partial_m + \frac{1}{4} \Omega_m^{ab} \bar{\sigma}_{ab} \right) \bar{\xi}_A = -i \bar{\sigma}_m \xi'_A, & D_m \xi'_A &= -\frac{i}{4\ell^2} \sigma_m \bar{\xi}_A.
\end{aligned} \tag{10.2.1}$$

This is a coupled first-order differential equation for 16 spinor components, and therefore has 16 independent solutions corresponding to the fermionic generators of the 4D  $\mathcal{N} = 2$  superconformal algebra. Lagrangian theories of vector multiplets and massless hypermultiplets are all superconformal at the classical level, so they can be unambiguously defined on the round  $S^4$  in this way. For massive theories on  $S^4$ , the superconformal symmetry is broken to a subgroup  $OSp(2|4)$ . This means that the mass terms are constructed in such a way that a subset of supercharges corresponding to the Killing spinors

$$D_m \xi_A = -\frac{i}{2\ell} \sigma_m \bar{\xi}_B \cdot t^B_A, \quad D_m \bar{\xi}_A = -\frac{i}{2\ell} \bar{\sigma}_m \xi_B \cdot \bar{t}^B_A \tag{10.2.2}$$

is preserved. Here  $t, \bar{t}$  are constant traceless  $U(2)$  matrices satisfying  $t\bar{t} = \bar{t}t = \mathbf{1}$ . They can be brought into a standard form, say  $t = \bar{t} = \tau_3$ , using R-symmetry.

### 10.2.2 Generalized Killing spinors and $\mathcal{N} = 2$ Supergravity

Off-shell supergravity allows to construct supersymmetric field theories on more general curved backgrounds [30]. The independent fields in the standard gravity multiplet (also called

*Weyl multiplet*) in 4D  $\mathcal{N} = 2$  supergravity [67–70] (see also reviews [71, 72]) are listed in Table 10.2.1. Supergravity backgrounds are specified by the classical values of all the bosonic fields, while the fermionic fields are all taken to vanish. A background is supersymmetric if the local SUSY variation of fermions, (we quote the formula from [72] with certain rescalings of fields)

$$\begin{aligned}
\mathbf{Q}\psi_{mA} &= D_m\xi_A + T^{kl}\sigma_{kl}\sigma_m\bar{\xi}_A + i\sigma_m\bar{\xi}'_A, \\
\mathbf{Q}\bar{\psi}_{mA} &= D_m\bar{\xi}_A + \bar{T}^{kl}\bar{\sigma}_{kl}\bar{\sigma}_m\xi_A + i\bar{\sigma}_m\xi'_A, \\
\mathbf{Q}\eta_A &= 8\sigma^{mn}\sigma^l\bar{\xi}_A D_l T_{mn} + 16iT^{kl}\sigma_{kl}\xi'_A - 3\tilde{M}\xi_A + 2i\sigma^{mn}\xi_B(V_{mn})^B_A + 4i\sigma^{mn}\xi_A\tilde{V}_{mn}, \\
\mathbf{Q}\bar{\eta}_A &= 8\bar{\sigma}^{mn}\bar{\sigma}^l\xi_A D_l\bar{T}_{mn} + 16i\bar{T}^{kl}\bar{\sigma}_{kl}\bar{\xi}'_A - 3\tilde{M}\bar{\xi}_A + 2i\bar{\sigma}^{mn}\bar{\xi}_B(V_{mn})^B_A - 4i\bar{\sigma}^{mn}\bar{\xi}_A\tilde{V}_{mn},
\end{aligned} \tag{10.2.3}$$

all vanish for a suitable choice of spinor fields  $(\xi_A, \bar{\xi}_A)$  and  $(\xi'_A, \bar{\xi}'_A)$ . Here the covariant derivatives are with respect to the local Lorentz as well as  $SU(2) \times U(1)$  R-symmetries. For example,

$$D_m\xi_A \equiv \left( \partial_m + \frac{1}{4}\Omega_m^{ab}\sigma_{ab} \right) \xi_A + i\xi_B(V_m)^B_A - i\tilde{V}_m\xi_A. \tag{10.2.4}$$

We also denoted the  $U(1)_R$  gauge field strength by  $\partial_m\tilde{V}_n - \partial_n\tilde{V}_m \equiv \tilde{V}_{mn}$  and similarly for the  $SU(2)_R$  field strength  $(V_{mn})^B_A$ . With the simplifying assumption

$$\tilde{V}_m = 0, \tag{10.2.5}$$

the above BPS condition can be transformed into the form presented in [32],

$$\begin{aligned}
D_m\xi_A + T^{kl}\sigma_{kl}\sigma_m\bar{\xi}_A &= -i\sigma_m\bar{\xi}'_A, \\
D_m\bar{\xi}_A + \bar{T}^{kl}\bar{\sigma}_{kl}\bar{\sigma}_m\xi_A &= -i\bar{\sigma}_m\xi'_A, \\
\sigma^m\bar{\sigma}^n D_m D_n \xi_A + 4D_l T_{mn}\sigma^{mn}\sigma^l\bar{\xi}_A &= M\xi_A, \\
\bar{\sigma}^m\sigma^n D_m D_n \bar{\xi}_A + 4D_l \bar{T}_{mn}\bar{\sigma}^{mn}\bar{\sigma}^l\xi_A &= M\bar{\xi}_A,
\end{aligned} \tag{10.2.6}$$

where  $M \equiv \tilde{M} - \frac{1}{3}R$ . This gives a consistent generalization of the conformal Killing spinor equation (10.2.1) on  $S^4$ . Hereafter we use  $M$  rather than  $\tilde{M}$  in accordance with [32], but note that the latter has a better transformation property under Weyl rescaling. The equations (10.2.6) are invariant under  $g_{mn} \rightarrow e^{2\rho}g_{mn}$  if accompanied by

$$\begin{aligned}
\xi_A &\rightarrow e^{\frac{1}{2}\rho}\xi_A, & \xi'_A &\rightarrow e^{-\frac{1}{2}\rho}\xi'_A, & T_{mn} &\rightarrow e^{-\rho}T_{mn}, & \tilde{M} &\rightarrow e^{-2\rho}\tilde{M}, \\
\bar{\xi}_A &\rightarrow e^{\frac{1}{2}\rho}\bar{\xi}_A, & \bar{\xi}'_A &\rightarrow e^{-\frac{1}{2}\rho}\bar{\xi}'_A, & \bar{T}_{mn} &\rightarrow e^{-\rho}\bar{T}_{mn}.
\end{aligned} \tag{10.2.7}$$

### 10.2.3 Transformation laws and Lagrangians

Supergravity also gives a description of local SUSY-invariant couplings of matter systems to gravity. By sending the Newton constant to zero in such a description, one can decouple gravity from the matter and treat the fields in gravity multiplet as classical background

fields. In this way one can systematically construct rigid SUSY theories on various curved backgrounds.

Vector multiplet consists of a gauge field  $A_m$ , scalars  $\phi, \bar{\phi}$ , gauginos  $\lambda_{\alpha A}, \bar{\lambda}_{\dot{\alpha} A}$  and an  $SU(2)_R$ -triplet auxiliary scalar  $D_{AB}$ . They transform under supersymmetry as

$$\begin{aligned}
\mathbf{Q}A_m &= i\xi^A \sigma_m \bar{\lambda}_A - i\bar{\xi}^A \bar{\sigma}_m \lambda_A, \\
\mathbf{Q}\phi &= -i\xi^A \lambda_A, \\
\mathbf{Q}\bar{\phi} &= +i\bar{\xi}^A \bar{\lambda}_A, \\
\mathbf{Q}\lambda_A &= \frac{1}{2}\sigma^{mn}\xi_A(F_{mn} + 8\bar{\phi}\bar{T}_{mn}) + 2\sigma^m\bar{\xi}_A D_m\phi + \sigma^m D_m\bar{\xi}_A\phi + 2i\xi_A[\phi, \bar{\phi}] + D_{AB}\xi^B, \\
\mathbf{Q}\bar{\lambda}_A &= \frac{1}{2}\bar{\sigma}^{mn}\bar{\xi}_A(F_{mn} + 8\phi\bar{T}_{mn}) + 2\bar{\sigma}^m\xi_A D_m\bar{\phi} + \bar{\sigma}^m D_m\xi_A\bar{\phi} - 2i\bar{\xi}_A[\phi, \bar{\phi}] + D_{AB}\bar{\xi}^B, \\
\mathbf{Q}D_{AB} &= -i\bar{\xi}_A\bar{\sigma}^m D_m\lambda_B - i\xi_B\bar{\sigma}^m D_m\lambda_A + i\xi_A\sigma^m D_m\bar{\lambda}_B + i\xi_B\sigma^m D_m\bar{\lambda}_A \\
&\quad - 2[\phi, \bar{\xi}_A\bar{\lambda}_B + \bar{\xi}_B\bar{\lambda}_A] + 2[\bar{\phi}, \xi_A\lambda_B + \xi_B\lambda_A].
\end{aligned} \tag{10.2.8}$$

Note that the following combination of vector and scalar fields is  $\mathbf{Q}$ -invariant,

$$\hat{\Phi} \equiv 2i\xi^A\xi_A\bar{\phi} - 2i\bar{\xi}^A\bar{\xi}_A\phi - 2i\bar{\xi}^A\bar{\sigma}^m\xi_A A_m, \tag{10.2.9}$$

which will become important later. SUSY invariant Yang-Mills kinetic Lagrangian reads

$$\begin{aligned}
\mathcal{L}_{\text{YM}} &= \frac{1}{g^2}\text{Tr}\left(\frac{1}{2}F_{mn}F^{mn} + 16F_{mn}(\bar{\phi}T^{mn} + \phi\bar{T}^{mn}) + 64\bar{\phi}^2 T_{mn}T^{mn} + 64\phi^2\bar{T}_{mn}\bar{T}^{mn}\right. \\
&\quad \left. - 4D_m\bar{\phi}D^m\phi + 2M\bar{\phi}\phi - 2i\lambda^A\sigma^m D_m\bar{\lambda}_A - 2\lambda^A[\bar{\phi}, \lambda_A] + 2\bar{\lambda}^A[\phi, \bar{\lambda}_A]\right. \\
&\quad \left. + 4[\phi, \bar{\phi}]^2 - \frac{1}{2}D^{AB}D_{AB}\right) + \frac{i\theta}{32\pi^2}\text{Tr}\left(\varepsilon^{klmn}F_{kl}F_{mn}\right).
\end{aligned} \tag{10.2.10}$$

One instanton factor is  $q = e^{2\pi i\tau}$  with  $\tau = \frac{\theta}{2\pi} + \frac{4\pi i}{g^2}$ .

For  $U(1)$  vector multiplets one can also construct a Feyet-Illiopoulos type invariant. Let  $w^{AB} = w^{BA}$  be an  $SU(2)_R$ -triplet background field satisfying

$$\begin{aligned}
w^{AB}\xi_B &= \frac{1}{2}\sigma^n D_n\bar{\xi}^A + 2T_{kl}\sigma^{kl}\xi^A, \\
w^{AB}\bar{\xi}_B &= \frac{1}{2}\bar{\sigma}^n D_n\xi^A + 2\bar{T}_{kl}\bar{\sigma}^{kl}\bar{\xi}^A.
\end{aligned} \tag{10.2.11}$$

Then the following is SUSY-invariant.

$$\mathcal{L}_{\text{FI}} = \zeta \left\{ w^{AB}D_{AB} - M(\phi + \bar{\phi}) - 64\phi T^{kl}T_{kl} - 64\bar{\phi}\bar{T}^{kl}\bar{T}_{kl} - 8F^{kl}(T_{kl} + \bar{T}_{kl}) \right\}. \tag{10.2.12}$$

Note that this term breaks the conformal invariance. By comparing with the Killing spinor equation (10.2.2), one finds  $t_{AB} = \bar{t}_{AB} = i\ell w_{AB}$  on the round  $S^4$  of radius  $\ell$ .

The system of  $r$  hypermultiplets consists of scalars  $q_{IA}$  and fermions  $\psi_{\alpha I}, \bar{\psi}_{\dot{\alpha} I}$ , with  $I = 1, \dots, 2r$ . The scalars obey the reality condition

$$(q_{IA})^\dagger = q^{AI} = \epsilon^{AB}\Omega^{IJ}q_{JB}, \tag{10.2.13}$$

where  $\Omega^{IJ}$  is the real antisymmetric  $Sp(r)$ -invariant tensor satisfying

$$(\Omega^{IJ})^* = -\Omega_{IJ}, \quad \Omega^{IJ}\Omega_{JK} = \delta_K^I.$$

The tensor  $\Omega^{IJ}$  and its inverse are used to raise or lower the  $Sp(r)$  indices. The pair of  $Sp(r)$  indices will be suppressed in the following when contracted in the top-left, bottom-right order, like  $q^{AI}q_{IA} = q^A q_A$ . The hypermultiplet fields can be coupled to vector multiplet by embedding the gauge group into  $Sp(r)$ . The covariant derivative of  $q_{IA}$ , for example, is then given by

$$D_m q_{IA} \equiv \partial_m q_{IA} - i(A_m)_I{}^J q_{JA} + i q_{IB}(V_m)^B{}_A. \quad (10.2.14)$$

It is a little intricate to write down an off-shell SUSY transformation rule for hypermultiplet fields explicitly. As is well known, for rigid  $\mathcal{N} = 2$  SUSY theories with hypermultiplets on flat space, there is no formalism which realizes all the 8 supercharges at once with finite number of auxiliary fields. However, when applying localization method, one always picks up one of the supercharges corresponding to a particular choice of Killing spinor  $\xi_A, \bar{\xi}_A$ , and requires that particular supercharge to be realized off-shell. What we will present here is an off-shell realization of just one supercharge.

To balance the number of bosons and fermions in hypermultiplet, we need to introduce the auxiliary scalar fields  $F_{I\check{A}}$ , where  $I$  is the  $Sp(r)$  index and  $\check{A} = 1, 2$  is a new auxiliary index. We also introduce [32] the spinor fields  $\check{\xi}_{\check{A}}, \check{\bar{\xi}}_{\check{A}}$  satisfying

$$\begin{aligned} \xi_A \check{\xi}_{\check{B}} - \bar{\xi}_A \check{\bar{\xi}}_{\check{B}} &= 0, \\ \xi^A \xi_A + \check{\xi}^{\check{A}} \check{\bar{\xi}}_{\check{A}} &= 0, \\ \bar{\xi}^A \bar{\xi}_A + \check{\bar{\xi}}^{\check{A}} \check{\xi}_{\check{A}} &= 0, \\ \xi^A \sigma^m \bar{\xi}_A + \check{\xi}^{\check{A}} \sigma^m \check{\bar{\xi}}_{\check{A}} &= 0. \end{aligned} \quad (10.2.15)$$

A solution to the above conditions is given by

$$\check{\xi}_{\check{A}} = c^{\frac{1}{2}} \xi_A, \quad \check{\bar{\xi}}_{\check{A}} = -c^{-\frac{1}{2}} \bar{\xi}_A \quad (A = \check{A} = 1, 2) \quad \text{where } c = -\frac{\bar{\xi}^A \bar{\xi}_A}{\xi^B \xi_B}. \quad (10.2.16)$$

There are more solutions since the equations (10.2.15) is invariant under local  $SL(2)$  transformations acting  $\check{\xi}_{\check{A}}$  and  $\check{\bar{\xi}}_{\check{A}}$  through the index  $\check{A}$ , but one can show the solution is unique up to this  $SL(2)$ . Using them the SUSY transformation rule for hypermultiplet can be expressed as follows,

$$\begin{aligned} \mathbf{Q}q_A &= -i\xi_A \psi + i\bar{\xi}_A \bar{\psi}, \\ \mathbf{Q}\psi &= 2\sigma^m \bar{\xi}_A D_m q^A + \sigma^m D_m \bar{\xi}_A q^A - 4i\xi_A \bar{\phi} q^A + 2\check{\xi}_{\check{A}} F^{\check{A}}, \\ \mathbf{Q}\bar{\psi} &= 2\bar{\sigma}^m \xi_A D_m q^A + \bar{\sigma}^m D_m \xi_A q^A - 4i\bar{\xi}_A \phi q^A + 2\check{\bar{\xi}}_{\check{A}} F^{\check{A}}, \\ \mathbf{Q}F_{\check{A}} &= i\check{\xi}_{\check{A}} \sigma^m D_m \bar{\psi} - 2\check{\xi}_{\check{A}} \phi \psi - 2\check{\xi}_{\check{A}} \lambda_B q^B + 2i\check{\xi}_{\check{A}} (\sigma^{kl} T_{kl}) \psi \\ &\quad - i\check{\bar{\xi}}_{\check{A}} \bar{\sigma}^m D_m \psi + 2\check{\bar{\xi}}_{\check{A}} \bar{\phi} \bar{\psi} + 2\check{\bar{\xi}}_{\check{A}} \bar{\lambda}_B q^B - 2i\check{\bar{\xi}}_{\check{A}} (\bar{\sigma}^{kl} \bar{T}_{kl}) \bar{\psi}. \end{aligned} \quad (10.2.17)$$

Similar off-shell transformation rule was used in [9] for 4D  $\mathcal{N} = 4$  SYM theory using Berkovits construction of 10D  $\mathcal{N} = 1$  SYM theory [73]. The SUSY invariant kinetic Lagrangian is

$$\begin{aligned}\mathcal{L}_{\text{mat}} = & \frac{1}{2}D_m q^A D^m q_A - q^A \{\phi, \bar{\phi}\} q_A + \frac{i}{2} q^A D_{AB} q^B + \frac{1}{8}(M + R) q^A q_A \\ & - \frac{i}{2} \bar{\psi} \bar{\sigma}^m D_m \psi - \frac{1}{2} \psi \phi \psi + \frac{1}{2} \bar{\psi} \bar{\phi} \bar{\psi} + \frac{i}{2} \psi \sigma^{kl} T_{kl} \psi - \frac{i}{2} \bar{\psi} \bar{\sigma}^{kl} \bar{T}_{kl} \bar{\psi} \\ & - q^A \lambda_A \psi + \bar{\psi} \bar{\lambda}_A q^A - \frac{1}{2} F^{\dot{A}} F_{\dot{A}}.\end{aligned}\quad (10.2.18)$$

The auxiliary symmetry transforms  $F_{I\dot{A}}$ ,  $\check{\xi}_{\dot{A}}$  and  $\bar{\xi}_{\dot{A}}$  all as doublets, and it is actually  $SU(2)$  since we need to impose  $F_{I\dot{A}}$  a reality condition similar to (10.2.13). To complete the off-shell formalism for hypermultiplets, one needs to specify the background gauge field  $(\check{V}_m)^{\dot{A}}_{\dot{B}}$  for this auxiliary symmetry which we call  $SU(2)_{\check{R}}$ .

The commutant of the gauge group within  $Sp(r)$  gives the global symmetry. One can introduce the mass for hypermultiplets by coupling an abelian subgroup of the global symmetry to background vector multiplets. Mass parameters are identified with the constant value of their scalar components  $\phi, \bar{\phi}$ . They have to be chosen not to break supersymmetry, so the fermion components of the background vector multiplet must have vanishing SUSY variation. The classical values

$$\phi = \bar{\phi} = \text{constant}, \quad D_{AB} = 2w_{AB}\phi \quad (10.2.19)$$

preserve the supersymmetry if the corresponding Killing spinor satisfy (10.2.11).

The square of supersymmetry  $\mathbf{Q}$  yields a sum of bosonic symmetry transformations including the translation by  $v^m \equiv 2\bar{\xi}^A \bar{\sigma}^m \xi_A$ ,

$$\begin{aligned}\mathbf{Q}^2 = & i\mathcal{L}_v \\ & + \text{Gauge} \left[ 2\phi \bar{\xi}^A \bar{\xi}_A - 2\bar{\phi} \xi^A \xi_A + v^m A_m \right] \\ & + \text{Lorentz} \left[ D_{[a} v_{b]} + v^m \Omega_{mab} \right] \\ & + \text{Scale} \left[ -\frac{i}{2} \xi^A \sigma^m D_m \bar{\xi}_A - \frac{i}{2} D_m \xi^A \sigma^m \bar{\xi}_A \right] \\ & + \text{R}_{U(1)} \left[ -\frac{i}{4} \xi^A \sigma^m D_m \bar{\xi}_A + \frac{i}{4} D_m \xi^A \sigma^m \bar{\xi}_A \right] \\ & + \text{R}_{SU(2)} \left[ -i \xi_{(A} \sigma^m D_m \bar{\xi}_{B)} + i D_m \xi_{(A} \sigma^m \bar{\xi}_{B)} + v^m V_{mAB} \right] \\ & + \check{\text{R}}_{SU(2)} \left[ 2i \check{\xi}_{(A} \sigma^m D_m \check{\xi}_{B)} - 2i D_m \check{\xi}_{(A} \sigma^m \check{\xi}_{B)} \right. \\ & \quad \left. + 4i \check{\xi}_{(A} \sigma^{kl} T_{kl} \check{\xi}_{B)} - 4i \check{\xi}_{(A} \bar{\sigma}^{kl} \bar{T}_{kl} \check{\xi}_{B)} + v^m \check{V}_{mAB} \right].\end{aligned}\quad (10.2.20)$$

Note that the Killing spinor  $(\xi_A, \bar{\xi}_A)$ , the auxiliary spinor  $(\check{\xi}_{\dot{A}}, \bar{\check{\xi}}_{\dot{A}})$  as well as all the background fields belonging to the gravity multiplet have to be invariant under  $\mathbf{Q}^2$ . This can be used to determine the form of  $(\check{V}_m)^{\dot{A}}_{\dot{B}}$ . Note also that, if one wants to introduce the mass or FI terms into the theory, the Killing spinor has to satisfy an extra condition (10.2.11). This implies

$$\xi^A \sigma^m D_m \bar{\xi}_A = \bar{\xi}^A \bar{\sigma}^m D_m \xi_A = 0, \quad (10.2.21)$$

so that  $\mathbf{Q}^2$  does not yield scale or  $U(1)_{\text{R}}$  transformations.

## 10.2.4 Examples of SUSY backgrounds

Let us review here some important examples of classical supergravity backgrounds with rigid SUSY.

**Topological twist** It is known that 4D  $\mathcal{N} = 2$  theories can be put on any 4D spaces preserving a single scalar supercharge by a procedure called Donaldson-Witten topological twist [4]. In the supergravity framework, topological twist corresponds to turning on a background  $SU(2)_R$  gauge field which equals the self-dual part of spin connection,

$$\frac{1}{4}\Omega_m^{ab}(\bar{\sigma}_{ab})^A_B + i(V_m)^A_B = 0, \quad (10.2.22)$$

so that the constant spinor  $\xi_{\alpha A} = 0$ ,  $\bar{\xi}_A^{\dot{\alpha}} = \delta_A^{\dot{\alpha}}$  satisfies the Killing spinor equation (10.2.3). The supersymmetry  $\mathbf{Q}$  is nilpotent up to gauge transformations, so that one can define physical observables by cohomology of  $\mathbf{Q}$  acting on gauge-invariant operators.

The choice of the background  $SU(2)_R$  gauge field allows one to identify the indices  $A, B, \dots$  with the dotted spinor indices. The chiral gaugino  $\lambda_{\alpha A}$  then turns into a vector  $\psi_m$  which is the superpartner of  $A_m$  under  $\mathbf{Q}$ , whereas the anti-chiral gaugino  $\bar{\lambda}_A^{\dot{\alpha}}$  gives rise to a scalar  $\eta$  and a self-dual tensor  $\chi_{mn}^+$ . The fermion  $\chi_{mn}^+$  and its superpartner play the role of Lagrange multiplier which reduces the path integral over the gauge field to a finite-dimensional moduli space of instanton configurations satisfying  $\frac{1}{2}\varepsilon_{klmn}F^{mn} = -F_{kl}$ . The contribution from  $k$ -instanton configurations is weighted by  $e^{2\pi i k \tau} = q^k$  since the SYM action can be written as

$$S_{\text{YM}} = 2\pi i \tau \cdot \frac{1}{8\pi^2} \int \text{Tr} F \wedge F + \mathbf{Q}(\dots). \quad (10.2.23)$$

Similarly, by setting  $SU(2)_R$  gauge field equal to the anti-self-dual part of spin connection, one obtains a supersymmetric background corresponding to anti-twisted theory for which the path integrals localize to moduli space of anti-instantons.

**Omega backgrounds** Omega background is a deformation of topologically twisted theory such that  $\mathbf{Q}$  is not nilpotent but squares to an isometry of the background metric. The simplest example is the Omega-deformation of flat space often denoted as  $\mathbb{R}_{\epsilon_1, \epsilon_2}^4$ . Path integrals of gauge theories on such a background reduce to equivariant integrals on instanton moduli space, that is the problem of counting the configurations of point-like instantons localized at the origin, and gives the definition of Nekrasov's instanton partition function [5–8].

To be a little more explicit, the Omega background  $\mathbb{R}_{\epsilon_1, \epsilon_2}^4$  is characterized by a scalar supercharge which squares to a rotation,

$$\mathbf{Q}^2 = i\mathcal{L}_v + (\dots), \quad v \equiv \epsilon_1 \left( x_1 \frac{\partial}{\partial x_2} - x_2 \frac{\partial}{\partial x_1} \right) + \epsilon_2 \left( x_3 \frac{\partial}{\partial x_4} - x_4 \frac{\partial}{\partial x_3} \right). \quad (10.2.24)$$

To realize it within the supergravity framework, one chooses the Killing spinor with constant  $\bar{\xi}_A$  as before, and also a nonvanishing  $\xi_A$  so that  $2\bar{\xi}^A\bar{\sigma}^m\xi_A = v^m$  holds. More explicitly,

$$\bar{\xi}_A^{\dot{\alpha}} = \frac{1}{\sqrt{2}}\delta_A^{\dot{\alpha}}, \quad \xi_{\alpha A} = -\frac{1}{2}v_m(\sigma^m)_{\alpha\dot{\alpha}}\bar{\xi}_A^{\dot{\alpha}}. \quad (10.2.25)$$

In order for this to satisfy the equation (10.2.6) one needs to put

$$M = \bar{T}_{kl} = 0, \quad T_{kl} = -\frac{1}{8}D_{[k}v_{l]} \quad \left( \text{or } \frac{1}{2}T_{kl}dx^kdx^l = \frac{\epsilon_2 - \epsilon_1}{16}(dx^1dx^2 - dx^3dx^4) \right) \quad (10.2.26)$$

Note that for  $\epsilon_1 = \epsilon_2$  no background auxiliary fields need to be turned on. A related remark is that the orientation reversal of one of the coordinate axes (“parity”) leads to the sign flip of either  $\epsilon_1$  or  $\epsilon_2$ , but at the same time flips the definition of chirality for spinors. Therefore, twisted theory on  $\mathbb{R}_{\epsilon_1, \epsilon_2}^4$  and anti-twisted theory on  $\mathbb{R}_{\epsilon_1, -\epsilon_2}^4$  are related by parity.

For the choice of Killing spinor (10.2.25), the simplest solution to the equation (10.2.15) is

$$\check{\xi}_\alpha^{\check{A}} = \frac{1}{\sqrt{2}}\delta_\alpha^{\check{A}}, \quad \bar{\xi}^{\dot{\alpha}\check{A}} = \frac{1}{2}v_m(\bar{\sigma}^m)^{\dot{\alpha}\alpha}\check{\xi}_\alpha^{\check{A}}. \quad (10.2.27)$$

Therefore the  $SU(2)_R$  indices are identified with dotted spinor indices as before, whereas the  $SU(2)_{\check{R}}$  indices are identified as undotted spinor indices.

More generally, starting from a topologically twisted theory on a manifold with an isometry generated by a Killing vector field  $v$ , one can introduce Omega-deformation by choosing the Killing spinor as (10.2.25) and the background fields as in (10.2.26).

**The sphere and ellipsoids** Here we review the construction of a supersymmetric ellipsoid background following [32]. The ellipsoid of our interest is defined as a hypersurface embedded in the flat  $\mathbb{R}^5$ ,

$$\frac{x_0^2}{r^2} + \frac{x_1^2 + x_2^2}{\ell^2} + \frac{x_3^2 + x_4^2}{\tilde{\ell}^2} = 1. \quad (10.2.28)$$

with  $U(1) \times U(1)$  isometry. Note that here we are interested in the “physical” SUSY and not the SUSY of topologically twisted theories, so that the observables should depend non-trivially on some of the axis-length parameters  $\ell, \tilde{\ell}, r$ . The square of the SUSY will include a linear combinations of the two  $U(1)$  isometries rotating the 12- and 34-planes about the origin.

A convenient set of coordinates is the polar angles  $(\rho, \theta, \varphi, \chi)$  which are related to the Cartesian coordinates on  $\mathbb{R}^5$  as

$$\begin{aligned} x_0 &= r \cos \rho, \\ x_1 &= \ell \sin \rho \cos \theta \cos \varphi, \\ x_2 &= \ell \sin \rho \cos \theta \sin \varphi, \\ x_3 &= \tilde{\ell} \sin \rho \sin \theta \cos \chi, \\ x_4 &= \tilde{\ell} \sin \rho \sin \theta \sin \chi. \end{aligned} \quad (10.2.29)$$

The two  $U(1)$  isometries of the ellipsoid are generated by Killing vectors  $\partial_\varphi$  and  $\partial_\chi$ . The north pole ( $\rho = 0$ ) and the south pole ( $\rho = \pi$ ) are the two fixed points of the isometry. Using the above polar angle coordinate system, we see the ellipsoid as a squashed  $S^3$  (with coordinates  $\theta, \varphi, \chi$ ) fibred over a segment  $0 \leq \rho \leq \pi$ .

For the round  $S^4$  with  $\ell = \tilde{\ell} = r$  the metric becomes

$$ds^2 = \ell^2(d\rho^2 + \sin^2 \rho \cdot ds_{(S^3)}^2) = E^1 E^1 + \dots + E^4 E^4. \quad (10.2.30)$$

A standard choice for the vielbein one-forms  $E^a$  is

$$E^1 = \ell \sin \rho \cos \theta d\varphi, \quad E^2 = \ell \sin \rho \sin \theta d\chi, \quad E^3 = \ell \sin \rho d\theta, \quad E^4 = \ell d\rho. \quad (10.2.31)$$

Note that  $E^1, E^2, E^3$  are proportional to the vielbein on the round  $S^3$ . A nice fact about this choice of frames is that one can relate part of the Killing spinor equation on  $S^4$  to that on  $S^3$ , so that the independent Killing spinors on  $S^4$  are all given by those on  $S^3$  multiplied by some functions of  $\rho$ . Let us choose the following particular solution,

$$\begin{aligned} \xi_{A=1} &= \sin \frac{\rho}{2} \cdot \kappa_+, & \bar{\xi}_{A=1} &= +i \cos \frac{\rho}{2} \cdot \kappa_+, & \kappa_\pm &= \frac{1}{2} \begin{pmatrix} e^{\frac{i}{2}(\pm\varphi \pm \chi - \theta)} \\ \mp e^{\frac{i}{2}(\pm\varphi \pm \chi + \theta)} \end{pmatrix}. \end{aligned} \quad (10.2.32)$$

The square of the corresponding SUSY includes a rotation  $v = \epsilon(\partial_\varphi + \partial_\chi)$  with  $\epsilon = \ell^{-1}$ . The theory near the north pole is thus approximately the topologically twisted theory on  $\mathbb{R}_{\epsilon, \epsilon}^4$ , whereas the theory near the south pole is the anti-twisted theory on  $\mathbb{R}_{\epsilon, -\epsilon}^4$ , where the minus sign accounts for the relative orientation flip between the two polar regions. It then follows from SUSY localization that, as long as we are interested in supersymmetric observables, the instantons and anti-instantons have to be localized at the north and south poles respectively. Their contributions are thus expressed by products of two Nekrasov partition functions with  $\epsilon_1 = \epsilon_2 = \ell^{-1}$  [9].

It is natural to ask whether there are supersymmetric deformations of the round sphere geometry which approach the general Omega background, with  $\epsilon_1$  and  $\epsilon_2$  independent, near the two poles. A reasonable guess would be that there should be a supersymmetric ellipsoid background with nonzero auxiliary fields in gravity multiplet, such that (10.2.32) remains a Killing spinor. If that is the case, the Killing vector field  $v$  appearing in the square of supersymmetry is

$$v \equiv 2\bar{\xi}^A \bar{\sigma}^m \xi_A \partial_m = \epsilon_1 \partial_\varphi + \epsilon_2 \partial_\chi, \quad \left( \epsilon_1 \equiv \frac{1}{\ell}, \quad \epsilon_2 \equiv \frac{1}{\tilde{\ell}} \right) \quad (10.2.33)$$

which indeed approach the desired rotation generator near the poles.

It was shown in [32] that the above naive guess is actually right. The generalized Killing spinor equation (10.2.6), with the above form of  $\xi_A$  and  $\bar{\xi}_A$  assumed, can be regarded as a linear algebraic equation for the auxiliary fields  $T_{mn}, \bar{T}_{mn}, (V_m)^A_B, M$  in gravity multiplet. Though the set of equations looks highly over-determined, it was shown to have a family of solutions. The explicit form of the background fields was obtained in [32]. The square of the supersymmetry was shown to be given by

$$\mathbf{Q}^2 = i\mathcal{L}_v + \text{Gauge}[\hat{\Phi}] + \text{R}_{SU(2)}[\Theta^A_B] + \check{\text{R}}_{SU(2)}[\check{\Theta}^{\check{A}}_{\check{B}}], \quad \Theta = \check{\Theta} = -\frac{\epsilon_1 + \epsilon_2}{2} \boldsymbol{\tau}^3 \quad (10.2.34)$$

where we used the standard solution for  $\check{\xi}_{\check{A}}, \bar{\xi}_{\check{A}}$  (10.2.16) to fix the gauge for local  $SU(2)_{\check{R}}$  symmetry, and  $\hat{\Phi}$  was defined in (10.2.9).

It is an interesting exercise to study the behavior of the supersymmetric ellipsoid background near the poles. Near the north pole one can use the Cartesian coordinates

$$x_1 = \ell \rho \cos \theta \cos \varphi, \quad x_2 = \ell \rho \cos \theta \sin \varphi, \quad x_3 = \tilde{\ell} \rho \sin \theta \cos \chi, \quad x_4 = \tilde{\ell} \rho \sin \theta \sin \chi, \quad (10.2.35)$$

assuming  $|x| \ll \ell \sim \tilde{\ell}$ . There the chiral component  $\xi_A$  of the Killing spinor (10.2.6) vanishes linearly in  $\rho$ , whereas the anti-chiral component  $\bar{\xi}_A$  stays finite. Therefore, by a suitable local Lorentz and  $SU(2)_{\check{R}}$  rotations it can be transformed into the form (10.2.25). Using  $\epsilon_1 = \ell^{-1}$  and  $\epsilon_2 = \tilde{\ell}^{-1}$ , one can show the auxiliary field  $T_{mn}$  agrees with (10.2.26) and  $\bar{T}_{mn} = 0$  to the leading order in small  $\epsilon_i |x|$ . However, the ellipsoids have nonvanishing curvature tensor, and accordingly the  $SU(2)_{\check{R}}$  gauge field is also non-vanishing. The nonzero components of the Riemann tensor  $R_{mn}^{ab}$  and the  $SU(2)_{\check{R}}$  gauge field strength  $(V_{mn})^A_B$ , measured in Cartesian coordinates, are of the order  $\epsilon_i^2$ . See [74] for the full details.

**Local  $T^2$ -bundle fibrations** It was shown in [74] that the ellipsoid backgrounds of [32] can be regarded as an example of supersymmetric *local  $T^2$ -bundle fibrations*, for which one can apply the same procedure as explained above to determine the necessary background auxiliary fields for general squashing parameters.

## 10.3 Partition function

Let us review here the application of localization principle to  $\mathcal{N} = 2$  supersymmetric path integrals on  $S^4$ , with some close look into the use of index theorem and the fixed point formula. We also present a closed form for the partition function, and review how it simplifies to a Gaussian matrix integral for  $\mathcal{N} = 2^*$  theories for special choices of mass parameter.

### 10.3.1 Localization principle

Let us recall how the SUSY localization principle simplifies the problems of path integration. Suppose a quantum field theory with an action  $S$  and a path-integral measure  $f$  has a supersymmetry  $\mathbf{Q}$ , which means that the expectation values of  $\mathbf{Q}$ -exact observables all vanish.

$$\langle \mathbf{Q}\mathcal{O} \rangle = \int e^{-S} \cdot \mathbf{Q}\mathcal{O} = 0. \quad (10.3.1)$$

In such a theory, expectation values of  $\mathbf{Q}$ -invariant observable are invariant under any deformation of the action of the form  $S \rightarrow S + t\mathbf{Q}V$ , where the parameter  $t$  is arbitrary and  $\mathbf{Q}^2V = 0$ . It is standard to construct  $V$  as the bilinear of all the fermions  $\Psi$  and their

$\mathbf{Q}$ -variations, because  $\mathbf{Q}V$  will then have manifestly positive-definite bosonic part.

$$\begin{aligned} V &= \int d^4x \sqrt{g} \sum_{\Psi} (\mathbf{Q}\Psi)^\dagger \Psi, \\ \mathbf{Q}V &= \int d^4x \sqrt{g} \left[ \sum_{\Psi} (\mathbf{Q}\Psi)^\dagger \mathbf{Q}\Psi + \dots \right]. \end{aligned} \quad (10.3.2)$$

The values of supersymmetric observables should be  $t$ -independent, so one may evaluate them at a very large  $t$ . There the deformed action is dominated by the term  $\mathbf{Q}V$ , and nonzero contribution to the path integral arise only from the vicinity of saddle points characterized by

$$\mathbf{Q}\Psi = 0 \text{ for all the fermions } \Psi. \quad (10.3.3)$$

Let us apply this to the general  $\mathcal{N} = 2$  gauge theories of vector and hypermultiplets on ellipsoids. It is easy to check that the saddle point equation (10.3.3) is solved by

$$\begin{aligned} \text{vector multiplet} &: A_m = 0, \quad \phi = \bar{\phi} = -\frac{i}{2} a_0 \text{ (constant)}, \quad D_{AB} = -i a_0 w_{AB}, \\ \text{hypermultiplet} &: q_A = F_{\tilde{A}} = 0, \end{aligned} \quad (10.3.4)$$

where  $w_{AB}$  was introduced in (10.2.11). What is more non-trivial is to prove there are no other saddle points: this has been done explicitly only for the case of round  $S^4$  [9]. Assuming that it continues to be the case for more general ellipsoid backgrounds, one can argue that the path integral reduces to a finite-dimensional integral over the space of saddle points parametrized by a Lie algebra-valued constant  $a_0$ .

An important subtlety in solving the saddle point equation is that, if one relaxes the condition that the solution be smooth everywhere, the gauge field is allowed to take nonzero singular values localized at the two poles [9]. The field strength must be anti-self-dual at the north pole and self-dual at the south pole. This is how the (anti-)instanton can make nonperturbative contribution to supersymmetric observables. As was explained in the previous section, their contribution is precisely given by Nekrasov's partition function, with argument  $q$  for instantons at the north pole and  $\bar{q}$  for the anti-instantons at the south pole.

Localization principle thus leads to the following formula for partition function,

$$Z = \int d^r a_0 e^{-S_{\text{cl}}(a_0)} Z_{1\text{-loop}}(a_0, m, \epsilon_1, \epsilon_2) Z_{\text{inst}}(a_0, m, q, \epsilon_1, \epsilon_2) Z_{\text{inst}}(a_0, m, \bar{q}, \epsilon_1, \epsilon_2). \quad (10.3.5)$$

Here the identification  $\epsilon_1 = 1/\ell$ ,  $\epsilon_2 = 1/\tilde{\ell}$  was used.  $S_{\text{cl}}(a_0)$  is the original action evaluated at saddle points, and the product of Nekrasov's partition function  $Z_{\text{inst}}$  expresses the contribution of (anti-)instantons at the poles. The one-loop factor  $Z_{1\text{-loop}}$  arises from path integrating over all the modes orthogonal to the saddle point locus, for which Gaussian approximation gives an exact answer thanks to localization principle. Finally, although the saddle points are labeled by a Lie-algebra valued parameter  $a_0$ , the integral can be reduced to its Cartan subalgebra. As is well known, the invariant measure  $[da_0]$  on a Lie algebra is related to the measure  $d^r a_0$  on its Cartan subalgebra by

$$[da_0] = d^r a_0 \cdot \prod_{\alpha \in \Delta_+} (a_0 \cdot \alpha)^2. \quad (10.3.6)$$

In the formula (10.3.5), the Vandermode factor is understood to be contained in  $Z_{1\text{-loop}}$ .

The SUSY invariant action in general consists of the Yang-Mills term (10.2.10), the Feyet-Illiopoulos term (10.2.12) and the hypermultiplet kinetic term (10.2.18). Its classical value at the saddle point  $a_0$  is therefore given by the sum of the following,

$$S_{\text{YM}} = \frac{8\pi^2}{g^2} \ell \tilde{\ell} \text{Tr}(a_0^2), \quad S_{\text{FI}} = -16i\pi^2 \ell \tilde{\ell} \zeta a_0, \quad S_{\text{mat}} = 0. \quad (10.3.7)$$

In fact, one can show that  $S_{\text{mat}}$  is exact under the supersymmetry corresponding to Killing spinors satisfying  $\xi^A \xi_A - \bar{\xi}^A \bar{\xi}_A = 1$ .

### 10.3.2 Gauge fixing

We now turn to the explicit path-integration. The first thing we have to do is to fix a gauge. Following the standard prescription, we introduce the ghost  $c$ , anti-ghost  $\bar{c}$  and a Lagrange multiplier boson  $B$ . We also introduce a nilpotent symmetry  $\mathbf{Q}_B$  which acts on every physical field  $X$  as a gauge transformation by parameter  $c$ ,

$$\mathbf{Q}_B X = \text{Gauge}[c]X. \quad \left( \text{example: } \mathbf{Q}_B A_m = D_m c, \quad \mathbf{Q}_B \lambda_A = i\{c, \lambda_A\} \right) \quad (10.3.8)$$

To achieve nilpotency, the ghost fields should transform by  $\mathbf{Q}_B$  as follows,

$$\mathbf{Q}_B c = icc, \quad \mathbf{Q}_B \bar{c} = B, \quad \mathbf{Q}_B B = 0. \quad (10.3.9)$$

Here we decide *not* to fix the coordinate-independent part of the gauge symmetry by this procedure. Therefore the fields  $c, \bar{c}, B$  are assumed to have no constant modes. (One could alternatively eliminate the constant modes of those fields by introducing constant “ghost-for-ghost” fields [9, 32].) We also define the action of  $\mathbf{Q}$  on the ghost fields

$$\mathbf{Q}c = a_0 - \hat{\Phi}, \quad \mathbf{Q}\bar{c} = 0, \quad \mathbf{Q}B = i\mathcal{L}_v \bar{c} + i[a_0, \bar{c}], \quad (10.3.10)$$

so that the square of the total supercharge  $\hat{\mathbf{Q}} \equiv \mathbf{Q} + \mathbf{Q}_B$  acts on all the fields as follows (compare with the formula (10.2.34) for  $\mathbf{Q}^2$ ),

$$\hat{\mathbf{Q}}^2 = i\mathcal{L}_v + \text{Gauge}[a_0] + \text{R}_{SU(2)}\left[-\frac{1}{2}(\epsilon_1 + \epsilon_2)\boldsymbol{\tau}^3\right] + \check{\text{R}}_{SU(2)}\left[-\frac{1}{2}(\epsilon_1 + \epsilon_2)\boldsymbol{\tau}^3\right]. \quad (10.3.11)$$

Usual gauge fixing proceeds by choosing an arbitrary gauge-fixing functional  $G$ , for example the Lorentz gauge  $G = \partial_m A^m$ , and modifying the action by the addition of gauge-fixing term  $\mathbf{Q}_B(\bar{c}G)$ . As was shown in [9], one can replace the gauge-fixing term by  $\hat{\mathbf{Q}}(\bar{c}G)$  without changing the value of partition function. The total supersymmetry  $\hat{\mathbf{Q}}$  is then preserved and can be used for localization argument.

### 10.3.3 Determinants and index

We now turn to the gauge-fixed path integral with respect to fluctuations around saddle points. We take the  $\hat{\mathbf{Q}}$ -exact deformation term (including the gauge-fixing term)

$$\hat{\mathbf{Q}}\hat{V} = \hat{\mathbf{Q}}(V + \bar{c}G), \quad (10.3.12)$$

to be very large, so that Gaussian approximation becomes actually exact and path integral simply gives rise to determinants. We also notice that, after the introduction of ghost fields, the number of bosons and fermions agree off-shell: a vector multiplet consists of ten bosons  $(A_m, \phi, \bar{\phi}, D_{AB}, B)$  and ten fermions  $(\lambda_{\alpha A}, \bar{\lambda}_A^{\dot{\alpha}}, c, \bar{c})$ , likewise a hypermultiplet consists of four bosons  $(q_A, F_{\check{A}})$  and four fermions  $(\psi_{\alpha}, \bar{\psi}^{\dot{\alpha}})$ . This is of course important for the localization principle to work.

We move to a new set of fields which is particularly useful for evaluating the fluctuation determinant. We first define fermions without spinor indices from gauginos,

$$\Psi \equiv -i\xi^A \lambda_A - i\bar{\xi}^{\dot{A}} \bar{\lambda}_A, \quad \Psi_m \equiv i\xi^A \sigma_m \bar{\lambda}_A - i\bar{\xi}^{\dot{A}} \bar{\sigma}_m \lambda_A, \quad \Xi_{AB} \equiv 2\bar{\xi}_{(A} \bar{\lambda}_{B)} - 2\xi_{(A} \lambda_{B)}, \quad (10.3.13)$$

so that the supersymmetry transformation rule simplifies.

$$\mathbf{Q}\phi_2 = \Psi, \quad \mathbf{Q}A_m = \Psi_m, \quad \mathbf{Q}\Xi_{AB} = D_{AB} + (\dots). \quad (10.3.14)$$

Likewise, from the fermion in hypermultiplet we define

$$\begin{aligned} \Psi_A &\equiv -i\xi_A \psi + i\bar{\xi}_A \bar{\psi}, & \mathbf{Q}q_A &= \Psi_A, \\ \Xi_{\check{A}} &\equiv \check{\xi}_{\check{A}} \psi - \check{\xi}_{\check{A}} \bar{\psi}, & \mathbf{Q}\Xi_{\check{A}} &= F_{\check{A}} + (\dots). \end{aligned} \quad (10.3.15)$$

It is then convenient to take five bosons  $\mathbf{X} = (A_m, \phi_2 \equiv \phi - \bar{\phi})$ , five fermions  $\Xi = (\Xi_{AB}, \bar{c}, c)$  and their  $\hat{\mathbf{Q}}$ -superpartners as independent variables for vector multiplet. Similarly, for hypermultiplet we take two bosons  $\mathbf{X} = q_A$ , two fermions  $\Xi = \Xi_{\check{A}}$  and their  $\hat{\mathbf{Q}}$ -superpartners as independent variables.

In quadratic approximation, the  $\hat{\mathbf{Q}}$ -exact deformation term (10.3.12) decomposes into vectormultiplet and hypermultiplet parts, and each term has the structure

$$\begin{aligned} \hat{V} \Big|_{\text{quad.}} &= (\hat{\mathbf{Q}}\mathbf{X}, \Xi) \begin{pmatrix} D_{00} & D_{01} \\ D_{10} & D_{11} \end{pmatrix} \begin{pmatrix} \mathbf{X} \\ \hat{\mathbf{Q}}\Xi \end{pmatrix} \\ \hat{\mathbf{Q}}\hat{V} \Big|_{\text{quad.}} &= (\mathbf{X}, \hat{\mathbf{Q}}\Xi) \underbrace{\begin{pmatrix} -\mathbf{H} & 0 \\ 0 & 1 \end{pmatrix}}_{=K_b} \begin{pmatrix} D_{00} & D_{01} \\ D_{10} & D_{11} \end{pmatrix} \begin{pmatrix} \mathbf{X} \\ \hat{\mathbf{Q}}\Xi \end{pmatrix} \\ &\quad - (\hat{\mathbf{Q}}\mathbf{X}, \Xi) \underbrace{\begin{pmatrix} D_{00} & D_{01} \\ D_{10} & D_{11} \end{pmatrix}}_{=K_f} \begin{pmatrix} 1 & 0 \\ 0 & \mathbf{H} \end{pmatrix} \begin{pmatrix} \hat{\mathbf{Q}}\mathbf{X} \\ \Xi \end{pmatrix}, \end{aligned} \quad (10.3.16)$$

where we denoted  $\mathbf{H} = \hat{\mathbf{Q}}^2$ . The Gaussian integral thus gives the square root of the following ratio of determinants,

$$\frac{\det K_f}{\det K_b} = \frac{\det_{\Xi} \mathbf{H}}{\det_{\mathbf{X}} \mathbf{H}} = \frac{\det_{\text{Coker} D_{10}} \mathbf{H}}{\det_{\text{Ker} D_{10}} \mathbf{H}}. \quad (10.3.17)$$

The last equality follows from the fact that the fields  $\mathbf{X}$  and  $\Xi$  take values on the spaces related by the operator  $D_{10}$ , and that  $\mathbf{H}$  commutes with  $D_{10}$ . The ratio of determinants is closely related to the index defined by

$$\text{Ind}(D_{10}) \equiv \text{Tr}_{\text{Ker} D_{10}}(e^{-i\mathbf{H}t}) - \text{Tr}_{\text{Coker} D_{10}}(e^{-i\mathbf{H}t}). \quad (10.3.18)$$

The index can be evaluated using the fixed-point formula, which is based on the following simple idea. We are interested in the trace of the operator  $e^{-i\mathbf{H}t}$  involving a finite diffeomorphism  $x^m \rightarrow \tilde{x}^m$ , and the index is the difference of the traces evaluated at the space of fields  $\mathbf{X}$  and  $\Xi$ . Since the trace of a matrix is the sum of diagonal elements, the trace of a finite diffeomorphism operator should be expressed as a  $d^4x$  integral of a function involving  $\delta^4(\tilde{x} - x)$ . The index is thus expressed as a sum over fixed point contributions,

$$\text{Ind}(D_{10}) = \sum_{x_0: \text{fixed points}} \frac{\text{Tr}_{\mathbf{X}}(e^{-i\mathbf{H}t})|_{x_0} - \text{Tr}_{\Xi}(e^{-i\mathbf{H}t})|_{x_0}}{\det(1 - \partial\tilde{x}/\partial x)}. \quad (10.3.19)$$

Defining  $z_1 = x_1 + ix_2$  and  $z_2 = x_3 + ix_4$  from the local Cartesian coordinate near the poles, one can express the action of  $e^{-i\mathbf{H}t}$  as

$$\tilde{z}_1 = z_1 q_1 = z_1 e^{\frac{it}{\ell}}, \quad \tilde{z}_2 = z_2 q_2 = z_2 e^{\frac{it}{\ell}}. \quad (10.3.20)$$

The determinant in the denominator is therefore given by

$$\det(1 - \partial\tilde{x}/\partial x) = |(1 - q_1)(1 - q_2)|^2. \quad (10.3.21)$$

The numerator is the difference of the trace of  $e^{-i\mathbf{H}t}$  acting on fields  $\mathbf{X}$  and  $\Xi$  at fixed points. For vector multiplet fields at the north pole it becomes

$$\begin{aligned} & \text{Tr}_{\mathbf{X}}(e^{-i\mathbf{H}t})|_{\text{NP}} - \text{Tr}_{\Xi}(e^{-i\mathbf{H}t})|_{\text{NP}} \\ &= \text{Tr}_{\text{adj}}(e^{a_0 t}) \times \left\{ \underbrace{(q_1 + q_2 + \bar{q}_1 + \bar{q}_2 + 1)}_{A_m} \underbrace{\phi_2}_{\phi_2} - \underbrace{(q_1 q_2 + 1 + \bar{q}_1 \bar{q}_2 + 1 + 1)}_{D_{AB}} \underbrace{1}_{\tilde{c}, c} \right\} \end{aligned} \quad (10.3.22)$$

The contribution to the index from the North pole is therefore

$$\text{Ind}(D_{10})|_{\text{NP}} = \text{Tr}_{\text{adj}}(e^{a_0 t}) \times \frac{(q_1 + q_2 + \bar{q}_1 + \bar{q}_2 + 1) - (q_1 q_2 + 1 + \bar{q}_1 \bar{q}_2 + 1 + 1)}{(1 - q_1)(1 - q_2)(1 - \bar{q}_1)(1 - \bar{q}_2)}. \quad (10.3.23)$$

Neglecting some fields whose contribution is trivial, one can identify the above result with the index of the self-dual complex  $(D_{\text{SD}} : \Omega^0 \xrightarrow{d} \Omega^1 \xrightarrow{d^+} \Omega^{2+})$  valued in the adjoint representation of the gauge group, defined by the instanton equation and gauge equivalence.

If the four factors in the denominator were all expanded into geometric series, the result would be interpreted as the trace of  $e^{-i\mathbf{H}t}$  evaluated by expanding all the fields into the basis of monomial functions  $z_1^k z_2^l \bar{z}_1^m \bar{z}_2^n$ . However, such a trace would not make sense because there would be infinitely many degenerate eigenmodes for each eigenvalue of  $\mathbf{H}$ . The index does not suffer from the problem of infinite degeneracy, because the fraction on the right hand side of (10.3.23) is reducible reflecting the cancellation between the fields  $\mathbf{X}$  and  $\Xi$ . But there remains another more subtle issue which requires a careful regularization, as we will see below.

After simplifying the fraction, combining the contributions from the two poles and recalling that the fields  $c, \bar{c}$  do not have constant modes, the index is given by

$$\text{Ind}(D_{10})|_{\text{vec}} = \text{Tr}_{\text{adj}}(e^{a_0 t}) \times \left\{ \left[ -\frac{1+q_1 q_2}{(1-q_1)(1-q_2)} \right]_{\text{NP}} + \left[ -\frac{1+q_1 q_2}{(1-q_1)(1-q_2)} \right]_{\text{SP}} + 2 \right\} \quad (10.3.24)$$

for vector multiplet. Similarly, for hypermultiplet in the representation  $R$  of the gauge group the index becomes

$$\text{Ind}(D_{10})_{\text{hyp}} = \text{Tr}_{R+\bar{R}}(e^{a_0 t}) \times \left\{ \left[ \frac{(q_1 q_2)^{\frac{1}{2}}}{(1-q_1)(1-q_2)} \right]_{\text{NP}} + \left[ \frac{(q_1 q_2)^{\frac{1}{2}}}{(1-q_1)(1-q_2)} \right]_{\text{SP}} \right\}. \quad (10.3.25)$$

To read from the index the spectrum of  $\mathbf{H}$  which is necessary for the computation of one-loop determinant, one needs to expand the above expressions into series in  $q_1, q_2$ . But a priori there is no natural choice whether to expand in positive or negative series in  $q$ 's. We have seen above that fixed point formula allows one to express the index as a sum of pole contributions, but it does not give us any further information about which eigenmode of  $\mathbf{H}$  is supported around which pole. Indeed, although the index of a differential operator  $D_{10}$  depends only on the term of highest order in the derivative, the detailed behavior of its zeromodes depends on the subleading terms as well. One can choose the subleading term in any convenient manner so that each eigenmode of  $\mathbf{H}$  has localized support near one of the poles. The index should of course be independent of such regularizations.

Let us look into this point in more detail, taking the hypermultiplet index as an example. To the leading order in the derivatives, the differential operator  $D_{10}$  is given by

$$\Xi^{\check{A}}(D_{10})_{\check{A}B} q^B = \Xi^{\check{A}} \left( i \check{\xi}_{\check{A}} \bar{\sigma}^m \xi_B - i \check{\xi}_{\check{A}} \sigma^m \bar{\xi}_B \right) D_m q^B. \quad (10.3.26)$$

We are interested in how the zeromode wavefunctions get localized near the poles depending on the choice of the non-derivative terms. Since  $D_{10}$  has to commute with  $\mathbf{H}$ , we follow the suggestion in [9] and introduce a non-derivative term in  $D_{10}$  through the modification  $D_m \rightarrow D_m - 2isv_m$ , where  $s$  is an arbitrary real parameter. Similar modification of differential operators was considered in the study of Morse theory [75] and in particular the derivation of holomorphic Morse inequality in [76].

Near the north pole one may identify  $\Xi^{\check{A}}$  as a chiral spinor and  $q^A$  as an anti-chiral spinor,

and  $(D_{10})_{\alpha\dot{\beta}}$  is then simply the Dirac operator

$$D_{10} = \frac{1}{2}\sigma^m(i\partial_m + sv_m) = \begin{pmatrix} \partial_{\bar{z}_2} + s\epsilon_2 z_2 & \partial_{z_1} - s\epsilon_1 z_1 \\ \partial_{z_1} + s\epsilon_1 z_1 & -\partial_{\bar{z}_2} + s\epsilon_2 z_2 \end{pmatrix}. \quad (10.3.27)$$

For vector multiplet, the relevant differential operator near the north pole has the index structure  $(D_{10})_{\dot{\alpha}\dot{\beta},\gamma\delta}$ , and is the adjoint of the operator above twisted by an anti-chiral spinor bundle. Assuming that  $\epsilon_1 = \ell^{-1}$  and  $\epsilon_2 = \tilde{\ell}^{-1}$  are both positive, the operator  $D_{10}$  can be shown to have no  $\Xi$ -zeromodes, but it has  $q$ -zeromodes of the following form,

$$\begin{aligned} s > 0 &\implies q^A = \begin{pmatrix} z_1^m z_2^n e^{-s(\epsilon_1|z_1|^2 + \epsilon_2|z_2|^2)} \\ 0 \end{pmatrix}, & e^{-i\mathbf{H}t} = e^{a_0 t} \cdot q_1^{m+\frac{1}{2}} q_2^{n+\frac{1}{2}}, \\ s < 0 &\implies q^A = \begin{pmatrix} 0 \\ \bar{z}_1^m \bar{z}_2^n e^{+s(\epsilon_1|z_1|^2 + \epsilon_2|z_2|^2)} \end{pmatrix}, & e^{-i\mathbf{H}t} = e^{a_0 t} \cdot q_1^{-m-\frac{1}{2}} q_2^{-n-\frac{1}{2}}. \end{aligned} \quad (10.3.28)$$

This indicates one should expand the north-pole contribution to the index into positive (negative) series in  $q_1, q_2$  if  $s > 0$  (resp.  $s < 0$ ). The analysis goes similarly near the south pole, with the result that one has to series-expand in the opposite way. We thus arrive at the formula for the index,

$$\begin{aligned} \text{Ind}(D_{10})|_{\text{vec}} &= \text{Tr}_{\text{adj}}(e^{a_0 t}) \left\{ 2 - \sum_{m,n \geq 0} \left( q_1^m q_2^n + q_1^{m+1} q_2^{n+1} + q_1^{-m} q_2^{-n} + q_1^{-m-1} q_2^{-n-1} \right) \right\}, \\ \text{Ind}(D_{10})|_{\text{hyp}} &= \text{Tr}_{R+\bar{R}}(e^{a_0 t}) \sum_{m,n \geq 0} \left( q_1^{m+\frac{1}{2}} q_2^{n+\frac{1}{2}} + q_1^{-m-\frac{1}{2}} q_2^{-n-\frac{1}{2}} \right). \end{aligned} \quad (10.3.29)$$

Note the operator  $D_{10}$  has infinitely many zeromodes, owing to the fact that it is not elliptic but only transversely elliptic [77].

The one-loop determinant factor  $Z_{1\text{-loop}}$  in (10.3.5) can be easily obtained from the above formula for the index. We assume  $a_0$  to be in Cartan subalgebra and neglect  $a_0$ -independent factors. One then finds that  $Z_{1\text{-loop}}$  is a product of contributions from vector and hypermultiplets,

$$\begin{aligned} Z_{1\text{-loop}}^{\text{vec}} &= \prod_{\alpha \in \Delta_+} \frac{\Upsilon(i\hat{a}_0 \cdot \alpha) \Upsilon(-i\hat{a}_0 \cdot \alpha)}{(\hat{a}_0 \cdot \alpha)^2} \times (\hat{a}_0 \cdot \alpha)^2 = \prod_{\alpha \in \Delta} \Upsilon(i\hat{a}_0 \cdot \alpha), \\ Z_{1\text{-loop}}^{\text{hyp}} &= \prod_{\rho \in R} \Upsilon\left(\frac{Q}{2} + i\hat{a}_0 \cdot \rho\right)^{-1}, \end{aligned} \quad (10.3.30)$$

where we included the Vandermonde determinant (10.3.6) into  $Z_{1\text{-loop}}^{\text{vec}}$ . Here  $\hat{a}_0 = \sqrt{\ell\bar{\ell}}a_0$  is the normalized saddle-point parameter,  $\alpha \in \Delta_+$  runs over positive roots of the gauge Lie algebra and  $\rho \in R$  runs over weights of the representation  $R$ . The function  $\Upsilon(x)$  is defined as an infinite product,

$$\Upsilon(x) = \text{const} \cdot \prod_{m,n \geq 0} (x + mb + nb^{-1})(Q - x + mb + nb^{-1}), \quad \left(Q = b + \frac{1}{b}\right) \quad (10.3.31)$$

where the parameter  $b$  is related to the ellipsoid geometry by  $b = (\ell/\tilde{\ell})^{\frac{1}{2}}$ . It appears frequently in observables of Liouville or Toda CFTs with coupling  $b$ . See for example [78], where some important properties of  $\Upsilon(x)$  are also summarized.

Note that one can read off an information on one-loop running of the gauge coupling from the behavior of  $Z_{1\text{-loop}}$  for  $\ell\tilde{\ell} \ll a_0^2$ ,

$$S_{\text{YM}} = \frac{8\pi^2}{g^2} \text{Tr}(\hat{a}_0^2), \quad -\ln Z_{1\text{-loop}} \sim \ln(\ell\tilde{\ell})^{\frac{1}{2}} \cdot \left\{ \text{Tr}_{\text{adj}}(\hat{a}_0^2) - \text{Tr}_R(\hat{a}_0^2) \right\}. \quad (10.3.32)$$

Here we used the asymptotic behavior of  $\Upsilon(x)$  at large  $|x|$ ,

$$\ln \Upsilon(x) \sim \left(x - \frac{Q}{2}\right)^2 \ln x + \left(\frac{1}{6} - \frac{Q^2}{12}\right) \ln x - \frac{3}{2} \left(x - \frac{Q}{2}\right)^2 + \dots. \quad (10.3.33)$$

### 10.3.4 $\mathcal{N} = 4$ SYM and Gaussian matrix model

$\mathcal{N} = 2$  gauge theory with massless adjoint hypermultiplet has an enhanced supersymmetry and is called  $\mathcal{N} = 4$  SYM. Application of localization principle to this model is particularly interesting since one can expect to obtain nontrivial and precise evidences for the AdS/CFT correspondence. In this respect, there was a long standing conjecture that the expectation value of circular Wilson loops in  $\mathcal{N} = 4$  SYM is given by a simple Gaussian matrix integral [10, 11]. Pestun's work [9] gave an analytic proof of this conjecture.

The  $\mathcal{N} = 4$  SYM can be deformed to the so-called  $\mathcal{N} = 2^*$  theory by making the adjoint hypermultiplet massive. The measure and the one-loop determinant part of the ellipsoid partition function for this theory read

$$Z_{1\text{-loop}} = \prod_{\alpha \in \Delta_+} \frac{\Upsilon(i\hat{a}_0 \cdot \alpha) \Upsilon(-i\hat{a}_0 \cdot \alpha)}{\Upsilon(\frac{Q}{2} + i\hat{m} + i\hat{a}_0 \cdot \alpha) \Upsilon(\frac{Q}{2} + i\hat{m} - i\hat{a}_0 \cdot \alpha)}, \quad (10.3.34)$$

where  $\hat{m}$  is the normalized (dimensionless) hypermultiplet mass. Note that it is invariant under sign-flip of  $\hat{m}$  since  $\Upsilon(x) = \Upsilon(Q - x)$ .

An obvious special value of the mass is  $\hat{m} = \pm iQ/2$ , for which the  $\Upsilon$  functions in the denominator and numerator cancel precisely. Similar simplification happens also to Nekrasov's partition function. For example for  $U(N)$  gauge group,  $Z_{\text{inst}}$  is simply given by a sum over the sets of  $N$  Young diagrams weighted by  $q^k$ , where  $k$  is the total number of boxes in the  $N$  diagrams. Therefore

$$Z_{\text{inst}} = \prod_{k \geq 1} (1 - q^k)^{-N}. \quad (10.3.35)$$

The only  $a_0$ -dependence remaining in the integrand is the classical action  $S_{\text{YM}}$ . The  $a_0$  integral can be easily performed and gives  $(\text{Im}\tau)^{-N/2}$ . The result agrees with the torus partition function of the 2D CFT of  $N$  massless scalars, but is different from Gaussian matrix integral.

Another special value of the mass is  $\hat{m} = \pm \frac{i}{2}(b^{-1} - b)$ , for which the measure and the determinant become

$$Z_{1\text{-loop}} = \prod_{\alpha \in \Delta_+} \frac{\Upsilon(i\hat{a}_0 \cdot \alpha) \Upsilon(-i\hat{a}_0 \cdot \alpha)}{\Upsilon(b^{\pm 1} + i\hat{a}_0 \cdot \alpha) \Upsilon(b^{\pm 1} - i\hat{a}_0 \cdot \alpha)} = \prod_{\alpha \in \Delta_+} (\hat{a}_0 \cdot a)^2, \quad (10.3.36)$$

which is the natural measure for matrix integral. At the same time, the Nekrasov partition function becomes trivial for this special value of  $\hat{m}$ , namely  $Z_{\text{inst}} = 1$ , due to the emergence of fermionic zero modes in the moduli space of  $k(\geq 1)$  instantons. As was argued in [12], the additional fermion zero mode is the consequence of supersymmetry enhancement. Thus the SUSY path integral reduces to the Gaussian matrix integral for this special choice of  $\hat{m}$ .

## 10.4 Supersymmetric observables

We review here the application of localization principle to the evaluation of supersymmetric non-local observables – Wilson loops, 't Hooft loops and surface operators.

### 10.4.1 Wilson loops

Having understood how to compute partition function using localization principle, it is straightforward to include Wilson loop operators. Wilson loops are defined as usual by holonomy integrals along closed paths, but in supersymmetric Wilson loops the gauge field is accompanied by scalar fields in vector multiplet. Also, the loops have to be aligned with the direction of the isometry generated by  $\mathbf{Q}^2$ . For generic mutually incommensurable choice of  $\ell, \tilde{\ell}$ , there are only two types of supersymmetric closed paths:

$$\begin{aligned} S_\varphi^1(\rho) &: (x_0, x_1, x_2, x_3, x_4) = (r \cos \rho, \ell \sin \rho \cos \varphi, \ell \sin \rho \sin \varphi, 0, 0), \\ S_\chi^1(\rho) &: (x_0, x_1, x_2, x_3, x_4) = (r \cos \rho, 0, 0, \tilde{\ell} \sin \rho \cos \chi, \tilde{\ell} \sin \rho \sin \chi). \end{aligned} \quad (10.4.1)$$

Namely,  $S_\varphi^1(\rho)$  is a circle within an  $(x_1, x_2)$ -plane at a fixed  $x_0$  and  $x_3 = x_4 = 0$ , and similarly  $S_\chi^1(\rho)$  is a circle within an  $(x_3, x_4)$ -plane. The corresponding Wilson loop operators are

$$\begin{aligned} W_\varphi(R) &\equiv \text{Tr}_R \text{P exp } i \int_{S_\varphi^1(\rho)} d\varphi \left( A_\varphi - 2\ell(\phi \cos^2 \frac{\rho}{2} + \bar{\phi} \sin^2 \frac{\rho}{2}) \right), \\ W_\chi(R) &\equiv \text{Tr}_R \text{P exp } i \int_{S_\chi^1(\rho)} d\varphi \left( A_\chi - 2\tilde{\ell}(\phi \cos^2 \frac{\rho}{2} + \bar{\phi} \sin^2 \frac{\rho}{2}) \right). \end{aligned} \quad (10.4.2)$$

Note that the integrand is proportional to  $\hat{\Phi}$  of (10.2.9) evaluated along the path, so the SUSY invariance is very easy to check. The expectation values of these operators can thus be evaluated by just inserting their classical values

$$W_\varphi(R) = \text{Tr}_R \exp(-2\pi b \hat{a}_0), \quad W_\chi(R) = \text{Tr}_R \exp(-2\pi b^{-1} \hat{a}_0). \quad (10.4.3)$$

into the integrand of (10.3.5).

### 10.4.2 't Hooft loops

't Hooft loops play an equally important role as Wilson loops. They were originally introduced in [79] as a probe to distinguish different phases of gauge theories. Also, in 4D  $\mathcal{N} = 2$  SUSY gauge theories, the Wilson and 't Hooft loop operators are known to transform among one another under duality.

**Definition of 't Hooft operator** A 't Hooft operator introduces a Dirac monopole singularity along a path in a 4D space, and its charge is specified by a coweight  $B$  of the gauge group. Insertions of 't Hooft operators therefore not only changes the classical SYM action  $S_{\text{cl}}$ , but also affects the one-loop and instanton parts of the formula (10.3.5) since it changes the boundary condition for the path integration variables. This problem was analyzed in detail in [53] for a single 't Hooft operator inserted along a great circle in the equator  $S^3$  of the round sphere.

Let us first study the operator lying along the  $x^1$ -axis ( $x^2 = x^3 = x^4 = 0$ ) in the flat  $\mathbb{R}^4$ . The behavior of the magnetic field around it is

$$F \sim -\frac{B}{4} \epsilon_{ijk} \frac{x^i dx^j dx^k}{|x|^3} \quad (i, j, k = 2, 3, 4). \quad (10.4.4)$$

When the  $\theta$ -angle is nonzero, the presence of magnetic charge changes the quantization condition of electric charge [80]. This implies that the 't Hooft operator also induces nonzero electric field proportional to  $\theta$ ,

$$F_{1i} \sim \frac{i\theta g^2 B}{16\pi^2} \frac{x^i}{|x|^3}. \quad (10.4.5)$$

If we require the 't Hooft operator to be half-BPS, the scalars are also required to take non-zero values around it. If the unbroken supersymmetry is characterized by  $\xi_A = \sigma_1 \bar{\xi}_A e^{i\alpha}$ , the scalars have to behave near the 't Hooft operator as follows,

$$\phi \sim e^{i\alpha} \left( \frac{1}{4} - \frac{i\theta g^2}{32\pi^2} \right) \frac{B}{|x|}, \quad \bar{\phi} \sim e^{-i\alpha} \left( -\frac{1}{4} - \frac{i\theta g^2}{32\pi^2} \right) \frac{B}{|x|}. \quad (10.4.6)$$

Consider now general  $\mathcal{N} = 2$  SUSY theories on the round  $S^4$  with radius  $\ell$ , and put a 't Hooft operator with charge  $B$  along the circle  $S^1_\varphi$  at  $\rho = \pi/2$ , namely the intersection of the sphere (10.2.28) with  $x_0 = x_3 = x_4 = 0$ . Our Killing spinor (10.2.32) satisfies  $\xi_A = -\sigma_1 \bar{\xi}_A$  there, so we substitute  $e^{i\alpha} = -1$  into the above expressions for fields on  $\mathbb{R}^4$  and then map to  $S^4$ . Using the Cartesian coordinates  $x_0, \dots, x_4$  introduced in (10.2.28), the value of gauge and scalar fields is

$$F = -\frac{B}{4|x|^3} \epsilon_{ijk} x_i dx_j dx_k + \frac{i\theta g^2 B}{16\pi^2} \frac{\ell dx_1 dx_2}{|x|^3}, \quad (i, j, k = 0, 3, 4)$$

$$\phi = \left( -\frac{1}{4} + \frac{i\theta g^2}{32\pi^2} \right) \frac{B}{|x|} - \frac{ia_0}{2}, \quad \bar{\phi} = \left( \frac{1}{4} + \frac{i\theta g^2}{32\pi^2} \right) \frac{B}{|x|} - \frac{ia_0}{2}. \quad (10.4.7)$$

Here we used  $|x| \equiv \sqrt{x_0^2 + x_3^2 + x_4^2}$ , and we also included the constant terms for the scalars. It was shown in [53] that the above expression with  $[B, a_0] = 0$  exhausts all the saddle point configurations with the correct singular behavior of fields around the loop.

**Localization computation** To compute the expectation values of 't Hooft operators, one needs to work out the classical action on the saddle-point configuration (10.4.7), one-loop

determinant and instanton contribution. All of them receive nontrivial modification from 't Hooft operator, as we will now review.

The classical SYM action integral diverges near the 't Hooft loop since it corresponds to the self-energy of monopole. It can be regularized by removing a neighborhood of the loop  $B_3 \times S^1$  from the integration domain, and adding the boundary term

$$S_{\text{boundary}} = i\ell \int_{S^2 \times S^1} \frac{d\varphi}{2\pi} \text{Tr} \left( e^{-i\alpha} \tau \phi + e^{i\alpha} \bar{\tau} \bar{\phi} \right) F. \quad (10.4.8)$$

Here  $\varphi$  is the coordinate along the loop and  $\tau$  is the complexified gauge coupling. The total classical action evaluated on the saddle point (10.4.7) is thus finite,

$$\begin{aligned} (S_{\text{YM}} + S_{\text{boundary}}) \Big|_{\text{cl}} &= -i\pi\tau \text{Tr}(\hat{a}_{\text{N}}^2) + i\pi\bar{\tau} \text{Tr}(\hat{a}_{\text{S}}^2), \\ \hat{a}_{\text{N}} &\equiv a_0\ell - \frac{\theta g^2 B}{16\pi^2} + \frac{iB}{2}, \quad \hat{a}_{\text{S}} \equiv a_0\ell - \frac{\theta g^2 B}{16\pi^2} - \frac{iB}{2}. \end{aligned} \quad (10.4.9)$$

We notice here that  $\hat{a}_{\text{N}}$  and  $\hat{a}_{\text{S}}$  are the values of the scalar  $\hat{\Phi}$  (10.2.9) at the two poles, which are relevant in the evaluation of equivariant integrals over the instanton moduli spaces there. Therefore the argument of Nekrasov's partition functions representing the effect of instantons at the north pole (anti-instantons at the south pole) should be changed from  $\hat{a}_0$  to  $\hat{a}_{\text{N}}$  (resp.  $\hat{a}_{\text{S}}$ ).

Actually there is a subtlety in identifying  $\hat{a}_{\text{N}}, \hat{a}_{\text{S}}$  with the value of  $\hat{\Phi}$ , since the latter contains the gauge potential  $A_m$  and there is no globally well-defined expression for it in the presence of the 't Hooft operator. By integrating the expression for the field strength (10.4.7) one finds

$$\begin{aligned} A &= -\frac{B}{2} \left( \frac{x_0}{|x|} - C \right) d\chi + \frac{i\theta g^2 B}{16\pi^2} \left( \frac{\ell}{|x|} - 1 \right) d\varphi, \\ \left( d\chi = \frac{x_3 dx_4 - x_4 dx_3}{x_3^2 + x_4^2}, \quad d\varphi = \frac{x_1 dx_2 - x_2 dx_1}{x_1^2 + x_2^2}, \quad |x| = \sqrt{x_0^2 + x_3^2 + x_4^2} \right) \end{aligned} \quad (10.4.10)$$

Near the north and south poles, we choose the integration constant  $C$  as  $+1$  or  $-1$  to avoid Dirac string singularity and find  $\hat{\Phi} = \hat{a}_{\text{N}}$  or  $\hat{\Phi} = \hat{a}_{\text{S}}$ , respectively. Near the equator, the natural choice  $C = 0$  leads to

$$\hat{\Phi} = \hat{a}_{\text{E}} \equiv a_0\ell - \frac{\theta g^2 B}{16\pi^2}. \quad (10.4.11)$$

Let us next turn to the evaluation of one-loop Gaussian integral over fluctuations from the above saddle points. As in the previous section one can relate it to an index and express it as a sum over contributions from fixed points. In addition to the north and south poles, this time there is a nontrivial contribution from the equator in the vicinity of the loop, due to the change in the boundary condition of fields there. We introduce the coordinates  $\varphi \sim \varphi + 2\pi$  and  $y_1, y_2, y_3$  to parametrize the local geometry  $S^1 \times \mathbb{R}^3$  near the loop, assuming the loop is at the origin of  $\mathbb{R}^3$ . The coordinate  $\varphi$  here is the same as the angle coordinate  $\varphi$  in (10.2.29),

while the other angle coordinate  $\chi$  there corresponds to the rotation angle in  $(y_1, y_2)$ -plane here.

Our Killing spinor  $\xi_A, \bar{\xi}_A$  (10.2.32) and  $\check{\xi}_{\check{A}}, \bar{\check{\xi}}_{\check{A}}$  are anti-periodic in  $\varphi$ . It is convenient to use a local  $J_3$  transformations in  $SU(2)_R$  and  $SU(2)_{\check{R}}$  to make them all independent of  $\varphi$ . Then vector multiplet fields become all periodic in  $\varphi$ , while hypermultiplet fields are all antiperiodic. The index involves the trace of  $e^{-it\mathbf{H}}$ , where

$$\mathbf{H} = \hat{\mathbf{Q}}^2 = \frac{1}{\ell} \left( i\partial_\varphi + i\partial_\chi + \text{Gauge}[\hat{a}_E] \right) \equiv \frac{i}{\ell} \partial_\varphi + \mathbf{H}_{(3)}. \quad (10.4.12)$$

Kaluza-Klein expansion with respect to  $\varphi$  thus relates the equatorial contribution to the index of our interest to a 3D index. The reduction takes the following schematic form

$$\text{Ind}(D_{(4)}) \Big|_{\text{eq}} = \sum_n e^{\frac{int}{\ell}} \text{Ind}(D_{(3)}). \quad (10.4.13)$$

The sum with respect to  $n$  is over integers for vector multiplet index and half-odd integers for hypermultiplets. For vector multiplet, the natural choice for the operator  $D_{(3)}^{\text{vec}}$  is the one associated with the gauge equivalence classes of small fluctuations around the singular solution to Bogomolny equation  $F + *D\phi_2 = 0$ ,

$$F = -\frac{B}{4|y|^3} \epsilon_{ijk} y_i dy_j dy_k, \quad \phi_2 = -\frac{1}{2} \frac{B}{|y|}. \quad (10.4.14)$$

For hypermultiplet, the natural choice is the 3D Dirac operator  $D_{(3)}^{\text{hyp}} = i\boldsymbol{\tau}^i (\partial_{y_i} - iA_i) + \phi_2$ .

In [53] the 3D indices were evaluated by using Kronheimer's construction of  $U(1)$ -invariant instantons [81]. Consider Gibbons-Hawking parametrization of flat  $\mathbb{C}^2$ ,

$$\begin{aligned} dz_1 d\bar{z}_1 + dz_2 d\bar{z}_2 &= \frac{1}{4r} (dr^2 + r^2 d\vartheta^2 + r^2 \sin^2 \vartheta d\chi^2) + r(d\psi - \frac{1}{2} \cos \vartheta d\chi)^2 \\ &= \frac{1}{4|y|} dy_i dy_i + |y| (d\psi + \omega)^2. \\ \left( z_1 = \sqrt{r} \cos \frac{\vartheta}{2} e^{\frac{i\chi}{2} - i\psi}, \quad z_2 = \sqrt{r} \sin \frac{\vartheta}{2} e^{\frac{i\chi}{2} + i\psi} \right) \end{aligned} \quad (10.4.15)$$

An important fact here is that, if  $(A, \phi_2)$  satisfies Bogomolny equation on  $\mathbb{R}^3$ , then

$$\mathcal{A} = A - 2|y|\phi_2(d\psi + \omega), \quad (10.4.16)$$

is an anti-self-dual and  $\psi$ -translation invariant gauge field configuration on  $\mathbb{C}^2$ . Note also that the singular monopole solution (10.4.14) corresponds to a pure gauge  $\mathcal{A} = B d\psi$  under this map. This map also relates the 3D indices of interest to the restricted 4D indices, where the trace is taken only over the space of  $\psi$ -independent wave functions. For example, the index of  $D_{(3)}^{\text{vec}}$  can be computed from the index of 4D self-dual complex  $D_{\text{SD}}$  associated to the gauge equivalence class of fluctuations from an anti-self-dual connection  $\mathcal{A}$ , restricted to

$\psi$ -independent wave functions. The 3D index is thus obtained by averaging the 4D index over  $\psi$ -translations

$$\begin{aligned}
\text{Ind}(D_{(3)}^{\text{vec}}) &= \int_0^{2\pi} \frac{d\nu}{2\pi} \left\{ \text{Tr}_{\text{Ker}D_{\text{SD}}} (e^{-it\mathbf{H}_{(3)}+\nu\partial_\psi}) - \text{Tr}_{\text{Coker}D_{\text{SD}}} (e^{-it\mathbf{H}_{(3)}+\nu\partial_\psi}) \right\}_{\mathcal{A}=Bd\psi} \\
&= \int_0^{2\pi} \frac{d\nu}{2\pi} \left\{ \text{Tr}_{\text{Ker}D_{\text{SD}}} (e^{-it\mathbf{H}_{(3)}+\nu(\partial_\psi+iB)}) - \text{Tr}_{\text{Coker}D_{\text{SD}}} (e^{-it\mathbf{H}_{(3)}+\nu(\partial_\psi+iB)}) \right\}_{\mathcal{A}=0} \\
&= \int_0^{2\pi} \frac{d\nu}{2\pi} \frac{\text{Tr}_{\text{adj}}(e^{\hat{a}_{\text{E}t}+i\nu B}) \times (1+e^{-\frac{i\nu}{\ell}})(1-e^{\frac{i\nu}{2\ell}+i\nu})(1-e^{\frac{i\nu}{2\ell}-i\nu})}{(1-\delta e^{\frac{i\nu}{2\ell}-i\nu})(1-\delta e^{\frac{i\nu}{2\ell}+i\nu})(1-\delta e^{-\frac{i\nu}{2\ell}-i\nu})(1-\delta e^{-\frac{i\nu}{2\ell}+i\nu})}. \quad (10.4.17)
\end{aligned}$$

Here in the second line we similarity-transform all the operators involved by a gauge rotation, and in the last line we introduced a parameter  $\delta$  ( $0 < \delta < 1$  and  $\delta \rightarrow 1$ ) to indicate expansions into geometric series. The index of  $D_{(3)}^{\text{hyp}}$  is related to the 4D Dirac index in the same way. The final result is

$$\begin{aligned}
\text{Ind}(D_{(3)}^{\text{vec}}) &= -\frac{1}{2}(u+u^{-1}) \sum_{\alpha \in \Delta_+} (e^{\alpha \cdot \hat{a}_{\text{E}t}} + e^{-\alpha \cdot \hat{a}_{\text{E}t}}) \frac{u^{|\alpha \cdot B|} - u^{-|\alpha \cdot B|}}{u - u^{-1}}, \\
\text{Ind}(D_{(3)}^{\text{hyp}}) &= \frac{1}{2} \sum_{\rho \in R} (e^{\rho \cdot \hat{a}_{\text{E}t} - \hat{m}t} + e^{-\rho \cdot \hat{a}_{\text{E}t} + \hat{m}t}) \frac{u^{|\rho \cdot B|} - u^{-|\rho \cdot B|}}{u - u^{-1}}. \quad (10.4.18)
\end{aligned}$$

Here we used  $u \equiv e^{it/2\ell}$ , and  $\hat{m}$  is the normalized mass parameter for the hypermultiplet. Note also that by definition of coweight  $B$  the inner products  $\alpha \cdot B$  and  $\rho \cdot B$  are always integers.

Let us now present the formula for the expectation value of a 't Hooft operator  $T_B$ . Without loss of generality we can choose the charge  $B$  to be the highest weight vector of an irreducible representation of  ${}^L G$  (Langlands dual of the gauge group). For ‘‘small’’ charge  $B$ , all the weight vectors of the corresponding representation are Weyl images of  $B$ . In such cases, the expectation value of the 't Hooft operator can be expressed by combining all the arguments reviewed above,

$$\begin{aligned}
\langle T_B \rangle &= \int [d\hat{a}_{\text{E}}] q^{\frac{1}{2}\text{Tr}(\hat{a}_{\text{N}})^2} Z_{1\text{-loop}}(\hat{a}_{\text{N}}, \hat{m})^{\frac{1}{2}} Z_{\text{inst}}(\hat{a}_{\text{N}}, \hat{m}, q) \cdot Z_{1\text{-loop}}^{(\text{eq})}(\hat{a}_{\text{E}}, \hat{m}, B) \\
&\quad \cdot \bar{q}^{\frac{1}{2}\text{Tr}(\hat{a}_{\text{S}})^2} Z_{1\text{-loop}}(\hat{a}_{\text{S}}, \hat{m})^{\frac{1}{2}} Z_{\text{inst}}(\hat{a}_{\text{S}}, \hat{m}, \bar{q}) \\
&\quad \hat{a}_{\text{N}} = \hat{a}_{\text{E}} + \frac{iB}{2}, \quad \hat{a}_{\text{S}} = \hat{a}_{\text{E}} - \frac{iB}{2}. \quad (10.4.19)
\end{aligned}$$

This can be rewritten further as a sum over Weyl images of  $B$ . As an example, consider  $SU(N)$   $\mathcal{N} = 2^*$  theory on  $S^4$  and take as  $B$  the highest weight vector for fundamental representation, namely  $B = h_1 = (\frac{N-1}{N}, -\frac{1}{N}, \dots, -\frac{1}{N})$ . Then the expectation value is expressed as a sum over weight vectors  $h_k$ ,

$$\begin{aligned}
\langle T_B \rangle &= \frac{1}{N} \sum_{k=1}^N \int d^r \hat{a} q^{\frac{1}{2}\text{Tr}(\hat{a} + \frac{i}{2}h_k)^2} Z_{1\text{-loop}}(\hat{a} + \frac{i}{2}h_k, \hat{m})^{\frac{1}{2}} Z_{\text{inst}}(\hat{a} + \frac{i}{2}h_k, \hat{m}, q) Z_{1\text{-loop}}^{(\text{eq})}(\hat{a}, \hat{m}, h_k) \\
&\quad \cdot \bar{q}^{\frac{1}{2}\text{Tr}(\hat{a} - \frac{i}{2}h_k)^2} Z_{1\text{-loop}}(\hat{a} - \frac{i}{2}h_k, \hat{m})^{\frac{1}{2}} Z_{\text{inst}}(\hat{a} - \frac{i}{2}h_k, \hat{m}, \bar{q}), \quad (10.4.20)
\end{aligned}$$

where the one-loop determinant factor from the equator is

$$Z_{1\text{-loop}}^{(\text{eq})}(\hat{a}, \hat{m}, h_k) = \prod_{j \neq k} \frac{\{\cosh \pi(\hat{a}_k - \hat{a}_j + \hat{m}) \cosh \pi(\hat{a}_k - \hat{a}_j - \hat{m})\}^{\frac{1}{2}}}{\cosh \pi(\hat{a}_k - \hat{a}_j)}. \quad (10.4.21)$$

This result was shown to agree with the expectation value of Verlinde's loop operators in  $A_{N-1}$  Toda CFT.

**Monopole screening** As in (10.4.20), the expectation value of a 't Hooft operator  $\langle T_B \rangle$  in  $S^4$  for general magnetic charge  $B$  involves the sum over weight vectors  $h$  of the highest weight representation  $B$  of the group  ${}^L G$ . The weight vector  $h$  appearing in the argument of  $Z_{1\text{-loop}}$  and  $Z_{\text{inst}}$  has an interpretation as the value of magnetic charge measured at the polar regions. Now for a "large" charge  $B$ , the corresponding representation has more weight vectors than just the Weyl images of  $B$ . Some of the weight vectors will therefore have reduced length as compared to the length of  $B$ . This is interpreted as monopole screening: smooth monopoles can surround the 't Hooft operator inserted at the equator and screen its magnetic charge, so that the magnetic charge  $h$  observed at the polar region is "smaller" than the charge  $B$  of the monopole inserted.

There should be solutions to the Bogomolny equation describing monopole screening, which are therefore labeled by  $B$  and  $h$  and form a finite dimensional moduli space. Via Kronheimer's construction, such solutions should be mapped to ASD connections on  $\mathbb{C}^2$  which are invariant under  $\psi$ -translation symmetry  $U(1)_\psi$ . Therefore, for  $U(N)$  gauge group the moduli space of monopoles is parametrized by the ADHM data

$$\left\{ B_1 (k \times k), B_2 (k \times k), I (k \times N), J (N \times k) \right\} \text{ s.t. } [B_1, B_2] + IJ = 0$$

satisfying also the condition of  $U(1)_\psi$  invariance. The number  $k$  and the action of  $U(1)_\psi$  are determined in the following way. Consider solutions to Bogomolny equation in which the charge of a singular monopole  $M$  is reduced to  $M'$  by screening effect. The charges  $M, M'$  here are regarded as  $N \times N$  diagonal matrices. Then there should be a diagonal matrix  $K$ , whose size  $k$  and elements are determined by the formula

$$\text{Tr}(x^M) = \text{Tr}(x^{M'}) + (x + x^{-1} - 2) \text{Tr}(x^K). \quad (10.4.22)$$

Then the condition of  $U(1)_\psi$  invariance is given by

$$[K, B_1] + B_1 = [K, B_2] - B_2 = KI - IM' = M'J - JK = 0. \quad (10.4.23)$$

Equivariant integral on this moduli space contributes another factor to the integrand of (10.4.19). The detail of the analysis is presented in [53] for the example of 't Hooft operators of higher spin representations of  $SU(2)$ .

### 10.4.3 Surface operators

Another important example of supersymmetric observables are surface operators, which are non-local operators supported on two-dimensional submanifolds. It will be a challenging problem to give a complete classification of surface operators for general 4D gauge theories, but a major progress have been made for BPS surface operators in  $\mathcal{N} = 2$  supersymmetric theories, as we review here.

For  $\mathcal{N} = 2$  theories of class S where M5-brane interpretation is available, a natural question is how to identify the surface operators describing other M-branes ending on or intersecting the M5-branes [51, 57]. For those surface operators, the calculations in gauge theories can be checked against the prediction from AGT correspondence. Another approach is to realize  $\mathcal{N} = 2$  SUSY theories geometrically using Calabi-Yau compactification of type IIA string, where D4-branes wrapping Lagrangian submanifolds give rise to surface operators [58]. In this setting, the results of gauge theory analysis can be compared with topological string amplitudes for which there are powerful formalisms known such as refined topological vertex.

For  $\mathcal{N} = 2$  SUSY theories on Omega-background  $\mathbb{R}_{\epsilon_1, \epsilon_2}^4$  with coordinates  $z_1 = x_1 + ix_2, z_2 = x_3 + ix_4$ , one can introduce surface operators along the surfaces  $z_2 = 0$  or  $z_1 = 0$  without braking supersymmetry. For theories on the ellipsoid (10.2.28), one can introduce BPS surface operators along the  $S^2$  defined by  $x_3 = x_4 = 0$  or  $x_1 = x_2 = 0$ .

**Coupled 2D-4D systems** One way to describe surface operators is in terms of 2D quantum field theories on its worldvolume. For 4D  $\mathcal{N} = 2$  theories realized on  $S_b^4$ , the objects of interest are the half-BPS surface operators which support  $\mathcal{N} = (2, 2)$  field theories on a squashed  $S^2$ . The supersymmetry for the coupled 2D-4D system is such that the  $S_b^4$  and  $S^2$  have the north and south poles in common, that is where the instantons of 4D gauge theory and vortices of 2D theory get localized.

If the 4D theory has a Lagrangian description, one can simplify the problem by turning off the 4D gauge coupling. The system is then reduced to a 2D interacting theory and 4D free matter theory both coupled to some frozen 4D vector multiplets. One can still learn a great deal about surface operators from this simplified system [64]. The partition function is then a product of the 4D free hypermultiplet path integral,  $Z_{1\text{-loop}}^{\text{hyp}}$  of (10.3.30), and the  $S^2$  partition function [17, 18] of the 2D theory. The classical value of the frozen 4D vector multiplet enters the formula as the common mass for 2D and 4D fields.

As an example, take a system of  $N^2$  free hypermultiplets. One can regard it as a bifundamental of the group  $S[U(N) \times U(N)]$  and turn on the masses  $(m_1, \dots, m_N; \tilde{m}_1, \dots, \tilde{m}_N)$ . The  $S_b^4$  partition function is then

$$\prod_{i,j=1}^N \Upsilon\left(\frac{Q}{2} + i(m_i - \tilde{m}_j)\right)^{-1}. \quad (10.4.24)$$

This simple theory is known to correspond to  $N$  M5-branes wrapped on a sphere with three (one *simple* and two *full*) punctures. AGT relation identifies (10.4.24) with the corresponding three-point function in Toda conformal field theory. Now introduce a  $\mathcal{N} = (2, 2)$  theory

with the same global symmetry  $S[U(N) \times U(N)]$  on the surface operator. The simplest class of examples is a 2D  $U(K)$  gauge theory with  $N$  fundamental and  $N$  anti-fundamental chiral multiplets. A systematic study and detailed comparison with Toda CFT correlators were made in [64]. It was shown that, if a suitable mass is turned on for the 2D theory, which is related to  $(m_i; \tilde{m}_i)$  by a suitable rescaling and imaginary shift, then the 2D-4D combined partition function reproduces the Toda four-point functions with various degenerate insertions [51].

**Singularity along a surface** Another way to define surface operators is to require that the gauge field and possibly other fields develop singularities along the surface. As an example, take an  $SU(N)$  gauge theory on  $\mathbb{C}^2$  with coordinate  $z_1 = x_1 + ix_2$  and  $z_2 = x_3 + ix_4$ . One can then introduce a surface operator along  $z_2 = 0$  by imposing the singular boundary condition

$$A \simeq A_\chi \cdot d\chi \left( \chi \equiv \arg(z_2), A_\chi \equiv \text{diag}(\underbrace{\nu_1, \dots, \nu_1}_{n_1 \text{ times}}, \underbrace{\nu_2, \dots, \nu_2}_{n_2 \text{ times}}, \dots, \underbrace{\nu_s, \dots, \nu_s}_{n_s \text{ times}}) \right). \quad (10.4.25)$$

This breaks the gauge symmetry  $SU(N)$  to a Levi subgroup

$$\mathbb{L} = S[U(n_1) \times \dots \times U(n_s)], \quad \sum_{i=1}^s n_i = N \quad (10.4.26)$$

on the surface. The parameters  $\nu_i$  satisfy  $\nu_1 > \dots > \nu_s > \nu_1 - 1$ , which in turn set the order of  $n_i$  appearing in the partition of  $N$ . For half-BPS surface operators in  $\mathcal{N} = 2$  supersymmetric theories, one needs to turn on the auxiliary field  $D_{AB}$  to ensure the SUSY variation of gaugino to vanish. For a suitable choice of unbroken supersymmetry one finds

$$D_{11} = D_{22} = 0, \quad D_{12} = iF_{12} = 2\pi i A_\chi \cdot \delta(x_3)\delta(x_4). \quad (10.4.27)$$

We have seen two different descriptions of surface operators, but there are some surface operators described in both ways. For example, the surface operators of type (10.4.25) in pure  $\mathcal{N} = 2$  SYM theory can also be described by a 2D  $\mathcal{N} = (2, 2)$  supersymmetric quiver gauge theory which flows to a sigma model on a flag manifold  $SU(N)/\mathbb{L}$ . Here the ordering of  $n_i$  makes a subtle effect: different orderings leads to different ultraviolet gauge theory descriptions, which flow to a non-linear sigma model on the same flag manifold but with different complex structures [63].

**Localization computation** Let us consider the surface operator of the type (10.4.25) introduced along the  $S^2$  inside the ellipsoid (10.2.28) defined by  $x_3 = x_4 = 0$ . In terms of the polar coordinates  $(\rho, \theta, \varphi, \chi)$  the surface operator is at  $\theta = 0$ . The singular behavior of the gauge field is then expressed as follows,

$$A = A_\chi \cdot d\chi. \quad (\text{near } \theta = 0) \quad (10.4.28)$$

At supersymmetric saddle points the gauge field takes precisely this form. The value of classical action at the saddle points labeled by  $\phi = \bar{\phi} = -ia_0/2$  is

$$S_{\text{YM}} = \frac{8\pi^2}{g^2} \text{Tr} \left( \ell \tilde{\ell} a_0^2 - 2i\ell a_0 A_\chi \right), \quad S_{\text{FI}} = -16i\pi^2 \zeta \left( \ell \tilde{\ell} a_0 - iA_\chi \ell \right), \quad S_{\text{mat}} = 0. \quad (10.4.29)$$

The saddle points can also have point-like instantons or anti-instantons localized at the north or south poles. Due to the presence of surface operator, the topology of gauge field configuration near the north pole is characterized by instanton number  $k$  as well as magnetic flux  $m_i$  defined by

$$\frac{1}{2\pi} \int_{\text{surface op}} \text{Tr}(A_\chi \cdot F) = \sum_{i=1}^s \nu_i m_i. \quad \left( \sum_{i=1}^s m_i = 0 \right) \quad (10.4.30)$$

Such topologically non-trivial gauge field configurations are called ramified instantons. The saddle points with point-like ramified instantons labeled by  $k, m_i$  are thus weighted by a factor  $q^{k-\nu_i m_i}$  in the path integral. Similarly, anti-instantons localized at the south pole are labeled by  $\tilde{k}, \tilde{m}_i$  and make contributions proportional to  $\tilde{q}^{k-\nu_i \tilde{m}_i}$ . Those contributions are organized into a generalization of Nekrasov's instanton partition function.

Nekrasov's partition function for ramified instantons is a generating function of equivariant integrals over the moduli spaces  $\mathcal{M}_{k, \tilde{m}; \tilde{n}}^{\text{ram}}$ . In mathematics literature these spaces are called Affine Laumon space. The equivariant parameters are  $\epsilon_1 = \ell^{-1}$ ,  $\epsilon_2 = \tilde{\ell}^{-1}$  and the constant value of the field  $\hat{\Phi}$  at saddle points

$$\hat{\Phi} = a_0 - \frac{iA_\chi}{\tilde{\ell}}. \quad (10.4.31)$$

Actually, this space  $\mathcal{M}_{k, \tilde{m}; \tilde{n}}^{\text{ram}}$  is known to be mathematically equivalent to another space which should be more familiar to physicists, that is the moduli space of  $U(N)$  instantons in orbifold  $\mathbb{C} \times (\mathbb{C}/\mathbb{Z}_s)$  [82]. Here the  $\mathbb{Z}_s$  is understood to act on fields through spacetime rotation as well as gauge transformation: it acts on the fundamental representation of  $U(N)$  as the multiplication by the diagonal matrix

$$\Omega_{\tilde{n}} \equiv \text{diag} \left( \underbrace{\omega, \dots, \omega}_{n_1}, \dots, \underbrace{\omega^s, \dots, \omega^s}_{n_s} \right); \quad \omega \equiv e^{\frac{2\pi i}{s}}. \quad (10.4.32)$$

Each instanton is assigned a  $\mathbb{Z}_s$  charge, and the moduli space is denoted as  $\mathcal{M}_{k; \tilde{n}}^{\text{orb}}$  with  $k_i$  the number of instantons with  $\mathbb{Z}_s$  charge  $i$  (we work with the convention  $k_i = k_{s+i}$ ). The two moduli spaces are related as follows,

$$\mathcal{M}_{k, \tilde{m}; \tilde{n}}^{\text{ram}} = \mathcal{M}_{\tilde{k}; \tilde{n}}^{\text{orb}} \quad \text{if} \quad k_s = k, \quad k_{i+1} = k_i + m_i. \quad (10.4.33)$$

For more explanation, see [63] and references therein.

The moduli space  $\mathcal{M}_{k; \tilde{n}}^{\text{orb}}$  can be parametrized by ADHM matrices. Let us denote  $K \equiv \sum_{i=1}^s k_i$ , then the set of matrices

$$\left\{ B_1(K \times K), B_2(K \times K), I(K \times N), J(N \times K) \right\} \quad \text{s.t.} \quad [B_1, B_2] + IJ = 0, \quad (10.4.34)$$

subject to the  $\otimes_i GL(k_i)$  equivalence and the  $\mathbb{Z}_s$  orbifold projection,

$$\begin{aligned}
\Omega_{\vec{k}} B_1 \Omega_{\vec{k}}^{-1} &= B_1, \\
\Omega_{\vec{k}} B_2 \Omega_{\vec{k}}^{-1} &= \omega B_2, \\
\Omega_{\vec{k}} I \Omega_{\vec{n}}^{-1} &= I, \\
\Omega_{\vec{n}} J \Omega_{\vec{k}}^{-1} &= \omega J.
\end{aligned}
\tag{10.4.35}$$

gives a parametrization of the moduli space  $\mathcal{M}_{k;\vec{n}}^{\text{orb}}$ . Here  $\Omega_{\vec{k}}$  is a diagonal matrix defined similarly to (10.4.32), with eigenvalue  $\omega^i$  appearing  $k_i$  times. The chain-saw quiver describes the components of ADHM matrices which survive the orbifold projection.

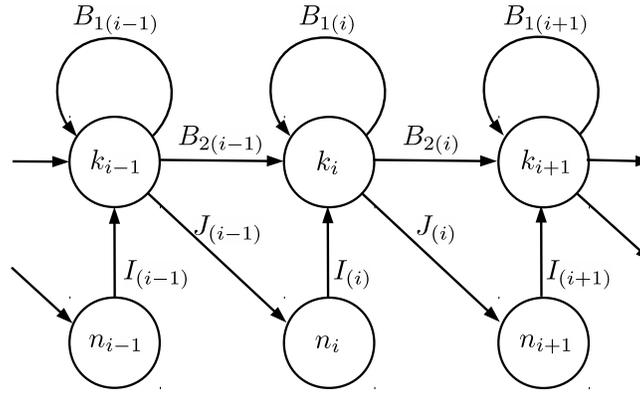

Ramified instanton partition functions and their correspondence with conformal blocks for general  $W_N$  algebra were studied in [57, 59–63].

The correspondence between ramified instantons and instantons in orbifolds will be a key to fully understand how to define and compute observables in the surface defect backgrounds. This was used in [65] for surface operators in  $\mathcal{N} = 2$  pure SYM and  $\mathcal{N} = 2^*$  SYM theories on  $S^4$ , and should be extended to more general cases. The exact formulae for observables obtained this way will also help clarifying how various descriptions of surface operators are related with each other.

## Acknowledgments

The author thanks Naofumi Hama for collaboration on the topics discussed in this review. He also thanks Heng-Yu Chen and Hee-Cheol Kim for useful discussions.

## References

- [1] V. Pestun and M. Zabzine, eds., *Localization techniques in quantum field theory*, vol. xx. Journal of Physics A, 2016. 1608.02952. <https://arxiv.org/src/1608.02952/anc/LocQFT.pdf>, <http://pestun.ihes.fr/pages/LocalizationReview/LocQFT.pdf>.

- [2] N. Seiberg and E. Witten, “Electric - magnetic duality, monopole condensation, and confinement in  $\mathcal{N} = 2$  supersymmetric Yang-Mills theory,” *Nucl. Phys.* **B426** (1994) 19–52, [arXiv:hep-th/9407087 \[hep-th\]](#). [Erratum: Nucl. Phys.B430,485(1994)].
- [3] N. Seiberg and E. Witten, “Monopoles, duality and chiral symmetry breaking in  $\mathcal{N} = 2$  supersymmetric QCD,” *Nucl. Phys.* **B431** (1994) 484–550, [arXiv:hep-th/9408099 \[hep-th\]](#).
- [4] E. Witten, “Topological Quantum Field Theory,” *Commun. Math. Phys.* **117** (1988) 353.
- [5] N. A. Nekrasov, “Seiberg-Witten prepotential from instanton counting,” *Adv. Theor. Math. Phys.* **7** (2003) no. 5, 831–864, [arXiv:hep-th/0206161 \[hep-th\]](#).
- [6] A. Losev, N. Nekrasov, and S. L. Shatashvili, “Issues in topological gauge theory,” *Nucl. Phys.* **B534** (1998) 549–611, [arXiv:hep-th/9711108 \[hep-th\]](#).
- [7] G. W. Moore, N. Nekrasov, and S. Shatashvili, “Integrating over Higgs branches,” *Commun. Math. Phys.* **209** (2000) 97–121, [arXiv:hep-th/9712241 \[hep-th\]](#).
- [8] A. Losev, N. Nekrasov, and S. L. Shatashvili, “Testing Seiberg-Witten solution,” in *Strings, branes and dualities. Proceedings, NATO Advanced Study Institute, Cargese, France, May 26-June 14, 1997*. 1997. [arXiv:hep-th/9801061 \[hep-th\]](#).
- [9] V. Pestun, “Localization of gauge theory on a four-sphere and supersymmetric Wilson loops,” *Commun. Math. Phys.* **313** (2012) 71–129, [arXiv:0712.2824 \[hep-th\]](#).
- [10] J. K. Erickson, G. W. Semenoff, and K. Zarembo, “Wilson loops in  $\mathcal{N} = 4$  supersymmetric Yang-Mills theory,” *Nucl. Phys.* **B582** (2000) 155–175, [arXiv:hep-th/0003055 \[hep-th\]](#).
- [11] N. Drukker and D. J. Gross, “An Exact prediction of  $\mathcal{N} = 4$  SUSYM theory for string theory,” *J. Math. Phys.* **42** (2001) 2896–2914, [arXiv:hep-th/0010274 \[hep-th\]](#).
- [12] T. Okuda and V. Pestun, “On the instantons and the hypermultiplet mass of  $\mathcal{N} = 2^*$  super Yang-Mills on  $S^4$ ,” *JHEP* **03** (2012) 017, [arXiv:1004.1222 \[hep-th\]](#).
- [13] K. Zarembo, “Localization and AdS/CFT Correspondence,” *Journal of Physics A* **xx** (2016) 000, [1608.02963](#).
- [14] A. Kapustin, B. Willett, and I. Yaakov, “Exact Results for Wilson Loops in Superconformal Chern-Simons Theories with Matter,” *JHEP* **03** (2010) 089, [arXiv:0909.4559 \[hep-th\]](#).
- [15] D. L. Jafferis, “The Exact Superconformal R-Symmetry Extremizes  $Z$ ,” *JHEP* **05** (2012) 159, [arXiv:1012.3210 \[hep-th\]](#).
- [16] N. Hama, K. Hosomichi, and S. Lee, “Notes on SUSY Gauge Theories on Three-Sphere,” *JHEP* **03** (2011) 127, [arXiv:1012.3512 \[hep-th\]](#).
- [17] F. Benini and S. Cremonesi, “Partition Functions of  $\mathcal{N} = (2, 2)$  Gauge Theories on  $S^2$  and Vortices,” *Commun. Math. Phys.* **334** (2015) no. 3, 1483–1527, [arXiv:1206.2356 \[hep-th\]](#).
- [18] N. Doroud, J. Gomis, B. Le Floch, and S. Lee, “Exact Results in  $D = 2$  Supersymmetric Gauge Theories,” *JHEP* **05** (2013) 093, [arXiv:1206.2606 \[hep-th\]](#).
- [19] J. Källén, J. Qiu, and M. Zabzine, “The perturbative partition function of supersymmetric 5D Yang-Mills theory with matter on the five-sphere,” *JHEP* **08** (2012) 157, [arXiv:1206.6008 \[hep-th\]](#).
- [20] H.-C. Kim and S. Kim, “M5-branes from gauge theories on the 5-sphere,” *JHEP* **05** (2013) 144, [arXiv:1206.6339 \[hep-th\]](#).
- [21] H.-C. Kim, J. Kim, and S. Kim, “Instantons on the 5-sphere and M5-branes,” [arXiv:1211.0144 \[hep-th\]](#).

- [22] E. Gerchkovitz, J. Gomis, and Z. Komargodski, “Sphere Partition Functions and the Zamolodchikov Metric,” *JHEP* **11** (2014) 001, [arXiv:1405.7271 \[hep-th\]](#).
- [23] J. Gomis and N. Ishtiaque, “Kähler potential and ambiguities in 4d  $\mathcal{N} = 2$  SCFTs,” *JHEP* **04** (2015) 169, [arXiv:1409.5325 \[hep-th\]](#). [JHEP04,169(2015)].
- [24] D. Gaiotto, “ $\mathcal{N} = 2$  dualities,” *JHEP* **08** (2012) 034, [arXiv:0904.2715 \[hep-th\]](#).
- [25] L. F. Alday, D. Gaiotto, and Y. Tachikawa, “Liouville Correlation Functions from Four-dimensional Gauge Theories,” *Lett. Math. Phys.* **91** (2010) 167–197, [arXiv:0906.3219 \[hep-th\]](#).
- [26] Y. Tachikawa, “A brief review of the 2d/4d correspondences,” *Journal of Physics A* **xx** (2016) 000, [1608.02964](#).
- [27] N. Wyllard, “ $A_{N-1}$  conformal Toda field theory correlation functions from conformal  $\mathcal{N} = 2$   $SU(N)$  quiver gauge theories,” *JHEP* **11** (2009) 002, [arXiv:0907.2189 \[hep-th\]](#).
- [28] N. Hama, K. Hosomichi, and S. Lee, “SUSY Gauge Theories on Squashed Three-Spheres,” *JHEP* **05** (2011) 014, [arXiv:1102.4716 \[hep-th\]](#).
- [29] Y. Imamura and D. Yokoyama, “ $\mathcal{N} = 2$  supersymmetric theories on squashed three-sphere,” *Phys. Rev.* **D85** (2012) 025015, [arXiv:1109.4734 \[hep-th\]](#).
- [30] G. Festuccia and N. Seiberg, “Rigid Supersymmetric Theories in Curved Superspace,” *JHEP* **06** (2011) 114, [arXiv:1105.0689 \[hep-th\]](#).
- [31] T. Dumitrescu, “An Introduction to Supersymmetric Field Theories in Curved Space,” *Journal of Physics A* **xx** (2016) 000, [1608.02957](#).
- [32] N. Hama and K. Hosomichi, “Seiberg-Witten Theories on Ellipsoids,” *JHEP* **09** (2012) 033, [arXiv:1206.6359 \[hep-th\]](#). [Addendum: JHEP10,051(2012)].
- [33] H. Samtleben and D. Tsimpis, “Rigid supersymmetric theories in 4d Riemannian space,” *JHEP* **05** (2012) 132, [arXiv:1203.3420 \[hep-th\]](#).
- [34] T. T. Dumitrescu, G. Festuccia, and N. Seiberg, “Exploring Curved Superspace,” *JHEP* **08** (2012) 141, [arXiv:1205.1115 \[hep-th\]](#).
- [35] D. Cassani, C. Klare, D. Martelli, A. Tomasiello, and A. Zaffaroni, “Supersymmetry in Lorentzian Curved Spaces and Holography,” *Commun. Math. Phys.* **327** (2014) 577–602, [arXiv:1207.2181 \[hep-th\]](#).
- [36] J. T. Liu, L. A. Pando Zayas, and D. Reichmann, “Rigid Supersymmetric Backgrounds of Minimal Off-Shell Supergravity,” *JHEP* **10** (2012) 034, [arXiv:1207.2785 \[hep-th\]](#).
- [37] T. T. Dumitrescu and G. Festuccia, “Exploring Curved Superspace (II),” *JHEP* **01** (2013) 072, [arXiv:1209.5408 \[hep-th\]](#).
- [38] C. Klare and A. Zaffaroni, “Extended Supersymmetry on Curved Spaces,” *JHEP* **10** (2013) 218, [arXiv:1308.1102 \[hep-th\]](#).
- [39] T. Nosaka and S. Terashima, “Supersymmetric Gauge Theories on a Squashed Four-Sphere,” *JHEP* **12** (2013) 001, [arXiv:1310.5939 \[hep-th\]](#).
- [40] A. Cabo-Bizet, E. Gava, V. I. Giraldo-Rivera, M. N. Muteeb, and K. S. Narain, “Partition Function of  $\mathcal{N} = 2$  Gauge Theories on a Squashed  $S^4$  with  $SU(2) \times U(1)$  Isometry,” *Nucl. Phys.* **B899** (2015) 149–164, [arXiv:1412.6826 \[hep-th\]](#).
- [41] A. Bawane, G. Bonelli, M. Ronzani, and A. Tanzini, “ $\mathcal{N} = 2$  supersymmetric gauge theories on  $S^2 \times S^2$  and Liouville Gravity,” *JHEP* **07** (2015) 054, [arXiv:1411.2762 \[hep-th\]](#).
- [42] M. Sinamuli, “On  $\mathcal{N} = 2$  supersymmetric gauge theories on  $S^2 \times S^2$ ,” [arXiv:1411.4918 \[hep-th\]](#).

- [43] S. Murthy and V. Reys, “Functional determinants, index theorems, and exact quantum black hole entropy,” *JHEP* **12** (2015) 028, [arXiv:1504.01400 \[hep-th\]](#).
- [44] R. K. Gupta, Y. Ito, and I. Jeon, “Supersymmetric Localization for BPS Black Hole Entropy: 1-loop Partition Function from Vector Multiplets,” *JHEP* **11** (2015) 197, [arXiv:1504.01700 \[hep-th\]](#).
- [45] D. Butter, G. Inverso, and I. Lodato, “Rigid 4D  $\mathcal{N} = 2$  supersymmetric backgrounds and actions,” *JHEP* **09** (2015) 088, [arXiv:1505.03500 \[hep-th\]](#).
- [46] T. Nishioka and I. Yaakov, “Supersymmetric Rényi Entropy,” *JHEP* **10** (2013) 155, [arXiv:1306.2958 \[hep-th\]](#).
- [47] X. Huang and Y. Zhou, “ $\mathcal{N} = 4$  Super-Yang-Mills on conic space as hologram of STU topological black hole,” *JHEP* **02** (2015) 068, [arXiv:1408.3393 \[hep-th\]](#).
- [48] M. Crossley, E. Dyer, and J. Sonner, “Super-Rényi entropy & Wilson loops for  $\mathcal{N} = 4$  SYM and their gravity duals,” *JHEP* **12** (2014) 001, [arXiv:1409.0542 \[hep-th\]](#).
- [49] N. Hama, T. Nishioka, and T. Ugajin, “Supersymmetric Rényi entropy in five dimensions,” *JHEP* **12** (2014) 048, [arXiv:1410.2206 \[hep-th\]](#).
- [50] Y. Zhou, “Universal Features of Four-Dimensional Superconformal Field Theory on Conic Space,” *JHEP* **08** (2015) 052, [arXiv:1506.06512 \[hep-th\]](#).
- [51] L. F. Alday, D. Gaiotto, S. Gukov, Y. Tachikawa, and H. Verlinde, “Loop and surface operators in  $\mathcal{N} = 2$  gauge theory and Liouville modular geometry,” *JHEP* **01** (2010) 113, [arXiv:0909.0945 \[hep-th\]](#).
- [52] N. Drukker, J. Gomis, T. Okuda, and J. Teschner, “Gauge Theory Loop Operators and Liouville Theory,” *JHEP* **02** (2010) 057, [arXiv:0909.1105 \[hep-th\]](#).
- [53] J. Gomis, T. Okuda, and V. Pestun, “Exact Results for ’t Hooft Loops in Gauge Theories on  $S^4$ ,” *JHEP* **05** (2012) 141, [arXiv:1105.2568 \[hep-th\]](#).
- [54] F. Fucito, J. F. Morales, and R. Poghossian, “Wilson loops and chiral correlators on squashed spheres,” *JHEP* **11** (2015) 064, [arXiv:1507.05426 \[hep-th\]](#).
- [55] S. Gukov, “Surface Operators,” in *New Dualities of Supersymmetric Gauge Theories*, J. Teschner, ed., pp. 223–259. Springer International Publishing, 2016. [arXiv:1412.7127 \[hep-th\]](#).
- [56] S. Gukov and E. Witten, “Gauge Theory, Ramification, And The Geometric Langlands Program,” [arXiv:hep-th/0612073 \[hep-th\]](#).
- [57] L. F. Alday and Y. Tachikawa, “Affine  $SL(2)$  conformal blocks from 4d gauge theories,” *Lett. Math. Phys.* **94** (2010) 87–114, [arXiv:1005.4469 \[hep-th\]](#).
- [58] T. Dimofte, S. Gukov, and L. Hollands, “Vortex Counting and Lagrangian 3-manifolds,” *Lett. Math. Phys.* **98** (2011) 225–287, [arXiv:1006.0977 \[hep-th\]](#).
- [59] H. Awata, H. Fuji, H. Kanno, M. Manabe, and Y. Yamada, “Localization with a Surface Operator, Irregular Conformal Blocks and Open Topological String,” *Adv. Theor. Math. Phys.* **16** (2012) no. 3, 725–804, [arXiv:1008.0574 \[hep-th\]](#).
- [60] C. Kozcaz, S. Pasquetti, F. Passerini, and N. Wyllard, “Affine  $sl(N)$  conformal blocks from  $\mathcal{N} = 2$   $SU(N)$  gauge theories,” *JHEP* **01** (2011) 045, [arXiv:1008.1412 \[hep-th\]](#).
- [61] N. Wyllard, “W-algebras and surface operators in  $\mathcal{N} = 2$  gauge theories,” *J. Phys.* **A44** (2011) 155401, [arXiv:1011.0289 \[hep-th\]](#).
- [62] N. Wyllard, “Instanton partition functions in  $\mathcal{N} = 2$   $SU(N)$  gauge theories with a general surface operator, and their W-algebra duals,” *JHEP* **02** (2011) 114, [arXiv:1012.1355 \[hep-th\]](#).

- [63] H. Kanno and Y. Tachikawa, “Instanton counting with a surface operator and the chain-saw quiver,” *JHEP* **06** (2011) 119, [arXiv:1105.0357 \[hep-th\]](#).
- [64] J. Gomis and B. Le Floch, “M2-brane surface operators and gauge theory dualities in Toda,” [arXiv:1407.1852 \[hep-th\]](#).
- [65] S. Nawata, “Givental  $J$ -functions, Quantum integrable systems, AGT relation with surface operator,” [arXiv:1408.4132 \[hep-th\]](#).
- [66] J. Wess and J. Bagger, *Supersymmetry and supergravity*. Princeton Univ. Pr., 1992.
- [67] B. de Wit, J. W. van Holten, and A. Van Proeyen, “Transformation Rules of  $\mathcal{N} = 2$  Supergravity Multiplets,” *Nucl. Phys.* **B167** (1980) 186.
- [68] B. de Wit, J. W. van Holten, and A. Van Proeyen, “Structure of  $\mathcal{N} = 2$  Supergravity,” *Nucl. Phys.* **B184** (1981) 77. [Erratum: *Nucl. Phys.*B222,516(1983)].
- [69] B. de Wit, P. G. Lauwers, R. Philippe, and A. Van Proeyen, “Noncompact  $\mathcal{N} = 2$  Supergravity,” *Phys. Lett.* **B135** (1984) 295.
- [70] B. de Wit, P. G. Lauwers, and A. Van Proeyen, “Lagrangians of  $\mathcal{N} = 2$  Supergravity - Matter Systems,” *Nucl. Phys.* **B255** (1985) 569.
- [71] T. Mohaupt, “Black hole entropy, special geometry and strings,” *Fortsch. Phys.* **49** (2001) 3–161, [arXiv:hep-th/0007195 \[hep-th\]](#).
- [72] D. Z. Freedman and A. Van Proeyen, *Supergravity*. Cambridge Univ. Press, Cambridge, UK, 2012.
- [73] N. Berkovits, “A Ten-dimensional superYang-Mills action with off-shell supersymmetry,” *Phys. Lett.* **B318** (1993) 104–106, [arXiv:hep-th/9308128 \[hep-th\]](#).
- [74] V. Pestun, “Localization for  $\mathcal{N} = 2$  Supersymmetric Gauge Theories in Four Dimensions,” in *New Dualities of Supersymmetric Gauge Theories*, J. Teschner, ed., pp. 159–194. Springer International Publishing, 2016. [arXiv:1412.7134 \[hep-th\]](#).
- [75] E. Witten, “Supersymmetry and Morse theory,” *J. Diff. Geom.* **17** (1982) no. 4, 661–692.
- [76] E. Witten, “Holomorphic Morse inequalities,” in *Algebraic and differential topology, global differential geometry*, G. M. Rassias, ed., Teubner-Texte zur Mathematik, pp. 318–333. Teubner, 1984.
- [77] M. F. Atiyah, *Elliptic operators and compact groups*. Springer-Verlag Berlin, 1974.
- [78] A. B. Zamolodchikov and A. B. Zamolodchikov, “Structure constants and conformal bootstrap in Liouville field theory,” *Nucl. Phys.* **B477** (1996) 577–605, [arXiv:hep-th/9506136 \[hep-th\]](#).
- [79] G. ’t Hooft, “On the Phase Transition Towards Permanent Quark Confinement,” *Nucl. Phys.* **B138** (1978) 1–25.
- [80] E. Witten, “Dyons of Charge  $e\theta/2\pi$ ,” *Phys. Lett.* **B86** (1979) 283–287.
- [81] P. Kronheimer, “Monopoles and Taub-NUT metrics,” *MSc. Thesis (Oxford University)* (1986) .
- [82] I. Biswas, “Parabolic bundles as orbifold bundles,” *Duke Math. J.* **88** (1997) 305–325.

# Chapter 11

## Localization and AdS/CFT Correspondence

Konstantin Zarembo

*Nordita, KTH Royal Institute of Technology and Stockholm University, Roslagstullsbacken 23,  
SE-106 91 Stockholm, Sweden*

*Department of Physics and Astronomy, Uppsala University, SE-751 08 Uppsala, Sweden  
zaremb@nordita.org*

### Abstract

An interplay between localization and holography is reviewed with the emphasis on the  $AdS_5/CFT_4$  correspondence.

### Contents

|                                                                  |            |
|------------------------------------------------------------------|------------|
| <b>11.1 Introduction</b>                                         | <b>431</b> |
| <b>11.2 <math>\mathcal{N} = 4</math> Super-Yang-Mills theory</b> | <b>432</b> |
| <b>11.3 Circular Wilson loop</b>                                 | <b>433</b> |
| <b>11.4 Higher representations and D-branes</b>                  | <b>440</b> |
| <b>11.5 Wavy lines, cusp and latitude</b>                        | <b>449</b> |
| <b>11.6 Operator Product Expansion</b>                           | <b>457</b> |
| <b>11.7 Massive theory</b>                                       | <b>464</b> |
| <b>11.8 Conclusions</b>                                          | <b>468</b> |
| <b>References</b>                                                | <b>469</b> |

## 11.1 Introduction

The holographic duality [2–4] can be understood as a precise string reformulation of the large- $N$  expansion [5]. Which gauge theories (perhaps all?) have exact holographic duals is

an interesting open problem. So far the classical gravity approximation has been the most useful holographic setup. This approximation is restricted to the regime of a very large 't Hooft coupling and is obviously difficult to access by ordinary methods of quantum field theory. Any exact result that can be reliably extended to strong coupling and consequently confronted with the predictions of holography is very valuable in this respect. A number of such results can be obtained with the help of supersymmetric localization [6]. Localization is thus instrumental in connecting holography with down-to-earth quantum field theory calculations, and opens a window onto genuine non-perturbative dynamics of gauge fields.

The aim of these notes is to review the large- $N$  expansion of localization formulas, with the aim to connect them to string theory and holographic duality. The review almost exclusively deals with the maximally supersymmetric  $\mathcal{N} = 4$  super-Yang-Mills (SYM) theory in four dimensions, apart from a rather cryptic discussion of its less supersymmetric non-conformal cousins. According to the AdS/CFT correspondence,  $\mathcal{N} = 4$  SYM is equivalent to string theory on  $AdS_5 \times S^5$  [2]. The AdS/CFT correspondence is the first and best studied model of holographic duality. While holographic uses of localization are not restricted to this setup, other cases are extensively covered elsewhere. Localization in three dimensions and its applications to the  $AdS_4/CFT_3$  duality are covered in [7] and in Chapter 7. Massive theories in four dimensions are treated in more detail in [8]. An overview of early developments in  $\mathcal{N} = 4$  SYM, with applications to the  $AdS_5/CFT_4$  correspondence, can be found in [9].

## 11.2 $\mathcal{N} = 4$ Super-Yang-Mills theory

The field content of the  $\mathcal{N} = 4$  SYM [10, 11] consists of the gauge potentials  $A_\mu$ , six scalars  $\Phi_I$  and four Majorana fermions  $\Psi_{\alpha A}$ , all in the adjoint representation of the gauge group. The scalars and fermions transform in the **6** and **4** (vector and spinor) representations of the  $SO(6)$  R-symmetry group. The Lagrangian of  $\mathcal{N} = 4$  SYM can be obtained by dimensionally reducing  $D = 10$ ,  $\mathcal{N} = 1$  Yang-Mills theory to four dimensions [10, 11]. The ten-dimensional origin of the theory is reflected in its field content: the bosons ( $A_\mu, \Phi_I$ ) combine into the ten-dimensional vector potential and  $\Psi_{\alpha A}$  are components of a single ten-dimensional Majorana-Weyl spinor. The action takes a rather concise form in the 10d notations, which is very useful for practical purposes:

$$S = \frac{1}{g_{\text{YM}}} \int d^4x \operatorname{tr} \left[ -\frac{1}{2} F_{\mu\nu}^2 + (D_\mu \Phi_I)^2 + \frac{1}{2} [\Phi_I, \Phi_J]^2 + i \bar{\Psi} \gamma^\mu D_\mu \Psi + \bar{\Psi} \gamma^I [\Phi_I, \Psi] \right], \quad (11.2.1)$$

The Dirac matrices  $\gamma^M = (\gamma^\mu, \gamma^I)$  form the ten-dimensional Clifford algebra, the fermions satisfy  $\gamma^{11} \Psi = \Psi$  and  $\bar{\Psi} = \Psi^t C$ , where  $\Gamma^{11}$  and  $C$  are the ten-dimensional chirality and charge-conjugation matrices, respectively. One can choose  $\gamma^I = \gamma^5 \Gamma^I$ , where  $\Gamma^I$  are the six-dimensional Dirac matrices, and assume that  $\gamma^\mu$  only act on the 4d spinor indices  $\alpha$  and  $\Gamma^I$  only act the R-symmetry indices  $A$ .

The  $\mathcal{N} = 4$  supersymmetry is the largest possible in non-gravitational theories in four dimensions and is powerful enough to protect the coupling constant  $g_{\text{YM}}$  from renormalization. The coupling therefore does not run with the energy scale and as a consequence the classical conformal invariance of the SYM action is not broken by quantum corrections. The  $\mathcal{N} = 4$  SYM therefore constitutes a continuous family of conformal field theories parameterized by the gauge coupling  $g_{\text{YM}}$ , the theta angle (which we have so far set to zero), and the gauge group, here taken to be  $U(N)$ .

The AdS/CFT duality relates  $\mathcal{N} = 4$  SYM to type IIB superstring theory on  $AdS_5 \times S^5$  [2–4]. The duality is naturally formulated within the large- $N$  expansion and is especially simple in the large- $N$  limit, in which the 't Hooft coupling

$$\lambda = g_{\text{YM}}^2 N \tag{11.2.2}$$

is kept fixed while  $N \rightarrow \infty$ . The string coupling and the dimensionless string tension are related to the parameters of the SYM theory as [2]

$$g_s = \frac{\lambda}{4\pi N} \quad T \equiv \frac{R_{\text{AdS}}^2}{2\pi\alpha'} = \frac{\sqrt{\lambda}}{2\pi}. \tag{11.2.3}$$

The planar (infinite- $N$ ) limit of the gauge theory thus maps to the non-interacting string theory, which is still a fairly complicated quantum-mechanical system. The string tension  $T$  is defined as the coupling multiplying the string action. The radius of AdS  $R_{\text{AdS}}$  and the string length  $\sqrt{\alpha'}$  can only appear in this combination, and never alone, because any dimensionful parameter is forbidden by scale invariance.

The AdS metric, written in the units where the AdS radius  $R_{\text{AdS}}$  is set to one, is given by

$$ds^2 = \frac{dx_\mu^2 + dz^2}{z^2}. \tag{11.2.4}$$

The holographic radial coordinate  $z$  ranges from zero to infinity. The gauge-theory observables are located at the boundary of AdS at  $z = 0$ . There is a precise map between correlation functions in the SYM theory and string amplitudes in  $AdS_5 \times S^5$  (with sources at the boundary). Moreover, when  $\lambda \gg 1$  the radius of AdS is large in the string units and the string amplitudes can be approximated by gravitational perturbations classically propagating on the AdS background [4]. The holographic duality is oftentimes identified with this simplified setup.

### 11.3 Circular Wilson loop

One of the operators with a well established holographic dual and which at the same time can be computed by localization, is the Wilson loop, defined as [12]

$$W_{\mathcal{R}}(C, \mathbf{n}) = \left\langle \text{tr}_{\mathcal{R}} \text{P exp} \left[ \oint_C ds \left( i\dot{x}^\mu A_\mu + |\dot{x}| n^I \Phi_I \right) \right] \right\rangle. \tag{11.3.1}$$

The Wilson loop is characterized by a contour  $C = \{x^\mu(s) | s \in (0, 2\pi)\}$  in the four-dimensional space-time (we concentrate on space-like Wilson loops, for which  $\dot{x}^2 > 0$  in the  $-+++$  metric), a contour on  $S^5$  (parameterized by a six-dimensional unit vector  $n^I$ ), and representation  $\mathcal{R}$  of the  $U(N)$  gauge group. For the defining representation ( $\mathcal{R} = \square$ ), the representation label will be omitted.

An important property of the Wilson loop operator is its local invariance under supersymmetry transformations. The general supersymmetry variation of the Wilson loop is

$$\delta_\epsilon W = \left\langle \text{tr}_{\mathcal{R}} \text{P} \oint d\tau \bar{\epsilon} \left( i\dot{x}^\mu \gamma_\mu + |\dot{x}| \gamma^5 n^I \Gamma_I \right) \Psi \exp \left[ \int_\tau^{\tau+2\pi} ds \left( i\dot{x}^\mu A_\mu + |\dot{x}| n^I \Phi_I \right) \right] \right\rangle.$$

As soon as the 6-vector  $n^I$  has the unit norm the combination of the Dirac matrices that enters the variation is degenerate, because it squares to zero:

$$\left( i\dot{x}^\mu \gamma_\mu + |\dot{x}| \gamma^5 n^I \Gamma_I \right)^2 = 0.$$

Alternatively, the spinor product in the variation can be written as

$$\bar{\epsilon} \left( i\dot{x}^\mu \gamma_\mu + |\dot{x}| \gamma^5 n^I \Gamma_I \right) \Psi = i\bar{\epsilon} \mathcal{P}^+ \dot{x}^\mu \gamma_\mu \Psi, \quad (11.3.2)$$

where

$$\mathcal{P}^\pm = 1 \pm i \frac{\dot{x}^\mu}{|\dot{x}|} \gamma_\mu \gamma^5 n^I \Gamma_I, \quad (11.3.3)$$

are orthogonal half-rank projectors.

Choosing

$$\bar{\epsilon} = \bar{\epsilon}_0 \mathcal{P}^-, \quad (11.3.4)$$

forces the supervariation of the Wilson loop to vanish. The projectors  $\mathcal{P}^\pm$  however depend on the position on the contour, through the velocity vector  $\dot{x}^\mu$ , and so does the parameter of variation  $\bar{\epsilon}$ . For the Wilson loop to be a real supersymmetric invariant,  $\bar{\epsilon}$  must be constant. An example is the straight line, for which the projectors  $\mathcal{P}^\pm$  are constant. As a consequence the straight Wilson line preserves half of the supersymmetry and does not receive any quantum corrections due to supersymmetry protection. A more general construction allows for arbitrary space-time dependence, but involves a non-trivial contour on  $S^5$  correlated with the space-time contour  $C$  [13].

The local super-invariance is not an honest symmetry of the action, but it is sufficient to protect Wilson loops from divergent quantum corrections. The UV divergences arise from small-scale fluctuations of quantum fields, and at short distances any smooth contour resembles the straight line, which is supersymmetric. Supersymmetry is not sufficient to cancel all quantum corrections for arbitrary Wilson loops, but it makes them UV finite.

An interesting intermediate case between completely trivial supersymmetric Wilson loops and too complicated generic observables are Wilson loops invariant under superconformal transformations. They are not entirely protected from quantum corrections, but superconformal invariance entails massive cancellations and leaves behind a relatively simple result, that sometimes can be computed by localization of the path integral.

The supersymmetry variation is a superconformal transformation if the spinor  $\bar{\epsilon}$  is a linear function of  $x^\mu$ :

$$\bar{\epsilon} = \bar{\eta} + \bar{\chi} x^\mu \gamma_\mu, \quad (11.3.5)$$

where  $\bar{\eta}$  and  $\bar{\chi}$  are arbitrary, coordinate-independent 10d Majorana-Weyl spinors. Superconformally invariant Wilson loops can be completely classified [14]. We begin with the simplest case – the circular loop. The expectation value for the circle can be computed exactly and reduces to a zero-dimensional Gaussian matrix model, as was initially conjectured on account of perturbative calculations [15, 16] and then proved by computing the path integral of  $\mathcal{N} = 4$  SYM with the help of localization [6].

Let us show that the circular Wilson loop is invariant under half of superconformal transformations. For the circle in the (34) plane,

$$\dot{x}^a = \varepsilon^{ab} x_b, \quad \gamma_a \gamma^5 = \varepsilon_{ab} \gamma^0 \gamma^1 \gamma^b, \quad (11.3.6)$$

where indices  $a$  and  $b$  take values 3 and 4. Taking these identities into account, the projectors (11.3.3) can be brought to the following form:

$$\mathcal{P}^\pm = 1 \pm i \gamma^0 \gamma^1 n^I \Gamma_I x^a \gamma_a. \quad (11.3.7)$$

On a contour in the (34) plane  $x^a \gamma_a = x^\mu \gamma_\mu$ , and the spinor (11.3.4) then has the requisite form (11.3.5) for any constant  $\bar{\epsilon}_0$ . The circular Wilson loop therefore is 1/2 BPS, commuting with 8 superconformal generators.

Another way to see that the circle preserves half of the superconformal symmetry is to notice that it can be mapped to a straight line by a conformal transformation. The expectation values of the circle and the straight line, however, are different, which can be understood as an anomaly associated with the boundary conditions at infinity [9, 16].

When the theory is compactified on  $S^4$ , the BRST generator used for localization of the path integral [6] is among the supersymmetries preserved by the Wilson loop that runs along the big circle of the sphere. In a conformal theory such as  $\mathcal{N} = 4$  SYM correlation functions on the sphere are equivalent to those on the plane, and therefore an expectation value of the circular Wilson loop (be it on  $\mathbb{R}^4$  or on  $S^4$ ) can be computed by localization [6].

The path integral on  $S^4$  localizes to zero modes of one of the scalar fields (for consistency, this has to be the same scalar that appears in the Wilson loop operator), and the partition function reduces to the Gaussian Hermitian matrix model:

$$Z = \int d^{N^2} \Phi e^{-\frac{8\pi^2 N}{\lambda} \text{tr} \Phi^2}. \quad (11.3.8)$$

The matrix-model action originates from the  $\mathcal{R} \text{tr} \Phi^2$  coupling to the curvature of the sphere, which is necessary to maintain the supersymmetry on  $S^4$ . The big-circle Wilson loop maps onto the exponential average in this simple matrix model [6, 15, 16]:

$$W_{\mathcal{R}}(C_{\text{circle}}) = \langle \text{tr}_{\mathcal{R}} e^{2\pi\Phi} \rangle. \quad (11.3.9)$$

The details of the path-integral localization that leads to this formula can be found in Chapter 10 or in [6].

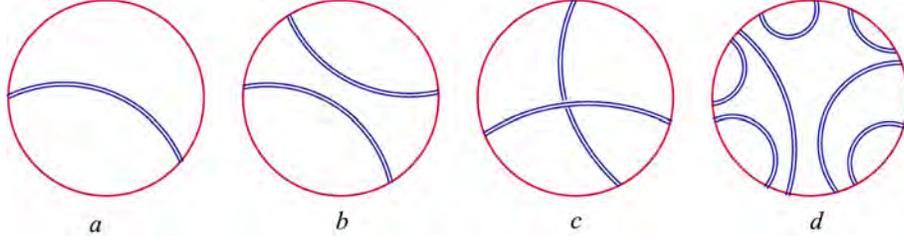

Figure 11.3.1: Rainbow diagrams that contribute to the expectation values of the circular Wilson loop. Each line is a sum of gluon and scalar propagators.

The same result can be derived by resumming the Feynman diagrams of perturbation theory [15, 16]. Consider the first perturbative correction (diagram a in fig. 11.3.1):

$$\frac{1}{N} W(C) = 1 + \frac{\lambda}{16\pi^2} \oint_C ds_1 \oint_C ds_2 \frac{|\dot{x}_1| |\dot{x}_2| - \dot{x}_1 \cdot \dot{x}_2}{(x_1 - x_2)^2} + \dots \quad (11.3.10)$$

The first term in the integral comes from the scalar exchange and the second from the vector propagator. For the circle in the canonical parameterization, the numerator equals  $1 - x_1 \cdot x_2$ , and the denominator  $(x_1 - x_2)^2 = 2 - 2x_1 \cdot x_2$ . The sum of the scalar and vector exchanges combines into a constant, equal to  $\lambda/16\pi^2$ . We can regard this constant as the propagator of an effective zero-dimensional field theory (11.3.8). The two diagrams that contribute at the next order are planar and non-planar rainbow graphs, diagrams b and c in fig. 11.3.1. Other one-loop diagrams appear to cancel among themselves [15]. All propagators in the rainbow graphs are effectively constant and the result is again the same as the second-order perturbation theory in the matrix model. The zero-dimensional average (11.3.9) is a combinatorial tool to generate the sum of rainbow diagrams. The diagrams with internal vertices cancel among themselves and never contribute at any order in perturbation theory [16].

The expectation value (11.3.9), being zero-dimensional and Gaussian, can be calculated exactly [16]:

$$W(C_{\text{circle}}) = e^{\frac{\lambda}{8N}} L_{N-1}^1 \left( -\frac{\lambda}{4N} \right), \quad (11.3.11)$$

where  $L_n^m(x)$  are the Laguerre polynomials. In order to connect to the AdS/CFT duality, we need to take the large- $N$  limit, which amounts to summing planar rainbow graphs. A typical diagram of this type is shown in fig. 11.3.1d. The large- $N$  result can be extracted from (11.3.11), but it is instructive to compute the planar expectation value of the circular loop by standard methods of random matrix theory [17], without using the exact result.

The matrix integral (11.3.8) can be reduced to eigenvalues:

$$Z = \int d^N a \prod_{i < j} (a_i - a_j)^2 e^{-\frac{8\pi^2 N}{\lambda} \sum_i a_i^2}. \quad (11.3.12)$$

At large  $N$ , the saddle-point approximation becomes exact (because the action is  $\mathcal{O}(N^2)$  and there are only  $\mathcal{O}(N)$  integration variables). The distribution of eigenvalues that minimizes the effective action satisfies the following set of equations:

$$\frac{1}{N} \sum_{j \neq i} \frac{1}{a_i - a_j} = \frac{8\pi^2}{\lambda} a_i. \quad (11.3.13)$$

This is an equilibrium condition for  $N$  particles with logarithmic pairwise repulsion in the common harmonic potential. The tendency of eigenvalues to fall into the bottom of the potential is counteracted by repulsion, which causes a finite spread of the eigenvalue distribution. In the thermodynamic (large- $N$ ) limit the distribution is characterized by a continuous density:

$$\rho(x) = \frac{1}{N} \sum_i \delta(x - a_i). \quad (11.3.14)$$

In terms of the density, the saddle-point equations take a form of a singular integral equation:

$$\int_{-\mu}^{\mu} \frac{dy \rho(y)}{x - y} = \frac{8\pi^2}{\lambda} x, \quad x \in (-\mu, \mu). \quad (11.3.15)$$

For  $\mu$  fixed this equation has a unique solution, provided that  $\rho(\pm\mu) = 0$  [18]. The maximal eigenvalue  $\mu$  is then determined by the normalization condition. Altogether, the eigenvalue distribution takes the well-known Wigner form:

$$\rho(x) = \frac{2}{\pi\mu^2} \sqrt{\mu^2 - x^2} \quad (11.3.16)$$

with

$$\mu = \frac{\sqrt{\lambda}}{2\pi}. \quad (11.3.17)$$

The circular Wilson loop can be calculated from (11.3.9):

$$\frac{1}{N} W(C_{\text{circle}}) = \int_{-\mu}^{\mu} dx \rho(x) e^{2\pi x}, \quad (11.3.18)$$

which gives [15]:

$$\frac{1}{N} W(C_{\text{circle}}) = \frac{2}{\sqrt{\lambda}} I_1(\sqrt{\lambda}). \quad (11.3.19)$$

where  $I_\nu(x)$  is the modified Bessel function. The appearance of the square root of  $\lambda$  here is to some extent fictitious, because  $I_1(x)$  is an odd function and the weak-coupling expansion goes in the powers of  $\lambda$  as it should.

But at large argument the Bessel function has an essential singularity and expands in an asymptotic, non-Borel-summable series in  $1/\sqrt{\lambda}$ . To the leading order:

$$\frac{1}{N} W(C_{\text{circle}}) \stackrel{\lambda \rightarrow \infty}{\simeq} \sqrt{\frac{2}{\pi}} \lambda^{-\frac{3}{4}} e^{\sqrt{\lambda}}. \quad (11.3.20)$$

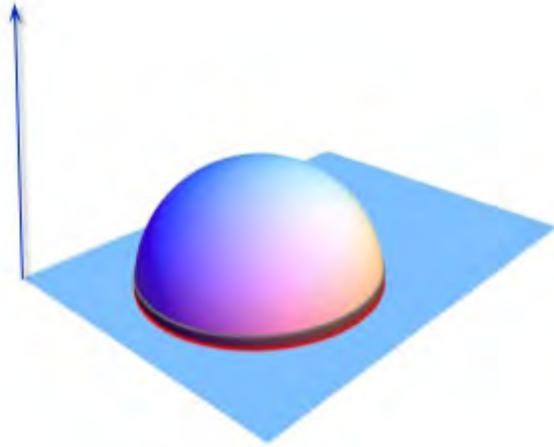

Figure 11.3.2: The minimal surface for the circular Wilson loop. Its area is regularized by cutting out a boundary layer of thickness  $\varepsilon$ .

Now the square root of  $\lambda$  appears for real, as actually expected, because the  $\hbar$  of the string sigma-model according to (11.2.3) is  $2\pi/\sqrt{\lambda}$ , such that  $1/\sqrt{\lambda}$  plays the rôle of the loop counting parameter on the worldsheet.

We now have an explicit result at strong coupling at our disposal, computed directly from the path integral of  $\mathcal{N} = 4$  SYM. According to the AdS/CFT duality, the Wilson loop expectation value maps to a disc amplitude in string theory [12, 19]:

$$W(C, \mathbf{n}) = \int \mathcal{D}h_{ab} \mathcal{D}X^M \mathcal{D}\theta^\alpha e^{-\frac{\sqrt{\lambda}}{2\pi} S_{\text{str}}[h_{ab}, X^M, \theta^\alpha]}, \quad (11.3.21)$$

where  $h_{ab}$ ,  $X^M$  and  $\theta^\alpha$  are the worldsheet metric, the string embedding coordinates and the worldsheet fermions. The full string action is known explicitly [20], but for our classical analysis the bosonic part of the sigma-model in  $AdS_5$  will suffice:

$$S_{\text{str}} = \frac{1}{2} \int d\tau d\sigma \sqrt{-h} h^{ab} \frac{1}{Z^2} (\partial_a X^\mu \partial_b X_\mu + \partial_a Z \partial_b Z) + \dots \quad (11.3.22)$$

The dependence on the shape of the loop originates from the boundary conditions for the string embedding coordinates: the string worldsheet should end on the contour  $C$  on the boundary of AdS (at  $z = 0$  in the Poincaré parameterization (11.2.4)) and on the contour  $n^I$  on  $S^5$ :

$$X^\mu(\sigma, 0) = x^\mu(\sigma), \quad Z(\sigma, 0) = 0, \quad N^I(\sigma, 0) = n^I(\sigma). \quad (11.3.23)$$

At  $\lambda \rightarrow \infty$  the string path integral is saturated by a saddle point and the Wilson loop expectation value obeys the minimal area law in  $AdS_5 \times S^5$ .

We thus need to find the minimal surface in the Anti-de-Sitter space that ends on a circle on the boundary. The solution can actually be obtained without solving any equations, just

by exploiting the symmetries of the problem. For the straight line  $x^\mu(\sigma) = n_1^\mu/(2R) + \sigma n_2^\mu$ , where  $n_1^\mu$  and  $n_2^\mu$  are two orthogonal unit vectors, the minimal surface is obvious:

$$X^\mu = \frac{n_1^\mu}{2R} + \sigma n_2^\mu, \quad Z = \tau, \quad (11.3.24)$$

which is an  $AdS_2$  hyperplane embedded in  $AdS_5$ . The metric of  $AdS_5$  admits the following isometry, which on the boundary reduces to the inversion accompanied by a translation:

$$X^\mu \rightarrow \frac{X^\mu}{Z^2 + X^2} - R n_1^\mu \quad Z \rightarrow \frac{Z}{Z^2 + X^2}. \quad (11.3.25)$$

This transformation leaves the string action invariant, and consequently maps solutions of the equations of motion to solutions. Applying this map to (11.3.24), and changing the worldsheet coordinates as

$$\frac{\tau}{R} \frac{1}{\frac{1}{4R^2} + \tau^2 + \sigma^2} \rightarrow \tanh \tau, \quad \frac{\sigma}{R} \frac{1}{\frac{1}{4R^2} - \tau^2 - \sigma^2} \rightarrow \tan \sigma, \quad (11.3.26)$$

we arrive at the minimal surface for the circle [21, 22]:

$$X^\mu = \frac{R}{\cosh \tau} (n_1^\mu \cos \sigma + n_2^\mu \sin \sigma), \quad Z = R \tanh \tau. \quad (11.3.27)$$

Geometrically this solution represents a hemisphere  $X^2 + Z^2 = R^2$  in the bulk of AdS (fig. 11.3.2).

The solution for the circle, written as (11.3.27), is already in the conformal gauge, and to compute the area one can just plug it in the string action with  $h_{ab} = \delta_{ab}$ . The  $\tau$  integral then diverges because of the  $1/Z^2$  factor in the AdS metric and has to be regularized. The correct renormalization prescription, justified in [22], is to cut off a boundary layer  $Z < \varepsilon$  (as illustrated in fig. 11.3.2), compute the regularized area, and apply an operator  $1 + \varepsilon \partial/\partial\varepsilon$  to the result. The sole function of the last step is to remove the singular  $1/\varepsilon$  term. After that one can send  $\varepsilon$  to zero. Applying this procedure to the minimal surface (11.3.27), we find:

$$S_{\text{str,ren}}(C_{\text{circle}}) = 2\pi \lim_{\varepsilon \rightarrow 0} \left( 1 + \varepsilon \frac{\partial}{\partial \varepsilon} \right) \int_\varepsilon^\infty \frac{d\tau}{\sinh^2 \tau} = -2\pi, \quad (11.3.28)$$

For the Wilson loop expectation value we thus get:

$$W(C_{\text{circle}}) \simeq e^{\sqrt{\lambda}}, \quad (11.3.29)$$

in complete agreement with the exact result (11.3.20) [15]. The prefactor in the asymptotic expansion of the exact formula should come from string fluctuations around the minimal surface (11.3.27). The factor of  $\lambda^{-3/4}$  was interpreted in [16] as a leftover of the residual  $SL(2, \mathbb{R})$  symmetry of the disc partition function. Each of the  $SL(2, \mathbb{R})$  generators is accompanied by a factor of  $\hbar^{1/2} \sim \lambda^{-1/4}$  giving in total  $\lambda^{-3/4}$ . The numerical constant, apart of the fluctuation determinants computed in [23], depends on the structure and normalization

of the measure in the string path integral [24], a delicate issue that has not been sorted out yet (see [25–27] for a recent discussion).

On the matrix model side, the leading exponential behavior of the Wilson loop is dictated by the largest eigenvalue:

$$W(C_{\text{circle}}) \simeq e^{2\pi\mu}, \quad (11.3.30)$$

because the measure in the integral (11.3.18) is exponentially peaked at the rightmost edge of the eigenvalue density. The strong-coupling expansion of the Wilson loop can be systematically constructed by expanding the eigenvalue density in power series in  $\mu - x$ . The integral representation (11.3.18) can then be regarded as the Borel transform of perturbation series in  $1/\sqrt{\lambda}$ , with the Borel variable  $t = \sqrt{\lambda} - 2\pi x$ . The square-root branch cut at the smallest eigenvalue, corresponding to  $t = 2\sqrt{\lambda}$ , renders the strong-coupling expansion non-Borel-summable. Interestingly, it has an instanton interpretation. There is an unstable solution of the string sigma-model with the action equal to  $+2\pi$  [28], which by the standard argument produces a singularity in the Borel plane at  $t = 2\sqrt{\lambda}$ .

## 11.4 Higher representations and D-branes

The circular loop in the fundamental representation probes the AdS/CFT duality at the planar level or, in the string-theory language, at the leading order in the string coupling. It is possible to access all orders in  $1/N$  while still remaining in the realm of classical gravity by considering Wilson loops in large representations whose rank scales with  $N$ :  $k \sim N$ . The fundamental string that ends on the Wilson line then puffs into a D-brane [29], which behaves classically at large  $N$  and large  $\lambda$ . On the field theory side, the regime of  $k \sim N$  requires resummation of all terms in the  $1/N$  expansion enhanced by powers of  $k$ .

We concentrate on completely symmetric and completely anti-symmetric representations (in the latter case  $k$  is bounded  $N$ ; for symmetric representations  $k$  is arbitrary; more general representations are discussed in [30, 31]):

$$\mathcal{R}_k^+ = \overbrace{\square \square \square \dots \square}^k \quad \mathcal{R}_k^- = \left. \begin{array}{c} \square \\ \square \\ \square \\ \vdots \\ \square \end{array} \right\} k. \quad (11.4.1)$$

Wilson loops in these representations depend on two variables in the large- $N$  limit:

$$W_{\pm} \left( \lambda, \frac{k}{N} \right) = W_{\mathcal{R}_k^{\pm}}(C_{\text{circle}}). \quad (11.4.2)$$

The characters of symmetric and anti-symmetric representations are conveniently packaged into the generating functions

$$\chi_{\pm}(\nu, \Phi) = \sum_k e^{-2\pi k\nu} \text{tr}_{\mathcal{R}_k^{\pm}} e^{2\pi\Phi}. \quad (11.4.3)$$

When expressed through eigenvalues, the generating functions of symmetric/anti-symmetric characters are equivalent to Bose or Fermi distributions:

$$\chi_{\pm}(\nu, \Phi) = \prod_{i=1}^N [1 \mp e^{2\pi(a_i - \nu)}]^{-1}. \quad (11.4.4)$$

Consequently,

$$W_{\pm}(\lambda, f) = -i \left\langle \int_{\Lambda - \frac{i}{2}}^{\Lambda + \frac{i}{2}} d\nu e^{2\pi N f \nu} \prod_{i=1}^N [1 \mp e^{2\pi(a_i - \nu)}]^{-1} \right\rangle, \quad (11.4.5)$$

where  $\Lambda$  is some large number, bigger than any  $a_i$ .

It is convenient to think of eigenvalues as (random) energy levels,  $\nu$  then plays the rôle of the chemical potential and  $f$  has the meaning of the particle density. The last formula then relates canonical and grand canonical partition functions of an  $N$ -level system of  $k$  non-interacting particles.

The Bose/Fermi partition functions in (11.4.5) are exponentially large, but not as large as the action in the matrix integral – the exponent is  $O(N)$  compared to the  $O(N^2)$  action. The insertion of the Wilson loop with  $k \sim N$  therefore does not backreact on the saddle point of the matrix model, and the average over the ensemble of random eigenvalues can be replaced, at large  $N$ , by average over the Wigner distribution (11.3.16). The integration over  $\nu$  is also saturated by a saddle point, and we get [32]:

$$W_{\pm}(\lambda, f) \simeq e^{2\pi N F_{\pm}(\lambda, \nu)}, \quad (11.4.6)$$

where the free energy is given by

$$F_{\pm}(\lambda, \nu) = f \nu \mp \frac{1}{2\pi} \int_{-\mu}^{\mu} dx \rho(x) \ln \left( 1 \mp e^{2\pi(x - \nu)} \right). \quad (11.4.7)$$

The chemical potential  $\nu$  is determined by minimizing the free energy:

$$0 = \frac{\partial F_{\pm}}{\partial \nu} = f - \int_{-\mu}^{\mu} \frac{dx \rho(x)}{e^{2\pi(\nu - x)} \mp 1}. \quad (11.4.8)$$

These are the standard textbook formulas for the partition function of a non-interacting Bose/Fermi gas with the single-particle level density  $\rho(x)$ . We are mostly interested in the strong-coupling regime, when the effective temperature (of order one) is much smaller than the typical "energy" (that is, typical eigenvalue), which at strong coupling scales as  $\sqrt{\lambda}$ . Symmetric and anti-symmetric representations behave very differently in the low-temperature regime, and will be considered separately.

We begin with the anti-symmetric case. At low temperature the Fermi distribution is well approximated by the step function, and eq. (11.4.8) simplifies to

$$f = \int_{\nu}^{\mu} dx \rho(x), \quad (11.4.9)$$

which for the Wigner density (11.3.16) gives:

$$\pi f = \theta - \frac{1}{2} \sin 2\theta, \quad (11.4.10)$$

with

$$\cos \theta = \frac{\nu}{\mu}. \quad (11.4.11)$$

For the free energy we get, in the same approximation [32, 33]:

$$F_- = \int_{\nu}^{\mu} dx \rho(x)x = \frac{\sqrt{\lambda}}{3\pi^2} \sin^3 \theta. \quad (11.4.12)$$

The standard low-temperature expansion of the Fermi-gas partition function generates the strong-coupling expansion of the Wilson loop. Explicit results for higher orders in  $1/\sqrt{\lambda}$  can be found in [34].

When the chemical potential  $\nu$  changes between  $+\mu$  to  $-\mu$ , the density  $f$  increases from 0 to 1. This is consistent with the fact that anti-symmetric representations only exist for  $k < N$ , and so  $f$  cannot exceed 1. Moreover, representations with  $k$  and  $N - k$  boxes are complex conjugate to one another. In the above formulas the conjugation symmetry acts as  $\theta \rightarrow \pi - \theta$  and leaves all the equations invariant as it should.

The symmetric case is more subtle, because the chemical potential for bosons must be negative, which in our conventions means that  $\nu > \mu$ . But as  $\nu$  decreases from infinity to  $\mu$ ,  $f$  according to eq. (11.4.8) grows from zero to a finite value

$$f_c = \frac{1}{2\pi} \int_{-\mu}^{\mu} \frac{dx \rho(x)}{\mu - x} = \frac{2}{\sqrt{\lambda}}, \quad (11.4.13)$$

which moreover becomes very small at strong coupling. At larger densities equation (11.4.8) has no solutions. In the statistical mechanics analogy this corresponds to the Bose-Einstein condensation. The Wilson loop expectation value, however, does not have any thermodynamic singularity at  $f = f_c$ , and can be analytically continued past the critical point [32, 35].

In the Bose-Einstein condensed phase a contribution of the largest eigenvalue to the average (11.4.5) is macroscopically large, allowing for  $f > f_c$  in thermodynamic equilibrium. Alternatively one can compute the Wilson loop at  $f < f_c$  and analytically continue the result past the critical point [32]. The equivalence of the two prescriptions is not obvious, but can be proven under very general assumptions [36]. We follow the derivation based on the condensation picture.

A contribution of the largest eigenvalue is singled out by contour deformation in (11.4.5) shown in fig. 11.4.1. The integral then picks a residue at the largest of  $a_i$ 's, which we denote simply by  $a$ . It is important to emphasize that  $a$  is actually different from  $\mu$ . There is a non-zero, albeit small probability to find an eigenvalue outside of the interval on which the macroscopic density is defined. The smallness of this probability is counterbalanced by the exponentially large statistical weight in (11.4.5). Taking into account the extra price of

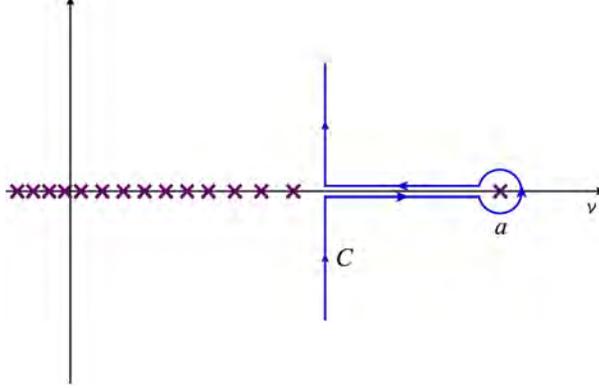

Figure 11.4.1: The contour of integration that singles out the contribution of the largest eigenvalue (from [36]).

pulling out an eigenvalue out of the macroscopic distribution, we get for the leading pole term in (11.4.5):

$$W_{\pm} = \int_{\mu}^{\infty} da P(a) e^{2\pi N f a} \prod_i \frac{1}{1 - e^{2\pi(a_i - a)}} \quad (11.4.14)$$

where  $P(a)$  is the probability to find the largest eigenvalue at  $a$ . The latter can be read off from the partition function (11.3.12):

$$P(a) = \text{const} e^{-\frac{8\pi^2 N}{\lambda} a^2} \prod_i (a - a_i)^2. \quad (11.4.15)$$

The normalization constant is determined by the condition that  $P(\mu) = O(1)$ , so the exponent should vanish at  $a = \mu$ .

Evaluating the integral (11.4.14) in the saddle-point approximation we find for the free energy defined in (11.4.6):

$$F_+ = f a - \frac{4\pi}{\lambda} a^2 + \frac{1}{2\pi} \int_{-\mu}^{\mu} dx \rho(x) \ln \frac{(a-x)^2}{1 - e^{2\pi(x-a)}} + F_0, \quad (11.4.16)$$

where

$$F_0 = \frac{4\pi}{\lambda} \mu^2 - \frac{1}{\pi} \int_{-\mu}^{\mu} dx \rho(x) \ln(\mu - x) = \frac{1}{2\pi} \ln \frac{16\pi^2 e}{\lambda}. \quad (11.4.17)$$

The largest eigenvalue  $a$  is determined by the saddle-point equation  $\partial F_+ / \partial a = 0$ :

$$f = \frac{8\pi a}{\lambda} + \int_{-\mu}^{\mu} dx \rho(x) \left[ \frac{1}{e^{2\pi(a-x)} - 1} - \frac{1}{\pi} \frac{1}{a-x} \right]. \quad (11.4.18)$$

At strong coupling when  $a - \mu \sim \sqrt{\lambda}$ , the first term under the integral is exponentially small in  $\sqrt{\lambda}$  and can be neglected, which gives:

$$f \simeq \frac{8\pi a}{\lambda} - \frac{1}{\pi} \int_{-\mu}^{\mu} \frac{dx \rho(x)}{a-x} = \frac{2}{\pi \mu^2} \sqrt{a^2 - \mu^2} \quad (11.4.19)$$

Introducing the rescaled variable

$$\kappa = \frac{\sqrt{\lambda}f}{4}, \quad (11.4.20)$$

we find that  $a = \mu\sqrt{1 + \kappa^2}$  and [29, 32]

$$\pi F_+ = \kappa\sqrt{1 + \kappa^2} + \operatorname{arcsinh} \kappa. \quad (11.4.21)$$

The string dual of a Wilson loop in the rank- $k$  representation is an object that carries  $k$  units of the string charge. When  $k$  is large, of order  $N$ , a natural candidate is a D-brane [29, 33, 37–41]. This can be justified by considering brane intersections [37, 39], and relies on the following mechanism. Consider a D $_p$ -brane whose  $(p+1)$ -dimensional worldvolume locally looks like  $\Sigma \times S^{p-1}$ , where  $\Sigma$  is a two-dimensional surface that we identify with the string worldsheet. For the sake of the argument we may visualize  $\Sigma$  as being "macroscopic", extending to large distances, while  $S^{p-1}$  being "very small", such that from far apart the worldvolume appears two-dimensional. For the D-brane to carry the correct string charge it should couple to the  $B_{MN}$  field as the fundamental string does.

The D-brane coupling to  $B_{MN}$  arises from the DBI action:

$$S_{\text{DBI}} = T_{\text{Dp}} \int d^{p+1}\sigma \sqrt{\det \left( g_{\mu\nu} + B_{\mu\nu} + \frac{1}{T_{\text{F1}}} F_{\mu\nu} \right)}, \quad (11.4.22)$$

where  $g_{\mu\nu}$  and  $B_{\mu\nu}$  are pullbacks of the target-space fields,  $F_{\mu\nu}$  is the internal gauge field on the D-brane worldvolume,  $T_{\text{Dp}}$  is the D-brane tension and  $T_{\text{F1}}$  is the tension of the fundamental string. Expanding to the linear order in  $B_{\mu\nu}$ , we find:

$$S_{\text{DBI}} \ni T_{\text{F1}} \int d^{p+1}\sigma B_{\mu\nu} \Pi^{\mu\nu} + \dots, \quad (11.4.23)$$

where

$$\Pi^{\mu\nu} = \frac{\delta S_{\text{DBI}}}{\delta F_{\mu\nu}}. \quad (11.4.24)$$

This should be compared to the string coupling to  $B_{MN}$  (the coupling is pure imaginary if the worldsheet is Euclidean):

$$S_{\text{str}} \ni \frac{i}{2} T_{\text{F1}} \int d^2\sigma B_{ab} \varepsilon^{ab}, \quad (11.4.25)$$

where  $B_{ab}$  is the pullback of  $B_{MN}$  onto the worldsheet. The D-brane will carry the correct amount  $k$  of the string charge provided that the electric field  $\Pi^{\mu\nu}$  has components only along  $\Sigma$ , upon averaging over the sphere, and is normalized as

$$\int_{S^{p-1}} d^{p-1}\sigma \Pi^{ab} = \frac{ik}{2} \varepsilon^{ab}. \quad (11.4.26)$$

This can be achieved by adding a Lagrange multiplier to the D-brane action:

$$S_{\text{L.m.}} = -\frac{ik}{2} \int_{\Sigma} d^2\sigma \varepsilon^{ab} F_{ab} = -ik \oint_C d\sigma^a A_a. \quad (11.4.27)$$

Here  $C$  is the contour on the boundary of  $AdS_5$  at which the D-brane ends:  $\partial\Sigma = C$ .

In the natural AdS units, in which the radius of  $AdS_5$  is set to one, the D-brane tensions can be obtained from the standard formulas [42] by replacing  $\alpha' \rightarrow 1/\sqrt{\lambda}$ ,  $g_s \rightarrow \lambda/4\pi N$ :

$$T_{F1} = \frac{\sqrt{\lambda}}{2\pi}, \quad T_{D1} = \frac{2N}{\sqrt{\lambda}}, \quad T_{D3} = \frac{N}{2\pi^2}, \quad T_{D5} = \frac{N\sqrt{\lambda}}{8\pi^4}. \quad (11.4.28)$$

The D-brane tensions are factor of  $N$  larger than the tension of the fundamental string. The D1-brane is dual to the 't Hooft loop in the gauge theory, the D3-branes describe Wilson loops in the symmetric representations [39, 40], and the D5-brane in the anti-symmetric [33, 37]. The rank of the representation is determined by the electric flux on the D-brane world volume, as we have discussed above.

Consider first the D3-brane [29]. Collecting together the DBI action, the Wess-Zumino coupling to the five-form potential and the Lagrange-multiplier term we get for the D3-brane action:

$$S_{D3} = \frac{N}{2\pi^2} \int d^4x \left[ \sqrt{\det_{\mu\nu} \left( g_{\mu\nu} + \frac{2\pi}{\sqrt{\lambda}} F_{\mu\nu} \right)} - \frac{1}{4!} \varepsilon^{\mu\nu\lambda\rho} C_{\mu\nu\lambda\rho} \right] - ik \oint_C A \quad (11.4.29)$$

As before, we will first solve the problem for the straight line and then get the result for the circle by a conformal transformation.

The D3-brane dual to the straight line has an  $AdS_2 \times S^2$  shape, where  $AdS_2$  is the original string worldsheet in the  $(xz)$  plane, and  $S^2$  is the round sphere linking the  $x$  axis in  $\mathbb{R}^4$ . The radius of the sphere evolves along the holographic direction, such that the D-brane embedding can be parameterized by  $r = r(z)$ . At the boundary of  $AdS_5$  the D-brane should shrink to the Wilson line so the boundary condition at  $z = 0$  is  $r(0) = 0$ . The potential of the RR five-form that supports the  $AdS_5 \times S^5$  geometry, in a convenient gauge is given by

$$C = \frac{r^2}{z^4} dx \wedge dr \wedge \text{Vol}(S^2). \quad (11.4.30)$$

Introducing the rescaled field strength,

$$F \equiv \frac{2\pi}{\sqrt{\lambda}} F_{xz}, \quad (11.4.31)$$

we arrive at the reduced D-brane action:

$$S_{D3} = \frac{2N}{\pi} \int dx dz \left[ \frac{r^2}{z^4} \left( \sqrt{\dot{r}^2 + 1 + z^4 F^2} - \dot{r} \right) - i\kappa F \right], \quad (11.4.32)$$

where  $\kappa$  is defined in (11.4.20).

The equations of motion that follow from this action are

$$\frac{r^2 F}{\sqrt{\dot{r}^2 + 1 + z^4 F^2}} = i\kappa$$

$$\left[ \frac{r^2}{z^4} \left( \frac{\dot{r}}{\sqrt{\dot{r}^2 + 1 + z^4 F^2}} - 1 \right) \right]' = \frac{2r}{z^4} \left( \sqrt{\dot{r}^2 + 1 + z^4 F^2} - \dot{r} \right). \quad (11.4.33)$$

In spite of their complicated appearance, they have a simple solution:

$$r = \kappa z, \quad F = \frac{i}{z^2}. \quad (11.4.34)$$

The action on this solution diverges, but cutting off the divergence at  $z = \varepsilon$  and applying  $1 + \varepsilon \partial/\partial\varepsilon$  we get zero, in accord with non-renormalization of the straight Wilson line, whose expectation value is  $W_k(\text{line}) = 1$  as expected.

The solution for the circular loop can be obtained by inversion, but looks rather complicated in the standard Poincaré coordinates. The problem can be greatly simplified by a judicious choice of coordinates [33]. Applying a coordinate transformation  $(r, z) \rightarrow (u, \zeta)$ :

$$r = \zeta \tanh u, \quad z = \frac{\zeta}{\cosh u}, \quad (11.4.35)$$

and substituting it into the  $AdS_5$  metric

$$ds_{AdS_5}^2 = \frac{dz^2 + dx^2 + dr^2 + r^2 d\Omega_{S^2}^2}{z^2}, \quad (11.4.36)$$

we get:

$$\begin{aligned} ds_{AdS_5}^2 &= du^2 + \cosh^2 u \frac{d\zeta^2 + dx^2}{\zeta^2} + \sinh^2 u d\Omega_{S^2}^2 \\ &= du^2 + \cosh^2 u d\Omega_{AdS_2}^2 + \sinh^2 u d\Omega_{S^2}^2. \end{aligned} \quad (11.4.37)$$

The boundary is now at  $u \rightarrow \infty$  (or  $\zeta \rightarrow 0$ ) and has the geometry of  $AdS_2 \times S^2$ . This slicing of the AdS space may look unusual, but there is no contradiction, since  $\mathbb{R}^4$  is conformally equivalent to  $AdS_2 \times S^2$ . This is easily seen by writing the Euclidean metric as

$$ds_{\mathbb{R}^4}^2 = r^2 \left( \frac{dx^2 + dr^2}{r^2} + d\Omega_{S^2}^2 \right). \quad (11.4.38)$$

The solution (11.4.34) in the new coordinates is simply

$$\sinh u = \kappa, \quad F = \frac{i\sqrt{1 + \kappa^2}}{\zeta^2}. \quad (11.4.39)$$

The D-brane sits at constant  $u$ , and the electric field is proportional to the volume form of  $AdS_2$ .

To obtain the solution for the circle we simply replace the Poincaré coordinates in  $AdS_2$  by the global coordinates:

$$ds_{AdS_5}^2 = du^2 + \cosh^2 u \left( d\chi^2 + \sinh^2 \chi d\varphi^2 \right) + \sinh^2 u d\Omega_{S^2}^2. \quad (11.4.40)$$

The boundary at  $u = \infty$  is still  $AdS_2 \times S^2$  conformally equivalent to  $\mathbb{R}^4$ . For the D-brane solution we again can take the hypersurface that spans  $AdS_2 \times S^2$  at constant  $u$ , with the electric field proportional to the volume form on  $AdS_2$ :

$$\sinh u = \kappa, \quad F \equiv \frac{2\pi}{\sqrt{\lambda}} F_{\varphi\chi} = i\sqrt{1 + \kappa^2} \sinh \chi. \quad (11.4.41)$$

The four-form potential in these coordinates is

$$C = \frac{1}{2} \left( 2 \sinh^3 u \cosh u + \sinh u \cosh u - u \right) \sinh \chi \, d\varphi \wedge d\chi \wedge \text{Vol}(S^2). \quad (11.4.42)$$

Substituting the solution into the D3-brane action (11.4.29) we get:

$$S_{\text{D3}} = \frac{N}{2\pi^2} \times \frac{1}{2} \left( \kappa \sqrt{1 + \kappa^2} + \text{arcsinh } \kappa \right) \times \text{Vol}(S^2) \times \int_0^{2\pi} d\varphi \int_0^{\ln \frac{2}{\varepsilon}} d\chi \sinh \chi. \quad (11.4.43)$$

The last, divergent factor is the volume of  $AdS_2$ , which as usual should be regularized by subtracting the  $1/\varepsilon$  term. The renormalized volume of  $AdS_2$  then equals  $-2\pi$ , and for the D-brane action we get [29]:

$$S_{\text{D3,ren}} = -2N \left( \kappa \sqrt{1 + \kappa^2} + \text{arcsinh } \kappa \right), \quad (11.4.44)$$

in complete agreement with the matrix-model prediction (11.4.6), (11.4.21).

If  $\kappa$  is small,

$$W_+ \simeq e^{4N\kappa} = e^{\sqrt{\lambda}k}. \quad (11.4.45)$$

This is just the  $k$ -th power of the Wilson loop in the fundamental representation (11.3.29). The character of a rank- $k$  representation can be expressed through ordinary traces and for small  $k \ll N$  only the term with the largest number of traces contributes due to the large- $N$  factorization:

$$\langle \text{tr}_{\mathcal{R}_k^\pm} e^{2\pi\Phi} \rangle = \frac{1}{k!} \left\langle \left( \text{tr} e^{2\pi\Phi} \right)^k \right\rangle + \langle \mathcal{O}(\text{tr}^{k-1}) \rangle = \frac{N^k}{k!} W_\square^k + \mathcal{O}(N^{k-1}). \quad (11.4.46)$$

For larger  $\kappa$  the result starts to deviate from the simple  $k$ -th power of the fundamental loop and consequently non-planar diagrams start to contribute. The complete result entails resummation of the  $(\lambda k^2/N^2)^n$  terms in the perturbative series and thus receives contributions from all orders of the  $1/N$  expansion. This calculation therefore probes the AdS/CFT duality beyond the planar approximation.

A Wilson loop in an anti-fundamental representation is dual to a D5-brane. The classical solution in that case [33] is quite a bit simpler, because the D5-brane expands in  $S^5$  rather than  $AdS_5$ . The expanded geometry has the direct product structure  $\Sigma \times S^4$  not just locally but over the whole worldvolume of the D-brane. The four-sphere wraps a latitude on  $S^5$  at a fixed polar angle  $\theta$ . The action of the D5-brane is

$$S_{\text{D5}} = \frac{N\sqrt{\lambda}}{8\pi^4} \left[ \int d^6x \sqrt{\det \left( g_{\mu\nu} + \frac{2\pi}{\sqrt{\lambda}} F_{\mu\nu} \right)} - \frac{2\pi i}{\sqrt{\lambda}} \int F \wedge C \right] - ik \oint_C A. \quad (11.4.47)$$

As before it is convenient to represent the last term as a volume integral over  $\Sigma$ . Using the product structure of the D-brane's worldvolume, one can integrate by parts the Wess-Zumino term, and since  $dC = -4\text{Vol}(S^5)$ , the integral of  $C$  gives four times the volume enclosed by  $S^4$  inside  $S^5$ :

$$\int_{S^4} C = -4 \times \frac{8\pi^2}{3} \int_0^\theta d\psi \sin^4 \psi = -4\pi^2 \left( \theta - \sin \theta \cos \theta - \frac{2}{3} \sin^3 \theta \cos \theta \right). \quad (11.4.48)$$

Parametrizing  $\Sigma$  by the holographic coordinate  $z$  and the polar angle  $\varphi$  on the boundary, and absorbing the factor of  $2\pi/\sqrt{\lambda}$  into  $F_{\varphi z}$ , we get:

$$S_{D5} = \frac{N\sqrt{\lambda}}{\pi^2} \int d\varphi dz \left[ \frac{A}{z^2} \sqrt{r^2(\dot{r}^2 + 1) + z^4 F^2} - iBF \right], \quad (11.4.49)$$

where

$$\begin{aligned} A &= \frac{1}{3} \sin^4 \theta \\ B &= \frac{1}{2} \left( \pi f - \theta + \sin \theta \cos \theta + \frac{2}{3} \sin^3 \theta \cos \theta \right). \end{aligned} \quad (11.4.50)$$

Here  $f = k/N$  and does not depend on  $\sqrt{\lambda}$ , in contradistinction to the D3-brane case. This is because a D5-brane is a factor of  $\sqrt{\lambda}$  heavier than a D3-brane.

The equations of motion for (11.4.49) are

$$\begin{aligned} \frac{Az^2 F}{\sqrt{r^2(\dot{r}^2 + 1) + z^4 F^2}} &= iB \\ \left( \frac{r^2}{z^2} \frac{\dot{r}}{\sqrt{r^2(\dot{r}^2 + 1) + z^4 F^2}} \right)' &= \frac{r}{z^2} \frac{\dot{r}^2 + 1}{\sqrt{r^2(\dot{r}^2 + 1) + z^4 F^2}} \end{aligned} \quad (11.4.51)$$

Their solution is very simple – the string worldsheet in AdS is undeformed:

$$r = \sqrt{R^2 - z^2}, \quad (11.4.52)$$

and the field strength is equal to

$$F = i \frac{B}{\sqrt{A^2 + B^2}} \frac{R}{z^2}. \quad (11.4.53)$$

Plugging this into the action (11.4.49) we get:

$$S_{D5} = \frac{2N\sqrt{\lambda}}{\pi} \sqrt{A^2 + B^2} R \int_{\varepsilon}^R \frac{dz}{z^2}. \quad (11.4.54)$$

After subtracting the  $1/\varepsilon$  divergence, this becomes

$$S_{D5,\text{ren}} = -\frac{2N\sqrt{\lambda}}{\pi} \sqrt{A^2 + B^2} \quad (11.4.55)$$

The position of the D5-brane on  $S^5$  is determined by minimization of the on-shell action in  $\theta$ . Using the equality  $\partial B/\partial\theta = -4A$ , we find:

$$\frac{\partial}{\partial\theta} (A^2 + B^2) = 2A \left( \frac{\partial A}{\partial\theta} - 4B \right) = \frac{4}{3} \sin^4 \theta (\theta - \sin \theta \cos \theta - \pi f). \quad (11.4.56)$$

Consequently,

$$\pi f = \theta - \frac{1}{2} \sin 2\theta. \quad (11.4.57)$$

For the renormalized action we thus get:

$$S_{\text{D5,ren}} = -\frac{2N\sqrt{\lambda}}{3\pi} \sin^3 \theta. \quad (11.4.58)$$

Again this is in perfect agreement [33] with the matrix-model predictions (11.4.6), (11.4.10) and (11.4.12).

The holographic calculations described above are purely classical, which is justified by a combination of the large- $N$  and strong-coupling limits. Since the D-brane tension is proportional to  $N$ , quantum fluctuations are  $1/N$  suppressed. The one-loop fluctuation corrections have been actually calculated for the D5-brane in [43, 44] and for the D3-brane in [44, 45], but the results so far disagree with the  $1/N$  corrections in the matrix model, which can also be accounted for. The disagreement does not necessarily mean that the relationship between Wilson loops and D-branes only holds at the leading order. It may well be that the  $1/N$  expansion on the matrix-model side contains some subtle contributions which have been overlooked, or the backreaction of the D-branes on the geometry (which for a single D-brane is a  $1/N$  effect) has not been properly taken into account. It would be very interesting to resolve this apparent contradiction.

## 11.5 Wavy lines, cusp and latitude

In this section we consider, following [46], a number of Wilson loop observables – the wavy lines, the cusp anomalous dimension, the heavy quark potential and the circular latitude on  $S^5$ . At first sight they seem unrelated but in fact can be expressed through one another, and some of them can be computed with the help of localization.

A wavy line [47, 48] (fig. 11.5.1a) is the straight line with a small perturbation on top:  $x^\mu(t) = \delta_0^\mu t + \xi^\mu(t)$ . Its expectation value starts at the quadratic order in waviness. The functional form of the leading piece is completely fixed by translational invariance and scale symmetry [48]:

$$\frac{1}{N} W(C_\xi) - 1 = \frac{B}{2} \int_{-\infty}^{+\infty} dt_1 dt_2 \frac{(\dot{\xi}(t_1) - \dot{\xi}(t_2))^2}{(t_1 - t_2)^2} + \mathcal{O}(\xi^4). \quad (11.5.1)$$

The coefficient  $B \equiv B(\lambda)$  is called the Bremsstrahlung function [46].

It is instructive to see how this structure arises at the leading order in perturbation theory. Expanding the sum of scalar and vector propagators, eq. (11.3.10), in  $\xi$  we get:

$$\frac{|1 + \dot{\xi}_1| |1 + \dot{\xi}_2| - (1 + \dot{\xi}_1 \cdot \dot{\xi}_2)}{(t_1 - t_2)^2 + (\xi_1 - \xi_2)^2} = \frac{1}{2} \frac{(\dot{\xi}(t_1) - \dot{\xi}(t_2))^2}{(t_1 - t_2)^2} + \mathcal{O}(\xi^4), \quad (11.5.2)$$

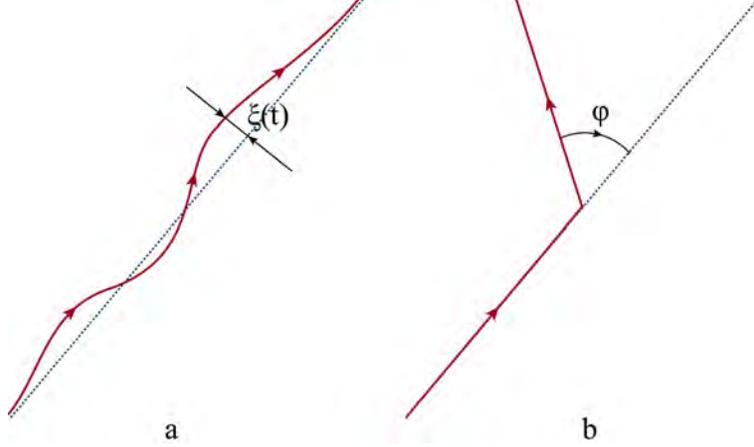

Figure 11.5.1: (a) A wavy line. (b) Cusp with an opening angle  $\pi - \phi$ .

which gives for the weak-coupling asymptotics of the Bremsstrahlung function [48]:

$$B(\lambda) \simeq \frac{\lambda}{16\pi^2} \quad (\lambda \rightarrow 0). \quad (11.5.3)$$

In QED, where only the vector exchange is present, the wavy line could be brought to the same form by subtracting the linearly divergent self-energy. The Bremsstrahlung function then is  $B_{\text{QED}} = 2\alpha/3\pi$  at the leading order of perturbation theory.

Another quantity of interest is the cusp anomalous dimension. If a contour has a cusp, the associated Wilson loop develops a logarithmic singularity due to locally divergent diagrams [49]. Since the anomaly is a local effect, it can be studied by zooming onto the vicinity of the cusp and considering the contour shown in fig. 11.5.1b. The expectation value of an infinite cusp diverges both in the UV and in the IR, and needs regularization. The natural IR cutoff is the scale  $L$  at which the Wilson loop starts to deviate from the simple straight-line cusp. To implement the UV cutoff one can round off the tip of the cusp on the scale of order  $\varepsilon \ll L$ .

The expectation of a Wilson loop with a cusp behaves as

$$W(C_{\text{cusp}}) = \text{const} \left( \frac{L}{\varepsilon} \right)^{\Gamma_{\text{cusp}}(\phi, \lambda)}. \quad (11.5.4)$$

The exponent  $\Gamma_{\text{cusp}}(\varphi, \lambda)$  is called the cusp anomalous dimension and depends on the opening angle of the cusp and the 't Hooft coupling. It can be computed order by order in perturbation theory. The cusp anomalous dimension has important applications in QCD [50], and has been extensively studied in the context of the AdS/CFT duality [22, 51–54].

At the first order of perturbation theory, we get from (11.3.10):

$$\begin{aligned} \frac{1}{N} W(C_{\text{cusp}}) &= 1 + \frac{\lambda}{8\pi^2} \int_{\varepsilon}^L ds dt \frac{1 - \cos \phi}{s^2 + t^2 + 2st \cos \phi} \\ &= 1 + \frac{\lambda}{8\pi^2} \phi \frac{1 - \cos \phi}{\sin \phi} \int_{\varepsilon}^L \frac{dt}{t} + \text{finite}. \end{aligned} \quad (11.5.5)$$

The integral over  $t$  produces the divergent logarithm, and for the one-loop cusp anomaly we obtain [22]:

$$\Gamma_{\text{cusp}}(\phi, \lambda) = \frac{\lambda}{8\pi^2} \phi \tan \frac{\phi}{2} \quad (\lambda \rightarrow 0). \quad (11.5.6)$$

This formula has a number of interesting limits. It can be analytically continued to pure imaginary angles:  $\phi \rightarrow i\theta$ , which is equivalent to changing the Euclidean cusp into a contour in the Minkowski space. The cusp then corresponds to a trajectory of a real particle that experiences an instantaneous acceleration. As can be seen from the leading-order result (11.5.6), but is true more generally, the cusp anomaly is a growing function of rapidity with linear asymptotics:

$$\Gamma_{\text{cusp}}(i\theta, \lambda) = -4f(\lambda)\theta \quad (\theta \rightarrow \infty). \quad (11.5.7)$$

The function  $f(\lambda)$ , that characterizes the light-like cusp, is also referred to as the cusp anomalous dimension. It is related to the scaling dimensions of twist-2 local operators:

$$\mathcal{O}_S = \text{tr} Z D_+^S Z, \quad (11.5.8)$$

where  $Z = \Phi_1 + i\Phi_2$  and  $D = D_1 + D_2$ . The twist-2 anomalous dimension grows logarithmically with the spin, and the coefficient coincides with the cusp anomaly:

$$\gamma_S(\lambda) \simeq f(\lambda) \ln S \quad (S \rightarrow \infty). \quad (11.5.9)$$

When the opening angle approaches  $\pi$  (equivalently,  $\phi \rightarrow 0$ ), the cusp becomes the straight line, whose expectation values is finite, and is actually trivial in  $\mathcal{N} = 4$  SYM. The anomalous dimension should consequently vanish at  $\phi = 0$ . Its Taylor expansion starts at the second order and is expressed through the Bremsstrahlung function. The explicit one-loop result (11.5.6) is in accord with these observations. Indeed, the cusp with a very small deflection angle can be viewed as a particular case of the wavy line, and its expectation value can be thus extracted from the general formula (11.5.1) by substituting  $\dot{\xi}^\mu = \theta(t)\phi n^\mu$ , where  $n^\mu$  is the unit normal to the first segment of the cusp:

$$\frac{1}{N} W(C_{\text{cusp}}) - 1 \stackrel{\phi \rightarrow 0}{\simeq} B\phi^2 \int_\varepsilon^L \frac{dt_1 dt_2}{(t_1 + t_2)^2} = B\phi^2 \ln \frac{L}{\varepsilon}, \quad (11.5.10)$$

which implies that

$$\Gamma_{\text{cusp}}(\phi, \lambda) \stackrel{\phi \rightarrow 0}{\simeq} B(\lambda)\phi^2. \quad (11.5.11)$$

Finally, the quark-anti-quark potential can be also expressed through the cusp anomaly. Because of the conformal invariance, the potential in  $\mathcal{N} = 4$  SYM obeys the Coulomb law:

$$V(L, \lambda) = -\frac{\alpha(\lambda)}{L}, \quad (11.5.12)$$

and is characterized by a single functions of the 't Hooft coupling, the Coulomb charge  $\alpha$ .

Normally, the quark-anti-quark potential is associated with the long rectangular contour, but it can also be extracted from the cusp anomaly. The cusped Wilson loop physically

corresponds to a quark-anti-quark pair created at the tip of the cusp, the two particles flying apart at constant velocity. When the opening angle of the cusp is very small ( $\phi \rightarrow \pi$ ), the relative velocity is also small and the interaction between the particles is dominated by the quasi-static Coulomb energy:

$$\ln W(C_{\text{cusp}}) \simeq \int_{\varepsilon}^L dt \frac{\alpha}{2t \sin \frac{\pi-\phi}{2}} \simeq \frac{\alpha}{\pi-\phi} \ln \frac{L}{\varepsilon}. \quad (11.5.13)$$

Consequently,

$$\alpha(\lambda) = \lim_{\phi \rightarrow \pi} (\pi - \phi) \Gamma_{\text{cusp}}(\phi, \lambda). \quad (11.5.14)$$

In particular, at weak coupling we get:

$$\alpha(\lambda) = \frac{\lambda}{4\pi} \quad (\lambda \rightarrow 0). \quad (11.5.15)$$

At strong coupling the cusp anomalous dimension is determined by the area of the minimal surface in  $AdS_5$  ending on the cusp at the boundary [22]. Due to the symmetries of the problem, the solution has a self-similar form. In the polar coordinates  $(r, \varphi)$  centred at the tip of the cusp the minimal surface can be parameterized as

$$z = ru(\varphi). \quad (11.5.16)$$

The Nambu-Goto action evaluated on this ansatz is

$$S_{\text{str}} = \frac{\sqrt{\lambda}}{2\pi} \int \frac{dr}{r} d\varphi \frac{1}{u^2} \sqrt{1 + u^2 + \dot{u}^2}. \quad (11.5.17)$$

Integration over  $r$  diverges logarithmically and gives the requisite  $\ln(L/\varepsilon)$  factor.

The equations of motion for  $u$  admit a first integral, due to translational symmetry in the angular direction, which can be used to solve for  $\dot{u}$ :

$$\dot{u} = \frac{1}{u^2} \sqrt{(u_0^2 - u^2)(u^2 + 1) \left( u^2 + \frac{u_0^2}{1 + u_0^2} \right)}, \quad (11.5.18)$$

where  $u_0$  is the constant of integration. Geometrically,  $u_0$  is the maximum of  $u(\varphi)$ , which due to the symmetries of the problem is reached at  $\varphi = (\pi - \phi)/2$ . Consequently,

$$\frac{\pi - \phi}{2} = \int_0^{u_0} \frac{du}{\dot{u}}. \quad (11.5.19)$$

The integration yields:

$$\frac{\pi - \phi}{2} = \frac{1}{u_0} \sqrt{\frac{1 + u_0^2}{2 + u_0^2}} \left[ (1 + u_0^2) \Pi(-u_0^2) - K \right], \quad (11.5.20)$$

where  $\Pi(n) \equiv \Pi(n|m)$  and  $K \equiv K(m)$  are the standard elliptic integrals of the third and first kind with the modulus given by

$$m = \frac{1}{2 + u_0^2}. \quad (11.5.21)$$

Changing the integration variable in (11.5.17) from  $\varphi$  to  $u$  with the help of (11.5.18), and subtracting the usual  $1/\varepsilon$  divergence near the boundary, we get for the cusp anomaly at strong coupling [22, 55]:

$$\Gamma_{\text{cusp}} = \frac{\sqrt{\lambda}}{\pi u_0 \sqrt{2 + u_0^2}} \left[ (2 + u_0^2) E - (1 + u_0^2) K \right], \quad (11.5.22)$$

where  $u_0$  is expressed through  $\phi$  by inverting (11.5.20).

The strong-coupling behavior of the Coulomb charge can be extracted from the above formulas by taking the  $u_0 \rightarrow 0$  limit and using (11.5.14), which gives [12, 19]:

$$\alpha(\lambda) \simeq \frac{4\pi^2 \sqrt{\lambda}}{\Gamma^4\left(\frac{1}{4}\right)} \quad (\lambda \rightarrow \infty). \quad (11.5.23)$$

The opposite limit  $u_0 \rightarrow \infty$ , according to (11.5.11), yields the Bremsstrahlung function [48]:

$$B(\lambda) \simeq \frac{\sqrt{\lambda}}{4\pi^2} \quad (\lambda \rightarrow \infty). \quad (11.5.24)$$

The cusped Wilson loop or a generic wavy line cannot be computed by localization directly, because in general they do not preserve any supersymmetry. However, using universality of the wavy line and the fact that some deformations of the circular Wilson loop are supersymmetric, one can use localization to compute the Bremsstrahlung function exactly [46]. Generalizations of these result to other observables and less supersymmetric theories have been studied in [56–60].

The coupling to scalars that preserved enough supersymmetry for localization to apply is the latitude:  $\mathbf{n} = (0, 0, \cos \tau \sin \theta, \sin \tau \sin \theta, \cos \theta, 0)$ , where  $\theta$  is constant. The spacial part of the Wilson loop is the circle in the standard parameterization. The supersymmetry projectors (11.3.3) for the latitude are of the form

$$\mathcal{P}^\pm = 1 \pm i \sin \theta \dot{x}^a \dot{x}^b \gamma_a \Gamma_b \gamma^5 \pm i \cos \theta \gamma^0 \gamma^1 \Gamma_5 x^a \gamma_a, \quad (11.5.25)$$

where in the last term we used the identities (11.3.6). Not all of the spinors  $\bar{\epsilon}_0 \mathcal{P}^-$  are of the form (11.3.5) necessary for superconformal invariance, because of the middle term in the projector. We can get rid of this term by imposing an extra condition on  $\bar{\epsilon}_0$ :

$$\bar{\epsilon}_0 (\gamma_3 \Gamma_4 + \gamma_4 \Gamma_3) = 0, \quad (11.5.26)$$

or equivalently

$$\bar{\epsilon}_0 \gamma_{(a} \Gamma_{b)} = \frac{1}{2} \delta_{ab} \bar{\epsilon}_0 \gamma^c \Gamma_c. \quad (11.5.27)$$

Then,

$$\bar{\epsilon} \equiv \bar{\epsilon}_0 \mathcal{P}^- = \bar{\epsilon}_0 \left( 1 - \frac{i}{2} \sin \theta \gamma^a \Gamma_a \gamma^5 - i \cos \theta \gamma^0 \gamma^1 \Gamma_5 x^a \gamma_a \right), \quad (11.5.28)$$

which is now a conformal Killing spinor. The extra condition (11.5.26) reduces the number of allowed supersymmetries by half, so the latitude is 1/4 BPS [28].

When  $\theta = \pi/2$ , the spinor (11.5.28) does not depend on  $x^\mu$  at all, and the equatorial latitude is invariant under 1/4 of the rigid supersymmetry [13]. Its expectation value equals to one due to supersymmetry protection. For  $\theta = 0$  the contour on  $S^5$  shrinks to a point, and we get back to the circular Wilson loop discussed in sec. 11.3.

As conjectured in [28] and proved rigorously in [61], the exact expectation value of the latitude is given by the sum of rainbow diagrams for any  $\theta$ , not just  $\theta = 0$ . The basic line-to-line propagator is equal to

$$\frac{\lambda}{8\pi^2} \frac{|\dot{x}_1| |\dot{x}_2| \mathbf{n}_1 \cdot \mathbf{n}_2 - \dot{x}_1 \cdot \dot{x}_2}{(x_1 - x_2)^2} = \frac{\lambda \cos^2 \theta}{16\pi^2}, \quad (11.5.29)$$

and is again a constant, rescaled by a factor of  $\cos^2 \theta$  compared to the circular loop case. The expectation value of the latitude is consequently given by the same expression (11.3.19), under a simple replacement  $\lambda \rightarrow \lambda \cos^2 \theta$ :

$$\frac{1}{N} W(C_{\text{latitude}}) = \frac{2}{\sqrt{\lambda} \cos \theta} I_1(\sqrt{\lambda} \cos \theta). \quad (11.5.30)$$

At strong coupling:

$$W(C_{\text{latitude}}) \simeq e^{\sqrt{\lambda} \cos \theta}. \quad (11.5.31)$$

This result is in perfect agreement with the AdS/CFT duality. The minimal surface for the latitude [62] is the direct product of the hemisphere (11.3.27) in space-time and a solid angle with apex  $2\theta$  on  $S^5$  – in the conformal gauge the solutions in  $AdS_5$  and  $S^5$  are independent provided each of them separately satisfies the Virasoro constraints. The regularized area of the hemisphere is  $-2\pi$ , while the solid angle subtended by the latitude is  $+2\pi(1 - \cos \theta)$ , which altogether gives the area of  $-2\pi \cos \theta$ , to be multiplied by the string tension  $\sqrt{\lambda}/2\pi$ . The exponent of the string amplitude that determines the expectation value of the latitude holographically is thus exactly the same as the one in (11.5.31).

The latitude with  $\theta \rightarrow 0$  can be regarded as a small perturbation of the circular Wilson loop. Even though the wavy line was originally defined by contour deformation in space-time, the quadratic part for the deviation on  $S^5$  is controlled by the same Bremsstrahlung function [46]:

$$\frac{W(C_{\text{latitude}}) - W(C_{\text{circle}})}{W(C_{\text{circle}})} = -\frac{1}{2\pi^2} B(\lambda) \theta^2 + \dots \quad (11.5.32)$$

Since the expectation value for the latitude is obtained from that for the circle by replacing  $\lambda \rightarrow \lambda \cos^2 \theta \approx \lambda(1 - \theta^2)$ , we get:

$$B(\lambda) = \frac{1}{2\pi^2} \frac{\partial \ln W(C_{\text{circle}})}{\partial \ln \lambda}. \quad (11.5.33)$$

The exact result for the circle (11.3.19) then implies [46]:

$$B(\lambda) = \frac{\sqrt{\lambda} I_2(\sqrt{\lambda})}{4\pi^2 I_1(\sqrt{\lambda})}. \quad (11.5.34)$$

This is an exact result valid for arbitrary  $\lambda$  and large  $N$  (the finite- $N$  result can be obtained by differentiating (11.3.11)). At strong coupling it agrees with the AdS/CFT prediction (11.5.24), since the ratio of the two Bessel functions approaches one when their arguments go to infinity.

Interestingly, the same function  $B(\lambda)$  appears in the correlator of the straight Wilson line with the Lagrangian density operator inserted at infinity [56], thus reconfirming an interpretation of the Bremsstrahlung function in terms of the dipole radiation of an accelerated quark [46, 63, 64]. This relationship was recently elaborated further for  $\mathcal{N} = 2$  theories [58–60].

Localization determines the leading order in the expansion of the cusp anomalous dimension around the supersymmetric configuration (the straight line). The other two limits considered above,  $\phi \rightarrow \pi$  and  $\phi \rightarrow i\infty$ , are not supersymmetric. However, exact non-perturbative results are available even in this case, due to remarkable integrability properties of the planar  $\mathcal{N} = 4$  SYM. In fact the whole function  $\Gamma_{\text{cusp}}(\phi, \lambda)$  can be computed from Thermodynamic Bethe Ansatz equations (TBA). The light-like cusp is described by the asymptotic Bethe ansatz at any value of the coupling constant [65], via its relationship to the twist-two local operators. The full machinery of TBA yields a set of more general functional equations which determine the cusp anomaly at any  $\phi$  and any  $\lambda$  [66–69]. The non-perturbative expression for the Bremsstrahlung function (11.5.34) can be recovered from the TBA equations, and can be generalized to include local operators inserted at the tip of the cusp [70].

The latitude belongs to a larger class of 1/8 supersymmetric Wilson loops, all of which can be computed by localization. Suppose that the contour  $C$  is restricted to lie on the surface of a two-dimensional sphere  $S^2 \subset \mathbb{R}^4$ , such that at any  $s$ ,  $x^0(s) = 0$ , and  $x^i(s)$  form a three-dimensional unit vector. The 1/8 BPS Wilson loop [71] is then defined as

$$W_{2d}(C) = \left\langle \text{tr P exp} \left[ \oint_C dx^i (iA_i + \varepsilon_{ijk} x^j \Phi^k) \right] \right\rangle. \quad (11.5.35)$$

It depends on three out of six scalar fields. The supersymmetry projectors (11.3.3) for this type of Wilson loops are

$$\mathcal{P}^\pm = 1 \pm i \dot{x}^l \gamma_l \dot{x}^i x^j \varepsilon_{ijk} \gamma^5 \Gamma^k. \quad (11.5.36)$$

Using the identity

$$\gamma_l = \frac{1}{2} \varepsilon_{lij} \gamma^5 \gamma^0 \gamma^i \gamma^j, \quad (11.5.37)$$

the supersymmetry projector can be brought to a more concise form:

$$\mathcal{P}^\pm = 1 \pm i \gamma^0 \Gamma^i \gamma_{ij} x^j. \quad (11.5.38)$$

The transformation parameter  $\bar{\varepsilon} = \bar{\varepsilon}_0 \mathcal{P}^-$  is not really a Killing spinor (11.3.5), unless extra conditions are imposed. The minimal set of conditions turns out to be

$$\bar{\varepsilon}_0 (\gamma_{ij} + \Gamma_{ij}) = 0, \quad (11.5.39)$$

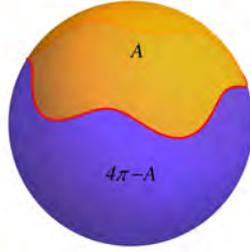

Figure 11.5.2: Wilson loop on  $S^2$ .

where indices  $i$  and  $j$  run from 1 to 3. Only two of these conditions are independent, because the gamma matrices used for the projection form a closed algebra under commutation. These conditions imply that

$$\bar{\epsilon}_0 \Gamma^i = \frac{1}{3} \bar{\epsilon}_0 \Gamma_j \gamma^j \gamma^i. \quad (11.5.40)$$

The parameter of supersymmetry transformations (11.3.4) then becomes

$$\bar{\epsilon} = \bar{\epsilon}_0 \mathcal{P}^- = \bar{\epsilon}_0 - \frac{2i}{3} \bar{\epsilon}_0 \gamma^0 \Gamma_j \gamma^j x^i \gamma_i, \quad (11.5.41)$$

which is a superconformal Killing spinor. The two conditions (11.5.39) reduce the number of eligible constant spinors by a quarter, and the  $\mathcal{P}^-$  projection by another half, so the Wilson loops defined in (11.5.35) are indeed 1/8 BPS.

Quite remarkably, localization reduces the expectation values of the 1/8 BPS Wilson loops to Wilson loops in the bosonic two-dimensional Yang-Mills theory restricted to the zero-instanton sector [55, 72]. The path integral of  $\mathcal{N} = 4$  SYM localizes on two-dimensional field configurations of the gauge field. The  $S^2$  Wilson loops remain invariant under the action of the BRST operator used in localizing the path integral in this way [61]. The 4d and 2d coupling constants are related as  $\lambda_{2d} = -\lambda/4\pi R^2$ , where  $R$  is the radius of the sphere. Since, the 2d coupling is negative, the localization partition function should be defined with care and requires complexification of the gauge group [61].

The two-dimensional Yang-Mills theory is invariant under area-preserving diffeomorphisms, so the Wilson loop without self-intersections can only depend on the area  $A$  it encloses on  $S^2$ , in other words on the solid angle at which the loop is seen from the middle of the sphere (fig. 11.5.2). It should also be symmetric under the interchange of the solid angle  $A$  and its complement:  $A \rightarrow 4\pi - A$ . The exact expectation value of a general  $S^2$  Wilson loop is given

by [55, 72]:

$$\frac{1}{N} W_{2d}(C) = \frac{4\pi}{\sqrt{\lambda A (4\pi - A)}} I_1 \left( \frac{\sqrt{\lambda A (4\pi - A)}}{2\pi} \right). \quad (11.5.42)$$

The latitude (11.5.30), for which  $A = 2\pi(1 - \sin \theta)$ , is a particular example of this class of Wilson loops.

## 11.6 Operator Product Expansion

In addition to expectation values some correlation functions involving Wilson loops can also be computed with the help of localization. We will concentrate on the two-point functions of Wilson loops with local gauge-invariant operators. In that case the problem can be reformulated in terms of the operator product expansion.

When probed from distances much larger than its size, a Wilson loop behaves as a local object, and can be approximated by a local operator insertion. This can be formalized by the operator product expansion of the loop operator [73]:

$$W(C, \mathbf{n}) = \sum_i \mathbb{C}_i[C, \mathbf{n}] \mathcal{O}_i(0), \quad (11.6.1)$$

where  $\mathcal{O}_i$  is a complete set of local gauge-invariant operators, and  $\mathbb{C}_i[C, \mathbf{n}]$  are numerical coefficients that depend on the shape of the contour  $C$  and on the path  $\mathbf{n}$  on the five-sphere. The OPE translates into an expansion of correlation functions of the Wilson loop in powers of  $R/|x|$ , where  $R$  is the characteristic size of the loop and  $|x|$  is a typical scale of the problem. For instance, a two-point function of a Wilson loop and a conformal primary scalar operator can be expanded as

$$\langle W(C, \mathbf{n}) \mathcal{O}_i(x) \rangle = \frac{\mathbb{C}_i[C, \mathbf{n}]}{|x|^{2\Delta_i}} + \text{descendants}, \quad (11.6.2)$$

where  $\Delta_i$  is the scaling dimension of  $\mathcal{O}_i$ . The contribution of descendants contains higher powers of  $1/|x|$ .

Our basic example is the circular Wilson loop. In that case, the two-point correlator with a scalar primary is entirely determined by conformal symmetry, which is best seen after a conformal transformation that maps the circle to a line. In the setup illustrated in fig. 11.6.1 this transformation is an inversion centered at the point  $A$ . The correlator of a local operator and a Wilson line depends only on one length scale and therefore is fixed by scale invariance up to an overall constant. The inverse transformation then determines the correlator with a circle. The overall constant can be identified with the OPE coefficient by matching to (11.6.2) at large distances [21, 74–76]:

$$\langle W(C_{\text{circle}}) \mathcal{O}_i(x) \rangle = \frac{\mathbb{C}_i}{\left[ h^2 + (r - R)^2 \right]^{\frac{\Delta_i}{2}} \left[ h^2 + (r + R)^2 \right]^{\frac{\Delta_i}{2}}}. \quad (11.6.3)$$

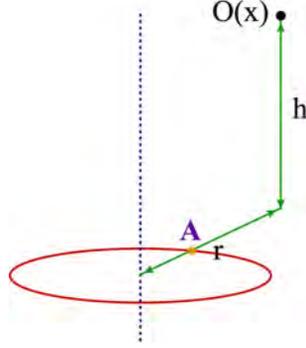

Figure 11.6.1: Correlator of the circular Wilson loop and a local operator.

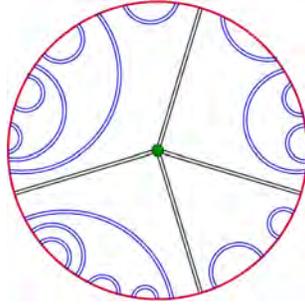

Figure 11.6.2: The only diagrams that contribute to the correlation functions of the circular Wilson loop and a chiral primary operator are the rainbow diagrams without internal vertices.

Here  $h$  is the distance from the point  $x$  to the plane of the circle and  $r$  the distance from  $x$  to the circle's axis of symmetry (fig. 11.6.1).

We are going to concentrate on the correlator of the circular loop with  $\mathbf{n} = (1, \mathbf{0})$  and chiral primary operators (CPO):

$$\mathcal{O}_J = \frac{1}{\sqrt{J}} \left( \frac{4\pi^2}{\lambda} \right)^{\frac{J}{2}} \text{tr} Z^J, \quad (11.6.4)$$

where  $Z = \Phi_1 + i\Phi_2$ . The chiral primaries are supersymmetry-protected and do not receive anomalous dimensions. The normalization factor is chosen such that the two-point function of  $\mathcal{O}_J$  is unit-normalized:

$$\langle \mathcal{O}_J^\dagger(x) \mathcal{O}_J(0) \rangle = \frac{1}{|x|^{2J}}. \quad (11.6.5)$$

The correlation functions  $\langle W(C_{\text{circle}}) \mathcal{O}_J \rangle$  can be computed exactly using localization. The exact answer can again be obtained by summing the rainbow diagrams [77], whereas a rigorous derivation relies on localization of the path integral on  $S^2$  [78]. The rainbow graphs now

contain two types of propagators, those that connect the operator to the loop, and those that connect two different points on the loop, fig. 11.6.2. These diagrams can be resummed by a brute-force account of combinatorics [77]. A more elegant derivation is based on mapping the problem to a Gaussian two-matrix model [78–81].

Both types of propagators in fig. 11.6.2 are effectively constant: the loop-to-loop propagator is equal to  $\lambda/16\pi^2$ , while the operator-to-loop propagator contributes a factor of  $\lambda/8\pi^2|x|^2$  for the operator inserted far away from the loop. These two types of propagators are accounted for by introducing two zero-dimensional fields,  $\Phi$  and  $Z$ , with propagators

$$\begin{array}{c} \Phi \\ \hline \square \end{array} \Phi = \frac{\lambda}{16^2} \quad \begin{array}{c} Z \\ \hline \square \end{array} \Phi = \frac{\lambda}{8\pi^2 i} \quad (11.6.6)$$

The factor of  $i$  in the  $Z\Phi$  propagator makes the quadratic form of the effective matrix model positive-definite. Since there are exactly  $J$   $Z\Phi$  propagators in each diagram, this factor is easily absorbed into an overall normalization of the correlator. The necessity to introduce the factors of  $i$  can be traced back to the fact that the 2d Yang-Mills theory, to which  $\mathcal{N} = 4$  SYM localizes, has a negative coupling and requires complexification of the gauge group [61].

A Gaussian matrix integral that reproduces these propagators is

$$\mathcal{Z}_{2MM} = \int dZ d\Phi e^{-\frac{2\pi^2 N}{\lambda} \text{tr}(Z^2 + 4iZ\Phi)}. \quad (11.6.7)$$

Integrating out  $Z$  we get back to the matrix model (11.3.8) for the circular Wilson loop as expected.

The OPE coefficients map to the following correlation function in the two-matrix matrix model (11.6.7):

$$\mathbb{C}_J^{\text{CPO}} = \frac{R^J}{\sqrt{J}} \left( -\frac{4\pi^2}{\lambda} \right)^{\frac{J}{2}} \langle \text{tr} Z^J \text{tr} e^{2\pi\Phi} \rangle. \quad (11.6.8)$$

To calculate this correlator, we first get rid of one of the  $Z$ 's by Wick contracting it with a  $\Phi$  in the exponential. The problem then reduces to computing single-trace expectation values

$$W_k(s) = \left\langle \frac{1}{N} \text{tr} e^{s\Phi} Z^k \right\rangle, \quad (11.6.9)$$

which are easier to deal with. In terms of those,

$$\mathbb{C}_J^{\text{CPO}} = \frac{\lambda R^J}{4\pi i \sqrt{J}} \left( -\frac{4\pi^2}{\lambda} \right)^{\frac{J}{2}} W_{J-1}(2\pi). \quad (11.6.10)$$

To calculate the mixed correlator (11.6.9) we use the standard method of Schwinger-Dyson equations [82, 83]. The Schwinger-Dyson equations for the two-matrix model (11.6.7) follow from the identity:

$$\int dZ d\Phi \text{tr} \left( \frac{\partial}{\partial \Phi^t} e^{s\Phi} Z^k \right) e^{-\frac{2\pi^2 N}{\lambda} \text{tr}(Z^2 + 4iZ\Phi)} = 0, \quad (11.6.11)$$

where  $\partial/\partial\Phi^t$  acts on everything to the right, making the integrand a total derivative. Performing differentiation we find:

$$\left\langle \int_0^s dt \operatorname{tr} e^{t\Phi} \operatorname{tr} e^{(s-t)\Phi} Z^k - \frac{8\pi^2 i N}{\lambda} \operatorname{tr} e^{s\Phi} Z^{k+1} \right\rangle = 0. \quad (11.6.12)$$

At large- $N$  the expectation value of the double trace appearing in the first term factorizes, and we get a closed system of equations for the matrix-model loop amplitudes (11.6.9):

$$W_{k+1}(s) = \frac{\lambda}{8\pi^2 i} \int_0^s dt W_0(t) W_k(s-t). \quad (11.6.13)$$

A systematic way to solve these equations is to Laplace transform in  $s$ , which maps convolution to a product. We will not go through all the details, because the answer can be guessed after a number of easy sample computations.

The average without insertions  $W_0(s)$  coincides with the expectation value of the circular loop (11.3.19), up to a rescaling of the coupling constant:

$$W_0(s) = \frac{4\pi}{s\sqrt{\lambda}} I_1 \left( \frac{s\sqrt{\lambda}}{2\pi} \right), \quad (11.6.14)$$

The Schwinger-Dyson equation (11.6.13) can thus be viewed as a recursion relation that fixes  $W_{k+1}$  in terms of  $W_k$ .

The first step of recursion can be done with the help of the convolution formula for the Bessel functions:

$$\int_0^a \frac{dx}{x(a-x)} I_\mu(c(a-x)) I_\nu(cx) = \frac{\mu + \nu}{a\mu\nu} I_{\mu+\nu}(ca). \quad (11.6.15)$$

For  $W_1$  we then get the Bessel function again, but now with index two. The next iteration boils down to the same convolution formula, which produces  $I_3$ , and so on. It is now easy to guess the general pattern:

$$W_k(s) = \frac{2(k+1)}{is} \left( -\frac{\lambda}{4\pi^2} \right)^{\frac{k-1}{2}} I_{k+1} \left( \frac{s\sqrt{\lambda}}{2\pi} \right). \quad (11.6.16)$$

which can be straightforwardly checked to solve the recursion relations (11.6.13) by virtue of the convolution formula (11.6.15).

Substituting the solution into (11.6.10) we get a remarkably simple result for the OPE coefficient [77]:

$$\mathbb{C}_J^{\text{CPO}} = \sqrt{J} R^J I_J(\sqrt{\lambda}). \quad (11.6.17)$$

This results holds at any  $\lambda$ , and at strong coupling can be compared to the predictions of the AdS/CFT correspondence.

In string theory, a local operator is dual to a closed string state and a Wilson loop to a boundary state. In the most common situation the string dual of a local operator is well

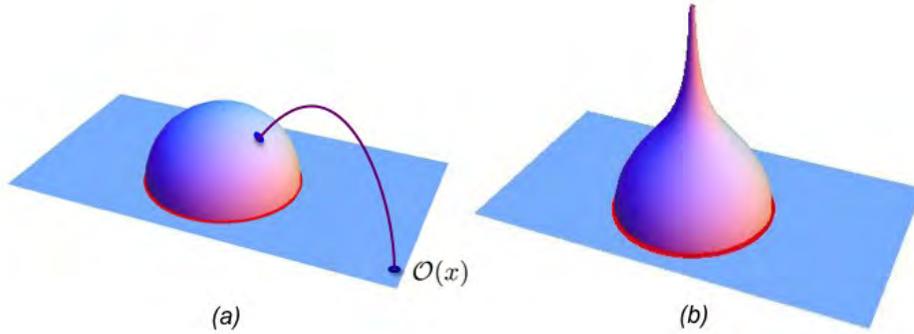

Figure 11.6.3: The correlation function  $\langle W(C)\mathcal{O}(x) \rangle$  in string theory: (a) a bulk-to-boundary propagator stretched between the operator and the string worldsheet, (b) emission of a macroscopic string state (the local operator in this case is inserted at infinity).

approximated by a supergravity field in the bulk. This is certainly true for the chiral primary operators (11.6.4) unless  $J$  is parametrically large. The correlation function  $\langle W(C)\mathcal{O}(x) \rangle$  corresponds then to the following process: the operator insertion at the boundary emits a supergravity mode which is subsequently absorbed by the worldsheet created by the Wilson loop. This is illustrated in fig. 11.6.3a. When the operator is itself dual to a semiclassical string (an example is a CPO with  $J \sim \sqrt{\lambda}$ ), the whole process is described by a single worldsheet as shown in fig. 11.6.3b.

In general, the two-point function  $\langle W(C, \mathbf{n})\mathcal{O}_i(x) \rangle$  (or the OPE coefficient  $\mathbb{C}_i[C, \mathbf{n}]$ , if the operator is placed at infinity) is computed by the string path integral (11.3.21) with a vertex operator inserted. Dividing by the Wilson loop vev to normalize by the disc amplitude without insertions we get:

$$\frac{\mathbb{C}_i[C, \mathbf{n}]}{W(C, \mathbf{n})} = \left\langle \int_{\Sigma} d^2\sigma_o \sqrt{h} V_i(\sigma_o) \right\rangle, \quad (11.6.18)$$

where the vertex operator  $V_i(\sigma_o)$  represents the local operator  $\mathcal{O}_i$  in SYM, and may depend on the string embedding coordinates  $X^M(\sigma_o)$ , their derivatives, worldsheet curvature, fermions and so on.

The one-to-one map  $V_i \longleftrightarrow \mathcal{O}_i$  is a core ingredient of the AdS/CFT duality, and yet it has never been worked out in any detail. Reason for that is a poor knowledge of string theory in  $AdS_5 \times S^5$ . Not many vertex operators are actually known. The chiral primaries (11.6.4) constitute a fortunate exception. The string vertex operators, dual to CPOs, can be calculated from the first principles, by expanding the string action in general supergravity fields around the  $AdS_5 \times S^5$  background [21]:

$$V_J^{\text{CPO}} = \frac{(J+1)\sqrt{J\lambda}}{8\pi N} (n_1 + in_2)^J z^J \left[ \frac{(\partial x)^2 - (\partial z)^2}{z^2} - (\partial \mathbf{n})^2 \right]. \quad (11.6.19)$$

The dependence on  $n_1 + in_2$  and  $z$  is dictated by the quantum numbers of the operator – its R-charge and scaling dimension which are both equal to  $J$ . The normalization of the vertex operator and the structure of the second-derivative terms are dictated by the AdS/CFT dictionary and by the couplings of the supergravity fields to the string worldsheet.

To calculate the OPE coefficient at the leading order in strong coupling it is enough to substitute the classical solution (11.3.27) with constant  $\mathbf{n} = (1, \mathbf{0})$  into the vertex operator (11.6.19) and integrate the latter over the worldsheet. The result of this calculation [21] is

$$\frac{\mathbb{C}_J^{\text{CPO}}}{W(C_{\text{circle}})} \stackrel{\lambda \rightarrow \infty}{=} \frac{(J+1)R^J\sqrt{J\lambda}}{2N} \int_0^\infty d\tau \frac{\tanh^J \tau}{\cosh^2 \tau} = \frac{R^J\sqrt{J\lambda}}{2N}. \quad (11.6.20)$$

Taking into account that the ratio of the Bessel functions approaches one at infinity, we find that the string-theory calculation is in complete agreement with the exact results (11.6.17) and (11.3.19).

Another tractable case is a BMN-like [84] limit in which  $J$  goes to infinity simultaneously with  $\lambda$  at fixed

$$j = \frac{J}{\sqrt{\lambda}}. \quad (11.6.21)$$

The backreaction of the vertex operator cannot be ignored in this case because of its exponential dependence on the large quantum number  $J$ . A heavy vertex operator produces a source in the classical equations of motion of the sigma-model that distorts the shape of the macroscopic string worldsheet [85].

Since the vertex operator (11.6.19) carries an R-charge the string worldsheet will extend in  $S^5$ . In the parameterization  $n_1 + in_2 = \cos \psi e^{i\varphi}$ , the string sitting at  $\psi = 0$  will maximize the weight in the path integral. The string action for the remaining degrees of freedom (in the conformal gauge) takes the form:

$$S_{\text{str}} = \frac{1}{2} \int d^2\sigma \left[ \frac{(\partial x)^2 + (\partial z)^2}{z^2} + (\partial\varphi)^2 \right] - 2\pi j \ln z(\sigma_o) - 2\pi i j \varphi(\sigma_o). \quad (11.6.22)$$

The equations of motion for  $z$  and  $\varphi$  acquire source terms, due to the vertex operator insertion:

$$\begin{aligned} -\partial^2 \varphi &= 2\pi i j \delta(\sigma - \sigma_o) \\ -\partial^2 \ln z - \frac{(\partial x)^2}{z^2} &= 2\pi j \delta(\sigma - \sigma_o) \\ -\partial^a \left( \frac{\partial_a x^\mu}{z^2} \right) &= 0. \end{aligned}$$

The source terms produce singularities at  $\sigma = \sigma_o$ :

$$\varphi \rightarrow -ij \ln |\sigma - \sigma_o|, \quad z \rightarrow \frac{\text{const}}{|\sigma - \sigma_o|^j} \quad (\sigma \rightarrow \sigma_o), \quad (11.6.23)$$

which can be viewed as boundary conditions for the equations of motion. The normalized OPE coefficient is given by the action  $S_{\text{str}}(j)$  evaluated on-shell:

$$\frac{\mathbb{C}_J^{\text{CPO}}}{W(C)} \simeq e^{-\frac{\sqrt{\lambda}}{2\pi}(S_{\text{str}}(j) - S_{\text{str}}(0))}. \quad (11.6.24)$$

The  $z$  and  $\varphi$  parts of the string action (11.6.22) are separately log-divergent at the vertex operator insertion, but the total divergence actually cancels. This is a manifestation of marginality of the vertex operator.

It may seem that the solution is not unique, due to the dependence on the insertion point  $\sigma_o$ . But this is not the case. The insertion point is actually not arbitrary. The solution has to satisfy the Virasoro constraints, and this condition picks a unique  $\sigma_o$ . Alternatively one can start with (11.6.18), where  $\sigma_o$  is an integration variable, and notice that at large  $\lambda$  and  $J$  the integral over  $\sigma_o$  is semiclassical. Then  $\sigma_o$  is determined by the saddle-point conditions. It can be shown that the saddle-point equations on  $\sigma_o$  are equivalent to the Virasoro constraints [86], again due to marginality of the vertex operator.

The solution of the equations of motion for the circular Wilson loop was found in [87] and is most easily written in the exponential parameterization of the disc:  $\sigma_0 + i\sigma_1 = e^{-\tau + is}$ . The vertex operator, for symmetry reasons, should be inserted at  $\sigma = 0$ , or equivalently at  $\tau = \infty$ . Then,

$$\begin{aligned}\varphi &= ij\tau \\ x^1 + ix^2 &= \frac{\sqrt{j^2 + 1} e^{j\tau + is}}{\cosh(\sqrt{j^2 + 1}\tau + \xi)} \\ z &= e^{j\tau} \left[ \sqrt{j^2 + 1} \tanh(\sqrt{j^2 + 1}\tau + \xi) - j \right]\end{aligned}\tag{11.6.25}$$

with

$$\xi = \ln(\sqrt{j^2 + 1} + j).\tag{11.6.26}$$

The solution is shown in fig. 11.6.3b. The worldsheet has the shape of a funnel with an infinite spike that goes up to the horizon. The spike disappears once  $j \rightarrow 0$  and the solution smoothly matches with the minimal surface (11.3.27) for the circular Wilson loop.

The action evaluated on the classical solution gives [87]:

$$\frac{\mathbb{C}_J^{\text{CPO}}}{W(C_{\text{circle}})} \simeq e^{-\sqrt{\lambda} \left[ 1 - \sqrt{j^2 + 1} - j \ln(\sqrt{j^2 + 1} - j) \right]}.\tag{11.6.27}$$

This is to be compared with the exact result (11.6.17) in which  $J$  and  $\lambda$  simultaneously go to infinity. The limit can be derived from the integral representation of the modified Bessel function:

$$I_J(\sqrt{\lambda}) = \frac{\left(\frac{\sqrt{\lambda}}{2}\right)^J}{\sqrt{\pi}\Gamma\left(J + \frac{1}{2}\right)} \int_{-1}^1 dt (1 - t^2)^{J - \frac{1}{2}} e^{\sqrt{\lambda}t}.\tag{11.6.28}$$

For large  $\lambda$  and  $J$  the integral has a saddle point at  $t = \sqrt{j^2 + 1} - j$ , and with exponential accuracy:

$$I_J(\sqrt{\lambda}) \simeq e^{\sqrt{\lambda} \left[ \sqrt{j^2 + 1} + j \ln(\sqrt{j^2 + 1} - j) \right]}.\tag{11.6.29}$$

Normalization by the expectation value of the Wilson (11.3.20) brings this result into the full agreement with the string-theory calculation.

Localization allows one to study much wider class of correlation functions involving Wilson loops of different shape [78, 88], in higher representations of the gauge group [74], 't Hooft loops [74, 89, 90], correlators of two Wilson loops [79–81, 91] as well as multi-point correlation functions [81].

## 11.7 Massive theory

A minimal amount of supersymmetry sufficient to localize a path integral on  $S^4$  is  $\mathcal{N} = 2$  [6]. While  $\mathcal{N} = 4$  SYM is unique, there are many  $\mathcal{N} = 2$  gauge theories and their localization partition functions have qualitatively new features compared to the  $\mathcal{N} = 4$  case. The resulting matrix models are not Gaussian any more, and there is no simple map between Feynman diagrams and the matrix integral<sup>1</sup>. The instantons, that did not contribute to the partition function of  $\mathcal{N} = 4$  SYM, survive localization in generic  $\mathcal{N} = 2$  theories. At large- $N$  the instantons are exponentially suppressed and will actually be neglected in what follows. Finally, and perhaps most interestingly, localization does not rely on conformal symmetry and applies to massive theories as well.

Breaking supersymmetry and introducing a mass scale in holographic duality is conceptually simple. A feature in the bulk (typically a domain wall or a black hole horizon) distance  $z_0 = 1/M$  away from the boundary sets the mass scale  $M$  in the dual gauge theory. Difficulties lie in formulating the holographic dictionary at the string level, which requires the resulting geometry to be a consistent string background. Perhaps the most reliable approach is to start with  $\mathcal{N} = 4$  SYM deformed by a relevant operator. The string dual then is a continuous deformation of  $AdS_5 \times S^5$ . Switching on a relevant perturbation corresponds to imposing boundary conditions and evolving the bulk fields according to the supergravity equations of motion away from the boundary. The only relevant deformation of  $\mathcal{N} = 4$  SYM that preserves  $\mathcal{N} = 2$  supersymmetry is known as the  $\mathcal{N} = 2^*$  theory. The dual supergravity background is known explicitly in this case [94].

The  $\mathcal{N} = 2$  decomposition of the  $\mathcal{N} = 4$  supermultiplet consists of the vector multiplet, containing the gauge fields  $A_\mu$ , two scalars  $\Phi$  and  $\Phi'$  and two Majorana fermions, and two CPT conjugate hypermultiplets, containing two complex scalars  $Z_i$  and a Dirac fermion. The only relevant operator that one can add to the original  $\mathcal{N} = 4$  Lagrangian without breaking  $\mathcal{N} = 2$  supersymmetry is the mass term for the hypermultiplet<sup>2</sup>.

The path integral of the  $\mathcal{N} = 2^*$  theory compactified on  $S^4$  localizes to the following

---

<sup>1</sup>It is interesting, in this respect, to compare explicit perturbative calculations in the  $\mathcal{N} = 2$  superconformal QCD [92] with localization. A three-loop propagator correction, the first diagram that goes beyond the rainbow approximation [92], can be identified in the matrix model [93]. This correction involves a  $\zeta(3)$  transcendentality from the loop integration, while in the matrix model  $\zeta(3)$  appears directly in the action (see [60] for further discussion of transcendental numbers appearing in the localization formulas and their comparison to perturbation theory).

<sup>2</sup>In components, it yields the dimension-2  $\bar{Z}^i Z_i$  mass term, the dimension-3 mass term for the Dirac fermion, the  $\Phi' \varepsilon^{ij} \text{Im}(Z_i Z_j)$  trilinear coupling, which breaks symmetry between  $\Phi$  and  $\Phi'$ , and certain Yukawa couplings.

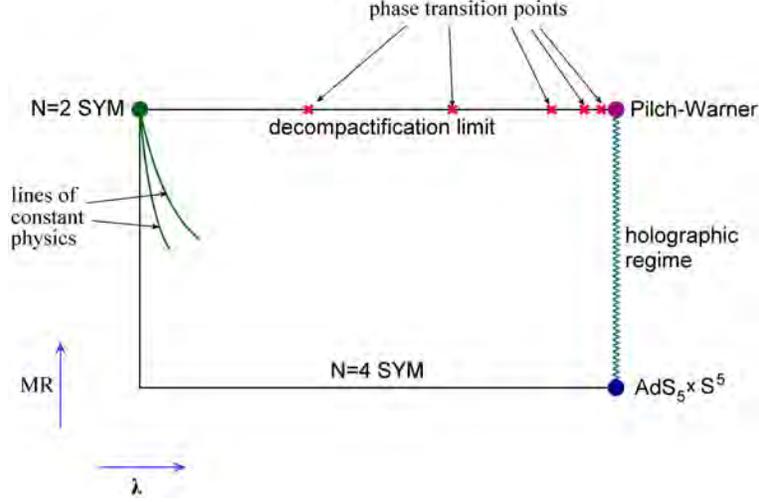

Figure 11.7.1: The phase diagram of  $\mathcal{N} = 2^*$  theory on  $S^4$  (from [95]).

eigenvalue model [6]:

$$Z = \int d^N a \prod_{i < j} \frac{(a_i - a_j)^2 H^2(a_i - a_j)}{H(a_i - a_j + M) H(a_i - a_j - M)} e^{-\frac{8\pi^2 N}{\lambda} \sum_i a_i^2}, \quad (11.7.1)$$

where the function  $H(x)$  is defined by an infinite product

$$H(x) = \prod_{n=1}^{\infty} \left(1 + \frac{x^2}{n^2}\right)^n e^{-\frac{x^2}{n}}. \quad (11.7.2)$$

We have neglected instantons, keeping in mind that they are suppressed in the large- $N$  limit. The integration variables are the eigenvalues of the zero mode of the scalar  $\Phi$ :

$$\Phi = \text{diag}(a_1, \dots, a_N). \quad (11.7.3)$$

The expectation value of the Wilson loop along the big circle of  $S^4$  is given by the same formula (11.3.9), provided the original Wilson loop operator couples exactly to the same scalar. Because the theory at hand is not conformal any more, the circular loop on  $S^4$  cannot be mapped back to  $\mathbb{R}^4$ . The dependence on the radius  $R$  of  $S^4$  also does not scale away. For brevity we have set  $R = 1$ , so dimensionful quantities such as  $M$ ,  $\Phi$  and  $a_i$  should be understood as  $MR$ ,  $\Phi R$  and  $a_i R$ .

The saddle-point equations for the eigenvalue model (11.7.1) are

$$\frac{1}{N} \sum_{j \neq i} \left( \frac{1}{a_i - a_j} - \mathcal{K}(a_i - a_j) + \frac{1}{2} \mathcal{K}(a_i - a_j + M) + \frac{1}{2} \mathcal{K}(a_i - a_j - M) \right) = \frac{8\pi^2}{\lambda} a_i, \quad (11.7.4)$$

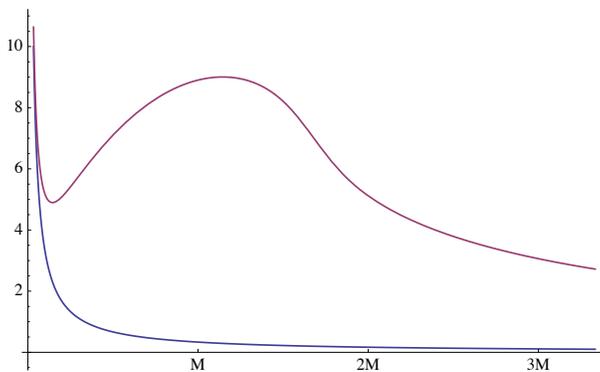

Figure 11.7.2: The two-body force acting between the eigenvalues in the  $\mathcal{N} = 2^*$  localization matrix model for  $M = 3$  (upper curve) and in the Gaussian model (lower curve).

where

$$\mathcal{K}(x) = -\frac{H'(x)}{H(x)}. \quad (11.7.5)$$

These equations were studied in [95–101], and although their general solution is not known, the phase diagram in the  $(M, \lambda)$  plane can be mapped in a fair amount of detail, and turns out to be rather non-trivial, fig. 11.7.1.

When  $M \rightarrow \infty$  and  $\lambda \rightarrow 0$  simultaneously, the hypermultiplets can be integrated out leaving behind pure  $\mathcal{N} = 2$  SYM. The mass scale  $M$  plays the rôle of a UV cutoff in the low-energy theory, while  $\lambda$  is identified with the bare coupling. The beta-function of the  $\mathcal{N} = 2$  SYM then generates a dynamical scale  $\Lambda = M e^{-4\pi^2/\lambda}$  (green lines in fig. 11.7.1 are the lines of constant  $\Lambda$ ). The saddle-point equations of the localization matrix model reproduce [97] in this corner of the phase diagram the large- $N$  solution of  $\mathcal{N} = 2$  SYM, known from the Seiberg-Witten theory [102, 103].

The one-body potential in the  $\mathcal{N} = 2^*$  matrix model is still Gaussian, while the two-body potential gets modified by the mass deformation. The two-body force between eigenvalues has a rather intricate shape (fig. 11.7.2). Remaining universally repulsive, it does not decrease with distance as fast as in the Gaussian model, and can compete with the attractive one-body potential. This competition causes an infinite sequence of quantum phase transitions in the decompactification limit  $R \rightarrow \infty$  (which in the dimensionless variables that we use corresponds to  $M \rightarrow \infty$ ) [99]<sup>3</sup>. Physically the phase transitions arise because of the resonances on nearly massless hypermultiplets. Indeed, the masses of the hypermultiplet fields in the Higgs background (11.7.3) are  $m_{ij}^h = |a_i - a_j \pm M|$  and can become small if the distance between a pair of eigenvalues gets close to  $M$ .

Since we mainly focus on an interplay between localization and holography, we are

<sup>3</sup>The phase transitions happen at  $\lambda_c^{(1)} = 35.42\dots$ ,  $\lambda_c^{(2)} = 84.6 \pm 1.0$ ,  $\lambda_c^{(3)} = 153.0 \pm 0.7$ , and asymptotically at  $\lambda_c^{(n)} \simeq \pi^2 n^2$ . The first critical coupling is known exactly [99]. The numerical results for secondary transitions improve on estimates of [99] and are obtained with the help of the formalism developed in [101].

interested in the strong-coupling limit of  $\mathcal{N} = 2^*$  SYM [98, 100, 101]. Drawing intuition from the solution of the Gaussian model (11.3.16), (11.3.17), we may assume that the width of the eigenvalue distribution grows with  $\lambda$  and will be much larger than any other scale in the problem at strong coupling. This is certainly true for small  $M$ , and will be checked *a posteriori* for arbitrary  $M$ . Treating  $M$  as a small parameter, and using the large-distance asymptotics of the function  $\mathcal{K}(x)$ , we find:

$$\frac{1}{2}\mathcal{K}(x+M) + \frac{1}{2}\mathcal{K}(x-M) - \mathcal{K}(x) \approx M^2\mathcal{K}''(x) \approx \frac{M^2}{x}$$

Hence only the tail of the two-body force in fig. 11.7.2 is important at strong coupling, and its sole effect is to renormalize the  $1/x$  interaction of the Gaussian model. The saddle-point distribution then obeys the Wigner law (11.3.16) with [98]

$$\mu = \frac{\sqrt{\lambda\left(M^2 + \frac{1}{R^2}\right)}}{2\pi}. \quad (11.7.6)$$

We have re-instated the dependence on  $R$  and the canonical mass dimension of  $\mu$  and  $M$ . When  $M=0$ , there are no dimensionful parameters in the problem and  $\mu$  scales away as  $1/R$ , while in the  $\mathcal{N} = 2^*$  theory it freezes at the scale that is parametrically larger than the bare mass in the Lagrangian, in accord with our original assumption.

The strong-coupling asymptotics of the circular Wilson loop is governed by the largest eigenvalue:  $W(C_{\text{circle}}) \simeq e^{\sqrt{\lambda}MR}$ . Although we cannot calculate any Wilson loop apart from the circle, it is natural to assume that expectation values for sufficiently large loops are universal, and hence should obey perimeter law with the coefficient fixed by localization:

$$W(C) \simeq e^{\frac{\sqrt{\lambda}}{2\pi}L(C)}. \quad (11.7.7)$$

This prediction can be checked using the explicit form of the dual supergravity background [98]. The relevant part of the metric is [94]

$$ds^2 = \frac{AM^2}{c^2-1} dx_\mu^2 + \frac{1}{A(c^2-1)^2} dc^2, \quad A = c + \frac{c^2-1}{2} \ln \frac{c-1}{c+1}. \quad (11.7.8)$$

The holographic coordinate  $c$  is related to  $z$  in (11.2.4) by

$$c = 1 + \frac{z^2 M^2}{2} + \dots \quad (11.7.9)$$

so the boundary is at  $c = 1$ . One can check that near the boundary the metric indeed asymptotes to that of  $AdS_5$ .

The minimal surface for a sufficiently big contour is approximately a cylinder, repeating the shape of the Wilson loop for any  $c$ , as long as  $c \ll ML$ . Because the metric decreases with  $c$  very fast, most part of the area will come from this region, and we can neglect the bending and eventual closure of the minimal surface in computing the area:

$$A_{\text{min}}(C) = ML \int_{1+\frac{M^2\varepsilon^2}{2}}^{\infty} \frac{dc}{(c^2-1)^{\frac{3}{2}}} = \frac{L}{\varepsilon} - ML. \quad (11.7.10)$$

The divergent term is subtracted by regularization and, taking into account that the dimensionless string tension must be the same as in  $AdS_5 \times S^5$ ,  $T = \sqrt{\lambda}/2\pi$ , we get perimeter law with exactly the same coefficient (11.7.7) as inferred from localization.

As shown in [104] the free energy of the matrix model agrees with the on-shell action of the supergravity on the solution that has  $S^4$  as a boundary. Corrections in  $1/\sqrt{\lambda}$  to the leading-order strong-coupling result (11.7.6) have been calculated on the matrix model side [100, 101], and it would be very interesting to compare them to quantum corrections due to string fluctuations in the bulk.

## 11.8 Conclusions

Localization is a powerful tool to explore supersymmetric gauge theories in the non-perturbative domain. Although limited to a restricted class of observables, localization relies on a direct evaluation of the path integral, without recourse to any assumptions or uncontrollable approximations. Via holography these first-principle calculations can be confronted with string theory and can give us additional hints on how string description emerges from summing planar diagrams.

Localization predictions are sometimes rather detailed. This review focusses on just a few examples, and in particular leaves aside theories for which a holographic dual is not really well established or has no weakly coupled regime. One interesting example of this class is  $\mathcal{N} = 2$  superconformal QCD – an  $\mathcal{N} = 2$  supersymmetric gauge theory with  $N_f = 2N_c$  fundamental hypermultiplets. This theory has zero beta-function, and is presumably dual to strings on  $AdS_5 \times X_5$ , where  $X_5$  may not be geometric (see [105] for a concrete proposal). The strong-coupling solution of the matrix model for  $\mathcal{N} = 2$  super-QCD is very different from the  $\mathcal{N} = 4$  and  $\mathcal{N} = 2^*$  cases [93]. Potential implications of this result for holography have not been worked out so far. Another class of examples are two-dimensional theories with  $\mathcal{N} = 4$  supersymmetry, which are dual to strings on  $AdS_3 \times S^3 \times T^4$  supported by the RR flux. Here on the contrary the planar diagram expansion on the gauge-theory side is not easy to develop (see [106] and [107] for two different proposals). Localization on  $S^2$  [108, 109] (see Chapter 3) may be very useful in this respect, and it would be interesting to solve the resulting matrix model at large- $N$ .

An interplay between holography and localization has been studied in much detail in three dimensions (see [7] for a review), and in dimensions higher than four [110–114]. It is also possible to localize on manifolds different from  $S^4$  (see Chapter 10), which has a number of interesting applications to holography. Entanglement entropy of a spherical region can be computed that way [115, 116] and compared to the Ryu-Takayanagi prescription [117] at strong coupling. Bremsstahlung function in generic  $\mathcal{N} = 2$  theories can be also extracted from localization [58]. Localization of  $\mathcal{N} = 4$  SYM on a large class of manifolds of the form  $S^1 \times M_3$  [118] yields supersymmetric indices that can be compared [119] to the supergravity action on geometries found in [120].

## Acknowledgements

I would like to thank X. Chen-Lin, A. Dekel, N. Drukker, J. Gordon, D. Medina Rincon, J. Russo and G. Semenoff for many useful discussions on localization, AdS/CFT correspondence, and matrix models. This work was supported by the Marie Curie network GATIS of the European Union's FP7 Programme under REA Grant Agreement No 317089, by the ERC advanced grant No 341222, by the Swedish Research Council (VR) grant 2013-4329, and by RFBR grant 15-01-99504.

## References

- [1] V. Pestun and M. Zabzine, eds., *Localization techniques in quantum field theory*, vol. xx. Journal of Physics A, 2016. [1608.02952](https://arxiv.org/src/1608.02952/anc/LocQFT.pdf). <https://arxiv.org/src/1608.02952/anc/LocQFT.pdf>, <http://pestun.ihep.fr/pages/LocalizationReview/LocQFT.pdf>.
- [2] J. M. Maldacena, “*The large  $N$  limit of superconformal field theories and supergravity*”, *Adv. Theor. Math. Phys.* 2, 231 (1998), [hep-th/9711200](https://arxiv.org/abs/hep-th/9711200).
- [3] S. S. Gubser, I. R. Klebanov and A. M. Polyakov, “*Gauge theory correlators from non-critical string theory*”, *Phys. Lett.* B428, 105 (1998), [hep-th/9802109](https://arxiv.org/abs/hep-th/9802109).
- [4] E. Witten, “*Anti-de Sitter space and holography*”, *Adv. Theor. Math. Phys.* 2, 253 (1998), [hep-th/9802150](https://arxiv.org/abs/hep-th/9802150).
- [5] G. 't Hooft, “*A Planar Diagram Theory for Strong Interactions*”, *Nucl.Phys.* B72, 461 (1974).
- [6] V. Pestun, “*Localization of gauge theory on a four-sphere and supersymmetric Wilson loops*”, *Commun.Math.Phys.* 313, 71 (2012), [0712.2824](https://arxiv.org/abs/0712.2824).
- [7] M. Marino, “*Lectures on localization and matrix models in supersymmetric Chern-Simons-matter theories*”, *J.Phys.A* A44, 463001 (2011), [1104.0783](https://arxiv.org/abs/1104.0783).
- [8] J. G. Russo and K. Zarembo, “*Localization at Large  $N$* ”, [1312.1214](https://arxiv.org/abs/1312.1214).
- [9] G. W. Semenoff and K. Zarembo, “*Wilson loops in SYM theory: From weak to strong coupling*”, *Nucl.Phys.Proc.Suppl.* 108, 106 (2002), [hep-th/0202156](https://arxiv.org/abs/hep-th/0202156).
- [10] F. Gliozzi, J. Scherk and D. I. Olive, “*Supersymmetry, Supergravity Theories and the Dual Spinor Model*”, *Nucl. Phys.* B122, 253 (1977).
- [11] L. Brink, J. H. Schwarz and J. Scherk, “*Supersymmetric Yang-Mills Theories*”, *Nucl.Phys.* B121, 77 (1977).
- [12] J. M. Maldacena, “*Wilson loops in large  $N$  field theories*”, *Phys. Rev. Lett.* 80, 4859 (1998), [hep-th/9803002](https://arxiv.org/abs/hep-th/9803002).
- [13] K. Zarembo, “*Supersymmetric Wilson loops*”, *Nucl. Phys.* B643, 157 (2002), [hep-th/0205160](https://arxiv.org/abs/hep-th/0205160).
- [14] A. Dymarsky and V. Pestun, “*Supersymmetric Wilson loops in  $N=4$  SYM and pure spinors*”, *JHEP* 1004, 115 (2010), [0911.1841](https://arxiv.org/abs/0911.1841).
- [15] J. K. Erickson, G. W. Semenoff and K. Zarembo, “*Wilson loops in  $N = 4$  supersymmetric Yang-Mills theory*”, *Nucl. Phys.* B582, 155 (2000), [hep-th/0003055](https://arxiv.org/abs/hep-th/0003055).
- [16] N. Drukker and D. J. Gross, “*An exact prediction of  $N = 4$  SUSYM theory for string theory*”, *J. Math. Phys.* 42, 2896 (2001), [hep-th/0010274](https://arxiv.org/abs/hep-th/0010274).
- [17] E. Brezin, C. Itzykson, G. Parisi and J. B. Zuber, “*Planar Diagrams*”, *Commun. Math. Phys.* 59, 35 (1978).
- [18] F. Gakhov, “*Boundary value problems*”, Dover Publications (1990).

- [19] S.-J. Rey and J.-T. Yee, “*Macroscopic strings as heavy quarks in large  $N$  gauge theory and anti-de Sitter supergravity*”, Eur. Phys. J. C22, 379 (2001), [hep-th/9803001](#).
- [20] R. R. Metsaev and A. A. Tseytlin, “*Type IIB superstring action in  $AdS_5 \times S^5$  background*”, Nucl. Phys. B533, 109 (1998), [hep-th/9805028](#).
- [21] D. E. Berenstein, R. Corrado, W. Fischler and J. M. Maldacena, “*The operator product expansion for Wilson loops and surfaces in the large  $N$  limit*”, Phys. Rev. D59, 105023 (1999), [hep-th/9809188](#).
- [22] N. Drukker, D. J. Gross and H. Ooguri, “*Wilson loops and minimal surfaces*”, Phys. Rev. D60, 125006 (1999), [hep-th/9904191](#).
- [23] M. Kruczenski and A. Tirziu, “*Matching the circular Wilson loop with dual open string solution at 1-loop in strong coupling*”, JHEP 0805, 064 (2008), [0803.0315](#).
- [24] C. Kristjansen and Y. Makeenko, “*More about One-Loop Effective Action of Open Superstring in  $AdS_5 \times S^5$* ”, JHEP 1209, 053 (2012), [1206.5660](#).
- [25] R. Bergamin and A. A. Tseytlin, “*Heat kernels on cone of  $AdS_2$  and  $k$ -wound circular Wilson loop in  $AdS_5 \times S^5$  superstring*”, J. Phys. A49, 14LT01 (2016), [1510.06894](#).
- [26] V. Forini, V. Giangreco, M. Puletti, L. Griguolo, D. Seminara and E. Vescovi, “*Precision calculation of 1/4-BPS Wilson loops in  $AdS_5 \times S^5$* ”, JHEP 1602, 105 (2016), [1512.00841](#).
- [27] A. Faraggi, L. A. Pando Zayas, G. A. Silva and D. Trancanelli, “*Toward precision holography with supersymmetric Wilson loops*”, JHEP 1604, 053 (2016), [1601.04708](#).
- [28] N. Drukker, “*1/4 BPS circular loops, unstable world-sheet instantons and the matrix model*”, JHEP 0609, 004 (2006), [hep-th/0605151](#).
- [29] N. Drukker and B. Fiol, “*All-genus calculation of Wilson loops using D-branes*”, JHEP 0502, 010 (2005), [hep-th/0501109](#).
- [30] T. Okuda and D. Trancanelli, “*Spectral curves, emergent geometry, and bubbling solutions for Wilson loops*”, JHEP 0809, 050 (2008), [0806.4191](#).
- [31] B. Fiol and G. Torrents, “*Exact results for Wilson loops in arbitrary representations*”, JHEP 1401, 020 (2014), [1311.2058](#).
- [32] S. A. Hartnoll and S. P. Kumar, “*Higher rank Wilson loops from a matrix model*”, JHEP 0608, 026 (2006), [hep-th/0605027](#).
- [33] S. Yamaguchi, “*Wilson loops of anti-symmetric representation and D5-branes*”, JHEP 0605, 037 (2006), [hep-th/0603208](#).
- [34] M. Horikoshi and K. Okuyama, “ *$\alpha'$ -expansion of Anti-Symmetric Wilson Loops in  $\mathcal{N} = 4$  SYM from Fermi Gas*”, [1607.01498](#).
- [35] G. Grignani, J. L. Karczmarek and G. W. Semenoff, “*Hot Giant Loop Holography*”, Phys.Rev. D82, 027901 (2010), [0904.3750](#).
- [36] X. Chen-Lin and K. Zarembo, “*Higher Rank Wilson Loops in  $N = 2^*$  Super-Yang-Mills Theory*”, JHEP 1503, 147 (2015), [1502.01942](#).
- [37] J. Gomis and F. Passerini, “*Holographic Wilson loops*”, JHEP 0608, 074 (2006), [hep-th/0604007](#).
- [38] D. Rodriguez-Gomez, “*Computing Wilson lines with dielectric branes*”, Nucl.Phys. B752, 316 (2006), [hep-th/0604031](#).
- [39] J. Gomis and F. Passerini, “*Wilson loops as D3-branes*”, JHEP 0701, 097 (2007), [hep-th/0612022](#).
- [40] S. Yamaguchi, “*Semi-classical open string corrections and symmetric Wilson loops*”, JHEP 0706, 073 (2007), [hep-th/0701052](#).

- [41] B. Fiol, A. Güijosa and J. F. Pedraza, “*Branes from Light: Embeddings and Energetics for Symmetric  $k$ -Quarks in  $\mathcal{N} = 4$  SYM*”, JHEP 1501, 149 (2015), [1410.0692](#).
- [42] J. Polchinski, “*String theory*”, Cambridge University Press (1998), Cambridge, UK New York.
- [43] A. Faraggi, W. Mueck and L. A. Pando Zayas, “*One-loop Effective Action of the Holographic Antisymmetric Wilson Loop*”, Phys. Rev. D85, 106015 (2012), [1112.5028](#).
- [44] A. Faraggi, J. T. Liu, L. A. Pando Zayas and G. Zhang, “*One-loop structure of higher rank Wilson loops in AdS/CFT*”, Phys.Lett. B740, 218 (2015), [1409.3187](#).
- [45] E. Buchbinder and A. Tseytlin, “*The  $1/N$  correction in the D3-brane description of circular Wilson loop at strong coupling*”, Phys.Rev. D89, 126008 (2014), [1404.4952](#).
- [46] D. Correa, J. Henn, J. Maldacena and A. Sever, “*An exact formula for the radiation of a moving quark in  $N=4$  super Yang Mills*”, JHEP 1206, 048 (2012), [1202.4455](#).
- [47] A. M. Polyakov and V. S. Rychkov, “*Gauge fields - strings duality and the loop equation*”, Nucl. Phys. B581, 116 (2000), [hep-th/0002106](#).
- [48] G. W. Semenoff and D. Young, “*Wavy Wilson line and AdS/CFT*”, Int. J. Mod. Phys. A20, 2833 (2005), [hep-th/0405288](#).
- [49] A. M. Polyakov, “*Gauge Fields as Rings of Glue*”, Nucl. Phys. B164, 171 (1980).
- [50] G. P. Korchemsky and G. Marchesini, “*Structure function for large  $x$  and renormalization of Wilson loop*”, Nucl. Phys. B406, 225 (1993), [hep-ph/9210281](#).
- [51] Y. Makeenko, P. Olesen and G. W. Semenoff, “*Cusped SYM Wilson loop at two loops and beyond*”, Nucl.Phys. B748, 170 (2006), [hep-th/0602100](#).
- [52] N. Drukker and V. Forini, “*Generalized quark-antiquark potential at weak and strong coupling*”, JHEP 1106, 131 (2011), [1105.5144](#).
- [53] D. Correa, J. Henn, J. Maldacena and A. Sever, “*The cusp anomalous dimension at three loops and beyond*”, JHEP 1205, 098 (2012), [1203.1019](#).
- [54] J. M. Henn and T. Huber, “*The four-loop cusp anomalous dimension in  $\mathcal{N} = 4$  super Yang-Mills and analytic integration techniques for Wilson line integrals*”, JHEP 1309, 147 (2013), [1304.6418](#).
- [55] N. Drukker, S. Giombi, R. Ricci and D. Trancanelli, “*Supersymmetric Wilson loops on  $S^3$* ”, JHEP 0805, 017 (2008), [0711.3226](#).
- [56] B. Fiol, B. Garolera and A. Lewkowycz, “*Exact results for static and radiative fields of a quark in  $N=4$  super Yang-Mills*”, JHEP 1205, 093 (2012), [1202.5292](#).
- [57] A. Lewkowycz and J. Maldacena, “*Exact results for the entanglement entropy and the energy radiated by a quark*”, JHEP 1405, 025 (2014), [1312.5682](#).
- [58] B. Fiol, E. Gerchkovitz and Z. Komargodski, “*The Exact Bremsstrahlung Function in  $N=2$  Superconformal Field Theories*”, Phys. Rev. Lett. 116, 081601 (2016), [1510.01332](#).
- [59] B. Fiol, B. Garolera and G. Torrents, “*Probing  $\mathcal{N} = 2$  superconformal field theories with localization*”, JHEP 1601, 168 (2016), [1511.00616](#).
- [60] V. Mitev and E. Pomoni, “*Exact Bremsstrahlung and Effective Couplings*”, JHEP 1606, 078 (2016), [1511.02217](#).
- [61] V. Pestun, “*Localization of the four-dimensional  $N=4$  SYM to a two-sphere and  $1/8$  BPS Wilson loops*”, JHEP 1212, 067 (2012), [0906.0638](#).
- [62] N. Drukker and B. Fiol, “*On the integrability of Wilson loops in  $AdS_5 \times S^5$ : Some periodic ansatze*”, JHEP 0601, 056 (2006), [hep-th/0506058](#).

- [63] A. Mikhailov, “Nonlinear waves in AdS / CFT correspondence”, [hep-th/0305196](#).
- [64] P. Banerjee and B. Sathiapalan, “Zero Temperature Dissipation and Holography”, JHEP 1604, 089 (2016), [1512.06414](#).
- [65] N. Beisert, B. Eden and M. Staudacher, “Transcendentality and crossing”, J. Stat. Mech. 0701, P021 (2007), [hep-th/0610251](#).
- [66] N. Drukker, “Integrable Wilson loops”, JHEP 1310, 135 (2013), [1203.1617](#).
- [67] D. Correa, J. Maldacena and A. Sever, “The quark anti-quark potential and the cusp anomalous dimension from a TBA equation”, JHEP 1208, 134 (2012), [1203.1913](#).
- [68] N. Gromov and F. Levkovich-Maslyuk, “Quantum Spectral Curve for a Cusped Wilson Line in  $N=4$  SYM”, JHEP 1604, 134 (2016), [1510.02098](#).
- [69] N. Gromov and F. Levkovich-Maslyuk, “Quark–anti-quark potential in  $N=4$  SYM”, [1601.05679](#).
- [70] N. Gromov and A. Sever, “Analytic Solution of Bremsstrahlung TBA”, JHEP 1211, 075 (2012), [1207.5489](#).
- [71] N. Drukker, S. Giombi, R. Ricci and D. Trancanelli, “More supersymmetric Wilson loops”, Phys. Rev. D76, 107703 (2007), [0704.2237](#).
- [72] N. Drukker, S. Giombi, R. Ricci and D. Trancanelli, “Wilson loops: From four-dimensional SYM to two-dimensional YM”, Phys. Rev. D77, 047901 (2008), [0707.2699](#).
- [73] M. A. Shifman, “Wilson Loop in Vacuum Fields”, Nucl. Phys. B173, 13 (1980).
- [74] J. Gomis, S. Matsuura, T. Okuda and D. Trancanelli, “Wilson loop correlators at strong coupling: from matrices to bubbling geometries”, JHEP 0808, 068 (2008), [0807.3330](#).
- [75] L. F. Alday and A. A. Tseytlin, “On strong-coupling correlation functions of circular Wilson loops and local operators”, J. Phys. A44, 395401 (2011), [1105.1537](#).
- [76] E. I. Buchbinder and A. A. Tseytlin, “Correlation function of circular Wilson loop with two local operators and conformal invariance”, Phys. Rev. D87, 026006 (2013), [1208.5138](#).
- [77] G. W. Semenoff and K. Zarembo, “More exact predictions of SUSYM for string theory”, Nucl. Phys. B616, 34 (2001), [hep-th/0106015](#).
- [78] S. Giombi and V. Pestun, “Correlators of local operators and  $1/8$  BPS Wilson loops on  $S^2$  from 2d YM and matrix models”, JHEP 1010, 033 (2010), [0906.1572](#).
- [79] S. Giombi, V. Pestun and R. Ricci, “Notes on supersymmetric Wilson loops on a two-sphere”, JHEP 1007, 088 (2010), [0905.0665](#).
- [80] A. Bassetto, L. Griguolo, F. Pucci, D. Seminara, S. Thambyahpillai and D. Young, “Correlators of supersymmetric Wilson-loops, protected operators and matrix models in  $N=4$  SYM”, JHEP 0908, 061 (2009), [0905.1943](#).
- [81] S. Giombi and V. Pestun, “Correlators of Wilson Loops and Local Operators from Multi-Matrix Models and Strings in AdS”, JHEP 1301, 101 (2013), [1207.7083](#).
- [82] A. A. Migdal, “Loop Equations and  $1/N$  Expansion”, Phys. Rept. 102, 199 (1983).
- [83] Yu. Makeenko, “Loop equations in matrix models and in 2-D quantum gravity”, Mod. Phys. Lett. A6, 1901 (1991).
- [84] D. E. Berenstein, J. M. Maldacena and H. S. Nastase, “Strings in flat space and pp waves from  $N = 4$  super Yang Mills”, JHEP 0204, 013 (2002), [hep-th/0202021](#).
- [85] A. Polyakov, “Talk at Strings 2002”, [www.damtp.cam.ac.uk/strings02/avt/polyakov/](http://www.damtp.cam.ac.uk/strings02/avt/polyakov/).

- [86] K. Zarembo, “Holographic three-point functions of semiclassical states”, JHEP 1009, 030 (2010), [1008.1059](#).
- [87] K. Zarembo, “Open string fluctuations in  $AdS_5 \times S^5$  and operators with large  $R$  charge”, Phys. Rev. D66, 105021 (2002), [hep-th/0209095](#).
- [88] T. Enari and A. Miwa, “Semi-classical correlator for  $1/4$  BPS Wilson loop and chiral primary operator with large  $R$ -charge”, Phys. Rev. D86, 106004 (2012), [1208.0821](#).
- [89] S. Giombi and V. Pestun, “The  $1/2$  BPS ’t Hooft loops in  $N=4$  SYM as instantons in 2d Yang-Mills”, J. Phys. A46, 095402 (2013), [0909.4272](#).
- [90] A. Bassetto and S. Thambyahpillai, “Quantum ’t Hooft loops of SYM  $N=4$  as instantons of YM<sub>2</sub> in dual groups  $SU(N)$  and  $SU(N)/Z_N$ ”, Lett. Math. Phys. 98, 97 (2011), [1011.0638](#).
- [91] A. Bassetto, L. Griguolo, F. Pucci, D. Seminara, S. Thambyahpillai and D. Young, “Correlators of supersymmetric Wilson loops at weak and strong coupling”, JHEP 1003, 038 (2010), [0912.5440](#).
- [92] R. Andree and D. Young, “Wilson Loops in  $N=2$  Superconformal Yang-Mills Theory”, JHEP 1009, 095 (2010), [1007.4923](#).
- [93] F. Passerini and K. Zarembo, “Wilson Loops in  $N=2$  Super-Yang-Mills from Matrix Model”, JHEP 1109, 102 (2011), [1106.5763](#).
- [94] K. Pilch and N. P. Warner, “ $N=2$  supersymmetric RG flows and the IIB dilaton”, Nucl.Phys. B594, 209 (2001), [hep-th/0004063](#).
- [95] J. Russo and K. Zarembo, “Massive  $N=2$  Gauge Theories at Large  $N$ ”, JHEP 1311, 130 (2013), [1309.1004](#).
- [96] J. G. Russo, “A Note on perturbation series in supersymmetric gauge theories”, JHEP 1206, 038 (2012), [1203.5061](#).
- [97] J. Russo and K. Zarembo, “Large  $N$  Limit of  $N=2$   $SU(N)$  Gauge Theories from Localization”, JHEP 1210, 082 (2012), [1207.3806](#).
- [98] A. Buchel, J. G. Russo and K. Zarembo, “Rigorous Test of Non-conformal Holography: Wilson Loops in  $N=2^*$  Theory”, JHEP 1303, 062 (2013), [1301.1597](#).
- [99] J. G. Russo and K. Zarembo, “Evidence for Large- $N$  Phase Transitions in  $N=2^*$  Theory”, JHEP 1304, 065 (2013), [1302.6968](#).
- [100] X. Chen-Lin, J. Gordon and K. Zarembo, “ $\mathcal{N} = 2^*$  super-Yang-Mills theory at strong coupling”, JHEP 1411, 057 (2014), [1408.6040](#).
- [101] K. Zarembo, “Strong-Coupling Phases of Planar  $N=2^*$  Super-Yang-Mills Theory”, Theor.Math.Phys. 181, 1522 (2014), [1410.6114](#).
- [102] M. R. Douglas and S. H. Shenker, “Dynamics of  $SU(N)$  supersymmetric gauge theory”, Nucl.Phys. B447, 271 (1995), [hep-th/9503163](#).
- [103] F. Ferrari, “The Large  $N$  limit of  $N=2$  superYang-Mills, fractional instantons and infrared divergences”, Nucl.Phys. B612, 151 (2001), [hep-th/0106192](#).
- [104] N. Bobev, H. Elvang, D. Z. Freedman and S. S. Pufu, “Holography for  $N = 2^*$  on  $S^4$ ”, JHEP 1407, 001 (2014), [1311.1508](#).
- [105] A. Gadde, E. Pomoni and L. Rastelli, “The Veneziano Limit of  $N = 2$  Superconformal QCD: Towards the String Dual of  $N = 2$   $SU(N_c)$  SYM with  $N_f = 2N_c$ ”, [0912.4918](#).
- [106] A. Pakman, L. Rastelli and S. S. Razamat, “Diagrams for Symmetric Product Orbifolds”, JHEP 0910, 034 (2009), [0905.3448](#).

- [107] O. O. Sax, A. Sfondrini and B. Stefanski, “*Integrability and the Conformal Field Theory of the Higgs branch*”, JHEP 1506, 103 (2015), [1411.3676](#).
- [108] F. Benini and S. Cremonesi, “*Partition Functions of  $\mathcal{N} = (2, 2)$  Gauge Theories on  $S^2$  and Vortices*”, Commun. Math. Phys. 334, 1483 (2015), [1206.2356](#).
- [109] N. Doroud, J. Gomis, B. Le Floch and S. Lee, “*Exact Results in D=2 Supersymmetric Gauge Theories*”, JHEP 1305, 093 (2013), [1206.2606](#).
- [110] J. Kallen, J. A. Minahan, A. Nedelin and M. Zabzine, “ *$N^3$ -behavior from 5D Yang-Mills theory*”, JHEP 1210, 184 (2012), [1207.3763](#).
- [111] D. L. Jafferis and S. S. Pufu, “*Exact results for five-dimensional superconformal field theories with gravity duals*”, JHEP 1405, 032 (2014), [1207.4359](#).
- [112] J. A. Minahan, A. Nedelin and M. Zabzine, “*5D super Yang-Mills theory and the correspondence to  $AdS_7/CFT_6$* ”, J.Phys. A46, 355401 (2013), [1304.1016](#).
- [113] J. A. Minahan and M. Zabzine, “*Gauge theories with 16 supersymmetries on spheres*”, JHEP 1503, 155 (2015), [1502.07154](#).
- [114] J. A. Minahan, “*Localizing gauge theories on  $S^d$* ”, JHEP 1604, 152 (2016), [1512.06924](#).
- [115] X. Huang and Y. Zhou, “ *$\mathcal{N} = 4$  Super-Yang-Mills on conic space as hologram of STU topological black hole*”, JHEP 1502, 068 (2015), [1408.3393](#).
- [116] M. Crossley, E. Dyer and J. Sonner, “*Super-Renyi entropy & Wilson loops for  $\mathcal{N} = 4$  SYM and their gravity duals*”, JHEP 1412, 001 (2014), [1409.0542](#).
- [117] S. Ryu and T. Takayanagi, “*Holographic derivation of entanglement entropy from AdS/CFT*”, Phys. Rev. Lett. 96, 181602 (2006), [hep-th/0603001](#).
- [118] B. Assel, D. Cassani and D. Martelli, “*Localization on Hopf surfaces*”, JHEP 1408, 123 (2014), [1405.5144](#).
- [119] P. B. Genolini, D. Cassani, D. Martelli and J. Sparks, “*The holographic supersymmetric Casimir energy*”, [1606.02724](#).
- [120] D. Cassani and D. Martelli, “*The gravity dual of supersymmetric gauge theories on a squashed  $S^1 \times S^3$* ”, JHEP 1408, 044 (2014), [1402.2278](#).

# Chapter 12

## A brief review of the 2d/4d correspondences

Yuji Tachikawa

*Kavli Institute for the Physics and Mathematics of the Universe,  
University of Tokyo, Kashiwa, Chiba 277-8583, Japan*  
yuji.tachikawa@ipmu.jp

### Abstract

An elementary introduction to the 2d/4d correspondences is given. After quickly reviewing the 2d  $q$ -deformed Yang-Mills theory and the Liouville theory, we will introduce 4d theories obtained by coupling trifundamentals to  $SU(2)$  gauge fields. We will then see concretely that the supersymmetric partition function of these theories on  $S^3 \times S^1$  and on  $S^4$  is given respectively by the  $q$ -deformed Yang-Mills theory and the Liouville theory. After giving a short discussion on how this correspondence may be understood from the viewpoint of the 6d  $\mathcal{N} = (2, 0)$  theory, we conclude the review by enumerating future directions. Most of the technical points will be referred to more detailed review articles.

### Contents

|                                                      |            |
|------------------------------------------------------|------------|
| <b>12.1 Introduction</b>                             | <b>476</b> |
| <b>12.2 Two two-dimensional theories</b>             | <b>477</b> |
| 12.2.1 Two-dimensional Yang-Mills theories           | 477        |
| 12.2.2 The Liouville theory                          | 483        |
| <b>12.3 A class of four-dimensional theories</b>     | <b>489</b> |
| 12.3.1 $\mathcal{N}=2$ supersymmetric gauge theories | 490        |
| 12.3.2 Class S theories of type $SU(2)$              | 491        |
| <b>12.4 Two supersymmetric backgrounds</b>           | <b>494</b> |
| 12.4.1 General yoga of supersymmetric localization   | 494        |

|                   |                                                      |            |
|-------------------|------------------------------------------------------|------------|
| 12.4.2            | $S^1 \times S^3$                                     | 496        |
| 12.4.3            | $S^4$                                                | 498        |
| <b>12.5</b>       | <b>Two correspondences and an interpretation</b>     | <b>502</b> |
| 12.5.1            | $S^1 \times S^3$ and the two-dimensional Yang-Mills  | 502        |
| 12.5.2            | $S^4$ and the Liouville theory                       | 504        |
| 12.5.3            | Six-dimensional interpretation                       | 506        |
| <b>12.6</b>       | <b>Future directions</b>                             | <b>509</b> |
| 12.6.1            | Two unsolved problems in the SU(2) case              | 510        |
| 12.6.2            | More objects in the SU(2) case                       | 510        |
| 12.6.3            | Using 6d $\mathcal{N}=(2,0)$ theories of other types | 511        |
| 12.6.4            | Other spacetimes, other theories                     | 513        |
| <b>References</b> |                                                      | <b>514</b> |

## 12.1 Introduction

The aim of this review article is to give an elementary account of the 2d/4d correspondence, originally found in [2,3]. Let us begin by presenting the essential idea, which is in fact quite simple.

We start from a certain six-dimensional quantum field theory  $\mathcal{S}$ , and consider its partition function on a product manifold  $X_4 \times C_2$ , where  $X_4$  is four-dimensional and  $C_2$  is two-dimensional. Let us further suppose that thanks to the supersymmetric twists, the resulting partition function depends on the shapes but not on the sizes of  $X_4$  and  $C_2$ . Then the six-dimensional partition function  $\mathcal{S}(X_4 \times C_2)$  can be evaluated in two ways. On the one hand, if we make  $C_2$  very small, we first have a four-dimensional theory  $\mathcal{S}(C_2)$ , and then we can consider its partition function on  $X_4$ , namely  $\mathcal{S}(C_2)(X_4)$ . On the other hand, if we make  $X_4$  very small, we first have a two-dimensional theory  $\mathcal{S}(X_4)$ , and then we can consider its partition function on  $C_2$ , namely  $\mathcal{S}(X_4)(C_2)$ . We now have an equality

$$\mathcal{S}(X_4)(C_2) = \mathcal{S}(C_2)(X_4). \quad (12.1.1)$$

So far the construction is extremely general. To get something concrete, we need to make a choice. As an example, let us take  $\mathcal{S}$  to be the 6d  $\mathcal{N}=(2,0)$  theory of type  $A_1$ , and  $C_2$  to be an arbitrary two-dimensional surface. The 4d theory  $\mathcal{S}(C_2)$  thus obtained is often called a class S theory of type  $A_1$ , and is an  $\mathcal{N}=2$  supersymmetric theory with a number of SU(2) gauge group factors coupled to a number of trifundamental fields [4].

If we choose  $X_4 = S^4$ , the partition function  $\mathcal{S}(C_2)(X_4)$  can be computable by localization [5,6], and from the results of the computation, one sees that  $\mathcal{S}(S^4)$  is the Liouville theory, which is a non-compact 2d conformal field theory [2]. If we choose  $X_4 = S^3 \times S^1$ , the partition function  $\mathcal{S}(C_2)(X_4)$  is called the superconformal index [7,8], and from the results of the computation, one sees that  $\mathcal{S}(S^3 \times S^1)$  is the  $q$ -deformed SU(2) Yang-Mills theory [3,9]. These are the simplest cases of the correspondences, and various generalizations are possible and have been carried out.

It is already five years since these correspondences were originally found<sup>1</sup>, and countless pages of original articles have been already wasted to describe the details and the generalizations. The number of the review articles devoted to this topic is also already quite large. However, this huge amount of information can also be somewhat daunting, and the author therefore feels that it would be not completely useless to have another concise review, so that a newly interested reader can quickly go through to have an idea of how this correspondence came to be known, where the details can be learned, and what are still unsolved problems s/he might want to study.

This article is therefore intentionally meant to be a shallow overview. Many of the facts will be stated as facts and will not be explained. Details and subtleties will be mentioned but will not be treated in full; references to review or original articles will be given instead.<sup>2</sup> The presentation will not be completely logical either. It would be most systematic to start from six dimensions, to analyze the compactification very carefully, and to arrive at the correspondence at the last step. Thanks to the recent developments, it would not be impossible to write a review in this order. This will, however, be a hard read for people new to this field.

Instead, this review will be organized to explain *how* the correspondence works instead of *why* there is the correspondence. In Sec. 12.2, we begin by learning two two-dimensional field theories that will be important for us: the two-dimensional  $q$ -deformed Yang-Mills theory and the Liouville theory. In Sec. 12.3, we introduce the class S theories of type SU(2), directly as four-dimensional field theories defined by Lagrangian associated to Riemann surfaces with decompositions to three-punctured spheres. In Sec. 12.4, we quickly introduce the technique of supersymmetric localization, and describe how the partition functions on  $S^1 \times S^3$  or on  $S^4$  can be computed. In Sec. 12.5, we apply the supersymmetric localization to the class S theories of type SU(2). We will see that the partition functions on  $S^3 \times S^1$  and on  $S^4$  are given by the  $q$ -deformed Yang-Mills and by the Liouville theory, respectively. We then explain how this correspondence can be understood in terms of the 6d  $\mathcal{N}=(2,0)$  theory. We will conclude in Sec. 12.6 by going over possible future directions.

## 12.2 Two two-dimensional theories

### 12.2.1 Two-dimensional Yang-Mills theories

Let us first study two-dimensional Yang-Mills theories. We will first deal with the standard undeformed gauge theories, and will indicate how it can be  $q$ -deformed at the end. Every detail of the undeformed theory can be found in the great review [10].

---

<sup>1</sup>The bulk of this article was written in August 2014, with only a minor update on the references in the summer of 2016.

<sup>2</sup>The references are not at all exhaustive, and not even extensive either. The author will happily include more in the arXiv version, so please do not hesitate to email him.

## Action

The 2d Yang-Mills theory with the gauge group  $G$  has the Lagrangian

$$S \propto \frac{1}{e^2} \int d^2x \sqrt{\det \mathbf{g}} \operatorname{tr} F_{\mu\nu} F^{\mu\nu}. \quad (12.2.1)$$

Here we consider the theory on a curved manifold with the background metric  $\mathbf{g}$ , in the Euclidean signature. The coupling constant  $e$  can be removed by rescaling  $\mathbf{g}$ .

Recall that in two dimensions, the only nonzero component of the field strength  $F_{\mu\nu}$  is  $F_{01}$ . The kinetic term can then be written as

$$\operatorname{tr} F_{\mu\nu} F^{\mu\nu} \propto (\mathbf{g}^{00} \mathbf{g}^{11} - \mathbf{g}^{01} \mathbf{g}^{10}) \operatorname{tr}(F_{01})^2 = (\det \mathbf{g})^{-1} \operatorname{tr}(F_{01})^2. \quad (12.2.2)$$

This means that in the action (12.2.1) we do not have individual components of the metric  $\mathbf{g}$ : the only combination that appears is  $\det \mathbf{g}$ . Put differently, the 2d Yang-Mills theory can be formulated on a 2d surface not quite equipped with the metric which allows us to measure the distance; all what we need is the volume form  $dx^0 dx^1 \sqrt{\det \mathbf{g}}$  which allows us to measure the area. The only invariant of the 2d surface is then its genus and the total area of the surface, on which alone the partition function can depend.

## On the cylinder

Let us now analyze the theory on a cylinder  $x^1 \sim x^1 + L$  with  $x^0$  as the time direction, see Fig. 12.2.1. We take the temporal gauge  $A_0 = 0$ . At a constant time slice  $x^0 = 0$ , the gauge-invariant data is the holonomy of the gauge field around the circle:

$$U := P \exp \int_0^L A_1 dx^1 \in G, \quad (12.2.3)$$

considered up to the adjoint  $G$ -action  $U \mapsto gUg^{-1}$ .

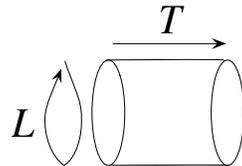

Figure 12.2.1: A cylinder with circumference  $L$

Then the wavefunction of the system is a function  $\psi(U)$  defined on  $G$ , such that we have the invariance

$$\psi(U) = \psi(gUg^{-1}). \quad (12.2.4)$$

It is a standard fact in group theory that such functions are given by a linear combination of traces

$$\chi_R(U) = \operatorname{tr}_R U \quad (12.2.5)$$

in irreducible representations  $R$ . Note that they are orthonormal under the natural measure on  $G$ :

$$\int_G \chi_R(U) \chi_{R'}(U)^* dU = \delta_{RR'}. \quad (12.2.6)$$

Decomposing  $A_1 = A_1^a T_a$ , where  $a = 1, \dots, \dim G$ , the Hamiltonian obtained from (12.2.1) is

$$H \propto \int_0^L \frac{\delta}{\delta A_1^a(x)} \frac{\delta}{\delta A_1^a(x)} dx^1. \quad (12.2.7)$$

Acting on  $\chi_R(U) = \text{tr}_R P \exp \int_0^L A_1 dx^1$ , we find

$$H \chi_R(U) \propto \text{tr}_R \int_0^L T^a T^a dx^1 P \exp \left( \int_0^L A_1 dx^1 \right) \propto L c_2(R) \chi_R(U) \quad (12.2.8)$$

where  $c_2(R)$  is the value of the quadratic Casimir in the irreducible representation  $R$ . We fix the proportionality constants by demanding that  $H \chi_R = L c_2(R) \chi_R$ .

Now we can evaluate the partition function  $Z$  on a torus  $x^1 \sim x^1 + L$ ,  $x^0 \sim x^0 + T$ :

$$Z = \text{tr} e^{-TH} = \sum_R e^{-TL c_2(R)}. \quad (12.2.9)$$

Note that the final result only depends on the total area  $TL$  of the torus, as it should be.

### On a general surface

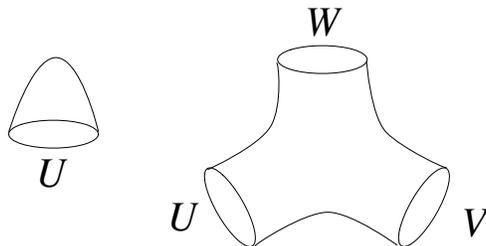

Figure 12.2.2: A disk and a three-holed sphere, with holonomies around the boundaries specified

Next, let us study the theory on a general 2d surface. First, consider the case of a disk with area  $A$ , see Fig. 12.2.2. We specify the holonomy  $U$  around the boundary circle; then we can perform the partition function under this condition. We can denote it as  $Z_A(U)$ . This can also be thought of as defining a wavefunction on the boundary  $S^1$ , and can be denoted as  $\psi_A(U) = Z_A(U)$ . Therefore, in the following, we use the terminology the partition function  $Z$  and the wavefunction  $\psi$  interchangeably. This method of defining a wavefunction via a path-integral over a disk (or more generally a ball in higher dimensions) was pioneered by Hartle and Hawking, and therefore this is often called the Hartle-Hawking wavefunction.

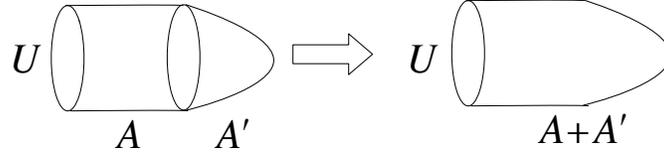

Figure 12.2.3: The area of a disk can be changed by gluing a cylinder

So, what is this wavefunction  $\psi_A(U)$  associated to the disk? First, note that we can glue a cylinder of area  $A$  to a disk of area  $A'$  to have a disk of area  $A + A'$ , see Fig. 12.2.3. This means

$$\psi_{A+A'}(U) = e^{-Ac_2} \psi_{A'}(U) \quad (12.2.10)$$

where  $c_2$  is the operator acting by  $c_2(R)$  on  $\chi_R(U)$ . Therefore it suffices to determine  $\psi_{A=0}(U)$ . When the area is zero,  $U$  is forced to be an identity element, and therefore  $\psi_{A=0}(U) = \alpha \delta(U)$  where  $\delta(U)$  is the delta function at the identity on the group manifold of the group  $G$  and  $\alpha$  is a proportionality constant. We can write

$$\delta(U) = \sum_R d_R \chi_R(U) \quad (12.2.11)$$

where  $d_R$  can be found from the orthonormality property (12.2.6):

$$d_R = \int_G \delta(U) \chi_R(U) dU = \text{tr}_R 1 = \dim R. \quad (12.2.12)$$

This way we find

$$\psi_A(U) = \alpha \sum_R e^{-Ac_2(R)} (\dim R) \chi_R(U). \quad (12.2.13)$$

Second, it is useful at this point to rewrite the Hamiltonian on the cylinder we found above as the amplitude on the cylinder whose boundary holonomies are  $U, V$ :

$$\psi_A(U, V) = \sum_R e^{-Ac_2(R)} \chi_R(U) \chi_R(V^{-1}). \quad (12.2.14)$$

Third, note that any 2d surface can be cut into pieces, such that each piece is a sphere with three holes, see Fig. 12.2.2. Let us say the area is  $A$  and the holonomies around the three holes are  $U, V$  and  $W$ . What is the wavefunction  $\psi_A(U, V, W)$ ? The crucial property is that when a disk is sewed to a hole, it becomes a cylinder, see Fig. 12.2.4. In terms of an equation, this becomes

$$\int_G \psi_A(U, V, W) \psi_{A'}(W^{-1}) dW = \psi_A(U, V). \quad (12.2.15)$$

Using (12.2.13) and (12.2.14), one finds that the unique solution is

$$\psi_A(U, V, W) = \frac{1}{\alpha} \sum_R e^{-Ac_2(R)} (\dim R)^{-1} \chi_R(U) \chi_R(V) \chi_R(W). \quad (12.2.16)$$

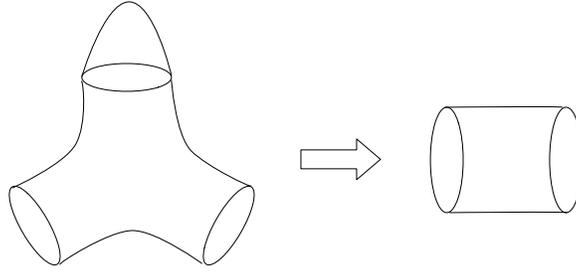

Figure 12.2.4: Sewing a disk to a hole makes a three-holed sphere into a cylinder

The result can be easily generalized to arbitrary surface of area  $A$ , genus  $g$  and  $n$  holes with holonomies  $U_{i=1,\dots,n}$ , by gluing  $\psi_A(U, V, W)$ . The answer is

$$\psi_{A,g}(U_i) = \alpha^{2-2g-n} \sum_R e^{-Ac_2(R)} \frac{\prod_i \chi_R(U_i)}{(\dim R)^{2g-2+n}}. \quad (12.2.17)$$

Note that this final answer automatically satisfies the associativity of the sewing of two three-punctured spheres as shown in Fig. 12.2.5.

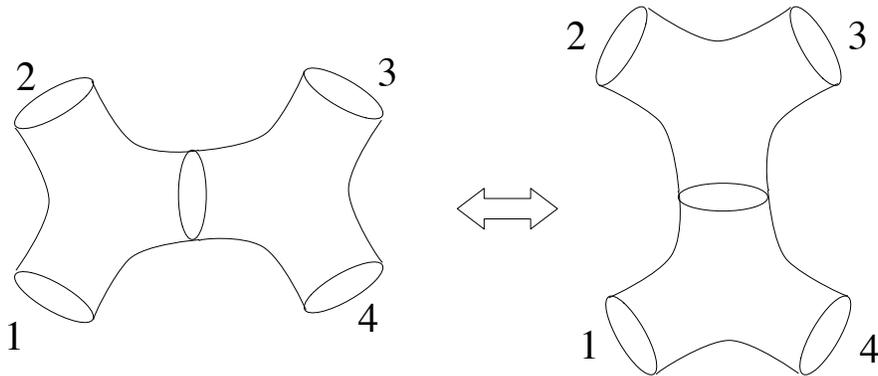

Figure 12.2.5: The amplitude does not depend on how one cuts a four-holed sphere into two three-holed spheres

Finally let us briefly discuss the dependence on  $\alpha$  of various quantities found above. In the action (12.2.1) we can include a local term

$$\delta S = \beta \int d^2x \sqrt{g} R \quad (12.2.18)$$

where  $R$  is the Riemann curvature of the metric  $g$ . On a surface without punctures, this integrates to  $\beta(2 - 2g)$ , and is therefore topological. When the surface has punctures, there is a natural boundary term that makes the integral  $\beta(2 - 2g - n)$ . By including this local but topological term (12.2.18), the factors  $\alpha^{2-2g-n}$  we saw above shifts to  $(e^\beta \alpha)^{2-2g-n}$ .

A term of the form (12.2.18) can be easily generated by changing the regularization scheme and/or the renormalization scheme of a quantum field theory. Therefore there is not much sense in asking what value of  $\alpha$  we get when we start from  $\beta = 0$  in the original Lagrangian (12.2.1).

### $q$ -deformation

So far, we solved the 2d Yang-Mills theory starting from the action (12.2.1). We can instead start from the lattice formulation. Namely, we draw a sufficiently fine mesh on the 2d surface. At each edge  $e$ , we assign a dynamical variable  $U_e$  taking values in the group  $G$ , and at each face  $f$ , we assign a Boltzmann weight

$$\psi_f = \sum_R e^{-A_f c_2(R)} \text{tr}_R \prod_e U_e \quad (12.2.19)$$

where the product is taken around the edges  $e$  around the face  $f$ . Then the path integral defined as

$$Z = \int \prod_e dU_e \prod_f \psi_f \quad (12.2.20)$$

gives the partition function (12.2.17).

An interesting deformation of this theory is obtained by declaring that edge variables  $U_e$  take values in the quantum group  $G_q$ , instead of in the ordinary group  $G$ . The quantum groups are obtained by making non-commutative the matrix entries of the group. For example, the quantum group  $\text{SU}(2)_q$  is given by considering  $2 \times 2$  matrices  $U_i^j = \begin{pmatrix} \alpha & \beta \\ \gamma & \delta \end{pmatrix}$  with the relations

$$\alpha\beta = q^{1/2}\beta\alpha, \quad \alpha\gamma = q^{1/2}\gamma\alpha, \quad \beta\delta = q^{1/2}\delta\beta, \quad \gamma\delta = q^{1/2}\delta\gamma, \quad \beta\gamma = \gamma\beta \quad (12.2.21)$$

and

$$\alpha\delta - q^{1/2}\gamma\beta = \delta\alpha - q^{-1/2}\gamma\beta = 1, \quad (12.2.22)$$

with their complex conjugates given by

$$\bar{U}_i^{\bar{j}} = \begin{pmatrix} \alpha^* & \beta^* \\ \gamma^* & \delta^* \end{pmatrix} = \begin{pmatrix} \delta & -q^{1/2}\gamma \\ -q^{-1/2}\beta & \alpha \end{pmatrix}. \quad (12.2.23)$$

Since the matrix entries themselves are non-commutative, it is slightly tricky to come up with a correct ordering of variables in the lattice path integral (12.2.20) but this can be done [11, 12].

Let us see how a complication would arise, in a simple example. From the explicit commutation relations of the matrix entries of  $\text{SU}_q(2)$  given above, it is easy to check that we have

$$\delta_{j\bar{j}} U_i^j \bar{U}_i^{\bar{j}} = \delta_{i\bar{i}}. \quad (12.2.24)$$

However, due to the non-commutativity of the entries, we have

$$\delta^{i\bar{i}} U_i^j \bar{U}_i^{\bar{j}} \neq \delta^{j\bar{j}}. \quad (12.2.25)$$

Instead, we have

$$D^{i\bar{i}} U_i^j \bar{U}_i^{\bar{j}} = D^{j\bar{j}} \quad (12.2.26)$$

where

$$D^{i\bar{i}} = \begin{pmatrix} q^{-1/2} & 0 \\ 0 & q^{1/2} \end{pmatrix}. \quad (12.2.27)$$

Therefore, the natural combination  $\delta^{i\bar{i}} \delta_{i\bar{i}}$  of the undeformed  $SU(2)$  is modified to

$$\delta^{i\bar{i}} \delta_{i\bar{i}} = 2 \quad \rightsquigarrow \quad D^{i\bar{i}} \delta_{i\bar{i}} = q^{1/2} + q^{-1/2} \quad (12.2.28)$$

in the representation theory of  $SU_q(2)$ . The right hand side is called the quantum dimension of the two-dimensional representation of  $SU_q(2)$ .

At the end of the day, the only change in the final expression (12.2.17) of the partition function, due to the fact that the gauge group is now the quantum group, is that the dimension  $\dim R$  is replaced by the quantum dimension  $\dim_q R$ . For the general  $SU(N)$  case, the quantum dimension is given by

$$\dim_q R = \text{tr}_R \text{diag}(q^{(N-1)/2}, q^{(N-3)/2}, \dots, q^{(1-N)/2}), \quad (12.2.29)$$

and therefore the partition function of the  $q$ -deformed theory is

$$\psi_{A,g}(U_i) = \alpha^{2-2g-n} \sum_R e^{-Ac_2(R)} \frac{\prod_i \chi_R(U_i)}{(\dim_q R)^{2g-2+n}}. \quad (12.2.30)$$

It is known that the same deformation arises also string theoretically [13], although the underlying quantum group is not directly visible there.

## 12.2.2 The Liouville theory

We will now study the second two-dimensional field theory, known as the Liouville theory. It is the prime example of so-called irrational conformal field theory. Here we cover only extremely shallow aspects of this beautiful and rich theory. An interested reader is referred to the classic reviews such as [14, 15]. We will mainly use a more axiomatic approach, pioneered and reviewed in [16]. Before getting there, let us quickly recall the free boson theory.

### Free boson theory

A massless boson  $\phi$  in two dimensions in the Euclidean signature satisfies the equation of motion

$$\Delta\phi = \bar{\partial}\partial\phi = 0. \quad (12.2.31)$$

A general solution is then

$$\phi(z, \bar{z}) = f(z) + \bar{f}(\bar{z}) \quad (12.2.32)$$

where  $f(z)$  is a holomorphic function.

From this we see that the classical theory has a symmetry under arbitrary holomorphic changes of the coordinate  $z \mapsto g(z)$ . Denote the generator of the infinitesimal transformation  $z \rightarrow z(1 + \epsilon z^n)$  by  $L_n$ . Classically they satisfy the commutation relation  $[L_m, L_n] = (m - n)L_{m+n}$ .

In the quantum theory, the basic operator product expansion of the free boson theory is

$$\partial\phi(z)\partial\phi(w) \sim -\frac{1}{2(z-w)^2} \quad (12.2.33)$$

and

$$e^{2ia\phi(z, \bar{z})}e^{-2ia\phi(w, \bar{w})} \sim \frac{1}{|z-w|^{2a^2}}. \quad (12.2.34)$$

The generator  $L_0$  rescales the coordinate as  $z \mapsto e^{-\epsilon L_0}z$ . Correspondingly, when the two-point function behaves as  $(z-w)^{-2\Delta}(\bar{z}-\bar{w})^{-2\bar{\Delta}}$ , we say that the operator has the holomorphic dimension  $L_0 = \Delta$  and the anti-holomorphic dimension  $\bar{L}_0 = \bar{\Delta}$ . We find  $\partial\phi$  has  $(L_0, \bar{L}_0) = (1, 0)$  and  $e^{2ia\phi}$  has  $(L_0, \bar{L}_0) = (a^2, a^2)$ .

Quantum mechanically, the algebra generated by  $L_n$  is modified to

$$[L_m, L_n] = (m-n)L_{m+n} + c\frac{m^3-m}{12}\delta_{m,-n} \quad (12.2.35)$$

where  $c$  is a number called the central charge. This is the celebrated Virasoro algebra. We package them into a field  $T(z) = \sum L_n z^{n-2}$ . The commutation relation above is equivalent to the operator product expansion

$$T(z)T(w) = \frac{c}{2}\frac{1}{(z-w)^4} + \frac{2}{(z-w)^2}T(w) + \frac{1}{z-w}T'(w) + \dots \quad (12.2.36)$$

In a free-boson theory, the energy-momentum tensor  $T(z)$  is given by  $T(z) = (1/2)\partial\phi\partial\phi$ . A short computation reveals that it satisfies the relation (12.2.36) with  $c = 1$ . We now consider a slightly modified free-boson theory where the energy momentum tensor is given by

$$T(z) = \partial\phi\partial\phi + iQ\partial^2\phi. \quad (12.2.37)$$

We find that this satisfies the relation (12.2.36) with

$$c = 1 + 6Q^2. \quad (12.2.38)$$

This modification corresponds to having the Lagrangian density

$$\mathcal{L} = g^{ij}\partial_i\phi\partial_j\phi + Q\phi R \quad (12.2.39)$$

where  $R$  is the curvature of the 2d surface. When computing the correlators on the sphere, we can map it to a flat infinite plane, with the caveat that there is still a concentration of the

curvature at  $z = \infty$ . This effectively place an operator  $e^{-2Q\phi}$  at  $z = \infty$ . From this reason the parameter  $Q$  is often called the background charge. This modifies the basic correlator of the exponential fields (12.2.34) to

$$e^{2(Q/2+ia)\phi(z,\bar{z})} e^{2(Q/2-ia)\phi(w,\bar{w})} \sim \frac{1}{|z-w|^{2a^2+Q^2/2}}. \quad (12.2.40)$$

In particular, the exponential operator  $e^{2(Q/2+ia)\phi}$  has  $L_0 = a^2 + Q^2/4$ . More generally, we say that the operator  $e^{2a\phi}$  has

$$L_0 = a(Q - a). \quad (12.2.41)$$

### Interacting theory

Suppose now that we want to change this free boson theory with background charge  $Q$  into a full-fledged interacting theory without destroying the conformal invariance. At leading order, a new term in the Lagrangian should have the dimension  $(L_0, \bar{L}_0) = (1, 1)$  to preserve the conformal invariance. From (12.2.41), we find that the operator  $e^{2b\phi}$  does the job, when

$$Q = b + \frac{1}{b}. \quad (12.2.42)$$

Now the Lagrangian density is

$$\mathcal{L} = g^{ij} \partial_i \phi \partial_j \phi + Q \phi R + 4\pi \mu e^{2b\phi} \quad (12.2.43)$$

where the parameter  $\mu$  is often called the cosmological constant.

This parameter  $\mu$  can be set to any value one wants, by shifting the origin of  $\phi$ , so it is not easy to do a perturbation theory in terms of this interaction term. Put differently, the potential term  $e^{2b\phi}$  is exponential, and cannot be considered as a small deformation from the free theory with the Lagrangian (12.2.39). But after a series of impressive works, we now know that the Lagrangian density (12.2.43) determines an interacting conformal field theory with the central charge

$$c = 1 + 6Q^2 = 1 + 6\left(b + \frac{1}{b}\right)^2. \quad (12.2.44)$$

One crucial difference from the free theory is as follows. In the free theory, the operator  $e^{2ip\phi}$  with  $L_0 = p^2$  gives rise to a state with momentum  $p$  moving the direction parameterized by  $\phi$ , under the state-operator correspondence. In particular, two operators  $e^{2ip\phi}$  and  $e^{-2ip\phi}$  are two distinct states.

Similarly, in the Liouville theory, the operator  $e^{(Q+2ip)\phi}$  with  $L_0 = p^2 + (Q/2)^2$  corresponds to a state with momentum  $p$  in the  $\phi$ -space. Here the shift of the exponent by  $Q$  is necessary to keep  $L_0$  real and positive. Due to the exponential interaction  $e^{2b\phi}$ , the wave coming from the negative  $\phi$  region cannot penetrate to the positive  $\phi$  region. Instead, it gets reflected by the exponential potential wall. This means that two operators  $e^{(Q+2ip)\phi}$  and  $e^{(Q-2ip)\phi}$  give one and the same state:

$$e^{(Q+2ip)\phi} = R(p) e^{(Q-2ip)\phi} \quad (12.2.45)$$

where  $R(p)$  is a phase called the reflection coefficient. The asymptotic behavior of  $R(p)$  can be computed from the quantum mechanical scattering problem by the exponential potential, and the constraints on further corrections to  $R(p)$  from the conformal invariance was one of the starting points of the full solution of the Liouville theory.

We now know that a unitary conformal theory can be uniquely specified by the condition that its spectrum is given by a family of primary operators  $V_p(z)$  for a real number  $p \geq 0$  with  $L_0 = \bar{L}_0 = p^2 + (Q/2)^2$ . The central charge is (12.2.44). The three-point function on the sphere was originally found independently by [17] and [18]. Using conformal invariance, we can put one operator at  $z = \infty$ , another at  $z = 1$ , and the third at  $z = 0$ . Then it is given by

$$C(\alpha_1, \alpha_2, \alpha_3) := \langle e^{2(Q-\alpha_1)\phi(\infty)} e^{2\alpha_2\phi(1)} e^{2\alpha_3\phi(0)} \rangle = [\pi\mu\gamma(b^2)b^{2-2b^2}]^{(Q-\alpha_1-\alpha_2-\alpha_3)/b} \\ \times \frac{\Upsilon'(0)\Upsilon(2\alpha_1)\Upsilon(2\alpha_2)\Upsilon(2\alpha_3)}{\Upsilon(\alpha_1 + \alpha_2 + \alpha_3 - Q)\Upsilon(\alpha_1 + \alpha_2 - \alpha_3)\Upsilon(\alpha_1 - \alpha_2 + \alpha_3)\Upsilon(-\alpha_1 + \alpha_2 + \alpha_3)}. \quad (12.2.46)$$

Here,

$$\gamma(x) = \Gamma(x)/\Gamma(1-x) \quad (12.2.47)$$

and

$$\Upsilon(x) = \frac{1}{\Gamma_2(x|b, b^{-1})\Gamma_2(Q-x|b, b^{-1})} \quad (12.2.48)$$

where  $\Gamma_2(x|\epsilon_1, \epsilon_2)$  is Barnes' double Gamma function obtained by regularizing the infinite product

$$\Gamma_2(x|\epsilon_1, \epsilon_2) \propto \prod_{m,n \geq 0} (x + m\epsilon_1 + n\epsilon_2)^{-1}. \quad (12.2.49)$$

We will need the following properties of the double Gamma function later in this review. First,  $\Gamma_2(x|\epsilon_1, \epsilon_2)$  is real when  $x$  is real, assuming  $\epsilon_{1,2}$  are real. Then, from analytic continuation, we have

$$\Gamma_2(x^*|\epsilon_1, \epsilon_2) = \Gamma_2(x|\epsilon_1, \epsilon_2)^*. \quad (12.2.50)$$

Another relation we need is

$$\Gamma_2(x + \epsilon_1|\epsilon_1, \epsilon_2)\Gamma_2(x + \epsilon_2|\epsilon_1, \epsilon_2) = x\Gamma_2(x|\epsilon_1, \epsilon_2)\Gamma_2(x + \epsilon_1 + \epsilon_2|\epsilon_1, \epsilon_2). \quad (12.2.51)$$

Before proceeding further, note that the two- and three-point functions are essentially invariant under the exchange  $b \rightarrow b^{-1}$ , as the first line in (12.2.46) can be absorbed into the definition of the primary operators. This invariance under the inversion of  $b$  is rather surprising from the point of view of the Lagrangian description using (12.2.43), as it cannot be seen classically at all. The invariance played a crucial role when people first solved the Liouville theory.

### Four-point function: general structure

In the 2d gauge theory case, the knowledge of the cylinder partition function and the partition function for the sphere with three holes were enough to compute the partition function on

arbitrary surface with any number of holes. Similarly, also for the Liouville theory, the knowledge of the two-point function and the three-point function is sufficient to obtain the correlation function on arbitrary surface with any number of insertions of operators.

Let us illustrate the method by computing the four point function. Using the conformal invariance, we can put three operators at  $z = \infty$ ,  $z = 1$  and  $z = 0$ . Let  $q$  be the position of the fourth operator, and we would like to obtain

$$\langle e^{2(Q-\alpha_1)\phi(\infty)} e^{2\alpha_2\phi(1)} e^{2\alpha_3\phi(q,\bar{q})} e^{2\alpha_4\phi(0)} \rangle. \quad (12.2.52)$$

This is done by inserting the complete set of states between  $e^{2\alpha_2\phi(1)}$  and  $e^{2\alpha_3\phi(q,\bar{q})}$ , see Fig. 12.2.6.

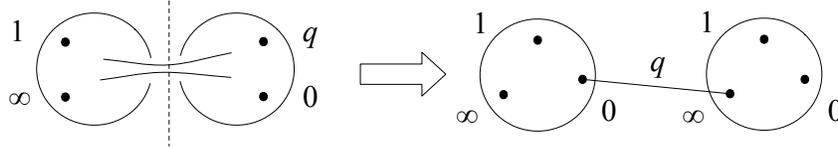

Figure 12.2.6: A four-punctured sphere is composed from two three-punctured sphere by gluing

At the level of the geometry, we have a three-punctured sphere with a local coordinate  $z$ , and another with a local coordinate  $z'$ . Both have three punctures at  $z, z' = \infty, 1, 0$ . We connect  $z = 0$  and  $z' = \infty$ ; this is done as follows. The local coordinate at  $z' = \infty$  is better thought of as  $w = 0$ , where  $wz' = 1$ . Now, the gluing of two punctures with parameter  $q$ , one at  $z = 0$  and another at  $w = 0$  is done by performing the identification  $zw = q$ . We end up having a four-punctured sphere with coordinate  $z$ , with punctures at  $z = \infty, 1, q$  and  $0$ .

The complete set of states are given by the operators

$$O_{p,\{n\},\{\tilde{n}\}} := L_{-n_1} L_{-n_2} \cdots L_{-n_k} \bar{L}_{-\tilde{n}_1} \bar{L}_{-\tilde{n}_2} \cdots \bar{L}_{-\tilde{n}_{\tilde{k}}} e^{2(Q/2+ip)\phi} \quad (12.2.53)$$

where  $p \geq 0$  is real and positive, and the positive integers

$$n_1 \geq n_2 \geq \cdots \geq n_k, \quad \tilde{n}_1 \geq \tilde{n}_2 \geq \cdots \geq \tilde{n}_{\tilde{k}} \quad (12.2.54)$$

specify the descendants of the Virasoro algebra. Note that  $k$  or  $\tilde{k}$  can be zero. The four-point function is then decomposed as

$$\langle e^{2(Q-\alpha_1)\phi(\infty)} e^{2\alpha_2\phi(1)} e^{2\alpha_3\phi(z,\bar{z})} e^{2\alpha_4\phi(0)} \rangle = \int_0^\infty dp \sum_{\{n\},\{\tilde{n}\},\{n'\},\{\tilde{n}'\}} \langle e^{2(Q-\alpha_1)\phi(\infty)} e^{2\alpha_2\phi(1)} O_{p,\{n\},\{\tilde{n}\}} \rangle z^{-\sum n} \bar{z}^{-\sum \tilde{n}} |z|^{-2\Delta_p} G^{\{n\},\{n'\}} G^{\{\tilde{n}\},\{\tilde{n}'\}} \langle O_{p,\{n'\},\{\tilde{n}'\}}^\dagger e^{2\alpha_3\phi(1)} e^{2\alpha_4\phi(0)} \rangle \quad (12.2.55)$$

where  $\Delta_p = p^2 + Q^2/4$  and  $G_p^{\{n\},\{n'\}} G_p^{\{\tilde{n}\},\{\tilde{n}'\}}$  is the inverse matrix of

$$G_{p,\{n\},\{n'\}} G_{p,\{\tilde{n}\},\{\tilde{n}'\}} = \langle O_{p,\{n'\},\{\tilde{n}'\}}^\dagger O_{p,\{n\},\{\tilde{n}\}} \rangle = \langle e^{(Q-2ip)\phi(\infty)} L_{n'_1} \cdots L_{n'_{k'}} \bar{L}_{\tilde{n}'_1} \cdots \bar{L}_{\tilde{n}'_{\tilde{k}'}} L_{-n_1} \cdots L_{-n_k} \bar{L}_{-\tilde{n}_1} \cdots \bar{L}_{-\tilde{n}_{\tilde{k}}} e^{(Q+2ip)\phi(0)} \rangle. \quad (12.2.56)$$

We will soon see that  $G_{p,\{n\},\{n'\}}$  can be computed using only the Virasoro algebra.

We can also write

$$\langle e^{2(Q-\alpha_1)\phi(\infty)} e^{2\alpha_2\phi(1)} O_{p,\{n\},\{\tilde{n}\}} \rangle = l_{\alpha_1,\alpha_2,\alpha,\{n\}} l_{\alpha_1,\alpha_2,\alpha,\{\tilde{n}\}} C(\alpha_1, \alpha_2, \alpha) \quad (12.2.57)$$

$$\langle O_{p,\{n'\},\{\tilde{n}'\}}^\dagger e^{2\alpha_3\phi(1)} e^{2\alpha_4\phi(0)} \rangle = r_{\{n'\},Q-\alpha,\alpha_3,\alpha_4} r_{\{\tilde{n}'\},Q-\alpha,\alpha_3,\alpha_4} C(Q - \alpha, \alpha_3, \alpha_4) \quad (12.2.58)$$

where  $\alpha = Q/2 + ip$ , and the functions  $l$  and  $r$  can again be computed using only the Virasoro algebra.

Plugging these relations back in (12.2.55), we have

$$\langle e^{2(Q-\alpha_1)\phi(\infty)} e^{2\alpha_2\phi(1)} e^{2\alpha_3\phi(q,\bar{q})} e^{2\alpha_4\phi(0)} \rangle = \int_0^\infty dp |q|^{2\Delta_p} C(\alpha_1, \alpha_2, \frac{Q}{2} + ip) C(\frac{Q}{2} - ip, \alpha_3, \alpha_4) F_{\alpha_1,\alpha_2,Q/2+ip,\alpha_3,\alpha_4}(q) \overline{F_{\alpha_1,\alpha_2,Q/2+ip,\alpha_3,\alpha_4}(q)} \quad (12.2.59)$$

where

$$F_{\alpha_1,\alpha_2,Q/2+ip,\alpha_3,\alpha_4}(q) = \sum_{\{n\},\{n'\}} q^{\sum n} l_{\alpha_1,\alpha_2,Q/2+ip,\{n\}} G_p^{\{n\},\{n'\}} r_{\{\tilde{n}'\},Q/2-ip,\alpha_3,\alpha_4} \quad (12.2.60)$$

is known as the four-point conformal block.

Note that the expression (12.2.59) was obtained by inserting a complete set of states between pairs  $\alpha_1, \alpha_2$  at  $z = \infty, 1$  and  $\alpha_3, \alpha_4$  at  $z = q, 0$ . The same correlator can also be obtained by inserting a complete set of states between pairs  $\alpha_1, \alpha_3$  at  $z = \infty, q$  and  $\alpha_2, \alpha_4$  at  $z = 1, 0$  or between pairs  $\alpha_1, \alpha_4$  at  $z = \infty, 0$  and  $\alpha_2, \alpha_3$  at  $z = 1, q$ . The equality of the resulting expressions is not at all trivial, but has been proved in [16, 19].

### Four-point function: explicit expressions

Let us determine the conformal block explicitly to the first few orders. For the zeroth order term, we just have  $G_{p,0,0} = l_{\alpha_1,\alpha_2,Q/2+ip,0} = r_{Q/2-ip,\alpha_3,\alpha_4,0} = 1$ , and so  $F_{\alpha_1,\alpha_2,Q/2+ip,\alpha_3,\alpha_4}(q) = 1 + O(q)$ .

In the next order, we first compute

$$\langle e^{(Q-2ip)\phi(\infty)} L_1 L_{-1} e^{(Q+2ip)\phi(0)} \rangle \quad (12.2.61)$$

using the commutation relation

$$L_1 L_{-1} = L_{-1} L_1 + 2L_0, \quad (12.2.62)$$

and the fact  $L_1$  annihilates the primary  $e^{(Q+2ip)\phi}$ . As  $L_0$  is  $\Delta_p = p^2 + (Q/2)^2$ , we find

$$G_{p,\{1\},\{1\}} = 2\Delta_p. \quad (12.2.63)$$

At the next order, we find

$$\begin{pmatrix} G_{p,\{2\},\{2\}} & G_{p,\{2\},\{1,1\}} \\ G_{p,\{1,1\},\{2\}} & G_{p,\{1,1\},\{1,1\}} \end{pmatrix} = \begin{pmatrix} 4\Delta_p + c/2 & 6\Delta_p \\ 6\Delta_p & 4\Delta_p + 8\Delta_0^2 \end{pmatrix}. \quad (12.2.64)$$

Next, we need to evaluate

$$\langle e^{2(Q-\alpha_1)\phi(\infty)} e^{2\alpha_2\phi(1)} L_{-1} e^{2\alpha\phi(0)} \rangle. \quad (12.2.65)$$

To do this, we commute  $e^{2\alpha_2\phi(1)}$  and  $L_{-1}$ . The term  $L_{-1}e^{2\alpha_2\phi(1)}$  has  $L_{-1}$  acting from the right on the primary  $e^{2(Q-\alpha_1)\phi(\infty)}$ , which annihilates it and gives zero. The computation of the commutator  $[e^{2\alpha_2\phi(1)}, L_{-1}]$  boils down to reinstating the position dependence by replacing  $\phi(1)$  with  $\phi(z)$ , taking the derivative with respect to  $z$ , and setting  $z = 1$  again. From the conformal invariance the  $z$  dependence is just  $z^{-h_{\alpha_1+h_{\alpha_2}+h_{Q/2+ip}}}$  where

$$h_\alpha = \alpha(Q - \alpha), \quad \Delta_p = h_{Q/2+ip} = p^2 + (Q/2)^2. \quad (12.2.66)$$

Then we have

$$l_{\alpha_1, \alpha_2, \frac{Q}{2}+ip, \{1\}} = -h_{\alpha_1} + h_{\alpha_2} + \Delta_p, \quad r_{\{1\}, \frac{Q}{2}-ip, \alpha_3, \alpha_4} = \Delta_p + h_{\alpha_3} - h_{\alpha_4}. \quad (12.2.67)$$

The next order terms are

$$l_{\alpha_1, \alpha_2, \frac{Q}{2}+ip, \{2\}} = -h_{\alpha_1} + 2h_{\alpha_2} + \Delta_p, \quad (12.2.68)$$

$$r_{\{2\}, \frac{Q}{2}-ip, \alpha_3, \alpha_4} = \Delta_p + 2h_{\alpha_3} - h_{\alpha_4}, \quad (12.2.69)$$

$$l_{\alpha_1, \alpha_2, \frac{Q}{2}+ip, \{1,1\}} = (-h_{\alpha_1} + h_{\alpha_2} + \Delta_p)(1 - h_{\alpha_1} + h_{\alpha_2} + \Delta_p), \quad (12.2.70)$$

$$r_{\{1,1\}, \frac{Q}{2}-ip, \alpha_3, \alpha_4} = (\Delta_p + h_{\alpha_3} - h_{\alpha_4})(1 + \Delta_p + h_{\alpha_3} - h_{\alpha_4}). \quad (12.2.71)$$

Combining the results, we find

$$F_{\alpha_1, \alpha_2, Q/2+ip, \alpha_3, \alpha_4}(q) = 1 + \frac{(-h_{\alpha_1} + h_{\alpha_2} + \Delta_p)(\Delta_p + h_{\alpha_3} - h_{\alpha_4})}{2\Delta_p} q + O(q^2). \quad (12.2.72)$$

The order  $q^2$  term can be computed from the data shown above, but is too lengthy to be included here.

It is tedious but not difficult to obtain terms of higher order in  $q$  in the conformal block  $F(q)$ . Note that this is determined purely by the property of the Virasoro algebra, and the final result is expressed in terms of  $h_{\alpha_i} = \alpha_i(Q - \alpha_i)$  and  $\Delta_p$ , that are the  $L_0$  of the primary fields  $e^{2\alpha_i\phi}$  and  $e^{(Q+2ip)\phi}$ , and the central charge  $c$  only. It is instructive at this point to write a program in a computer algebra system of the reader's choice to compute the conformal block to the arbitrary order in  $q$ .

## 12.3 A class of four-dimensional theories

In this section we introduce a class of four-dimensional  $\mathcal{N}=2$  supersymmetric gauge theories, commonly known as class S theories of type SU(2) in the literature. This class of theories was first introduced in [4]. For an extensive review, see e.g. [20]. We start by quickly recalling the very basics of  $\mathcal{N}=2$  Lagrangians.

### 12.3.1 $\mathcal{N}=2$ supersymmetric gauge theories

We assume the reader knows the basics of  $\mathcal{N}=1$  superfields. The  $\mathcal{N}=2$  theories we deal with can be obtained by imposing an  $SU(2)_R$  symmetry that does *not* commute with the  $\mathcal{N}=1$  supersymmetry apparent in the  $\mathcal{N}=1$  formalism.

Let us start with the  $\mathcal{N}=2$  vector multiplet. This consists of an  $\mathcal{N}=1$  vector multiplet  $V$  of a gauge group  $G$ , together with an  $\mathcal{N}=1$  chiral multiplet  $\Phi$  in the adjoint representation of  $G$ . We consider the Lagrangian

$$\frac{\Im\tau}{4\pi} \int d^4\theta \operatorname{tr} \Phi^\dagger e^{[V,\cdot]} \Phi + \int d^2\theta \frac{-i}{8\pi} \tau \operatorname{tr} W_\alpha W^\alpha + cc. \quad (12.3.1)$$

where  $\tau = 4\pi i/g^2 + \theta/2\pi$  is the complexified gauge coupling. By expanding the superfields into components, we see that the gaugino  $\lambda$  in  $V$  and the chiralino  $\psi$  in  $\Phi$  have exactly the same couplings with the other fields, thus realizing  $SU(2)_R$  symmetry.

Next, we introduce the  $\mathcal{N}=2$  hypermultiplet, in the representation  $R$  of the gauge group  $G$ . This consists of a pair of  $\mathcal{N}=1$  chiral multiplets  $Q, \tilde{Q}$  in the representation  $R$  and  $\bar{R}$ . The Lagrangian is

$$\int d^4\theta (Q^\dagger e^V Q + \tilde{Q} e^{-V} \tilde{Q}^\dagger) + \left( \int d^2\theta \tilde{Q} \Phi Q + cc. \right) \quad (12.3.2)$$

where  $\mu$  is the mass term. Here, the  $SU(2)_R$  symmetry rotates the scalar components of  $Q$  and  $\tilde{Q}^\dagger$ .

The Lagrangian above describes a massless hypermultiplet. To give a mass term, we can give a vev to  $\Phi$  in the Lagrangian above. For example, take a pair of hypermultiplets  $Q_i^a$  and  $\tilde{Q}_a^i$  where  $a = 1, \dots, N_c$  and  $i = 1, \dots, N_f$ . This is in the bifundamental representation of  $SU(N_c) \times U(N_f)$ , and as such we have the coupling

$$\tilde{Q}_a^i \Phi_b^a Q_i^b + \tilde{Q}_a^i \underline{\Phi}_j^i Q_j^a \quad (12.3.3)$$

in the Lagrangian, where  $\Phi$  is in the adjoint of  $SU(N_c)$  and  $\underline{\Phi}$  is in the adjoint of  $U(N_f)$ . Now we regard  $\underline{\Phi}$  and its associated  $\mathcal{N}=1$  vector multiplet as external, background fields and just give a vev  $\langle \underline{\Phi} \rangle_j^i = m_j^i$ . We end up having a mass term of the form  $m_j^i \tilde{Q}^i Q_j$ . To preserve  $SU(2)_R$  invariance, we require  $[m, m^\dagger] = 0$ , which means that  $m$  is diagonalizable. It is known that this is the only way to give masses to hypermultiplets.

When  $m = 0$ , the  $U(N_f)$  symmetry is a global flavor symmetry. With generic nonzero diagonal  $m$ , this  $U(N_f)$  symmetry is further explicitly broken to  $U(1)^{N_f}$ . We usually say that this mass term  $m_j^i \tilde{Q}^i Q_j$  is associated to the flavor symmetry  $U(N_f)$ . We often abuse the terminology and say that the theory has the  $U(N_f)$  flavor symmetry even when  $m \neq 0$ .

Finally let us introduce the half-hypermultiplet. When the representation  $R$  is pseudoreal, i.e. when  $R$  and  $\bar{R}$  are equivalent as representations and when there is a gauge-invariant antisymmetric two-form  $\epsilon_{ab}$ , we can impose the condition

$$Q_a = \epsilon_{ab} (\tilde{Q}^\dagger)^b \quad (12.3.4)$$

compatible with the  $SU(2)_R$  invariance. This is called a half-hypermultiplet in the representation  $R$ . Note that this consists of a single  $\mathcal{N}=1$  chiral multiplet in the representation  $R$ .

## 12.3.2 Class S theories of type SU(2)

### Construction from three-punctured spheres and cylinders

In Sec. 12.2, we recalled the properties of two two-dimensional field theories. Very abstractly, two-dimensional field theories associate complex numbers to two-dimensional surfaces. There, the essential point was to find the amplitude associated to a three-punctured sphere or a three-holed sphere, and the amplitude associated to a cylinder.

Here, we introduce a way to associate four-dimensional field theories instead of complex numbers to two-dimensional surfaces. Again, the important point is to consider what to associate to a three-punctured sphere or a cylinder.

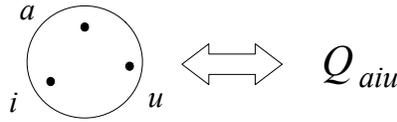

Figure 12.3.1: A three punctured sphere corresponds to  $Q_{aiu}$ , with  $SU(2)^3$  symmetry.

First, take a three-punctured sphere, see Fig. 12.3.1. We associate an  $SU(2)$  flavor symmetry for each of the three punctures. The fundamental representation of  $SU(2)$  is pseudoreal. Furthermore, the tensor product of an odd number of pseudoreal representations is pseudoreal. Therefore, the  $\mathcal{N}=1$  chiral multiplet in the representation  $(2, 2, 2)$  of  $SU(2)_1 \times SU(2)_2 \times SU(2)_3$ , which we denote as

$$Q_{aiu}, \quad a = 1, 2; i = 1, 2; u = 1, 2 \quad (12.3.5)$$

forms a half-hypermultiplet. Here  $a, i, u$  are the indices for  $SU(2)_{1,2,3}$ , respectively.

Next, take a cylinder, see Fig. 12.3.2. We assign to it a complex number  $\tau = 4\pi i/g^2 + \theta/2\pi$ , where  $g$  is real and  $\theta \sim \theta + 2\pi$ . We then associate to it an  $\mathcal{N}=2$  vector multiplet with gauge group  $SU(2)$ , whose complexified coupling is  $\tau$ .

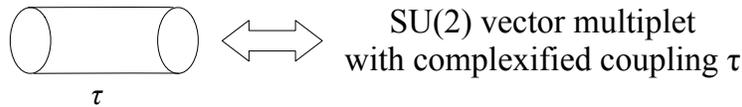

Figure 12.3.2: A cylinder with parameter  $\tau$  corresponds to an  $SU(2)$  vector multiplet.

Now, given a collection of three-punctured spheres, we pick two punctures. Let us say that the first puncture is at  $z = 0$  in a local coordinate  $z$  and the second is at  $w = 0$  in a local coordinate  $w$ . We take a cylinder with parameter  $\tau$ , and make the identification

$$zw = e^{2\pi i\tau}. \quad (12.3.6)$$

We also often use the notation  $q = e^{2\pi i\tau}$ .

Correspondingly, we perform the following operation on the four-dimensional gauge theory side. By choosing two punctures, we picked up two  $SU(2)$  flavor symmetries. We now couple them to a dynamical  $SU(2)$  gauge field, whose complexified coupling constant is  $\tau$ .

### One-punctured torus

Take one three-punctured sphere, and connect two punctures out of three, by a cylinder of parameter  $\tau$ . The result is a torus of modulus  $\tau$  with a puncture, see Fig. 12.3.3. As a gauge theory operation, we start from a trifundamental  $Q_{aiu}$ . Pick the indices  $a$  and  $i$ , and we couple it to a single  $SU(2)$  gauge field. We now regard two  $SU(2)$  symmetries acting on  $a$  and  $i$  as one and the same; as a doublet times a doublet is a triplet plus a singlet, we relabel  $Q_{aiu}$  as  $A_{Iu}$  ( $I = 1, 2, 3$ ) and  $H_u$ , where the index  $u = 1, 2$  is still for an  $SU(2)$  flavor symmetry.

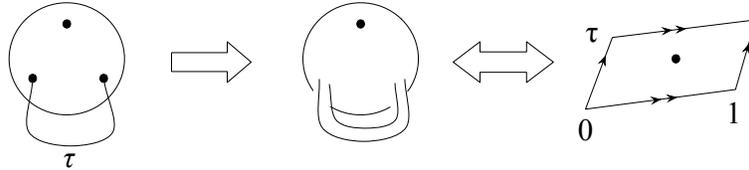

Figure 12.3.3: A punctured torus can be obtained from gluing two points of a three-punctured sphere.

We end up with an  $\mathcal{N}=2$   $SU(2)$  gauge theory with a triplet hypermultiplet formed by  $A_I := A_{I,u=1}$ ,  $\tilde{A}_I := A_{I,u=2}$  and a decoupled hypermultiplet formed by  $H := H_{u=1}$ ,  $\tilde{H} := H_{u=2}$ . An  $\mathcal{N}=2$  gauge theory with gauge group  $G$ , together with a hypermultiplet in the adjoint representation of  $G$ , has an enhanced  $\mathcal{N}=4$  supersymmetry, and commonly known just as  $\mathcal{N}=4$  supersymmetric Yang-Mills. We can give a mass term using  $SU(2)$  flavor symmetry, still preserving  $\mathcal{N}=2$  supersymmetry. The resulting theory is often called  $\mathcal{N}=2^*$  theory.

Note that the gauge theory we obtained has zero one-loop beta function. The high-degree of supersymmetry guarantees that the beta function is zero even non-perturbatively. Therefore the complexified coupling  $\tau$  remains a dimensionless parameter in the gauge theory.

An important property of  $\mathcal{N}=4$  super Yang-Mills is its S-duality: the theory with gauge group  $G$  with coupling constant  $\tau$  is equivalent to the theory with dual gauge group  $G^\vee$  with coupling constant  $-1/\tau$ . We only use the case  $G = SU(2)$ , where the dual gauge group  $G^\vee$  happens to be the same as the original one, so  $G = G^\vee = SU(2)$ .

This has a nice interpretation in our geometric construction of gauge theories: we can construct a one-punctured torus with modular parameter  $\tau$  in two ways from a three-punctured sphere and a cylinder, namely with a cylinder with parameter  $\tau$  or with parameter  $-1/\tau$ .

Correspondingly, for this once-punctured torus, we have two gauge theories associated under our rule:  $\mathcal{N}=4$  theory with gauge group  $SU(2)$ , with complexified gauge coupling  $\tau$  or the same theory with gauge coupling  $-1/\tau$ . The S-duality guarantees that these two theories are the same.

### Four-punctured sphere

Next, take two three-punctured spheres, and connect one puncture from a sphere and another puncture from another sphere, with a cylinder with parameter  $\tau$ . This gives a four-punctured sphere.

In the gauge theory language, we have two trifundamentals  $Q_{aiu}$  and  $Q'_{usx}$ . The indices  $a, i, s, x = 1, 2$  are for four  $SU(2)$  symmetries, and we have a dynamical  $SU(2)$  gauge multiplet acting on the index  $u = 1, 2$ . The one-loop beta function is zero. Again, the beta function is zero even non-perturbatively, and the complexified coupling constant is a genuine dimensionless parameter of the theory.

We can reorganize the chiral matter fields into  $q_{uI}$  where  $u = 1, 2$  and  $I = 1, \dots, 8$ . The superpotential coupling is

$$\delta^{IJ} q_{uI} \Phi_{uv} q_{vJ} \quad (12.3.7)$$

where  $\Phi$  is the adjoint chiral scalar of the  $SU(2)$  gauge multiplet. The indices  $uv$  are symmetric, and therefore  $\delta_{IJ}$  is symmetric too. This means that the flavor symmetry is  $SO(8)$ . This theory is often called  $SU(2)$  gauge theory with  $N_f = 4$  flavors. The four  $SU(2)$ s are subgroups of this  $SO(8)$ :

$$SU(2)_a \times SU(2)_i \times SU(2)_s \times SU(2)_x \subset SO(8) \quad (12.3.8)$$

and the chiral matter fields transform as

$$2_a \otimes 2_i \oplus 2_s \otimes 2_x = 8_V \quad (12.3.9)$$

where  $8_V$  is the vector representation of the  $SO(8)$  flavor symmetry.

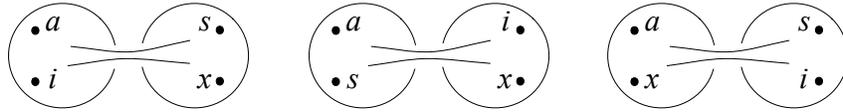

Figure 12.3.4: A four-punctured sphere can be decomposed in three different ways.

Now, a four-punctured sphere can be obtained in three distinct ways from two three-punctured spheres, see Fig. 12.3.4. We described one already. Two others also give  $SU(2)$  theories with  $N_f = 4$  flavors, but with different  $SO(8)$  representation and with different coupling constants. Namely, the matter fields in

$$2_a \otimes 2_s \oplus 2_i \otimes 2_x = 8_S \quad (12.3.10)$$

with coupling  $q' = 1/q$  and the matter fields in

$$2_a \otimes 2_x \oplus 2_s \otimes 2_i = 8_C \quad (12.3.11)$$

with coupling  $q'' = 1 - q$ . Here,  $8_S$  and  $8_C$  are positive and negative chirality spinors of  $SO(8)$ , and we used the exponentiated complexified coupling constants  $q = e^{2\pi i\tau}$ ,  $q' = e^{2\pi i\tau'}$ ,  $q'' = e^{2\pi i\tau''}$ . Again, the S-duality guaranteeing the equivalence of these three descriptions has been known for quite some time.

## General consideration

Let us recapitulate what we have introduced so far. First, we gave a method to construct an  $\mathcal{N}=2$  gauge theory. The data was encoded in terms of the three-punctured spheres and cylinders connecting pairs of punctures. As can be easily checked, every gauge group corresponding to any cylinder has zero one-loop beta function. The  $\mathcal{N}=2$  supersymmetry then guarantees that all beta functions are zero even non-perturbatively, and therefore all gauge coupling constants remain genuine dimensionless parameters of the theory. The punctures that remain unused for connection via cylinders provide  $SU(2)$  flavor symmetries. With  $k$  punctures we have  $SU(2)^k$  flavor symmetries, and if desired, we can turn on the corresponding  $k$  mass parameters. At this point, we have a Lagrangian field theory for a given Riemann surface with punctures, with the decomposition into three-punctured spheres specified.

Second, we considered a torus with one puncture can be constructed from two three-punctured spheres in two ways. The corresponding gauge theories were both  $\mathcal{N}=4$  super Yang-Mills with gauge group  $SU(2)$  with a decoupled hypermultiplet, but with different coupling  $\tau$  and  $-1/\tau$ . They are known to be S-dual. Therefore, a torus with one puncture in fact corresponded to a single theory.

Third, we considered a sphere with four-punctures. This can be constructed in three ways from two three-punctured spheres. The three corresponding gauge theories were  $SU(2)$  theories with  $N_f = 4$  flavors, but with hypermultiplets in distinct  $SO(8)$  flavor representations and with distinct coupling constants. Again, they are known to be S-dual. Therefore, a four-punctured sphere in fact corresponded to a single theory.

In general, given a single Riemann surface with a number of punctures, there are multiple ways to cut it into three-punctured spheres and cylinders. Each of such decompositions gives rise to a distinct Lagrangian of  $\mathcal{N}=2$  supersymmetric gauge theory. However, by combining the two S-dualities recalled above, any such decompositions can be related. Therefore, we conclude that a single Riemann surface with a number of punctures in fact corresponds to a single quantum field theory, of which various distinct Lagrangians are just avatars.

## 12.4 Two supersymmetric backgrounds

In this section we first discuss the general idea of supersymmetric localization, following the approach pioneered by [21] and reviewed in Chapter 5. We then discuss two explicit supersymmetric backgrounds, one based on  $S^1 \times S^3$  and another based on  $S^4$ . More details on the former and the latter can be found in Chapter 13 and in Chapter 10, respectively.

### 12.4.1 General yoga of supersymmetric localization

The energy-momentum tensor  $T_{\mu\nu}$  of a quantum field theory describes how it couples to an external metric perturbation. Namely, let  $Z$  be the partition function as a functional of the metric. Then we have  $\delta \log Z = \int \delta g_{\mu\nu} T^{\mu\nu} d^d x$ . By integrating this small variation, we know how a quantum field theory behaves in a general curved manifold.

In a supersymmetric theory, the energy-momentum tensor  $T_{\mu\nu}$  sits in a supermultiplet, containing the supercurrent  $S_{\mu\alpha}$  and other components, depending on the dimension of the spacetime, the number of supersymmetries, and other subtler properties. In this review we are interested in  $\mathcal{N}=2$  theory in four dimensions. We then have the R-current  $J_\mu^R$  and a scalar component  $X$ , both in the adjoint of  $SU(2)_R$ .

The energy-momentum tensor  $T_{\mu\nu}$  knows how the theory couples to the metric  $g_{\mu\nu}$ . Similarly, the supercurrent  $S_{\mu\alpha}$  knows how it couples to the gravitino background  $\psi_{\mu\alpha}$ . The R-current  $J_\mu^R$  knows how it couples to the R-symmetry background  $A_\mu^R$ , and the scalar component  $X$  knows how it couples to the scalar background  $M$ . In short, the supermultiplet  $(T_{\mu\nu}, S_{\mu\alpha}, J_\mu^R, X, \dots)$  knows how it couples to the external supergravity background  $(g_{\mu\nu}, \psi_{\mu\alpha}, A_\mu^R, M, \dots)$ . There are many definitions of supermanifolds in the mathematical literature, but from the point of view of the supersymmetric field theories, the most natural super-version of a curved manifold is a manifold with the full supergravity background specified. This point of view was emphasized first in [21] and reviewed in more detail in Chapter 5.

Similarly, if a theory has a global flavor symmetry group  $G$ , it has a flavor current  $J_\mu$ , which knows how the theory couples to the flavor symmetry background  $A_\mu$ . When the theory is  $\mathcal{N}=2$  supersymmetric in four dimensions,  $J_\mu$  sits in a supermultiplet containing a scalar operator  $K$ , that knows how to couple to a background scalar  $\Phi$ , where both  $K$  and  $\Phi$  are adjoint of  $G$ . In fact, the mass term of  $\mathcal{N}=2$  theory is just a special case of this construction, as we recalled in Sec. 12.3.1.

Now, given a quantum field theory on a curved manifold with isometry  $\xi$ , we have  $\langle \delta_\xi O \rangle = 0$  for any operator  $O$ . Similarly, given a supersymmetric field theory on a supersymmetric background, i.e. a supergravity background with at least one superisometry  $\epsilon$ , we have  $\langle \delta_\epsilon O \rangle = 0$  for any operator  $O$ .

It often happens that many natural bosonic operators in the Lagrangian can be written as  $\delta_\epsilon O$ . For example, suppose a coupling  $\lambda$  in the Lagrangian multiplies an operator  $X = \delta_\epsilon O$ . Then, the partition function is independent of  $\lambda$ , because

$$\frac{\partial}{\partial \lambda} \log Z = \langle X \rangle = \langle \delta_\epsilon O \rangle = 0. \quad (12.4.1)$$

Also, note that the superisometry variation of the supercurrent itself,  $\delta_\epsilon S_{\mu\alpha}$ , is given by a linear combination of the energy-momentum tensor and other bosonic components of the supermultiplet. This means that a certain variation of the metric can be combined with corresponding particular variations of R-symmetry and scalar backgrounds so that the partition function is independent of it. This makes the partition function on a supersymmetric background oblivious to detailed choice of the metric. Sometimes it depends only on the topology or the complex structure of the spacetime. When  $\delta_\epsilon^2$  generates a bosonic isometry of the background, the partition function only depends on the topological property of that isometry, etc.

It also often happens that we can choose a fermionic operator  $O$  such that

$$\delta_\epsilon^2 O = 0, \quad \delta_\epsilon O \simeq \sum_\psi |\delta\psi|^2. \quad (12.4.2)$$

where  $\psi$  runs over the dynamical fermion fields in the theory. We then consider the deformation

$$S \rightarrow S(t) = S + t \int d^d x \delta_\epsilon O. \quad (12.4.3)$$

Thanks to  $\delta_\epsilon^2 O = 0$ , the deformed Lagrangian is still invariant under the supersymmetry  $\epsilon$ . Then

$$\frac{\partial}{\partial t} \log Z(t) = \int d^d x \langle \delta_\epsilon O \rangle = 0 \quad (12.4.4)$$

for arbitrary  $t$ . In the large  $t$  limit, the integral localizes to the configurations satisfying

$$\delta\psi = 0 \quad (12.4.5)$$

and fluctuations around them. For this reason we often call  $\delta_\epsilon O$  as the localizing term.

We parameterize the solutions to (12.4.5) by a space  $\mathcal{M} = \sqcup_i \mathcal{M}_i$  where  $i$  is some label distinguishing the components. Then we have the equality

$$Z = \sum_i \int_{\mathcal{M}_i} Z_{\text{classical}} Z_{\text{quadr. fluct.}}, \quad (12.4.6)$$

where  $Z_{\text{classical}}$  is the exponential of the classical action evaluated at a configuration satisfying (12.4.5), and  $Z_{\text{quadr. fluct.}}$  is the result of the Gaussian integrals of bosonic and fermionic fluctuations. The interaction terms do not contribute in the  $t \rightarrow \infty$  limit.

Often, each of the components  $\mathcal{M}_i$  is finite dimensional, and therefore the partition function  $Z$  is given as a sum of explicit multiple integrals. Evaluating it is still a formidable task, but is infinitely simpler than the original infinite-dimensional path integral expression.

Now, let us discuss two particular classes of supersymmetric backgrounds for four-dimensional  $\mathcal{N}=2$  theories, on which the localization has been worked out in detail. The first is  $S^1 \times S^3$  and the second is  $S^4$ . We do not discuss the detailed derivations of the facts mentioned below. Happily, all the details can be found in Chapter 13 for  $S^1 \times S^3$  and in Chapter 10 for  $S^4$ .

## 12.4.2 $S^1 \times S^3$

First, we consider  $\mathcal{N}=2$  superconformal theory on  $S^1 \times S^3$ . An  $\mathcal{N}=2$  superconformal theory has  $SU(2)_R \times U(1)_R$  R-symmetry. A class of supersymmetric backgrounds, where the supersymmetric localization can be performed, is specified by the ratio  $\beta$  of the radii of  $S^1$  and  $S^3$ , and two holonomies of  $SU(2)_R$  and  $U(1)_R$  around  $S^1$ . In total there are three parameters, commonly denoted by  $(p, q, t)$ . Note that this  $q$  is independent of the exponentiated complexified coupling, also often denoted by  $q$  and is equal to  $e^{2\pi i \tau}$ . In fact, the vector multiplet Lagrangian is of the form  $\sim \tau \delta_\epsilon O$ , and therefore the partition function on this background is independent of the complexified gauge coupling  $\tau$ .

For brevity of the exposition, we only use the one-dimensional slice where  $p = 0$ ,  $q = t$ . In this case  $q = e^{-\beta}$ . When the  $\mathcal{N}=2$  theory in question has a flavor symmetry  $G$ , we can choose an element  $g \in G$  such that there is a background  $G$  gauge field around  $S^1$  given by  $g$ . Then the partition function on this background is just a function of  $q = e^{-\beta}$  and  $g \in G$ .

By considering the  $S^1$  direction as the time direction, the partition function can be written as

$$Z(q, g) = \text{tr}_{\mathcal{H}}(-1)^F q^{\Delta-R} g. \quad (12.4.7)$$

Here,  $\mathcal{H}$  is the Hilbert space of the superconformal theory on  $S^3$ , which is equivalent to the space of point-like operators of the conformal theory on the flat space, via the state-operator correspondence.  $\Delta$  is then the scaling dimension of the operator, and  $R$  is the third component of the  $SU(2)_R$  charge. From this structure this partition function is often called the superconformal index. For four-dimensional quantum field theories, this concept was introduced in [7, 8].

Correspondingly, the computation of  $Z(q, g)$  for an  $\mathcal{N}=2$  Lagrangian field theory can be done either by counting the operators on a flat space, or by performing the path integral on  $S^1 \times S^3$ . In most of the literature it is done using the operator approach; for a thorough discussion for  $\mathcal{N}=2$  case, see [9]. For a path-integral approach for  $\mathcal{N}=4$ , see [25].

Either way, we find the following results. We first represent the holonomy  $g \in G$  around  $S^1$  using complex numbers in the form

$$g = (z_1, \dots, z_r) \in U(1)^r \subset G \quad (12.4.8)$$

where  $r$  is the rank of  $G$ . We can have an arbitrary flavor holonomy. The gauge holonomy parameterizes the BPS configurations over which we integrate.

For an  $\mathcal{N}=2$  hypermultiplet consisting of  $\mathcal{N}=1$  chiral multiplet in a representation  $R$  of a symmetry  $G$ , the partition function is

$$Z_R(q, g) = \prod_{n \geq 0} \prod_w \frac{1}{1 - q^{n+1/2} z^w} \quad (12.4.9)$$

where  $w = (w_1, \dots, w_r)$  runs over weights of  $R$  and  $z^w := \prod z_i^{w_i}$ .

For a gauge theory with gauge group  $G$ , the partition function is

$$Z(q) = \frac{1}{|W_G|} \oint \prod_{i=1}^r \frac{dz_i}{2\pi\sqrt{-1}z_i} \prod_{\alpha} (1 - z^{\alpha}) K(z)^{-2} \times (\text{matter contribution}) \quad (12.4.10)$$

where

$$K(z)^{-1} = \prod_{n \geq 0} \left[ (1 - q^{n+1})^r \prod_{\alpha} (1 - q^{n+1} z^{\alpha}) \right]. \quad (12.4.11)$$

Here, the product on  $\alpha$  runs over the roots  $\alpha$  of  $G$ ,  $|W_G|$  is the order of the Weyl group of  $G$ , and the integral takes the residues at the origin.

As an example, the partition function of  $\mathcal{N}=4$  supersymmetric Yang-Mills of gauge group  $SU(N)$ , considered as an  $\mathcal{N}=2$  theory with  $SU(2)$  flavor symmetry, is given as follows. The  $SU(2)$  element  $g$  is written as  $(a, a^{-1}) \in SU(2)$ . The  $SU(N)$  element is written as

$(z_1, \dots, z_N) \in \text{SU}(N)$ , with the understanding that  $\prod z_i = 1$ . Then, we have

$$Z(q, a) = \frac{1}{N!} \oint \prod_{i=1}^{N-1} \frac{dz_i}{2\pi\sqrt{-1}z_i} \prod_{i,j} (1 - z_i/z_j)^2 \times \frac{\prod_{n \geq 0} (1 - q^{n+1})^{2r} \prod_{i,j} (1 - q^{n+1} z_i/z_j)^2}{\prod_{\pm} \prod_{n \geq 0} (1 - q^{n+1/2} a^{\pm 1})^r \prod_{i,j} (1 - q^{n+1/2} z_i/z_j a^{\pm 1})}. \quad (12.4.12)$$

This looks complicated, but it is quite explicit, and its  $q$ -expansion can be readily computed.

### 12.4.3 $S^4$

As a second supersymmetric background, we consider  $S^4$ . The localization on a round  $S^4$  was first done in [6], and this was later extended to squashed  $S^4$  in [26]. We call both backgrounds just  $S^4$ . A review of the localization on general backgrounds with two isometries can be found in [27].

#### General structure

To describe the localization, we first write  $S^4$  as a hypersurface in a five-dimensional space parameterized by a real number  $x$  and two complex numbers  $z_{1,2}$ :

$$x^2 + |z_1|^2 + |z_2|^2 = 1. \quad (12.4.13)$$

Write  $z_i = r_i e^{\sqrt{-1}\phi_i}$ , and we endow  $S^4$  with background supergravity fields invariant under the arbitrary shift of  $\phi_1$  and  $\phi_2$ . The metric and other supergravity fields can be suitably chosen so that there is a superisometry  $\epsilon$  such that  $\delta_{\epsilon}^2$  generates a rotation

$$\phi_i \rightarrow \phi_i + \epsilon_i. \quad (12.4.14)$$

Note that  $x = 1, z_i = 0$  and  $x = -1, z_i = 0$  are two fixed points under this rotation. We call them the north pole and the south pole.

The field configurations that contribute to the partition function under the localization are as follows. For the hypermultiplets, the vev should be all zero. For the vector multiplets, the adjoint scalar  $\Phi$  is such that  $\Phi$  can have a non-zero spacetime-independent vev but  $\bar{\Phi} = 0$ . This vev is customarily denoted by  $a$ . We take the convention that  $a$  is purely imaginary. When the vector multiplet is non-dynamical, this vev  $a$  gives the mass term of the hypermultiplets, and is often denoted by  $m$ . In addition, there can be point-like instantons supported on the north pole and point-like anti-instantons supported on the south pole.

Correspondingly, the partition function of the theory on  $S^4$  with gauge group  $G$  has the form

$$Z = \frac{1}{|W_G|} \int d^r a Z(a) \overline{Z(a)} \quad (12.4.15)$$

where  $|W_G|$  is the order of the Weyl group, the integral is over the space of vevs of the real part of  $\Phi$  that is gauge-fixed to lie on the Cartan subalgebra. Then  $Z(a)$  is the contribution

from the northern hemisphere given the vev  $a$ , and its complex conjugate  $\overline{Z(a)}$  gives the contribution from the southern hemisphere.

The contribution  $Z(a)$  is often called Nekrasov's partition function, and is composed of the following ingredients:

$$Z(a) = Z_{\text{classical}}(a)Z_{\text{one-loop}}(a)Z_{\text{instanton}}(a). \quad (12.4.16)$$

In the following, we give explicit forms of these three factors. We will be cavalier about the overall factors independent of the vev of the adjoint scalars, mass parameters and gauge coupling constants.

### Classical and one-loop factors

The first factor is the exponentiated classical action, given by the product of

$$e^{-\frac{1}{\epsilon_1\epsilon_2}2\pi\sqrt{-1}\tau(a,a)} \quad (12.4.17)$$

over various gauge multiplets, where  $\tau$  is the complexified gauge coupling. The second factor is the one-loop contributions from the vector multiplets and the hypermultiplets. From a gauge multiplet, we have

$$Z_{\text{one-loop}}^G = \prod_{\alpha>0} \frac{1}{\Gamma_2(\alpha \cdot a + \epsilon_1 + \epsilon_2 | \epsilon_1, \epsilon_2) \Gamma_2(\alpha \cdot a | \epsilon_1, \epsilon_2)} \quad (12.4.18)$$

where the product runs over the positive roots  $\alpha$ . From a hypermultiplet in the representation  $R$ , we have

$$Z_{\text{one-loop}}^R = \prod_w \Gamma_2(w \cdot a + \frac{\epsilon_1 + \epsilon_2}{2} | \epsilon_1, \epsilon_2) \quad (12.4.19)$$

where the product runs over the weights of  $R$ . For a half-hypermultiplet in  $R$ , the product runs over arbitrary half of the weights of  $R$ ; the final contribution to the instanton integral (12.4.15) does not depend on this split into halves.

The mass term of hypermultiplets can be incorporated by giving a vev to the scalar in the flavor background gauge multiplet. Effectively, this just replaces  $w \cdot a \rightarrow w \cdot a + m$ . Note also that in our convention  $a$  is purely imaginary but  $\epsilon_{1,2}$  are real. Therefore, to get the contribution  $\overline{Z(a)}$  from the southern hemisphere, we just replace  $a$  by  $-a$  in the argument of the double Gamma function.

### Instanton contributions

The instanton contribution is much more complicated to present and the explicit form is only known for SU gauge groups and with full hypermultiplets, due to various technical problems. Even for SU gauge groups, the computation involves a certain regularization that introduces spurious contributions, which is often said to come from replacing SU groups by U groups and therefore has the name U(1) factors. Here we just quote the known results, including the spurious or U(1) factor. For a more detailed discussion, see [28].

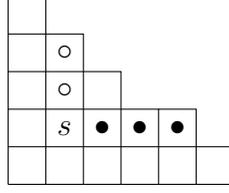

Figure 12.4.1: Young diagram  $Y = (5, 4, 3, 2, 2, 1)$  and a box  $s = (2, 2)$ , and its arm and leg length.

A point-like instanton configuration of a  $U(N)$  gauge multiplet is labeled by an  $N$ -tuple of Young diagrams  $\vec{Y} = (Y_1, \dots, Y_N)$ . A Young diagram  $Y$  is just a non-decreasing sequence of natural numbers  $Y = (\lambda_1 \geq \lambda_2 \geq \dots)$ . Here we visualize them by considering  $\lambda_i$  as the height of the  $i$ -th column from the left, and we set  $\lambda_i = 0$  when  $i$  is larger than the width of the diagram. This is not the standard convention in the literature of Young diagrams, but is the standard one in the instanton computations. We denote by  $|Y|$  the number of boxes, i.e.  $|Y| = \sum \lambda_i$  and then we define  $|\vec{Y}| = \sum |Y_i|$ .

We denote by  $Y^T$  its transpose,  $Y^T = (\lambda'_1 \geq \lambda'_2 \geq \dots)$ . For a box  $s$  at the coordinate  $(i, j)$ , its arm-length  $A_Y(s)$  and the leg-length  $L_Y(s)$  are defined to be

$$A_Y(s) = \lambda_i - j, \quad L_Y(s) = \lambda'_j - i. \quad (12.4.20)$$

Note that  $s$  can be outside of the Young diagram  $Y$ . We then let

$$E(a, Y_1, Y_2, s) = a - \epsilon_1 L_{Y_2}(s) + \epsilon_2 (A_{Y_1}(s) + 1). \quad (12.4.21)$$

Now we can finally write down the instanton contribution. For example, consider an  $SU(N) \times SU(M)$  gauge theory with a bifundamental hypermultiplet. Its instanton contribution is a sum over possible point-like instanton configurations:

$$Z_{\text{instanton}}(\vec{a}; \vec{b}) = \sum_{\vec{Y}, \vec{W}} q^{|\vec{Y}|} q'^{|\vec{W}|} Z(\vec{a}, \vec{Y}; \vec{b}, \vec{W}) \quad (12.4.22)$$

where  $\vec{a} = (a_1, \dots, a_N)$  and  $\vec{b} = (b_1, \dots, b_M)$  are the vevs of the real part of the adjoint scalars in the vector multiplets of  $SU(N)$  and  $SU(M)$ , and  $\vec{Y} = (Y_1, \dots, Y_N)$ ,  $\vec{W} = (W_1, \dots, W_M)$  label the point-like instanton configurations. The prefactors  $q$ ,  $q'$  are given by  $q = e^{2\pi\sqrt{-1}\tau}$  and  $q' = e^{2\pi\sqrt{-1}\tau'}$  where  $\tau$ ,  $\tau'$  are the complexified gauge couplings of two gauge factors.

The contribution from each fixed point,  $Z(\vec{a}, \vec{Y}; \vec{b}, \vec{W})$ , is given by the product of the contributions from each multiplet. The vector multiplet of  $SU(N)$  contributes by

$$Z_{\text{instanton}}^{\text{vector}, SU(N)}(\vec{a}, \vec{Y}) = \frac{1}{\prod_{i,j=1}^N \prod_{s \in Y_i} E(a_i - a_j, Y_i, Y_j, s) \prod_{t \in Y_j} (\epsilon_1 + \epsilon_2 - E(a_j - a_i, Y_j, Y_i, t))}, \quad (12.4.23)$$

and the contribution from  $SU(M)$  can be obtained similarly. The contribution from the bifundamental of mass  $m$  is

$$Z_{\text{instanton}}^{\text{hyper,bifundamental}}(\vec{a}, \vec{Y}; \vec{b}, \vec{W}; m) = \prod_i^N \prod_j^M \prod_{s \in Y_i} (E(a_i - b_j, Y_i, W_j, s) - m - \frac{\epsilon_1 + \epsilon_2}{2}) \prod_{t \in W_j} (E(b_j - a_i, W_j, Y_i, t) - m + \frac{\epsilon_1 + \epsilon_2}{2}). \quad (12.4.24)$$

The contributions from an adjoint hypermultiplet of  $SU(N)$  can be obtained by setting  $\vec{a} = \vec{b}$  and  $\vec{Y} = \vec{W}$ . Similarly, the contributions from  $N_f$  fundamental hypermultiplet of  $SU(N)$  can be obtained by letting  $M = N_f$  and regarding the  $SU(M)$  part as a background gauge field, setting  $W_i = 0$ . Then  $\vec{b}$  becomes the  $SU(N_f)$  part of the mass parameters. As an example, the partition function of  $SU(N)$  gauge theory with an adjoint hypermultiplet of mass  $m$  is

$$Z(\tau, m) = \frac{1}{N!} \int d^{N-1} a |q^{-\frac{1}{\epsilon_1 \epsilon_2} \sum a_i^2}|^2 \times \prod_{i,j} \frac{\Gamma_2((a_i - a_j) + m + \frac{\epsilon_1 + \epsilon_2}{2} | \epsilon_1, \epsilon_2) \Gamma_2((a_i - a_j) - m + \frac{\epsilon_1 + \epsilon_2}{2} | \epsilon_1, \epsilon_2)}{\Gamma_2((a_i - a_j) + \epsilon_1 + \epsilon_2 | \epsilon_1, \epsilon_2) \Gamma_2((a_i - a_j) | \epsilon_1, \epsilon_2)} \times \left| \sum_{\vec{Y}} q^{|\vec{Y}|} \prod_{i,j} \frac{\prod_{s \in Y_i} (E(a_i - a_j, Y_i, Y_j, s) - m - \frac{\epsilon_1 + \epsilon_2}{2}) \prod_{t \in Y_j} (E(a_j - a_i, Y_j, Y_i, t) - m + \frac{\epsilon_1 + \epsilon_2}{2})}{\prod_{s \in Y_i} E(a_i - a_j, Y_i, Y_j, s) \prod_{t \in Y_j} (\epsilon_1 + \epsilon_2 - E(a_j - a_i, Y_j, Y_i, t))} \right|^2 \quad (12.4.25)$$

This expression is horrible, but quite explicit nonetheless. The matter content of the theory is the same as  $\mathcal{N}=4$  super Yang-Mills with gauge group  $SU(N)$ , and the supersymmetry on this supergravity background is believed to enhance when  $m = \pm(\epsilon_1 - \epsilon_2)/2$ . Then the expression simplifies greatly [29]. In this case, the instanton correction is trivial, because when  $|Y| \geq 1$ , there is a box that causes at least one factor of the numerator to be zero. For each choice of  $(i, j)$ , the one-loop factor gives

$$\frac{\Gamma_2((a_i - a_j) + \epsilon_1 | \epsilon_1, \epsilon_2) \Gamma_2((a_i - a_j) + \epsilon_2 | \epsilon_1, \epsilon_2)}{\Gamma_2((a_i - a_j) | \epsilon_1, \epsilon_2) \Gamma_2((a_i - a_j) + \epsilon_1 + \epsilon_2 | \epsilon_1, \epsilon_2)} = a_i - a_j. \quad (12.4.26)$$

Then the integral boils down to

$$Z(\tau, \frac{\epsilon_1 - \epsilon_2}{2}) = \frac{1}{N!} \int d^{N-1} a \prod_{i,j} (a_i - a_j) |q^{-\frac{1}{\epsilon_1 \epsilon_2} \sum a_i^2}|^2 = \int d^{N^2-1} A |q|^{-\frac{2}{\epsilon_1 \epsilon_2} \text{tr} AA^\dagger}, \quad (12.4.27)$$

that is, this is just an Hermitean random matrix model. This was originally observed in [30, 31], and the  $S^4$  localization of [6] was originally conceived to derive this fact quantum field theoretically.

## 12.5 Two correspondences and an interpretation

Here comes the crux: we compute the partition functions of the class of 4d  $\mathcal{N}=2$  theories associated to Riemann surfaces with punctures introduced in Sec. 12.3 on two supersymmetric backgrounds introduced in Sec. 12.4. We will find that they are given by the two two-dimensional theories introduced in Sec. 12.2.

### 12.5.1 $S^1 \times S^3$ and the two-dimensional Yang-Mills

Let us first consider the partition function on  $S^1 \times S^3$ . Take a three-punctured sphere. In Sec. 12.3 we associated to it a half-hypermultiplet in  $2 \otimes 2 \otimes 2$  of  $SU(2)_1 \times SU(2)_2 \times SU(2)_3$ . Its partition function  $Z(a_1, a_2, a_3)$  on  $S^1 \times S^3$ , when the holonomy of  $SU(2)_i$  is  $(a_i, 1/a_i) \in SU(2)_i$ , is given using (12.4.9) by

$$Z(a_1, a_2, a_3) = \prod_{\pm \pm \pm} \prod_{n \geq 0} \frac{1}{1 - q^{n+1/2} a_1^{\pm 1} a_2^{\pm 1} a_3^{\pm 1}}. \quad (12.5.1)$$

It so happens that it has an alternative expression as an infinite sum

$$Z(a_1, a_2, a_3) = \frac{K(a_1)K(a_2)K(a_3)}{K_0} \sum_{n \geq 0} \frac{\chi_n(a_1)\chi_n(a_2)\chi_n(a_3)}{\chi_n(q^{1/2})}, \quad (12.5.2)$$

where

$$K(a)^{-1} = \prod_{n \geq 0} \left[ (1 - q^{n+1}) \prod_{\pm} (1 - q^{n+1} a^{\pm 2}) \right] \quad (12.5.3)$$

is the same function introduced in (12.4.11),

$$K_0^{-1} = \prod_{n \geq 0} (1 - q^{2+n}), \quad (12.5.4)$$

and

$$\chi_n(a) = a^{n-1} + a^{n-3} + \dots + a^{3-n} + a^{1-n} \quad (12.5.5)$$

is the character of  $(a, 1/a) \in SU(2)$  in the  $n$ -dimensional irreducible representation of  $SU(2)$ . At this point, the reader should try to prove this equality (12.5.2), or at least check it by expanding both sides to, say,  $O(q^3)$ .

We see that this infinite sum expression is equal to the amplitude of the three-holed sphere of the 2d  $q$ -deformed  $SU(2)$  Yang-Mills, introduced in Sec. 12.2.30, in the zero area limit, apart from the prefactor involving  $K(a_i)$  and  $K(0)$ .

Next, consider the four-punctured sphere. The corresponding four-dimensional theory is obtained by taking two half-hypermultiplets of  $SU(2)_1 \times SU(2)_2 \times SU(2)$  and  $SU(2) \times SU(2)_3 \times SU(2)_4$ , and coupling them by a dynamical  $SU(2)$  gauge multiplet. Correspondingly,

the partition function on  $S^1 \times S^3$  is given by the formula (12.4.10):

$$Z(a_1, a_2; a_3, a_4) = \frac{1}{2} \oint \frac{dz}{2\pi iz} (1 - z^2) \left(1 - \frac{1}{z^2}\right) K(z)^{-2} Z(a_1, a_2, z) Z(z, a_3, a_4) \quad (12.5.6)$$

$$\begin{aligned} &= \frac{1}{2} \oint \frac{dz}{2\pi iz} (1 - z^2) \left(1 - \frac{1}{z^2}\right) K(z)^{-2} \\ &\quad \times \prod_{\pm\pm\pm} \prod_{n \geq 0} \frac{1}{1 - q^{n+1/2} a_1^{\pm 1} a_2^{\pm 1} z^{\pm 1}} \prod_{\pm\pm\pm} \prod_{n \geq 0} \frac{1}{1 - q^{n+1/2} z^{\pm 1} a_3^{\pm 1} a_4^{\pm 1}} \end{aligned} \quad (12.5.7)$$

where we used the infinite product form of the contribution from the half-hypermultiplet, (12.5.1). In this form it is not clear that this expression is symmetric under the permutation of variables  $a_{1,2,3,4}$ .

Plugging in the infinite-sum form (12.5.2) instead, one finds

$$\begin{aligned} Z(a_1, a_2; a_3, a_4) &= \frac{1}{2} \oint \frac{dz}{2\pi iz} (1 - z^2) \left(1 - \frac{1}{z^2}\right) \frac{K(a_1)K(a_2)K(a_3)K(a_4)}{K_0^2} \\ &\quad \times \sum_{n \geq 0} \frac{\chi_n(a_1)\chi_n(a_2)\chi_n(z)}{\chi_n(q^{1/2})} \sum_{m \geq 0} \frac{\chi_m(z)\chi_m(a_2)\chi_n(a_3)}{\chi_m(q^{1/2})} \end{aligned} \quad (12.5.8)$$

$$= \frac{K(a_1)K(a_2)K(a_3)K(a_4)}{K_0^2} \sum_{n \geq 0} \frac{\chi_n(a_1)\chi_n(a_2)\chi_n(a_3)\chi_n(a_4)}{\chi_n(q^{1/2})^2}. \quad (12.5.9)$$

Here, we used the orthogonality of the  $SU(2)$  characters under the natural measure

$$\frac{1}{2} \oint \frac{dz}{2\pi iz} (1 - z^2) \left(1 - \frac{1}{z^2}\right) \chi_n(z)\chi_m(z) = \delta_{mn} \quad (12.5.10)$$

which is just a special version of (12.2.6). The factor  $(1 - z^2)(1 - z^{-2})$  is a measure factor introduced by restricting the group variable  $z \in SU(2)$  into its Cartan torus.

We find that the partition function (12.5.9) is again equal to the amplitude of the four-holed sphere of the  $q$ -deformed  $SU(2)$  Yang-Mills, apart from the prefactor involving  $K(a)$  and  $K_0$ , and the fact that the area  $A$  needs to be set to zero.

This computation can easily be generalized to arbitrary class S theories of type  $SU(2)$ . On the four-dimensional side, we consider the partition function on  $S^1 \times S^3$  of the theory associated to a Riemann surface of genus  $g$  with  $n$  punctures, where we put the holonomy  $(a_i, 1/a_i) \in SU(2)_i$  for the flavor symmetry for the  $i$ -th puncture. On the two-dimensional side, we take the  $q$ -deformed  $SU(2)$  Yang-Mills on the same Riemann surface, where we regard punctures as holes, with the holonomy  $(a_i, 1/a_i) \in SU(2)$  specified around the  $i$ -th hole. Then we have the general relation

$$Z_{4d,g,n}(a_i) = \frac{\prod_i K(a_i)}{K_0^{2g-2+n}} Z_{2d,g,n,A=0}(a_i). \quad (12.5.11)$$

The factor  $K(a)/K_0$  for each puncture can be absorbed into a redefinition of the hole-introducing operator on the two-dimensional side. Similarly, we can always add a local counter-term in a two-dimensional non-gravitational theory given by

$$S_{2d} \rightarrow S_{2d} + c \int \sqrt{g} R_g = S_{2d} + c(2 - 2g) \quad (12.5.12)$$

where  $R_g$  is the curvature scalar of the two-dimensional metric. This can absorb the factor  $K_0^{2-2g}$ . Therefore, we conclude that the  $S^1 \times S^3$  partition function of the class S theory of type  $SU(2)$  associated to a punctured Riemann surface is always given by the partition function of the  $q$ -deformed  $SU(2)$  Yang-Mills considered on the same punctured Riemann surface. This is the correspondence first found in [3].

## 12.5.2 $S^4$ and the Liouville theory

Let us next consider the partition function on  $S^4$ , which will be a function of the parameters  $\epsilon_{1,2}$  in the supergravity background, the masses  $m_i$ , and the complexified gauge couplings  $\tau_i$ . Note that  $\epsilon_{1,2}$  and  $m_i$  all have mass dimension 1. We fix the scale by demanding  $\epsilon_1\epsilon_2 = 1$ .

Take a three-punctured sphere. The corresponding four-dimensional theory associated in Sec. 12.3 is a half-hypermultiplet in  $2 \otimes 2 \otimes 2$  of  $SU(2)_1 \times SU(2)_2 \times SU(2)_3$ . Its partition function  $Z_{S^4}^{\text{trifund}}(m_1, m_2, m_3)$  on  $S^4$ , when the mass parameters of  $SU(2)_i$  is  $(m_i/2, -m_i/2) \in SU(2)_i$ , is given by  $|Z_{\text{n.h.}}(m_1, m_2, m_3)|^2$  as in (12.4.15). Here the contribution from the northern hemisphere,  $Z_{\text{n.h.}}^{\text{trifund}}(m_1, m_2, m_3)$  is given in (12.4.19):

$$Z_{\text{n.h.}}^{\text{trifund}}(m_1, m_2, m_3) = \prod_{\pm\pm} \Gamma_2\left(\frac{m_1 \pm m_2 \pm m_3}{2} + \frac{\epsilon_1 + \epsilon_2}{2} | \epsilon_1, \epsilon_2\right) \quad (12.5.13)$$

and therefore we have

$$Z_{S^4}^{\text{trifund}}(m_1, m_2, m_3) = \prod_{\pm\pm\pm} \Gamma_2\left(\frac{\pm m_1 \pm m_2 \pm m_3}{2} + \frac{\epsilon_1 + \epsilon_2}{2} | \epsilon_1, \epsilon_2\right). \quad (12.5.14)$$

Note that we used our convention that  $m_i$  are all purely imaginary.

We see that this is equal to the denominator of the three-point function (12.2.46) of the Liouville theory, under the identification

$$\alpha_i = m_i + \frac{b + 1/b}{2}, \quad (\epsilon_1, \epsilon_2) = \left(b, \frac{1}{b}\right), \quad (12.5.15)$$

after substituting the definition (12.2.48) of the function  $\Upsilon$ . Most of the factors in the numerator can also be accounted for by identifying the two-dimensional operator

$$V_{\alpha_i} := \Upsilon(2\alpha_i)e^{2\alpha_i\phi} \quad (12.5.16)$$

with the puncture with mass  $m_i$  in the class S construction. Then, most of the mass-dependent terms of the Liouville three-point function is in the partition function of the trifundamental half-hypermultiplet. Let us denote this as an equation:

$$Z_{S^4}^{\text{trifund}}(m_1, m_2, m_3) = \langle V_{\alpha_1}(\infty)V_{\alpha_2}(1)V_{\alpha_3}(0) \rangle_{\text{Liouville}} \quad (12.5.17)$$

where the equality is up to a multiplication by functions independent of  $m_i$ .

Now, let us consider the four-punctured sphere. The corresponding four-dimensional theory is obtained by taking two trifundamentals, one for  $SU(2)_1 \times SU(2)_2 \times SU(2)$  and

another for  $SU(2) \times SU(2)_3 \times SU(3)_4$ , and coupling it to an  $SU(2)$  vector multiplet. The  $S^4$  partition function is, according to (12.4.15),

$$Z_{S^4}(m_1, m_2; m_3, m_4; \tau) = \frac{1}{2} \int da |q|^{2a^2} Z_{S^4}^{\text{trifund}}(m_1, m_2, a) Z_{S^4}^{\text{trifund}}(a, m_3, m_4) \times Z_{S^4}^{\text{gauge, one-loop}}(a) |Z_{n.p.}^{\text{instanton}}(a, m_i, q)|^2. \quad (12.5.18)$$

Here,  $m_i$  are the mass parameters for  $SU(2)_i$ ,  $Z_{n.p.}^{\text{instanton}}(a, m_i, q)$  is the instanton contribution from the north pole, and  $Z_{S^4}^{\text{gauge, one-loop}}(a)$  is the one-loop contribution from the gauge multiplet. Let us start with the gauge one-loop factor, which is

$$Z_{S^4}^{\text{gauge, one-loop}}(a) = \prod_{\pm} \frac{1}{\Gamma_2(\pm a | \epsilon_1, \epsilon_2) \Gamma_2(\pm a + \epsilon_1 \epsilon_2 | \epsilon_1, \epsilon_2)} = \Upsilon(a) \Upsilon(Q - a). \quad (12.5.19)$$

Together with the factors  $Z_{S^4}^{\text{trifund}}(m_1, m_2, a)$  and  $Z_{S^4}^{\text{trifund}}(a, m_3, m_4)$ , this provides the product of three-point functions in the expression of the Liouville four-point function (12.2.59).

This strongly suggests that the rest of the factors should match, namely, that the conformal block  $F$  in (12.2.59) and the instanton partition function  $Z_{n.p.}^{\text{instanton}}$  should agree:

$$F_{\alpha_1, \alpha_2, ip+Q/2, \alpha_3, \alpha_4}(q) \quad " = " \quad Z_{n.p.}^{\text{instanton}}(a, m_i, q) \quad (12.5.20)$$

under the identification

$$\alpha_i = m_i + \frac{Q}{2}, \quad ip + \frac{Q}{2} = a + \frac{Q}{2}. \quad (12.5.21)$$

The equality (12.5.20) almost works, in the following sense. As already mentioned in Sec. 12.4.3, we can only compute the instanton contribution of the  $U(2)$  gauge fields, for which no half-hypermultiplet exists, since the doublet and the anti-doublet are different for  $U(2)$ . The half-hypermultiplet in the trifundamental  $SU(2)_1 \times SU(2)_2 \times SU(2)$  with mass parameters  $m_1, m_2$  is regarded as two fundamental hypermultiplets in  $U(2)$ , with masses  $m_1 + m_2$  and  $-m_1 + m_2$ . The contribution from these two fundamental hypermultiplets can be computed using the formula (12.4.24) for the bifundamental of  $U(2) \times U(2)$ . Similarly, we regard the half-hypermultiplet in the trifundamental  $SU(2) \times SU(2)_3 \times SU(2)_4$  as two fundamental hypermultiplets in  $U(2)$ , with masses  $m_3 + m_4$  and  $m_3 - m_4$ .

The concrete version of (12.5.20) is then

$$Z_{n.p., U(2)}^{\text{instanton}}(a, m_i, q) = (1 - q)^{2(m_2 - Q/2)(Q/2 - m_3)} F_{\alpha_1, \alpha_2, ip+Q/2, \alpha_3, \alpha_4}(z). \quad (12.5.22)$$

The factor which is a fractional power of  $(1 - q)$  is the spurious contribution that is already alluded to in Sec. 12.4.3. The reader is advised at this point to compute both sides of the equation above to order  $q^2$  and check the equality. This can be done by using only the formulas already quoted in this review.<sup>3</sup>

---

<sup>3</sup>The author joined the collaboration that led to [2] at a rather late stage, and his contribution was only to provide the Mathematica code that does the instanton counting that was used to check this equality.

This spurious prefactor should be dropped for the physically correct version of the partition function, so we just set

$$Z_{n.p.,\text{corrected}}^{\text{instanton}}(a, m_i, q) = F_{\alpha_1, \alpha_2, ip+Q/2, \alpha_3, \alpha_4}(z). \quad (12.5.23)$$

We then have the equality

$$Z_{S^4}(m_1, m_2; m_3, m_4; \tau) = \langle V_{\alpha_1}(\infty)V_{\alpha_2}(1)V_{\alpha_3}(z)V_{\alpha_4}(0) \rangle_{\text{Liouville}} \quad (12.5.24)$$

where the equality is again up to multiplication by a function independent of  $m_i$  and  $z$ .<sup>4</sup>

This analysis can be extended to a linear quiver and a circular quiver with  $SU(2)^n$  gauge group. The restriction comes from our inability to compute the instanton partition function with a trifundamental half-hypermultiplet when all three  $SU(2)$ s couple to dynamical gauge fields.

### 12.5.3 Six-dimensional interpretation

Let us summarize what we saw so far. In Sec. 12.3, we introduced a class of four-dimensional  $\mathcal{N}=2$  theories associated to a Riemann surface with punctures. With  $n$  punctures, the corresponding theory has  $SU(2)^n$  flavor symmetry. In Sec. 12.5.1, we computed the partition function of these theories on  $S^1 \times S^3$ , using the formulas reviewed in Sec. 12.4.2. We found that it is equivalent to the two-dimensional  $q$ -deformed  $SU(2)$  Yang-Mills theory on the same Riemann surface that we recalled in Sec. 12.2.1

In Sec. 12.5.2, we computed the partition function of these theories on  $S^4$ , using the formulas reviewed in Sec. 12.4.3. We found that it is equivalent to the Liouville theory on the same Riemann surface that we recalled in Sec. 12.2.2. How should we understand these correspondences? We already gave the outline in Sec. 12.1. Here let us see slightly more details.

#### 6d $\mathcal{N}=(2,0)$ theory and 4d class S theories

We start from the six-dimensional  $\mathcal{N}=(2,0)$  theory of type  $SU(2)$ , and we put it on a Riemann surface  $C$ . Let us discuss a few features of this theory that will be important for us. When compactified on  $S^1$ , it becomes the maximally supersymmetric  $SU(2)$  Yang-Mills theory in five dimensions. The precise sense in which it ‘becomes’ the five-dimensional theory is hotly debated. One strange fact is that the instanton number of the five-dimensional theory should be identified with the Kaluza-Klein momentum of the six-dimensional theory on  $S^1$ . Practically, it is known that, as far as the quantities protected by the supersymmetry are concerned, we just have to include the supersymmetric instanton contributions in the

---

<sup>4</sup>For example, in (12.5.18) the integrand involves  $|q|^{2a^2}$  while in (12.2.59) the integrand involves  $|q|^{2a^2+Q^2/2}$ . Therefore, there is naively a mismatch (among others) of a factor  $|q|^{Q^2/2}$  between the two expressions. But note that  $\mathcal{N}=2$  supersymmetric theories on curved spaces such as  $S^4$  have local supersymmetric counterterms [32–34] that can change the partition function by a multiplication of the form  $|f(\tau)|$  where  $f$  is some holomorphic function. This ambiguity accounts for the mismatch  $|q|^{Q^2/2}$ .

computation. More details of this point can be found in Chapter 17. We should definitely *not* include Kaluza-Klein towers of massive fields in five dimensions, as it would lead to overcounting.

This six-dimensional theory has codimension-2 operators, such that on each one of them we have an  $SU(2)$  flavor symmetry. The reader would surely be already familiar with operators supported on points. Computing correlation functions of these point-operators is almost the first thing we learn in quantum field theory. Operators supported on lines are also quite familiar: in a four-dimensional gauge theory with gauge group  $G$ , we can consider the trace of the path-ordered exponential of the gauge field along a line  $L$ , in any representation  $R$  of  $G$ . This defines the Wilson line on  $L$  in the representation  $R$ . This introduces an external electrically charged particle whose worldline is  $L$ . Similarly, we can introduce an external magnetically charged particle on a given worldline: this determines a 't Hooft loop operator. The codimension-2 operator of the six-dimensional theory is similar: it extends along four directions in the six-dimensional spacetime. This four-dimensional subspace can have its own external  $SU(2)$  background field, coupled to its flavor symmetry.

So, given a Riemann surface  $C$  endowed with a metric and  $n$  chosen points  $p_i$  on it, we consider the spacetime of the form  $\mathbb{R}^{1,3} \times C$  and the  $\mathcal{N}=(2,0)$  theory of type  $SU(2)$  on it, together with a codimension-2 operator on  $\mathbb{R}^{1,3} \times p_i$  for each  $i$ . By making the area of  $C$  very small, this defines a four-dimensional theory with  $SU(2)^n$  flavor symmetry. To preserve a number of supersymmetry, we use the  $SO(5)_R$  symmetry of the  $\mathcal{N}=(2,0)$  theory. The curvature of  $C$  makes the spinor bundle over  $C$  non-trivial; but the supercharges of the six-dimensional theory is charged not only under the  $SO(2)$  metric curvature of  $C$  but under the  $SO(5)_R$  symmetry. So, we pick an  $SO(2)$  subgroup of  $SO(5)_R$ , and put a compensating curvature there, so that some of the supercharge lives in the trivial bundle over  $C$ . This method is often called the partial topological twisting.

The most naive choice would be to take the subgroup  $SO(2)_R \times SO(3)_R \subset SO(5)_R$ , and use this  $SO(2)_R$  for the partial topological twisting. The resulting theory is  $\mathcal{N}=2$  supersymmetric in four dimensions. This partial topological twisting has an additional feature that the most of the computable four-dimensional physics only depends on the total area and on the complex structure of the two-dimensional surface, and not on the detailed choice of the metric.

This allows us to perform the following operation: we pick a decomposition of the punctured Riemann surface into three-punctured spheres connected by a thin, long cylinders. For each of the cylinder, we first perform the reduction around  $S^1$ . Then, we just have the five-dimensional  $SU(2)$  super Yang-Mills on an edge, which gives a four-dimensional  $SU(2)$  gauge multiplet. The complexified coupling of the resulting gauge multiplet can be argued to be given by  $\tau$ , the complex parameter geometrically associated to the cylinder. For each of the three-punctured spheres, we have some four-dimensional  $\mathcal{N}=2$  theory with  $SU(2)^3$  symmetry: this is our favorite theory, i.e. the half-hypermultiplet in the trifundamental representation of  $SU(2)^3$ .

The four-dimensional theory  $\mathcal{S}(C)$  thus obtained is determined intrinsically by the two-dimensional Riemann surface  $C$  with punctures. The Riemann surface, however, has multiple decompositions into three-punctured spheres. Each of such decompositions gives rise to a

four-dimensional Lagrangian description. Starting with a genus  $g$  surface with  $n$  punctures, we always have  $3g - 3 + n$   $SU(2)$  gauge multiplets and  $2g - 2 + n$  half-hypermultiplets in the trifundamental, but the  $3g - 3 + n$  coupling constants of two different decompositions are related in a complicated manner, and the  $n$  flavor symmetries of various trifundamentals are permuted in an interesting way. Most often, an elementary field in one Lagrangian description arises as a monopole or a monopole bound state in another Lagrangian description.

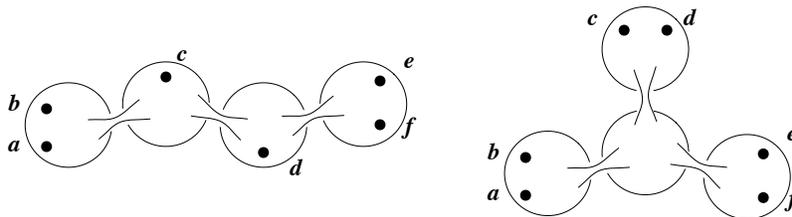

Figure 12.5.1: A sphere with six punctures under two different decompositions

As an illustration, consider a sphere with six punctures, see Fig. 12.5.1. This can be built from four three-punctured spheres connected by three tubes. Therefore the gauge group is  $SU(2)^3$  and there are four trifundamentals. The decomposition on the left and on the right are rather different, however. For example, one trifundamental coming from the sphere at the center of the decomposition on the right has all three  $SU(2)$  symmetries coupled to dynamical gauge fields. But we also know that these two decompositions can be continuously deformed to each other. This represents an S-duality from the 4d Lagrangian perspective.

### Alternative derivations of the correspondences

In Sec. 12.5.1 and Sec. 12.5.2, we computed the partition function of  $\mathcal{S}(C)$  on  $S^1 \times S^3$  and on  $S^4$ , and we found that it is given by two-dimensional  $q$ -deformed  $SU(2)$  Yang-Mills on  $C$  and by the Liouville theory on  $C$ . In view of the relation  $\mathcal{S}(X_4)(C_2) = \mathcal{S}(C_2)(X_4)$  when the partition function does not depend on the size, we now conclude that

$$\mathcal{S}(S^1 \times S^3) = \text{two-dimensional } q\text{-deformed } SU(2) \text{ Yang-Mills}, \quad (12.5.25)$$

$$\mathcal{S}(S^4) = \text{Liouville theory}. \quad (12.5.26)$$

See Fig. 12.5.2 for an illustration.

These two equalities are remarkable: usually in the physics literature, the equality is between numbers. Here, it is between quantum field theories! This, the author believes, shows our steady progress towards a better understanding of quantum field theories in general.

We have arrived at the two equations (12.5.25), (12.5.26) on  $\mathcal{S}(X_4)$  in a rather roundabout way, first by studying the four-dimensional theories  $\mathcal{S}(C)$ , second by computing their partition functions via localization, and finally by identifying the results with the known two-dimensional theories. Is there a more direct way to obtain these relations?

An obstacle is that we do not know the Lagrangian of the six-dimensional theory. A practical method to proceed is to use an  $S^1$  reduction first. When  $X_4 = S^1 \times S^3$ , we

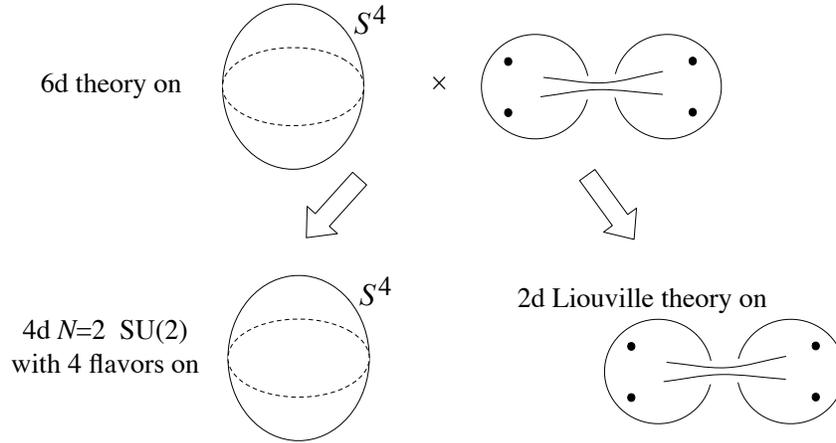

Figure 12.5.2: 6d theory on  $S^4 \times$  a Riemann surface, and its dimensional reduction

obviously have an  $S^1$ . We first compactify the six-dimensional theory on this  $S^1$ . Then we just have the five-dimensional super Yang-Mills on  $S^3$ . Its path integral can be localized to constant modes along  $S^3$ , and it essentially gives SU(2) Yang-Mills theory on the remaining two-directions. The one-loop fluctuations on  $S^3$  then gives a required modification to make it to the  $q$ -deformed Yang-Mills. This analysis was done in [36].

When  $X_4 = S^4$ , we do not directly see an  $S^1$ . But  $S^4$  can be seen as an  $S^3$  fibration over a segment, such that at the two ends  $S^3$  further degenerates. Now,  $S^3$  is an  $S^1$  fibration over  $S^2$ . So we can first reduce the system on this  $S^1$ . The system is now the five-dimensional SU(2) super Yang-Mills on an  $S^2$  fibration over a segment, with a funny boundary condition at both ends. The five-dimensional SU(2) super Yang-Mills on  $S^2$  can be localized to give an SL(2) Chern-Simons on the remaining three dimensions, and the boundary conditions at the end of the segments are such that its compactification down to two dimensions gives rise to the Liouville theory. The details can be found in the paper [37].

## 12.6 Future directions

At this point we have gone through the very basics of the 2d/4d correspondence: we started from the six-dimensional  $\mathcal{N}=(2,0)$  theory of type SU(2). Its compactification on a punctured Riemann surface can be given a Lagrangian description in terms of SU(2) vector multiplets and trifundamental half-hypermultiplets. We can then compute its partition function on  $S^1 \times S^3$  or on  $S^4$ . We saw that the partition function equals that of the two-dimensional  $q$ -deformed SU(2) Yang-Mills or that of the Liouville theory, respectively. We now have a way to understand this result by directly studying the six-dimensional theory on  $S^1 \times S^3$  or on  $S^4$ .

There are still gaps in our understanding in this basic case; and there are many avenues of generalizations. Let us conclude this review by going over these points. It would be a great pleasure for some of the readers to get involved and solve some of the problems mentioned; it

would be even more fantastic if some would open up new directions not even mentioned here.

### 12.6.1 Two unsolved problems in the $SU(2)$ case

In this most basic case, most of the mathematical relations, that are just claimed to hold in this review, have been even rigorously proved. The one big gap in our understanding on the Liouville theory side is in the localization of general class S theory of type  $SU(2)$  on  $S^4$ : we still do not know how to obtain the instanton contribution from a genuine half-hypermultiplet in the trifundamental of  $SU(2)^3$ , see e.g. [38]. Due to this problem, the  $S^4$  partition function can only be computed for linear or circular quivers. The author hopes an interested reader would find a way to proceed on this point.

On the side of  $S^1 \times S^3$  partition function, we only discussed a one-parameter slice of the general superconformal indices with three parameters  $(p, q, t)$ . In the two-parameter slice  $(p = 0, q, t)$ , it is known that the  $S^1 \times S^3$  partition function gives the  $(q, t)$ -deformed Yang-Mills theory, where the characters  $\chi_\lambda(a)$  in the Yang-Mills partition function are replaced by the Macdonald polynomials  $P_\lambda(a|q, t)$ . In the most general three-parameter case, the basic associativity of the four-point function was shown mathematically, but not as we did by rewriting the infinite product into an infinite sum, over a further generalization  $P_\lambda(a|p, q, t)$  of Macdonald polynomials, see e.g. [39].

### 12.6.2 More objects in the $SU(2)$ case

So far in this review, we only used one particular type of codimension-2 operators of the six-dimensional  $\mathcal{N}=(2, 0)$  theory of type  $SU(2)$ . It preserves the superconformal symmetry that maps the worldvolume of the operator to itself; such operator is often called regular. Compactifications on a Riemann surface with regular punctures give superconformal theories in four dimensions, and we discussed them exclusively up to this point.

There are also irregular codimension-2 operators, that breaks the superconformal symmetry. Compactifications with irregular punctures can lead to asymptotically-free theories in four dimensions, and also superconformal theories of a rather different type, called Argyres-Douglas theories. The  $S^4$  partition function of asymptotically-free theories can be written down, but that of the Argyres-Douglas theories are not well understood from the 4d point of view. The corresponding Liouville correlators are being explored, see e.g. [40, 41]. There was a progress in the understanding of the  $S^1 \times S^3$  partition functions of the Argyres-Douglas theories in 2015, see e.g. [42, 43].

The six-dimensional  $\mathcal{N}=(2, 0)$  theory of type  $SU(2)$  also has codimension-4 operators, labeled by irreducible  $SU(2)$  representations. The ones labeled by trivial 1-dimensional representation are trivial, and the basic nontrivial ones are labeled by the doublet representation. Recall the basic set-up of the 2d/4d correspondence, where we have the six-dimensional theory on  $X_4 \times C_2$ . As codimension-4 operators have two-dimensional world-volume, we can have the following three situations, roughly speaking:

- The operator extends in two directions in  $X_4$ , and sits at a point in  $C_2$ . This gives a

so-called surface operator of the four-dimensional theory. Its gauge theory description is by now well understood. In the Liouville theory this is an insertion of a degenerate operator. Its manifestation in the  $q$ -deformed Yang-Mills was studied in [44].

- The operator extends in one direction in  $X_4$ , and in one direction in  $C_2$ . This gives a line operator of the four-dimensional theory. In fact, all possible line operators of the class S theories of type  $SU(2)$  can be nicely described in this way. They also give line operators in the Liouville theory [45, 46].
- The operator sits at a point in  $X_4$ , and covers the entire  $C_2$ . This just gives a point-operator of the four-dimensional theory. When  $C_2$  is the three-punctured sphere, this operator is the trifundamental operator itself.

These appear to be more or less understood; they are more interesting when we generalize from  $SU(2)$  to something larger.

The codimension-2 operators can also be put into this setup in various ways:

- The operator extends in four directions in  $X_4$ , and sits at a point in  $C_2$ . This is the puncture we have been talking about, and changes the four-dimensional theory.
- The operator extends in three directions in  $X_4$ , and wraps a line in  $C_2$ . This should give a domain wall operator in the class S theory, but does not appear to have been studied.
- The operator extends in two directions in  $X_4$ , and wraps the entire  $C_2$ . This gives a surface operator in the four-dimensional theory, and changes the theory on  $C_2$ . When  $X_4 = S^4$ , the theory on  $C_2$  is the  $SL(2)$  WZW theory [47]; the instanton contribution was studied earlier [48].

### 12.6.3 Using 6d $\mathcal{N}=(2, 0)$ theories of other types

So far we only discussed the case where we start from the 6d  $\mathcal{N}=(2, 0)$  theory of type  $SU(2)$ . The 6d  $\mathcal{N}=(2, 0)$  theories are believed to fall into the ADE classification, i.e. there are theories of type  $G = A_n, D_n$  and  $E_{n=6,7,8}$ . We can put these theories on  $X_4 \times C_2$ , and have a lot of fun working out the resulting 2d/4d correspondences.

Without any additional objects in the setup,  $\mathcal{S}_G(S^1 \times S^3)$  gives the two-dimensional  $q$ -deformed Yang-Mills with gauge group  $G$ , or its  $(q, t)$  and  $(p, q, t)$  generalizations.  $\mathcal{S}_G(S^4)$  gives a natural generalization of the Liouville theory, known as the two-dimensional Toda theory of type  $G$ , which has a two-dimensional symmetry called the  $W_G$  algebra, that is a generalization of the Virasoro algebra.

In the  $\mathcal{N}=(2, 0)$  theory of type  $G$ , there are also codimension-2 and codimension-4 operators. The codimension-2 operators can be classified into regular ones and irregular ones. The latter are not very well understood, see e.g. [49]. The former are quite well understood: they are labeled by a homomorphism  $\mathfrak{su}(2) \rightarrow \mathfrak{g}$ , see e.g. [50]. The basic one is when the map sends the whole  $\mathfrak{su}(2)$  to zero. This is often called the full codimension-2 operator, and

is the one that appears when we split a Riemann surface into two. All the other regular codimension-2 operator can be obtained by giving a vev to the point-operators living on the codimension-2 operator.

The four-dimensional theories obtained by putting the six-dimensional  $\mathcal{N}=(2,0)$  theory of type  $G$  on a Riemann surface with punctures are called class S theories of type  $G$ . As always, they can be decomposed into the cylinders that basically give rise to  $G$  gauge multiplets in four dimensions, and the four-dimensional theory for each of the three-punctured spheres. The theory corresponding to the sphere with three full punctures is called the  $T_G$  theory, or  $T_N$  theory when  $G = \text{SU}(N)$ . The  $T_2$  theory is then the free theory of a half-hypermultiplet in the trifundamental of  $\text{SU}(2)^3$ . The other  $T_G$  theories do not admit, however, any useful Lagrangian description. In a sense the  $\text{SU}(2)$  case was the exception: the six-dimensional  $\mathcal{N}=(2,0)$  theory itself does not have any useful Lagrangian, and therefore we should not expect one in four dimensions in general.

This presents a big difficulty in the localization computation, since the localization only applies to the Lagrangian part of the theory. Fortunately, we can still apply the localization to the vector multiplets coming from the cylinders. For example, from this alone, we can conjecture that the instanton partition function of the  $G$  gauge theory when  $G$  is one of  $A_n$ ,  $D_n$  or  $E_{n=6,7,8}$  should be controlled by the  $W_G$  algebra. This aroused a not quite insignificant interest in the mathematics community, and is now rigorously proved [51–53]. However, the  $S^4$  partition function of the  $T_G$  theory is not yet known. Under the 2d/4d correspondence, this should map to the three-point function of the Toda theory of type  $G$  with general momenta. This is again not known unless  $G$  is of type  $\text{SU}(2)$ . Here we see the conservation law of the difficulty at work: something that is difficult on one side of the correspondence is also difficult on the other side. At the same time, we can say that a breakthrough on either side of the correspondence will have a huge impact on the other. The author hopes that an interested reader will do make such an epoch-making step. The  $S^1 \times S^3$  partition function of the  $T_G$  theory has been deduced from the associativity alone, at least in the two-dimensional  $(q, t)$  slice. This information has been used to understand the  $T_G$  theory better.

We can put a regular codimension-2 operator specified by a homomorphism  $\phi$  on  $S^4 \times C_2$  such that it wraps the entire  $C_2$  and occupy an  $S^2 \subset S^4$ . This is known to modify the  $W_G$  symmetry on  $C_2$  to a more general  $W$ -algebra  $W(G, \phi)$  obtained by the quantum Drinfeld-Sokolov reduction. But the two-dimensional theory itself has not been worked out.

Let us now briefly discuss codimension-4 operators of the six-dimensional theory of type  $G$ . They are labeled by irreducible representations of  $G$ . When three representations  $R_{1,2,3}$  have an invariant tensor  $\varphi : R_1 \otimes R_2 \otimes R_3 \rightarrow \mathbb{C}$ , we can consider a junction of three codimension-4 operator along a one-dimensional locus. We can place such a junction in  $X_4 \times C_2$  in many ways; analyzing the setup from the point of view of the four-dimensional theory on  $X_4$  and from that of the two-dimensional theory on  $C_2$  generate various correspondences, some of which have been worked out.

## 12.6.4 Other spacetimes, other theories

In this review, we only discussed putting the six-dimensional  $\mathcal{N}=(2,0)$  theory on a particular spacetime of the form  $X_4 \times C_2$ , where we perform the partial topological twist along  $C_2$  to have  $\mathcal{N}=2$  supersymmetry on  $X_4$ . In fact the choices we actually used in this review were even more restricted. Namely, we only considered just two cases,  $X_4 = S^1 \times S^3$  and  $X_4 = S^4$ . Clearly this very short list can be extended. There are a few works on  $X_4 = S^1 \times S^3/\mathbb{Z}_k$  and on  $X_4 = S^4/\mathbb{Z}_k$ . For example, the six-dimensional  $\mathcal{N}=(2,0)$  theory of type  $SU(2)$  on  $S^4/\mathbb{Z}_2$  is known to lead to the  $\mathcal{N}=(1,1)$  super Liouville theory on the two-dimensional side.

Another choice is to take compact complex toric surfaces as  $X_4$ . For this, the final formula of the localization computation was announced by Nekrasov in [54]; the details were recently provided by different authors in [55]. The corresponding two-dimensional theories labeled by  $X_4$  were not understood yet, though.

We can also consider non-compact complex surfaces as  $X_4$ . In this case we do not obtain a full-fledged 2d theory; rather, the supersymmetric localization on it gives rise to 2d chiral algebras. The case  $X_4 = \mathbb{R}^4$  was originally studied by [5] and gives the instanton contribution we discussed in Sec. 12.4.3. There are also various studies when  $X_4$  is an ALE space, which was pioneered by [56]. For a sample of references, see e.g. [57–76].<sup>5</sup>

We can of course consider other decompositions of the six-dimensional spacetime. For example, we can consider putting the six-dimensional  $\mathcal{N}=(2,0)$  theory on spacetimes of the form  $X_{6-d} \times C_d$  where we perform the partial topological twist along  $C_d$ , so that the preserved supersymmetry squared generates an isometry in  $X_{6-d}$ . Note that this setup is not symmetric under the exchange  $d \leftrightarrow 6-d$ . In this review we only discussed the case  $d=2$ ; the other cases  $d=3,4$  have been analyzed, mainly for six-dimensional  $\mathcal{N}=(2,0)$  theory of type  $SU(N)$ . For example, the reader can find some discussion on the 3d-3d case in Chapter 9. We can have even more fun by including various codimension-2 and codimension-4 operators into this general setup.

Just considering six-dimensional  $\mathcal{N}=(2,0)$  theories on product manifolds give us such plethora of correspondences of lower-dimensional quantum field theories that are being worked out. Then a natural direction would be to look for theories other than six-dimensional  $\mathcal{N}=(2,0)$  theories as the starting point. In six dimensions, there are many other  $\mathcal{N}=(1,0)$  supersymmetric theories that are believed to be ultraviolet complete. They are even less understood than  $\mathcal{N}=(2,0)$  theories, but there are recent activities to explore their properties systematically. Once basic features are understood, it should not be impossible to consider them on product manifolds, which hopefully would lead to completely new types of 4d-2d and other correspondences.

Of course we can start from lower-dimensional, more familiar gauge theories on product manifolds of the form  $X_{D-d} \times C_d$ . For example,  $\mathcal{N}=4$  super Yang-Mills theory with gauge group  $G$  was considered on the spacetime of the form  $X_2 \times C_2$ , with a partial topological twisting along  $C_2$ , and this is the basis of Witten’s approach to the geometric Langlands correspondence. The two-dimensional theory one obtains on  $X_2$  is a non-linear sigma model

---

<sup>5</sup>The author thanks F. Sala for the help in compiling this list of references.

on the moduli space of the  $G$ -Hitchin system on  $C_2$ , and does not seem to have a nice cut-and-paste description when  $C_2$  is split into two, as was possible in case of the four-dimensional class S theory. It sounds strange that a four-dimensional gauge theory with known Lagrangian behaves in a more complicated way upon compactification on  $C_2$  than a mysterious six-dimensional theory without Lagrangian behaves. The main difference seems to lie in the fact that the possible supersymmetric configuration of the gauge fields on the Riemann surface  $C_2$  is quite rich, since  $C_2$  can have various nontrivial one-cycles, around which the gauge fields can have nontrivial holonomies. In the case of the six-dimensional  $\mathcal{N}=(2,0)$  theory, we do not have a useful Lagrangian description; very naively, people say that it is a theory of non-abelian two-form fields. Whatever this statement means, it suggests that there can not be too much supersymmetric configuration on the Riemann surface  $C_2$ , since there is only one two-cycle in  $C_2$ . That said, having an explicit Lagrangian description at the starting point, it should in principle be possible to work out every aspect of the correspondences of the lower-dimensional field theories on  $X_{D-d}$  and on  $C_d$ , which the author thinks worth while to pursue.

## Acknowledgment

It is a pleasure to thank Tatsuma Nishioka for carefully reading the draft and giving various useful comments. This work is supported in part by JSPS Grant-in-Aid for Scientific Research No. 25870159 and in part by WPI Initiative, MEXT, Japan at IPMU, the University of Tokyo.

## References

- [1] V. Pestun and M. Zabzine, eds., *Localization techniques in quantum field theory*, vol. xx. Journal of Physics A, 2016. 1608.02952. <https://arxiv.org/src/1608.02952/anc/LocQFT.pdf>, <http://pestun.ihep.fr/pages/LocalizationReview/LocQFT.pdf>.
- [2] L. F. Alday, D. Gaiotto, and Y. Tachikawa, “Liouville Correlation Functions from Four-Dimensional Gauge Theories,” *Lett. Math. Phys.* **91** (2010) 167–197, [arXiv:0906.3219](https://arxiv.org/abs/0906.3219) [hep-th].
- [3] A. Gadde, L. Rastelli, S. S. Razamat, and W. Yan, “The 4D Superconformal Index from  $q$ -Deformed 2D Yang-Mills,” *Phys. Rev. Lett.* **106** (2011) 241602, [arXiv:1104.3850](https://arxiv.org/abs/1104.3850) [hep-th].
- [4] D. Gaiotto, “ $\mathcal{N} = 2$  Dualities,” *JHEP* **1208** (2012) 034, [arXiv:0904.2715](https://arxiv.org/abs/0904.2715) [hep-th].
- [5] N. A. Nekrasov, “Seiberg-Witten Prepotential from Instanton Counting,” *Adv. Theor. Math. Phys.* **7** (2004) 831–864, [arXiv:hep-th/0206161](https://arxiv.org/abs/hep-th/0206161).
- [6] V. Pestun, “Localization of Gauge Theory on a Four-Sphere and Supersymmetric Wilson Loops,” *Commun. Math. Phys.* **313** (2012) 71–129, [arXiv:0712.2824](https://arxiv.org/abs/0712.2824) [hep-th].
- [7] C. Romelsberger, “Counting Chiral Primaries in  $\mathcal{N} = 1$ ,  $d = 4$  Superconformal Field Theories,” *Nucl. Phys.* **B747** (2006) 329–353, [arXiv:hep-th/0510060](https://arxiv.org/abs/hep-th/0510060) [hep-th].
- [8] J. Kinney, J. M. Maldacena, S. Minwalla, and S. Raju, “An Index for 4 Dimensional Super Conformal Theories,” *Commun. Math. Phys.* **275** (2007) 209–254, [arXiv:hep-th/0510251](https://arxiv.org/abs/hep-th/0510251) [hep-th].

- [9] A. Gadde, L. Rastelli, S. S. Razamat, and W. Yan, “Gauge Theories and Macdonald Polynomials,” *Commun.Math.Phys.* **319** (2013) 147–193, [arXiv:1110.3740 \[hep-th\]](#).
- [10] S. Cordes, G. W. Moore, and S. Ramgoolam, “Lectures on 2-D Yang-Mills Theory, Equivariant Cohomology and Topological Field Theories,” *Nucl.Phys.Proc.Suppl.* **41** (1995) 184–244, [arXiv:hep-th/9411210 \[hep-th\]](#).
- [11] E. Buffenoir and P. Roche, “Two-Dimensional Lattice Gauge Theory Based on a Quantum Group,” *Commun.Math.Phys.* **170** (1995) 669–698, [arXiv:hep-th/9405126 \[hep-th\]](#).
- [12] A. Y. Alekseev, H. Grosse, and V. Schomerus, “Combinatorial Quantization of the Hamiltonian Chern-Simons Theory. 2.,” *Commun.Math.Phys.* **174** (1995) 561–604, [arXiv:hep-th/9408097 \[hep-th\]](#).
- [13] M. Aganagic, H. Ooguri, N. Saulina, and C. Vafa, “Black Holes,  $q$ -Deformed 2D Yang-Mills, and Non-Perturbative Topological Strings,” *Nucl.Phys.* **B715** (2005) 304–348, [arXiv:hep-th/0411280 \[hep-th\]](#).
- [14] N. Seiberg, “Notes on Quantum Liouville Theory and Quantum Gravity,” *Prog. Theor. Phys. Suppl.* **102** (1990) 319–349.
- [15] Y. Nakayama, “Liouville Field Theory: a Decade After the Revolution,” *Int. J. Mod. Phys.* **A19** (2004) 2771–2930, [arXiv:hep-th/0402009](#).
- [16] J. Teschner, “Liouville theory revisited,” *Class. Quant. Grav.* **18** (2001) R153–R222, [arXiv:hep-th/0104158](#).
- [17] H. Dorn and H. J. Otto, “Two and Three Point Functions in Liouville Theory,” *Nucl. Phys.* **B429** (1994) 375–388, [arXiv:hep-th/9403141](#).
- [18] A. B. Zamolodchikov and A. B. Zamolodchikov, “Structure Constants and Conformal Bootstrap in Liouville Field Theory,” *Nucl. Phys.* **B477** (1996) 577–605, [arXiv:hep-th/9506136](#).
- [19] B. Ponsot and J. Teschner, “Liouville Bootstrap via Harmonic Analysis on a Noncompact Quantum Group,” [arXiv:hep-th/9911110](#).
- [20] Y. Tachikawa, “ $\mathcal{N}=2$  supersymmetric dynamics for pedestrians,” *Lect. Notes Phys.* **890** (2013) 194, [arXiv:1312.2684 \[hep-th\]](#).  
<http://inspirehep.net/record/1268680/files/arXiv:1312.2684.pdf>.
- [21] G. Festuccia and N. Seiberg, “Rigid Supersymmetric Theories in Curved Superspace,” *JHEP* **1106** (2011) 114, [arXiv:1105.0689 \[hep-th\]](#).
- [22] T. Dumitrescu, “An Introduction to Supersymmetric Field Theories in Curved Space,” *Journal of Physics A* **xx** (2016) 000, [1608.02957](#).
- [23] L. Rastelli and S. Razamat, “The supersymmetric index in four dimensions,” *Journal of Physics A* **xx** (2016) 000, [1608.02965](#).
- [24] K. Hosomichi, “ $\mathcal{N} = 2$  SUSY gauge theories on  $S^4$ ,” *Journal of Physics A* **xx** (2016) 000, [1608.02962](#).
- [25] S. Nawata, “Localization of  $\mathcal{N} = 4$  Superconformal Field Theory on  $S^1 \times S^3$  and Index,” *JHEP* **1111** (2011) 144, [arXiv:1104.4470 \[hep-th\]](#).
- [26] N. Hama and K. Hosomichi, “Seiberg-Witten Theories on Ellipsoids,” *JHEP* **1209** (2012) 033, [arXiv:1206.6359 \[hep-th\]](#).
- [27] V. Pestun, “Localization for  $\mathcal{N} = 2$  Supersymmetric Gauge Theories in Four Dimensions,” in *New Dualities of Supersymmetric Gauge Theories*, J. Teschner, ed., pp. 159–194. Springer, 2016. [arXiv:1412.7134 \[hep-th\]](#).

- [28] Y. Tachikawa, “A review on instanton counting and  $W$ -algebras,” in *New Dualities of Supersymmetric Gauge Theories*, J. Teschner, ed., pp. 79–120. Springer, 2016. [arXiv:1412.7121 \[hep-th\]](#).
- [29] T. Okuda and V. Pestun, “On the Instantons and the Hypermultiplet Mass of  $\mathcal{N} = 2^*$  Super Yang-Mills on  $S^4$ ,” *JHEP* **1203** (2012) 017, [arXiv:1004.1222 \[hep-th\]](#).
- [30] J. Erickson, G. Semenoff, and K. Zarembo, “Wilson Loops in  $\mathcal{N} = 4$  Supersymmetric Yang-Mills Theory,” *Nucl.Phys.* **B582** (2000) 155–175, [arXiv:hep-th/0003055 \[hep-th\]](#).
- [31] N. Drukker and D. J. Gross, “An Exact Prediction of  $\mathcal{N} = 4$  SUSYM Theory for String Theory,” *J.Math.Phys.* **42** (2001) 2896–2914, [arXiv:hep-th/0010274 \[hep-th\]](#).
- [32] E. Gerchkovitz, J. Gomis, and Z. Komargodski, “Sphere Partition Functions and the Zamolodchikov Metric,” *JHEP* **1411** (2014) 001, [arXiv:1405.7271v2 \[hep-th\]](#).
- [33] J. Gomis and N. Ishtiaque, “Kähler Potential and Ambiguities in 4D  $\mathcal{N} = 2$  SCFTs,” [arXiv:1409.5325 \[hep-th\]](#).
- [34] J. Gomis, P.-S. Hsin, Z. Komargodski, A. Schwimmer, N. Seiberg, and S. Theisen, “Anomalies, Conformal Manifolds, and Spheres,” *JHEP* **03** (2016) 022, [arXiv:1509.08511 \[hep-th\]](#).
- [35] S. Kim and K. Lee, “Indices for 6 dimensional superconformal field theories,” *Journal of Physics A* **xx** (2016) 000, [1608.02969](#).
- [36] Y. Fukuda, T. Kawano, and N. Matsumiya, “5D SYM and 2D  $q$ -Deformed YM,” [arXiv:1210.2855 \[hep-th\]](#).
- [37] C. Cordova and D. L. Jafferis, “Toda Theory From Six Dimensions,” [arXiv:1605.03997 \[hep-th\]](#).
- [38] L. Hollands, C. A. Keller, and J. Song, “Towards a 4D/2D Correspondence for Sicilian Quivers,” *JHEP* **10** (2011) 100, [arXiv:1107.0973 \[hep-th\]](#).
- [39] S. S. Razamat, “On the  $\mathcal{N} = 2$  Superconformal Index and Eigenfunctions of the Elliptic RS Model,” *Lett.Math.Phys.* **104** (2014) 673–690, [arXiv:1309.0278 \[hep-th\]](#).
- [40] D. Gaiotto and J. Teschner, “Irregular Singularities in Liouville Theory and Argyres-Douglas Type Gauge Theories, I,” [arXiv:1203.1052 \[hep-th\]](#).
- [41] J. Gomis and B. Le Floch, “M2-brane surface operators and gauge theory dualities in Toda,” [arXiv:1407.1852 \[hep-th\]](#).
- [42] M. Buican and T. Nishinaka, “On the superconformal index of Argyres–Douglas theories,” *J. Phys.* **A49** (2016) no. 1, 015401, [arXiv:1505.05884 \[hep-th\]](#).
- [43] C. Cordova and S.-H. Shao, “Schur Indices, BPS Particles, and Argyres-Douglas Theories,” *JHEP* **01** (2016) 040, [arXiv:1506.00265 \[hep-th\]](#).
- [44] L. F. Alday, M. Bullimore, M. Fluder, and L. Hollands, “Surface Defects, the Superconformal Index and  $q$ -Deformed Yang-Mills,” [arXiv:1303.4460 \[hep-th\]](#).
- [45] L. F. Alday, D. Gaiotto, S. Gukov, Y. Tachikawa, and H. Verlinde, “Loop and Surface Operators in  $\mathcal{N} = 2$  Gauge Theory and Liouville Modular Geometry,” *JHEP* **1001** (2010) 113, [arXiv:0909.0945 \[hep-th\]](#).
- [46] N. Drukker, J. Gomis, T. Okuda, and J. Teschner, “Gauge Theory Loop Operators and Liouville Theory,” *JHEP* **02** (2010) 057, [arXiv:0909.1105 \[hep-th\]](#).
- [47] S. Nawata, “Givental J-functions, Quantum integrable systems, AGT relation with surface operator,” [arXiv:1408.4132 \[hep-th\]](#).
- [48] L. F. Alday and Y. Tachikawa, “Affine  $SL(2)$  Conformal Blocks from 4D Gauge Theories,” *Lett.Math.Phys.* **94** (2010) 87–114, [arXiv:1005.4469 \[hep-th\]](#).

- [49] D. Xie, “General Argyres–Douglas Theory,” *JHEP* **1301** (2013) 100, [arXiv:1204.2270 \[hep-th\]](#).
- [50] O. Chacaltana, J. Distler, and Y. Tachikawa, “Nilpotent Orbits and Codimension-Two Defects of 6D  $N=(2,0)$  Theories,” *Int.J.Mod.Phys.* **A28** (2013) 1340006, [arXiv:1203.2930 \[hep-th\]](#).
- [51] O. Schiffmann and E. Vasserot, “Cherednik algebras, W algebras and the equivariant cohomology of the moduli space of instantons on  $\mathbb{A}^2$ ,” *Publications mathématiques de l’IHÉS* **118** (2013) no. 1, 213–342, [arXiv:1202.2756 \[math.QA\]](#).
- [52] D. Maulik and A. Okounkov, “Quantum Groups and Quantum Cohomology,” [arXiv:1211.1287 \[math.AG\]](#).
- [53] A. Braverman, M. Finkelberg, and H. Nakajima, “Instanton Moduli Spaces and  $\mathcal{W}$ -Algebras,” [arXiv:1406.2381 \[math.QA\]](#).
- [54] N. Nekrasov, “Localizing gauge theories,” in *XIVth International Congress on Mathematical Physics*, J.-C. Zambrini, ed., pp. 645–654. Mar., 2006. <http://www.ihes.fr/~nikita/IMAGES/Lisbon.ps>.
- [55] M. Bershtein, G. Bonelli, M. Ronzani, and A. Tanzini, “Exact results for  $\mathcal{N} = 2$  supersymmetric gauge theories on compact toric manifolds and equivariant Donaldson invariants,” [arXiv:1509.00267 \[hep-th\]](#).
- [56] F. Fucito, J. F. Morales, and R. Poghossian, “Multi instanton calculus on ALE spaces,” *Nucl. Phys.* **B703** (2004) 518–536, [arXiv:hep-th/0406243](#).
- [57] F. Fucito, J. F. Morales, and R. Poghossian, “Instanton on toric singularities and black hole countings,” *JHEP* **12** (2006) 073, [arXiv:hep-th/0610154 \[hep-th\]](#).
- [58] L. Griguolo, D. Seminara, R. J. Szabo, and A. Tanzini, “Black holes, instanton counting on toric singularities and q-deformed two-dimensional Yang–Mills theory,” *Nucl. Phys.* **B772** (2007) 1–24, [arXiv:hep-th/0610155 \[hep-th\]](#).
- [59] R. Dijkgraaf and P. Sulkowski, “Instantons on ALE spaces and orbifold partitions,” *JHEP* **03** (2008) 013, [arXiv:0712.1427 \[hep-th\]](#).
- [60] V. Belavin and B. Feigin, “Super Liouville conformal blocks from  $N=2$   $SU(2)$  quiver gauge theories,” *JHEP* **07** (2011) 079, [arXiv:1105.5800 \[hep-th\]](#).
- [61] G. Bonelli, K. Maruyoshi, and A. Tanzini, “Instantons on ALE spaces and Super Liouville Conformal Field Theories,” [arXiv:1106.2505 \[hep-th\]](#).
- [62] A. Belavin, V. Belavin, and M. Bershtein, “Instantons and 2d Superconformal field theory,” *JHEP* **1109** (2011) 117, [arXiv:1106.4001 \[hep-th\]](#).
- [63] G. Bonelli, K. Maruyoshi, and A. Tanzini, “Gauge Theories on ALE Space and Super Liouville Correlation Functions,” [arXiv:1107.4609 \[hep-th\]](#).
- [64] N. Wyllard, “Coset conformal blocks and  $N=2$  gauge theories,” [arXiv:1109.4264 \[hep-th\]](#).
- [65] Y. Ito, “Ramond sector of super Liouville theory from instantons on an ALE space,” *Nucl.Phys.* **B861** (2012) 387–402, [arXiv:1110.2176 \[hep-th\]](#).
- [66] M. Alfimov and G. Tarnopolsky, “Parafermionic Liouville field theory and instantons on ALE spaces,” *JHEP* **1202** (2012) 036, [arXiv:1110.5628 \[hep-th\]](#).
- [67] A. Belavin, M. Bershtein, B. Feigin, A. Litvinov, and G. Tarnopolsky, “Instanton moduli spaces and bases in coset conformal field theory,” [arXiv:1111.2803 \[hep-th\]](#).
- [68] G. Bonelli, K. Maruyoshi, A. Tanzini, and F. Yagi, “ $N=2$  gauge theories on toric singularities, blow-up formulae and  $W$ -algebras,” [arXiv:1208.0790 \[hep-th\]](#).

- [69] A. Belavin, M. Bershtein, and G. Tarnopolsky, “Bases in coset conformal field theory from AGT correspondence and Macdonald polynomials at the roots of unity,” [arXiv:1211.2788 \[hep-th\]](#).
- [70] Y. Ito, K. Maruyoshi, and T. Okuda, “Scheme dependence of instanton counting in ALE spaces,” [arXiv:1303.5765 \[hep-th\]](#).
- [71] M. N. Alfimov, A. A. Belavin, and G. M. Tarnopolsky, “Coset conformal field theory and instanton counting on  $C^2/Z_p$ ,” *JHEP* **08** (2013) 134, [arXiv:1306.3938 \[hep-th\]](#).
- [72] H. Itoyama, T. Oota, and R. Yoshioka, “2d-4d Connection between  $q$ -Virasoro/W Block at Root of Unity Limit and Instanton Partition Function on ALE Space,” *Nucl. Phys.* **B877** (2013) 506–537, [arXiv:1308.2068 \[hep-th\]](#).
- [73] U. Bruzzo, M. Pedrini, F. Sala, and R. J. Szabo, “Framed sheaves on root stacks and supersymmetric gauge theories on ALE spaces,” *Adv. Math.* **288** (2016) 1175–1308, [arXiv:1312.5554 \[math.AG\]](#).
- [74] M. Pedrini, F. Sala, and R. J. Szabo, “AGT relations for abelian quiver gauge theories on ALE spaces,” *J. Geom. Phys.* **103** (2016) 43–89, [arXiv:1405.6992 \[math.RT\]](#).
- [75] L. Spodyneiko, “AGT correspondence: Ding-Iohara algebra at roots of unity and Lepowsky-Wilson construction,” *J. Phys.* **A48** (2015) 275404, [arXiv:1409.3465 \[hep-th\]](#).
- [76] U. Bruzzo, F. Sala, and R. J. Szabo, “ $\mathcal{N} = 2$  Quiver Gauge Theories on A-type ALE Spaces,” *Lett. Math. Phys.* **105** (2015) no. 3, 401–445, [arXiv:1410.2742 \[hep-th\]](#).
- [77] T. Dimofte, “Perturbative and nonperturbative aspects of complex Chern-Simons Theory,” *Journal of Physics A* **xx** (2016) 000, [1608.02961](#).

# Chapter 13

## The supersymmetric index in four dimensions

Leonardo Rastelli<sup>1</sup> and Shlomo S. Razamat<sup>2</sup>

<sup>1</sup> *C. N. Yang Institute for Theoretical Physics, Stony Brook University, Stony Brook, NY  
11794-3840, USA*

<sup>2</sup> *Department of Physics, Technion, Haifa, 32000, Israel*

leonardo.rastelli@stonybrook.edu, razamat@physics.technion.ac.il

### Abstract

We review the calculation and properties of the supersymmetric index for four dimensional  $\mathcal{N} = 1$  theories, illustrating its physical significance in several examples.

### Contents

|                                                    |            |
|----------------------------------------------------|------------|
| <b>13.1 Introduction</b>                           | <b>520</b> |
| <b>13.2 Definition of the index</b>                | <b>521</b> |
| 13.2.1 Index as a trace                            | 522        |
| 13.2.2 Index as a partition function               | 523        |
| 13.2.3 Computation of the index                    | 524        |
| <b>13.3 Index of sigma models</b>                  | <b>527</b> |
| <b>13.4 Index of gauge theories</b>                | <b>529</b> |
| <b>13.5 Index spectroscopy</b>                     | <b>534</b> |
| 13.5.1 An example                                  | 537        |
| <b>13.6 Dualities and Identities</b>               | <b>538</b> |
| 13.6.1 Symmetries and transformations of the index | 538        |
| 13.6.2 $\mathcal{N} = 4$ dualities                 | 540        |
| 13.6.3 Seiberg dualities                           | 541        |
| 13.6.4 Kutasov-Schwimmer dualities                 | 541        |

|                                                                   |            |
|-------------------------------------------------------------------|------------|
| <b>13.7 Limits</b> . . . . .                                      | <b>542</b> |
| 13.7.1 Small $\tau$ limit, $\mathbb{S}^1 \rightarrow 0$ . . . . . | 542        |
| 13.7.2 Large $\tau$ limit, $\mathbb{S}^3 \rightarrow 0$ . . . . . | 546        |
| 13.7.3 Poles and residues . . . . .                               | 548        |
| 13.7.4 Large $N$ limit . . . . .                                  | 551        |
| <b>13.8 Other topics and open problems</b> . . . . .              | <b>553</b> |
| <b>References</b> . . . . .                                       | <b>554</b> |

## 13.1 Introduction

The technique of supersymmetric localization allows to compute the partition functions of several supersymmetric field theories on certain compact manifolds preserving some of the supersymmetry. In favorable cases, the procedure of localization reduces the computation of the infinite dimensional path integral to a finite dimensional integral or to a discrete sum. Many of the computable supersymmetric partition functions in dimension  $d \leq 4$  are related to one another, see figure 1. The relations take two forms. First, different partition functions might be related by taking various limits of their parameters. For example, a partition function on a compact manifold can depend on the relative size of different components – sending that size to zero corresponds to computing a partition function of a theory in a lower dimension. Such limits are represented by solid lines in the figure. Second, partition functions on compact manifolds can sometimes be computed by gluing together partition functions on non-compact manifolds with prescribed boundary conditions at infinity. Different patterns of gluing of the same non-compact partition functions can lead to two different compact partition functions. For example, both the  $\mathbb{S}^2 \times \mathbb{S}^1$  partition function (the three-dimensional supersymmetric index) and the  $\mathbb{S}^3$  partition function are obtained by gluing partition functions on  $\mathbb{C} \times \mathbb{S}^1$ . Such relations are denoted by dashed lines in the figure. Some of the relations indicated in the figure are well studied while for others only some partial understanding is available.<sup>1</sup>

The main focus of this review article will be the  $\mathbb{S}^3 \times \mathbb{S}^1$  partition function, also known as the four-dimensional supersymmetric index, because it can be understood as the Witten index of the theory quantized on  $\mathbb{S}^3 \times \mathbb{R}$ , refined by fugacities that keep track of the relevant quantum numbers. This is the simplest and arguably the most important observable in the network of partition functions shown in figure 1. For theories that admit a Lagrangian description, the four-dimensional index can be obtained by solving a simple counting problem: one enumerates (with signs) local gauge invariant operators built from elementary fields in the four dimensional theory, in the limit of vanishing coupling. By contrast, the supersymmetric index in other dimensions gets contributions from more complicated objects, such as instantons in five dimensions, monopoles in three dimensions, and local supersymmetric

---

<sup>1</sup>This picture could be extended to a larger network of relations starting from higher dimensional theories – the  $\mathbb{S}^4$  partition function [2] (see Chapter 10), notably absent in figure 1, would be part of such an extended picture.

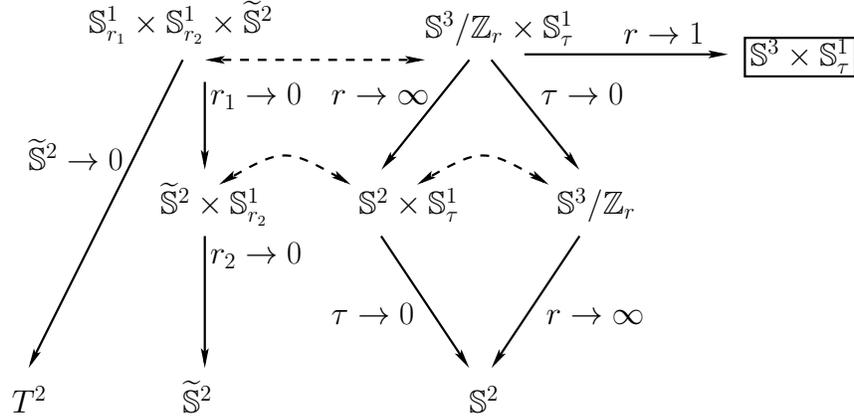

Figure 13.1.1: Different supersymmetric partition functions in dimensions 4, 3, 2 are related by limits of parameters (solid lines) and block decompositions (dashed lines). The  $\mathbb{S}^3 \times \mathbb{S}^1$  partition function (also known as the four-dimensional index) is one of the simplest and most useful partition functions.

defects in two dimensions. The four-dimensional counting problem is efficiently encoded by a simple matrix integral, which could be equivalently obtained by applying the recipe of supersymmetric localization to the  $\mathbb{S}^3 \times \mathbb{S}^1$  partition function. While the four-dimensional index is computationally simpler than other partition functions, its properties and the technology needed to extract physical information from it are of more universal applicability.

This review article is organized as follows. In section 2 we discuss the definition of the supersymmetric index and the prescription to compute it in any Lagrangian theory. In section 3 properties of the index of theories built from chiral fields with superpotential interactions are reviewed. In section 4 we discuss basic properties of the index of gauge theories. In section 5 we review superconformal representation theory and the way different multiplets are encoded in the index. In particular we review how to extract easily the spectrum of relevant and exactly marginal deformations. In section 6 we discuss briefly some of the mathematical properties of indices. In particular we review symmetries of the index and identities between indices of different looking theories related by dualities. In section 7 we review different physically important limits of the index. Finally, in section 8 we mention several topics not covered in detail in this review.

## 13.2 Definition of the index

There are two equivalent ways to define the supersymmetric index. It can be defined as the supersymmetric partition function on  $\mathbb{S}^3 \times \mathbb{S}^1$ , which depends holomorphically on two complex structure moduli (conventionally denoted  $p$  and  $q$ ) and on holonomies for background gauge fields coupling to the flavor symmetries of the theory. Alternatively, it is given by an

appropriately weighted trace over the states of the theory quantized on  $\mathbb{S}^3 \times \mathbb{R}$ . If the theory is conformal, one can use the state/operator map to interpret these states as local operators. Only in such cases it is appropriate to refer to the index as the *superconformal* index. There are many important examples of  $\mathcal{N} = 1$  superconformal field theories that can be reached as infrared fixed points of RG flows starting from weakly-coupled Lagrangian theories. One of the most useful properties of the index (most easily argued using its definition as a partition function) is its invariance under RG flow. This provides a powerful way to obtain the index of an IR fixed point, by performing a simple calculation in the UV.

### 13.2.1 Index as a trace

The index of a  $4d$  superconformal field theory is defined as the Witten index of the theory in radial quantization. Let  $\mathcal{Q}$  be one of the Poincaré supercharges, and  $\mathcal{Q}^\dagger = \mathcal{S}$  the conjugate conformal supercharge. Schematically, the index is defined as [4-6]

$$\mathcal{I}(\mu_i) = \text{Tr} (-1)^F e^{-\beta \delta} e^{-\mu_i \mathcal{M}_i}, \quad (13.2.1)$$

where the trace is over the Hilbert space of the theory quantized on  $\mathbb{S}^3$ ,  $\delta \equiv \frac{1}{2}\{\mathcal{Q}, \mathcal{Q}^\dagger\}$ ,  $\mathcal{M}_i$  are  $\mathcal{Q}$ -closed conserved charges and  $\mu_i$  the associated chemical potentials. Since states with  $\delta > 0$  come in boson/fermion pairs, only the  $\delta = 0$  states contribute, and the index is independent of  $\beta$ . There are infinitely many states with  $\delta = 0$  – this is true even for a single short irreducible representation of the superconformal algebra, because some of the non-compact generators (some of the spacetime derivatives) have  $\delta = 0$ . The introduction of the chemical potentials  $\mu_i$  serves both to regulate this divergence and to achieve a more refined counting.

For  $\mathcal{N} = 1$ , the supercharges are  $\{\mathcal{Q}_\alpha, \mathcal{S}^\alpha \equiv \mathcal{Q}^{\dagger\alpha}, \tilde{\mathcal{Q}}_{\dot{\alpha}}, \tilde{\mathcal{S}}^{\dot{\alpha}} \equiv \tilde{\mathcal{Q}}^{\dagger\dot{\alpha}}\}$ , where  $\alpha = \pm$  and  $\dot{\alpha} = \pm$  are respectively  $SU(2)_1$  and  $SU(2)_2$  indices, with  $SU(2)_1 \times SU(2)_2 = Spin(4)$  the isometry group of the  $\mathbb{S}^3$ . The relevant anticommutators are

$$\{\mathcal{Q}_\alpha, \mathcal{Q}^{\dagger\beta}\} = E + 2M_\alpha^\beta + \frac{3}{2}r \quad (13.2.2)$$

$$\{\tilde{\mathcal{Q}}_{\dot{\alpha}}, \tilde{\mathcal{Q}}^{\dagger\dot{\beta}}\} = E + 2\tilde{M}_{\dot{\alpha}}^{\dot{\beta}} - \frac{3}{2}r, \quad (13.2.3)$$

where  $E$  is the conformal Hamiltonian,  $M_\alpha^\beta$  and  $\tilde{M}_{\dot{\alpha}}^{\dot{\beta}}$  the  $SU(2)_1$  and  $SU(2)_2$  generators, and  $r$  the generator of the  $U(1)_r$  R-symmetry. In our conventions, the  $\mathcal{Q}$ s have  $r = -1$  and  $\tilde{\mathcal{Q}}$ s have  $r = +1$ , and of course the dagger operation flips the sign of  $r$ .

One can define two inequivalent indices, a “left-handed” index  $\mathcal{I}^L(t, y)$  and a “right-handed”

index  $\mathcal{I}^{\text{R}}(t, y)$ . For the left-handed index, we pick say<sup>2</sup>  $\mathcal{Q} \equiv \mathcal{Q}_-$ ,

$$\mathcal{I}^{\text{L}}(p, q) \equiv \text{Tr} (-1)^F p^{\frac{1}{3}(E+j_1)+j_2} q^{\frac{1}{3}(E+j_1)-j_2} = \text{Tr} (-1)^F p^{j_1+j_2-\frac{1}{2}r} q^{j_1-j_2-\frac{1}{2}r}, \quad \delta = E-2j_1+\frac{3}{2}r, \quad (13.2.4)$$

where  $j_1$  and  $j_2$  are the Cartan generators of  $SU(2)_1$  and  $SU(2)_2$ . The two ways of writing the exponent of  $t$  are equivalent since they differ by a  $\mathcal{Q}$ -exact term. For the right-handed index, we pick say  $\mathcal{Q} \equiv \tilde{\mathcal{Q}}_-$ ,

$$\mathcal{I}^{\text{R}}(p, q) \equiv \text{Tr} (-1)^F p^{\frac{1}{3}(E+j_2)+j_1} q^{\frac{1}{3}(E+j_2)-j_1} = \text{Tr} (-1)^F p^{j_1+j_2+\frac{1}{2}r} q^{j_2-j_1+\frac{1}{2}r}, \quad \delta = E-2j_2-\frac{3}{2}r. \quad (13.2.5)$$

One may also introduce chemical potentials for global symmetries of the theory which commute with the supersymmetry algebra and thus conserve the index property of the trace. Such fugacities can be turned on for continuous and/or discrete symmetries as we will see in what follows.<sup>3</sup>

If the theory is *not* conformal, and is described instead by an RG flow from a free UV fixed point to an IR fixed point, one can still define the index from (13.2.1), evaluating the trace over the local operators at the UV fixed point, but making sure that the allowed symmetries are preserved along the flow. (In particular, the R-charge assignments must correspond to a non-anomalous R symmetry). Since the index is an RG invariant, this gives a recipe to evaluate the superconformal index of the IR fixed point. At intermediate scales on the flow, the index is interpreted as the partition function on  $\mathbb{S}^3 \times \mathbb{S}^1$ , or equivalently, as the trace over the states of the theory quantized on  $\mathbb{S}^3$ .

## 13.2.2 Index as a partition function

Alternatively, the index can be defined as the supersymmetric partition function on  $\mathbb{S}^3 \times \mathbb{S}^1_\tau$ . As was argued in [8] (see also [9] any  $\mathcal{N} = 1$  supersymmetric theory can be put in a supersymmetric way on  $\mathbb{S}^3 \times \mathbb{S}^1_\tau$  provided it possesses anomaly free  $U(1)_r$  R symmetry. We refer to Chapter 5 for a detailed treatment and mention here only some of the salient points.

The  $\mathbb{S}^3 \times \mathbb{S}^1_\tau$  partition function depends holomorphically on the complex structure moduli  $p$  and  $q$ , and on the holonomies associated to flavor symmetries. It does *not* depend on gauge and superpotential couplings<sup>4</sup>, and is invariant under RG flow (Chapter 5). The partition function can be evaluated by localization techniques [11, 12], and the result is the same matrix integral that we will obtain in the next subsection by enumeration of gauge invariant operators.

<sup>2</sup>Picking  $\mathcal{Q} \equiv \mathcal{Q}_+$  would amount to the replacement  $j_1 \leftrightarrow -j_1$ , which is an equivalent choice because of  $SU(2)_1$  symmetry. The same consideration applies to the right-handed index, which can be defined either choosing  $\tilde{\mathcal{Q}}_-$  or  $\tilde{\mathcal{Q}}_+$ .

<sup>3</sup>One can consider additional generalizations of the index such as introduction of charge conjugation [7] to the trace but we will refrain from doing so here.

<sup>4</sup>But of course, the presence of a superpotential restricts the possible R charge assignments.

The precise equivalence of the trace formula for the index and the computation of the partition function requires a bit of care. When computing the index using the trace formula we implicitly normalize it so the vacuum (assuming it is unique) contributes +1 to the index. In particular in the large radius limit,  $\tau \rightarrow \infty$  the index computed as a counting problem receives only contributions from the vacua, and assuming there is a unique vacuum (preserving certain global symmetries) the index in the limit is 1. However, while computing the partition function in the large radius limit one finds a contribution coming from the Casimir energy of the theory,

$$\lim_{\tau \rightarrow \infty} \mathcal{Z}_{\mathbb{S}^3 \times \mathbb{S}^1} \sim e^{-\tau E_{\text{Casimir}}} . \quad (13.2.6)$$

The trace formulation of the index and the partition function formulation thus differ by the multiplicative factor  $e^{-\tau E_{\text{Casimir}}}$ . The Casimir energy can be computed from the trace formulation of the index [13–16],

$$E_{\text{Casimir}} = - \lim_{\tau \rightarrow \infty} \frac{d}{d\tau} \log \mathcal{I}(p = e^{-\tau\omega_1}, q = e^{-\tau\omega_2}, u_a = e^{im_a\tau}) \quad (13.2.7)$$

$$= \frac{2}{3}(a - c)(\omega_1 + \omega_2) + \frac{2}{27}(3c - 2a) \frac{(\omega_1 + \omega_2)^3}{\omega_1\omega_2} , \quad (13.2.8)$$

where  $a$  and  $c$  are the Weyl anomaly coefficients.

### 13.2.3 Computation of the index

By the state/operator correspondence the computation of the index of a conformal gauge theory proceeds by listing all the possible operators we can construct from modes of the fields and projecting out gauge non invariant ones. The different modes of the fields are usually called “letters” and the operators are words constructed using this alphabet.

The “letters” of an  $\mathcal{N} = 1$  chiral multiplet are enumerated in table 13.2.1. We assume that in the IR the  $U(1)_r$  charge of the lowest component of the multiplet  $\phi$  is some arbitrary  $r_{IR} = r$  (determined in a concrete theory by anomaly cancellation and in subtle cases  $a$ -maximization). According to the prescription we have just reviewed, the index receives contributions from the letters with  $\delta_{UV} = 0$ , and each letter contributes as  $(-1)^F p^{j_1+j_2-\frac{1}{2}r_{IR}} q^{j_1-j_2-\frac{1}{2}r_{IR}}$  to the left-handed index and as  $(-1)^F p^{j_1+j_2+\frac{1}{2}r_{IR}} q^{j_2-j_1+\frac{1}{2}r_{IR}}$  to the right-handed index. To keep track of the gauge and flavor quantum numbers, we introduce characters. We assume that the chiral multiplet transforms in the representation  $\mathcal{R}$  of the gauge  $\times$  flavor group, and denote by  $\chi_{\mathcal{R}}(U, V)$ ,  $\chi_{\bar{\mathcal{R}}}(U, V)$  the characters of  $\mathcal{R}$  and of the conjugate representation  $\bar{\mathcal{R}}$ , with  $U$  and  $V$  gauge and flavor group matrices respectively. All in all, the single-letter left- and right-handed indices for a chiral multiplet are [17]

$$i_{\chi(r)}^{\text{L}}(p, q, U, V) = \frac{(pq)^{\frac{1}{2}r} \chi_{\bar{\mathcal{R}}}(U, V) - (pq)^{\frac{2-r}{2}} \chi_{\mathcal{R}}(U, V)}{(1-p)(1-q)} \quad (13.2.9)$$

$$i_{\chi(r)}^{\text{R}}(p, q, U, V) = \frac{(pq)^{\frac{1}{2}r} \chi_{\mathcal{R}}(U, V) - (pq)^{\frac{2-r}{2}} \chi_{\bar{\mathcal{R}}}(U, V)}{(1-p)(1-q)} . \quad (13.2.10)$$

| Letters              | $E_{UV}$      | $j_1$            | $j_2$            | $r_{UV}$       | $r_{IR}$ | $\delta_{UV}^L$     | $\mathcal{I}^L$         | $\delta_{UV}^R$      | $\mathcal{I}^R$         |
|----------------------|---------------|------------------|------------------|----------------|----------|---------------------|-------------------------|----------------------|-------------------------|
| $\phi$               | 1             | 0                | 0                | $\frac{2}{3}$  | $r$      | 2                   | —                       | 0                    | $(pq)^{\frac{1}{2}r}$   |
| $\psi$               | $\frac{3}{2}$ | $\pm\frac{1}{2}$ | 0                | $-\frac{1}{3}$ | $r-1$    | $0^+, 2^-$          | $-(pq)^{\frac{2-r}{2}}$ | 2                    | —                       |
| $\partial\psi$       | $\frac{5}{2}$ | 0                | $\pm\frac{1}{2}$ | $-\frac{1}{3}$ | $r-1$    | 2                   | —                       | $4^+, 2^-$           | —                       |
| $\square\phi$        | 3             | 0                | 0                | $\frac{2}{3}$  | $r$      | 4                   | —                       | 2                    | —                       |
| $\bar{\phi}$         | 1             | 0                | 0                | $-\frac{2}{3}$ | $-r$     | 0                   | $(pq)^{\frac{1}{2}r}$   | 2                    | —                       |
| $\bar{\psi}$         | $\frac{3}{2}$ | 0                | $\pm\frac{1}{2}$ | $\frac{1}{3}$  | $-r+1$   | 2                   | —                       | $2^+, 0^-$           | $-(pq)^{\frac{2-r}{2}}$ |
| $\partial\bar{\psi}$ | $\frac{5}{2}$ | $\pm\frac{1}{2}$ | 0                | $\frac{1}{3}$  | $-r+1$   | $2^+, 4^-$          | —                       | 2                    | —                       |
| $\square\bar{\phi}$  | 3             | 0                | 0                | $-\frac{2}{3}$ | $-r$     | 2                   | —                       | 4                    | —                       |
| $\partial_{\pm\pm}$  | 1             | $\pm\frac{1}{2}$ | $\pm\frac{1}{2}$ | 0              | 0        | $0^{\pm}, 2^{\pm-}$ | $p, q$                  | $0^{+\pm}, 2^{-\pm}$ | $p, q$                  |

Table 13.2.1: The “letters” of an  $\mathcal{N} = 1$  chiral multiplet and their contributions to the index. Here  $\delta^L = E - 2j_1 + \frac{3}{2}r_{UV}$  and  $\delta_{UV}^R = E - 2j_2 - \frac{3}{2}r_{UV}$ . A priori we have to take into account the free equations of motion  $\partial\psi = 0$  and  $\square\phi = 0$ , which imply constraints on the possible words, but we see that in this case equations of motions have  $\delta_{UV} \neq 0$  so they do not change the index. Finally there are two spacetime derivatives contributing to the index, and their multiple action on the fields is responsible for the denominator of the index,  $\frac{1}{(1-p)(1-q)} = \sum_{n,m=0}^{\infty} p^n q^m$ .

The denominators encode the action of the two spacetime derivatives with  $\delta = 0$ . Note that the left-handed and right-handed indices differ by conjugation of the gauge and flavor quantum numbers. As a basic consistency check [6], consider a single free massive chiral multiplet (no gauge or flavor indices). In the UV, we neglect the mass deformation and as always  $r_{UV} = \frac{2}{3}$ . In the IR, the quadratic superpotential implies  $r_{IR} = 1$ , and one finds  $i_{r=1}^L = i_{r=1}^R \equiv 0$ . As expected, a massive superfield decouples and does not contribute to the IR index.

Finding the contribution to the index of an  $\mathcal{N} = 1$  vector multiplet is even easier, since the  $R$ -charge of a vector superfield  $W_\alpha$  is fixed at the canonical value  $+1$  all along the flow. For both left- and the right-handed index, the single-letter index of a vector multiplet is [4]

$$i_V(p, q, U) = \frac{2pq - p - q}{(1-p)(1-q)} \chi_{adj}(U). \quad (13.2.11)$$

Armed with the single-letter indices, the full index is obtained by enumerating all the words and then projecting onto gauge-singlets by integrating over the Haar measure of the gauge group. Schematically,

$$\mathcal{I}(t, y, V) = \int [dU] \prod_k \text{PE}[i_k(p, q, U, V)], \quad (13.2.12)$$

where  $k$  labels the different supermultiplets, and  $\text{PE}[i_k]$  is the plethystic exponential of the single-letter index of the  $k$ -th multiplet. The plethystic exponential,

$$\text{PE}[i_k(t, y, U, V)] \equiv \exp \left\{ \sum_{m=1}^{\infty} \frac{1}{m} i_k(p^m, q^m, V^m) \chi_{\mathcal{R}_k}(U^m, V^m) \right\}, \quad (13.2.13)$$

implements the combinatorics of symmetrization of the single letters, see *e.g.* [18, 19]. As usual, one can gauge fix the integral over the gauge group and reduce it to an integral over the maximal torus, with the usual extra factor arising of van der Monde determinant.

The multi-letter contribution to the index of a chiral multiplet (the plethystic exponential of its single-letter index) can be elegantly written as a product of elliptic Gamma functions [17]. For a chiral superfield in the fundamental representation  $\square$  of  $SU(N_c)$ , and with IR R-charge equal to  $r$ , one has

$$\begin{aligned} \text{PE}[i_r(p, q, U)] &\equiv \prod_{i=1}^{N_c} \Gamma((pq)^{\frac{1}{2}r} z_i; p, q), \\ \Gamma(z; p, q) &\equiv \prod_{k,m=0}^{\infty} \frac{1 - p^{k+1} q^{m+1} / z}{1 - p^k q^m z}. \end{aligned} \quad (13.2.14)$$

Here  $\{z_k\}$ ,  $k = 1, \dots, N_c$  are complex numbers of unit modulus, obeying  $\prod_{k=1}^{N_c} z_k = 1$ , which parametrize the Cartan subalgebras of  $SU(N_c)$ .

Similarly, the multi-letter contribution of a vector multiplet in the adjoint of  $SU(N)$  combines with the  $SU(N)$  Haar measure to give the compact expression [17, 20]

$$\frac{\kappa^{N-1}}{N!} \oint_{\mathbb{T}^{N-1}} \prod_{i=1}^{N-1} \frac{dz_i}{2\pi i z_i} \prod_{k \neq \ell} \frac{1}{\Gamma(z_k/z_\ell; p, q)} \cdots \quad (13.2.15)$$

The dots indicate that this is to be understood as a building block of the full matrix integral. Here  $\kappa$  is taken to be,

$$\kappa \equiv (p; p)(q; q) \quad (13.2.16)$$

where  $(a; b) \equiv \prod_{k=0}^{\infty} (1 - ab^k)$ . Note that  $\kappa$  is the index of  $U(1)$  free vector multiplet and we will sometimes denote  $\kappa = \mathcal{I}_V$ . We will often leave implicit the  $q$  and  $p$  dependence of the elliptic gamma functions,  $\Gamma(z; p, q) \rightarrow \Gamma(z)$ . Also, we will often use the shorthand notation

$$\Gamma(Az^{\pm 1}) \equiv \Gamma(Az)\Gamma(Az^{-1}). \quad (13.2.17)$$

If the gauge group of the theory has abelian factors, one can turn on FI terms. On  $\mathbb{S}^3 \times \mathbb{S}_\tau^1$  such FI terms should be quantized [21]. Indeed, on  $\mathbb{S}^3 \times \mathbb{R}$  with sphere of radius  $r_3$  the FI parameter  $\zeta$  appears in the action as,

$$\zeta \int d^4x \sqrt{g} (D - \frac{2i}{r_3} A_4), \quad (13.2.18)$$

where  $A_4$  is the component of the gauge field along  $\mathbb{R}$  and  $D$  is the auxiliary field of the  $\mathcal{N} = 1$  vector multiplet. Upon compactification of  $\mathbb{R}$  to  $\mathbb{S}_\tau^1$  we have to insure that this term is invariant under large gauge transformations,  $A_4 \rightarrow A_4 + \frac{1}{\tau}$ . Under such a transformation,

$$\zeta \int d^4x \sqrt{g} (D - \frac{2i}{r_3} A_4) \rightarrow \zeta \int d^4x \sqrt{g} (D - \frac{2i}{r_3} A_4) + 8\pi^3 i \zeta r_3^3, \quad (13.2.19)$$

which implies that  $\zeta = \frac{1}{4\pi^2 r_3^3} n$  with  $n \in \mathbb{Z}$ . The FI parameter for the  $U(1)_u$  gauge factor will introduce the term  $u^n$  in the matrix integral that computes the index.

The index does not depend on any continuous coupling of the theory. However, the functional form of the superpotential restricts the possible global symmetries and hence the fugacities that the index can depend on. In turning on a certain set of fugacities, we are computing the index for all possible choices of superpotentials consistent with the symmetries associated to those fugacities.

### 13.3 Index of sigma models

We now turn to discuss basic properties of the index of some of simplest  $\mathcal{N} = 1$  theories: sigma models built from chiral fields with no gauge interactions.

- *Mass terms* – Invariance along the RG flow is a basic property of the index. A simple implication is that the index for a massive theory with a single supersymmetric vacuum must be equal to 1. Let's check this fact in the theory of two chiral fields with a superpotential mass term

$$W = m Q_a Q_b. \quad (13.3.1)$$

As the superpotential has R-charge two, the R-charges of the two fields satisfy

$$r_a + r_b = 2. \quad (13.3.2)$$

Moreover there is one  $U(1)$  symmetry under which the two fields are oppositely charged. Let us turn on a fugacity  $u$  for this symmetry and assign charge +1 to field  $a$ . From our general rules, the index of this theory is

$$\Gamma((pq)^{\frac{1}{2}r_a}u)\Gamma((pq)^{\frac{1}{2}(2-r_a)}u^{-1}) = \prod_{i,j=0}^{\infty} \frac{1 - (pq)^{1-\frac{1}{2}r_a}p^i q^j u^{-1}}{1 - (pq)^{\frac{1}{2}r_a}p^i q^j u} \prod_{i,j=0}^{\infty} \frac{1 - (pq)^{1-\frac{1}{2}(2-r_a)}p^i q^j u}{1 - (pq)^{\frac{1}{2}(2-r_a)}p^i q^j u^{-1}} = 1, \quad (13.3.3)$$

as expected.

- *F-term supersymmetry breaking* – As another degenerate example, consider the theory of a chiral field with linear superpotential,  $W = \eta Q$ , the Polonyi model. This model has no supersymmetric vacuum and thus breaks supersymmetry spontaneously. The field  $Q$  has R-charge 2 and is not charged under any global symmetry. The index is

$$\Gamma(pq) = 0, \quad (13.3.4)$$

consistently with the absence of a supersymmetric vacuum. The vanishing the index can be traced to the presence of a fermionic letter that contributes -1 (see Table 1): this mode should be interpreted as the Goldstino of supersymmetry breaking. In general, models with

spontaneous supersymmetry breaking of O’Raifeartaigh type will involve fields with R-charge two neutral under all global symmetries – resulting in a vanishing index.

- *Runaway vacuum* – We can consider a slight modification of the above model to restore the supersymmetric vacuum but at infinity in field space. We take

$$W = \eta Q + \frac{1}{2} \lambda Q^2 S. \quad (13.3.5)$$

The potential of this model has a minimum at zero as  $S$  goes to infinity – a runaway behavior. Indeed, the F-term equations read

$$\eta + \lambda QS = 0, \quad Q^2 = 0. \quad (13.3.6)$$

The vacuum is reached by taking the limit

$$Q \rightarrow 0, \quad S \rightarrow \infty, \quad QS = -\frac{\eta}{\lambda}. \quad (13.3.7)$$

The field  $Q$  has R-charge +2 and contributes zero to the index (because of the fermionic zero mode mentioned above), while  $S$  has R-charge  $-2$  and contributes infinity, making the index of this model ill-defined. The divergence in the index of the  $S$  field can be traced to the existence of a bosonic zero mode, namely  $\partial_{-+} \partial_{++} \phi$ , which contributes in the plethystic exponential with weight 1 (see Table 1). As we will soon discuss, divergences in the index signal the appearance of flat directions. In this example, the vacuum at infinity has a flat direction since the F-term equations are projective – it is this flat direction that gives rise to the divergent contribution.

- *Non-trivial chiral ring* – Next, let us consider a superpotential of the form  $W = \lambda Q^{h+1}$  for some integer  $h$ . This model has a chiral ring relation  $Q^h \sim 0$ . The field  $Q$  has R-charge  $\frac{2}{h+1}$ , it is not charged under any continuous global symmetries, but can carry charge under  $\mathbb{Z}_{h+1}$ . Let us denote by  $g$  ( $g^{h+1} = 1$ ) the fugacity for  $\mathbb{Z}_{h+1}$  and write the index of this model as

$$\Gamma((pq)^{\frac{1}{1+h}} g) = \text{PE} \left[ \frac{(pq)^{\frac{1}{1+h}} g - ((pq)^{\frac{1}{1+h}} g)^h}{(1-p)(1-q)} \right]. \quad (13.3.8)$$

Recall that the numerator in the plethystic exponential of a chiral field comes from the bosonic mode  $\phi$  and a fermionic mode  $\bar{\psi}$ , while the denominator comes from the derivatives,  $\partial_{\pm+}$ . Note that  $\bar{\psi}$  contributes to the index the  $h$ th power of the contribution of  $\phi$  with an opposite sign. This implies that the contribution of  $\phi^h$  is cancelled by the contribution of  $\bar{\psi}$ , in accordance with the chiral ring relation discussed above.

## 13.4 Index of gauge theories

• *D-term supersymmetry breaking* – Let us first discuss the simplest gauge theory,  $U(1)$  theory with an FI parameter  $\zeta$ , which as we discussed should be integer. The index of this model is given by

$$\kappa \oint \frac{dz}{2\pi iz} z^\zeta = \kappa \delta_{\zeta,0}. \quad (13.4.1)$$

For non-zero FI parameter the index vanishes, signalling D-term supersymmetry breaking. As we discussed in the previous section, pairs of chiral fields with a mass term superpotential do not affect the index. The index (13.4.1) can then be interpreted as the index of a  $U(1)$  gauge theory with any number of such pairs. Although the details of the dynamics of the model may depend on existence of such fields and on the relative values of the gauge coupling/FI term and masses, the index is always zero, capturing only the fact that supersymmetry is broken.

• *IR duality* –  $\mathcal{N} = 1$  gauge theories in four dimensions exhibit a variety of remarkable properties one of which is the ubiquity of IR dualities first discussed by Seiberg [22]. A basic example is  $\mathcal{N} = 1$   $SU(2)$  gauge theory with three flavors of fundamental and anti-fundamental quarks. This theory flows in the IR to a free theory in which is given by a sigma model of the collection of the mesonic and baryonic fields. The index of this gauge theory is given by

$$\mathcal{I}_{gauge} = \kappa \oint \frac{dz}{4\pi iz} \frac{1}{\Gamma(z^{\pm 2})} \prod_{i=1}^3 \Gamma((pq)^{\frac{1}{6}} b u_i z^{\pm 1}) \Gamma((pq)^{\frac{1}{6}} b^{-1} v_i z^{\pm 1}). \quad (13.4.2)$$

Here  $\prod_{i=1}^3 u_i = \prod_{i=1}^3 v_i = 1$ , with these fugacities parametrizing the  $SU(3)_u \times SU(3)_v$  flavor symmetry rotating the fundamental and anti-fundamental quarks, while  $b$  parametrizes the baryonic  $U(1)_b$ . The distinction between fundamental and anti-fundamental matter here is artificial because of the pseudo-reality of the representations and is motivated by higher rank generalizations. In particular the  $SU(3)_u \times SU(3)_v \times U(1)_b$  flavor symmetry enhances to  $SU(6)_t$  with  $\{t_i\} = \{b u_i, b^{-1} v_i\}$ . The index of the free mesons and baryons is given by

$$\mathcal{I}_{sigma} = \prod_{i < j} \Gamma((pq)^{\frac{1}{3}} t_i t_j). \quad (13.4.3)$$

If the index is to be independent of the RG flow  $\mathcal{I}_{gauge}$  should be equal to  $\mathcal{I}_{sigma}$ , which is indeed a proven mathematical fact. This identity is known as Spiridonov's beta function identity in math literature [23]. On the sigma model side we have fifteen chiral fields but the flavor symmetry has only rank five. The remaining symmetries rotating the chiral fields are broken by the superpotential which is the Pfaffian of the antisymmetric matrix one can build from these fields. This superpotential is encoded in the index through the restriction of the fugacities to the ones of the  $SU(6)_t$  symmetry.

In evaluating the index, we have used the anomaly free R-charges for the quarks,  $R = \frac{1}{3}$ . Mathematically, the anomaly free condition translates into a constraint on the arguments of

the Gamma functions appearing in the numerator of the integrand. In this case we have,

$$\prod_{i=1}^6 ((pq)^{\frac{1}{6}} t_i) = pq. \quad (13.4.4)$$

Such constraints are called balancing conditions in the math literature [24].

- *Higgsing/mass deformations* – As discussed above, giving a mass to a pair of chiral fields trivializes their contribution to the index. If the theory has a dual IR description, the mass deformation corresponds to turning on a vacuum expectation value that Higgses the gauge symmetry on the other side of the duality. Let us discuss how this happens at the level of the index in a simple example. We consider theory A to be an  $SU(2)$  gauge theory with four flavors. This model has an  $SU(4)_u \times SU(4)_v \times U(1)_b$  flavor symmetry. Its index is given

$$\mathcal{I}_A(\mathbf{u}, \mathbf{v}, b) = \kappa \oint \frac{dz}{4\pi iz} \frac{1}{\Gamma(z^{\pm 2})} \prod_{i=1}^4 \Gamma((pq)^{\frac{1}{4}} b u_i z^{\pm 1}) \Gamma((pq)^{\frac{1}{4}} b^{-1} v_i z^{\pm 1}), \quad (13.4.5)$$

where the fugacities satisfy the  $SU(4)$  constraint

$$\prod_{i=1}^4 u_i = \prod_{i=1}^4 v_i = 1. \quad (13.4.6)$$

This model enjoys an IR duality. The Seiberg dual of it is a gauge theory with same rank and same charged matter content. However the charges of the quarks under global symmetries are different, they are in the conjugate representation of the  $SU(3)_u \times SU(3)_v$  flavor group. There are moreover gauge singlet fields having same charges as the mesons of the theory on side A and coupling to the mesons of the gauge theory on side B through a superpotential. The index of the theory on side B is

$$\mathcal{I}_B(\mathbf{u}, \mathbf{v}, b) = \mathcal{I}_A(\mathbf{u}^{-1}, \mathbf{v}^{-1}, b) \prod_{i,j=1}^4 \Gamma((pq)^{\frac{1}{2}} u_i v_j). \quad (13.4.7)$$

The product over the Gamma functions is the product over the singlet fields. Thanks to an identity proved by Rains [25], the indices on side A and side B coincide

$$\mathcal{I}_A = \mathcal{I}_B, \quad (13.4.8)$$

as expected from the duality. Again it was important here to use the anomaly free R-charges for the fields.

Let us now consider giving a mass to a pair of quarks on side A. This should give us the  $SU(2)$  gauge theory with three flavors we discussed in the previous bullet. We break the flavor symmetry from  $SU(3)_u \times SU(3)_v$  down to  $SU(2)_u \times SU(2)_v$ . This breaking of symmetry through mass terms is encoded in the index by specializing the corresponding fugacities. For example, let us turn on a mass term  $m Q_1 \tilde{Q}_1$ . The weight of the mesonic

operator  $Q_1\tilde{Q}_1$  in the index before turning on the mass term is  $(pq)^{\frac{1}{2}}u_1v_1$ . After turning on the mass it should be  $pq$  corresponding to R-charge +2 and no other charges. Thus turning on the mass term in the index corresponds to specializing the fugacities to be

$$u_1v_1 = (pq)^{\frac{1}{2}}. \quad (13.4.9)$$

We now define  $u_1 = (pq)^{\frac{1}{4}}a$ ,  $v_1 = (pq)^{\frac{1}{4}}a^{-1}$ , and find from (13.4.6),

$$\prod_{i=2}^4 u_i = (pq)^{-\frac{1}{4}}a^{-1}, \quad \prod_{i=2}^4 v_i = (pq)^{-\frac{1}{4}}a. \quad (13.4.10)$$

Redefining

$$u_i \equiv \tilde{u}_{i-1}(pq)^{-\frac{1}{12}}a^{-\frac{1}{3}}, \quad v_i \equiv \tilde{v}_{i-1}(pq)^{-\frac{1}{12}}a^{\frac{1}{3}}, \quad b = \tilde{b}a^{\frac{1}{3}}, \quad (13.4.11)$$

we obtain

$$\prod_{i=1}^3 \tilde{u}_i = \prod_{i=1}^3 \tilde{v}_i = 1. \quad (13.4.12)$$

After mass deformation, the index on side A becomes

$$\mathcal{I}_A \rightarrow \kappa \oint \frac{dz}{2\pi iz} \frac{1}{\Gamma(z^{\pm 1})} \prod_{i=1}^3 \Gamma((pq)^{\frac{1}{6}}\tilde{b}\tilde{u}_i z^{\pm 1}) \Gamma((pq)^{\frac{1}{6}}\tilde{b}^{-1}\tilde{v}_i z^{\pm 1}), \quad (13.4.13)$$

which coincides with (13.4.2) as expected.

Let us now discuss what happens on side B of the duality. Here the physics is more interesting. We gave a mass field to the meson  $Q_1\tilde{Q}_1$  on side A of the duality. On side B it maps to a singlet field,  $M_{11}$ , and thus the mass deformation adds a linear term to the superpotential. The superpotential involving the field  $M_{11}$  is thus of the form

$$mM_{11} + q_1\tilde{q}_1M_{11}, \quad (13.4.14)$$

where  $q_i$  and  $\tilde{q}_i$  are the quarks of the side B of the duality. The F-term equation thus impose a vacuum expectation value for the meson  $q_1\tilde{q}_1$ . Turning such a vev Higgses the gauge  $SU(2)$  gauge group and brings us to the sigma model of the previous bullet. Let us see what happens at the level of the index. The singlet  $M_{11}$  contributes to the index as  $\Gamma((pq)^{\frac{1}{2}}u_1v_1)$  and thus setting the fugacities to satisfy (13.4.9) turns this into  $\Gamma(pq)$  which is vanishing. Let us analyze carefully what happens to the  $SU(2)$  integral in (13.4.7). The integrand here has many poles in  $z$ . For example there are two poles coming from  $\Gamma((pq)^{\frac{1}{4}}bu_1z^{\pm 1})$  and two poles from  $\Gamma((pq)^{\frac{1}{4}}b^{-1}v_1z^{\pm 1})$  located at

$$z^{\pm 1} = (pq)^{\frac{1}{4}}bu_1, \quad (pq)^{\frac{1}{4}}bv_1. \quad (13.4.15)$$

Two of these poles are inside the  $z$  integration contour and two are outside. Note then that if we specialize the fugacities to satisfy (13.4.9) these four poles pinch the integration contour pairwise producing a divergence. The leading, divergent, contribution to the integral in the

mass limit we consider thus comes only from two poles in the  $z$  integral. These two poles are related by Weyl symmetry in the limit and thus give the same residues. The divergence coming from the pinching is precisely canceled against the zero coming from the meson  $M_{11}$  in the mass limit. The index on side B in the limit is given then by

$$\begin{aligned} \mathcal{I}_B(\mathbf{u}^{-1}, \mathbf{v}^{-1}, b) &\rightarrow \tag{13.4.16} \\ \text{Res}_{z \rightarrow (pq)^{\frac{1}{4}} b u_1, u_1 v_1 \rightarrow (pq)^{\frac{1}{2}}} &\left[ \frac{1}{\Gamma(z^{\pm 2})} \prod_{i=1}^4 \Gamma((pq)^{\frac{1}{4}} b u_i z^{\pm 1}) \Gamma((pq)^{\frac{1}{4}} b^{-1} v_i z^{\pm 1}) \prod_{i,j=1}^4 \Gamma((pq)^{\frac{1}{2}} u_i v_j) \right] \\ &\rightarrow \prod_{i < j} \Gamma((pq)^{\frac{1}{3}} \tilde{t}_i \tilde{t}_j), \end{aligned}$$

where  $\{\tilde{t}_i\} = \{\tilde{b}\tilde{u}_i, \tilde{b}^{-1}\tilde{v}_i\}$ . We thus rederived the identity for the index following from the duality of  $SU(2)$  theory with three flavors to sigma model from the duality of  $SU(2)$  theory with four flavors by following the RG flow triggered by mass term on one side of the duality and vev on the other side.

The general lesson to be learned here is that Higgsing gauge symmetries by vevs for gauge invariant operators manifests itself at the level of the index as reducing the number of integrals in the matrix model through the pinching procedure. In general a vev is possible when a flat direction opens up in the field space and this leads the index to have a pole. The index of the theory obtained in the IR of such an RG flow is given by the residue of the pole.

- *Spontaneously broken global symmetries* – We discussed spontaneous supersymmetry breaking above; here we will study a case of flavor symmetry breaking. The example we consider is  $SU(2)$  gauge theory with two flavors, *i.e.* two fundamental and two anti-fundamental quarks. This theory has an  $SU(4)$  flavor symmetry at the classical level rotating the four quarks. However, at the quantum level the model can be described in terms of the six gauge singlet chiral fields  $M_{ij} = Q_i Q_j$  with a quadratic constraint  $\text{Pf } M = \Lambda^4$  where  $\Lambda$  is the dynamical scale of the gauge theory. This dynamical superpotential breaks the  $SU(4)$  symmetry down to  $Sp(4)$ .

Let us see what happens here at the level of the index. The gauge theory at hand can be obtained from the  $SU(2)$  theory with three flavors we already considered by giving a mass to one of the flavors. Let us denote the six quarks by  $Q_i$  and rotate them with  $SU(6)_t$  symmetry. We can turn on a mass term of the form  $m Q_1 Q_2$ . The theory with three flavors has an IR dual in terms of a sigma model and the analysis is simpler to perform on that side of the duality. Here we have a collection of fifteen singlet fields with a superpotential. The field  $Q_1 Q_2$  is dual to singlet  $M_{12}$ . Turning on the mass term the superpotential on the sigma model side involving field  $M_{12}$  will become schematically

$$m M_{12} + M_{12}(M_{34} M_{56} + M_{36} M_{45} - M_{35} M_{46}). \tag{13.4.17}$$

In particular the F term coming from  $M_{12}$  imposes the constraint we discussed above,

$$m \sim M_{34} M_{56} + M_{36} M_{45} - M_{35} M_{46}. \tag{13.4.18}$$

The weight of field  $M_{12}$  before turning on the linear superpotential is  $(pq)^{\frac{1}{3}}t_1t_2$  and after turning it on it becomes  $pq$ . Thus in the index we need to specialize the parameters as

$$t_1t_2 = (pq)^{\frac{2}{3}}. \quad (13.4.19)$$

We parametrize the fugacities as

$$t_1 = (pq)^{\frac{1}{3}}a, \quad t_2 = (pq)^{\frac{1}{3}}a^{-1}, \quad t_{i>2} = (pq)^{-\frac{1}{6}}\tilde{t}_{i-2}, \quad \prod_{i=1}^4 \tilde{t}_i = 1. \quad (13.4.20)$$

Fugacities  $a$  and  $\tilde{t}_i$  parametrize  $u(1)_a \times su(3)_{\tilde{t}} = su(4)$  classical symmetry of the model. Then after this specification the index of the sigma model becomes

$$\mathcal{I}_{sigma} \rightarrow \Gamma(pq) \prod_{i=1}^4 \Gamma((pq)^{\frac{1}{2}}a^{\pm 1}\tilde{t}_i) \prod_{i<j} \Gamma(\tilde{t}_i\tilde{t}_j). \quad (13.4.21)$$

This expression vanishes for generic values of  $\tilde{t}_j$ . In other words, if we insist on turning on fugacities for the classical  $SU(4)$  symmetry the index vanishes indicating that there is no vacuum of the model having this symmetry. On the other hand let us further take  $\tilde{t}_1 = \tilde{t}_2^{-1} \equiv c$ . This also implies that  $\tilde{t}_3 = \tilde{t}_4^{-1} \equiv d$ . The symmetry we now parametrize is  $su(2)_c \times su(2)_d \subset sp(4)$ . After this specialization the index becomes

$$\mathcal{I}_{sigma} \rightarrow \Gamma(pq) \Gamma(1)^2 \Gamma((pq)^{\frac{1}{2}}a^{\pm 1}c^{\pm 1}) \Gamma((pq)^{\frac{1}{2}}a^{\pm 1}d^{\pm 1}) \Gamma(c^{\pm 1}d^{\pm 1}) = \Gamma(pq) \Gamma(1)^2 \Gamma(c^{\pm 1}d^{\pm 1}). \quad (13.4.22)$$

Note that the fields charged under  $U(1)_a$  can form mass terms and their contribution to the index trivializes. Since  $\Gamma(z)$  has a simple pole as  $z \rightarrow 1$  and a simple zero as  $z \rightarrow pq$ , this expression diverges. We can thus summarize that unless we specialize the  $SU(4)$  fugacities to parametrize an  $Sp(4)$  subgroup the index vanishes and diverges otherwise. The residue of the divergence is given by

$$\Gamma(c^{\pm 1}d^{\pm 1}), \quad (13.4.23)$$

which is the index of the collection of the chiral fields in any given quantum vacuum of the model.

Let us consider the  $SU(2)$  gauge theory with two flavors with the  $Sp(4)$  flavor quantum symmetry, theory A, and some other theory with an  $SU(2)_c$  flavor symmetry. which we will call theory B. Let us also assume that we can gauge in anomaly free fashion the diagonal combination of the  $SU(2)_c$  symmetry of theory B and an  $SU(2)$  sub-group of the  $Sp(4)$  symmetry of theory A. Note that at a generic point of the moduli space of theory A operator charged under  $SU(2)_c$  obtains a vev. This Higgses the  $SU(2)_c$  gauge group. Careful analysis reveals that the theory in the IR is identical to theory B with an addition of two singlet fields. We denote the index of theory B by  $\mathcal{I}_B(c)$  where  $c$  is fugacity for the  $SU(2)_c$  symmetry. The index of the combined theory is then

$$\mathcal{I}(d, g) = \kappa^2 \oint \frac{dc}{4\pi ic} \frac{1}{\Gamma(c^{\pm 2})} \oint \frac{dz}{4\pi iz} \frac{1}{\Gamma(z^{\pm 2})} \Gamma(g c^{\pm 1} z^{\pm 1}) \Gamma(g^{-1} d^{\pm 1} z^{\pm 1}) \mathcal{I}_B(c). \quad (13.4.24)$$

One has to be careful here with the contour of integration since the poles of the index coming from the quarks of theory A sit on the unit circle. The contour can be obtained by carefully taking the mass limit from the theory with three flavors and we call it  $\mathcal{C}$ . This contour separates the sequences of poles these Gamma functions have converging to infinity and zero. Computation of this index reveals that it satisfies,

$$\mathcal{I}(d, g) = \Gamma(g^{\pm 2}) \mathcal{I}_B(d). \quad (13.4.25)$$

We have seen that the index of theory A vanishes except for a subset of fugacities where it diverges, and the above computation reveals that this index can be thought of as a delta function in the space of fugacities. See [26] for more details. The identity (13.4.25) is known as an integral inversion formula of Spiridonov-Warnaar [27].

## 13.5 Index spectroscopy

The supersymmetric index contains useful information about the protected spectrum of the theory. The index counts (with signs) short multiplets up to the equivalence relation that sets to zero sets of short multiplets that may recombine into long ones. In general, it is not possible to deduce unambiguously from the index the precise spectrum of short multiplets. However, for certain special multiplets corresponding to relevant and marginal operators, useful statements with a direct physical interpretation can be made. We will follow closely the discussion in [28].

A generic long multiplet  $\mathcal{A}_{r(j_1, j_2)}^\Delta$  of  $\mathcal{N} = 1$  superconformal algebra is generated by the action of the four Poincaré supercharges  $(\mathcal{Q}_\alpha, \tilde{\mathcal{Q}}_{\dot{\alpha}})$  on a superconformal primary state, which by definition is annihilated by superconformal charges  $(\mathcal{S}_\alpha, \tilde{\mathcal{S}}_{\dot{\alpha}})$ . The multiplet is labeled by the charges  $(\Delta, r, j_1, j_2)$  of the primary with respect to the dilatations, R-symmetry, and the two angular momenta respectively. The absence of negative norm states in the multiplet imposes certain inequalities on these quantum numbers,

$$\Delta \geq 2 - 2\delta_{j_1, 0} + 2j_1 - \frac{3}{2}r, \quad (13.5.1)$$

$$\Delta \geq 2 - 2\delta_{j_2, 0} + 2j_2 + \frac{3}{2}r, \quad (13.5.2)$$

$$\Delta \notin \left(-\frac{3}{2}r, 2 - \frac{3}{2}r\right), \quad \text{if } j_1 = 0, \quad (13.5.3)$$

$$\Delta \notin \left(\frac{3}{2}r, 2 + \frac{3}{2}r\right), \quad \text{if } j_1 = 0, \quad (13.5.4)$$

$$\Delta \geq 2 + j_1 + j_2, \quad \text{if } j_1 \neq 0, \quad j_2 \neq 0, \quad (13.5.5)$$

$$\Delta \geq 1 + j_1 + j_2, \quad \text{if } j_1 = 0 \text{ or } j_2 = 0. \quad (13.5.6)$$

When these inequalities are saturated, some combination of the Poincaré supercharges will annihilate the primary as well, resulting in a shortened multiplet. The relevant property of

these short multiplets is that they must always saturate the unitarity bound in order to be free of negative normed states, and so their conformal dimension is fixed in terms of other quantum numbers and is protected against corrections as one changes the parameters of the theory.

The possible shortening conditions of the  $\mathcal{N} = 1$  superconformal algebra are summarized in Table 13.5.1. Note that  $\mathcal{D}$  and  $\bar{\mathcal{D}}$  multiplets correspond to free fields and our general results below will not hold for them.

| Shortening Conditions |                                                                                                                                                               |                                    |                                                                   | Multiplet                                                          |
|-----------------------|---------------------------------------------------------------------------------------------------------------------------------------------------------------|------------------------------------|-------------------------------------------------------------------|--------------------------------------------------------------------|
| $\mathcal{B}$         | $\mathcal{Q}_\alpha r\rangle^{h.w.} = 0$                                                                                                                      | $j_1 = 0$                          | $\Delta = -\frac{3}{2}r$                                          | $\mathcal{B}_{r(0,j_2)}$                                           |
| $\bar{\mathcal{B}}$   | $\bar{\mathcal{Q}}_{\dot{\alpha}} r\rangle^{h.w.} = 0$                                                                                                        | $j_2 = 0$                          | $\Delta = \frac{3}{2}r$                                           | $\bar{\mathcal{B}}_{r(j_1,0)}$                                     |
| $\hat{\mathcal{B}}$   | $\mathcal{B} \cap \bar{\mathcal{B}}$                                                                                                                          | $j_1, j_2, r = 0$                  | $\Delta = 0$                                                      | $\hat{\mathcal{B}}$                                                |
| $\mathcal{C}$         | $\epsilon^{\alpha\beta}\mathcal{Q}_\beta r\rangle_{\dot{\alpha}}^{h.w.} = 0$<br>$(\mathcal{Q})^2 r\rangle^{h.w.} = 0$ for $j_1 = 0$                           |                                    | $\Delta = 2 + 2j_1 - \frac{3}{2}r$<br>$\Delta = 2 - \frac{3}{2}r$ | $\mathcal{C}_{r(j_1,j_2)}$<br>$\mathcal{C}_{r(0,j_2)}$             |
| $\bar{\mathcal{C}}$   | $\epsilon^{\dot{\alpha}\dot{\beta}}\bar{\mathcal{Q}}_{\dot{\beta}} r\rangle_{\alpha}^{h.w.} = 0$<br>$(\bar{\mathcal{Q}})^2 r\rangle^{h.w.} = 0$ for $j_2 = 0$ |                                    | $\Delta = 2 + 2j_2 + \frac{3}{2}r$<br>$\Delta = 2 + \frac{3}{2}r$ | $\bar{\mathcal{C}}_{r(j_1,j_2)}$<br>$\bar{\mathcal{C}}_{r(j_1,0)}$ |
| $\hat{\mathcal{C}}$   | $\mathcal{C} \cap \bar{\mathcal{C}}$                                                                                                                          | $\frac{3}{2}r = (j_1 - j_2)$       | $\Delta = 2 + j_1 + j_2$                                          | $\hat{\mathcal{C}}_{(j_1,j_2)}$                                    |
| $\mathcal{D}$         | $\mathcal{B} \cap \bar{\mathcal{C}}$                                                                                                                          | $j_1 = 0, -\frac{3}{2}r = j_2 + 1$ | $\Delta = -\frac{3}{2}r = 1 + j_2$                                | $\mathcal{D}_{(0,j_2)}$                                            |
| $\bar{\mathcal{D}}$   | $\bar{\mathcal{B}} \cap \mathcal{C}$                                                                                                                          | $j_2 = 0, \frac{3}{2}r = j_1 + 1$  | $\Delta = \frac{3}{2}r = 1 + j_1$                                 | $\bar{\mathcal{D}}_{(j_1,0)}$                                      |

Table 13.5.1: Shortening conditions for the  $SU(2, 2|1)$  superconformal algebra.

If the charges of a collection of short multiplets obey certain relations, they can combine to form a long multiplet which is no longer protected. Alternatively, one can understand this recombination in reverse, as a long multiplet decomposing into a collection short multiplets as the conformal dimension of its primary hits the BPS bound. This phenomenon plays a crucial role in extracting spectral information about an SCFT from its index because the index counts short multiplets of the theory *up to recombination*. The collective contributions to the index from short multiplets that can recombine vanishes. The recombination equations for  $\mathcal{N} = 1$  superconformal algebra are as follows:

$$\begin{aligned}
\mathcal{A}_{r(j_1,j_2)}^{2+2j_1-\frac{3}{2}r} &\longrightarrow \mathcal{C}_{r(j_1,j_2)} \oplus \mathcal{C}_{r-1(j_1-\frac{1}{2},j_2)} , \\
\mathcal{A}_{r(j_1,j_2)}^{2+2j_2+\frac{3}{2}r} &\longrightarrow \bar{\mathcal{C}}_{r(j_1,j_2)} \oplus \bar{\mathcal{C}}_{r+1(j_1,j_2-\frac{1}{2})} , \\
\mathcal{A}_{\frac{2}{3}(j_1-j_2)(j_1,j_2)}^{2+j_1+j_2} &\longrightarrow \hat{\mathcal{C}}_{(j_1,j_2)} \oplus \mathcal{C}_{\frac{2}{3}(j_1-j_2)-1(j_1-\frac{1}{2},j_2)} \oplus \bar{\mathcal{C}}_{\frac{2}{3}(j_1-j_2)+1(j_1,j_2-\frac{1}{2})} .
\end{aligned} \tag{13.5.7}$$

$\mathcal{B}$  multiplets can be formally treated as a special case of  $\mathcal{C}$  multiplets with unphysical spin quantum numbers,

$$\mathcal{B}_{r(0,j_2)} =: \mathcal{C}_{r+1(-\frac{1}{2},j_2)} , \quad \bar{\mathcal{B}}_{r(j_1,0)} =: \bar{\mathcal{C}}_{r-1(j_1,-\frac{1}{2})} . \tag{13.5.8}$$

Thus the discussion can be phrased entirely in terms of  $\mathcal{C}$  type multiplets.

An important example of recombination is for the long multiplet  $\mathcal{A}_{0(0,0)}^{2+-\frac{3}{2}r}$  as  $r \rightarrow 0$ . The multiplet hits the BPS bound and splits into three short multiplets according to the third rule in (13.5.7),

$$\mathcal{A}_{0(0,0)}^2 \longrightarrow \hat{\mathcal{C}}_{(0,0)} \oplus \mathcal{C}_{-1(-\frac{1}{2},0)} \oplus \bar{\mathcal{C}}_{1(0,-\frac{1}{2})} = \hat{\mathcal{C}}_{(0,0)} \oplus (\mathcal{B}_{-2(0,0)} \oplus \bar{\mathcal{B}}_{2(0,0)}) \quad (13.5.9)$$

The multiplet  $\hat{\mathcal{C}}_{(0,0)}$  contains a conserved current, while the multiplet  $\mathcal{B}_{-2(0,0)}$  contains a chiral primary  $\mathcal{O}$  of dimension three and an associated marginal F-term deformation  $\int d^2\theta \mathcal{O}$ . The recombination described above demonstrates the fact that a marginal operator can fail to be exactly marginal if and only if it combines with a conserved current corresponding to a broken global symmetry. This particular recombination and its implications for the space of exactly marginal deformations of an SCFT has been studied in detail in [29].

The  $\mathcal{C}$  ( $\bar{\mathcal{C}}$ ) multiplets contribute only to the left-handed index (right-handed index), while  $\hat{\mathcal{C}}$  multiplets contribute to both. We restrict our attention to  $\mathcal{I}^L$  and treat  $\hat{\mathcal{C}}$  as a special case of  $\mathcal{C}$  with  $r = \frac{2}{3}(j_1 - j_2)$ . The recombination rules allow us to define equivalence classes of short representations which make identical contributions to the index,

$$\begin{aligned} [\tilde{r}, j_2]_+ &\equiv \left\{ \mathcal{C}_{r(j_1, j_2)} \mid 2j_1 - r = \tilde{r}, \quad j_1 \in \mathbb{Z}_{\geq 0} \right\}, \\ [\tilde{r}, j_2]_- &\equiv \left\{ \mathcal{C}_{r(j_1, j_2)} \mid 2j_1 - r = \tilde{r}, \quad j_1 \in -\frac{1}{2} + \mathbb{Z}_{\geq 0} \right\}. \end{aligned} \quad (13.5.10)$$

For a  $\mathcal{B}$  type multiplet, the unitarity bounds of Equation (13.5.1) imply that  $\tilde{r} \geq -\frac{4}{3} + \frac{2}{3}j_2$ , while for a  $\mathcal{C}$  multiplet they imply  $\tilde{r} \geq \frac{4}{3}j_1 + \frac{2}{3}j_2$ . Consequently, there are a finite number of representations in a fixed equivalence class — for fixed  $\tilde{r}$ , there is an upper limit on  $j_1$  such that these bounds can be satisfied.

The contribution to the left-handed superconformal index from any short multiplet in a given class is given by

$$\mathcal{I}_{[\tilde{r}, j_2]_+}^L = -\mathcal{I}_{[\tilde{r}, j_2]_-}^L = (-1)^{2j_2+1} \frac{(pq)^{\frac{1}{2}(\tilde{r}+2)} \chi_{j_2}(p/q)}{(1-p)(1-q)}. \quad (13.5.11)$$

We define the *net degeneracy* for a given choice of  $(\tilde{r}, j_2)$ ,

$$\text{ND}[\tilde{r}, j_2] := \# [\tilde{r}, j_2]_+ - \# [\tilde{r}, j_2]_-, \quad (13.5.12)$$

and the extractable content of the superconformal index is encapsulated in precisely the integers  $\text{ND}[\tilde{r}, j_2]$ . If the index of an  $\mathcal{N} = 1$  SCFT is known, the net degeneracies can be systematically extracted by means of a *sieve algorithm* (see for example [28]). The most precise information about actual operators we can extract from the index comes from the equivalence classes with a small number of representatives.

The optimal case is the chiral primary operators that lie in multiplets  $\mathcal{B}_{r(0, j_2)}$  and have  $-2 - \frac{2}{3}j_2 < r \leq -\frac{2}{3} - \frac{2}{3}j_2$ . These have  $\tilde{r} \in [-\frac{4}{3} + \frac{2}{3}j_2, \frac{2}{3}j_2)$ , and they are the *only representatives*

of the equivalence class  $[\tilde{r}, 0]_-$  for this range of  $\tilde{r}$ . Furthermore, there are no unitary representations in the corresponding class  $[\tilde{r}, 0]_+$ . Consequently, we can read off the exact number of such operators from the superconformal index. Specializing to  $j_2 = 0$ , these are precisely the relevant deformations of the SCFT. The number of such deformations is simply the coefficient of  $(pq)^{-\frac{1}{2}r}(p/q)^0$  in the index after subtracting out any non-trivial  $SU(2)_2$  characters at the same power of  $pq$ .

The next best case is for  $\tilde{r} \in [\frac{2}{3}j_2, \frac{2}{3} + \frac{2}{3}j_2)$ . Both  $[\tilde{r}, j_2]_+$  and  $[\tilde{r}, j_2]_-$  have only a single representative in this range, and so the index computes the difference in the number of such operators. For  $j_2 = \tilde{r} = 0$  in particular, the representatives are  $\hat{\mathcal{C}}_{(0,0)}$  and  $\mathcal{B}_{-2(0,0)}$ , respectively. The cancellation between these multiplets corresponds to precisely the recombination described in the example above, and we see that the index computes

$$\begin{aligned} \text{ND}[0, 0] &= \# \mathcal{B}_{-2(0,0)} - \# \hat{\mathcal{C}}_{(0,0)} \\ &= \# \text{marginal operators} - \# \text{conserved currents} . \end{aligned} \tag{13.5.13}$$

If all global flavor symmetries are broken at a generic point on the conformal manifold, then this net degeneracy will precisely capture the actual dimension of that conformal manifold. However, not all recombinations of the type discussed in the example necessarily take place, and in this case one must account for conserved currents in extracting the dimension of the conformal manifold. Again, this net degeneracy is easily computed by expanding the index to order  $pq$  and subtracting out all nontrivial characters for  $SU(2)_2$ .

For  $\tilde{r} \geq \frac{2}{3}$ , there will be several representatives that are indistinguishable to the index, and the cancellations among them do not correspond to any obvious physical phenomenon such as symmetry breaking. Thus, the most immediate spectroscopic use of the index is the analysis of relevant and marginal operators at a fixed point.

### 13.5.1 An example

As an example we discuss  $SU(N)$   $\mathcal{N} = 4$  SYM. In  $\mathcal{N} = 1$  notation we have here three adjoint chiral fields,  $\Phi_j$ , with R-charge  $\frac{2}{3}$  rotated by  $SU(3)_t$  global symmetry. The superconformal R-charge is that of a free field since the conformal manifold passes through the free point. The index is given by

$$\mathcal{I}_N(t, p, q) = \frac{1}{N!} \kappa^{N-1} \oint \prod_{j=1}^{N-1} \frac{dz_j}{2\pi i z_j} \prod_{j \neq k} \frac{\Gamma((pq)^{\frac{1}{3}} t_1 z_j / z_k) \Gamma((pq)^{\frac{1}{3}} t_2 z_j / z_k) \Gamma((pq)^{\frac{1}{3}} \frac{1}{t_1 t_2} z_j / z_k)}{\Gamma(z_j / z_k)} . \tag{13.5.14}$$

For  $N > 2$ , the first few terms in the  $p, q$  expansion are

$$\mathcal{I}_N(t, p, q) = 1 + \mathbf{6}_t (pq)^{\frac{2}{3}} + \mathbf{3}_t (p+q) (pq)^{\frac{1}{3}} + (1 + \mathbf{10}_t - \mathbf{8}_t) pq + \dots . \tag{13.5.15}$$

Following the general prescription of this section we read off the relevant operators to be  $\mathbf{6}_t$  which are the six quadratic operators  $\Phi_{(j}\Phi_{k)}$ . We have also operators charged under

$j_2$  at order  $(p+q)(pq)^{\frac{1}{3}}$  which do not correspond to relevant operators. At order  $pq$  we have the marginal operators. The contribution here is  $1 + \mathbf{10}_t - \mathbf{8}_t$ . The generators of the global symmetry form the  $\mathbf{8}_t$  which is subtracted the marginal operators are the gauge coupling and the  $\mathbf{10}_t$  symmetric cubic combinations of the adjoint chirals. At a generic point on the conformal manifold the  $SU(3)_t$  symmetry is broken and the dimension of it is  $1 + 10 - 8 = 3$  as expected. These exactly marginal deformations are the gauge coupling, the  $\beta$  deformation (adding  $\text{Tr}\Phi_1\{\Phi_2, \Phi_3\}$  to superpotential), and the  $\gamma$  deformation (adding also  $\text{Tr}(\Phi_1^3 + \Phi_2^3 + \Phi_3^3)$ ).

The case of  $N = 2$  is special and there the expansion of the index coincides with (13.5.15) except that  $\mathbf{10}_t$  term is missing. Here the conformal manifold is actually only one dimensional and corresponds to the gauge coupling. On any point of this manifold the  $SU(3)_t$  symmetry is unbroken consistently with the index. The reason here two directions are missing is that a general marginal superpotential cubic in the chiral fields can be decomposed as a sum of two terms, in one of which the gauge indices are contracted with  $\epsilon_{abc}$  and the other with  $d_{abc} = \text{Tr} T_a\{T_b, T_c\}$ . The latter structure is non zero only for  $N > 2$ .

## 13.6 Dualities and Identities

Perhaps the most important application of the supersymmetric index as a test of non-perturbative dualities. Since the index is an RG invariant quantity and does not depend on the marginal couplings, it should be the same when computed for two theories flowing to the same fixed point or two different descriptions of the same conformal theory. Physical dualities translates into mathematical identities between elliptic hypergeometric integrals. Such identities are very non-trivial and give the strongest checks to date of many dualities. In several cases, these identities have already appeared in the mathematical literature, but in many others they are new – they are undoubtedly true since they can be checked to very high orders in a series expansion, but a rigorous proof is still lacking.

### 13.6.1 Symmetries and transformations of the index

Before discussing relations between indices of dual theories, it is useful to pause and consider the symmetry properties of the index of a single theory. The index is a function  $\mathcal{I}(a_1, a_2, \dots, a_s, p, q)$ . The parameters  $a_i$  are fugacities for  $U(1)$  global symmetries forming the maximal torus of the (possibly non-abelian) global symmetry. If the symmetry enhances to a non-abelian symmetry the index should be invariant under the action of the Weyl group acting on the fugacities. For example, if the  $a_i$ 's parametrize an  $SU(s+1)$  symmetry, the index should be invariant under permutations of the  $a_i$ 's and under the transformation of any of the  $a_j$  as  $a_j \rightarrow \frac{1}{a_1 a_2 \dots a_s}$ .

We can also ask the converse question: what happens if the index is invariant under the action of certain discrete group  $\mathcal{W}$  on the flavor fugacities? There are two interesting physical

possibilities. First, it might be that the flavor symmetry enhances to a non-abelian group such that  $\mathcal{W}$  serves as its Weyl group. A second physical possibility is that such a discrete symmetry signals self-duality of the theory. An example is  $SU(2) \mathcal{N} = 2$  SYM with four flavors. Here the flavour group (in  $\mathcal{N} = 2$  language) is rank four, and let us parametrize it by four fugacities  $a_i$ . In  $\mathcal{N} = 1$  language the index is given by

$$\mathcal{I}(a_1, a_2, a_3, a_4) = \frac{\kappa \Gamma((pq)^{\frac{1}{3}} t^{-2})}{2} \oint \frac{dz}{2\pi i z} \frac{\Gamma((pq)^{\frac{1}{3}} t^{-2} z^{\pm 2})}{\Gamma(z^{\pm 2})} \Gamma((pq)^{\frac{1}{3}} t a_1^{\pm 1} a_2^{\pm 1} z^{\pm 1}) \Gamma((pq)^{\frac{1}{3}} t a_3^{\pm 1} a_4^{\pm 1} z^{\pm 1}). \quad (13.6.1)$$

Here  $t$  is fugacity for a  $U(1)$  symmetry related to the bigger R-symmetry of  $\mathcal{N} = 2$ . The flavor symmetry here enhance to  $SO(8)$  and the index is manifestly invariant under the Weyl group of  $SO(8)$ . This group is generated by  $a_i \rightarrow a_i^{-1}$  and by  $a_1 \leftrightarrow a_2$ ,  $a_3 \leftrightarrow a_4$ . However, the index is also invariant under exchanging  $a_1$  and  $a_3$ . This is not part of  $SO(8)$  Weyl symmetry and is not manifest in the integral above. This discrete symmetry is the manifestation of the self S-duality (or rather triality) that the theory enjoys. This is a strong/weak type of duality relating the same theory with different values of coupling. This invariance property of the index was proven in [30]. In fact the full discrete symmetry of the index, the one coming from Weyl of  $SO(8)$  and the one coming from the duality, is the Weyl group of  $F_4$ . We are not aware of a physical interpretation for the full  $F_4$  symmetry – it would be nice to figure out whether there is any.

Another similar example is that of  $\mathcal{N} = 1$   $SU(2)$  theory with four flavors, *i.e.* the same theory as above but without the adjoint chiral field. The theory has flavor symmetry of rank seven, the  $SU(8)$  symmetry rotating the different matter fields. This theory enjoys Seiberg-duality as we already discussed, but in fact there are many more dualities as discussed in [31]. This theory in fact has 72 dual descriptions. The different descriptions correspond to the action of the Weyl group of  $E_7$  on the fugacities. In the different duality frames the gauge structure is the same as in the original one but there are additional singlet fields and superpotentials. It was argued in [32] that taking two copies of this theory coupled through a quartic superpotential the theory is exactly self-dual and that there should be a point on the conformal manifold of this theory where the flavor symmetry is actually enhanced to  $E_7$ .

We can also ask whether there are interesting properties of the index involving manipulations of both the flavor fugacities and the superconformal fugacities  $p$  and  $q$ . A simple example is as follows. One can consider assigning different anomaly free R-charges to the fields by mixing a given R-symmetry with the flavor symmetry. For example give a flavor symmetry  $U(1)_a$  we can redefine the R-symmetry to be  $R \rightarrow R + s q_a$  with  $q_a$  being the charge under  $U(1)_a$ . At the level of the index this transformation corresponds to

$$R \rightarrow R + s q_a \Rightarrow \mathcal{I}(a, p, q) \rightarrow \mathcal{I}((pq)^{\frac{s}{2}} a, p, q). \quad (13.6.2)$$

Let us consider shifting flavor fugacity  $a$  to  $q^{\tilde{s}} p^s a$ . When  $s$  and  $\tilde{s}$  are the same this is just a redefinition of the R-charge. From the definition of the index the shift in  $a$  amounts to

$$\mathcal{I} = \text{Tr}(-1)^F p^{j_1+j_2+\frac{r}{2}} q^{j_2-j_1+\frac{r}{2}} a^{q_a} \rightarrow \text{Tr}(-1)^F p^{j_1+j_2+\frac{r}{2}+s q_a} q^{j_2-j_1+\frac{r}{2}+\tilde{s} q_a} a^{q_a}. \quad (13.6.3)$$

To interpret this expression as an index we can redefine

$$\hat{r} = r + (s + \tilde{s})q_a, \quad \hat{j}_1 = j_1 + \frac{s - \tilde{s}}{2}q_a. \quad (13.6.4)$$

In particular for  $s \neq \tilde{s}$  this breaks Lorentz symmetry and does not make sense as a pure  $4d$  index. However, such a transformation might make sense as an index of a coupled 4d-2d system. A simple example is the following important identity of the index of a chiral field,

$$\mathcal{I}^{(R)}(pa) = \Gamma((pq)^{\frac{R}{2}}pa) = \theta((pq)^{\frac{R}{2}}a; q) \mathcal{I}^{(R)}(a). \quad (13.6.5)$$

The index on the right-hand side can be interpreted as an index of chiral field in four dimensions coupled to a Fermi  $(0, 2)$  multiplet in two dimensions. Similarly we have

$$\mathcal{I}^{(R)}(p^{-1}a) = \Gamma((pq)^{\frac{R}{2}}p^{-1}a) = \frac{1}{\theta((pq)^{\frac{R}{2}}p^{-1}a; q)} \mathcal{I}^{(R)}(a). \quad (13.6.6)$$

Here the right hand side is a chiral field in four dimensions coupled to a chiral  $(0, 2)$  field in two dimension. Such a transformation of the index will become important while discussing indices in presence of surface defects [33–35] and we will comment on this more in what follows.

### 13.6.2 $\mathcal{N} = 4$ dualities

A basic example of a duality implying a non-trivial mathematical identity is the S-duality between  $SO(2n + 1)$   $\mathcal{N} = 4$  SYM and  $USp(2n)$   $\mathcal{N} = 4$  SYM. We use an  $\mathcal{N} = 1$  language with the three adjoint chiral multiplets having R-charge  $\frac{2}{3}$ . Then the index of the  $SO(2n + 1)$  model is given by

$$\mathcal{I}_{so} = \kappa^n \prod_{i=1}^3 \Gamma((pq)^{\frac{1}{3}}t_i) \frac{1}{2^n n!} \oint \prod_{i=1}^n \frac{dz_i}{2\pi i z_i} \prod_{i < k} \frac{\prod_{j=1}^3 \Gamma((pq)^{\frac{1}{3}}t_j z_i^{\pm 1} z_k^{\pm 1})}{\Gamma(z_i^{\pm 1} z_k^{\pm 1})} \prod_{i=1}^n \frac{\prod_{j=1}^3 \Gamma((pq)^{\frac{1}{3}}t_j z_i^{\pm 1})}{\Gamma(z_i^{\pm 1})}, \quad (13.6.7)$$

while for the  $USp(2n)$  model we get

$$\mathcal{I}_{sp} = \kappa^n \prod_{i=1}^3 \Gamma((pq)^{\frac{1}{3}}t_i) \frac{1}{2^n n!} \oint \prod_{i=1}^n \frac{dz_i}{2\pi i z_i} \prod_{i < k} \frac{\prod_{j=1}^3 \Gamma((pq)^{\frac{1}{3}}t_j z_i^{\pm 1} z_k^{\pm 1})}{\Gamma(z_i^{\pm 1} z_k^{\pm 1})} \prod_{i=1}^n \frac{\prod_{j=1}^3 \Gamma((pq)^{\frac{1}{3}}t_j z_i^{\pm 2})}{\Gamma(z_i^{\pm 2})}. \quad (13.6.8)$$

Fugacities  $t_j$  parametrize  $SU(3)_t$  symmetry rotating the three adjoint chirals. We have decomposed the  $SU(4)$  R-symmetry of  $\mathcal{N} = 4$  to  $U(1)$  R-symmetry of  $\mathcal{N} = 1$  and  $SU(3)_t$ . For  $n = 1$  and  $n = 2$  the  $SO(2n + 1)$  and  $USp(2n)$  algebras are isomorphic<sup>5</sup> and there is a simple change of integration variables making the two expressions above manifestly the

<sup>5</sup>The global form of the gauge group is inessential here – the spectrum of local gauge-invariant operators captured by the index depends only on the gauge algebra.

same.<sup>6</sup> For  $n > 2$ , one can check that the two expressions coincide to very high orders in a series expansion in fugacities, but no proof is available yet except in certain degeneration limits [36].

### 13.6.3 Seiberg dualities

Seiberg dualities are the basic examples of IR dualities – two theories flowing to the same fixed point. The simplest example is of an  $SU(N)$  gauge theory with  $N_f$  on side A being equivalent to  $SU(N_f - N)$  gauge theory with  $N_f$  flavors, conjugate representation of the flavor group, and a bunch of gauge singlet fields dual to the mesons of side A on side B. The index of side A is given by

$$\mathcal{I}_N^{N_f}(\mathbf{u}, \mathbf{v}, b) = \kappa^{N-1} \frac{1}{N!} \oint \prod_{i=1}^{N-1} \frac{dz_i}{2\pi i z_i} \prod_{i \neq j} \frac{1}{\Gamma(z_i/z_j)} \prod_{i=1}^{N_f} \prod_{j=1}^N \Gamma((pq)^{\frac{N_f-N}{2N_f}} b u_i z_j) \Gamma((pq)^{\frac{N_f-N}{2N_f}} v_i z_j^{-1} b^{-1}). \quad (13.6.9)$$

Here  $\mathbf{u}$ ,  $\mathbf{v}$ , and  $b$  are parametrizing the  $SU(N_f)_u \times SU(N_f)_v \times U(1)_b$  global symmetry of the theory. on side B we have

$$\begin{aligned} \tilde{\mathcal{I}}_{N_f-N}^{N_f}(\mathbf{u}, \mathbf{v}, b) &= \left( \prod_{i,j=1}^{N_f} \Gamma((pq)^{\frac{N_f-N}{N_f}} u_i v_j) \right) \kappa^{N_f-N-1} \frac{1}{(N_f-N)!} \oint \prod_{i=1}^{N_f-N-1} \frac{dz_i}{2\pi i z_i} \prod_{i \neq j} \frac{1}{\Gamma(z_i/z_j)} \\ &\prod_{i=1}^{N_f} \prod_{j=1}^{N_f-N} \Gamma((pq)^{\frac{N}{2N_f}} b^{\frac{N}{N_f-N}} u_i^{-1} z_j) \Gamma((pq)^{\frac{N}{2N_f}} v_i^{-1} z_j^{-1} b^{-\frac{N}{N_f-N}}). \end{aligned} \quad (13.6.10)$$

Duality implies that the two indices above should be equal and indeed it was shown by Rains that they are [25]. The proof is rather non trivial but in section 7 we will discuss a proof for a certain limit of the parameters.

### 13.6.4 Kutasov-Schwimmer dualities

Let us give yet another example of duality which implies a mathematical identity of indices yet to be proven rigorously. The example is that of Kutasov-Schwimmer dualities where in addition to  $N_f$  flavors of fundamental matter of  $SU(N)$  gauge group one introduces two, or one, adjoint fields. The superpotentials for the adjoint fields follow *ADE* classification,

$$\begin{aligned} A_k &: \quad \text{Tr } X^{k+1}, & (13.6.11) \\ D_{k+2} &: \quad \text{Tr } X^{k+1} + \text{Tr } XY^2, \\ E_6 &: \quad \text{Tr } X^4 + \text{Tr } Y^3, & E_7 &: \quad \text{Tr } X^3 Y + \text{Tr } Y^3, & E_8 &: \quad \text{Tr } X^5 + \text{Tr } Y^3. \end{aligned}$$

<sup>6</sup>The two root systems define dual lattices in  $n$  dimensions. In  $n = 1, 2$  there is a linear transformation taking one into the other (line dual to line, and square dual to square), while for  $n > 2$  there is not.

These superpotentials fix the R-charge assignments for the adjoint fields. Dual descriptions are known in the  $A$ ,  $D$ , [37–39] and  $E_7$  [40] cases. The dual has gauge group of  $SU(\alpha N_f - N)$  with  $\alpha$  depending on the superpotential for the adjoint matter,

$$\begin{aligned} A_k &: & \alpha &= k, \\ D_{k+2} &: & \alpha &= 3k, \\ E_7 &: & \alpha &= 30. \end{aligned} \tag{13.6.12}$$

One also has to introduce a variety of singlet fields coupled through a superpotential to gauge singlet operators on the dual side. For details the reader is referred to [41]. One can write down the corresponding identities for the supersymmetric indices, see *e.g.* [17], and check that they are true in series expansion in fugacities or in certain limits such as large  $N$ . However no proof is known to date.

We have focussed on the simplest representative examples of dualities and there are many more, see the discussion in [42, 43]. The mathematics of these identities is a very active area of research, see *e.g.* [24, 44–46] for reviews.

## 13.7 Limits

In previous sections we have discussed how the index encodes information about four-dimensional physics. Upon taking appropriate limits, the index can also be related to physical quantities in other spacetime dimensions. We will discuss here the two most natural limits of this kind.

### 13.7.1 Small $\tau$ limit, $\mathbb{S}^1 \rightarrow 0$

We consider taking all the fugacities to 1. This limit in the partition function language corresponds to taking the limit of the size of  $\mathbb{S}^1$  to zero. Since the index and the partition function differ only by the  $e^{-\tau E_{Casimir}}$  factor the two coincide in the limit. Moreover it was argued on general grounds that in this limit the index has generically the following divergent behavior [47]

$$\mathcal{I}(\tau \rightarrow 0) = \mathcal{Z}_{\mathbb{S}^3 \times \mathbb{S}^1}(\tau \rightarrow 0) = e^{-\frac{16\pi^2}{3} \frac{1}{\tau}(a-c)} \times \mathcal{Z}_{\mathbb{S}^3}. \tag{13.7.1}$$

This asymptotic behavior can be corrected by subleading power-law terms in  $\tau$  when the theory has moduli spaces on the circle [14, 48].<sup>7</sup> Let us discuss how this comes about in detail in a particular example.<sup>8</sup>

---

<sup>7</sup>However, in certain non-generic situations even the leading behavior is modified, see [14] for a careful discussion. Perhaps the simplest example that exhibits this non-generic behavior is the ISS model [49] (see also [50] for a discussion of the index of this theory).

<sup>8</sup>We follow here the discussion in appendix B of [21].

• *Dimensional reduction of the index of a chiral field* – Let us make the relation between the geometry and the index a bit more precise. We compute the partition function on  $\mathbb{S}^3 \times \mathbb{S}^1$  with radii  $r_3$  and  $r_1$ , twisted by fugacities for various global symmetries. Equivalently, after a change of variables it can be thought of as a partition function on  $\mathbb{S}_b^3 \times \tilde{\mathbb{S}}^1$  with the fugacities responsible for the geometric twisting absorbed in the geometry [51]. Here  $\mathbb{S}_b^3$  is the squashed sphere. We can compute the index as a partition function by first reducing the theory on  $\tilde{\mathbb{S}}^1$  of finite radius, and then computing the  $3d$  partition function of the resulting  $3d$  theory, including all the KK modes on the  $\tilde{\mathbb{S}}^1$ . The fugacities corresponding to flavor symmetries can be thought of as couplings to background gauge fields along the  $\mathbb{S}^1$  direction. The gauge fields along the  $\mathbb{S}^1$  have the meaning of real mass parameters for global symmetries in three dimensions. In addition, as we go once around the  $\mathbb{S}^1$ , we should rotate the  $\mathbb{S}^3$  along the Hopf fiber by an angle depending on the fugacities  $p$  and  $q$ . This has the effect of changing the geometry. As discussed in [51], there is a change of coordinates, where the metric becomes that of an  $\mathbb{S}_b^3 \times \tilde{\mathbb{S}}^1$ , where the  $\tilde{\mathbb{S}}^1$  factor is rotated on the  $\mathbb{S}_b^3$  base. The parameters are related by

$$p = e^{-2\pi b \frac{\tilde{r}_1}{r_3}} \quad ; \quad q = e^{-2\pi b^{-1} \frac{\tilde{r}_1}{r_3}}, \quad \tilde{r}_1 = \frac{2}{b + b^{-1}} r_1. \quad (13.7.2)$$

This procedure leads to the action used in [51] to compute the supersymmetric partition function on  $\mathbb{S}_b^3$ . Then, we can write the  $4d$  index as coming from a theory on  $\mathbb{S}_b^3$ , with an infinite tower of KK modes. We refer the reader to the references above and to appendix B of [21] for more details.

For a free chiral field (of R-charge  $R$  and charged under a  $U(1)_u$  symmetry) we are interested in rewriting the index in the following form,

$$\mathcal{Z}_{\mathbb{S}^3 \times \mathbb{S}^1}^{(R)}(p, q, u) \propto \prod_{n=-\infty}^{\infty} \mathcal{Z}^{(R)}(\omega_1, \omega_2, m + \frac{n}{\tilde{r}_1}), \quad (13.7.3)$$

where  $\mathcal{Z}_{\mathbb{S}_b^3}$  is the  $\mathbb{S}_b^3$  partition function of a chiral field depending on the squashing parameter, real mass for  $U(1)_u$ , and the R-charge,

$$\mathcal{Z}_{\mathbb{S}_b^3} = \Gamma_h(\omega R + \sum_a m_a e_a; \omega_1, \omega_2), \quad (13.7.4)$$

$$\Gamma_h(z; \omega_1, \omega_2) = e^{\frac{\pi i}{2\omega_1 \omega_2} \left( (z-\omega)^2 - \frac{\omega_1^2 + \omega_2^2}{12} \right)} \prod_{\ell=0}^{\infty} \frac{1 - e^{\frac{2\pi i}{\omega_1}(\omega_2 - z)} e^{\frac{2\pi i \omega_2 \ell}{\omega_1}}}{1 - e^{-\frac{2\pi i}{\omega_2} z} e^{-\frac{2\pi i \omega_1 \ell}{\omega_2}}}.$$

The parameters on the two sides in (13.7.3) are related as

$$u = e^{2\pi i \tilde{r}_1 m}, \quad p = e^{2\pi i \tilde{r}_1 \omega_1}, \quad q = e^{2\pi i \tilde{r}_1 \omega_2}, \quad \omega = \frac{1}{2}(\omega_1 + \omega_2). \quad (13.7.5)$$

On the left-hand side we have the  $4d$  index of a chiral superfield, and on the right-hand side the product over  $3d$   $\mathbb{S}_b^3$  partition functions of the KK modes on  $\tilde{\mathbb{S}}^1$ . The inverse radius of  $\tilde{\mathbb{S}}^1$ ,  $1/\tilde{r}_1$ , plays the role of a real mass coupled to the KK momentum.

The expression on the right hand side of (13.7.3) as it stands is divergent and needs to be properly regularized and defined. Moreover one needs to be careful to include the Casimir energy in the definition of the partition function in four dimensions. Concretely, the twisted partition function of the chiral field on  $\mathbb{S}^3 \times \mathbb{S}^1$  can be written as

$$\mathcal{Z}_{\mathbb{S}^3 \times \mathbb{S}^1}^{(0)}(p, q, u) = e^{\mathcal{I}_0} \Gamma(u; p, q). \quad (13.7.6)$$

Here we chose to take R charge to be zero for simplicity with non trivial R charge easily reintroduced by mixing in the flavor symmetry. The factor  $e^{\mathcal{I}_0}$  relates the two different natural normalizations. It is computed in [13],

$$\tilde{r}_1^{-1} \mathcal{I}_0 = \frac{1}{4} \left( r^{-1} \frac{d}{dr} \left( r \Gamma_0(e^{2\pi r i m}; e^{2\pi r i \omega_1}, e^{2\pi r i \omega_2}) \right) \right) \Big|_{r=0}, \quad (13.7.7)$$

where  $\Gamma_0(z; p, q)$  is the so called single particle index, defined by

$$\Gamma(u; p, q) = \exp \left[ \sum_{n=1}^{\infty} \frac{1}{n} \Gamma_0(z^n; p^n, q^n) \right] \rightarrow \Gamma_0(z; p, q) = \frac{z - pqz^{-1}}{(1-p)(1-q)}. \quad (13.7.8)$$

Using the fact that  $\Gamma_0$  has a simple pole at  $r = 0$  and a vanishing constant term in the expansion around  $r = 0$ , equation (13.7.7) leads to

$$\mathcal{I}_0 = \frac{\pi i \tilde{r}_1 (m - \omega) (2m(m - 2\omega) + \omega_1 \omega_2)}{6 \omega_1 \omega_2}. \quad (13.7.9)$$

Next we compute the right-hand side of (13.7.3),

$$\prod_{n=-\infty}^{\infty} \mathcal{Z}^{(0)}(\omega_1, \omega_2, m + \frac{n}{\tilde{r}_1}) = \prod_{n=-\infty}^{\infty} \Gamma_h(m + \frac{n}{\tilde{r}_1}; \omega_1, \omega_2). \quad (13.7.10)$$

The infinite product over  $n$  here diverges, since for large  $n$  the hyperbolic Gamma functions approach a divergent exponential behavior,

$$\begin{aligned} \log (\Gamma_h(\omega R + \rho(\sigma) + \tau(\mu + s \mu_o))) &= \quad (13.7.11) \\ \text{sign}(\tau(\mu_o)) \frac{\pi i}{2 \omega_1 \omega_2} \left( [\omega(R - 1) + \rho(\sigma) + \tau(\mu + s \mu_o)]^2 - \frac{\omega_1^2 + \omega_2^2}{12} \right) &+ \mathcal{O}(e^{-\alpha s}), \end{aligned}$$

We can regularize this divergence using zeta-function regularization ( $\sum_{n=1}^{\infty} n^s = \zeta(-s)$ )<sup>9</sup>

$$\begin{aligned} \prod_{n=-\infty}^{\infty} e^{-\text{sign}(n) \frac{\pi i}{2 \omega_1 \omega_2} \left( (m + \frac{n}{\tilde{r}_1} - \omega)^2 - \frac{\omega_1^2 + \omega_2^2}{12} \right)} &\longrightarrow \quad (13.7.12) \\ \exp(\Delta) \equiv \exp \left( \frac{i\pi (2m(3m \tilde{r}_1 + 1) - 2(1 - 6m \tilde{r}_1)\omega + \tilde{r}_1(\omega_1^2 + \omega_2^2 + 3\omega_1 \omega_2))}{12 \tilde{r}_1 \omega_1 \omega_2} \right). \end{aligned}$$

<sup>9</sup> Here we defined  $\text{sign}(n = 0) = -1$ .

The precise statement of (13.7.3) is then the following equality

$$e^{\mathcal{I}_0} \Gamma(u; p, q) = e^{-\Delta} \prod_{n=-\infty}^{\infty} \left[ e^{-\text{sign}(n) \frac{\pi i}{2\omega_1 \omega_2} \left( (m + \frac{n}{\tilde{r}_1} - \omega)^2 - \frac{\omega_1^2 + \omega_2^2}{12} \right)} \Gamma_h \left( m + \frac{n}{\tilde{r}_1}; \omega_1, \omega_2 \right) \right]. \quad (13.7.13)$$

The infinite product on the right-hand side is now well-defined, and in fact by using (13.7.4) and (13.2.14) it can be written as a product of two elliptic Gamma functions,

$$\Gamma(u; p, q) = e^{-\Delta - \mathcal{I}_0} \frac{\Gamma(e^{2\pi i \frac{m}{\omega_1}}; e^{2\pi i \frac{\omega_2}{\omega_1}}, e^{-2\pi i \frac{1}{\tilde{r}_1 \omega_1}})}{\Gamma(e^{2\pi i \frac{m - \omega_1}{\omega_2}}; e^{-2\pi i \frac{1}{\tilde{r}_1 \omega_2}}, e^{-2\pi i \frac{\omega_1}{\omega_2}})}. \quad (13.7.14)$$

This equality is discussed in [52]. It is sometimes viewed as an indication of an  $SL(3, \mathbb{Z})$  structure. Taking the  $3d$  limit by sending  $\tilde{r}_1$  to zero, we decouple the massive KK modes on the  $\tilde{S}^1$ . The only term surviving the limit on the right-hand side of (13.7.13) has  $n = 0$ , and we obtain

$$\lim_{\tilde{r}_1 \rightarrow 0} \left[ \Gamma(e^{2\pi i \tilde{r}_1 (\omega R + m)}; e^{2\pi i \tilde{r}_1 \omega_1}, e^{2\pi i \tilde{r}_1 \omega_2}) e^{\frac{\pi i}{6\omega_1 \omega_2 \tilde{r}_1} (m - \omega(1-R))} \right] = \Gamma_h(\omega R + m; \omega_1, \omega_2). \quad (13.7.15)$$

Note that the divergent factor is after turning on flavor fugacity and going to unsquashed sphere,  $\omega_1 = \omega_2 = \frac{1}{2\pi}i$  and  $\tilde{r}_1 = \tau$ ,

$$e^{\frac{\pi i}{6\omega_1 \omega_2 \tilde{r}_1} \omega(1-R)} = e^{\frac{\pi^2}{3\tau}(1-R)} = e^{-\frac{16\pi^2}{3\tau}(a-c)}, \quad (13.7.16)$$

in agreement with (13.7.1) since the anomalies of the chiral field are given by

$$a = \frac{1}{32}(9(R-1)^3 - 3(R-1)), \quad c = \frac{1}{32}(9(R-1)^3 - 5(R-1)), \quad a - c = \frac{1}{16}(R-1). \quad (13.7.17)$$

- *Reduction of gauge theories* – We can also consider the limit of small  $\tau$  for gauge theories. We will not review this in detail here, and only mention the salient features. Up to the divergent factor appearing in (13.7.1), and its generalization when flavor fugacities are present, the matrix model for the index reduces to the matrix model [53] used to compute  $\mathbb{S}_b^3$  partition function of the dimensionally reduced theory [21, 54–56]. Two comments are in order. First, the theories in four dimensions might have classical symmetries which are anomalous in the quantum theory. When reducing the theory on a circle a superpotential is produced which explicitly breaks these symmetries [21]. In the partition this manifests itself as a lack of real mass parameter for the symmetry which is anomalous in four dimension. These superpotentials are extremely important to understand what physics IR dualities in four dimensions reduce to in three dimensions. Second, in certain cases [14, 48] the three dimensional partition function in (13.7.1) is by itself divergent. Such examples include reductions of  $SO(N)$  gauge theories with  $\mathcal{N} = 1$  supersymmetry and  $SU(N)$  gauge theories with  $\mathcal{N} = 4$  supersymmetry. We refer the reader to Chapter 6 for details of the  $\mathbb{S}_b^3$  partition function.

### 13.7.2 Large $\tau$ limit, $\mathbb{S}^3 \rightarrow 0$

In this limit the radius of  $\mathbb{S}^3$  is much smaller than the radius of the circle and we effectively compactify the theory to quantum mechanics on a circle. The supersymmetric index in this limit computes the usual Witten index of the resulting quantum mechanics, that is the number of supersymmetric vacua. More concretely,

$$\mathcal{Z}_{\mathbb{S}^3 \times \mathbb{S}^1_{\tau \rightarrow \infty}} \rightarrow e^{-\tau E_{\text{Casimir}}} \#_{\text{vacua}}. \quad (13.7.18)$$

In particular since in the index we strip off the Casimir energy contribution it computes in the limit just the number of supersymmetric vacua. However, often a given theory might have a moduli space of vacua and the limit will diverge. In some examples we can keep some of the flavor fugacities which will regulate this divergence and give a finite result.

For  $\tau$  large,<sup>10</sup>

$$p, q \rightarrow 0. \quad (13.7.19)$$

We assume implicitly that the index we obtain is finite in the limit because we have enough flavor fugacities to lift the degeneracy of the moduli space (this is not always possible). The fugacities  $p$  and  $q$  couple to charges  $j_2 \pm j_1 + \frac{1}{2}r$ . Setting these fugacities to zero is well defined if for all states contributing to the index  $j_2 \pm j_1 + \frac{1}{2}r \geq 0$ . Let us assume that this is the case and soon we will discuss several examples. Then, the states which contribute to the index satisfy

$$j_2 \pm j_1 + \frac{1}{2}r = 0, \quad \rightarrow \quad j_1 = 0 \quad j_2 = -\frac{1}{2}r. \quad (13.7.20)$$

Moreover, since states contributing to the index satisfy  $E - 2j_2 - \frac{3}{2}r = 0$  we also get that  $E = \frac{1}{2}r$ . Now, from unitarity,

$$E \pm 2j_1 + \frac{3}{2}r \geq 0, \quad E \pm 2j_2 - \frac{3}{2}r \geq 0, \quad (13.7.21)$$

which imply that the states contributing to the limit we discuss have all charges vanishing,

$$E = r = j_1 = j_2 = 0. \quad (13.7.22)$$

Such states parametrize vacua of the model, *i.e.* the moduli space, as expected. Again, for the index to be well defined we will have to keep some of the flavor fugacities under which the operators contributing to the limit are charged.

Let us discuss the limit for a free chiral field. The limit is well defined if the R-charge is between zero and two. For R-charge vanishing the index is  $\frac{1}{1-u}$  where  $u$  is fugacity for the  $U(1)$  symmetry rotating the chiral. The index is give just by powers of the scalar component. This is the case when we can give a vacuum expectation value to the scalar parametrizing the moduli space, which will also break the  $U(1)_u$  symmetry. For  $r > 0$  but less than two the index is 1. For  $r = 2$  it becomes  $1 - u^{-1}$ . Note that R-charge two is outside the unitarity

<sup>10</sup>This limit has also been considered in [42].

bounds for free chiral and thus there is no physical meaning for this result. However, such an R-charge would be acceptable for a gauge non-invariant chiral matter field in gauge theory.

We now give a more interesting example. Pure  $SU(N)$  SYM has  $N$  vacua, however it also has a discrete R symmetry. To define the index we need continuous R symmetry and thus we will not discuss this example but rather turn on flavors. Consider  $SU(N)$  SQCD with  $N_f$  flavors. The standard choice of anomaly R-charge is  $\frac{N_f - N}{N_f}$  for all the matter fields. This choice keeps all the flavor symmetry manifest. Our limit is well defined here. The limit of  $p, q \rightarrow 0$  in this case is trivial, the index is 1 meaning that only the vacuum in the origin of field space satisfies (13.7.22). However, we can change the choice of R-charges keeping the condition for R-charges to be anomaly free,

$$\sum R_i + \sum \tilde{R}_i = 2N_f - 2N. \quad (13.7.23)$$

For example, let us assign  $N$  quarks and  $N$  anti-quarks R-charge zero, and the remaining matter R-charge one. The anomaly free condition above is satisfied. Taking our limit the index becomes

$$\mathcal{I}^{(N)}(\{t, \tilde{t}\}_{i=1}^N) = \frac{1}{N!} \oint \prod_{i=1}^{N-1} \frac{dz_i}{2\pi i z_i} \prod_{i \neq j} (1 - z_i/z_j) \prod_{i=1}^N \frac{1}{1 - t_i z_i} \frac{1}{1 - \tilde{t}_i z_i^{-1}}. \quad (13.7.24)$$

Note that  $N_f$  does not appear here anymore and there is no condition on fugacities  $t_i, \tilde{t}_i$ . This integral can be easily computed to give

$$\mathcal{I}^{(N)}(\{t, \tilde{t}\}_{i=1}^N) = (1 - \prod_{i=1}^N t_i \tilde{t}_i) \frac{1}{1 - \prod_{i=1}^N t_i} \frac{1}{1 - \prod_{i=1}^N \tilde{t}_i} \prod_{i,j=1}^N \frac{1}{1 - t_i \tilde{t}_j}. \quad (13.7.25)$$

This can be easily understood. The product is the product over the mesonic operators surviving the limit parametrizing a slice of the moduli space. The second and third terms are the baryon and the anti-baryon. The first term is an obvious constraint on this moduli space. We see that the index captures neatly a slice of the moduli space of the theory. This is equivalent to the so called Hilbert series of this slice (for discussion of Hilbert series see for example [58, 59]). We can ask how this limit behaves under Seiberg duality. On side B of the duality we will have  $SU(N_f - N)$  theory with  $N_f$  quarks/anti-quarks and gauge singlets dual to the mesons. The dual quarks in this case have again R-charges zero and one in our case, now  $N$  have R-charge 1 and  $N_f - N$  R-charge zero. The mesons which survive the limit have R-charge zero and R-charges two. Note that as we said above the latter cannot be physical because of the violation of unitarity bounds. The index of the dual theory is

$$\left[ \prod_{i,j=1}^N \frac{1}{1 - t_i \tilde{t}_j} \prod_{i,j=N+1}^{N_f} (1 - t_i^{-1} \tilde{t}_j^{-1}) \right] \times \mathcal{I}^{(N_f - N)}(\{ \frac{(\prod_{k=1}^{N_f} t_k)^{\frac{1}{N_f - N}}}{t_i}, \frac{(\prod_{k=1}^{N_f} \tilde{t}_k)^{\frac{1}{N_f - N}}}{\tilde{t}_i} \}_{i=N+1}^{N_f}). \quad (13.7.26)$$

We can now plug in the result from (13.7.25) for  $\mathcal{I}^{(N_f - N)}$  and

$$\prod_{k=1}^{N_f} \tilde{t}_k \prod_{k=1}^{N_f} t_k = 1, \quad (13.7.27)$$

from anomaly cancellation to obtain that the above is equal to

$$\begin{aligned}
& \left[ \prod_{i,j=1}^N \frac{1}{1-t_i \tilde{t}_j} \prod_{i,j=N+1}^{N_f} (1-t_i^{-1} \tilde{t}_j^{-1}) \right] \times \left( 1 - \prod_{i=N+1}^{N_f} t_i^{-1} \tilde{t}_i^{-1} \right) \tag{13.7.28} \\
& \frac{1}{1 - \prod_{k=1}^{N_f} t_k \prod_{i=N+1}^{N_f} t_i^{-1}} \frac{1}{1 - \prod_{k=1}^{N_f} \tilde{t}_k \prod_{i=N+1}^{N_f} \tilde{t}_i^{-1}} \prod_{i,j=N+1}^{N_f} \frac{1}{1 - t_i^{-1} \tilde{t}_j^{-1}} = \\
& \frac{1}{1 - \prod_{k=1}^N t_k} \frac{1}{1 - \prod_{k=1}^N \tilde{t}_k} \left( 1 - \prod_{i=1}^N t_i \tilde{t}_i \right) \prod_{i,j=1}^N \frac{1}{1 - t_i \tilde{t}_j},
\end{aligned}$$

in agreement with (13.7.25).

Note that naively it is important in the gauge theory for the limit to be well defined to have the R-charges of all the chiral fields to be between zero and two. However, even if some of the charges of chirals are outside of this region the limit might be well behaved. Consider for example giving R-charge zero to  $N_f + N$  chiral fields and R-charge two to  $N_f - N$ . This is an anomaly free R-charge. Assuming that  $N_f + N$  is even, we might split the choice above equally between the quarks and anti-quarks, that is giving R-charge zero to  $\frac{N_f+N}{2}$  flavors. In such a case the R-charges of the dual theory are one for  $\frac{N_f+N}{2}$  flavors and  $-1$  for  $\frac{N_f-N}{2}$ . Thus although naively the limit of the matter is singular from the duality we know that the limit for the gauge invariant operators has to be well defined.

In summary, the  $p, q$  to zero limit captures protected information associated to a certain submanifold of the moduli space of the theory. The precise submanifold is determined by the choice of the R-charges. One can in principle consider other limits on fugacities coupling to combinations of charges which for a given model are non-negative for states contributing to the index. However since the index gets contributions from fermions and bosons in conjugate representations the index would usually get contributions from both negatively and positively charged objects unless the limit is for an R-symmetry. In certain cases the information captured in this limit is equivalent to the Hilbert series of the moduli space. An example is given by [60] the limit of the index of  $\mathcal{N} = 2$  theories corresponding to genus zero Riemann surfaces in class  $\mathcal{S}$  terminology [61]. See also [62–64] for the 3d variants of such limits.

### 13.7.3 Poles and residues

The index is a meromorphic function of the fugacities and in general has numerous poles. Let us assume the index has a behavior of the following form,

$$\mathcal{I}_0(a_1, a_2, \dots) = \frac{\mathcal{I}'(a_1, a_2, \dots)}{1 - a_1}, \tag{13.7.29}$$

where  $a_i$  are some fugacities and we assume  $\mathcal{I}'$  has no zeros or poles at  $a_1 = 1$ . From the trace interpretation of the index we deduce that there is a bosonic operator in the theory,  $\mathcal{O}$ , with charges such that it contributes with weight  $a_1$  to the index. Moreover, any power of

this operator also contributes to the index. The pole at  $a_1 = 1$  corresponds to computing the index while giving weight 1 to  $\mathcal{O}$ . Putting it differently, we consider turning on only fugacities for symmetries consistent with giving a vacuum expectation value for  $\mathcal{O}$ . It is thus natural to interpret the residue of the pole as the index of the theory obtained as the IR fixed point of an RG flow triggered by vacuum expectation value for  $\mathcal{O}$ .

We have encountered an example of the effect of vacuum expectation values while discussing Higgsing in section 13.4. Let us give several additional examples. First let us consider a sigma model with two chiral fields and a superpotential

$$W = \Phi_1 \Phi_2^2. \quad (13.7.30)$$

We have one  $U(1)_a$  global symmetry preserved by the superpotential and we choose  $\Phi_1$  to have charge  $-2$  and  $\Phi_2$  has charge  $+1$ . We also assign R-charge  $2R$  to  $\Phi_1$  and  $1 - R$  to  $\Phi_2$ . The index of the model is given by

$$\mathcal{I}(a) = \Gamma((pq)^R a^{-2}) \Gamma((pq)^{\frac{1-R}{2}} a). \quad (13.7.31)$$

Note that the chiral ring here has the relations

$$\Phi_1 \Phi_2 \sim 0, \quad \Phi_2^2 \sim 0. \quad (13.7.32)$$

In particular, as we already discussed not all powers of the scalar component of  $\Phi_2$  contribute to the index, but any power of the scalar from  $\Phi_1$  appears. This index has many poles one of which is at  $a = (pq)^{\frac{R}{2}}$ . The operator which leads to the divergence is the scalar component of  $\Phi_1$ . The residue is given by

$$\mathcal{I}(a) \sim \frac{1}{1 - (pq)^R a^{-2}} \Gamma((pq)^{\frac{1}{2}}) \mathcal{I}_V^{-1} + O(1). \quad (13.7.33)$$

The index of  $\Phi_2$  becomes  $\Gamma((pq)^{\frac{1}{2}}) = 1$ , which is the index of a massive fields since the vacuum expectation value for  $\Phi_1$  generates a mass term for  $\Phi_2$ . The index of field  $\Phi_1$  stripping off the divergence is  $\Gamma(1)' = \frac{1}{(q;q)(p;p)} = \mathcal{I}_V^{-1}$  which is the index of the Nambu-Goldstone boson corresponding to the broken  $U(1)_a$  symmetry. The residue is thus just given by the index of the Nambu-Goldstone boson as expected as the theory is empty in the IR. It is thus natural to write the general relation

$$\mathcal{I}_0(a_1 \rightarrow 1) = \frac{1}{1 - a_1} \mathcal{I}_{IR}(a_2, \dots) \mathcal{I}_{Nam.-Gold.} + O(1). \quad (13.7.34)$$

We consider now a more involved example of a gauge theory. The theory we discuss is  $SU(2) \times SU(2)$  quiver gauge theory of figure 13.7.1. The superpotential is

$$W = Q_1 \Phi_1 \tilde{Q}_1 + Q_2 \Phi_2 \tilde{Q}_2. \quad (13.7.35)$$

We will assign R-charge zero to the  $Q_i$  and  $\tilde{Q}_i$  fields and R-charge two to  $\Phi_j$ . This model has three abelian global symmetries which we will denote by  $U(1)_T \times U(1)_X \times U(1)_Y$ . The different fields have the charges specified in Table 3.

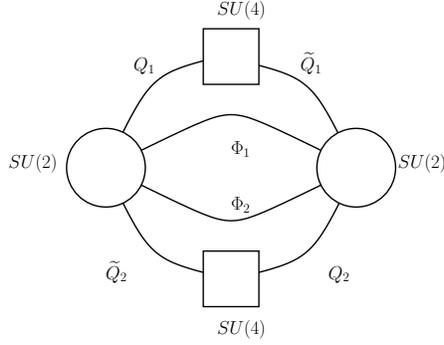

Figure 13.7.1: An  $SU(2) \times SU(2)$  quiver gauge theory.

|               | $U(1)_T$ | $U(1)_X$ | $U(1)_Y$ | $U(1)_R$ |
|---------------|----------|----------|----------|----------|
| $\Phi_1$      | -2       | +2       | 0        | 2        |
| $\Phi_2$      | -2       | -2       | 0        | 2        |
| $Q_1$         | +1       | -1       | +1       | 0        |
| $\tilde{Q}_1$ | +1       | -1       | -1       | 0        |
| $Q_2$         | +1       | +1       | -1       | 0        |
| $\tilde{Q}_2$ | +1       | +1       | +1       | 0        |

Table 13.7.1: Abelian charges of fields.

We can consider giving a vacuum expectation value to a baryonic operator of the form  $B_Q = \epsilon \cdot Q_1^2$ . This will Higgs one of the  $SU(2)$  gauge groups and reduce the rank of the flavor group by one. Let us analyze how this comes about from the index. The index of the model is given by,

$$\mathcal{I} = \kappa^2 \oint \frac{dz_1}{4\pi i z_1 \Gamma(z_1^{\pm 1})} \oint \frac{dz_2}{4\pi i z_2 \Gamma(z_2^{\pm 2})} \Gamma\left(\frac{pq}{T^2} X^{\pm 2} z_1^{\pm 1} z_2^{\pm 1}\right) \times \quad (13.7.36)$$

$$\prod_{i=1}^4 \Gamma\left(\frac{TY}{X} u_i z_1^{\pm 1}\right) \Gamma(TY X v_i^{-1} z_2^{\pm 1}) \Gamma\left(\frac{T}{YX} u_i^{-1} z_2^{\pm 1}\right) \Gamma\left(\frac{TX}{Y} v_i z_1^{\pm 1}\right).$$

We have two  $SU(4)$  symmetries with fugacities  $u_i$  and  $v_i$ . Baryon  $B_Q$  contributes to the index with weight  $\frac{T^2 Y^2}{X^2} u_1 u_2$  where we have made a choice of the subgroup of  $SU(4)_u$  under which  $B_Q$  is charged. Giving a vacuum expectation value to  $B_Q$  we set the weight of the operator to one,

$$\frac{T^2 Y^2}{X^2} u_1 u_2 = 1.$$

With this specification of parameters the field  $Q_1$  contributes to the index as,

$$\Gamma\left(\frac{TY}{X}u_iz_1^{\pm 1}\right) \rightarrow \Gamma\left(\frac{1}{\sqrt{u_1u_2}}u_iz_1^{\pm 1}\right). \quad (13.7.37)$$

Before the specification this field had poles in  $z_1$  at, among others,

$$z_1 = \frac{TY}{X}u_1, \frac{TY}{X}u_2, \quad z_1 = \frac{X}{TY}u_1^{-1}, \frac{X}{TY}u_2^{-1},$$

with the former inside the unit circle and latter outside assuming that  $|T| < 1$  and all other fugacities for global symmetries being phases. The integration contour thus lies between these poles. However after the specification the poles above inside and outside of the circle collide and pinch the integration contour at  $z_1 = \sqrt{\frac{u_1}{u_2}}, \sqrt{\frac{u_2}{u_1}}$ . This causes the integral over  $z_1$  to diverge. The residue of this divergence is,

$$2\kappa \text{Res}_{\frac{T^2Y^2}{X^2}u_1u_2 \rightarrow 1} \mathcal{I} = \prod_{i=3}^4 \Gamma\left(\frac{u_i}{u_1}\right) \Gamma\left(\frac{u_i}{u_2}\right) \prod_{i=1}^4 \Gamma(T^2v_iu_1) \Gamma(T^2v_iu_2) \times \quad (13.7.38)$$

$$\kappa \oint \frac{dz_2}{4\pi iz_2 \Gamma(z_2^{\pm 2})} \Gamma\left(\frac{pq}{T^4Y^2} \frac{1}{u_1u_2} \left(\sqrt{\frac{u_1}{u_2}}\right)^{\pm 1} z_2^{\pm 1}\right) \prod_{i=3}^4 \Gamma\left(\frac{1}{Y^2} \frac{u_i^{-1}}{\sqrt{u_1u_2}} z_2^{\pm 1}\right) \prod_{i=1}^4 \Gamma(T^2Y^2v_i^{-1} \sqrt{u_1u_2} z_2^{\pm 1}).$$

This is the index of  $\mathcal{N} = 1$   $SU(2)$  SCFT with four flavors and additional singlet fields coupled to the charged matter through a superpotential. This is exactly the matter content one would expect after giving a vacuum expectation value to baryon  $B_Q$ .

More general poles correspond to turning on vacuum expectation values to derivatives of operators and thus break explicitly Lorentz invariance. The theory in the IR is expected to have co-dimension two defects. The residue computes then an index of a theory in presence of such defects. Such flows and corresponding defects were discussed in the  $\mathcal{N} = 2$  context in [33] and in  $\mathcal{N} = 1$  context in [65] (see [66] for a review). The IR theory here has  $4d$  degrees of freedom coupled to  $2d$  ones, and the index is often expressible as some difference operator, shifting flavor fugacities by general powers of  $p$  and  $q$ , acting on the four dimensional index [33, 35, 65, 67]. This is reminiscent of the observation below (13.6.5).

### 13.7.4 Large $N$ limit

The matrix models of indices of gauge theories can be simplified and explicitly evaluated in the limit of large number of colors using large  $N$  matrix model techniques (see *e.g.* [4, 19]). Let us here give a general result for the large  $N$  limit of an index of a quiver gauge theory with  $U(N)$  gauge groups. We follow here the discussion and notations of [68].

We consider a quiver theory with gauge group  $\prod_{a=1}^s U(N_a)_{u_a}$ . Let  $\{e^{\alpha_{ai}}\}_{i=1}^{N_a}$  denote the  $N_a$  eigenvalues of  $u_a$ . Then the matrix model integral (13.2.12) is,

$$\mathcal{I}(x) = \int \prod_{a,i} [d\alpha_{ai}] \exp \left\{ - \sum_{ai \neq bj} V_b^a(\alpha_{ai} - \alpha_{bj}) \right\}. \quad (13.7.39)$$

Here, the potential  $V$  is the following function

$$V_b^a(\theta) = \delta_b^a(\ln 2) + \sum_{n=1}^{\infty} \frac{1}{n} [\delta_b^a - i_b^a(x^n)] \cos n\theta, \quad (13.7.40)$$

where,  $i_b^a(x)$  is the total single letter index in the representation  $r^a \otimes r_b$  and  $x$  stands for all the fugacities we can turn on. Writing the density of the eigenvalues  $\{e^{\alpha_{ai}}\}$  at the point  $\theta$  on the circle as  $\rho_a(\theta)$ , we reduce it to the functional integral problem,

$$\mathcal{I}(x) = \int \prod_a [d\rho_a] \exp\left\{-\int d\theta_1 d\theta_2 \sum_{a,b} n_a n_b \rho_a(\theta_1) V_b^a(\theta_1 - \theta_2) \rho_b^\dagger(\theta_2)\right\}. \quad (13.7.41)$$

For large  $N$ , we can evaluate this expression with the saddle point approximation,

$$\mathcal{I}(x) = \prod_k \frac{1}{\det(1 - i(x^k))}.$$

For  $SU(N)$  gauge groups instead of  $U(N)$ , the result is modified as follows,

$$\mathcal{I}(x) = \prod_k \frac{e^{-\frac{1}{k} \text{tr } i(x^k)}}{\det(1 - i(x^k))}. \quad (13.7.42)$$

Here  $i(x)$  is the matrix with entries  $i_b^a(x)$ .

The single-trace partition function can be obtained from the full partition function,

$$\mathcal{I}_{s.t.} = \sum_{n=1}^{\infty} \frac{\mu(n)}{n} \log \mathcal{I}(x^n) \quad (13.7.43)$$

$$= -\sum_{k=1}^{\infty} \frac{\varphi(k)}{k} \log[\det(1 - i(x^k))] - \sum_{n=1}^{\infty} \frac{\mu(n)}{n} \sum_{k=1}^{\infty} \frac{\text{tr } i(x^{nk})}{k} \quad (13.7.44)$$

$$= -\sum_{k=1}^{\infty} \frac{\varphi(k)}{k} \log[\det(1 - i(x^k))] - \text{tr } i(x). \quad (13.7.45)$$

The second term in the summation would be absent for the  $U(N)$  gauge theories. Here  $\mu(n)$  is the Möbius function ( $\mu(1) \equiv 1$ ,  $\mu(n) \equiv 0$  if  $n$  has repeated prime factors and  $\mu(n) \equiv (-1)^k$  if  $n$  is the product of  $k$  distinct primes) and  $\varphi(n)$  is the Euler Phi function, defined as the number of positive integers less than  $n$  that are coprime to  $n$ . We have used the properties

$$\sum_{d|n} d\mu\left(\frac{n}{d}\right) = \varphi(n), \quad \sum_{d|n} \mu(d) = \delta_{n,1}. \quad (13.7.46)$$

Indices in the large  $N$  limit can be used to check holographic dualities. For example the index of  $\mathcal{N} = 4$  SYM in this limit can be matched with the spectrum of fields in  $AdS_5$  computed in supergravity [4]. The large  $N$  indices [68] of a variety of  $Y_{p,q}$  models [69] were also matched with the holographic duals [70]. In general the field theory expressions in the large  $N$  limit are rather simple though the dual holographic computation can be involved, see [70]. For example, the index of  $\mathcal{N} = 2$  class  $\mathcal{S}$  theories [61] of genus  $\mathfrak{g}$  is explicitly known in large  $N$  limit [60] though that simple result was not yet reproduced from the gravity side [71].

## 13.8 Other topics and open problems

There are many other interesting related topics that we could review here. We conclude with a brief mention of a few of them:

- *Holomorphic blocks* – The localization procedure leading directly to the trace-formula formulation of the index is the so called Coulomb branch localization. The computation reduces to a matrix integral over the zero modes of the vector field in the direction of  $\mathbb{S}_r^1$ . The name comes from the fact that these components upon reduction to three dimensions become scalar components in the vector multiplet and parametrize the Coulomb branch. However, there is a different localization procedure one can employ [72–74]. The dimensional reduction of this procedure to three dimensions leads to the so called Higgs branch localization form for the index [75–77]. In this localization procedure the index can be written as a finite sum over vortex/anti-vortex partition functions which are effectively partition functions on  $\mathbb{C} \times T^2$ . This “holomorphic block” factorization of the partition function is extremely powerful since it connects together a priori unrelated partition functions. By gluing differently the blocks one can obtain various geometry and thus relate the supersymmetric index for example to  $\mathbb{S}^2 \times T^2$  partition function. Let us mention here only the simplest example of such a factorization in the case of a free chiral field. Here we have

$$\mathcal{I}^{(R)}(a) = \Gamma((pq)^{\frac{R}{2}} a; p, q) = \Gamma((pq)^{\frac{R}{2}} a; p, pq) \Gamma((pq)^{\frac{R}{2}} qa; q, pq). \quad (13.8.1)$$

There are many interesting results yet to be uncovered following this direction.

- *Lens space index* – As was mentioned in the introduction the supersymmetric index is a special case of a sequence of partition functions, the lens space indices  $\mathbb{S}^3/\mathbb{Z}_r \times \mathbb{S}^1$  [78]. As a counting problem the lens index is computed as follows. Since the geometry involves an orbifold projection the lens index receives contributions from local operators consistent with the action of the orbifold. Let us call this sector the “untwisted” one. Let us again here give just an example of the lens index of a free chiral field in the “untwisted” sector,

$$\mathcal{I}_r^{(R)}(a) = \Gamma((pq)^{\frac{R}{2}} a; p^r, pq) \Gamma((pq)^{\frac{R}{2}} q^r a; q^r, pq). \quad (13.8.2)$$

On the other hand, for  $r > 1$  the lens space  $\mathbb{S}^3/\mathbb{Z}_r$  has a non-contractable torsion cycle, and upon quantizing the theory on this space one should consider configurations wrapping this cycle. This leads to a finite number, since the cycle is torsion, of “twisted” sectors which receive contributions from extended objects in the theory. Thus although the supersymmetric index,  $r = 1$ , gets contributions only from local operators, the lens index captures a much larger variety of objects. Moreover, the spectrum of the non-local objects is sensitive to the global structure of the gauge groups [79] and not just to the Lie algebras making lens indices a more refined characteristic of the physics.

Taking the limit of large  $r$  the non-trivial cycle of the lens space shrinks to zero size and  $S^3/\mathbb{Z}_r$  becomes  $S^2$ . In this limit the lens index in four dimensions reduces to the supersymmetric index in three dimensions. The finite sum over the twisted sectors becomes an infinite sum over monopoles sectors in three dimensions. Although there are several works studying the lens index it has been largely neglected and there are many avenues for farther research.

- *Relations to integrable models* – Finally let us mention that the supersymmetric index is closely related to quantum mechanical integrable systems. These relations come in different forms. For example the (lens) index itself can be related to partition function of two dimensional lattice integrable models [80,81]. On the other hand, as we discussed in the previous sections, computing indices of theories in presence of surface defects amounts to acting on indices without defects with difference operators [33,65,82]. Such difference operators are Hamiltonians for well known Ruijsenaars-Schneider integrable systems when the theories are  $\mathcal{N} = 2$  [33,67,83–85], and give rise to novel integrable models when one has  $\mathcal{N} = 1$  supersymmetry [65,86,87]. These relations deserve a much more thorough investigation.

## Acknowledgements

We would like to thank Ofer Aharony, Chris Beem, Abhijit Gadde, Davide Gaiotto, Guido Festuccia, Zohar Komargodski, Nathan Seiberg, Brian Willett, Wenbin Yan for fruitful collaborations and numerous discussions on the topics reviewed here. LR is supported in part by NSF Grant PHY-1316617. SSR is a Jacques Lewiner Career Advancement Chair fellow. This research was also supported by Israel Science Foundation under grant no. 1696/15 and by I-CORE Program of the Planning and Budgeting Committee.

## References

- [1] V. Pestun and M. Zabzine, eds., *Localization techniques in quantum field theory*, vol. xx. Journal of Physics A, 2016. 1608.02952. <https://arxiv.org/src/1608.02952/anc/LocQFT.pdf>, <http://pestun.ihep.fr/pages/LocalizationReview/LocQFT.pdf>.
- [2] V. Pestun, “Localization of gauge theory on a four-sphere and supersymmetric Wilson loops,” [arXiv:0712.2824](https://arxiv.org/abs/0712.2824) [hep-th].
- [3] K. Hosomichi, “ $\mathcal{N} = 2$  SUSY gauge theories on  $S^4$ ,” *Journal of Physics A* **xx** (2016) 000, 1608.02962.
- [4] J. Kinney, J. M. Maldacena, S. Minwalla, and S. Raju, “An index for 4 dimensional super conformal theories,” *Commun. Math. Phys.* **275** (2007) 209–254, [arXiv:hep-th/0510251](https://arxiv.org/abs/hep-th/0510251).
- [5] C. Romelsberger, “Counting chiral primaries in  $\mathcal{N} = 1$ ,  $d=4$  superconformal field theories,” *Nucl. Phys.* **B747** (2006) 329–353, [arXiv:hep-th/0510060](https://arxiv.org/abs/hep-th/0510060).
- [6] C. Romelsberger, “Calculating the Superconformal Index and Seiberg Duality,” [arXiv:0707.3702](https://arxiv.org/abs/0707.3702) [hep-th].

- [7] B. I. Zwiebel, “Charging the Superconformal Index,” *JHEP* **01** (2012) 116, [arXiv:1111.1773 \[hep-th\]](#).
- [8] G. Festuccia and N. Seiberg, “Rigid Supersymmetric Theories in Curved Superspace,” *JHEP* **1106** (2011) 114, [arXiv:1105.0689 \[hep-th\]](#).
- [9] D. Sen, “Supersymmetry in the Space-time  $R \times S^{*3}$ ,” *Nucl. Phys.* **B284** (1987) 201.
- [10] T. Dumitrescu, “An Introduction to Supersymmetric Field Theories in Curved Space,” *Journal of Physics A* **xx** (2016) 000, [1608.02957](#).
- [11] C. Closset and I. Shamir, “The  $\mathcal{N} = 1$  Chiral Multiplet on  $T^2 \times S^2$  and Supersymmetric Localization,” *JHEP* **03** (2014) 040, [arXiv:1311.2430 \[hep-th\]](#).
- [12] B. Assel, D. Cassani, and D. Martelli, “Localization on Hopf surfaces,” *JHEP* **08** (2014) 123, [arXiv:1405.5144 \[hep-th\]](#).
- [13] H.-C. Kim and S. Kim, “M5-branes from gauge theories on the 5-sphere,” [arXiv:1206.6339 \[hep-th\]](#).
- [14] A. A. Ardehali, “High-temperature asymptotics of supersymmetric partition functions,” [arXiv:1512.03376 \[hep-th\]](#).
- [15] B. Assel, D. Cassani, L. Di Pietro, Z. Komargodski, J. Lorenzen, and D. Martelli, “The Casimir Energy in Curved Space and its Supersymmetric Counterpart,” *JHEP* **07** (2015) 043, [arXiv:1503.05537 \[hep-th\]](#).
- [16] N. Bobev, M. Bullimore, and H.-C. Kim, “Supersymmetric Casimir Energy and the Anomaly Polynomial,” *JHEP* **09** (2015) 142, [arXiv:1507.08553 \[hep-th\]](#).
- [17] F. A. Dolan and H. Osborn, “Applications of the Superconformal Index for Protected Operators and q-Hypergeometric Identities to  $N=1$  Dual Theories,” *Nucl. Phys.* **B818** (2009) 137–178, [arXiv:arXiv:0801.4947 \[hep-th\]](#).
- [18] S. Benvenuti, B. Feng, A. Hanany, and Y.-H. He, “Counting BPS operators in gauge theories: Quivers, syzygies and plethystics,” *JHEP* **11** (2007) 050, [arXiv:hep-th/0608050](#).
- [19] O. Aharony, J. Marsano, S. Minwalla, K. Papadodimas, and M. Van Raamsdonk, “The Hagedorn / deconfinement phase transition in weakly coupled large  $N$  gauge theories,” *Adv. Theor. Math. Phys.* **8** (2004) 603–696, [arXiv:hep-th/0310285](#).
- [20] A. Gadde, E. Pomoni, L. Rastelli, and S. S. Razamat, “S-duality and 2d Topological QFT,” *JHEP* **03** (2010) 032, [arXiv:0910.2225 \[hep-th\]](#).
- [21] O. Aharony, S. S. Razamat, N. Seiberg, and B. Willett, “3d dualities from 4d dualities,” *JHEP* **07** (2013) 149, [arXiv:1305.3924 \[hep-th\]](#).
- [22] N. Seiberg, “Electric - magnetic duality in supersymmetric nonAbelian gauge theories,” *Nucl. Phys.* **B435** (1995) 129–146, [arXiv:hep-th/9411149 \[hep-th\]](#).
- [23] V. Spiridonov, “On the elliptic beta function,” *Russian Mathematical Surveys* **56:1** (2001) 185.
- [24] V. Spiridonov, “Essays on the theory of elliptic hypergeometric functions,” *Uspekhi Mat. Nauk* **63 no 3** (2008) 3–72, [arXiv:0805.3135](#).
- [25] E. M. Rains, “Transformations of Elliptic Hypergeometric Integrals ,” [math/0309252](#).
- [26] V. Spiridonov and G. Vartanov, “Elliptic hypergeometric integrals and ’t Hooft anomaly matching conditions,” *JHEP* **1206** (2012) 016, [arXiv:1203.5677 \[hep-th\]](#).
- [27] V. P. Spiridonov and S. O. Warnaar, “Inversions of integral operators and elliptic beta integrals on root systems ,” *Adv. Math.* **207** (2006) 91–132, [math/0411044](#).

- [28] C. Beem and A. Gadde, “The  $N = 1$  superconformal index for class  $S$  fixed points,” *JHEP* **1404** (2014) 036, [arXiv:1212.1467 \[hep-th\]](#).
- [29] D. Green, Z. Komargodski, N. Seiberg, Y. Tachikawa, and B. Wecht, “Exactly Marginal Deformations and Global Symmetries,” *JHEP* **06** (2010) 106, [arXiv:1005.3546 \[hep-th\]](#).
- [30] F. J. van de Bult, “An elliptic hypergeometric integral with  $W(F_4)$  symmetry,” [arXiv:0909.4793](#).
- [31] V. P. Spiridonov and G. S. Vartanov, “Superconformal indices for  $\mathcal{N} = 1$  theories with multiple duals,” *Nucl. Phys.* **B824** (2010) 192–216, [arXiv:0811.1909 \[hep-th\]](#).
- [32] T. Dimofte and D. Gaiotto, “An E7 Surprise,” *JHEP* **10** (2012) 129, [arXiv:1209.1404 \[hep-th\]](#).
- [33] D. Gaiotto, L. Rastelli, and S. S. Razamat, “Bootstrapping the superconformal index with surface defects,” *JHEP* **01** (2013) 022, [arXiv:1207.3577 \[hep-th\]](#).
- [34] D. Gaiotto and H.-C. Kim, “Surface defects and instanton partition functions,” *ArXiv e-prints* (2014) , [arXiv:1412.2781 \[hep-th\]](#).
- [35] A. Gadde and S. Gukov, “2d index and surface operators,” *Journal of High Energy Physics* **3** (2014) 80, [arXiv:1305.0266 \[hep-th\]](#).
- [36] V. Spiridonov and G. Vartanov, “Superconformal indices of  $N=4$  SYM field theories,” [arXiv:1005.4196 \[hep-th\]](#).
- [37] D. Kutasov, “A Comment on duality in  $N=1$  supersymmetric nonAbelian gauge theories,” *Phys. Lett.* **B351** (1995) 230–234, [arXiv:hep-th/9503086 \[hep-th\]](#).
- [38] D. Kutasov and A. Schwimmer, “On duality in supersymmetric Yang-Mills theory,” *Phys. Lett.* **B354** (1995) 315–321, [arXiv:hep-th/9505004 \[hep-th\]](#).
- [39] K. A. Intriligator and B. Wecht, “RG fixed points and flows in SQCD with adjoints,” *Nucl. Phys.* **B677** (2004) 223–272, [arXiv:hep-th/0309201 \[hep-th\]](#).
- [40] D. Kutasov and J. Lin, “Exceptional  $N=1$  Duality,” [arXiv:1401.4168 \[hep-th\]](#).
- [41] D. Kutasov and J. Lin, “ $N=1$  Duality and the Superconformal Index,” [arXiv:1402.5411 \[hep-th\]](#).
- [42] V. P. Spiridonov and G. S. Vartanov, “Elliptic hypergeometry of supersymmetric dualities,” [arXiv:0910.5944 \[hep-th\]](#).
- [43] V. Spiridonov and G. Vartanov, “Elliptic hypergeometry of supersymmetric dualities II. Orthogonal groups, knots, and vortices,” [arXiv:1107.5788 \[hep-th\]](#).
- [44] V. Spiridonov, “Elliptic hypergeometric terms,” [arXiv:1003.4491 \[math.CA\]](#).
- [45] V. Spiridonov, “Classical elliptic hypergeometric functions and their applications ,” *Rokko Lect. in Math. Vol. 18, Dept. of Math, Kobe Univ.* (2005) 253–287, [arXiv:math/0511579](#).
- [46] V. Spiridonov, “Elliptic hypergeometric functions,” [arXiv:0704.3099](#).
- [47] C. Closset, T. T. Dumitrescu, G. Festuccia, and Z. Komargodski, “Supersymmetric Field Theories on Three-Manifolds,” *JHEP* **05** (2013) 017, [arXiv:1212.3388 \[hep-th\]](#).
- [48] O. Aharony, S. S. Razamat, N. Seiberg, and B. Willett, “3d dualities from 4d dualities for orthogonal groups,” *JHEP* **1308** (2013) 099, [arXiv:1307.0511](#).
- [49] K. A. Intriligator, N. Seiberg, and S. H. Shenker, “Proposal for a simple model of dynamical SUSY breaking,” *Phys. Lett.* **B342** (1995) 152–154, [arXiv:hep-ph/9410203 \[hep-ph\]](#).
- [50] G. Vartanov, “On the ISS model of dynamical SUSY breaking,” *Phys.Lett.* **B696** (2011) 288–290, [arXiv:1009.2153 \[hep-th\]](#).

- [51] Y. Imamura and D. Yokoyama, “N=2 supersymmetric theories on squashed three-sphere,” *Phys. Rev.* **D85** (2012) 025015, [arXiv:1109.4734 \[hep-th\]](#).
- [52] G. Felder and A. Varchenko, “The elliptic gamma function and  $SL(3, Z) \times \mathbb{Z}^3$ ,” *ArXiv Mathematics e-prints* (1999) , [math/9907061](#).
- [53] A. Kapustin, B. Willett, and I. Yaakov, “Exact Results for Wilson Loops in Superconformal Chern-Simons Theories with Matter,” *JHEP* **03** (2010) 089, [arXiv:0909.4559 \[hep-th\]](#).
- [54] F. Dolan, V. Spiridonov, and G. Vartanov, “From 4d superconformal indices to 3d partition functions,” [arXiv:1104.1787 \[hep-th\]](#).
- [55] Y. Imamura, “Relation between the 4d superconformal index and the  $S^3$  partition function,” [arXiv:1104.4482 \[hep-th\]](#).
- [56] A. Gadde and W. Yan, “Reducing the 4d Index to the  $S^3$  Partition Function,” *JHEP* **1212** (2012) 003, [arXiv:1104.2592 \[hep-th\]](#).
- [57] B. Willett, “Localization on three-dimensional manifolds,” *Journal of Physics A* **xx** (2016) 000, [1608.02958](#).
- [58] J. Gray, A. Hanany, Y.-H. He, V. Jejjala, and N. Mekareeya, “SQCD: A Geometric Apercu,” *JHEP* **0805** (2008) 099, [arXiv:0803.4257 \[hep-th\]](#).
- [59] A. Hanany and N. Mekareeya, “Counting Gauge Invariant Operators in SQCD with Classical Gauge Groups,” *JHEP* **10** (2008) 012, [arXiv:0805.3728 \[hep-th\]](#).
- [60] A. Gadde, L. Rastelli, S. S. Razamat, and W. Yan, “Gauge Theories and Macdonald Polynomials,” *Commun.Math.Phys.* **319** (2013) 147–193, [arXiv:1110.3740 \[hep-th\]](#).
- [61] D. Gaiotto, “N=2 dualities,” [arXiv:arXiv:0904.2715 \[hep-th\]](#).
- [62] S. S. Razamat and B. Willett, “Down the rabbit hole with theories of class S,” [arXiv:1403.6107 \[hep-th\]](#).
- [63] S. Cremonesi, “The Hilbert series of 3d  $\mathcal{N} = 2$  Yang-Mills theories with vectorlike matter,” *J. Phys.* **A48** (2015) no. 45, 455401, [arXiv:1505.02409 \[hep-th\]](#).
- [64] A. Hanany, C. Hwang, H. Kim, J. Park, and R.-K. Seong, “Hilbert Series for Theories with Aharony Duals,” *JHEP* **11** (2015) 132, [arXiv:1505.02160 \[hep-th\]](#). [Addendum: *JHEP*04,064(2016)].
- [65] D. Gaiotto and S. S. Razamat, “ $\mathcal{N} = 1$  theories of class  $\mathcal{S}_k$ ,” *JHEP* **07** (2015) 073, [arXiv:1503.05159 \[hep-th\]](#).
- [66] L. Rastelli and S. S. Razamat, “The Superconformal Index of Theories of Class  $\mathcal{S}$ ,” in *New Dualities of Supersymmetric Gauge Theories*, J. Teschner, ed., pp. 261–305. 2016. [arXiv:1412.7131 \[hep-th\]](#).
- [67] L. F. Alday, M. Bullimore, M. Fluder, and L. Hollands, “Surface defects, the superconformal index and q-deformed Yang-Mills,” [arXiv:1303.4460 \[hep-th\]](#).
- [68] A. Gadde, L. Rastelli, S. S. Razamat, and W. Yan, “On the Superconformal Index of N=1 IR Fixed Points: A Holographic Check,” *JHEP* **1103** (2011) 041, [arXiv:1011.5278 \[hep-th\]](#).
- [69] S. Benvenuti, S. Franco, A. Hanany, D. Martelli, and J. Sparks, “An infinite family of superconformal quiver gauge theories with Sasaki-Einstein duals,” *JHEP* **06** (2005) 064, [arXiv:hep-th/0411264](#).
- [70] R. Eager, J. Schmude, and Y. Tachikawa, “Superconformal Indices, Sasaki-Einstein Manifolds, and Cyclic Homologies,” *Adv. Theor. Math. Phys.* **18** (2014) no. 1, 129–175, [arXiv:1207.0573 \[hep-th\]](#).
- [71] D. Gaiotto and J. Maldacena, “The gravity duals of N=2 superconformal field theories,” [arXiv:arXiv:0904.4466 \[hep-th\]](#).

- [72] W. Peelaers, “Higgs branch localization of  $\mathcal{N} = 1$  theories on  $S^3 \times S^1$ ,” *JHEP* **08** (2014) 060, [arXiv:1403.2711 \[hep-th\]](#).
- [73] Y. Yoshida, “Factorization of 4d  $\mathcal{N}=1$  superconformal index,” [arXiv:1403.0891 \[hep-th\]](#).
- [74] F. Nieri and S. Pasquetti, “Factorisation and holomorphic blocks in 4d,” *JHEP* **11** (2015) 155, [arXiv:1507.00261 \[hep-th\]](#).
- [75] S. Pasquetti, “Factorisation of  $\mathcal{N} = 2$  Theories on the Squashed 3-Sphere,” *JHEP* **1204** (2012) 120, [arXiv:1111.6905 \[hep-th\]](#).
- [76] C. Beem, T. Dimofte, and S. Pasquetti, “Holomorphic Blocks in Three Dimensions,” [arXiv:1211.1986 \[hep-th\]](#).
- [77] F. Benini and W. Peelaers, “Higgs branch localization in three dimensions,” *JHEP* **05** (2014) 030, [arXiv:1312.6078 \[hep-th\]](#).
- [78] F. Benini, T. Nishioka, and M. Yamazaki, “4d Index to 3d Index and 2d TQFT,” [arXiv:1109.0283 \[hep-th\]](#).
- [79] S. S. Razamat and B. Willett, “Global Properties of Supersymmetric Theories and the Lens Space,” *Commun. Math. Phys.* **334** (2015) no. 2, 661–696, [arXiv:1307.4381 \[hep-th\]](#).
- [80] V. P. Spiridonov, “Elliptic beta integrals and solvable models of statistical mechanics,” *Contemp. Math.* **563** (2012) 181–211, [arXiv:1011.3798 \[hep-th\]](#).
- [81] M. Yamazaki, “New Integrable Models from the Gauge/YBE Correspondence,” *J. Statist. Phys.* **154** (2014) 895, [arXiv:1307.1128 \[hep-th\]](#).
- [82] D. Gaiotto and H.-C. Kim, “Surface defects and instanton partition functions,” [arXiv:1412.2781 \[hep-th\]](#).
- [83] M. Bullimore, M. Fluder, L. Hollands, and P. Richmond, “The superconformal index and an elliptic algebra of surface defects,” [arXiv:1401.3379 \[hep-th\]](#).
- [84] L. F. Alday, M. Bullimore, and M. Fluder, “On S-duality of the Superconformal Index on Lens Spaces and 2d TQFT,” [arXiv:1301.7486 \[hep-th\]](#).
- [85] S. S. Razamat and M. Yamazaki, “S-duality and the  $\mathcal{N}=2$  Lens Space Index,” *JHEP* **1310** (2013) 048, [arXiv:1306.1543 \[hep-th\]](#).
- [86] J. Yagi, “Quiver gauge theories and integrable lattice models,” *JHEP* **10** (2015) 065, [arXiv:1504.04055 \[hep-th\]](#).
- [87] K. Maruyoshi and J. Yagi, “Surface defects as transfer matrices,” [arXiv:1606.01041 \[hep-th\]](#).

# Chapter 14

## Review of localization for 5d supersymmetric gauge theories

Jian Qiu<sup>a,b,c</sup> and Maxim Zabzine<sup>c</sup>

<sup>a</sup> *Max-Planck-Institut für Mathematik,  
Vivatsgasse 7, 53111 Bonn, Germany*

<sup>b</sup> *Department of Mathematics, Uppsala University,  
Box 480, SE-75106 Uppsala, Sweden*

<sup>c</sup> *Department of Physics and Astronomy, Uppsala university,  
Box 516, SE-75120 Uppsala, Sweden*  
jian.qiu@math.uu.se, Maxim.Zabzine@physics.uu.se

### Abstract

We give a pedagogical review of the localization of supersymmetric gauge theory on 5d toric Sasaki-Einstein manifolds. We construct the cohomological complex resulting from supersymmetry and consider its natural toric deformations with all equivariant parameters turned on. We also give detailed discussion on how the Sasaki-Einstein geometry permeates every aspect of the calculation, from Killing spinor, vanishing theorems to the index theorems.

### Contents

|                                                              |            |
|--------------------------------------------------------------|------------|
| <b>14.1 Introduction</b>                                     | <b>560</b> |
| <b>14.2 The basic setup</b>                                  | <b>562</b> |
| 14.2.1 5d SYM on flat space                                  | 562        |
| 14.2.2 SYM on the simply connected Sasaki-Einstein manifolds | 563        |
| 14.2.3 Field Content and Susy transformation                 | 565        |

|                                                                  |            |
|------------------------------------------------------------------|------------|
| <b>14.3 The cohomological complex</b> . . . . .                  | <b>566</b> |
| 14.3.1 Finite dimensional toy model . . . . .                    | 566        |
| 14.3.2 Change of variable . . . . .                              | 568        |
| 14.3.3 Deformation of the complex . . . . .                      | 572        |
| <b>14.4 Analysis of the fixed points</b> . . . . .               | <b>573</b> |
| 14.4.1 Vector multiplet and contact instantons . . . . .         | 573        |
| 14.4.2 Hyper-multiplet and vanishing theorems . . . . .          | 575        |
| <b>14.5 Gauge fixing and the determinant</b> . . . . .           | <b>578</b> |
| 14.5.1 The determinant . . . . .                                 | 580        |
| 14.5.2 Schmude’s approach . . . . .                              | 581        |
| 14.5.3 Generalised multiple sine . . . . .                       | 583        |
| 14.5.4 Conjecture for the full answer . . . . .                  | 584        |
| <b>14.6 Asymptotics and comparison with flat space</b> . . . . . | <b>584</b> |
| 14.6.1 Comparison with flat space . . . . .                      | 585        |
| 14.6.2 The 1-loop effective action . . . . .                     | 586        |
| <b>14.7 Appendix. Geometrical setting</b> . . . . .              | <b>589</b> |
| 14.7.1 Some basics of contact geometry . . . . .                 | 589        |
| 14.7.2 Toric Sasaki manifolds . . . . .                          | 592        |
| <b>References</b> . . . . .                                      | <b>597</b> |

## 14.1 Introduction

The localisation technique in computing exact partition functions has had a long history by now: from Witten’s work on 2D Yang-Mills [2], then on the 3d side, the non-abelian localisation for Chern-Simons theory [3], and a more direct approach by embedding Chern-Simons in the  $N = 2$  supersymmetric Chern-Simons theory [4], and finally on 4d there is the groundbreaking work of Pestun [5]. The techniques used in these calculations simplify as one gains more and more insight into what is essential for the localisation and what are mere frills. For example the work of Källén [6], by using a nifty field redefinition, a large part of the work in the calculation of [4] can be circumvented. The similar field redefinitions were later used in the work [7] that started a series of work on the localisation in 5 dimension. Though the context of localisation may be very different, there is a common thread that unifies all of the above approach, namely the Duistermaat-Heckman formula [8] in equivariant cohomology. Let  $(X^{2n}, \omega)$  be a  $2n$  dimensional closed symplectic manifold, if there is a  $U(1)$  action on  $X$  with moment map  $\mu$ . Assuming that this action has only isolated fixed points, then the integral

$$\int_X \frac{\omega^n}{n!} e^{-\mu} = \sum_i \frac{e^{-\mu(p_i)}}{e(p_i)}$$

can be written as a sum of contributions from the fixed points  $\{p_i\}$ , and  $e(p_i) = \prod_a m_a(p_i)$  is the product of the weights  $m_a(p_i)$  of the  $U(1)$  action on the tangent space at  $p_i$ . This formula

has a generalisation to the case of just having a vector field  $V$  on  $X$  with only isolated fixed points [9], as the whole localisation revolves around this formula, we shall review it quickly here to make the paper self-contained. Let a  $V$  be a vector field on  $X$  with isolated zeros and assume that it is Killing with respect to a given metric  $g$ . With this data one can define an operator

$$d_V = d + \iota_V , \tag{14.1.1}$$

such that  $d_V^2 = L_V$ . This operator would be the equivariant differential had  $V$  been induced by a  $U(1)$  action. Let  $\alpha$  be a differential form that is closed under  $d_V$ , note that  $\alpha$  necessarily contains forms of different degrees. The integral of  $\alpha$  is then given by

$$\int_X \alpha = \sum_{p_i} \frac{\pi^n \alpha|_{p_i}}{\det^{1/2} L_V|_{p_i}} , \tag{14.1.2}$$

where the sum is over fixed points of  $V$ . At each  $p_i$  the Lie derivative  $L_V$  acts as an automorphism of  $T_{p_i}X$  and we can compute its determinant. The normalized infinitesimal form of  $V$  at point  $p_i$  is

$$V = 2\pi \sum_a m_a \left( x_a \frac{\partial}{\partial y_a} - y_a \frac{\partial}{\partial x_a} \right) , \tag{14.1.3}$$

where the positive integers  $m_a(p_i)$  are the weights of the  $U(1)$  action at  $p_i$ . The proof of this formula using the Grassmann variables will be given in section 14.3.1.

The formula (14.1.2) is the basis of our localisation technique. In fact, what one shall do is to find, in a given supersymmetric theory, a particular combination of the supersymmetry generator that behaves just like the operator (14.1.1) and then apply (14.1.2). In the infinite dimensional (path integral) setting, the vector field  $V$  is acting on the space of fields, and usually involves a combination of gauge transformation plus a Lie derivative along some vector field on the manifold where our gauge theory is formulated. Our task is to review the details of this procedure for 5d supersymmetric gauge theories. The review is organized as follows: in section 14.2 we review 5d supersymmetric Yang-Mills theory on flat space and on curved spaces. In section 14.3 we turn the susy algebra of section 14.2 into the desired form (14.1.1) and discuss its natural deformations. In section 14.4 we find the localization locus which gives us an interesting set of differential equations on 5-manifold. In section 14.5 we perform the localization and express the final perturbative answer as the matrix model with generalised triple sine function, see Chapter 15 for the study of these matrix models. We also conjecture the full answer for the partition function, see also Chapter 16 for further discussion. Finally in section 14.6 we discuss the relation between the curved space computations and the 1-loop perturbation computation on a flat space. In the appendices 14.7 we collect the necessary material on the geometrical setting of the 5d theory, namely the 5d toric Sasaki-Einstein manifolds.

## 14.2 The basic setup

### 14.2.1 5d SYM on flat space

We discuss briefly the setting on the flat space, since later we will extract from our curved space computation certain quantity such as the  $\beta$ -function, which can be compared to the explicit 1-loop computation on flat space.

We are interested in Euclidean version of  $N = 1$  supersymmetric Yang-Mills theory on  $\mathbb{R}^5$  which can be obtained by the reduction of 6d  $N = 1$  theory on  $\mathbb{R}^{5,1}$ . The 5d supersymmetric Yang-Mills action on flat space is

$$S = \frac{1}{g_{YM}^2} \text{Tr}_f \int_{\mathbb{R}^5} d^5x \left[ \frac{1}{2} F^{mn} F_{mn} + i \lambda_I \not{D} \lambda^I - (D^m \sigma)(D_m \sigma) - \lambda_I [\sigma, \lambda^I] - \frac{1}{2} D_{IJ} D^{IJ} \right] \quad (14.2.1)$$

where  $\text{Tr}_f$  is normalised as  $\text{Tr}_f [t^a t^b] = \delta^{ab}/2$  and  $D_m$  is covariant derivative. The various fields are:  $F$  is the field strength of the gauge connection  $F_{ij} = \partial_{[i} A_{j]} - i A_{[i} A_{j]}$ ,  $i, j = 1, \dots, 5$ ; and  $\sigma$  is an adjoint scalar (its kinetic term has the wrong sign because  $\sigma$  is in fact the temporal component of the gauge field  $\sigma \sim A^0$ , since the theory comes from a compactification of a 6d theory on  $\mathbb{R}^{1,5}$ ); while the field  $D_{IJ}$  is an auxiliary field in adjoint that is an isotriplet, i.e.  $D_{IJ} = D_{JI}$  and  $I, J = 1, 2$  are the isospin indices. The fermions  $\lambda^I$  above are the gaugini in adjoint, here the pairing of the spinors above uses only transposition

$$\psi \Gamma^{i_1} \dots \Gamma^{i_n} \chi \stackrel{\text{def}}{=} \psi^T C \Gamma^{i_1} \dots \Gamma^{i_n} \chi, \quad (14.2.2)$$

where  $C$  is the charge conjugation matrix satisfying  $C \Gamma^i C^{-1} = (\Gamma^i)^T$  ( $C$  is the product of all the gamma matrices that are imaginary or real). The  $\lambda_I$  are symplectic Majorana spinors satisfying

$$(\lambda^I)^* = \epsilon_{IJ} C \lambda^J. \quad (14.2.3)$$

Sometimes there is debate about the treatment of the reality condition for fermions when one passes from Lorentz to Euclidean signatures. However in the action above, the pairing of spinors uses only the transposition. Since the conjugation of a fermion never appears, while the integration over fermions is a formal integral<sup>1</sup>, the problem of how to treat the reality condition properly will not affect our calculation.

The field content of 5d SYM can also be understood from the 4d point of view. The 5d  $N=1$  susy reduces to the 4d  $N=2$  susy and the field content is quite familiar. The vector multiplet part of the action written in terms of the 4d  $N=1$  super fields is

$$S = \frac{1}{4\pi} \text{Im} \left( \frac{1}{2} \int d^2\theta d^5x \frac{\partial^2 \mathcal{F}}{\partial \mathcal{A}^i \partial \mathcal{A}^j} W^i W^j + \int d^4\theta d^5x \bar{\mathcal{A}}^i \frac{\partial \mathcal{F}}{\partial \mathcal{A}^i} \right). \quad (14.2.4)$$

Here  $W$  is a spinor fermionic chiral superfield, its leading component is the gaugino and it also contains the self-dual part of the field strength. The field  $\mathcal{A}$  is a chiral superfield that

<sup>1</sup>By this we mean there is no need to choose a cycle for the integration, in contrast to when one integrates a holomorphic form.

contains the other gaugino and the scalar in the vector multiplet. The object  $\mathcal{F}(\mathcal{A})$  is called the prepotential and is holomorphic in  $\mathcal{A}$ . In 5d the real part of the complex scalar becomes the 5<sup>th</sup> component of the gauge field leaving behind a real scalar that was called  $\sigma$  in (14.2.1).

It is a remarkable feature that in 5d, the prepotential  $\mathcal{F}$  has the following most general form [12]

$$\mathcal{F} = h_{ij} \mathcal{A}^i \mathcal{A}^j + c_{ijk} \mathcal{A}^i \mathcal{A}^j \mathcal{A}^k , \quad (14.2.5)$$

where  $i$  is the index of the adjoint representation. For example, in the standard case

$$h_{ij} = \left( \frac{\theta}{2\pi} + \frac{4\pi i}{g_{YM}^2} \right) \delta_{ij} .$$

The cubic term would then contribute a Chern-Simons term [13] (remember that the leading component of  $\mathcal{A}$  contains the fifth component of the gauge field)

$$\begin{aligned} \frac{c}{6} \text{Tr} \mathcal{A}^3 &\rightarrow CS_5 + \frac{c}{2\pi^2} \text{Tr} \int \sigma \left( F \wedge *F + (D\sigma) \wedge *(D\sigma) + \dots \right) , \\ CS_5 &= \frac{-ic}{24\pi^2} \text{Tr} \int_{M^5} \left( A(dA)^2 - \frac{3i}{2} A^3 dA - \frac{3}{5} A^5 \right) . \end{aligned} \quad (14.2.6)$$

The coupling of the Chern-Simons term, which is proportional  $c$ , must be quantized. This is one way of seeing that one cannot have any higher power terms in (14.2.5), since those would lead to a Chern-Simons term with a field dependent coupling, which is not allowed.

Note that in flat space, even if one sets the cubic term in (14.2.5) to zero to start with, it will be generated at 1-loop. By dimension counting,  $h$  has dimension of mass while  $c$  is a number, so  $c$  cannot depend on  $h$  and hence this is a 1-loop effect only. To perform the actual calculation, one can use the background field method and then we can compare it to our localization result at the flat space limit. The two results agree, but in an indirect way.

## 14.2.2 SYM on the simply connected Sasaki-Einstein manifolds

The theory (14.2.1) was constructed on the five sphere in [14], and a more systematic way of placing a supersymmetric theory on curved space was presented in [15]. The general method is that one starts from a suitable supergravity theory and then sends  $M_{pl} \rightarrow \infty$ , i.e. one freezes gravity. It is a large enterprise to study and classify the geometry arising this way that supports at least a fraction of the supersymmetry, see [16–18] and also [19].

We will not focus on the most general supersymmetric 5d gauge theories and instead we shall study the simplest case namely Sasaki-Einstein geometry. It turns out that in 5d one can freeze gravity if one can solve the Killing spinor equation

$$D_m \xi = \pm \frac{i}{2} \Gamma_m \xi_J , \quad (14.2.7)$$

where  $D$  is the spin covariant derivative. The number of independent solutions will determine the number of supersymmetry possessed by the theory. The Killing equation actually leads

to Sasaki-Einstein geometry, see [20] and also the review in [21]. For example to see that it is Einstein, apply (14.2.7) twice, one gets

$$D_m D_n \xi = -\frac{1}{4} \Gamma_n \Gamma_m \xi ,$$

whose antisymmetric part forces  $R_{mnpq} \Gamma^{pq} \xi = 2 \Gamma_{mn} \xi$ . Multiplying both sides by  $\Gamma^n$

$$\Gamma^n R_{mnpq} \Gamma^{pq} \xi = 2 \Gamma^n \Gamma_{mn} \xi \stackrel{\text{Bianchi}}{\Rightarrow} R_{mq} \Gamma^q \xi = 4 \Gamma_m \xi \Rightarrow R_{mn} = 4 g_{mn} .$$

The basic trick of the trade is to construct some tensors out of the Killing spinors, and apply (14.2.7) to determine what sort of differential identities these tensors obey. Then with some luck, one can classify the geometry.

From now on we focus on the simply connected 5d Sasaki-Einstein (SE) manifolds<sup>2</sup>, then the solution can be organized as doublets

$$D_m \xi_I = \frac{1}{r} t_I^J \Gamma_m \xi_J , \quad t_I^J = \frac{i}{2} (\sigma_3)_I^J , \quad (\xi_I \xi_J) = -\frac{1}{2} \epsilon_{IJ} , \quad (14.2.8)$$

where we have inserted  $r$  as a dimensionful parameter (the size of manifold, which can be ignored for now); and  $\sigma_3 = \text{diag}[1, -1]$ .

We pause to highlight some key features of the simply connected 5d SE manifolds, which will be used in the formulation of the susy theory, leaving a more detailed review to the appendix.

Out of the solution to (14.2.8), one can construct two tensors (we shall leave out  $r$  next)

$$R^p = \xi_I \Gamma^p \xi^I , \quad J_m{}^n = -2 t^{IJ} \xi_I \Gamma_m{}^n \xi_J , \quad (14.2.9)$$

these quantities satisfy

- $R$  has constant norm 1 and it is a Killing vector field, called the *Reeb* vector field
- $J$  is horizontal with respect to  $R$ , i.e.  $R^m J_m{}^n = 0$
- $J$  defines a complex structure transverse to  $R$ , i.e.  $J$  squares to  $-1$  restricted to the plane perpendicular to  $R$
- $Jg$  is the Kähler form transverse to  $R$

The Sasaki condition implies also the equation

$$\nabla_m J^p{}_q = -v^p g_{mq} + \delta_m^p \kappa_q .$$

That transverse to  $R$ , there is a Kähler structure is particularly important, both in bulding a convenient spin representation and in the index computation of Schmude [23], see later. We also remark that the transverse Kähler structure is Kähler-Einstein ( $R_{pq}^\perp = 6g_{pq}^\perp$ ).

---

<sup>2</sup>By theorem 7.5.27 in [22], such manifolds are spin

### 14.2.3 Field Content and Susy transformation

In this section we recall the action of 5d SYM for both the vector and hyper-multiplet, and their susy transformation. The same formula is valid for  $S^5$  or more general SE manifolds, the only difference is the number of solutions to the Killing spinor equation, i.e. the number of susy. In the former case, one get eight susy while only two for the latter.

The field content of the vector-multiplet is as in the flat space case, the off-shell supersymmetry reads transformation

$$\begin{aligned}
\delta A_m &= i\xi_I \Gamma_m \lambda^I , \\
\delta \sigma &= i\xi_I \lambda^I , \\
\delta \lambda_I &= -\frac{1}{2}(\Gamma^{mn} \xi_I) F_{mn} + (\Gamma^m \xi_I) D_m \sigma - \xi^J D_{JI} + \frac{2}{r} t_I^J \xi_J \sigma , \\
\delta D_{IJ} &= -i\xi_I \Gamma^m D_m \lambda_J + [\sigma, \xi_I \lambda_J] + \frac{i}{r} t_I^K \xi_K \lambda_J + (I \leftrightarrow J) ,
\end{aligned} \tag{14.2.10}$$

where  $\xi_I$  is a spinor satisfying the Killing equation (14.2.8). The susy invariant action is

$$\begin{aligned}
S_{vec} &= \frac{1}{g_{YM}^2} \int \text{Vol}_M \text{Tr} \left[ \frac{1}{2} F_{mn} F^{mn} - D_m \sigma D^m \sigma - \frac{1}{2} D_{IJ} D^{IJ} + \frac{2}{r} \sigma t^{IJ} D_{IJ} - \frac{10}{r^2} t^{IJ} t_{IJ} \sigma^2 \right. \\
&\quad \left. + i \lambda_I \Gamma^m D_m \lambda^I - \lambda_I [\sigma, \lambda^I] - \frac{i}{r} t^{IJ} \lambda_I \lambda_J \right] ,
\end{aligned} \tag{14.2.11}$$

where one see that compared to (14.2.1), certain  $1/r$  corrections appeared. Upon sending  $r \rightarrow \infty$  we recover the flat action (14.2.1) and flat supersymmetry transformations. We point out a technical detail that the vev  $D_{IJ} \sim (2/r)t_{IJ}\sigma$  from solving the eom above is not a susy background, but in contrast  $D_{IJ} \sim -(2/r)t_{IJ}\sigma$  is. The difference vanishes in the flat space limit.

The hyper-multiplet consists of an  $SU(2)_R$ -doublet of complex scalars  $q_I^A$ ,  $I = 1, 2$  and an  $SU(2)_R$ -singlet fermion  $\psi^A$ , with the reality conditions ( $A = 1, 2, \dots, 2N$ )

$$(q_I^A)^* = \Omega_{AB} \epsilon^{IJ} q_J^B , \quad (\psi^A)^* = \Omega_{AB} C \psi^B , \tag{14.2.12}$$

where  $\Omega_{AB}$  is the invariant tensor of  $USp(2N)$

$$\Omega = \begin{vmatrix} 0 & \mathbf{1}_N \\ -\mathbf{1}_N & 0 \end{vmatrix} ,$$

and  $C$  is the charge conjugation matrix as before.

The gauge group will be a subgroup of  $USp(2N)$ , in particular we consider the hyper-multiplet with the representation  $\underline{N} \oplus \bar{\underline{N}}$  of  $SU(N)$ , which is embedded in  $USp(2N)$  in the standard manner

$$U \rightarrow \begin{vmatrix} U & 0 \\ 0 & U^{-T} \end{vmatrix} , \quad U \in SU(N) .$$

Suppressing the gauge group index, the on-shell supersymmetry transformations are written as:

$$\begin{aligned}\delta q_I &= -2i\xi_I\psi , \\ \delta\psi &= \Gamma^m\xi_I(D_m q^I) + i\sigma\xi_I q^I - \frac{3}{r}t^{IJ}\xi_I q_J .\end{aligned}\tag{14.2.13}$$

The off-shell version of this transformations will be discussed later. The Lagrangian invariant under (14.2.13) is

$$\begin{aligned}L_{hyp} &= \epsilon^{IJ}\Omega_{AB}D_m q_I^A D^m q_J^B - \epsilon^{IJ}q_I^A \sigma_{AC}\sigma^C{}_{B}q_J^B + \frac{15}{2r^2}\epsilon^{IJ}\Omega_{AB}t^2 q_I^A q_J^B \\ &\quad - 2i\Omega_{AB}\psi^A \not{D}\psi^B - 2\psi^A \sigma_{AB}\psi^B - 4\Omega_{AB}\psi^A \lambda_I q^{IB} - iq_I^A D_{AB}^{IJ} q_J^B ,\end{aligned}\tag{14.2.14}$$

where  $t^2 = t^{IJ}t_{IJ} = 1/2$  and  $\sigma_{AB} = \Omega_{AC}\sigma^C{}_{B}$ . The covariant derivative  $D$  includes both the Levi-Civita connection and the gauge connection.

Here as in the vector case, the action is written without complex conjugation, and the fermion integrals are done formally.

## 14.3 The cohomological complex

### 14.3.1 Finite dimensional toy model

Here we give a simple proof of (14.1.2) in a way that makes its connection to supersymmetry apparent. We recommend a nice review [24] that covers large part of this section.

Recall the setting of (14.1.2) from section 14.1. We have a vector field  $V$  acting on a manifold  $X$ . We denote the coordinates of  $X$  as  $x^i$ ,  $i = 1, \dots, 2n$ . One can use the fermionic variables  $\psi^i$  to represent the 1-forms  $dx^i$ , and hence a function  $\mathcal{O}(x, \psi)$  is just a differential form on  $X$ . An integral of a differential form is then written as a Grassmann integral

$$I = \int d^{2n}x d^{2n}\psi \mathcal{O}(x, \psi) .$$

Assume that the differential form  $\mathcal{O}(x, \psi)$  on  $X$  is invariant under an odd symmetry

$$\delta_V x^i = \psi^i , \quad \delta_V \psi^i = L_V x^i = V^i(x) .\tag{14.3.1}$$

In fact this complex is nothing but the Cartan formula for the Lie-derivative  $L_V = \{d, \iota_V\}$ , where  $\iota_V : \Omega^i \rightarrow \Omega^{i-1}$  is the contraction of forms with  $V$ , represented as  $V^i \partial_{\psi^i}$  now.

Pick an odd function  $W$  satisfying  $\delta_V^2 W = 0$  then we can insert into the integral a factor

$$I(t) = \int d^{2n}x d^{2n}\psi \mathcal{O}(x, \psi) e^{-t\delta_V W} , \quad \delta_V^2 W = 0 ,\tag{14.3.2}$$

without changing the value of the integral. The last statement can be seen by differentiating with respect to  $t$

$$\frac{d}{dt}I(t) = - \int d^{2n}x d^{2n}\psi \mathcal{O}(x, \psi) (\delta_V W) e^{-t\delta_V W} = - \int d^{2n}x d^{2n}\psi \delta_V (\mathcal{O}(x, \psi) W e^{-t\delta_V W}) ,$$

in the last integral, we can replace  $\delta_V$  with  $d = \psi^i \partial_i$  since the integral will only pick up terms top degree in  $\psi$ . In this way, one can use Stokes theorem and the result  $dI/dt = 0$  follows.

We assume that  $\delta_V W$  is a well-behaved function, i.e. providing sufficient damping at infinity and whose critical points are isolated, we can then send  $t \rightarrow \infty$  in (14.3.2) and the integral will be concentrated at the critical points of the even part of  $\delta W$

$$\lim_{t \rightarrow \infty} \int d^{2n}x d^{2n}\psi \mathcal{O}(x, \psi) e^{-t\delta_V W} = \sum_{\text{cr pt}} \frac{\pi^n \mathcal{O}_0}{\sqrt{\det(\delta_V W)''}} , \quad (14.3.3)$$

Again so long as  $\delta_V W$  is well-behaved in the above sense, the determinant appearing in (14.3.3) is (up to a phase) independent of  $W$ . To see this, pick a critical point, say  $x = 0$  and assume that  $\delta_V W$  has the expansion

$$\delta_V W = c + \frac{1}{2} g_{ij} x^i x^j + \frac{1}{2} b_{ij} \psi^i \psi^j + \dots ,$$

then  $\delta_V^2 W = 0$  implies

$$0 = \delta_V^2 W = g_{ij} x^i \psi^j + b_{ij} V^i \psi^j + \dots ,$$

for this to be zero, one must have  $V^i \sim x^j \partial_j V^i + \dots$ , and

$$g_{ij} = -\partial_i V^k b_{kj} .$$

This leads to

$$\det g = (-1)^n \det V' \det b , \quad \frac{\text{pf } b}{\sqrt{\det g}} = \pm \frac{1}{\sqrt{\det dV}} ,$$

where  $dV$  is the derivative of  $V$  at  $x = 0$ , regarded as an endomorphism of  $T_0 X$ . The precise sign can be worked out, but as it is not crucial to the path integral, we just set it to be  $+$ . Thus in conclusion

$$\int_X \mathcal{O} = \sum_{x_0 \in \text{cr pt}} \frac{\pi^{\frac{\dim X}{2}} \mathcal{O}}{\sqrt{\det(dV)}|_{x_0}} . \quad (14.3.4)$$

There is also holomorphic version of the story. Let  $\delta_V$  and  $V$  act holomorphically

$$\delta x^i = \psi^i , \quad \delta x^{\bar{i}} = \psi^{\bar{i}} , \quad \delta \psi^i = V^i , \quad \delta \psi^{\bar{i}} = V^{\bar{i}} ,$$

then we have some modification to the above argument. Assume that  $\delta W$  has the expansion

$$\delta W = c + g_{i\bar{j}} x^i x^{\bar{j}} + b_{i\bar{j}} \psi^i \psi^{\bar{j}} + \dots ,$$

and  $\delta^2 W = 0$  implies

$$0 = g_{i\bar{j}} \psi^i x^{\bar{j}} + b_{i\bar{j}} V^i \psi^{\bar{j}} + c.c + \dots = x^i (g_{i\bar{j}} + b_{j\bar{i}} (\partial_i V^j)) \psi^{\bar{j}} + \dots$$

hence  $g_{i\bar{j}} = -b_{j\bar{j}}(\partial_i V^j)$ , and the determinant to be computed turns into

$$\frac{\det b_{j\bar{j}}}{\det g_{j\bar{j}}} = (-1)^{\dim_{\mathbb{C}} X} \frac{1}{\det(\partial_i V^j)} = (-1)^{\dim_{\mathbb{C}} X} \frac{1}{\det(\partial_i V^{\bar{j}})} .$$

This case is applicable to the hyper-multiplet.

In fact the setting can be more general, in that  $x$  itself can be both even and odd, with  $\psi$  being of the opposite parity.

**Remark** Based on the fact that the eventual determinant only depends on the vector field  $V$  and not on the details of  $W$  (provided of course the appropriate  $W$  exists), one might tend to skip the step of finding  $W$ . This is viable in a finite dimensional setting above, as the fixed points are really points. But when we come to infinite dimensional path integral setting, the fixed points of  $V$  are described by certain differential equations in the fields, and so one would prefer to find a  $W$  such that its critical points *imply* the given differential equations, and desirably a bit more, so that one can study effectively the fixed points.

It is straightforward to generalise the above to the case when the zero of  $V$  is a submanifold  $Z$  of codimension  $p$ ,

$$(14.3.4) = \int_Z \frac{\pi^{\text{codim } Z/2} \mathcal{O}}{\sqrt{\det(dV)}} , \quad (14.3.5)$$

where  $dV$  is now regarded as an endomorphism of the normal bundle  $N_Z$  of  $Z$  in  $X$ .

### 14.3.2 Change of variable

Our goal next will be to put the vector and hyper multiplet into the complex of the form (14.3.1). We suggest the reader to take a look at the appendix where various geometrical objects of the SE manifold are explained. The most important one we shall use is the projector

$$P_{\pm} = \frac{1}{2}(\iota_R \kappa \pm \iota_R^*) : \Omega^2 \rightarrow \Omega_H^{2\pm} , \quad (14.3.6)$$

where  $\kappa$  is the contact 1-form. In the current setting it is just  $\kappa = g_R$  and it satisfies

$$\iota_R \kappa = 1 , \quad \iota_R dk = 0 , \quad \frac{1}{8} \kappa dk d\kappa = \text{Vol} .$$

We see that  $d\kappa$  is nondegenerate on the plane transverse to  $R$  (in fact it is proportional to the transverse Kähler form). Further  $\Omega_H^{2\pm}$  are the horizontal (anti)-self-dual 2-forms, so the projector (14.3.6) is the 5d lift of the usual 4d self-duality projector, we will see shortly the 5d instantons are also the lift of the usual 4d anti-self-dual instantons.

Schematically the anti-commutator of two susy transformations is

$$\{\delta_1, \delta_2\} = \text{translation} + \text{R-rotation} + \text{dilatation} + \text{gauge transformation} , \quad (14.3.7)$$

where by translation we mean the infinitesimal diffeomorphism along a vector field. The Killing spinors  $\xi$  single out one particular susy  $\delta_\xi$  that has a simpler anti-commutator

$$\delta_\xi^2 = \text{translation} + \text{gauge transformation} , \quad (14.3.8)$$

next we exhibit this for the vector and hyper-multiplet cases.

*Vector-multiplet*

We use the Killing spinor to turn the gaugino into some odd differential forms. Define

$$\Psi_m = \xi_I \Gamma_m \lambda^I , \quad \chi_{mn} = \xi_I \Gamma_{mn} \lambda^I + R_{[m} \xi_I \Gamma_{n]} \lambda^I , \quad (14.3.9)$$

the 2-form  $\chi$  satisfies the same conditions as  $J$ :

$$\iota_R \chi = 0 , \quad \iota_R * \chi = \chi . \quad (14.3.10)$$

This change of variable is invertible

$$\lambda_I = -\frac{1}{2} \xi^J (\xi_J \Gamma^{mn} \xi_I) \chi_{mn} + (\Gamma^m \xi_I) \Psi_m , \quad (14.3.11)$$

with  $\Psi_m$  having 5 components and  $\chi_{mn}$  having 3 components.

With the new variables the susy transformation reads (where we just write  $\delta$  for  $\delta_\xi$ )

$$\begin{aligned} \delta A &= i\Psi , & \delta \Psi &= -\iota_R F + D\sigma , \\ \delta \chi &= H , & \delta H &= -iL_R^A \chi - [\sigma, \chi] , \\ \delta \sigma &= -i\iota_R \Psi , \\ \delta^2 &= -iL_R + iG_\Phi , & \Phi &= \sigma + \iota_R A . \end{aligned} \quad (14.3.12)$$

Here  $H$  is the bosonic partner of  $\chi$  and hence has exactly the same property (14.3.10), explicitly it is related to the auxiliary  $D_{IJ}$  as

$$H_{mn} = 2(F_H^+)_{mn} + (\xi^I \Gamma_{mn} \xi^J) (D_{IJ} + \frac{2}{r} t_{IJ} \sigma) , \quad F_H^+ = P_+ F . \quad (14.3.13)$$

Further  $G_\Phi$  is the gauge transformation with respect to parameter  $\Phi$ , defined as<sup>3</sup>

$$G_\epsilon A = D\epsilon , \quad G_\epsilon \phi = i\epsilon \phi ,$$

with  $\phi$  in any representation (e.g., if  $\phi$  is in the adjoint then  $\epsilon \phi = [\epsilon, \phi]$ ). Finally  $L_R^A = L_R + i[\ , \iota_R A]$  is the Lie derivative combined with gauge transformation. So we see that the square of the susy transformation has the promised form (14.3.8).

---

<sup>3</sup>Our convention is that the Lie algebra  $u(n)$  is given by Hermitian matrices, and  $D = d - iA = d - iA^a t^a$  for a basis  $\{t^a\}$  of the Lie algebra. This choice engenders awkward  $i$ 's everywhere, something that we came to regret.

**Remark** Intuitively, we can understand the simplification from (14.3.7) to (14.3.8) as follows. In our redefinition of fields, we combined the  $SU(2)$  doublet  $\lambda^I$  with another doublet  $\xi_I$ , forming a singlet, and so the R-rotation vanishes from right hand side of (14.3.8). As for the dilatation, it would have the divergence  $\text{div } R$  as its parameter, but since  $R$  is Killing, this vanishes too.

### *Hyper-multiplet*

Knowing that one should form  $SU(2)$  singlets to eliminate R-rotation from the square of the susy transformation, we combine the scalar  $q_I$  with the Killing spinors, and leave the fermion  $\psi$  alone as it is already a singlet. Thus the twisted hyper-complex is formulated in terms of spinors. The change of variables reads

$$q = \xi_I q^I, \quad q_I = -2\xi_I q,$$

where  $q$  is a spinor and we remind the reader about the spinor pairing  $\xi_I q \stackrel{def}{=} \xi_I^T C q$ . To see that the above change of variables is invertible one has to use the Fierz identities, see [25].

From the reality condition satisfied by  $\xi_I$  and  $q_I$  one can see that the spinor field  $q$  now satisfies the same reality condition as  $\psi$

$$(q^A)^* = \Omega_{AB} C q^B.$$

Assuming that the gauge group is  $SU(N) \subset USp(2N)$ , one can solve this constraint by splitting

$$q^A \Rightarrow \left| \begin{array}{c} q^\alpha \\ -C q_\beta^* \end{array} \right|, \quad (14.3.14)$$

where  $q^\alpha$  is now an unconstrained Dirac spinor transforming in a representation of  $SU(N)$ , indexed by  $\alpha$ . The field  $\psi$  can be dealt with in exactly the same way.

We will also split  $\psi$  according to its chirality under

$$\gamma_5 = -R \cdot \Gamma, \quad (14.3.15)$$

i.e.  $\psi = \psi_+ + \psi_-$ ,  $\gamma_5 \psi_\pm = \pm \psi_\pm$ . Note that the spinor  $q$  has  $\gamma_5 q = +q$  always due to the special property of the Killing spinors (see the review in section 2.3 [21]). After some massive use of the Fierz identities and introducing an auxiliary field  $\mathcal{F}$  with  $-1$   $\gamma_5$ -eigenvalue, we get the off-shell complex

$$\begin{aligned} \delta q &= i\psi_+, \\ \delta \psi_+ &= (-L_R^s + G_\Phi)q, \\ \delta \psi_- &= \mathcal{F}, \\ \delta \mathcal{F} &= (-iL_R^s + iG_\Phi)\psi_-, \end{aligned} \quad (14.3.16)$$

$$\delta^2 = -iL_R^s + iG_\Phi, \quad (14.3.17)$$

where  $G_\Phi$  is the same gauge transformation as in (14.3.12). We have also introduced the spinorial Lie derivative  $L_X^s$ , defined for Killing vectors  $X$ , see [26]<sup>4</sup>

$$\begin{aligned} L_X^s &= D_X + \frac{1}{8} \nabla_{[m} X_n] \Gamma^{mn} , \\ [L_X^s, L_Y^s] &= L_{[X, Y]}^s, \quad [D_m, L_X^s] = 0 , \end{aligned}$$

where  $\nabla$  is the Levi-Civita connection and  $D$  is the spin covariant derivative. The last property shows that by using Killing vectors one can generate new solutions of the Killing spinor equation.

*A Convenient Spin Representation.*

For later computation, we would like to choose a convenient spin representation in terms of anti-holomorphic forms. Let

$$W_{can} = \bigoplus \Omega_H^{0,\cdot}(M) , \quad (14.3.18)$$

where  $\Omega_H^{0,\cdot}$  consists of horizontal forms anti-holomorphic with respect to  $J$ . One then has a representation of the Clifford algebra: let  $\psi$  be any section of  $W_{can}$  and  $\chi$  a 1-form, define the Clifford action

$$\chi \cdot \psi = \begin{cases} \sqrt{2} \chi \wedge \psi & \chi \in \Omega_H^{0,1}(M) \\ \sqrt{2} \iota_{g^{-1}\chi} \psi & \chi \in \Omega_H^{1,0}(M) \\ (-1)^{\deg+1} \psi & \chi = \kappa \end{cases} . \quad (14.3.19)$$

In this way, one has a  $\text{spin}^c$ -structure whose characteristic line bundle (see chapter 5 in [27]) is the anti-canonical line bundle associated with the complex structure  $J$ .

**Remark** In this representation, the two Killing spinors are (0,0) and the (0,2) forms respectively. In particular, that a non-vanishing section of (0,2) forms exists follows from the triviality of the canonical bundle of the horizontal complex structure. The latter in turn follows from the Kähler Einstein condition: the curvature of the canonical bundle is the (1,1) part of the Ricci tensor which is proportional to  $d\kappa$  and hence is trivial.

Thus one has a representation where  $q, \psi_+ \in \Omega_H^{0,0} \oplus \Omega_H^{0,2}$ , and  $\psi_-, \mathcal{F} \in \Omega_H^{0,1}$ . Furthermore with SE metric the spinorial Lie derivative is related to the usual Lie derivative as

$$L_X^s = L_X + i f_X , \quad (14.3.20)$$

where  $f_X$  is a real constant. In the toric SE case  $f_X$  can be read off easily from the toric data and  $f_R = 3/2$ . To summarize, the hyper complex reads

$$\begin{aligned} \delta q &= i \psi_+ , \quad \delta \psi_+ = (-L_R - i f_R + G_\Phi) q , \\ \delta \psi_- &= \mathcal{F} , \quad \delta \mathcal{F} = i(-L_R - i f_R + G_\Phi) \psi_- . \end{aligned} \quad (14.3.21)$$

---

<sup>4</sup>There is a sign difference in our second term compared to that of [26], the reason is the difference in the convention of the Clifford algebra  $\{\Gamma_p, \Gamma_q\} = 2g_{pq}$  in this paper, while it is  $-2g_{pq}$  there.

We need also the formula for the spinor pairing for later use. If one works through the spinor-form correspondence, the pairing is

$$\begin{array}{c|c|c} \text{as spinors} & \xi^T C \eta & \xi^\dagger \eta \\ \text{as forms} & -(-1)^{d(d-1)/2} \frac{\xi \wedge \eta}{2\bar{\varrho}} & \xi^* \wedge * \eta \end{array} \quad (14.3.22)$$

where  $d = \deg \xi$  and  $\bar{\varrho}$  is the nowhere vanishing section of  $\Omega_H^{0,2}$ , which exists in the SE geometry, and assume that it is normalised to be of norm 1. In the text, the first pairing is denoted as just  $\xi\eta$ , and we denote it in the form language as  $\langle \xi, \eta \rangle$ , this pairing is known as the Mukai pairing.

### 14.3.3 Deformation of the complex

One of the advantages of reformulating the susy complex in terms of differential forms is that there is natural deformation of the cohomological complex.

Looking at (14.3.12), one has the freedom to deform  $R$ , and in the case of toric SE geometry, the deformation has a very simple parameterisation, see later. Putting aside some positivity conditions, the deformation is valid provided one also deforms  $\kappa$  and subsequently the horizontal plane correspondingly. One can allow  $R$  to have a small imaginary part in order to get the stronger localisation locus. The deformed complex looks exactly the same as (14.3.12) so we shall not write it again.

In a series of works [28–31], one tried to set up susy theories on the squashed three (five) sphere. These manifolds are topologically the same but the metric is no longer SE, so the Killing equations (14.2.7) must be modified. In other words, more background fields from the supergravity multiplet have to be turned on, and these fields modify the right hand side of (14.2.7). The net result is that one gets a fairly complicated susy theory, but if one tries to rewrite them in terms of differential forms (14.3.12), no change occurred other than replacing  $R$  with the deformed one. Thus as far as computation is concerned, one can take (14.3.12) as the starting point.

The deformation of the hyper-multiplet complex is a bit more tricky. We can take the formulation in (14.3.16) and deform  $R$  as before, keeping in mind that the chirality operator  $\gamma_5 = -R \cdot \Gamma$  has to be deformed accordingly. The only problem is that the spinorial Lie derivative  $L_R^s$  depends on the choice of the spin connection, and thus the deformation seems less canonical. Alternatively, one can take the reformulation of hypermultiplet in terms of differential forms (14.3.21) as the starting point with the Lie derivative acting on forms canonically. The only remaining problem is to determine the shift  $f_R$  and this can be done by using the consistency checks for SE metric.

In particular, we shall deform the metric and horizontal complex structure for the SE manifolds; in the toric SE case, these deformations are easily parameterized, see appendix 14.7.2. Now we focus on the toric case, by assumption we still have a nowhere vanishing section  $\varrho \in \Omega_H^{0,2}$ , which shall be constructed also in the appendix, and we show that

$$2i f_R \varrho = L_R \varrho . \quad (14.3.23)$$

In particular, when the metric is SE, one always has  $L_R \varrho = 3i\varrho$  and so  $f_R = 3/2$  agreeing with the shift for SE case. And now we use (14.3.23) as a definition of the shift  $f_R$ . Later we will see that this shift has some other virtues.

## 14.4 Analysis of the fixed points

As we did for the toy model section 14.3.1, we have to find an appropriate functional  $W$  and deform the action by  $-t \int \delta W$  so as to localize the path integral on the fixed points of the vector field  $\delta^2 = -iL_R^{(s)} + iG_\Phi$ .

### 14.4.1 Vector multiplet and contact instantons

*An observable*

Beside the supersymmetric Yang-Mills action the vector multiplet also possesses an observable that is  $\delta$ -closed but not  $\delta$ -exact

$$\begin{aligned} \mathcal{O} &= CS_{3,2}(A + \kappa\sigma) + i\text{Tr} \int \kappa \wedge d\kappa \wedge \Psi \wedge \Psi, \\ CS_{3,2} &= \text{Tr} \int d\kappa \wedge (A \wedge dA - \frac{2i}{3} A \wedge A \wedge A) = \text{Tr} \int \kappa \wedge F \wedge F. \end{aligned} \quad (14.4.1)$$

The bosonic part of  $\mathcal{O}$  reads

$$\mathcal{O}|_{bos} = \text{Tr} \int \kappa \wedge F \wedge F + 2\sigma\kappa \wedge d\kappa \wedge F + \sigma^2\kappa \wedge d\kappa \wedge d\kappa.$$

One can in fact also write an observable associated with the 5d Chern-Simons term, see [7].

Next we collect the bosonic part of the classical action (14.2.11) (set  $r = 1$ )

$$\begin{aligned} S_{vec}|_{bos} &= \text{Tr} \int \iota_R F \wedge *(\iota_R F) - \kappa \wedge F \wedge F - (D\sigma) \wedge *(D\sigma) \\ &\quad - \frac{1}{2} H \wedge *H + 2\kappa \wedge F \wedge H + \frac{1}{r} \sigma\kappa \wedge d\kappa \wedge H - \frac{2}{r} \sigma\kappa \wedge d\kappa \wedge F - \frac{8}{r^2} \sigma^2\kappa \wedge d\kappa \wedge d\kappa. \end{aligned} \quad (14.4.2)$$

Now we can choose  $W$

$$W_{vec}(s) = \text{Tr} \left[ \Psi \wedge *(-\iota_R F - D\sigma) - \frac{1}{2} \chi \wedge *H + 2\chi \wedge *F + s\sigma\kappa \wedge d\kappa \wedge \chi \right],$$

where  $s$  is some parameter and  $F_H^+ = P_+ F$ , with  $P_+$  defined in (14.3.6). We can check that the classical action is reproduced as

$$S_{vec} = -\mathcal{O} + \int \delta W_{vec}(1).$$

But for the deforming part, we take  $t \int W_{vec}(0)$ , and it is easy to check that

$$\int \delta W_{vec}(0)|_{bos} = \text{Tr} \int \iota_R F \wedge *(\iota_R F) - (D\sigma) \wedge *(D\sigma) - \frac{1}{2} H \wedge *H + 2F_H^+ \wedge *H. \quad (14.4.3)$$

The fields  $H$  and  $\sigma$  should be to Wick rotated  $H \rightarrow iH$  and  $\sigma \rightarrow i\sigma$ , in order to have a positive kinetic term and stronger localization locus. Next we integrate out  $H$  leaving a perfect square. Thus the localisation locus is

$$F_H^+ = 0, \quad \iota_R F = 0, \quad D\sigma = 0. \quad (14.4.4)$$

The first two equations came to be called the 'contact instanton' and they can be combined in one equation

$$*F = -\kappa \wedge F, \quad (14.4.5)$$

while the last equation in (14.4.4) says  $\sigma$  is a covariant constant.

**Remark** Recall in the 4d case, (anti)-self-duality of  $F$  would imply the Yang-Mills equation. In 5d same thing happens

$$D_A(*F) = D_A(\kappa \wedge F) = d\kappa \wedge F - \kappa \wedge D_A F = d\kappa \wedge F,$$

but the rhs is zero

$$d\kappa \wedge F = (\iota_R * d\kappa) \wedge F = \iota_R(*d\kappa \wedge F) = \iota_R(d\kappa \wedge *F) = d\kappa \wedge \iota_R F = -d\kappa \wedge F.$$

We leave it to the reader to check that the same equation (14.4.4) but with  $F_H^- = 0$  will not imply the Yang-Mills equation.

**Remark** We comment also that (14.4.4) is not an elliptic system, so studying its deformation is slightly unconventional (see [32–34]). However, one can embed this set of equations into another set [35], which is a 5d lift of the Vafa-Witten equation, now called the Haydys-Witten equation [36–38]. The latter set has interesting vanishing theorems so is perhaps better adapted for studying the moduli problem.

The Yang-Mills action saturates a bound at the instanton background

$$\begin{aligned} \int F \wedge *F &= \int (\kappa \iota_R F + F_H) \wedge *(\kappa \iota_R F + F_H) = \int (\iota_R F) \wedge *(\iota_R F) + F_H^+ \wedge *F_H^+ + F_H^- \wedge *F_H^- \\ &= \int (\iota_R F) \wedge *(\iota_R F) + 2F_H^+ \wedge *F_H^+ - \kappa \wedge F \wedge F, \end{aligned} \quad (14.4.6)$$

where we have used the orthogonality of different subspaces. The term  $\int \kappa \wedge F \wedge F$  provides a weighting for the instantons. Since this term is not topological, so it is not immediately clear that its value is bounded away from zero. This gap is important in that it allows us to take the large  $N$  limit and decouple the instanton sector, see Chapter 15. In the simple case of a round  $S^5$ , it is possible to further analyse the contact instanton configuration, and show that for  $SU(2)$  gauge group the contact instantons are in 1-1 correspondence with the instantons on  $\mathbb{C}P^2$ , see section 3.2.2. of [25]<sup>5</sup>. So in this case, we do have a gap and this gap

---

<sup>5</sup>Due to a historical accident, the choice of volume form in [25] is opposite to the current one. The reader should bear this in mind when comparing results between the two papers, especially some anti-self-dualities there will become self-dualities here.

will be stable against small perturbations of the geometry. For the general case, we believe that if one carries out some careful analysis, one can show the existence of the gap, but we did not investigate it any further.

The round  $S^5$  case is special because the Reeb vector field  $R$  forms closed orbits everywhere, in fact it is the  $U(1)$  rotation along the fibre of the Hopf fibration  $U(1) \rightarrow S^5 \rightarrow \mathbb{C}P^2$ . However what is more interesting is the opposite extreme: when the Reeb flows are not closed except at a few isolated loci. In this situation, the instanton partition functions are conjectured to concentrate along those few orbits, this conjecture is supported by evidence from the perturbative sector, see Chapter 16. For the rest of the review, we focus on the perturbative, i.e. zero instanton sector. To summarise, the localisation locus for the vector multiplet is

$$A = 0, \quad \sigma = a = \text{const} \in i\mathfrak{g}, \quad \Psi = 0. \quad (14.4.7)$$

Evaluating the classical action (14.4.2) at this background we get

$$S_{vec} = -\text{Tr} \int \kappa (d\kappa)^2 \sigma^2 = -8\text{Vol} \text{Tr}[a^2], \quad (14.4.8)$$

this quadratic term will be the Gaussian damping for the matrix model resulting from localisation.

## 14.4.2 Hyper-multiplet and vanishing theorems

As explained at the end of section 14.3.3, if one sticks to the SE geometry, then one can use (14.3.16) as his starting point, while if one deforms the SE geometry then (14.3.21) is a more convenient starting point.

We first deal with the case of SE metric, i.e. (14.3.16), where one can give a concise proof of a vanishing theorem. We can add the following exact term  $-t\delta \int W_{hyp}$  to the path integral, where

$$W_{hyp} = \frac{1}{2} \Omega_{AB} \left[ \psi_+^A (-L_R^{As} - G_\sigma) q^B + \psi_-^A \mathcal{F}^B + 2i \psi_-^A \not{D} q^B \right],$$

where the notation  $L_X^{As}$  denotes the spinorial Lie derivative coupled to the gauge potential. Note that the last two terms are designed to produce a kinetic term for  $q$  and the fermions. The bosonic part of  $\delta W_{hyp}$  is

$$\delta W_{hyp}|_{bos} = \frac{1}{2} \Omega^{AB} \left[ (L_R^{As} q)^A (L_R^{As} q)^B - (G_\sigma q)^A (G_\sigma q)^B + \mathcal{F}^A \mathcal{F}^B + 2i \mathcal{F}^A \not{D} q^B \right]. \quad (14.4.9)$$

In the last term, only the negative  $\gamma_5$  chirality part of  $\not{D} q$  will survive since  $\gamma_5 \mathcal{F} = -\mathcal{F}$ . Now integrating out  $\mathcal{F}$  produces a good kinetic term  $(\not{D} q)^2$ . To this end, it is now convenient to take the gauge group to be  $SU(N)$  and solve the constraint as in (14.3.14), then (14.4.9) turns into

$$\delta W_{hyp}|_{bos} = (L_R^{As} q)^\dagger L_R^{As} q - q^\dagger \sigma^2 q + \mathcal{F}^\dagger \mathcal{F} + i \left[ \mathcal{F}^\dagger \not{D} q + c.c. \right], \quad (14.4.10)$$

where we have used the same symbol for the fields before and after the rewriting (14.3.14). Now we can integrate over  $\mathcal{F}$  and get

$$W_{hyp}|_{bos} = (\mathcal{D} - \frac{1}{4}\mathcal{J}q)^\dagger (\mathcal{D} - \frac{1}{4}\mathcal{J}q) - q^\dagger \sigma^2 q ,$$

where the key relation used in the step above is

$$\frac{1}{2}(1 + \gamma_5) \left( \mathcal{D} - \frac{1}{4}\mathcal{J} \right) q = -L_R^{As} q .$$

Remembering that  $\sigma$  is Wick rotated, we get the localisation locus

$$\left( -\frac{1}{4}\mathcal{J} + \mathcal{D} \right) q = 0 , \quad \sigma q = 0 . \tag{14.4.11}$$

We prove next that this set of conditions implies  $q = 0$ .

**Proof** We start from the equation  $(\mathcal{D} - \mathcal{J}/4)q = 0$  and so

$$0 = (\mathcal{D} - \mathcal{J}/4)^2 q = (\mathcal{D}^2 - \frac{1}{4}\mathcal{J}\mathcal{D} - \frac{1}{4}\mathcal{D}\mathcal{J} + \frac{1}{16}\mathcal{J}^2)q = (\mathcal{D}^2 - \frac{1}{4}\mathcal{D}\mathcal{J})q .$$

Now put this under the integral

$$0 = \int q^\dagger (-\mathcal{D}^2 + \frac{1}{4}\mathcal{D}\mathcal{J})q \stackrel{ibp}{=} \int q^\dagger (-\mathcal{D}^2 - \frac{1}{4}\overleftarrow{\mathcal{D}}\mathcal{J})q = \int q^\dagger (-\mathcal{D}^2 + \frac{1}{16}\mathcal{J}^2)q ,$$

note that in our convention the gamma matrices are hermitian, so  $\Gamma_p^\dagger = \Gamma_p$ ,  $\Gamma_{pq}^\dagger = -\Gamma_{pq}$ . The two terms in the integral are

$$\mathcal{D}^2 = D^2 - 5 - \frac{i}{2}\mathcal{F} , \quad \mathcal{J}^2 = -8(1 + \gamma_5) .$$

We also put the gauge field in an instanton configuration (14.4.4). Then we have

$$q^\dagger \mathcal{F} q = q^\dagger (F_H^+)_{mn} \Gamma^{mn} q = 0 ,$$

since  $q^\dagger \Gamma^{mn} q$  is horizontal self-dual and  $F_H^+ = 0$ . Assembling everything altogether

$$0 = \int q^\dagger \left( \frac{1}{16}\mathcal{J}^2 - D^2 + 5 \right) q = \int q^\dagger \left( -D^2 + 4 \right) q = \int (D_m q)^\dagger (D^m q) + 4 \int q^\dagger q .$$

So we must have  $q = 0$  ■

The key perennial trick is to relate two quadratic differential operators, e.g.  $\mathcal{D}^2$  and  $D * D$  hoping to produce some constant terms. This technique will be exploited again shortly.

*Now we deviate from the SE metric*, but keeping the topology type. It is more convenient to do so in the form formulation of (14.3.21). Remember that  $q, \psi_+ \in \Omega_H^{0,0} \oplus \Omega_H^{0,2}$  and  $\psi_-, \mathcal{F} \in \Omega_H^{0,1}$ ,

we denote the 0-form component of  $q, \psi_+$  as  $h, \lambda$  and the 2-form component as  $B, \Sigma$ , while  $\psi_-, \mathcal{F}$  are always 1-forms, we still call them  $\psi_-, \mathcal{F}$ .

We add an exact term  $-t\delta \int W_{hyp}$ , which is the same as (14.4.10) except the appropriate replacements

$$\not{D}q \Rightarrow (Dh)^{0,1} - 4D^\dagger B; L_R^{As} \Rightarrow L_R^A + if_R.$$

After integrating out  $\mathcal{F}$ , the bosonic part of  $\delta W_{hyp}$  is<sup>6</sup>

$$\begin{aligned} \delta W_{hyp}|_{\text{bos}} &= \int \left( (-L_R^A - if_R)q \right)^\dagger * (-L_R^A - if_R)q - (G_\sigma q)^\dagger * G_\sigma q \\ &\quad + (D^{0,1}h - 4D^\dagger B)^\dagger * (D^{0,1}h - 4D^\dagger B). \end{aligned}$$

So the localisation locus, written in differential forms, is

$$(L_R^A + if_R)h = (L_R^A + if_R)B = 0, \quad D^{0,1}h - 4D^\dagger B = 0. \quad (14.4.12)$$

Next we give a convenient criteria for the vanishing of all fields in the hypermultiplet. Consider the integral

$$0 = \int (D^{0,1}h - 4D^\dagger B)^\dagger * (D^{0,1}h - 4D^\dagger B) = \|D^{0,1}h\|^2 + 16\|D^\dagger B\|^2. \quad (14.4.13)$$

Note that the cross term between  $D^{0,1}h$  and  $D^\dagger B$  can be shown to vanish by using (14.4.4).

Now focus on the last three terms, we apply a Weizenbock formula (see (14) in sec.2.5 of [35])

$$\begin{aligned} \|D^\dagger B\|^2 + \frac{1}{2}\|L_R^A B\|^2 &= \|DB\|^2 - \frac{1}{2}\|L_R^A B\|^2 \\ &= \int if_b^a * (B_a^\dagger \times B^b) - \frac{1}{4}(8-s)B^\dagger * B + \frac{1}{4}\langle \nabla B^\dagger, \nabla B \rangle \end{aligned} \quad (14.4.14)$$

where  $s$  is the scalar curvature,  $a, b$  are indices in the fundamental of  $SU(N)$ ,  $\langle -, - \rangle$  is defined in (14.7.12) and the  $\times$  operation is defined as

$$\Omega_H^{2+} \ni (X \times Y)_{mn} = X_{mp}Y_n{}^p - X_{np}Y_m{}^p, \quad X, Y \in \Omega_H^{2+}.$$

The term in (14.4.14) involving the curvature vanishes, since  $B_a^\dagger \times B^b$  is horizontal self-dual and  $F$  is horizontal anti-self-dual. And the last term in (14.4.14) can be broken further into

$$\begin{aligned} \langle \nabla B^\dagger, \nabla B \rangle &= \langle (\nabla B^\dagger)_H, (\nabla B)_H \rangle + \langle (L_R^A - 2i)B^\dagger, (L_R^A + 2i)B \rangle + 2\langle B^\dagger, B \rangle \\ &= \langle (\nabla B^\dagger)_H, (\nabla B)_H \rangle + (2 + (2 - f_R)^2)\langle B^\dagger, B \rangle. \end{aligned}$$

Thus (14.4.13) equals (using (14.4.12))

$$14.4.13 = \|D^{0,1}h\|^2 + 16 \int \left( \frac{s}{4} + 1 - 2f_R \right) B^\dagger * B + \frac{1}{4}\langle (\nabla B^\dagger)_H, (\nabla B)_H \rangle.$$

---

<sup>6</sup>Here  $D^\dagger$  is the adjoint of  $D$ , and  $B^\dagger$  is the hermitian conjugate of  $B$ , hopefully, there will be no confusion.

so we can conclude the vanishing of  $B$  if  $s + 4 - 8f_R > 0$  everywhere.

Assuming that the condition above is satisfied and so  $B = 0$ . To prove the vanishing of  $h$ , we need a trick, note that  $\varrho(L_R^A + if_R)h = (L_R^A - if_R)(\varrho h)$ , then we can combine  $\bar{\varrho}h$  into a 2-form. The equation (14.4.12) plus a choice of  $\varrho$  such that  $D^{0,1}\varrho = 0$  leads to that

$$D^{(0,1)}(\varrho h) = 0 = (L_R^A - if_R)(\varrho h)$$

The rest of the treatment for  $h$  will be as for  $B$ . One has

$$0 = \|D^{0,1}(\varrho h)\|^2 = \|D(\varrho h)\|^2 - \|L_R^A \varrho h\|^2.$$

Now apply the second half of Weizenbock formula (14.4.14), and arrives at

$$0 = \int \left( \frac{s}{4} + 1 - 2f_R \right) (\varrho h) * (\varrho h)^\dagger + \frac{1}{4} \langle (\nabla \varrho h)_H, (\nabla (\varrho h)^\dagger)_H \rangle$$

and hence the same vanishing condition. So the conclusion is that if

$$s + 4 - 8f_R > 0 \tag{14.4.15}$$

then the hyper-multiplet vanishes at the localisation locus. Again at the SE point, the lhs above equals  $20 + 4 - 8 \cdot 3/2 = 12$  corroborating with the direct proof after (14.4.11). Now one can perturb the geometry in an open neighbourhood round the SE point and still retain the vanishing result. We have not carried out the detailed calculation of  $s$  away from the SE point, but it is likely that, for the type of deformation we consider in this paper, this condition is true always.

**Remark** The sign in front of  $if_R$  in (14.4.12) is crucial. In fact, we shall see that the equation

$$(L_R - ic)h = D^{0,1}h = 0$$

has non-trivial solutions for infinitely many positive values of  $c$ . These solutions represent the Kohn-Rossi cohomology. But when  $c \geq 0$ , the vanishing theorem is rendered impotent, since one needs to replace the combination  $s + 4 - 8f_R$  in (14.4.15) with

$$s + 4 - 8(c + 2f_R)$$

which can just escape the vanishing theorem, say, at the SE point for  $c \geq 0$ . This is a nice consistency check on our manipulations with the Weizenbock formula.

## 14.5 Gauge fixing and the determinant

Now we are ready to apply the abstract model in section 14.3.1 to the gauge theory and we follow closely the original work by Pestun [5]. The hyper complex (14.3.16) is perfectly analogous to (14.3.1), however the vector complex (14.3.12) is not, in that the combination  $\Phi = \iota_R A + \sigma$  has no susy variation. Besides this, there is the problem of gauge fixing. We

first fix the gauge bundle to be topologically trivial, since we are only interested in the zero instanton sector, in particular, the connection  $A$  is a global adjoint 1-form.

We will take a shortcut and arrive at the answer faster though admittedly less rigorously. Up to gauge transformation, the fixed points are given by (14.4.7), and we use the gauge freedom to fix  $\Phi$  at  $\Phi = a$ . Doing this will incur a Fadeev-Popov determinant

$$J_{FP} = \det_{\Omega^0}(-iL_R + iG_a) ,$$

since the gauge transformation of  $\Phi$  is  $G_\epsilon \Phi = L_R \epsilon + i[\epsilon, \Phi]$ . With  $\Phi$  fixed, the rest of the fields contribute to a determinant factor as in (14.3.5)

$$\text{sdet}_{\Omega^1 \oplus \Omega_H^{2+}}^{1/2}(-iL_R + iG_a) ,$$

where  $\Omega^1$  comes from  $A$  and  $\Omega_H^{2+}$  from  $\chi$ . Combining this with the Fadeev-Popov determinant

$$J_{vec} = \text{sdet}_{2\Omega^0 \oplus \Omega^1 \oplus \Omega_H^{2+}}^{1/2}(-iL_R + iG_a) ,$$

but one needs to exclude from the zero forms their constant mode since these are not treated as gauge symmetry but as moduli of the Colomb branch. The hyper contribution is more straightforward, one uses the analogue of the toy model given in sec.14.3.1

$$J_{hyp} = \text{sdet}_{\Omega_H^{0,\cdot}}^{-1}(-iL_R^s + iG_a) ,$$

where as a reminder  $L_R^s$  is the spinor Lie derivative whose relation to the usual Lie derivative is given in (14.3.20).

To evaluate the first determinant, the complex can be decomposed into

$$2\Omega^0 \oplus \Omega^1 \oplus \Omega_H^{2+} = \Omega^{0,0} \oplus \Omega_H^{0,1} \oplus \Omega_H^{0,2} \bigoplus c.c. ,$$

so we just need to compute the determinant taken on the complex  $\Omega_H^{0,\cdot}$ , which is the Kohn-Rossi complex with the differential  $\bar{\partial}_H$  given in (14.7.16). It will be explained in detail in sec.14.5.1 that the super-determinant cancels out totally except those that are in the  $\bar{\partial}_H$  cohomology, leaving only

$$J_{vec} = \text{sdet}_{H_{\bar{\partial}_H}^{0,\cdot}}(-iL_R + iG_a) ,$$

$$J_{hyp} = \text{sdet}_{H_{\bar{\partial}_H}^{0,\cdot}}^{-1}(-iL_R^s + iG_a) .$$

For the vector multiplet, we needed to take a square root but we will ignore the possible phase, and we also remember that we exclude the constant mode.

Assemble the two determinants together with the classical action evaluated at (14.4.7), and Wick rotate  $a \rightarrow ia$

$$Z^{pert} = \int_{\mathfrak{su}} da e^{-\frac{8\pi^3 r}{9YM} \rho \text{Tr}[a^2]} \cdot \frac{\det'_{adj} \text{sdet}_{\Omega_H^{0,\cdot}}(-iL_R - G_a)}{\det_{\underline{R}} \text{sdet}_{\Omega_H^{0,\cdot}}(-iL_R^s - G_a)} \cdot \frac{1}{\det'_{adj}(-G_a)} ,$$

in fact the last term can be absorbed if one writes the integral of  $a$  not over  $\mathfrak{su}(N)$  but over its cartan  $\mathfrak{t}$

$$Z^{pert} = \int_{\mathfrak{t}} da e^{-\frac{8\pi^3 r}{9YM} \rho \text{Tr}[a^2]} \cdot \frac{\det'_{adj} \text{sdet}_{\Omega_H^{0,\cdot}}(-iL_R - G_a)}{\det_{\underline{R}} \text{sdet}_{\Omega_H^{0,\cdot}}(-iL_R^s - G_a)} . \quad (14.5.1)$$

### 14.5.1 The determinant

This section makes heavy use of differential geometrical properties of the toric Sasaki-Einstein manifolds. We try to provide enough stepping stones in the text, further details can be found in the appendix.

From the travail of previous sections, the whole localisation reduces to the computation of the super determinant in (14.5.1)

$$s \det_{\mathcal{V}}(-iL_R + x) , \quad \mathcal{V} = \oplus \Omega_H^{0,\bullet} \quad (14.5.2)$$

taken over the horizontal anti-holomorphic forms  $\mathcal{V} = \Omega_H^{0,\bullet}$ . Even though  $\mathcal{V}$  is infinite dimensional, the presence of susy guarantees massive cancellation in the super determinant. The problem is to how to keep track of the cancellation, and more importantly, the remainders after the cancellation.

Let  $P$  (respectively  $P_+$  and  $P_-$ ) be the projectors that projects a 1-form to its horizontal (respectively horizontal hollomorphic and anti-holomorphic) components, defined in (14.7.13). We define an operator that acts on horizontal  $(p, q)$  forms

$$\bar{\partial}_H \omega = dx^r (P_-)_r{}^s \nabla_s \omega + iq\kappa \wedge \omega , \quad \omega \in \Omega_H^{p,q} . \quad (14.5.3)$$

One can check that it sends  $\Omega_H^{p,q} \rightarrow \Omega_H^{p,q+1}$  and it is nilpotent, i.e. it is a differential of the complex  $\Omega_H^{p,\bullet}$ . The cohomology of  $\bar{\partial}_H$  is known as the *Kohn-Rossi* cohomology (see [39], we shall soon show that  $\bar{\partial}_H$  is the restriction of the Dolbeault operator on the cone  $C(M)$  to the boundary  $M$ , which is the setting of [39]). One can also couple  $\bar{\partial}_H$  to the gauge connection, and all properties still hold if the gauge curvature is horizontal anti-self-dual; hence this operator is a differential at any instanton background.

The  $\bar{\partial}_H$ -complex is not elliptic: clearly the symbol of  $\bar{\partial}_H$  is not exact along the  $R$  direction; thus its cohomology is of infinite dimension. But fortunately, for the toric Sasaki manifolds, we have a powerful index theorem that can handle the difficulty. For toric Sasaki geometry, the isometry contains  $G = U(1)^3$ , and the Reeb is a linear combination of the three  $U(1)$ 's. Then the  $\bar{\partial}_H$ -complex is an elliptic complex transverse to the  $G$ -action, since its symbol is elliptic transverse to the Reeb. Furthermore,  $\bar{\partial}_H$  is invariant under the  $G$ -action, since all structures appearing in (14.5.3), the metric,  $R$ ,  $\kappa$  (and hence also  $J$ , since  $J \sim d\kappa$ ) are invariant under the  $G = U(1)^3$  isometry. Then we have the decomposition of the  $\bar{\partial}_H$  cohomology into the representations of  $G$  (see Theorem 2.2 [40])

$$H_{\bar{\partial}_H}^{0,p} = \bigoplus_i m_i^p R_i , \quad m_i^p \in \mathbb{Z}_{\geq 0} , \quad (14.5.4)$$

where the  $m$ 's are multiplicities of the representation of  $R_i$ . In the case  $G = U(1)^3$ , the representations are just labelled by 3 charges, which we will organize into an integer valued 3-vector.

The localisation technique for transversely elliptic operators due to Atiyah [40] allows us to compute the alternating differences of  $m_i$ . However this is a fairly involved task, so we present first a technique sketched by Schmude [23].

## 14.5.2 Schmude's approach

The key observation is that the Dolbeault operator  $\bar{\partial}^6$  on the 6d Kähler cone acts as

$$\bar{\partial}^6 = \frac{1}{2}(t^{-1}dt - i\kappa)(L_{t\partial_t} + iL_R) - \frac{i}{2}d\kappa \iota_{t\partial_t} + \bar{\partial}_H^5, \quad (14.5.5)$$

where we have inserted 5, 6 to indicate whether an object is a 5d or 6d one.

Consider  $H_{\bar{\partial}_H}^{0,\bullet}$ , and decompose it according to (14.5.4), meaning that we can discuss  $H_{\bar{\partial}_H}^{0,\bullet}$  assuming a fixed  $U(1)^3$  charge. In all our considerations we assume the toric setup. Take  $\alpha$  a representative of  $H_{\bar{\partial}_H}^{0,\bullet}$ , we can assume that it has charge vector  $\vec{q}$ , then its  $L_R$  eigenvalue is  $L_R\alpha = i(\vec{R} \cdot \vec{q})\alpha$ , where we have used an integer 3-vector  $\vec{R}$  to express the Reeb as a linear combination of the three  $U(1)$  isometry. We can now extend  $\alpha$  to the Kähler cone as

$$\alpha \rightarrow \tilde{\alpha} = t^{\vec{R} \cdot \vec{q}}\alpha, \quad (14.5.6)$$

looking at (14.5.5),  $\tilde{\alpha}$  will be annihilated by  $\bar{\partial}^6$ . If  $\vec{R}$  is assumed to be within the dual cone (see sec.14.7.2) then  $\vec{R} \cdot \vec{q} \geq 0$  and so  $\tilde{\alpha}$  is well-defined within the 6d Kähler cone.

On the other hand if  $\alpha = \bar{\partial}_H\beta$ , then

$$\tilde{\alpha} = \bar{\partial}^6\tilde{\beta},$$

where  $\tilde{\beta} = t^{\vec{R} \cdot \vec{q}}\beta$ . Thus we have a well-defined map of cohomology

$$H_{\bar{\partial}_H}^{0,\bullet}(M) \rightarrow H_{\bar{\partial}^6}^{0,\bullet}(C(M)). \quad (14.5.7)$$

The left inverse to the extension map (14.5.6) is the restriction map that restricts a form to the surface  $t = 1$ . This already shows that the restriction map is onto, while the extension map is into. From the injectivity we deduce

$$H_{\bar{\partial}_H}^{0,1}(M) = 0$$

since  $\pi_1(C(M))$  is at most torsion, and  $C(M)$  is Kähler.

We turn now to  $H_{\bar{\partial}_H}^{0,0}$ . Since  $H_{\bar{\partial}^6}^{0,0}(C(M))$  are the holomorphic functions on  $C(M)$  and the latter has a very convenient description in the toric case: they correspond to integer lattice points in the cone  $C$ . One can read off the charges under  $U(1)^3$  of the function from the coordinates of the lattice point that represents the function. This also shows that the restriction to  $t = 1$  is injective, since there is one unique holomorphic function with a given  $U(1)^3$  charge, two functions with different charges cannot cancel each other when restricted to  $t = 1$ . In this way we have a complete answer for (14.5.4) at degree zero and one.

For degree two, one can also show that (14.5.6) is an extension and compute  $H_{\bar{\partial}^6}^{0,2}(C(M))$  using Serre duality. But we can in fact make the Serre-duality explicit here. Let  $\bar{\varrho} \in \Omega_H^{0,2}$  satisfying  $\partial_H\bar{\varrho} = 0$  (from this we also have  $d^\dagger\bar{\varrho} = 0$ ). Now any section of  $\Omega_H^{0,2}$  is of the form  $\bar{f}\bar{\varrho}$  for some function  $\bar{f}$ , we only need to sift out the  $\bar{\partial}_H$ -exact ones to get  $H_{\bar{\partial}_H}^{0,2}$ . On  $(0, 2)$  forms we have

$$\bar{\partial}_H^\dagger(\bar{f}\bar{\varrho}) = d^\dagger(\bar{f}\bar{\varrho}) = -g^{pq}(\partial_p\bar{f})\bar{\varrho}_{qr}dx^r.$$

The right hand side is zero iff  $\bar{f}$  satisfies  $\partial_H \bar{f} = 0$ . Note that if  $\bar{\partial}_H^\dagger(\bar{f}\bar{\varrho}) = 0$ , then  $\bar{f}\bar{\varrho}$  is orthogonal to any  $\bar{\partial}_H$ -exact forms, so we reach the conclusion that

$$H_{\bar{\partial}_H}^{0,0}(M) \xrightarrow{f \rightarrow \bar{f}\bar{\varrho}} H_{\bar{\partial}_H}^{0,2}(M) \quad (14.5.8)$$

is an isomorphism <sup>7</sup>

Now we can wrap up the lengthy discussion and get the index. We introduce some formal variables  $s_a$ ,  $a = 1, 2, 3$  and use monomials of such to denote a representation of  $U(1)^3$ . For example  $s_1^2 s_2^{-5} s_3$  is a representation of charge 2 under the 1st  $U(1)$ , charge  $-5$  under the 2nd and charge 1 under the 3rd. Then the index

$$\text{ind}_{U(1)^3} \bar{\partial}_H = \sum_{\vec{m} \in C \cap \mathbb{Z}^3} \bar{s}^{\vec{m}} + \sum_{-\vec{m} \in C^\circ \cap \mathbb{Z}^3} \bar{s}^{-\vec{m}}, \quad (14.5.9)$$

where

$$\begin{aligned} \bar{s}^{\vec{m}} &= s_1^{m_1} s_2^{m_2} s_3^{m_3}, \\ C &= \{\vec{r} \in \mathbb{R}^3, \vec{r} \cdot \vec{v}_i \geq 0\}, \\ C^\circ &= \{\vec{r} \in \mathbb{R}^3, \vec{r} \cdot \vec{v}_i > 0\}, \end{aligned}$$

where  $i$  runs over all faces of the cone. The first summand comes from  $H_{\bar{\partial}_H}^{0,0}$  and is straightforward. For the second term, since we see from (14.5.8) that  $H_{\bar{\partial}_H}^{0,2}$  are also 1-1 to lattice points in the cone, but the  $U(1)^3$ -charge is reversed and then shifted by the charge of  $\bar{\varrho}$ . So we should have written the second summand as  $\sum_{-\vec{m} \in C \cap \mathbb{Z}^3} \bar{s}^{-\vec{m}-\vec{\xi}}$  where  $-\vec{\xi}$  is the charge vector for  $\bar{\varrho}$ . But if we use the 1-Gorenstein condition  $\vec{\xi} \cdot \vec{v}_i = 1, \forall i$  (see the discussion around (14.7.23)), we can write the sum as in (14.5.9). But note that (14.5.9) is valid even for toric Sasaki manifolds, i.e. when  $\bar{\varrho}$  does not exist.

We continue our computation of the determinant. From the index, we read off

$$\text{sdet}_{\Omega_H^{0,\cdot}}(-iL_R + x) = \prod_{\vec{n} \in C \cap \mathbb{Z}^3} (\vec{n} \cdot \vec{R} + x) (-\vec{n} \cdot \vec{R} - 2f_R + x), \quad (14.5.10)$$

where the first product comes from  $H_{\bar{\partial}_H}^{0,0}$  and  $\vec{n} \cdot \vec{R}$  is the  $-iL_R$ -eigenvalue; the second term comes from  $H_{\bar{\partial}_H}^{0,2}$  and their  $-iL_R$  eigenvalue has been explained in the last paragraph.

**Example** As a more familiar example, take  $M = S^5$ . Then the cone is just the first octant  $C = \mathbb{R}_{\geq 0}^3$ . Take also  $\vec{R} = [1, 1, 1]$ , then  $f_R = 3$  and

$$\text{sdet} = \prod_{m \geq 0} (m + x)^{(m+1)(m+2)/2} (-m - 3 + x)^{(m+1)(m+2)/2}. \quad (14.5.11)$$

The multiplicity  $(m + 1)(m + 2)/2$  comes as follows. Fixing the plane  $\vec{n} \cdot \vec{R} = m$ , then its intersection with the cone contains  $(m + 1)(m + 2)/2$  lattice points.

---

<sup>7</sup>In the proof, we have not treated some analytical issues carefully, such as how to define the Hilbert space where the horizontal forms reside, but this is slightly of the topic of the paper. The same omission was in the treatment of [41], but we believe that the our result will not be affected by these technicalities.

In fact, with the Reeb given by its charge  $[1, 1, 1]$ , it corresponds to the  $U(1)$  vector field in the Hopf fibration  $U(1) \rightarrow S^5 \rightarrow \mathbb{C}P^2$ . In this case one can compute the  $\bar{\partial}_H$ -cohomology using a 'Fourier transform'. For example computing  $H_{\bar{\partial}_H}^{0,0}(S^5)$  with fixed  $(-iL_R)$ -eigenvalue  $m$  amounts to computing  $H^0(\mathbb{C}P^2, \mathcal{O}(m))$ , and the answer is  $(m+1)(m+2)/2$  for  $m \geq 0$  (which is the number of monomials homogeneous of degree  $m$  in three variables) and zero otherwise. In general

$$\begin{aligned} \dim H^{0,0}(\mathbb{C}P^2, \mathcal{O}(n)) &= \begin{cases} \frac{1}{2}(n+1)(n+2) & n \geq 0 \\ 0 & n < 0 \end{cases}, \\ \dim H^{0,1}(\mathbb{C}P^2, \mathcal{O}(n)) &= 0 \\ \dim H^{0,2}(\mathbb{C}P^2, \mathcal{O}(n)) &= \begin{cases} \frac{1}{2}(n+1)(n+2) & n \leq -3 \\ 0 & n > -3 \end{cases}. \end{aligned} \quad (14.5.12)$$

The group  $H_{\bar{\partial}_H}^{0,2}(S^5) \sim H^2(\mathbb{C}P^2, \mathcal{O}(m)) \sim H^0(\mathbb{C}P^2, \mathcal{O}(-m-3))^*$ , where the last duality is the Serre duality and takes the place of (14.5.8). After a change of summation variable, we get the second exponential in (14.5.11).

### 14.5.3 Generalised multiple sine

Up to an overall sign, the product of (14.5.10) is an interesting generalisation of the multiple sine functions. Recall that the usual multiple sine function is defined as

$$S_r(x|\omega) = \prod_{m_a \geq 0} \left( \sum_{a=1}^r m_a \omega_a + x \right) \prod_{m_a > 0} \left( \sum_{a=1}^r m_a \omega_a - x \right)^{(-1)^{r-1}}. \quad (14.5.13)$$

One can define a generalised version of multiple sines associated with a cone in  $\mathbb{R}^r$ ,

$$S_r^C = \prod_{\vec{m} \in C \cap \mathbb{Z}^r} (\vec{\omega} \cdot \vec{m} + x) \prod_{\vec{m} \in C^\circ \cap \mathbb{Z}^r} (\vec{\omega} \cdot \vec{m} - x)^{(-1)^{r-1}}. \quad (14.5.14)$$

So the standard multiple sine corresponds to the cone that is the first orthant of  $\mathbb{R}^r$ . For more properties of (generalised) multiple sines, see [42] and [43]

For our problem, we have the cone  $C \subset \mathbb{R}^3$  which is also the image of the moment map of  $C(M)$ . So (14.5.10) can be written as the generalised triple sine function associated with this cone

$$(14.5.10) \sim S_3^C(x|\vec{R}) = \prod_{\vec{m} \in C(X) \cap \mathbb{Z}^3} (\vec{m} \cdot \vec{R} + x) \prod_{\vec{m} \in C^\circ(X) \cap \mathbb{Z}^3} (\vec{m} \cdot \vec{R} - x).$$

We mainly focus on the case when  $M$  is simply connected SE, then  $C$  is 1-Gorenstein. As we saw, one has  $\vec{\xi} \in \mathbb{Z}^3$  such that  $\vec{\xi} \cdot \vec{v}_i = 1$  and the second product can be written as

$$\prod_{\vec{m} \in C(X) \cap \mathbb{Z}^3} (\vec{m} \cdot \vec{R} + \vec{\xi} \cdot \vec{R} - x) \text{ and } \vec{\xi} \cdot \vec{R} \text{ is precisely the shift } 2f_R.$$

So we have finished our localisation computation for the zero instanton sector

$$Z^{\text{pert}} = \int_{\mathfrak{t}} da e^{-\frac{8\pi^3 r}{g_{YM}^2} e^{\text{Tr}[a^2]}} \cdot \frac{\det'_{\text{adj}} S_3^C(ia|\vec{R})}{\det_{\underline{R}} S_3^C(ia + im + \vec{\xi} \cdot \vec{R}/2|\vec{R})}, \quad (14.5.15)$$

where a mass  $m$  is generated for the hyper-multiplet by a simple shift of  $a$ , i.e.  $m$  is regarded as a background gauge connection coupled to the hyper. The matrix model (14.5.15) is discussed further in Chapter 15.

### 14.5.4 Conjecture for the full answer

The answer (14.5.15) corresponds to the contribution of the trivial connection. In order to derive the full answer we have to analyze the contact instantons (14.4.5) and perform the one-loop calculations over every non-trivial solutions. As it stands the problem is hard to solve from the first principles. However it is natural to expect that only the configurations invariant under full  $U(1)^3$  action will contribute to the integral. The invariant configurations will tend to localise around the close Reeb orbits (for the generic choice of  $\kappa$  there will be only a few closed orbits and they are called Reeb orbits). Thus around every Reeb orbit the complex and the calculation will boil down to the calculation on  $\mathbb{C}^2 \times S^1$ , very much in analogy with Pestun's calculation [5] on  $S^4$  and its reduction to  $\mathbb{C}^2$ . In order to conjecture the full answer we need to identify the parameters on toric SE manifold with the parameters of Nekrasov's instanton partition function on  $\mathbb{C}^2 \times S^1$  corresponding to each closed Reeb orbit. This can be done either geometrically or by studying the factorisation properties of the perturbative answer [41]. The full answer is written as

$$Z^{full} = \int_{\mathfrak{t}} da e^{-\frac{8\pi^3 r}{g_{YM}^2} \varrho \text{Tr}[a^2]} \cdot \frac{\det'_{adj} S_3^C(ia|\vec{R})}{\det_{\underline{R}} S_3^C(ia + im + \vec{\xi} \cdot \vec{R}/2|\vec{R})} \prod_{i=1}^n Z_{\mathbb{C}^2 \times S^1}^{\text{Nekrasov}}(\beta_i, \epsilon_i, \epsilon'_i), \quad (14.5.16)$$

where  $\beta_i$  is radius of  $S^1$ ,  $\epsilon_i, \epsilon'_i$  are equivariant parameters on  $\mathbb{C}^2$ . Here  $n$  is the number of closed Reeb orbits and the parameters  $\beta_i, \epsilon_i, \epsilon'_i$  can be read off from the toric data [41]. This conjecture is discussed further in Chapter 16.

## 14.6 Asymptotics and comparison with flat space

In this section, we will compare our result with a one-loop flat space computation, in particular, we will obtain a match between the precise coefficient of the effective  $\mathcal{A}^3$  term generated at 1-loop.

We first analyze the large  $x$  behaviour of the generalised triple sine functions. The process is a bit technical and we start from a toy model

$$S_1 = \prod_{n=0}^{\infty} (x + n\omega) \cdot \prod_{n=0}^{\infty} (\omega - x + n\omega) = 2 \sin \frac{\pi x}{\omega}.$$

Here we assume that all infinite product are regularized. Take the first product and write it using the zeta function regularisation

$$\begin{aligned} \log \prod_{n=0}^{\infty} (x + n\omega) &= -\frac{\partial}{\partial s} \frac{1}{\Gamma(s)} \int_0^{\infty} \sum_{n=0}^{\infty} e^{-(n\omega+x)t} t^{s-1} dt \Big|_{s=0} \\ &= -\frac{\partial}{\partial s} \frac{1}{\Gamma(s)} \int_0^{\infty} \frac{e^{-xt}}{1 - e^{-\omega t}} t^{s-1} dt \Big|_{s=0}, \end{aligned}$$

where it is assumed  $\text{Re } \omega > \text{Re } x > 0$  and we are interested in  $\text{Im } x \gg 0$ . In this regime, one can replace  $(1 - e^{-\omega t})^{-1}$  with its Laurent expansion at  $t = 0$ , the error is of order  $x^{-1}$  (see sec.6.1 of [21]). Furthermore since  $\lim_{s \rightarrow 0} \Gamma(s)^{-1} \rightarrow 0$ , one needs only keep the singular terms from the integral. Thus one keeps only terms of order  $t^{-1}$ ,  $t^0$  in the previous Laurent series. These terms will produce  $\Gamma(s - 1)$ ,  $\Gamma(s)$  and therefore survive the limit  $s \rightarrow 0$ . The net result is

$$\log \prod_{n=0}^{\infty} (x + n\omega) = -\frac{1}{\omega} (x \log x - x) - \frac{1}{2} \log x + \mathcal{O}(x^{-1}).$$

One replaces  $x$  with  $\omega - x$  in the second product, and in total one gets

$$\log S_1(x|\omega) = \frac{\pi}{\omega} |\text{Im } x| - \frac{i\pi}{2} \text{sgn}(\text{Im } x) + \mathcal{O}(x^{-1}).$$

In the higher dimension case, we have the following formula that expresses the asymptotic behaviour of a generalised triple sine in terms of the geometrical data of the cone (we assume that the cone is 1-Gorenstein)

$$\log S_3^C(x|\vec{R}) \sim -i\pi \text{sgn}(\text{Im } x) \left( \left( \frac{x^3}{3R^1} + \frac{R^1 x}{6} \right) \sum_i \frac{4}{|v_i|} A_i + \frac{x}{12} \frac{1}{2\pi} \sum_i \beta_i \right) = -V_{vec}(x) \quad (14.6.1)$$

$$\log S_3^C(x + \frac{1}{2} \vec{\xi} \cdot \vec{R} | \vec{R}) \sim -i\pi \text{sgn}(\text{Im } x) \left( \left( \frac{x^3}{3R^1} - \frac{R^1 x}{12} \right) \sum_i \frac{4}{|v_i|} A_i + \frac{x}{12} \frac{1}{2\pi} \sum_i \beta_i \right) = V_{hyp}(x) \quad (14.6.2)$$

In the above one should understand  $x$  as  $x^i t_i$  for some basis  $\{t_i\}$  of the Lie algebra, and  $\text{Im } x$  takes the imaginary part of each  $x^i$ . The rest of the term in this asymptotic formula can all be read off from the geometry of the cone. The  $\beta_i$  are the length of the closed Reeb orbits

$$\beta_i = \frac{2\pi}{\det[\vec{v}_i, \vec{v}_{i+1}, \vec{R}]},$$

where  $\vec{v}_i, \vec{v}_{i+1}$  are the normals of the two faces that intersect at the  $i^{\text{th}}$  edge of the cone. For the  $A_i$ 's, let us cut the cone off with the plane  $\vec{y} \cdot \vec{R} = 1/2$ ,  $\vec{y} \in \mathbb{R}^3$ , then  $A_i$  is the area of the  $i^{\text{th}}$  face.

To summarise, asymptotically, the matrix model integral is given by

$$Z^{\text{pert}} \sim \int_{\mathfrak{t}} da e^{-\frac{8\pi^3 r}{g_{YM}^2} \text{Tr}[a^2]} \cdot \exp \left( -\text{Tr}_{ad} V_{vec}(iar) - \text{Tr}_{\underline{R}} V_{hyp}(iar) \right), \quad (14.6.3)$$

with  $V_{vec, hyp}$  given in (14.6.1) and (14.6.2), and  $r$  is of dimension length that controls the size of the manifold.

### 14.6.1 Comparison with flat space

In particular, we can consider the  $S^5$  case, where the cone is the standard one. Then  $A_i = 1/8$ ,  $R^1 = \sum \omega_i$ , and  $\beta_i = 2\pi \omega_i^{-1}$ ,  $i = 1, 2, 3$ . If the sphere is the round one all  $\omega_i = 1$ , we get then

the effective potentials

$$\begin{aligned}
 V_{vec}^{S^5}(x) &\sim i\pi \operatorname{sgn}(\operatorname{Im} x) \left( \frac{x^3}{6} + x \right), \\
 V_{hyp}^{S^5}(x) &\sim -i\pi \operatorname{sgn}(\operatorname{Im} x) \left( \frac{x^3}{6} - \frac{x}{8} \right).
 \end{aligned}
 \tag{14.6.4}$$

The relevance of the asymptotic behaviour is that it controls the flat space limit. If one restores the dimensionful parameter  $r$ , which is the radius of  $S^5$ , we obtain the effective action

$$S_{eff} = \frac{8\pi^3 r^3}{g_{YM}^2} \operatorname{Tr}_f[a^2] + \sum_{\alpha \in \text{roots}} \left( \frac{r^3}{6} |\langle a, \alpha \rangle|^3 - r |\langle a, \alpha \rangle| \right) - \sum_{\mu \in \text{weights}} \left( \frac{r^3}{6} |\langle a, \mu \rangle|^3 + \frac{r}{8} \langle a, \mu \rangle \right)
 \tag{14.6.5}$$

From this one notices that since the volume of  $S^5$  is  $\pi^3 r^5$ , the effective potential is suppressed by  $r^{-2}$

$$V_{eff} = \frac{8}{r^2 g_{YM}^2} \operatorname{Tr}_f[a^2] + \sum_{\alpha \in \text{roots}} \frac{1}{6r^2} |\langle a, \alpha \rangle|^3 - \sum_{\mu \in \text{weights}} \frac{1}{6r^2} |\langle a, \mu \rangle|^3 + \mathcal{O}(r^{-4}),
 \tag{14.6.6}$$

i.e.  $V_{eff}$  computed in the Coulomb branch vanishes as  $r \rightarrow \infty$  and the  $V_{eff}$  we have above is due entirely to the curved space effect. But this is not surprising, since  $a$  is the bottom component of the superfield  $\mathcal{A}$ , and if the only nonzero background of  $\mathcal{A}$  is  $a = \text{const}$ , then nothing will survive the superspace integral. Therefore the comparison with the flat space computation will take an indirect route. The comparison goes as the following chart 14.6.1.

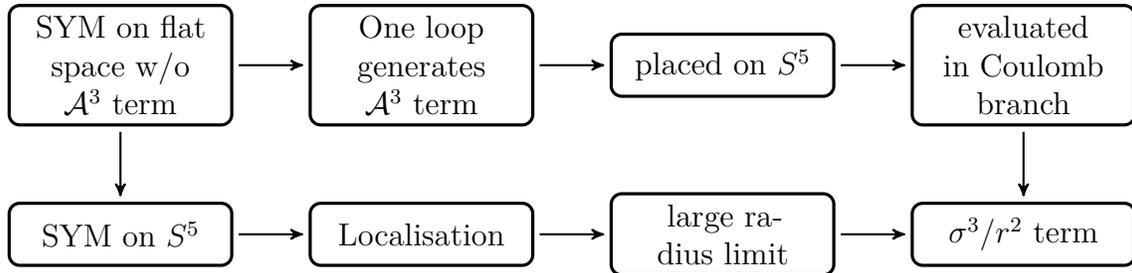

Figure 14.6.1: One starts from super Yang-Mills on flat space without the  $\mathcal{A}^3$  term in the prepotential. The one loop contribution generates an  $\mathcal{A}^3$  term, then the whole system can still be put on  $S^5$  and evaluated in Coulomb branch and will produce  $\sigma^3$  term. On the other hand, one can first place the theory on  $S^5$ , perform localisation, take  $r \rightarrow \infty$  limit and obtain the  $\sigma^3/r^2$  term.

## 14.6.2 The 1-loop effective action

Consider the flat space action (14.2.1) and we will compute the 1-loop effective action at some background. The computation is standard (see for example [44]), one just needs to

compute the determinant

$$S_{eff}(\phi_{cl}) - S_0(\phi_{cl}) = \text{sTr} \frac{1}{2} \log \frac{\partial^2 S_0(\phi)}{\partial \phi \partial \phi} \Big|_{\phi=\phi_{cl}}. \quad (14.6.7)$$

It is also easier to consider its 6d lift of the 5d action, for which  $\sigma$  becomes the temporal component of the gauge field, and hence we just have the gauge fields, fermions plus the ghosts. Split the gauge field as  $A = \mathbf{A} + a$ , with  $\mathbf{A}$  some background, denote by  $\mathbf{D}$  the covariant derivative with  $\mathbf{A}$  and  $\mathbf{F}$  its curvature. For fields of different spins we have a uniform description of the quadratic term

$$S''(\phi_{cl}) = -\mathbf{D}^2 + \mathbf{F}_{mn} J^{mn},$$

where  $J$  is the angular momentum generator

$$\begin{aligned} J^{mn} &= 0 \text{ spin } 0; \quad J^{mn} = \frac{i}{2} \Gamma^{mn} \text{ spin } 1/2, \quad (J^{mn})_{pq} = i \delta_{pq}^{mn} \text{ spin } 1, \\ \text{Tr}[J^{rs} J^{pq}] &= C(j) g^{r[p} g^{q]s} \end{aligned} \quad (14.6.8)$$

with  $C(1) = 2$  and  $C(1/2) = 1$  for the last two cases. The determinant (14.6.7) reduces to

$$\det \Delta_{r,j} = \det(-\partial^2 + \Delta^1 + \Delta^2 + \Delta^J),$$

for each field of representation  $r$  and spin  $j$ . The various terms read

$$\Delta^1 = i(\partial^m \mathbf{A}_m + \mathbf{A}_m \partial^m), \quad \Delta^2 = \mathbf{A}^m \mathbf{A}_m, \quad \Delta^J = \mathbf{F}_{pq} J^{pq}.$$

Out of the computation we aim to get the coefficient of the term  $\sigma F * F$ , so we choose a convenient (supersymmetric) background  $\mathbf{A}^{1-5} \in \mathfrak{h} = \text{Lie } H$ , and  $\sigma = \mathbf{A}^0 \in \mathfrak{h}$  a constant. We compute the determinant up to second order in  $\mathbf{A}^{1-5}$ , so the relevant diagrams are in fig.14.6.2. The first two diagrams give

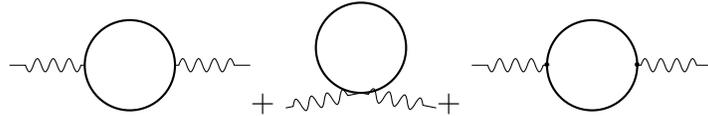

Figure 14.6.2: The 1-loop diagrams. In the third diagram  $\bullet$  represents the insertion  $F_{pq} J^{pq}$ . And the momentum in the loop is to run clockwise.

$$\begin{aligned} I + II &= -\frac{1}{2} d(j) \sum_{\mu \in \text{wght}} \int \frac{d^d k}{(2\pi)^d} \langle \mu | \mathbf{A}_m(k) \mathbf{A}_n(-k) | \mu \rangle \frac{\Gamma(2-d/2)}{(4\pi)^{d/2}} (k^2 g^{mn} - k^m k^n) \\ &\quad \int_0^1 dx (1-4x^2)(x(1-x)k^2 + \langle \mu | \sigma | \mu \rangle^2)^{d/2-2}, \end{aligned} \quad (14.6.9)$$

where  $d(j)$  is the dimension of the spin  $j$  representation. The third diagram gives

$$III = -2C(j) \sum_{\mu \in \text{wght}} \int \frac{d^d k}{(2\pi)^d} \langle \mu | \mathbf{A}_m(k) \mathbf{A}_n(-k) | \mu \rangle (k^2 g_{mn} - k_m k_n) \frac{\Gamma(2-d/2)}{(4\pi)^{d/2}} \int_0^1 dx (x(1-x)k^2 + \langle \mu | \sigma | \mu \rangle^2)^{d/2-2}, \quad (14.6.10)$$

with  $C(j)$  being the Casimir defined in (14.6.8).

From the three contributions, one can extract the term  $\sigma \mathbf{F} * \mathbf{F}$ , for a spin  $j$  field of representation  $r$ , one gets

$$\begin{aligned} X_{r,j} = (I + II) + III &= \sum_{\mu \in \text{wght}} \langle \mu | \mathbf{F} * \mathbf{F} | \mu \rangle \frac{\Gamma(2-d/2)}{(4\pi)^{d/2}} \left( \frac{1}{6} d(j) - 2C(j) \right) |\langle \mu | \sigma | \mu \rangle^2|^{d/2-2} \\ &= -\frac{1}{16\pi^2} \left( \frac{1}{6} d(j) - 2C(j) \right) \text{Tr} [\mathbf{F} * \mathbf{F} | \sigma |]. \end{aligned}$$

Adding up the field content for the vector multiplet ( $n_f = 1$  is the number of Dirac fermions in 5d, the  $1/2$  is because  $\det \Delta_{ad,1/2}$  computes the determinant of  $\not{D}^2$ )

$$X_{ad,1}^{-1/2} + X_{ad,0} + X_{ad,1/2}^{n_f/2} + X_{ad,0}^{-1/2} = -\frac{1}{16\pi^2} \text{Tr}_{ad} [\mathbf{F} * \mathbf{F} | \sigma |],$$

and for the hyper-multiplet

$$X_{r_h,1/2}^{1/2} + X_{r_h,0}^{-4/2} = \frac{1}{16\pi^2} \text{Tr}_{r_h} [\mathbf{F} * \mathbf{F} | \sigma - m |].$$

Thus the effective potential is

$$\frac{1}{V} S_{eff}(\mathbf{A}) = \frac{1}{2g^2} \sum_a \mathbf{F}^a * \mathbf{F}^a + \frac{1}{16\pi^2} \text{Tr}_{ad} [\mathbf{F} * \mathbf{F} | \sigma |] - \frac{1}{16\pi^2} \text{Tr}_{r_h} [\mathbf{F} * \mathbf{F} | \sigma - m |]. \quad (14.6.11)$$

The  $\sigma \mathbf{F} * \mathbf{F}$  term appearing above comes from the  $\mathcal{A}^3$  term in the prepotential. Recall (14.2.6) that from  $c/6 \mathcal{A}^3$ , one gets in the action

$$\frac{c}{6} \mathcal{A}^3 \rightarrow \frac{c}{2\pi^2} \text{Tr} \left[ \sigma \int F \wedge *F + (D\sigma) * (D\sigma) + \dots \right] + CS(5).$$

Also in passing from  $\mathbb{R}^5$  to  $S^5$ , (14.2.6) undergoes the change

$$\int \sqrt{g} d^6 x \text{Tr} [\sigma (D\sigma)^2] \rightarrow \int \sqrt{g} d^5 x \text{Tr} \left[ \sigma \left( D\sigma^2 + \frac{R}{12} \sigma^2 + \frac{1}{r^2} \sigma^2 \right) \right].$$

The role of  $R\sigma^2/12$  term is clear, it is there to make  $D\sigma^2$  term conformal invariant<sup>8</sup>. As for the last  $\sigma^3/r^2$  term, it comes from the  $D^2$  term in (14.2.11), by plugging in the expectation

<sup>8</sup>Under an infinitesimal conformal transform  $\delta g_{ij} = 2g_{ij}\phi$ , one has  $\delta\sigma = \sigma\phi(2-d)/3$  and  $\delta R = 2(1-d)\square\phi - 2\phi R$ .

value  $D_{IJ} = -2r^{-1}\sigma t_{IJ}$  in (14.2.1), one gets an extra  $\sigma^3/r^2$ . Now use  $R = 20/r^2$ , one gets the association

$$\sigma F \wedge *F \sim \frac{8}{3r^2}\sigma^3$$

Thus from the effective potential (14.6.11), one gets on  $S^5$  a potential term

$$\frac{1}{16\pi^2} \frac{8}{3r^2} \left( \sum_{\beta \in \text{root}} |\langle \sigma, \beta \rangle|^3 - \sum_{\mu \in \text{wght}} |\langle \sigma, \mu \rangle - m|^3 \right).$$

This matches perfectly with (14.6.6).

**Acknowledgements** We thank Tobias Ekholm, Johan Källén, Joseph Minahan, Anton Nedelin, Vasily Pestun, Luigi Tizzano and Jacob Winding for discussions and for the collaborations on this and related subjects. The research of J.Q. is supported in part by the Max-Planck Institute for Mathematics in Bonn. The research of M.Z. is supported in part by Vetenskapsrådet under grant #2014-5517, by the STINT grant and by the grant "Geometry and Physics" from the Knut and Alice Wallenberg foundation.

## 14.7 Appendix. Geometrical setting

### 14.7.1 Some basics of contact geometry

- **Contact structure.** A contact structure on a 5-manifold  $M$  is a smooth distribution of contact element  $\xi$ , which is a 4d subspace of the tangent space  $TM$ . This distribution is required to be non-integrable, and in this review  $\xi$  will be called the transverse or horizontal plane. If  $\xi$  is given by the kernel of a 1-form  $\kappa$ , then the non-integrability says that  $\kappa(d\kappa)^2 \neq 0$  everywhere. Note that this condition implies  $d\kappa$  is non-degenerate on  $\xi$ , and serves as an analogue of the symplectic structure. Also from the same condition one has a unique vector field  $R$  called the Reeb vector field such that

$$\iota_R \kappa = 1, \quad \iota_R d\kappa = 0. \tag{14.7.1}$$

One can split  $TM$  into vertical and horizontal components using the projector

$$P = 1 - R \otimes \kappa.$$

- **Contact metric structure.** In analogy with the symplectic case, one can construct purely algebraically an endomorphism  $J : \xi \rightarrow \xi$  and  $J^2 = -1$ . The triple  $(\xi, \kappa, J)$  is said to be a contact metric structure on  $M$  if  $J$  is compatible with  $d\kappa$  in the sense that  $1/2d\kappa J$  is a metric for  $\xi$ . We also extend  $J$  to an endomorphism of the entire  $TM$  by defining its action on  $R$  as zero  $JR = 0$ , leading to

$$J^2 = -P = -1 + R \otimes \kappa.$$

One can write down a metric of the tangent bundle as the direct sum of the one on  $\xi = \ker \kappa$  and the one along  $R$

$$g = \frac{1}{2}d\kappa J + \kappa \otimes \kappa . \quad (14.7.2)$$

As a consequence

$$\begin{aligned} g(JX, JY) &= g(X, Y) - \kappa(X)\kappa(Y) , \\ d\kappa &= -2gJ , \\ R &= g^{-1}\kappa . \end{aligned} \quad (14.7.3)$$

**Remark** As a note of the general convention of the review, we do not make any distinction of  $J$  when it serves as an endomorphism of  $TM$ , or of  $T^*M$  or a 2-form on  $M$ , all of which are related by raising or lower an appropriate index with the metric.

Let us fix the volume form of  $M$  as<sup>9</sup>

$$\text{vol} = \frac{1}{2}\kappa \wedge J \wedge J = \frac{1}{8}\kappa \wedge d\kappa \wedge d\kappa , \quad (14.7.4)$$

and one can define a duality operator for the horizontal 2-forms as

$$\omega \rightarrow *_R\omega = \iota_R * \omega , \quad \omega \in \Omega_H^2(M) . \quad (14.7.5)$$

The following relations are quite useful

$$\kappa \wedge *\omega = (-1)^{p-1} * \iota_R\omega , \quad \iota_R * \omega = (-1)^p * (\kappa\omega) , \quad \omega \in \Omega^p(M) . \quad (14.7.6)$$

• K-contact structure. If  $R$  is a Killing vector field with respect to  $g$  of (14.7.2), then  $(\kappa, R, J)$  gives a K-contact structure, the Killing condition is equivalent to

$$\nabla_X R = JX , \quad \forall X \in TM . \quad (14.7.7)$$

• Sasaki manifolds. From  $M$ , one can construct a manifold  $C(M)$  which is a cone over  $M$  with metric, symplectic and almost complex structures

$$\begin{aligned} C(M) &= \mathbb{R}^{>0} \times M , \\ \mathcal{G} &= dt^2 + t^2g , \\ \omega &= d(t^2\kappa) , \\ \mathcal{J} &= 2\omega^{-1}\mathcal{G} . \end{aligned} \quad (14.7.8)$$

A Sasaki manifold is a K-contact manifold such that  $(C(M), \mathcal{G}, \omega, \mathcal{J})$  is Kähler. The complex structure is written explicitly as

$$\mathcal{J} = J + t^{-1}R \otimes dt - t\partial_t \otimes \kappa ,$$

---

<sup>9</sup>We remind the reader that the choice of volume form in [25] is minus the current one.

it is easy to check  $\mathcal{J}^2 = -1_6$ . The vector field

$$\epsilon = t \frac{\partial}{\partial t} \quad (14.7.9)$$

generates a scaling along the  $t$ -direction and is called the *homothetic* vector field. It is clear that

$$\mathcal{J}(\epsilon) = R . \quad (14.7.10)$$

The Kähler condition is equivalent to the covariant constancy of  $\mathcal{J}$  with respect to the Levi-Civita connection. Thus a K-contact manifold is Sasaki iff  $J$  satisfies the integrability condition

$$\langle Z, (\nabla_X J)Y \rangle = -\kappa(Z)\langle X, Y \rangle + \langle Z, X \rangle \kappa(Y) , \quad (14.7.11)$$

where  $\langle -, - \rangle$  is the inner product using the metric

$$\langle A, B \rangle = A_{i_1 \dots i_p} B_{j_1 \dots j_p} g^{i_1 j_1} \dots g^{i_p j_p} . \quad (14.7.12)$$

From (14.7.11) one can derive a wealth of relations, some of which will be needed later. Define first some more projectors

$$(P_{\pm})_p^q = \frac{1}{2}(P \pm iJ)_p^q , \quad (14.7.13)$$

where  $P$  is the projection to the horizontal component of a vector or a form, with its indices written out  $P_s^r = \delta_s^r - R^r_{R_s}$ . The two projectors project to the horizontal (1,0) or (0,1) component with respect to the complex structure  $J$ . Keeping in mind the Kähler property of the cone  $C(M)$  will lead to the vanishing of (0,2) and (2,0) components of the curvature tensor, which translates in 5d as

$$\begin{aligned} R_{mnpq} - J_p^u J_q^v R_{mnuv} &= g_{p[m} g_{n]q} + J_{p[m} J_{n]q} , \\ R_{mnpq} R^p &= -g_{q[m} R_{n]} . \end{aligned} \quad (14.7.14)$$

The first equation says that

$$(P_-)_p^s (P_-)_q^t R_{mnst} = (P_-)_{pm} (P_-)_{qn} - (m \leftrightarrow n) , \quad (14.7.15)$$

i.e. the (0,2) component of the curvature, though not vanishing, can be written as something elementary.

It is useful to think of a Sasaki-manifold as an odd-dimensional analogue of a Kähler manifold. In fact, not only is the cone Kähler, there is also a Kähler structure transverse to the Reeb foliation (see [45] or section 7 of [22]). One can develop a transverse Dolbeault or even the appropriate Hodge theory. We define an operator

$$\bar{\partial}_H : \Omega_H^{p,q} \rightarrow \Omega_H^{p,q+1} , \quad \bar{\partial}_H = dx^r (P_-)_r^s \nabla_s + iq\kappa . \quad (14.7.16)$$

It is a differential that sends  $\Omega_H^{p,q} \rightarrow \Omega_H^{p,q+1}$ . It is a bit lengthy but straightforward to check the claimed properties of this operator, so we suppress the proof, but one needs to make use of equations (14.7.7) (14.7.11) and (14.7.14). It is also useful to transcribe the 6d Dolbeault operator in 5d language

$$\bar{\partial}^6 = \frac{1}{2}(t^{-1}dt - i\kappa)(L_\epsilon + iL_R) + (P_-)_{pq}dx^p dx^q \iota_\epsilon + \bar{\partial}_H . \quad (14.7.17)$$

• Sasaki-Einstein manifolds. If the cone metric is in addition Ricci-flat, i.e. the cone is Calabi-Yau, then  $M$  is said to be Sasaki-Einstein (SE), which is the central player in this review. The Ricci flatness of the cone is equivalent to 5d condition

$$R_{mn} = 4g_{mn} . \quad (14.7.18)$$

The CY property implies that there is a nowhere vanishing section of (3,0) forms on the cone, let us pick a harmonic representative  $\Omega$ , i.e.  $\bar{\partial}^6\Omega = 0$  (since the cone is neither compact nor smooth, one needs to construct the harmonic representative explicitly). From  $\Omega$  we define  $\varrho = \iota_\epsilon\Omega = -i\iota_R\Omega$ , the restriction of  $\varrho$  to the surface  $t = 1$ , i.e. to  $M$  will be a nowhere vanishing section of  $\Omega_H^{2,0}(M)$  already appearing in sec.14.4.2. From  $\bar{\partial}^6\Omega = 0$  and the relation (14.7.17)

$$0 = \bar{\partial}^6\Omega = \frac{i}{2}t^{-1}dt\kappa(L_{\epsilon-i_R}\varrho) - \frac{1}{2}(t^{-1}dt + i\kappa)\bar{\partial}_H\varrho .$$

Since  $L_{\epsilon-i_R}\varrho \in \Omega_H^{2,0}$  and  $\bar{\partial}_H\varrho \in \Omega_H^{2,1}$ , we have

$$L_{\epsilon-i_R}\varrho = 0 = \bar{\partial}_H\varrho .$$

From the last equation we also get

$$\nabla^\dagger\varrho = 0 .$$

## 14.7.2 Toric Sasaki manifolds

This section presents the construction of examples for the manifolds discussed in the previous subsection. To construct Sasaki-manifolds, it is easier to start from its Kähler cone, which can be obtained through Kähler reduction from a flat space.

Consider  $\mathbb{C}^4$  with the standard Kähler structure. Let  $\mathbf{e}_i$ ,  $i = 1, \dots, 4$  be four  $U(1)$ 's that rotate the phase of each  $\mathbb{C}$  factor. The  $U(1)$  actions are Hamiltonian with moment map

$$\vec{\mu} = \frac{1}{2}(|z_1|^2, \dots, |z_4|^2) .$$

Let  $U(1)_T = T^i\mathbf{e}_i$  be a particular combination of these  $U(1)$ 's, we can assume that  $T$  is primitive, i.e. the four components of  $T$  have greatest common divisor 1. The action of  $U(1)_T$  is has moment map

$$\mu_T = \vec{T} \cdot \vec{\mu} = \frac{1}{2} \sum_{i=1}^4 |z_i|^2 T^i ,$$

suppose that the four components of  $T$  are not all positive or negative, then  $\mu_T^{-1}(0)$  is non-trivial. Let

$$C(M) = \mu_T^{-1}(0)/U(1)_T$$

be the Kähler reduction of  $\mathbb{C}^4$ . Since  $\mu_T^{-1}(0)$  is invariant under the simultaneous scaling  $z_i \rightarrow \lambda z_i$ ,  $\lambda \in \mathbb{R}^\times$ , hence  $\mu_T^{-1}(0)$  and  $C(M)$  have the structure of a cone. Note that the action of  $U(1)_T$  on  $\mu_T^{-1}(0)$  is not free, so  $C(M)$  will always be singular.

From  $C(M)$ , we can get to  $M$  by imposing a constraint to fix the scaling freedom above, by intersecting the  $C_\mu(M)$  with a hyper-surface. We pick a 4-vector (not necessarily integer)  $\vec{\omega}$  and consider the surface

$$H_\omega = \{z_i \in \mathbb{C} \mid \sum_{i=1}^4 \omega_i |z_i|^2 = 1\} . \quad (14.7.19)$$

The  $U(1)_T$  action on the intersection  $H_\omega \cap \mu_T^{-1}(0)$  can be free if  $T, \omega$  are appropriately chosen. As an example, let  $T = [p + q, p - q, -p, -p]$ , with  $p > q > 1$  and  $\delta(p, q) = 1$ . Also choose  $\omega_i > 0$ ,  $i = 1, \dots, 4$ , then the intersection is topologically  $S^3 \times S^3$ . The loci where  $U(1)_T$  action is non-free is at  $z_1 = z_2 = 0$  or  $z_3 = z_4 = 0$ , both of which are excluded by the intersection. With a free action secured, the quotient

$$M = H_\omega \cap \mu_T^{-1}(0)/U(1)_T$$

is a smooth 5d manifold. In fact, the  $U(1)$  determined by  $\sum_{i=1}^4 \omega_i \mathbf{e}_i$  serves as the Reeb vector field on  $M$ .

We can give a more intrinsic description of  $C(M)$  and  $M$ . Out of the four  $U(1)$ 's acting on  $z_i$ , there will be only three independent  $U(1)$ 's left after the Kähler reduction, let us pick a basis  $e^a = 1, 2, 3$  for them. An explicit such basis can be chosen as follows. With our assumption on the primitiveness of  $T$ , we can find a  $4 \times 4$  matrix  $A \in SL(4, \mathbb{Z})$  with  $T$  as the last column, then the linear combinations

$$e_a = \sum_{i=1}^4 \mathbf{e}_i A_a^i, \quad a = 1, 2, 3$$

give a basis of the three  $U(1)$ 's acting on  $C(M)$ . Denote the Hamiltonian of the three  $U(1)$ 's as  $y_a$ ,  $a = 1, 2, 3$ . The  $y_a$  is an explicit parametrisation of the hyperplane  $\sum_i T^i |z_i|^2 = 0$ .

Write now

$$(A^{-1})_i^a = \left[ \begin{array}{cccc} \vec{v}_1 & \vec{v}_2 & \vec{v}_3 & \vec{v}_4 \\ \dots & \dots & \dots & \dots \end{array} \right]_{4 \times 4},$$

where  $\vec{v}_i$  are integer 3-vectors. On the hyperplane  $\sum_i T^i |z_i|^2 = 0$ , the  $|z_i|^2$  are solved as

$$0 \leq \frac{1}{2} |z_i|^2 = \sum_a y_a v_i^a . \quad (14.7.20)$$

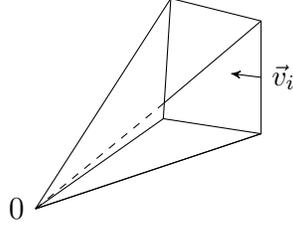

Figure 14.7.1: The moment map cone  $C_\mu(M)$

The inequalities (14.7.20) demarcates the domain of  $\{y_a\}$  as being a polytope cone. This cone actually contains almost all information about the geometry, so we give it a name  $C_\mu(M)$ . Referring to fig.14.7.1, the inward pointing normals are  $\vec{v}_i$ ,  $i = 1, \dots, 4$  (though the order may not be the same as how they appear in  $A^{-1}$ ). A good way to visualize the geometry of  $C(M)$  is that it is a torus fibration over  $C_\mu(M)$ . A generic fibre is  $U(1)^3$ , but the tori may degenerate at the boundaries of the cone. At the codim 1 faces, say face 1, the  $U(1)$  singled out by  $\vec{v}_1$ , i.e.  $\sum_a e_a v_i^a$  degenerates, while at the intersection of faces 1 and 2, two  $U(1)$ 's singled out by  $\vec{v}_{1,2}$  degenerate, etc.

To complete our translation of the geometry of  $M$  into that of  $C_\mu(M)$ , let  $\vec{R}$  be a 3-vector with components

$$R^a = \sum_{i=1}^4 v_i^a \omega_i . \quad (14.7.21)$$

The 3-vector  $\vec{R}$  gives a linear combination of  $U(1)$ 's:  $\sum_{a=1}^3 R^a e_a$ , this  $U(1)$  is the Reeb vector field on  $M$ , now written in purely 6d terms. Due to the correspondence (14.7.21), we will call both  $\vec{\omega}$ ,  $\vec{R}$  the Reeb vector (that they represent).

Furthermore the condition  $H_\omega$  of (14.7.19) translates to

$$\vec{R} \cdot \vec{y} = \frac{1}{2} .$$

The intersection of this hyper-plane with  $C_\mu(M)$  is a compact polygon iff  $\vec{R}$  is within the dual cone of the cone  $C_\mu(M)$ , i.e.  $\vec{R} = \sum_{i=1}^4 \lambda_i \vec{v}_i$ ,  $\lambda_i > 0$ . This compact polygon is the base of  $U(1)^3$  fibration, whose total space is the celebrated  $Y^{p,q}$  manifold [46]. We have also an easy generalisation

**Example** A close cousin of  $Y^{p,q}$  is obtained by taking  $T = [a, b, -c, -a - b + c]$  such that  $a, b, a + b - c > 0$ ,  $\delta(a, c) = \delta(a, d) = \delta(b, c) = \delta(b, d) = 1$ , known as the  $L^{a,b,c}$  space.

Then  $T$  can be completed into an  $SL(4, \mathbb{Z})$  matrix

$$A = \begin{bmatrix} 0 & m & 0 & a \\ 0 & 0 & 1 & b \\ 0 & n & 0 & -c \\ 1 & -m - n & -1 & -a - b + c \end{bmatrix} , \quad mc + na = 1 .$$

And its inverse is

$$A^{-1} = \begin{bmatrix} 1 & 1 & 1 & 1 \\ c & 0 & a & 0 \\ -bn & 1 & bm & 0 \\ n & 0 & -m & 0 \end{bmatrix},$$

and from the first three rows we read off the inward normals (in their right order)

$$\vec{v}_1 = [1, c, -bn], \quad \vec{v}_2 = [1, a, bm], \quad \vec{v}_3 = [1, 0, 1], \quad \vec{v}_4 = [1, 0, 0]. \quad (14.7.22)$$

These are two of the few SE manifolds, for which we know the explicit metric [46] [47].

The same story above can be repeated starting from  $\mathbb{C}^{n+3}$  and a Kähler reduction with respect to  $\mathfrak{n}$ -charges. But we stress that one does not have to take the route of the Kähler reduction, rather one may start from the more fundamental object  $C_\mu(M)$ . For example, one can postulate a polytope cone  $C \subset \mathbb{R}^n$ , with inward pointing normals  $\vec{v}_i$ ,  $i = 1 \cdots N$  (assumed to be primitive of course), then Lehman [48] showed that if at the intersection of  $k$  ( $k \leq n - 1$ ) faces, the  $k$  normals  $\vec{v}_1, \cdots, \vec{v}_k$  satisfy

$$\text{span}_{\mathbb{Z}} \langle \vec{v}_1, \cdots, \vec{v}_k \rangle = \text{span}_{\mathbb{R}} \langle \vec{v}_1, \cdots, \vec{v}_k \rangle \cap \mathbb{Z}^n,$$

then the cone gives rise to a smooth toric contact manifold. These conditions can be explicitly checked for the  $Y^{p,q}$ ,  $L^{a,b,c}$  cases above (the explicit normals and a more convenient criteria are given in [41]).

*Toric Sasaki-Einstein manifolds.* By definition if  $M$  is toric SE, then its metric cone is CY and then in the Kähler reduction construction of  $C(M)$  the charges of  $U(1)_T$  must sum to zero. This has a very simple implication when translated into the cone language: there exists a primitive  $\vec{\xi} \in \mathbb{Z}^3$  such that

$$\vec{\xi} \cdot \vec{v}_i = 1, \quad i = 1, \cdots, n \quad (14.7.23)$$

known as the 1-Gorenstein condition. The proof of this fact is not difficult and is left to the reader. Referring to the example above (14.7.22), all  $\vec{v}_i$  has its first component equal to 1, and so one chooses simply  $\vec{\xi} = [1, 0, 0]$ .

Since  $C(M)$  has flat canonical bundle, and if it is also simply connected, we will have a nowhere vanishing section  $\Omega$ , whose contraction with  $\epsilon$  gives the  $\varrho$  in the previous section.

*Deformations.*

So far we have given the Reeb vector field, but not quite the rest of the contact structures. Let us denote by  $\mathcal{J}_0$  the standard complex structure on  $\mathbb{C}^4$ , then it descends through the Kähler reduction to a complex structure on  $C(M)$ . Let also  $\epsilon$  be the homothetic vector that scales all  $z_i$ , it is easy to observe

$$\mathcal{J}_0(\epsilon) = \mathcal{J}_0 \sum_{i=1}^4 (z_i \partial_{z_i} + c.c) = i \sum_{i=1}^4 (z^i \partial_{z^i} - c.c) = \sum_{i=1}^4 \mathbf{e}_i.$$

Comparing this with (14.7.10), we have the Reeb  $\vec{\omega} = [1, 1, 1, 1]$ , or using (14.7.21)

$$\vec{R}_0 = \sum_{i=1}^4 \vec{v}_i ,$$

which is certainly within the dual cone. We call this the standard Reeb and the corresponding complex structure the standard complex structure. But to obtain general Reeb vector fields, one needs to deform  $\mathcal{J}$ , which can be done in a very transparent manner in the toric setting. As these deformations are reflected in the partition function, so using susy gauge theory as a means to study these geometries is an interesting enterprise.

Since we are interested in toric deformations, it is convenient to use  $y^i = |z_i|^2/2$ ,  $\theta_i = \arg z_i$  as coordinates of  $\mathbb{C}^{n+3}$ , we just take  $n = 1$  as an illustration. The material here is taken from the marvelous paper [49]. One can write a metric

$$\begin{aligned} \mathcal{G} &= G_{ij} dy^i dy^j + G^{ij} d\theta_i d\theta_j , \quad G_{ij} = \partial_{y^i} \partial_{y^j} G , \quad G^{ij} = G_{ij}^{-1} , \\ G &= \frac{1}{2} \sum_{i=1}^4 y^i \log y^i + \frac{1}{2} (\vec{\omega} \cdot \vec{y}) \log (\vec{\omega} \cdot \vec{y}) - \frac{1}{2} (\vec{\omega}_0 \cdot \vec{y}) \log (\vec{\omega}_0 \cdot \vec{y}) , \end{aligned}$$

where  $\vec{\omega}_0 = [1, 1, 1, 1]$ . Even though  $\mathcal{G}$  appear to have singularities at  $y^i = 0$ , they are only coordinate singularities, in fact, when  $y^1 \sim 0$

$$\mathcal{G} \sim \frac{1}{2} \frac{dy^1 dy^1}{y^1} + 2y^1 d\theta_1 d\theta_1 + \dots ,$$

and is perfectly smooth at  $y^1 = 0$  after reverting to Cartesian coordinates. We need not worry too much about the positivity of  $\mathcal{G}$ , as  $\mathcal{G}$  is certainly so when  $\omega = \omega_0$ , and thus there is an open neighbourhood round  $\omega = \omega_0$  in which positivity is secured.

The complex structure is

$$\mathcal{J} = -G_{ij} dy^i \otimes \partial_{\theta_j} + G^{ij} d\theta_i \otimes \partial_{y^j} . \quad (14.7.24)$$

To see that it is integrable, consider the (0,1)-forms  $d\theta_i + iG_{ij} dy^j$ , since  $d(d\theta_i + iG_{ij} dy^j) = iG_{ij,k} dy^k \wedge dy^j = 0$ , the distribution  $\cap_i \ker(d\theta_i + iG_{ij} dy^j)$  is integrable, and  $\mathcal{J}$  is integrable. In fact, if one works out explicitly the Levi-Civita connection, then  $\mathcal{J}$  is covariantly constant, i.e. we have a Kähler structure  $\mathbb{C}^4$ .

Since all structures here descend through the Kähler reduction, we have a deformed Kähler structure on the cone  $C(M)$ . In particular

$$J(\epsilon) = 2J(y^i \partial_i) = 2G_{ij} y^j \partial_{\theta_i} = \sum \omega^i \partial_{\theta_i} ,$$

comparing with (14.7.10), and using the correspondence (14.7.21) of two presentations of the Reeb before and after the Kähler reduction, one reaches the desired Reeb vector field.

So far we have held the symplectic structure of the cone fixed and deformed the complex structure, and hence the use of the symplectic coordinates  $y, \theta$ . In the subsequent discussion

of deformation of the symplectic structure (which we will not need in this paper, since the partition function only depends on the complex moduli), one must switch to the complex coordinates. From the explicit complex structure above, one can identify the (1,0)-forms

$$(1 + i\mathcal{J})d\theta_i = d\theta_i - iG_{ij}dy^j = d(\theta_i - iG_i) .$$

Thus we let the complex coordinates be

$$z_i = \exp(G_i + i\theta_i) .$$

For example letting  $R = R_0$  in (14.7.24), one can check that  $z_i$  is a constant multiple of the standard complex coordinates of  $\mathbb{C}^4$ .

With the explicit complex coordinates one can construct a harmonic representative of the holomorphic volume form  $\Omega$  from the Kähler reduction picture. Take  $\Omega_0 = dz_1 \wedge \cdots \wedge dz_4$ , which is smooth and is also invariant under (the complexified)  $U(1)_T$  action since the charges of  $U(1)_T$  sums to zero. Now let  $\Omega = \iota_T \Omega_0$ , where  $T_i$  are the vector fields induced by the  $U(1)_T$  action. Thus  $\Omega$  is a basic form with respect to  $U(1)_T$  and thus descends through the Kähler reduction and becomes the holomorphic volume form of  $C(M)$ . Moreover as  $\Omega_0$  is annihilated by  $\bar{\partial}$  and so will be  $\Omega$ , thus  $\Omega$  is a harmonic representative of  $H^{0,3}(C(M))$ . It is easily checked that  $\Omega$  scales under  $\epsilon$  with weight  $\sum_k \omega_k$ , subsequently has weight  $i \sum_k \omega_k$  under  $L_R$ . This is how one can obtain the weight of  $\varrho$  under  $L_R$ .

## References

- [1] V. Pestun and M. Zabzine, eds., *Localization techniques in quantum field theory*, vol. xx. Journal of Physics A, 2016. 1608.02952. <https://arxiv.org/src/1608.02952/anc/LocQFT.pdf>, <http://pestun.ihes.fr/pages/LocalizationReview/LocQFT.pdf>.
- [2] E. Witten, “Two-dimensional gauge theories revisited,” *J. Geom. Phys.* **9** (1992) 303–368, [arXiv:hep-th/9204083](https://arxiv.org/abs/hep-th/9204083) [hep-th].
- [3] C. Beasley and E. Witten, “Non-Abelian localization for Chern-Simons theory,” *J. Diff. Geom.* **70** (2005) no. 2, 183–323, [arXiv:hep-th/0503126](https://arxiv.org/abs/hep-th/0503126) [hep-th].
- [4] A. Kapustin, B. Willett, and I. Yaakov, “Exact Results for Wilson Loops in Superconformal Chern-Simons Theories with Matter,” *JHEP* **03** (2010) 089, [arXiv:0909.4559](https://arxiv.org/abs/0909.4559) [hep-th].
- [5] V. Pestun, “Localization of gauge theory on a four-sphere and supersymmetric Wilson loops,” *Commun.Math.Phys.* **313** (2012) 71–129, [arXiv:0712.2824](https://arxiv.org/abs/0712.2824) [hep-th].
- [6] J. Kallen, “Cohomological localization of Chern-Simons theory,” *JHEP* **08** (2011) 008, [arXiv:1104.5353](https://arxiv.org/abs/1104.5353) [hep-th].
- [7] J. Källén and M. Zabzine, “Twisted supersymmetric 5D Yang-Mills theory and contact geometry,” *JHEP* **1205** (2012) 125, [arXiv:1202.1956](https://arxiv.org/abs/1202.1956) [hep-th].
- [8] J. Duistermaat and G. Heckman, “On the Variation in the Cohomology of the Symplectic Form of the Reduced Phase Space.,” *Inventiones mathematicae* **69** (1982) 259–268. <http://eudml.org/doc/142953>.
- [9] E. Witten, “Supersymmetry and Morse theory,” *Journal of Differential Geometry* **17** (1982) no. 4, 661–692. <http://projecteuclid.org/euclid.jdg/1214437492>.

- [10] J. Minahan, “Matrix models for 5D super Yang-Mills,” *Journal of Physics A* **xx** (2016) 000, [1608.02967](#).
- [11] S. Pasquetti, “Holomorphic blocks and the 5d AGT correspondence,” *Journal of Physics A* **xx** (2016) 000, [1608.02968](#).
- [12] N. Seiberg, “Five-dimensional SUSY field theories, nontrivial fixed points and string dynamics,” *Phys. Lett.* **B388** (1996) 753–760, [arXiv:hep-th/9608111](#) [[hep-th](#)].
- [13] H.-C. Kim, S.-S. Kim, and K. Lee, “5-dim Superconformal Index with Enhanced En Global Symmetry,” *JHEP* **1210** (2012) 142, [arXiv:1206.6781](#) [[hep-th](#)].
- [14] K. Hosomichi, R.-K. Seong, and S. Terashima, “Supersymmetric Gauge Theories on the Five-Sphere,” *Nucl.Phys.* **B865** (2012) 376–396, [arXiv:1203.0371](#) [[hep-th](#)].
- [15] G. Festuccia and N. Seiberg, “Rigid Supersymmetric Theories in Curved Superspace,” *JHEP* **1106** (2011) 114, [arXiv:1105.0689](#) [[hep-th](#)].
- [16] T. T. Dumitrescu, G. Festuccia, and N. Seiberg, “Exploring Curved Superspace,” *JHEP* **1208** (2012) 141, [arXiv:1205.1115](#) [[hep-th](#)].
- [17] T. T. Dumitrescu and G. Festuccia, “Exploring Curved Superspace (II),” *JHEP* **1301** (2013) 072, [arXiv:1209.5408](#) [[hep-th](#)].
- [18] C. Closset, T. T. Dumitrescu, G. Festuccia, and Z. Komargodski, “Supersymmetric Field Theories on Three-Manifolds,” *JHEP* **1305** (2013) 017, [arXiv:1212.3388](#) [[hep-th](#)].
- [19] Y. Pan, “Rigid Supersymmetry on 5-dimensional Riemannian Manifolds and Contact Geometry,” [arXiv:1308.1567](#) [[hep-th](#)].
- [20] T. Friedrich and I. Kath, “Einstein Manifolds of Dimension Five with Small First Eigenvalue of the Dirac Operator,” *J. Differential Geometry* **29** (1989) 263–279.
- [21] J. Qiu and M. Zabzine, “5D Super Yang-Mills on  $Y^{p,q}$  Sasaki-Einstein manifolds,” *Commun. Math. Phys.* **333** (2015) no. 2, 861–904, [arXiv:1307.3149](#) [[hep-th](#)].
- [22] C. P. Boyer and K. Galicki, *Sasakian geometry*. Oxford Mathematical Monographs. Oxford University Press, Oxford, 2008.
- [23] J. Schmude, “Localisation on Sasaki-Einstein manifolds from holomorphic functions on the cone,” [arXiv:1401.3266](#) [[hep-th](#)].
- [24] A. Alekseev, “Notes on Equivariant Localization,” in *Geometry and Quantum Physics*, H. Gausterer, L. Pittner, and H. Grosse, eds., vol. 543 of *Lecture Notes in Physics*, pp. 1–24. Springer Berlin Heidelberg, 2000. [http://dx.doi.org/10.1007/3-540-46552-9\\_1](http://dx.doi.org/10.1007/3-540-46552-9_1).
- [25] J. Källén, J. Qiu, and M. Zabzine, “The perturbative partition function of supersymmetric 5D Yang-Mills theory with matter on the five-sphere,” *JHEP* **1208** (2012) 157, [arXiv:1206.6008](#) [[hep-th](#)].
- [26] J. M. Figueroa-O’Farrill, “On the supersymmetries of Anti-de Sitter vacua,” *Class.Quant.Grav.* **16** (1999) 2043–2055, [arXiv:hep-th/9902066](#) [[hep-th](#)].
- [27] D. Salamon, *Spin geometry and Seiberg-Witten invariants*. 1996.
- [28] N. Hama, K. Hosomichi, and S. Lee, “SUSY Gauge Theories on Squashed Three-Spheres,” *JHEP* **1105** (2011) 014, [arXiv:1102.4716](#) [[hep-th](#)].
- [29] Y. Imamura and D. Yokoyama, “N=2 supersymmetric theories on squashed three-sphere,” *Phys.Rev.* **D85** (2012) 025015, [arXiv:1109.4734](#) [[hep-th](#)].
- [30] Y. Imamura, “Supersymmetric theories on squashed five-sphere,” [arXiv:1209.0561](#) [[hep-th](#)].

- [31] Y. Imamura, “Perturbative partition function for squashed  $S^5$ ,” [arXiv:1210.6308 \[hep-th\]](#).
- [32] M. Wolf, “Contact Manifolds, Contact Instantons, and Twistor Geometry,” *JHEP* **1207** (2012) 074, [arXiv:1203.3423 \[hep-th\]](#).
- [33] D. Baraglia and P. Hekmati, “Moduli Spaces of Contact Instantons,” [arXiv:1401.5140 \[math.DG\]](#).
- [34] Y. Pan, “Note on a Cohomological Theory of Contact-Instanton and Invariants of Contact Structures,” [arXiv:1401.5733 \[hep-th\]](#).
- [35] J. Qiu and M. Zabzine, “On twisted N=2 5D super Yang-Mills theory,” *Lett. Math. Phys.* **106** (2016) no. 1, 1–27, [arXiv:1409.1058 \[hep-th\]](#).
- [36] A. Haydys, “Fukaya-Seidel category and gauge theory,” *ArXiv e-prints* (2010) , [arXiv:1010.2353](#).
- [37] E. Witten, “Fivebranes and Knots,” [arXiv:1101.3216 \[hep-th\]](#).
- [38] S. A. Cherkis, “Octonions, Monopoles, and Knots,” [arXiv:1403.6836 \[hep-th\]](#).
- [39] J. J. Kohn and H. Rossi, “On the Extension of Holomorphic Functions from the Boundary of a Complex Manifold,” *Annals of Mathematics* **81** (1965) no. 2, pp. 451–472. <http://www.jstor.org/stable/1970624>.
- [40] M. F. Atiyah, *Elliptic operators and compact groups*, vol. 401. Springer-Verlag, Berlin, 1974.
- [41] J. Qiu, L. Tizzano, J. Winding, and M. Zabzine, “Gluing Nekrasov partition functions,” *Commun. Math. Phys.* **337** (2015) no. 2, 785–816, [arXiv:1403.2945 \[hep-th\]](#).
- [42] A. Narukawa, “The modular properties and the integral representations of the multiple elliptic gamma functions,” *Adv. Math.* **189** (2004) no. 2, 247–267. <http://dx.doi.org/10.1016/j.aim.2003.11.009>.
- [43] L. Tizzano and J. Winding, “Multiple sine, multiple elliptic gamma functions and rational cones,” *ArXiv e-prints* (2015) , [arXiv:1502.05996](#).
- [44] M. E. Peskin and D. V. Schroeder, *An Introduction To Quantum Field Theory*. Frontiers in Physics. Westview Press; First Edition, 1995.
- [45] J. Sparks, “Sasaki-Einstein Manifolds,” *ArXiv e-prints* (2010) , [arXiv:1004.2461](#).
- [46] J. P. Gauntlett, D. Martelli, J. Sparks, and D. Waldram, “Sasaki-Einstein metrics on  $S^2 \times S^3$ ,” *Adv.Theor.Math.Phys.* **8** (2004) 711–734, [arXiv:hep-th/0403002 \[hep-th\]](#).
- [47] M. Cvetic, H. Lu, D. N. Page, and C. Pope, “New Einstein-Sasaki spaces in five and higher dimensions,” *Phys.Rev.Lett.* **95** (2005) 071101, [arXiv:hep-th/0504225 \[hep-th\]](#).
- [48] E. Lerman, “Contact toric manifolds,” *J. Symplectic Geom.* **1** (2002) no. 4, 659–828, [arXiv:math/0107201 \[math\]](#). <http://projecteuclid.org/getRecord?id=euclid.jsg/1092749569>.
- [49] D. Martelli, J. Sparks, and S.-T. Yau, “The Geometric dual of a-maximisation for Toric Sasaki-Einstein manifolds,” *Commun.Math.Phys.* **268** (2006) 39–65, [arXiv:hep-th/0503183 \[hep-th\]](#).

# Chapter 15

## Matrix models for 5d super Yang-Mills

Joseph A. Minahan

*Department of Physics and Astronomy, Uppsala university,  
Box 516, SE-75120 Uppsala, Sweden  
joseph.minahan@physics.uu.se*

### Abstract

In this contribution to the review on localization in gauge theories we investigate the matrix models derived from localizing  $\mathcal{N} = 1$  super Yang-Mills on  $S^5$ . We consider the large- $N$  limit and attempt to solve the matrix model by a saddle-point approximation. In general it is not possible to find an analytic solution, but at the weak and the strong limits of the 't Hooft coupling there are dramatic simplifications that allows us to extract most of the interesting information. At weak coupling we show that the matrix model is close to the Gaussian matrix model and that the free-energy scales as  $N^2$ . At strong coupling we show that if the theory contains one adjoint hypermultiplet then the free-energy scales as  $N^3$ . We also find the expectation value of a supersymmetric Wilson loop that wraps the equator. We demonstrate how to extract the effective couplings and reproduce results of Seiberg. Finally, we compare to results for the six-dimensional  $(2, 0)$  theory derived using the AdS/CFT correspondence. We show that by choosing the hypermultiplet mass such that the supersymmetry is enhanced to  $\mathcal{N} = 2$ , the Wilson loop result matches the analogous calculation using AdS/CFT. The free-energies differ by a rational fraction.

### Contents

|                                                                                               |            |
|-----------------------------------------------------------------------------------------------|------------|
| <b>15.1 Introduction</b> . . . . .                                                            | <b>601</b> |
| <b>15.2 Matrix model for <math>\mathcal{N} = 1</math> 5d Yang-Mills with matter</b> . . . . . | <b>602</b> |
| <b>15.3 <math>\mathcal{N} = 1^*</math> 5d super Yang-Mills</b> . . . . .                      | <b>606</b> |

|                                                |            |
|------------------------------------------------|------------|
| <b>15.4 Supergravity comparisons</b> . . . . . | <b>609</b> |
| <b>15.5 Discussion</b> . . . . .               | <b>611</b> |
| <b>References</b> . . . . .                    | <b>612</b> |

## 15.1 Introduction

In this installment of the review on localization we analyze the matrix models that result from localizing five-dimensional  $\mathcal{N} = 1$  super Yang-Mills on a five-sphere of radius  $r$ . In five dimensions the supermultiplets have one vector multiplet and some hypermultiplets. In this generic case there are a total of eight supersymmetries. The most interesting case for us is when there is one hypermultiplet in the adjoint representation with a particular mass,  $M$ . We will refer to such theories as  $\mathcal{N} = 1^*$  theories. When  $M = i/(2r)$  the supersymmetry is enhanced to  $\mathcal{N} = 2$ , with 16 total supersymmetries. This is the maximal amount of supersymmetry in five dimensions (without gravity), so we will refer to this as maximally supersymmetric Yang-Mills (MSYM).

The reason that the  $\mathcal{N} = 2$  enhancement is interesting is that the mysterious six-dimensional  $(2, 0)$  superconformal field theory when compactified on a circle reduces to MSYM, with the radius related to the Yang-Mills coupling by

$$R_6 = \frac{g_{YM}^2}{8\pi^2}. \tag{15.1.1}$$

This relation follows from identifying the Kaluza-Klein modes of the  $(2, 0)$  theory with the instanton particles in the 5d MSYM [2]. These  $(2, 0)$  theories are difficult to study because they have no free parameters and no Lagrangian description, and thus no perturbative prescription. However, they do have an  $AdS_7 \times S^4$  dual, so certain strong coupling data can be extracted using supergravity. The hope then is that one can use the localization results from the MSYM to say something about the  $(2, 0)$  theory. For example, one can now say much about the supersymmetric indices of the  $(2, 0)$  theories using MSYM (see Chapter 17).

One thing to keep in mind about this discussion is that the MSYM is non-renormalizable and hence requires a UV completion. The  $(2, 0)$  theory on the circle is believed to be a consistent UV completion <sup>1</sup>. The observables we compute using localization are however finite because of the supersymmetry and would be expected to match with the same observables in the UV complete theory.

Localization results in a complicated matrix model that is not analytically solvable in general. However, we will show that in the large- $N$  limit at strong coupling the analysis of the matrix model simplifies dramatically. One of the main results is that free-energy scales as  $N^3$  [9, 10] with a coefficient that depends on  $M$  [10]. The supergravity analysis of the  $(2, 0)$

---

<sup>1</sup>It had been proposed that MSYM could be used to actually define the  $(2, 0)$  theories [4–6], and while not renormalizable, might actually be finite [4]. However, an explicit calculation shows that the four-point amplitude is UV divergent at six loops [7] and hence requires a UV completion. For a possible way around this see [8].

theory also exhibits  $N^3$  behavior for the free-energy [11, 12], suggesting that the degrees of freedom are more than for a weakly coupled gauge theory, where one finds  $N^2$  scaling in the free-energy. However, at the MSYM point, the coefficient in front of the  $N^3$  term differs by a factor of 4/5 with the  $N^3$  term in the supergravity calculation. This remains an unresolved problem.

Nevertheless one can study another supersymmetric observable, the expectation value of a Wilson loop along the equator. Here one finds a match at the MSYM point with a parallel computation done using supergravity [13].

The rest of the paper is organized as follows. In section 15.2 we give some details of the matrix model resulting from localization of 5d SYM and study limits at large volume or large hypermultiplet mass, reproducing results in [14, 15] for the effective couplings. In section 15.3 we consider the large  $N$  behavior of the  $\mathcal{N} = 1^*$  theories. We calculate the free energy and the expectation value of a supersymmetric Wilson loop in the weak and strong coupling limits. We also generalize these results to  $\mathbb{Z}_k$  quiver theories. In section 15.4 we compute the free energy and the Wilson loop expectation value starting from the supergravity dual of the (2, 0) theory on  $S^5 \times R$ , and then compactifying the  $R$  to an  $S^1$  and identifying the radius as in (15.1.1). We show that there is a mismatch with the free-energy result from section 15.3 by a factor of 4/5, but the Wilson loop results agree. In section 15.5 we give a brief summary discuss some open problems.

## 15.2 Matrix model for $\mathcal{N} = 1$ 5d Yang-Mills with matter

The perturbative partition function was derived in [16] for massless hypermultiplets and in [17] for MSYM. Its derivation is given in Chapter 14. In this section we show how the results of the effective couplings in [14, 15] can be extracted from the resulting matrix model.

We consider a theory with a semi-simple compact gauge group  $G$ . This has an  $\mathcal{N} = 1$  vector multiplet and  $\mathcal{N} = 1$  massless hypermultiplets in representation  $R_i$  with splittings into half-multiplets when  $R_i$  is complex. The partition function of this gauge theory on  $S^5$  is then given by

$$Z = \int_{\text{Cartan}} [d\phi] e^{-\frac{8\pi^3 r}{g_{YM}^2} \text{Tr}(\phi^2) - \frac{\pi k}{3} \text{Tr}(\phi^3)} Z_{1\text{-loop}}^{\text{vect}}(\phi) \prod_i Z_{1\text{-loop}}^i(\phi) + \mathcal{O}(e^{-\frac{16\pi^3 r}{g_{YM}^2}}), \quad (15.2.1)$$

where the one-loop contributions are given by the infinite products

$$Z_{1\text{-loop}}^{\text{vect}}(\phi) = \prod_{\beta} \prod_{t \neq 0} (t - \langle \beta, i\phi \rangle)^{(1 + \frac{3}{2}t + \frac{1}{2}t^2)}, \quad (15.2.2)$$

and

$$Z_{1\text{-loop}}^i(\phi) = \prod_{\mu \in R_i} \prod_t \left( t - \langle i\phi, \mu \rangle + \frac{3}{2} \right)^{-(1 + \frac{3}{2}t + \frac{1}{2}t^2)}, \quad (15.2.3)$$

with  $\beta$  the roots and  $\mu$  the weights in  $R_i$ .

The path integral in (15.2.1) has a contribution from a Chern-Simons term with level  $k$ . We have also absorbed the radius  $r$  into the integration variable  $\phi = -ir\sigma$ . As in the 4D case [19], we must Wick rotate and integrate over real  $\phi$  in order to have a well-defined path integral.

The infinite products that appear in (15.2.2) and (15.2.3) are divergent and need to be regularized. Each one-loop contribution has the form

$$\mathcal{P} = x \prod_{t=1}^{\infty} (t+x)^{(1+\frac{3}{2}t+\frac{1}{2}t^2)} (t-x)^{(1-\frac{3}{2}t+\frac{1}{2}t^2)}, \quad (15.2.4)$$

whose log can be written as

$$\log \mathcal{P} = \sum_{t=1}^{\infty} \left( 3x - \frac{x^2}{2} \right) + \text{convergent part}. \quad (15.2.5)$$

Therefore, the infinite product can be regulated by replacing it with the triple sine function [20]

$$S_3(x) = 2\pi e^{-\zeta'(-2)} x e^{\frac{x^2}{4} - \frac{3}{2}x} \prod_{t=1}^{\infty} \left( \left( 1 + \frac{x}{t} \right)^{(1+\frac{3}{2}t+\frac{1}{2}t^2)} \left( 1 - \frac{x}{t} \right)^{(1-\frac{3}{2}t+\frac{1}{2}t^2)} e^{\frac{x^2}{2} - 3x} \right), \quad (15.2.6)$$

As an alternative we can regularize the divergence by introducing a UV cut-off that stops the mode expansion at  $n_0 = \pi\lambda r$ , and leaving the log of the one-loop determinants to be

$$\begin{aligned} \log(Z_{1\text{-loop}}^{\text{vect}}(\phi) \prod_i Z_{1\text{-loop}}^i(\phi)) &= -\frac{\pi\lambda r}{2} \sum_{\beta} (\langle \beta, i\phi \rangle)^2 + \frac{\pi\lambda r}{2} \sum_{\mu \in R_i} (\langle i\phi, \mu \rangle)^2 + \text{convergent part} \\ &= \pi\lambda r \left( C_2(\text{adj}) - \sum_i C_2(R_i) \right) \text{Tr}(\phi^2) + \text{convergent part}, \end{aligned} \quad (15.2.7)$$

where  $\text{Tr}(T_A T_B) = C_2(R)\delta_{AB}$  and  $\sum_{\mu \in R_i} (\langle \phi, \mu \rangle)^2 = 2C_2(R_i) \text{Tr}(\phi^2)$ . The linear piece cancels since the gauge group is semi-simple. Hence, the divergent piece is proportional to  $\text{Tr}(\phi^2)$  and can be absorbed into an effective coupling given by

$$\frac{1}{g_{eff}^2} = \frac{1}{g_{YM}^2} - \frac{\lambda}{8\pi^2} \left( C_2(\text{adj}) - \sum_i C_2(R_i) \right). \quad (15.2.8)$$

This renormalization of the coupling agrees with the flat space results in [21, 22].

The convergent part of (15.2.4) can be replaced by  $S_3(x)e^{-\frac{x^2}{4}+\frac{3}{2}x}$  up to  $x$ -independent (and hence irrelevant) constants. The extra exponential factor leads to a further finite shift in the coupling constant. Notice that the UV divergence cancels if there is only one hypermultiplet and it sits in the adjoint representation.

Using the regularized determinants, we can rewrite the matrix model in terms of triple sine functions  $S_3(x)$

$$Z = \int d\phi e^{-\frac{8\pi^3 r}{9} \text{Tr}(\phi^2) - \frac{\pi k}{3} \text{Tr}(\phi^3)} \det_{Ad} \left( S_3(i\phi) \right) \prod_i \det_{R_i}^{-1} \left( S_3 \left( i\phi + \frac{3}{2} \right) \right), \quad (15.2.9)$$

where from now on we assume that  $g_{YM}$  is the renormalized coupling. The triple sine function  $S_3(x)$  has the symmetry property

$$S_3(-x) = S_3(x+3), \quad S_3\left(x + \frac{3}{2}\right) = S_3\left(-x + \frac{3}{2}\right). \quad (15.2.10)$$

The weights are mapped from  $\mu$  to  $-\mu$  when exchanging representation  $R$  with  $\bar{R}$ . Hence, the one-loop contribution of a massless hypermultiplet has the property

$$\det_R\left(S_3\left(i\phi + \frac{3}{2}\right)\right) = \det_R\left(S_3\left(-i\phi + \frac{3}{2}\right)\right) = \det_{\bar{R}}\left(S_3\left(i\phi + \frac{3}{2}\right)\right). \quad (15.2.11)$$

and the representations  $R$  and  $\bar{R}$  are automatically symmetrized in the determinants.

Hypermultiplet masses can be turned on by using an auxiliary  $U(1)$  vector multiplet. One takes a  $G \times U(1)$  matrix model, but excludes the integration over the  $U(1)$  direction. Thus the contribution of massive hypermultiplets is given by

$$Z = \int d\phi e^{-\frac{8\pi^3 r}{g_{YM}^2} \text{Tr}(\phi^2) - \frac{\pi k}{3} \text{Tr}(\phi^3)} \det_{Ad}\left(S_3(i\phi)\right) \prod_i \det_{R_i}^{-1}\left(S_3\left(i\phi + im_i + \frac{3}{2}\right)\right), \quad (15.2.12)$$

where  $m_i$  are dimensionless parameters related to the actual hypermultiplet masses by  $m_i = rM_i$ . Using the triple sine's symmetry we find the relation

$$\det_{R_i}\left(S_3\left(i\phi + im_i + \frac{3}{2}\right)\right) = \det_{\bar{R}_i}\left(S_3\left(i\phi - im_i + \frac{3}{2}\right)\right). \quad (15.2.13)$$

Hence, the partition function with massive hypermultiplets can be written as

$$\begin{aligned} & \int d\phi e^{-\frac{8\pi^3 r}{g_{YM}^2} \text{Tr}(\phi^2) - \frac{\pi k}{3} \text{Tr}(\phi^3)} \det_{Ad}\left(S_3(i\phi)\right) \\ & \times \prod_i \det_{R_i}^{-1/2}\left(S_3\left(i\phi + im_i + \frac{3}{2}\right)\right) \det_{\bar{R}_i}^{-1/2}\left(S_3\left(i\phi - im_i + \frac{3}{2}\right)\right) \end{aligned} \quad (15.2.14)$$

Let us consider (15.2.14) in the large volume limit by taking  $r \rightarrow \infty$ . We can write (15.2.14) in the form

$$\int d\phi e^{-\mathcal{F}}, \quad (15.2.15)$$

where

$$\mathcal{F} = \frac{8\pi^3 r}{g_{YM}^2} \text{Tr}(\phi^2) + \frac{\pi k}{3} \text{Tr}(\phi^3) - \sum_{\beta} \log S_3(\langle i\phi, \beta \rangle) + \sum_i \sum_{\mu_i} \log S_3\left(\langle i\phi, \mu_i \rangle + im_i + \frac{3}{2}\right).$$

We then restore the  $r$  dependence by the rescaling  $\phi \rightarrow r\phi$  and  $m \rightarrow rm$ . Using the asymptotic expansion for  $|\text{Im}z| \rightarrow \infty$  and  $0 \leq \text{Re}z < 3$

$$\log S_3(z) \sim -\text{sgn}(\text{Im}z)\pi i \left(\frac{1}{6}z^3 - \frac{3}{4}z^2 + z + \dots\right), \quad (15.2.16)$$

we obtain the expression

$$\frac{1}{2\pi r^3} \mathcal{F} = \frac{4\pi^2}{g_{YM}^2} \text{Tr}(\phi^2) + \frac{k}{6} \text{Tr}(\phi^3) + \frac{1}{12} \left( \sum_{\beta} |\langle \phi, \beta \rangle|^3 - \sum_i \sum_{\mu_i} |\langle \phi, \mu_i \rangle + m_i|^3 \right) + O(r^{-2}). \quad (15.2.17)$$

Up to a constant which we have absorbed into the definition of the coupling, (15.2.17) matches the quantum prepotential in the flat-space limit [15]. The normalization of the quadratic term is fixed either by a direct one-loop calculation in flat space [22] or by matching the superpotential in 5d with the corresponding one in 4D [21].

The matrix model is well-defined if  $\mathcal{F}$  is a convex positive function in the large  $\phi$  limit. In this limit  $\mathcal{F}$  takes the asymptotic form

$$\begin{aligned} \mathcal{F} = & \frac{8\pi^3 r}{g_{YM}^2} \text{Tr}(\phi^2) + \frac{\pi k}{3} \text{Tr}(\phi^3) + \frac{\pi}{6} \left( \sum_{\beta} |\langle \phi, \beta \rangle|^3 - \sum_i \sum_{\mu_i} |\langle \phi, \mu_i \rangle|^3 \right) \\ & - \pi \sum_{\beta} |\langle \phi, \beta \rangle| - \frac{\pi}{2} \sum_i \sum_{\mu_i} \left( m_i \text{sgn}(\langle \phi, \mu_i \rangle) (\langle \phi, \mu_i \rangle)^2 + (m_i^2 + \frac{1}{4}) |\langle \phi, \mu_i \rangle| \right) + \dots, \end{aligned} \quad (15.2.18)$$

where the ellipsis stands for terms suppressed at large  $\phi$ . Analyzing the convexity of (15.2.18) it is clear that the cubic terms dominate. Hence, the analysis is identical to that in [15] and the same conditions apply. In special cases the cubic terms cancel each other, for example in the case of single adjoint hypermultiplet [10] or for the superconformal  $USp(2N)$  theory described in [23].

Suppose we now take the hypermultiplet masses to infinity. For large  $|m_i|$  the leading terms in (15.2.16) are

$$\begin{aligned} \mathcal{F} = & \frac{8\pi^3 r}{g_{YM}^2} \text{Tr}(\phi^2) + \frac{\pi k}{3} \text{Tr}(\phi^3) - \sum_{\beta} \log S_3(\langle i\phi, \beta \rangle) \\ & - \sum_i \text{sgn}(m_i) \frac{\pi}{2} \sum_{\mu_i} \left( \frac{1}{3} (\langle \phi, \mu_i \rangle)^3 + m (\langle \phi, \mu_i \rangle)^2 \right). \end{aligned}$$

The two last terms in (15.2.19) can be absorbed by a redefinition of  $k$  and  $g_{YM}$ . To see this, note that

$$\text{Tr}(T_A T_B T_C + T_A T_C T_B) = C_3(\mathbb{R}) d_{ABC}, \quad (15.2.19)$$

where

$$\sum_{\mu} (\langle \phi, \mu \rangle)^3 = C_3(\mathbb{R}) \text{Tr}(\phi^3). \quad (15.2.20)$$

The coefficient  $C_3$  satisfies  $C_3(\bar{\mathbb{R}}) = -C_3(\mathbb{R})$ , hence it is zero for real representations. For the lower complex representations in  $SU(N)$  it is 1 for the fundamental,  $N - 4$  for the antisymmetric, and  $N + 4$  for the symmetric representations. Hence, from (15.2.19) and (15.2.20) we get

$$k_{eff} = k - \sum_i \text{sgn}(m_i) \frac{C_3(\mathbb{R}_i)}{2}, \quad (15.2.21)$$

the same result in [14, 15]. A similar analysis of the quadratic terms gives

$$\frac{r}{g_{eff}^2} = \frac{r}{g_{YM}^2} - \sum_i \frac{|m_i|}{8\pi^2} C_2(R_i). \quad (15.2.22)$$

### 15.3 $\mathcal{N} = 1^*$ 5d super Yang-Mills

We now turn to  $\mathcal{N} = 1^*$  super Yang-Mills, where there is a single adjoint hypermultiplet with mass parameter  $m$ . We further assume that the gauge group is  $SU(N)$ .

To analyze the resulting matrix model (15.2.14) we rewrite the triple sine function  $S_3(z)$  in (15.2.6) as

$$S_3(z) = 2e^{-\zeta'(-2)} \sin(\pi z) e^{\frac{1}{2}f(z)} e^{\frac{3}{2}l(z)}, \quad (15.3.1)$$

where  $l(z)$  and  $f(z)$  are given by [24, 25]

$$l(z) = -z \log(1 - e^{2\pi iz}) + \frac{i}{2} \left( \pi z^2 + \frac{1}{\pi} \text{Li}_2(e^{2\pi iz}) \right) - \frac{i\pi}{12} \quad (15.3.2)$$

$$f(z) = \frac{i\pi z^3}{3} + z^2 \log(1 - e^{-2\pi iz}) + \frac{iz}{\pi} \text{Li}_2(e^{-2\pi iz}) + \frac{1}{2\pi^2} \text{Li}_3(e^{-2\pi iz}) - \frac{\zeta(3)}{2\pi^2} \quad (15.3.3)$$

While these functions are rather ugly, their derivatives have the much nicer form

$$\frac{df(z)}{dz} = \pi z^2 \cot(\pi z); \quad \frac{dl(z)}{dz} = -\pi z \cot(\pi z); \quad (15.3.4)$$

The matrix model path integral (15.2.14) can then be rewritten as

$$Z = \int_{\text{Cartan}} [d\phi] e^{-\frac{8\pi^3 r}{g_{YM}^2} \text{Tr}(\phi^2)} \prod_{\beta} (\sin(\pi \langle \beta, i\phi \rangle) e^{-\frac{1}{4}l(\frac{1}{2}-im-\langle \beta, i\phi \rangle) - \frac{1}{4}l(\frac{1}{2}-im+\langle \beta, i\phi \rangle)} \\ \times e^{\frac{1}{2}f(\langle \beta, i\phi \rangle) - \frac{1}{4}f(\frac{1}{2}-im-\langle \beta, i\phi \rangle) - \frac{1}{4}f(\frac{1}{2}-im+\langle \beta, i\phi \rangle)} + \dots) \quad (15.3.5)$$

up to instanton terms, where we have dropped the Chern-Simons term. From now on we assume that the gauge group is  $U(N)$ . Defining the t' Hooft coupling constant to be

$$\lambda = \frac{g_{YM}^2 N}{r},$$

and taking the large  $N$  limit for fixed  $\lambda$ , all instanton contributions are suppressed. We can then re-express (15.3.5) as the integral over the eigenvalues  $\phi_i$

$$Z \sim \int \prod_{i=1}^N d\phi_i \exp \left( -\frac{8\pi^3 N}{\lambda} \sum_i \phi_i^2 + \sum_{j \neq i} \sum_i \left[ \log [\sinh(\pi(\phi_i - \phi_j))] \right. \right. \\ \left. \left. - \frac{1}{4}l\left(\frac{1}{2} - im + i(\phi_i - \phi_j)\right) - \frac{1}{4}l\left(\frac{1}{2} - im - i(\phi_i - \phi_j)\right) + \frac{1}{2}f(i(\phi_i - \phi_j)) - \right. \right. \\ \left. \left. - \frac{1}{4}f\left(\frac{1}{2} - im + i(\phi_i - \phi_j)\right) - \frac{1}{4}f\left(\frac{1}{2} - im - i(\phi_i - \phi_j)\right) \right] \right). \quad (15.3.6)$$

In the large  $N$  limit the partition function in (15.3.6) is dominated by the saddle point. Using the derivatives in (15.3.4), the  $\phi_i$  at the saddle point satisfy

$$\begin{aligned} \frac{16\pi^3 N}{\lambda} \phi_i = \pi \sum_{j \neq i} & \left[ \left( 2 - (\phi_i - \phi_j)^2 \right) \coth(\pi(\phi_i - \phi_j)) \right. \\ & + \frac{1}{2} \left( \frac{1}{4} + (\phi_i - \phi_j - m)^2 \right) \tanh(\pi(\phi_i - \phi_j - m)) \\ & \left. + \frac{1}{2} \left( \frac{1}{4} + (\phi_i - \phi_j + m)^2 \right) \tanh(\pi(\phi_i - \phi_j + m)) \right]. \end{aligned} \quad (15.3.7)$$

In general this equation is not solvable, but it simplifies a lot both at weak ( $\lambda \ll 1$ ) and strong ( $\lambda \gg 1$ ) coupling.

For weak coupling, the contribution from the hypermultiplet plays no role and (15.3.7) reduces to

$$\frac{16\pi^3 N}{\lambda} \phi_i \approx 2 \sum_{j \neq i} \frac{1}{\phi_i - \phi_j}. \quad (15.3.8)$$

This is the same equation one finds for a Gaussian matrix model and in the large- $N$  limit its solution has the Wigner distribution

$$\rho(\phi) \equiv \frac{1}{N} \frac{dn}{d\phi} = \frac{2}{\pi\phi_0^2} \sqrt{\phi_0^2 - \phi^2}, \quad \phi_0 = \sqrt{\frac{\lambda}{4\pi^3}}, \quad (15.3.9)$$

where the eigenvalue density is normalized to

$$\int \rho(\phi) d\phi = 1. \quad (15.3.10)$$

The free energy then has the typical weak coupling form

$$F = -\log Z \approx -N^2 \log \sqrt{\lambda}. \quad (15.3.11)$$

At strong coupling and with  $|m| \ll \lambda$  we can simplify (15.3.7) by making the ansatz  $|\phi_i - \phi_j| \gg 1$ . In general this is not the case for every pair  $(i, j)$ , but it will be true for most of them. The saddle point equation then simplifies to

$$\frac{16\pi^3 N}{\lambda} \phi_i = \pi \left( \frac{9}{4} + m^2 \right) \sum_{j \neq i} \text{sgn}(\phi_i - \phi_j). \quad (15.3.12)$$

If we assume the  $\phi_i$  are ordered, we get

$$\phi_i = \frac{(9 + 4m^2) \lambda}{64\pi^2 N} (2i - N). \quad (15.3.13)$$

Hence the eigenvalue density is constant over its support,

$$\begin{aligned} \rho(\phi) &= \frac{32\pi^2}{(9 + 4m^2) \lambda}, & |\phi| \leq \phi_m, & \quad \phi_m = \frac{(9 + 4m^2) \lambda}{64\pi^2} \\ &= 0 & |\phi| > \phi_m. & \end{aligned} \quad (15.3.14)$$

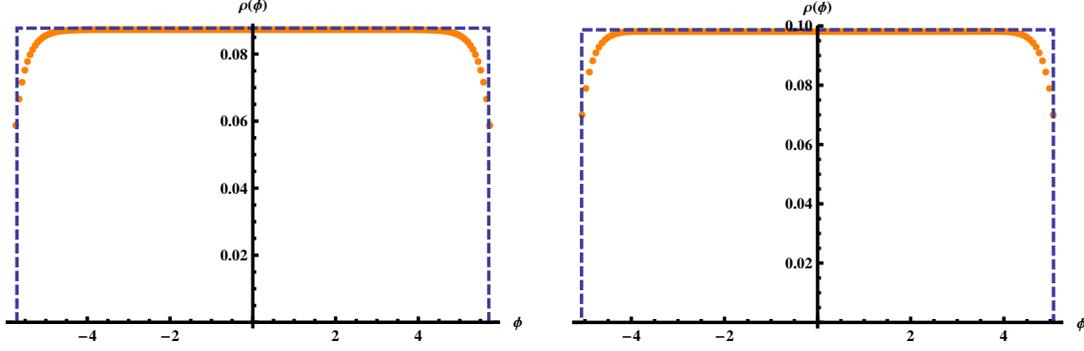

Figure 15.3.1: Numerical results for the eigenvalue density  $\rho(\phi)$  for (left)  $m = 0$ ,  $N = 200$ ,  $\lambda = 400$  and (right)  $m = \frac{1}{2}$ ,  $N = 160$ ,  $\lambda = 320$ . The dashed blue lines are the strong coupling solutions in (15.3.14).

In figure 15.3.1 we compare the approximation in (15.3.14) with numerical results using the full kernel in (15.3.7). As one can see the approximation is very good except with a slight deterioration at the end-points.

Using the strong-coupling ansatz, the partition function in (15.3.5) simplifies to

$$Z \sim \int \prod_i d\phi_i e^{-\frac{8\pi^3 N}{\lambda} \sum_i \phi_i^2 + \frac{\pi}{2} (9 + m^2) \sum_{j \neq i} \sum_i |\phi_i - \phi_j|}. \quad (15.3.15)$$

Applying the saddle point solution (15.3.13), we find for the free energy

$$F \equiv -\log Z \approx -\frac{g_{YM}^2 N^3}{96\pi r} \left( \frac{9}{4} + m^2 \right)^2 + O(N^2). \quad (15.3.16)$$

Thus we see that the free energy crosses over from the  $N^2$  dependence expected in a weakly coupled gauge theory to an  $N^3$  behavior when going from weak to strong coupling.

The other interesting observable we can compute using localization is a supersymmetric Wilson loop [13, 26, 27]. Such loops in five-dimensional flat space were first considered in [28]. On  $S^5$ , the loop must run along an  $S^1$  fiber over a base  $\mathbb{C}P^2$  in order to preserve some of the supersymmetries. The supersymmetric Wilson loop is given by

$$\langle W \rangle = \frac{1}{N} \left\langle \text{Tr} \left( \text{P exp} \left( i \oint_{S^1} (A_M v^M) ds \right) \right) \right\rangle. \quad (15.3.17)$$

where we have written the bosonic fields  $A_M$  in the 10D notation of [19, 29]. The vector  $v^M$  is the 10-dimensional vector  $v^M = \epsilon \Gamma^M \epsilon$  where the components  $M = 1, \dots, 5$  reduce to the Reeb vector on  $S^5$  and  $v^0 = 1$ , where  $A_0 = \sigma$ . All other components of  $v^M$  are zero. Hence, along the localization locus in the zero instanton sector we have  $A_M v^M = \sigma$ . After Wick rotation the Wilson loop then becomes

$$\langle W \rangle = \frac{1}{N} \langle \text{Tr} e^{2\pi\phi} \rangle = \frac{1}{N} \left\langle \sum_i e^{2\pi\phi_i} \right\rangle. \quad (15.3.18)$$

In the large  $N$  limit the  $\sum_i e^{2\pi\phi_i}$  term has a negligible back-reaction on the saddle point solutions. Thus in this limit the Wilson loop is well-approximated by the integral

$$\langle W \rangle = \int d\phi \rho(\phi) e^{2\pi\phi}. \quad (15.3.19)$$

At weak coupling where the density has support only for  $|\phi| \ll 1$  we can approximate the integral as

$$\langle W \rangle \approx \int d\phi \rho(\phi) (1 + 2\pi^2 \phi^2) = 1 + \frac{\lambda}{8\pi} \approx \exp\left(\frac{\lambda}{8\pi}\right). \quad (15.3.20)$$

At strong coupling, where the density is approximately constant along its support, we find

$$\langle W \rangle \approx \frac{32\pi^2}{(9 + 4m^2)\lambda} \int_{-\phi_m}^{\phi_m} e^{2\pi\phi} d\phi \sim \exp\left(\frac{\lambda}{8\pi} \left(\frac{9}{4} + m^2\right)\right), \quad (15.3.21)$$

where we have dropped the prefactor since it can be affected by our approximation and besides is not particularly important for the rest of the discussion. Interestingly, and unlike 4D, the argument in the exponent still has linear  $\lambda$  dependence at strong coupling, with the coefficient changed by the factor  $\left(\frac{9}{4} + m^2\right)$  as compared to the weak coupling result.

The results for the free-energy and the Wilson loop can be generalized to a  $\mathbb{Z}_k$  quiver of the  $\mathcal{N} = 1^*$  theory [10, 13]. The quiver has an  $SU(N)^k$  gauge group with equal mass hypermultiplets transforming in the bifundamental representations,  $(N, \bar{N}, 1, \dots, 1)$ ,  $(1, N, \bar{N}, 1, \dots)$ , *etc.* The eigenvalues of (15.3.7) divide into  $k$  groups  $\psi_i^{(r)}$ , where  $r = 1, \dots, k$ ,  $i = 1, \dots, N$ , resulting in the equations of motion

$$\begin{aligned} \frac{16\pi^3 N}{\lambda} \psi_i^{(r)} &= \pi \left[ \sum_{j \neq i} \left( 2 - (\psi_i^{(r)} - \psi_j^{(r)})^2 \right) \coth(\pi(\psi_i^{(r)} - \psi_j^{(r)})) \right. \\ &\quad + \left( \sum_j \left[ \frac{1}{4} \left( \frac{1}{4} + (\psi_i^{(r)} - \psi_j^{(r+1)} - m)^2 \right) \tanh(\pi(\psi_i^{(r)} - \psi_j^{(r+1)} - m)) \right. \right. \\ &\quad \left. \left. + \frac{1}{4} \left( \frac{1}{4} + (\psi_i^{(r)} - \psi_j^{(r-1)} - m)^2 \right) \tanh(\pi(\psi_i^{(r)} - \psi_j^{(r-1)} - m)) \right] \right) \\ &\quad \left. + (m \rightarrow -m) \right). \end{aligned} \quad (15.3.22)$$

Equations (15.3.22) have a solution where  $\psi_i^{(r)} = \psi_i^{(s)}$  for all  $r$  and  $s$ . Hence, if we take the same strong coupling ansatz as before, we find the eigenvalues set to  $\psi_i^{(r)} = \phi_i$ , where  $\phi_i$  are the values in (15.3.13). The free energy is  $F_k = kF$ , where  $F$  is the free-energy in (15.3.16). The Wilson loop is the same as in (15.3.21).

## 15.4 Supergravity comparisons

In this section we compare the results for strongly coupled 5d SYM with the corresponding results found using the AdS/CFT correspondence [10, 13].

We begin by reviewing the supergravity computation of the free energy [10]. We consider supergravity on  $AdS_7 \times S^4$  where the  $AdS_7$  boundary is  $S^1 \times S^5$ . The radii of  $AdS_7$  and  $S^4$  are  $\ell$  and  $\ell/2$  respectively, where  $\ell = 2\ell_{pl}(\pi N)^{1/3}$ . The  $AdS_7$  metric in global coordinates is given by

$$ds^2 = \ell^2(\cosh^2 \rho d\tau^2 + d\rho^2 + \sinh^2 \rho d\Omega_5^2), \quad (15.4.1)$$

where  $d\Omega_5^2$  is the unit 5-sphere metric. The Euclidean time direction is compactified and has the identification  $\tau \equiv \tau + 2\pi R_6/r$ , while  $R_6$  and  $r$  are the boundary radii of  $S^1$  and  $S^5$ .

Under the AdS/CFT correspondence, the supergravity classical action equals the free energy of the boundary field theory. The action needs to be regulated by adding counterterms [30–33]. There can be scheme dependence in the regulation [32], but we will follow a minimal subtraction type prescription, which is the normal procedure when regulating the action. The full action then has the form

$$I_{AdS} = I_{\text{bulk}} + I_{\text{surface}} + I_{\text{ct}}, \quad (15.4.2)$$

where

$$I_{\text{bulk}} = -\frac{1}{16\pi G_N} \text{Vol}(S^4) \int d^7x \sqrt{g} (R - 2\lambda) \quad (15.4.3)$$

is the action in the bulk with Newton's constant related to the 11-dimensional Planck length as  $G_N = 16\pi^7 \ell_{pl}^9$ . The other terms in (15.4.2) are the surface contribution  $I_{\text{surf}}$  and the counterterm  $I_{\text{ct}}$ , written in terms of the boundary metric and which cancels off divergences in  $I_{\text{bulk}}$ . One then finds the equations of motion

$$R - 2\lambda = -\frac{12}{\ell^2}, \quad (15.4.4)$$

and hence the action

$$I_{\text{bulk}} = -\frac{1}{256\pi^8 \ell_{pl}^9} \left( \frac{\pi^2 \ell^4}{6} \right) \frac{2\pi R_6}{r} \pi^3 (-12\ell^5) \int_0^{\rho_0} \cosh \rho \sinh^5 \rho d\rho = \frac{4\pi R_6}{3r} N^3 \sinh^6 \rho_0. \quad (15.4.5)$$

The integral diverges as  $\rho_0 \rightarrow \infty$  and corresponds to a UV divergence in the boundary theory. We then set  $\lambda = e^{\rho_0}$  where  $\lambda$  is the UV cutoff of the boundary theory, from which we obtain the expansion

$$\sinh^6 \rho_0 = \frac{1}{64} \lambda^6 - \frac{3}{32} \lambda^4 + \frac{15}{64} \lambda^2 - \frac{5}{16} + \mathcal{O}(\lambda^{-2}). \quad (15.4.6)$$

The surface term contributes to the divergent pieces, but not the finite part of (15.4.5), while the counterterm cancels off the remaining divergent pieces with a minimal subtraction prescription. Hence, the regularized action is [31]

$$I_{AdS} = -\frac{5\pi R_6}{12r} N^3. \quad (15.4.7)$$

The Wilson loop expectation value can also be computed using supergravity [34]. Here, one considers an M2 brane that wraps the Euclidean time direction and the equator, while the

brane's third direction drops straight down into the bulk. The Wilson loop is then dominated by the extremum of the world-volume action of the M2 brane,

$$\langle W \rangle \sim e^{-T^{(2)} \int dV}, \quad (15.4.8)$$

where the tension of the brane is  $T^{(2)} = \frac{1}{(2\pi)^2 l_p^3}$ . The M2 brane volume is given by

$$\int dV = l^3 \int_0^{\frac{2\pi R_6}{r}} d\tau \int_0^{2\pi} d\phi \int_0^{\rho_0} d\rho \sinh(\rho) \cosh(\rho) \quad (15.4.9)$$

Using the same UV cutoff as in (15.4.5) we find

$$T^{(2)} \int dV = \frac{\pi N R_6}{r} (\lambda - 2 + \lambda^{-1}). \quad (15.4.10)$$

The integral is again regulated using the minimal subtraction procedure and gives the regulated Wilson loop

$$\langle W \rangle \sim \exp\left(\frac{2\pi N R_6}{r}\right) \quad (15.4.11)$$

Using the identification in (15.1.1) we see that (15.4.11) matches with (15.3.21) if  $m = i/2$ , which is the enhancement point to  $\mathcal{N} = 2$  supersymmetry [17, 29]. However, for this value of  $m$  the free-energy results in (15.4.7) and (15.3.16) differ by a factor of 5/4. Curiously, if we were to replace (15.1.1) with

$$R_6 = \frac{g_{YM}^2}{16\pi^2} \left(\frac{9}{4} + m^2\right). \quad (15.4.12)$$

such that the Wilson loops agree for any value of  $m$ , then the free-energies in (15.4.7) and (15.3.16) agree for  $m = 1/2$ . At present we do not have an explanation for this.

We can also compare supergravity results for the quiver. This effectively replaces the  $S^4$  with  $S^4/\mathbb{Z}_k$ , reducing the volume of this space by a factor of  $k$ , while at the same time replacing  $N$  with  $Nk$ . Therefore the free-energy becomes

$$I_{AdS} = -\frac{5\pi R_6 k^2}{12 r} N^3. \quad (15.4.13)$$

Likewise,  $R_6$  should be replaced with  $R_6/k$ . Hence we have the same sort of matching/mismatching between the gauge theory and supergravity as in the unquivered theory.

## 15.5 Discussion

In this review we have shown how to extract perturbative results for five-dimensional  $\mathcal{N} = 1^*$  Yang-Mills theory on  $S^5$ . There are of course many other interesting phenomena that one can explore. For example, one can squash the  $S^5$  [35] which modifies the determinant factors

in (15.2.3). Interestingly, the free-energy is the same as in (15.3.16), multiplied by the ratio of the squashed to unsquashed volume factors [35].

Also of interest are phase transitions. Here we will describe two types. The first is a transition between a Yang-Mills phase and a Chern-Simons phase [36]. Here it is possible to show that there is a third order phase transition when the ratio

$$\kappa \equiv \frac{8\pi^2}{k g_{YM}^2} \tag{15.5.1}$$

equals the critical value

$$\kappa_c = \sqrt{\frac{27\pi\lambda}{2}} \tag{15.5.2}$$

at weak coupling and

$$\kappa_c = 4\pi^2(9 + 4m^2)\lambda \tag{15.5.3}$$

at strong coupling.

Another type of phase transition occurs when taking the infinite volume limit [37], in a manner similar to what happens in four dimensions [38, 39], there occur an infinite number of transitions as the actual 't Hooft coupling,  $t \equiv g_{YM}^2 N$ , is taken to infinity. For an adjoint hypermultiplet with mass  $M$ , at strong coupling one finds a series of critical points at [37]

$$t_c^{(n)} = \frac{8\pi^2}{M}(n+1), \quad n \in \mathbb{Z}_+, \tag{15.5.4}$$

or in terms of the dimensionless 't Hooft coupling and mass parameter,

$$\lambda_c^{(n)} = \frac{8\pi^2}{m}(n+1), \quad n \in \mathbb{Z}_+. \tag{15.5.5}$$

An important open problem is the mismatch of the free-energies between the 5d gauge theory calculation and the supergravity computation of the (2,0) theory. One possibility is that this is a scheme dependence problem. In any event, we hope to see this discrepancy resolved in the near future.

## Acknowledgement:

This research is supported in part by Vetenskapsrådet under grant #2012-3269. I thank my co-authors J. Källén, A. Nedelin and M. Zabzine for very enjoyable collaborations. I also thank the CTP at MIT for kind hospitality during the course of this work.

## References

- [1] V. Pestun and M. Zabzine, eds., *Localization techniques in quantum field theory*, vol. xx. Journal of Physics A, 2016. 1608.02952. <https://arxiv.org/src/1608.02952/anc/LocQFT.pdf>, <http://pestun.ihe.fr/pages/LocalizationReview/LocQFT.pdf>.

- [2] E. Witten, “String Theory Dynamics in Various Dimensions,” *Nucl.Phys.* **B443** (1995) 85–126, [arXiv:hep-th/9503124](#) [hep-th].
- [3] S. Kim and K. Lee, “Indices for 6 dimensional superconformal field theories,” *Journal of Physics A* **xx** (2016) 000, [1608.02969](#).
- [4] M. R. Douglas, “On D=5 super Yang-Mills theory and (2,0) theory,” *JHEP* **1102** (2011) 011, [arXiv:1012.2880](#) [hep-th].
- [5] N. Lambert, C. Papageorgakis, and M. Schmidt-Sommerfeld, “M5-Branes, D4-Branes and Quantum 5D Super-Yang-Mills,” *JHEP* **1101** (2011) 083, [arXiv:1012.2882](#) [hep-th].
- [6] S. Bolognesi and K. Lee, “Instanton Partons in 5-dim SU(N) Gauge Theory,” *Phys.Rev.* **D84** (2011) 106001, [arXiv:1106.3664](#) [hep-th].
- [7] Z. Bern, J. J. Carrasco, L. J. Dixon, M. R. Douglas, M. von Hippel, *et al.*, “D = 5 Maximally Supersymmetric Yang-Mills Theory Diverges at Six Loops,” [arXiv:1210.7709](#) [hep-th].
- [8] C. Papageorgakis and A. B. Royston, “Revisiting Soliton Contributions to Perturbative Amplitudes,” *JHEP* **09** (2014) 128, [arXiv:1404.0016](#) [hep-th].
- [9] H.-C. Kim and S. Kim, “M5-branes from gauge theories on the 5-sphere,” [arXiv:1206.6339](#) [hep-th].
- [10] J. Kallen, J. Minahan, A. Nedelin, and M. Zabzine, “ $N^3$ -behavior from 5D Yang-Mills theory,” *JHEP* **1210** (2012) 184, [arXiv:1207.3763](#) [hep-th].
- [11] I. R. Klebanov and A. A. Tseytlin, “Entropy of Near Extremal Black P-Branes,” *Nucl.Phys.* **B475** (1996) 164–178, [arXiv:hep-th/9604089](#) [hep-th].
- [12] M. Henningson and K. Skenderis, “The Holographic Weyl Anomaly,” *JHEP* **9807** (1998) 023, [arXiv:hep-th/9806087](#) [hep-th].
- [13] J. A. Minahan, A. Nedelin, and M. Zabzine, “5D Super Yang-Mills Theory and the Correspondence to  $AdS_7/CFT_6$ ,” *J.Phys.* **A46** (2013) 355401, [arXiv:1304.1016](#) [hep-th].
- [14] N. Seiberg, “Five-Dimensional SUSY Field Theories, Nontrivial Fixed Points and String Dynamics,” *Phys.Lett.* **B388** (1996) 753–760, [arXiv:hep-th/9608111](#) [hep-th].
- [15] K. A. Intriligator, D. R. Morrison, and N. Seiberg, “Five-Dimensional Supersymmetric Gauge Theories and Degenerations of Calabi-Yau Spaces,” *Nucl.Phys.* **B497** (1997) 56–100, [arXiv:hep-th/9702198](#) [hep-th].
- [16] J. Kallen, J. Qiu, and M. Zabzine, “The perturbative partition function of supersymmetric 5D Yang-Mills theory with matter on the five-sphere,” *JHEP* **1208** (2012) 157, [arXiv:1206.6008](#) [hep-th].
- [17] H.-C. Kim and S. Kim, “M5-branes from gauge theories on the 5-sphere,” *JHEP* **1305** (2013) 144, [arXiv:1206.6339](#) [hep-th].
- [18] J. Qiu and M. Zabzine, “Review of localization for 5D supersymmetric gauge theories,” *Journal of Physics A* **xx** (2016) 000, [1608.02966](#).
- [19] V. Pestun, “Localization of Gauge Theory on a Four-Sphere and Supersymmetric Wilson Loops,” *Commun.Math.Phys.* **313** (2012) 71–129, [arXiv:0712.2824](#) [hep-th].
- [20] S.-Y. Koyama and N. Kurokawa, “Zeta functions and normalized multiple sine functions,” *Kodai Math. J.* **28** (2005) no. 3, 534–550. <http://dx.doi.org/10.2996/kmj/1134397767>.
- [21] N. Nekrasov, “Five dimensional gauge theories and relativistic integrable systems,” *Nucl.Phys.* **B531** (1998) 323–344, [arXiv:hep-th/9609219](#) [hep-th].

- [22] T. Flacke, “Covariant quantization of  $N = 1$ ,  $D = 5$  supersymmetric Yang-Mills theories in 4D superfield formalism,” *DESY-thesis-2003-047* (2003) .
- [23] D. L. Jafferis and S. S. Pufu, “Exact results for five-dimensional superconformal field theories with gravity duals,” [arXiv:1207.4359](#) [[hep-th](#)].
- [24] D. L. Jafferis, “The Exact Superconformal R-Symmetry Extremizes  $Z$ ,” *JHEP* **1205** (2012) 159, [arXiv:1012.3210](#) [[hep-th](#)].
- [25] J. Kallen and M. Zabzine, “Twisted supersymmetric 5D Yang-Mills theory and contact geometry,” *JHEP* **1205** (2012) 125, [arXiv:1202.1956](#) [[hep-th](#)].
- [26] H.-C. Kim, J. Kim, and S. Kim, “Instantons on the 5-Sphere and M5-Branes,” [arXiv:1211.0144](#) [[hep-th](#)].
- [27] B. Assel, J. Estes, and M. Yamazaki, “Wilson Loops in 5D  $\mathcal{N} = 1$  SCFTs and AdS/CFT,” [arXiv:1212.1202](#) [[hep-th](#)].
- [28] D. Young, “Wilson Loops in Five-Dimensional Super-Yang-Mills,” *JHEP* **1202** (2012) 052, [arXiv:1112.3309](#) [[hep-th](#)].
- [29] J. A. Minahan and M. Zabzine, “Gauge Theories with 16 Supersymmetries on Spheres,” *JHEP* **1503** (2015) 155, [arXiv:1502.07154](#) [[hep-th](#)].
- [30] V. Balasubramanian and P. Kraus, “A Stress Tensor for Anti-de Sitter Gravity,” *Commun.Math.Phys.* **208** (1999) 413–428, [arXiv:hep-th/9902121](#) [[hep-th](#)].
- [31] R. Emparan, C. V. Johnson, and R. C. Myers, “Surface Terms as Counterterms in the AdS / CFT Correspondence,” *Phys.Rev.* **D60** (1999) 104001, [arXiv:hep-th/9903238](#) [[hep-th](#)].
- [32] S. de Haro, S. N. Solodukhin, and K. Skenderis, “Holographic Reconstruction of Space-Time and Renormalization in the AdS / CFT Correspondence,” *Commun.Math.Phys.* **217** (2001) 595–622, [arXiv:hep-th/0002230](#) [[hep-th](#)].
- [33] A. M. Awad and C. V. Johnson, “Higher Dimensional Kerr - AdS Black Holes and the AdS / CFT Correspondence,” *Phys.Rev.* **D63** (2001) 124023, [arXiv:hep-th/0008211](#) [[hep-th](#)].
- [34] D. E. Berenstein, R. Corrado, W. Fischler, and J. M. Maldacena, “The Operator product expansion for Wilson loops and surfaces in the large N limit,” *Phys.Rev.* **D59** (1999) 105023, [arXiv:hep-th/9809188](#) [[hep-th](#)].
- [35] J. Qiu and M. Zabzine, “5D Super Yang-Mills on  $Y^{p,q}$  Sasaki-Einstein Manifolds,” *Commun.Math.Phys.* **333** (2015) no. 2, 861–904, [arXiv:1307.3149](#) [[hep-th](#)].
- [36] J. A. Minahan and A. Nedelin, “Phases of Planar 5-Dimensional Supersymmetric Chern-Simons Theory,” *JHEP* **1412** (2014) 049, [arXiv:1408.2767](#) [[hep-th](#)].
- [37] A. Nedelin, “Phase Transitions in 5D Super Yang-Mills Theory,” [arXiv:1502.07275](#) [[hep-th](#)].
- [38] J. G. Russo and K. Zarembo, “Evidence for Large-N Phase Transitions in  $\mathcal{N} = 2^*$  Theory,” *JHEP* **1304** (2013) 065, [arXiv:1302.6968](#) [[hep-th](#)].
- [39] J. Russo and K. Zarembo, “Massive  $\mathcal{N} = 2$  Gauge Theories at Large N,” *JHEP* **1311** (2013) 130, [arXiv:1309.1004](#) [[hep-th](#)].

# Chapter 16

## Holomorphic blocks and the 5d AGT correspondence

Sara Pasquetti

*Dipartimento di Fisica, Università di Milano-Bicocca, Piazza della Scienza 3, I-20126 Milano, Italy*  
sara.pasquetti@gmail.com

### Abstract

We review the holomorphic block factorisation of partition functions of supersymmetric theories on compact manifolds in various dimensions. We then show how to interpret 3d and 5d partition functions as correlation functions with underlying symmetry given by a deformation of the Virasoro algebra.

### Contents

|                                                                                    |            |
|------------------------------------------------------------------------------------|------------|
| <b>16.1 Introduction</b>                                                           | <b>616</b> |
| <b>16.2 Compact manifolds and Holomorphic Block factorisation</b>                  | <b>617</b> |
| 16.2.1 Factorisation and Holomorphic blocks in 3d and 4d                           | 617        |
| 16.2.2 Factorisation and Holomorphic blocks in 5d                                  | 623        |
| 16.2.3 Codimension-two defects via Higgsing                                        | 629        |
| <b>16.3 Chiral 5d AGT</b>                                                          | <b>633</b> |
| 16.3.1 Deformed Virasoro algebras and chiral blocks                                | 633        |
| 16.3.2 $\mathcal{V}ir_{q,t}$ chiral blocks and instanton-vortex counting           | 638        |
| <b>16.4 3d &amp; 5d partition functions as <math>q</math>-deformed correlators</b> | <b>644</b> |
| <b>16.5 Appendix</b>                                                               | <b>649</b> |
| <b>References</b>                                                                  | <b>652</b> |

## 16.1 Introduction

Over the last 10 years, starting from the seminal work by Pestun [2], Witten’s localisation has been extensively applied to supersymmetric theories defined on compact manifolds of various dimensions. This has led to the derivation of a large number of exact results such as the evaluation of partition functions and vevs of various BPS observables like Wilson-loops and surface operators.

Thanks to these results it has been possible to perform impressive large  $N$  tests of various holographic dualities as summarised in the contributions Chapter 7, Chapter 11, Chapter 15 of this review. It has also been possible to do precision checks of various non-perturbative dualities such as Seiberg-like dualities and 3d mirror symmetry. For example, as reviewed in Chapter 6, 3d partition functions are protected under RG flow hence one can explicitly compute partition functions of pairs of UV Lagrangian supposed to flow to the same SCFT in the IR, and show that they are indeed equal.

Localisation has played a key role also in the discovery of new surprising correspondences relating QFTs in different dimensions and with different types of symmetries. This is the case of the celebrated Alday-Gaiotto-Tachikawa (AGT) correspondence [7] relating  $S^4$  partition functions of  $\mathcal{N} = 2$  theories to Toda CFT correlators. This correspondence together with its variation involving the superconformal index or  $S^3 \times S^1$  partition functions of  $\mathcal{N} = 2$  theories is reviewed in Chapter 12. A similar correspondence relating 3d  $\mathcal{N} = 2$  theories to complex Chern-Simons theories is reviewed in Chapter 9.

The interest in studying SUSY theories on compact manifolds has led to the development of a comprehensive approach to the formulation of supersymmetric theories on curved space initiated by Festuccia and Seiberg [10] and reviewed in Chapter 5. In particular it has been possible to derive general theorems to determine the amount of supersymmetry preserved by a given background and the dependence of partition functions on the data specifying the background.

It has also been observed that if the manifold  $M$  on which the theory is formulated can be decomposed into simpler building blocks, as for example in the case of the solid tori decomposition of a three-sphere, then also the partition function  $Z_M$  can be expressed in terms of the partition functions of the building blocks, the so-called holomorphic-blocks. In the first part of this review article we will illustrate several examples of this block decomposition in 3d, 4d and 5d.

Holomorphic blocks in various dimensions are interesting mathematical objects with intricate transformation properties under dualities which often involve non-trivial Stokes phenomena, for an extensive analysis of the properties of the 3d holomorphic blocks see [12]. 3d and 5d blocks are related to open and closed topological string amplitudes while 3d blocks appear also as Chern-Simons wave functions in the context of the 3d-3d correspondence discussed in Chapter 9.

In this review article we focus instead on the interpretation of the holomorphic blocks in the context of AGT-like correspondences. Via the AGT correspondence partition functions of  $\mathcal{N} = 2$  theories on  $S^4$  can be mapped to Toda/CFT correlators and the holomorphic blocks, which in this case coincide with the two hemi-sphere partition functions, are mapped to the

Toda chiral conformal blocks. Correlators involving degenerate operators are instead mapped to  $\mathcal{N} = 2$  theories on  $S^4$  with surface operators inserted on a codimension-two  $S^2$  and the holomorphic blocks of the codimension-two defect theory correspond to degenerate chiral conformal blocks.

In the second part of this review we will argue that a similar correspondence can be established between  $\mathcal{N} = 1$  theories on a large class of 5-manifolds and correlators with underlying symmetry given by a deformation of the Virasoro algebra. Also in this case codimension-two defect theories and 3d holomorphic blocks can be mapped to degenerate deformed Virasoro correlators.

The plan of the review is the following: we discuss the holomorphic block factorisation in 3d and 4d in section 16.2.1 and in 5d in section 16.2.2. In section 16.2.3 we consider the insertion of codimension-2 defect operators via Higgsing in 5d theories focusing on some simple cases. We then move to the discussion of the dual deformed Virasoro side. After introducing the deformed Virasoro algebra in section 16.3.1, we collect some of the evidences of the mapping of degenerate and non-degenerate deformed Virasoro chiral blocks to vortex and instanton partition functions in section 16.3.2. Finally in section 16.4 we discuss how to combine deformed Virasoro blocks to construct correlators and how these can be mapped to 3d and 5d partition functions.

## 16.2 Compact manifolds and Holomorphic Block factorisation

### 16.2.1 Factorisation and Holomorphic blocks in 3d and 4d

In this section we discuss the holomorphic block factorisation in 4d theories defined on Hermitian manifolds of the form  $M^{4d} = M^{3d} \times S^1$ , where  $M^{3d}$  is a possibly non-trivial  $U(1)$  fibration over the 2-sphere, and their 3d reductions. More precisely we focus on the following  $\mathcal{N} = 1$  backgrounds: the  $S^3 \times S^1$  and lens  $L_r \times S^1$  indexes, the  $S^2 \times T^2$  background and their 3d  $\mathcal{N} = 2$  reductions: the squashed sphere  $S^3$ , the lens space  $L_r$ , the  $S^2 \times S^1$  index and the twisted  $S^2 \times S^1$  index.

The 3-manifolds listed above can all be realised by gluing two solid tori  $D^2 \times S^1$  with an element  $g \in SL(2, \mathbb{Z})$ , we call them  $M_g^{3d}$ . Similarly all the 4-manifolds above can be constructed from the fusion of two solid tori  $D^2 \times T^2$  with appropriate elements in  $g \in SL(3, \mathbb{Z})$  and we call them  $M_g^{4d}$ .

As reviewed in Chapter 5 partition functions on these backgrounds are metric independent, they do however depend on other data specifying the background (for example in the 4d case they depend on the complex structure and holomorphic vector bundles associated to the flavour symmetries) so they are not properly topological objects, nevertheless, as we will review, there is evidence that the following chain of identities holds:

$$Z^{M_g^{3d/4d}} = \sum_g \left\| \Upsilon^{3d/4d} \right\|_g^2 = \sum_c \left\| \mathcal{B}_c^{3d/4d} \right\|_g^2 = \sum_c \left\| \oint_{\Gamma_c} \Upsilon^{3d/4d} \right\|_g^2. \quad (16.2.1)$$

The first equality states the factorisation into a “ $g$ -square” of the integrand of the Coulomb branch partition function<sup>1</sup> given by a classical and 1-loop contribution:

$$Z_{\text{cl}}^{M_g^{3d/4d}} Z_{1\text{-loop}}^{M_g^{3d/4d}} = \left\| \Upsilon^{3d/4d} \right\|_g^2. \quad (16.2.2)$$

The functions  $\Upsilon^{3d/4d}$  can be interpreted as integrands of the  $D^2 \times S^1$  or  $D^2 \times T^2$  partition functions. The data specialising the manifold  $M_g^{3d/4d}$  are all encoded in the gluing rule  $g$ .

To explain this first equality we consider the case of the simplest 3d  $\mathcal{N} = 2$  theory: the free chiral with (minus) half Chern-Simon unit, which we add to remove the parity anomaly. This theory is often referred to as the tetrahedron theory since in the context of the 3d-3d correspondence it computes the quantum volume of the ideal tetrahedron [13], [14], [15].

If we specialise to the squashed 3-sphere  $S_b^3 = \{(x, y) \in \mathbb{C}^2 \mid b^2|x|^2 + b^{-2}|y|^2 = 1\}$ , as reviewed in Chapter 6, the contribution of a charge plus chiral multiplet with canonical R-charge and real mass  $X$  for the background vector multiplet associated to the  $U(1)$  flavour symmetry, is given in terms of the double-sine function  $s_b$  defined in the Appendix 16.5. When combined with the Gaussian contribution of the  $-1/2$  CS unit, the partition function admits a factorised form:

$$Z_{\Delta}^{S_b^3}(X) = e^{\frac{i\pi X^2}{2}} s_b\left(\frac{iQ}{2} - X\right) = \frac{(qx^{-1}; q)_{\infty}}{(\tilde{x}^{-1}; \tilde{q}^{-1})_{\infty}} = \left\| \mathcal{B}_{\Delta}^{3d}(x; q) \right\|_S^2, \quad (16.2.3)$$

where  $Q = b + b^{-1}$  and the *holomorphic* variables are defined as

$$\begin{aligned} q &= e^{2\pi i b^2} = e^{2\pi i \tau}, & \tilde{q} &= e^{\frac{2\pi i}{b^2}} = e^{\frac{2\pi i}{\tau}}, \\ x &= e^{2\pi b X} = e^{2\pi i \chi}, & \tilde{x} &= e^{2\pi \frac{X}{b}} = e^{2\pi i \frac{\chi}{\tau}}. \end{aligned} \quad (16.2.4)$$

The 3d holomorphic block  $\mathcal{B}_{\Delta}^{3d}(x; q) = (qx^{-1}; q)_{\infty}$  is the partition function on the solid torus or Melvin cigar  $D^2 \times S^1$  of the tetrahedron theory. Notice that when  $|q| < 1$  we have  $|\tilde{q}| > 1$  and

$$(x; q)_{\infty} = \sum_{n=0}^{\infty} \frac{(-1)^n q^{\frac{n(n-1)}{2}} x^n}{(q; q)_n} = \begin{cases} \prod_{r=0}^{\infty} (1 - q^r x) & \text{if } |q| < 1 \\ \prod_{r=0}^{\infty} (1 - q^{-r-1} x)^{-1} & \text{if } |q| > 1. \end{cases} \quad (16.2.5)$$

Basically blocks in  $x, q$ , and  $\tilde{x}, \tilde{q}$ , share the same series expansion but they converge to different functions. This is a key feature of holomorphic blocks which has been extensively discussed in [12]. The two blocks are glued through the  $S$ -gluing acting on  $\tau$ , the modular parameter of the boundary  $T^2$ , and on the flavour variable  $\chi$  as:

$$\tau \rightarrow \tilde{\tau} = -S(\tau) = \frac{1}{\tau}, \quad \chi \rightarrow \tilde{\chi} = \frac{\chi}{\tau}. \quad (16.2.6)$$

---

<sup>1</sup>The symbol  $\sum$  indicates that the Coulomb branch partition might include a sum over a discrete index besides the integration over the constant values of the fields parameterising the Coulomb branch.

This gluing corresponds to the element  $S \in SL(2, \mathbb{Z})$  (composed with orientation inversion) realising a three-sphere from a pair of solid tori.

There is an similar factorisation of the tetrahedron theory on the lens space  $L_r$ . This smooth 3-manifold is the free  $\mathbb{Z}_r$  orbifold of the squashed 3-sphere with the identification

$$(x, y) \sim (e^{\frac{2\pi i}{r}} x, e^{-\frac{2\pi i}{r}} y) . \quad (16.2.7)$$

In this case, as reviewed in Chapter 6, the contribution of the chiral multiplet is expressed in terms of the modified double-sine function which takes into account the periodicity inherited from the  $\mathbb{Z}_r$  quotient. The factorisation properties of the modified double-sine are somewhat subtle and we refer the reader to [16] for details, in the end when combined with the appropriate half Chern-Simons unit one finds:

$$Z_{\Delta}^{L_r}(X, H) = \left\| \mathcal{B}_{\Delta}^{3d}(x; q) \right\|_r^2 . \quad (16.2.8)$$

Where we have turned on for the flavour symmetry a continuous real mass  $X$  and a discrete holonomy  $H \in \mathbb{Z}_r$ , parameterising the topological sectors. The holomorphic variables are now defined as

$$\begin{aligned} x &= e^{\frac{2\pi}{r} bX} e^{\frac{2\pi i}{r} H} = e^{2\pi i \chi} e^{\frac{2\pi i}{r} H}, & \tilde{x} &= e^{\frac{2\pi}{rb} X} e^{-\frac{2\pi i}{r} H} = e^{2\pi i \frac{\chi}{r\tau-1}} e^{-\frac{2\pi i}{r} H}, \\ q &= e^{2\pi i \frac{bQ}{r}} = e^{2\pi i \tau}, & \tilde{q} &= e^{2\pi i \frac{Q}{br}} = e^{2\pi i \frac{\tau}{r\tau-1}} . \end{aligned} \quad (16.2.9)$$

The two blocks are glued through the  $r$ -pairing acting as

$$\tau \rightarrow \tilde{\tau} = -\hat{r}(\tau) = \frac{\tau}{r\tau - 1}, \quad \chi \rightarrow \tilde{\chi} = \frac{\chi}{r\tau - 1}, \quad H \rightarrow \tilde{H} = r - H . \quad (16.2.10)$$

This gluing rule as expected coincides with the  $\hat{r} \in SL(2, \mathbb{Z})$  element (composed with the orientation inversion) realising the  $L_r$  geometry from a pair of solid tori. The factorisation on the more general  $L(p, q)$  Lens spaces has been discussed in [17].

The next example we discuss is the  $S^2 \times S^1$  background. Localisation on this background is reviewed in in Chapter 6. For the tetrahedron with a fugacity  $\zeta$  which we take to be a phase, and the integer  $m \in \mathbb{Z}$  for the background magnetic flux through  $S^2$ , we find:

$$Z_{\Delta}^{S^2 \times S^1}(\zeta, m) = \left\| (qx^{-1}; q)_{\infty} \right\|_{id}^2 ,$$

where the holomorphic variables

$$\begin{aligned} x &= \zeta q^{m/2} = e^{2\pi i \chi}, & \tilde{x} &= \zeta^{-1} q^{m/2} = e^{2\pi i \bar{\chi}}, \\ q &= e^{2\pi i \tau}, & \tilde{q} &= q^{-1} = e^{-2\pi i \tau} . \end{aligned} \quad (16.2.11)$$

The two blocks are glued through the  $id$ -pairing (combined with orientation reverse) acting as

$$\tau \rightarrow \tilde{\tau} = -id(\tau) = -\tau, \quad \chi \rightarrow \tilde{\chi} = \bar{\chi}. \quad (16.2.12)$$

This gluing rule as expected coincides with the  $id \in SL(2, \mathbb{Z})$  element (composed with orientation inversion). Finally as discussed in [16], there is a similar factorisation also in the case of the twisted index background [18].

Generic interacting theories, with no parity anomaly, that is with integer effective Chern-Simons couplings, can be constructed by gauging products of tetrahedron theories and then adding integers units of Chern-Simons terms and the contribution of vector multiplets. This observation allow us to *take the square root* of the integrand of generic theories whenever there is no parity anomaly. Indeed we have just reviewed how to take tetrahedron theories as squares of tetrahedron blocks, thanks to these special functions identities we can easily factorise the matter and vector multiplet contributions. Chern-Simons terms at integer level, can instead be dealt with by using the properties of the theta function:

$$\theta(x; q) := (-q^{1/2}x; q)_\infty (-q^{1/2}x^{-1}; q)_\infty, \quad (16.2.13)$$

which for example satisfies

$$\left\| \theta\left((-q^{1/2})^c x^a; q\right) \right\|_S^2 = C^{-2} e^{-i\pi\left(a\frac{x}{2i\pi b} + c\frac{Q}{2}\right)^2}, \quad C = e^{-\frac{i\pi}{12}(b^2 + \frac{1}{b^2})}.$$

We can use this identity to express Chern-Simons terms on  $S^3$  as squares of theta functions depending on the holomorphic variables. Chern-Simons terms on other 3-manifolds  $M_g^{3d}$  are similarly factorised in terms of  $g$ -squares of theta functions.

To make a concrete example we consider the SQED partition function on  $S_b^3$ , with masses  $\tilde{m}_i$  for the  $N_f$  charge plus chirals, masses  $m_i$  for the  $N_f$  charge minus chirals and an FI parameter  $\xi$ :

$$Z^{S_b^3}[SQED] = \int d\sigma e^{2\pi i\sigma\xi} \prod_{j,k=1}^{N_f} s_b(\sigma + m_j + iQ/2) s_b(-\sigma - \tilde{m}_k + iQ/2). \quad (16.2.14)$$

In this case the classical (FI term) and 1-loop term can be factorised as

$$\Upsilon^{3d}[SQED] = \frac{\theta(xu; q)}{\theta(u; q)\theta(x; q)} \prod_{j,k=1}^{N_f} \frac{(qx_j x^{-1}; q)_\infty}{(y_k x^{-1}; q)_\infty}, \quad (16.2.15)$$

with the following definition of holomorphic variables:

$$\begin{aligned} x &= e^{2\pi b\sigma}, & x_i &= e^{2\pi b m_i}, & y_i &= e^{2\pi b \tilde{m}_i}, & z &= e^{2\pi b \xi}, & q &= e^{2\pi i b^2}, \\ \tilde{x} &= e^{2\pi\sigma/b}, & \tilde{x}_i &= e^{2\pi m_i/b}, & \tilde{y}_i &= e^{2\pi \tilde{m}_i/b}, & \tilde{z} &= e^{2\pi \xi/b}, & \tilde{q} &= e^{2\pi i/b^2}, \end{aligned} \quad (16.2.16)$$

and

$$\prod_{j,k=1}^{N_f} x_j y_k^{-1} = r, \quad u = (-q^{\frac{1}{2}})^{N_f} r^{\frac{1}{2}} z^{-1}. \quad (16.2.17)$$

The discussion of the first equality in the chain of identities (16.2.1) for the 4-manifolds case is similar. Here the factorisation of the integrand in terms of the  $D^2 \times T^2$  integrand  $\Upsilon^{4d}$

again involves several non-trivial identities for the special functions appearing in the one-loop contributions but this time the necessary and sufficient condition for the factorisation is the cancellation of the cubic anomaly. This was observed in [16] building on the discovery of the surprising relation between the modular properties of the superconformal index and the appearance of the anomaly polynomial [19].

The next equality in the chain of identities (16.2.1) is the block-factorisation of the Coulomb branch partition function. 1-loop factors are meromorphic functions and it is possible to evaluate the integral by taking residues at their poles by choosing suitable convergent integration contours. The result takes the form of a sum over the supersymmetric vacua (critical points of the effective twisted of superpotential) of the semiclassical (2, 2) theory on the  $\mathbb{R}^2 \times S^1$  and  $\mathbb{R}^2 \times T^2$  solid tori:

$$Z^{M_g^{3d/4d}} = \sum_c \left( Z_{\text{cl}}^{M_g^{3d/4d}} Z_{1\text{-loop}}^{M_g^{3d/4d}} \right)_c \left\| \mathcal{Z}_V^{3d/4d,c} \right\|_g^2. \quad (16.2.18)$$

The contribution of each vacua consists of the product of classical and 1-loop terms evaluated at the  $c$ -th vacuum and of the vortex  $\mathcal{Z}_V^{3d/4d,c}$  partition function. This is the partition function of the theory placed on the cigars or  $\mathbb{R}^2 \times S^1$  or  $\mathbb{R}^2 \times T^2$  with the Omega background turned on  $\mathbb{R}^2$  [20] and enumerates finite energy BPS vortex configurations. Typically vortex partition functions expressed in terms of  $q$ -deformed or elliptic hypergeometric series.

We can also factorise the one-loop and classical contributions as discussed above and present the partition function as a sum of  $g$ -squares of 3d or 4d holomorphic blocks defined as:

$$\mathcal{B}_c^{3d/4d} = \Upsilon^{3d/4d} \Big|_c \mathcal{Z}_V^{3d/4d,c}. \quad (16.2.19)$$

To make a concrete example we consider again the the SQED partition function on  $S_b^3$ . To evaluate the integral (16.2.14) we can close the contour in the upper half plane and take the contributions of poles located at  $x = -m_i + imb + in/b$ , see [21] for details. The result reads

$$Z^{S_b^3[SQED]} = \sum_{i=1}^{N_f} e^{-2\pi i \xi m_i} \prod_{j,k=1}^{N_f} \frac{s_b(m_j - m_i + iQ/2)}{s_b(\tilde{m}_k - m_i - iQ/2)} \left\| \mathcal{Z}_V^{(i)} \right\|_S^2, \quad (16.2.20)$$

where the various terms are given by the FI and 1-loop contributions with the Coulomb branch parameter fixed at  $x = -m_i$  and the vortex partition function

$$\begin{aligned} \mathcal{Z}_V^{(i)} &= \sum_{n \geq 0} \prod_{j,k=1}^{N_f} \frac{(y_k x_i^{-1}; q)_n}{(q x_j x_i^{-1}; q)_n} u^n = \\ &= {}_{N_f} \Phi_{N_f-1}(x_i^{-1} y_1, \dots, x_i^{-1} y_{N_f}; q x_i^{-1} x_1, \dots, q x_i^{-1} x_{N_f}; u). \end{aligned} \quad (16.2.21)$$

where  ${}_{N_f} \Phi_{N_f-1}$  is the basic hypergeometric function. The classical and 1-loop term can also

be factorised to obtain the 3d block:

$$\mathcal{B}_i^{3d} = \frac{\theta(x_i u; q)}{\theta(u; q)\theta(x_i; q)} \prod_{j,k=1}^{N_f} \frac{(qx_j x_i^{-1}; q)_\infty}{(y_k x_i^{-1}; q)_\infty} \times {}_{N_f}\Phi_{N_f-1}(x_i^{-1}y_1, \dots, x_i^{-1}y_{N_f}; qx_i^{-1}x_1, \dots, qx_i^{-1}x_{N_f}; u). \quad (16.2.22)$$

Explicit examples of block factorisation have been obtained for various theories and backgrounds including  $S_b^3$ , lens space  $L_r$ , the superconformal index  $S^2 \times S^1$ , the twisted index, [21], [12], [22], [23], [24], [25], [16], [18].

Similar residue computations yield the block factorisation of  $\mathcal{N} = 1$  theories on  $S^3 \times S^1$ ,  $L_r \times S^1$ ,  $S^2 \times T^2$  [26], [27], [16], [28] and on the ellipsoid [29], and, as reviewed in Chapter 3 in 2d  $\mathcal{N} = (2, 2)$  theories on  $S^2$  [31], [32], [33].

The block factorisation of  $M_g^{3d/4d}$  partition function can also be interpreted as the result of an alternative localisation scheme known as Higgs branch localisation. As reviewed in Chapter 3 the Higgs branch localisation was originally introduced for the (2,2) theories in [32], [34], and later applied to other backgrounds in [31], [35], [27], [26], see also the chapter Chapter 3 in this review.

Another perspective on the factorisation in the  $S_b^3$  case was provided in [36], where it was shown that it is possible to deform the three-sphere geometry into two cigars  $D^2 \times S^1$  connected by a long tube without changing the value of the partition function. This deformation has exactly the effect of projecting down the theory into the SUSY ground states which are the only states contributing to the overlap of the two blocks. It should be possible to extend this argument to other 3d and 4d backgrounds. In 2d a similar proof of the block-decomposition of the two-sphere was provided in [37]. The 2d holomorphic block in this case are the cigar partition functions appearing in the Cecotti-Vafa  $tt^*$  set-up [38], [39] and their overlap computes the exact Kähler potential as reviewed in Chapter 4.

To explain the last equality in (16.2.1) we begin by observing a key property of the 3d (or 4d) holomorphic blocks: they are annihilated by a set of difference equations which can be interpreted as Ward identities for Wilson loops (or surface operators) wrapping the circle  $S^1$  (or the torus  $T^2$ ) and acting at the tip of the cigar. There are in fact two commuting sets of difference operators annihilating respectively the holomorphic and the anti-holomorphic blocks. This set of difference operators can be systematically derived from the UV Lagrangian [13], [14], [15]. Building on this in [12] it was developed an integral formalism to compute the 3d holomorphic blocks by integrating the meromorphic one-form  $\Upsilon^{3d}$  on a basis of middle-dimensional cycles in  $(\mathbb{C}^*)^{|G|}$

$$\mathcal{B}_c^{3d} = \oint_{\Gamma_c} \Upsilon^{3d}. \quad (16.2.23)$$

Each contour is associated to a critical point of the integrand, which in turn is related to a supersymmetric ground state and it is chosen so that the integral converges and solves the set of difference equations. The space of blocks can then be viewed as the vector space of solutions to the system of difference equations. Closely connected to this constructions are

the global transformations properties of the blocks in parameter space. It was shown that by fixing  $q$  and varying  $x$  the holomorphic blocks are subject to Stokes phenomena. We refer the reader to [12] for a detailed discussion of the block integrals and the interplay between mirror symmetry and Stokes phenomenon. See also [41] for a derivation of the block integrals from localisation on  $D^2 \times S^1$ .

In the context of the 3d-3d correspondence reviewed in the contribution Chapter 5, 3d blocks are identified with complex Chern-Simons wave-functions. In the second part of this chapter we will instead see how 3d blocks can be identified with  $q$ -deformed Virasoro correlators.

We should also mention that factorisation and the definition of the blocks suffer an intrinsic ambiguity. By defining blocks as solutions to difference equations we have the possibility to multiply them by  $q$ -constant which satisfy  $c(xq; q) = c(x; q)$ . By requiring that these constants don't modify the compact space results we restrict to  $q$ -constants with unit  $g$ -square  $\|c(x; q)\|_g^2 = 1$ . These are elliptic ratios of theta functions and have a trivial semiclassical limit ( $q = e^h$   $h \rightarrow 0$ ). These functions represent our ambiguity.

A block integral formulation for 4d holomorphic blocks leading to the last equality in (16.2.1) has been proposed in [16]. The definition of the integration contours for 4d block integrals is quite subtle and a careful study of their properties is still missing. For example it would be interesting to study their behaviour under various 4d dualities. It should also be possible to re-derive the 4d block integrand prescription via localisation on  $D^2 \times T^2$ . The relation of 4d block integrals to free field correlators in an elliptic deformation of the Virasoro algebra has been explored in [42].

## 16.2.2 Factorisation and Holomorphic blocks in 5d

As reviewed in Chapter 14, localisation can be applied to 5d  $\mathcal{N} = 1$  theories formulated on a large class of 5d manifolds. The aim of this section is to show that partition functions on these manifolds can be obtained by gluing the so-called 5d holomorphic blocks  $\mathcal{B}^{5d}$ , which are partition functions on  $\mathbb{R}_{\epsilon_1, \epsilon_2}^4 \times S^1$ . The gluing rule can be read out from the geometric data of the 5d manifolds.

### Squashed $S^5$ partition functions and 5d holomorphic blocks

We begin our discussion with the squashed  $S^5$ , the simplest example of toric Sasaki-Einstein 5-manifold. It is convenient to think the  $S^5$  as  $T^3$  fibration over the interior of a triangle, with the fiber degenerating to a torus on the faces and to a circle over the vertices.

As reviewed in Chapter 14, the partition function of 5d  $\mathcal{N} = 1$  theories on this background takes the following form:

$$Z^{S^5} = \int d\vec{\sigma} Z_{\text{cl}}^{S^5}(\vec{\sigma}) Z_{\text{1-loop}}^{S^5}(\vec{\sigma}, \vec{M}) Z_{\text{inst}}^{S^5}(\vec{\sigma}, \vec{M}). \quad (16.2.24)$$

The integral is over the zero-mode of the vector multiplets scalars  $\vec{\sigma}$  taking value in the

Cartan subalgebra of the gauge group,  $\vec{M}$  indicate the hypermultiplet masses.

The non-perturbative  $Z_{\text{inst}}^{S^5}(\sigma, \vec{M})$  receives contributions from the three fixed points of the Hopf fibration over the  $\mathbb{CP}^2$  base and takes the following factorized form [44, 45]:

$$Z_{\text{inst}}^{S^5}(\vec{\sigma}, \vec{M}) = \prod_{k=1}^3 (\mathcal{Z}_{\text{inst}})_k = \left\| \mathcal{Z}_{\text{inst}} \right\|_S^3, \quad (16.2.25)$$

where  $\mathcal{Z}_{\text{inst}}$  coincides with the equivariant instanton partition function on  $\mathbb{R}^4 \times S^1$  [46, 47] with Coulomb and mass parameters appropriately rescaled and with equivariant parameters  $\epsilon_1 = \frac{e_1}{e_3}$  and  $\epsilon_2 = \frac{e_2}{e_3}$ :

$$\mathcal{Z}_{\text{inst}} = \mathcal{Z}_{\text{inst}}^{\mathbb{R}^4 \times S^1} \left( \frac{i\vec{\sigma}}{e_3}, \frac{\vec{m}}{e_3}; \frac{e_1}{e_3}, \frac{e_2}{e_3} \right), \quad (16.2.26)$$

where  $m = iM + E/2$  and  $E = \omega_1 + \omega_2 + \omega_3$ . The sub-index  $k = 1, 2, 3$  in eq. (16.2.25) refers to the following identification of the parameters  $e_1, e_2, e_3$  to the squashing parameters  $\omega_1, \omega_2, \omega_3$  in each sector:

| sector | $e_1$      | $e_2$      | $e_3$      |
|--------|------------|------------|------------|
| 1      | $\omega_3$ | $\omega_2$ | $\omega_1$ |
| 2      | $\omega_1$ | $\omega_3$ | $\omega_2$ |
| 3      | $\omega_1$ | $\omega_2$ | $\omega_3$ |

(16.2.27)

The three sectors correspond to the loci where the Reeb vector forms closed orbits (in the round  $S^5$  case they close everywhere). For more general toric SE manifolds, it is conjectured that the non-perturbative contributions are indeed localised at these isolated loci.

Actually the instanton partition function depends on the squashing parameters through the combination

$$q = e^{2\pi i e_1/e_3}, \quad t = e^{2\pi i e_2/e_3}, \quad (16.2.28)$$

from which we see that the product  $\left\| \cdots \right\|_S^3$  enjoys an  $SL(3, \mathbb{Z})$  symmetry which acts as *S-dualizing* the couplings  $q$  and  $t$ .

The classical Yang-Mills action can also be expressed in the  $SL(3, \mathbb{Z})$  factorized form as the instanton contribution [48]: <sup>2</sup>

$$Z_{\text{cl}}^{S^5}(\sigma) = e^{\frac{2\pi i}{\omega_1 \omega_2 \omega_3 g^2} \text{Tr}(\sigma^2)} = e^{-\frac{2\pi i}{\omega_1 \omega_2 \omega_3 g^2 2C_2(ad)} \sum_{\alpha} [i\alpha(\sigma)]^2} = \left\| \mathcal{Z}_{\text{cl}} \right\|_S^3, \quad (16.2.29)$$

where

$$\mathcal{Z}_{\text{cl}} = \prod_{\alpha} \frac{\Gamma_{q,t} \left( \frac{1}{e_3} \left( i\alpha(\sigma) + \frac{1}{g^2 2C_2(ad)} + \frac{E}{2} \right) \right)}{\Gamma_{q,t} \left( \frac{1}{e_3} \left( \frac{1}{g^2 2C_2(ad)} + \frac{E}{2} \right) \right)}, \quad (16.2.30)$$

---

<sup>2</sup>To simplify this expression we defined  $g^2 = \frac{g_{YM}^2}{4i\pi^2}$  and used that  $2C_2(ad) \sum_{\rho} \rho(\sigma)^2 = \sum_{\alpha} \alpha(\sigma)^2$ .

and we denoted by  $\alpha$  the roots of the gauge group Lie algebra. To arrive at this expression we first need to write the Gaussian term as a combination of Bernoulli polynomial  $B_{33}$  defined in Appendix 16.5 and then use the identity [49]

$$e^{-\frac{2\pi i}{3!}B_{33}(z)} = \prod_{k=1}^3 \Gamma_{q,t} \left( \frac{z}{e_3} \right)_k = \left\| \Gamma_{q,t} \left( \frac{z}{e_3} \right) \right\|_S^3 \quad (16.2.31)$$

where the elliptic gamma function  $\Gamma_{q,t}$  is defined in the Appendix 16.5. We can therefore write the partition function as:

$$Z_{S^5} = \int d\sigma Z_{1\text{-loop}}^{S^5}(\sigma, \vec{M}) \left\| \mathcal{Z}_{\text{cl}} \mathcal{Z}_{\text{inst}} \right\|_S^3, \quad (16.2.32)$$

where  $\mathcal{Z}_{\text{cl}}$  and  $\mathcal{Z}_{\text{inst}}$  are given respectively in (16.2.30) and (16.2.26).

The 1-loop contribution to the partition function is expressed in terms of the triple sine function  $S_3$  defined in appendix 16.5:

$$Z_{1\text{-loop}}^{S^5}(\vec{\sigma}, \vec{M}) = \frac{\prod_{\alpha>0} S_3(i\alpha(\sigma)) S_3(E + i\alpha(\sigma))}{\prod_R \prod_{\rho \in R} S_3(i\rho(\sigma) + iM + \frac{E}{2})}, \quad (16.2.33)$$

where  $\rho$  is the weight of the representation  $R$ . As suggested in [44], using the relation (16.5.5), the 1-loop contribution to the partition function can be factorised as:

$$Z_{1\text{-loop}}^{S^5}(\vec{\sigma}, \vec{M}) = \prod_R \prod_{\rho \in R} e^{-\frac{\pi i}{3!}[B_{33}(i\alpha(\sigma)) - B_{33}(i\rho(\sigma) + m)]} \prod_{k=1}^3 \frac{(e^{\frac{2\pi i}{e_3}[i\alpha(\sigma)]}; q, t)_k}{(e^{\frac{2\pi i}{e_3}[i\rho(\sigma) + m_R]}; q, t)_k} \quad (16.2.34)$$

where  $(z; q, t) = \prod_{i,j \geq 0} (1 - zq^i t^j)$  denotes the double  $(q, t)$ -factorial and the sub-index  $k$  indicates that  $q, t$  defined in (16.2.28) are related to the squashing parameters according to the  $k$ -th entry in table (16.2.27). Each factor of the  $k$ -product can in turn be identified with the 1-loop contribution to the  $\mathbb{R}^4 \times S^1$  theory:

$$\mathcal{Z}_{1\text{-loop}} = \mathcal{Z}_{1\text{-loop}}^{\mathbb{R}^4 \times S^1} \left( \frac{i\sigma}{e_3}, \frac{\vec{m}}{e_3}; \frac{e_1}{e_3}, \frac{e_2}{e_3} \right) = \prod_R \prod_{\rho \in R} \frac{(e^{\frac{2\pi i}{e_3}[i\alpha(\sigma)]}; q, t)}{(e^{\frac{2\pi i}{e_3}[i\rho(\sigma) + m_R]}; q, t)}. \quad (16.2.35)$$

If we consider (pseudo) real representations, for each weight  $\rho$  there is the opposite weight  $-\rho$  and the sum of the Bernoulli is a quadratic polynomial. For example consider the case with  $N_f$  fundamentals of mass  $M_f$  and  $N_f$  anti-fundamentals of mass  $\bar{M}_f$ , with  $f = 1, \dots, N_f$ , and  $N_a$  adjoints of mass  $M_a$ ,  $a = 1, \dots, N_a$ . The total contribution from the Bernoulli's in the 1-loop terms is (up to a  $\sigma$ -independent constant)

$$\text{Ber} = e^{-\frac{2\pi i}{\omega_1 \omega_2 \omega_3} \frac{\sum_{\alpha} [i\alpha(\sigma)]^2}{2C_2(ad)} \left[ \frac{E}{4} N_f - \frac{1}{4} \sum_f (m_f + \bar{m}_f) + C_2(ad) \left( \frac{E}{2} (N_a - 1) - \sum_a m_a \right) \right]}, \quad (16.2.36)$$

which, once combined with the classical terms, amounts to the shift of the coupling constant

$$\frac{1}{g^2} \rightarrow \frac{1}{g_{eff}^2} = \frac{1}{g^2} + \frac{E}{4} N_f - \frac{1}{4} \sum_f (m_f + \bar{m}_f) + C_2(ad) \left( \frac{E}{2} (N_a - 1) - \sum_a m_a \right). \quad (16.2.37)$$

Combining all these observations one arrives at the completely factorized form [48] (up to constant prefactors):

$$Z^{S^5} = \int d\sigma \left\| \mathcal{B}^{5d} \right\|_S^3, \quad (16.2.38)$$

where  $\mathcal{B}^{5d}$ , the 5d holomorphic block, is defined as

$$\mathcal{B}^{5d} = \mathcal{Z}_{1\text{-loop}} \mathcal{Z}_{\text{cl}} \mathcal{Z}_{\text{inst}}, \quad (16.2.39)$$

with  $\mathcal{Z}_{\text{cl}}$  defined as in eq. (16.2.30) with  $g^2 \rightarrow g_{eff}^2$ . As in the 3d case there is an ambiguity in the definition of the 5d blocks, this is discussed in [48].

We will now see that the partition functions on a large class of 5-manifolds can be expressed in terms of the 5d blocks  $\mathcal{B}^{5d}$ .

### Block-factorisation of 5d toric Sasaki-Einstein partition functions

As reviewed in Chapter 14 localisation can be performed on general simply connected toric Sasaki-Einstein (SE) manifolds  $\mathcal{M}^n$ . These backgrounds preserve 2 supersymmetries.

As in the  $S^5$  case it is convenient to think of these 5-manifolds as  $T^3$  fibration over the interior of a polygon, with the fiber degenerating to a torus on the  $n$  faces and to circle over the  $n$  vertices.

The perturbative partition function on a SE manifold  $\mathcal{M}^n$  is again a Coulomb branch integral

$$Z^{\mathcal{M}^n} = \int d\vec{\sigma} Z_{\text{cl}}^{\mathcal{M}^n}(\vec{\sigma}) Z_{1\text{-loop}}^{\mathcal{M}^n}(\vec{\sigma}, \vec{M}). \quad (16.2.40)$$

The 1-loop contribution  $Z_{1\text{-loop}}^{\mathcal{M}^n}(\vec{\sigma}, \vec{M})$  takes the same form as in the  $S^5$  case (16.2.33) with the triple-sine functions replaced by the generalised triple-sine function defined as:

$$S_3^{\mathcal{M}^n}(X) \sim \prod_{\vec{m} \in C_\mu(\mathcal{M}^n) \cap \mathbb{Z}^3} (\vec{m} \cdot \vec{R} + X)(\vec{m} \cdot \vec{R} + \vec{\xi} \cdot \vec{R} - X). \quad (16.2.41)$$

In the above expression the product is over the integers in the moment map cone:

$$C_\mu(\mathcal{M}^n) = \left\{ \vec{m} \in \mathbb{R}^3 \mid \vec{m} \cdot \vec{v}_i \geq 0, i = 1, \dots, n \right\}, \quad (16.2.42)$$

the three-component vector  $\vec{R}$  parameterises the Reeb vector field, the vector  $\vec{\xi}$  satisfies  $\vec{\xi} \cdot \vec{v}_i = 1$  for  $i = 1, \dots, n$  and  $\vec{v}_i$  are the inward pointing normals of the  $n$  faces. The constant  $E$  in (16.2.33) is also replaced by  $E \rightarrow \vec{\xi} \cdot \vec{R}$ .

In [50], [51] it was derived a factorisation formula for the generalised 3-ple sine functions:

$$S_3^{\mathcal{M}^n}(X) = \text{Ber} \prod_{k=1}^n \left( e^{\frac{2\pi i X}{e_3}} ; e^{\frac{2\pi i e_1}{e_3}}, e^{\frac{2\pi i e_2}{e_3}} \right)_k, \quad (16.2.43)$$

where we denoted by Ber the contribution of the exponential of the cubic Bernoulli polynomials and in each sector the equivariant parameters map to the toric data via the following table

| sector | $e_1$                                   | $e_2$                               | $e_3$                                     |
|--------|-----------------------------------------|-------------------------------------|-------------------------------------------|
| $k$    | $\det[\vec{R}, \vec{v}_{k+1}, \vec{n}]$ | $\det[\vec{v}_k, \vec{R}, \vec{n}]$ | $\det[\vec{v}_k, \vec{v}_{k+1}, \vec{R}]$ |

(16.2.44)

where  $\vec{n}$  is chosen to satisfy the condition  $\det[\vec{v}_i, \vec{v}_{i+1}, \vec{n}] = 1$ . Proceeding as in the  $S^5$  case, we apply the identity (16.2.43) to decompose the 1-loop part into  $n$ -copies of the 1-loop Nekrasov partition function  $\mathcal{Z}_{1\text{loop}}$ .

The classical contribution is given by

$$Z_{\text{cl}}^{\mathcal{M}^n}(\vec{\sigma}) = e^{\frac{2\pi i r \rho}{g^2} \text{Tr}(\vec{\sigma}^2)} \quad (16.2.45)$$

where  $r$  is the overall scale of  $\mathcal{M}^n$  and  $\rho$  is the squashed volume normalised to  $\text{vol}(S^5) = \pi^3$ . By repeatedly using the Gamma function identities (16.5.19) and (16.5.18) it is possible to show that

$$Z_{\text{cl}}^{\mathcal{M}^n}(\vec{\sigma}) = \prod_{k=1}^n (\mathcal{Z}_{\text{cl}})_k \quad (16.2.46)$$

with  $\mathcal{Z}_{\text{cl}}$  defined as in (16.2.30) and in each sector the equivariant parameters are related to the toric data according to the table (16.2.44).

By collecting the Bernoulli factors Ber from the factorisation of each generalised 3-ple sine one obtains a quadratic polynomial which produces the usual renormalisation of the gauge coupling. This allows us to write

$$Z_{\text{cl}}^{\mathcal{M}^n}(\vec{\sigma}) Z_{1\text{-loop}}^{\mathcal{M}^n}(\vec{\sigma}, \vec{M}) = \prod_{k=1}^n (\mathcal{Z}_{\text{cl}} \mathcal{Z}_{1\text{loop}})_k \quad (16.2.47)$$

where  $\mathcal{Z}_{\text{cl}}$  is defined as in eq. (16.2.30) with  $g^2 \rightarrow g_{\text{eff}}^2$ .

In [50] it has been conjectured that the full non-perturbative partition function on  $\mathcal{M}^n$  would receive contributions only from instantons solutions localised around closed Reeb orbits. Around each orbit the instanton contribution is given by a copy of the  $\mathbb{R}^4 \times S^1$  instanton partition function  $\mathcal{Z}_{\text{inst}}$ , leading to the following fully factorised proposal

$$Z_{\text{full}}^{\mathcal{M}^n} = \int \prod_{k=1}^n (\mathcal{B}^{5d})_k. \quad (16.2.48)$$

Proving this conjecture would require a careful study of the contact instanton equation which are quite difficult to analyse. At the moment we cannot rule out the possibility that other solutions will contribute to the full partition function.

In 3d and 4d, partition functions on the lens space  $S^3/\mathbb{Z}_r$  and on the lens index  $S^3/\mathbb{Z}_r \times S^1$  admit a block factorised form only when all the flat connections are summed over [16]. The contribution of a fixed flat connection to the partition function is not factorised. In the  $\mathcal{M}^n$  case instead, as we have just seen, the perturbative result in the trivial flat connection is already factorised. This fact could be a hint that the proposal (16.2.48) is indeed complete or perhaps just an accident. In conclusion further studies are necessary to shed light on this point.

### $S^4 \times S^1$ partition functions and 5d holomorphic blocks

The next case we consider is 5d index or  $S^4 \times S^1$  partition function.  $\mathcal{N} = 1$  gauge theories on this background have been studied in [52–54]. The partition function takes the form of a Coulomb branch integral

$$Z^{S^4 \times S^1} = \int d\vec{\sigma} Z_{1\text{-loop}}^{S^4 \times S^1}(\vec{\sigma}, \vec{M}) Z_{\text{inst}}^{S^4 \times S^1}(\vec{\sigma}, \vec{M}), \quad (16.2.49)$$

with instantons contributions from the fixed points at north and south poles of the  $S^4$ :

$$Z_{\text{inst}}^{S^4 \times S^1} = \prod_{k=1}^2 (\mathcal{Z}_{\text{inst}})_k = \left\| \mathcal{Z}_{\text{inst}} \right\|_{id}^2. \quad (16.2.50)$$

Each pole contributes with a copy of the  $\mathbb{R}^4 \times S^1$  partition function  $\mathcal{Z}_{\text{inst}}$  (16.2.26) with  $m = iM + Q_0/2$  and  $Q_0 = b_0 + 1/b_0$  and the following identification

| sector | $e_1$      | $e_2$ | $e_3$       |
|--------|------------|-------|-------------|
| 1      | $b_0^{-1}$ | $b_0$ | $2\pi i/R$  |
| 2      | $b_0^{-1}$ | $b_0$ | $-2\pi i/R$ |

where  $R$  is the circumference of  $S^1$  and  $b_0$  the squashing parameter of  $S^4$ .

Due to the property (16.5.19) of the elliptic Gamma function, the classical term  $\mathcal{Z}_{\text{cl}}$  defined in eq. (16.2.30) “squares” to one  $\left\| \mathcal{Z}_{\text{cl}} \right\|_{id}^2 = 1$ , we can therefore write

$$Z_{S^4 \times S^1} = \int d\sigma Z_{1\text{-loop}}^{S^4 \times S^1}(\sigma, \vec{M}) \left\| \mathcal{Z}_{\text{cl}} \mathcal{Z}_{\text{inst}} \right\|_{id}^2. \quad (16.2.51)$$

The 1-loop contributions of vector and hyper multiplets are given by

$$Z_{1\text{-loop}}^{S^4 \times S^1, \text{vect}}(\vec{\sigma}) = \frac{\prod_{\alpha > 0} \Upsilon^R(i\alpha(\sigma)) \Upsilon^R(-i\alpha(\sigma))}{\prod_{\rho \in R} \Upsilon^R(i\rho(\sigma) + iM + \frac{Q_0}{2})}, \quad (16.2.52)$$

where the special function  $\Upsilon^R$  is defined in appendix 16.5. Also in this case it is possible to bring the 1-loop term in a factorized form hence the 5d index can be factorised in terms of the same 5d blocks  $\mathcal{B}^{5d}$  we found in the  $S^5$  case [48]:

$$Z^{S^4 \times S^1} = \int d\sigma \left\| \mathcal{B}^{5d} \right\|_{id}^2. \quad (16.2.53)$$

### 16.2.3 Codimension-two defects via Higgsing

Codimension-two half BPS defects in SUSY gauge theories, such as surface operators in 4d, are an important class of non-local operators which can be used to probe the dynamics of gauge theories. For a recent review on surface operators see [55] and Chapter 10. They can be defined by prescribing a singular behaviour of the fields on the codimension-two locus where defect operators live, this has the effect of breaking the gauge group  $G$  to a Levi sub-group  $L$ . Another possibility to define defects in gauge theories is by a coupled system with extra degrees of freedom leaving on the defects. A related construction, the so called Higgsing procedure, introduced in [57] involves turning on a position dependent vev or vortex configuration in a UV theory  $T'$  and following the RG flow to an IR point described by a theory  $T$ . This construction should be indeed equivalent to coupling the 4d gauge fields to a 2d sigma model with target space the vortex moduli space.

The Higgsing prescription gives rise to a large class of  $\mathcal{N} = 2$  and  $\mathcal{N} = 1$  theories with surface operators insertions. Some of these systems can be realised in Hanany-Witten brane set ups with surface operators engineered by extra branes [58] as show in Fig. 16.2.1 and admit a description in terms of a 2d GLSM coupled to the bulk theory [59]. Although this is not the most general type of surface operator, we will restrict to this class in the following.

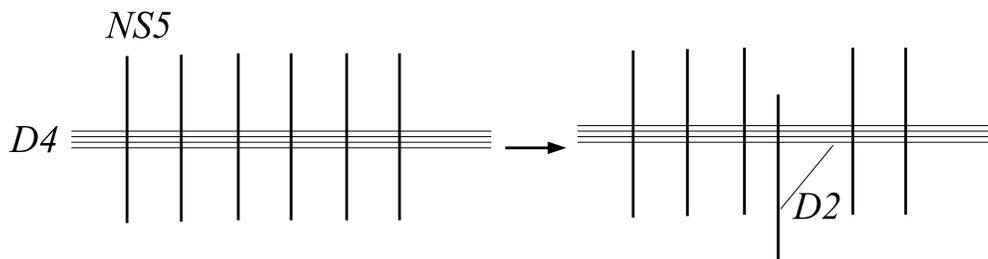

Figure 16.2.1: The Hanany-Witten brane setup for a linear quiver. On the RHS a surface operator corresponding to a position-dependent vev is engineered by an extra D2 brane.

In recent years there has been much progress in computing partition functions and indices of theories with the insertion of these operators. In 4d one can compute the superconformal index ( $S^3 \times S^1$  partition function) of a theory  $T$  enriched by a surface operator via Higgsing by tuning the flavour fugacities of the theory  $T'$  to special values. This causes the integration contour to pinch a set of poles. The index is then evaluated by taking the residue at these poles and the result yields the index of theory  $T$  enriched by a surface operator. If the surface operators admit a description in terms of a 2d GLSM coupled to the bulk theory [59] the index for the coupled 2d-4d system is decorated with the elliptic genus of the 2d GLSM [60].

It is also possible to compute the  $\mathbb{R}_{\epsilon_1, \epsilon_2}^4$  instanton partition function for 4d theory in presence of a surface defect. This takes the form of a double expansion (see for example [20])

$$\sum_{n=0}^{\infty} \sum_{m \in \Lambda} Q^n z^m Z_{n,m}^{inst+vortex}, \quad (16.2.54)$$

where  $n, Q$  are respectively the instanton number and the instanton counting parameter,  $m \in \Lambda \sim H_2(G/L; Z)$  (where  $L$  is the Levi subgroup of the gauge group  $G$ ) are the monopole numbers, and  $z$  is the vortex counting parameter. By decoupling the bulk theory (sending  $Q \rightarrow 0$  and focusing on the  $n = 0$  sector) one gets the purely 2d vortex counting partition function.

At the level of the Hanany-Witten brane setup, as shown in the second line of Fig. 16.2.2, decoupling the bulk theory amounts to sending to infinity all the NS5 branes far from the insertion point. The 4d theory is then just a collection of free 4d hypers coupled to the 2d theory on the stretched D2 brane. Also in this case the combined instanton-vortex counting partition function can be obtained via Higgsing, by tuning the mass parameters to special values [61].

Another option to compute the instanton-vortex partition function is geometric engineering, where  $\mathcal{N} = 2$  gauge theories are obtained via type II strings compactified on toric Calab-Yau threefolds. The refined A-model topological string partition function on these targets [62], [63] coincides with the  $\mathbb{R}_{\epsilon_1, \epsilon_2}^4 \times S^1$  instanton partition function, while open topological strings amplitudes in presence of toric branes reproduce the instanton-vortex counting [20], [64], [65], [66].

In the context of the AGT correspondence [7], two types of surface defects in class  $\mathcal{S}$  theories were discussed. The first type is realised by M2 branes with two directions extending in the 4d space-time and sitting at a point on the Gaiotto curve  $\mathcal{C}_{g,n}$ . The second type of surface operators is instead realised by M5 branes wrapping  $\mathcal{C}_{g,n}$  and with two directions extending in the 4d space-time. In [67] it was proposed to relate the first type class of surface operators to degenerate primary operators in the dual CFT. Indeed it was later shown that it is possible to match the instanton-vortex partition function for these surface operators to the conformal blocks with degenerate insertions as sketched in Fig. 16.2.2, [20], [64], [66].

The compact space version of the AGT+surface operators correspondence was proposed in [32], [68] where it was shown that degenerate correlators can be mapped to partition functions of class  $\mathcal{S}$  theories on  $S^4$ , coupled to a 2d GLSM describing the surface defects defined on  $S^2$ .

As a simple example we consider the  $SU(2)$  theory with 4 flavours on  $S^4$ . When a combination of the masses is tuned to the ‘‘Higgsing condition’’  $m_1 + m_2 = -b_0$ , where  $b_0$  is the squashing parameter of the ellipsoid, the integration contour pinches two poles. The sum of the residue of the partition function at these two points can be identified with the  $S^2$  partition function of the  $(2, 2)$  SQED with 2 flavours multiplied by the contributions of the free 4d hypers. Via the AGT dictionary, which relates the mass parameters to the four external momenta in the CFT correlator, the Higgsing condition is translated into the analytic continuation of one momentum to a degenerate value  $\alpha_2 \rightarrow -b_0/2$ .<sup>3</sup> Summarising

---

<sup>3</sup>Via the AGT dictionary the squashing parameter  $b_0$  is identified with the parameter appearing in central charge  $c = 1 + 6(b_0 + b_0^{-1})^2$  of the dual CFT.

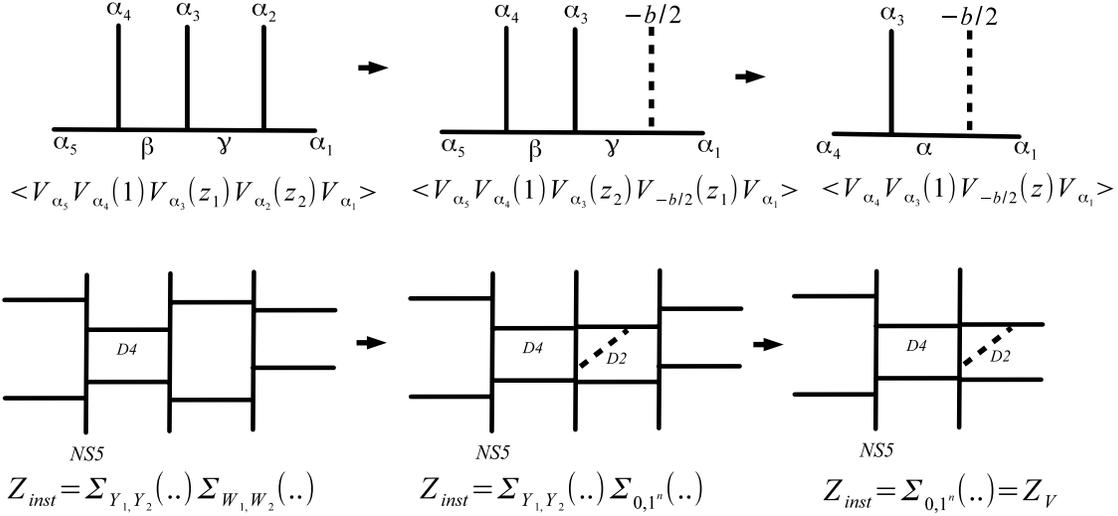

Figure 16.2.2: Higgsing a linear quiver and dual CFT interpretation. The first column represents an  $2 + SU(2) \times SU(2) + 2$  linear quiver and its dual CFT 5-point block, the instanton partition functions involves summing over two 2-vectors of Young tableaux associated to the two  $SU(2)$  nodes. The second column represents the analytic continuation of the mass/momenta to the Higgsing/degeneration condition. Correspondently the sum over the second vector of Young tableaux reduces to a sum over a column-diagram. In the third column the bulk theory is decoupled and the instanton partition function reduces to a vortex partition function which is mapped to the conformal block with 3 non-degenerate and one degenerate-primaries.

we have the following web of correspondences:<sup>4</sup>

$$\begin{array}{ccc}
 Z^{S^4}[2 + SU(2) + 2] & \xrightarrow{\text{Higgsing}} & Z^{S^2}[U(1) + 2] \\
 \text{AGT} \updownarrow & & \text{AGT} \updownarrow \\
 \langle V_{\alpha_1} V_{\alpha_2} V_{\alpha_3} V_{\alpha_4} \rangle & \xrightarrow{\text{Degeneration}} & \langle V_{\alpha_1} V_{-b_0/2} V_{\alpha_3} V_{\alpha_4} \rangle .
 \end{array}$$

We conclude our digression on surface operators in 4d theories by mentioning that for surface operators realised in terms of M5 branes the standard instanton moduli space is replaced by the  $\tilde{\text{O}}$ ramified instantons  $\tilde{\text{O}}$  moduli space and the CFT duals, studied for example in [69], [70] and recently in [71], have affine  $sl(N)$  symmetries. More general surface operators and CFT duals have been studied in [72] and [73], for a review see [74].

Codimension-two half BPS defects can be introduced also in 5d  $\mathcal{N} = 1$  theories. In [75] the Higgsing prescription has been applied to obtain the 5d index ( $S^4 \times S^1$  partition function), decorated by the 3d index ( $S^2 \times S^1$  partition function) of codimension-two defects. Here

<sup>4</sup>The expressions obtained via Higgsing/degenerations have been normalised respectively by the contribution of 4d free hypers and by the 3-point function of the non-degenerate primaries.

we will consider codimension-two defects defined via Higgsing on  $S^5$  and  $S^4 \times S^1$ . We will restrict again to the simple case of free 5d hypers coupled to the codimension-two defect partition function. We consider the case of the  $SU(2)$  theory with four fundamental hyper multiplets with masses  $M_f$ ,  $f = 1, \dots, 4$  on  $S^5$ . As shown in [48], if we tune the masses to satisfy the condition:

$$M_1 + M_2 = i(\omega_3 + E) \quad \text{or} \quad m_1 + m_2 = -\omega_3, \quad (16.2.55)$$

where  $m_j = iM_j + E/2$ , the 1-loop factor develops poles which pinch the integration contour. The partition functions can then be defined via a meromorphic analytic continuation which prescribes to take the residues at the two poles trapped along the integration path located at

$$a_1 = m_1 = -m_2 - \omega_3 = -a_2, \quad a_1 = m_1 + \omega_3 = -m_2 = -a_2. \quad (16.2.56)$$

By analogy with the 4d case, we expect that by taking the residues at these poles, will reconstruct the  $S_b^3$  partition function of 3d SQED with 2 flavours.

Indeed if we evaluate the instanton partition function (16.2.25) at the first pole we find that in the first two sectors the sum over Young tableaux degenerates respectively to the sum over a single column and single row yielding two copies of the  $q$ -deformed hypergeometric  ${}_2\Phi_1$ . The third sector instead gets contribution only from the empty diagrams. In particular all the parameters enter exactly to reconstruct the  $S$ -pairing of two vortex partition functions:

$$\left\| \mathcal{Z}_{\text{inst}} \right\|_S^3 \xrightarrow{(a_1, a_2) \rightarrow (m_1, m_2 + \omega_3)} \left\| {}_2\Phi_1(A, B; C, e^{2\pi i \frac{\omega_2}{\omega_1}}; u) \right\|_S^2 = \left\| \mathcal{Z}_V^{(1)} \right\|_S^2. \quad (16.2.57)$$

The coefficients  $A, B, C$  of the basic hypergeometric function depend on the 5d mass parameters, if we identify them with those of the vortex partition function  $\mathcal{Z}_V^{(1)}$ , we obtain the following dictionary between 3d and 5d masses:

$$m_1^{3d} = -im_1, \quad m_2^{3d} = -im_2, \quad \tilde{m}_1^{3d} = im_3, \quad \tilde{m}_2^{3d} = im_4, \quad (16.2.58)$$

while by matching the expansion parameters we find  $i\xi = 1/\tilde{g}^2$ . We also identify  $\omega_2 = \frac{1}{\omega_1} = b$ . In complete analogy, for the other pole, located at  $a_1 = m_1 + \omega_3 = -m_2 = -a_2$  we find

$$\left\| \mathcal{Z}_{\text{inst}} \right\|_S^3 \xrightarrow{(a_1, a_2) \rightarrow (m_1 + \omega_3, m_2)} \left\| \mathcal{Z}_V^{(2)} \right\|_S^2. \quad (16.2.59)$$

The last step is the identification of the residue at the  $i$ -th pole of the  $S^5$  classical and one loop contributions with  $S_b^3$  classical and one loop contributions evaluated on the  $i$ -th vacuum, in the end after normalising by the contribution of the free 5d hypers, one obtains the promised result:

$$Z^{S^5}[2 + SU(2) + 2] \xrightarrow{m_1 + m_2 = -\omega_3} \sum_{i=1,2} \left( Z_{\text{cl}}^{S_b^3} Z_{1\text{-loop}}^{S_b^3} \right)_i \left\| \mathcal{Z}_V^{(i)} \right\|_S^2 = Z^{S_b^3}[U(1) + 2]. \quad (16.2.60)$$

Notice that there are two extra choices for the degeneration condition, which would have led to the same result:

$$m_1 + m_2 = -\omega_{1,2}, \quad \text{with} \quad \omega_{2,1} = \omega_3^{-1} = b. \quad (16.2.61)$$

The three possibilities correspond to the three maximal squashed 3-spheres inside the squashed 5-sphere.

In a similar manner, it is possible to show that the partition function of the SCQCD on  $S^4 \times S^1$ , when two of the masses satisfy the condition

$$m_1 + m_2 = -b_0, \quad (16.2.62)$$

reduces to the SQED partition function on  $S^2 \times S^1$ :

$$\begin{aligned} Z^{S^4 \times S^1} [2 + SU(2) + 2] &\xrightarrow{m_1 + m_2 = -b_0} \sum_{i=1,2} \left( Z_{\text{cl}}^{S^2 \times S^1} Z_{1\text{-loop}}^{S^2 \times S^1} \right)_i \left\| \mathcal{Z}_V^{(i)} \right\|_{\text{id}}^2 \\ &= Z^{S^2 \times S^1} [U(1) + 2], \end{aligned} \quad (16.2.63)$$

with the 3d angular momentum fugacity  $q$  related to the 5d parameters by  $q = e^{R/b_0}$ . Also in this case there is another possible degeneration condition  $m_1 + m_2 = -\frac{1}{b_0}$ , which leads to the same result but with the identification  $q = e^{Rb_0}$ . The two choices correspond to the two maximal  $S^2$  inside the squashed  $S^4$ .

By paralleling the 4d case we will reinterpret the 5d-3d Higgsing (16.2.60), (16.2.63) as the analytic continuation of a 4-point  $q$ -deformed correlator to the  $q$ -correlator of three non-degenerate and one-degenerate primaries.

Before doing so in next section we will focus on the  $q$ -deformation of the chiral version of the AGT correspondence where we review how  $\mathbb{R}^4 \times S^1$  instanton and  $\mathbb{R}^2 \times S^1$  vortex counting can be mapped to chiral blocks of deformed Virasoro primaries.

## 16.3 Chiral 5d AGT

### 16.3.1 Deformed Virasoro algebras and chiral blocks

Deformed Virasoro and  $\mathcal{W}_N$  algebras were introduced independently in the mid 90s by various groups [76, 77], [78–80], [81, 82], see [83] for a review. The  $\mathcal{Vir}_{q,t}$  algebra is a deformation of the Virasoro algebra, it depends on two complex parameters  $q, t$  and is generated by an infinite set of generators  $T_n$  with  $n \in \mathbb{Z}$ , satisfying the commutation relations

$$[T_n, T_m] = - \sum_{l=1}^{+\infty} f_l (T_{n-l} T_{m+l} - T_{m-l} T_{n+l}) - \frac{(1-q)(1-t^{-1})(p^n - p^{-n})}{1-p} \delta_{m+n,0} \quad (16.3.1)$$

where  $p = \frac{q}{t}$  and the functions  $f_l$  are determined by the expansion

$$f(z) = \sum_{l=0}^{+\infty} f_l z^l = \exp \left[ \sum_{l=1}^{+\infty} \frac{1}{n} \frac{(1-q^n)(1-t^{-n})}{1+p^n} z^n \right]. \quad (16.3.2)$$

The algebra  $\mathcal{V}ir_{q,t}$  is invariant under  $(q, t) \rightarrow (q^{-1}, t^{-1})$  and  $(q, t) \rightarrow (t, q)$ .

As in the Virasoro algebra, the representations of  $\mathcal{V}ir_{q,t}$  can be constructed using Verma modules [76]. The highest weight state  $|\lambda\rangle$  satisfies

$$T_0|\lambda\rangle = \lambda|\lambda\rangle, \quad T_n|\lambda\rangle = 0 \quad \text{for } n > 0, \quad (16.3.3)$$

and the Verma module is constructed acting on the highest weight state  $|\lambda\rangle$  with the operators  $T_{-n}$  with  $n > 0$ . Singular states in the Verma module can be detected using the Kac determinant. In particular there is a level two singular vector when  $\lambda$  takes the following values

$$\lambda_1 = p^{1/2}q^{1/2} + p^{-1/2}q^{-1/2}, \quad \lambda_2 = p^{1/2}t^{-1/2} + p^{-1/2}t^{1/2}. \quad (16.3.4)$$

The states  $\lambda_1$  and  $\lambda_2$  are mapped into each other by the exchange  $(q, t) \rightarrow (t, q)$  and are left invariant by  $(q, t) \rightarrow (q^{-1}, t^{-1})$ .

The algebra  $\mathcal{V}ir_{q,t}$  can be related to other known algebras by taking suitable limits on parameters  $q, t$  [84]. In particular the ordinary Virasoro algebra is recovered by setting  $t = q^\beta$ ,  $q = e^{\hbar}$  and expanding the deformed Virasoro current  $T(z) = \sum_{n \in \mathbb{Z}} T_n z^{-n}$ :

$$T(z) = 2 + T^{(2)}\hbar^2 + T^{(4)}\hbar^4 + \dots \quad (16.3.5)$$

In the second term of the expansion we recognise the Virasoro current  $L(z) = \sum_{n \in \mathbb{Z}} L_n z^{-n-2}$

$$T^{(2)} = \beta \left( z^2 L(z) + \frac{(1 - \beta)^2}{4\beta} \right) \quad (16.3.6)$$

with the identification  $\beta = -b_0^2$ . From the expansion (16.3.5) we see that to control the deformed theory we need all the higher spin currents  $T^{(n)}(z)$ , while in the undeformed case the current  $L(z)$  constraints completely the conformal blocks. We also notice that since in the  $\hbar \rightarrow 0$  limit the  $(q, t) \rightarrow (t, q)$  symmetry of  $\mathcal{V}ir_{q,t}$  reduces to the  $b_0 \leftrightarrow \frac{1}{b_0}$  symmetry, it is natural to identify the states  $\lambda_1, \lambda_2$  (16.3.4) as the  $q$ -deformation of the level-two degenerate states  $\alpha^{(1,2)} = -\frac{b_0}{2}$  and  $\alpha^{(2,1)} = -\frac{1}{2b_0}$  of the undeformed Virasoro case.

Correlation functions in 2d CFTs can be computed by decomposing them into 3-point functions and conformal blocks, by the insertion of complete sets of Virasoro descendants. 3-point functions can be determined by the bootstrap approach by requiring the associativity of the OPE, which is equivalent to the modular invariance and single valuedness of the correlators [85]. Conformal blocks can in turn be computed as series expansions in powers of the cross ratios, with coefficients obtained by repeated applications of the commutations rules of the Virasoro generators with the primary operators such as:

$$[L_m, V_\alpha(z)] = z^{m+1} \frac{\partial}{\partial z} V_\alpha(z) + \Delta(\alpha)(m+1)z^m V_\alpha(z). \quad (16.3.7)$$

There is also an alternative approach due to Dotsenko-Fateev [86] (see also [87]) which consists in deriving a Feigin-Fuchs integral representations for conformal blocks as  $n$ -point functions

of Coulomb gas vertex operators.

In the deformed case, the analogue of eq. (16.3.7) is not known and so far most of the results have been obtained via the free boson integral approach. In [76] the deformed Virasoro algebra and its free field realisation was introduced to construct singular vectors which are eigenvectors of the Macdonald operator hence proportional to the Macdonald symmetric functions. In ordinary CFT there is a similar relation between singular vectors of the Virasoro algebra and the Jack symmetric functions which in turn appears in the description of excited states in the Calogero-Sutherland model (CSM). Generalising the CFT-CSM correspondence to the  $q$ -deformed case was indeed the motivation to study the deformed Virasoro algebra in [76].

The free boson integral formulation was the central tool also in the series of works [78–80] which led to an independent derivation of the deformed Virasoro algebra. In these works the authors focused on the algebra of chiral vertex operators

$$\Phi_{\Delta_1}^{\nu_3 \nu_4}(z_1) \Phi_{\Delta_2}^{\nu_4 \nu_1}(z_2) \Big|_{\mathcal{L}_{\nu_1}} = \sum_{\nu_2} W_{\Delta_1 \Delta_2} \left[ \frac{\nu_3 \nu_2}{\nu_4 \nu_1} \right] \Phi_{\Delta_2}^{\nu_3 \nu_2}(z_2) \Phi_{\Delta_1}^{\nu_2 \nu_1}(z_1), \quad (16.3.8)$$

where the primary operators

$$\Phi_{\Delta}^{\lambda \nu}(z) : \mathcal{L}_{\lambda} \otimes \mathbb{C}[z] z^{\Delta_{\lambda} - \Delta_{\nu}}, \quad (16.3.9)$$

interpolate between irreducible representation of the algebra  $\mathcal{L}_{\lambda}$  specified by highest weight  $\Delta_{\lambda}$ . In the Virasoro case the matrix  $W_{\Delta_1 \Delta_2}$  is a constant (independent on  $z_1 z_2^{-1}$ ) solution of the Yang-Baxter equation. The idea of [78] was to consider a suitable deformation of the bosonization construction to realise chiral vertex operators which satisfy the commutation relations (16.3.8) with elliptic  $W_{\Delta_1 \Delta_2}$  matrices. Remarkably in this way they obtained the same deformed Virasoro algebra considered in [76]. This deformation of the Virasoro algebra was also identified as the dynamical symmetry of the Andrews-Baxter-Forrester (ABF) model in [79].

Recently the integral representation of the deformed Virasoro chiral blocks has been reconsidered in [88], before reviewing this work we record the integral representation of ordinary Virasoro conformal blocks. An  $M + 2$ -point conformal block is obtained by inserting  $M + 2$  vertex operators with momenta  $\alpha_a$  at positions  $z_a$ ,  $a = 0, \dots, M + 1$ , with  $z_{M+1} = \infty$ , in the background of  $N$  screening charge integrals

$$\mathcal{B}_{M+2} = \left\langle \oint dw_1 \cdots \oint dw_N V_{\alpha_0}(0) \cdots V_{\alpha_M}(z_M) S(w_1) \cdots S(w_N) \right\rangle. \quad (16.3.10)$$

The vertex operators and screening charges are given in terms of the Liouville field  $\phi(z)$ :

$$V_{\alpha}(z) =: e^{-\frac{\alpha \phi(z)}{b_0}} : , \quad S(z) =: e^{2b_0 \phi(z)} : . \quad (16.3.11)$$

It is convenient to represent conformal blocks by means of comb diagrams as shown in Fig. 16.3.1. The momentum  $\alpha_{M+1}$  is determined by remaining  $M + 1$  momenta and by the total

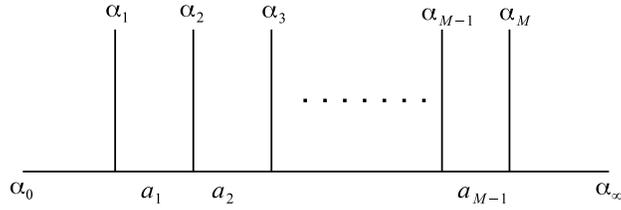

Figure 16.3.1: The comb conformal diagram for the  $M + 2$  block.

number of screening charges  $N$

$$\sum_{a=0}^{M+1} \alpha_a + 2\beta N = 2 - 2\beta. \quad (16.3.12)$$

By expanding in modes the Liouville field:

$$\phi(z) = \frac{\phi_0}{b_0} + \frac{h_0 \log z}{b_0} + \frac{1}{b_0} \sum_{k \neq 0} h_k \frac{z^{-k}}{k}, \quad (16.3.13)$$

and using the modes commutation rule

$$[h_n, h_m] = \frac{-b_0^2}{2} n \delta_{n+m, 0}, \quad (16.3.14)$$

the conformal block reduces to the following Dotsenko-Fateev (DF) integral

$$\mathcal{B}_{M+2} = \frac{1}{\prod_{a=1}^N N_a!} \oint_{\mathcal{C}_1 \dots \mathcal{C}_M} dw_1 \dots dw_N \prod_{1 \leq i \neq j \leq N} (w_i - w_j)^\beta \prod_{a=0}^M \prod_{i=1}^N (w_i - z_a)^{\alpha_a}. \quad (16.3.15)$$

The integration contour is defined by splitting the  $N$  screening integrals into  $M$  groups with  $N_a$  screening integrals each:

$$N = \sum_{a=1}^M N_a. \quad (16.3.16)$$

The contour for the  $a$ -th group encircles the segments  $\mathcal{C}_a$

$$\mathcal{C}_a : \quad [0, z_a], \quad a = 1, \dots, M. \quad (16.3.17)$$

Naively the integral (16.3.15) seems to miss some parameters. As shown in in Fig. 16.3.1, the conformal block depends in fact on the internal momenta  $a_1, \dots, a_{M-1}$ . The missing parameters are precisely the fractions of screening charges integrated along each contour [89–94], with the identifications

$$a_1 = \alpha_0 + \alpha_1 + 2\beta N_1, \quad a_k = a_{k-1} + \alpha_k + 2\beta N_k, \quad k = 2, \dots, M - 1. \quad (16.3.18)$$

In the deformed Virasoro case one promotes the modes commutation rule to a  $q$ -deformed commutation

$$[h_n, h_m] = \frac{-b_0^2}{2} n \delta_{n+m,0} \quad \rightarrow \quad [h_n, h_m] = \frac{1}{1 + (t/q)^n} \frac{1 - t^n}{1 - q^n} n \delta_{n+m,0}, \quad (16.3.19)$$

and defines bosonised vertex operators and screening charges as

$$\hat{V}_\alpha(z) = : e^{\left( -\frac{\alpha}{b_0^2} \phi_0 - \frac{\alpha}{b_0^2} h_0 \log z + \sum_{n \neq 0} \frac{1-q^{-\alpha n}}{n(1-t^{-n})} h_n z^{-n} \right)} : \quad (16.3.20)$$

$$\hat{S}(z) = : e^{\left( 2\phi_0 + 2h_0 \log z + \sum_{n \neq 0} \frac{1+(t/q)^n}{n} h_n z^n \right)} : . \quad (16.3.21)$$

The  $q$ -deformed chiral block with  $M + 2$  insertions then reads [88], [76]:

$$\mathcal{B}_{M+2}^q = \langle \oint dw_1 \cdots \oint dw_N \hat{V}_{\alpha_0}(0) \cdots \hat{V}_{\alpha_M}(z_M) \hat{S}(w_1) \cdots \hat{S}(w_N) \rangle. \quad (16.3.22)$$

By using the commutation rules (16.3.19) the block (16.3.22) reduces to the following  $q$ -deformed DF integral:

$$\mathcal{B}_{M+2}^q = \frac{C}{\prod_{a=1}^N N_a!} \oint_{\mathcal{C}_1 \cdots \mathcal{C}_M} dw_1 \cdots dw_N \Delta_{q,t}^2(w) \prod_{a=0}^M V_a(w, z_a), \quad (16.3.23)$$

where

$$\Delta_{q,t}^2(w) = \prod_{1 \leq i \neq j \leq N} \frac{(w_i/w_j; q)_\infty}{(tw_i/w_j; q)_\infty}, \quad V_a(w, z_a) = \prod_{i=1}^N \frac{(q^{\alpha_a} z_a/w_i; q)_\infty}{(z_a/w_i; q)_\infty}. \quad (16.3.24)$$

The higher rank case, involving the  $q$ - $\mathcal{W}_N$  algebra is studied in [95].

In the literature we find often another presentation of the DF integrals:

$$\begin{aligned} \mathcal{B}_{M+2} &= \int_0^1 d^{N_1} w \int_0^{\Lambda_2^{-1}} d^{N_2} w \cdots \int_0^{\Lambda_2^{-1} \cdots \Lambda_M^{-1}} d^{N_M} w \prod_{1 \leq i \neq j \leq N} \left(1 - \frac{w_i}{w_j}\right)^\beta \times \\ &\times \prod_{i=1}^{N_1 + \cdots + N_M} w_i^{\alpha_0} (1 - w_i)^{v_1} (1 - \Lambda_2 w_i)^{v_2} \cdots (1 - \Lambda_2 \cdots \Lambda_M w_i)^{v_M}, \end{aligned} \quad (16.3.25)$$

it is easy to find a dictionary relating the parameters  $v_i$  to the momenta  $\alpha_i$  and the cross ratios  $\Lambda_i$  to the  $z_i$  in eq. (16.3.15), so the two presentations are equivalent. The DF integral (16.3.25) can be promoted to the  $q$ -deformed case by replacing

$$\prod_{1 \leq i \neq j \leq N} (w_i - w_j)^\beta \rightarrow \prod_{1 \leq i \neq j \leq N} \prod_{k=0}^{\beta} (w_i - q^k w_j), \quad (1-x)^c \rightarrow \prod_{n=0}^{c-1} (1 - q^n x), \quad (16.3.26)$$

and the integration measure by the Jackson measure  $dx \rightarrow d_q x$  defined as

$$\int_0^1 f(x) d_q x = (1-q) \sum_{k=0}^{\infty} q^k f(q^k). \quad (16.3.27)$$

In the end one arrives at the  $q$ -deformed DF integral [96]:

$$\begin{aligned} \mathcal{B}_{M+2}^q &= \int_0^1 d_q^{N_1} w \int_0^{\Lambda_2^{-1}} d_q^{N_2} w \cdots \int_0^{\Lambda_2^{-1} \cdots \Lambda_M^{-1}} d_q^{N_M} w \prod_{1 \leq i \neq j \leq N} \prod_{k=0}^{\beta-1} \left(1 - q^k \frac{w_i}{w_j}\right)^\beta \\ &\times \prod_{i=1}^{N_1 + \cdots + N_M} w_i^{\alpha_0} \prod_{k=0}^{v_1-1} (1 - q^k w_i) \prod_{k=0}^{v_2-1} (1 - q^k \Lambda_2 w_i) \cdots \prod_{k=0}^{v_M-1} (1 - q^k \Lambda_2 \cdots \Lambda_M w_i), \end{aligned} \quad (16.3.28)$$

which can be shown to be equivalent to (16.3.23) for integer values of  $\beta$  and of the momenta. Actually the expressions in (16.3.24) provide the analytic continuation to non-integer values of the products in (16.3.26).

### 16.3.2 $\mathcal{Vir}_{q,t}$ chiral blocks and instanton-vortex counting

In this section we will discuss the map between  $\mathcal{Vir}_{q,t}$  chiral blocks and  $\mathbb{R}^4 \times S^1$  instantons or  $\mathbb{R}^2 \times S^1$  vortex partition functions. The  $q, t$  parameter appearing in the deformed Virasoro algebra are identified with the equivariant parameters in the instanton partition function  $q = e^{R\epsilon_1}$ ,  $t = e^{-R\epsilon_2}$  with  $R$  the radius of the  $S^1$ .<sup>5</sup>

The first evidence of this map is the very neat result of [97] (see also [98]) where the  $q$ -deformed version of the so-called Gaiotto-Whittaker states [99] was constructed. The deformed analogue of the Gaiotto-Whittaker states  $|G\rangle$  are states in the Verma module  $M_h$  satisfying:

$$T_1|G\rangle = \Lambda^2 G, \quad T_n|G\rangle = 0 \quad (n \geq 2) \quad \Lambda^2 \in \mathbb{C}, \quad (16.3.29)$$

and normalised such that  $|G\rangle = |h\rangle + \cdots$  where  $|h\rangle$  is an highest weight vector ( $T_n|h\rangle = 0$ , for  $n > 0$ ,  $T_0|h\rangle = h|h\rangle$ ,  $h \in \mathbb{C}$ ). The inner product  $\langle G|G\rangle$  can be computed using the free boson realisation of  $\mathcal{Vir}_{q,t}$  and it can be shown that

$$\langle G|G\rangle = \mathcal{Z}_{inst}^{5d}[SU(2)], \quad (16.3.30)$$

where  $\mathcal{Z}_{inst}^{5d}[SU(2)]$  is the instanton partition function of the  $5d \mathcal{N} = 1$  pure  $SU(2)$  theory and the parameter  $\Lambda^2$  is identified with the instanton counting parameter. This result has been generalised to higher rank in [100].

Moving to multipoint correlators, we have to rely on the  $q$ -DF integral representation discussed in the previous section since, as we mentioned, the OPE approach in the  $q$ -deformed case is not well developed. This fact also implies that at the moment we cannot evaluate the correlators at generic values of external and internal momenta since they will have to satisfy conditions like (16.3.12), hence we can only test the correspondence with 5d instanton partition functions at special points in the moduli space.

The undeformed AGT correspondence associates to the sphere with  $M + 2$  punctures the  $M + 2$ -point correlator on the CFT side and the  $\mathcal{N} = 2$ ,  $2 + SU(2)^{M-1} + 2$  linear quiver on

---

<sup>5</sup>The parameter  $t$  in this section is the inverse of the parameter  $t$  appearing in section 16.2.2.

the gauge theory side, one would then expect an analogous map between the  $M + 2$ -point block in  $\mathcal{V}ir_{q,t}$  and the 5d  $\mathcal{N} = 1, 2 + SU(2)^{M-1} + 2$  quiver theory.

However it is important to notice that in 5d the  $2 + SU(2)^{M-1} + 2$  theory is dual to the  $M + SU(M) + M$  theory (more generally the duality relates  $K + SU(K)^{M-1} + K$  to  $M + SU(M)^{K-1} + M$  theories) [101,102]. A neat way to understand this duality is to consider the geometric engineering perspective. In fact both theories can be engineered by a IIA compactification on the same toric Calabi-Yau threefold, whose toric diagram for the  $M = 3$  case is depicted in Fig. 16.3.2. The topological string partition function  $Z_{top}$  on this CY

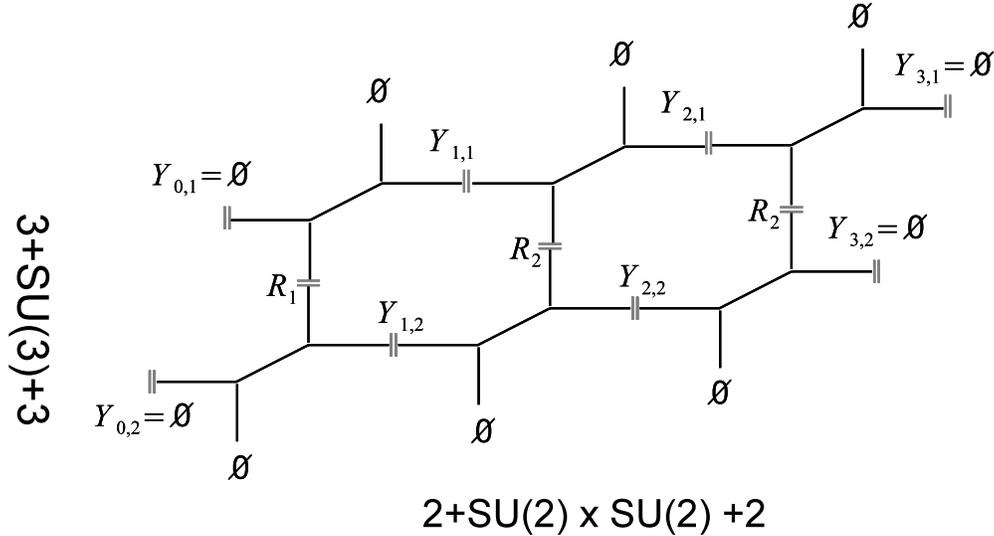

Figure 16.3.2: The toric diagram of the CY geometry engineering either  $3 + SU(3) + 3$  or  $2 + SU(2)^2 + 2$ .

can be computed by means of the refined vertex formalism [63]. One has to glue trivalent vertices by summing over sets of representations associated to each internal leg. In general it is not possible to perform all the sums in a closed form and one typically gets a perturbative expansion in powers of the Kähler parameters of the legs with representations left to sum.

For example in the case of Fig. 16.3.2 one can resum all the reps associated to the diagonal and vertical legs and obtain a perturbative expansion in the Kähler parameters of the horizontal legs with Young tableaux  $Y_{1,1}, Y_{1,2}$  and  $Y_{2,1}, Y_{2,2}$ . The result one gets in this way can be identified with the 5d  $2 + SU(2)^2 + 2$  instanton partition function with the Kähler parameters of the horizontal legs mapped to 5d gauge couplings of the two nodes.

Alternatively one can resum first the diagonal and horizontal legs and obtain a perturbative expansion in the Kähler parameters associated to the vertical legs with Young tableaux  $R_1, R_2, R_3$ . This expansion can be mapped to the  $3 + SU(3) + 3$  instanton partition function. The fact that the two ways of performing the sum are equivalent requires the non-trivial slicing invariance property of the refined topological vertex. The dictionary relating the topological string Kähler parameters to the Coulomb, gauge coupling and mass parameters

in two dual gauge theories can be found in [103].

As a result of the discussion above, the  $M + 2$ -point  $q$ -DF block is expected to be related to both these 5d theories. As we will see it turns out that there are two distinct evaluation methods which yield the two instanton expansions.

In [88] it was devised a procedure to evaluate the  $q$ -DF  $M + 2$ -point block (16.3.23) by residues computation. The integrand in (16.3.23) is a meromorphic function, poles come from the zeros of the  $q$ -products  $\prod_{k=1}^{\infty}(1 - q^k z)$  in the denominator located at  $z = q^{-k}$ . By taking into account carefully that certain poles are cancelled by the zeros of the  $q$ -products in the numerator, it can be shown that the poles enclosed by each integration contour  $\mathcal{C}_a$  where  $N_a$  screening charges are integrated, are labelled by Young tableaux  $R_a$  with at most  $N_a$  rows. Basically one finds:

$$\frac{1}{N_1!} \oint_{\mathcal{C}_1} dw^{N_1} \cdots \frac{1}{N_M!} \oint_{\mathcal{C}_M} dw^{N_M} \rightarrow \sum_{R_1, \dots, R_M} . \quad (16.3.31)$$

By taking the residues at these sets of poles in (16.3.23) the result very nicely organises as the 5d Nekrasov partition function for the  $M + SU(M) + M$  theory:

$$\mathcal{B}_{M+2}^q = \sum_{R_1, \dots, R_M} \Lambda^{\sum_a |R_a|} \frac{z_{fund}(\vec{R}) z_{anti-fund}(\vec{R})}{z_{vec}(\vec{R})} = Z_{inst}^{5d}[M + SU(M) + M]. \quad (16.3.32)$$

where  $\vec{R} = (R_1, \dots, R_M)$ . For details on how the gauge theory parameters are mapped to the  $q$ -DF we refer the reader to [88], [104]. Notice that, since as discussed above the sets of representations are non-generic and the mass and Coulomb parameters via the dictionary are identified with momenta satisfying the conditions (16.3.18), the 5d theory is at a special point in the moduli space where the Higgs branch and the Coulomb branch meet at the origin. The non-restricted 5d theory was conjectured to emerge via geometric-transition in the large N limit.

In [88], [95], it was also observed that the  $M + 2$ -point block (16.3.23) can be directly identified with the block integral  $Z^{3d}$ , discussed in section 16.2.1, of a 3d  $SU(N)$  theory with  $2M$  flavours and one adjoint. Indeed the screening charge contributions  $\Delta_{q,t}^2(w)$  and the vertices  $V_a(w, z_a)$  in eq. (16.3.24) can be respectively identified with the vector and hypermultiplets contribution to the 3d block integral. In the end one finds a triality relation:

$$\mathcal{B}_{M+2}^q = Z^{3d} = Z_{inst}^{5d}[M + SU(M) + M]. \quad (16.3.33)$$

The 3d theory is interpreted as the theory studied in [58], [105], on charge N vortices in the 5d gauge theory.

The relation between free field correlators in  $q$ -Virasoro and 3d gauge theories partition functions has been recently discussed in [106]. The authors showed that it is possible to map 3d  $\mathcal{N} = 2$  partition functions on the 3-manifolds  $M_g^{3d}$  to free field correlators of the  $q$ -Virasoro modular double.

We now turn to the second evaluation method of the  $q$ -DF integrals yielding the dual instanton expansion. We begin by recording the schematic form of the instanton expansion of the  $2 + SU(2)^{M-1} + 2$  quiver theory:

$$\frac{Z_{inst}^{5d}[2 + SU(2)^{M-1} + 2] = \sum_{\vec{Y}_a} \Lambda_1^{|\vec{Y}_1|} \cdots \Lambda_{M-1}^{|\vec{Y}_{M-1}|} z_{fund}(\vec{Y}_1) z_{bifund}(\vec{Y}_1, \vec{Y}_2) \cdots z_{bifund}(\vec{Y}_{M-1}, \vec{Y}_{M-1}) z_{anti-fund}(\vec{Y}_{M-1})}{z_{vec}(\vec{Y}_1) z_{vec}(\vec{Y}_2) \cdots z_{vec}(\vec{Y}_{M-1})}, \quad (16.3.34)$$

where  $\vec{Y}_a$  is a two component Young Tableau and  $\Lambda_1 \cdots \Lambda_{M-1}$  the gauge couplings. In the 4d/undeformed case this structure suggested to look for an analogous decomposition of conformal blocks on a basis of states labelled by the Young tableaux  $\vec{Y}_a$ , this is the so-called Nekrasov decomposition of the conformal blocks:

$$\begin{aligned} & \langle V_{\alpha_0}(0) V_{\alpha_1}(1) V_{\alpha_2}(\alpha_2) \cdots V_{\alpha_{M+1}}(\infty) \rangle \sim \\ & \sum_{\vec{Y}_a} \langle V_{\alpha_0}(0) | V_{\alpha_1}(1) | \tilde{\alpha}_1, \vec{Y}_1 \rangle \langle \tilde{\alpha}_1, \vec{Y}_1 | V_{\alpha_2}(\alpha_2) | \tilde{\alpha}_2, \vec{Y}_2 \rangle \cdots \\ & \cdots \langle \tilde{\alpha}_{M-1}, \vec{Y}_{M-1} | V_{\alpha_M}(\alpha_M) | V_{\alpha_{M+1}}(\infty) \rangle, \end{aligned} \quad (16.3.35)$$

where the symbol  $\sim$  is due to the omission of the so-called  $U(1)$  factor that one needs to strip-off from the Nekrasov partition function in order to match with the CFT results. This factor plays a crucial role in [107], [108] where this basis was identified as a special orthogonal basis of states for the algebra  $Vir \otimes \mathcal{H}$ , the tensor product of Virasoro and Heisenberg algebras. Besides rendering much simpler the evaluation of the coefficients of the OPE this basis has a clear interpretation as the class of fixed points in the equivariant cohomology of the instanton moduli space.<sup>6</sup>

Unfortunately lifting directly this approach to the deformed case is problematic since, as we already mentioned, the OPE approach in the deformed case is not known, however one can try to find a similar decomposition of the  $q$ -DF integrals in terms of these states. This idea has been developed in a series of papers [93, 94, 111, 112]. The authors initially focused on the 4-point block in the undeformed Virasoro case which can be schematically expressed as:

$$\mathcal{B}_{2+2} = \int_{\mathcal{C}_1} d\mu(x) \int_{\mathcal{C}_2} d\mu(y) \mathbb{I}^2(x, y), \quad (16.3.36)$$

where  $x = (x_1, \cdots, x_{N_1})$  and  $y = (y_1, \cdots, y_{N_2})$  indicate the two sets of screening charges variables integrated on the first and second contours respectively. We refer the reader to [112] for the explicit definition of the factors  $d\mu(x)$ ,  $d\mu(y)$ , which can be identified with the so-called Selberg measure, and of the cross term  $\mathbb{I}^2(x, y)$ . The idea was to express the cross term by means of the completeness of a set of new orthogonal polynomials  $K_{\vec{Y}}(x)$  labelled by Young tableaux  $\vec{Y} = Y_1, Y_2$ . These polynomials are a generalisation of Jack polynomials depending on two reps which, in the  $\beta = 1$  case, reduce to the products of two Schur polynomials  $K_{\vec{Y}}(x) = \chi_{Y_1} \chi_{Y_2}$ . Using the completeness of these polynomials

$$\mathbb{I}^2(x, y) = \sum_{\vec{Y}} \Lambda^{|\vec{Y}|} K_{\vec{Y}}(x) K_{\vec{Y}}^*(y), \quad (16.3.37)$$

---

<sup>6</sup> The action of the  $W_N$  algebra on the instanton moduli space is discussed [109], [110].

the 4-point function can be expressed as a double Selberg average:

$$\mathcal{B}_{2+2} = \int_{\mathcal{C}_1} d\mu(x) \int_{\mathcal{C}_2} d\mu(y) \mathbb{I}^2(x, y) = \sum_{\vec{Y}} \Lambda^{|\vec{Y}|} \int_{\mathcal{C}_1} d\mu(x) K_{\vec{Y}}(x) \int_{\mathcal{C}_2} d\mu(y) K_{\vec{Y}}^*(y). \quad (16.3.38)$$

The explicit evaluation of these Selberg averages remarkably yields

$$\int_{\mathcal{C}_1} d\mu(x) K_{\vec{Y}}(x) \int_{\mathcal{C}_2} d\mu(y) K_{\vec{Y}}^*(y) = \frac{z_{fund}(\vec{Y}) z_{antifund}(\vec{Y})}{z_{vec}(\vec{Y})}, \quad (16.3.39)$$

hence one reconstructs the instanton expansion for the  $2 + SU(2) + 2$  theory:

$$\mathcal{B}_{2+2} = \sum_{\vec{Y}} \Lambda^{|\vec{Y}|} \frac{z_{fund}(\vec{Y}) z_{antifund}(\vec{Y})}{z_{vec}(\vec{Y})} = Z_{inst}^{4d}[2 + SU(2) + 2]. \quad (16.3.40)$$

This result has been generalised to the  $q$ -deformed case for  $q = t$  in [96] and then for generic  $q, t$  in [113]. In this latter case one needs to introduce a new set of polynomials, combinations of Macdonalds polynomials to prove that

$$\mathcal{B}_{2,2}^q = Z_{inst}^{5d}[2 + SU(2) + 2]. \quad (16.3.41)$$

The generalisation to multipoint blocks has been studied in [114]. We refer the reader to the original paper, here we record only the key steps leading to the final result. First one introduces an object called *generalised bifundamental kernel*  $\widetilde{N}_{\vec{Y}_{a-1}, \vec{Y}_a}$ . For  $q = t$  this kernel admits a factorised form in terms of skew Schur polynomials:

$$\widetilde{N}_{\vec{Y}_{a-1}, \vec{Y}_a} = N_{Y_{a-1,1} Y_{a,1}} N_{Y_{a-1,2} Y_{a,2}}, \quad N_{A,B}[x] = \sum_C \chi_{A/C}^*[y] \chi_{B/C}[y]. \quad (16.3.42)$$

The first result is that one can express the  $M + 2$ -point block in terms of  $q$ -Selberg averages of the generalised bifundamental kernels:

$$\mathcal{B}_{M+2}^q = \sum_{\vec{Y}_a} \prod_{a=1}^M \Lambda_a^{|\vec{Y}_a|} \langle \widetilde{N}_{\vec{Y}_{a-1}, \vec{Y}_a} \rangle, \quad (16.3.43)$$

with  $\vec{Y}_0 = \vec{Y}_M = \emptyset$ . One can then prove that:

$$\langle \widetilde{N}_{\vec{Y}_{a-1}, \vec{Y}_a} \rangle \sim \frac{z_{bif}[\vec{Y}_{a-1}, \vec{Y}_a]}{z_{vec}(\vec{Y}_{a-1})^{1/2} z_{vec}(\vec{Y}_a)^{1/2}}, \quad (16.3.44)$$

which, by considering the form of the quiver instanton partition function in (16.3.34), leads to

$$\mathcal{B}_{M+2}^q = Z_{inst}^{5d}[2 + SU(2)^{M-1} + 2]. \quad (16.3.45)$$

This provides a proof of the “standard” 5d lift of the AGT correspondence. However [114] managed to prove that there is a finer structure. They showed that the  $q$ -DF integral can

in fact be directly decomposed in terms of resolved conifold topological string amplitudes  $[Z_{top}]_{Y_1, Y_2}^{R_1, R_2}$ , where  $R_{1,2}$  and  $Y_{1,2}$  are the representations respectively carried by the external vertical and horizontal legs. In particular the average of the bifundamental kernel decomposes as:

$$\langle \widetilde{N}_{\vec{Y}_{a-1}, \vec{Y}_a} \rangle \sim \sum_R Q_f^{|R|} [Z_{top}]_{Y_{a-1,1}, Y_{a,1}}^{0, R^T} [Z_{top}]_{Y_{a-1,2}, Y_{a,2}}^{R, 0} =$$

The sum over the representation  $R$  is the result of the  $q$  average. As we have already mentioned the integrands are typically meromorphic functions and integrals are evaluated by summing sets of poles labelled by Young tableaux (with finite number of rows). The Kähler parameter  $Q_f$ , associated to the internal vertical leg carrying the representation  $R$ , is related to Coulomb branch parameter. In conclusion the  $M + 2$ -point block can be directly mapped to the topological string partition function for the CY geometry depicted (for  $M = 3$ ) in Fig. 16.3.2:

$$\mathcal{B}_{M+2} = \sum_{\vec{Y}_a} \sum_{R_a} \prod_{a=1}^M \Lambda_a^{|\vec{Y}_a|} Q_{f_a}^{|R_a|} [Z_{top}]_{Y_{a-1,1}, Y_{a,1}}^{0, R_a^T} [Z_{top}]_{Y_{a-1,2}, Y_{a,2}}^{R_a, 0}, \quad (16.3.46)$$

with  $\vec{Y}_0 = \vec{Y}_M = \emptyset$ . This is the most fundamental decomposition of the  $q$ -deformed DF blocks.

Recently it has been observed that DF and gauge theory matrix integrals can be considered as special cases of a more general class of matrix models, the so-called network matrix models which have a direct topological string interpretation. The symmetry of these matrix models is the Ding-Iohara-Miki algebra which has been conjectured to be the underlying symmetry of the AGT correspondence, see for example [115] and references therein.

We close this section by mentioning a further approach to the evaluation of (deformed) DF-integrals. In [92] it was shown that  $q$ -deformed blocks involving 3-generic primaries operators plus any number of operators with specialised momentum (corresponding to level-2 degenerates) are given by multivariate basic hypergeometric series. For example it is easy to see that if in the  $q$ -DF integral (16.3.23) we take arbitrary  $\alpha_0, \alpha_1, \alpha_{M+1}$  and specialise  $\alpha_i = -1$  for  $i = 2, \dots, M$  such that the corresponding vertices become

$$V_i(w, x_i) = \prod_{j=1}^N \frac{(q^{\alpha_i} x_i / w_j; q)_\infty}{(x_i / w_j; q)_\infty} \rightarrow \prod_{j=1}^N (1 - q^{-1} x_i / w_j), \quad (16.3.47)$$

the integral can be mapped to the Jackson integral studied in [116].<sup>7</sup> This integral can be exactly evaluated and yields (up to prefactors) a basic hypergeometric functions of  $M$  variables:

$$\mathcal{B}_{M+2}(x_1, \dots, x_M) \sim {}_2\Phi_1(A, B; C; x_1, \dots, x_M),$$

where the coefficients  $A, B, C$  are functions of the 3 generic momenta. For example, in the case of a 4-point block with 3 generic and one degenerate insertion one finds:

$$\mathcal{B}_{2+2}(z) = {}_2\Phi_1(A, B; C; z), \quad (16.3.48)$$

which is annihilated by the difference operator

$$D(A, B; C; q; z)\mathcal{B}_{\alpha_0, \alpha_1, \alpha_2}(z) = 0, \quad (16.3.49)$$

$$D(A, B; C; q; z) = h_2 \frac{\partial_q^2}{\partial_q z^2} + h_1 \frac{\partial_q}{\partial_q z} + h_0, \quad (16.3.50)$$

where  $\frac{\partial_q}{\partial_q z} f(z) = \frac{f(qz) - f(z)}{z(q-1)}$  and the coefficients  $h_2, h_1, h_0$  are defined by

$$\begin{aligned} h_2 &= z(C - ABqz), \\ h_1 &= \frac{1 - C}{1 - q} + \frac{(1 - A)(1 - B) - (1 - ABq)}{(1 - q)} z, \\ h_0 &= -\frac{(1 - A)(1 - B)}{(1 - q)^2}. \end{aligned} \quad (16.3.51)$$

By removing the  $q$ -deformation this difference operator reduces to the familiar hypergeometric differential operator acting on level-two degenerate 4-point correlators.

As we discussed in section 16.2.3, we expect a map between  $\mathcal{V}ir_{q,t}$  blocks with some of the momenta analytically continued to degenerate values and instanton-vortex partition functions associated to linear quivers with defects obtained via Higgsing. In particular the block  $\mathcal{B}_{2+2}$  in (16.3.48), in analogy with the undeformed case, is expected to be mapped to the vortex partition function of the 3d  $\mathcal{N} = 2$  QED with 2 flavours, describing the codimension-two defect theory obtained by Higgsing the 5d  $2 + SU(2) + 2$  theory (after normalizing by the contributions of 3-point functions and 5d free hypers). Indeed we see that  $\mathcal{B}_{2+2}$  is given by a  $q$ -deformed hypergeometric series as the  $\mathcal{N} = 2$  QED vortex partition function, so the two quantities can be mapped with a suitable dictionary.

## 16.4 3d & 5d partition functions as $q$ -deformed correlators

Having reviewed the identification of instanton/vortex partition functions with non-degenerate/degenerate chiral  $\mathcal{V}ir_{q,t}$  blocks we now move to the construction of  $\mathcal{V}ir_{q,t}$  correlators and discuss their map to 3d and 5d partition functions.

<sup>7</sup>The measure in [116] is different from the Macdonald measure in (16.3.23) but they actually give the same results up to prefactors independent on  $x$ , see for example the discussion in Appendix C of [117].

The first question one needs to address is how to combine  $\mathcal{V}ir_{q,t}$  chiral blocks into a correlator. In the undeformed 2d CFT case, the underlying symmetry is the product of the holomorphic and anti-holomorphic copies of the Virasoro algebra and correlators are constructed by taking the modulus square of the holomorphic and anti-holomorphic conformal blocks. This ensures that the monodromies acquired by the chiral blocks under change of channel (or ordering of the OPE) cancel out in the physical correlators which are modular invariant and single-value objects.  $\mathcal{V}ir_{q,t}$  chiral blocks don't have monodromies since, they have lines of poles rather than branch-cuts. This is clear if we consider for example the degenerate chiral blocks discussed in the previous section, given by  $q$ -deformed hypergeometric series.

In [118], [48] it was proposed to define deformed correlators by combining  $\mathcal{V}ir_{q,t}$  chiral blocks with the  $SL(3, \mathbb{Z})$  gluing rules described in section 16.2.2. In particular the authors considered the  $S^4 \times S^1$  and  $S^5$  gluings and defined two families of correlators with respectively  $\mathcal{V}ir_{q,t} \otimes \mathcal{V}ir_{q,t}$  and  $\mathcal{V}ir_{q,t} \otimes \mathcal{V}ir_{q,t} \otimes \mathcal{V}ir_{q,t}$  symmetry. In the first case the blocks are glued with the  $id$ -gluing (16.2.51), while in the second case with the  $S$ -gluing (16.2.27). Correspondingly these two families were called  $id$ - and  $S$ -correlators and it was proposed the following 5d-lift of the AGT correspondence relating  $M + 2$ -point  $id$ - and  $S$ -correlators to  $S^4 \times S^1$  and  $S^5$  partition functions of the  $2 + SU(2)^{M-1} + 2$  linear quiver:

$$\begin{aligned} Z^{S^5} [2 + SU(2)^{M-1} + 2] &= \int d\sigma Z_{1\text{-loop}}^{S^5}(\sigma, \vec{M}) \left\| \mathcal{Z}_{cl} \mathcal{Z}_{inst}^{5d} \right\|_S^3 = \\ &= \int da C^S \dots C^S \left\| \mathcal{C}_q \mathcal{B}_{M+2}^q \right\|_S^3 = \langle V_{\alpha_\infty}(\infty) V_{\alpha_M}(z_M) \dots V_{\alpha_1}(z_1) V_{\alpha_0}(0) \rangle_S, \end{aligned} \quad (16.4.1)$$

$$\begin{aligned} Z^{S^4 \times S^1} [2 + SU(2)^{M-1} + 2] &= \int d\sigma Z_{1\text{-loop}}^{S^4 \times S^1}(\sigma, \vec{M}) \left\| \mathcal{Z}_{cl} \mathcal{Z}_{inst}^{5d} \right\|_{id}^2 = \\ &= \int da C^{id} \dots C^{id} \left\| \mathcal{C}_q \mathcal{B}_{M+2}^q \right\|_{id}^3 = \langle V_{\alpha_\infty}(\infty) V_{\alpha_M}(z_M) \dots V_{\alpha_1}(z_1) V_{\alpha_0}(0) \rangle_{id}. \end{aligned} \quad (16.4.2)$$

In detail the map goes as follows. The instanton and classical contributions are identified with the  $\mathcal{V}ir_{q,t}$  chiral blocks:

$$\mathcal{Z}_{cl} \mathcal{Z}_{inst}^{5d} = \mathcal{C}_q \mathcal{B}_{M+2}. \quad (16.4.3)$$

In the previous section we have discussed the map  $\mathcal{Z}_{inst}^{5d} = \mathcal{B}_{M+2}$  for special values of the momenta and mentioned that the match should extend to generic momenta via geometric transition.

The classical terms are instead conjectured to map to the factors  $\mathcal{C}_q$ , which were interpreted as the deformed version of the conformal factors, to which they reduce in the  $q \rightarrow 1$  limit. In the undeformed case these factors follow from the conformal Ward identities. In the  $q$ -deformed case at present it is not know how to derive the analogue of these identities, however an interesting discussion on the  $q$ -deformation of the  $SU(1, 1)$  Ward identities can be found in [119].

The key point is then to map the 1-loop factors to the 3-point functions contribution which we schematically indicated as  $C^S \dots C^S$  or  $C^{id} \dots C^{id}$ . We will discuss this point in

a moment, before doing so it is useful to note that the correspondences (16.4.1), (16.4.2), generate via analytic continuation/Higgsing, a series of secondary correspondences between  $id$ ,  $S$ -correlators with degenerate insertions and  $S^4 \times S^1$ ,  $S^5$  partition functions decorated by the  $S^2 \times S^1$ ,  $S^3$  partition functions describing the codimension-two defects. For example one expects the map of the  $id$  and  $S$ -correlators of 3 generic primaries and one level-two degenerate primary  $V_{\alpha_2}(z) = V_{deg}(z)$  (normalised by the 3-point function of the non-degenerate primaries) to the partition functions of the  $\mathcal{N} = 2$  SQED with 2 flavours on  $S^2 \times S^1$ ,  $S^3$  (normalised by the contribution of the free 5d hypers):

$$Z_{S^3}^{SQED} = \sum_i^2 G_{1\text{-loop}}^{(i)} \left\| \mathcal{G}_{cl}^{(i)} \mathcal{Z}_V^{(i)} \right\|_S^2 = \langle V_{\alpha_4}(\infty) V_{\alpha_3}(1) V_{deg}(z) V_{\alpha_0}(0) \rangle_S, \quad (16.4.4)$$

$$Z_{S^2 \times S^1}^{SQED} = \sum_i^2 G_{1\text{-loop}}^{(i)} \left\| \mathcal{G}_{cl}^{(i)} \mathcal{Z}_V^{(i)} \right\|_{id}^2 = \langle V_{\alpha_4}(\infty) V_{\alpha_3}(1) V_{deg}(z) V_{\alpha_0}(0) \rangle_{id}. \quad (16.4.5)$$

The correspondences (16.4.4) and (16.4.5) indicate that the degenerate 4-point correlators will be  $SL(2, \mathbb{Z})$   $id$ - or  $S$ -squares of degenerate blocks hence, they will be annihilated by two hypergeometric difference operators (see also the discussion on the evaluation of the degenerate block integral (16.3.48)):

$$\langle V_{\alpha_4}(\infty) V_{\alpha_3}(1) V_{deg}(z) V_{\alpha_1}(0) \rangle_* \sim G(z, \tilde{z}), \quad (16.4.6)$$

$$D(A, B; C; q; z) G(z, \tilde{z}) = 0, \quad D(\tilde{A}, \tilde{B}; \tilde{C}; \tilde{q}; \tilde{z}) G(z, \tilde{z}) = 0. \quad (16.4.7)$$

The parameters  $A, B, C$  are functions of the momenta  $\alpha_1, \alpha_3, \alpha_4$ , un-tilded and tilded variables denote the parameters in the two chiral blocks and the subscript  $*$  indicate either the  $id$  or  $S$  gluing.

This observation was used in [118] to derive 3-point functions by means of the bootstrap approach [85], [120]. Eqs. (16.4.7) imply that  $G(z, \tilde{z})$  can be expressed as a bi-linear combination of solutions of the  $q$ -hypergeometric difference equation. Let  $I_{1,2}^{(s)}$  be a basis of two linearly independent solutions in the neighbourhood of  $z = 0$ , then we can write:

$$\langle V_{\alpha_4}(\infty) V_{\alpha_3}(1) V_{deg}(z) V_{\alpha_1}(0) \rangle_* \sim \sum_{i=1}^2 K_i^{(s)} \left\| I_i^{(s)}(z; q) \right\|_*^2, \quad (16.4.8)$$

where the coefficients  $K_i^{(s)}$  are related to the 3-point function factor associated to the diagram on the left of Fig. 16.4.1.

Similarly in the  $u$ -channel the correlation function is a bilinear combination of solutions  $I_{1,2}^{(u)}$  in the neighbourhood of  $z = \infty$ :

$$\langle V_{\alpha_4}(\infty) V_{\alpha_3}(r) V_{deg}(z) V_{\alpha_1}(0) \rangle \sim \sum_{i=1}^2 K_i^{(u)} \left\| I_i^{(u)}(z; q) \right\|_*^2, \quad (16.4.9)$$

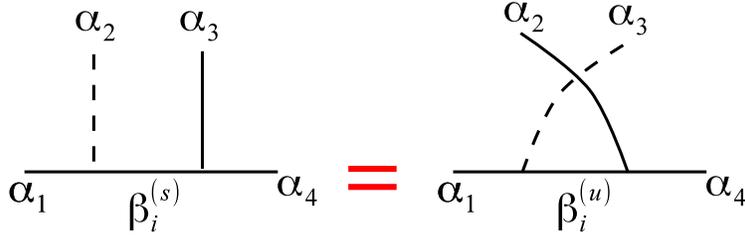

Figure 16.4.1: Crossing symmetry requires the equality of correlations involving chiral blocks in the  $s$ -channel (on the LHS) and in the  $u$ -channel (on the RHS).

with coefficient  $K_i^{(u)}$  related to the 3-point functions factor associated to the diagram on the right of Fig. 16.4.1.

To bootstrap the 3-point functions we now impose crossing symmetry requiring the equality of  $s$ - and  $u$ -channel correlators:

$$K_1^{(s)} \left\| \left\| I_1^{(s)} \right\|_* \right\|^2 + K_2^{(s)} \left\| \left\| I_2^{(s)} \right\|_* \right\|^2 = K_1^{(u)} \left\| \left\| I_1^{(u)} \right\|_* \right\|^2 + K_2^{(u)} \left\| \left\| I_2^{(u)} \right\|_* \right\|^2. \quad (16.4.10)$$

We then take the analytic continuation to the neighbourhood of  $\infty$  of the solutions  $I_i^{(s)}$  and express them as linear combination of  $u$ -channel solutions. At this point eq. (16.4.10) yields a set of non-trivial equations for the coefficients  $K_i^{(s)}$  and  $K_i^{(u)}$  which determine the 3-point functions uniquely once the gluing rule is specified.

In the case of  $id$ -gluing there are two types of level-two degenerate primaries:  $\alpha_2 = -\frac{b_0^{\pm 1}}{2}$  (corresponding to the two  $S^2 \times S^1$  defects inside  $S^4 \times S^1$ ) and we can write two sets of equations for the 3-point function. The unique solution (up to  $q$ -constants) to these equations is given by:

$$C^{id}(\alpha_3, \alpha_2, \alpha_1) = \frac{1}{\Upsilon^R(2\alpha_T - Q_0)} \prod_{i=1}^3 \frac{\Upsilon^R(2\alpha_i)}{\Upsilon^R(2\alpha_T - 2\alpha_i)}, \quad (16.4.11)$$

where  $2\alpha_T = \alpha_1 + \alpha_2 + \alpha_3$  while the parameter  $R$  is related to the deformation parameter of the algebra and to the  $S^1$  radius of the  $S^4 \times S^1$  geometry on the gauge theory side. The definition and useful properties of the  $\Upsilon^R(X)$  function are collected in the Appendix 16.5.

Similarly, for  $S$ -correlators there are three types of degenerations  $\alpha_2 = -\frac{\omega_i}{2}$  for  $i = 1, 2, 3$  (corresponding to the three large  $S^3$  inside  $S^5$ ) and we can write three sets of equations with unique solution given by:

$$C^S(\alpha_3, \alpha_2, \alpha_1) = \frac{1}{S_3(2\alpha_T - E)} \prod_{i=1}^3 \frac{S_3(2\alpha_i)}{S_3(2\alpha_T - 2\alpha_i)}. \quad (16.4.12)$$

We can now complete the map between  $q$ -deformed correlators and partition functions. For example it is easy to check that the 3-point functions factor in the 4-point  $S$ -correlator

can be mapped to the  $S^5$  one-loop contribution of the  $2 + SU(2) + 2$  theory:

$$C^S(\alpha_1, \alpha_2, \alpha)C^S(E - \alpha, \alpha_3, \alpha_4) = Z_{1\text{-loop}}^{S^5, \text{vect}}(\sigma) \prod_{i=1}^4 Z_{1\text{-loop}}^{S^5, \text{hyper}}(\sigma, m_i),$$

where the 1-loop factors for the vector multiplet and for the fundamental hypers are defined in eqs. (16.2.33), and masses and momenta are mapped by the following dictionary:

$$\alpha = i\sigma + \frac{E}{2}, \quad \alpha_1 \pm \alpha_2 = im_{1,2} + E, \quad \alpha_3 \pm \alpha_4 = im_{3,4} + E. \quad (16.4.13)$$

Similarly for  $id$ -correlators one can show that:

$$C_{id}(\alpha_1, \alpha_2, \alpha)C_{id}(Q_0 - \alpha, \alpha_3, \alpha_4) = Z_{1\text{-loop}}^{S^4 \times S^1, \text{vect}}(\sigma) \prod_{i=1}^4 Z_{1\text{-loop}}^{S^4 \times S^1, \text{hyper}}(\sigma, m_i), \quad (16.4.14)$$

with the following dictionary:

$$\alpha = i\sigma + \frac{Q_0}{2}, \quad \alpha_1 \pm \alpha_2 = im_{1,2} + Q_0, \quad \alpha_3 \pm \alpha_4 = im_{3,4} + Q_0. \quad (16.4.15)$$

3-point functions factor in higher point  $S$ ,  $id$ -correlators can be similarly mapped to 1-loop contributions in  $S^5$  and  $S^4 \times S^1$  linear quiver partition functions. In [48] it was also shown that the 3-point function contribution to the 1-punctured torus  $S$ ,  $id$ -correlators can be mapped to the 1-loop factor of the  $SU(2)$  theory with a massive adjoint hyper on  $S^5$  and  $S^4 \times S^1$ .

It is possible to take a smooth limit which removes the  $q$ -deformation and reduces  $id$ -correlators to Liouville correlators. On the gauge theory side this limit corresponds to shrinking the  $S^1$  radius and reducing to the  $S^4$  partition function. Indeed for  $R \rightarrow 0$ , the 3-point function (16.4.11) smoothly reduces to the familiar DOZZ formula for the Liouville 3-point function [121], [122], [120], which via AGT is mapped to 1-loop factors on  $S^4$ .  $S$ -correlators instead don't admit a smooth undeformed limit. In [48] reflection coefficients, constructed from  $id$  and  $S$  3-point functions, were given a geometric interpretation as Harish-Chandra  $c$ -functions for certain quantum symmetric spaces. These  $c$ -functions were in turn related to the Jost functions describing scattering processes in two different limits of the XYZ spin chain.

The 3-point function (16.4.11) was earlier derived in [64], building on the results of [123], by using the topological string partition function on a particular toric CY threefold, the blow up of the  $\mathbb{C}^2/[\mathbb{Z}_2 \times \mathbb{Z}_2]$  orbifold. In [123] it was proposed that a five-dimensional version of the  $T_N$  theory could be obtained in a IIB setup in terms of a junction of  $N$  D5-branes,  $N$  NS5-branes and  $N$  (1,1) 5-branes which realises the blow up of the  $\mathbb{C}^2/[\mathbb{Z}_N \times \mathbb{Z}_N]$  orbifold. The 4d  $T_N$  theory is the non-Lagrangian theory of  $N$  M5 branes on the sphere with 3 full punctures and it is mapped via AGT to the Toda 3-point function. For this reason one expects that the topological string partition function on the  $T_N$  geometry maps to the  $q$ -deformed Toda 3-point function with 3 full primaries. The determination of the Toda 3-point function

with 3 full primaries is a long standing open problem and the possibility of extracting the answer from the  $T_N$  geometry has been explored in [124], [125].

The work done on the correspondence between deformed  $\mathcal{V}ir_{q,t}$  correlators and partition functions has focused on establishing a direct map between the terms contributing to the partition functions and the terms contributing to the  $\mathcal{V}ir_{q,t}$  correlators. At a deeper level one would like to be able to identify how symmetries are mapped across the correspondence. In the AGT case the generalised S-duality of 4d  $\mathcal{N} = 2$  gauge theories was beautifully identified with the Moore-Seiberg duality groupoid acting on 2d CFT correlators. This observation for example made it possible to borrow from the CFT the sophisticated machinery of Verlinde-loop operators and apply it to the exact computation of vevs of line operators on the gauge theory side [67], [126]. More recently in [68] the map of symmetries has been understood also in the case where surface operators engineered by M2 branes are included. Remarkably in this case all the gauge theory dualities of the combined 4d-2d system describing the surface operator, can be identified with symmetries of the Toda correlators involving extra degenerate primaries. It would be very interesting to establish an analogous complete map between 3d/5d gauge theory dualities and symmetries of  $q$ -correlators. An encouraging step in this direction was taken in [48] where it was pointed out that the crossing symmetry of the degenerate 4-point  $\mathcal{V}ir_{q,t}$  correlator, which was used to derive the 3-point functions, can be identified with the flop symmetry of the 3d SQED, which acts by swapping the sign of the Fayet-Iliopoulos and exchanging charge plus with charge minus chiral multiplets. Understanding the map of symmetries should open up the possibility to retrace in  $q$ -deformed case, the various applications of the gauge/CFT correspondence to the study of defects operators in gauge theories.

## Acknowledgments

I would like to thank Fabrizio Nieri, Filippo Passerini and Alessandro Torrielli for enjoyable collaborations on these topics. S.P. is partially supported by the ERC-STG grant 637844-HBQFTNCER.

## 16.5 Appendix

In this appendix we collect the definition and some properties of the special functions used in the main text.

## Bernoulli polynomials

The Bernoulli polynomials  $B_{rr}(z|\vec{\omega})$  are defined by [127]

$$\begin{aligned} B_{11}(z|\vec{\omega}) &= \frac{z}{\omega_1} - \frac{1}{2} \\ B_{22}(z|\vec{\omega}) &= \frac{z^2}{\omega_1\omega_2} - \frac{\omega_1 + \omega_2}{\omega_1\omega_2}z + \frac{\omega_1^2 + \omega_2^2 + 3\omega_1\omega_2}{\omega_1\omega_2} \\ B_{33}(z|\vec{\omega}) &= \frac{z^3}{\omega_1\omega_2\omega_3} - \frac{3(\omega_1 + \omega_2 + \omega_3)}{2\omega_1\omega_2\omega_3}z^2 + \frac{\omega_1^2 + \omega_2^2 + \omega_3^2 + 3(\omega_1\omega_2 + \omega_2\omega_3 + \omega_3\omega_1)}{2\omega_1\omega_2\omega_3}z \\ &\quad - \frac{(\omega_1 + \omega_2 + \omega_3)(\omega_1\omega_2 + \omega_2\omega_3 + \omega_3\omega_1)}{4\omega_1\omega_2\omega_3}, \end{aligned} \tag{16.5.1}$$

where  $\vec{\omega} := (\omega_1, \dots, \omega_r)$ . We will use the shorthand  $B_{rr}(z) := B_{rr}(z|\vec{\omega})$ .

## Multiple Gamma and Sine functions

The Barnes  $r$ -Gamma function  $\Gamma_r(z|\vec{\omega})$  can be defined as the  $\zeta$ -regularized infinite product [127]

$$\Gamma_r(z|\vec{\omega}) \sim \prod_{\vec{n} \in \mathbb{Z}_0^+} \frac{1}{(z + \vec{\omega} \cdot \vec{n})}. \tag{16.5.2}$$

When there is no possibility of confusion, we will simply set  $\Gamma_r(z) := \Gamma_r(z|\vec{\omega})$ .

The  $r$ -Sine function is defined according to [127]

$$S_r(z|\vec{\omega}) = \frac{\Gamma_r(E_r - z)^{(-1)^r}}{\Gamma_r(z)} \tag{16.5.3}$$

where we defined  $E_r := \sum_i \omega_i$ . We will also denote  $S_r(z) := S_r(z|\vec{\omega})$  when there is no confusion. Also, introducing the multiple  $q$ -shifted factorial

$$(z; q_1, \dots, q_r) := \prod_{k_1, \dots, k_r \geq 0} (1 - zq_1^{k_1} \cdots q_r^{k_r}) \tag{16.5.4}$$

the  $r$ -sine function has the following product representation ( $r \geq 2$ ) [127]

$$S_r(z) = e^{(-1)^r \frac{i\pi}{r!} B_{rr}(z)} \prod_{k=1}^r \left( e^{\frac{2\pi i}{\omega_k} z}; e^{2\pi i \frac{\omega_1}{\omega_k}}, \dots, e^{2\pi i \frac{\omega_{k-1}}{\omega_k}}, e^{2\pi i \frac{\omega_{k+1}}{\omega_k}}, \dots, e^{2\pi i \frac{\omega_r}{\omega_k}} \right) \tag{16.5.5}$$

whenever  $\text{Im}(\omega_j/\omega_k) \neq 0$  (for  $j \neq k$ ). General useful identities are

$$S_r(z)S_r(E_r - z)^{(-1)^r} = 1 \tag{16.5.6}$$

$$S_r(\lambda z|\lambda\vec{\omega}) = S_r(z|\vec{\omega}); \quad \lambda \in \mathbb{C}/\{0\} \tag{16.5.7}$$

$$\frac{S_r(z + \omega_i)}{S_r(z)} = \frac{1}{S_{r-1}(z|\omega_1, \dots, \omega_{i-1}, \omega_{i+1}, \dots, \omega_r)}. \quad (16.5.8)$$

For  $r = 2$  the multi-sine function is related to the double sine function

$$s_b(z) = S_2(Q/2 - iz|b, b^{-1}) \sim \prod_k \frac{n_1\omega_1 + n_2\omega_2 + Q/2 - iz}{n_1\omega_1 + n_2\omega_2 + Q/2 + iz} \quad (16.5.9)$$

where we take  $Q = \omega_1 + \omega_2$  and  $b = \omega_1 = \omega_2^{-1}$ .

## $\Upsilon^R$ function

The  $\Upsilon^R$  function is defined as the regularized infinite product

$$\Upsilon^R(z) \sim \prod_{n_1, n_2 \geq 0} \sinh \left[ \frac{R}{2} (z + n_1 b_0 + n_2 b_0^{-1}) \right] \sinh \left[ \frac{R}{2} (Q_0 - z + n_1 b_0 + n_2 b_0^{-1}) \right].$$

Important defining properties are

$$\Upsilon^R(z) = \Upsilon^R(Q_0 - z) \quad (16.5.10)$$

$$\frac{\Upsilon^R(z + b_0^{\pm 1})}{\Upsilon^R(z)} \sim \frac{(e^{R(b_0^{\mp 1} - z)}; e^{Rb_0^{\mp 1}})}{(e^{Rz}; e^{Rb_0^{\mp 1}})}. \quad (16.5.11)$$

In the  $R \rightarrow 0$  limit it reduces to the  $\Upsilon(z)$  function appearing in Liouville field theory

$$\Upsilon(z) = \Gamma_2(z|b_0, b_0^{-1})^{-1} \Gamma_2(Q_0 - z|b_0, b_0^{-1})^{-1} \quad (16.5.12)$$

where  $Q_0 := b_0 + b_0^{-1}$ .

## Jacobi Theta and elliptic Gamma functions

The Jacobi  $\Theta$  function is defined by [128]

$$\Theta(z; \tau) = (e^{2\pi iz}; e^{2\pi i\tau}) (e^{2\pi i\tau} e^{-2\pi iz}; e^{2\pi i\tau}) \quad (16.5.13)$$

and satisfies the functional relation

$$\frac{\Theta(\tau + z; \tau)}{\Theta(z; \tau)} = -e^{-2\pi iz}. \quad (16.5.14)$$

Another relevant property is [127]

$$\Theta\left(\frac{z}{\omega_1}; \frac{\omega_2}{\omega_1}\right) \Theta\left(\frac{z}{\omega_2}; \frac{\omega_1}{\omega_2}\right) = e^{-i\pi B_{22}(z)}. \quad (16.5.15)$$

The elliptic Gamma function  $\Gamma_{q,t}$  is defined by [128]

$$\Gamma_{q,t}(z) = \frac{(qt e^{-2\pi iz}, q, t)}{(e^{2\pi iz}, q, t)}; \quad q = e^{2\pi i\tau}; \quad t = e^{2\pi i\sigma} \quad (16.5.16)$$

and satisfies the functional relations

$$\frac{\Gamma_{q,t}(\tau + z)}{\Gamma_{q,t}(z)} = \Theta(z; \sigma); \quad \frac{\Gamma_{q,t}(\sigma + z)}{\Gamma_{q,t}(z)} = \Theta(z; \tau). \quad (16.5.17)$$

Other relevant properties are [49]

$$\Gamma_{q,t} \left( \frac{z}{e_3} \right)_1 \Gamma_{q,t} \left( \frac{z}{e_3} \right)_2 \Gamma_{q,t} \left( \frac{z}{e_3} \right)_3 = e^{-\frac{i\pi}{3} B_{33}(z)} \quad (16.5.18)$$

where  $q, t$  are expressed via the  $e_1, e_2, e_3$  parameters as described in (16.2.27), (16.2.28) and

$$\Gamma_{q,t} \left( \frac{z}{e_3} \right) \Gamma_{q,t} \left( \frac{e_1 + e_2 - z}{e_3} \right) = 1. \quad (16.5.19)$$

## References

- [1] V. Pestun and M. Zabzine, eds., *Localization techniques in quantum field theory*, vol. xx. Journal of Physics A, 2016. 1608.02952. <https://arxiv.org/src/1608.02952/anc/LocQFT.pdf>, <http://pestun.ihes.fr/pages/LocalizationReview/LocQFT.pdf>.
- [2] V. Pestun, “Localization of gauge theory on a four-sphere and supersymmetric Wilson loops,” *Commun. Math. Phys.* **313** (2012) 71–129, [arXiv:0712.2824](https://arxiv.org/abs/0712.2824) [hep-th].
- [3] M. Mariño, “Localization at large  $N$  in Chern-Simons-matter theories,” *Journal of Physics A* **xx** (2016) 000, 1608.02959.
- [4] K. Zarembo, “Localization and AdS/CFT Correspondence,” *Journal of Physics A* **xx** (2016) 000, 1608.02963.
- [5] J. Minahan, “Matrix models for 5D super Yang-Mills,” *Journal of Physics A* **xx** (2016) 000, 1608.02967.
- [6] B. Willett, “Localization on three-dimensional manifolds,” *Journal of Physics A* **xx** (2016) 000, 1608.02958.
- [7] L. F. Alday, D. Gaiotto, and Y. Tachikawa, “Liouville Correlation Functions from Four-dimensional Gauge Theories,” *Lett.Math.Phys.* **91** (2010) 167–197, [arXiv:0906.3219](https://arxiv.org/abs/0906.3219) [hep-th].
- [8] Y. Tachikawa, “A brief review of the 2d/4d correspondences,” *Journal of Physics A* **xx** (2016) 000, 1608.02964.
- [9] T. Dimofte, “Perturbative and nonperturbative aspects of complex Chern-Simons Theory,” *Journal of Physics A* **xx** (2016) 000, 1608.02961.
- [10] G. Festuccia and N. Seiberg, “Rigid Supersymmetric Theories in Curved Superspace,” *JHEP* **06** (2011) 114, [arXiv:1105.0689](https://arxiv.org/abs/1105.0689) [hep-th].
- [11] T. Dumitrescu, “An Introduction to Supersymmetric Field Theories in Curved Space,” *Journal of Physics A* **xx** (2016) 000, 1608.02957.

- [12] C. Beem, T. Dimofte, and S. Pasquetti, “Holomorphic Blocks in Three Dimensions,” [arXiv:1211.1986 \[hep-th\]](#).
- [13] T. Dimofte, D. Gaiotto, and S. Gukov, “3-Manifolds and 3d Indices,” *Adv. Theor. Math. Phys.* **17** (2013) no. 5, 975–1076, [arXiv:1112.5179 \[hep-th\]](#).
- [14] T. Dimofte, D. Gaiotto, and S. Gukov, “Gauge Theories Labelled by Three-Manifolds,” *Commun. Math. Phys.* **325** (2014) 367–419, [arXiv:1108.4389 \[hep-th\]](#).
- [15] T. Dimofte and S. Gukov, “Chern-Simons Theory and S-duality,” *JHEP* **05** (2013) 109, [arXiv:1106.4550 \[hep-th\]](#).
- [16] F. Nieri and S. Pasquetti, “Factorisation and holomorphic blocks in 4d,” [arXiv:1507.00261 \[hep-th\]](#).
- [17] T. Dimofte, “Complex Chern-Simons theory at level  $k$  via the 3d-3d correspondence,” [arXiv:1409.0857 \[hep-th\]](#).
- [18] F. Benini and A. Zaffaroni, “A topologically twisted index for three-dimensional supersymmetric theories,” [arXiv:1504.03698 \[hep-th\]](#).
- [19] V. P. Spiridonov and G. S. Vartanov, “Elliptic hypergeometric integrals and ’t Hooft anomaly matching conditions,” *JHEP* **06** (2012) 016, [arXiv:1203.5677 \[hep-th\]](#).
- [20] T. Dimofte, S. Gukov, and L. Hollands, “Vortex Counting and Lagrangian 3-manifolds,” *Lett. Math. Phys.* **98** (2011) 225–287, [arXiv:1006.0977 \[hep-th\]](#).
- [21] S. Pasquetti, “Factorisation of  $\mathcal{N} = 2$  Theories on the Squashed 3-Sphere,” *JHEP* **1204** (2012) 120, [arXiv:1111.6905 \[hep-th\]](#).
- [22] M. Taki, “Holomorphic Blocks for 3d Non-abelian Partition Functions,” [arXiv:1303.5915 \[hep-th\]](#).
- [23] C. Hwang, H.-C. Kim, and J. Park, “Factorization of the 3d superconformal index,” *JHEP* **1408** (2014) 018, [arXiv:1211.6023 \[hep-th\]](#).
- [24] C. Hwang and J. Park, “Factorization of the 3d superconformal index with an adjoint matter,” [arXiv:1506.03951 \[hep-th\]](#).
- [25] Y. Imamura, H. Matsuno, and D. Yokoyama, “Factorization of the  $S^3/\mathbb{Z}_n$  partition function,” *Phys. Rev.* **D89** (2014) no. 8, 085003, [arXiv:1311.2371 \[hep-th\]](#).
- [26] Y. Yoshida, “Factorization of 4d  $\mathcal{N}=1$  superconformal index,” [arXiv:1403.0891 \[hep-th\]](#).
- [27] W. Peelaers, “Higgs branch localization of  $\mathcal{N} = 1$  theories on  $S^3 \times S^1$ ,” *JHEP* **1408** (2014) 060, [arXiv:1403.2711 \[hep-th\]](#).
- [28] H.-Y. Chen and H.-Y. Chen, “Heterotic Surface Defects and Dualities from 2d/4d Indices,” *JHEP* **10** (2014) 004, [arXiv:1407.4587 \[hep-th\]](#).
- [29] H.-Y. Chen and T.-H. Tsai, “On Higgs Branch Localization of Seiberg-Witten Theories on Ellipsoid,” [arXiv:1506.04390 \[hep-th\]](#).
- [30] F. Benini and B. Le Floch, “Supersymmetric localization in two dimensions,” *Journal of Physics A* **xx** (2016) 000, [1608.02955](#).
- [31] F. Benini and S. Cremonesi, “Partition functions of  $\mathcal{N} = (2, 2)$  gauge theories on  $S^2$  and vortices,” [arXiv:1206.2356 \[hep-th\]](#).
- [32] N. Doroud, J. Gomis, B. Le Floch, and S. Lee, “Exact Results in D=2 Supersymmetric Gauge Theories,” *JHEP* **05** (2013) 093, [arXiv:1206.2606 \[hep-th\]](#).
- [33] C. Closset, S. Cremonesi, and D. S. Park, “The equivariant A-twist and gauged linear sigma models on the two-sphere,” *JHEP* **1506** (2015) 076, [arXiv:1504.06308 \[hep-th\]](#).

- [34] F. Benini and W. Peelaers, “Higgs branch localization in three dimensions,” *JHEP* **1405** (2014) 030, [arXiv:1312.6078 \[hep-th\]](#).
- [35] M. Fujitsuka, M. Honda, and Y. Yoshida, “Higgs branch localization of 3d  $\mathcal{N} = 2$  theories,” *PTEP* **2014** (2014) no. 12, 123B02, [arXiv:1312.3627 \[hep-th\]](#).
- [36] L. F. Alday, D. Martelli, P. Richmond, and J. Sparks, “Localization on Three-Manifolds,” *JHEP* **1310** (2013) 095, [arXiv:1307.6848 \[hep-th\]](#).
- [37] J. Gomis and S. Lee, “Exact Kahler Potential from Gauge Theory and Mirror Symmetry,” *JHEP* **04** (2013) 019, [arXiv:1210.6022 \[hep-th\]](#).
- [38] S. Cecotti and C. Vafa, “Topological antitopological fusion,” *Nucl. Phys.* **B367** (1991) 359–461.
- [39] S. Cecotti, D. Gaiotto, and C. Vafa, “ $tt^*$  geometry in 3 and 4 dimensions,” *JHEP* **1405** (2014) 055, [arXiv:1312.1008 \[hep-th\]](#).
- [40] D. Morrison, “Gromov-Witten invariants and localization,” *Journal of Physics A* (2016) , 1608.02956.
- [41] Y. Yoshida and K. Sugiyama, “Localization of 3d  $\mathcal{N} = 2$  Supersymmetric Theories on  $S^1 \times D^2$ ,” [arXiv:1409.6713 \[hep-th\]](#).
- [42] F. Nieri, “An elliptic Virasoro symmetry in 6d,” [arXiv:1511.00574 \[hep-th\]](#).
- [43] J. Qiu and M. Zabzine, “Review of localization for 5D supersymmetric gauge theories,” *Journal of Physics A* **xx** (2016) 000, 1608.02966.
- [44] G. Lockhart and C. Vafa, “Superconformal Partition Functions and Non-perturbative Topological Strings,” [arXiv:1210.5909 \[hep-th\]](#).
- [45] H.-C. Kim, J. Kim, and S. Kim, “Instantons on the 5-sphere and M5-branes,” [arXiv:1211.0144 \[hep-th\]](#).
- [46] N. A. Nekrasov, “Seiberg-Witten prepotential from instanton counting,” *Adv.Theor.Math.Phys.* **7** (2004) 831–864, [arXiv:hep-th/0206161 \[hep-th\]](#).
- [47] N. Nekrasov and A. Okounkov, “Seiberg-Witten theory and random partitions,” [arXiv:hep-th/0306238 \[hep-th\]](#).
- [48] F. Nieri, S. Pasquetti, F. Passerini, and A. Torrielli, “5D partition functions, q-Virasoro systems and integrable spin-chains,” *JHEP* **12** (2014) 040, [arXiv:1312.1294 \[hep-th\]](#).
- [49] G. Felder and A. Varchenko, “The elliptic gamma function and  $SL(3, \mathbb{Z}) \ltimes \mathbb{Z}^3$ ,” *Adv. Math.* **156** (2000) 44–76.
- [50] J. Qiu, L. Tizzano, J. Winding, and M. Zabzine, “Gluing Nekrasov partition functions,” *Commun. Math. Phys.* **337** (2015) no. 2, 785–816, [arXiv:1403.2945 \[hep-th\]](#).
- [51] L. Tizzano and J. Winding, “Multiple sine, multiple elliptic gamma functions and rational cones,” [arXiv:1502.05996 \[math.CA\]](#).
- [52] H.-C. Kim, S.-S. Kim, and K. Lee, “5-dim Superconformal Index with Enhanced  $E_n$  Global Symmetry,” *JHEP* **1210** (2012) 142, [arXiv:1206.6781 \[hep-th\]](#).
- [53] S. Terashima, “On Supersymmetric Gauge Theories on  $S^4 \times S^1$ ,” [arXiv:1207.2163 \[hep-th\]](#).
- [54] A. Iqbal and C. Vafa, “BPS Degeneracies and Superconformal Index in Diverse Dimensions,” [arXiv:1210.3605 \[hep-th\]](#).
- [55] S. Gukov, “Surface Operators,” *Math. Phys. Stud.* **9783319187693** (2016) 223–259, [arXiv:1412.7127 \[hep-th\]](#).
- [56] K. Hosomichi, “ $\mathcal{N} = 2$  SUSY gauge theories on  $S^4$ ,” *Journal of Physics A* **xx** (2016) 000, 1608.02962.

- [57] D. Gaiotto, L. Rastelli, and S. S. Razamat, “Bootstrapping the superconformal index with surface defects,” *JHEP* **01** (2013) 022, [arXiv:1207.3577 \[hep-th\]](#).
- [58] A. Hanany and D. Tong, “Vortices, instantons and branes,” *JHEP* **07** (2003) 037, [arXiv:hep-th/0306150 \[hep-th\]](#).
- [59] A. Hanany and K. Hori, “Branes and N=2 theories in two-dimensions,” *Nucl. Phys.* **B513** (1998) 119–174, [arXiv:hep-th/9707192 \[hep-th\]](#).
- [60] A. Gadde and S. Gukov, “2d Index and Surface operators,” *JHEP* **03** (2014) 080, [arXiv:1305.0266 \[hep-th\]](#).
- [61] A. Mironov and A. Morozov, “The Power of Nekrasov Functions,” *Phys. Lett.* **B680** (2009) 188–194, [arXiv:0908.2190 \[hep-th\]](#).
- [62] M. Aganagic, A. Klemm, M. Marino, and C. Vafa, “The Topological vertex,” *Commun. Math. Phys.* **254** (2005) 425–478, [arXiv:hep-th/0305132 \[hep-th\]](#).
- [63] A. Iqbal, C. Kozcaz, and C. Vafa, “The Refined topological vertex,” *JHEP* **10** (2009) 069, [arXiv:hep-th/0701156 \[hep-th\]](#).
- [64] C. Kozcaz, S. Pasquetti, and N. Wyllard, “A and B model approaches to surface operators and Toda theories,” *JHEP* **1008** (2010) 042, [arXiv:1004.2025 \[hep-th\]](#).
- [65] G. Bonelli, A. Tanzini, and J. Zhao, “The Liouville side of the Vortex,” *JHEP* **1109** (2011) 096, [arXiv:1107.2787 \[hep-th\]](#).
- [66] G. Bonelli, A. Tanzini, and J. Zhao, “Vertices, Vortices and Interacting Surface Operators,” *JHEP* **06** (2012) 178, [arXiv:1102.0184 \[hep-th\]](#).
- [67] L. F. Alday, D. Gaiotto, S. Gukov, Y. Tachikawa, and H. Verlinde, “Loop and surface operators in  $\mathcal{N} = 2$  gauge theory and Liouville modular geometry,” *JHEP* **1001** (2010) 113, [arXiv:0909.0945 \[hep-th\]](#).
- [68] J. Gomis and B. Le Floch, “M2-brane surface operators and gauge theory dualities in Toda,” [arXiv:1407.1852 \[hep-th\]](#).
- [69] L. F. Alday and Y. Tachikawa, “Affine  $SL(2)$  conformal blocks from 4d gauge theories,” *Lett. Math. Phys.* **94** (2010) 87–114, [arXiv:1005.4469 \[hep-th\]](#).
- [70] C. Kozcaz, S. Pasquetti, F. Passerini, and N. Wyllard, “Affine  $sl(N)$  conformal blocks from N=2  $SU(N)$  gauge theories,” *JHEP* **01** (2011) 045, [arXiv:1008.1412 \[hep-th\]](#).
- [71] E. Frenkel, S. Gukov, and J. Teschner, “Surface Operators and Separation of Variables,” [arXiv:1506.07508 \[hep-th\]](#).
- [72] N. Wyllard, “W-algebras and surface operators in N=2 gauge theories,” *J. Phys.* **A44** (2011) 155401, [arXiv:1011.0289 \[hep-th\]](#).
- [73] N. Wyllard, “Instanton partition functions in N=2  $SU(N)$  gauge theories with a general surface operator, and their W-algebra duals,” *JHEP* **02** (2011) 114, [arXiv:1012.1355 \[hep-th\]](#).
- [74] Y. Tachikawa, “A review on instanton counting and W-algebras,” *Math. Phys. Stud.* **9783319187693** (2016) 79–120, [arXiv:1412.7121 \[hep-th\]](#).
- [75] D. Gaiotto and H.-C. Kim, “Surface defects and instanton partition functions,” [arXiv:1412.2781 \[hep-th\]](#).
- [76] J. Shiraishi, H. Kubo, H. Awata, and S. Odake, “A Quantum deformation of the Virasoro algebra and the Macdonald symmetric functions,” *Lett. Math. Phys.* **38** (1996) 33–51, [arXiv:q-alg/9507034 \[q-alg\]](#).

- [77] H. Awata, H. Kubo, S. Odake, and J. Shiraishi, “Quantum  $W(N)$  algebras and Macdonald polynomials,” *Commun.Math.Phys.* **179** (1996) 401–416, [arXiv:q-alg/9508011 \[q-alg\]](#).
- [78] S. L. Lukyanov and Y. Pugai, “Bosonization of ZF algebras: Direction toward deformed Virasoro algebra,” *J.Exp.Theor.Phys.* **82** (1996) 1021–1045, [arXiv:hep-th/9412128 \[hep-th\]](#).
- [79] S. L. Lukyanov and Y. Pugai, “Multipoint local height probabilities in the integrable RSOS model,” *Nucl.Phys.* **B473** (1996) 631–658, [arXiv:hep-th/9602074 \[hep-th\]](#).
- [80] S. L. Lukyanov, “A Note on the deformed Virasoro algebra,” *Phys.Lett.* **B367** (1996) 121–125, [arXiv:hep-th/9509037 \[hep-th\]](#).
- [81] E. Frenkel and N. Reshetikhin, “Quantum Affine Algebras and Deformations of the Virasoro and  $W$ -algebras,” *Commun.Math.Phys.* **178** (1996) 237–264, [arXiv:q-alg/9505025 \[q-alg\]](#).
- [82] B. Feigin and E. Frenkel, “Quantum  $W$  algebras and elliptic algebras,” *Commun.Math.Phys.* **178** (1996) 653–678, [arXiv:q-alg/9508009 \[q-alg\]](#).
- [83] S. Odake, “Beyond CFT: Deformed Virasoro and elliptic algebras,” in *Theoretical physics at the end of the twentieth century. Proceedings, Summer School, Banff, Canada, June 27-July 10, 1999*, pp. 307–449. 1999. [arXiv:hep-th/9910226 \[hep-th\]](#).  
<http://alice.cern.ch/format/showfull?sysnb=0332345>.
- [84] H. Awata, H. Kubo, S. Odake, and J. Shiraishi, “Virasoro type symmetries in solvable models,” [arXiv:hep-th/9612233 \[hep-th\]](#).
- [85] A. Belavin, A. M. Polyakov, and A. Zamolodchikov, “Infinite Conformal Symmetry in Two-Dimensional Quantum Field Theory,” *Nucl.Phys.* **B241** (1984) 333–380.
- [86] V. Dotsenko and V. Fateev, “Conformal Algebra and Multipoint Correlation Functions in Two-Dimensional Statistical Models,” *Nucl.Phys.* **B240** (1984) 312.
- [87] G. Felder, “BRST approach to minimal model,” *J.Exp.Theor.Phys.* **317** (1989) 215–236.
- [88] M. Aganagic, N. Haouzi, C. Kozcaz, and S. Shakirov, “Gauge/Liouville Triality,” [arXiv:1309.1687 \[hep-th\]](#).
- [89] R. Dijkgraaf and C. Vafa, “Toda Theories, Matrix Models, Topological Strings, and  $N=2$  Gauge Systems,” [arXiv:0909.2453 \[hep-th\]](#).
- [90] H. Itoyama, K. Maruyoshi, and T. Oota, “The Quiver Matrix Model and 2d-4d Conformal Connection,” *Prog.Theor.Phys.* **123** (2010) 957–987, [arXiv:0911.4244 \[hep-th\]](#).
- [91] T. Eguchi and K. Maruyoshi, “Seiberg-Witten theory, matrix model and AGT relation,” *JHEP* **1007** (2010) 081, [arXiv:1006.0828 \[hep-th\]](#).
- [92] R. Schiappa and N. Wyllard, “An  $A(r)$  threesome: Matrix models, 2d CFTs and 4d  $\mathcal{N} = 2$  gauge theories,” *J.Math.Phys.* **51** (2010) 082304, [arXiv:0911.5337 \[hep-th\]](#).
- [93] A. Mironov, A. Morozov, and S. Shakirov, “Matrix Model Conjecture for Exact BS Periods and Nekrasov Functions,” *JHEP* **1002** (2010) 030, [arXiv:0911.5721 \[hep-th\]](#).
- [94] A. Mironov, A. Morozov, and S. Shakirov, “Conformal blocks as Dotsenko-Fateev Integral Discriminants,” *Int.J.Mod.Phys.* **A25** (2010) 3173–3207, [arXiv:1001.0563 \[hep-th\]](#).
- [95] M. Aganagic, N. Haouzi, and S. Shakirov, “ $A_n$ -Triality,” [arXiv:1403.3657 \[hep-th\]](#).
- [96] A. Mironov, A. Morozov, S. Shakirov, and A. Smirnov, “Proving AGT conjecture as HS duality: extension to five dimensions,” *Nucl.Phys.* **B855** (2012) 128–151, [arXiv:1105.0948 \[hep-th\]](#).
- [97] H. Awata and Y. Yamada, “Five-dimensional AGT Conjecture and the Deformed Virasoro Algebra,” *JHEP* **1001** (2010) 125, [arXiv:0910.4431 \[hep-th\]](#).

- [98] S. Yanagida, “Five-dimensional SU(2) AGT conjecture and recursive formula of deformed Gaiotto state,” *J.Math.Phys.* **51** (2010) 123506, [arXiv:1005.0216 \[math.QA\]](#).
- [99] D. Gaiotto, “Asymptotically free  $\mathcal{N} = 2$  theories and irregular conformal blocks,” *J.Phys.Conf.Ser.* **462** (2013) no. 1, 012014, [arXiv:0908.0307 \[hep-th\]](#).
- [100] M. Taki, “On AGT-W Conjecture and q-Deformed W-Algebra,” [arXiv:1403.7016 \[hep-th\]](#).
- [101] S. Katz, P. Mayr, and C. Vafa, “Mirror symmetry and exact solution of 4-D N=2 gauge theories: 1.,” *Adv.Theor.Math.Phys.* **1** (1998) 53–114, [arXiv:hep-th/9706110 \[hep-th\]](#).
- [102] O. Aharony, A. Hanany, and B. Kol, “Webs of (p,q) five-branes, five-dimensional field theories and grid diagrams,” *JHEP* **9801** (1998) 002, [arXiv:hep-th/9710116 \[hep-th\]](#).
- [103] L. Bao, V. Mitev, E. Pomoni, M. Taki, and F. Yagi, “Non-Lagrangian Theories from Brane Junctions,” [arXiv:1310.3841 \[hep-th\]](#).
- [104] M. Aganagic and S. Shakirov, “Gauge/Vortex duality and AGT,” *Math. Phys. Stud.* **9783319187693** (2016) 419–448, [arXiv:1412.7132 \[hep-th\]](#).
- [105] A. Hanany and D. Tong, “Vortex strings and four-dimensional gauge dynamics,” *JHEP* **04** (2004) 066, [arXiv:hep-th/0403158 \[hep-th\]](#).
- [106] A. Nedelin, F. Nieri, and M. Zabzine, “q-Virasoro modular double and 3d partition functions,” [arXiv:1605.07029 \[hep-th\]](#).
- [107] V. A. Alba, V. A. Fateev, A. V. Litvinov, and G. M. Tarnopolskiy, “On combinatorial expansion of the conformal blocks arising from AGT conjecture,” *Lett.Math.Phys.* **98** (2011) 33–64, [arXiv:1012.1312 \[hep-th\]](#).
- [108] A. A. Belavin, M. A. Bershtein, B. L. Feigin, A. V. Litvinov, and G. M. Tarnopolsky, “Instanton moduli spaces and bases in coset conformal field theory,” *Commun. Math. Phys.* **319** (2013) 269–301, [arXiv:1111.2803 \[hep-th\]](#).
- [109] D. Maulik and A. Okounkov, “Quantum Groups and Quantum Cohomology,” [arXiv:1211.1287 \[math.AG\]](#).
- [110] O. Schiffmann and E. Vasserot, “Cherednik algebras, W algebras and the equivariant cohomology of the moduli space of instantons on  $A^2$ ,” [arXiv:1202.2756 \[math.QA\]](#).
- [111] A. Mironov, A. Morozov, and S. Shakirov, “A direct proof of AGT conjecture at beta = 1,” *JHEP* **1102** (2011) 067, [arXiv:1012.3137 \[hep-th\]](#).
- [112] A. Morozov and A. Smirnov, “Towards the Proof of AGT Relations with the Help of the Generalized Jack Polynomials,” *Lett.Math.Phys.* **104** (2014) no. 5, 585–612, [arXiv:1307.2576 \[hep-th\]](#).
- [113] Y. Zenkevich, “Generalized Macdonald polynomials, spectral duality for conformal blocks and AGT correspondence in five dimensions,” [arXiv:1412.8592 \[hep-th\]](#).
- [114] A. Morozov and Y. Zenkevich, “Decomposing Nekrasov Decomposition,” [arXiv:1510.01896 \[hep-th\]](#).
- [115] H. Awata, H. Kanno, T. Matsumoto, A. Mironov, A. Morozov, A. Morozov, Y. Ohkubo, and Y. Zenkevich, “Explicit examples of DIM constraints for network matrix models,” [arXiv:1604.08366 \[hep-th\]](#).
- [116] J. Kaneko, “Constant term identities of Forrester-Zeilberger-Cooper,” *Discrete Mathematics* **173** (1997) 79–90.
- [117] H. Awata and Y. Yamada, “Five-dimensional AGT Relation and the Deformed beta-ensemble,” *Prog.Theor.Phys.* **124** (2010) 227–262, [arXiv:1004.5122 \[hep-th\]](#).

- [118] F. Nieri, S. Pasquetti, and F. Passerini, “3d & 5d gauge theory partition functions as q-deformed CFT correlators,” [arXiv:1303.2626 \[hep-th\]](#).
- [119] D. Bernard and A. LeClair, “ $q$  deformation of  $SU(1,1)$  conformal Ward identities and  $q$ -strings,” *Phys.Lett.* **B227** (1989) 417–423.
- [120] J. Teschner, “On the Liouville three point function,” *Phys.Lett.* **B363** (1995) 65–70, [arXiv:hep-th/9507109 \[hep-th\]](#).
- [121] H. Dorn and H. Otto, “Two and three point functions in Liouville theory,” *Nucl.Phys.* **B429** (1994) 375–388, [arXiv:hep-th/9403141 \[hep-th\]](#).
- [122] A. B. Zamolodchikov and A. B. Zamolodchikov, “Structure constants and conformal bootstrap in Liouville field theory,” *Nucl.Phys.* **B477** (1996) 577–605, [arXiv:hep-th/9506136 \[hep-th\]](#).
- [123] F. Benini, S. Benvenuti, and Y. Tachikawa, “Webs of five-branes and N=2 superconformal field theories,” *JHEP* **09** (2009) 052, [arXiv:0906.0359 \[hep-th\]](#).
- [124] V. Mitev and E. Pomoni, “Toda 3-Point Functions From Topological Strings,” *JHEP* **06** (2015) 049, [arXiv:1409.6313 \[hep-th\]](#).
- [125] M. Isachenkov, V. Mitev, and E. Pomoni, “Toda 3-Point Functions From Topological Strings II,” [arXiv:1412.3395 \[hep-th\]](#).
- [126] N. Drukker, J. Gomis, T. Okuda, and J. Teschner, “Gauge Theory Loop Operators and Liouville Theory,” *JHEP* **02** (2010) 057, [arXiv:0909.1105 \[hep-th\]](#).
- [127] A. Narukawa, “The modular properties and the integral representations of the multiple elliptic gamma functions,” [arXiv:math/0306164 \[Math.QA\]](#).
- [128] G. Gasper and M. Rahman, “Basic Hypergeometric Series,” *2nd edition, Cambridge University Press* (2004) .

# Chapter 17

## Indices for 6 dimensional superconformal field theories

Seok Kim<sup>1</sup> and Kimyeong Lee<sup>2</sup>

<sup>1</sup>*Department of Physics and Astronomy & Center for Theoretical Physics,  
Seoul National University, Seoul 151-747, Korea*

<sup>2</sup>*School of Physics, Korea Institute for Advanced Study, Seoul 130-722, Korea  
skim@phya.snu.ac.kr, klee@kias.re.kr*

### Abstract

We review some recent developments in the 6 dimensional  $(2, 0)$  superconformal field theories, focusing on their BPS spectra in the Coulomb and symmetric phases computed by various Witten indices. We shall discuss the instanton partition function of 5d maximal super-Yang-Mills theory, and the 6d superconformal index.

### Contents

|                                                                           |            |
|---------------------------------------------------------------------------|------------|
| <b>17.1 Introduction</b>                                                  | <b>660</b> |
| <b>17.2 Coulomb branch indices for the self-dual strings</b>              | <b>663</b> |
| 17.2.1 Elliptic Genus Method                                              | 663        |
| 17.2.2 Instanton Partition Method                                         | 666        |
| <b>17.3 Superconformal indices of the 6d <math>(2, 0)</math> theories</b> | <b>670</b> |
| 17.3.1 The partition function on $S^5$                                    | 671        |
| 17.3.2 The $(2, 0)$ index, $W_N$ characters and Casimir energy            | 674        |
| 17.3.3 The partition function on $\mathbb{CP}^2 \times S^1$               | 686        |
| <b>17.4 Discussions</b>                                                   | <b>691</b> |
| <b>17.5 Appendix. Off-shell supergravity analysis on <math>S^5</math></b> | <b>693</b> |
| <b>References</b>                                                         | <b>696</b> |

## 17.1 Introduction

With various string dualities found in mid 90's, interacting quantum field theories in spacetime dimensions larger than 4 were discovered from string theory [2–4]. Many aspects of these QFTs are counterintuitive from the conventional viewpoint and have enriched our notion on what quantum field theory is. The higher dimensional QFTs are also the key to understanding the strong-coupling aspects of string and M theories. Multiple M5-branes and 6d (2, 0) theories are such examples.

However, we still do not know their intrinsic definitions. For instance, they are strongly interacting CFTs, and no Lagrangian descriptions are known. Despite this situation, in the last few years there has been interesting progress in our understanding on the 5 and 6 dimensional superconformal field theories, based on various effective descriptions of these theories. In particular, we shall focus on the advances in supersymmetric observables of these higher dimensional field theories.

There have been many works on the BPS observables of 5d and 6d SCFTs, especially from 2012 when the techniques of curved space SUSY QFT were applied to higher dimensions. For instance, in 5d SCFTs, there have been extensive studies on the partition functions on  $S^4 \times S^1$  [5–8] and  $S^5$  [9–11]. There have also been many studies on 6d SCFTs. Their partition functions were studied on  $S^5 \times S^1$  [12–18],  $S^3 \times S^1 \times M_2$  [19],  $S^2 \times S^1 \times M_3$  [20, 21], and  $S^3 \times M_3$  [22], where  $M_2$  and  $M_3$  are 2 and 3 dimensional manifolds. Various 6d defect partition functions on curved manifolds were also studied, such as the dimension 2 surfaces [16, 17, 23, 24] and dimension 4 surfaces [24, 25]. The progress was made possible largely due to the technical advances in 5d super-Yang-Mills theories on curved manifolds. See [12, 26–29] and references therein for some early developments, [30] for some systematic formulations on 5d maximal SYM on curved backgrounds, [5, 15, 16, 31–33] for the factorizations of 5d partition functions on  $S^4 \times S^1$  and  $S^5$ , [34] for the saddle point structures of the supersymmetric path integral of 5d SYM on Sasaki-Einstein spaces. Often, via factorization, some curved space observables are related to those of the same QFT on flat spacetime, such as  $\mathbb{R}^4 \times S^1$  or  $\mathbb{R}^4 \times T^2$ , in the Coulomb phase. The last Coulomb phase observables have been studied from relatively long time ago, after the pioneering works by Nekrasov et al. [35, 36]. There have been continuing developments in these observables [37–45], especially in the recent few years after the realization of their relations to the conformal phase observables.

Especially in this review paper, we shall discuss the BPS spectra of these theories captured by Witten index partition functions. The main objects will be the partition functions of 6d SCFTs on the Omega deformed  $\mathbb{R}^4 \times T^2$  in the Coulomb phase, and also the superconformal index partition function on  $S^5 \times S^1$ . We shall mostly discuss the (2, 0) CFTs, since major progress has been made only for these theories so far. We shall however comment on possible generalizations to a wider class of (1, 0) CFTs at various places. It will mostly be reviews of some papers cited above, but contains some unpublished materials as well. In the rest of the introduction, we shall briefly motivate the objects that we study in this paper and also our methods and approaches.

One observable discussed in this paper is the superconformal index of the 6d SCFT [46]. This is a Witten index which counts BPS local operators of the CFT on  $\mathbb{R}^6$ . Or equivalently,

it counts BPS states of the radially quantized CFT on  $S^5 \times \mathbb{R}$ , weighted by various chemical potentials. Being a supersymmetric version of the thermal partition function, we can regard it as the partition function on  $S^5 \times S^1$  with supersymmetric boundary conditions of fields along  $S^1$ . Schematically, we shall be considering expressions for this index of the form

$$Z_{S^5 \times S^1}(\mu) = \int [d\phi] e^{-S_0(\phi)} Z_{\mathbb{R}^4 \times T^2}^{(1)}(\phi, \mu) Z_{\mathbb{R}^4 \times T^2}^{(2)}(\phi, \mu) Z_{\mathbb{R}^4 \times T^2}^{(3)}(\phi, \mu), \quad (17.1.1)$$

where  $\phi$  denotes the ‘scalar VEV in the Coulomb branch’ which is integrated over in the above expression, and  $S_0(\phi)$  is the so-called ‘classical action’ which shall be explained later. The three ingredients  $Z_{\mathbb{R}^4 \times T^2}^{(i)}(\phi, \mu)$  are the Coulomb branch Witten index of the circle compactified 6d theory on flat space, which we shall explain in detail in section 2.  $\mu$  collectively denotes the chemical potentials. In particular, it will contain the (dimensionless) ‘inverse temperature’ like variable  $\beta = \frac{2\pi r_1}{r_5}$ , where  $r_1, r_5$  are the radii of the  $S^1$  and  $S^5$  factor, respectively. Other chemical potentials, in our parametrization, will be the three rotation chemical potentials  $\omega_1, \omega_2, \omega_3$  on  $S^5$ , and those for the flavor symmetries.

The expression above is just one of the many occasions in which the SUSY QFT partition functions on compact manifolds are related to the Coulomb branch partition functions. A canonical example can be found for gauge theories on  $S^4$  [47], related to the Coulomb phase partition function on  $\mathbb{R}^4$ . The Coulomb branch partition function has been an extremely useful observable by itself, for many reasons, and has been extensively studied since [35, 36]. In the context of 6d CFTs, it provides useful information on the BPS spectrum of wrapped self-dual strings [48, 49]. Also, understanding its properties better has been (and will be) the key to the developments in the conformal phase observables, such as (17.1.1). So our section 2 will review the old and new developments on the Coulomb branch partition function on  $\mathbb{R}^4 \times T^2$ . Somewhat interestingly, the recent demand on refined understanding of this observable triggered a technically clearer derivation of this rather old observable, especially for many subtle QFTs for which this partition function could not be computed before.

Coming back to the superconformal index (17.1.1), we do not have a self-contained formulation to justify it. However, considering the regime with small circle,  $\beta \ll 1$ , we can try to understand the structure of (17.1.1) using a 5 dimensional effective description. When  $\beta \ll 1$ , the expression (17.1.1) admits a ‘weak coupling’ expansion in  $\beta$ , either perturbative one in power series of  $\beta$ , or nonperturbative one in a series of  $e^{2\pi i \tau_i} \ll 1$ , where  $\tau_i = \frac{2\pi i}{\beta \omega_i}$ . The last ‘weak coupling’ expansion acquires a more precise sense when the 6d SCFT compactified on a small circle admits a weakly coupled 5d Yang-Mills theory description. For instance, when we compactify the 6d (2, 0) CFT of ADE type on small  $S^1$  with radius  $r_1$ , then at low energy we would have a 5 dimensional maximal super-Yang-Mills description on  $S^5$ .<sup>1</sup> Such a 5d SYM limit exists for some other (1, 0) SCFTs.<sup>2</sup> The radius  $r_1$  of the circle gets mapped to

<sup>1</sup>‘Maximal SYM’ will often mean a QFT with the field content of maximal SYM, subject to deformations due to curvature and chemical potential parameters. So the number of preserved SUSY could be less than 16. For instance, mass-deformed maximal SYM, the  $\mathcal{N} = 2^*$  theory, will often be called just maximal SYM.

<sup>2</sup>We shall comment on cases in which no 5d SYM limits exist, in which case the expression (17.1.1) could still make sense.

the 5d gauge coupling  $g_{YM}$  via

$$\frac{4\pi^2}{g_{YM}^2} = \frac{1}{r_1}, \quad (17.1.2)$$

in our convention for  $g_{YM}$ . So here, the small  $\beta$  expansion is indeed the weak coupling expansion.

The partition function  $Z_{\mathbb{R}^4 \times T^2}^{(i)}$  at  $\beta \ll 1$  thus reduces to 5d SYM partition functions on  $\mathbb{R}^4 \times S^1$ , which has been studied in great detail since [35]. This decomposes into the perturbative part and instanton corrections,

$$Z_{\mathbb{R}^4 \times T^2}^{(i)} = Z_{\text{pert}}^{(i)}(\phi, \omega, m) Z_{\text{inst}}^{(i)}(\beta, \phi, \omega, m), \quad (17.1.3)$$

where  $Z_{\text{pert}}^{(i)}$  is the 1-loop contribution which is independent of  $\beta$ , and

$$Z_{\text{inst}}^{(i)} = \sum_{k=0}^{\infty} e^{-\frac{4\pi^2 k}{\beta \omega_i}} Z_k^{(i)}(\phi, \omega, m) \quad (17.1.4)$$

with  $Z_0 \equiv 1$  acquires contributions from Yang-Mills instantons localized on  $\mathbb{R}^4$  and extended along  $S^1$ . These instanton solitons in 5d SYM are interpreted as Kaluza-Klein modes of the 6d CFT compactified on circle, so captures nontrivial  $\beta$  dependence even after compactification on small circle.  $S_0(\phi)$  in (17.1.1) can also be computed from 5d SYM. So pragmatically, we shall be able to understand all the ingredients of (17.1.1) from 5d SYM. Having obtained the weakly coupled expression (17.1.1) for the 6d index, one may sum over the  $k$  series and re-expand the result at  $\beta \gg 1$  if one has a good technical control over  $Z_{\text{inst}}^{(i)}$ . The strong coupling result is useful because the spectral information can be obtained only after the expansion in the small fugacity  $e^{-\beta} \ll 1$ . We explain in section 3.2 how to explicitly do this in some special cases.

At this point, we also note that there is another version of the 6d index formula taking the form (17.1.1), which is obtained from 5d SYM on  $\mathbb{CP}^2 \times S^1$ . This expression takes a manifest form of the index, given as an expansion in  $e^{-\beta}$  at  $\beta \gg 1$ . We shall explain it for the (2,0) theory in section 3.3, emphasizing its virtue and new physics visible from this setting.

Conceptually, it will be interesting to understand whether the formulae of the type (17.1.1) are correct for all 6d SCFTs without relying on 5d SYM descriptions. Also, it would be nice to understand whether it is the unexpected feature of 5d SYM or our specific choice of SUSY observables which made 5d SYM useful here. For the Coulomb phase index explained in section 2, we can completely bypass the 5d SYM description logically (although it is still useful), and directly compute the index from string/M-theory by taking decoupling limits and starting from UV complete 1d or 2d gauge theories. We do not know whether we can bypass the 5d SYM description for the superconformal index.

The remaining part of this paper is organized as follows. In section 2, we explain the computation and physics of the Coulomb branch indices of 6d CFTs on Omega deformed  $\mathbb{R}^4 \times T^2$ , mainly from 1 dimensional gauge theories (also with detailed comments on studies from 2d gauge theories). In section 3, we explain the 6d (2,0) superconformal index and the physics contained in it. Section 4 concludes with open questions and comments. Appendix A

elaborates on the SUSY gauge theory on  $S^5$ , including background supergravity construction for the vector multiplets.

## 17.2 Coulomb branch indices for the self-dual strings

In this section, we study the spectrum of self-dual strings in the Coulomb phase of the 6d SCFTs. On one hand, this will be interesting data of the theory by itself. On the other hand, these Coulomb phase observables play important roles in understanding supersymmetric partition functions at the conformal point, such as the 6d superconformal index [46].

In the ‘Coulomb phase,’ scalars in the 6d tensor multiplets assume nonzero expectation values  $v^I$ . In such a phase, there appear tensionful self-dual strings whose tension is proportional to the Coulomb VEV. Let us first explain the SUSY preserved by these strings, when they are extended along a straight line. The 6d theory in the Coulomb phase preserves  $\mathcal{N} = (1, 0)$  or  $(2, 0)$  Poincare supersymmetry. We only use the  $(1, 0)$  part of the SUSY to define our BPS self-dual strings. For our purpose, we write the 8 supercharges as  $Q_\alpha^A, Q_{\dot{\alpha}}^A$ .  $A = 1, 2$  is the doublet index for the  $SU(2)_R$  R-symmetry.  $\alpha = 1, 2, \dot{\alpha} = 1, 2$  are the doublet indices of the  $SU(2)_l \times SU(2)_r = SO(4)$  spatial rotation on the 6d field theory direction  $\mathbb{R}^4$ , transverse to the string. These supercharges are subject to the reality condition

$$(Q_\alpha^A)^\dagger = \epsilon_{AB} \epsilon^{\alpha\beta} Q_\beta^B, \quad (Q_{\dot{\alpha}}^A)^\dagger = \epsilon_{AB} \epsilon^{\dot{\alpha}\dot{\beta}} Q_{\dot{\beta}}^B. \quad (17.2.1)$$

The supersymmetry algebra contains the following anti-commutatioaon relations:

$$\begin{aligned} \{Q_\alpha^A, Q_\beta^B\} &= \epsilon^{AB} \epsilon_{\alpha\beta} (H + P + Rv^I n_I), \quad \{Q_{\dot{\alpha}}^A, Q_{\dot{\beta}}^B\} = \epsilon^{AB} \epsilon_{\dot{\alpha}\dot{\beta}} (H - P - Rv^I n_I), \\ \{Q_\alpha^A, Q_{\dot{\beta}}^B\} &= \epsilon^{AB} (\sigma^m)_{\alpha\dot{\beta}} P_m, \end{aligned} \quad (17.2.2)$$

where  $H$  is energy,  $P$  is momentum along the string, and  $P_m$  is the momenta along  $\mathbb{R}^4$ . Here we have compactified one direction of the 6d theory on  $S^1$  with radius  $R$ , and wrapped the strings on that circle. We shall study the self-dual strings whose 5d masses saturate the BPS bound  $H \geq P + Rv^I n_I$ , so preserve 4 supercharges  $Q_{\dot{\alpha}}^A$ . The other half-BPS states preserving  $Q_\alpha^A$  would have similar spectrum.

### 17.2.1 Elliptic Genus Method

In particular, we shall be interested in the Witten index which counts the BPS degeneracies of these strings wrapping the circle. Namely, the 6d CFT is put on  $\mathbb{R}^{4,1} \times S^1$ , and there are  $r$  real scalar VEVs  $v^I$  ( $I = 1, \dots, r$ ). The index is defined by

$$Z_{\{n_I\}}(\tau, \epsilon_{1,2}, m) = \text{Tr} \left[ (-1)^F q^{\frac{H'+P}{2}} e^{-\epsilon_1(J_1+J_R) - \epsilon_2(J_2+J_R)} e^{-m \cdot F} \right], \quad (17.2.3)$$

where  $H'$  is the energy over the string rest mass  $Rv^I n_I$ ,  $q \equiv e^{2\pi i \tau}$ ,  $J_1 \equiv J_l + J_r$ ,  $J_2 \equiv J_r - J_l$ , and  $F$  collectively denotes all the other conserved global charges which commute with the

supercharges. The charges appearing inside the trace is chosen so that they commute with the two supercharges  $Q_1^1, Q_2^2$ , among  $Q_\alpha^A$ . From the algebra (17.2.2), the most general states preserving these two supercharges will be the  $\frac{1}{2}$ -BPS states preserving all  $Q_\alpha^A$ . So with this index we are counting the states in the  $\frac{1}{2}$ -BPS multiplet, with a further refinement given by  $J_r + J_R$  (which does not commute with all four  $Q_\alpha^A$ ). We also define the partition function  $Z(v^I, \tau, \epsilon_{1,2}, m)$  by summing over the winding numbers of the self-dual strings,

$$Z(v^I, \tau, \epsilon_{1,2}, m) = \sum_{n_1, \dots, n_r=0}^{\infty} e^{-v^I n_I} Z_{n_I}(\tau, \epsilon_{1,2}, m), \quad (17.2.4)$$

where  $Z_{n_I=0} \equiv 1$ . Here, we introduce the (dimensionless) chemical potentials  $v^I$  conjugate to the winding numbers  $n_I$ . These are just scaled version of the scalar VEVs  $v^I$  that we used above but should not be confused with them.

$Z(v^I, \tau, \epsilon_{1,2}, m)$  is computed in various ways. Currently, in most nontrivial theories, it is only computable in series expansions. One series expansion takes the form of (17.2.4), and the coefficients  $Z_{n_I}(\tau, \epsilon_{1,2}, m)$  are computed from the elliptic genera of suitable 2 dimensional supersymmetric quantum field theories living on the worldsheets of these strings [38, 39, 42, 45]. A different kind of series expansion can be made in  $q = e^{2\pi i \tau}$ , when  $q \ll 1$ :

$$Z(v^I, \tau, \epsilon_{1,2}, m) = \sum_{k=0}^{\infty} q^k Z_k(v^I, \epsilon_{1,2}, m). \quad (17.2.5)$$

The momentum charge  $k$  on  $S^1$  is given a weight  $q^k$ . These Kaluza-Klein momentum states are regarded as massive particles in 5d.  $Z_k(v^I, \epsilon_{1,2}, m)$  can be computed from the quantum mechanics of the ‘instanton solitons’ of 5 dimensional gauge theory, if one has a 5d weakly coupled SYM description at small radius. In this section, we shall mostly focus on the latter quantum mechanical index. The usefulness of these two approaches will be commented later.

We first explain the general ideas of computing the two types of coefficients  $Z_{n_I}(q, \epsilon_{1,2}, m)$  and  $Z_k(v^I, \epsilon_{1,2}, m)$ , before studying an example. Both computations essentially rely on the string theory completion of the 6d SCFT, and suitable decoupling limits when the contribution of some charges to the BPS mass become large.

Let us first explain the strategy of computing  $Z_{n_I}(q, \epsilon_{1,2}, m)$ . Firstly, as the 6d SCFT lacks intrinsic definition, we rely on its string theory or M-theory engineering. In all such constructions, one engineers suitable string/M-theory backgrounds, and takes suitable low energy decoupling limits in which the 6 dimensional states decouple from the bulk states (e.g. 10/11 dimensional gravity, stringy states, so on). After this limit, certain 6 dimensional decoupled sector of 6d SCFT exists. Furthermore, we are interested in the 1+1 dimensional strings in the Coulomb phase, with nonzero VEV for the 6d scalar  $v$  whose mass dimension is 2. The tension of the self-dual strings is proportional to  $v$ . At energy scale much below  $v^{\frac{1}{2}}$ , the 6d system will again exhibit a decoupling, between the 2d QFT on the strings and the rest of the 6d system.  $Z_{n_I}(q, \epsilon_{1,2}, m)$  is computed by studying the last 2d QFT living on the strings’ worldsheet. We generally expect the 2d QFT to be an interacting conformal field theory. The computation of the observables is generally very difficult with strongly

interacting QFT. Here, the crucial step is to engineer a 2d gauge theory which is weakly coupled in UV, and flows to the desired interacting CFT in the IR. The construction of the UV gauge theory will often be easy with brane construction engineering of the 6d SCFT and the associated self-dual strings. Such UV gauge theories are constructed for the self-dual strings of a few interesting 6d CFTs, such as ‘M-strings’ [39], ‘E-strings’ [42], and some others [45]. The UV gauge theories for many interesting self-dual strings are still unknown at the moment and are under active studies. With a weakly-coupled UV gauge theory which flows to the desired CFT, the elliptic genus can in principle be easily computed from the UV theory, as the elliptic genus is independent of the continuous coupling parameters of the theory. In fact the general elliptic genus formula for 2d SUSY Yang-Mills theories was recently derived in [51, 52].

$Z_k(v^I, \epsilon_{1,2}, m)$  can also be computed in a similar manner, for some classes of self-dual strings. This approach is applicable to the cases in which the circle compactification of the 6d theory yields weakly coupled 5d Yang-Mills theories at low energy. Then, the momentum  $k$  is given by the topological charge

$$k = \frac{1}{8\pi^2} \int_{\mathbb{R}^4} \text{tr}(F \wedge F) \in \mathbb{Z} \quad (17.2.6)$$

carried by the Yang-Mills instanton solitons of the 5d gauge theory. The dynamics of these solitons are often described by a quantum mechanical gauge theory.  $Z_k(v^I, \epsilon_{1,2}, m)$  is essentially computed by the quantum mechanical index for the  $k$  instantons. More precisely, one finds

$$Z_k(v^I, \epsilon_{1,2}, m) = Z_{\text{pert}}(v^I, \epsilon_{1,2}, m) Z_{k,\text{inst}}(v^I, \epsilon_{1,2}, m), \quad (17.2.7)$$

where  $Z_{\text{pert}}$  is computed from the perturbative degrees of freedom in 5d SYM, and  $Z_{k,\text{inst}}$  is given by the instanton quantum mechanics. The last instanton partition function has been first computed in [35, 36], and has been intensively studied since then for various reasons. Although we used the notion of 5d SYM to explain the strategy, we can often get the quantum mechanical gauge theory description from the full string theory set up by taking a suitable decoupling limit, bypassing the UV incomplete 5d SYM description at all. For instance, for the (2, 0) theory compactified on circle, one just obtains the quantum mechanics from the D0-D4 system by taking a low energy decoupling limit, without relying on 5d SYM description at all.

The two quantities  $Z_{n_I}(q, \epsilon_{1,2}, m)$  and  $Z_k(v^I, \epsilon_{1,2}, m)$  are supersymmetric indices of the 2d and 1d gauge theories on  $T^2$  and  $S^1$ , respectively. Although both types of indices have been extensively studied in the literature from long time ago, their general structures for gauge theories have been fully clarified only recently. See [50–52] for the developments in the 2d elliptic genus, and [41, 53, 54] for the 1d Witten index.

Before proceeding with concrete examples, we also comment that the quantity  $Z(v^I, \tau, \epsilon_{1,2}, m)$  can often be computed from topological string amplitudes on suitable Calabi-Yau 3-folds. This happens when the 6d SCFTs are engineered from F-theory on singular elliptic Calabi-Yau 3-folds [55–57]. Changing the moduli of CY<sub>3</sub> in a way that specific 2-cycles shrink to zero volume, one obtains a 6 dimensional singularity which supports decoupled degrees of freedom

at low energy, defining 6d SCFTs. One important ingredient of these theories is D3-branes wrapping these collapsing 2-cycles, which yield self-dual strings that become tensionless in the singular limit. Therefore, the volume moduli of these 2-cycles are the Coulomb branch VEVs  $v^I$  in the 6d tensor supermultiplets.

So in this setting, we consider the F-theory on  $\mathbb{R}^{4,1} \times S^1 \times \text{CY}_3$  in the Coulomb phase. We wrap D3-branes along  $S^1$  times the 2-cycles in  $\text{CY}_3$ . This system can be T-dualized on  $S^1$  to the dual circle  $\tilde{S}^1$  of the type IIA theory. The D3-branes map to D2-branes transverse to  $\tilde{S}^1$ . Consider the regime with large  $S^1$ , or equivalently small  $\tilde{S}^1$ , and make an M-theory uplift on an extra circle  $S^1_M$ . Then  $\tilde{S}^1$  and  $S^1_M$  combine to a torus and fiber the 4d base of the original  $\text{CY}_3$  we started from, meaning that we get M-theory on the same  $\text{CY}_3$ . The self-dual string winding numbers over the 2-cycles maps to the M2-brane winding numbers on the same cycles. The momentum on  $S^1$  maps to M2-brane winding number on the  $T^2$  fiber. So the counting of the self-dual string states maps to counting the wrapped M2-branes on  $\text{CY}_3$  in M-theory. The last BPS spectrum is computed by the topological string partition function on  $\text{CY}_3$  [58, 59]. In particular, consider an expansion of  $Z_{\mathbb{R}^4 \times T^2}$  in the rotation parameters  $\epsilon_1, \epsilon_2$  given by

$$Z_{\mathbb{R}^4 \times T^2}(v^I, q, \epsilon_{1,2}, m) = \exp \left[ \sum_{n \geq 0, g \geq 0} (\epsilon_1 + \epsilon_2)^n (\epsilon_1 \epsilon_2)^{g-1} F^{(n,g)}(v^I, q, m) \right]. \quad (17.2.8)$$

The coefficients of the expansion  $F^{(n,g)}(v^I, q, m) = \sum_{n_I, k, f} e^{-v^I n_I} q^k e^{-m \cdot f} F_{n_I, k, f}^{(n,g)}$  are computed by the topological string amplitudes on  $\text{CY}_3$ . The series in (17.2.8) is the genus expansion of refined topological string. So from this viewpoint, the elliptic genus we study in this section is the all genus sum of the topological string amplitudes. A few low genus expansions are known for many interesting 6d self-dual strings. This provides an alternative method of computing some data of the full elliptic genus when neither 2d nor 1d gauge theories are known. For instance, see [45] for the results 6d strings engineered by F-theory on Hirzebruch surfaces, where many such strings do not have known gauge theory descriptions yet.

## 17.2.2 Instanton Partition Method

With the above comments in mind, we shall now explain the studies of the Coulomb branch indices from 1d gauge theories. We shall specifically explain the 6d (2, 0) SCFT of  $A_{N-1}$  type, to be concrete. Although this quantity has been studied in the context of ‘instanton counting’ of 5d SYM [35], one does not have to rely on 5d SYM description at all, as everything can be directly understood from the full string theory setting. For applications of the similar techniques to the Coulomb branch CFTs with (1, 0) SUSY, see [41, 42].

The maximal superconformal field theory in 6d of  $A_{N-1}$  type is engineered by taking  $N$  M5-branes on top of another, in the flat M-theory background. In the low energy limit, the system contains a 6d SCFT on M5-branes’ worldvolume which is decoupled from the bulk. In the Coulomb branch, we take  $N$  M5-branes separated along one of the five transverse directions of  $\mathbb{R}^5$ . The self-dual strings are suspended between separated M5-branes along this direction, and also wrap  $\mathbb{R}^{1,1} \subset \mathbb{R}^{5,1}$  of the 5-brane worldvolume.

We are interested in the index of the circle compactified self-dual strings. The index is invariant under the change of continuous parameters of the theory, and also of the background parameters as long as they do not appear in the supercharges that are associated with the definition of the Witten index. So we can take the circle radius to be very small, and use the type IIA string theory description for the computation. Let us denote by  $v^I$  (with  $I = 1, \dots, N$ ) the  $N$  scalar VEVs, or positions of  $N$  M5-branes along a line in  $\mathbb{R}^5$ . These are related to the 5d VEVs by a multiplication of  $R$ . Let  $n_I$  denote the number of self-dual strings ending on a given M5-branes, with orientations taken into account. If the strings have  $k$  units of Kaluza-Klein momentum, one obtains in the small  $R$  limit a system of  $k$  D0-branes bound to fundamental strings with charges  $n_I$  stretched between the  $N$  D4-branes. In particular, the energy of the compactified self-dual strings is bounded as

$$E \geq \frac{k}{R} + v^I n_I . \quad (17.2.9)$$

In the regime with very small  $R$ , where we plan to compute the index, we can use the effective description with fixed  $k$ , as the particles with large rest mass  $\sim R^{-1}$  become non-relativistic. So the quantum mechanics of  $k$  D0-branes bound to  $N$  D4-branes would capture the exact index  $Z_{k,\text{inst}}(v^I, \epsilon_{1,2}, m)$ . The quantum numbers  $n_I$  will be realized as  $SU(N)$  Noether charges of this mechanical system. This is simply the decoupling limit of the  $k$  D0-branes bound to D4-branes, and could also be regarded as the discrete lightcone quantization (DLCQ) of M5-branes [60].

The quantum mechanics of  $k$  D0-branes on  $N$  D4-branes (in the Coulomb phase) preserves 8 SUSY, since the D0-D4 system preserves  $\frac{1}{4}$  of the type IIA SUSY. The system has  $SO(4)_1 \sim SU(2)_{1L} \times SU(2)_{1R}$  rotation symmetry on D4 worldvolume transverse to D0, and  $SO(5)$  rotation transverse to the D4's. When D4's are displaced along one of the five directions of  $\mathbb{R}^5$ , with VEV  $v = \text{diag}(v_1, \dots, v_N)$ ,  $SO(5)$  is broken to  $SO(4)_2 \sim SU(2)_{2L} \times SU(2)_{2R}$ . We denote by  $\alpha, \dot{\alpha}, a, \dot{a}$  the doublet indices of the four  $SU(2)$ 's, respectively, in the order presented above. The 8 supercharges can be written by  $Q_{\dot{\alpha}}^a, Q_{\alpha}^{\dot{a}}$  with reality conditions similar to (17.2.1). The degrees of freedom are:

$$\begin{aligned} \text{D0-D0 strings} & : U(k) \text{ adjoint } A_0 , \quad (\varphi^{1,2,3,4} \sim \varphi_{a\dot{a}}, \varphi^5) , \quad \lambda_{\dot{\alpha}}^a , \quad \lambda_{\alpha}^{\dot{a}} \\ & \quad U(k) \text{ adjoint } a_m \sim a_{\alpha\dot{\alpha}} , \quad \lambda_{\alpha}^a , \quad \lambda_{\alpha}^{\dot{a}} \\ \text{D0-D4 strings} & : U(k) \times U(N) \text{ bi-fundamental } q_{\dot{\alpha}} , \quad \psi^a , \quad \psi^{\dot{a}} \end{aligned} \quad (17.2.10)$$

with  $m = 1, \dots, 4$ . The D4-D4 strings move along  $\mathbb{R}^4$  transverse to the D0's, and decouple at low energy. (These will be perturbative 5d SYM degrees.) This system can be formally obtained by a dimensional reduction of a 2 dimensional  $\mathcal{N} = (4, 4)$  SUSY gauge theory, in which  $Q_{\dot{\alpha}}^a$  and  $Q_{\alpha}^{\dot{a}}$  respectively define 4 left-moving and right-moving supercharges. The first line of the above field content is called the vector multiplet. The second and third line separately form a hypermultiplet. The action of this system is very standard, and could be found e.g. in [37], whose notations we followed here.

The index  $Z_{k,\text{inst}}(v^I, \epsilon_{1,2}, m)$  is defined in this quantum mechanics by

$$Z_{k,\text{inst}}(v^I, \epsilon_{1,2}, m) = \text{Tr} \left[ (-1)^F e^{-\beta\{Q, Q^\dagger\}} e^{-v \cdot n} e^{-2\epsilon_+ (J_{1R} + J_{2R})} e^{-2\epsilon_- J_{1L}} e^{-m J_{2L}} \right] , \quad (17.2.11)$$

where  $n = (n_1, \dots, n_N)$  denotes the  $U(1)^N \subset U(N)$  charge,  $\epsilon_{\pm} \equiv \frac{\epsilon_1 \pm \epsilon_2}{2}$ , and  $J_{1L}, J_{1R}, J_{2L}, J_{2R}$  are the Cartans of  $SU(2)_{1L}, SU(2)_{1R}, SU(2)_{2L}, SU(2)_{2R}$ , respectively.  $\beta$  is the usual regulator parameter which does not appear in the index. The trace is over the Hilbert space of the quantum mechanics. Note that the measure in the trace commutes with two supercharges  $Q = Q_1^{\dagger}, Q^{\dagger} = -Q_2^{\dagger}$  among  $Q_{\alpha}^{\dagger}$ , as we explained at the beginning of this section. This index was computed by Nekrasov [35] in 2002. We shall briefly review it with adding more recent clarifications on the computational step, for which Nekrasov wrote down a prescription for computation. These clarification of the prescriptions is somewhat crucial to compute the  $Z_{k,\text{inst}}$  indices for more general 6d (1, 0) SCFTs [41, 42].

The 1d gauge theory for D0-D4 system that we explained above is strongly coupled at low energy, since the quantum mechanical gauge coupling has dimension  $[g_{QM}^2] = M^3$ . We can however compute the index in the  $g_{QM} \rightarrow 0$  limit, as the Witten index is generically expected to be insensitive to the changes of continuous parameters of the theory. This is what Nekrasov has done in [35], and also in more recent studies of [41, 53, 54]. The computation of the index is done by going to the path integral representation of the index with Euclidean quantum mechanics, put on a circle with circumference  $\beta$ , and computing it in the  $g_{QM} \rightarrow 0$  limit. The computation consists of (1) identifying the zero modes of the quantum mechanical path integral on  $S^1$ , in the limit  $g_{QM} \rightarrow 0$  (carefully defined in [41, 51, 52, 54]); (2) Gaussian path integral over the non-zero modes; (3) finally making an exact integration over the zero modes.

We briefly explain the results of these three steps, within our example for simplicity. Firstly, the zero modes in the  $g_{QM} \rightarrow 0$  limit consist of the constant modes of  $\varphi^5$  and  $A_{\tau}$  which commute with each other. Here,  $A_{\tau}$  is the Wick-rotated variable  $A_{\tau} = -iA_0$  in the Euclidean quantum mechanics on  $S^1$ . More precisely,  $U \equiv e^{i\beta A_{\tau}}$  defines a holonomy of the gauge group  $U(k)$  along the circle. For the  $U(k)$  gauge group, one can take  $\phi \equiv \varphi^5 + iA_{\tau}$  to be

$$\phi = \text{diag}(\phi_1, \dots, \phi_k) \quad (17.2.12)$$

using  $U(k)$  rotation, locally labeled by  $k$  complex parameters. Each parameter satisfies  $\phi_i \sim \phi_i + 2\pi i$ , so lives on a cylinder. These variables are subject to further identification given by permuting the  $k$  variables. This is the permutation subgroup of  $U(k)$  which acts within (17.2.12). For gauge groups other than  $G = U(k)$ , especially for disconnected groups, the zero mode structure could be more complicated. See [41] for examples. There are also some fermionic zero modes in the strict  $g_{QM} = 0$  limit, which we shall not explain here, but plays important roles in the final step (3) above.

Secondly, in the above background, the 1-loop determinants over non-zero modes yield the following factor:

$$\begin{aligned} Z_{1\text{-loop}}(\phi, \epsilon_{1,2}, m) &= \frac{\prod_{I \neq J} 2 \sinh \frac{\phi_{IJ}}{2} \cdot \prod_{I,J=1}^k 2 \sinh \frac{\phi_{IJ} + 2\epsilon_+}{2}}{\prod_{I,J=1}^k 2 \sinh \frac{\phi_{IJ} + \epsilon_1}{2} \cdot 2 \sinh \frac{\phi_{IJ} + \epsilon_2}{2}} \cdot \prod_{I,J=1}^k \frac{2 \sinh \frac{\phi_{IJ} \pm m - \epsilon_-}{2}}{2 \sinh \frac{\phi_{IJ} \pm m - \epsilon_+}{2}} \\ &\cdot \prod_{I=1}^k \prod_{i=1}^N \frac{2 \sinh \frac{m \pm (\phi_I - v_i)}{2}}{2 \sinh \frac{\epsilon_{\pm} (\phi_I - v_i)}{2}}, \end{aligned} \quad (17.2.13)$$

where  $\phi_{IJ} \equiv \phi_I - \phi_J$ , and the sinh expressions with  $\pm$  in the arguments mean multiplying the sinh factors with all possible signs. The factor on the second line comes from the integral over the fundamental hypermultiplet  $q_{\hat{\alpha}}, \psi^a, \psi^{\hat{a}}$ , and the second factor on the right hand side of the first line comes from the adjoint hypermultiplet  $a_m, \lambda_{\hat{\alpha}}^a, \lambda_{\hat{\alpha}}^{\hat{a}}$ . Finally, the first factor on the first line comes from the vector multiplet nonzero modes  $A_{\tau}, \varphi^I, \lambda_{\hat{\alpha}}^a, \lambda_{\hat{\alpha}}^{\hat{a}}$ .

The final task is to integrate over the  $k$  complex, or  $2k$  real, variables  $\phi_I$ . Naively, it appears that one has to do a  $2k$  dimensional integral on copies of cylinders, with a meromorphic measure given by (17.2.13). This naive prescription will not work because the measure will diverge at various poles, implying that the integration over non-zero modes becomes subtle near the poles even in the  $g_{QM} \rightarrow 0$  limit. In [35], Nekrasov gave a  $k$  dimensional contour integral prescription, rather than a  $2k$  dimensional real integral, with the measure (17.2.13). The result is the sum over residues for a subset of poles in the integrand (17.2.13). The relevant poles are labeled by all possible  $N$ -tuple of Young diagrams  $Y = (Y_1, Y_2, \dots, Y_N)$  with  $k$  total number of boxes. These are sometimes called  $N$ -colored Young diagrams with  $k$  boxes. The summation of residues from these poles is given by [37, 61, 62]

$$Z_{k,\text{inst}}(v, \epsilon_{1,2}, m) = \sum_{|Y|=k} \prod_{i,j=1}^N \prod_{s \in Y_i} \frac{\sinh \frac{E_{ij}+m-\epsilon_+}{2} \sinh \frac{E_{ij}-m-\epsilon_+}{2}}{\sinh \frac{E_{ij}}{2} \sinh \frac{E_{ij}-2\epsilon_+}{2}} \quad (17.2.14)$$

with

$$E_{ij} = v_i - v_j - \epsilon_1 h_i(s) + \epsilon_2 (v_j(s) + 1) . \quad (17.2.15)$$

Here,  $s$  labels the boxes in the  $i$ 'th Young diagram  $Y_i$ .  $h_i(s)$  is the distance from the box  $s$  to the edge on the right side of  $Y_i$  that one reaches by moving horizontally to the right.  $v_j(s)$  is the distance from  $s$  to the edge on the bottom side of  $Y_j$  that one reaches by moving down (and  $v_j(s)$  may be negative if one has to move up to the bottom of  $Y_j$ ). See [37, 61, 62] for more detailed explanations on notation. This result can be obtained from the following rule for the contour. First of all, the contours will be a closed curve on the  $z_I = e^{\phi_I}$  plane. The rules of the contour choices, or equivalently the residues to be kept by the contour integral, are as follows: (1) exclude all the poles in (17.2.13) coming from the sinh factors whose arguments include  $m$  (from 5d SYM, this amounts to ignoring all the poles coming from 5d adjoint hypermultiplet); (2) exclude all poles at  $z_I = 0$  or  $\infty$ ; (3) as for the remaining poles, take  $\epsilon_+ \gg 1$ , and include all poles within the unit circles  $|z_I| < 1$ .

Although well known and used, this prescription was given a satisfactory derivation only rather recently [41], using and generalizing the methods of [51, 52]. The strategy of [51, 52] is to carefully re-do the supersymmetric path integral computation when  $\phi$  is near its pole location, and also carefully considering the lift of some gaugino zero modes [51]. After some analysis, the final contour integral reduces to a set of residue sum, which is called the Jeffrey-Kirwan residue [63]. The Jeffrey-Kirwan residue rules are slightly different from the above (1), (2), (3) in general, but it was shown for the above  $U(k)$  theory that the two rules yield the same result [41].

The result (17.2.14) is useful to understand various aspects of the  $(2, 0)$  theory in Coulomb phase, and its self-dual strings compactified on a circle [37]. It is also useful to understand the conformal phase (with zero Coulomb VEV) of the theory. An early finding of this sort

was that (17.2.14) could be used to study the index of the DLCQ (2, 0) theory, which is the 6d CFT compactified on a light-like circle. Namely, one takes (17.2.14) and suitably integrates over the Coulomb VEV  $v$  with Haar measure inserted, to extract out the gauge invariant spectrum [37]. More recently, and this will be reviewed in our section 3, (17.2.14) was used as the building block of more sophisticated CFT observable, the superconformal index on  $S^5 \times S^1$ . Again several factors of the form (17.2.14) are multiplied (with other factors that we shall call the ‘classical measure,’ see section 3), and we suitably integrate over the Coulomb VEV parameter  $v$ .

Here, we find one virtue of the index (17.2.5) obtained by 1d gauge theory, over (17.2.4) which is obtained by 2d gauge theory. Namely, in many recent applications,  $q = e^{2\pi i\tau}$  is kept as a fixed fugacity, while the Coulomb VEV is introduced temporarily and should be integrated over to obtain CFT observables. The computations explained in this subsection keeps the  $v$  dependence exact, at a given order  $q^k$  in  $q$ . So in this sense, knowing the coefficients of (17.2.5) exactly could be more useful, rather than knowing those of (17.2.4).

On the other hand, the elliptic genus (17.2.4) has the virtue of making the modular property under the  $SL(2, \mathbb{Z})$  transformation clear, with the modular parameter  $\tau$ . So when one has to make a strong coupling re-expansion of the partition function, as explained in the introduction and section 3.2, this could potentially be very useful. Also, the elliptic genus (17.2.4) can often be computed when the circle reduction of 6d CFT does not flow to weakly coupled SYM, so that the 1d approach of this section becomes difficult to apply [42, 45]. However, (17.2.4) takes the form of the Coulomb VEV expansion when  $v$  acquires large expectation values (compared to other parameters such as  $\tau, m, \epsilon_{1,2}$ ). So apparently it is unclear how to integrate over them in the curved space partition functions.

### 17.3 Superconformal indices of the 6d (2, 0) theories

In this section, we explain the current status of our understanding on the superconformal index of the 6d (2, 0) theories. Possible extensions to the 6d (1, 0) theories have not yet been developed in detail, on which we shall just make general statements and brief comments.

6d (1, 0) SCFT has  $OSp(8^*|2)$  superconformal symmetry, as well as possible global symmetries whose charges we collectively call  $F$ . The bosonic part of the superconformal symmetry is  $SO(6, 2) \times SU(2)_R$ . We are interested in the radially quantized CFT, living on  $S^5 \times \mathbb{R}$ . Then the maximal commuting set of charges of the bosonic subgroup are taken to be  $R \in SU(2)_R$  in the R-symmetry,  $j_1, j_2, j_3 \in SO(6)$  which are rotations on  $S^5$ , and  $E$  for the translational symmetry along the time direction  $\mathbb{R}$ . Often, we make  $E$  dimensionless by multiplying the radius  $r$  of  $S^5$ . We normalize  $R, j_i$  to have  $\pm\frac{1}{2}$  eigenvalues for spinors. The superconformal index of a general 6 dimensional SCFT is defined by [46]

$$Z_{S^5 \times S^1}(\beta, m, a_i) \equiv \text{Tr} \left[ (-1)^F e^{-\beta(E-R)} e^{-\beta a_i j_i} e^{-\beta m \cdot F} \right] , \quad (17.3.1)$$

where  $a_1 + a_2 + a_3 = 0$ , and  $\text{Tr}$  is the trace over the Hilbert space of the CFT on  $S^5 \times \mathbb{R}$ . Note that the 6d (1, 0) SCFT has 8 Poincare supercharges  $Q_{s_1 s_2 s_3}^A$ , with  $A = \pm\frac{1}{2}$  for the

R-symmetry, and  $(s_1, s_2, s_3) = (\pm\frac{1}{2}, \pm\frac{1}{2}, \pm\frac{1}{2})$  for the  $SO(6)$  symmetry, where the last three  $\pm$  signs are constrained by  $\pm\pm\pm = -$ . These supercharges have energy ( $\sim$  scale dimension)  $E = \frac{1}{2}$ . The 8 conformal supercharges are given by  $S_{s_1 s_2 s_3}^A$ , where this time the three signs for  $s_i = \pm\frac{1}{2}$  are constrained by  $\pm\pm\pm = +$ . They have scale dimension  $E = -\frac{1}{2}$ . Among these 16 supercharges, the measure of (17.3.1) commutes with  $Q = Q_{---}^+$ ,  $S = S_{+++}^-$ . So the index counts BPS states (with minus sign for fermions) which are annihilated by at least these two supercharges. Equivalently, by the operator-state map, the index counts BPS local operators of the CFT on  $\mathbb{R}^6$ . The energies (dimensions) of the BPS states (operators) are given by  $E = 4R + j_1 + j_2 + j_3$ , from the vanishing of  $\{Q, S\}$  acting on these BPS states.

Specifying to the 6d (2, 0) SCFTs, the superalgebra is  $OSp(8^*|4)$ , and there are no extra flavor symmetries. The supercharges are now given by  $Q_{s_1 s_2 s_3}^{R_1 R_2}$ ,  $S_{s_1 s_2 s_3}^{R_1 R_2}$ , where  $R_1 = \pm\frac{1}{2}$ ,  $R_2 = \pm\frac{1}{2}$  are the two  $SO(5) \sim Sp(4)$  spinor charges.  $s_1, s_2, s_3$  are given and constrained in the same way as the previous paragraph. We can pick  $Q = Q_{---}^{++}$  and  $S = S_{+++}^-$  and define the index

$$Z_{S^5 \times S^1}(\beta, m, a_i) \equiv \text{Tr} \left[ (-1)^F e^{-\beta(E - \frac{R_1 + R_2}{2})} e^{-\beta a_i j_i} e^{\beta m \frac{R_1 - R_2}{2}} \right]. \quad (17.3.2)$$

The BPS states counted by this index satisfy  $E = 2(R_1 + R_2) + j_1 + j_2 + j_3$ . (17.3.2) can be regarded as a specialization of (17.3.1) by regarding  $R = \frac{R_1 + R_2}{2}$  as the (1, 0) R-charge, and  $\frac{R_1 - R_2}{2}$  as a flavor symmetry of the (1, 0) superconformal subalgebra.

Even without a microscopic formulation of the 6d SCFTs, we have fairly well-motivated expressions for these partition functions (17.3.1), (17.3.2). We shall write down two such expressions, one in section 3.1 and another in section 3.3. Both of them are inspired by 5 dimensional super-Yang-Mills theories, obtained by circle reductions of 6d SCFTs on  $S^5 \times S^1$  down to 5d.

### 17.3.1 The partition function on $S^5$

The first expression for the partition function  $Z_{S^5 \times S^1}$ , is given as follows. It uses the Coulomb branch partition function  $Z_{\mathbb{R}^4 \times T^2}(\tau, v, \epsilon_1, \epsilon_2, m_0)$  that we explained in section 2, and is given by

$$\begin{aligned} Z_{S^5 \times S^1}(\beta, m, a_i) &= \frac{e^{-S_{\text{bkgd}}}}{|W(G_r)|} \int_{-\infty}^{\infty} \left[ \prod_{I=1}^r d\phi_I \right] e^{-S_0(\phi, \beta, a_i)} Z_{\mathbb{R}^4 \times T^2} \left( \frac{2\pi i}{\beta \omega_1}, \frac{\phi}{\omega_1}, \frac{2\pi i \omega_{21}}{\omega_1}, \frac{2\pi i \omega_{31}}{\omega_1}, 2\pi i \left( \frac{m}{\omega_1} + \frac{3}{2} \right) \right) \\ &\cdot Z_{\mathbb{R}^4 \times T^2} \left( \frac{2\pi i}{\beta \omega_2}, \frac{\phi}{\omega_2}, \frac{2\pi i \omega_{32}}{\omega_2}, \frac{2\pi i \omega_{12}}{\omega_2}, 2\pi i \left( \frac{m}{\omega_2} + \frac{3}{2} \right) \right) Z_{\mathbb{R}^4 \times T^2} \left( \frac{2\pi i}{\beta \omega_3}, \frac{\phi}{\omega_3}, \frac{2\pi i \omega_{13}}{\omega_3}, \frac{2\pi i \omega_{23}}{\omega_3}, 2\pi i \left( \frac{m}{\omega_3} + \frac{3}{2} \right) \right), \\ S_0 &= \frac{2\pi^2 \text{tr}(\phi^2)}{\beta \omega_1 \omega_2 \omega_3}, \end{aligned} \quad (17.3.3)$$

where  $\omega_i \equiv 1 + a_i$ ,  $\omega_{ij} \equiv \omega_i - \omega_j = a_i - a_j$ . ( $\frac{2\pi i \omega_{ij}}{\omega_j}$  appearing in the arguments may be replaced by  $\frac{2\pi i \omega_i}{\omega_j}$ , as was more commonly used in [15, 32], using the  $2\pi i$  period shifts of the arguments.) Here,  $G_r$  is the gauge group of the low energy 5d SYM that one obtains by reducing the 6d SCFT, and  $W(G_r)$  is the Weyl group of  $G_r$ . More abstractly, in the 6d CFT,

$W(G_r)$  acquires meaning as the Weyl group acting on the Coulomb branch as  $\mathbb{R}^r/W(G_r)$ , and  $\phi_I$  parametrizes the Coulomb branch  $\mathbb{R}^r$ .  $S_{\text{bkgd}}$  is a term which depends only on the background parameters  $\beta, \omega_i, m$ , which we shall explain further below. This expression has been proposed with two different motivations. See [15] for discussions involving topological strings. Here, we explain how (17.3.3) was proposed from the viewpoint of 5 dimensional supersymmetric Yang-Mills theory.

First consider the 6d theory on  $S^5 \times \mathbb{R}$ . The partition function (17.3.1) would be computed by a Euclidean 6d theory path integral on  $S^5 \times S^1$ , where the  $S^1$  has circumference  $\beta$  and various fields satisfy twisted boundary conditions due to the extra insertion  $-R + a_i j_i + m \cdot \frac{R_1 - R_2}{2}$ .<sup>3</sup> The twisted boundary conditions given by  $a_i j_i$  can be represented by deforming the background metric of  $S^5 \times S^1$  in a ‘complex’ manner as follows [16]:

$$\begin{aligned} ds^2(S^5 \times S^1) &= r^2 \sum_{i=1}^3 \left[ dn_i^2 + n_i^2 \left( d\phi_i + \frac{ia_i}{r} d\tau \right)^2 \right] + d\tau^2 \\ &= r^2 \sum_i \left[ dn_i^2 + n_i^2 d\phi_i^2 + \alpha^2 \left( \sum_j a_j n_j^2 d\phi_j \right)^2 \right] + \alpha^{-2} \left( d\tau + i\alpha^2 r \sum_j a_j n_j^2 d\phi_j \right)^2 \\ &\equiv g_{\mu\nu} dx^\mu dx^\nu + \alpha^{-2} (d\tau + rC)^2, \end{aligned} \tag{17.3.4}$$

where  $\alpha^{-2} \equiv 1 - \sum_j n_j^2 a_j^2$  and  $C \equiv i\alpha^2 \sum_j a_j n_j^2 d\phi_j$ . Here  $n_i$ ’s satisfy  $n_1^2 + n_2^2 + n_3^2 = 1$ , and  $\tau \sim \tau + \beta$ ,  $\phi \sim \phi_i + 2\pi$  periodicities are assumed. If one is uncomfortable about the complex metric, one can simply take the chemical potentials  $a_i$ ’s to be imaginary first, and later continue to real  $a_i$ ’s in the partition function (17.3.3) or 5d SYM. (It will be deforming the action to be complex.) We would like to understand the partition function (17.3.1) first in the regime  $\beta \ll 1$ , in which case one can make the Kaluza-Klein reduction of the 6d theory on a small circle to a 5d SYM on  $S^5$ .  $\beta = \frac{2\pi r_1}{r}$  in the dimensionless convention is the ratio of the radii of  $S^1$  and  $S^5$ . In particular, when  $\beta \ll 1$ , this is identified with the 5d SYM gauge coupling  $g_{YM}^2$  as  $\beta = \frac{g_{YM}^2}{2\pi r}$ . All terms in  $Z_{\mathbb{R}^4 \times T^2}$  appearing in the right hand side can be understood as non-perturbative instanton corrections for small  $\beta$  even from the 5d viewpoint, as we saw in the section 2.<sup>4</sup>

If we Kaluza-Klein reduce the 6d metric on  $\tau$  circle, one would naturally expect to have a supersymmetric Yang-Mills theory on a ‘squashed’  $S^5$  whose metric is given by  $g_{\mu\nu}$  above, also with a background ‘dilaton’ field  $\alpha$  and the background ‘gravi-photon’ field  $C$ . The last statement can be made more precise by finding (17.3.4) as a 5 dimensional off-shell supergravity background [69]. We find that this is the case. More precisely, we divide the construction of 5d SYM on  $S^5$  with metric  $g_{\mu\nu}$  into two steps. We first obtaining the vector

<sup>3</sup>For the convenience of arguments, we formally assume the existence of a 6d Lagrangian description and the path integral representation of (17.3.1). This is true for the free Abelian (2, 0) theory. For interacting theories, concrete arguments will only rely on the Lagrangian formulation of the 5d SYM at low energy, which exists.

<sup>4</sup>Sometimes, (17.3.3) makes sense even if the small circle reduction does not yield weakly-coupled 5d SYM. For instance, some 6d (1, 0) SCFTs on a circle flow to strongly interacting 5d SCFTs rather than 5d SYMs. However, viewing  $Z_{\mathbb{R}^4 \times T^2}$ ,  $\phi$  as the 6d partition functions and 6d scalars, (17.3.3) still makes sense, although we do not know how to derive it.

multiplet part of the action using off-shell supergravity methods, which is more cumbersome to achieve in a more conventional method. We then construct the hypermultiplet part of the action in a more brutal manner. The former can be easily done by using the 5d off-shell supergravity of [70], which realizes 8 off-shell SUSY of the background gravity and the dynamical vector multiplets. Construction of the hypermultiplet part of the action with one off-shell SUSY closely follows [27]. The results are summarized in appendix A.

At this point, let us comment that the metric  $g_{\mu\nu}$  of (17.3.4) may be just one special way of geometrizing the chemical potentials  $\omega_i$ . In the literature, alternative geometric realizations are also discussed, which lead to the same supersymmetric partition function (17.3.3) [15, 32].

With the action, SUSY and notations on the squashed  $S^5$  summarized in appendix A, we can understand the partition function (17.3.3) in more detail from 5d SYM. We first study the classical action at the possible saddle points. Expanding three  $\mathbb{Z}_{\mathbb{R}^4 \times T^2}$  factors in the series of  $e^{-\frac{4\pi^2 k_i}{\beta \omega_i}}$ , with  $i = 1, 2, 3$ , we find the following factor at each value of  $k_1, k_2, k_3$  and given  $\phi$ ,

$$\exp \left[ -\frac{1}{\beta} \left( \frac{2\pi^2 \text{tr}(\phi^2)}{\omega_1 \omega_2 \omega_3} + \sum_{i=1}^3 \frac{4\pi^2 k_i}{\omega_i} \right) \right]. \quad (17.3.5)$$

The exponent can be understood as the action of the following supersymmetric configurations. The SUSY transformation of the gaugino  $\chi^A$  in the vector multiplet is given by

$$\delta \chi^A = \frac{i}{2} (F_{\mu\nu} - \alpha^{-1} \phi V_{\mu\nu}) \gamma^{\mu\nu} \epsilon^A + \alpha D_\mu (\alpha^{-1} \phi) \gamma^\mu \epsilon^i - (D - i\alpha \phi \sigma_3)_B^A \epsilon^B, \quad (17.3.6)$$

where  $V = dC$ . Some off-shell supersymmetric configurations are given by taking  $\chi = 0$  and

$$F_{\mu\nu} = \phi_0 V_{\mu\nu}, \quad \phi = \alpha \phi_0, \quad D = i\alpha^2 \phi_0 \sigma_3 \quad (17.3.7)$$

with constant  $\phi_0$ , as explained in appendix A.  $\phi_0$  can be taken to be in the Cartan subalgebra, using the global part of the gauge transformation. This is not the most general supersymmetric configurations. To understand more general possibilities, we consider

$$(\delta \chi_A)^\dagger (\delta \chi^A) = \frac{1}{2f} (\hat{F}_{\mu\nu} \xi^\nu)^2 + \frac{1}{2f} \left( f \hat{F}_{\mu\nu} - \frac{1}{2} \epsilon_{\mu\nu\alpha\beta\gamma} \hat{F}^{\alpha\beta} \xi^\gamma \right)^2 + \alpha^2 f [D_\mu (\alpha^{-1} \phi)]^2 + f (i\hat{D})^2, \quad (17.3.8)$$

with  $\hat{F}_{\mu\nu} \equiv F_{\mu\nu} - \alpha^{-1} \phi V_{\mu\nu}$ ,  $\hat{D} \equiv D - i\alpha \phi \sigma_3$ . The vector  $\xi = \sum_{i=1}^3 \omega_i \frac{\partial}{\partial \phi_i}$  is a Killing spinor bilinear: see appendix A. So the following equations define supersymmetric configurations:

$$\hat{F}_{\mu\nu} \xi^\nu = 0, \quad \hat{F}_{\mu\nu} = \frac{1}{2} \epsilon_{\mu\nu\alpha\beta\gamma} \hat{F}^{\alpha\beta} \xi^\gamma / f, \quad D_\mu (\alpha^{-1} \phi) = 0, \quad D = i\alpha \phi \sigma_3. \quad (17.3.9)$$

The configuration (17.3.7) is a special solution to these equations with  $\hat{F}_{\mu\nu} = 0$ . Here, the first two equations are deformations of the so-called contact instanton equations [26, 64]. Locally, the first two equations demand that  $\hat{F}_{\mu\nu}$  is orthogonal to the vector  $\xi$ , and on the orthogonal 4-plane  $\hat{F}_{\mu\nu}$  satisfies the self-duality condition. Locally, it may look like be a self-duality equation on  $\mathbb{R}^4$ , namely an instanton string along  $\xi$ . But it is highly nontrivial if there would

be globally well defined solutions extending the flat space instanton solutions, or perhaps a completely new class of solutions on curved space which do not admit ‘instanton string’ picture from the flat space intuition. In particular, for generic  $\omega_i$ , the vector  $\xi$  generally does not generate a closed orbit on  $T^3$  spanned by the three angles  $\phi_i$ . So naively trying to extend the flat space instanton strings in curved space is likely to fail.

We have little idea on the general solutions to the above equations. There is one class of solutions in which the flat space solutions can be easily embedded in  $S^5$ . To understand this, first note that the  $\xi$  orbit on  $T^3$  closes at  $(n_1, n_2, n_3) = (1, 0, 0)$ ,  $(0, 1, 0)$  and  $(0, 0, 1)$ . This is because  $T^3$  degenerates to  $S^1$  at these points. So taking the small instanton strings in flat space (having zero sizes), and letting them wind one of these three circles, will generate singular configurations with finite action. With nonzero scalar  $\phi = \alpha\phi_0$ , we generically should embed these instantons to  $U(1)^r \subset G_r$  so that the field strength commutes with  $\phi_0$ . Let us assign  $k_1, k_2, k_3$  instanton strings to the above three locations. This can be superposed with the special solutions (17.3.7) since they are all in  $U(1)^r$ . As explained in appendix A, plugging in this configuration to the classical action precisely provides the weight (17.3.5). This motivates  $S_0$  and  $\tau_i = \frac{2\pi i}{\omega_i}$  appearing in the formula (17.3.3). Rigorous treatment is missing at this stage. See also [32, 34] for detailed discussions on this issue.

With these supersymmetric configurations identified, one should introduce  $Q$ -exact deformations which would yield (17.3.9) as saddle point equations, and then compute the 1-loop determinants. A factorization like [47] was assumed for the 1-loop determinant in [16] to identify the measure as given by (17.3.3). On  $S^4$ , the factorization happened due to such a property of the index theorem which captures the BPS modes contributing to the determinant, and we expect our factorization in (17.3.3) could be derived by a similar careful treatment.<sup>5</sup> More pragmatically, the factorization has been also shown at a perturbative level by an independent computation [32, 33], which then very naturally suggests the factorized result (17.3.3) at the full non-perturbative level. The same factorized formula has been obtained by exploring the relation between topological strings and supersymmetric partition functions [15]. With this factorized measure, one should integrate and sum over the saddle point parameters  $\phi_0, k_1, k_2, k_3$ , which leads to (17.3.3). (We dropped the subscript of  $\phi_0$  in 17.3.3.)

In the next subsection, we shall study the physics of (17.3.3) for the  $(2, 0)$  theory, in various cases in which (17.3.3) can be handled more concretely.

### 17.3.2 The $(2, 0)$ index, $W_N$ characters and Casimir energy

The index (17.3.3) has been studied in more detail for the  $(2, 0)$  SCFTs, especially in the  $A_{N-1}$  case in which the 5d instanton counting has been best understood. The technical issue concerning the expression (17.3.3) is that it is given in a ‘weak coupling’ expansion form, taking the form of series expansion in  $\beta$  and  $e^{-\frac{4\pi^2}{\beta\omega_i}}$  when  $\beta \ll 1$  after  $\phi$  integral. However, the index structure of  $Z_{S^5 \times S^1}$  will be best visible in the regime  $\beta \gg 1$ , as a series expansion in  $e^{-\beta}$ . At the moment, this re-expansion in the regime  $\beta \gg 1$  has been achieved only in two

<sup>5</sup>Once the factorization is assumed, the effective  $\epsilon_1, \epsilon_2, m$  parameters can be determined by investigating the coefficients of the bosonic symmetry appearing on the right hand side of  $\{Q, S\}$  algebra.

special cases. One is the 6d Abelian (2, 0) index with all fugacities turned on, and another is the non-Abelian index with all but one fugacities tuned to special values. In this subsection, we shall explain these two.<sup>6</sup>

**Abelian (2, 0) index:** We should first explain what is the virtue of studying the Abelian theory, as the 6d theory is free. In fact the superconformal index of the free 6d (2, 0) tensor multiplet is computed in [46]. In our convention, it is given by

$$Z_{S^5 \times S^1}(\beta, m, a_i) = e^{-\beta\epsilon_0} \exp \left[ \sum_{n=1}^{\infty} \frac{1}{n} f(n\beta, nm, na_i) \right], \quad (17.3.10)$$

$$f(\beta, m, a_i) = \frac{e^{-\frac{3\beta}{2}}(e^{\beta m} + e^{-\beta m}) - (e^{-\beta(\omega_1+\omega_2)} + e^{-\beta(\omega_2+\omega_3)} + e^{-\beta(\omega_3+\omega_1)}) + e^{-3\beta}}{(1 - e^{-\beta\omega_1})(1 - e^{-\beta\omega_2})(1 - e^{-\beta\omega_3})},$$

where we used  $\omega_i = 1 + a_i$ .  $\epsilon_0$  is the ‘zero point energy’ factor, which is in general regularization scheme dependent. We shall explain this factor in more detail below in this subsection. Since we know this (trivial) index concretely, one might wonder what is the virtue of getting it from (17.3.3). The first reason is simply to check that (17.3.3) correctly provides the well known results. The second reason is to emphasize the precise meaning of the formula (17.3.3). The equation (17.3.10) is given in the form of a series expansion in  $e^{-\beta} \ll 1$ . By expanding  $f(\beta, m, a_i)$  in a series in  $e^{-\beta}$ , one would obtain an infinite product expression for  $Z_{S^5 \times S^1}$  for the Abelian theory:

$$q^{\epsilon_0} \prod_{n_1=0}^{\infty} \prod_{n_2=0}^{\infty} \prod_{n_3=0}^{\infty} \frac{(1 - q^{2+n_1+n_2+n_3} \zeta_1^{n_1-1} \zeta_2^{n_2} \zeta_3^{n_3})(1 - q^{2+n_1+n_2+n_3} \zeta_1^{n_1} \zeta_2^{n_2-1} \zeta_3^{n_3})(1 - q^{2+n_1+n_2+n_3} \zeta_1^{n_1} \zeta_2^{n_2} \zeta_3^{n_3-1})}{(1 - yq^{\frac{3}{2}+n_1+n_2+n_3} \zeta_1^{n_1} \zeta_2^{n_2} \zeta_3^{n_3})(1 - y^{-1}q^{\frac{3}{2}+n_1+n_2+n_3} \zeta_1^{n_1} \zeta_2^{n_2} \zeta_3^{n_3})(1 - q^{3+n_1+n_2+n_3} \zeta_1^{n_1} \zeta_2^{n_2} \zeta_3^{n_3})},$$

where  $q = e^{-\beta}$ ,  $\zeta_i = e^{-\beta a_i}$ ,  $y = e^{-\beta m}$ . This is well defined for small enough  $q$ .

Now to see if this index is reproduced from (17.3.3), we should sum over all the  $q$  series appearing in the  $Z_{\mathbb{R}^4 \times T^2}$  factors, and make a ‘strong coupling’ expansion to compare with (17.3.11). Alternatively, one can make a ‘weakly coupled’ expansion of (17.3.10) and confirm that we obtain (17.3.3). Using suitable contour integral expression for  $\log Z_{S^5 \times S^1}$  obtained from (17.3.10) [18] or using some properties of the triple sine functions [15], one could make an expansion of (17.3.10) which is given by

$$Z_{S^5 \times S^1} = \left[ \frac{\beta\omega_1\omega_2\omega_3}{2\pi} \right]^{\frac{1}{2}} e^{-\beta\epsilon_0 - \frac{\beta}{24} \left( 1 + \frac{2a_1 a_2 a_3 + (1-a_1 a_2 - a_2 a_3 - a_3 a_1)(\frac{1}{4} - m^2) + (\frac{1}{4} - m^2)^2}{\omega_1 \omega_2 \omega_3} \right)} e^{\frac{\pi^2(\omega_1^2 + \omega_2^2 + \omega_3^2 - 2\omega_1\omega_2 - 2\omega_2\omega_3 - \omega_3\omega_1 + 4m^2)}{24\beta\omega_1\omega_2\omega_3}}$$

$$\cdot Z_{\text{pert}} \left( \frac{2\pi i \omega_{21}}{\omega_1}, \frac{2\pi i \omega_{31}}{\omega_1}, 2\pi i \left( \frac{m}{\omega_1} + \frac{3}{2} \right) \right) Z_{\text{inst}} \left( \frac{2\pi i}{\beta\omega_1}, \frac{2\pi i \omega_{21}}{\omega_1}, \frac{2\pi i \omega_{31}}{\omega_1}, 2\pi i \left( \frac{m}{\omega_1} + \frac{3}{2} \right) \right)$$

$$\cdot \left( 1, 2, 3 \rightarrow 2, 3, 1 \right) \left( 1, 2, 3 \rightarrow 3, 1, 2 \right), \quad (17.3.11)$$

---

<sup>6</sup>In principle, there would be an issue of whether we know the exact form of  $Z_{\mathbb{R}^4 \times T^2}$  from various expansions only, as explained in section 2. In all cases in which we made concrete studies, we were able to find exact expressions which yield the known series expansions in  $\beta^n e^{-\frac{4\pi^2 k}{\beta}}$  with non-negative integers  $n, k$  at  $\beta \ll 1$

where the last two factors the repetitions of the second line with the 1, 2, 3 subscripts of  $\omega_i$  permuted,  $Z_{\text{pert}}$  is the perturbative  $U(1)$  maximal SYM partition function on the  $\Omega$  deformed  $\mathbb{R}^4 \times S^1$ , and  $Z_{\text{inst}}$  is the ‘instanton’ part of the  $U(1)$  maximal SYM on  $\mathbb{R}^4 \times S^1$  [35, 36, 71]

$$Z_{\text{inst}}(\tau, \epsilon_1, \epsilon_2, m_0) = \exp \left[ \sum_{n=1}^{\infty} \frac{1}{n} \frac{\sinh \frac{n(m_0 + \epsilon_-)}{2} \sinh \frac{n(m_0 - \epsilon_-)}{2}}{\sinh \frac{n\epsilon_1}{2} \sinh \frac{n\epsilon_2}{2}} \frac{e^{2\pi i n \tau}}{1 - e^{2\pi i n \tau}} \right], \quad (17.3.12)$$

which is identical to (17.2.14) when we expand (17.3.12) in  $e^{2\pi i \tau}$ . Note that neither  $Z_{\text{pert}}$ ,  $Z_{\text{inst}}$  depends on the  $U(1)$  Coulomb VEV  $\phi$ . So the first factor  $[\frac{\beta\omega_1\omega_2\omega_3}{2\pi}]^{\frac{1}{2}}$  can be replaced by

$$\left( \frac{\beta\omega_1\omega_2\omega_3}{2\pi} \right)^{\frac{1}{2}} = \int_{-\infty}^{\infty} d\phi \exp \left( -\frac{2\pi^2\phi^2}{\beta\omega_1\omega_2\omega_3} \right), \quad (17.3.13)$$

which is the Gaussian integral in (17.3.3) with the measure  $e^{S_0}$ . So the known index (17.3.10) would be completely agreeing with (17.3.3) if we identify  $Z_{\mathbb{R}^4 \times T^2} = Z_{\text{pert}}Z_{\text{inst}}$  and if we take

$$\begin{aligned} \epsilon_0 &= -\frac{1}{24} \left[ 1 + \frac{2a_1a_2a_3 + (1 - a_1a_2 - a_2a_3 - a_3a_1)(\frac{1}{4} - m^2) + (\frac{1}{4} - m^2)^2}{\omega_1\omega_2\omega_3} \right], \\ S_{\text{bkgd}} &= -\frac{\pi^2(\omega_1^2 + \omega_2^2 + \omega_3^2 - 2\omega_1\omega_2 - 2\omega_2\omega_3 - \omega_3\omega_1 + 4m^2)}{24\beta\omega_1\omega_2\omega_3}. \end{aligned} \quad (17.3.14)$$

We shall explain these three identifications about  $\epsilon_0$ ,  $S_{\text{bkgd}}$  and  $Z_{\text{inst}}$ , in turn.

Firstly,  $\epsilon_0$  is the vacuum ‘Casimir energy’ which we shall explain later in this subsection. For now, we simply regard (17.3.3) as giving a specific value of the vacuum energy at  $\beta \gg 1$  expansion. Secondly,  $S_{\text{bkgd}}$  couples the parameters  $g_{YM}^2, m$  of the theory to the background parameters of  $S^5$ , such as  $r, \omega_i$ . In particular, it takes the form of the leading free energy in the ‘high temperature’ regime  $\beta \ll 1$ . From the analysis of one lower dimension on  $S^5$ , this data cannot be determined in a self-contained way, and should be given as an input. One can think about it in two different viewpoints. One may first regard  $S_{\text{bkgd}}$  as our ignorance, but demand that we tune it so that the strong coupling expansion of (17.3.3) becomes an index. It is an extremely nontrivial request that tuning  $S_{\text{bkgd}}$  in negative powers of  $\beta$  yields an index at  $\beta \gg 1$ . As the above results in the Abelian theory shows, it completely fixes  $S_{\text{bkgd}}$  if one can freely do both weak and strong coupling expansions. Furthermore, the general structures of the high temperature asymptotics of the the 6d SCFT index was proposed in [72]. They only considered the angular momentum chemical potentials  $\omega_i$ , with  $m = 0$ , and completely fixed the  $\beta, \omega_i$  dependence apart from a few central charge coefficients. Of course their proposal is consistent with (17.3.14) at  $m = 0$ .

So we finally explain  $Z_{\mathbb{R}^4 \times T^2} = Z_{\text{pert}}Z_{\text{inst}}$ . At first sight, it sounds strange that 5d  $U(1)$  maximal SYM exhibits such a nontrivial ‘instanton’ factor  $Z_{\text{inst}}$ , as  $U(1)$  adjoint theory looks free. However, one should understand how Nekrasov’s ‘instanton calculus’ yielded a nontrivial result (17.3.12). This is because Nekrasov actually did not work with this free QFT, but worked with a UV completion of it. Namely, just as we explained in section 2, without any logical reference to 5d SYM, what we call Nekrasov’s ‘instanton partition function’ is a string

theory result, especially for non-renormalizable QFTs. The equation (17.3.12) gains a solid meaning as the index for  $k$  D0-branes bound to 1 D4-brane. In our context,  $Z_{\mathbb{R}^4 \times T^2}$  is the true 6d CFT observable computed from the string or M-theory engineering. So although we attempted to find motivations and supports of the expression (17.3.3) from 5d SYM, our true claim is that the integrand  $Z_{\mathbb{R}^4 \times T^2}$  should naturally be understood as the 6d observable, without necessarily relying on the UV incomplete 5d SYM. See [41] for more discussions on  $Z_{\text{inst}}$  as a more abstract 6d observable. So understanding that we should use  $Z_{\mathbb{R}^4 \times T^2}$  computed from string theory, the identification  $Z_{\mathbb{R}^4 \times T^2} = Z_{\text{pert}} Z_{\text{inst}}$  with (17.3.12) is justified. **Unrefined non-Abelian (2, 0) indices:** Now we turn to more interesting non-Abelian indices. Again we shall restrict our interest to the (2, 0) theory here, as we shall crucially use simplifications coming from extra SUSY when some chemical potentials are tuned. Namely, consider the following tuning of the  $U(1) \subset SO(5)_R$  chemical potential for  $\frac{R_1 - R_2}{2}$ :

$$m = \frac{1}{2} - a_3 . \quad (17.3.15)$$

The index can then be written as

$$Z_{S^5 \times S^1}(\beta, \frac{1}{2} - a_3, a_i) = \text{Tr} \left[ (-1)^F e^{-\beta(E - R_1)} e^{-\beta a_1(j_1 - j_3 - \frac{R_1 - R_2}{2})} e^{-\beta(j_2 - j_3 - \frac{R_1 - R_2}{2})} \right] . \quad (17.3.16)$$

Apart from the supercharges  $Q \equiv Q_{--}^{++}$ ,  $S \equiv S_{++}^{--}$  which commute with this measure by construction, two extra supercharges  $Q_{+-}^{+-}$ ,  $S_{-+}^{-+}$  commute with it at (17.3.15). So the index exhibits more cancellations of bosons/fermions paired by the extra supercharges, which will make the index simpler. The SYM on  $S^5$  will also preserve more SUSY. We will show shortly that the equation (17.3.3) can be exactly computed at this point. We also note that further tunings

$$m = \frac{1}{2} , \quad a_1 = a_2 = a_3 = 0 \quad (17.3.17)$$

will leave only one chemical potential  $\beta$ , in which case the measure of the index

$$Z_{S^5 \times S^1}(\beta, \frac{1}{2}, 0) = \text{Tr} \left[ (-1)^F e^{-\beta(E - R_1)} \right] \quad (17.3.18)$$

commutes with 16 of the 32 supercharges of the (2, 0) theory. Namely, the following 8 complex supercharges  $Q_{\pm\pm\pm}^{\pm\pm}$  (with the  $\pm$  subscripts satisfying  $\pm\pm\pm = -$ ) and their conjugates  $S_{\pm\pm\pm}^{-\pm}$  (with subscripts satisfying  $\pm\pm\pm = +$ ) commute with  $e^{-\beta(E - R_1)}$ . The presence of 16 SUSY will have special implication on the index, especially concerning the ‘zero point energy’ of the vacuum which is captured by the index. Also, one would naturally expect that the circle reduction of the 6d theory at (17.3.17) will yield a maximal SYM which actually preserves 16 supercharges. This is indeed the case [12]. See also [17].

To understand the simplification at the level of the formula (17.3.3), we first study how the  $\Omega$  background parameters and the mass parameters simplify. In the notation of section 2,

the effective  $\Omega$  parameters  $\epsilon_1, \epsilon_2$  and the mass  $m_0$  in the three  $Z_{\mathbb{R}^4 \times T^2}$  factors are given by

$$\begin{aligned} \frac{1}{2\pi i}(\epsilon_1, \epsilon_2, m_0) &= \left( \frac{\omega_2 - \omega_1}{\omega_1}, \frac{\omega_3 - \omega_1}{\omega_1}, \frac{m}{\omega_1} + \frac{3}{2} \right) \sim \left( \frac{\omega_2 - \omega_1}{\omega_1}, \frac{\omega_3 - \omega_1}{\omega_1}, \frac{m}{\omega_1} - \frac{1}{2} \right) : \text{1st} \\ &\left( \frac{\omega_3 - \omega_2}{\omega_2}, \frac{\omega_1 - \omega_2}{\omega_2}, \frac{m}{\omega_2} - \frac{1}{2} \right) : \text{2nd} \\ &\left( \frac{\omega_1 - \omega_3}{\omega_3}, \frac{\omega_2 - \omega_3}{\omega_3}, \frac{m}{\omega_3} - \frac{1}{2} \right) : \text{3rd} . \end{aligned} \quad (17.3.19)$$

We use  $m_0$  for the effective mass parameter on  $\mathbb{R}^4 \times T^2$ , to avoid confusions with the actual mass parameter of 5d SYM on  $S^5$ , or the chemical potential  $\beta m$  of the 6d index. Also, we used the fact that all parameters  $\epsilon_1, \epsilon_2, m_0$  are periodic variables in  $2\pi i$  shifts. So at (17.3.15), one finds

$$\begin{aligned} \frac{1}{2\pi i}(\epsilon_1, \epsilon_2, m_0) &= \left( \frac{\omega_2 - \omega_1}{\omega_1}, \frac{\omega_3 - \omega_1}{\omega_1}, \frac{\omega_2 - \omega_3}{2\omega_1} \right) : \text{1st} \\ &\left( \frac{\omega_3 - \omega_2}{\omega_2}, \frac{\omega_1 - \omega_2}{\omega_2}, \frac{\omega_1 - \omega_3}{2\omega_2} \right) : \text{2nd} \\ &\left( \frac{\omega_1 - \omega_3}{\omega_3}, \frac{\omega_2 - \omega_3}{\omega_3}, \frac{\omega_1 + \omega_2 - 2\omega_3}{2\omega_3} \right) : \text{3rd} . \end{aligned} \quad (17.3.20)$$

Defining  $\epsilon_{\pm} \equiv \frac{\epsilon_1 \pm \epsilon_2}{2}$ , we find that these effective parameters satisfy  $m_0 = \epsilon_-$  in the first factor,  $m_0 = -\epsilon_-$  in the second factor, and  $m = \epsilon_+$  in the third factor.

Let us explain that the partition function  $Z_{\mathbb{R}^4 \times T^2}$  simplifies in all the three factors. Note that  $Z_{\mathbb{R}^4 \times T^2}(q, v, \epsilon_{1,2}, m_0)$  takes the following form:

$$\begin{aligned} Z_{\mathbb{R}^4 \times T^2} &= Z_{\text{pert}}(v, \epsilon_{1,2}, m_0) Z_{\text{inst}}(q, v, \epsilon_{1,2}, m_0) , \quad (17.3.21) \\ Z_{\text{pert}} &= \widetilde{PE} \left[ \frac{1}{2} \frac{\sin \frac{m_0 + \epsilon_+}{2} \sin \frac{m_0 - \epsilon_+}{2}}{\sin \frac{\epsilon_1}{2} \sin \frac{\epsilon_2}{2}} \chi_{\text{adj}}(v) \right] , \end{aligned}$$

where  $Z_{\text{inst}}$  is given in section 2, and

$$\chi_{\text{adj}}(v) = \sum_{\alpha \in \text{adj}(G)} e^{\alpha(v)} . \quad (17.3.22)$$

$\widetilde{PE}$  is defined by expanding the function in  $\widetilde{PE}[\dots]$  in  $e^{-\epsilon_{1,2}}, e^{-m_0}, e^{-\alpha(v_i)}$ , and imposing

$$\widetilde{PE}[ne^{-x}] = \left[ 2 \sinh \frac{x}{2} \right]^n = \left[ \frac{e^{-\frac{x}{2}}}{1 - e^{-x}} \right]^n , \quad \widetilde{PE}[f + g] = \widetilde{PE}[f] \widetilde{PE}[g] . \quad (17.3.23)$$

As for  $Z_{\text{inst}}$ , the  $U(N)$  result is known well in the series expansion in  $q$ , as explained in section 2. For  $D_N$  cases, the  $SO(2N)$  partition function is in principle computable from [41], but not very much have been done in detail so far. For  $E_N$ , almost nothing is known, although we shall say something about it below. Here we would like to emphasize the general structure of  $Z_{\text{pert}}$  and  $Z_{\text{inst}}$ . Since  $Z_{\text{pert}}$  and  $Z_{\text{inst}}$  count BPS particles on  $\mathbb{R}^{4,1}$  in the Coulomb phase,

they carry universal prefactors from their center-of-mass supermultiplets. In particular, since perturbative particles and instantons preserve different 8 supercharges among the full 16 as massive vector and tensor multiplets, respectively, the prefactors appearing in the two parts are different. It is easy to check [37] that

$$Z_{\text{pert}} = \widetilde{PE} [I_+(\epsilon_{1,2}, m_0)(\dots)] \quad , \quad Z_{\text{inst}} = \widetilde{PE} [I_-(\epsilon_{1,2}, m_0)(\dots)] \quad . \quad (17.3.24)$$

( $\dots$ ) are the contributions from internal degrees of freedom of the BPS states, which are regular in  $\epsilon_1 = \epsilon_2 = m_0 = 0$  the limit, and

$$I_{\pm}(\epsilon_{1,2}, m_0) \equiv \frac{\sin \frac{m_0 + \epsilon_{\pm}}{2} \sin \frac{m_0 - \epsilon_{\pm}}{2}}{\sin \frac{\epsilon_1}{2} \sin \frac{\epsilon_2}{2}} \quad . \quad (17.3.25)$$

For  $Z_{\text{pert}}$ , this structure is already manifest in (17.3.21).

Firstly, at  $m_0 = \pm\epsilon_-$ , one finds from (17.3.25) and (17.3.24) that  $I_-(\epsilon_{1,2}, \pm\epsilon_-) = 0$  and  $Z_{\text{inst}} = 1$ . Therefore, in the unrefined limit (17.3.15), one finds that the first and second  $Z_{\mathbb{R}^4 \times T^2}$  factors in (17.3.3) reduces to the perturbative contributions at this point. Note also from (17.3.25) that  $I_+(\epsilon_{1,2}, \pm\epsilon_-) = -1$ . So applying this to (17.3.21), one obtains

$$Z_{\mathbb{R}^4 \times T^2} \rightarrow \widetilde{PE} \left[ -\frac{1}{2} \chi_{\text{adj}}(v) \right] \quad (17.3.26)$$

at  $m_0 = \pm\epsilon_-$ . So applying this to the first and second factors of (17.3.3), one obtains

$$Z_{\mathbb{R}^4 \times T^2}^{(1)} Z_{\mathbb{R}^4 \times T^2}^{(2)} \rightarrow \widetilde{PE} \left[ -\frac{1}{2} (\chi_{\text{adj}}(v/\omega_1) + \chi_{\text{adj}}(v/\omega_2)) \right] = \prod_{\alpha > 0} 2 \sinh \frac{\alpha(v)}{\omega_1} \cdot 2 \sinh \frac{\alpha(v)}{\omega_2} \quad , \quad (17.3.27)$$

where the product is over positive roots of  $G$ , up to a possible overall sign on which we are not very careful. We then turn to  $Z_{\mathbb{R}^4 \times T^2}^{(3)}$  at  $m_0 = \epsilon_+$ . From (17.3.24) or (17.3.21), it is obvious that  $Z_{\text{pert}} = 1$  at  $m_0 = \epsilon_+$ , since  $I_+ = 0$ . So  $Z_{\mathbb{R}^4 \times T^2}$  acquires  $Z_{\text{inst}}$  contribution only at  $m = \epsilon_+$ . For  $U(N)$ , one can easily show from the  $U(N)$  instanton partition function of section 2 that

$$Z_{\text{inst}}(\beta, \epsilon_{1,2}, m_0 = \pm\epsilon_+) = \frac{1}{\eta(\tau)^N} = e^{-\frac{\pi N i \tau}{12}} \prod_{n=1}^{\infty} \frac{1}{(1 - e^{2\pi n i \tau})^N} \quad . \quad (17.3.28)$$

where  $\tau = \frac{2\pi i}{\beta}$ . Here, we have included the extra factor of

$$e^{-S_{\text{bkgd}}} = e^{-\frac{\pi N i \tau}{12}} = e^{\frac{\pi^2 N}{6\beta}} \quad , \quad (17.3.29)$$

which will be justified below. More generally, we shall present below nontrivial evidences that

$$e^{-S_{\text{bkgd}}} Z_{\text{inst}}(\beta, \epsilon_{1,2}, m_0 = \pm\epsilon_+) = \frac{1}{\eta(\tau)^N} \quad (17.3.30)$$

for all  $U(N)$ ,  $D_N = SO(2N)$ ,  $E_N$  groups. If one wishes to consider the interacting  $A_{N-1}$  part only, instead of  $U(N)$ , one simply takes  $Z_{\text{inst}} = \eta(\tau)^{-(N-1)}$  by dropping an overall  $U(1)$  factor  $Z_{\text{inst}}^{U(1)} = \eta(\tau)^{-1}$ . So  $e^{-S_{\text{bkgd}}} Z_{\mathbb{R}^4 \times T^2}^{(3)}$  simplifies to

$$e^{-S_{\text{bkgd}}} Z_{\mathbb{R}^4 \times T^2}^{(3)} \rightarrow \frac{1}{\eta(\tau/\omega_3)^N} = \frac{1}{\eta\left(\frac{2\pi i}{\beta\omega_3}\right)^N} \quad (17.3.31)$$

in the limit (17.3.15), for all  $A_N$ ,  $D_N$ ,  $E_N$  series.

With all the simplifications (17.3.27), (17.3.31), the partition function (17.3.3) on  $S^5$  reduces to

$$Z_{S^5 \times S^1}(\beta, m = \frac{1}{2} - a_3, a_i) = \frac{1}{\eta\left(\frac{2\pi i}{\beta\omega_3}\right)^N} \cdot \frac{1}{W(G_N)} \int \prod_{I=1}^N d\phi_I e^{-\frac{2\pi^2 \text{tr}(\phi^2)}{\beta\omega_1\omega_2\omega_3}} \prod_{\alpha>0} 2 \sinh \frac{\alpha(\phi)}{\omega_1} \cdot 2 \sinh \frac{\alpha(\phi)}{\omega_2}. \quad (17.3.32)$$

The integral over  $\phi_I$  is simply a Gaussian integral. The result of the integral is

$$Z_{S^5 \times S^1}(\beta, m = \frac{1}{2} - a_3, a_i) = \left(\frac{\beta\omega_3}{2\pi}\right)^{\frac{N}{2}} \frac{1}{\eta\left(\frac{2\pi i}{\beta\omega_3}\right)^N} e^{\frac{\beta c_2 |G|}{24} \omega_3 \left(\frac{\omega_1}{\omega_2} + \frac{\omega_2}{\omega_1}\right)} \prod_{\alpha>0} 2 \sinh \left(\beta\omega_3 \frac{\alpha \cdot \rho}{2}\right), \quad (17.3.33)$$

where  $\rho$  is the Weyl vector. Since  $\eta(\tau)$  is a modular form, its expansion in the  $\beta \gg 1$  regime is easy to understand. The result is given by

$$\begin{aligned} Z_{S^5 \times S^1}(\beta, \frac{1}{2} - a_3, a_i) &= e^{\beta \frac{c_2 |G|}{24} \frac{\omega_3}{\omega_1 \omega_2} (\omega_1 + \omega_2)^2} \prod_{\alpha>0} (1 - e^{-\beta\omega_3 \alpha \cdot \rho}) \cdot \frac{1}{\eta\left(\frac{i\beta\omega_3}{2\pi}\right)^N} \\ &= e^{\beta \frac{c_2 |G|}{24} \frac{\omega_3}{\omega_1 \omega_2} (\omega_1 + \omega_2)^2 + \frac{N\beta\omega_3}{24}} \prod_{\alpha>0} (1 - e^{-\beta\omega_3 \alpha \cdot \rho}) \cdot \prod_{n=1}^{\infty} \frac{1}{(1 - e^{-n\beta\omega_3})^N}. \end{aligned} \quad (17.3.34)$$

After a little computation for the cases  $G = U(N)$ ,  $D_N$ ,  $E_N$  (the reference [16] for the  $A$  and  $D$  cases), one obtains

$$Z_{S^5 \times S^1}(\beta, \frac{1}{2} - a_3, a_i) = e^{\beta \frac{c_2 |G|}{24} \frac{\omega_3}{\omega_1 \omega_2} (\omega_1 + \omega_2)^2 + \frac{N\beta\omega_3}{24}} \prod_{s=0}^{\infty} \prod_{d=\text{deg}[C(G)]} \frac{1}{1 - e^{-\beta\omega_3(d+s)}} \quad (17.3.35)$$

where  $d$  runs over the degrees of the possible Casimir operators  $C(G)$  of the group  $G$ . More concretely, the degrees of the Casimir operators are

$$\begin{aligned} U(N) &: 1, 2, \dots, N \\ SO(2N) &: 2, 4, \dots, 2N - 2 \text{ and } N \\ E_6 &: 2, 5, 6, 8, 9, 12 \\ E_7 &: 2, 6, 8, 10, 12, 14, 18 \\ E_8 &: 2, 8, 12, 14, 18, 20, 24, 30 \end{aligned} \quad (17.3.36)$$

for all ADE groups. We shall shortly give physical interpretations of these results.

Before proceeding to the interpretation of the result, we emphasize that the expression (17.3.3) obtained at  $\beta \ll 1$  successfully becomes an index (or more generally, partition function which counts states) in the  $\beta \gg 1$  regime, meaning that an expansion in  $e^{-\beta} \ll 1$  has integer coefficients only. At this stage, we can justify the choice of  $S_{\text{bkgd}} = -\frac{\pi^2 N}{6\beta}$ . Just as in the Abelian case, we had to add this part by hand, as our supports on (17.3.3) came from one lower dimension in the high temperature regime. Namely, the leading singular behaviors of the free energy (coming in negative powers of  $\beta$ ) have to be inputs in this approach. This input is all encoded in  $S_{\text{bkgd}}$ , in the form of the couplings of the parameters of the theory to the background gravity fields. As in the Abelian case,  $S_{\text{bkgd}}$  in negative powers of  $\beta$  is uniquely fixed by demanding the full quantity to be an index at  $\beta \gg 1$ . The structure of such couplings  $S_{\text{bkgd}}$  has been explored in [72] in the case of  $S^3 \times S^1$  using 3 dimensional supergravity, and similar studies are made on  $S^5 \times S^1$ . In particular, the absence of a term proportional to  $\beta^{-3}$  in our  $S_{\text{bkgd}}$  is consistent with what [72] proposes for the (2, 0) theory.

Also note that the choice (17.3.30) for all ADE group is consistent with the requirement to have an index at  $\beta \gg 1$ , because the modular transformation of  $\eta^{-N}$  to go to the  $\beta \gg 1$  regime exactly absorbs the factor  $\left(\frac{\beta\omega_3}{2\pi}\right)^{\frac{N}{2}}$  in (17.3.33), which could have obstructed the index interpretation. Below we shall provide more support of our choice (17.3.30) for DE groups.

We now study the physics of (17.3.35). We first consider the ‘spectrum’ part of this index,

$$\prod_{s=0}^{\infty} \prod_{d=\text{deg}[C(G)]} \frac{1}{1 - q^{d+s}} = PE \left[ \frac{\sum_{d=\text{deg}[C(G)]} q^d}{1 - q} \right], \quad (17.3.37)$$

where we defined  $q \equiv e^{-\beta\omega_3}$ , and  $PE$  here is defined in a more standard manner,  $PE[f(x)] \equiv \exp \left[ \sum_{n=1}^{\infty} \frac{1}{n} f(x^n) \right]$ , without including the zero point energy factors. All coefficients of this index in  $q$  expansion has positive coefficients, implying the possibility that this could actually be a partition function counting bosonic states/operators only. This is independently supported by other studies on the 6d (2, 0) theory [73], which identified a closed 2d bosonic chiral subsector of the operator product expansions of local operators.

To give a more intuitive feelings on (17.3.37), we shall first explain an analogous situation in the 4d  $\mathcal{N} = 4$  Yang-Mills theory with ADE gauge groups, in which (17.3.37) also emerges as the partition function of a class of BPS operators. In the 4d SYM, we are interested in gauge invariant BPS operators in the weakly coupled theory, consisting of one complex scalar  $\Phi$  and one of the two holomorphic derivatives on  $\mathbb{R}^4$ , which we call  $\partial$ . The spectrum of these operators in the weakly coupled regime is worked out in [74]. In particular, we are interested in local operators  $\mathcal{O}$  which are annihilated by a specific  $Q$ ,  $Q\mathcal{O} = 0$ , with the equivalence relation  $\mathcal{O} \sim \mathcal{O} + Q\lambda$ , so we are interested in the cohomology elements. It was shown that the cohomology elements can be constructed using the  $\Phi$  letters with  $\partial$  derivatives only. The cohomology elements can be constructed by multiplying elements of the form

$$\partial^s f(\Phi), \quad (17.3.38)$$

where  $f(\Phi)$  is any gauge invariant expression for the matrix  $\Phi$ , and then linearly superposing all possible operators constructed this way. So the question is to find the independent

‘generators’ taking the form of (17.3.38). Note that if  $f$  satisfies  $f(\Phi) = g(\Phi)h(\Phi)$  or  $f(\Phi) = g(\Phi) + h(\Phi)$  with other gauge invariant expressions  $g(\Phi), h(\Phi)$ , then (17.3.38) is no longer an independent generator. With these considerations, if one takes  $f(\Phi)$  to be all possible independent Casimir operators of the gauge group, then (17.3.38) forms the complete set of generators of the cohomology. The dimension of  $\Phi$  is 1, so the dimension of the operator  $f(\Phi)$  is the degree of the Casimir operator. So for instance, for ADE gauge groups, this leads to the scale dimension spectrum (17.3.36) of the  $f(\Phi)$  appearing in the generator (17.3.38). For instance, the generators for  $U(N)$  are  $f(\Phi) = \text{tr}(\Phi^n)$  with  $n = 1, \dots, N$ . The generators for  $SU(N)$  also takes the same form, with  $n = 2, \dots, N$ . The generators for  $SO(2N)$  are  $f(\Phi) = \text{tr}(\Phi^2), \dots, \text{tr}(\Phi^{2N-2})$  and  $\text{Pf}(\Phi) = \sqrt{\det \Phi}$ . Thus the partition function for these generators, where the letters with scale dimension  $\Delta$  are weighted by  $q^\Delta$ , is given by

$$z(q)_{\text{letter}} = \sum_{s=0}^{\infty} \sum_{d \in \text{deg}[C(G)]} q^{d+s} = \frac{\sum_{d \in \text{deg}[C(G)]} q^d}{1 - q}, \quad (17.3.39)$$

where  $\Delta[\Phi] = \Delta[\partial] = 1$ . Now the full set of the cohomology is obtained by forming the Fock space of the generators (17.3.38), and the partition function over this space is given by (17.3.37).

To summarize, from 4d maximal SYM, we obtained the same partition function as what we got for the 6d (2,0) theory. This is not strange. For instance, had we been counting gauge invariant operators made of scalar  $\Phi$  only without any derivatives, this would have given us the half-BPS states whose partition function is given by  $PE[\sum_{d \in \text{deg}[C(G)]} q^d]$ . The half-BPS partition function is known to be universal in all maximal superconformal field theories, in 3,4,6 dimensions. There is also an explanation of this universality, by quantizing and counting the states of half-BPS giant gravitons in the AdS duals [75, 76]. Even after including one derivative, one can follow the D3-brane giant graviton counting of the partition function (17.3.37) in  $AdS_5 \times S^5$  [74, 77], to quantize and count the M5-brane giant gravitons on  $AdS_7 \times S^4$  to obtain the same partition function (at least for the A and D series). At this point, let us mention that the large  $N$  limits of (17.3.37) for  $U(N)$  and  $SO(2N)$  completely agree with the supergravity indices on  $AdS_7 \times S^4$  and  $AdS_7 \times S^4/\mathbb{Z}_2$ , respectively [12, 16]. It is also reassuring to find that the chiral algebra arguments of [73] naturally suggest the same partition function (17.3.37), for all ADE cases. So turning the logic around, the natural result (17.3.37) also supports our conjecture (17.3.30) on the instanton correction for the gauge groups DE. (The case with  $SO(2N)$  may be derivable with the results of [41].)

The partition function (17.3.37), with  $d$  running over the degrees of the Casimir operators of  $G = SU(N), SO(2N), E_N$ , is known to be the vacuum character of the  $W_G$  algebra. The appearance of the  $W_G$  algebra in the superconformal index, and more generally in the chiral subsector of the 6d BPS operators, was asserted in [73] to be closely related to the appearance of the 2d Toda theories in the AGT correspondence [78, 79]. In fact the appearance of  $W_G$  algebra and relation to the AGT relation are further supported recently, by considering the superconformal index with various defect operators [24]. Namely, for the  $A_{N-1}$  theories, insertions of various dimension 2 and/or 4 defect operators to the unrefined index yielded the characters of various degenerate and semi-degenerate representations of  $W_N$  algebra, and

also the characters of the so-called  $W_N^\rho$  representations when the dimension 4 operator is wrapped over the 2d plane where the chiral operators live. This appears to be very concrete supports of the predictions of the AGT correspondence [80] from the 6d index.

Finally, let us explain the prefactor of (17.3.35), which takes the form of  $e^{-\beta(\epsilon_0)_{\text{SUSY}}}$  with

$$(\epsilon_0)_{\text{SUSY}} = -\frac{c_2|G|}{24} \frac{\omega_3}{\omega_1\omega_2} (\omega_1 + \omega_2)^2 - \frac{N\omega_3}{24}. \quad (17.3.40)$$

This formally takes the form of the ‘vacuum energy’ as it is conjugate to the chemical potential  $\beta$  in the index. However, one needs to understand vacuum energies with care. As is obvious already in the free quantum field theory, vacuum energy is the summation of zero point energies of infinitely many harmonic oscillators, which is formally divergent. It is a quantity that has to be carefully defined and computed with regularization/renormalization. Since the regularization and renormalization are constrained by symmetry, it will be simplest to start the discussion with the special case (17.3.17), (17.3.18) of our index. In this case, (17.3.40) simplifies to

$$(\epsilon_0)_{\text{SUSY}} = -\frac{c_2|G|}{6} - \frac{N}{24}. \quad (17.3.41)$$

More general cases will be commented on later.

Since  $\beta$  is conjugate to  $E - R_1$  in (17.3.18), the formal definition of  $(\epsilon_0)_{\text{SUSY}}$  is given by the ‘expectation value’ of the charge  $E - R_1$  for the vacuum on  $S^5 \times \mathbb{R}$ ,

$$\langle E - R_1 \rangle = -\left. \frac{\partial}{\partial \beta} \log Z_{S^5 \times S^1} \right|_{\beta \rightarrow \infty}. \quad (17.3.42)$$

This quantity has to be carefully defined. To concretely illustrate the subtleties, it will be illustrative to consider the free  $(2, 0)$ , consisting of an Abelian tensor multiplet. Then, (17.3.42) is given by the collection of the zero point values of  $E - R_1$  for the free particle oscillators:

$$(\epsilon_0)_{\text{SUSY}} = \text{tr} \left[ (-1)^F \frac{E - R_1}{2} \right] = \sum_{\text{bosonic modes}} \frac{E - R_1}{2} - \sum_{\text{fermionic modes}} \frac{E - R_1}{2}. \quad (17.3.43)$$

The trace is over the infinitely many free particle modes, and  $E, R_1$  appearing in the sum are the values of  $E, R_1$  carried by modes. This is similar to the ordinary Casimir energy defined by

$$\epsilon_0 \equiv \text{tr} \left[ (-1)^F \frac{E}{2} \right] = \sum_{\text{bosonic modes}} \frac{E}{2} - \sum_{\text{fermionic modes}} \frac{E}{2}, \quad (17.3.44)$$

which appears when one computes the partition function of a QFT on  $S^n \times \mathbb{R}$  with inverse-temperature  $\beta$  conjugate to the energy  $E$  [81]. Both expressions are formal, and should be supplemented by a suitable regularization of the infinite sums. As in [81] for the latter quantity, one can use the charges carried by the summed-over states to provide regularizations. The charges that can be used in the regulator are constrained by the symmetries of the problem under considerations, which are different between (17.3.43) and (17.3.44). The

latter is what is normally called the Casimir energy. Let us call  $(\epsilon_0)_{\text{SUSY}}$  the supersymmetric Casimir energy [82].

For (17.3.44), the only charge that one can use to regularize the sum is energy  $E$  [81]. This is because the symmetry of the path integral for the partition function on  $S^n \times S^1$  includes all the internal symmetry of the theory, together with the rotation symmetry on  $S^n$ . Firstly, non-Abelian rotation symmetries forbid nonzero vacuum expectation values of angular momenta on  $S^n$ . Also, there are no sources which will give nonzero values for the internal charges: its expectation value is zero either if the internal symmetry is non-Abelian, or if there are sign flip symmetries of the Abelian internal symmetries. On the other hand, energy  $E$  can be used in the regulator function. The remaining procedure of properly defining (17.3.44) is explained in [81]. One introduces a regulator function  $f(E/\Lambda)$  with a UV cut-off  $\Lambda$  (to be sent back to infinity at the final stage) which satisfies the properties  $f(0) = 1$ ,  $f(\infty) = 0$  and is sufficiently flat at  $E/\Lambda = 0$ :  $f'(0) = 0$ ,  $f''(0) = 0$ , etc. The rigorous definition replacing (17.3.44) is given by

$$\text{tr} \left[ (-1)^F \frac{E}{2} f(E/\Lambda) \right] . \quad (17.3.45)$$

When energy level  $E$  has an integer-spacing,  $E = \frac{m}{R}$  with  $m = 1, 2, 3, \dots$ , and the degeneracy for given  $m$  is a polynomial of  $m$  (as in [81]), one can show that this definition is the same as

$$\text{tr} \left[ (-1)^F \frac{E}{2} e^{-\beta' E} \right] = -\frac{1}{2} \frac{d}{d\beta'} \text{tr} \left[ (-1)^F e^{-\beta' E} \right] , \quad (17.3.46)$$

where small  $\beta'$  is the regulator here. We shall use the latter regulator in our discussions.

On the other hand, the correct regularization of (17.3.43) is constrained by different symmetries. At  $m = \pm \frac{1}{2}$ ,  $a_i = 0$ , the symmetry of the path integral is  $SU(4|2)$  subgroup of  $OSp(8^*|4)$ , containing 16 supercharges. For instance, this is visible on the 5d SYM on  $S^5$  [12], and is also manifest in (17.3.18). This subgroup is defined by elements of  $OSp(8^*|4)$  which commute with  $E - R_1$ . So to respect the  $SU(4|2)$  symmetry, only  $E - R_1$  can be used to regularize the sum (17.3.43). So this sum can be regularized as  $\text{tr} \left[ (-1)^F \frac{E - R_1}{2} f\left(\frac{E - R_1}{\Lambda}\right) \right]$ , or equivalently as

$$\text{tr} \left[ (-1)^F \frac{E - R_1}{2} e^{-\beta'(E - R_1)} \right] = -\frac{1}{2} \frac{d}{d\beta'} \text{tr} \left[ (-1)^F e^{-\beta'(E - R_1)} \right] . \quad (17.3.47)$$

The quantities

$$f_{\text{SUSY}}(\beta') = \text{tr} \left[ (-1)^F e^{-\beta'(E - R_1)} \right] , \quad f(\beta') = \text{tr} \left[ (-1)^F e^{-\beta' E} \right] \quad (17.3.48)$$

are computed in [18, 46] for the free (2, 0) tensor multiplet, given by

$$\begin{aligned} f(x) &= \frac{5x^2(1 - x^2) - 16x^{\frac{5}{2}}(1 - x) + (10x^3 - 15x^4 + 6x^5 - x^6)}{(1 - x)^6} , \\ f_{\text{SUSY}}(x) &= \frac{x}{1 - x} , \end{aligned} \quad (17.3.49)$$

where  $x \equiv e^{-\frac{\beta'}{r}}$  with the  $S^5$  radius  $r$ . From these expressions, one obtains

$$-\frac{1}{2} \frac{d}{d\beta'} f(x) = \frac{5r}{16(\beta')^2} - \frac{25}{384r} + r^{-3} \mathcal{O}(\beta')^2 \quad (17.3.50)$$

and

$$-\frac{1}{2} \frac{d}{d\beta'} f_{\text{SUSY}}(x) = \frac{r}{2(\beta')^2} - \frac{1}{24r} + r^{-3} \mathcal{O}(\beta')^2, \quad (17.3.51)$$

as  $\beta' \rightarrow 0$ . As explained in [81], the first term  $\frac{5r}{16(\beta')^2} \sim \frac{5}{16} r \Lambda^2$  of (17.3.50) should be canceled by a counterterm. This is because the vacuum value of  $E$  has to be zero in the flat space limit  $r \rightarrow \infty$  from the conformal symmetry. A counterterm of the form  $\Lambda^2 \int_{S^5 \times S^1} d^6 x \sqrt{g} R^2$  or  $(\beta')^{-2} \int_{S^5 \times S^1} d^6 x \sqrt{g} R^2$  can cancel this divergence. Similarly, the first term of (17.3.51) has to be canceled by a counterterm of the same form. This is because the vacuum value of  $E - R_1$  has to vanish in the flat space limit, required by the superconformal symmetry. After these subtractions and removing the regulator  $\beta' \rightarrow 0$ , one obtains

$$\epsilon_0 = -\frac{25}{384r}, \quad (\epsilon_0)_{\text{SUSY}} = -\frac{1}{24r}. \quad (17.3.52)$$

So although conceptually closely related, the two quantities are different observables. At least with the Abelian example above, we hope that we clearly illustrated the difference.

Considering that our  $S^5$  partition function is constrained by  $SU(4|2)$  SUSY in the path integral, it is very natural to expect that  $(\epsilon_0)_{\text{SUSY}}$  of (17.3.41) is the supersymmetric Casimir energy. Note also that,  $(\epsilon_0)_{\text{SUSY}} = -\frac{1}{24r}$  computed above for the free 6d theory agrees with the zero point energy (17.3.41) computed from the  $S^5$  partition function at  $N = 1$ , which concretely supports this natural expectation. (Note that  $c_2|G| \equiv f^{abc} f^{abc} = 0$  for Abelian gauge group, and also that we absorbed the factor  $\frac{1}{r}$  into  $\beta$ .) Even in the non-Abelian case, we think that (17.3.41) should be the supersymmetric Casimir energy  $(\epsilon_0)_{\text{SUSY}}$ , and not  $\epsilon_0$ .

The more conventional Casimir energy  $\epsilon_0$  in the large  $N$  limit has been computed in the  $AdS_7 \times S^4$  gravity dual in the literature. The result is given by [13, 83]

$$\epsilon_0 = -\frac{5N^3}{24r}, \quad (17.3.53)$$

while from the 5d maximal SYM with  $U(N)$  gauge group, we obtain from (17.3.41)

$$(\epsilon_0)_{\text{SYM}} = -\frac{N(N^2 - 1)}{6r} \xrightarrow{N \rightarrow \infty} -\frac{N^3}{6r}. \quad (17.3.54)$$

From the interpretation in our previous paragraph, we think it is likely that the disagreement of the two quantities is simply due to the fact that the gravity dual and the 5d SYM computed different observables.<sup>7</sup> Assuming our interpretation, it will be interesting to study what kind of computation should be done in the gravity side to reproduce  $(\epsilon_0)_{\text{SUSY}}$ . We think the key is

<sup>7</sup>See, however, the reference [17] for discussions on different possibilities of interpreting these results.

to keep SUSY manifest in the holographic renormalization computations, as this was what yielded two different Abelian observables (17.3.52).

We also mention in passing that one can define a ‘supersymmetric version’ of Renyi entropy [84] in SUSY QFTs. This supersymmetric version can be computed more easily in SUSY QFTs, similar to the supersymmetric version of the Casimir energy that we explained here. We expect that there should be many supersymmetric observables of this sort.

Finally, let us consider (17.3.40) at more general points in the chemical potential space. For instance, if one tries to repeat the computation of Casimir energies from the free QFT consideration, clearly we have less symmetries which constrain the regulator in the oscillator sum. So it might be that the quantity could depend on the regularization scheme, and the localization computation might have made an implicit assumption on it to get the result (17.3.40). Since the maximal SUSY point (17.3.17) appears to remove all such possible ambiguities, we expect that any implicit assumptions that could have been made in the path integral will not spoil (17.3.41). On the other hand, even after turning on many chemical potentials, observables like ‘Casimir force’ that can be derived from the Casimir energy should be physical. So one should be able to define both versions of Casimir energies  $\epsilon_0$ ,  $(\epsilon_0)_{\text{SUSY}}$  at most general values of chemical potentials. It is not clear to us whether our computation captures such a physical quantity at general value of chemical potential at all.

### 17.3.3 The partition function on $\mathbb{CP}^2 \times S^1$

In this subsection, we discuss another expression of the superconformal index of the (2, 0) theory of the same schematic form (17.1.1), which this time takes a manifest index form. Following [18], let us explain this index for the  $U(N)$  gauge group only. The index takes the following form:

$$\begin{aligned}
Z_{S^5 \times S^1}(\beta, m, a_i) &= \frac{1}{N!} \sum_{s_1, \dots, s_N = -\infty}^{\infty} \oint \prod_{I=1}^N d\lambda_I e^{-S_0(\lambda, s, \beta)} Z_{\mathbb{R}^4 \times T^2} \left( \frac{i\beta\omega_1}{2\pi}, i\lambda - s\beta a_1, \omega_{21}, \omega_{31}, m - \frac{\omega_1}{2} \right) \\
&\quad \cdot Z_{\mathbb{R}^4 \times T^2} \left( \frac{i\beta\omega_2}{2\pi}, i\lambda - s\beta a_2, \omega_{32}, \omega_{12}, m - \frac{\omega_2}{2} \right) \cdot Z_{\mathbb{R}^4 \times T^2} \left( \frac{i\beta\omega_2}{2\pi}, i\lambda - s\beta a_2, \omega_{32}, \omega_{12}, m - \frac{\omega_2}{2} \right), \\
S_0(\lambda, \beta) &= \beta \sum_{I=1}^N \left( -\frac{s_I^2}{2} + i s_I \lambda_I \right), \tag{17.3.55}
\end{aligned}$$

where again the index  $Z_{\mathbb{R}^4 \times T^2}(\tau, v, \beta, \epsilon_{1,2}, m_0)$  is used as building blocks, and we use the notation  $\omega_i = 1 + a_i$ ,  $\omega_{ij} = \omega_i - \omega_j$ . The ‘Coulomb VEV’ parameter  $\lambda$  is taken to be  $\lambda_I \equiv \lambda'_I - i s \beta \zeta$  with any positive  $\zeta$ , where  $\lambda'_I$  are variables whose integration contours are almost at the real axis in the range  $0 \leq \lambda'_I \leq 2\pi$ . The precise integration contour will be explained below, which goes around the poles in a specific manner.  $\zeta$  appeared in [18] as a freedom to choose the path integral contour for some fields, and can be any number as long as it is positive. (The index will not depend on its value. In [18], it was parametrized by  $\zeta = \frac{4}{\xi-1}$  with  $\xi > 0$ .)

The contour for  $\lambda'_I$  was heuristically motivated in [18], and was checked to yield reasonable results, but it is not rigorously derived so far. The contour prescription is obtained as follows.

We first take all  $a_i$  parameters and  $m - \frac{1}{2}$  to be imaginary, in which case there will be many poles in the  $Z_{\mathbb{R}^4 \times T^2}$  factors at the line  $\text{Im}(\lambda_I) = 0$ . When one considers an integral with all  $s_I \neq s_J$ , the integral contour is taken to be along real  $\lambda'_I$  line between  $1 \leq \lambda'_I \leq 2\pi$ , which does not hit any poles. When some  $s_I$ 's are equal, then the above real axis contour will hit some poles on the real axis. In such a case, we slightly deform the contour, or equivalently the poles away from the real axis, as follows. In each  $Z_{\mathbb{R}^4 \times T^2}$  factor, the effective Omega parameters  $\epsilon_1, \epsilon_2$  are taken to be imaginary. The pole or contour deformation is obtained by giving infinitesimal real shifts to these imaginary parameters as

$$\epsilon_1 + \varepsilon, \quad \epsilon_2 + \varepsilon, \quad (17.3.56)$$

with  $0 < \varepsilon \ll 1$ . This effectively deforms the contour to go around the poles in a specific way. Although with some motivations about this rule presented in [18], we should stress that this is just a working prescription at the moment of writing this review.

This formula was derived from a 5d SYM on  $\mathbb{CP}^2 \times \mathbb{R}$ , which was obtained by first considering 6d (2,0) theory on a supersymmetric  $S^5/\mathbb{Z}_K \times \mathbb{R}$  orbifold [14, 18]. The orbifold acts as follows. Considering the round  $S^5$  as a Hopf fibration over  $\mathbb{CP}^2$ , its metric is given by

$$ds^2(S^5) = r^2 \left[ ds^2(\mathbb{CP}^2) + (dy + V)^2 \right], \quad (17.3.57)$$

where  $y \sim y + 2\pi$  and  $V$  is related to the Kahler 2-form  $J$  of  $\mathbb{CP}^2$  by  $J = \frac{1}{2}dV$ .  $S^5/\mathbb{Z}_K$  is obtained by modding out the fiber direction by

$$y \sim y + \frac{2\pi}{K}. \quad (17.3.58)$$

Our strategy is to first consider the regime with large  $K$ , and obtain a 5d Yang-Mills theory on  $\mathbb{CP}^2 \times \mathbb{R}$  whose gauge coupling is proportional to  $\frac{1}{K}$ . The coupling will be small for large  $K$ , or in the energy scale  $\frac{1}{r} \sim E \ll \frac{K}{r}$ . Of course our eventual interest is the case with  $K = 1$ , in which case the 5d SYM is strongly coupled at all energy scale  $E \gtrsim \frac{1}{r}$ . The expression (17.3.55) is obtained by studying this 5d Yang-Mills theory on  $\mathbb{CP}^2 \times \mathbb{R}$  at strong coupling.

We would like to consider supersymmetric orbifold, as this would yield 5d supersymmetric Yang-Mills theory which admits some exact computations. However, the above action leaves none of the (2,0) Killing spinors invariant [14]. To make a supersymmetric  $\mathbb{Z}_K$  orbifold, one can make a simultaneous rotation on the spatial angle (17.3.58) in  $SO(6)$ , and also on the internal  $SO(5)$  R-symmetry. In [18], an infinite family of rotations by  $\frac{2\pi}{K}$  angle was considered with the rotation generator

$$j_1 + j_2 + j_3 + \frac{3}{2}(R_1 + R_2) + n(R_1 - R_2), \quad (17.3.59)$$

where the  $\frac{2\pi}{K}$  rotation with  $j_1 + j_2 + j_3$  generates (17.3.58). To make the  $2\pi$  rotation with this charge to be an identity, we should take  $n$  to be half an odd integer. By construction of the charge (17.3.59), this  $\mathbb{Z}_K$  commutes with a pair of supercharges  $Q = Q_{---}$  and  $S = S_{+++}$  that we used to define the superconformal index. At  $K \neq 1$ , various 5d SYMs labeled by

different  $n$  will describe inequivalent systems, as  $\mathbb{Z}_K$  orbifolds are all different. At the strong coupling point  $K = 1$ , there is no orbifolding, so different 5d SYMs on  $\mathbb{CP}^2 \times \mathbb{R}$  are expected to be all equivalent at the quantum level. In particular, we expect SUSY enhancement to  $OSp(8^*|4)$ .

At  $K = 1$ , the index (17.3.2) is computed from 5d SYM on  $\mathbb{CP}^2 \times S^1$ , with suitable twisted boundary conditions of fields on  $S^1$  by the chemical potentials [14, 18]. Although we expect that all SYMs labeled by  $n$  would yield equivalent results, 5d SYMs are very different at different values of  $n$ . The formula (17.3.55) is obtained from the SYM associated with  $n = -\frac{1}{2}$ , which has a virtue of showing 8 supercharges explicitly in the 5d SYM action, including  $Q, S$  above. The QFT at  $n = -\frac{3}{2}$  was first discovered in [14], and the perturbative index (without including instantons) of this QFT at large  $K$  was also computed.

The action and SUSY transformation of fields are explained in [18], which we shall not repeat here. The derivation of the index (17.3.55) goes in a similar way as that of the index (17.3.3) from the  $S^5$  partition function, which can be found in [18]. (Just like on  $S^5$ , the ‘derivation’ again assumes some localized nature of the instanton saddle point configurations.) Here we would just like to stress a few qualitative differences in the formula (17.3.55), compared to (17.3.3).

Firstly, the complex structure parameter  $\tau_i = \frac{i\beta\omega_i}{2\pi}$  in each  $Z_{\mathbb{R}^4 \times T^2}$  provides the factor  $e^{2\pi i\tau_i k_i} = e^{-\beta\omega_i k_i}$  in the  $k_i$  instanton coefficients. So the expression (17.3.55) manifestly takes the form of an index at  $\beta \gg 1$ . This should be clear since the 5d SYM is put on  $\mathbb{CP}^2 \times S^1$ , explicitly having a time direction, with  $\beta$  being the circumference length of the circle. This is in contrast to the  $S^5$  partition function, where the time direction had to ‘emerge’ at strong coupling  $\beta \gg 1$ .

Secondly, apart from the three instanton summations in  $Z_{\mathbb{R}^4 \times T^2}$  factors, the expression (17.3.55) has extra summations over integers  $s_1, \dots, s_N$ . This originates from a more complicated saddle point structure of the path integral. To explain it, let us first fix our orientation convention on  $\mathbb{CP}^2$ . We can decompose 2-forms  $\mathbb{CP}^2$  to self-dual and anti-self-dual 2-forms. Our convention is such that the Kahler 2-form  $J$  is in the anti-self-dual part. Then, the saddle point first admits singular self-dual instantons, localized at the fixed points of the  $U(1)^2$  rotations generated by  $j_1 - j_2, j_2 - j_3$ . The summation over these instanton numbers generate the series expansion with  $e^{2\pi i\tau_i k_i}$  in the three  $Z_{\mathbb{R}^4 \times T^2}$  factors. With nonzero  $\lambda$  which breaks  $U(N)$  to  $U(1)^N$ , these self-dual instantons are all  $U(1)^N$  instantons, just like the instantons appearing in the Nekrasov partition functions. On top of these, it turns out that one could also have anti-self-dual field configurations  $F^- = \frac{2s}{r^2}J$ , where  $s = \text{diag}(s_1, \dots, s_N)$  with integer eigenvalues. The  $-\beta \sum_I \frac{s_I^2}{2}$  term in  $S_0$  is the contribution of these anti-self-dual instantons to the energy  $E$  in (17.3.2). These extra anti-self-dual instantons play very nontrivial roles in making (17.3.2) to work.

One might worry that, summation over all the integers  $s_I$  with unbound negative energy weight  $e^{\beta \sum_I \frac{s_I^2}{2}}$  will make the expression (17.3.55) divergent. However, the  $\lambda$  integration contour explained above will project this infinite sum over  $s_I$  into a finite sum. The state which contributes with the most negative energy will be the vacuum. (Here, by ‘energy’ we mean  $E - \frac{R_1 + R_2}{2}$ .)

In [18], the expression (17.3.55) was used to study various aspects of the (2, 0) theory. Here we shall explain two studies made there. Firstly, we shall explain how the unrefined index of section 2.2 appears from this approach, as this will illustrate how the formula (17.3.55) works in the simplest setting. Secondly, we shall explain the systematic series expansion of the expression (17.3.55) in terms of fugacities at some finite  $N (> 1)$ , keeping all independent chemical potentials generic. This should probably be the strongest virtue of the expression (17.3.55).

We first consider the unrefined index at  $m = \frac{1}{2} - a_3$ . From the expressions of  $\epsilon_1, \epsilon_2, m_0$  appearing in the three factors of the expression (17.3.55), one can show that they satisfy  $m = \epsilon_-$  in the first factor,  $m = -\epsilon_-$  in the second factor, and  $m = \epsilon_+$  in the third factor. So the simplification pattern of the integrand is similar to the  $S^5$  partition function. Thus, one obtains [18]

$$\frac{1}{\eta\left(\frac{i\beta\omega_3}{2\pi}\right)^N} \cdot \frac{1}{N!} \oint [d\lambda_I] \sum_{s_1, \dots, s_N = -\infty}^{\infty} e^{\frac{\beta}{2} \sum_I s_I^2 - i \sum_I s_I \lambda_I} \prod_{I < J} 2 \sinh \frac{i\lambda_{IJ} - \beta s_{IJ} a_1}{2} \cdot 2 \sinh \frac{i\lambda_{IJ} - \beta s_{IJ} a_2}{2}, \quad (17.3.60)$$

where the first factor  $\eta\left(\frac{i\beta}{2\pi}\right)^{-N}$  comes from  $Z_{\text{inst}}$  from the third factor of the expression (17.3.55) at  $m = \epsilon_+$ .<sup>8</sup> The integrand is so much simplified that there are no poles of  $\lambda'_I$  on their real axes. Thus, the contour integral can be taken along the real axes of  $\lambda'_I$ , or along the  $\text{Im}\lambda_I = -s_I\beta\zeta$  line. Consider the complex variable  $z_I = e^{-i\lambda_I}$ . Since the only pole of the integrand appears at  $z_I = 0$ , one can continuously deform the integration contour to the unit circles  $|z_I| = 1$  (namely  $\text{Im}\lambda_I = 0$ ). The integral (17.3.60) can be done easily [18], which yields

$$e^{\beta\omega_3 \frac{N(N^2-1)}{6}} \eta\left(\frac{i\beta\omega_3}{2\pi}\right)^{-N} \prod_{n=1}^{N-1} (1 - e^{-n\beta\omega_3})^{N-n} = e^{\beta\omega_3 \left(\frac{N(N^2-1)}{6} + \frac{N}{24}\right)} \prod_{s=0}^{\infty} \prod_{d=1}^N \frac{1}{1 - e^{-\beta\omega_3(d+s)}}. \quad (17.3.61)$$

The spectrum part of this index is exactly the same as (17.3.37), with  $d = 1, \dots, N$  for  $U(N)$  Casimir operators.

We next consider the vacuum energy factor. First of all, we go back to the integral expression (17.3.60) and trace where the vacuum is coming from, among the various saddle points of the 5d SYM. The vacuum comes from the configuration in which  $e^{\frac{\beta}{2} \sum_I s_I^2}$  factor in (17.3.60) is the largest. Apparently, taking all  $s_I$ 's to be arbitrary large, it might look that one can make this factor as large as possible. If this were the case, then the index (17.3.55) would not have made sense. But from the structure of the contour integral (17.3.60), one cannot make  $s_I$  to be arbitrary large. This is due to the term  $e^{-i \sum_I s_I \lambda_I}$ , which is part of the classical action. Physically, this term comes from a term of the form [14]

$$\int J \wedge \text{tr} \left( A \wedge dA - \frac{2i}{3} A^3 \right) \quad (17.3.62)$$

in the action on  $\mathbb{C}\mathbb{P}^2 \times S^1$  [14, 18]. Namely, a magnetic flux  $F \sim J$  induces an electric charge via the Kahler-Chern-Simons term (17.3.62). This induces a phase  $e^{-i \sum_I s_I \lambda_I}$  in (17.3.60).

<sup>8</sup>We have included the zero point energy factors of these instanton particles, to obtain  $\eta^{-N}$ .

So for the contour integral to be nonzero, the rest of the measure in (17.3.60) should provide a phase which can cancel  $e^{-i \sum_I s_I \lambda_I}$ . Since the measure consists of a product of  $N^2 - N$  sine functions, there are only finitely many values of  $s_1, \dots, s_N$  for which the integral is nonzero. It turns out that the maximal value of  $e^{\frac{\beta}{2} \sum_I s_I^2}$  is obtained at

$$(s_1, \dots, s_N) = (N - 1, N - 3, \dots, -(N - 3), -(N - 1)) , \quad (17.3.63)$$

or any other configurations obtained by permuting the above  $s_I$  fluxes. Summing over  $N!$  such fluxes, one obtains the following contribution

$$\frac{1}{N!} \cdot N! e^{\frac{\beta}{2}((N-1)^2 + (N-3)^2 + \dots + (-N+1)^2)} = e^{\beta \frac{N(N^2-1)}{6}} . \quad (17.3.64)$$

Collecting the other factors coming from the sine functions, one finds extra  $e^{\frac{a_3 \beta N(N^2-1)}{6}}$ , and by expanding the instanton correction  $\eta(\frac{i\beta}{2\pi})^{-N}$ , one obtains  $e^{\frac{N\beta\omega_3}{24}}$  at lowest energy. So combining all, one finds  $1 \cdot \exp\left[\beta\omega_3\left(\frac{N(N^2-1)}{6} + \frac{N}{24}\right)\right]$ . This illustrates that, from the viewpoint of SYM on  $\mathbb{CP}^2 \times \mathbb{R}$ , the 6d CFT vacuum and its energy  $\sim N^3$  appear in a highly nontrivial manner, by ‘exciting’ many non-perturbative anti-self-dual instantons. It should be very interesting to understand this vacuum structure more directly.

We find that the vacuum energy

$$(\epsilon_0)_{\text{SUSY}} = -\omega_3 \left( \frac{N(N^2 - 1)}{6} + \frac{N}{24} \right) \quad (17.3.65)$$

is *not* the same as (17.3.40) computed from the  $S^5$  partition function in general. This is not surprising because, as we explained in the previous subsection, we have not too strong symmetry in general which could constrain the regularization/renormalization of the path integral, so the two SYM computations on  $S^5$  and  $\mathbb{CP}^2 \times S^1$  could have implicitly chosen inequivalent regularization schemes. It is not clear to us at the moment if any of the two is physically meaningful. However, when  $m = \frac{1}{2}$  and  $a_i = 0$ , recall that we have maximal SUSY  $SU(4|2)$  which we expect to constrain the regularization completely. Indeed, at this point ( $\omega_i = 1$ ), the two results (17.3.40) and (17.3.65) agrees with each other, supporting our expectation.

The final subject of this subsection is the general index with all four chemical potentials turned on. The full expression (17.3.55) is too complicated for us to handle exactly, but now we can systematically make a low energy fugacity expansion. This has been done in [18] for various values of  $N$  until a few low orders in  $e^{-\beta}$ .

Let us define  $q \equiv e^{-\beta}$ ,  $y \equiv e^{\beta(m-\frac{1}{2})}$ ,  $y_i \equiv e^{-\beta a_i}$  (satisfying  $y_1 y_2 y_3 = 1$ ). We shall be expanding the index by assuming  $q \ll 1$ , keeping  $y, y_i$  to be of order 1. Firstly, for general  $N$ , the expression (17.3.55) was computed up to  $\mathcal{O}(q^2)$ . The result apart from the zero point energy factor is

$$Z_{S^5 \times S^1} = 1 + qy + q^2 \left[ 2y^2 + y(y_1 + y_2 + y_3) - (y_1^{-1} + y_2^{-1} + y_3^{-1}) + y^{-1} \right] + \mathcal{O}(q^3) \quad (17.3.66)$$

for  $N \geq 2$ . (The exact index at  $N = 1$  was worked out in [18] separately.) The result is independent of  $N$  for  $N \geq 2$ . In fact, empirically in all studies done in [18], the index will turn out to be independent of  $N$  at  $q^k$  order if  $k \leq N$ . This is a natural thing to expect for a CFT with large  $N$  gravity dual. This is because  $E \ll N$  is the regime in which supergravity approximation of the string/M-theory is valid, and the gravity spectrum is independent of  $N$ . Of course, the  $N$  independence of the spectrum up to the threshold  $E = N$  is too much to expect, but it often happens at least in the BPS sector that  $E \sim N$  is the threshold beyond which the ‘stringy exclusion’ behaviors [85] start to appear. The  $N$  independent index (17.3.66) completely agrees with the large  $N$  supergravity index on  $AdS_7 \times S^4$ , which is a consistency check of the expression (17.3.55).

As explained in [18], the analysis at higher orders in  $q$  becomes quickly complicated, due to the appearance of many instanton saddle points contributing to the formula (17.3.55). The studies are made for  $N = 2, 3$  till  $q^3$  order in [18]. After adding many contributions from various saddle points, each of them acquiring contributions from many residues in the contour integral, the  $q^3$  order corrections to (17.3.66) for  $N = 2, 3$  are given by

$$U(2) : q^3 \left[ 2y^3 + 2y^2(y_1 + y_2 + y_3) + y \left( y_1^2 + y_2^2 + y_3^2 - \frac{1}{y_1} - \frac{1}{y_2} - \frac{1}{y_3} \right) - \left( \frac{y_1}{y_2} + \frac{y_2}{y_1} + \frac{y_2}{y_3} + \frac{y_3}{y_2} + \frac{y_3}{y_1} + \frac{y_1}{y_3} \right) + y^{-1}(y_1 + y_2 + y_3) \right] \quad (17.3.67)$$

$$U(3) : q^3 \left[ 3y^3 + 2y^2(y_1 + y_2 + y_3) + y \left( y_1^2 + y_2^2 + y_3^2 - \frac{1}{y_1} - \frac{1}{y_2} - \frac{1}{y_3} \right) - \left( \frac{y_1}{y_2} + \frac{y_2}{y_1} + \frac{y_2}{y_3} + \frac{y_3}{y_2} + \frac{y_3}{y_1} + \frac{y_1}{y_3} \right) + y^{-1}(y_1 + y_2 + y_3) \right] \quad (17.3.68)$$

The  $U(3)$  result (17.3.68) completely agrees with the large  $N$  supergravity index on  $AdS_7 \times S^4$ , presumably because  $k = N$  is the threshold until which the BPS spectrum is independent of  $N$ . For  $U(2)$ , we see from (17.3.67) that one state is missing compared to the large  $N$  index, i.e.  $2y^3$  vs.  $3y^3$  in the first terms. It will be interesting to study the  $U(2)$  index at very high order in  $q$ , and investigate a truly unexplored sector of the 6d (2, 0) theory beyond supergravity.

## 17.4 Discussions

In this review, we explained the recent progress on the 6d SCFT partition functions in the Coulomb and the symmetric phases, focusing on the Coulomb branch indices in the Omega background and the superconformal index on  $S^5 \times S^1$ . The two observables are closely related, and we explained their relations and the physics contained in these indices with the example of (2, 0) theory. In this section, we discuss some open problems, and some recent progress on this subject that we could not properly review in this work.

As we tried to emphasize in section 2, the computation of the indices in the Coulomb phase does not really rely on the 5d SYM description. We can rather understand it as a direct

string theory computation, in the very background which is used to engineer the 6d SCFT itself. The references [41, 42] discuss more subtle  $(1, 0)$  theories in the Coulomb phase in a similar manner, such as those living on the M5-M9-brane system. [41] also explain how one can extract out the 6d Coulomb branch partition functions from string theory computations. So we claim that the expressions like (17.3.3) and (17.3.55) for the 6d superconformal indices should be using such ‘intrinsic’ partition functions on  $\mathbb{R}^4 \times T^2$ , which are defined and computed without referring to the 5d SYM. However, it seems (at least so far) that we have no way to even motivate the curved space partition functions results like (17.3.3) and (17.3.55), set aside derivations, without using the the 5d SYM descriptions. Of course one can hope these formulae to be true even when small circle reductions of the 6d CFT does not flow to weakly coupled 5d SYM, as all the ingredients appearing in these formulae can be addressed without referring to 5d SYM. This makes us suspect that there should be a more abstract way of understanding these formulae, perhaps directly using string theory. However, we do not know if we can realize  $S^5 \times \mathbb{R}$  background and put 6d CFT there directly in the string theory setting.

We have presented two different expressions (17.3.3) and (17.3.55) for the superconformal indices for a given theory, and found the same physics in various sectors of the  $(2, 0)$  theory when we could make concrete studies of them. Of course more basic question is whether the two partition functions are identically the same, perhaps modulo the Casimir energy factors which might be ambiguous in general. Answering this question would have to do with making a strong-coupling re-expansion of the ingredients  $Z_{\mathbb{R}^4 \times T^2}$  in (17.3.3).

Related to the last question, and also for applying our findings to more general  $(1, 0)$  SCFTs, it would be very important to understand the modular properties of the partition functions (17.2.4) and (17.2.5) better. Knowing its modular property under  $\tau \rightarrow -\frac{1}{\tau}$  means that we can make a strong coupling expansion of (17.3.3). At this point, we should emphasize the studies of the elliptic genus which appears as the coefficients of (17.2.4) for various self-dual strings. Namely, assuming large Coulomb VEV  $v$ ,  $Z_{n_I}(\tau, \epsilon_{1,2}, m)$  were computed from various 2d gauge theories living on the self-dual strings. It has been first studied for the  $A_{N-1}$  type  $(2, 0)$  strings in [38, 39], which are called M-strings. More interesting  $(1, 0)$  self-dual strings have been studied this way. For instance, the  $(1, 0)$  strings for M2-branes suspended between M5-M9 branes are called E-strings, whose elliptic genera were systematically computed from 2d QFT [42]. Some other strings for  $(1, 0)$  theory engineered by F-theory were studied recently in [45]. With these elliptic genera known, it will be in principle possible to trace how to make a strong coupling re-expansion of the integrand of (17.3.3), and address the index for a variety of  $(1, 0)$  CFTs.<sup>9</sup>

Even if one forgets about the application to the symmetric phase observables, computing the elliptic genera of various  $(1, 0)$  self-dual strings would be very valuable by itself. And this is quite challenging in general, as engineering a weakly coupled 2d gauge theory on the worldsheet is not always easy. For instance, the task becomes relatively easier if the self-dual

---

<sup>9</sup>Note that the studies of this paper either used special properties of the Abelian theory, or relied on SUSY enhancement which are not available for  $(1, 0)$  theories. Also, the  $\mathbb{CP}^2 \times S^1$  index might have used too many ingredients of the  $(2, 0)$  theory, so it is not clear whether the strategy will go through well for all  $(1, 0)$  CFTs.

strings can be engineered using D-branes subject to various boundary conditions [38,39,42,45]. However, many interesting 6d CFTs are engineered from F-theory, which involves exotic 7-branes. It will be interesting to see how much we can learn about them from 2d gauge theories.

Finally, it should be interesting to explore the 6d CFT partition functions on other curved manifolds, presumably using various 5d SYM approaches. In this paper we tried not to mention 5d SYM description when unnecessary, e.g. in section 2, for the sake of consistency and also for logical clarity. But of course 5d SYM provides extremely useful viewpoint to study this system. In the very limited class of SUSY observables that we studied, the only subtlety of 5d SYM that we could find was the small instanton issue. So we would very much like to know how much 5d SYM can be teaching us about higher dimensional CFTs [86].

## Acknowledgements

We would like to thank Chiung Hwang, Hee-Cheol Kim, Joonho Kim, Sung-Soo Kim, Eunkyung Koh, Sungjay Lee, Jaemo Park, Cumrun Vafa for their collaborations with the authors, on the materials covered in this paper. We would also like to thank Dario Martelli, Shiraz Minwalla and especially Hee-Cheol Kim for helpful discussions on the related subjects while we were writing this review. We also like to thank Yuji Tachikawa for careful reading of this manuscript and many useful comments. This work is supported in part by the National Research Foundation of Korea (NRF) Grant No. 2012R1A1A2042474 (SK), 2012R1A2A2A02046739 (SK), 2015R1A2A2A01003124 (SK), 2006-0093850 (KL).

## 17.5 Appendix. Off-shell supergravity analysis on $S^5$

By making the KK reduction from  $S^5 \times S^1$  with twists by  $a_i$ , our background fields are given by

$$C = i\alpha^2 a_i n_i^2 d\phi_i, \quad \alpha^2 = \frac{1}{1 - a_i^2 n_i^2}. \quad (17.5.1)$$

The field  $C$  is imaginary. By comparing the gravitino SUSY condition of [70] and the 5d reduction of the Killing spinor equation for the two spinors on our background, one finds that  $v_{\mu\nu} = -\frac{i}{4\alpha}(dC)_{\mu\nu}$  for the antisymmetric field in the Weyl multiplet,  $b_\mu = 0$  for the dilatation gauge field, and  $V_\mu = -C_\mu \frac{\sigma_3}{2}$  for the  $SU(2)_R$  gauge field. The Killing spinor equation is

$$D_a \epsilon = \left[ \frac{i}{8\alpha} \gamma_{abc} (dC)^{bc} + i\gamma_a \left( -\alpha \frac{\sigma_3}{2} - \frac{1}{4\alpha} \gamma_{bc} V^{bc} + \frac{i}{2\alpha} \gamma^b \nabla_b \alpha \right) \right] \epsilon, \quad (17.5.2)$$

where  $D_a \epsilon = \left( \nabla_a + C_a \frac{\sigma_3}{2} \right) \epsilon$ .  $a, b, c, \dots$  are frame indices. The conjugate spinor  $\epsilon^\dagger$  is literally taken to be the Hermitian conjugate in our Euclidean theory, so it satisfies

$$D_a \epsilon^\dagger = \epsilon^\dagger \left[ -\frac{i}{8\alpha} \gamma_{abc} V^{bc} - i \left( -\alpha \frac{\sigma_3}{2} - \frac{1}{4\alpha} \gamma_{bc} V^{bc} - \frac{i}{2\alpha} \gamma^b \nabla_b \alpha \right) \gamma_a \right], \quad (17.5.3)$$

where  $D_a \epsilon^\dagger = \nabla_a \epsilon^\dagger - \epsilon^\dagger C_a \frac{\sigma_3}{2}$ . The imaginary nature of  $C, V$  is all taken into account. Below we shall study some bosonic equations which are derived from the above Killing spinor

equation, from which we determine various geometric quantities. As we are physically quite confident from 6d arguments that (17.3.4) should be a SUSY background, we shall only study a subset of the bosonic equations to determine the fields, rather than completely solving them.

We study the differential conditions satisfied by the spinor bilinears. One first obtains

$$\nabla_a (\alpha \epsilon^\dagger \epsilon) = -i\xi^b (dC)_{ab} . \quad (17.5.4)$$

where  $\xi^a \equiv \epsilon^\dagger \gamma^a \epsilon$ . One similarly obtains the following condition for the vector bilinear:

$$\nabla_b \xi_a = -\frac{i}{4\alpha} (\epsilon^\dagger \gamma_{abcd} \epsilon) (dC)^{cd} + i\alpha (\epsilon^\dagger \sigma_3 \gamma_{ab} \epsilon) + \frac{i}{\alpha} (\epsilon^\dagger \epsilon) (dC)_{ab} - \frac{2}{\alpha} \xi_{[a} \nabla_{b]} \alpha - \frac{1}{\alpha} \delta_{ab} \xi^c \nabla_c \alpha . \quad (17.5.5)$$

Note that all but the last term is antisymmetric in  $a, b$ . So one obtains

$$\nabla_a \xi_b + \nabla_b \xi_a = -2g_{ab} \frac{\xi \cdot \nabla \alpha}{\alpha} \quad (17.5.6)$$

and

$$d\xi = \frac{i}{4\alpha} \star (V \wedge \xi) - \frac{i}{\alpha} f V + \frac{2}{\alpha} \xi \wedge d\alpha + 2\alpha X^3 , \quad (17.5.7)$$

where  $f = \epsilon^\dagger \epsilon$ ,  $V_{\mu\nu} \equiv (dC)_{\mu\nu}$ ,  $X^3_{\mu\nu} = -\frac{i}{2} \epsilon^\dagger \sigma^3 \gamma_{\mu\nu} \epsilon$ . We shall need the expression for  $X^3$  from (17.5.7) later. There are more differential conditions for the tensor bilinears. We will not need to consider them. We also study the algebraic conditions satisfied by the bilinears. In our Euclidean theory, the algebraic conditions become

$$\xi^\mu \xi_\mu = f^2 , \quad i_\xi X^3 = 0 , \quad i_\xi \star X^3 = -f X^3 , \quad 4(X^3 \cdot X^3)_{\mu\nu} = -f^2 g_{\mu\nu} + \xi_\mu \xi_\nu \quad (17.5.8)$$

etc. We shall not consider other 2-form bilinears  $X^1, X^2$  in this paper.

A possible guess for  $\xi = \xi^\mu \partial_\mu$  is the following. A highly well-motivated conjecture for  $\xi$  is that it should generate the bosonic symmetry for  $\mathcal{Q}^2$  algebra, where  $\mathcal{Q} = Q + S$  is the supercharge associated with our index. So we try

$$\xi = \sum_{i=1}^3 \omega_i \partial_{\phi_i} . \quad (17.5.9)$$

Firstly, this trivially solves (17.5.6), since  $\xi$  is a Killing vector which leaves  $\alpha$  invariant. Then we plug this  $\xi$  into the right hand side of (17.5.4). Here we can nontrivially test our educated guess (17.5.9), since  $-i\xi^b (dC)_{ab}$  is integrable with the above  $\xi$ . The solution to (17.5.4) with  $f = \epsilon^\dagger \epsilon$  is

$$f = \frac{1 + a_i n_i^2}{\sqrt{1 - a_i^2 n_i^2}} . \quad (17.5.10)$$

One can check that this result is also compatible with the algebraic conditions (17.5.8).

The only background fields of [70] that we have not determined yet are D in the Weyl multiplet, and the background vector multiplet fields. D can be determined in the above

background by studying the Weyl multiplet gaugino SUSY variation. Contracting the SUSY condition with  $\epsilon^\dagger$ , one obtains

$$fD = \frac{i}{2\alpha}\xi_a \left( \nabla_b V^{ba} - \frac{i}{4\alpha}\epsilon^{abcde}V_{bc}V_{de} + \frac{\nabla_b\alpha}{\alpha}V^{ba} \right) - 2iX_{ab}^3V^{ab} - \frac{f}{2\alpha^2}V^{ab}V_{ab} . \quad (17.5.11)$$

Inserting (17.5.7) for  $X^3$ , and plugging in  $g_{\mu\nu}$ ,  $V = dC$ ,  $\alpha$  of (17.3.4),  $\xi$  of (17.5.9),  $f$  of (17.5.10), one finds a big simplification, after which D is simply given by

$$D = 2(a_1^2 + a_2^2 + a_3^2)\alpha^2 . \quad (17.5.12)$$

We also need to determine the background vector field of various sorts. There are various flavor background gauge fields, coupling to the hypermultiplet, and also one auxiliary vector multiplet whose scalar VEV should provide the Yang-Mills coupling. In the notation of [70], SUSY condition for gauge multiplet gaugino is given by

$$\begin{aligned} \delta\chi^A &= \frac{i}{2}F_{\mu\nu}\gamma^{\mu\nu}\epsilon^A + \gamma^\mu D_\mu\phi\epsilon^A - D^A_B\epsilon^B + 2\phi\eta^A \\ &= \frac{i}{2}(F_{\mu\nu} - \alpha^{-1}\phi V_{\mu\nu})\gamma^{\mu\nu}\epsilon^A + \alpha D_\mu(\alpha^{-1}\phi)\gamma^\mu\epsilon^A + (i\alpha\phi\sigma_3 - D)^A_B\epsilon^B \end{aligned} \quad (17.5.13)$$

in our notation and normalization for fields, with

$$\eta_\pm = i \left( \alpha\sigma_3/2 - \frac{1}{4\alpha}V_{\mu\nu}\gamma^{\mu\nu} + \frac{i}{2\alpha}\nabla_\mu\alpha\gamma^\mu \right) \epsilon_\pm . \quad (17.5.14)$$

The  $\pm$  signs are for the  $SU(2)_R$  doublet, containing  $R$  or  $\frac{R_1+R_2}{2}$  as the Cartan. The supersymmetric configurations, apart from possible singular behaviors, are

$$F_{\mu\nu} = \alpha^{-1}\phi(dC)_{\mu\nu} , \quad D_\mu(\alpha^{-1}\phi) = 0 , \quad D = i\alpha\phi\sigma_3 . \quad (17.5.15)$$

This is solved by  $\phi = \alpha\phi_0$  with a constant  $\phi_0$ , and  $A_\mu = \phi_0 C_\mu$ ,  $D = i\alpha^2\phi_0\sigma_3$ . For various background vector multiplet fields, this will be enough. However, these configurations are also legitimate saddle point configurations for the dynamical vector multiplet fields in the path integral. There it will be necessary to include singular configurations to the above solutions. There is only one background vector multiplet field appearing in the vector multiplet action, whose nonzero scalar VEV sets the Yang-Mills coupling scale. Namely, we take  $(A_\mu^I, \chi^{IA}, \phi^I)$  with  $I = 0, 1, \dots, n_V$ , where  $n_V$  is the number of matter vector multiplet fields. In our case,  $n_V = |G|$ . There is one auxiliary scalar  $\phi^0$ , and the remaining  $n_V$  scalars are arranged into a matrix  $\phi$ . The matter-gravity coupling action is given by the cubic function  $\mathcal{N} = C_{IJK}\phi^I\phi^J\phi^K$ , which we take as  $\mathcal{N} = \phi^0\text{tr}(\phi\phi)$  in our case. The background fields are given by  $A_\mu^0 = C_\mu$ ,  $\phi^0 = \alpha$ ,  $D^0 = i\alpha^2\sigma_3$ . So these background fields are the ‘gravi-photon/dilaton’ background. The vector multiplet action can be read off from [70]. For instance, the bosonic part of the vector multiplet action is given by

$$\begin{aligned} 2g_{YM}^2 e^{-1}\mathcal{L}_V &= \left( -\frac{1}{2}D + \frac{1}{4}R + \frac{3}{16\alpha^2}V^2 \right) \alpha\phi^2 - \frac{1}{2\alpha}\phi^2V^2 + \phi \left( 2\partial^a\alpha D_a\phi - \frac{i}{4}\alpha^2(\sigma_3)_{AB}D^{AB} \right) \\ &\quad + \frac{\alpha}{2}F_{ab}F^{ab} + \alpha D^a\phi D_a\phi + \frac{\alpha}{2}D_{AB}D^{AB} + e^{-1}\frac{i}{4}\epsilon^{\mu\nu\rho\sigma\tau}C_\mu F_{\nu\rho}F_{\sigma\tau} , \end{aligned} \quad (17.5.16)$$

where trace is assumed. The first order term  $2\phi\partial^a\alpha D_a\phi$  on the first line can be integrated by part, to yield the mass term  $-(\partial^2\alpha)\phi^2$ .

Now we consider the special SUSY configuration  $A_\mu = \phi_0 C_\mu$ ,  $D = i\alpha^2\phi_0\sigma_3$ ,  $\phi = \alpha\phi_0$  for *dynamical* vector multiplet fields. Plugging this into the action (17.5.16), the saddle point action is given by

$$S_0 = \frac{4\pi^3\text{tr}(\phi_0^2)}{g_{YM}^2\omega_1\omega_2\omega_3} . \quad (17.5.17)$$

Restoring  $r$  and making all parameters dimensionless  $\beta = \frac{g_{YM}^2}{2\pi r}$ ,  $r\phi_0 = \phi_{\text{new}}$ , one obtains

$$S_0 = \frac{2\pi^2\text{tr}(\phi^2)}{\beta\omega_1\omega_2\omega_3} , \quad (17.5.18)$$

which is the classical measure used in (17.3.3). When singular self-dual instanton strings are put on  $S^5$  along  $S^1$  at  $(n_1, n_2, n_3) = (1, 0, 0), (0, 1, 0), (0, 0, 1)$ , as mentioned in section 3.1, there is an extra contribution to the classical action. Supposing that  $k_1, k_2, k_3$  self-dual instanton strings are put at three circles in  $U(1)^r \subset G_r$  part of the gauge group, the first and last term of the second line of (17.5.16) makes additional contribution to the action. The net action is [16]

$$S_0 = \frac{2\pi^2\text{tr}(\phi^2)}{\beta\omega_1\omega_2\omega_3} + \sum_{i=1}^3 \frac{4\pi^2 k_i}{\beta\omega_i} . \quad (17.5.19)$$

For the charged hypermultiplets, one should rely on a bit brute-force method of constructing the SUSY action and transformation. One can follow [27], which constructs the action with one off-shell supersymmetry. For the hypermultiplet with scalar  $q_A$ , complex fermion  $\psi$ , we introduce two complex auxiliary fields  $F_{A'}$ , following [27]. The supersymmetric action (also coupling with vector multiplet fields) is given by

$$\begin{aligned} \mathcal{L}_H = & |D_\mu q^A|^2 + |[\phi, q^A]|^2 - \bar{q}_A(\sigma^I)^A_B [D^I, q^B] + (4 - \alpha^2/4) |q^A|^2 - \bar{F}_{A'} F^{A'} \\ & + i\psi^\dagger \gamma^\mu D_\mu \psi + i\psi^\dagger [\phi, \psi] + \sqrt{2}i\psi^\dagger [\chi_A, q^A] - \sqrt{2}i[\bar{q}_A, \chi^{\dagger A}] \psi - \frac{1}{8\alpha} \psi^\dagger V_{ab} \gamma^{ab} \psi + \frac{i}{2\alpha} \partial_a \alpha \psi^\dagger \gamma^a \psi . \end{aligned} \quad (17.5.20)$$

We presented the result for adjoint hypermultiplet, but the action for other representations should also be clear. The action is invariant under the SUSY transformation

$$\begin{aligned} \delta q^A &= \sqrt{2}i\epsilon^{\dagger A} \psi , \quad \delta \bar{q}_A = \sqrt{2}i\psi^\dagger \epsilon_A , \\ \delta \psi &= \sqrt{2} \left[ -D_\mu q_A \gamma^\mu \epsilon^A + [\phi, q_A] \epsilon^A + \frac{3i}{2} \alpha q_A (\sigma^3)^A_B \epsilon^B + \left( \frac{i}{2\alpha} V_{ab} \gamma^{ab} + \frac{2}{\alpha} \partial_a \alpha \gamma^a \right) q_A \epsilon^A - iF_{A'} \hat{\epsilon}^{A'} \right] , \\ \delta F^{A'} &= \sqrt{2} \hat{\epsilon}^{\dagger A'} \left[ -\gamma^\mu \nabla_\mu \psi - [\phi, \psi] + \frac{i}{8\alpha} V_{ab} \gamma^{ab} \psi + \frac{1}{2\alpha} \partial_a \alpha \gamma^a \psi \right] , \end{aligned} \quad (17.5.21)$$

and the spinor  $\hat{\epsilon}$  satisfies [27]

$$\epsilon^\dagger \epsilon = \hat{\epsilon}^\dagger \hat{\epsilon} , \quad (\epsilon^A)^T C \hat{\epsilon}^{B'} = 0 , \quad \epsilon^\dagger \gamma^\mu \epsilon + \hat{\epsilon}^\dagger \gamma^\mu \hat{\epsilon} = 0 . \quad (17.5.22)$$

To turn on the hypermultiplet mass  $m$ , we introduce one more background vector multiplet for the hypermultiplet flavor symmetry, and give them supersymmetric background values with  $\phi^0 \sim m$ . Then one can couple this background vector field with the above hypermultiplet in the same way as the dynamical vector fields couple to the hypermultiplets above.

## References

- [1] V. Pestun and M. Zabzine, eds., *Localization techniques in quantum field theory*, vol. xx. Journal of Physics A, 2016. 1608.02952. <https://arxiv.org/src/1608.02952/anc/LocQFT.pdf>, <http://pestun.ihep.fr/pages/LocalizationReview/LocQFT.pdf>.
- [2] E. Witten, In \*Los Angeles 1995, Future perspectives in string theory\* 501-523 [hep-th/9507121].
- [3] N. Seiberg and E. Witten, Nucl. Phys. B **471**, 121 (1996) [hep-th/9603003].
- [4] N. Seiberg, Phys. Lett. B **388**, 753 (1996) [hep-th/9608111].
- [5] H. C. Kim, S. S. Kim and K. Lee, JHEP **1210**, 142 (2012) [arXiv:1206.6781 [hep-th]].
- [6] O. Bergman, D. Rodriguez-Gomez and G. Zafrir, JHEP **1308**, 081 (2013) [arXiv:1305.6870 [hep-th]]; O. Bergman, D. Rodriguez-Gomez and G. Zafrir, JHEP **1401**, 079 (2014) [arXiv:1310.2150 [hep-th]]; O. Bergman, D. Rodriguez-Gomez and G. Zafrir, JHEP **1403**, 112 (2014) [arXiv:1311.4199 [hep-th]]; G. Zafrir, JHEP **1412**, 116 (2014) [arXiv:1408.4040 [hep-th]]; O. Bergman and G. Zafrir, arXiv:1410.2806 [hep-th].
- [7] H. Hayashi, H. C. Kim and T. Nishinaka, JHEP **1406**, 014 (2014) [arXiv:1310.3854 [hep-th]]; H. Hayashi and G. Zoccarato, JHEP **1501**, 093 (2015) [arXiv:1409.0571 [hep-th]].
- [8] L. Bao, V. Mitev, E. Pomoni, M. Taki and F. Yagi, JHEP **1401**, 175 (2014) [arXiv:1310.3841 [hep-th]]; M. Taki, arXiv:1310.7509 [hep-th]; M. Taki, arXiv:1401.7200 [hep-th]; V. Mitev, E. Pomoni, M. Taki and F. Yagi, arXiv:1411.2450 [hep-th].
- [9] D. L. Jafferis and S. S. Pufu, JHEP **1405**, 032 (2014) [arXiv:1207.4359 [hep-th]].
- [10] L. F. Alday, M. Fluder, P. Richmond and J. Sparks, Phys. Rev. Lett. **113**, no. 14, 141601 (2014) [arXiv:1404.1925 [hep-th]]; L. F. Alday, M. Fluder, C. M. Gregory, P. Richmond and J. Sparks, JHEP **1409**, 067 (2014) [arXiv:1405.7194 [hep-th]].
- [11] B. Assel, J. Estes and M. Yamazaki, Annales Henri Poincare **15**, 589 (2014) [arXiv:1212.1202 [hep-th]].
- [12] H. C. Kim and S. Kim, JHEP **1305**, 144 (2013) [arXiv:1206.6339 [hep-th]].
- [13] J. Kallen, J. A. Minahan, A. Nedelin and M. Zabzine, JHEP **1210**, 184 (2012) [arXiv:1207.3763 [hep-th]].
- [14] H. C. Kim and K. Lee, JHEP **1307**, 072 (2013) [arXiv:1210.0853 [hep-th]].
- [15] G. Lockhart and C. Vafa, arXiv:1210.5909 [hep-th].
- [16] H. C. Kim, J. Kim and S. Kim, arXiv:1211.0144 [hep-th].
- [17] J. A. Minahan, A. Nedelin and M. Zabzine, J. Phys. A **46**, 355401 (2013) [arXiv:1304.1016 [hep-th]].
- [18] H. C. Kim, S. Kim, S. S. Kim and K. Lee, arXiv:1307.7660.
- [19] T. Kawano and N. Matsumiya, Phys. Lett. B **716**, 450 (2012) [arXiv:1206.5966 [hep-th]]. Y. Fukuda, T. Kawano and N. Matsumiya, Nucl. Phys. B **869**, 493 (2013) [arXiv:1210.2855 [hep-th]].
- [20] J. Yagi, JHEP **1308**, 017 (2013) [arXiv:1305.0291 [hep-th]].
- [21] S. Lee and M. Yamazaki, JHEP **1312**, 035 (2013) [arXiv:1305.2429 [hep-th]].
- [22] C. Cordova and D. L. Jafferis, arXiv:1305.2891 [hep-th].
- [23] H. Mori and S. Yamaguchi, Phys. Rev. D **90**, no. 2, 026005 (2014) [arXiv:1404.0930 [hep-th]].
- [24] M. Bullimore and H. C. Kim, arXiv:1412.3872 [hep-th].
- [25] F. Nieri, S. Pasquetti and F. Passerini, Lett. Math. Phys. **105**, no. 1, 109 (2015) [arXiv:1303.2626 [hep-th]].

- [26] J. Kallen and M. Zabzine, JHEP **1205**, 125 (2012) [arXiv:1202.1956 [hep-th]].
- [27] K. Hosomichi, R. K. Seong and S. Terashima, Nucl. Phys. B **865**, 376 (2012) [arXiv:1203.0371 [hep-th]].
- [28] J. Kallen, J. Qiu and M. Zabzine, JHEP **1208**, 157 (2012) [arXiv:1206.6008 [hep-th]].
- [29] Y. Imamura, arXiv:1210.6308 [hep-th].
- [30] C. Cordova and D. L. Jafferis, arXiv:1305.2886 [hep-th].
- [31] F. Nieri, S. Pasquetti, F. Passerini and A. Torrielli, JHEP **1412**, 040 (2014) [arXiv:1312.1294 [hep-th], arXiv:1312.1294v2].
- [32] J. Qiu and M. Zabzine, Phys. Rev. D **89**, no. 6, 065040 (2014) [arXiv:1312.3475 [hep-th]].
- [33] J. Qiu, L. Tizzano, J. Winding and M. Zabzine, arXiv:1403.2945 [hep-th].
- [34] J. Qiu and M. Zabzine, arXiv:1409.1058 [hep-th].
- [35] N. A. Nekrasov, Adv. Theor. Math. Phys. **7**, 831 (2004) [arXiv:hep-th/0206161].
- [36] N. Nekrasov and A. Okounkov, arXiv:hep-th/0306238.
- [37] H. C. Kim, S. Kim, E. Koh, K. Lee and S. Lee, JHEP **1112**, 031 (2011) [arXiv:1110.2175 [hep-th]].
- [38] B. Haghighat, A. Iqbal, C. Kozcaz, G. Lockhart and C. Vafa, arXiv:1305.6322 [hep-th].
- [39] B. Haghighat, C. Kozcaz, G. Lockhart and C. Vafa, Phys. Rev. D **89**, no. 4, 046003 (2014) [arXiv:1310.1185 [hep-th]].
- [40] B. Haghighat, G. Lockhart and C. Vafa, Phys. Rev. D **90**, no. 12, 126012 (2014) [arXiv:1406.0850 [hep-th]].
- [41] C. Hwang, J. Kim, S. Kim and J. Park, arXiv:1406.6793 [hep-th].
- [42] J. Kim, S. Kim, K. Lee, J. Park and C. Vafa, arXiv:1411.2324 [hep-th].
- [43] W. Cai, M. x. Huang and K. Sun, JHEP **1501**, 079 (2015) [arXiv:1411.2801 [hep-th]].
- [44] D. Gaiotto and H. C. Kim, arXiv:1412.2781 [hep-th].
- [45] B. Haghighat, A. Klemm, G. Lockhart and C. Vafa, arXiv:1412.3152 [hep-th].
- [46] J. Bhattacharya, S. Bhattacharyya, S. Minwalla and S. Raju, JHEP **0802**, 064 (2008) [arXiv:0801.1435 [hep-th]].
- [47] V. Pestun, Commun. Math. Phys. **313**, 71 (2012) [arXiv:0712.2824 [hep-th]].
- [48] A. Strominger, Phys. Lett. B **383**, 44 (1996) [hep-th/9512059].
- [49] P. S. Howe, N. D. Lambert and P. C. West, Nucl. Phys. B **515**, 203 (1998) [hep-th/9709014].
- [50] A. Gadde and S. Gukov, JHEP **1403** (2014) 080 [arXiv:1305.0266 [hep-th]].
- [51] F. Benini, R. Eager, K. Hori and Y. Tachikawa, Lett. Math. Phys. **104**, 465 (2014) [arXiv:1305.0533 [hep-th]].
- [52] F. Benini, R. Eager, K. Hori and Y. Tachikawa, arXiv:1308.4896 [hep-th].
- [53] C. Cordova and S. -H. Shao, arXiv:1406.7853 [hep-th].
- [54] K. Hori, H. Kim and P. Yi, arXiv:1407.2567 [hep-th].
- [55] D. R. Morrison and C. Vafa, Nucl. Phys. B **473**, 74 (1996) [hep-th/9602114].
- [56] D. R. Morrison and C. Vafa, Nucl. Phys. B **476**, 437 (1996) [hep-th/9603161].
- [57] E. Witten, Nucl. Phys. B **471**, 195 (1996) [hep-th/9603150].

- [58] R. Gopakumar and C. Vafa, hep-th/9809187.
- [59] R. Gopakumar and C. Vafa, hep-th/9812127.
- [60] O. Aharony, M. Berkooz, S. Kachru, N. Seiberg and E. Silverstein, Adv. Theor. Math. Phys. **1**, 148 (1998) [hep-th/9707079]; O. Aharony, M. Berkooz and N. Seiberg, Adv. Theor. Math. Phys. **2**, 119 (1998) [hep-th/9712117].
- [61] R. Flume and R. Poghossian, Int. J. Mod. Phys. A **18**, 2541 (2003) [hep-th/0208176].
- [62] U. Bruzzo, F. Fucito, J. F. Morales and A. Tanzini, JHEP **0305**, 054 (2003) [hep-th/0211108].
- [63] L. C. Jeffrey and F. C. Kirwan, Topology **34** no. 2, 291 (1995) [arXiv:alg-geom/9307001]; A. Szenes and M. Vergne, Invent. Math. **158** no. 3, 453 (2004) [arXiv:math/0306311 [math.AT]].
- [64] D. Harland and C. Nolle, JHEP **1203**, 082 (2012) [arXiv:1109.3552 [hep-th]]; M. Wolf, JHEP **1207**, 074 (2012) [arXiv:1203.3423 [hep-th]].
- [65] A. Hanany and A. Zaffaroni, Nucl. Phys. B **529**, 180 (1998) [hep-th/9712145]; D. Gaiotto and A. Tomasiello, JHEP **1412**, 003 (2014) [arXiv:1404.0711 [hep-th]].
- [66] J. J. Heckman, D. R. Morrison and C. Vafa, JHEP **1405**, 028 (2014) [arXiv:1312.5746 [hep-th]]; M. Del Zotto, J. J. Heckman, A. Tomasiello and C. Vafa, arXiv:1407.6359 [hep-th].
- [67] M. R. Douglas and G. W. Moore, hep-th/9603167.
- [68] P. Horava and E. Witten, Nucl. Phys. B **460**, 506 (1996) [hep-th/9510209].
- [69] G. Festuccia and N. Seiberg, JHEP **1106**, 114 (2011) [arXiv:1105.0689 [hep-th]].
- [70] T. Kugo and K. Ohashi, Prog. Theor. Phys. **105**, 323 (2001) [hep-ph/0010288]; K. Hanaki, K. Ohashi and Y. Tachikawa, Prog. Theor. Phys. **117**, 533 (2007) [hep-th/0611329].
- [71] A. Iqbal, C. Kozcaz and K. Shabbir, Nucl. Phys. B **838**, 422 (2010) [arXiv:0803.2260 [hep-th]].
- [72] L. Di Pietro and Z. Komargodski, JHEP **1412**, 031 (2014) [arXiv:1407.6061 [hep-th]].
- [73] C. Beem, L. Rastelli and B. C. van Rees, arXiv:1404.1079 [hep-th].
- [74] L. Grant, P. A. Grassi, S. Kim and S. Minwalla, JHEP **0805**, 049 (2008) [arXiv:0803.4183 [hep-th]].
- [75] G. Mandal and N. V. Suryanarayana, JHEP **0703**, 031 (2007) [hep-th/0606088].
- [76] S. Bhattacharyya and S. Minwalla, JHEP **0712**, 004 (2007) [hep-th/0702069 [HEP-TH]].
- [77] S. K. Ashok and N. V. Suryanarayana, JHEP **0905**, 090 (2009) [arXiv:0808.2042 [hep-th]].
- [78] L. F. Alday, D. Gaiotto and Y. Tachikawa, Lett. Math. Phys. **91**, 167 (2010) [arXiv:0906.3219 [hep-th]].
- [79] N. Wyllard, JHEP **0911**, 002 (2009) [arXiv:0907.2189 [hep-th]].
- [80] L. F. Alday, D. Gaiotto, S. Gukov, Y. Tachikawa and H. Verlinde, JHEP **1001**, 113 (2010) [arXiv:0909.0945 [hep-th]].
- [81] O. Aharony, J. Marsano, S. Minwalla, K. Papadodimas and M. Van Raamsdonk, Adv. Theor. Math. Phys. **8**, 603 (2004) [hep-th/0310285].
- [82] D. Cassani and D. Martelli, JHEP **1408**, 044 (2014) [arXiv:1402.2278 [hep-th]].
- [83] A. M. Awad and C. V. Johnson, Phys. Rev. D **63**, 124023 (2001) [hep-th/0008211].
- [84] T. Nishioka and I. Yaakov, JHEP **1310**, 155 (2013) [arXiv:1306.2958 [hep-th]].
- [85] J. McGreevy, L. Susskind and N. Toumbas, JHEP **0006**, 008 (2000) [hep-th/0003075].
- [86] M. R. Douglas, JHEP **1102** (2011) 011; N. Lambert, C. Papageorgakis and M. Schmidt-Sommerfeld, JHEP **1101**, 083 (2011);
